# Supplementary material for: High-throughput Investigations of Topological and Nodal Superconductors
Source: arXiv:2106.11985 ancillary file (2022-03-04)
Supplement: Supplementary file 1 [file SM-I.pdf]

# Supplemental Materials for "High-throughput Investigations of Topological and Nodal Superconductors"

Feng Tang,[1,*] Seishiro Ono,[2,*] Xiangang Wan,[1] and Haruki Watanabe[2]

[1]National Laboratory of Solid State Microstructures and School of Physics, Nanjing University, Nanjing 210093, China and Collaborative Innovation Center of Advanced Microstructures, Nanjing University, Nanjing 210093, China

[2]Department of Applied Physics, University of Tokyo, Tokyo 113-8656, Japan

## CONTENTS

A. Cooper pair and its symmetry 2

B. Details of constructing $\{\mathrm{BS}\}$ for each magnetic space group 4
1. Remarks 4
2. Construction of $\{\mathrm{BS}\}_f$ and $\{\mathrm{AI}\}_f$ bases 4
a. Representation of MSG operation in the Bloch basis 5
b. BLs for a given $k$ 6
c. CRs of irreps of little groups 7
d. CRs for BLs and BS space for Bogoliubov excitations 7
e. Constructing basis vectors of $\{\mathrm{BS}\}_f$ space 7
f. Constructing ALs exhaustively and find basis vectors of $\{\mathrm{AI}\}_f$ space 8
g. Get regularized basis vectors of $\{\mathrm{BS}\}_f$ and $X_f$ 9

C. The strategy of dealing with cases when pairing breaking colored symmetry 10

D. Remarks on the Bilbao notations 10

E. Subroutine *TopologicalSupercon* 12
1. Generating inputs 12
a. Formatting results of first-principles calculations 12
b. Precautions on convention 12

F. Details of analyses of material examples 14
1. BaPtP with ${}^1E$ pairing 14
2. BaPtP with $T$ pairing 14
3. BaPtSb with $A_1''$ pairing 15
4. Detailed information on $CsV_3Sb_5$ 16

References 17

* These two authors contribute equally to this work.

In this supplemental materials, we provide theoretical details in our work.

## A. COOPER PAIR AND ITS SYMMETRY

In this section, we discuss how irreducible representations describe the pairing symmetries[1].

The superconducting order parameter is described by

$$\hat{\Delta} = \frac{1}{2}\sum_{\boldsymbol{k}}\sum_{\sigma\sigma'}\Delta_{\sigma\sigma'}(\boldsymbol{k})\hat{c}^{\dagger}_{\sigma}(\boldsymbol{k})\hat{c}^{\dagger}_{\sigma'}(-\boldsymbol{k}) + \text{h.c.}, \tag{1}$$

where $\hat{c}^{\dagger}_{\sigma}(\boldsymbol{k})$ is the creation operator of an electron with momentum $\boldsymbol{k}$ and $\sigma$ denotes the degree of freedom of the system.

Let $g$ be a space group symmetry of the normal phase, which satisfies

$$\hat{g}\hat{c}^{\dagger}_{\sigma}(\boldsymbol{k})\hat{g}^{-1} = \sum_{\sigma'}\hat{c}^{\dagger}_{\sigma'}(p_g\boldsymbol{k})[u_{\boldsymbol{k}}(g)]_{\sigma'\sigma}, \tag{2}$$

where $p_g$ is an $\mathrm{O}(3)$ representation of $g$ and $u(g)$ is a unitary representation of $g$. Then, the superconducting order parameter is transformed by

$$\hat{g}\hat{\Delta}\hat{g}^{-1} = \frac{1}{2}\sum_{\boldsymbol{k}}\sum_{\sigma\sigma'}\sum_{l,l'}\hat{c}^{\dagger}_{l}(p_g\boldsymbol{k})[u_{\boldsymbol{k}}(g)]_{l\sigma}\Delta_{\sigma\sigma'}(\boldsymbol{k})[u_{-\boldsymbol{k}}(g)]_{l'\sigma'}\hat{c}^{\dagger}_{l'}(-p_g\boldsymbol{k}) + \text{h.c.}, \tag{3}$$

$$= \frac{1}{2}\sum_{\boldsymbol{k}}\sum_{\sigma\sigma'}\hat{c}^{\dagger}_{\sigma}(p_g\boldsymbol{k})\left(u_{\boldsymbol{k}}(g)\Delta(\boldsymbol{k})u^{T}_{-\boldsymbol{k}}(g)\right)_{\sigma\sigma'}\hat{c}^{\dagger}_{\sigma'}(-p_g\boldsymbol{k}) + \text{h.c.}, \tag{4}$$

In the following, we discuss the transformation of $\Delta(\boldsymbol{k})$ under PG operations. Irreps of PGs play an important role in this purpose [1]. Here, we consider one-dimensional irreps and higher-dimensional ones, separately.

(i) one-dimensional irrep.

We define the case where a superconducting order parameter belongs to a one-dimensional irrep by

$$u_{\boldsymbol{k}}(g)\Delta(\boldsymbol{k})u^{T}_{-\boldsymbol{k}}(g) = e^{i\theta_g}\Delta(p_g\boldsymbol{k}) \ \ (e^{i\theta_g} \in \mathrm{U}(1)). \tag{5}$$

In such a case, by redefining $u'(g) = e^{-i\theta_g/2}u(g)$, we find that $\hat{g}\hat{\Delta}\hat{g}^{-1} = \hat{\Delta}$. Thus, $g$ is a symmetry of the superconducting phase.

(ii) higher-dimensional irrep.

For an order parameter that belongs to a $N$-dimensional irrep, $\Delta(\boldsymbol{k})$ is described by

$$\Delta(\boldsymbol{k}) = \sum_{a=1}^{N}\eta_a\Delta_a(\boldsymbol{k}) \tag{6}$$

such that

$$u_{\boldsymbol{k}}(g)\Delta_a(\boldsymbol{k})u^{T}_{-\boldsymbol{k}}(g) = \sum_{b=1}^{N}\Delta_b(p_g\boldsymbol{k})[u^{\alpha}]_{ba}, \tag{7}$$

where $u^{\alpha}$ is a $N$-dimensional irrep. Depending on the parameters $\{\eta_a\}_{a=1}^{N}$, the remaining symmetries are different, as shown in the following example.

Let us discuss $E_u$ representation of PG $D_{4h}$. Here, to see how the point group is lowered, it is enough to consider PG part of the space group. For simplicity, we here consider the two orbital system. Then, according to Ref. [1], the superconducting order parameters are described by

$$\Delta(\boldsymbol{k}) = \eta_1\Delta_1(\boldsymbol{k}) + \eta_2\Delta_2(\boldsymbol{k}), \tag{8}$$

$$= \eta_1 k_x\sigma_x + \eta_2 k_y\sigma_x. \tag{9}$$

---

[1] This section is based on discussions with Ken Shiozaki. Seishiro Ono would like to thank Ken Shiozaki for explaining the case of higher-dimensional irreducible representations to him.

For a PG operation $g$, $\Delta(\boldsymbol{k})$ is transformed as

$$u(g)\Delta(\boldsymbol{k})u^T(g) = \begin{pmatrix} u(g)\Delta_1(\boldsymbol{k})u^T(g) & u(g)\Delta_2(\boldsymbol{k})u^T(g) \end{pmatrix} \begin{pmatrix} \eta_1 \\ \eta_2 \end{pmatrix} \tag{10}$$

$$= \begin{pmatrix} \Delta_1(p_g\boldsymbol{k}) & \Delta_2(p_g\boldsymbol{k}) \end{pmatrix} u^{E_u}(g) \begin{pmatrix} \eta_1 \\ \eta_2 \end{pmatrix} \tag{11}$$

Since $u(g)$ can be chosen such that $e^{-i(\theta_g/2)\boldsymbol{n}_g\cdot\boldsymbol{\sigma}}$, we find that

$$u(C_4^z)\Delta(\boldsymbol{k})u^T(C_4^z) = e^{-i\frac{\pi}{4}\sigma_z}\Delta(\boldsymbol{k})e^{-i\frac{\pi}{4}\sigma_z}$$

$$= \begin{pmatrix} \Delta_1(-k_y, k_x) & \Delta_2(-k_y, k_x) \end{pmatrix} \begin{pmatrix} 0 & -1 \\ 1 & 0 \end{pmatrix} \begin{pmatrix} \eta_1 \\ \eta_2 \end{pmatrix}, \tag{12}$$

$$u(C_2^z)\Delta(\boldsymbol{k})u^T(C_2^z) = e^{-i\frac{\pi}{2}\sigma_z}\Delta(\boldsymbol{k})e^{-i\frac{\pi}{2}\sigma_z}$$

$$= \begin{pmatrix} \Delta_1(-\boldsymbol{k}) & \Delta_2(-\boldsymbol{k}) \end{pmatrix} \begin{pmatrix} -1 & 0 \\ 0 & -1 \end{pmatrix} \begin{pmatrix} \eta_1 \\ \eta_2 \end{pmatrix}, \tag{13}$$

$$u(C_2^x)\Delta(\boldsymbol{k})u^T(C_2^x) = e^{-i\frac{\pi}{2}\sigma_x}\Delta(\boldsymbol{k})e^{-i\frac{\pi}{2}\sigma_x}$$

$$= \begin{pmatrix} \Delta_1(k_x, -k_y) & \Delta_2(k_x, -k_y) \end{pmatrix} \begin{pmatrix} -1 & 0 \\ 0 & 1 \end{pmatrix} \begin{pmatrix} \eta_1 \\ \eta_2 \end{pmatrix}, \tag{14}$$

$$u(I)\Delta(\boldsymbol{k})u^T(I) = \sigma_0\Delta(\boldsymbol{k})\sigma_0$$

$$= \begin{pmatrix} \Delta_1(-\boldsymbol{k}) & \Delta_2(-\boldsymbol{k}) \end{pmatrix} \begin{pmatrix} -1 & 0 \\ 0 & -1 \end{pmatrix} \begin{pmatrix} \eta_1 \\ \eta_2 \end{pmatrix}. \tag{15}$$

(16)

When we consider $(\eta_1, \eta_2) = (1, 0)$, while the $C_4$ is no longer a symmetry of the system, $C_2^x, C_2^z$, and $I$ are still symmetries. Then, $\Delta_1(\boldsymbol{k})$ belongs to $B_{2u}$ irrep of PG $D_{2h}$.

Indeed, we can consider the order parameter in a different basis, i.e.,

$$\Delta(\boldsymbol{k}) = \eta_1'\Delta_1'(\boldsymbol{k}) + \eta_2'\Delta_2'(\boldsymbol{k}), \tag{17}$$

where

$$\begin{pmatrix} \Delta_1' & \Delta_2' \end{pmatrix} = \begin{pmatrix} \Delta_1 & \Delta_2 \end{pmatrix} V, \quad \begin{pmatrix} \eta_1' \\ \eta_2' \end{pmatrix} = V^{-1} \begin{pmatrix} \eta_1 \\ \eta_2 \end{pmatrix}. \tag{18}$$

For example, we take $V = \begin{pmatrix} 1 & -1 \\ i & i \end{pmatrix}$, and then $V^{-1}\begin{pmatrix} 0 & -1 \\ 1 & 0 \end{pmatrix} V = \mathrm{diag}(-i, i)$. In this case, the transformations are

$$u(C_4^z)\Delta(\boldsymbol{k})u^T(C_4^z) = e^{-i\frac{\pi}{4}\sigma_z}\Delta(\boldsymbol{k})e^{-i\frac{\pi}{4}\sigma_z}$$

$$= \begin{pmatrix} \Delta_1'(-k_y, k_x) & \Delta_2'(-k_y, k_x) \end{pmatrix} \begin{pmatrix} -i & 0 \\ 0 & i \end{pmatrix} \begin{pmatrix} \eta_1' \\ \eta_2' \end{pmatrix}, \tag{19}$$

$$u(C_2^z)\Delta(\boldsymbol{k})u^T(C_2^z) = e^{-i\frac{\pi}{2}\sigma_z}\Delta(\boldsymbol{k})e^{-i\frac{\pi}{2}\sigma_z}$$

$$= \begin{pmatrix} \Delta_1'(-\boldsymbol{k}) & \Delta_2'(-\boldsymbol{k}) \end{pmatrix} \begin{pmatrix} -1 & 0 \\ 0 & -1 \end{pmatrix} \begin{pmatrix} \eta_1' \\ \eta_2' \end{pmatrix}, \tag{20}$$

$$u(C_2^x)\Delta(\boldsymbol{k})u^T(C_2^x) = e^{-i\frac{\pi}{2}\sigma_x}\Delta(\boldsymbol{k})e^{-i\frac{\pi}{2}\sigma_x}$$

$$= \begin{pmatrix} \Delta_1'(k_x, -k_y) & \Delta_2'(k_x, -k_y) \end{pmatrix} \begin{pmatrix} 0 & 1 \\ 1 & 0 \end{pmatrix} \begin{pmatrix} \eta_1' \\ \eta_2' \end{pmatrix}, \tag{21}$$

$$u(I)\Delta(\boldsymbol{k})u^T(I) = \sigma_0\Delta(\boldsymbol{k})\sigma_0$$

$$= \begin{pmatrix} \Delta_1'(-\boldsymbol{k}) & \Delta_2'(-\boldsymbol{k}) \end{pmatrix} \begin{pmatrix} -1 & 0 \\ 0 & -1 \end{pmatrix} \begin{pmatrix} \eta_1' \\ \eta_2' \end{pmatrix}. \tag{22}$$

(23)

When we consider $(\eta_1', \eta_2') = (1, 0)$ $[(\eta_1, \eta_2) = (1, i)]$, while the $C_2^x$ is no longer a symmetry of the system, $C_4^z$ and $I$ are still symmetries. Then, $\Delta_1'(\boldsymbol{k}) = \Delta_1(\boldsymbol{k}) + i\Delta_2(\boldsymbol{k}) = (k_x + ik_y)\sigma_x$, which is well-known as the order parameter of chiral $p$-wave superconductors, belongs to ${}^1E_u$ irrep of PG $C_{4h}$.

As shown above, the PG symmetry could be lowered by pairings that belongs to higher-dimensional irreps. A strategy to enumerate all lowered PGs is that we consider all inequivalent bases such that the representation matrices of the higher-dimensional irrep for some symmetries are diagonal simultaneously and parameters $\{\eta_a\}_{a=1}^N$ in each basis. To find such bases is achieved by to decompose the higher-dimensional irrep into several one-dimensional irreps of the sub-point group (sub-PG) of the original PG. In this work, we focus on maximal sub-PGs (namely, no other sub-PGs are their supergroups) and the cases where only one parameter $\eta_a$ is one and the others are zero in each basis. Although it is true that superconducting order parameters can have multiple components of irreps of the lowered PG, we think that such a case should be rare. For example, $D_{4h}$ is reduced to $C_{2h}$ $[(\eta_1, \eta_2) = (1, 1)$ in the above example]. In such a case, one can use our subroutine to diagnose topological/nodal superconductivity.

## B. DETAILS OF CONSTRUCTING $\{\mathrm{BS}\}$ FOR EACH MAGNETIC SPACE GROUP

### 1. Remarks

For each space group (SG), or more generally, magnetic space group (MSG), assuming the pairing symmetry which belongs to 1D single-valued irreducible representation (irrep) of the point group, one can determine the band structure (BS) space of superconductors whose base can be written as $\mathbf{b}_i, i = 1, 2, \ldots, d$ and the atomic insulator (AI) bases can be determined through $\mathbf{a}_i = s_i \mathbf{b}_i$. Here $\mathbf{b}_i$'$s$ contain band labels (BLs) that are consistent with a gapped superconductor or superconductor only allowing node in generic point. And $\mathbf{a}_i$'$s$ contain BLs that are consistent with trivial superconductors. Later, we show explicitly the factors $S = (s_1, s_2, \ldots, s_d)$ and $\{\mathbf{b}_i\}_{i=1}^d$ for all 230 space groups (type-II MSGs) considering spin-orbit coupling for any pairing symmetries (described by 1D single-valued irreps of point group), which are used in our high-throughput investigations. Note that some BL may be $\mathbb{Z}_2$-valued, thus for any calculated BLs collected as $n_{\mathrm{SC}}$, to expand it on the BS base, we need to consider the following expression:

$$n_{\mathrm{SC}} = \sum_i r_i \mathbf{b}_i + \sum_j m_j p_{\xi_j}, \tag{24}$$

where $m_j$ is integer and $p_{\xi_j}$ means that the $\xi_j$-th component of $n_{\mathrm{SC}}$ is $\mathbb{Z}_2$-valued and in $p_{\xi_j}$, only the $\xi_j$-th component is 2 while the rest are all 0. Note that $p_{\xi_j}$ must belong to AI space. Eq. 24 may result in different solutions $\{r_i\}$ but all solutions give the same diagnosis result: One may directly find solutions of $\{r_i\}$ given some $\{m_j\}$. In the following, we show one method to solve for $\{r_i\}$ but we should point out that the reader can apply other method he/she prefers:

Step 1: For the vector space spanned by $\{\mathbf{b}_i\}_i \oplus \{p_{\xi_j}\}_j$ with integer-valued coefficients, one can obtain basis vectors (actually, the resulting space is called auxiliary BS space, denoted by $\{\mathrm{BS}\}_f$) from Smith decomposition. Suppose that the basis vectors are $\mathbf{b}^f_{i'} = \sum_i P_{ii'} \mathbf{b}_i + \sum_j Q_{ji'} p_{\xi_j}$ where $P_{ii'}$ and $Q_{ji'}$ are all integers.

Step 2: Expand $n_{\mathrm{SC}}$ on the basis vectors of $\{\mathrm{BS}\}_f$: $n_{SC} = \sum_{i'} r^f_{i'} \mathbf{b}^f_{i'}$. Note that $r^f_{i'}$ should be all integers for $n_{\mathrm{SC}}$ belong to the BS space.

Step 3: From the results in the former two steps, $n_{\mathrm{SC}} = \sum_{i'} r^f_{i'} \mathbf{b}^f_{i'} = \sum_{i'i} r^f_{i'} P_{ii'} \mathbf{b}_i + \sum_{i'j} r^f_{i'} Q_{ji'} p_{\xi_j}$. Compared with Eq. 24, we can obtain that $r_i = \sum_{i'} P_{ii'} r^f_{i'}$.

### 2. Construction of $\{\mathbf{BS}\}_f$ and $\{\mathbf{AI}\}_f$ bases

As stated before, due to possibly existing $\mathbb{Z}_2$ valued BLs, it is thus necessary to introduce an auxiliary space to generalize the BLs to constitute an integer-valued vector. After that, the construction of $\{\mathrm{BS}\}_f$ and $\{\mathrm{AI}\}_f$ space is almost the same as those for normal states. However, as shown later, we should perform both analysis for $\{\mathrm{BS}\}_f$ and $\{\mathrm{AI}\}_f$ different from that for normal states, for which the BS space can be deduced from the AI space (thus analysis of AI space is enough for normal states). For $\{\mathrm{BS}\}$, one may be encountered with compatibility relations (CRs) that are $\mathbb{Z}_2$. Note that some component (or BL) in $n_{SC}$ may also be $\mathbb{Z}_2$-valued. In the following, we first show how to derive CRs for BLs at high-symmetry points (HSPs), from which we can obtain the space $\{\mathrm{BS}\}_f$ when releasing $\mathbb{Z}_2$-ness of some BLs to $\mathbb{Z}$-ness. The BLs are determined by effective Altland-Zirnbauer (EAZ) class as shown in Table 1 for any $k$ point in Brillouin zone (BZ). Denote the total symmetry group of the normal state as $\mathcal{M}$, one of 1651 MSGs, which can be written as $\mathcal{M} = \mathcal{G}$ for 230 type-I SGs where $\mathcal{G}$ is composed of only unitary spatial operations whose point parts constitute the point group (PG) $\mathcal{G}_0$ and translation subgroup is denoted by $T$, and :

$$\mathcal{M} = \mathcal{G} + A\mathcal{G}, \tag{25}$$

for type-II, III, IV MSGs, where $A = \mathcal{T}, \{\beta|\boldsymbol{\tau}\}\mathcal{T}(\beta \notin \mathcal{G}_0), \{E|\boldsymbol{\tau}\}\mathcal{T}(\{E|\boldsymbol{\tau}\} \notin T)$, respectively [2] ($\mathcal{T}$ is time-reversal transformation). Hereafter, we called elements in $A\mathcal{G}$ as colored symmetries and are also antiunitary. Any $k$ in BZ is subject to symmetries as defined by those which leave $k$ invariant up to a reciprocal lattice vector, constituting the little group $\mathcal{G}_k$ which may contain colored operations.

### *a. Representation of MSG operation in the Bloch basis*

Choosing some Bloch basis, characterized by $k$ in BZ, the total normal-state Hamiltonian can be written as the direct sum of matrices $H(\mathbf{k})$ for all $k$'s in BZ. In the same basis, the operation in the MSG can be expressed by, $U_{g\mathbf{k},\mathbf{k}}(g), g \in \mathcal{G}$ and $U_{A\mathbf{k},\mathbf{k}}(A)\mathcal{K}$ ($\mathcal{K}$ is complex conjugate). Hence, $H(\mathbf{k})$ should satisfy:

$$U_{g\mathbf{k},\mathbf{k}}(g)H(\mathbf{k})U_{g\mathbf{k},\mathbf{k}}(g)^{\dagger} = H(g\mathbf{k}), \tag{26}$$

and,

$$U_{A\mathbf{k},\mathbf{k}}(A)H(\mathbf{k})^{*}U_{A\mathbf{k},\mathbf{k}}(A)^{\dagger} = H(A\mathbf{k}). \tag{27}$$

In this work, the pairing term $\Delta(\mathbf{k})$ can be classified using the one 1D irrep (single-valued) of $\mathcal{G}_0$, whose character is denoted as $\chi_g$ ($|\chi_g|^2 = 1$), and more concretely,

$$U_{g\mathbf{k},\mathbf{k}}(g)\Delta(\mathbf{k})U_{-g\mathbf{k},-\mathbf{k}}(g)^{\top} = \chi_g\Delta(g\mathbf{k}), \tag{28}$$

viewing $\Delta(\mathbf{k})$ as the basis function of the irrep. From Eq. 28 it is easy to obtain that $\chi_{gg'} = \chi_g\chi_{g'}$ noting $U_{gg'\mathbf{k},g'\mathbf{k}}(g)U_{g'\mathbf{k},\mathbf{k}}(g') = U_{gg'\mathbf{k},\mathbf{k}}(gg')$. With respect to $A$, any colored symmetry, which could exist for type-II, III or IV MSGs, we can always require that,

$$U_{A\mathbf{k},\mathbf{k}}(A)\Delta(\mathbf{k})^{*}U_{-A\mathbf{k},-\mathbf{k}}(A)^{\top} = \Delta(A\mathbf{k}). \tag{29}$$

Hence, the single-valued irrep $\chi_g$ should satisfy that,

$$\frac{1}{|\mathcal{G}|}\sum_{g\in\mathcal{G}}\chi_{(Ag)^2} = 1, \tag{30}$$

which leads to that,

$$\chi^{*}_{A^{-1}gA} = \chi_g. \tag{31}$$

In this work, we consider all 1D single-valued irreps of the PG $\mathcal{G}_0$, which may not satisfy Eq. 30, namely the MSG $\mathcal{M}$ is reduced to $\mathcal{G}$. For this case, we discuss how to obtain $\{\mathrm{BS}\}_f$ and $\{\mathrm{AI}\}_f$ in Sec. C.

Then, the Bogoliubov-de Gennes (BdG) Hamiltonian $H^{\mathrm{BdG}}(\mathbf{k}) = \begin{pmatrix} H(\mathbf{k}) & \Delta(\mathbf{k}) \\ \Delta(\mathbf{k})^{\dagger} & -H(-\mathbf{k})^{*} \end{pmatrix}$ should satisfy the following constraints:

$$U^{\mathrm{BdG}}_{g\mathbf{k},\mathbf{k}}(g)H^{\mathrm{BdG}}(\mathbf{k})U^{\mathrm{BdG}}_{g\mathbf{k},\mathbf{k}}(g)^{\dagger} = H^{\mathrm{BdG}}(g\mathbf{k}), \tag{32}$$

and,

$$U^{\mathrm{BdG}}_{A\mathbf{k},\mathbf{k}}(A)H^{\mathrm{BdG}}(\mathbf{k})^{*}U^{\mathrm{BdG}}_{A\mathbf{k},\mathbf{k}}(A)^{\dagger} = H^{\mathrm{BdG}}(A\mathbf{k}), \tag{33}$$

once we choose:

$$U^{\mathrm{BdG}}_{g\mathbf{k},\mathbf{k}}(g) = \begin{pmatrix} U_{g\mathbf{k},\mathbf{k}}(g) & 0 \\ 0 & \chi_g U_{-g\mathbf{k},-\mathbf{k}}(g)^{*} \end{pmatrix}, \tag{34}$$

and,

$$U^{\mathrm{BdG}}_{A\mathbf{k},\mathbf{k}}(A) = \begin{pmatrix} U_{A\mathbf{k},\mathbf{k}}(A) & 0 \\ 0 & U_{-A\mathbf{k},-\mathbf{k}}(A)^{*} \end{pmatrix}. \tag{35}$$

A natural symmetry operation for the BdG Hamiltonian is particle-hole transformation $\mathcal{C} = \begin{pmatrix} 0 & 1 \\ 1 & 0 \end{pmatrix} \mathcal{K}$, where $0, 1$ should be understood as null- and identity- matrices of the same dimnension as $H(\mathbf{k})$, respectively. Thus,

$$\mathcal{C} H^{\mathrm{BdG}}(\mathbf{k}) \mathcal{C}^{\dagger} = -H^{\mathrm{BdG}}(-\mathbf{k}), \tag{36}$$

by which, it is easy to find that:

Assuming $\Psi_{\mathbf{k}}$ is the eigenvector of $H^{\mathrm{BdG}}(\mathbf{k})$ with eigenvalue $E_{\mathbf{k}}$ , $\mathcal{C}\Psi_{\mathbf{k}}$ is the eigenvector of $H^{\mathrm{BdG}}(-\mathbf{k})$ with eigenvalue $-E_{\mathbf{k}}$.

Similarly, assuming $u^{\alpha}_{\mathbf{k}}$ is $\alpha$ irrep of $\mathcal{G}(\mathbf{k})$ (more strictly, the unitary part of the little group) whose basis vectors denoted as $\Psi^{\alpha}_{\mathbf{k},s}, s = 1, 2, \ldots, d_{\alpha}$, $\mathcal{C}\Psi^{\alpha}_{\mathbf{k},s}$ are basis vectors of $\mathcal{G}(-\mathbf{k}) = \mathcal{G}(\mathbf{k})$ whose irrep is denoted as $\tilde{\alpha}$ of $\mathcal{G}(-\mathbf{k})$. Formally, we can denote such transformation as $(\mathbf{k}, \alpha) \to (-\mathbf{k}, \tilde{\alpha})$ by $\mathcal{C}$.

For any $k$ in BZ, we can assign EAZ class to each irrep of the little group $\mathcal{G}_{\mathbf{k}}$ as described in the following.

### *b. BLs for a given k*

The EAZ class $(W^{\alpha}_k(\mathcal{T}), W^{\alpha}_k(\mathcal{C}), W^{\alpha}_k(\Gamma))$ assigned to irrep $\alpha$ for $k$ in BZ can be found as follows:

For $W^{\alpha}_k(\mathcal{T})$, if there is no colored symmetries in $\mathcal{M}$ (the MSG is type-I) or the Cooper pair breaks the colored symmetries, $W^{\alpha}_k(\mathcal{T})$ must be zero, otherwise, we should check whether there exist elements in $A\mathcal{G}$ which leave $k$ invariant up to a reciprocal lattice vector. These elements constitute a set denoted by $\mathcal{T}_k = R_{\mathcal{T}}\mathcal{G}_k$, where $R_{\mathcal{T}}$ is a representative element (colored). Hence,

$$W^{\alpha}_k(\mathcal{T}) = \frac{1}{|\mathcal{T}_k|} \sum_{R \in \mathcal{T}_k} \chi^{\alpha}_k(R^2), \tag{37}$$

which can be 0,1,or $-1$ and we use $\chi^{\alpha}_k$ to denote the character of irrep $\alpha$ at $k$, or $(k, \alpha)$. Note that when $|\mathcal{T}_k| = 0$, $W^{\alpha}_k(\mathcal{T}) = 0$.

For $W^{\alpha}(\mathcal{C})$, we should check whether there exist elements in $\mathcal{G}$ which leave $k$ to be $-k$ up to a reciprocal lattice vector, constituting a set $\mathcal{C}_k = R_{\mathcal{C}}\mathcal{G}_k$ where $R_{\mathcal{C}}$ is a representative element. If there is no such element, $W^{\alpha}_k(\mathcal{C}) = 0$. Then,

$$W^{\alpha}_k(\mathcal{C}) = \frac{1}{|\mathcal{C}_k|} \sum_{R \in \mathcal{C}_k} \chi^{\alpha}_k((\mathcal{C}R)^2), \tag{38}$$

which can be 0,1,or $-1$. Note that in Eq. 38, $\chi^{\alpha}_k((\mathcal{C}R)^2) = \chi^{*}_R \chi^{\alpha}_k(R^2)$. It is easy to find that when $W^{\alpha}_k(\mathcal{C}) = 1$ or $-1$, the BL $N^{\alpha}_k$, if defined, must be zero.

For $W^{\alpha}_k(\Gamma)$, when there exists no element in $A\mathcal{G}$ leaving $k$ to be $-k$ up to a reciprocal lattice vector, it is 0, and otherwise, denote $\Gamma_k = R_{\Gamma}\mathcal{G}_k$ as a set composed of these elements in $A\mathcal{G}$ leaving $k$ to $-k$ up to a reciprocal lattice vector, it can be 0 or 1, corresponding to that $\mathcal{C}R_{\Gamma}$ transforms irrep $\alpha$ to another irrep or itself, respectively. When the pairing breaks colored symmetries or $\mathcal{M}$ is type-I MSG, $W^{\alpha}_k(\Gamma)$ is 0.

Supplementary Table 1. The classification of EAZ symmetry classes. Here $p^{\alpha}_k$ and $N^{\alpha}_k$ denotes the $\mathbb{Z}_2$- and $\mathbb{Z}$-valued BLs. The triple $(W^{\alpha}_k(\mathcal{T}), W^{\alpha}_k(\mathcal{C}), W^{\alpha}_k(\Gamma))$ represents the result of Wigner criteria. In the fifth column, we show the explicit expression of BLs in terms of $n^{\alpha}_k$ (occupied number of irrep $\alpha$ at $k$ point in normal state) assuming weak coupling.

| EAZ | $(W^{\alpha}_k(\mathcal{T}), W^{\alpha}_k(\mathcal{C}), W^{\alpha}_k(\Gamma))$ | classification | BL | BL as normal state property |
|---|---|---|---|---|
| A | $(0, 0, 0)$ | $\mathbb{Z}$ | $N^{\alpha}_k$ | $n^{\alpha}_k - n^{\tilde{\alpha}}_{-k}$ |
| AIII | $(0, 0, 1)$ | 0 | 0 | 0 |
| AI | $(1, 0, 0)$ | $\mathbb{Z}$ | $N^{\alpha}_k$ | $n^{\alpha}_k - n^{\tilde{\alpha}}_{-k}$ |
| BDI | $(1, 1, 1)$ | $\mathbb{Z}_2$ | $p^{\alpha}_k$ | $n^{\alpha}_k \mod 2$ |
| D | $(0, 1, 0)$ | $\mathbb{Z}_2$ | $p^{\alpha}_k$ | $n^{\alpha}_k \mod 2$ |
| DIII | $(-1, 1, 1)$ | 0 | 0 | 0 |
| AII | $(-1, 0, 0)$ | $2\mathbb{Z}$ | $N^{\alpha}_k$ | $n^{\alpha}_k - n^{\tilde{\alpha}}_{-k}$ |
| CII | $(-1, -1, 1)$ | 0 | 0 | 0 |
| C | $(0, -1, 0)$ | 0 | 0 | 0 |
| CI | $(1, -1, 1)$ | 0 | 0 | 0 |

### c. CRs of irreps of little groups

In the following, we discuss the CRs for irreps of related wave vectors in BZ. Suppose $k$ is connected with $k_l$ while $k$ owns a higher (or equal ) symmetry than $k_l$, thus their irreps should be related. Denote the little group of $k_l$ as $\mathcal{G}_{k_l}$, which should be a subgroup of $\mathcal{G}_k$. The irrep $\alpha$ of $\mathcal{G}_k$ is then related with irreps of $\alpha_l$ of $\mathcal{G}_{k_l}$, calculated by the following formula,

$$\begin{aligned} &(k,\alpha) \to \sum_{\alpha_l} c_{k,\alpha}^{k_l,\alpha_l}(k_l,\alpha_l), \\ &c_{k,\alpha}^{k_l,\alpha_l} = \frac{1}{|\mathcal{G}_{k_l}|}\sum_{R\in\mathcal{G}_{k_l}} e^{i(\mathbf{k}-\mathbf{k}_l)\cdot\mathbf{t}_R}(\chi_{k_l}^{\alpha_l})^*\chi_k^\alpha, \end{aligned} \tag{39}$$

where we use $(k,\alpha)$ to represent the irrep $\alpha$ of $\mathcal{G}_k$ as shown before, and note that here $R$ in the summation is taken to be uncolored. Thus the occurrences $n_k^\alpha$ (for gapped normal-state band structures) of irreps should be subject to the following constraints,

$$n_{k_l}^{\alpha_l} = \sum_\alpha c_{k,\alpha}^{k_l,\alpha_l} n_k^\alpha. \tag{40}$$

### d. CRs for BLs and BS space for Bogoliubov excitations

Then we consider the CRs for BLs at $k$ and $k_l$. The relations between BLs at these two wave vectors that would be useful in deriving constraints on BLs at HSPs are classified to the following two types:

*Type 1.* When the EAZ class of $(k_l,\alpha_l)$ is A, AI or AII, the BL should be $N_{k_l}^{\alpha_l}$ and we should require that,

$$N_{k_l}^{\alpha_l} = \sum_\alpha c_{k,\alpha}^{k_l,\alpha_l} N_k^\alpha, \tag{41}$$

where in the summation over $\alpha$, the corresponding EAZ class is also one of A, AI or AII.

*Type 2.* When the EAZ class of $(k_l,\alpha_l)$ is D or BDI, the BL should be $p_{k_l}^{\alpha_l}$ and we should require that,

$$p_{k_l}^{\alpha_l} = \sum_\alpha c_{k,\alpha}^{k_l,\alpha_l} p_k^\alpha + \sum_{\alpha'} c_{k,\alpha'}^{k_l,\alpha_l} N_k^{\alpha'}, \tag{42}$$

where in the first summation over $\alpha$, the corresponding EAZ class is B or BDI while in the second summation, the EAZ class for $\alpha'$ is A, AI or AII. Besides, for the second summation, we only consider one in the pair due to chiral symmetry or particle-hole symmetry of $\mathbf{k}$: $\mathcal{C}R_\mathcal{C}$ or $\mathcal{C}R_\Gamma$ must pair $N_k^{\alpha'}$ with $N_k^{\tilde{\alpha'}}$ or $N_k^{\alpha'}$ with $N_k^{\bar{\alpha'}}$ so that they are inverse with each other. Here $(k,\alpha')$ and $(k,\bar{\alpha'})$ are related by the chiral symmetry.

### e. Constructing basis vectors of $\{BS\}_f$ space

Then we are ready to calculate the $\{\mathrm{BS}\}_f$ space, following three steps.

**Step 1:** Obtain constraint equation $Cn_{\mathrm{SC}} = 0$ from all CRs between BLs. Each row of $C$ corresponds a constraint of $n_{\mathrm{SC}}$, which may be of $\mathbb{Z}_2$-type: e.g. if the $i$-th row of the constraint equation is of $\mathbb{Z}_2$-type, it should be viewed as $\sum_{i'} C_{ii'} n_{\mathrm{SC},i'} = 0 \mod 2$. We first consider the constraints on BLs at a given HSP $k$.

The simplest constraint is that for irrep at this HSP owning EAZ class AIII, DIII, CII, C or CI, the BL must be zero (or strictly speaking, there is no BL attributed).

Then consider $R_\mathcal{T}$ which may pair BLs $N_k^\alpha$ or $p_k^\alpha$: If $\alpha$ and $\alpha'$ are paired by $R_\mathcal{T}$, $N_k^\alpha = N_k^{\alpha'}$ or $p_k^\alpha = p_k^{\alpha'} \mod 2$ depending on the EAZ class of $\alpha$ (or $\alpha'$).

In addition, $\mathcal{C}R_\mathcal{C}$ could require that $N_k^\alpha$ and another $N_k^{\tilde{\alpha}}$ are inverse, namely, $N_k^\alpha + N_k^{\tilde{\alpha}} = 0$. Similarly, $\mathcal{C}R_\Gamma$ could also impose similar constraints.

Then we consider the constraints on BLs at two HSPs $k_1$ and $k_2$ which are related with a common $k_l$ as following ($k_l$ can be high-symmetry line, high-symmetry plane, or even generic point),

$$\begin{aligned} R_1k_1 \to k_l, \\ R_2k_2 \to k_l, \end{aligned} \tag{43}$$

where $R_1$ and $R_2$ are MSG elements. Since the irreps at $k_1$ and $R_1k_1$ are related through $R_1$ as well as their BLs, the BLs at $k_1$ are thus related with the BLs at $k_l$. Similarly, the BLs at $k_2$ are related with those at $k_1$.

For *Type 1* constraint, namely, the EAZ class of $\alpha_l$ at $k_l$ is A, AI or AII while the EAZ class of $\alpha_{1(2)}$ at $k_{1(2)}$ is A, AI or AII at $k_1(2)$, we have,

$$\begin{aligned}&\sum_{\alpha_1} c^{k_l,\alpha_l}_{R_1k_1,R_1\alpha_1} N^{\alpha_1}_{k_1} = \\ &\sum_{\alpha_2} c^{k_l,\alpha_l}_{R_2k_2,R_2\alpha_2} N^{\alpha_2}_{k_2},\end{aligned} \tag{44}$$

where $(R_1k_1, R_1\alpha_1)$ represent the irrep at $R_1\alpha_1$ from $\alpha_1$ at $k_1$ by $R_1$ and the same is for others.

For *Type 2* constraint, namely, the EAZ class of $\alpha_l$ at $k_l$ is D or BDI, the EAZ class of $\alpha_{1(2)}$ at $k_{1(2)}$ is A, AI or AII, we would have,

$$\begin{aligned}&\sum_{\alpha_1} c^{k_l,\alpha_l}_{R_1k_1,R_1\alpha_1} p^{\alpha_1}_{k_1} + \sum_{\alpha_1'} c^{k_l,\alpha_l}_{R_1k_1,R_1\alpha_1'} N^{\alpha_1'}_{k_1} = \\ &\sum_{\alpha_2} c^{k_l,\alpha_l}_{R_2k_2,R_2\alpha_2} p^{\alpha_2}_{k_2} + \sum_{\alpha_2'} c^{k_l,\alpha_l}_{R_2k_2,\alpha_2'} N^{\alpha_2'}_{k_2} \mod 2.\end{aligned} \tag{45}$$

Other than the above constraints, we may be encountered with the following situation, since the HSPs we consider are thought to be inequivalent with each other when they can not be related with any other by MSG operation, thus there is a possibility that two HSPs can be related by $\mathcal{C}$, denoted as $k_1$ and $k_2$ and $\mathcal{C}$ can pair $N^{\alpha_1}_{k_1}$ with $N^{\alpha_2}_{k_2}$ by $N^{\alpha_1}_{k_1} + N^{\alpha_2}_{k_2} = 0$.

Consider all inequivalent $\{k_l\}$'$s$ (namely, they are not related by any MSG operation) and all the above constraints, we thus obtain $Cn_{\text{SC}} = 0$, some row of which may be $\mathbb{Z}_2$-CR. Then we go to the next step.

**Step 2.** First release the possible $\mathbb{Z}_2$-CRs to be $\mathbb{Z}$-ones. Suppose $\eta_1$ is a set containing all row indices of $Cn_{\text{SC}} = 0$ corresponding to normal $\mathbb{Z}$ CRs while $\eta_2$ is a set containing all row indices which correspond to $\mathbb{Z}_2$-CRs. Hence, we write $Cn_{\text{SC}} = 0$ as the following form,

$$\begin{aligned}&\sum_{j=1}^{D} C_{i_1j} n^f_{\text{SC}j} = 0, \\ &\sum_{j=1}^{D} C_{i_2j} n^f_{\text{SC}j} = 0 \mod 2 \Rightarrow \sum_{i_2\in r_2} C_{i_2j} n^f_{\text{SC}j} + 2n'_{i_2} = 0,\end{aligned} \tag{46}$$

where $i_{1(2)} \in \eta_{1(2)}$, $D$ is the length of $n_{\text{SC}}$, and we attribute superscript $f$ in $n_{\text{SC}}$ indicating that the $\mathbb{Z}_2$-components have also been released to take any integers. Besides, we also extend $n^f_{\text{SC}}$ to be $n'' = (n^f_{\text{SC}}, n')$ (the length of $n'$ is the number of $\mathbb{Z}_2$-CRs). From Eq. 46, we thus obtain a new constraint equation, of which each constraint is integer-valued,

$$C'n'' = 0, \tag{47}$$

whose solution can be found as a combination of basis vectors $\{v_i\}$ with the combination coefficients $c_i$ being integers:

$$n'' = \sum_{i=1}^{d'} c_i v_i. \tag{48}$$

**Step 3.** From Eq. 48, we can obtain the basis vectors of $\{\text{BS}\}_f$ by taking only the first $D$ entries of each $v_i$, denoted as $\mathbf{b}'_i$. Note that any basis vector in $\{v_i\}_i$ would not own common factor larger than 1, but for $\{\mathbf{b}'_i\}$, it is allowed that some basis vector may own common factor large than 1. This is why we need to construct bases for both BS and AI spaces for superconductors.

### *f. Constructing ALs exhaustively and find basis vectors of $\{AI\}_f$ space*

The $\{\text{AI}\}_f$ space can be obtained in a similar way as constructing AI space for normal states, while the only point that need to be taken care of is a different definition of BS as $n_{\text{SC}}$, which can derived from $n^{\alpha}_{k}$ and $n^{\alpha'}_{-k}$. To exhaustively construct all possible

AIs for superconductors, one only need to exhaustively consider all Wyckoff positions and all corresponding site-symmetry group irreps or co-irreps (when the site-symmetry group contains colored elements). Given a Wyckoff position, which contains a finite number $d_s$ of sites in the primitive unit cell which are related by MSG operations, denoted as $\{\boldsymbol{\tau}_1, \boldsymbol{\tau}_2, \boldsymbol{\tau}_3, \ldots, \boldsymbol{\tau}_{d_s}\}$. Focus on the first site $\boldsymbol{\tau}_1$. Let all MSG operations that leave the site to be itself constitute a group $\mathcal{M}_{\boldsymbol{\tau}_1}$, which should be isomorphic to a point group which may be of type-I,II or III. Any other site can be generated through an MSG operation from $\boldsymbol{\tau}_1$: $\boldsymbol{\tau}_i = R_i\boldsymbol{\tau}_1$. For type I and II MSGs, all $\{R_i\}$'$s$ can be chosen to be uncolored. For type-III and IV MSGs, if $\mathcal{M}_{\tau_1}$ owns colored elements, it is found that all $R_i$'$s$ can be chosen to be uncolored otherwise half of $R_i$'$s$ can be chosen to be uncolored, while the rest half cannot.

Take an irrep or co-irrep $\xi$ (whose dimension is $d_\xi$) of $\mathcal{M}_{\boldsymbol{\tau}_1}$, whose basis functions are denoted by $\phi_j^\xi(\mathbf{r}-\boldsymbol{\tau}_1), j = 1, 2, d_\xi$. Thus the basis functions for the whole MSG can be found as $\{E|\mathbf{R}_l\}R_i\phi_j^\xi(\mathbf{r}-\boldsymbol{\tau}_1)$. To obtain $n_{\text{SC}}$ for such basis functions, we can obtain the following Bloch summations for HSP $k$ and $-k$,

$$
\begin{aligned}
\phi^\xi_{j,\tau_i,\mathbf{k}} &= \sum_l e^{i\mathbf{k}\cdot\mathbf{R}_l}\{E|\mathbf{R}_l\}R_i\phi_j^\xi(\mathbf{r}-\boldsymbol{\tau}_1), \text{and},\\
\phi^\xi_{j,\tau_i,-\mathbf{k}} &= \sum_l e^{-i\mathbf{k}\cdot\mathbf{R}_l}\{E|\mathbf{R}_l\}R_i\phi_j^\xi(\mathbf{r}-\boldsymbol{\tau}_1),
\end{aligned} \tag{49}
$$

respectively, and then operate little group operation (uncolored) $\{\alpha|\mathbf{t}\} \in \mathcal{G}_\mathbf{k}$ on them:

$$
\begin{aligned}
\{\alpha|\mathbf{t}\}\phi^\xi_{j,\tau_i,\mathbf{k}} &= \sum_l e^{i\mathbf{k}\cdot\mathbf{R}_l}\{E|\alpha\mathbf{R}_l+\mathbf{R}\}R_{i'}O\phi_j^\xi(\mathbf{r}-\boldsymbol{\tau}_1), \text{and},\\
\{\alpha|\mathbf{t}\}\phi^\xi_{j,\tau_i,-\mathbf{k}} &= \sum_l e^{-i\mathbf{k}\cdot\mathbf{R}_l}\{E|\alpha\mathbf{R}_l+\mathbf{R}\}R_{i'}O\phi_j^\xi(\mathbf{r}-\boldsymbol{\tau}_1),
\end{aligned} \tag{50}
$$

where $\{\alpha|\mathbf{t}\}R_i = \{E|\mathbf{R}\}R_{i'}O$ $(O \in \mathcal{M}_{\tau_1})$. Hence, the character of $\{\alpha|\mathbf{t}\}$ should be:

$$
\begin{aligned}
\chi(\{\alpha|\mathbf{t}\}) &= \sum_i \delta_{ii'}e^{-i\mathbf{k}\cdot\mathbf{R}}\chi^\xi(O), \text{and},\\
\chi(\{\alpha|\mathbf{t}\}) &= \sum_i \delta_{ii'}e^{i\mathbf{k}\cdot\mathbf{R}}\chi^\xi(O),
\end{aligned} \tag{51}
$$

respectively.

Using Eq. 51, we thus can obtain $n_k^\alpha$ and $n_{-k}^{\alpha'}$. Then from EAZ classes for HSPs, we can obtain the corresponding BLs, or $n_{\text{SC}}$. Consider all Wyckoff positions and all site-symmetry-group irreps or co-irreps, we thus obtain a set of $\{n_{\text{SC}}^{\tau_1,\xi}\}$'$s$.

Any AI should be written as linear combinations of these AIs with the coefficients being non-negative integers while we can extend the coefficients to take any integers. Furthermore, when some BL is $\mathbb{Z}_2$-valued, supposed to be the $p$-th component, we introduce an additional "AI" (denoted as $n_{a,p}$) which also owns $D$ entries with only the $p$-th entry being 2 while the rest vanishing. Hence, we obtain $\{\text{AI}\}^f$ from $n_{\text{SC}}^{\tau_1,\xi}$'$s$ and $n_{a,p}$'$s$. The $d'$ basis vectors of the resulting $\{\text{AI}\}_f$ space can then be found through standard Smith decomposition: $\mathbf{a}_i', i = 1, 2, \ldots, d'$ so that any AI can be expressed as integer multiples of them. Note that here the dimension $d'$ is the same as that of $\{\text{BS}\}^f$ space.

### g. *Get regularized basis vectors of* $\{BS\}_f$ *and* $X_f$

So far we have got ready to derive the symmetry-indicator (SI) group for the MSG assuming a pairing belonging to the 1D single-valued irrep of the PG. Since any AI should satisfy the constraints $Cn_{\text{SC}} = 0$, $\mathbf{a}_i'$ can be expressed by

$$
\mathbf{a}_i' = \sum_j \Lambda_{ji}\mathbf{b}_j', \Lambda_{ji} \in \mathbb{Z}. \tag{52}
$$

Through Smith decomposition of $\Lambda_{ji}$, we can find a integer-valued transformation matrix $P$ (whose inverse is also integer-valued), so that $\Lambda P = (\mathbf{e}_1, \mathbf{e}_2, \ldots, \mathbf{e}_{d'})$ where $\mathbf{e}_i$ has been made own large common factor as far as possible and the common factors $s_i$ of $\mathbf{e}_i, i = 1, 2, \ldots, d'$ satisfy: $s_1 \le s_2 \le s_3 \ldots \le s_{d'-1} \le s_{d'}$. Thus we obtain the regularized basis vectors for $\{\text{AI}\}_f$ space, $\mathbf{a}_i$ and $\{\text{BS}\}_f$ space, $\mathbf{b}_i$:

$$
\begin{aligned}
\mathbf{a}_i &= \sum_j (\Lambda P)_{ji}\mathbf{b}_j',\\
\mathbf{b}_i &= \frac{\mathbf{a}_i}{s_i}.
\end{aligned} \tag{53}
$$

From basis vectors of $\{\text{BS}\}_f$ and $X_f$, we can obtain bases for $\{\text{BS}\}$ and the factors $S$ by recovering the $\mathbb{Z}_2$-ness in $n_{\text{SC}}$.

## C. THE STRATEGY OF DEALING WITH CASES WHEN PAIRING BREAKING COLORED SYMMETRY

As mentioned before, we may be encountered with superconducting pairings that belong to 1D single-valued irreps of PG but violate Eq. 30, namely, breaking colored-symmetries in $A\mathcal{G}$ (reducing $\mathcal{M} = \mathcal{G} + A\mathcal{G}$ to $\mathcal{G}$). Here we show a strategy of dealing with such as in the following. We may even be encountered with higher-dimensional irreps or multiple 1D irreps characterizing the pairings, which could also break symmetries in $\mathcal{G}$. We leave this general symmetry-breaking situation as a future study.

Due to the lack of colored symmetries, $W_k^\alpha(\mathcal{C})$ and $W_k^\alpha(\Gamma)$ would always be zero. For the construction of $\{\text{BS}\}_f$ space, we only need to note that: 1. Constraints on $N_{\mathbf{k}}^\alpha$ and $N_{\mathbf{k}}^{\alpha'}$ which should be equal due to $R_{\mathcal{T}}\mathcal{T}$, should be released. So are those on $p_{\mathbf{k}}^\alpha$ and $p_{\mathbf{k}}^{\alpha'}$;

2. The constraints arising from $R_1 k_1 \to k_l, R_2 k_2 \to k_l$ should be released when $R_1$ or $R_2$ must be colored elements.

Following the same steps shown above, we can solve the released constraint equation $C n_{\text{SC}} = 0$, and obtain the corresponding basis vectors of $\{\text{BS}\}_f$.

With respect to AIs. We classify the original Wyckoff positions into two types: For one type, the symmetry group $\mathcal{G}_{\boldsymbol{\tau}_1}$ owns colored elements while for the other, $\mathcal{G}_{\boldsymbol{\tau}_1}$ contains only uncolored elements. For the former case, the sites $\{\boldsymbol{\tau}_i = R_i \boldsymbol{\tau}_1\}$ are not changed and $R_i$ which can always be chosen to be uncolored. When $A$-breaking pairing is formed, all colored elements are lost. Then $\mathcal{G}_{\boldsymbol{\tau}_1}$ is reduced.

For the latter case, where the number of sites in one primitive unit cell should be even, namely $d_s \mod 2 = 0$. With no loss of generality, we require that $R_i, i = 1, 2, \ldots, d_s/2$ are uncolored while the rest are colored. When $A$-breaking pairing is formed, the sites in the original setting would split into two parts: $\{\boldsymbol{\tau}_1, \boldsymbol{\tau}_2, \ldots, \boldsymbol{\tau}_{d_s/2}\}$ and $\{\boldsymbol{\tau}_{d_s/2+1}, \boldsymbol{\tau}_{d_s/2+2}, \ldots, \boldsymbol{\tau}_{d_s}\}$. We then consider each site separately. It is worth pointing out that these two sets of sites can be related with the colored element in the original MSG, thus their AIs are also related by the colored element.

After obtaining all $n_{\text{SC}}$'s for all AIs in this case, we can thus obtain the basis vectors for $\{\text{AI}\}_f$ space. Then following Sec. B 2 g, we can obtain $S = (s_1, s_2, \ldots, s_d)$ and $\{\mathbf{b}_i\}_{i=1}^d$ for the $A$-breaking pairing.

## D. REMARKS ON THE BILBAO NOTATIONS

We perform the construction of BS bases as well as the first-principles calculations of irreps at $k$ points based on our order of $k$ points, little group operations and the irreps (the convention, namely, the origin and orientation of crystal axes, is exactly the same as that of default setting on the Bilbao server). We compare our $k$ points and the irreps of little groups. We first note that the character of translation operation is given by $e^{i\mathbf{k}\cdot\mathbf{R}_l}$, while ours is its complex conjugate, thus we take complex conjugate of all irreps of little groups listed on the Bilbao server and then compare with ours. Besides, it should be pointed out that for SGs 22, 42,43, 69, 70, the $k$ points we use actually lie in HSLs. We list explicitly the coordinates of these $k$ points and the coordinates of HSLs on the Bilbao server in Table 2. The coordinates are all given based on the conventional lattice. Note that for HSLs $A$ and $B$ as listed in Table 2, the irreps of their little groups are related by SG operation with the explicit irreps of the HSLs $A$ and $B$ shown on the Bilbao server ($(u, 0, 1)$ and $(0, v, 1)$, respectively), namely, the HSLs $A$ and $B$ there and those here constitute a wave vector star.

| SG | $\mathbf{k}$ | HSL | $\mathcal{G}$ |
|---|---|---|---|
| 22,42,43,69,70 | $(\frac{1}{2}, 1, 0)$ | $A : (-u, 0, 1)$ | $(-3, 1, -1)$ |
| 22,42,43,69,70 | $(0, 1, -\frac{1}{2})$ | $H : (0, 1, w)$ | $(0, 0, -4)$ |
| 22,42,43,69,70 | $(-1, \frac{1}{2}, 0)$ | $B : (0, -v, 1)$ | $(-1, -3, -1)$ |

Supplementary Table 2. The $k$ points in SGs 22, 42, 43, 69, 70 used in our calculations, whose coordinates are given in the second column, actually lie in HSLs as listed on the Bilbao server (the third column). It is easy to find that $\mathbf{k} - \mathbf{G}$ (a reciprocal lattice vector), lie in the respective HSL.

Furthermore, for trigonal or hexagonal lattices, namely SGs 143-194, we adopt that the (right-hand) Cartesian system are chosen as schematically shown in Fig. 1, where $\mathbf{a}_H$ and $\mathbf{b}_H$ are hexagonal lattice basis vectors. This is necessary to compare the spin-space rotations.

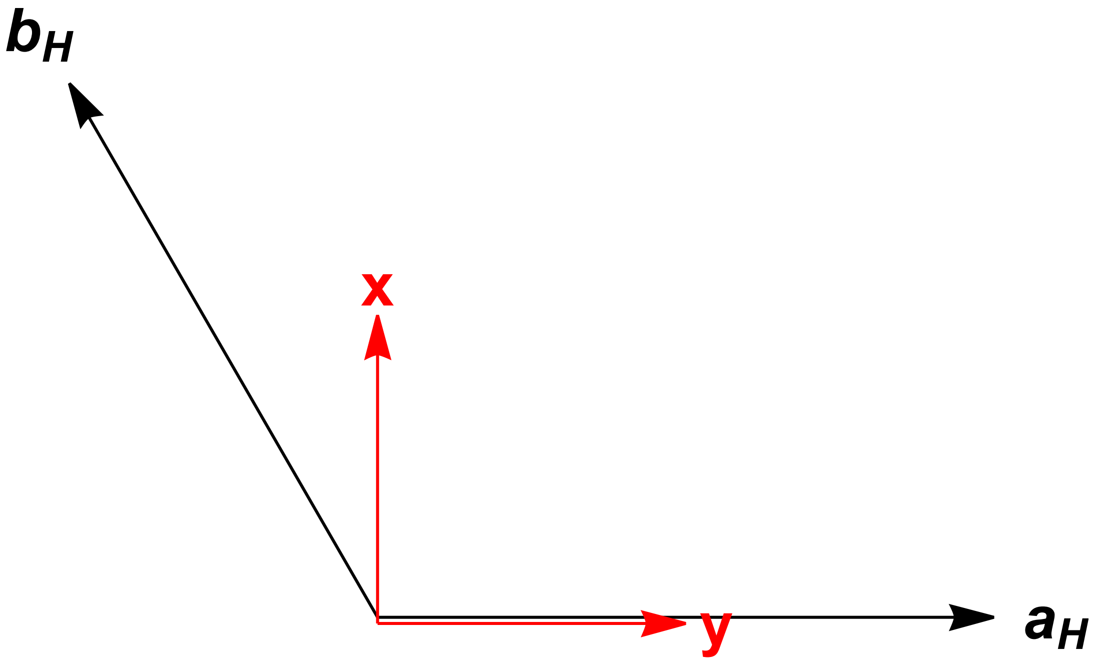


FIG. 1. The Cartesian system (right-hand) for SGs 143-194.

## E. SUBROUTINE *TOPOLOGICALSUPERCON*

### 1. Generating inputs

*TopologicalSupercon* is a subroutine, which can quickly diagnose possible topological and nodal superconductivity based on symmetry-indicator method for any material. Users can use this subroutine just by uploading a particularly formatted result of first-principles calculations. In this document, we explain how to prepare the input file and how to run the program.

#### a. *Formatting results of first-principles calculations*

The input file must contain symmetry operations and characters of irreducible representations for each band in a particular format. Although one can make it by oneself, three external programs (*vasp2trace* [3], *irvsp* [**?** ], and *qeirreps* [4]) can automatically generate it. To use our subroutine for superconductors, there are two additional things to do. One is to add the Fermi energy to the first line of the input produced by the above external programs. The other is to compute the characters of the hole-bands below the Fermi energy and include them in the input. In other words, one should take into account the partially filled bands in the computations for superconductors.

#### b. *Precautions on convention*

When one generates an input, one should pay attention to the convention. In first-principles calculations, one must follow the following settings (These assumptions will be removed from the next update):

(i) For space groups No. 3–15 (Monoclinic space groups), the rotation axis and the direction perpendicular to the mirror plane are set to the $+y$-axis.

(ii) For space groups No. 75–139 (Tetragonal space groups), the four-fold rotation axis is set to the $+z$-axis.

(iii) For space groups No. 143–194 (Trigonal and Hexagonal space groups), the three-fold or the six-fold rotation axes are set to the $+z$-axis.

(iv) For any space group, the spin-quantization axis is set to the $+z$-axis.

(v) The primitive lattice vectors $(\boldsymbol{a}, \boldsymbol{b}, \boldsymbol{c})$ are chosen in the same way as Table 3.

Supplementary Table 3. **Primitive lattice vectors.** When one performs first-principles calculations, one needs to choose the primitive lattice vectors in the same way as the following table. Here, $a, b, c$, and $\gamma$ are independent lattice parameters. In the output of the subroutine, the parameters are set to $a = b = c = 1$ and $\gamma = \pi/2$.

| Lattice | $(\boldsymbol{a}, \boldsymbol{b}, \boldsymbol{c})$ | Lattice | $(\boldsymbol{a}, \boldsymbol{b}, \boldsymbol{c})$ |
|---|---|---|---|
| Monoclinic primitive | $\begin{pmatrix} a & 0 & -c\cos(\gamma) \\ 0 & b & 0 \\ 0 & 0 & c\sin(\gamma) \end{pmatrix}$ | Monoclinic base-centered | $\begin{pmatrix} \frac{1}{2}a\sin(\gamma) & -\frac{1}{2}a\sin(\gamma) & 0 \\ \frac{b}{2} & \frac{b}{2} & 0 \\ \frac{1}{2}a\cos(\gamma) & -\frac{1}{2}a\cos(\gamma) & c \end{pmatrix}$ or $\begin{pmatrix} \frac{1}{2}a\sin(\gamma) & \frac{1}{2}a\sin(\gamma) & 0 \\ -\frac{b}{2} & \frac{b}{2} & 0 \\ \frac{1}{2}a\cos(\gamma) & -\frac{1}{2}a\cos(\gamma) & c \end{pmatrix}$ |
| Orthorhombic primitive | $\begin{pmatrix} a & 0 & 0 \\ 0 & b & 0 \\ 0 & 0 & c \end{pmatrix}$ | Orthorhombic base-centered | $\begin{pmatrix} \frac{a}{2} & -\frac{a}{2} & 0 \\ \frac{b}{2} & \frac{b}{2} & 0 \\ 0 & 0 & c \end{pmatrix}$ or $\begin{pmatrix} \frac{a}{2} & \frac{a}{2} & 0 \\ -\frac{b}{2} & \frac{b}{2} & 0 \\ 0 & 0 & c \end{pmatrix}$ |
| Orthorhombic body-centered | $\begin{pmatrix} -\frac{a}{2} & \frac{a}{2} & \frac{a}{2} \\ \frac{b}{2} & -\frac{b}{2} & \frac{b}{2} \\ \frac{c}{2} & \frac{c}{2} & -\frac{c}{2} \end{pmatrix}$ or $\begin{pmatrix} \frac{a}{2} & -\frac{a}{2} & \frac{a}{2} \\ \frac{b}{2} & -\frac{b}{2} & -\frac{b}{2} \\ \frac{c}{2} & \frac{c}{2} & -\frac{c}{2} \end{pmatrix}$ | Orthorhombic face-centered | $\begin{pmatrix} \frac{a}{2} & 0 & \frac{a}{2} \\ 0 & \frac{b}{2} & \frac{b}{2} \\ \frac{c}{2} & \frac{c}{2} & 0 \end{pmatrix}$ or $\begin{pmatrix} \frac{a}{2} & 0 & \frac{a}{2} \\ 0 & -\frac{b}{2} & -\frac{b}{2} \\ \frac{c}{2} & \frac{c}{2} & 0 \end{pmatrix}$ |
| Tetragonal primitive | $\begin{pmatrix} a & 0 & 0 \\ 0 & a & 0 \\ 0 & 0 & c \end{pmatrix}$ | Tetragonal body-centered | $\begin{pmatrix} -\frac{a}{2} & \frac{a}{2} & \frac{a}{2} \\ \frac{a}{2} & -\frac{a}{2} & \frac{a}{2} \\ \frac{c}{2} & \frac{c}{2} & -\frac{c}{2} \end{pmatrix}$ |
| Rhombohedral | $\begin{pmatrix} \frac{a}{2} & -\frac{a}{2} & 0 \\ \frac{a}{2\sqrt{3}} & \frac{a}{2\sqrt{3}} & -\frac{a}{\sqrt{3}} \\ \frac{c}{3} & \frac{c}{3} & \frac{c}{3} \end{pmatrix}$ | Hexagonal | $\begin{pmatrix} a & -\frac{a}{2} & 0 \\ 0 & \frac{\sqrt{3}}{2}a & 0 \\ 0 & 0 & c \end{pmatrix}$ |
| Cubic primitive | $\begin{pmatrix} a & 0 & 0 \\ 0 & a & 0 \\ 0 & 0 & a \end{pmatrix}$ | Cubic face-centered | $\begin{pmatrix} 0 & \frac{a}{2} & \frac{a}{2} \\ \frac{a}{2} & 0 & \frac{a}{2} \\ \frac{a}{2} & \frac{a}{2} & 0 \end{pmatrix}$ |
| Cubic body-centered | $\begin{pmatrix} -\frac{a}{2} & \frac{a}{2} & \frac{a}{2} \\ \frac{a}{2} & -\frac{a}{2} & \frac{a}{2} \\ \frac{a}{2} & \frac{a}{2} & -\frac{a}{2} \end{pmatrix}$ | A type lattices | $\begin{pmatrix} 0 & 0 & c \\ \frac{a}{2} & -\frac{a}{2} & 0 \\ \frac{b}{2} & \frac{b}{2} & 0 \end{pmatrix}$ or $\begin{pmatrix} c & 0 & 0 \\ 0 & \frac{a}{2} & -\frac{a}{2} \\ 0 & \frac{b}{2} & \frac{b}{2} \end{pmatrix}$ |

## F. DETAILS OF ANALYSES OF MATERIAL EXAMPLES

Here, we demonstrate our computation process using BaPtP with ${}^1E$ pairing and BaPtSb with $A_1''$ pairing as examples.

### 1. BaPtP with ${}^1E$ pairing

First, we identify the EAZ class for each irrep. The EAZ class for $\Gamma_6$ is class C; those for $M_5$, $R_5$, and $R_7$ are class D; those for the rest of irreps are class A. In other words, there are no BLs for $\Gamma_6$; $\mathbb{Z}_2$-valued BLs are assigned to $M_5$, $R_5$, and $R_7$; integer-valued BLs are defined for the rest of irreps.

Next, we perform the first-principles calculation and find counts of irreps at each high-symmetry momenta

$$\begin{aligned}&(n_\Gamma^5, n_\Gamma^6, n_\Gamma^7, n_X^2, n_X^3, n_X^4, n_X^5, n_M^5, n_R^4, n_R^5, n_R^6, n_R^7)\\&\quad= (31, 30, 30, 45, 45, 45, 45, 90, 14, 16, 16, 46).\end{aligned} \tag{54}$$

Using the formulas $p_{\boldsymbol{k}}^\alpha = n_{\boldsymbol{k}}^\alpha \bmod 2$ and $N_{\boldsymbol{k}}^\alpha = n_{\boldsymbol{k}}^\alpha - n_{\boldsymbol{k}}^\gamma$, we obtain the following $\boldsymbol{n}_{\mathrm{SC}}$ based on weak-pairing assumption:

$$\begin{aligned}\boldsymbol{n}_{\mathrm{SC}} &= (N_\Gamma^5, N_\Gamma^7, N_X^2, N_X^3, N_X^4, N_X^5, p_M^5, N_R^4, p_R^5, N_R^6, p_R^7),\\&= (1, -1, 0, 0, 0, 0, 0, -2, 0, 2, 0).\end{aligned}$$

Finally, we check whether the above BLs satisfy all CRs. We find that $C\boldsymbol{n}_{\mathrm{SC}} \neq \boldsymbol{0}$, which implies that the superconductor is a NSC. From nonzero elements in $C\boldsymbol{n}_{\mathrm{SC}}$, we find that CRs in the $\Gamma - R$ line are violated. More concretely, BLs should satisfy $N_\Gamma^7 = N_R^4$, $N_\Gamma^5 = N_R^6$, and $N_\Gamma^5 + N_\Gamma^7 = 0$ when the Bogoliubov quasi-particle spectrum is fully gapped. One can explicitly see that the first and second CRs are violated, which guarantees that two gapless points exist in this line. Furthermore, by checking the CRs between this line and its neighborhood, we find that the gapless points in this line are actually part of a surface node. The analysis is the same for the ${}^2E$ pairing.

To show that the system is expected to exhibit surface nodes, we here discuss a low-energy effective model along the $\Gamma$-R line. The little co-group of any point in the $\Gamma$-R line contains only the three-fold rotation symmetry along the line. Since there are two violated compatibility relations along the line, two gapless points must exist on the line. Let us start with the case where the two gapless points are at the same position. Then, the effective model is

$$\begin{aligned}h_{\boldsymbol{q}} &= q_1\sigma_x + q_2\sigma_y + q_3\sigma_z,\\U(C_3) &= \mathrm{diag}\left(-1, e^{-i\frac{\pi}{3}}\right),\end{aligned}$$

where $\boldsymbol{q} = (q_1, q_2, q_3)$ is the displacement from the gapless points. However, there are no reasons why the two gapless points on the line are forced to be in the same position. Indeed, we can add the mass term $M = m\sigma_0$, which shifts positions of the two gapless points. After computing the energy spectrum of $h_{\boldsymbol{q}} + M$, we obtain $E_{\boldsymbol{q}} = \pm\sqrt{q_1^2 + q_2^2 + q_3^2} + m$. Thus, one can find that the two gapless points are part of a spherical node.

### 2. BaPtP with $T$ pairing

Here, we consider the three-dimensional irrep $T$, which can be decomposed into $B_1 \oplus B_2 \oplus B_3$ of point group $D_2$ or $A \oplus^1 E \oplus^2 E$ of point group $C_3$. As discussed in the main text, when the pairing symmetry is a multi-dimensional irrep, some symmetries must be broken. Then, we here assume that $\mathcal{D}(g)$ is either one of $B_1$, $B_2$, or $B_3$ of $D_2$.

The first thing we have to do is map the counts of irreps in Eq. (54) to those in the lowered space group. This can be achieved by referring to Supplemental Materials II. We obtain the counts of irreps of space group $P2_12_12_1$

$$\begin{aligned}&(n_\Gamma^5, n_X^2, n_X^3, n_X^4, n_X^5, n_S^5, n_R^2, n_R^3, n_R^4, n_R^5, n_U^5, n_Z^2, n_Z^3, n_Z^4, n_Z^5, n_T^5, n_Y^2, n_Y^3, n_Y^4, n_Y^5)\\&\quad= (91, 45, 45, 45, 45, 90, 46, 46, 46, 46, 90, 45, 45, 45, 45, 90, 45, 45, 45, 45).\end{aligned} \tag{55}$$

Next, we discuss $B_1$ pairing. In the weak-pairing assumption, we get the following band labels:

$$\begin{aligned}&(p_\Gamma^5, N_X^2, N_X^3, N_X^4, N_X^5, N_R^2, N_R^3, N_R^4, N_R^5, p_Z^2, p_Z^3, p_Z^4, p_Z^5, N_Y^2, N_Y^3, N_Y^4, N_Y^5)\\&\quad= (1, 0, 0, 0, 0, 0, 0, 0, 0, 1, 1, 1, 1, 0, 0, 0, 0).\end{aligned}$$

There exists the following compatibility conditions

$$p_\Gamma^5 = p_Z^2 + p_Z^4 \mod 2;$$
$$p_\Gamma^5 = p_Z^3 + p_Z^5 \mod 2.$$

As one can see from Eq. 56, both compatibility conditions are violated. Thus, the gapless points must exist on the Γ-Z line. Furthermore, by checking the CRs between this line and its neighborhood, we find that the gapless points in this line are actually part of line nodes. The same analysis is applicable to $B_2$ and $B_3$ pairings.

### 3. BaPtSb with $A_1''$ pairing

In the same way as BaPtP, we analyze the topological and nodal nature. The EAZ classes for $\Gamma_7$, $M_5$, $A_7$, and $L_5$ are class BDI; those for the rest of irreps at high-symmetry momenta are class AI. That is, $\mathbb{Z}_2$-valued BLs are assigned to $\Gamma_7$, $M_5$, $A_7$, and $L_5$; integer-valued BLs are defined for the rest of irreps. Again, from the first-principle calculation, we find

$$\begin{aligned}&(n_\Gamma^7, n_\Gamma^8, n_\Gamma^9, n_M^5, n_K^7, n_K^8, n_K^9, n_K^{10}, n_K^{11}, n_K^{12},\\ &\quad n_A^7, n_A^8, n_A^9, n_L^5, n_H^7, n_H^8, n_H^9, n_H^{10}, n_H^{11}, n_H^{12})\\ &= (8, 9, 9, 28, 9, 10, 8, 9, 10, 8, 8, 8, 10, 28, 10, 9, 9, 9, 9, 10).\end{aligned}$$

Based on the above counts of irreps in the normal conducting phase, we obtain $\boldsymbol{n}_{\mathrm{SC}}$ as

$$\begin{aligned}\boldsymbol{n}_{\mathrm{SC}} &= (p_\Gamma^7, N_\Gamma^8, N_\Gamma^9, p_M^5, N_K^7, N_K^8, N_K^9, N_K^{10}, N_K^{11}, N_K^{12},\\ &\quad p_A^7, N_A^8, N_A^9, p_L^5, N_H^7, N_H^8, N_H^9, N_H^{10}, N_H^{11}, N_H^{12})\\ &= (0, 0, 0, 0, -1, 1, -1, 1, 2, -2, 0, -2, 2, 0, 1, -1, 0, 0, -1, 1).\end{aligned}$$

We can quickly find that $\boldsymbol{n}_{\mathrm{SC}}$ satisfies all CRs from the fact that we can expand $\boldsymbol{n}_{\mathrm{SC}}$ as $\boldsymbol{n}_{\mathrm{SC}} = 3\mathbf{b}_2 - 4\mathbf{b}_3 - 7\mathbf{b}_4 - 10\mathbf{b}_5 + 3\mathbf{b}_6 + 2\mathbf{b}_7 - \mathbf{b}_9 + 5\mathbf{b}_{10}$, where $\{\mathbf{b}_i\}_{i=1}^{10}$ are shown in

| | $\mathbf{b}_1$ | $\mathbf{b}_2$ | $\mathbf{b}_3$ | $\mathbf{b}_4$ | $\mathbf{b}_5$ | $\mathbf{b}_6$ | $\mathbf{b}_7$ | $\mathbf{b}_8$ | $\mathbf{b}_9$ | $\mathbf{b}_{10}$ |
|---|---|---|---|---|---|---|---|---|---|---|
| $s_i$ | 1 | 1 | 1 | 1 | 2 | 2 | 2 | 2 | 6 | 6 |
| $p_\Gamma^7$ | 1 | 0 | 0 | 0 | 0 | 0 | 0 | 1 | 0 | 0 |
| $N_\Gamma^8$ | 0 | 1 | −4 | 7 | −3 | 0 | 3 | −3 | 1 | −1 |
| $N_\Gamma^9$ | 0 | −1 | 4 | −7 | 3 | 0 | −3 | 3 | −1 | 1 |
| $p_{\mathrm{M}}^5$ | 1 | 1 | 0 | 1 | 0 | 0 | 0 | 1 | 1 | 1 |
| $N_{\mathrm{K}}^7$ | 0 | 0 | 2 | −1 | 0 | 0 | 0 | 0 | 0 | 0 |
| $N_{\mathrm{K}}^8$ | 0 | 0 | −2 | 1 | 0 | 0 | 0 | 0 | 0 | 0 |
| $N_{\mathrm{K}}^9$ | 0 | 1 | −5 | 12 | −6 | 0 | 6 | −6 | 2 | −2 |
| $N_{\mathrm{K}}^{10}$ | 0 | −1 | 5 | −12 | 6 | 0 | −6 | 6 | −2 | 2 |
| $N_{\mathrm{K}}^{11}$ | 0 | −1 | 3 | −11 | 6 | 0 | −6 | 6 | −2 | 2 |
| $N_{\mathrm{K}}^{12}$ | 0 | 1 | −3 | 11 | −6 | 0 | 6 | −6 | 2 | −2 |
| $p_{\mathrm{A}}^7$ | 1 | 0 | 0 | 0 | 0 | 0 | 0 | 0 | 0 | 0 |
| $N_{\mathrm{A}}^8$ | 0 | 1 | −2 | 3 | −1 | −1 | 3 | 0 | 0 | −1 |
| $N_{\mathrm{A}}^9$ | 0 | −1 | 2 | −3 | 1 | 1 | −3 | 0 | 0 | 1 |
| $p_{\mathrm{L}}^5$ | 1 | 1 | 0 | 1 | 0 | 0 | 0 | 0 | 0 | 0 |
| $N_{\mathrm{H}}^7$ | 0 | 0 | −2 | 7 | −4 | 1 | 3 | −6 | 2 | −1 |
| $N_{\mathrm{H}}^8$ | 0 | 0 | 2 | −7 | 4 | −1 | −3 | 6 | −2 | 1 |
| $N_{\mathrm{H}}^9$ | 0 | 1 | −1 | 4 | −2 | 0 | 3 | 0 | 0 | −1 |
| $N_{\mathrm{H}}^{10}$ | 0 | −1 | 1 | −4 | 2 | 0 | −3 | 0 | 0 | 1 |
| $N_{\mathrm{H}}^{11}$ | 0 | −1 | 3 | −11 | 6 | −1 | −6 | 6 | −2 | 2 |
| $N_{\mathrm{H}}^{12}$ | 0 | 1 | −3 | 11 | −6 | 1 | 6 | −6 | 2 | −2 |

As explained above, $\{r_i \bmod s_i\}_{i=1}^{10}$ tell us the entry of SIs. Then, the entry of SIs can be easily found to be $(0, 1, 0, 0, 5, 5) \in (\mathbb{Z}_2)^4 \times (\mathbb{Z}_6)^2$ in our choice of bases. Note that the entry of SIs depends on the choice of a basis set of $\{\mathrm{BS}\}$.

We can compute the mirror Chern numbers $C_M^{k_z=0,\pi}$ by the following formulas [5, 6]

$$C_M^{k_z=0} = N_\Gamma^8 - N_\Gamma^9 + \frac{3}{2}N_{\rm K}^7 + \frac{3}{2}N_{\rm K}^8 + \frac{1}{2}N_{\rm K}^9 - \frac{1}{2}N_{\rm K}^{10} - \frac{1}{2}N_{\rm K}^{11} + \frac{1}{2}N_{\rm K}^{12} \bmod 3,$$
$$C_M^{k_z=\pi} = N_A^8 - N_A^9 + \frac{3}{2}N_{\rm H}^7 + \frac{3}{2}N_{\rm H}^8 + \frac{1}{2}N_{\rm H}^9 - \frac{1}{2}N_{\rm H}^{10} - \frac{1}{2}N_{\rm H}^{11} + \frac{1}{2}N_{\rm H}^{12} \bmod 3.$$

Applying the formulas to $\boldsymbol{n}_{\rm SC}$, one can see $(C_M^{k_z=0}, C_M^{k_z=\pi}) = (0,1) \bmod 3$.

### 4. Detailed information on $\mathbf{CsV_3Sb_5}$

In this section, we show all results for 'Star of David' and 'Tri-Hexagonal' structures of $CsV_3Sb_5$, including the cases where the Fermi energies are changed. Here, we also discuss the symmetry indicators for the $A_{1u}$ representation of space group $P6/mmm$.

Although an entry of SIs might correspond to various topological phases, SIs can partially determine topology that must exist in the material. We define the following indices:

$$z_{8,I} \equiv \left[\left(N_\Gamma^7 + N_\Gamma^8 + N_\Gamma^9\right) + 3N_{\rm M}^5 + \left(N_{\rm A}^7 + N_{\rm A}^8 + N_\Gamma^9\right) + 3N_{\rm L}^5\right] \quad (56)$$
$$z_{m,C_6}^{k_z=0} \equiv \frac{1}{2}\left(N_\Gamma^9 - N_\Gamma^{12}\right) + \frac{3}{2}\left(N_\Gamma^{10} - N_\Gamma^7\right) + \frac{5}{2}\left(N_\Gamma^8 - N_\Gamma^{11}\right) + \frac{3}{2}\left(N_{\rm M}^6 - N_{\rm M}^5\right) + \left(-N_{\rm K}^8 + N_{\rm K}^9\right) \quad (57)$$
$$z_{m,C_6}^{k_z=\pi} \equiv \frac{1}{2}\left(N_{\rm A}^9 - N_{\rm A}^{12}\right) + \frac{3}{2}\left(N_{\rm A}^{10} - N_{\rm A}^7\right) + \frac{5}{2}\left(N_{\rm A}^8 - N_{\rm A}^{11}\right) + \frac{3}{2}\left(N_{\rm L}^6 - N_{\rm L}^5\right) + \left(-N_{\rm H}^8 + N_{\rm H}^9\right) \quad (58)$$

As discussed in Ref. [5], $z_{m,C_6}^{k_z=0}$ and $z_{m,C_6}^{k_z=\pi}$ mod 6 indicate the mirror Chern numbers mod 6 on $k_z = 0$ and $\pi$ planes, respectively. In addition, $z_{8,I} = 1 \bmod 2$ implies that the three-dimensional winding number is odd, i.e., the material must be a strong topological superconductor. When $z_{8,I} = 2 \bmod 4$ or $z_{8,I} = 4 \bmod 8$, the material must be either a topological crystalline superconductors or a strong topological superconductor with an even-valued winding number. For this pairing, we used the bases shown in Eq, (59). After computing the above indices for each basis $\mathbf{b}_i$, we find the following facts:

(i) $(z_{m,C_6}^{k_z=0}, z_{m,C_6}^{k_z=\pi}) = (0,5) \bmod 6$ for $\mathbf{b}_8$, $(z_{m,C_6}^{k_z=0}, z_{m,C_6}^{k_z=\pi}) = (5,5) \bmod 6$ for $\mathbf{b}_9$, $(z_{m,C_6}^{k_z=0}, z_{m,C_6}^{k_z=\pi}) = (1,2) \bmod 6$ for $\mathbf{b}_{10}$, and $(z_{m,C_6}^{k_z=0}, z_{m,C_6}^{k_z=\pi}) = (0,0) \bmod 6$ for the other bases;

(ii) $z_{8,I} = 4 \bmod 8$ for $\mathbf{b}_{5,6,7,8}$, $z_{8,I} = 2 \bmod 8$ for $\mathbf{b}_9$, $z_{8,I} = 1 \bmod 8$ for $\mathbf{b}_{10}$.

Then, the entries of SIs in this basis vectors tell us the topology indicated by SIs. In particular, the coefficient of $\mathbf{b}_{10}$ must be odd to have an odd-valued three-dimensional winding number.

$$\left(\begin{array}{c|cccccccccc}
\text{SG 191 } A_{1u} & \mathbf{b}_1 & \mathbf{b}_2 & \mathbf{b}_3 & \mathbf{b}_4 & \mathbf{b}_5 & \mathbf{b}_6 & \mathbf{b}_7 & \mathbf{b}_8 & \mathbf{b}_9 & \mathbf{b}_{10} \\
\hline
z_{8,I} & -8 & -8 & -8 & 24 & 4 & 4 & -36 & 84 & -46 & -9 \\
z_{m,C_6}^{k_z=0} & 0 & 6 & 0 & -6 & 0 & 0 & 6 & -18 & 11 & 1 \\
z_{m,C_6}^{k_z=\pi} & 0 & 6 & 0 & -6 & -6 & 0 & -30 & 17 & 23 & 2 \\
\hline
N_{\Gamma}^{7} & 0 & -1 & 0 & 0 & 0 & 0 & 0 & 0 & 0 & 0 \\
N_{\Gamma}^{8} & -1 & 0 & 0 & 3 & 0 & 0 & -3 & 9 & -5 & -1 \\
N_{\Gamma}^{9} & 0 & 0 & -1 & 0 & 0 & 0 & 0 & 0 & 0 & 0 \\
N_{\Gamma}^{10} & 0 & 1 & 0 & 0 & 0 & 0 & 0 & 0 & 0 & 0 \\
N_{\Gamma}^{11} & 1 & 0 & 0 & -3 & 0 & 0 & 3 & -9 & 8 & 1 \\
N_{\Gamma}^{12} & 0 & 0 & 1 & 0 & 0 & 0 & 0 & 0 & 0 & 0 \\
N_{\mathrm{M}}^{5} & -1 & -1 & -1 & 7 & 0 & 0 & -7 & 21 & -12 & -2 \\
N_{\mathrm{M}}^{6} & 1 & 1 & 1 & -7 & 0 & 0 & 7 & -21 & 12 & 2 \\
N_{\mathrm{K}}^{8} & -1 & 0 & 1 & 0 & 0 & 0 & 0 & 0 & 0 & 0 \\
N_{\mathrm{K}}^{9} & 1 & 0 & -1 & 0 & 0 & 0 & 0 & 0 & 0 & 0 \\
N_{\mathrm{A}}^{7} & 0 & -1 & 0 & 2 & 1 & 0 & -3 & 9 & -5 & -1 \\
N_{\mathrm{A}}^{8} & -1 & 0 & 0 & -1 & 0 & 0 & 0 & -3 & 2 & 0 \\
N_{\mathrm{A}}^{9} & 0 & 0 & -1 & 2 & 0 & 1 & -3 & 9 & -5 & -1 \\
N_{\mathrm{A}}^{10} & 0 & 1 & 0 & -2 & -1 & 0 & 3 & -9 & 8 & 1 \\
N_{\mathrm{A}}^{11} & 1 & 0 & 0 & 1 & 0 & 0 & 0 & 3 & -2 & 0 \\
N_{\mathrm{A}}^{12} & 0 & 0 & 1 & -2 & 0 & -1 & 3 & -9 & 8 & 1 \\
N_{\mathrm{L}}^{5} & -1 & -1 & -1 & -1 & 1 & 1 & -2 & -1 & 1 & 0 \\
N_{\mathrm{L}}^{6} & 1 & 1 & 1 & 1 & -1 & -1 & 2 & 1 & -1 & 0 \\
N_{\mathrm{H}}^{8} & -1 & 0 & 1 & 0 & 0 & -1 & 0 & 0 & 0 & 0 \\
N_{\mathrm{H}}^{9} & 1 & 0 & -1 & 0 & 0 & 1 & 0 & 0 & 0 & 0
\end{array}\right). \quad (59)$$

---


[1] Manfred Sigrist and Kazuo Ueda, "Phenomenological theory of unconventional superconductivity," Rev. Mod. Phys. **63**, 239–311 (1991).

[2] Christopher John Bradley and Arthur P Cracknell, *The Mathematical Theory of Symmetry in Solids: Representation Theory for Point Groups and Space Groups* (Oxford University Press, 2009).

[3] M. G. Vergniory and et al., "A complete catalogue of high-quality topological materials," Nature **566**, 480–485 (2019).

[4] Akishi Matsugatani, Seishiro Ono, Yusuke Nomura, and Haruki Watanabe, "qeirreps: An open-source program for quantum espresso to compute irreducible representations of bloch wavefunctions," Computer Physics Communications **264**, 107948 (2021).

[5] Seishiro Ono, Hoi Chun Po, and Haruki Watanabe, "Refined symmetry indicators for topological superconductors in all space groups," Science Advances **6**, eaaz8367 (2020).

[6] Zhida Song, Tiantian Zhang, Zhong Fang, and Chen Fang, "Quantitative mappings between symmetry and topology in solids," Nat. Commun. **9**, 3530 (2018).
