# Supplementary material for: High-throughput Investigations of Topological and Nodal Superconductors
Source: arXiv:2106.11985 ancillary file (2022-03-04)
Supplement: Supplementary file 2 [file SM-II.pdf]

# Supplementary Material II for “High-throughput Investigations of Topological and Nodal Superconductors”

Feng Tang,<sup>1,\*</sup> Seishiro Ono,<sup>2,\*</sup> Xiangang Wan,<sup>1,†</sup> and Haruki Watanabe<sup>2,‡</sup>

<sup>1</sup>National Laboratory of Solid State Microstructures and School of Physics, Nanjing University, Nanjing 210093, China and Collaborative Innovation Center of Advanced Microstructures, Nanjing University, Nanjing 210093, China

<sup>2</sup>Department of Applied Physics, University of Tokyo, Tokyo 113-8656, Japan

(Dated: February 16, 2022)

## CONTENTS

|                                                                             |    |
|-----------------------------------------------------------------------------|----|
| A. Preliminary remark on listing lowered SGs by higher-dimensional irreps   | 4  |
| B. Symmetry-lowering patterns for higher-dimensional irreps in space groups | 5  |
| 1. Lowered SGs by higher-dimensional irreps of pairings in SG 89            | 5  |
| 2. Lowered SGs by higher-dimensional irreps of pairings in SG 90            | 5  |
| 3. Lowered SGs by higher-dimensional irreps of pairings in SG 91            | 6  |
| 4. Lowered SGs by higher-dimensional irreps of pairings in SG 92            | 7  |
| 5. Lowered SGs by higher-dimensional irreps of pairings in SG 93            | 8  |
| 6. Lowered SGs by higher-dimensional irreps of pairings in SG 94            | 9  |
| 7. Lowered SGs by higher-dimensional irreps of pairings in SG 95            | 9  |
| 8. Lowered SGs by higher-dimensional irreps of pairings in SG 96            | 10 |
| 9. Lowered SGs by higher-dimensional irreps of pairings in SG 97            | 11 |
| 10. Lowered SGs by higher-dimensional irreps of pairings in SG 98           | 12 |
| 11. Lowered SGs by higher-dimensional irreps of pairings in SG 99           | 12 |
| 12. Lowered SGs by higher-dimensional irreps of pairings in SG 100          | 13 |
| 13. Lowered SGs by higher-dimensional irreps of pairings in SG 101          | 14 |
| 14. Lowered SGs by higher-dimensional irreps of pairings in SG 102          | 15 |
| 15. Lowered SGs by higher-dimensional irreps of pairings in SG 103          | 15 |
| 16. Lowered SGs by higher-dimensional irreps of pairings in SG 104          | 16 |
| 17. Lowered SGs by higher-dimensional irreps of pairings in SG 105          | 17 |
| 18. Lowered SGs by higher-dimensional irreps of pairings in SG 106          | 18 |
| 19. Lowered SGs by higher-dimensional irreps of pairings in SG 107          | 18 |
| 20. Lowered SGs by higher-dimensional irreps of pairings in SG 108          | 19 |
| 21. Lowered SGs by higher-dimensional irreps of pairings in SG 109          | 20 |
| 22. Lowered SGs by higher-dimensional irreps of pairings in SG 110          | 20 |
| 23. Lowered SGs by higher-dimensional irreps of pairings in SG 111          | 21 |
| 24. Lowered SGs by higher-dimensional irreps of pairings in SG 112          | 22 |
| 25. Lowered SGs by higher-dimensional irreps of pairings in SG 113          | 23 |
| 26. Lowered SGs by higher-dimensional irreps of pairings in SG 114          | 23 |
| 27. Lowered SGs by higher-dimensional irreps of pairings in SG 115          | 24 |
| 28. Lowered SGs by higher-dimensional irreps of pairings in SG 116          | 25 |
| 29. Lowered SGs by higher-dimensional irreps of pairings in SG 117          | 26 |
| 30. Lowered SGs by higher-dimensional irreps of pairings in SG 118          | 26 |
| 31. Lowered SGs by higher-dimensional irreps of pairings in SG 119          | 27 |
| 32. Lowered SGs by higher-dimensional irreps of pairings in SG 120          | 28 |
| 33. Lowered SGs by higher-dimensional irreps of pairings in SG 121          | 29 |
| 34. Lowered SGs by higher-dimensional irreps of pairings in SG 122          | 29 |
| 35. Lowered SGs by higher-dimensional irreps of pairings in SG 123          | 30 |
| 36. Lowered SGs by higher-dimensional irreps of pairings in SG 124          | 31 |

---

\* These two authors contribute equally to this work.

† [xgwan@nju.edu.cn](mailto:xgwan@nju.edu.cn)

‡ [hwatanabe@g.ecc.u-tokyo.ac.jp](mailto:hwatanabe@g.ecc.u-tokyo.ac.jp)



|                                                                     |     |
|---------------------------------------------------------------------|-----|
| 95. Lowered SGs by higher-dimensional irreps of pairings in SG 198  | 87  |
| 96. Lowered SGs by higher-dimensional irreps of pairings in SG 199  | 88  |
| 97. Lowered SGs by higher-dimensional irreps of pairings in SG 200  | 89  |
| 98. Lowered SGs by higher-dimensional irreps of pairings in SG 201  | 91  |
| 99. Lowered SGs by higher-dimensional irreps of pairings in SG 202  | 92  |
| 100. Lowered SGs by higher-dimensional irreps of pairings in SG 203 | 93  |
| 101. Lowered SGs by higher-dimensional irreps of pairings in SG 204 | 94  |
| 102. Lowered SGs by higher-dimensional irreps of pairings in SG 205 | 96  |
| 103. Lowered SGs by higher-dimensional irreps of pairings in SG 206 | 97  |
| 104. Lowered SGs by higher-dimensional irreps of pairings in SG 207 | 98  |
| 105. Lowered SGs by higher-dimensional irreps of pairings in SG 208 | 101 |
| 106. Lowered SGs by higher-dimensional irreps of pairings in SG 209 | 105 |
| 107. Lowered SGs by higher-dimensional irreps of pairings in SG 210 | 108 |
| 108. Lowered SGs by higher-dimensional irreps of pairings in SG 211 | 111 |
| 109. Lowered SGs by higher-dimensional irreps of pairings in SG 212 | 114 |
| 110. Lowered SGs by higher-dimensional irreps of pairings in SG 213 | 117 |
| 111. Lowered SGs by higher-dimensional irreps of pairings in SG 214 | 120 |
| 112. Lowered SGs by higher-dimensional irreps of pairings in SG 215 | 123 |
| 113. Lowered SGs by higher-dimensional irreps of pairings in SG 216 | 127 |
| 114. Lowered SGs by higher-dimensional irreps of pairings in SG 217 | 130 |
| 115. Lowered SGs by higher-dimensional irreps of pairings in SG 218 | 133 |
| 116. Lowered SGs by higher-dimensional irreps of pairings in SG 219 | 136 |
| 117. Lowered SGs by higher-dimensional irreps of pairings in SG 220 | 139 |
| 118. Lowered SGs by higher-dimensional irreps of pairings in SG 221 | 142 |
| 119. Lowered SGs by higher-dimensional irreps of pairings in SG 222 | 146 |
| 120. Lowered SGs by higher-dimensional irreps of pairings in SG 223 | 150 |
| 121. Lowered SGs by higher-dimensional irreps of pairings in SG 224 | 154 |
| 122. Lowered SGs by higher-dimensional irreps of pairings in SG 225 | 159 |
| 123. Lowered SGs by higher-dimensional irreps of pairings in SG 226 | 163 |
| 124. Lowered SGs by higher-dimensional irreps of pairings in SG 227 | 167 |
| 125. Lowered SGs by higher-dimensional irreps of pairings in SG 228 | 171 |
| 126. Lowered SGs by higher-dimensional irreps of pairings in SG 229 | 174 |
| 127. Lowered SGs by higher-dimensional irreps of pairings in SG 230 | 178 |
| References                                                          | 182 |

In this supplementary materials, we list all details of lowered space groups (SGs) by higher-dimensional irreps of the original PG in the rest sections.

### A. PRELIMINARY REMARK ON LISTING LOWERED SGS BY HIGHER-DIMENSIONAL IRREPS

Then we show details on how the superconducting pairings belonging to the higher-dimensional irreps of the PG break SG symmetry. We firstly show all the representative elements in the factor group (SG/T) where T is the corresponding translation group: Each element is expressed in the style following that in the Bilbao server (<https://www.cryst.ehu.es/>) (also, the convention also follows that of the default setting adopted in the Bilbao server). These elements are labeled by 1, 2, 3, . . . . As discussed above, the pairing belonging to higher-dimensional irrep might break some elements, thus only some are preserved. We show the preserved elements by the labels (printed in red) for the elements of SG/T. Then the PG is lowered and the SG is thus also lowered, denoted by  $SG'$  (the SG number of the original SG is denoted by  $SG$ ). To fit with the default convention (note that how the Bravais lattice is centered might also be changed), we might need a transformation including a rotation of the crystal axes and the origin shift: Denote the crystal axes of the original SG as  $\mathbf{a}_{SG}$ ,  $\mathbf{b}_{SG}$  and  $\mathbf{c}_{SG}$ , and those of the lowered SG as  $\mathbf{a}_{SG'}$ ,  $\mathbf{b}_{SG'}$  and  $\mathbf{c}_{SG'}$ , we then express then rotation of the crystal axes by  $(\mathbf{a}_{SG'}, \mathbf{b}_{SG'}, \mathbf{c}_{SG'}) = (\mathbf{a}_{SG}, \mathbf{b}_{SG}, \mathbf{c}_{SG})P$ , where  $P$  is an integer matrix. With respect to the origin shift, we show  $\overrightarrow{O_{SG}O_{SG'}}$  where  $O_{SG}$  ( $O_{SG'}$ ) is the origin of the original (lowered) SG. All possible reductions of the higher-dimensional irrep for the original PG to the one-dimensional irreps of the lowered PG are also given, and then one should consider these one-dimensional irreps one-by-one to diagnose the topological/nodal superconductivity in the lowered SG. For the example of PG  $D_{4h}$ , (see Sec. 37) the higher-dimensional irreps can be  $E_g$  and  $E_u$ , which are reduced to  $B_{1g} \oplus B_{3g}$  of the sub-PG  $D_{2h}$  and  $B_{1u} \oplus B_{3u}$  of the sub-PG  $D_{2h}$ , respectively. They can also be reduced to  ${}^2E_g \oplus {}^1E_g$  of the sub-PG  $C_{4h}$  and  ${}^2E_u \oplus {}^1E_u$  of the sub-PG  $C_{4h}$ , respectively. We also show the correspondences between the irreps at high-symmetry points (HSPs) of the lowered SG and those of the original SG:  $n_\alpha^{SG}$  means the number of occurrences of the irrep  $\alpha$  at some HSP for the original SG while  $n_{\alpha'}^{SG'}$  means the number of occurrences of the irrep  $\alpha'$  at some HSP for the lowered SG. Note that the notation of irrep of HSP follows that in the Bilbao server, which implies the information of the HSP involved.

We should point out that the label for each sub-SG (printed in red and bold), **1, 2, 3, . . .**, is presented in parentheses ( ) following the chemical formula in the database ([tncs.nju.edu.cn](https://tncs.nju.edu.cn)) (right after ,). The materials in the database with high-dimensional irreps of pairing symmetries are regarded as new entries, distinguished by the high-dimensional irrep for pairing symmetry of the original PG and the sub-SG label. For example, searching “059186” in the search box of ICSD number, we can obtain 9 results as shown in Fig. 1 below: The item with chemical formula being “Ba1Pt1Sb1” corresponds to results for one-dimensional irreps and the SG is not lowered (the original SG is SG 187). The rest 8 items are results for high-dimensional irreps for pairing symmetries where one can find that their SGs are lowered: The lowered SGs can be SGs 38 and 174. The chemical formulas contains parentheses ( ) where the high-dimensional irrep and sub-SG label are given: e.g. For the chemical formula being “Ba1Pt1Sb1(SG187:E”,4)”, it means that the high-dimensional irrep is E” and the sub-SG label is 4. Based on the content here, one can know concretely which elements of the original PG are preserved (white the rest are broken) for this item: The 1st, 7th, 9th, 2nd, 3rd and 8th elements in SG/T are preserved (All elements in the factor group SG/T of SG 187 are shown in order in a frame).

|    | Space Group number | ICSD number | Chemical formula      |
|----|--------------------|-------------|-----------------------|
| 1. | 187                | 059186      | Ba1Pt1Sb1             |
| 2. | 38                 | 059186      | Ba1Pt1Sb1(SG187:E",1) |
| 3. | 38                 | 059186      | Ba1Pt1Sb1(SG187:E",1) |
| 4. | 38                 | 059186      | Ba1Pt1Sb1(SG187:E",2) |
| 5. | 38                 | 059186      | Ba1Pt1Sb1(SG187:E",2) |
| 6. | 38                 | 059186      | Ba1Pt1Sb1(SG187:E",3) |
| 7. | 38                 | 059186      | Ba1Pt1Sb1(SG187:E",3) |
| 8. | 174                | 059186      | Ba1Pt1Sb1(SG187:E",4) |
| 9. | 174                | 059186      | Ba1Pt1Sb1(SG187:E",4) |

FIG. 1. Searching “059186” in the ICSD number box returns 9 items with the first for result of one-dimensional irrep and the rest for results of higher-dimensional irreps for pairings. The chemical formula indicates the original SG and the higher-dimensional irrep, as well as the lower SG (the integer  $i$  after , in the parentheses means that the sub-SG label is  $i$  and the concrete broken or preserved PG elements for sub-SG  $i$  are listed in Sec. 86).

In total, we have 282100 new entries when considering higher-dimensional irreps for pairings, around ten times the entries of only one-dimensional irreps. Finally, we should point out that SGs 1-88 own no higher-dimensional irreps of pairing symmetries, thus we start from SG 89 (whose PG is  $D_4$ ) in the following.

## B. SYMMETRY-LOWERING PATTERNS FOR HIGHER-DIMENSIONAL IRREPS IN SPACE GROUPS

### 1. Lowered SGs by higher-dimensional irreps of pairings in SG 89

The representative operations of SG/T for SG 89:

$$1 : (x, y, z), 2 : (-y, x, z), 3 : (y, -x, z), 4 : (x, -y, -z), 5 : (-x, y, -z), 6 : (-x, -y, z), 7 : (y, x, -z), 8 : (-y, -x, -z).$$

The lower SG is SG 16 when the preserved operations are: (**sub-SG label is 1**) 1, 4, 5, 6.

The transformation is:  $(\mathbf{a}_{16}, \mathbf{b}_{16}, \mathbf{c}_{16}) = (\mathbf{a}_{89}, \mathbf{b}_{89}, \mathbf{c}_{89}) \begin{pmatrix} 0 & 0 & 1 \\ 1 & 0 & 0 \\ 0 & 1 & 0 \end{pmatrix}, \overrightarrow{O_{89}O_{16}} = \frac{1}{2}\mathbf{a}_{16} + (\frac{1}{2})\mathbf{c}_{16}$

The reduction of higher dimensional irrep:

$$D_4 : E \rightarrow B_1 + B_3 \text{ of } D_2.$$

The correspondences of irreps at HSPs from original SG to lowered SG:

$$n_{GM5}^{16} = n_{GM6}^{89} + n_{GM7}^{89} n_{X5}^{16} = n_{X5}^{89} n_{S5}^{16} = n_{R5}^{89} n_{R5}^{16} = n_{A6}^{89} + n_{A7}^{89} n_{U5}^{16} = n_{M6}^{89} + n_{M7}^{89} n_{Z5}^{16} = n_{X5}^{89} n_{T5}^{16} = n_{R5}^{89} n_{Y5}^{16} = n_{Z6}^{89} + n_{Z7}^{89}$$

The lower SG is SG 21 when the preserved operations are: (**sub-SG label is 2**) 1, 6, 7, 8.

The transformation is:  $(\mathbf{a}_{21}, \mathbf{b}_{21}, \mathbf{c}_{21}) = (\mathbf{a}_{89}, \mathbf{b}_{89}, \mathbf{c}_{89}) \begin{pmatrix} 1 & -1 & 0 \\ 1 & 1 & 0 \\ 0 & 0 & 1 \end{pmatrix}, \overrightarrow{O_{89}O_{21}} = \frac{1}{2}\mathbf{c}_{21}$

The reduction of higher dimensional irrep:

$$D_4 : E \rightarrow B_2 + B_3 \text{ of } D_2.$$

The correspondences of irreps at HSPs from original SG to lowered SG:

$$n_{GM5}^{21} = n_{GM6}^{89} + n_{GM7}^{89} n_{Y5}^{21} = n_{M6}^{89} + n_{M7}^{89} n_{S4}^{21} = n_{X5}^{89} n_{S3}^{21} = n_{X5}^{89} n_{Z5}^{21} = n_{Z6}^{89} + n_{Z7}^{89} n_{T5}^{21} = n_{A6}^{89} + n_{A7}^{89} n_{R4}^{21} = n_{R5}^{89} n_{R3}^{21} = n_{R5}^{89}$$

The lower SG is SG 75 when the preserved operations are: (**sub-SG label is 3**) 1, 2, 3, 6.

The transformation is:  $(\mathbf{a}_{75}, \mathbf{b}_{75}, \mathbf{c}_{75}) = (\mathbf{a}_{89}, \mathbf{b}_{89}, \mathbf{c}_{89}) \begin{pmatrix} -1 & 0 & 0 \\ 0 & -1 & 0 \\ 0 & 0 & 1 \end{pmatrix}, \overrightarrow{O_{89}O_{75}} = -\frac{1}{2}\mathbf{a}_{75} + (\frac{1}{2})\mathbf{b}_{75}$

The reduction of higher dimensional irrep:

$$D_4 : E \rightarrow {}^2E + {}^1E \text{ of } C_4.$$

The correspondences of irreps at HSPs from original SG to lowered SG:

$$n_{GM5}^{75} = n_{GM6}^{89} n_{GM7}^{75} = n_{GM6}^{89} n_{GM8}^{75} = n_{GM7}^{89} n_{GM6}^{75} = n_{GM7}^{89} n_{X4}^{75} = n_{X5}^{89} n_{X3}^{75} = n_{X5}^{89} n_{M5}^{75} = n_{M7}^{89} n_{M7}^{75} = n_{M7}^{89} n_{M8}^{75} = n_{M6}^{89} n_{M6}^{75} = n_{M6}^{89} n_{A5}^{75} = n_{A7}^{89} n_{A7}^{75} = n_{A7}^{89} n_{A8}^{75} = n_{A6}^{89} n_{A6}^{75} = n_{A6}^{89} n_{R4}^{75} = n_{R5}^{89} n_{R3}^{75} = n_{R5}^{89} n_{Z5}^{75} = n_{Z6}^{89} n_{Z7}^{75} = n_{Z6}^{89} n_{Z8}^{75} = n_{Z7}^{89} = n_{Z7}^{89}$$

### 2. Lowered SGs by higher-dimensional irreps of pairings in SG 90

The representative operations of SG/T for SG 90:

$$1 : (x, y, z), 2 : (\frac{1}{2} - y, x + \frac{1}{2}, z), 3 : (y + \frac{1}{2}, \frac{1}{2} - x, z), 4 : (x + \frac{1}{2}, \frac{1}{2} - y, -z), 5 : (\frac{1}{2} - x, y + \frac{1}{2}, -z), 6 : (-x, -y, z), \\ 7 : (y, x, -z), 8 : (-y, -x, -z).$$

The lower SG is SG 18 when the preserved operations are: **(sub-SG label is 1) 1, 4, 5, 6.**

$$\text{The transformation is: } (\mathbf{a}_{18}, \mathbf{b}_{18}, \mathbf{c}_{18}) = (\mathbf{a}_{90}, \mathbf{b}_{90}, \mathbf{c}_{90}) \begin{pmatrix} -1 & 0 & 0 \\ 0 & 1 & 0 \\ 0 & 0 & -1 \end{pmatrix}, \overrightarrow{O_{90}O_{18}} = \mathbf{a}_{18} + (\frac{1}{2})\mathbf{c}_{18}$$

The reduction of higher dimensional irrep:

$$D_4 : E \rightarrow B_2 + B_3 \text{ of } D_2.$$

The correspondences of irreps at HSPs from original SG to lowered SG:

$$n_{GM5}^{18} = n_{GM6}^{90} + n_{GM7}^{90} n_{X4}^{18} = n_{X4}^{90} n_{X5}^{18} = n_{X3}^{90} n_{X3}^{18} = n_{X5}^{90} n_{X2}^{18} = n_{X2}^{90} n_{S5}^{18} = n_{M6}^{90} + n_{M7}^{90} n_{R5}^{18} = n_{A6}^{90} + n_{A7}^{90} n_{U4}^{18} = n_{R2}^{90} \\ n_{U5}^{18} = n_{R5}^{90} n_{U3}^{18} = n_{R3}^{90} n_{U2}^{18} = n_{R4}^{90} n_{Z5}^{18} = n_{Z6}^{90} + n_{Z7}^{90} n_{T3}^{18} = n_{R2}^{90} n_{T2}^{18} = n_{R3}^{90} n_{T4}^{18} = n_{R5}^{90} n_{T5}^{18} = n_{R4}^{90} n_{Y3}^{18} = n_{X4}^{90} n_{Y2}^{18} = \\ n_{X5}^{90} n_{Y4}^{18} = n_{X3}^{90} n_{Y5}^{18} = n_{X2}^{90}$$

The lower SG is SG 21 when the preserved operations are: **(sub-SG label is 2) 1, 6, 7, 8.**

$$\text{The transformation is: } (\mathbf{a}_{21}, \mathbf{b}_{21}, \mathbf{c}_{21}) = (\mathbf{a}_{90}, \mathbf{b}_{90}, \mathbf{c}_{90}) \begin{pmatrix} 1 & -1 & 0 \\ 1 & 1 & 0 \\ 0 & 0 & 1 \end{pmatrix}, \overrightarrow{O_{90}O_{21}} = \frac{1}{2}\mathbf{b}_{21} + (\frac{1}{2})\mathbf{c}_{21}$$

The reduction of higher dimensional irrep:

$$D_4 : E \rightarrow B_2 + B_3 \text{ of } D_2.$$

The correspondences of irreps at HSPs from original SG to lowered SG:

$$n_{GM5}^{21} = n_{GM6}^{90} + n_{GM7}^{90} n_{Y5}^{21} = n_{M6}^{90} + n_{M7}^{90} n_{S4}^{21} = n_{X2}^{90} + n_{X4}^{90} n_{S3}^{21} = n_{X3}^{90} + n_{X5}^{90} n_{Z5}^{21} = n_{Z6}^{90} + n_{Z7}^{90} n_{T5}^{21} = n_{A6}^{90} + n_{A7}^{90} \\ n_{R4}^{21} = n_{R2}^{90} + n_{R4}^{90} n_{R3}^{21} = n_{R3}^{90} + n_{R5}^{90}$$

The lower SG is SG 75 when the preserved operations are: **(sub-SG label is 3) 1, 2, 3, 6.**

$$\text{The transformation is: } (\mathbf{a}_{75}, \mathbf{b}_{75}, \mathbf{c}_{75}) = (\mathbf{a}_{90}, \mathbf{b}_{90}, \mathbf{c}_{90}) \begin{pmatrix} -1 & 0 & 0 \\ 0 & -1 & 0 \\ 0 & 0 & 1 \end{pmatrix}, \overrightarrow{O_{90}O_{75}} = \frac{1}{2}\mathbf{b}_{75}$$

The reduction of higher dimensional irrep:

$$D_4 : E \rightarrow {}^2E + {}^1E \text{ of } C_4.$$

The correspondences of irreps at HSPs from original SG to lowered SG:

$$n_{GM5}^{75} = n_{GM6}^{90} n_{GM7}^{75} = n_{GM6}^{90} n_{GM8}^{75} = n_{GM7}^{90} n_{GM6}^{75} = n_{GM7}^{90} n_{X4}^{75} = n_{X2}^{90} + n_{X4}^{90} n_{X3}^{75} = n_{X3}^{90} + n_{X5}^{90} n_{M5}^{75} = n_{M7}^{90} n_{M7}^{75} = \\ n_{M6}^{90} n_{M8}^{75} = n_{M7}^{90} n_{M6}^{75} = n_{M6}^{90} n_{A5}^{75} = n_{A7}^{90} n_{A7}^{75} = n_{A6}^{90} n_{A8}^{75} = n_{A7}^{90} n_{A6}^{75} = n_{A6}^{90} n_{R4}^{75} = n_{R2}^{90} + n_{R4}^{90} n_{R3}^{75} = n_{R3}^{90} + n_{R5}^{90} n_{Z5}^{75} = \\ n_{Z6}^{90} n_{Z7}^{75} = n_{Z6}^{90} n_{Z8}^{75} = n_{Z7}^{90} n_{Z6}^{75} = n_{Z7}^{90}$$

### 3. Lowered SGs by higher-dimensional irreps of pairings in SG 91

The representative operations of SG/T for SG 91:

$$1 : (x, y, z), 2 : (-y, x, z + \frac{1}{4}), 3 : (y, -x, z + \frac{3}{4}), 4 : (x, -y, \frac{1}{2} - z), 5 : (-x, y, -z), 6 : (-x, -y, z + \frac{1}{2}), 7 : (y, x, \frac{3}{4} - z), \\ 8 : (-y, -x, \frac{1}{4} - z).$$

The lower SG is SG 17 when the preserved operations are: **(sub-SG label is 1) 1, 4, 5, 6.**

$$\text{The transformation is: } (\mathbf{a}_{17}, \mathbf{b}_{17}, \mathbf{c}_{17}) = (\mathbf{a}_{91}, \mathbf{b}_{91}, \mathbf{c}_{91}) \begin{pmatrix} 0 & -1 & 0 \\ 1 & 0 & 0 \\ 0 & 0 & 1 \end{pmatrix}, \overrightarrow{O_{91}O_{17}} = \frac{1}{2}\mathbf{b}_{17} + (-)\mathbf{c}_{17}$$

The reduction of higher dimensional irrep:

$$D_4 : E \rightarrow B_3 + B_2 \text{ of } D_2.$$

The correspondences of irreps at HSPs from original SG to lowered SG:

$$n_{GM5}^{17} = n_{GM6}^{91} + n_{GM7}^{91} n_{X5}^{17} = n_{X5}^{91} n_{S5}^{17} = n_{M6}^{91} + n_{M7}^{91} n_{R5}^{17} = n_{A4}^{91} + n_{A5}^{91} n_{R4}^{17} = n_{A7}^{91} n_{R2}^{17} = n_{A7}^{91} n_{R3}^{17} = n_{A3}^{91} + n_{A6}^{91} n_{U5}^{17} = \\ n_{R5}^{91} n_{U4}^{17} = n_{R2}^{91} n_{U2}^{17} = n_{R4}^{91} n_{U3}^{17} = n_{R3}^{91} n_{Z4}^{17} = n_{Z3}^{91} + n_{Z6}^{91} n_{Z5}^{17} = n_{Z7}^{91} n_{Z3}^{17} = n_{Z7}^{91} n_{Z2}^{17} = n_{Z4}^{91} + n_{Z5}^{91} n_{T4}^{17} = n_{R5}^{91} n_{T5}^{17} = n_{R4}^{91}$$

$$n_{T3}^{17} = n_{R2}^{91} n_{T2}^{17} = n_{R3}^{91} n_{Y5}^{17} = n_{X5}^{91}$$

The lower SG is SG 20 when the preserved operations are: **(sub-SG label is 2) 1, 6, 7, 8.**

$$\text{The transformation is: } (\mathbf{a}_{20}, \mathbf{b}_{20}, \mathbf{c}_{20}) = (\mathbf{a}_{91}, \mathbf{b}_{91}, \mathbf{c}_{91}) \begin{pmatrix} 1 & 1 & 0 \\ 1 & -1 & 0 \\ 0 & 0 & -1 \end{pmatrix}, \overrightarrow{O_{91}O_{20}} = \frac{5}{8}\mathbf{c}_{20}$$

The reduction of higher dimensional irrep:

$$D_4 : E \rightarrow B_2 + B_3 \text{ of } D_2.$$

The correspondences of irreps at HSPs from original SG to lowered SG:

$$\begin{aligned} n_{GM5}^{20} &= n_{GM6}^{91} + n_{GM7}^{91} n_{Y5}^{20} = n_{M6}^{91} + n_{M7}^{91} n_{S4}^{20} = n_{X5}^{91} n_{S3}^{20} = n_{X5}^{91} n_{Z5}^{20} = n_{Z7}^{91} n_{Z4}^{20} = n_{Z5}^{91} + n_{Z6}^{91} n_{Z2}^{20} = n_{Z3}^{91} + n_{Z4}^{91} n_{Z3}^{20} = \\ n_{Z7}^{91} n_{T5}^{20} &= n_{A7}^{91} n_{T4}^{20} = n_{A5}^{91} + n_{A6}^{91} n_{T2}^{20} = n_{A3}^{91} + n_{A4}^{91} n_{T3}^{20} = n_{A7}^{91} n_{R4}^{20} = n_{R3}^{91} + n_{R5}^{91} n_{R3}^{20} = n_{R2}^{91} + n_{R4}^{91} \end{aligned}$$

The lower SG is SG 76 when the preserved operations are: **(sub-SG label is 3) 1, 2, 3, 6.**

$$\text{The transformation is: } (\mathbf{a}_{76}, \mathbf{b}_{76}, \mathbf{c}_{76}) = (\mathbf{a}_{91}, \mathbf{b}_{91}, \mathbf{c}_{91}) \begin{pmatrix} -1 & 0 & 0 \\ 0 & 1 & 0 \\ 0 & 0 & -1 \end{pmatrix}, \overrightarrow{O_{91}O_{76}} = \frac{1}{2}\mathbf{a}_{76} + \left(\frac{1}{2}\right)\mathbf{b}_{76} + \left(\frac{3}{4}\right)\mathbf{c}_{76}$$

The reduction of higher dimensional irrep:

$$D_4 : E \rightarrow {}^2E + {}^1E \text{ of } C_4.$$

The correspondences of irreps at HSPs from original SG to lowered SG:

$$\begin{aligned} n_{GM5}^{76} &= n_{GM6}^{91} n_{GM7}^{76} = n_{GM6}^{91} n_{GM8}^{76} = n_{GM7}^{91} n_{GM6}^{76} = n_{GM7}^{91} n_{X4}^{76} = n_{X5}^{91} n_{X3}^{76} = n_{X5}^{91} n_{M5}^{76} = n_{M7}^{91} n_{M7}^{76} = n_{M7}^{91} n_{M8}^{76} = \\ n_{M6}^{91} n_{M6}^{76} &= n_{M6}^{91} n_{A6}^{76} = n_{A3}^{91} + n_{A5}^{91} n_{A7}^{76} = n_{A7}^{91} n_{A8}^{76} = n_{A7}^{91} n_{A5}^{76} = n_{A4}^{91} + n_{A6}^{91} n_{R4}^{76} = n_{R2}^{91} + n_{R4}^{91} n_{R3}^{76} = n_{R3}^{91} + n_{R5}^{91} n_{Z8}^{76} = \\ n_{Z7}^{91} n_{Z5}^{76} &= n_{Z4}^{91} + n_{Z6}^{91} n_{Z6}^{76} = n_{Z3}^{91} + n_{Z5}^{91} n_{Z7}^{76} = n_{Z7}^{91} \end{aligned}$$

#### 4. Lowered SGs by higher-dimensional irreps of pairings in SG 92

The representative operations of SG/T for SG 92:

$$\begin{aligned} 1 : (x, y, z), 2 : \left(\frac{1}{2} - y, x + \frac{1}{2}, z + \frac{1}{4}\right), 3 : \left(y + \frac{1}{2}, \frac{1}{2} - x, z + \frac{3}{4}\right), 4 : \left(x + \frac{1}{2}, \frac{1}{2} - y, \frac{3}{4} - z\right), 5 : \left(\frac{1}{2} - x, y + \frac{1}{2}, \frac{1}{4} - z\right), \\ 6 : (-x, -y, z + \frac{1}{2}), 7 : (y, x, -z), 8 : (-y, -x, \frac{1}{2} - z). \end{aligned}$$

The lower SG is SG 19 when the preserved operations are: **(sub-SG label is 1) 1, 4, 5, 6.**

$$\text{The transformation is: } (\mathbf{a}_{19}, \mathbf{b}_{19}, \mathbf{c}_{19}) = (\mathbf{a}_{92}, \mathbf{b}_{92}, \mathbf{c}_{92}) \begin{pmatrix} -1 & 0 & 0 \\ 0 & 0 & 1 \\ 0 & 1 & 0 \end{pmatrix}, \overrightarrow{O_{92}O_{19}} = \mathbf{a}_{19} + \left(\frac{1}{8}\right)\mathbf{b}_{19} + \left(\frac{3}{4}\right)\mathbf{c}_{19}$$

The reduction of higher dimensional irrep:

$$D_4 : E \rightarrow B_1 + B_3 \text{ of } D_2.$$

The correspondences of irreps at HSPs from original SG to lowered SG:

$$\begin{aligned} n_{GM5}^{19} &= n_{GM6}^{92} + n_{GM7}^{92} n_{X4}^{19} = n_{X4}^{92} n_{X5}^{19} = n_{X3}^{92} n_{X3}^{19} = n_{X2}^{92} n_{X2}^{19} = n_{X5}^{92} n_{S5}^{19} = n_{R5}^{92} n_{R3}^{19} = n_{A4}^{92} + n_{A5}^{92} n_{R2}^{19} = n_{A7}^{92} n_{R4}^{19} = \\ n_{A3}^{92} + n_{A6}^{92} n_{R5}^{19} &= n_{A7}^{92} n_{Y5}^{19} = n_{M6}^{92} + n_{M7}^{92} n_{Z4}^{19} = n_{X5}^{92} n_{Z5}^{19} = n_{X4}^{92} n_{Z3}^{19} = n_{X3}^{92} n_{Z2}^{19} = n_{X2}^{92} n_{T5}^{19} = n_{R5}^{92} n_{Y3}^{19} = n_{Z7}^{92} n_{Y2}^{19} = \\ n_{Z3}^{92} + n_{Z6}^{92} n_{Y4}^{19} &= n_{Z7}^{92} n_{Y5}^{19} = n_{Z4}^{92} + n_{Z5}^{92} \end{aligned}$$

The lower SG is SG 20 when the preserved operations are: **(sub-SG label is 2) 1, 6, 7, 8.**

$$\text{The transformation is: } (\mathbf{a}_{20}, \mathbf{b}_{20}, \mathbf{c}_{20}) = (\mathbf{a}_{92}, \mathbf{b}_{92}, \mathbf{c}_{92}) \begin{pmatrix} -1 & -1 & 0 \\ -1 & 1 & 0 \\ 0 & 0 & -1 \end{pmatrix}, \overrightarrow{O_{92}O_{20}} = \frac{1}{2}\mathbf{a}_{20} + \left(\frac{1}{2}\right)\mathbf{b}_{20} + \left(-\frac{1}{2}\right)\mathbf{c}_{20}$$

The reduction of higher dimensional irrep:

$$D_4 : E \rightarrow B_2 + B_3 \text{ of } D_2.$$

The correspondences of irreps at HSPs from original SG to lowered SG:

$$\begin{aligned} n_{GM5}^{20} &= n_{GM6}^{92} + n_{GM7}^{92} n_{Y5}^{20} = n_{M6}^{92} + n_{M7}^{92} n_{S4}^{20} = n_{X3}^{92} + n_{X5}^{92} n_{S3}^{20} = n_{X2}^{92} + n_{X4}^{92} n_{Z5}^{20} = n_{Z7}^{92} n_{Z4}^{20} = n_{Z5}^{92} + n_{Z6}^{92} n_{Z2}^{20} = \\ n_{Z3}^{92} + n_{Z4}^{92} n_{Z3}^{20} &= n_{Z7}^{92} n_{T5}^{20} = n_{A7}^{92} n_{T4}^{20} = n_{A5}^{92} + n_{A6}^{92} n_{T2}^{20} = n_{A3}^{92} + n_{A4}^{92} n_{T3}^{20} = n_{A7}^{92} n_{R4}^{20} = n_{R5}^{92} n_{R3}^{20} = n_{R5}^{92} \end{aligned}$$

The lower SG is SG 76 when the preserved operations are: **(sub-SG label is 3) 1, 2, 3, 6.**

The transformation is:  $(\mathbf{a}_{76}, \mathbf{b}_{76}, \mathbf{c}_{76}) = (\mathbf{a}_{92}, \mathbf{b}_{92}, \mathbf{c}_{92}) \begin{pmatrix} -1 & 0 & 0 \\ 0 & 1 & 0 \\ 0 & 0 & -1 \end{pmatrix}, \overrightarrow{O_{92}O_{76}} = \mathbf{a}_{76} + (\frac{1}{2})\mathbf{b}_{76} + (-\frac{3}{8})\mathbf{c}_{76}$

The reduction of higher dimensional irrep:

$D_4 : E \rightarrow {}^2E + {}^1E$  of  $C_4$ .

The correspondences of irreps at HSPs from original SG to lowered SG:

$$\begin{aligned} n_{GM5}^{76} &= n_{GM6}^{92} n_{GM7}^{76} = n_{GM6}^{92} n_{GM8}^{76} = n_{GM7}^{92} n_{GM6}^{76} = n_{GM7}^{92} n_{X4}^{76} = n_{X3}^{92} + n_{X5}^{92} n_{X3}^{76} = n_{X2}^{92} + n_{X4}^{92} n_{M5}^{76} = n_{M6}^{92} n_{M7}^{76} = \\ n_{M7}^{92} n_{M8}^{76} &= n_{M6}^{92} n_{M6}^{76} = n_{M7}^{92} n_{A6}^{76} = n_{A7}^{92} n_{A7}^{76} = n_{A4}^{92} + n_{A6}^{92} n_{A8}^{76} = n_{A3}^{92} + n_{A5}^{92} n_{A5}^{76} = n_{A7}^{92} n_{R4}^{76} = n_{R5}^{92} n_{R3}^{76} = n_{R5}^{92} n_{Z8}^{76} = \\ n_{Z7}^{92} n_{Z5}^{76} &= n_{Z4}^{92} + n_{Z6}^{92} n_{Z6}^{76} = n_{Z3}^{92} + n_{Z5}^{92} n_{Z7}^{76} = n_{Z7}^{92} \end{aligned}$$

## 5. Lowered SGs by higher-dimensional irreps of pairings in SG 93

The representative operations of SG/T for SG 93:

$$\begin{aligned} 1 : (x, y, z), 2 : (-y, x, z + \frac{1}{2}), 3 : (y, -x, z + \frac{1}{2}), 4 : (x, -y, -z), 5 : (-x, y, -z), 6 : (-x, -y, z), 7 : (y, x, \frac{1}{2} - z), \\ 8 : (-y, -x, \frac{1}{2} - z). \end{aligned}$$

The lower SG is SG 16 when the preserved operations are: **(sub-SG label is 1) 1, 4, 5, 6.**

The transformation is:  $(\mathbf{a}_{16}, \mathbf{b}_{16}, \mathbf{c}_{16}) = (\mathbf{a}_{93}, \mathbf{b}_{93}, \mathbf{c}_{93}) \begin{pmatrix} 0 & 0 & 1 \\ 1 & 0 & 0 \\ 0 & 1 & 0 \end{pmatrix}, \overrightarrow{O_{93}O_{16}} = \frac{1}{2}\mathbf{a}_{16} + (\frac{1}{2})\mathbf{c}_{16}$

The reduction of higher dimensional irrep:

$D_4 : E \rightarrow B_1 + B_3$  of  $D_2$ .

The correspondences of irreps at HSPs from original SG to lowered SG:

$$\begin{aligned} n_{GM5}^{16} &= n_{GM6}^{93} + n_{GM7}^{93} n_{X5}^{16} = n_{X5}^{93} n_{S5}^{16} = n_{R5}^{93} n_{R5}^{16} = n_{A6}^{93} + n_{A7}^{93} n_{U5}^{16} = n_{M6}^{93} + n_{M7}^{93} n_{Z5}^{16} = n_{X5}^{93} n_{T5}^{16} = n_{R5}^{93} n_{Y5}^{16} = \\ n_{Z6}^{93} + n_{Z7}^{93} \end{aligned}$$

The lower SG is SG 21 when the preserved operations are: **(sub-SG label is 2) 1, 6, 7, 8.**

The transformation is:  $(\mathbf{a}_{21}, \mathbf{b}_{21}, \mathbf{c}_{21}) = (\mathbf{a}_{93}, \mathbf{b}_{93}, \mathbf{c}_{93}) \begin{pmatrix} 1 & -1 & 0 \\ 1 & 1 & 0 \\ 0 & 0 & 1 \end{pmatrix}, \overrightarrow{O_{93}O_{21}} = \frac{3}{4}\mathbf{c}_{21}$

The reduction of higher dimensional irrep:

$D_4 : E \rightarrow B_2 + B_3$  of  $D_2$ .

The correspondences of irreps at HSPs from original SG to lowered SG:

$$\begin{aligned} n_{GM5}^{21} &= n_{GM6}^{93} + n_{GM7}^{93} n_{Y5}^{21} = n_{M6}^{93} + n_{M7}^{93} n_{S4}^{21} = n_{X5}^{93} n_{S3}^{21} = n_{X5}^{93} n_{Z5}^{21} = n_{Z6}^{93} + n_{Z7}^{93} n_{T5}^{21} = n_{A6}^{93} + n_{A7}^{93} n_{R4}^{21} = n_{R5}^{93} n_{R3}^{21} = \\ n_{R5}^{93} \end{aligned}$$

The lower SG is SG 77 when the preserved operations are: **(sub-SG label is 3) 1, 2, 3, 6.**

The transformation is:  $(\mathbf{a}_{77}, \mathbf{b}_{77}, \mathbf{c}_{77}) = (\mathbf{a}_{93}, \mathbf{b}_{93}, \mathbf{c}_{93}) \begin{pmatrix} -1 & 0 & 0 \\ 0 & 1 & 0 \\ 0 & 0 & -1 \end{pmatrix}, \overrightarrow{O_{93}O_{77}} = \frac{1}{2}\mathbf{a}_{77} + (\frac{1}{2})\mathbf{b}_{77}$

The reduction of higher dimensional irrep:

$D_4 : E \rightarrow {}^2E + {}^1E$  of  $C_4$ .

The correspondences of irreps at HSPs from original SG to lowered SG:

$$\begin{aligned} n_{GM5}^{77} &= n_{GM6}^{93} n_{GM7}^{77} = n_{GM6}^{93} n_{GM8}^{77} = n_{GM7}^{93} n_{GM6}^{77} = n_{GM7}^{93} n_{X4}^{77} = n_{X5}^{93} n_{X3}^{77} = n_{X5}^{93} n_{M5}^{77} = n_{M7}^{93} n_{M7}^{77} = n_{M7}^{93} n_{M8}^{77} = \\ n_{M6}^{93} n_{M6}^{77} &= n_{M6}^{93} n_{A5}^{77} = n_{A7}^{93} n_{A8}^{77} = n_{A6}^{93} n_{A7}^{77} = n_{A7}^{93} n_{A6}^{77} = n_{A6}^{93} n_{R4}^{77} = n_{R5}^{93} n_{R3}^{77} = n_{R5}^{93} n_{Z6}^{77} = n_{Z7}^{93} n_{Z8}^{77} = n_{Z6}^{93} n_{Z7}^{77} = n_{Z7}^{93} \\ n_{Z5}^{77} &= n_{Z6}^{93} \end{aligned}$$

## 6. Lowered SGs by higher-dimensional irreps of pairings in SG 94

The representative operations of SG/T for SG 94:

$$1 : (x, y, z), 2 : (\frac{1}{2} - y, x + \frac{1}{2}, z + \frac{1}{2}), 3 : (y + \frac{1}{2}, \frac{1}{2} - x, z + \frac{1}{2}), 4 : (x + \frac{1}{2}, \frac{1}{2} - y, \frac{1}{2} - z), 5 : (\frac{1}{2} - x, y + \frac{1}{2}, \frac{1}{2} - z), \\ 6 : (-x, -y, z), 7 : (y, x, -z), 8 : (-y, -x, -z).$$

The lower SG is SG 18 when the preserved operations are: **(sub-SG label is 1) 1, 4, 5, 6.**

The transformation is:  $(\mathbf{a}_{18}, \mathbf{b}_{18}, \mathbf{c}_{18}) = (\mathbf{a}_{94}, \mathbf{b}_{94}, \mathbf{c}_{94}) \begin{pmatrix} -1 & 0 & 0 \\ 0 & 1 & 0 \\ 0 & 0 & -1 \end{pmatrix}, \overrightarrow{O_{94}O_{18}} = \mathbf{a}_{18} + (\frac{3}{4})\mathbf{c}_{18}$

The reduction of higher dimensional irrep:

$$D_4 : E \rightarrow B_2 + B_3 \text{ of } D_2.$$

The correspondences of irreps at HSPs from original SG to lowered SG:

$$n_{GM5}^{18} = n_{GM6}^{94} + n_{GM7}^{94} \quad n_{X4}^{18} = n_{X4}^{94} \quad n_{X5}^{18} = n_{X3}^{94} \quad n_{X3}^{18} = n_{X5}^{94} \quad n_{X2}^{18} = n_{X2}^{94} \quad n_{S5}^{18} = n_{M6}^{94} + n_{M7}^{94} \quad n_{R5}^{18} = n_{A6}^{94} + n_{A7}^{94} \quad n_{U4}^{18} = n_{R2}^{94} \\ n_{U5}^{18} = n_{R5}^{94} \quad n_{U3}^{18} = n_{R3}^{94} \quad n_{U2}^{18} = n_{R4}^{94} \quad n_{Z5}^{18} = n_{Z6}^{94} + n_{Z7}^{94} \quad n_{T3}^{18} = n_{R4}^{94} \quad n_{T2}^{18} = n_{R5}^{94} \quad n_{T4}^{18} = n_{R3}^{94} \quad n_{T5}^{18} = n_{R2}^{94} \quad n_{Y3}^{18} = n_{X4}^{94} \quad n_{Y2}^{18} = n_{X5}^{94} \\ n_{X5}^{94} \quad n_{Y4}^{18} = n_{X3}^{94} \quad n_{Y5}^{18} = n_{X2}^{94}$$

The lower SG is SG 21 when the preserved operations are: **(sub-SG label is 2) 1, 6, 7, 8.**

The transformation is:  $(\mathbf{a}_{21}, \mathbf{b}_{21}, \mathbf{c}_{21}) = (\mathbf{a}_{94}, \mathbf{b}_{94}, \mathbf{c}_{94}) \begin{pmatrix} 1 & -1 & 0 \\ 1 & 1 & 0 \\ 0 & 0 & 1 \end{pmatrix}, \overrightarrow{O_{94}O_{21}} = \frac{1}{2}\mathbf{b}_{21} + (\frac{1}{2})\mathbf{c}_{21}$

The reduction of higher dimensional irrep:

$$D_4 : E \rightarrow B_2 + B_3 \text{ of } D_2.$$

The correspondences of irreps at HSPs from original SG to lowered SG:

$$n_{GM5}^{21} = n_{GM6}^{94} + n_{GM7}^{94} \quad n_{Y5}^{21} = n_{A6}^{94} + n_{A7}^{94} \quad n_{S4}^{21} = n_{X2}^{94} + n_{X4}^{94} \quad n_{S3}^{21} = n_{X3}^{94} + n_{X5}^{94} \quad n_{Z5}^{21} = n_{Z6}^{94} + n_{Z7}^{94} \quad n_{T5}^{21} = n_{A6}^{94} + n_{A7}^{94} \\ n_{R2}^{21} = n_{R2}^{94} + n_{R4}^{94} \quad n_{R3}^{21} = n_{R3}^{94} + n_{R5}^{94}$$

The lower SG is SG 77 when the preserved operations are: **(sub-SG label is 3) 1, 2, 3, 6.**

The transformation is:  $(\mathbf{a}_{77}, \mathbf{b}_{77}, \mathbf{c}_{77}) = (\mathbf{a}_{94}, \mathbf{b}_{94}, \mathbf{c}_{94}) \begin{pmatrix} -1 & 0 & 0 \\ 0 & 1 & 0 \\ 0 & 0 & -1 \end{pmatrix}, \overrightarrow{O_{94}O_{77}} = \mathbf{a}_{77} + (\frac{1}{2})\mathbf{b}_{77} + (\frac{1}{4})\mathbf{c}_{77}$

The reduction of higher dimensional irrep:

$$D_4 : E \rightarrow {}^2E + {}^1E \text{ of } C_4.$$

The correspondences of irreps at HSPs from original SG to lowered SG:

$$n_{GM5}^{77} = n_{GM6}^{94} \quad n_{GM7}^{77} = n_{GM6}^{94} \quad n_{GM8}^{77} = n_{GM7}^{94} \quad n_{GM6}^{77} = n_{GM7}^{94} \quad n_{X4}^{77} = n_{X3}^{94} + n_{X5}^{94} \quad n_{X3}^{77} = n_{X2}^{94} + n_{X4}^{94} \quad n_{M5}^{77} = n_{M6}^{94} \quad n_{M7}^{77} = n_{M7}^{94} \quad n_{M8}^{77} = n_{M6}^{94} \quad n_{M6}^{77} = n_{M7}^{94} \quad n_{A5}^{77} = n_{A6}^{94} \quad n_{A8}^{77} = n_{A6}^{94} \quad n_{A7}^{77} = n_{A7}^{94} \quad n_{A6}^{77} = n_{A7}^{94} \quad n_{R4}^{77} = n_{R3}^{94} + n_{R5}^{94} \quad n_{R3}^{77} = n_{R2}^{94} + n_{R4}^{94} \quad n_{Z6}^{77} = n_{Z7}^{94} \quad n_{Z8}^{77} = n_{Z6}^{94} \quad n_{Z7}^{77} = n_{Z7}^{94} \quad n_{Z5}^{77} = n_{Z6}^{94}$$

## 7. Lowered SGs by higher-dimensional irreps of pairings in SG 95

The representative operations of SG/T for SG 95:

$$1 : (x, y, z), 2 : (-y, x, z + \frac{3}{4}), 3 : (y, -x, z + \frac{1}{4}), 4 : (x, -y, \frac{1}{2} - z), 5 : (-x, y, -z), 6 : (-x, -y, z + \frac{1}{2}), 7 : (y, x, \frac{1}{4} - z), \\ 8 : (-y, -x, \frac{3}{4} - z).$$

The lower SG is SG 17 when the preserved operations are: **(sub-SG label is 1) 1, 4, 5, 6.**

The transformation is:  $(\mathbf{a}_{17}, \mathbf{b}_{17}, \mathbf{c}_{17}) = (\mathbf{a}_{95}, \mathbf{b}_{95}, \mathbf{c}_{95}) \begin{pmatrix} 0 & -1 & 0 \\ 1 & 0 & 0 \\ 0 & 0 & 1 \end{pmatrix}, \overrightarrow{O_{95}O_{17}} = \frac{1}{2}\mathbf{b}_{17} + (-\frac{1}{2})\mathbf{c}_{17}$

The reduction of higher dimensional irrep:

$$D_4 : E \rightarrow B_3 + B_2 \text{ of } D_2.$$

The correspondences of irreps at HSPs from original SG to lowered SG:

$$\begin{aligned} n_{GM5}^{17} &= n_{GM6}^{95} + n_{GM7}^{95} n_{X5}^{17} = n_{X5}^{95} n_{S5}^{17} = n_{M6}^{95} + n_{M7}^{95} n_{R5}^{17} = n_{A7}^{95} n_{R4}^{17} = n_{A3}^{95} + n_{A6}^{95} n_{R2}^{17} = n_{A4}^{95} + n_{A5}^{95} n_{R3}^{17} = n_{A7}^{95} n_{U5}^{17} = \\ n_{R3}^{95} n_{U4}^{17} &= n_{R4}^{95} n_{U2}^{17} = n_{R2}^{95} n_{U3}^{17} = n_{R5}^{95} n_{Z4}^{17} = n_{Z7}^{95} n_{Z5}^{17} = n_{Z4}^{95} + n_{Z5}^{95} n_{Z3}^{17} = n_{Z3}^{95} + n_{Z6}^{95} n_{Z2}^{17} = n_{Z7}^{95} n_{T4}^{17} = n_{R5}^{95} n_{T5}^{17} = n_{R4}^{95} \\ n_{T3}^{17} &= n_{R2}^{95} n_{T2}^{17} = n_{R3}^{95} n_{Y5}^{17} = n_{X5}^{95} \end{aligned}$$

The lower SG is SG 20 when the preserved operations are: **(sub-SG label is 2) 1, 6, 7, 8.**

$$\text{The transformation is: } (\mathbf{a}_{20}, \mathbf{b}_{20}, \mathbf{c}_{20}) = (\mathbf{a}_{95}, \mathbf{b}_{95}, \mathbf{c}_{95}) \begin{pmatrix} 1 & 1 & 0 \\ 1 & -1 & 0 \\ 0 & 0 & -1 \end{pmatrix}, \overrightarrow{O_{95}O_{20}} = \frac{3}{8}\mathbf{c}_{20}$$

The reduction of higher dimensional irrep:

$$D_4 : E \rightarrow B_2 + B_3 \text{ of } D_2.$$

The correspondences of irreps at HSPs from original SG to lowered SG:

$$\begin{aligned} n_{GM5}^{20} &= n_{GM6}^{95} + n_{GM7}^{95} n_{Y5}^{20} = n_{M6}^{95} + n_{M7}^{95} n_{S4}^{20} = n_{X5}^{95} n_{S3}^{20} = n_{X5}^{95} n_{Z5}^{20} = n_{Z3}^{95} + n_{Z4}^{95} n_{Z4}^{20} = n_{Z7}^{95} n_{Z2}^{20} = n_{Z7}^{95} n_{Z3}^{20} = \\ n_{Z5}^{95} + n_{Z6}^{95} n_{T5}^{20} &= n_{A3}^{95} + n_{A4}^{95} n_{T4}^{20} = n_{A7}^{95} n_{T2}^{20} = n_{A7}^{95} n_{T3}^{20} = n_{A5}^{95} + n_{A6}^{95} n_{R4}^{20} = n_{R3}^{95} + n_{R5}^{95} n_{R3}^{20} = n_{R2}^{95} + n_{R4}^{95} \end{aligned}$$

The lower SG is SG 78 when the preserved operations are: **(sub-SG label is 3) 1, 2, 3, 6.**

$$\text{The transformation is: } (\mathbf{a}_{78}, \mathbf{b}_{78}, \mathbf{c}_{78}) = (\mathbf{a}_{95}, \mathbf{b}_{95}, \mathbf{c}_{95}) \begin{pmatrix} -1 & 0 & 0 \\ 0 & 1 & 0 \\ 0 & 0 & -1 \end{pmatrix}, \overrightarrow{O_{95}O_{78}} = \frac{1}{2}\mathbf{a}_{78} + \left(\frac{1}{2}\right)\mathbf{b}_{78} + \left(\frac{1}{4}\right)\mathbf{c}_{78}$$

The reduction of higher dimensional irrep:

$$D_4 : E \rightarrow {}^2E + {}^1E \text{ of } C_4.$$

The correspondences of irreps at HSPs from original SG to lowered SG:

$$\begin{aligned} n_{GM5}^{78} &= n_{GM6}^{95} n_{GM7}^{78} = n_{GM6}^{95} n_{GM8}^{78} = n_{GM7}^{95} n_{GM6}^{78} = n_{GM7}^{95} n_{X4}^{78} = n_{X5}^{95} n_{X3}^{78} = n_{X5}^{95} n_{M5}^{78} = n_{M7}^{95} n_{M7}^{78} = n_{M7}^{95} n_{M8}^{78} = \\ n_{M6}^{95} n_{M6}^{78} &= n_{M6}^{95} n_{A5}^{78} = n_{A7}^{95} n_{A7}^{78} = n_{A4}^{95} + n_{A6}^{95} n_{A8}^{78} = n_{A3}^{95} + n_{A5}^{95} n_{A6}^{78} = n_{A7}^{95} n_{R4}^{78} = n_{R2}^{95} + n_{R4}^{95} n_{R3}^{78} = n_{R3}^{95} + n_{R5}^{95} n_{Z7}^{78} = \\ n_{Z3}^{95} + n_{Z5}^{95} n_{Z6}^{78} &= n_{Z7}^{95} n_{Z5}^{78} = n_{Z7}^{95} n_{Z8}^{78} = n_{Z4}^{95} + n_{Z6}^{95} \end{aligned}$$

## 8. Lowered SGs by higher-dimensional irreps of pairings in SG 96

The representative operations of SG/T for SG 96:

$$\begin{aligned} 1 : (x, y, z), 2 : \left(\frac{1}{2} - y, x + \frac{1}{2}, z + \frac{3}{4}\right), 3 : \left(y + \frac{1}{2}, \frac{1}{2} - x, z + \frac{1}{4}\right), 4 : \left(x + \frac{1}{2}, \frac{1}{2} - y, \frac{1}{4} - z\right), 5 : \left(\frac{1}{2} - x, y + \frac{1}{2}, \frac{3}{4} - z\right), \\ 6 : \left(-x, -y, z + \frac{1}{2}\right), 7 : (y, x, -z), 8 : \left(-y, -x, \frac{1}{2} - z\right). \end{aligned}$$

The lower SG is SG 19 when the preserved operations are: **(sub-SG label is 1) 1, 4, 5, 6.**

$$\text{The transformation is: } (\mathbf{a}_{19}, \mathbf{b}_{19}, \mathbf{c}_{19}) = (\mathbf{a}_{96}, \mathbf{b}_{96}, \mathbf{c}_{96}) \begin{pmatrix} -1 & 0 & 0 \\ 0 & 0 & 1 \\ 0 & 1 & 0 \end{pmatrix}, \overrightarrow{O_{96}O_{19}} = \mathbf{a}_{19} + \left(-\frac{1}{8}\right)\mathbf{b}_{19} + \left(\frac{3}{4}\right)\mathbf{c}_{19}$$

The reduction of higher dimensional irrep:

$$D_4 : E \rightarrow B_1 + B_3 \text{ of } D_2.$$

The correspondences of irreps at HSPs from original SG to lowered SG:

$$\begin{aligned} n_{GM5}^{19} &= n_{GM6}^{96} + n_{GM7}^{96} n_{X4}^{19} = n_{X4}^{96} n_{X5}^{19} = n_{X3}^{96} n_{X3}^{19} = n_{X2}^{96} n_{X2}^{19} = n_{X5}^{96} n_{S5}^{19} = n_{R5}^{96} n_{R3}^{19} = n_{A7}^{96} n_{R2}^{19} = n_{A4}^{96} + n_{A5}^{96} n_{R4}^{19} = \\ n_{A7}^{96} n_{R5}^{19} &= n_{A3}^{96} + n_{A6}^{96} n_{U5}^{19} = n_{M6}^{96} + n_{M7}^{96} n_{Z4}^{19} = n_{X5}^{96} n_{Z5}^{19} = n_{X4}^{96} n_{Z3}^{19} = n_{X3}^{96} n_{Z2}^{19} = n_{X2}^{96} n_{T5}^{19} = n_{R5}^{96} n_{Y3}^{19} = n_{Z3}^{96} + n_{Z6}^{96} \\ n_{Y2}^{19} &= n_{Z7}^{96} n_{Y4}^{19} = n_{Z4}^{96} + n_{Z5}^{96} n_{Y5}^{19} = n_{Z7}^{96} \end{aligned}$$

The lower SG is SG 20 when the preserved operations are: **(sub-SG label is 2) 1, 6, 7, 8.**

$$\text{The transformation is: } (\mathbf{a}_{20}, \mathbf{b}_{20}, \mathbf{c}_{20}) = (\mathbf{a}_{96}, \mathbf{b}_{96}, \mathbf{c}_{96}) \begin{pmatrix} -1 & -1 & 0 \\ -1 & 1 & 0 \\ 0 & 0 & -1 \end{pmatrix}, \overrightarrow{O_{96}O_{20}} = \frac{1}{2}\mathbf{a}_{20} + \left(\frac{1}{2}\right)\mathbf{b}_{20}$$

The reduction of higher dimensional irrep:

$$D_4 : E \rightarrow B_2 + B_3 \text{ of } D_2.$$

The correspondences of irreps at HSPs from original SG to lowered SG:

$$\begin{aligned} n_{GM5}^{20} &= n_{GM6}^{96} + n_{GM7}^{96} n_{Y5}^{20} = n_{M6}^{96} + n_{M7}^{96} n_{S4}^{20} = n_{X3}^{96} + n_{X5}^{96} n_{S3}^{20} = n_{X2}^{96} + n_{X4}^{96} n_{Z5}^{20} = n_{Z3}^{96} + n_{Z4}^{96} n_{Z4}^{20} = n_{Z7}^{96} n_{Z2}^{20} = n_{Z7}^{96} \\ n_{Z3}^{20} &= n_{Z5}^{96} + n_{Z6}^{96} n_{T5}^{20} = n_{A3}^{96} + n_{A4}^{96} n_{T4}^{20} = n_{A7}^{96} n_{T2}^{20} = n_{A7}^{96} n_{T3}^{20} = n_{A5}^{96} + n_{A6}^{96} n_{R4}^{20} = n_{R5}^{96} n_{R3}^{20} = n_{R5}^{96} \end{aligned}$$

The lower SG is SG 78 when the preserved operations are: **(sub-SG label is 3) 1, 2, 3, 6.**

The transformation is:  $(\mathbf{a}_{78}, \mathbf{b}_{78}, \mathbf{c}_{78}) = (\mathbf{a}_{96}, \mathbf{b}_{96}, \mathbf{c}_{96}) \begin{pmatrix} -1 & 0 & 0 \\ 0 & 1 & 0 \\ 0 & 0 & -1 \end{pmatrix}, \overrightarrow{O_{96}O_{78}} = \mathbf{a}_{78} + \left(\frac{1}{2}\right)\mathbf{b}_{78} + \left(-\frac{1}{8}\right)\mathbf{c}_{78}$

The reduction of higher dimensional irrep:

$$D_4 : E \rightarrow {}^2E + {}^1E \text{ of } C_4.$$

The correspondences of irreps at HSPs from original SG to lowered SG:

$$\begin{aligned} n_{GM5}^{78} &= n_{GM6}^{96} n_{GM7}^{78} = n_{GM6}^{96} n_{GM8}^{78} = n_{GM7}^{96} n_{GM6}^{78} = n_{GM7}^{96} n_{X4}^{78} = n_{X3}^{96} + n_{X5}^{96} n_{X3}^{78} = n_{X2}^{96} + n_{X4}^{96} n_{M5}^{78} = n_{M6}^{96} n_{M7}^{78} = \\ n_{M7}^{96} n_{M8}^{78} &= n_{M6}^{96} n_{M6}^{78} = n_{M7}^{96} n_{A5}^{78} = n_{A4}^{96} + n_{A6}^{96} n_{A7}^{78} = n_{A7}^{96} n_{A8}^{78} = n_{A7}^{96} n_{A6}^{78} = n_{A3}^{96} + n_{A5}^{96} n_{R4}^{78} = n_{R5}^{96} n_{R3}^{78} = n_{R5}^{96} n_{Z7}^{78} = \\ n_{Z3}^{96} + n_{Z5}^{96} n_{Z6}^{78} &= n_{Z7}^{96} n_{Z5}^{78} = n_{Z7}^{96} n_{Z8}^{78} = n_{Z4}^{96} + n_{Z6}^{96} \end{aligned}$$

## 9. Lowered SGs by higher-dimensional irreps of pairings in SG 97

The representative operations of SG/T for SG 97:

$$1 : (x, y, z), 2 : (-y, x, z), 3 : (y, -x, z), 4 : (x, -y, -z), 5 : (-x, y, -z), 6 : (-x, -y, z), 7 : (y, x, -z), 8 : (-y, -x, -z).$$

The lower SG is SG 23 when the preserved operations are: **(sub-SG label is 1) 1, 4, 5, 6.**

The transformation is:  $(\mathbf{a}_{23}, \mathbf{b}_{23}, \mathbf{c}_{23}) = (\mathbf{a}_{97}, \mathbf{b}_{97}, \mathbf{c}_{97}) \begin{pmatrix} 0 & 0 & 1 \\ 1 & 0 & 0 \\ 0 & 1 & 0 \end{pmatrix}, \overrightarrow{O_{97}O_{23}} = -\frac{1}{2}\mathbf{b}_{23}$

The reduction of higher dimensional irrep:

$$D_4 : E \rightarrow B_1 + B_3 \text{ of } D_2.$$

The correspondences of irreps at HSPs from original SG to lowered SG:

$$\begin{aligned} n_{GM5}^{23} &= n_{GM6}^{97} + n_{GM7}^{97} n_{X5}^{23} = n_{M6}^{97} + n_{M7}^{97} n_{T4}^{23} = n_{N4}^{97} n_{T3}^{23} = n_{N3}^{97} n_{W5}^{23} = n_{P5}^{97} n_{R4}^{23} = n_{X5}^{97} n_{R3}^{23} = n_{X5}^{97} n_{S3}^{23} = n_{N4}^{97} n_{S4}^{23} = \\ n_{N3}^{97} \end{aligned}$$

The lower SG is SG 22 when the preserved operations are: **(sub-SG label is 2) 1, 6, 7, 8.**

The transformation is:  $(\mathbf{a}_{22}, \mathbf{b}_{22}, \mathbf{c}_{22}) = (\mathbf{a}_{97}, \mathbf{b}_{97}, \mathbf{c}_{97}) \begin{pmatrix} 1 & -1 & 0 \\ 1 & 1 & 0 \\ 0 & 0 & 1 \end{pmatrix}, \overrightarrow{O_{97}O_{22}} = \frac{1}{4}\mathbf{a}_{22} + \left(-\frac{1}{4}\right)\mathbf{b}_{22} + \left(-\frac{1}{4}\right)\mathbf{c}_{22}$

The reduction of higher dimensional irrep:

$$D_4 : E \rightarrow B_2 + B_3 \text{ of } D_2.$$

The correspondences of irreps at HSPs from original SG to lowered SG:

$$n_{GM5}^{22} = n_{GM6}^{97} + n_{GM7}^{97} n_{Y5}^{22} = n_{X5}^{97} n_{L2}^{22} = n_{N3}^{97} + n_{N4}^{97} n_{Z5}^{22} = n_{M6}^{97} + n_{M7}^{97} n_{T5}^{22} = n_{X5}^{97}$$

The lower SG is SG 79 when the preserved operations are: **(sub-SG label is 3) 1, 2, 3, 6.**

The transformation is:  $(\mathbf{a}_{79}, \mathbf{b}_{79}, \mathbf{c}_{79}) = (\mathbf{a}_{97}, \mathbf{b}_{97}, \mathbf{c}_{97}) \begin{pmatrix} 0 & 1 & 0 \\ -1 & 0 & 0 \\ 0 & 0 & 1 \end{pmatrix}, \overrightarrow{O_{97}O_{79}} = \frac{1}{2}\mathbf{a}_{79} + \left(\frac{1}{2}\right)\mathbf{b}_{79}$

The reduction of higher dimensional irrep:

$$D_4 : E \rightarrow {}^2E + {}^1E \text{ of } C_4.$$

The correspondences of irreps at HSPs from original SG to lowered SG:

$$\begin{aligned} n_{GM5}^{79} &= n_{GM6}^{97} n_{GM7}^{79} = n_{GM6}^{97} n_{GM8}^{79} = n_{GM7}^{97} n_{GM6}^{79} = n_{GM7}^{97} n_{M5}^{79} = n_{M6}^{97} n_{M7}^{79} = n_{M6}^{97} n_{M8}^{79} = n_{M7}^{97} n_{M6}^{79} = n_{M7}^{97} n_{X4}^{79} = \\ n_{X5}^{97} n_{X3}^{79} &= n_{X5}^{97} n_{P4}^{79} = n_{P5}^{97} n_{P3}^{79} = n_{P5}^{97} n_{N2}^{79} = n_{N3}^{97} + n_{N4}^{97} \end{aligned}$$

### 10. Lowered SGs by higher-dimensional irreps of pairings in SG 98

The representative operations of SG/T for SG 98:

$$1 : (x, y, z), 2 : (-y, x + \frac{1}{2}, z + \frac{1}{4}), 3 : (y, \frac{1}{2} - x, z + \frac{1}{4}), 4 : (x, \frac{1}{2} - y, \frac{1}{4} - z), 5 : (-x, y + \frac{1}{2}, \frac{1}{4} - z), 6 : (-x, -y, z), \\ 7 : (y, x, -z), 8 : (-y, -x, -z).$$

The lower SG is SG 24 when the preserved operations are: **(sub-SG label is 1) 1, 4, 5, 6.**

The transformation is:  $(\mathbf{a}_{24}, \mathbf{b}_{24}, \mathbf{c}_{24}) = (\mathbf{a}_{98}, \mathbf{b}_{98}, \mathbf{c}_{98}) \begin{pmatrix} 0 & 1 & 0 \\ 0 & 0 & 1 \\ 1 & 0 & 0 \end{pmatrix}, \overrightarrow{O_{98}O_{24}} = -\frac{1}{8}\mathbf{a}_{24} + (-\frac{1}{2})\mathbf{b}_{24} + (\frac{1}{4})\mathbf{c}_{24}$

The reduction of higher dimensional irrep:

$$D_4 : E \rightarrow B_1 + B_2 \text{ of } D_2.$$

The correspondences of irreps at HSPs from original SG to lowered SG:

$$n_{GM5}^{24} = n_{GM6}^{98} + n_{GM7}^{98} \quad n_{X5}^{24} = n_{M6}^{98} + n_{M7}^{98} \quad n_{T3}^{24} = n_{N4}^{98} \quad n_{T4}^{24} = n_{N3}^{98} \quad n_{W3}^{24} = n_{P2}^{98} \quad n_{W2}^{24} = n_{P4}^{98} \quad n_{W4}^{24} = n_{P3}^{98} \quad n_{W5}^{24} = n_{P5}^{98} \quad n_{R3}^{24} = n_{N3}^{98} \quad n_{R4}^{24} = n_{N4}^{98} \quad n_{S4}^{24} = n_{X5}^{98} \quad n_{S3}^{24} = n_{X5}^{98}$$

The lower SG is SG 22 when the preserved operations are: **(sub-SG label is 2) 1, 6, 7, 8.**

The transformation is:  $(\mathbf{a}_{22}, \mathbf{b}_{22}, \mathbf{c}_{22}) = (\mathbf{a}_{98}, \mathbf{b}_{98}, \mathbf{c}_{98}) \begin{pmatrix} 1 & -1 & 0 \\ 1 & 1 & 0 \\ 0 & 0 & 1 \end{pmatrix}, \overrightarrow{O_{98}O_{22}} = \frac{1}{4}\mathbf{a}_{22} + (-\frac{1}{4})\mathbf{b}_{22} + (-\frac{1}{4})\mathbf{c}_{22}$

The reduction of higher dimensional irrep:

$$D_4 : E \rightarrow B_2 + B_3 \text{ of } D_2.$$

The correspondences of irreps at HSPs from original SG to lowered SG:

$$n_{GM5}^{22} = n_{GM6}^{98} + n_{GM7}^{98} \quad n_{Y5}^{22} = n_{X5}^{98} \quad n_{L2}^{22} = n_{N3}^{98} + n_{N4}^{98} \quad n_{Z5}^{22} = n_{M6}^{98} + n_{M7}^{98} \quad n_{T5}^{22} = n_{X5}^{98}$$

The lower SG is SG 80 when the preserved operations are: **(sub-SG label is 3) 1, 2, 3, 6.**

The transformation is:  $(\mathbf{a}_{80}, \mathbf{b}_{80}, \mathbf{c}_{80}) = (\mathbf{a}_{98}, \mathbf{b}_{98}, \mathbf{c}_{98}) \begin{pmatrix} 0 & 1 & 0 \\ -1 & 0 & 0 \\ 0 & 0 & 1 \end{pmatrix}, \overrightarrow{O_{98}O_{80}} = \frac{1}{2}\mathbf{a}_{80} + (-\frac{1}{8})\mathbf{c}_{80}$

The reduction of higher dimensional irrep:

$$D_4 : E \rightarrow {}^2E + {}^1E \text{ of } C_4.$$

The correspondences of irreps at HSPs from original SG to lowered SG:

$$n_{GM5}^{80} = n_{GM6}^{98} \quad n_{GM7}^{80} = n_{GM6}^{98} \quad n_{GM8}^{80} = n_{GM7}^{98} \quad n_{GM6}^{80} = n_{GM7}^{98} \quad n_{M7}^{80} = n_{M6}^{98} \quad n_{M5}^{80} = n_{M6}^{98} \quad n_{M6}^{80} = n_{M7}^{98} \quad n_{M8}^{80} = n_{M7}^{98} \quad n_{X4}^{80} = n_{X5}^{98} \quad n_{X3}^{80} = n_{X5}^{98} \quad n_{P4}^{80} = n_{P3}^{98} + n_{P5}^{98} \quad n_{P3}^{80} = n_{P2}^{98} + n_{P4}^{98} \quad n_{N2}^{80} = n_{N3}^{98} + n_{N4}^{98}$$

### 11. Lowered SGs by higher-dimensional irreps of pairings in SG 99

The representative operations of SG/T for SG 99:

$$1 : (x, y, z), 2 : (-y, x, z), 3 : (y, -x, z), 4 : (-x, -y, z), 5 : (-x, y, z), 6 : (x, -y, z), 7 : (-y, -x, z), 8 : (y, x, z).$$

The lower SG is SG 25 when the preserved operations are: **(sub-SG label is 1) 1, 4, 5, 6.**

The transformation is:  $(\mathbf{a}_{25}, \mathbf{b}_{25}, \mathbf{c}_{25}) = (\mathbf{a}_{99}, \mathbf{b}_{99}, \mathbf{c}_{99}) \begin{pmatrix} 1 & 0 & 0 \\ 0 & 1 & 0 \\ 0 & 0 & 1 \end{pmatrix}, \overrightarrow{O_{99}O_{25}} = \frac{1}{2}\mathbf{a}_{25}$

The reduction of higher dimensional irrep:

$$C_{4v} : E \rightarrow B_1 + B_2 \text{ of } C_{2v}.$$

The correspondences of irreps at HSPs from original SG to lowered SG:

$$n_{GM5}^{25} = n_{GM6}^{99} + n_{GM7}^{99} \quad n_{X5}^{25} = n_{X5}^{99} \quad n_{S5}^{25} = n_{M6}^{99} + n_{M7}^{99} \quad n_{R5}^{25} = n_{A6}^{99} + n_{A7}^{99} \quad n_{U5}^{25} = n_{R5}^{99} \quad n_{Z5}^{25} = n_{Z6}^{99} + n_{Z7}^{99} \quad n_{T5}^{25} = n_{R5}^{99} \quad n_{Y5}^{25} = n_{R5}^{99}$$

$n_{X5}^{99}$ 

The lower SG is SG 35 when the preserved operations are: **(sub-SG label is 2) 1, 4, 7, 8.**

The transformation is:  $(\mathbf{a}_{35}, \mathbf{b}_{35}, \mathbf{c}_{35}) = (\mathbf{a}_{99}, \mathbf{b}_{99}, \mathbf{c}_{99}) \begin{pmatrix} 1 & -1 & 0 \\ 1 & 1 & 0 \\ 0 & 0 & 1 \end{pmatrix}, \overrightarrow{O_{99}O_{35}} = \mathbf{0}$

The reduction of higher dimensional irrep:

$C_{4v} : E \rightarrow B_1 + B_2$  of  $C_{2v}$ .

The correspondences of irreps at HSPs from original SG to lowered SG:

$$n_{GM5}^{35} = n_{GM6}^{99} + n_{GM7}^{99} n_{Y5}^{35} = n_{M6}^{99} + n_{M7}^{99} n_{S4}^{35} = n_{X5}^{99} n_{S3}^{35} = n_{X5}^{99} n_{Z5}^{35} = n_{Z6}^{99} + n_{Z7}^{99} n_{T5}^{35} = n_{A6}^{99} + n_{A7}^{99} n_{R4}^{35} = n_{R5}^{99} n_{R3}^{35} = n_{R5}^{99}$$

The lower SG is SG 75 when the preserved operations are: **(sub-SG label is 3) 1, 2, 3, 4.**

The transformation is:  $(\mathbf{a}_{75}, \mathbf{b}_{75}, \mathbf{c}_{75}) = (\mathbf{a}_{99}, \mathbf{b}_{99}, \mathbf{c}_{99}) \begin{pmatrix} -1 & 0 & 0 \\ 0 & -1 & 0 \\ 0 & 0 & 1 \end{pmatrix}, \overrightarrow{O_{99}O_{75}} = -\frac{1}{2}\mathbf{a}_{75} + (\frac{1}{2})\mathbf{b}_{75}$

The reduction of higher dimensional irrep:

$C_{4v} : E \rightarrow {}^2E + {}^1E$  of  $C_4$ .

The correspondences of irreps at HSPs from original SG to lowered SG:

$$n_{GM5}^{75} = n_{GM6}^{99} n_{GM7}^{75} = n_{GM6}^{99} n_{GM8}^{75} = n_{GM7}^{99} n_{GM6}^{75} = n_{GM7}^{99} n_{X4}^{75} = n_{X5}^{99} n_{X3}^{75} = n_{X5}^{99} n_{M5}^{75} = n_{M7}^{99} n_{M7}^{75} = n_{M7}^{99} n_{M8}^{75} = n_{M6}^{99} n_{M6}^{75} = n_{M6}^{99} n_{A5}^{75} = n_{A7}^{99} n_{A7}^{75} = n_{A7}^{99} n_{A8}^{75} = n_{A6}^{99} n_{A6}^{75} = n_{A6}^{99} n_{R4}^{75} = n_{R5}^{99} n_{R3}^{75} = n_{R5}^{99} n_{Z5}^{75} = n_{Z6}^{99} n_{Z7}^{75} = n_{Z6}^{99} n_{Z8}^{75} = n_{Z7}^{99} n_{Z6}^{75} = n_{Z7}^{99}$$

## 12. Lowered SGs by higher-dimensional irreps of pairings in SG 100

The representative operations of SG/T for SG 100:

$$1 : (x, y, z), 2 : (-y, x, z), 3 : (y, -x, z), 4 : (-x, -y, z), 5 : (\frac{1}{2} - x, y + \frac{1}{2}, z), 6 : (x + \frac{1}{2}, \frac{1}{2} - y, z), 7 : (\frac{1}{2} - y, \frac{1}{2} - x, z), 8 : (y + \frac{1}{2}, x + \frac{1}{2}, z).$$

The lower SG is SG 32 when the preserved operations are: **(sub-SG label is 1) 1, 4, 5, 6.**

The transformation is:  $(\mathbf{a}_{32}, \mathbf{b}_{32}, \mathbf{c}_{32}) = (\mathbf{a}_{100}, \mathbf{b}_{100}, \mathbf{c}_{100}) \begin{pmatrix} 1 & 0 & 0 \\ 0 & 1 & 0 \\ 0 & 0 & 1 \end{pmatrix}, \overrightarrow{O_{100}O_{32}} = \frac{1}{2}\mathbf{a}_{32} + (\frac{1}{2})\mathbf{b}_{32}$

The reduction of higher dimensional irrep:

$C_{4v} : E \rightarrow B_1 + B_2$  of  $C_{2v}$ .

The correspondences of irreps at HSPs from original SG to lowered SG:

$$n_{GM5}^{32} = n_{GM6}^{100} + n_{GM7}^{100} n_{X3}^{32} = n_{X2}^{100} n_{X5}^{32} = n_{X4}^{100} n_{X2}^{32} = n_{X5}^{100} n_{X4}^{32} = n_{X3}^{100} n_{S5}^{32} = n_{M6}^{100} + n_{M7}^{100} n_{R5}^{32} = n_{A6}^{100} + n_{A7}^{100} n_{U3}^{32} = n_{R2}^{100} n_{U5}^{32} = n_{R4}^{100} n_{U2}^{32} = n_{R5}^{100} n_{U4}^{32} = n_{R3}^{100} n_{Z5}^{32} = n_{Z6}^{100} + n_{Z7}^{100} n_{T5}^{32} = n_{R4}^{100} n_{T3}^{32} = n_{R2}^{100} n_{T4}^{32} = n_{R5}^{100} n_{T2}^{32} = n_{R3}^{100} n_{Y5}^{32} = n_{X4}^{100} n_{Y3}^{32} = n_{X2}^{100} n_{Y4}^{32} = n_{X5}^{100} n_{Y2}^{32} = n_{X3}^{100}$$

The lower SG is SG 35 when the preserved operations are: **(sub-SG label is 2) 1, 4, 7, 8.**

The transformation is:  $(\mathbf{a}_{35}, \mathbf{b}_{35}, \mathbf{c}_{35}) = (\mathbf{a}_{100}, \mathbf{b}_{100}, \mathbf{c}_{100}) \begin{pmatrix} 1 & -1 & 0 \\ 1 & 1 & 0 \\ 0 & 0 & 1 \end{pmatrix}, \overrightarrow{O_{100}O_{35}} = \frac{1}{4}\mathbf{a}_{35} + (\frac{1}{4})\mathbf{b}_{35}$

The reduction of higher dimensional irrep:

$C_{4v} : E \rightarrow B_1 + B_2$  of  $C_{2v}$ .

The correspondences of irreps at HSPs from original SG to lowered SG:

$$n_{GM5}^{35} = n_{GM6}^{100} + n_{GM7}^{100} n_{Y5}^{35} = n_{M6}^{100} + n_{M7}^{100} n_{S4}^{35} = n_{X2}^{100} + n_{X4}^{100} n_{S3}^{35} = n_{X3}^{100} + n_{X5}^{100} n_{Z5}^{35} = n_{Z6}^{100} + n_{Z7}^{100} n_{T5}^{35} = n_{A6}^{100} + n_{A7}^{100} n_{R4}^{35} = n_{R2}^{100} + n_{R4}^{100} n_{R3}^{35} = n_{R3}^{100} + n_{R5}^{100}$$

The lower SG is SG 75 when the preserved operations are: **(sub-SG label is 3) 1, 2, 3, 4.**

The transformation is:  $(\mathbf{a}_{75}, \mathbf{b}_{75}, \mathbf{c}_{75}) = (\mathbf{a}_{100}, \mathbf{b}_{100}, \mathbf{c}_{100}) \begin{pmatrix} -1 & 0 & 0 \\ 0 & -1 & 0 \\ 0 & 0 & 1 \end{pmatrix}, \overrightarrow{O_{100}O_{75}} = -\frac{1}{2}\mathbf{a}_{75} + (\frac{1}{2})\mathbf{b}_{75}$

The reduction of higher dimensional irrep:

$C_{4v} : E \rightarrow {}^2E + {}^1E$  of  $C_4$ .

The correspondences of irreps at HSPs from original SG to lowered SG:

$$\begin{aligned} n_{GM5}^{75} &= n_{GM6}^{100} n_{GM7}^{75} = n_{GM6}^{100} n_{GM8}^{75} = n_{GM7}^{100} n_{GM6}^{75} = n_{GM7}^{100} n_{X4}^{75} = n_{X2}^{100} + n_{X4}^{100} n_{X3}^{75} = n_{X3}^{100} + n_{X5}^{100} n_{M5}^{75} = n_{M7}^{100} n_{M7}^{75} = \\ n_{M6}^{100} n_{M8}^{75} &= n_{M7}^{100} n_{M6}^{75} = n_{M6}^{100} n_{A5}^{75} = n_{A7}^{100} n_{A7}^{75} = n_{A6}^{100} n_{A8}^{75} = n_{A7}^{100} n_{A6}^{75} = n_{A6}^{100} n_{R4}^{75} = n_{R2}^{100} + n_{R4}^{100} n_{R3}^{75} = n_{R3}^{100} + n_{R5}^{100} \\ n_{Z5}^{75} &= n_{Z6}^{100} n_{Z7}^{75} = n_{Z6}^{100} n_{Z8}^{75} = n_{Z7}^{100} n_{Z6}^{75} = n_{Z7}^{100} \end{aligned}$$

### 13. Lowered SGs by higher-dimensional irreps of pairings in SG 101

The representative operations of SG/T for SG 101:

$$1 : (x, y, z), 2 : (-y, x, z + \frac{1}{2}), 3 : (y, -x, z + \frac{1}{2}), 4 : (-x, -y, z), 5 : (-x, y, z + \frac{1}{2}), 6 : (x, -y, z + \frac{1}{2}), 7 : (-y, -x, z), 8 : (y, x, z).$$

The lower SG is SG 27 when the preserved operations are: **(sub-SG label is 1) 1, 4, 5, 6.**

The transformation is:  $(\mathbf{a}_{27}, \mathbf{b}_{27}, \mathbf{c}_{27}) = (\mathbf{a}_{101}, \mathbf{b}_{101}, \mathbf{c}_{101}) \begin{pmatrix} 1 & 0 & 0 \\ 0 & 1 & 0 \\ 0 & 0 & 1 \end{pmatrix}, \overrightarrow{O_{101}O_{27}} = \frac{1}{2}\mathbf{a}_{27}$

The reduction of higher dimensional irrep:

$C_{4v} : E \rightarrow B_1 + B_2$  of  $C_{2v}$ .

The correspondences of irreps at HSPs from original SG to lowered SG:

$$\begin{aligned} n_{GM5}^{27} &= n_{GM6}^{101} + n_{GM7}^{101} n_{X5}^{27} = n_{X5}^{101} n_{S5}^{27} = n_{M6}^{101} + n_{M7}^{101} n_{R5}^{27} = n_{A6}^{101} + n_{A7}^{101} n_{U5}^{27} = n_{R5}^{101} n_{Z5}^{27} = n_{Z6}^{101} + n_{Z7}^{101} n_{T5}^{27} = n_{R5}^{101} \\ n_{Y5}^{27} &= n_{X5}^{101} \end{aligned}$$

The lower SG is SG 35 when the preserved operations are: **(sub-SG label is 2) 1, 4, 7, 8.**

The transformation is:  $(\mathbf{a}_{35}, \mathbf{b}_{35}, \mathbf{c}_{35}) = (\mathbf{a}_{101}, \mathbf{b}_{101}, \mathbf{c}_{101}) \begin{pmatrix} 1 & -1 & 0 \\ 1 & 1 & 0 \\ 0 & 0 & 1 \end{pmatrix}, \overrightarrow{O_{101}O_{35}} = \mathbf{0}$

The reduction of higher dimensional irrep:

$C_{4v} : E \rightarrow B_1 + B_2$  of  $C_{2v}$ .

The correspondences of irreps at HSPs from original SG to lowered SG:

$$\begin{aligned} n_{GM5}^{35} &= n_{GM6}^{101} + n_{GM7}^{101} n_{Y5}^{35} = n_{M6}^{101} + n_{M7}^{101} n_{S4}^{35} = n_{X5}^{101} n_{S3}^{35} = n_{X5}^{101} n_{Z5}^{35} = n_{Z6}^{101} + n_{Z7}^{101} n_{T5}^{35} = n_{A6}^{101} + n_{A7}^{101} n_{R4}^{35} = n_{R5}^{101} \\ n_{R5}^{35} &= n_{R5}^{101} \end{aligned}$$

The lower SG is SG 77 when the preserved operations are: **(sub-SG label is 3) 1, 2, 3, 4.**

The transformation is:  $(\mathbf{a}_{77}, \mathbf{b}_{77}, \mathbf{c}_{77}) = (\mathbf{a}_{101}, \mathbf{b}_{101}, \mathbf{c}_{101}) \begin{pmatrix} -1 & 0 & 0 \\ 0 & 1 & 0 \\ 0 & 0 & -1 \end{pmatrix}, \overrightarrow{O_{101}O_{77}} = \frac{1}{2}\mathbf{a}_{77} + (\frac{1}{2})\mathbf{b}_{77}$

The reduction of higher dimensional irrep:

$C_{4v} : E \rightarrow {}^2E + {}^1E$  of  $C_4$ .

The correspondences of irreps at HSPs from original SG to lowered SG:

$$\begin{aligned} n_{GM5}^{77} &= n_{GM6}^{101} n_{GM7}^{77} = n_{GM6}^{101} n_{GM8}^{77} = n_{GM7}^{101} n_{GM6}^{77} = n_{GM7}^{101} n_{X4}^{77} = n_{X5}^{101} n_{X3}^{77} = n_{X5}^{101} n_{M5}^{77} = n_{M7}^{101} n_{M7}^{77} = n_{M7}^{101} n_{M8}^{77} = \\ n_{M6}^{101} n_{M6}^{77} &= n_{M6}^{101} n_{A5}^{77} = n_{A6}^{101} n_{A8}^{77} = n_{A6}^{101} n_{A7}^{77} = n_{A7}^{101} n_{A6}^{77} = n_{A7}^{101} n_{R4}^{77} = n_{R5}^{101} n_{R3}^{77} = n_{R5}^{101} n_{Z6}^{77} = n_{Z6}^{101} n_{Z8}^{77} = n_{Z6}^{101} n_{Z7}^{77} = \\ n_{Z7}^{101} n_{Z5}^{77} &= n_{Z7}^{101} \end{aligned}$$

#### 14. Lowered SGs by higher-dimensional irreps of pairings in SG 102

The representative operations of SG/T for SG 102:

$$1 : (x, y, z), 2 : \left(\frac{1}{2} - y, x + \frac{1}{2}, z + \frac{1}{2}\right), 3 : \left(y + \frac{1}{2}, \frac{1}{2} - x, z + \frac{1}{2}\right), 4 : (-x, -y, z), 5 : \left(\frac{1}{2} - x, y + \frac{1}{2}, z + \frac{1}{2}\right), \\ 6 : \left(x + \frac{1}{2}, \frac{1}{2} - y, z + \frac{1}{2}\right), 7 : (-y, -x, z), 8 : (y, x, z).$$

The lower SG is SG 34 when the preserved operations are: **(sub-SG label is 1) 1, 4, 5, 6.**

The transformation is:  $(\mathbf{a}_{34}, \mathbf{b}_{34}, \mathbf{c}_{34}) = (\mathbf{a}_{102}, \mathbf{b}_{102}, \mathbf{c}_{102}) \begin{pmatrix} 1 & 0 & 0 \\ 0 & 1 & 0 \\ 0 & 0 & 1 \end{pmatrix}, \overrightarrow{O_{102}O_{34}} = \frac{1}{2}\mathbf{b}_{34}$

The reduction of higher dimensional irrep:

$$C_{4v} : E \rightarrow B_1 + B_2 \text{ of } C_{2v}.$$

The correspondences of irreps at HSPs from original SG to lowered SG:

$$n_{GM5}^{34} = n_{GM6}^{102} + n_{GM7}^{102} n_{X3}^{34} = n_{X2}^{102} n_{X5}^{34} = n_{X4}^{102} n_{X2}^{34} = n_{X5}^{102} n_{X4}^{34} = n_{X3}^{102} n_{S5}^{34} = n_{M6}^{102} + n_{M7}^{102} n_{R5}^{34} = n_{A6}^{102} + n_{A7}^{102} n_{U3}^{34} = \\ n_{R4}^{102} n_{U5}^{34} = n_{R2}^{102} n_{U2}^{34} = n_{R3}^{102} n_{U4}^{34} = n_{R5}^{102} n_{Z5}^{34} = n_{Z6}^{102} + n_{Z7}^{102} n_{T5}^{34} = n_{R4}^{102} n_{T3}^{34} = n_{R2}^{102} n_{T4}^{34} = n_{R5}^{102} n_{T2}^{34} = n_{R3}^{102} n_{Y5}^{34} = n_{X4}^{102} \\ n_{Y3}^{34} = n_{X2}^{102} n_{Y4}^{34} = n_{X5}^{102} n_{Y2}^{34} = n_{X3}^{102}$$

The lower SG is SG 35 when the preserved operations are: **(sub-SG label is 2) 1, 4, 7, 8.**

The transformation is:  $(\mathbf{a}_{35}, \mathbf{b}_{35}, \mathbf{c}_{35}) = (\mathbf{a}_{102}, \mathbf{b}_{102}, \mathbf{c}_{102}) \begin{pmatrix} 1 & -1 & 0 \\ 1 & 1 & 0 \\ 0 & 0 & 1 \end{pmatrix}, \overrightarrow{O_{102}O_{35}} = \frac{1}{2}\mathbf{b}_{35}$

The reduction of higher dimensional irrep:

$$C_{4v} : E \rightarrow B_1 + B_2 \text{ of } C_{2v}.$$

The correspondences of irreps at HSPs from original SG to lowered SG:

$$n_{GM5}^{35} = n_{GM6}^{102} + n_{GM7}^{102} n_{Y5}^{35} = n_{M6}^{102} + n_{M7}^{102} n_{S4}^{35} = n_{X2}^{102} + n_{X4}^{102} n_{S3}^{35} = n_{X3}^{102} + n_{X5}^{102} n_{Z5}^{35} = n_{Z6}^{102} + n_{Z7}^{102} n_{T5}^{35} = n_{A6}^{102} + n_{A7}^{102} \\ n_{R4}^{35} = n_{R2}^{102} + n_{R4}^{102} n_{R3}^{35} = n_{R3}^{102} + n_{R5}^{102}$$

The lower SG is SG 77 when the preserved operations are: **(sub-SG label is 3) 1, 2, 3, 4.**

The transformation is:  $(\mathbf{a}_{77}, \mathbf{b}_{77}, \mathbf{c}_{77}) = (\mathbf{a}_{102}, \mathbf{b}_{102}, \mathbf{c}_{102}) \begin{pmatrix} -1 & 0 & 0 \\ 0 & 1 & 0 \\ 0 & 0 & -1 \end{pmatrix}, \overrightarrow{O_{102}O_{77}} = \mathbf{a}_{77} + \left(\frac{1}{2}\right)\mathbf{b}_{77}$

The reduction of higher dimensional irrep:

$$C_{4v} : E \rightarrow {}^2E + {}^1E \text{ of } C_4.$$

The correspondences of irreps at HSPs from original SG to lowered SG:

$$n_{GM5}^{77} = n_{GM6}^{102} n_{GM7}^{77} = n_{GM6}^{102} n_{GM8}^{77} = n_{GM7}^{102} n_{GM6}^{77} = n_{GM7}^{102} n_{X4}^{77} = n_{X3}^{102} + n_{X5}^{102} n_{X3}^{77} = n_{X2}^{102} + n_{X4}^{102} n_{M5}^{77} = n_{M6}^{102} n_{M7}^{77} = \\ n_{M7}^{102} n_{M8}^{77} = n_{M6}^{102} n_{M6}^{77} = n_{M7}^{102} n_{A5}^{77} = n_{A6}^{102} n_{A8}^{77} = n_{A7}^{102} n_{A7}^{77} = n_{A6}^{102} n_{A6}^{77} = n_{A7}^{102} n_{R4}^{77} = n_{R3}^{102} + n_{R5}^{102} n_{R3}^{77} = n_{R2}^{102} + n_{R4}^{102} \\ n_{Z6}^{77} = n_{Z6}^{102} n_{Z8}^{77} = n_{Z6}^{102} n_{Z7}^{77} = n_{Z7}^{102} n_{Z5}^{77} = n_{Z7}^{102}$$

#### 15. Lowered SGs by higher-dimensional irreps of pairings in SG 103

The representative operations of SG/T for SG 103:

$$1 : (x, y, z), 2 : (-y, x, z), 3 : (y, -x, z), 4 : (-x, -y, z), 5 : (-x, y, z + \frac{1}{2}), 6 : (x, -y, z + \frac{1}{2}), 7 : (-y, -x, z + \frac{1}{2}), \\ 8 : (y, x, z + \frac{1}{2}).$$

The lower SG is SG 27 when the preserved operations are: **(sub-SG label is 1) 1, 4, 5, 6.**

The transformation is:  $(\mathbf{a}_{27}, \mathbf{b}_{27}, \mathbf{c}_{27}) = (\mathbf{a}_{103}, \mathbf{b}_{103}, \mathbf{c}_{103}) \begin{pmatrix} 1 & 0 & 0 \\ 0 & 1 & 0 \\ 0 & 0 & 1 \end{pmatrix}, \overrightarrow{O_{103}O_{27}} = \frac{1}{2}\mathbf{a}_{27}$

The reduction of higher dimensional irrep:

$C_{4v} : E \rightarrow B_1 + B_2$  of  $C_{2v}$ .

The correspondences of irreps at HSPs from original SG to lowered SG:

$$\begin{aligned} n_{GM5}^{27} &= n_{GM6}^{103} + n_{GM7}^{103} n_{X5}^{27} = n_{X5}^{103} n_{S5}^{27} = n_{M6}^{103} + n_{M7}^{103} n_{R5}^{27} = n_{A6}^{103} + n_{A7}^{103} n_{U5}^{27} = n_{R5}^{103} n_{Z5}^{27} = n_{Z6}^{103} + n_{Z7}^{103} n_{T5}^{27} = n_{R5}^{103} \\ n_{Y5}^{27} &= n_{X5}^{103} \end{aligned}$$

The lower SG is SG 37 when the preserved operations are: **(sub-SG label is 2) 1, 4, 7, 8.**

$$\text{The transformation is: } (\mathbf{a}_{37}, \mathbf{b}_{37}, \mathbf{c}_{37}) = (\mathbf{a}_{103}, \mathbf{b}_{103}, \mathbf{c}_{103}) \begin{pmatrix} 1 & -1 & 0 \\ 1 & 1 & 0 \\ 0 & 0 & 1 \end{pmatrix}, \overrightarrow{O_{103}O_{37}} = \mathbf{0}$$

The reduction of higher dimensional irrep:

$C_{4v} : E \rightarrow B_1 + B_2$  of  $C_{2v}$ .

The correspondences of irreps at HSPs from original SG to lowered SG:

$$\begin{aligned} n_{GM5}^{37} &= n_{GM6}^{103} + n_{GM7}^{103} n_{Y5}^{37} = n_{M6}^{103} + n_{M7}^{103} n_{S4}^{37} = n_{X5}^{103} n_{S3}^{37} = n_{X5}^{103} n_{Z5}^{37} = n_{Z6}^{103} + n_{Z7}^{103} n_{T5}^{37} = n_{A6}^{103} + n_{A7}^{103} n_{R4}^{37} = n_{R5}^{103} \\ n_{R3}^{37} &= n_{R5}^{103} \end{aligned}$$

The lower SG is SG 75 when the preserved operations are: **(sub-SG label is 3) 1, 2, 3, 4.**

$$\text{The transformation is: } (\mathbf{a}_{75}, \mathbf{b}_{75}, \mathbf{c}_{75}) = (\mathbf{a}_{103}, \mathbf{b}_{103}, \mathbf{c}_{103}) \begin{pmatrix} -1 & 0 & 0 \\ 0 & -1 & 0 \\ 0 & 0 & 1 \end{pmatrix}, \overrightarrow{O_{103}O_{75}} = -\frac{1}{2}\mathbf{a}_{75} + \left(\frac{1}{2}\right)\mathbf{b}_{75}$$

The reduction of higher dimensional irrep:

$C_{4v} : E \rightarrow {}^2E + {}^1E$  of  $C_4$ .

The correspondences of irreps at HSPs from original SG to lowered SG:

$$\begin{aligned} n_{GM5}^{75} &= n_{GM6}^{103} n_{GM7}^{75} = n_{GM6}^{103} n_{GM8}^{75} = n_{GM7}^{103} n_{GM6}^{75} = n_{GM7}^{103} n_{X4}^{75} = n_{X5}^{103} n_{X3}^{75} = n_{X5}^{103} n_{M5}^{75} = n_{M7}^{103} n_{M7}^{75} = n_{M7}^{103} n_{M8}^{75} = \\ n_{M6}^{103} n_{M6}^{75} &= n_{M6}^{103} n_{A5}^{75} = n_{A7}^{103} n_{A7}^{75} = n_{A7}^{103} n_{A8}^{75} = n_{A6}^{103} n_{A6}^{75} = n_{A6}^{103} n_{R4}^{75} = n_{R5}^{103} n_{R3}^{75} = n_{R5}^{103} n_{Z5}^{75} = n_{Z6}^{103} n_{Z7}^{75} = n_{Z6}^{103} n_{Z8}^{75} = \\ n_{Z7}^{103} n_{Z6}^{75} &= n_{Z7}^{103} \end{aligned}$$

## 16. Lowered SGs by higher-dimensional irreps of pairings in SG 104

The representative operations of SG/T for SG 104:

$$1 : (x, y, z), 2 : (-y, x, z), 3 : (y, -x, z), 4 : (-x, -y, z), 5 : \left(\frac{1}{2} - x, y + \frac{1}{2}, z + \frac{1}{2}\right), 6 : \left(x + \frac{1}{2}, \frac{1}{2} - y, z + \frac{1}{2}\right), \\ 7 : \left(\frac{1}{2} - y, \frac{1}{2} - x, z + \frac{1}{2}\right), 8 : \left(y + \frac{1}{2}, x + \frac{1}{2}, z + \frac{1}{2}\right).$$

The lower SG is SG 34 when the preserved operations are: **(sub-SG label is 1) 1, 4, 5, 6.**

$$\text{The transformation is: } (\mathbf{a}_{34}, \mathbf{b}_{34}, \mathbf{c}_{34}) = (\mathbf{a}_{104}, \mathbf{b}_{104}, \mathbf{c}_{104}) \begin{pmatrix} 1 & 0 & 0 \\ 0 & 1 & 0 \\ 0 & 0 & 1 \end{pmatrix}, \overrightarrow{O_{104}O_{34}} = \frac{1}{2}\mathbf{a}_{34} + \left(\frac{1}{2}\right)\mathbf{b}_{34}$$

The reduction of higher dimensional irrep:

$C_{4v} : E \rightarrow B_1 + B_2$  of  $C_{2v}$ .

The correspondences of irreps at HSPs from original SG to lowered SG:

$$\begin{aligned} n_{GM5}^{34} &= n_{GM6}^{104} + n_{GM7}^{104} n_{X3}^{34} = n_{X2}^{104} n_{X5}^{34} = n_{X4}^{104} n_{X2}^{34} = n_{X5}^{104} n_{X4}^{34} = n_{X3}^{104} n_{S5}^{34} = n_{M6}^{104} + n_{M7}^{104} n_{R5}^{34} = n_{A6}^{104} + n_{A7}^{104} n_{U3}^{34} = \\ n_{R4}^{104} n_{U5}^{34} &= n_{R2}^{104} n_{U2}^{34} = n_{R3}^{104} n_{U4}^{34} = n_{R5}^{104} n_{Z5}^{34} = n_{Z6}^{104} + n_{Z7}^{104} n_{T5}^{34} = n_{R4}^{104} n_{T3}^{34} = n_{R2}^{104} n_{T4}^{34} = n_{R5}^{104} n_{T2}^{34} = n_{R3}^{104} n_{Y5}^{34} = n_{X4}^{104} \\ n_{Y3}^{34} &= n_{X2}^{104} n_{Y4}^{34} = n_{X5}^{104} n_{Y2}^{34} = n_{X3}^{104} \end{aligned}$$

The lower SG is SG 37 when the preserved operations are: **(sub-SG label is 2) 1, 4, 7, 8.**

$$\text{The transformation is: } (\mathbf{a}_{37}, \mathbf{b}_{37}, \mathbf{c}_{37}) = (\mathbf{a}_{104}, \mathbf{b}_{104}, \mathbf{c}_{104}) \begin{pmatrix} 1 & -1 & 0 \\ 1 & 1 & 0 \\ 0 & 0 & 1 \end{pmatrix}, \overrightarrow{O_{104}O_{37}} = \frac{1}{4}\mathbf{a}_{37} + \left(\frac{1}{4}\right)\mathbf{b}_{37}$$

The reduction of higher dimensional irrep:

$C_{4v} : E \rightarrow B_1 + B_2$  of  $C_{2v}$ .

The correspondences of irreps at HSPs from original SG to lowered SG:

$$\begin{aligned} n_{GM5}^{37} &= n_{GM6}^{104} + n_{GM7}^{104} n_{Y5}^{37} = n_{M6}^{104} + n_{M7}^{104} n_{S4}^{37} = n_{X2}^{104} + n_{X4}^{104} n_{S3}^{37} = n_{X3}^{104} + n_{X5}^{104} n_{Z5}^{37} = n_{Z6}^{104} + n_{Z7}^{104} n_{T5}^{37} = n_{A6}^{104} + n_{A7}^{104} \\ n_{R4}^{37} &= n_{R2}^{104} + n_{R4}^{104} n_{R3}^{37} = n_{R3}^{104} + n_{R5}^{104} \end{aligned}$$

The lower SG is SG 75 when the preserved operations are: **(sub-SG label is 3) 1, 2, 3, 4.**

$$\text{The transformation is: } (\mathbf{a}_{75}, \mathbf{b}_{75}, \mathbf{c}_{75}) = (\mathbf{a}_{104}, \mathbf{b}_{104}, \mathbf{c}_{104}) \begin{pmatrix} -1 & 0 & 0 \\ 0 & -1 & 0 \\ 0 & 0 & 1 \end{pmatrix}, \overrightarrow{O_{104}O_{75}} = -\frac{1}{2}\mathbf{a}_{75} + \left(\frac{1}{2}\right)\mathbf{b}_{75}$$

The reduction of higher dimensional irrep:

$$C_{4v} : E \rightarrow {}^2E + {}^1E \text{ of } C_4.$$

The correspondences of irreps at HSPs from original SG to lowered SG:

$$\begin{aligned} n_{GM5}^{75} &= n_{GM6}^{104} n_{GM7}^{75} = n_{GM6}^{104} n_{GM8}^{75} = n_{GM7}^{104} n_{GM6}^{75} = n_{GM7}^{104} n_{X4}^{75} = n_{X2}^{104} + n_{X4}^{104} n_{X3}^{75} = n_{X3}^{104} + n_{X5}^{104} n_{M5}^{75} = n_{M7}^{104} n_{M7}^{75} = \\ n_{M6}^{104} n_{M8}^{75} &= n_{M7}^{104} n_{M6}^{75} = n_{M6}^{104} n_{A5}^{75} = n_{A7}^{104} n_{A7}^{75} = n_{A6}^{104} n_{A8}^{75} = n_{A7}^{104} n_{A6}^{75} = n_{A6}^{104} n_{R4}^{75} = n_{R2}^{104} + n_{R4}^{104} n_{R3}^{75} = n_{R3}^{104} + n_{R5}^{104} \\ n_{Z5}^{75} &= n_{Z6}^{104} n_{Z7}^{75} = n_{Z6}^{104} n_{Z8}^{75} = n_{Z7}^{104} n_{Z6}^{75} = n_{Z7}^{104} \end{aligned}$$

### 17. Lowered SGs by higher-dimensional irreps of pairings in SG 105

The representative operations of SG/T for SG 105:

$$\begin{aligned} 1 : (x, y, z), 2 : (-y, x, z + \frac{1}{2}), 3 : (y, -x, z + \frac{1}{2}), 4 : (-x, -y, z), 5 : (-x, y, z), 6 : (x, -y, z), 7 : (-y, -x, z + \frac{1}{2}), \\ 8 : (y, x, z + \frac{1}{2}). \end{aligned}$$

The lower SG is SG 25 when the preserved operations are: **(sub-SG label is 1) 1, 4, 5, 6.**

$$\text{The transformation is: } (\mathbf{a}_{25}, \mathbf{b}_{25}, \mathbf{c}_{25}) = (\mathbf{a}_{105}, \mathbf{b}_{105}, \mathbf{c}_{105}) \begin{pmatrix} 1 & 0 & 0 \\ 0 & 1 & 0 \\ 0 & 0 & 1 \end{pmatrix}, \overrightarrow{O_{105}O_{25}} = \frac{1}{2}\mathbf{a}_{25}$$

The reduction of higher dimensional irrep:

$$C_{4v} : E \rightarrow B_1 + B_2 \text{ of } C_{2v}.$$

The correspondences of irreps at HSPs from original SG to lowered SG:

$$\begin{aligned} n_{GM5}^{25} &= n_{GM6}^{105} + n_{GM7}^{105} n_{X5}^{25} = n_{X5}^{105} n_{S5}^{25} = n_{M6}^{105} + n_{M7}^{105} n_{R5}^{25} = n_{A6}^{105} + n_{A7}^{105} n_{U5}^{25} = n_{R5}^{105} n_{Z5}^{25} = n_{Z6}^{105} + n_{Z7}^{105} n_{T5}^{25} = n_{R5}^{105} \\ n_{Y5}^{25} &= n_{X5}^{105} \end{aligned}$$

The lower SG is SG 37 when the preserved operations are: **(sub-SG label is 2) 1, 4, 7, 8.**

$$\text{The transformation is: } (\mathbf{a}_{37}, \mathbf{b}_{37}, \mathbf{c}_{37}) = (\mathbf{a}_{105}, \mathbf{b}_{105}, \mathbf{c}_{105}) \begin{pmatrix} 1 & -1 & 0 \\ 1 & 1 & 0 \\ 0 & 0 & 1 \end{pmatrix}, \overrightarrow{O_{105}O_{37}} = \mathbf{0}$$

The reduction of higher dimensional irrep:

$$C_{4v} : E \rightarrow B_1 + B_2 \text{ of } C_{2v}.$$

The correspondences of irreps at HSPs from original SG to lowered SG:

$$\begin{aligned} n_{GM5}^{37} &= n_{GM6}^{105} + n_{GM7}^{105} n_{Y5}^{37} = n_{M6}^{105} + n_{M7}^{105} n_{S4}^{37} = n_{X5}^{105} n_{S3}^{37} = n_{X5}^{105} n_{Z5}^{37} = n_{Z6}^{105} + n_{Z7}^{105} n_{T5}^{37} = n_{A6}^{105} + n_{A7}^{105} n_{R4}^{37} = n_{R5}^{105} \\ n_{R3}^{37} &= n_{R5}^{105} \end{aligned}$$

The lower SG is SG 77 when the preserved operations are: **(sub-SG label is 3) 1, 2, 3, 4.**

$$\text{The transformation is: } (\mathbf{a}_{77}, \mathbf{b}_{77}, \mathbf{c}_{77}) = (\mathbf{a}_{105}, \mathbf{b}_{105}, \mathbf{c}_{105}) \begin{pmatrix} -1 & 0 & 0 \\ 0 & 1 & 0 \\ 0 & 0 & -1 \end{pmatrix}, \overrightarrow{O_{105}O_{77}} = \frac{1}{2}\mathbf{a}_{77} + \left(\frac{1}{2}\right)\mathbf{b}_{77}$$

The reduction of higher dimensional irrep:

$$C_{4v} : E \rightarrow {}^2E + {}^1E \text{ of } C_4.$$

The correspondences of irreps at HSPs from original SG to lowered SG:

$$\begin{aligned} n_{GM5}^{77} &= n_{GM6}^{105} n_{GM7}^{77} = n_{GM6}^{105} n_{GM8}^{77} = n_{GM7}^{105} n_{GM6}^{77} = n_{GM7}^{105} n_{X4}^{77} = n_{X5}^{105} n_{X3}^{77} = n_{X5}^{105} n_{M5}^{77} = n_{M7}^{105} n_{M7}^{77} = n_{M7}^{105} n_{M8}^{77} = \\ n_{M6}^{105} n_{M6}^{77} &= n_{M6}^{105} n_{A5}^{77} = n_{A6}^{105} n_{A8}^{77} = n_{A6}^{105} n_{A7}^{77} = n_{A7}^{105} n_{A6}^{77} = n_{A7}^{105} n_{R4}^{77} = n_{R5}^{105} n_{R3}^{77} = n_{R5}^{105} n_{Z6}^{77} = n_{Z6}^{105} n_{Z8}^{77} = n_{Z6}^{105} n_{Z7}^{77} = \\ n_{Z7}^{105} n_{Z5}^{77} &= n_{Z7}^{105} \end{aligned}$$

### 18. Lowered SGs by higher-dimensional irreps of pairings in SG 106

The representative operations of SG/T for SG 106:

$$1 : (x, y, z), 2 : (-y, x, z + \frac{1}{2}), 3 : (y, -x, z + \frac{1}{2}), 4 : (-x, -y, z), 5 : (\frac{1}{2} - x, y + \frac{1}{2}, z), 6 : (x + \frac{1}{2}, \frac{1}{2} - y, z), \\ 7 : (\frac{1}{2} - y, \frac{1}{2} - x, z + \frac{1}{2}), 8 : (y + \frac{1}{2}, x + \frac{1}{2}, z + \frac{1}{2}).$$

The lower SG is SG 32 when the preserved operations are: **(sub-SG label is 1) 1, 4, 5, 6.**

The transformation is:  $(\mathbf{a}_{32}, \mathbf{b}_{32}, \mathbf{c}_{32}) = (\mathbf{a}_{106}, \mathbf{b}_{106}, \mathbf{c}_{106}) \begin{pmatrix} 1 & 0 & 0 \\ 0 & 1 & 0 \\ 0 & 0 & 1 \end{pmatrix}, \overrightarrow{O_{106}O_{32}} = \frac{1}{2}\mathbf{a}_{32} + (\frac{1}{2})\mathbf{b}_{32}$

The reduction of higher dimensional irrep:

$$C_{4v} : E \rightarrow B_1 + B_2 \text{ of } C_{2v}.$$

The correspondences of irreps at HSPs from original SG to lowered SG:

$$n_{GM5}^{32} = n_{GM6}^{106} + n_{GM7}^{106} \quad n_{X3}^{32} = n_{X2}^{106} \quad n_{X5}^{32} = n_{X4}^{106} \quad n_{X2}^{32} = n_{X4}^{106} \quad n_{X4}^{32} = n_{X5}^{106} \quad n_{X3}^{32} = n_{X5}^{106} \quad n_{S5}^{32} = n_{M6}^{106} + n_{M7}^{106} \quad n_{R5}^{32} = n_{A6}^{106} + n_{A7}^{106} \quad n_{U3}^{32} = \\ n_{R2}^{106} \quad n_{U5}^{32} = n_{R4}^{106} \quad n_{U2}^{32} = n_{R5}^{106} \quad n_{U4}^{32} = n_{R3}^{106} \quad n_{Z5}^{32} = n_{Z6}^{106} + n_{Z7}^{106} \quad n_{T5}^{32} = n_{R4}^{106} \quad n_{T3}^{32} = n_{R2}^{106} \quad n_{T4}^{32} = n_{R5}^{106} \quad n_{T2}^{32} = n_{R3}^{106} \quad n_{Y5}^{32} = n_{X4}^{106} \\ n_{Y3}^{32} = n_{X2}^{106} \quad n_{Y4}^{32} = n_{X5}^{106} \quad n_{Y2}^{32} = n_{X3}^{106}$$

The lower SG is SG 37 when the preserved operations are: **(sub-SG label is 2) 1, 4, 7, 8.**

The transformation is:  $(\mathbf{a}_{37}, \mathbf{b}_{37}, \mathbf{c}_{37}) = (\mathbf{a}_{106}, \mathbf{b}_{106}, \mathbf{c}_{106}) \begin{pmatrix} 1 & -1 & 0 \\ 1 & 1 & 0 \\ 0 & 0 & 1 \end{pmatrix}, \overrightarrow{O_{106}O_{37}} = \frac{1}{4}\mathbf{a}_{37} + (\frac{1}{4})\mathbf{b}_{37}$

The reduction of higher dimensional irrep:

$$C_{4v} : E \rightarrow B_1 + B_2 \text{ of } C_{2v}.$$

The correspondences of irreps at HSPs from original SG to lowered SG:

$$n_{GM5}^{37} = n_{GM6}^{106} + n_{GM7}^{106} \quad n_{Y5}^{37} = n_{M6}^{106} + n_{M7}^{106} \quad n_{S4}^{37} = n_{X2}^{106} + n_{X4}^{106} \quad n_{S3}^{37} = n_{X3}^{106} + n_{X5}^{106} \quad n_{Z5}^{37} = n_{Z6}^{106} + n_{Z7}^{106} \quad n_{T5}^{37} = n_{A6}^{106} + n_{A7}^{106} \\ n_{R4}^{37} = n_{R2}^{106} + n_{R4}^{106} \quad n_{R3}^{37} = n_{R3}^{106} + n_{R5}^{106}$$

The lower SG is SG 77 when the preserved operations are: **(sub-SG label is 3) 1, 2, 3, 4.**

The transformation is:  $(\mathbf{a}_{77}, \mathbf{b}_{77}, \mathbf{c}_{77}) = (\mathbf{a}_{106}, \mathbf{b}_{106}, \mathbf{c}_{106}) \begin{pmatrix} -1 & 0 & 0 \\ 0 & 1 & 0 \\ 0 & 0 & -1 \end{pmatrix}, \overrightarrow{O_{106}O_{77}} = \frac{1}{2}\mathbf{a}_{77} + (\frac{1}{2})\mathbf{b}_{77}$

The reduction of higher dimensional irrep:

$$C_{4v} : E \rightarrow {}^2E + {}^1E \text{ of } C_4.$$

The correspondences of irreps at HSPs from original SG to lowered SG:

$$n_{GM5}^{77} = n_{GM6}^{106} \quad n_{GM7}^{77} = n_{GM6}^{106} \quad n_{GM8}^{77} = n_{GM7}^{106} \quad n_{GM6}^{77} = n_{GM7}^{106} \quad n_{X4}^{77} = n_{X3}^{106} + n_{X5}^{106} \quad n_{X3}^{77} = n_{X2}^{106} + n_{X4}^{106} \quad n_{M5}^{77} = n_{M6}^{106} \quad n_{M7}^{77} = \\ n_{M7}^{106} \quad n_{M8}^{77} = n_{M6}^{106} \quad n_{M6}^{77} = n_{M7}^{106} \quad n_{A5}^{77} = n_{A7}^{106} \quad n_{A8}^{77} = n_{A6}^{106} \quad n_{A7}^{77} = n_{A7}^{106} \quad n_{A6}^{77} = n_{A6}^{106} \quad n_{R4}^{77} = n_{R3}^{106} + n_{R5}^{106} \quad n_{R3}^{77} = n_{R2}^{106} + n_{R4}^{106} \\ n_{Z6}^{77} = n_{Z6}^{106} \quad n_{Z8}^{77} = n_{Z6}^{106} \quad n_{Z7}^{77} = n_{Z7}^{106} \quad n_{Z5}^{77} = n_{Z7}^{106}$$

### 19. Lowered SGs by higher-dimensional irreps of pairings in SG 107

The representative operations of SG/T for SG 107:

$$1 : (x, y, z), 2 : (-y, x, z), 3 : (y, -x, z), 4 : (-x, -y, z), 5 : (-x, y, z), 6 : (x, -y, z), 7 : (-y, -x, z), 8 : (y, x, z).$$

The lower SG is SG 44 when the preserved operations are: **(sub-SG label is 1) 1, 4, 5, 6.**

The transformation is:  $(\mathbf{a}_{44}, \mathbf{b}_{44}, \mathbf{c}_{44}) = (\mathbf{a}_{107}, \mathbf{b}_{107}, \mathbf{c}_{107}) \begin{pmatrix} 1 & 0 & 0 \\ 0 & 1 & 0 \\ 0 & 0 & 1 \end{pmatrix}, \overrightarrow{O_{107}O_{44}} = -\frac{1}{2}\mathbf{b}_{44}$

The reduction of higher dimensional irrep:

$C_{4v} : E \rightarrow B_1 + B_2$  of  $C_{2v}$ .

The correspondences of irreps at HSPs from original SG to lowered SG:

$$\begin{aligned} n_{GM5}^{44} &= n_{GM6}^{107} + n_{GM7}^{107} n_{X5}^{44} = n_{M6}^{107} + n_{M7}^{107} n_{T4}^{44} = n_{X5}^{107} n_{T3}^{44} = n_{X5}^{107} n_{W4}^{44} = n_{P5}^{107} n_{W3}^{44} = n_{P5}^{107} n_{R4}^{44} = n_{N4}^{107} n_{R3}^{44} = n_{N3}^{107} \\ n_{S3}^{44} &= n_{N4}^{107} n_{S4}^{44} = n_{N3}^{107} \end{aligned}$$

The lower SG is SG 42 when the preserved operations are: **(sub-SG label is 2) 1, 4, 7, 8.**

The transformation is:  $(\mathbf{a}_{42}, \mathbf{b}_{42}, \mathbf{c}_{42}) = (\mathbf{a}_{107}, \mathbf{b}_{107}, \mathbf{c}_{107}) \begin{pmatrix} 1 & -1 & 0 \\ 1 & 1 & 0 \\ 0 & 0 & 1 \end{pmatrix}, \overrightarrow{O_{107}O_{42}} = \mathbf{0}$

The reduction of higher dimensional irrep:

$C_{4v} : E \rightarrow B_1 + B_2$  of  $C_{2v}$ .

The correspondences of irreps at HSPs from original SG to lowered SG:

$$n_{GM5}^{42} = n_{GM6}^{107} + n_{GM7}^{107} n_{Y5}^{42} = n_{X5}^{107} n_{L2}^{42} = n_{N3}^{107} + n_{N4}^{107} n_{Z5}^{42} = n_{M6}^{107} + n_{M7}^{107} n_{T5}^{42} = n_{X5}^{107}$$

The lower SG is SG 79 when the preserved operations are: **(sub-SG label is 3) 1, 2, 3, 4.**

The transformation is:  $(\mathbf{a}_{79}, \mathbf{b}_{79}, \mathbf{c}_{79}) = (\mathbf{a}_{107}, \mathbf{b}_{107}, \mathbf{c}_{107}) \begin{pmatrix} 0 & 1 & 0 \\ -1 & 0 & 0 \\ 0 & 0 & 1 \end{pmatrix}, \overrightarrow{O_{107}O_{79}} = \frac{1}{2}\mathbf{a}_{79} + (\frac{1}{2})\mathbf{b}_{79}$

The reduction of higher dimensional irrep:

$C_{4v} : E \rightarrow {}^2E + {}^1E$  of  $C_4$ .

The correspondences of irreps at HSPs from original SG to lowered SG:

$$\begin{aligned} n_{GM5}^{79} &= n_{GM6}^{107} n_{GM7}^{79} = n_{GM6}^{107} n_{GM8}^{79} = n_{GM7}^{107} n_{GM6}^{79} = n_{GM7}^{107} n_{M5}^{79} = n_{M6}^{107} n_{M7}^{79} = n_{M6}^{107} n_{M8}^{79} = n_{M7}^{107} n_{M6}^{79} = n_{M7}^{107} n_{X4}^{79} = \\ n_{X5}^{107} n_{X3}^{79} &= n_{X5}^{107} n_{P4}^{79} = n_{P5}^{107} n_{P3}^{79} = n_{P5}^{107} n_{N2}^{79} = n_{N3}^{107} + n_{N4}^{107} \end{aligned}$$

## 20. Lowered SGs by higher-dimensional irreps of pairings in SG 108

The representative operations of SG/T for SG 108:

$$1 : (x, y, z), 2 : (-y, x, z), 3 : (y, -x, z), 4 : (-x, -y, z), 5 : (-x, y, z + \frac{1}{2}), 6 : (x, -y, z + \frac{1}{2}), 7 : (-y, -x, z + \frac{1}{2}), 8 : (y, x, z + \frac{1}{2}).$$

The lower SG is SG 45 when the preserved operations are: **(sub-SG label is 1) 1, 4, 5, 6.**

The transformation is:  $(\mathbf{a}_{45}, \mathbf{b}_{45}, \mathbf{c}_{45}) = (\mathbf{a}_{108}, \mathbf{b}_{108}, \mathbf{c}_{108}) \begin{pmatrix} 1 & 0 & 0 \\ 0 & 1 & 0 \\ 0 & 0 & 1 \end{pmatrix}, \overrightarrow{O_{108}O_{45}} = -\frac{1}{2}\mathbf{b}_{45}$

The reduction of higher dimensional irrep:

$C_{4v} : E \rightarrow B_1 + B_2$  of  $C_{2v}$ .

The correspondences of irreps at HSPs from original SG to lowered SG:

$$\begin{aligned} n_{GM5}^{45} &= n_{GM6}^{108} + n_{GM7}^{108} n_{X5}^{45} = n_{M6}^{108} + n_{M7}^{108} n_{T4}^{45} = n_{X5}^{108} n_{T3}^{45} = n_{X5}^{108} n_{W4}^{45} = n_{P5}^{108} n_{W3}^{45} = n_{P5}^{108} n_{R4}^{45} = n_{N4}^{108} n_{R3}^{45} = n_{N3}^{108} \\ n_{S4}^{45} &= n_{N3}^{108} n_{S3}^{45} = n_{N4}^{108} \end{aligned}$$

The lower SG is SG 42 when the preserved operations are: **(sub-SG label is 2) 1, 4, 7, 8.**

The transformation is:  $(\mathbf{a}_{42}, \mathbf{b}_{42}, \mathbf{c}_{42}) = (\mathbf{a}_{108}, \mathbf{b}_{108}, \mathbf{c}_{108}) \begin{pmatrix} 1 & -1 & 0 \\ 1 & 1 & 0 \\ 0 & 0 & 1 \end{pmatrix}, \overrightarrow{O_{108}O_{42}} = \frac{1}{4}\mathbf{a}_{42} + (-\frac{1}{4})\mathbf{b}_{42}$

The reduction of higher dimensional irrep:

$C_{4v} : E \rightarrow B_1 + B_2$  of  $C_{2v}$ .

The correspondences of irreps at HSPs from original SG to lowered SG:

$$n_{GM5}^{42} = n_{GM6}^{108} + n_{GM7}^{108} n_{Y5}^{42} = n_{X5}^{108} n_{L2}^{42} = n_{N3}^{108} + n_{N4}^{108} n_{Z5}^{42} = n_{M6}^{108} + n_{M7}^{108} n_{T5}^{42} = n_{X5}^{108}$$

The lower SG is SG 79 when the preserved operations are: **(sub-SG label is 3) 1, 2, 3, 4.**

The transformation is:  $(\mathbf{a}_{79}, \mathbf{b}_{79}, \mathbf{c}_{79}) = (\mathbf{a}_{108}, \mathbf{b}_{108}, \mathbf{c}_{108}) \begin{pmatrix} 0 & 1 & 0 \\ -1 & 0 & 0 \\ 0 & 0 & 1 \end{pmatrix}, \overrightarrow{O_{108}O_{79}} = \frac{1}{2}\mathbf{a}_{79} + (\frac{1}{2})\mathbf{b}_{79}$

The reduction of higher dimensional irrep:

$C_{4v} : E \rightarrow {}^2E + {}^1E$  of  $C_4$ .

The correspondences of irreps at HSPs from original SG to lowered SG:

$$\begin{aligned} n_{GM5}^{79} &= n_{GM6}^{108} n_{GM7}^{79} = n_{GM6}^{108} n_{GM8}^{79} = n_{GM7}^{108} n_{GM6}^{79} = n_{GM7}^{108} n_{M5}^{79} = n_{M6}^{108} n_{M7}^{79} = n_{M6}^{108} n_{M8}^{79} = n_{M7}^{108} n_{M6}^{79} = n_{M7}^{108} n_{X4}^{79} = \\ n_{X5}^{108} n_{X3}^{79} &= n_{X5}^{108} n_{P4}^{79} = n_{P5}^{108} n_{P3}^{79} = n_{P5}^{108} n_{N2}^{79} = n_{N3}^{108} + n_{N4}^{108} \end{aligned}$$

## 21. Lowered SGs by higher-dimensional irreps of pairings in SG 109

The representative operations of SG/T for SG 109:

$$\begin{aligned} 1 : (x, y, z), 2 : (-y, x + \frac{1}{2}, z + \frac{1}{4}), 3 : (y, \frac{1}{2} - x, z + \frac{1}{4}), 4 : (-x, -y, z), 5 : (-x, y, z), 6 : (x, -y, z), 7 : \\ (-y, \frac{1}{2} - x, z + \frac{1}{4}), 8 : (y, x + \frac{1}{2}, z + \frac{1}{4}). \end{aligned}$$

The lower SG is SG 44 when the preserved operations are: **(sub-SG label is 1) 1, 4, 5, 6.**

The transformation is:  $(\mathbf{a}_{44}, \mathbf{b}_{44}, \mathbf{c}_{44}) = (\mathbf{a}_{109}, \mathbf{b}_{109}, \mathbf{c}_{109}) \begin{pmatrix} 1 & 0 & 0 \\ 0 & 1 & 0 \\ 0 & 0 & 1 \end{pmatrix}, \overrightarrow{O_{109}O_{44}} = -\frac{1}{2}\mathbf{b}_{44}$

The reduction of higher dimensional irrep:

$C_{4v} : E \rightarrow B_1 + B_2$  of  $C_{2v}$ .

The correspondences of irreps at HSPs from original SG to lowered SG:

$$\begin{aligned} n_{GM5}^{44} &= n_{GM6}^{109} + n_{GM7}^{109} n_{X5}^{44} = n_{M6}^{109} + n_{M7}^{109} n_{T4}^{44} = n_{X2}^{109} + n_{X4}^{109} n_{T3}^{44} = n_{X3}^{109} + n_{X5}^{109} n_{W4}^{44} = n_{P2}^{109} + n_{P4}^{109} n_{W3}^{44} = n_{P3}^{109} + n_{P5}^{109} \\ n_{R4}^{44} &= n_{N4}^{109} n_{R3}^{44} = n_{N3}^{109} n_{S3}^{44} = n_{N4}^{109} n_{S4}^{44} = n_{N3}^{109} \end{aligned}$$

The lower SG is SG 43 when the preserved operations are: **(sub-SG label is 2) 1, 4, 7, 8.**

The transformation is:  $(\mathbf{a}_{43}, \mathbf{b}_{43}, \mathbf{c}_{43}) = (\mathbf{a}_{109}, \mathbf{b}_{109}, \mathbf{c}_{109}) \begin{pmatrix} -1 & -1 & 0 \\ 1 & -1 & 0 \\ 0 & 0 & 1 \end{pmatrix}, \overrightarrow{O_{109}O_{43}} = \frac{1}{4}\mathbf{a}_{43} + (-\frac{1}{4})\mathbf{b}_{43}$

The reduction of higher dimensional irrep:

$C_{4v} : E \rightarrow B_1 + B_2$  of  $C_{2v}$ .

The correspondences of irreps at HSPs from original SG to lowered SG:

$$\begin{aligned} n_{GM5}^{43} &= n_{GM6}^{109} + n_{GM7}^{109} n_{X5}^{43} = n_{X2}^{109} n_{Y3}^{43} = n_{X4}^{109} n_{Y4}^{43} = n_{X3}^{109} n_{Y2}^{43} = n_{X5}^{109} n_{L2}^{43} = n_{N3}^{109} + n_{N4}^{109} n_{Z5}^{43} = n_{M6}^{109} + n_{M7}^{109} n_{T5}^{43} = \\ n_{X3}^{109} n_{T3}^{43} &= n_{X5}^{109} n_{T4}^{43} = n_{X4}^{109} n_{T2}^{43} = n_{X2}^{109} \end{aligned}$$

The lower SG is SG 80 when the preserved operations are: **(sub-SG label is 3) 1, 2, 3, 4.**

The transformation is:  $(\mathbf{a}_{80}, \mathbf{b}_{80}, \mathbf{c}_{80}) = (\mathbf{a}_{109}, \mathbf{b}_{109}, \mathbf{c}_{109}) \begin{pmatrix} 0 & 1 & 0 \\ -1 & 0 & 0 \\ 0 & 0 & 1 \end{pmatrix}, \overrightarrow{O_{109}O_{80}} = \frac{1}{2}\mathbf{a}_{80}$

The reduction of higher dimensional irrep:

$C_{4v} : E \rightarrow {}^2E + {}^1E$  of  $C_4$ .

The correspondences of irreps at HSPs from original SG to lowered SG:

$$\begin{aligned} n_{GM5}^{80} &= n_{GM6}^{109} n_{GM7}^{80} = n_{GM6}^{109} n_{GM8}^{80} = n_{GM7}^{109} n_{GM6}^{80} = n_{GM7}^{109} n_{M7}^{80} = n_{M7}^{109} n_{M5}^{80} = n_{M6}^{109} n_{M6}^{80} = n_{M7}^{109} n_{M8}^{80} = n_{M6}^{109} n_{X4}^{80} = \\ n_{X3}^{109} + n_{X5}^{109} n_{X3}^{80} &= n_{X2}^{109} + n_{X4}^{109} n_{P4}^{80} = n_{P3}^{109} + n_{P5}^{109} n_{P3}^{80} = n_{P2}^{109} + n_{P4}^{109} n_{N2}^{80} = n_{N3}^{109} + n_{N4}^{109} \end{aligned}$$

## 22. Lowered SGs by higher-dimensional irreps of pairings in SG 110

The representative operations of SG/T for SG 110:

$$1 : (x, y, z), 2 : (-y, x + \frac{1}{2}, z + \frac{1}{4}), 3 : (y, \frac{1}{2} - x, z + \frac{1}{4}), 4 : (-x, -y, z), 5 : (-x, y, z + \frac{1}{2}), 6 : (x, -y, z + \frac{1}{2}), \\ 7 : (\frac{1}{2} - y, -x, z + \frac{1}{4}), 8 : (y + \frac{1}{2}, x, z + \frac{1}{4}).$$

The lower SG is SG 45 when the preserved operations are: **(sub-SG label is 1) 1, 4, 5, 6.**

$$\text{The transformation is: } (\mathbf{a}_{45}, \mathbf{b}_{45}, \mathbf{c}_{45}) = (\mathbf{a}_{110}, \mathbf{b}_{110}, \mathbf{c}_{110}) \begin{pmatrix} 1 & 0 & 0 \\ 0 & 1 & 0 \\ 0 & 0 & 1 \end{pmatrix}, \overrightarrow{O_{110}O_{45}} = -\frac{1}{2}\mathbf{b}_{45}$$

The reduction of higher dimensional irrep:

$$C_{4v} : E \rightarrow B_1 + B_2 \text{ of } C_{2v}.$$

The correspondences of irreps at HSPs from original SG to lowered SG:

$$n_{GM5}^{45} = n_{GM6}^{110} + n_{GM7}^{110} \quad n_{X5}^{45} = n_{M6}^{110} + n_{M7}^{110} \quad n_{T4}^{45} = n_{X2}^{110} + n_{X4}^{110} \quad n_{T3}^{45} = n_{X3}^{110} + n_{X5}^{110} \quad n_{W4}^{45} = n_{P2}^{110} + n_{P4}^{110} \quad n_{W3}^{45} = n_{P3}^{110} + n_{P5}^{110} \\ n_{R4}^{45} = n_{N4}^{110} \quad n_{R3}^{45} = n_{N3}^{110} \quad n_{S4}^{45} = n_{N3}^{110} \quad n_{S3}^{45} = n_{N4}^{110}$$

The lower SG is SG 43 when the preserved operations are: **(sub-SG label is 2) 1, 4, 7, 8.**

$$\text{The transformation is: } (\mathbf{a}_{43}, \mathbf{b}_{43}, \mathbf{c}_{43}) = (\mathbf{a}_{110}, \mathbf{b}_{110}, \mathbf{c}_{110}) \begin{pmatrix} 1 & -1 & 0 \\ 1 & 1 & 0 \\ 0 & 0 & 1 \end{pmatrix}, \overrightarrow{O_{110}O_{43}} = \frac{1}{4}\mathbf{a}_{43} + (-\frac{1}{4})\mathbf{b}_{43}$$

The reduction of higher dimensional irrep:

$$C_{4v} : E \rightarrow B_1 + B_2 \text{ of } C_{2v}.$$

The correspondences of irreps at HSPs from original SG to lowered SG:

$$n_{GM5}^{43} = n_{GM6}^{110} + n_{GM7}^{110} \quad n_{Y5}^{43} = n_{X3}^{110} \quad n_{Y3}^{43} = n_{X5}^{110} \quad n_{Y4}^{43} = n_{X2}^{110} \quad n_{Y2}^{43} = n_{X4}^{110} \quad n_{L2}^{43} = n_{N3}^{110} + n_{N4}^{110} \quad n_{Z5}^{43} = n_{M6}^{110} + n_{M7}^{110} \quad n_{T5}^{43} = n_{X2}^{110} \quad n_{T3}^{43} = n_{X4}^{110} \quad n_{T4}^{43} = n_{X5}^{110} \quad n_{T2}^{43} = n_{X3}^{110}$$

The lower SG is SG 80 when the preserved operations are: **(sub-SG label is 3) 1, 2, 3, 4.**

$$\text{The transformation is: } (\mathbf{a}_{80}, \mathbf{b}_{80}, \mathbf{c}_{80}) = (\mathbf{a}_{110}, \mathbf{b}_{110}, \mathbf{c}_{110}) \begin{pmatrix} 0 & 1 & 0 \\ -1 & 0 & 0 \\ 0 & 0 & 1 \end{pmatrix}, \overrightarrow{O_{110}O_{80}} = \frac{1}{2}\mathbf{a}_{80}$$

The reduction of higher dimensional irrep:

$$C_{4v} : E \rightarrow {}^2E + {}^1E \text{ of } C_4.$$

The correspondences of irreps at HSPs from original SG to lowered SG:

$$n_{GM5}^{80} = n_{GM6}^{110} \quad n_{GM7}^{80} = n_{GM6}^{110} \quad n_{GM8}^{80} = n_{GM7}^{110} \quad n_{GM6}^{80} = n_{GM7}^{110} \quad n_{M7}^{80} = n_{M7}^{110} \quad n_{M5}^{80} = n_{M6}^{110} \quad n_{M6}^{80} = n_{M7}^{110} \quad n_{M8}^{80} = n_{M6}^{110} \quad n_{X4}^{80} = n_{X3}^{110} + n_{X5}^{110} \quad n_{X3}^{80} = n_{X2}^{110} + n_{X4}^{110} \quad n_{P4}^{80} = n_{P3}^{110} + n_{P5}^{110} \quad n_{P3}^{80} = n_{P2}^{110} + n_{P4}^{110} \quad n_{N2}^{80} = n_{N3}^{110} + n_{N4}^{110}$$

### 23. Lowered SGs by higher-dimensional irreps of pairings in SG 111

The representative operations of SG/T for SG 111:

$$1 : (x, y, z), 2 : (x, -y, -z), 3 : (-x, y, -z), 4 : (-x, -y, z), 5 : (y, -x, -z), 6 : (-y, x, -z), 7 : (-y, -x, z), \\ 8 : (y, x, z).$$

The lower SG is SG 16 when the preserved operations are: **(sub-SG label is 1) 1, 2, 3, 4.**

$$\text{The transformation is: } (\mathbf{a}_{16}, \mathbf{b}_{16}, \mathbf{c}_{16}) = (\mathbf{a}_{111}, \mathbf{b}_{111}, \mathbf{c}_{111}) \begin{pmatrix} 0 & 0 & 1 \\ 1 & 0 & 0 \\ 0 & 1 & 0 \end{pmatrix}, \overrightarrow{O_{111}O_{16}} = \frac{1}{2}\mathbf{a}_{16} + (\frac{1}{2})\mathbf{c}_{16}$$

The reduction of higher dimensional irrep:

$$D_{2d} : E \rightarrow B_1 + B_3 \text{ of } D_2.$$

The correspondences of irreps at HSPs from original SG to lowered SG:

$$n_{GM5}^{16} = n_{GM6}^{111} + n_{GM7}^{111} \quad n_{X5}^{16} = n_{X5}^{111} \quad n_{S5}^{16} = n_{R5}^{111} \quad n_{R5}^{16} = n_{A6}^{111} + n_{A7}^{111} \quad n_{U5}^{16} = n_{M6}^{111} + n_{M7}^{111} \quad n_{Z5}^{16} = n_{X5}^{111} \quad n_{T5}^{16} = n_{R5}^{111} \quad n_{Y5}^{16} = n_{Z6}^{111} + n_{Z7}^{111}$$

The lower SG is SG 35 when the preserved operations are: **(sub-SG label is 2) 1, 4, 7, 8.**

The transformation is:  $(\mathbf{a}_{35}, \mathbf{b}_{35}, \mathbf{c}_{35}) = (\mathbf{a}_{111}, \mathbf{b}_{111}, \mathbf{c}_{111}) \begin{pmatrix} 1 & -1 & 0 \\ 1 & 1 & 0 \\ 0 & 0 & 1 \end{pmatrix}, \overrightarrow{O_{111}O_{35}} = \mathbf{0}$

The reduction of higher dimensional irrep:

$D_{2d} : E \rightarrow B_1 + B_2$  of  $C_{2v}$ .

The correspondences of irreps at HSPs from original SG to lowered SG:

$$n_{GM5}^{35} = n_{GM6}^{111} + n_{GM7}^{111} n_{Y5}^{35} = n_{M6}^{111} + n_{M7}^{111} n_{S4}^{35} = n_{X5}^{111} n_{S3}^{35} = n_{X5}^{111} n_{Z5}^{35} = n_{Z6}^{111} + n_{Z7}^{111} n_{T5}^{35} = n_{A6}^{111} + n_{A7}^{111} n_{R4}^{35} = n_{R5}^{111}$$

$$n_{R3}^{35} = n_{R5}^{111}$$

The lower SG is SG 81 when the preserved operations are: **(sub-SG label is 3) 1, 5, 6, 4.**

The transformation is:  $(\mathbf{a}_{81}, \mathbf{b}_{81}, \mathbf{c}_{81}) = (\mathbf{a}_{111}, \mathbf{b}_{111}, \mathbf{c}_{111}) \begin{pmatrix} -1 & 0 & 0 \\ 0 & -1 & 0 \\ 0 & 0 & 1 \end{pmatrix}, \overrightarrow{O_{111}O_{81}} = \frac{1}{2}\mathbf{a}_{81} + (\frac{1}{2})\mathbf{b}_{81} + (\frac{1}{2})\mathbf{c}_{81}$

The reduction of higher dimensional irrep:

$D_{2d} : E \rightarrow {}^2E + {}^1E$  of  $S_4$ .

The correspondences of irreps at HSPs from original SG to lowered SG:

$$n_{GM7}^{81} = n_{GM6}^{111} n_{GM8}^{81} = n_{GM7}^{111} n_{GM5}^{81} = n_{GM6}^{111} n_{GM6}^{81} = n_{GM7}^{111} n_{X4}^{81} = n_{X5}^{111} n_{X3}^{81} = n_{X5}^{111} n_{M7}^{81} = n_{M7}^{111} n_{M8}^{81} = n_{M6}^{111} n_{M5}^{81} =$$

$$n_{M7}^{111} n_{M6}^{81} = n_{M6}^{111} n_{A7}^{81} = n_{A6}^{111} n_{A8}^{81} = n_{A7}^{111} n_{A5}^{81} = n_{A6}^{111} n_{A6}^{81} = n_{A7}^{111} n_{R4}^{81} = n_{R5}^{111} n_{R3}^{81} = n_{R5}^{111} n_{Z7}^{81} = n_{Z7}^{111} n_{Z8}^{81} = n_{Z6}^{111} n_{Z5}^{81} =$$

$$n_{Z7}^{111} n_{Z6}^{81} = n_{Z6}^{111}$$

#### 24. Lowered SGs by higher-dimensional irreps of pairings in SG 112

The representative operations of SG/T for SG 112:

$$1 : (x, y, z), 2 : (x, -y, \frac{1}{2} - z), 3 : (-x, y, \frac{1}{2} - z), 4 : (-x, -y, z), 5 : (y, -x, -z), 6 : (-y, x, -z), 7 : (-y, -x, z + \frac{1}{2}),$$

$$8 : (y, x, z + \frac{1}{2}).$$

The lower SG is SG 16 when the preserved operations are: **(sub-SG label is 1) 1, 2, 3, 4.**

The transformation is:  $(\mathbf{a}_{16}, \mathbf{b}_{16}, \mathbf{c}_{16}) = (\mathbf{a}_{112}, \mathbf{b}_{112}, \mathbf{c}_{112}) \begin{pmatrix} 0 & 0 & 1 \\ 1 & 0 & 0 \\ 0 & 1 & 0 \end{pmatrix}, \overrightarrow{O_{112}O_{16}} = \frac{1}{2}\mathbf{a}_{16} + (\frac{1}{4})\mathbf{b}_{16} + (\frac{1}{2})\mathbf{c}_{16}$

The reduction of higher dimensional irrep:

$D_{2d} : E \rightarrow B_1 + B_3$  of  $D_2$ .

The correspondences of irreps at HSPs from original SG to lowered SG:

$$n_{GM5}^{16} = n_{GM6}^{112} + n_{GM7}^{112} n_{X5}^{16} = n_{X5}^{112} n_{S5}^{16} = n_{R5}^{112} n_{R5}^{16} = n_{A6}^{112} + n_{A7}^{112} n_{U5}^{16} = n_{M6}^{112} + n_{M7}^{112} n_{Z5}^{16} = n_{X5}^{112} n_{T5}^{16} = n_{R5}^{112} n_{Y5}^{16} =$$

$$n_{Z6}^{112} + n_{Z7}^{112}$$

The lower SG is SG 37 when the preserved operations are: **(sub-SG label is 2) 1, 4, 7, 8.**

The transformation is:  $(\mathbf{a}_{37}, \mathbf{b}_{37}, \mathbf{c}_{37}) = (\mathbf{a}_{112}, \mathbf{b}_{112}, \mathbf{c}_{112}) \begin{pmatrix} 1 & -1 & 0 \\ 1 & 1 & 0 \\ 0 & 0 & 1 \end{pmatrix}, \overrightarrow{O_{112}O_{37}} = \mathbf{0}$

The reduction of higher dimensional irrep:

$D_{2d} : E \rightarrow B_1 + B_2$  of  $C_{2v}$ .

The correspondences of irreps at HSPs from original SG to lowered SG:

$$n_{GM5}^{37} = n_{GM6}^{112} + n_{GM7}^{112} n_{Y5}^{37} = n_{M6}^{112} + n_{M7}^{112} n_{S4}^{37} = n_{X5}^{112} n_{S3}^{37} = n_{X5}^{112} n_{Z5}^{37} = n_{Z6}^{112} + n_{Z7}^{112} n_{T5}^{37} = n_{A6}^{112} + n_{A7}^{112} n_{R4}^{37} = n_{R5}^{112}$$

$$n_{R3}^{37} = n_{R5}^{112}$$

The lower SG is SG 81 when the preserved operations are: **(sub-SG label is 3) 1, 5, 6, 4.**

The transformation is:  $(\mathbf{a}_{81}, \mathbf{b}_{81}, \mathbf{c}_{81}) = (\mathbf{a}_{112}, \mathbf{b}_{112}, \mathbf{c}_{112}) \begin{pmatrix} -1 & 0 & 0 \\ 0 & -1 & 0 \\ 0 & 0 & 1 \end{pmatrix}, \overrightarrow{O_{112}O_{81}} = \frac{1}{2}\mathbf{a}_{81} + (\frac{1}{2})\mathbf{b}_{81} + (\frac{1}{2})\mathbf{c}_{81}$

The reduction of higher dimensional irrep:

$D_{2d} : E \rightarrow {}^2E + {}^1E$  of  $S_4$ .

The correspondences of irreps at HSPs from original SG to lowered SG:

$$\begin{aligned} n_{GM7}^{81} &= n_{GM6}^{112} n_{GM8}^{81} = n_{GM7}^{112} n_{GM5}^{81} = n_{GM6}^{112} n_{GM6}^{81} = n_{GM7}^{112} n_{X4}^{81} = n_{X5}^{112} n_{X3}^{81} = n_{X5}^{112} n_{M7}^{81} = n_{M7}^{112} n_{M8}^{81} = n_{M6}^{112} n_{M5}^{81} = \\ n_{M7}^{112} n_{M6}^{81} &= n_{M6}^{112} n_{A7}^{81} = n_{A7}^{112} n_{A8}^{81} = n_{A6}^{112} n_{A5}^{81} = n_{A6}^{112} n_{A6}^{81} = n_{A7}^{112} n_{R4}^{81} = n_{R5}^{112} n_{R3}^{81} = n_{R5}^{112} n_{Z7}^{81} = n_{Z6}^{112} n_{Z8}^{81} = n_{Z7}^{112} n_{Z5}^{81} = \\ n_{Z7}^{112} n_{Z6}^{81} &= n_{Z6}^{112} \end{aligned}$$

## 25. Lowered SGs by higher-dimensional irreps of pairings in SG 113

The representative operations of SG/T for SG 113:

$$\begin{aligned} 1 : (x, y, z), \quad 2 : (x + \frac{1}{2}, \frac{1}{2} - y, -z), \quad 3 : (\frac{1}{2} - x, y + \frac{1}{2}, -z), \quad 4 : (-x, -y, z), \quad 5 : (y, -x, -z), \quad 6 : (-y, x, -z), \\ 7 : (\frac{1}{2} - y, \frac{1}{2} - x, z), \quad 8 : (y + \frac{1}{2}, x + \frac{1}{2}, z). \end{aligned}$$

The lower SG is SG 18 when the preserved operations are: **(sub-SG label is 1) 1, 2, 3, 4.**

The transformation is:  $(\mathbf{a}_{18}, \mathbf{b}_{18}, \mathbf{c}_{18}) = (\mathbf{a}_{113}, \mathbf{b}_{113}, \mathbf{c}_{113}) \begin{pmatrix} -1 & 0 & 0 \\ 0 & 1 & 0 \\ 0 & 0 & -1 \end{pmatrix}$ ,  $\overrightarrow{O_{113}O_{18}} = \frac{1}{2}\mathbf{a}_{18} + (\frac{1}{2})\mathbf{c}_{18}$

The reduction of higher dimensional irrep:

$D_{2d} : E \rightarrow B_2 + B_3$  of  $D_2$ .

The correspondences of irreps at HSPs from original SG to lowered SG:

$$\begin{aligned} n_{GM5}^{18} &= n_{GM6}^{113} + n_{GM7}^{113} n_{X4}^{18} = n_{X2}^{113} n_{X5}^{18} = n_{X5}^{113} n_{X3}^{18} = n_{X3}^{113} n_{X2}^{18} = n_{X4}^{113} n_{S5}^{18} = n_{M6}^{113} + n_{M7}^{113} n_{R5}^{18} = n_{A6}^{113} + n_{A7}^{113} n_{U4}^{18} = \\ n_{R4}^{113} n_{U5}^{18} &= n_{R3}^{113} n_{U3}^{18} = n_{R5}^{113} n_{U2}^{18} = n_{R2}^{113} n_{Z5}^{18} = n_{Z6}^{113} + n_{Z7}^{113} n_{T3}^{18} = n_{R2}^{113} n_{T2}^{18} = n_{R3}^{113} n_{T4}^{18} = n_{R5}^{113} n_{T5}^{18} = n_{R4}^{113} n_{Y3}^{18} = n_{X4}^{113} \\ n_{Y2}^{18} &= n_{X5}^{113} n_{Y4}^{18} = n_{X3}^{113} n_{Y5}^{18} = n_{X2}^{113} \end{aligned}$$

The lower SG is SG 35 when the preserved operations are: **(sub-SG label is 2) 1, 4, 7, 8.**

The transformation is:  $(\mathbf{a}_{35}, \mathbf{b}_{35}, \mathbf{c}_{35}) = (\mathbf{a}_{113}, \mathbf{b}_{113}, \mathbf{c}_{113}) \begin{pmatrix} 1 & -1 & 0 \\ 1 & 1 & 0 \\ 0 & 0 & 1 \end{pmatrix}$ ,  $\overrightarrow{O_{113}O_{35}} = \frac{1}{4}\mathbf{a}_{35} + (\frac{1}{4})\mathbf{b}_{35}$

The reduction of higher dimensional irrep:

$D_{2d} : E \rightarrow B_1 + B_2$  of  $C_{2v}$ .

The correspondences of irreps at HSPs from original SG to lowered SG:

$$\begin{aligned} n_{GM5}^{35} &= n_{GM6}^{113} + n_{GM7}^{113} n_{Y5}^{35} = n_{M6}^{113} + n_{M7}^{113} n_{S4}^{35} = n_{X2}^{113} + n_{X4}^{113} n_{S3}^{35} = n_{X3}^{113} + n_{X5}^{113} n_{Z5}^{35} = n_{Z6}^{113} + n_{Z7}^{113} n_{T5}^{35} = n_{A6}^{113} + n_{A7}^{113} \\ n_{R4}^{35} &= n_{R2}^{113} + n_{R4}^{113} n_{R3}^{35} = n_{R3}^{113} + n_{R5}^{113} \end{aligned}$$

The lower SG is SG 81 when the preserved operations are: **(sub-SG label is 3) 1, 5, 6, 4.**

The transformation is:  $(\mathbf{a}_{81}, \mathbf{b}_{81}, \mathbf{c}_{81}) = (\mathbf{a}_{113}, \mathbf{b}_{113}, \mathbf{c}_{113}) \begin{pmatrix} -1 & 0 & 0 \\ 0 & -1 & 0 \\ 0 & 0 & 1 \end{pmatrix}$ ,  $\overrightarrow{O_{113}O_{81}} = \frac{1}{2}\mathbf{a}_{81} + (\frac{1}{2})\mathbf{b}_{81} + (\frac{1}{2})\mathbf{c}_{81}$

The reduction of higher dimensional irrep:

$D_{2d} : E \rightarrow {}^2E + {}^1E$  of  $S_4$ .

The correspondences of irreps at HSPs from original SG to lowered SG:

$$\begin{aligned} n_{GM7}^{81} &= n_{GM6}^{113} n_{GM8}^{81} = n_{GM7}^{113} n_{GM5}^{81} = n_{GM6}^{113} n_{GM6}^{81} = n_{GM7}^{113} n_{X4}^{81} = n_{X2}^{113} + n_{X4}^{113} n_{X3}^{81} = n_{X3}^{113} + n_{X5}^{113} n_{M7}^{81} = n_{M6}^{113} n_{M8}^{81} = \\ n_{M7}^{113} n_{M5}^{81} &= n_{M7}^{113} n_{M6}^{81} = n_{M6}^{113} n_{A7}^{81} = n_{A7}^{113} n_{A8}^{81} = n_{A6}^{113} n_{A5}^{81} = n_{A6}^{113} n_{A6}^{81} = n_{A7}^{113} n_{R4}^{81} = n_{R2}^{113} + n_{R4}^{113} n_{R3}^{81} = n_{R3}^{113} + n_{R5}^{113} \\ n_{Z7}^{81} &= n_{Z7}^{113} n_{Z8}^{81} = n_{Z6}^{113} n_{Z5}^{81} = n_{Z7}^{113} n_{Z6}^{81} = n_{Z6}^{113} \end{aligned}$$

## 26. Lowered SGs by higher-dimensional irreps of pairings in SG 114

The representative operations of SG/T for SG 114:

$$1 : (x, y, z), 2 : (x + \frac{1}{2}, \frac{1}{2} - y, \frac{1}{2} - z), 3 : (\frac{1}{2} - x, y + \frac{1}{2}, \frac{1}{2} - z), 4 : (-x, -y, z), 5 : (y, -x, -z), 6 : (-y, x, -z), \\ 7 : (\frac{1}{2} - y, \frac{1}{2} - x, z + \frac{1}{2}), 8 : (y + \frac{1}{2}, x + \frac{1}{2}, z + \frac{1}{2}).$$

The lower SG is SG 18 when the preserved operations are: **(sub-SG label is 1) 1, 2, 3, 4.**

$$\text{The transformation is: } (\mathbf{a}_{18}, \mathbf{b}_{18}, \mathbf{c}_{18}) = (\mathbf{a}_{114}, \mathbf{b}_{114}, \mathbf{c}_{114}) \begin{pmatrix} -1 & 0 & 0 \\ 0 & 1 & 0 \\ 0 & 0 & -1 \end{pmatrix}, \overrightarrow{O_{114}O_{18}} = \frac{1}{2}\mathbf{a}_{18} + (\frac{1}{4})\mathbf{c}_{18}$$

The reduction of higher dimensional irrep:

$$D_{2d} : E \rightarrow B_2 + B_3 \text{ of } D_2.$$

The correspondences of irreps at HSPs from original SG to lowered SG:

$$n_{GM5}^{18} = n_{GM6}^{114} + n_{GM7}^{114} \quad n_{X4}^{18} = n_{X2}^{114} \quad n_{X5}^{18} = n_{X3}^{114} \quad n_{X2}^{18} = n_{X4}^{114} \quad n_{X3}^{18} = n_{X5}^{114} \quad n_{S5}^{18} = n_{M6}^{114} + n_{M7}^{114} \quad n_{R5}^{18} = n_{A6}^{114} + n_{A7}^{114} \quad n_{U4}^{18} = \\ n_{R2}^{114} \quad n_{U5}^{18} = n_{R5}^{114} \quad n_{U3}^{18} = n_{R3}^{114} \quad n_{U2}^{18} = n_{R4}^{114} \quad n_{Z5}^{18} = n_{Z6}^{114} + n_{Z7}^{114} \quad n_{T3}^{18} = n_{R2}^{114} \quad n_{T2}^{18} = n_{R3}^{114} \quad n_{T4}^{18} = n_{R5}^{114} \quad n_{T5}^{18} = n_{R4}^{114} \quad n_{Y3}^{18} = n_{X4}^{114} \\ n_{Y2}^{18} = n_{X5}^{114} \quad n_{Y4}^{18} = n_{X3}^{114} \quad n_{Y5}^{18} = n_{X2}^{114}$$

The lower SG is SG 37 when the preserved operations are: **(sub-SG label is 2) 1, 4, 7, 8.**

$$\text{The transformation is: } (\mathbf{a}_{37}, \mathbf{b}_{37}, \mathbf{c}_{37}) = (\mathbf{a}_{114}, \mathbf{b}_{114}, \mathbf{c}_{114}) \begin{pmatrix} 1 & -1 & 0 \\ 1 & 1 & 0 \\ 0 & 0 & 1 \end{pmatrix}, \overrightarrow{O_{114}O_{37}} = \frac{1}{4}\mathbf{a}_{37} + (\frac{1}{4})\mathbf{b}_{37}$$

The reduction of higher dimensional irrep:

$$D_{2d} : E \rightarrow B_1 + B_2 \text{ of } C_{2v}.$$

The correspondences of irreps at HSPs from original SG to lowered SG:

$$n_{GM5}^{37} = n_{GM6}^{114} + n_{GM7}^{114} \quad n_{Y5}^{37} = n_{M6}^{114} + n_{M7}^{114} \quad n_{S4}^{37} = n_{X2}^{114} + n_{X4}^{114} \quad n_{S3}^{37} = n_{X3}^{114} + n_{X5}^{114} \quad n_{Z5}^{37} = n_{Z6}^{114} + n_{Z7}^{114} \quad n_{T5}^{37} = n_{A6}^{114} + n_{A7}^{114} \\ n_{R4}^{37} = n_{R2}^{114} + n_{R4}^{114} \quad n_{R3}^{37} = n_{R3}^{114} + n_{R5}^{114}$$

The lower SG is SG 81 when the preserved operations are: **(sub-SG label is 3) 1, 5, 6, 4.**

$$\text{The transformation is: } (\mathbf{a}_{81}, \mathbf{b}_{81}, \mathbf{c}_{81}) = (\mathbf{a}_{114}, \mathbf{b}_{114}, \mathbf{c}_{114}) \begin{pmatrix} -1 & 0 & 0 \\ 0 & -1 & 0 \\ 0 & 0 & 1 \end{pmatrix}, \overrightarrow{O_{114}O_{81}} = \frac{1}{2}\mathbf{a}_{81} + (\frac{1}{2})\mathbf{b}_{81} + (\frac{1}{2})\mathbf{c}_{81}$$

The reduction of higher dimensional irrep:

$$D_{2d} : E \rightarrow {}^2E + {}^1E \text{ of } S_4.$$

The correspondences of irreps at HSPs from original SG to lowered SG:

$$n_{GM7}^{81} = n_{GM6}^{114} \quad n_{GM8}^{81} = n_{GM7}^{114} \quad n_{GM5}^{81} = n_{GM6}^{114} \quad n_{GM6}^{81} = n_{GM7}^{114} \quad n_{X4}^{81} = n_{X2}^{114} + n_{X4}^{114} \quad n_{X3}^{81} = n_{X3}^{114} + n_{X5}^{114} \quad n_{M7}^{81} = n_{M6}^{114} \quad n_{M8}^{81} = \\ n_{M7}^{114} \quad n_{M5}^{81} = n_{M7}^{114} \quad n_{M6}^{81} = n_{M6}^{114} \quad n_{A7}^{81} = n_{A6}^{114} \quad n_{A8}^{81} = n_{A7}^{114} \quad n_{A5}^{81} = n_{A6}^{114} \quad n_{A6}^{81} = n_{A7}^{114} \quad n_{R4}^{81} = n_{R2}^{114} + n_{R4}^{114} \quad n_{R3}^{81} = n_{R3}^{114} + n_{R5}^{114} \\ n_{Z7}^{81} = n_{Z6}^{114} \quad n_{Z8}^{81} = n_{Z7}^{114} \quad n_{Z5}^{81} = n_{Z7}^{114} \quad n_{Z6}^{81} = n_{Z6}^{114}$$

## 27. Lowered SGs by higher-dimensional irreps of pairings in SG 115

The representative operations of SG/T for SG 115:

$$1 : (x, y, z), 2 : (-x, -y, z), 3 : (y, x, -z), 4 : (-y, -x, -z), 5 : (y, -x, -z), 6 : (-y, x, -z), 7 : (-x, y, z), \\ 8 : (x, -y, z).$$

The lower SG is SG 21 when the preserved operations are: **(sub-SG label is 1) 1, 2, 3, 4.**

$$\text{The transformation is: } (\mathbf{a}_{21}, \mathbf{b}_{21}, \mathbf{c}_{21}) = (\mathbf{a}_{115}, \mathbf{b}_{115}, \mathbf{c}_{115}) \begin{pmatrix} 1 & -1 & 0 \\ 1 & 1 & 0 \\ 0 & 0 & 1 \end{pmatrix}, \overrightarrow{O_{115}O_{21}} = \frac{1}{2}\mathbf{c}_{21}$$

The reduction of higher dimensional irrep:

$$D_{2d} : E \rightarrow B_2 + B_3 \text{ of } D_2.$$

The correspondences of irreps at HSPs from original SG to lowered SG:

$$n_{GM5}^{21} = n_{GM6}^{115} + n_{GM7}^{115} \quad n_{Y5}^{21} = n_{M6}^{115} + n_{M7}^{115} \quad n_{S4}^{21} = n_{X5}^{115} \quad n_{S3}^{21} = n_{X5}^{115} \quad n_{Z5}^{21} = n_{Z6}^{115} + n_{Z7}^{115} \quad n_{T5}^{21} = n_{A6}^{115} + n_{A7}^{115} \quad n_{R4}^{21} = n_{R5}^{115} \\ n_{R3}^{21} = n_{R5}^{115}$$

The lower SG is SG 25 when the preserved operations are: **(sub-SG label is 2) 1, 2, 7, 8.**

The transformation is:  $(\mathbf{a}_{25}, \mathbf{b}_{25}, \mathbf{c}_{25}) = (\mathbf{a}_{115}, \mathbf{b}_{115}, \mathbf{c}_{115}) \begin{pmatrix} 1 & 0 & 0 \\ 0 & 1 & 0 \\ 0 & 0 & 1 \end{pmatrix}, \overrightarrow{O_{115}O_{25}} = \frac{1}{2}\mathbf{a}_{25}$

The reduction of higher dimensional irrep:

$D_{2d} : E \rightarrow B_1 + B_2$  of  $C_{2v}$ .

The correspondences of irreps at HSPs from original SG to lowered SG:

$$\begin{aligned} n_{GM5}^{25} &= n_{GM6}^{115} + n_{GM7}^{115} n_{X5}^{25} = n_{X5}^{115} n_{S5}^{25} = n_{M6}^{115} + n_{M7}^{115} n_{R5}^{25} = n_{A6}^{115} + n_{A7}^{115} n_{U5}^{25} = n_{R5}^{115} n_{Z5}^{25} = n_{Z6}^{115} + n_{Z7}^{115} n_{T5}^{25} = n_{R5}^{115} \\ n_{Y5}^{25} &= n_{X5}^{115} \end{aligned}$$

The lower SG is SG 81 when the preserved operations are: **(sub-SG label is 3) 1, 5, 6, 2.**

The transformation is:  $(\mathbf{a}_{81}, \mathbf{b}_{81}, \mathbf{c}_{81}) = (\mathbf{a}_{115}, \mathbf{b}_{115}, \mathbf{c}_{115}) \begin{pmatrix} -1 & 0 & 0 \\ 0 & -1 & 0 \\ 0 & 0 & 1 \end{pmatrix}, \overrightarrow{O_{115}O_{81}} = \frac{1}{2}\mathbf{a}_{81} + (\frac{1}{2})\mathbf{b}_{81} + (\frac{1}{2})\mathbf{c}_{81}$

The reduction of higher dimensional irrep:

$D_{2d} : E \rightarrow {}^2E + {}^1E$  of  $S_4$ .

The correspondences of irreps at HSPs from original SG to lowered SG:

$$\begin{aligned} n_{GM7}^{81} &= n_{GM6}^{115} n_{GM8}^{81} = n_{GM7}^{115} n_{GM5}^{81} = n_{GM6}^{115} n_{GM6}^{81} = n_{GM7}^{115} n_{X4}^{81} = n_{X5}^{115} n_{X3}^{81} = n_{X5}^{115} n_{M7}^{81} = n_{M7}^{115} n_{M8}^{81} = n_{M6}^{115} n_{M5}^{81} = \\ n_{M7}^{115} n_{M6}^{81} &= n_{M6}^{115} n_{A7}^{81} = n_{A6}^{115} n_{A8}^{81} = n_{A7}^{115} n_{A5}^{81} = n_{A6}^{115} n_{A6}^{81} = n_{A7}^{115} n_{R4}^{81} = n_{R5}^{115} n_{R3}^{81} = n_{R5}^{115} n_{Z7}^{81} = n_{Z7}^{115} n_{Z8}^{81} = n_{Z6}^{115} n_{Z5}^{81} = \\ n_{Z7}^{115} n_{Z6}^{81} &= n_{Z6}^{115} \end{aligned}$$

## 28. Lowered SGs by higher-dimensional irreps of pairings in SG 116

The representative operations of SG/T for SG 116:

$$\begin{aligned} 1 : (x, y, z), 2 : (-x, -y, z), 3 : (y, x, \frac{1}{2} - z), 4 : (-y, -x, \frac{1}{2} - z), 5 : (y, -x, -z), 6 : (-y, x, -z), 7 : (-x, y, z + \frac{1}{2}), \\ 8 : (x, -y, z + \frac{1}{2}). \end{aligned}$$

The lower SG is SG 21 when the preserved operations are: **(sub-SG label is 1) 1, 2, 3, 4.**

The transformation is:  $(\mathbf{a}_{21}, \mathbf{b}_{21}, \mathbf{c}_{21}) = (\mathbf{a}_{116}, \mathbf{b}_{116}, \mathbf{c}_{116}) \begin{pmatrix} 1 & -1 & 0 \\ 1 & 1 & 0 \\ 0 & 0 & 1 \end{pmatrix}, \overrightarrow{O_{116}O_{21}} = \frac{3}{4}\mathbf{c}_{21}$

The reduction of higher dimensional irrep:

$D_{2d} : E \rightarrow B_2 + B_3$  of  $D_2$ .

The correspondences of irreps at HSPs from original SG to lowered SG:

$$\begin{aligned} n_{GM5}^{21} &= n_{GM6}^{116} + n_{GM7}^{116} n_{Y5}^{21} = n_{M6}^{116} + n_{M7}^{116} n_{S4}^{21} = n_{X5}^{116} n_{S3}^{21} = n_{X5}^{116} n_{Z5}^{21} = n_{Z6}^{116} + n_{Z7}^{116} n_{T5}^{21} = n_{A6}^{116} + n_{A7}^{116} n_{R4}^{21} = n_{R5}^{116} \\ n_{R3}^{21} &= n_{R5}^{116} \end{aligned}$$

The lower SG is SG 27 when the preserved operations are: **(sub-SG label is 2) 1, 2, 7, 8.**

The transformation is:  $(\mathbf{a}_{27}, \mathbf{b}_{27}, \mathbf{c}_{27}) = (\mathbf{a}_{116}, \mathbf{b}_{116}, \mathbf{c}_{116}) \begin{pmatrix} 1 & 0 & 0 \\ 0 & 1 & 0 \\ 0 & 0 & 1 \end{pmatrix}, \overrightarrow{O_{116}O_{27}} = \frac{1}{2}\mathbf{a}_{27}$

The reduction of higher dimensional irrep:

$D_{2d} : E \rightarrow B_1 + B_2$  of  $C_{2v}$ .

The correspondences of irreps at HSPs from original SG to lowered SG:

$$\begin{aligned} n_{GM5}^{27} &= n_{GM6}^{116} + n_{GM7}^{116} n_{X5}^{27} = n_{X5}^{116} n_{S5}^{27} = n_{M6}^{116} + n_{M7}^{116} n_{R5}^{27} = n_{A6}^{116} + n_{A7}^{116} n_{U5}^{27} = n_{R5}^{116} n_{Z5}^{27} = n_{Z6}^{116} + n_{Z7}^{116} n_{T5}^{27} = n_{R5}^{116} \\ n_{Y5}^{27} &= n_{X5}^{116} \end{aligned}$$

The lower SG is SG 81 when the preserved operations are: **(sub-SG label is 3) 1, 5, 6, 2.**

The transformation is:  $(\mathbf{a}_{81}, \mathbf{b}_{81}, \mathbf{c}_{81}) = (\mathbf{a}_{116}, \mathbf{b}_{116}, \mathbf{c}_{116}) \begin{pmatrix} -1 & 0 & 0 \\ 0 & -1 & 0 \\ 0 & 0 & 1 \end{pmatrix}, \overrightarrow{O_{116}O_{81}} = \frac{1}{2}\mathbf{a}_{81} + (\frac{1}{2})\mathbf{b}_{81} + (\frac{1}{2})\mathbf{c}_{81}$

The reduction of higher dimensional irrep:

$$D_{2d} : E \rightarrow {}^2E + {}^1E \text{ of } S_4.$$

The correspondences of irreps at HSPs from original SG to lowered SG:

$$\begin{aligned} n_{GM7}^{81} &= n_{GM6}^{116} n_{GM8}^{81} = n_{GM7}^{116} n_{GM5}^{81} = n_{GM6}^{116} n_{GM6}^{81} = n_{GM7}^{116} n_{X4}^{81} = n_{X5}^{116} n_{X3}^{81} = n_{X5}^{116} n_{M7}^{81} = n_{M7}^{116} n_{M8}^{81} = n_{M6}^{116} n_{M5}^{81} = \\ n_{M7}^{116} n_{M6}^{81} &= n_{M6}^{116} n_{A7}^{81} = n_{A7}^{116} n_{A8}^{81} = n_{A6}^{116} n_{A5}^{81} = n_{A6}^{116} n_{A6}^{81} = n_{A7}^{116} n_{R4}^{81} = n_{R5}^{116} n_{R3}^{81} = n_{R5}^{116} n_{Z7}^{81} = n_{Z6}^{116} n_{Z8}^{81} = n_{Z7}^{116} n_{Z5}^{81} = \\ n_{Z7}^{116} n_{Z6}^{81} &= n_{Z6}^{116} \end{aligned}$$

**29. Lowered SGs by higher-dimensional irreps of pairings in SG 117**

The representative operations of SG/T for SG 117:

$$\begin{aligned} 1 : (x, y, z), 2 : (-x, -y, z), 3 : (y + \frac{1}{2}, x + \frac{1}{2}, -z), 4 : (\frac{1}{2} - y, \frac{1}{2} - x, -z), 5 : (y, -x, -z), 6 : (-y, x, -z), \\ 7 : (\frac{1}{2} - x, y + \frac{1}{2}, z), 8 : (x + \frac{1}{2}, \frac{1}{2} - y, z). \end{aligned}$$

The lower SG is SG 21 when the preserved operations are: (sub-SG label is 1) 1, 2, 3, 4.

The transformation is:  $(\mathbf{a}_{21}, \mathbf{b}_{21}, \mathbf{c}_{21}) = (\mathbf{a}_{117}, \mathbf{b}_{117}, \mathbf{c}_{117}) \begin{pmatrix} -1 & -1 & 0 \\ 1 & -1 & 0 \\ 0 & 0 & 1 \end{pmatrix}, \overrightarrow{O_{117}O_{21}} = \frac{1}{4}\mathbf{a}_{21} + (\frac{1}{4})\mathbf{b}_{21} + (\frac{1}{2})\mathbf{c}_{21}$

The reduction of higher dimensional irrep:

$$D_{2d} : E \rightarrow B_2 + B_3 \text{ of } D_2.$$

The correspondences of irreps at HSPs from original SG to lowered SG:

$$\begin{aligned} n_{GM5}^{21} &= n_{GM6}^{117} + n_{GM7}^{117} n_{Y5}^{21} = n_{M6}^{117} + n_{M7}^{117} n_{S4}^{21} = n_{X2}^{117} + n_{X4}^{117} n_{S3}^{21} = n_{X3}^{117} + n_{X5}^{117} n_{Z5}^{21} = n_{Z6}^{117} + n_{Z7}^{117} n_{T5}^{21} = n_{A6}^{117} + n_{A7}^{117} \\ n_{R4}^{21} &= n_{R2}^{117} + n_{R4}^{117} n_{R3}^{21} = n_{R3}^{117} + n_{R5}^{117} \end{aligned}$$

The lower SG is SG 32 when the preserved operations are: (sub-SG label is 2) 1, 2, 7, 8.

The transformation is:  $(\mathbf{a}_{32}, \mathbf{b}_{32}, \mathbf{c}_{32}) = (\mathbf{a}_{117}, \mathbf{b}_{117}, \mathbf{c}_{117}) \begin{pmatrix} 1 & 0 & 0 \\ 0 & 1 & 0 \\ 0 & 0 & 1 \end{pmatrix}, \overrightarrow{O_{117}O_{32}} = \frac{1}{2}\mathbf{a}_{32} + (\frac{1}{2})\mathbf{b}_{32}$

The reduction of higher dimensional irrep:

$$D_{2d} : E \rightarrow B_1 + B_2 \text{ of } C_{2v}.$$

The correspondences of irreps at HSPs from original SG to lowered SG:

$$\begin{aligned} n_{GM5}^{32} &= n_{GM6}^{117} + n_{GM7}^{117} n_{X3}^{32} = n_{X4}^{117} n_{X5}^{32} = n_{X2}^{117} n_{X2}^{32} = n_{X3}^{117} n_{X4}^{32} = n_{X5}^{117} n_{S5}^{32} = n_{M6}^{117} + n_{M7}^{117} n_{R5}^{32} = n_{A6}^{117} + n_{A7}^{117} n_{U3}^{32} = \\ n_{R4}^{32} &= n_{R2}^{117} n_{U5}^{32} = n_{R2}^{117} n_{U2}^{32} = n_{R3}^{117} n_{U4}^{32} = n_{R5}^{117} n_{Z5}^{32} = n_{Z6}^{117} + n_{Z7}^{117} n_{T5}^{32} = n_{R4}^{117} n_{T3}^{32} = n_{R2}^{117} n_{T4}^{32} = n_{R5}^{117} n_{T2}^{32} = n_{R3}^{117} n_{Y5}^{32} = n_{X4}^{117} \\ n_{Y3}^{32} &= n_{X2}^{117} n_{Y4}^{32} = n_{X5}^{117} n_{Y2}^{32} = n_{X3}^{117} \end{aligned}$$

The lower SG is SG 81 when the preserved operations are: (sub-SG label is 3) 1, 5, 6, 2.

The transformation is:  $(\mathbf{a}_{81}, \mathbf{b}_{81}, \mathbf{c}_{81}) = (\mathbf{a}_{117}, \mathbf{b}_{117}, \mathbf{c}_{117}) \begin{pmatrix} -1 & 0 & 0 \\ 0 & -1 & 0 \\ 0 & 0 & 1 \end{pmatrix}, \overrightarrow{O_{117}O_{81}} = \frac{1}{2}\mathbf{a}_{81} + (\frac{1}{2})\mathbf{b}_{81} + (\frac{1}{2})\mathbf{c}_{81}$

The reduction of higher dimensional irrep:

$$D_{2d} : E \rightarrow {}^2E + {}^1E \text{ of } S_4.$$

The correspondences of irreps at HSPs from original SG to lowered SG:

$$\begin{aligned} n_{GM7}^{81} &= n_{GM6}^{117} n_{GM8}^{81} = n_{GM7}^{117} n_{GM5}^{81} = n_{GM6}^{117} n_{GM6}^{81} = n_{GM7}^{117} n_{X4}^{81} = n_{X2}^{117} + n_{X4}^{117} n_{X3}^{81} = n_{X3}^{117} + n_{X5}^{117} n_{M7}^{81} = n_{M6}^{117} n_{M8}^{81} = \\ n_{M7}^{117} n_{M5}^{81} &= n_{M7}^{117} n_{M6}^{81} = n_{M6}^{117} n_{A7}^{81} = n_{A7}^{117} n_{A8}^{81} = n_{A6}^{117} n_{A5}^{81} = n_{A6}^{117} n_{A6}^{81} = n_{A7}^{117} n_{R4}^{81} = n_{R2}^{117} + n_{R4}^{117} n_{R3}^{81} = n_{R3}^{117} + n_{R5}^{117} \\ n_{Z7}^{81} &= n_{Z7}^{117} n_{Z8}^{81} = n_{Z6}^{117} n_{Z5}^{81} = n_{Z7}^{117} n_{Z6}^{81} = n_{Z6}^{117} \end{aligned}$$

**30. Lowered SGs by higher-dimensional irreps of pairings in SG 118**

The representative operations of SG/T for SG 118:

$$1 : (x, y, z), 2 : (-x, -y, z), 3 : (y + \frac{1}{2}, x + \frac{1}{2}, \frac{1}{2} - z), 4 : (\frac{1}{2} - y, \frac{1}{2} - x, \frac{1}{2} - z), 5 : (y, -x, -z), 6 : (-y, x, -z), \\ 7 : (\frac{1}{2} - x, y + \frac{1}{2}, z + \frac{1}{2}), 8 : (x + \frac{1}{2}, \frac{1}{2} - y, z + \frac{1}{2}).$$

The lower SG is SG 21 when the preserved operations are: **(sub-SG label is 1) 1, 2, 3, 4.**

$$\text{The transformation is: } (\mathbf{a}_{21}, \mathbf{b}_{21}, \mathbf{c}_{21}) = (\mathbf{a}_{118}, \mathbf{b}_{118}, \mathbf{c}_{118}) \begin{pmatrix} -1 & -1 & 0 \\ 1 & -1 & 0 \\ 0 & 0 & 1 \end{pmatrix}, \overrightarrow{O_{118}O_{21}} = \frac{1}{4}\mathbf{a}_{21} + (\frac{1}{4})\mathbf{b}_{21} + (\frac{3}{4})\mathbf{c}_{21}$$

The reduction of higher dimensional irrep:

$$D_{2d} : E \rightarrow B_2 + B_3 \text{ of } D_2.$$

The correspondences of irreps at HSPs from original SG to lowered SG:

$$n_{GM5}^{21} = n_{GM6}^{118} + n_{GM7}^{118} \quad n_{Y5}^{21} = n_{M6}^{118} + n_{M7}^{118} \quad n_{S4}^{21} = n_{X2}^{118} + n_{X4}^{118} \quad n_{S3}^{21} = n_{X3}^{118} + n_{X5}^{118} \quad n_{Z5}^{21} = n_{Z6}^{118} + n_{Z7}^{118} \quad n_{T5}^{21} = n_{A6}^{118} + n_{A7}^{118} \\ n_{R4}^{21} = n_{R2}^{118} + n_{R4}^{118} \quad n_{R3}^{21} = n_{R3}^{118} + n_{R5}^{118}$$

The lower SG is SG 34 when the preserved operations are: **(sub-SG label is 2) 1, 2, 7, 8.**

$$\text{The transformation is: } (\mathbf{a}_{34}, \mathbf{b}_{34}, \mathbf{c}_{34}) = (\mathbf{a}_{118}, \mathbf{b}_{118}, \mathbf{c}_{118}) \begin{pmatrix} 1 & 0 & 0 \\ 0 & 1 & 0 \\ 0 & 0 & 1 \end{pmatrix}, \overrightarrow{O_{118}O_{34}} = \frac{1}{2}\mathbf{a}_{34} + (\frac{1}{2})\mathbf{b}_{34}$$

The reduction of higher dimensional irrep:

$$D_{2d} : E \rightarrow B_1 + B_2 \text{ of } C_{2v}.$$

The correspondences of irreps at HSPs from original SG to lowered SG:

$$n_{GM5}^{34} = n_{GM6}^{118} + n_{GM7}^{118} \quad n_{Y3}^{34} = n_{X4}^{118} \quad n_{X5}^{34} = n_{X2}^{118} \quad n_{X2}^{34} = n_{X3}^{118} \quad n_{X4}^{34} = n_{X5}^{118} \quad n_{S5}^{34} = n_{M6}^{118} + n_{M7}^{118} \quad n_{R5}^{34} = n_{A6}^{118} + n_{A7}^{118} \quad n_{U3}^{34} = n_{R4}^{118} \quad n_{U5}^{34} = n_{R2}^{118} \quad n_{U2}^{34} = n_{R3}^{118} \quad n_{U4}^{34} = n_{R5}^{118} \quad n_{Z5}^{34} = n_{Z6}^{118} + n_{Z7}^{118} \quad n_{T5}^{34} = n_{R4}^{118} \quad n_{T3}^{34} = n_{R2}^{118} \quad n_{T4}^{34} = n_{R5}^{118} \quad n_{T2}^{34} = n_{R3}^{118} \quad n_{Y5}^{34} = n_{X4}^{118} \\ n_{Y3}^{34} = n_{X2}^{118} \quad n_{Y4}^{34} = n_{X5}^{118} \quad n_{Y2}^{34} = n_{X3}^{118}$$

The lower SG is SG 81 when the preserved operations are: **(sub-SG label is 3) 1, 5, 6, 2.**

$$\text{The transformation is: } (\mathbf{a}_{81}, \mathbf{b}_{81}, \mathbf{c}_{81}) = (\mathbf{a}_{118}, \mathbf{b}_{118}, \mathbf{c}_{118}) \begin{pmatrix} -1 & 0 & 0 \\ 0 & -1 & 0 \\ 0 & 0 & 1 \end{pmatrix}, \overrightarrow{O_{118}O_{81}} = \frac{1}{2}\mathbf{a}_{81} + (\frac{1}{2})\mathbf{b}_{81} + (\frac{1}{2})\mathbf{c}_{81}$$

The reduction of higher dimensional irrep:

$$D_{2d} : E \rightarrow {}^2E + {}^1E \text{ of } S_4.$$

The correspondences of irreps at HSPs from original SG to lowered SG:

$$n_{GM7}^{81} = n_{GM6}^{118} \quad n_{GM8}^{81} = n_{GM7}^{118} \quad n_{GM5}^{81} = n_{GM6}^{118} \quad n_{GM6}^{81} = n_{GM7}^{118} \quad n_{X4}^{81} = n_{X2}^{118} + n_{X4}^{118} \quad n_{X3}^{81} = n_{X3}^{118} + n_{X5}^{118} \quad n_{M7}^{81} = n_{M6}^{118} \quad n_{M8}^{81} = n_{M7}^{118} \quad n_{M5}^{81} = n_{M7}^{118} \quad n_{M6}^{81} = n_{M6}^{118} \quad n_{A7}^{81} = n_{A6}^{118} \quad n_{A8}^{81} = n_{A7}^{118} \quad n_{A5}^{81} = n_{A6}^{118} \quad n_{A6}^{81} = n_{A7}^{118} \quad n_{R4}^{81} = n_{R2}^{118} + n_{R4}^{118} \quad n_{R3}^{81} = n_{R3}^{118} + n_{R5}^{118} \\ n_{Z7}^{81} = n_{Z6}^{118} \quad n_{Z8}^{81} = n_{Z7}^{118} \quad n_{Z5}^{81} = n_{Z7}^{118} \quad n_{Z6}^{81} = n_{Z6}^{118}$$

### 31. Lowered SGs by higher-dimensional irreps of pairings in SG 119

The representative operations of SG/T for SG 119:

$$1 : (x, y, z), 2 : (-x, -y, z), 3 : (y, x, -z), 4 : (-y, -x, -z), 5 : (y, -x, -z), 6 : (-y, x, -z), 7 : (-x, y, z), \\ 8 : (x, -y, z).$$

The lower SG is SG 22 when the preserved operations are: **(sub-SG label is 1) 1, 2, 3, 4.**

$$\text{The transformation is: } (\mathbf{a}_{22}, \mathbf{b}_{22}, \mathbf{c}_{22}) = (\mathbf{a}_{119}, \mathbf{b}_{119}, \mathbf{c}_{119}) \begin{pmatrix} 1 & -1 & 0 \\ 1 & 1 & 0 \\ 0 & 0 & 1 \end{pmatrix}, \overrightarrow{O_{119}O_{22}} = \frac{1}{4}\mathbf{a}_{22} + (-\frac{1}{4})\mathbf{b}_{22} + (-\frac{1}{4})\mathbf{c}_{22}$$

The reduction of higher dimensional irrep:

$$D_{2d} : E \rightarrow B_2 + B_3 \text{ of } D_2.$$

The correspondences of irreps at HSPs from original SG to lowered SG:

$$n_{GM5}^{22} = n_{GM6}^{119} + n_{GM7}^{119} \quad n_{Y5}^{22} = n_{X5}^{119} \quad n_{L2}^{22} = n_{N3}^{119} + n_{N4}^{119} \quad n_{Z5}^{22} = n_{M6}^{119} + n_{M7}^{119} \quad n_{T5}^{22} = n_{X5}^{119}$$

The lower SG is SG 44 when the preserved operations are: **(sub-SG label is 2) 1, 2, 7, 8.**

The transformation is:  $(\mathbf{a}_{44}, \mathbf{b}_{44}, \mathbf{c}_{44}) = (\mathbf{a}_{119}, \mathbf{b}_{119}, \mathbf{c}_{119}) \begin{pmatrix} 1 & 0 & 0 \\ 0 & 1 & 0 \\ 0 & 0 & 1 \end{pmatrix}, \overrightarrow{O_{119}O_{44}} = -\frac{1}{2}\mathbf{b}_{44}$

The reduction of higher dimensional irrep:

$D_{2d} : E \rightarrow B_1 + B_2$  of  $C_{2v}$ .

The correspondences of irreps at HSPs from original SG to lowered SG:

$$\begin{aligned} n_{GM5}^{44} &= n_{GM6}^{119} + n_{GM7}^{119} n_{X5}^{44} = n_{M6}^{119} + n_{M7}^{119} n_{T4}^{44} = n_{X5}^{119} n_{T3}^{44} = n_{X5}^{119} n_{W4}^{44} = n_{P5}^{119} + n_{P6}^{119} n_{W3}^{44} = n_{P7}^{119} + n_{P8}^{119} n_{R4}^{44} = n_{N4}^{119} \\ n_{R3}^{44} &= n_{N3}^{119} n_{S3}^{44} = n_{N4}^{119} n_{S4}^{44} = n_{N3}^{119} \end{aligned}$$

The lower SG is SG 82 when the preserved operations are: **(sub-SG label is 3) 1, 5, 6, 2.**

The transformation is:  $(\mathbf{a}_{82}, \mathbf{b}_{82}, \mathbf{c}_{82}) = (\mathbf{a}_{119}, \mathbf{b}_{119}, \mathbf{c}_{119}) \begin{pmatrix} 0 & 1 & 0 \\ -1 & 0 & 0 \\ 0 & 0 & 1 \end{pmatrix}, \overrightarrow{O_{119}O_{82}} = \frac{1}{2}\mathbf{a}_{82} + (-\frac{1}{2})\mathbf{b}_{82}$

The reduction of higher dimensional irrep:

$D_{2d} : E \rightarrow {}^2E + {}^1E$  of  $S_4$ .

The correspondences of irreps at HSPs from original SG to lowered SG:

$$\begin{aligned} n_{GM7}^{82} &= n_{GM6}^{119} n_{GM8}^{82} = n_{GM7}^{119} n_{GM5}^{82} = n_{GM6}^{119} n_{GM6}^{82} = n_{GM7}^{119} n_{M7}^{82} = n_{M6}^{119} n_{M8}^{82} = n_{M7}^{119} n_{M5}^{82} = n_{M6}^{119} n_{M6}^{82} = n_{M7}^{119} n_{X4}^{82} = \\ n_{X5}^{119} n_{X3}^{82} &= n_{X5}^{119} n_{P7}^{82} = n_{P6}^{119} n_{P8}^{82} = n_{P5}^{119} n_{P5}^{82} = n_{P8}^{119} n_{P6}^{82} = n_{P7}^{119} n_{N2}^{82} = n_{N3}^{119} + n_{N4}^{119} \end{aligned}$$

### 32. Lowered SGs by higher-dimensional irreps of pairings in SG 120

The representative operations of SG/T for SG 120:

$$\begin{aligned} 1 : (x, y, z), 2 : (-x, -y, z), 3 : (y, x, \frac{1}{2} - z), 4 : (-y, -x, \frac{1}{2} - z), 5 : (y, -x, -z), 6 : (-y, x, -z), 7 : (-x, y, z + \frac{1}{2}), \\ 8 : (x, -y, z + \frac{1}{2}). \end{aligned}$$

The lower SG is SG 22 when the preserved operations are: **(sub-SG label is 1) 1, 2, 3, 4.**

The transformation is:  $(\mathbf{a}_{22}, \mathbf{b}_{22}, \mathbf{c}_{22}) = (\mathbf{a}_{120}, \mathbf{b}_{120}, \mathbf{c}_{120}) \begin{pmatrix} 1 & -1 & 0 \\ 1 & 1 & 0 \\ 0 & 0 & 1 \end{pmatrix}, \overrightarrow{O_{120}O_{22}} = \frac{1}{4}\mathbf{a}_{22} + (-\frac{1}{4})\mathbf{b}_{22}$

The reduction of higher dimensional irrep:

$D_{2d} : E \rightarrow B_2 + B_3$  of  $D_2$ .

The correspondences of irreps at HSPs from original SG to lowered SG:

$$n_{GM5}^{22} = n_{GM6}^{120} + n_{GM7}^{120} n_{Y5}^{22} = n_{X5}^{120} n_{L2}^{22} = n_{N3}^{120} + n_{N4}^{120} n_{Z5}^{22} = n_{M6}^{120} + n_{M7}^{120} n_{T5}^{22} = n_{X5}^{120}$$

The lower SG is SG 45 when the preserved operations are: **(sub-SG label is 2) 1, 2, 7, 8.**

The transformation is:  $(\mathbf{a}_{45}, \mathbf{b}_{45}, \mathbf{c}_{45}) = (\mathbf{a}_{120}, \mathbf{b}_{120}, \mathbf{c}_{120}) \begin{pmatrix} 1 & 0 & 0 \\ 0 & 1 & 0 \\ 0 & 0 & 1 \end{pmatrix}, \overrightarrow{O_{120}O_{45}} = -\frac{1}{2}\mathbf{b}_{45}$

The reduction of higher dimensional irrep:

$D_{2d} : E \rightarrow B_1 + B_2$  of  $C_{2v}$ .

The correspondences of irreps at HSPs from original SG to lowered SG:

$$\begin{aligned} n_{GM5}^{45} &= n_{GM6}^{120} + n_{GM7}^{120} n_{X5}^{45} = n_{M6}^{120} + n_{M7}^{120} n_{T4}^{45} = n_{X5}^{120} n_{T3}^{45} = n_{X5}^{120} n_{W4}^{45} = n_{P5}^{120} + n_{P6}^{120} n_{W3}^{45} = n_{P7}^{120} + n_{P8}^{120} n_{R4}^{45} = n_{N4}^{120} \\ n_{R3}^{45} &= n_{N3}^{120} n_{S4}^{45} = n_{N4}^{120} n_{S3}^{45} = n_{N3}^{120} \end{aligned}$$

The lower SG is SG 82 when the preserved operations are: **(sub-SG label is 3) 1, 5, 6, 2.**

The transformation is:  $(\mathbf{a}_{82}, \mathbf{b}_{82}, \mathbf{c}_{82}) = (\mathbf{a}_{120}, \mathbf{b}_{120}, \mathbf{c}_{120}) \begin{pmatrix} 0 & 1 & 0 \\ -1 & 0 & 0 \\ 0 & 0 & 1 \end{pmatrix}, \overrightarrow{O_{120}O_{82}} = \frac{1}{2}\mathbf{a}_{82} + (-\frac{1}{2})\mathbf{b}_{82}$

The reduction of higher dimensional irrep:

$D_{2d} : E \rightarrow {}^2E + {}^1E$  of  $S_4$ .

The correspondences of irreps at HSPs from original SG to lowered SG:

$$\begin{aligned} n_{GM7}^{82} &= n_{GM6}^{120} n_{GM8}^{82} = n_{GM7}^{120} n_{GM5}^{82} = n_{GM6}^{120} n_{GM6}^{82} = n_{GM7}^{120} n_{M7}^{82} = n_{M6}^{120} n_{M8}^{82} = n_{M7}^{120} n_{M5}^{82} = n_{M6}^{120} n_{M6}^{82} = n_{M7}^{120} n_{X4}^{82} = \\ n_{X5}^{120} n_{X3}^{82} &= n_{X5}^{120} n_{P7}^{82} = n_{P5}^{120} n_{P8}^{82} = n_{P6}^{120} n_{P5}^{82} = n_{P7}^{120} n_{P6}^{82} = n_{P8}^{120} n_{N2}^{82} = n_{N3}^{120} + n_{N4}^{120} \end{aligned}$$

### 33. Lowered SGs by higher-dimensional irreps of pairings in SG 121

The representative operations of SG/T for SG 121:

$$1 : (x, y, z), 2 : (x, -y, -z), 3 : (-x, y, -z), 4 : (-x, -y, z), 5 : (y, -x, -z), 6 : (-y, x, -z), 7 : (-y, -x, z), 8 : (y, x, z).$$

The lower SG is SG 23 when the preserved operations are: (**sub-SG label is 1**) 1, 2, 3, 4.

$$\text{The transformation is: } (\mathbf{a}_{23}, \mathbf{b}_{23}, \mathbf{c}_{23}) = (\mathbf{a}_{121}, \mathbf{b}_{121}, \mathbf{c}_{121}) \begin{pmatrix} 0 & 0 & 1 \\ 1 & 0 & 0 \\ 0 & 1 & 0 \end{pmatrix}, \overrightarrow{O_{121}O_{23}} = -\frac{1}{2}\mathbf{b}_{23}$$

The reduction of higher dimensional irrep:

$$D_{2d} : E \rightarrow B_1 + B_3 \text{ of } D_2.$$

The correspondences of irreps at HSPs from original SG to lowered SG:

$$\begin{aligned} n_{GM5}^{23} &= n_{GM6}^{121} + n_{GM7}^{121} n_{X5}^{23} = n_{M6}^{121} + n_{M7}^{121} n_{T4}^{23} = n_{N4}^{121} n_{T3}^{23} = n_{N3}^{121} n_{W5}^{23} = n_{P6}^{121} + n_{P7}^{121} n_{R4}^{23} = n_{X5}^{121} n_{R3}^{23} = n_{X5}^{121} n_{S3}^{23} = \\ n_{N4}^{121} n_{S4}^{23} &= n_{N3}^{121} \end{aligned}$$

The lower SG is SG 42 when the preserved operations are: (**sub-SG label is 2**) 1, 4, 7, 8.

$$\text{The transformation is: } (\mathbf{a}_{42}, \mathbf{b}_{42}, \mathbf{c}_{42}) = (\mathbf{a}_{121}, \mathbf{b}_{121}, \mathbf{c}_{121}) \begin{pmatrix} 1 & -1 & 0 \\ 1 & 1 & 0 \\ 0 & 0 & 1 \end{pmatrix}, \overrightarrow{O_{121}O_{42}} = \mathbf{0}$$

The reduction of higher dimensional irrep:

$$D_{2d} : E \rightarrow B_1 + B_2 \text{ of } C_{2v}.$$

The correspondences of irreps at HSPs from original SG to lowered SG:

$$n_{GM5}^{42} = n_{GM6}^{121} + n_{GM7}^{121} n_{Y5}^{42} = n_{X5}^{121} n_{L2}^{42} = n_{N3}^{121} + n_{N4}^{121} n_{Z5}^{42} = n_{M6}^{121} + n_{M7}^{121} n_{T5}^{42} = n_{X5}^{121}$$

The lower SG is SG 82 when the preserved operations are: (**sub-SG label is 3**) 1, 5, 6, 4.

$$\text{The transformation is: } (\mathbf{a}_{82}, \mathbf{b}_{82}, \mathbf{c}_{82}) = (\mathbf{a}_{121}, \mathbf{b}_{121}, \mathbf{c}_{121}) \begin{pmatrix} 0 & 1 & 0 \\ -1 & 0 & 0 \\ 0 & 0 & 1 \end{pmatrix}, \overrightarrow{O_{121}O_{82}} = \frac{1}{2}\mathbf{a}_{82} + (-\frac{1}{2})\mathbf{b}_{82}$$

The reduction of higher dimensional irrep:

$$D_{2d} : E \rightarrow {}^2E + {}^1E \text{ of } S_4.$$

The correspondences of irreps at HSPs from original SG to lowered SG:

$$\begin{aligned} n_{GM7}^{82} &= n_{GM6}^{121} n_{GM8}^{82} = n_{GM7}^{121} n_{GM5}^{82} = n_{GM6}^{121} n_{GM6}^{82} = n_{GM7}^{121} n_{M7}^{82} = n_{M6}^{121} n_{M8}^{82} = n_{M7}^{121} n_{M5}^{82} = n_{M6}^{121} n_{M6}^{82} = n_{M7}^{121} n_{X4}^{82} = \\ n_{X5}^{121} n_{X3}^{82} &= n_{X5}^{121} n_{P7}^{82} = n_{P7}^{121} n_{P8}^{82} = n_{P6}^{121} n_{P5}^{82} = n_{P7}^{121} n_{P6}^{82} = n_{P6}^{121} n_{N2}^{82} = n_{N3}^{121} + n_{N4}^{121} \end{aligned}$$

### 34. Lowered SGs by higher-dimensional irreps of pairings in SG 122

The representative operations of SG/T for SG 122:

$$1 : (x, y, z), 2 : (x, \frac{1}{2} - y, \frac{1}{4} - z), 3 : (-x, y + \frac{1}{2}, \frac{1}{4} - z), 4 : (-x, -y, z), 5 : (y, -x, -z), 6 : (-y, x, -z), 7 : (-y, \frac{1}{2} - x, z + \frac{1}{4}), 8 : (y, x + \frac{1}{2}, z + \frac{1}{4}).$$

The lower SG is SG 24 when the preserved operations are: **(sub-SG label is 1) 1, 3, 2, 4.**

$$\text{The transformation is: } (\mathbf{a}_{24}, \mathbf{b}_{24}, \mathbf{c}_{24}) = (\mathbf{a}_{122}, \mathbf{b}_{122}, \mathbf{c}_{122}) \begin{pmatrix} 0 & 0 & 1 \\ 0 & -1 & 0 \\ 1 & 0 & 0 \end{pmatrix}, \overrightarrow{O_{122}O_{24}} = \frac{1}{8}\mathbf{a}_{24} + (-\frac{1}{2})\mathbf{b}_{24} + (\frac{1}{4})\mathbf{c}_{24}$$

The reduction of higher dimensional irrep:

$$D_{2d} : E \rightarrow B_1 + B_2 \text{ of } D_2.$$

The correspondences of irreps at HSPs from original SG to lowered SG:

$$\begin{aligned} n_{GM5}^{24} &= n_{GM6}^{122} + n_{GM7}^{122} n_{X5}^{24} = n_{M6}^{122} + n_{M7}^{122} n_{T3}^{24} = n_{N3}^{122} n_{T4}^{24} = n_{N4}^{122} n_{W3}^{24} = n_{P7}^{122} n_{W2}^{24} = n_{P7}^{122} n_{W4}^{24} = n_{P4}^{122} + n_{P5}^{122} n_{W5}^{24} = \\ n_{P3}^{122} + n_{P6}^{122} n_{R3}^{24} &= n_{N3}^{122} n_{R4}^{24} = n_{N4}^{122} n_{S4}^{24} = n_{X3}^{122} + n_{X5}^{122} n_{S3}^{24} = n_{X2}^{122} + n_{X4}^{122} \end{aligned}$$

The lower SG is SG 43 when the preserved operations are: **(sub-SG label is 2) 1, 4, 8, 7.**

$$\text{The transformation is: } (\mathbf{a}_{43}, \mathbf{b}_{43}, \mathbf{c}_{43}) = (\mathbf{a}_{122}, \mathbf{b}_{122}, \mathbf{c}_{122}) \begin{pmatrix} 1 & 1 & 0 \\ -1 & 1 & 0 \\ 0 & 0 & 1 \end{pmatrix}, \overrightarrow{O_{122}O_{43}} = \frac{1}{4}\mathbf{a}_{43} + (-\frac{1}{4})\mathbf{b}_{43}$$

The reduction of higher dimensional irrep:

$$D_{2d} : E \rightarrow B_1 + B_2 \text{ of } C_{2v}.$$

The correspondences of irreps at HSPs from original SG to lowered SG:

$$\begin{aligned} n_{GM5}^{43} &= n_{GM6}^{122} + n_{GM7}^{122} n_{Y3}^{43} = n_{X2}^{122} n_{Y3}^{43} = n_{X4}^{122} n_{Y4}^{43} = n_{X3}^{122} n_{Y2}^{43} = n_{X5}^{122} n_{L2}^{43} = n_{N3}^{122} + n_{N4}^{122} n_{Z5}^{43} = n_{M6}^{122} + n_{M7}^{122} n_{T5}^{43} = \\ n_{X4}^{122} n_{T3}^{43} &= n_{X2}^{122} n_{T4}^{43} = n_{X3}^{122} n_{T2}^{43} = n_{X5}^{122} \end{aligned}$$

The lower SG is SG 82 when the preserved operations are: **(sub-SG label is 3) 1, 5, 6, 4.**

$$\text{The transformation is: } (\mathbf{a}_{82}, \mathbf{b}_{82}, \mathbf{c}_{82}) = (\mathbf{a}_{122}, \mathbf{b}_{122}, \mathbf{c}_{122}) \begin{pmatrix} -1 & 0 & 0 \\ 0 & -1 & 0 \\ 0 & 0 & 1 \end{pmatrix}, \overrightarrow{O_{122}O_{82}} = \frac{1}{2}\mathbf{a}_{82} + (-\frac{1}{2})\mathbf{b}_{82}$$

The reduction of higher dimensional irrep:

$$D_{2d} : E \rightarrow {}^2E + {}^1E \text{ of } S_4.$$

The correspondences of irreps at HSPs from original SG to lowered SG:

$$\begin{aligned} n_{GM7}^{82} &= n_{GM8}^{122} n_{GM8}^{82} = n_{GM7}^{122} n_{GM5}^{82} = n_{GM6}^{122} n_{GM6}^{82} = n_{GM7}^{122} n_{M7}^{82} = n_{M7}^{122} n_{M8}^{82} = n_{M6}^{122} n_{M5}^{82} = n_{M6}^{122} n_{M6}^{82} = n_{M7}^{122} n_{X4}^{82} = \\ n_{X3}^{122} + n_{X5}^{122} n_{X3}^{82} &= n_{X2}^{122} + n_{X4}^{122} n_{P7}^{82} = n_{P7}^{122} n_{P8}^{82} = n_{P7}^{122} n_{P5}^{82} = n_{P4}^{122} + n_{P6}^{122} n_{P6}^{82} = n_{P3}^{122} + n_{P5}^{122} n_{N2}^{82} = n_{N3}^{122} + n_{N4}^{122} \end{aligned}$$

### 35. Lowered SGs by higher-dimensional irreps of pairings in SG 123

The representative operations of SG/T for SG 123:

$$\begin{aligned} 1 : (x, y, z), 2 : (-y, x, z), 3 : (y, -x, z), 4 : (x, -y, -z), 5 : (-x, y, -z), 6 : (-x, -y, z), 7 : (y, x, -z), 8 : \\ (-y, -x, -z), 9 : (-x, -y, -z), 10 : (y, -x, -z), 11 : (-y, x, -z), 12 : (-x, y, z), 13 : (x, -y, z), 14 : (x, y, -z), \\ 15 : (-y, -x, z), 16 : (y, x, z). \end{aligned}$$

The lower SG is SG 47 when the preserved operations are: **(sub-SG label is 1) 1, 4, 5, 6, 9, 12, 13, 14.**

$$\text{The transformation is: } (\mathbf{a}_{47}, \mathbf{b}_{47}, \mathbf{c}_{47}) = (\mathbf{a}_{123}, \mathbf{b}_{123}, \mathbf{c}_{123}) \begin{pmatrix} 0 & 0 & 1 \\ 1 & 0 & 0 \\ 0 & 1 & 0 \end{pmatrix}, \overrightarrow{O_{123}O_{47}} = \frac{1}{2}\mathbf{a}_{47} + (\frac{1}{2})\mathbf{c}_{47}$$

The reduction of higher dimensional irrep:

$$D_{4h} : E_g \rightarrow B_{1g} + B_{3g} \text{ of } D_{2h}.$$

$$D_{4h} : E_u \rightarrow B_{1u} + B_{3u} \text{ of } D_{2h}.$$

The correspondences of irreps at HSPs from original SG to lowered SG:

$$\begin{aligned} n_{GM6}^{47} &= n_{GM8}^{123} + n_{GM9}^{123} n_{GM5}^{47} = n_{GM6}^{123} + n_{GM7}^{123} n_{X6}^{47} = n_{X5}^{123} n_{X5}^{47} = n_{X6}^{123} n_{S6}^{47} = n_{R5}^{123} n_{S5}^{47} = n_{R6}^{123} n_{R6}^{47} = n_{A8}^{123} + n_{A9}^{123} n_{R5}^{47} = \\ n_{A6}^{123} + n_{A7}^{123} n_{U6}^{47} &= n_{M8}^{123} + n_{M9}^{123} n_{U5}^{47} = n_{M6}^{123} + n_{M7}^{123} n_{Z6}^{47} = n_{X5}^{123} n_{Z5}^{47} = n_{X6}^{123} n_{T6}^{47} = n_{R5}^{123} n_{T5}^{47} = n_{R6}^{123} n_{Y6}^{47} = n_{Z8}^{123} + n_{Z9}^{123} \\ n_{Y5}^{47} &= n_{Z6}^{123} + n_{Z7}^{123} \end{aligned}$$

The lower SG is SG 65 when the preserved operations are: **(sub-SG label is 2) 1, 6, 7, 8, 9, 14, 15, 16.**

The transformation is:  $(\mathbf{a}_{65}, \mathbf{b}_{65}, \mathbf{c}_{65}) = (\mathbf{a}_{123}, \mathbf{b}_{123}, \mathbf{c}_{123}) \begin{pmatrix} 1 & -1 & 0 \\ 1 & 1 & 0 \\ 0 & 0 & 1 \end{pmatrix}, \overrightarrow{O_{123}O_{65}} = \frac{1}{2}\mathbf{c}_{65}$

The reduction of higher dimensional irrep:

$$D_{4h} : E_g \rightarrow B_{2g} + B_{3g} \text{ of } D_{2h}.$$

$$D_{4h} : E_u \rightarrow B_{2u} + B_{3u} \text{ of } D_{2h}.$$

The correspondences of irreps at HSPs from original SG to lowered SG:

$$\begin{aligned} n_{GM6}^{65} &= n_{GM8}^{123} + n_{GM9}^{123} & n_{GM5}^{65} &= n_{GM6}^{123} + n_{GM7}^{123} & n_{Y6}^{65} &= n_{M8}^{123} + n_{M9}^{123} & n_{Y5}^{65} &= n_{M6}^{123} + n_{M7}^{123} & n_{S6}^{65} &= n_{X6}^{123} & n_{S4}^{65} &= n_{X5}^{123} & n_{S5}^{65} &= n_{R5}^{123} \\ n_{X6}^{123} n_{S3}^{65} &= n_{X5}^{123} n_{Z6}^{65} &= n_{Z6}^{123} + n_{Z7}^{123} & n_{Z5}^{65} &= n_{Z8}^{123} + n_{Z9}^{123} & n_{T6}^{65} &= n_{A6}^{123} + n_{A7}^{123} & n_{T5}^{65} &= n_{A8}^{123} + n_{A9}^{123} & n_{R6}^{65} &= n_{R5}^{123} & n_{R4}^{65} &= n_{R6}^{123} \\ n_{R5}^{65} &= n_{R5}^{123} & n_{R3}^{65} &= n_{R3}^{123} \end{aligned}$$

The lower SG is SG 83 when the preserved operations are: **(sub-SG label is 3) 1, 2, 3, 6, 9, 10, 11, 14.**

The transformation is:  $(\mathbf{a}_{83}, \mathbf{b}_{83}, \mathbf{c}_{83}) = (\mathbf{a}_{123}, \mathbf{b}_{123}, \mathbf{c}_{123}) \begin{pmatrix} -1 & 0 & 0 \\ 0 & -1 & 0 \\ 0 & 0 & 1 \end{pmatrix}, \overrightarrow{O_{123}O_{83}} = \frac{1}{2}\mathbf{c}_{83}$

The reduction of higher dimensional irrep:

$$D_{4h} : E_g \rightarrow {}^2E_g + {}^1E_g \text{ of } C_{4h}.$$

$$D_{4h} : E_u \rightarrow {}^2E_u + {}^1E_u \text{ of } C_{4h}.$$

The correspondences of irreps at HSPs from original SG to lowered SG:

$$\begin{aligned} n_{GM9}^{83} &= n_{GM8}^{123} & n_{GM5}^{83} &= n_{GM6}^{123} & n_{GM11}^{83} &= n_{GM8}^{123} & n_{GM7}^{83} &= n_{GM6}^{123} & n_{GM12}^{83} &= n_{GM9}^{123} & n_{GM8}^{83} &= n_{GM7}^{123} & n_{GM10}^{83} &= n_{GM9}^{123} & n_{GM6}^{83} &= n_{GM8}^{123} \\ n_{GM7}^{83} n_{X6}^{83} &= n_{X6}^{123} n_{X4}^{83} &= n_{X5}^{123} n_{X5}^{83} &= n_{X6}^{123} n_{X3}^{83} &= n_{X5}^{123} n_{M9}^{83} &= n_{M8}^{123} n_{M5}^{83} &= n_{M6}^{123} n_{M11}^{83} &= n_{M8}^{123} n_{M7}^{83} &= n_{M6}^{123} n_{M12}^{83} &= n_{M9}^{123} \\ n_{M8}^{83} &= n_{M7}^{123} n_{M10}^{83} &= n_{M9}^{123} n_{M6}^{83} &= n_{M7}^{123} n_{A9}^{83} &= n_{A6}^{123} n_{A5}^{83} &= n_{A8}^{123} n_{A11}^{83} &= n_{A6}^{123} n_{A7}^{83} &= n_{A8}^{123} n_{A12}^{83} &= n_{A7}^{123} n_{A8}^{83} &= n_{A9}^{123} n_{A10}^{83} \\ n_{A7}^{83} n_{A6}^{83} &= n_{A9}^{123} n_{R6}^{83} &= n_{R5}^{123} n_{R4}^{83} &= n_{R6}^{123} n_{R5}^{83} &= n_{R5}^{123} n_{R3}^{83} &= n_{R6}^{123} n_{Z9}^{83} &= n_{Z6}^{123} n_{Z5}^{83} &= n_{Z8}^{123} n_{Z11}^{83} &= n_{Z6}^{123} n_{Z7}^{83} &= n_{Z8}^{123} n_{Z12}^{83} \\ n_{Z7}^{83} n_{Z8}^{83} &= n_{Z9}^{123} n_{Z10}^{83} &= n_{Z7}^{123} n_{Z6}^{83} &= n_{Z9}^{123} \end{aligned}$$

### 36. Lowered SGs by higher-dimensional irreps of pairings in SG 124

The representative operations of SG/T for SG 124:

$$\begin{aligned} &1 : (x, y, z), 2 : (-y, x, z), 3 : (y, -x, z), 4 : (x, -y, \frac{1}{2} - z), 5 : (-x, y, \frac{1}{2} - z), 6 : (-x, -y, z), 7 : (y, x, \frac{1}{2} - z), \\ &8 : (-y, -x, \frac{1}{2} - z), 9 : (-x, -y, -z), 10 : (y, -x, -z), 11 : (-y, x, -z), 12 : (-x, y, z + \frac{1}{2}), 13 : (x, -y, z + \frac{1}{2}), \\ &14 : (x, y, -z), 15 : (-y, -x, z + \frac{1}{2}), 16 : (y, x, z + \frac{1}{2}). \end{aligned}$$

The lower SG is SG 49 when the preserved operations are: **(sub-SG label is 1) 1, 4, 5, 6, 9, 12, 13, 14.**

The transformation is:  $(\mathbf{a}_{49}, \mathbf{b}_{49}, \mathbf{c}_{49}) = (\mathbf{a}_{124}, \mathbf{b}_{124}, \mathbf{c}_{124}) \begin{pmatrix} 1 & 0 & 0 \\ 0 & 1 & 0 \\ 0 & 0 & 1 \end{pmatrix}, \overrightarrow{O_{124}O_{49}} = \frac{1}{2}\mathbf{a}_{49} + (\frac{1}{2})\mathbf{c}_{49}$

The reduction of higher dimensional irrep:

$$D_{4h} : E_g \rightarrow B_{2g} + B_{3g} \text{ of } D_{2h}.$$

$$D_{4h} : E_u \rightarrow B_{2u} + B_{3u} \text{ of } D_{2h}.$$

The correspondences of irreps at HSPs from original SG to lowered SG:

$$\begin{aligned} n_{GM6}^{49} &= n_{GM8}^{124} + n_{GM9}^{124} & n_{GM5}^{49} &= n_{GM6}^{124} + n_{GM7}^{124} & n_{X6}^{49} &= n_{X5}^{124} n_{X5}^{49} &= n_{X6}^{124} n_{S6}^{49} &= n_{M6}^{124} + n_{M7}^{124} & n_{S5}^{49} &= n_{M8}^{124} + n_{M9}^{124} & n_{R4}^{49} &= n_{R4}^{124} \\ n_{A5}^{124} + n_{A6}^{124} n_{R3}^{49} &= n_{A7}^{124} + n_{A8}^{124} & n_{U4}^{49} &= n_{R3}^{124} n_{U3}^{49} &= n_{R4}^{124} n_{Z4}^{49} &= n_{Z5}^{124} + n_{Z6}^{124} & n_{Z3}^{49} &= n_{Z7}^{124} + n_{Z8}^{124} & n_{T4}^{49} &= n_{R3}^{124} n_{T3}^{49} &= n_{R4}^{124} \\ n_{Y6}^{49} &= n_{X6}^{124} n_{Y5}^{49} &= n_{X5}^{124} \end{aligned}$$

The lower SG is SG 66 when the preserved operations are: **(sub-SG label is 2) 1, 6, 7, 8, 9, 14, 15, 16.**

The transformation is:  $(\mathbf{a}_{66}, \mathbf{b}_{66}, \mathbf{c}_{66}) = (\mathbf{a}_{124}, \mathbf{b}_{124}, \mathbf{c}_{124}) \begin{pmatrix} 1 & -1 & 0 \\ 1 & 1 & 0 \\ 0 & 0 & 1 \end{pmatrix}, \overrightarrow{O_{124}O_{66}} = \frac{1}{2}\mathbf{c}_{66}$

The reduction of higher dimensional irrep:

$$D_{4h} : E_g \rightarrow B_{2g} + B_{3g} \text{ of } D_{2h}.$$

$$D_{4h} : E_u \rightarrow B_{2u} + B_{3u} \text{ of } D_{2h}.$$

The correspondences of irreps at HSPs from original SG to lowered SG:

$$\begin{aligned} n_{GM6}^{66} &= n_{GM8}^{124} + n_{GM9}^{124} & n_{GM5}^{66} &= n_{GM6}^{124} + n_{GM7}^{124} & n_{Y6}^{66} &= n_{M8}^{124} + n_{M9}^{124} & n_{Y5}^{66} &= n_{M6}^{124} + n_{M7}^{124} & n_{S6}^{66} &= n_{X6}^{124} & n_{S4}^{66} &= n_{X5}^{124} & n_{S5}^{66} &= n_{X5}^{124} & n_{S5}^{66} &= n_{R3}^{124} \\ n_{X6}^{124} n_{S3}^{66} &= n_{X5}^{124} n_{Z4}^{66} & n_{Z5}^{124} &+ n_{Z6}^{124} & n_{Z3}^{66} &= n_{Z7}^{124} &+ n_{Z8}^{124} & n_{T4}^{66} &= n_{A5}^{124} &+ n_{A6}^{124} & n_{T3}^{66} &= n_{A7}^{124} &+ n_{A8}^{124} & n_{R6}^{66} &= n_{R4}^{124} & n_{R4}^{66} &= n_{R3}^{124} \\ n_{R5}^{66} &= n_{R3}^{124} & n_{R3}^{66} &= n_{R4}^{124} \end{aligned}$$

The lower SG is SG 83 when the preserved operations are: **(sub-SG label is 3) 1, 2, 3, 6, 9, 10, 11, 14.**

The transformation is:  $(\mathbf{a}_{83}, \mathbf{b}_{83}, \mathbf{c}_{83}) = (\mathbf{a}_{124}, \mathbf{b}_{124}, \mathbf{c}_{124}) \begin{pmatrix} -1 & 0 & 0 \\ 0 & -1 & 0 \\ 0 & 0 & 1 \end{pmatrix}, \overrightarrow{O_{124}O_{83}} = \frac{1}{2}\mathbf{c}_{83}$

The reduction of higher dimensional irrep:

$$D_{4h} : E_g \rightarrow {}^2E_g + {}^1E_g \text{ of } C_{4h}.$$

$$D_{4h} : E_u \rightarrow {}^2E_u + {}^1E_u \text{ of } C_{4h}.$$

The correspondences of irreps at HSPs from original SG to lowered SG:

$$\begin{aligned} n_{GM9}^{83} &= n_{GM8}^{124} & n_{GM5}^{83} &= n_{GM6}^{124} & n_{GM11}^{83} &= n_{GM8}^{124} & n_{GM7}^{83} &= n_{GM6}^{124} & n_{GM12}^{83} &= n_{GM9}^{124} & n_{GM8}^{83} &= n_{GM7}^{124} & n_{GM10}^{83} &= n_{GM9}^{124} & n_{GM6}^{83} &= n_{GM7}^{124} \\ n_{GM7}^{124} n_{X6}^{83} &= n_{X6}^{124} n_{X4}^{83} & n_{X4}^{83} &= n_{X5}^{124} & n_{X5}^{83} &= n_{X6}^{124} & n_{X3}^{83} &= n_{X5}^{124} & n_{M9}^{83} &= n_{M8}^{124} & n_{M5}^{83} &= n_{M6}^{124} & n_{M11}^{83} &= n_{M8}^{124} & n_{M7}^{83} &= n_{M6}^{124} & n_{M12}^{83} &= n_{M9}^{124} \\ n_{M8}^{83} &= n_{M7}^{124} & n_{M10}^{83} &= n_{M9}^{124} & n_{M6}^{83} &= n_{M7}^{124} & n_{A9}^{83} &= n_{A5}^{124} & n_{A5}^{83} &= n_{A7}^{124} & n_{A11}^{83} &= n_{A7}^{124} & n_{A7}^{83} &= n_{A5}^{124} & n_{A12}^{83} &= n_{A8}^{124} & n_{A8}^{83} &= n_{A6}^{124} & n_{A10}^{83} &= n_{A6}^{124} \\ n_{A6}^{124} n_{A6}^{83} &= n_{A8}^{124} n_{R6}^{83} & n_{R4}^{83} &= n_{R4}^{124} & n_{R4}^{83} &= n_{R3}^{124} & n_{R5}^{83} &= n_{R3}^{124} & n_{R3}^{83} &= n_{R4}^{124} & n_{Z9}^{83} &= n_{Z5}^{124} & n_{Z5}^{83} &= n_{Z7}^{124} & n_{Z11}^{83} &= n_{Z7}^{124} & n_{Z7}^{83} &= n_{Z5}^{124} & n_{Z12}^{83} &= n_{Z5}^{124} \\ n_{Z8}^{124} n_{Z8}^{83} &= n_{Z6}^{124} n_{Z10}^{83} & n_{Z6}^{124} n_{Z6}^{83} &= n_{Z8}^{124} \end{aligned}$$

### 37. Lowered SGs by higher-dimensional irreps of pairings in SG 125

The representative operations of SG/T for SG 125:

$$\begin{aligned} 1 : (x, y, z), & 2 : (\frac{1}{2} - y, x, z), & 3 : (y, \frac{1}{2} - x, z), & 4 : (x, \frac{1}{2} - y, -z), & 5 : (\frac{1}{2} - x, y, -z), & 6 : (\frac{1}{2} - x, \frac{1}{2} - y, z), & 7 : (y, x, -z), \\ 8 : (\frac{1}{2} - y, \frac{1}{2} - x, -z), & 9 : (-x, -y, -z), & 10 : (y + \frac{1}{2}, -x, -z), & 11 : (-y, x + \frac{1}{2}, -z), & 12 : (-x, y + \frac{1}{2}, z), & 13 : (x + \frac{1}{2}, -y, z), \\ 14 : (x + \frac{1}{2}, y + \frac{1}{2}, -z), & 15 : (-y, -x, z), & 16 : (y + \frac{1}{2}, x + \frac{1}{2}, z). \end{aligned}$$

The lower SG is SG 50 when the preserved operations are: **(sub-SG label is 1) 1, 4, 5, 6, 9, 12, 13, 14.**

The transformation is:  $(\mathbf{a}_{50}, \mathbf{b}_{50}, \mathbf{c}_{50}) = (\mathbf{a}_{125}, \mathbf{b}_{125}, \mathbf{c}_{125}) \begin{pmatrix} 1 & 0 & 0 \\ 0 & 1 & 0 \\ 0 & 0 & 1 \end{pmatrix}, \overrightarrow{O_{125}O_{50}} = \frac{1}{2}\mathbf{a}_{50} + (\frac{1}{2})\mathbf{b}_{50} + (\frac{1}{2})\mathbf{c}_{50}$

The reduction of higher dimensional irrep:

$$D_{4h} : E_g \rightarrow B_{2g} + B_{3g} \text{ of } D_{2h}.$$

$$D_{4h} : E_u \rightarrow B_{2u} + B_{3u} \text{ of } D_{2h}.$$

The correspondences of irreps at HSPs from original SG to lowered SG:

$$\begin{aligned} n_{GM6}^{50} &= n_{GM8}^{125} + n_{GM9}^{125} & n_{GM5}^{50} &= n_{GM6}^{125} + n_{GM7}^{125} & n_{X4}^{50} &= n_{X3}^{125} & n_{X3}^{50} &= n_{X4}^{125} & n_{S3}^{50} &= n_{M5}^{125} & n_{S4}^{50} &= n_{M5}^{125} & n_{R3}^{50} &= n_{A5}^{125} & n_{R4}^{50} &= n_{A5}^{125} \\ n_{U4}^{50} &= n_{R3}^{125} & n_{U3}^{50} &= n_{R4}^{125} & n_{Z6}^{50} &= n_{Z6}^{125} &+ n_{Z7}^{125} & n_{Z5}^{50} &= n_{Z8}^{125} &+ n_{Z9}^{125} & n_{T4}^{50} &= n_{R3}^{125} & n_{T3}^{50} &= n_{R4}^{125} & n_{Y4}^{50} &= n_{X3}^{125} & n_{Y3}^{50} &= n_{X4}^{125} \end{aligned}$$

The lower SG is SG 67 when the preserved operations are: **(sub-SG label is 2) 1, 6, 7, 8, 9, 14, 15, 16.**

The transformation is:  $(\mathbf{a}_{67}, \mathbf{b}_{67}, \mathbf{c}_{67}) = (\mathbf{a}_{125}, \mathbf{b}_{125}, \mathbf{c}_{125}) \begin{pmatrix} 1 & -1 & 0 \\ 1 & 1 & 0 \\ 0 & 0 & 1 \end{pmatrix}, \overrightarrow{O_{125}O_{67}} = \frac{1}{2}\mathbf{a}_{67} + (\frac{1}{2})\mathbf{b}_{67} + (\frac{1}{2})\mathbf{c}_{67}$

The reduction of higher dimensional irrep:

$$D_{4h} : E_g \rightarrow B_{2g} + B_{3g} \text{ of } D_{2h}.$$

$$D_{4h} : E_u \rightarrow B_{2u} + B_{3u} \text{ of } D_{2h}.$$

The correspondences of irreps at HSPs from original SG to lowered SG:

$$\begin{aligned} n_{GM6}^{67} &= n_{GM8}^{125} + n_{GM9}^{125} & n_{GM5}^{67} &= n_{GM6}^{125} + n_{GM7}^{125} & n_{Y6}^{67} &= n_{M5}^{125} & n_{Y5}^{67} &= n_{M5}^{125} & n_{S2}^{67} &= n_{X3}^{125} + n_{X4}^{125} & n_{Z6}^{67} &= n_{Z6}^{125} + n_{Z7}^{125} & n_{Z5}^{67} &= n_{Z6}^{125} \\ n_{Z8}^{125} + n_{Z9}^{125} & n_{T6}^{67} &= n_{A5}^{125} & n_{T5}^{67} &= n_{A5}^{125} & n_{R2}^{67} &= n_{R3}^{125} + n_{R4}^{125} \end{aligned}$$

The lower SG is SG 85 when the preserved operations are: **(sub-SG label is 3) 1, 2, 3, 6, 9, 10, 11, 14.**

The transformation is:  $(\mathbf{a}_{85}, \mathbf{b}_{85}, \mathbf{c}_{85}) = (\mathbf{a}_{125}, \mathbf{b}_{125}, \mathbf{c}_{125}) \begin{pmatrix} -1 & 0 & 0 \\ 0 & 1 & 0 \\ 0 & 0 & -1 \end{pmatrix}, \overrightarrow{O_{125}O_{85}} = \frac{1}{2}\mathbf{b}_{85} + (\frac{1}{2})\mathbf{c}_{85}$

The reduction of higher dimensional irrep:

$$D_{4h} : E_g \rightarrow {}^2E_g + {}^1E_g \text{ of } C_{4h}.$$

$$D_{4h} : E_u \rightarrow {}^2E_u + {}^1E_u \text{ of } C_{4h}.$$

The correspondences of irreps at HSPs from original SG to lowered SG:

$$\begin{aligned} n_{GM9}^{85} &= n_{GM8}^{125} n_{GM5}^{85} = n_{GM6}^{125} n_{GM11}^{85} = n_{GM8}^{125} n_{GM7}^{85} = n_{GM6}^{125} n_{GM12}^{85} = n_{GM9}^{125} n_{GM8}^{85} = n_{GM7}^{125} n_{GM10}^{85} = n_{GM9}^{125} n_{GM6}^{85} = \\ n_{GM7}^{125} n_{X2}^{85} &= n_{X3}^{125} + n_{X4}^{125} n_{M3}^{85} = n_{M5}^{125} n_{M4}^{85} = n_{M5}^{125} n_{A3}^{85} = n_{A5}^{125} n_{A4}^{85} = n_{A5}^{125} n_{R2}^{85} = n_{R3}^{125} + n_{R4}^{125} n_{Z9}^{85} = n_{Z6}^{125} n_{Z5}^{85} = n_{Z8}^{125} \\ n_{Z11}^{85} &= n_{Z6}^{125} n_{Z7}^{85} = n_{Z8}^{125} n_{Z12}^{85} = n_{Z7}^{125} n_{Z8}^{85} = n_{Z9}^{125} n_{Z10}^{85} = n_{Z7}^{125} n_{Z6}^{85} = n_{Z9}^{125} \end{aligned}$$

### 38. Lowered SGs by higher-dimensional irreps of pairings in SG 126

The representative operations of SG/T for SG 126:

$$\begin{aligned} 1 : (x, y, z), 2 : (\frac{1}{2}-y, x, z), 3 : (y, \frac{1}{2}-x, z), 4 : (x, \frac{1}{2}-y, \frac{1}{2}-z), 5 : (\frac{1}{2}-x, y, \frac{1}{2}-z), 6 : (\frac{1}{2}-x, \frac{1}{2}-y, z), 7 : (y, x, \frac{1}{2}-z), \\ 8 : (\frac{1}{2}-y, \frac{1}{2}-x, \frac{1}{2}-z), 9 : (-x, -y, -z), 10 : (y + \frac{1}{2}, -x, -z), 11 : (-y, x + \frac{1}{2}, -z), 12 : (-x, y + \frac{1}{2}, z + \frac{1}{2}), \\ 13 : (x + \frac{1}{2}, -y, z + \frac{1}{2}), 14 : (x + \frac{1}{2}, y + \frac{1}{2}, -z), 15 : (-y, -x, z + \frac{1}{2}), 16 : (y + \frac{1}{2}, x + \frac{1}{2}, z + \frac{1}{2}). \end{aligned}$$

The lower SG is SG 48 when the preserved operations are: (**sub-SG label is 1**) 1, 4, 5, 6, 9, 12, 13, 14.

$$\text{The transformation is: } (\mathbf{a}_{48}, \mathbf{b}_{48}, \mathbf{c}_{48}) = (\mathbf{a}_{126}, \mathbf{b}_{126}, \mathbf{c}_{126}) \begin{pmatrix} 0 & 0 & 1 \\ 1 & 0 & 0 \\ 0 & 1 & 0 \end{pmatrix}, \overrightarrow{O_{126}O_{48}} = \frac{1}{2}\mathbf{a}_{48}$$

The reduction of higher dimensional irrep:

$$D_{4h} : E_g \rightarrow B_{1g} + B_{3g} \text{ of } D_{2h}.$$

$$D_{4h} : E_u \rightarrow B_{1u} + B_{3u} \text{ of } D_{2h}.$$

The correspondences of irreps at HSPs from original SG to lowered SG:

$$\begin{aligned} n_{GM6}^{48} &= n_{GM8}^{126} + n_{GM9}^{126} n_{GM5}^{48} = n_{GM6}^{126} + n_{GM7}^{126} n_{X4}^{48} = n_{X3}^{126} n_{X3}^{48} = n_{X4}^{126} n_{S3}^{48} = n_{R3}^{126} n_{S4}^{48} = n_{R4}^{126} n_{R6}^{48} = n_{A5}^{126} n_{R5}^{48} = n_{A5}^{126} \\ n_{U3}^{48} &= n_{M5}^{126} n_{U4}^{48} = n_{M5}^{126} n_{Z4}^{48} = n_{X4}^{126} n_{Z3}^{48} = n_{X3}^{126} n_{T4}^{48} = n_{R3}^{126} n_{T3}^{48} = n_{R4}^{126} n_{Y4}^{48} = n_{Z7}^{126} + n_{Z8}^{126} n_{Y3}^{48} = n_{Z5}^{126} + n_{Z6}^{126} \end{aligned}$$

The lower SG is SG 68 when the preserved operations are: (**sub-SG label is 2**) 1, 6, 7, 8, 9, 14, 15, 16.

$$\text{The transformation is: } (\mathbf{a}_{68}, \mathbf{b}_{68}, \mathbf{c}_{68}) = (\mathbf{a}_{126}, \mathbf{b}_{126}, \mathbf{c}_{126}) \begin{pmatrix} 1 & -1 & 0 \\ 1 & 1 & 0 \\ 0 & 0 & 1 \end{pmatrix}, \overrightarrow{O_{126}O_{68}} = -\frac{1}{4}\mathbf{a}_{68} + (\frac{3}{4})\mathbf{b}_{68} + (\frac{1}{2})\mathbf{c}_{68}$$

The reduction of higher dimensional irrep:

$$D_{4h} : E_g \rightarrow B_{2g} + B_{3g} \text{ of } D_{2h}.$$

$$D_{4h} : E_u \rightarrow B_{2u} + B_{3u} \text{ of } D_{2h}.$$

The correspondences of irreps at HSPs from original SG to lowered SG:

$$\begin{aligned} n_{GM6}^{68} &= n_{GM8}^{126} + n_{GM9}^{126} n_{GM5}^{68} = n_{GM6}^{126} + n_{GM7}^{126} n_{Y6}^{68} = n_{M5}^{126} n_{Y5}^{68} = n_{M5}^{126} n_{S2}^{68} = n_{X3}^{126} + n_{X4}^{126} n_{Z4}^{68} = n_{Z5}^{126} + n_{Z6}^{126} n_{Z3}^{68} = \\ n_{Z7}^{126} + n_{Z8}^{126} n_{T4}^{68} &= n_{A5}^{126} n_{T3}^{68} = n_{A5}^{126} n_{R2}^{68} = n_{R3}^{126} + n_{R4}^{126} \end{aligned}$$

The lower SG is SG 85 when the preserved operations are: (**sub-SG label is 3**) 1, 2, 3, 6, 9, 10, 11, 14.

$$\text{The transformation is: } (\mathbf{a}_{85}, \mathbf{b}_{85}, \mathbf{c}_{85}) = (\mathbf{a}_{126}, \mathbf{b}_{126}, \mathbf{c}_{126}) \begin{pmatrix} -1 & 0 & 0 \\ 0 & 1 & 0 \\ 0 & 0 & -1 \end{pmatrix}, \overrightarrow{O_{126}O_{85}} = \frac{1}{2}\mathbf{a}_{85} + (\frac{1}{2})\mathbf{c}_{85}$$

The reduction of higher dimensional irrep:

$$D_{4h} : E_g \rightarrow {}^2E_g + {}^1E_g \text{ of } C_{4h}.$$

$$D_{4h} : E_u \rightarrow {}^2E_u + {}^1E_u \text{ of } C_{4h}.$$

The correspondences of irreps at HSPs from original SG to lowered SG:

$$\begin{aligned} n_{GM9}^{85} &= n_{GM8}^{126} n_{GM5}^{85} = n_{GM6}^{126} n_{GM11}^{85} = n_{GM8}^{126} n_{GM7}^{85} = n_{GM6}^{126} n_{GM12}^{85} = n_{GM9}^{126} n_{GM8}^{85} = n_{GM7}^{126} n_{GM10}^{85} = n_{GM9}^{126} n_{GM6}^{85} = \\ n_{GM7}^{126} n_{X2}^{85} &= n_{X3}^{126} + n_{X4}^{126} n_{M3}^{85} = n_{M5}^{126} n_{M4}^{85} = n_{M5}^{126} n_{A3}^{85} = n_{A5}^{126} n_{A4}^{85} = n_{A5}^{126} n_{R2}^{85} = n_{R3}^{126} + n_{R4}^{126} n_{Z9}^{85} = n_{Z7}^{126} n_{Z5}^{85} = n_{Z8}^{126} \\ n_{Z11}^{85} &= n_{Z5}^{126} n_{Z7}^{85} = n_{Z7}^{126} n_{Z12}^{85} = n_{Z6}^{126} n_{Z8}^{85} = n_{Z8}^{126} n_{Z10}^{85} = n_{Z8}^{126} n_{Z6}^{85} = n_{Z6}^{126} \end{aligned}$$

### 39. Lowered SGs by higher-dimensional irreps of pairings in SG 127

The representative operations of SG/T for SG 127:

$$1 : (x, y, z), 2 : (-y, x, z), 3 : (y, -x, z), 4 : (x + \frac{1}{2}, \frac{1}{2} - y, -z), 5 : (\frac{1}{2} - x, y + \frac{1}{2}, -z), 6 : (-x, -y, z), 7 : (y + \frac{1}{2}, x + \frac{1}{2}, -z), 8 : (\frac{1}{2} - y, \frac{1}{2} - x, -z), 9 : (-x, -y, -z), 10 : (y, -x, -z), 11 : (-y, x, -z), 12 : (\frac{1}{2} - x, y + \frac{1}{2}, z), 13 : (x + \frac{1}{2}, \frac{1}{2} - y, z), 14 : (x, y, -z), 15 : (\frac{1}{2} - y, \frac{1}{2} - x, z), 16 : (y + \frac{1}{2}, x + \frac{1}{2}, z).$$

The lower SG is SG 55 when the preserved operations are: **(sub-SG label is 1) 1, 4, 5, 6, 9, 12, 13, 14.**

$$\text{The transformation is: } (\mathbf{a}_{55}, \mathbf{b}_{55}, \mathbf{c}_{55}) = (\mathbf{a}_{127}, \mathbf{b}_{127}, \mathbf{c}_{127}) \begin{pmatrix} 1 & 0 & 0 \\ 0 & 1 & 0 \\ 0 & 0 & 1 \end{pmatrix}, \overrightarrow{O_{127}O_{55}} = \frac{1}{2}\mathbf{c}_{55}$$

The reduction of higher dimensional irrep:

$$D_{4h} : E_g \rightarrow B_{2g} + B_{3g} \text{ of } D_{2h}.$$

$$D_{4h} : E_u \rightarrow B_{2u} + B_{3u} \text{ of } D_{2h}.$$

The correspondences of irreps at HSPs from original SG to lowered SG:

$$\begin{aligned} n_{GM6}^{55} &= n_{GM8}^{127} + n_{GM9}^{127} & n_{GM5}^{55} &= n_{GM6}^{127} + n_{GM7}^{127} & n_{X4}^{55} &= n_{X4}^{127} & n_{X3}^{55} &= n_{X3}^{127} & n_{S6}^{55} &= n_{M8}^{127} + n_{M9}^{127} & n_{S5}^{55} &= n_{M6}^{127} + n_{M7}^{127} & n_{R6}^{55} &= n_{R3}^{127} \\ n_{A6}^{127} + n_{A7}^{127} & n_{B5}^{127} &= n_{A8}^{127} + n_{A9}^{127} & n_{U4}^{55} &= n_{R4}^{127} & n_{U3}^{55} &= n_{R3}^{127} & n_{Z6}^{55} &= n_{Z6}^{127} + n_{Z7}^{127} & n_{Z5}^{55} &= n_{Z8}^{127} + n_{Z9}^{127} & n_{T4}^{55} &= n_{R4}^{127} & n_{T3}^{55} &= n_{R3}^{127} \\ n_{Y4}^{55} &= n_{X4}^{127} & n_{Y3}^{55} &= n_{X3}^{127} \end{aligned}$$

The lower SG is SG 65 when the preserved operations are: **(sub-SG label is 2) 1, 6, 7, 8, 9, 14, 15, 16.**

$$\text{The transformation is: } (\mathbf{a}_{65}, \mathbf{b}_{65}, \mathbf{c}_{65}) = (\mathbf{a}_{127}, \mathbf{b}_{127}, \mathbf{c}_{127}) \begin{pmatrix} 1 & -1 & 0 \\ 1 & 1 & 0 \\ 0 & 0 & 1 \end{pmatrix}, \overrightarrow{O_{127}O_{65}} = -\frac{1}{4}\mathbf{a}_{65} + (\frac{1}{4})\mathbf{b}_{65} + (\frac{1}{2})\mathbf{c}_{65}$$

The reduction of higher dimensional irrep:

$$D_{4h} : E_g \rightarrow B_{2g} + B_{3g} \text{ of } D_{2h}.$$

$$D_{4h} : E_u \rightarrow B_{2u} + B_{3u} \text{ of } D_{2h}.$$

The correspondences of irreps at HSPs from original SG to lowered SG:

$$\begin{aligned} n_{GM6}^{65} &= n_{GM8}^{127} + n_{GM9}^{127} & n_{GM5}^{65} &= n_{GM6}^{127} + n_{GM7}^{127} & n_{Y6}^{65} &= n_{M6}^{127} + n_{M7}^{127} & n_{Y5}^{65} &= n_{M8}^{127} + n_{M9}^{127} & n_{S6}^{65} &= n_{X4}^{127} & n_{S4}^{65} &= n_{X4}^{127} & n_{S5}^{65} &= n_{X5}^{127} \\ n_{X3}^{127} & n_{S3}^{65} &= n_{X3}^{127} & n_{Z6}^{65} &= n_{Z6}^{127} + n_{Z7}^{127} & n_{Z5}^{65} &= n_{Z8}^{127} + n_{Z9}^{127} & n_{T6}^{65} &= n_{A8}^{127} + n_{A9}^{127} & n_{T5}^{65} &= n_{A6}^{127} + n_{A7}^{127} & n_{R6}^{65} &= n_{R4}^{127} & n_{R4}^{65} &= n_{R4}^{127} \\ n_{R5}^{65} &= n_{R3}^{127} & n_{R3}^{65} &= n_{R3}^{127} \end{aligned}$$

The lower SG is SG 83 when the preserved operations are: **(sub-SG label is 3) 1, 2, 3, 6, 9, 10, 11, 14.**

$$\text{The transformation is: } (\mathbf{a}_{83}, \mathbf{b}_{83}, \mathbf{c}_{83}) = (\mathbf{a}_{127}, \mathbf{b}_{127}, \mathbf{c}_{127}) \begin{pmatrix} -1 & 0 & 0 \\ 0 & -1 & 0 \\ 0 & 0 & 1 \end{pmatrix}, \overrightarrow{O_{127}O_{83}} = \frac{1}{2}\mathbf{a}_{83} + (\frac{1}{2})\mathbf{b}_{83} + (\frac{1}{2})\mathbf{c}_{83}$$

The reduction of higher dimensional irrep:

$$D_{4h} : E_g \rightarrow {}^2E_g + {}^1E_g \text{ of } C_{4h}.$$

$$D_{4h} : E_u \rightarrow {}^2E_u + {}^1E_u \text{ of } C_{4h}.$$

The correspondences of irreps at HSPs from original SG to lowered SG:

$$\begin{aligned} n_{GM9}^{83} &= n_{GM8}^{127} & n_{GM5}^{83} &= n_{GM6}^{127} & n_{GM11}^{83} &= n_{GM8}^{127} & n_{GM7}^{83} &= n_{GM6}^{127} & n_{GM12}^{83} &= n_{GM9}^{127} & n_{GM8}^{83} &= n_{GM7}^{127} & n_{GM10}^{83} &= n_{GM9}^{127} & n_{GM6}^{83} &= n_{GM7}^{127} \\ n_{X6}^{83} &= n_{X3}^{127} & n_{X4}^{83} &= n_{X3}^{127} & n_{X5}^{83} &= n_{X4}^{127} & n_{X3}^{83} &= n_{X4}^{127} & n_{M9}^{83} &= n_{M9}^{127} & n_{M5}^{83} &= n_{M7}^{127} & n_{M11}^{83} &= n_{M8}^{127} & n_{M7}^{83} &= n_{M6}^{127} & n_{M12}^{83} &= n_{M9}^{127} \\ n_{M8}^{83} &= n_{M7}^{127} & n_{M10}^{83} &= n_{M8}^{127} & n_{M6}^{83} &= n_{M6}^{127} & n_{A9}^{83} &= n_{A7}^{127} & n_{A5}^{83} &= n_{A9}^{127} & n_{A11}^{83} &= n_{A6}^{127} & n_{A7}^{83} &= n_{A8}^{127} & n_{A12}^{83} &= n_{A7}^{127} & n_{A8}^{83} &= n_{A9}^{127} & n_{A10}^{83} &= n_{A9}^{127} \\ n_{A6}^{127} & n_{A6}^{83} &= n_{A8}^{127} & n_{R6}^{83} &= n_{R3}^{127} & n_{R4}^{83} &= n_{R3}^{127} & n_{R5}^{83} &= n_{R4}^{127} & n_{R3}^{83} &= n_{R4}^{127} & n_{Z9}^{83} &= n_{Z6}^{127} & n_{Z5}^{83} &= n_{Z8}^{127} & n_{Z11}^{83} &= n_{Z6}^{127} & n_{Z7}^{83} &= n_{Z8}^{127} & n_{Z12}^{83} &= n_{Z9}^{127} \\ n_{Z7}^{83} & n_{Z8}^{83} &= n_{Z9}^{127} & n_{Z10}^{83} &= n_{Z7}^{127} & n_{Z6}^{83} &= n_{Z9}^{127} \end{aligned}$$

### 40. Lowered SGs by higher-dimensional irreps of pairings in SG 128

The representative operations of SG/T for SG 128:

$$1 : (x, y, z), 2 : (-y, x, z), 3 : (y, -x, z), 4 : (x + \frac{1}{2}, \frac{1}{2} - y, \frac{1}{2} - z), 5 : (\frac{1}{2} - x, y + \frac{1}{2}, \frac{1}{2} - z), 6 : (-x, -y, z), 7 : (y + \frac{1}{2}, x + \frac{1}{2}, \frac{1}{2} - z), 8 : (\frac{1}{2} - y, \frac{1}{2} - x, \frac{1}{2} - z), 9 : (-x, -y, -z), 10 : (y, -x, -z), 11 : (-y, x, -z), 12 : (\frac{1}{2} - x, y + \frac{1}{2}, z + \frac{1}{2}), 13 : (x + \frac{1}{2}, \frac{1}{2} - y, z + \frac{1}{2}), 14 : (x, y, -z), 15 : (\frac{1}{2} - y, \frac{1}{2} - x, z + \frac{1}{2}), 16 : (y + \frac{1}{2}, x + \frac{1}{2}, z + \frac{1}{2}).$$

The lower SG is SG 58 when the preserved operations are: **(sub-SG label is 1) 1, 4, 5, 6, 9, 12, 13, 14.**

The transformation is:  $(\mathbf{a}_{58}, \mathbf{b}_{58}, \mathbf{c}_{58}) = (\mathbf{a}_{128}, \mathbf{b}_{128}, \mathbf{c}_{128}) \begin{pmatrix} 1 & 0 & 0 \\ 0 & 1 & 0 \\ 0 & 0 & 1 \end{pmatrix}, \overrightarrow{O_{128}O_{58}} = \mathbf{0}$

The reduction of higher dimensional irrep:

$$D_{4h} : E_g \rightarrow B_{2g} + B_{3g} \text{ of } D_{2h}.$$

$$D_{4h} : E_u \rightarrow B_{2u} + B_{3u} \text{ of } D_{2h}.$$

The correspondences of irreps at HSPs from original SG to lowered SG:

$$\begin{aligned} n_{GM6}^{58} &= n_{GM8}^{128} + n_{GM9}^{128} & n_{GM5}^{58} &= n_{GM6}^{128} + n_{GM7}^{128} & n_{X4}^{58} &= n_{X4}^{128} & n_{X3}^{58} &= n_{X3}^{128} & n_{S6}^{58} &= n_{M8}^{128} + n_{M9}^{128} & n_{S5}^{58} &= n_{M6}^{128} + n_{M7}^{128} & n_{R4}^{58} &= n_{R3}^{128} + n_{R5}^{128} \\ n_{A7}^{128} + n_{A8}^{128} & n_{R3}^{58} &= n_{A5}^{128} + n_{A6}^{128} & n_{U7}^{58} &= n_{R9}^{128} & n_{U3}^{58} &= n_{R5}^{128} & n_{U6}^{58} &= n_{R6}^{128} & n_{U2}^{58} &= n_{R2}^{128} & n_{U8}^{58} &= n_{R8}^{128} & n_{U4}^{58} &= n_{R4}^{128} & n_{U9}^{58} &= n_{R7}^{128} & n_{U5}^{58} &= n_{R7}^{128} & n_{U5}^{58} &= n_{R7}^{128} \\ n_{R3}^{128} & n_{Z4}^{58} &= n_{Z7}^{128} + n_{Z8}^{128} & n_{Z3}^{58} &= n_{Z5}^{128} + n_{Z6}^{128} & n_{T8}^{58} &= n_{R8}^{128} & n_{T4}^{58} &= n_{R4}^{128} & n_{T9}^{58} &= n_{R9}^{128} & n_{T5}^{58} &= n_{R5}^{128} & n_{T7}^{58} &= n_{R7}^{128} & n_{T3}^{58} &= n_{R3}^{128} & n_{T6}^{58} &= n_{R6}^{128} \\ n_{R6}^{128} & n_{T2}^{58} &= n_{R2}^{128} & n_{Y4}^{58} &= n_{X4}^{128} & n_{Y3}^{58} &= n_{X3}^{128} \end{aligned}$$

The lower SG is SG 66 when the preserved operations are: **(sub-SG label is 2) 1, 6, 7, 8, 9, 14, 15, 16.**

The transformation is:  $(\mathbf{a}_{66}, \mathbf{b}_{66}, \mathbf{c}_{66}) = (\mathbf{a}_{128}, \mathbf{b}_{128}, \mathbf{c}_{128}) \begin{pmatrix} 1 & -1 & 0 \\ 1 & 1 & 0 \\ 0 & 0 & 1 \end{pmatrix}, \overrightarrow{O_{128}O_{66}} = -\frac{1}{4}\mathbf{a}_{66} + (\frac{1}{4})\mathbf{b}_{66} + (\frac{1}{2})\mathbf{c}_{66}$

The reduction of higher dimensional irrep:

$$D_{4h} : E_g \rightarrow B_{2g} + B_{3g} \text{ of } D_{2h}.$$

$$D_{4h} : E_u \rightarrow B_{2u} + B_{3u} \text{ of } D_{2h}.$$

The correspondences of irreps at HSPs from original SG to lowered SG:

$$\begin{aligned} n_{GM6}^{66} &= n_{GM8}^{128} + n_{GM9}^{128} & n_{GM5}^{66} &= n_{GM6}^{128} + n_{GM7}^{128} & n_{Y6}^{66} &= n_{M6}^{128} + n_{M7}^{128} & n_{Y5}^{66} &= n_{M8}^{128} + n_{M9}^{128} & n_{S6}^{66} &= n_{X4}^{128} & n_{S4}^{66} &= n_{X4}^{128} & n_{S5}^{66} &= n_{X4}^{128} & n_{S5}^{66} &= n_{X4}^{128} \\ n_{X3}^{128} & n_{S3}^{66} &= n_{X3}^{128} & n_{Z4}^{66} &= n_{Z5}^{128} + n_{Z6}^{128} & n_{Z3}^{66} &= n_{Z7}^{128} + n_{Z8}^{128} & n_{T4}^{66} &= n_{A5}^{128} + n_{A6}^{128} & n_{T3}^{66} &= n_{A7}^{128} + n_{A8}^{128} & n_{R6}^{66} &= n_{R3}^{128} + n_{R5}^{128} & n_{R4}^{66} &= n_{R3}^{128} + n_{R5}^{128} \\ n_{R7}^{128} + n_{R9}^{128} & n_{R5}^{66} &= n_{R2}^{128} + n_{R4}^{128} & n_{R3}^{66} &= n_{R6}^{128} + n_{R8}^{128} \end{aligned}$$

The lower SG is SG 83 when the preserved operations are: **(sub-SG label is 3) 1, 2, 3, 6, 9, 10, 11, 14.**

The transformation is:  $(\mathbf{a}_{83}, \mathbf{b}_{83}, \mathbf{c}_{83}) = (\mathbf{a}_{128}, \mathbf{b}_{128}, \mathbf{c}_{128}) \begin{pmatrix} -1 & 0 & 0 \\ 0 & -1 & 0 \\ 0 & 0 & 1 \end{pmatrix}, \overrightarrow{O_{128}O_{83}} = \frac{1}{2}\mathbf{a}_{83} + (\frac{1}{2})\mathbf{b}_{83} + (\frac{1}{2})\mathbf{c}_{83}$

The reduction of higher dimensional irrep:

$$D_{4h} : E_g \rightarrow {}^2E_g + {}^1E_g \text{ of } C_{4h}.$$

$$D_{4h} : E_u \rightarrow {}^2E_u + {}^1E_u \text{ of } C_{4h}.$$

The correspondences of irreps at HSPs from original SG to lowered SG:

$$\begin{aligned} n_{GM9}^{83} &= n_{GM8}^{128} & n_{GM5}^{83} &= n_{GM6}^{128} & n_{GM11}^{83} &= n_{GM8}^{128} & n_{GM7}^{83} &= n_{GM6}^{128} & n_{GM12}^{83} &= n_{GM9}^{128} & n_{GM8}^{83} &= n_{GM7}^{128} & n_{GM10}^{83} &= n_{GM9}^{128} & n_{GM6}^{83} &= n_{GM9}^{128} \\ n_{M8}^{128} & n_{X6}^{83} &= n_{X3}^{128} & n_{X4}^{83} &= n_{X3}^{128} & n_{X5}^{83} &= n_{X4}^{128} & n_{X3}^{83} &= n_{X4}^{128} & n_{M9}^{83} &= n_{M9}^{128} & n_{M5}^{83} &= n_{M7}^{128} & n_{M11}^{83} &= n_{M8}^{128} & n_{M7}^{83} &= n_{M6}^{128} & n_{M12}^{83} &= n_{M9}^{128} \\ n_{M8}^{83} &= n_{M7}^{128} & n_{M10}^{83} &= n_{M8}^{128} & n_{M6}^{83} &= n_{M6}^{128} & n_{A9}^{83} &= n_{A6}^{128} & n_{A5}^{83} &= n_{A7}^{128} & n_{A11}^{83} &= n_{A8}^{128} & n_{A7}^{83} &= n_{A5}^{128} & n_{A12}^{83} &= n_{A7}^{128} & n_{A8}^{83} &= n_{A6}^{128} & n_{A10}^{83} &= n_{A9}^{128} \\ n_{A5}^{128} & n_{A6}^{83} &= n_{A8}^{128} & n_{R6}^{83} &= n_{R6}^{128} + n_{R8}^{128} & n_{R4}^{83} &= n_{R2}^{128} + n_{R4}^{128} & n_{R5}^{83} &= n_{R7}^{128} + n_{R9}^{128} & n_{R3}^{83} &= n_{R3}^{128} + n_{R5}^{128} & n_{Z9}^{83} &= n_{Z5}^{128} & n_{Z5}^{83} &= n_{Z5}^{128} & n_{Z7}^{83} &= n_{Z7}^{128} \\ n_{Z11}^{83} &= n_{Z7}^{128} & n_{Z7}^{83} &= n_{Z5}^{128} & n_{Z12}^{83} &= n_{Z8}^{128} & n_{Z8}^{83} &= n_{Z6}^{128} & n_{Z10}^{83} &= n_{Z6}^{128} & n_{Z6}^{83} &= n_{Z6}^{128} \end{aligned}$$

**41. Lowered SGs by higher-dimensional irreps of pairings in SG 129**

The representative operations of SG/T for SG 129:

$$1 : (x, y, z), 2 : (\frac{1}{2} - y, x, z), 3 : (y, \frac{1}{2} - x, z), 4 : (x + \frac{1}{2}, -y, -z), 5 : (-x, y + \frac{1}{2}, -z), 6 : (\frac{1}{2} - x, \frac{1}{2} - y, z), 7 : (y + \frac{1}{2}, x + \frac{1}{2}, -z), 8 : (-y, -x, -z), 9 : (-x, -y, -z), 10 : (y + \frac{1}{2}, -x, -z), 11 : (-y, x + \frac{1}{2}, -z), 12 : (\frac{1}{2} - x, y, z), 13 : (x, \frac{1}{2} - y, z), 14 : (x + \frac{1}{2}, y + \frac{1}{2}, -z), 15 : (\frac{1}{2} - y, \frac{1}{2} - x, z), 16 : (y, x, z).$$

The lower SG is SG 59 when the preserved operations are: **(sub-SG label is 1) 1, 4, 5, 6, 9, 12, 13, 14.**

The transformation is:  $(\mathbf{a}_{59}, \mathbf{b}_{59}, \mathbf{c}_{59}) = (\mathbf{a}_{129}, \mathbf{b}_{129}, \mathbf{c}_{129}) \begin{pmatrix} 1 & 0 & 0 \\ 0 & 1 & 0 \\ 0 & 0 & 1 \end{pmatrix}, \overrightarrow{O_{129}O_{59}} = \frac{1}{2}\mathbf{b}_{59} + (\frac{1}{2})\mathbf{c}_{59}$

The reduction of higher dimensional irrep:

$$D_{4h} : E_g \rightarrow B_{2g} + B_{3g} \text{ of } D_{2h}.$$

$$D_{4h} : E_u \rightarrow B_{2u} + B_{3u} \text{ of } D_{2h}.$$

The correspondences of irreps at HSPs from original SG to lowered SG:

$$\begin{aligned} n_{GM6}^{59} &= n_{GM8}^{129} + n_{GM9}^{129} & n_{GM5}^{59} &= n_{GM6}^{129} + n_{GM7}^{129} & n_{X4}^{59} &= n_{X3}^{129} & n_{X3}^{59} &= n_{X4}^{129} & n_{S3}^{59} &= n_{M5}^{129} & n_{S4}^{59} &= n_{M5}^{129} & n_{R3}^{59} &= n_{A5}^{129} & n_{R4}^{59} &= n_{A5}^{129} \\ n_{U4}^{59} &= n_{R4}^{129} & n_{U3}^{59} &= n_{R3}^{129} & n_{Z6}^{59} &= n_{Z6}^{129} + n_{Z7}^{129} & n_{Z5}^{59} &= n_{Z8}^{129} + n_{Z9}^{129} & n_{T4}^{59} &= n_{R4}^{129} & n_{T3}^{59} &= n_{R3}^{129} & n_{Y4}^{59} &= n_{X3}^{129} & n_{Y3}^{59} &= n_{X4}^{129} \end{aligned}$$

The lower SG is SG 67 when the preserved operations are: **(sub-SG label is 2) 1, 6, 7, 8, 9, 14, 15, 16.**

The transformation is:  $(\mathbf{a}_{67}, \mathbf{b}_{67}, \mathbf{c}_{67}) = (\mathbf{a}_{129}, \mathbf{b}_{129}, \mathbf{c}_{129}) \begin{pmatrix} 1 & -1 & 0 \\ 1 & 1 & 0 \\ 0 & 0 & 1 \end{pmatrix}, \overrightarrow{O_{129}O_{67}} = \frac{1}{4}\mathbf{a}_{67} + (\frac{3}{4})\mathbf{b}_{67} + (\frac{1}{2})\mathbf{c}_{67}$

The reduction of higher dimensional irrep:

$$D_{4h} : E_g \rightarrow B_{2g} + B_{3g} \text{ of } D_{2h}.$$

$$D_{4h} : E_u \rightarrow B_{2u} + B_{3u} \text{ of } D_{2h}.$$

The correspondences of irreps at HSPs from original SG to lowered SG:

$$\begin{aligned} n_{GM6}^{67} &= n_{GM8}^{129} + n_{GM9}^{129} & n_{GM5}^{67} &= n_{GM6}^{129} + n_{GM7}^{129} & n_{Y6}^{67} &= n_{M5}^{129} & n_{Y5}^{67} &= n_{M5}^{129} & n_{S2}^{67} &= n_{X3}^{129} + n_{X4}^{129} & n_{Z6}^{67} &= n_{Z6}^{129} + n_{Z7}^{129} & n_{Z5}^{67} &= n_{Z8}^{129} + n_{Z9}^{129} & n_{T6}^{67} &= n_{A5}^{129} & n_{T5}^{67} &= n_{A5}^{129} & n_{R2}^{67} &= n_{R3}^{129} + n_{R4}^{129} \end{aligned}$$

The lower SG is SG 85 when the preserved operations are: **(sub-SG label is 3) 1, 2, 3, 6, 9, 10, 11, 14.**

The transformation is:  $(\mathbf{a}_{85}, \mathbf{b}_{85}, \mathbf{c}_{85}) = (\mathbf{a}_{129}, \mathbf{b}_{129}, \mathbf{c}_{129}) \begin{pmatrix} -1 & 0 & 0 \\ 0 & -1 & 0 \\ 0 & 0 & 1 \end{pmatrix}, \overrightarrow{O_{129}O_{85}} = \frac{1}{2}\mathbf{a}_{85} + (-\frac{1}{2})\mathbf{b}_{85} + (\frac{1}{2})\mathbf{c}_{85}$

The reduction of higher dimensional irrep:

$$D_{4h} : E_g \rightarrow {}^2E_g + {}^1E_g \text{ of } C_{4h}.$$

$$D_{4h} : E_u \rightarrow {}^2E_u + {}^1E_u \text{ of } C_{4h}.$$

The correspondences of irreps at HSPs from original SG to lowered SG:

$$\begin{aligned} n_{GM9}^{85} &= n_{GM8}^{129} & n_{GM5}^{85} &= n_{GM6}^{129} & n_{GM11}^{85} &= n_{GM8}^{129} & n_{GM7}^{85} &= n_{GM6}^{129} & n_{GM12}^{85} &= n_{GM9}^{129} & n_{GM8}^{85} &= n_{GM7}^{129} & n_{GM10}^{85} &= n_{GM9}^{129} & n_{GM6}^{85} &= n_{GM7}^{129} \\ n_{X2}^{85} &= n_{X3}^{129} + n_{X4}^{129} & n_{X1}^{85} &= n_{X3}^{129} & n_{M3}^{85} &= n_{M5}^{129} & n_{M4}^{85} &= n_{M5}^{129} & n_{A3}^{85} &= n_{A5}^{129} & n_{A4}^{85} &= n_{A5}^{129} & n_{R2}^{85} &= n_{R3}^{129} + n_{R4}^{129} & n_{Z9}^{85} &= n_{Z6}^{129} & n_{Z5}^{85} &= n_{Z8}^{129} & n_{Z8}^{85} &= n_{Z9}^{129} \\ n_{Z11}^{85} &= n_{Z6}^{129} & n_{Z7}^{85} &= n_{Z8}^{129} & n_{Z12}^{85} &= n_{Z7}^{129} & n_{Z8}^{85} &= n_{Z9}^{129} & n_{Z10}^{85} &= n_{Z7}^{129} & n_{Z6}^{85} &= n_{Z9}^{129} \end{aligned}$$

## 42. Lowered SGs by higher-dimensional irreps of pairings in SG 130

The representative operations of SG/T for SG 130:

$$\begin{aligned} 1 : (x, y, z), & 2 : (\frac{1}{2} - y, x, z), & 3 : (y, \frac{1}{2} - x, z), & 4 : (x + \frac{1}{2}, -y, \frac{1}{2} - z), & 5 : (-x, y + \frac{1}{2}, \frac{1}{2} - z), & 6 : (\frac{1}{2} - x, \frac{1}{2} - y, z), \\ 7 : (y + \frac{1}{2}, x + \frac{1}{2}, \frac{1}{2} - z), & 8 : (-y, -x, \frac{1}{2} - z), & 9 : (-x, -y, -z), & 10 : (y + \frac{1}{2}, -x, -z), & 11 : (-y, x + \frac{1}{2}, -z), \\ 12 : (\frac{1}{2} - x, y, z + \frac{1}{2}), & 13 : (x, \frac{1}{2} - y, z + \frac{1}{2}), & 14 : (x + \frac{1}{2}, y + \frac{1}{2}, -z), & 15 : (\frac{1}{2} - y, \frac{1}{2} - x, z + \frac{1}{2}), & 16 : (y, x, z + \frac{1}{2}). \end{aligned}$$

The lower SG is SG 56 when the preserved operations are: **(sub-SG label is 1) 1, 4, 5, 6, 9, 12, 13, 14.**

The transformation is:  $(\mathbf{a}_{56}, \mathbf{b}_{56}, \mathbf{c}_{56}) = (\mathbf{a}_{130}, \mathbf{b}_{130}, \mathbf{c}_{130}) \begin{pmatrix} 1 & 0 & 0 \\ 0 & 1 & 0 \\ 0 & 0 & 1 \end{pmatrix}, \overrightarrow{O_{130}O_{56}} = \mathbf{b}_{56} + (\frac{1}{2})\mathbf{c}_{56}$

The reduction of higher dimensional irrep:

$$D_{4h} : E_g \rightarrow B_{2g} + B_{3g} \text{ of } D_{2h}.$$

$$D_{4h} : E_u \rightarrow B_{2u} + B_{3u} \text{ of } D_{2h}.$$

The correspondences of irreps at HSPs from original SG to lowered SG:

$$\begin{aligned} n_{GM6}^{56} &= n_{GM8}^{130} + n_{GM9}^{130} & n_{GM5}^{56} &= n_{GM6}^{130} + n_{GM7}^{130} & n_{X4}^{56} &= n_{X3}^{130} & n_{X3}^{56} &= n_{X4}^{130} & n_{S3}^{56} &= n_{M5}^{130} & n_{S4}^{56} &= n_{M5}^{130} & n_{R3}^{56} &= n_{A5}^{130} & n_{R5}^{56} &= n_{A5}^{130} \\ n_{U3}^{56} &= n_{R4}^{130} & n_{U4}^{56} &= n_{R3}^{130} & n_{Z4}^{56} &= n_{Z5}^{130} + n_{Z6}^{130} & n_{Z3}^{56} &= n_{Z7}^{130} + n_{Z8}^{130} & n_{T4}^{56} &= n_{R3}^{130} & n_{T3}^{56} &= n_{R4}^{130} & n_{Y4}^{56} &= n_{X4}^{130} & n_{Y3}^{56} &= n_{X3}^{130} \end{aligned}$$

The lower SG is SG 68 when the preserved operations are: **(sub-SG label is 2) 1, 6, 7, 8, 9, 14, 15, 16.**

The transformation is:  $(\mathbf{a}_{68}, \mathbf{b}_{68}, \mathbf{c}_{68}) = (\mathbf{a}_{130}, \mathbf{b}_{130}, \mathbf{c}_{130}) \begin{pmatrix} 1 & -1 & 0 \\ 1 & 1 & 0 \\ 0 & 0 & 1 \end{pmatrix}, \overrightarrow{O_{130}O_{68}} = \mathbf{b}_{68} + \left(\frac{1}{2}\right)\mathbf{c}_{68}$

The reduction of higher dimensional irrep:

$$D_{4h} : E_g \rightarrow B_{2g} + B_{3g} \text{ of } D_{2h}.$$

$$D_{4h} : E_u \rightarrow B_{2u} + B_{3u} \text{ of } D_{2h}.$$

The correspondences of irreps at HSPs from original SG to lowered SG:

$$\begin{aligned} n_{GM6}^{68} &= n_{GM8}^{130} + n_{GM9}^{130} n_{GM5}^{68} = n_{GM6}^{130} + n_{GM7}^{130} n_{Y6}^{68} = n_{M5}^{130} n_{Y5}^{68} = n_{M5}^{130} n_{S2}^{68} = n_{X3}^{130} + n_{X4}^{130} n_{Z4}^{68} = n_{Z5}^{130} + n_{Z6}^{130} n_{Z3}^{68} = \\ n_{Z7}^{130} + n_{Z8}^{130} n_{T4}^{68} &= n_{A5}^{130} n_{T3}^{68} = n_{A5}^{130} n_{R2}^{68} = n_{R3}^{130} + n_{R4}^{130} \end{aligned}$$

The lower SG is SG 85 when the preserved operations are: **(sub-SG label is 3) 1, 2, 3, 6, 9, 10, 11, 14.**

The transformation is:  $(\mathbf{a}_{85}, \mathbf{b}_{85}, \mathbf{c}_{85}) = (\mathbf{a}_{130}, \mathbf{b}_{130}, \mathbf{c}_{130}) \begin{pmatrix} -1 & 0 & 0 \\ 0 & -1 & 0 \\ 0 & 0 & 1 \end{pmatrix}, \overrightarrow{O_{130}O_{85}} = \frac{1}{2}\mathbf{a}_{85} + \left(-\frac{1}{2}\right)\mathbf{b}_{85} + \left(\frac{1}{2}\right)\mathbf{c}_{85}$

The reduction of higher dimensional irrep:

$$D_{4h} : E_g \rightarrow {}^2E_g + {}^1E_g \text{ of } C_{4h}.$$

$$D_{4h} : E_u \rightarrow {}^2E_u + {}^1E_u \text{ of } C_{4h}.$$

The correspondences of irreps at HSPs from original SG to lowered SG:

$$\begin{aligned} n_{GM9}^{85} &= n_{GM8}^{130} n_{GM5}^{85} = n_{GM6}^{130} n_{GM11}^{85} = n_{GM8}^{130} n_{GM7}^{85} = n_{GM6}^{130} n_{GM12}^{85} = n_{GM9}^{130} n_{GM8}^{85} = n_{GM7}^{130} n_{GM10}^{85} = n_{GM9}^{130} n_{GM6}^{85} = \\ n_{GM7}^{130} n_{X2}^{85} &= n_{X3}^{130} + n_{X4}^{130} n_{M3}^{85} = n_{M5}^{130} n_{M4}^{85} = n_{M5}^{130} n_{A3}^{85} = n_{A5}^{130} n_{A4}^{85} = n_{A5}^{130} n_{R2}^{85} = n_{R3}^{130} + n_{R4}^{130} n_{Z9}^{85} = n_{Z5}^{130} n_{Z5}^{85} = n_{Z7}^{130} \\ n_{Z11}^{85} &= n_{Z7}^{130} n_{Z7}^{85} = n_{Z5}^{130} n_{Z12}^{85} = n_{Z8}^{130} n_{Z8}^{85} = n_{Z6}^{130} n_{Z10}^{85} = n_{Z6}^{130} n_{Z6}^{85} = n_{Z8}^{130} \end{aligned}$$

### 43. Lowered SGs by higher-dimensional irreps of pairings in SG 131

The representative operations of SG/T for SG 131:

$$\begin{aligned} 1 : (x, y, z), 2 : (-y, x, z + \frac{1}{2}), 3 : (y, -x, z + \frac{1}{2}), 4 : (x, -y, -z), 5 : (-x, y, -z), 6 : (-x, -y, z), 7 : (y, x, \frac{1}{2} - z), \\ 8 : (-y, -x, \frac{1}{2} - z), 9 : (-x, -y, -z), 10 : (y, -x, \frac{1}{2} - z), 11 : (-y, x, \frac{1}{2} - z), 12 : (-x, y, z), 13 : (x, -y, z), \\ 14 : (x, y, -z), 15 : (-y, -x, z + \frac{1}{2}), 16 : (y, x, z + \frac{1}{2}). \end{aligned}$$

The lower SG is SG 47 when the preserved operations are: **(sub-SG label is 1) 1, 4, 5, 6, 9, 12, 13, 14.**

The transformation is:  $(\mathbf{a}_{47}, \mathbf{b}_{47}, \mathbf{c}_{47}) = (\mathbf{a}_{131}, \mathbf{b}_{131}, \mathbf{c}_{131}) \begin{pmatrix} 0 & 0 & 1 \\ 1 & 0 & 0 \\ 0 & 1 & 0 \end{pmatrix}, \overrightarrow{O_{131}O_{47}} = \frac{1}{2}\mathbf{a}_{47} + \left(\frac{1}{2}\right)\mathbf{c}_{47}$

The reduction of higher dimensional irrep:

$$D_{4h} : E_g \rightarrow B_{1g} + B_{3g} \text{ of } D_{2h}.$$

$$D_{4h} : E_u \rightarrow B_{1u} + B_{3u} \text{ of } D_{2h}.$$

The correspondences of irreps at HSPs from original SG to lowered SG:

$$\begin{aligned} n_{GM6}^{47} &= n_{GM8}^{131} + n_{GM9}^{131} n_{GM5}^{47} = n_{GM6}^{131} + n_{GM7}^{131} n_{X6}^{47} = n_{X5}^{131} n_{X5}^{47} = n_{X6}^{131} n_{S6}^{47} = n_{R5}^{131} n_{S5}^{47} = n_{R6}^{131} n_{R6}^{47} = n_{A5}^{131} n_{R5}^{47} = n_{A5}^{131} \\ n_{U6}^{47} &= n_{M8}^{131} + n_{M9}^{131} n_{U5}^{47} = n_{M6}^{131} + n_{M7}^{131} n_{Z6}^{47} = n_{X5}^{131} n_{Z5}^{47} = n_{X6}^{131} n_{T6}^{47} = n_{R6}^{131} n_{T5}^{47} = n_{R5}^{131} n_{Y6}^{47} = n_{Z5}^{131} n_{Y5}^{47} = n_{Z5}^{131} \end{aligned}$$

The lower SG is SG 66 when the preserved operations are: **(sub-SG label is 2) 1, 6, 7, 8, 9, 14, 15, 16.**

The transformation is:  $(\mathbf{a}_{66}, \mathbf{b}_{66}, \mathbf{c}_{66}) = (\mathbf{a}_{131}, \mathbf{b}_{131}, \mathbf{c}_{131}) \begin{pmatrix} 1 & -1 & 0 \\ 1 & 1 & 0 \\ 0 & 0 & 1 \end{pmatrix}, \overrightarrow{O_{131}O_{66}} = \frac{1}{2}\mathbf{c}_{66}$

The reduction of higher dimensional irrep:

$$D_{4h} : E_g \rightarrow B_{2g} + B_{3g} \text{ of } D_{2h}.$$

$$D_{4h} : E_u \rightarrow B_{2u} + B_{3u} \text{ of } D_{2h}.$$

The correspondences of irreps at HSPs from original SG to lowered SG:

$$n_{GM6}^{66} = n_{GM8}^{131} + n_{GM9}^{131} n_{GM5}^{66} = n_{GM6}^{131} + n_{GM7}^{131} n_{Y6}^{66} = n_{M8}^{131} + n_{M9}^{131} n_{Y5}^{66} = n_{M6}^{131} + n_{M7}^{131} n_{S6}^{66} = n_{X6}^{131} n_{S4}^{66} = n_{X5}^{131} n_{S5}^{66} =$$

$$n_{X6}^{131} n_{S3}^{66} = n_{X5}^{131} n_{Z4}^{66} = n_{Z5}^{131} n_{Z3}^{66} = n_{Z5}^{131} n_{T4}^{66} = n_{A5}^{131} n_{T3}^{66} = n_{A5}^{131} n_{R6}^{66} = n_{R5}^{131} n_{R4}^{66} = n_{R6}^{131} n_{R5}^{66} = n_{R5}^{131} n_{R3}^{66} = n_{R6}^{131}$$

The lower SG is SG 84 when the preserved operations are: **(sub-SG label is 3) 1, 2, 3, 6, 9, 10, 11, 14.**

The transformation is:  $(\mathbf{a}_{84}, \mathbf{b}_{84}, \mathbf{c}_{84}) = (\mathbf{a}_{131}, \mathbf{b}_{131}, \mathbf{c}_{131}) \begin{pmatrix} -1 & 0 & 0 \\ 0 & -1 & 0 \\ 0 & 0 & 1 \end{pmatrix}, \overrightarrow{O_{131}O_{84}} = \frac{1}{2}\mathbf{c}_{84}$

The reduction of higher dimensional irrep:

$$D_{4h} : E_g \rightarrow {}^2E_g + {}^1E_g \text{ of } C_{4h}.$$

$$D_{4h} : E_u \rightarrow {}^2E_u + {}^1E_u \text{ of } C_{4h}.$$

The correspondences of irreps at HSPs from original SG to lowered SG:

$$\begin{aligned} n_{GM9}^{84} &= n_{GM8}^{131} n_{GM5}^{84} = n_{GM6}^{131} n_{GM11}^{84} = n_{GM8}^{131} n_{GM7}^{84} = n_{GM6}^{131} n_{GM12}^{84} = n_{GM9}^{131} n_{GM8}^{84} = n_{GM7}^{131} n_{GM10}^{84} = n_{GM9}^{131} n_{GM6}^{84} = \\ n_{GM7}^{131} n_{X6}^{84} &= n_{X6}^{131} n_{X4}^{84} = n_{X5}^{131} n_{X5}^{84} = n_{X6}^{131} n_{X3}^{84} = n_{X5}^{131} n_{M9}^{84} = n_{M8}^{131} n_{M5}^{84} = n_{M6}^{131} n_{M11}^{84} = n_{M8}^{131} n_{M7}^{84} = n_{M6}^{131} n_{M12}^{84} = n_{M9}^{131} \\ n_{M8}^{84} &= n_{M7}^{131} n_{M10}^{84} = n_{M9}^{131} n_{M6}^{84} = n_{M7}^{131} n_{A4}^{84} = n_{A5}^{131} n_{A3}^{84} = n_{A5}^{131} n_{R4}^{84} = n_{R6}^{131} n_{R6}^{84} = n_{R5}^{131} n_{R3}^{84} = n_{R6}^{131} n_{R5}^{84} = n_{R5}^{131} n_{R4}^{84} = \\ n_{Z5}^{131} n_{Z3}^{84} &= n_{Z5}^{131} \end{aligned}$$

#### 44. Lowered SGs by higher-dimensional irreps of pairings in SG 132

The representative operations of SG/T for SG 132:

$$\begin{aligned} 1 : (x, y, z), 2 : (-y, x, z + \frac{1}{2}), 3 : (y, -x, z + \frac{1}{2}), 4 : (x, -y, \frac{1}{2} - z), 5 : (-x, y, \frac{1}{2} - z), 6 : (-x, -y, z), 7 : (y, x, -z), \\ 8 : (-y, -x, -z), 9 : (-x, -y, -z), 10 : (y, -x, \frac{1}{2} - z), 11 : (-y, x, \frac{1}{2} - z), 12 : (-x, y, z + \frac{1}{2}), 13 : (x, -y, z + \frac{1}{2}), \\ 14 : (x, y, -z), 15 : (-y, -x, z), 16 : (y, x, z). \end{aligned}$$

The lower SG is SG 49 when the preserved operations are: **(sub-SG label is 1) 1, 4, 5, 6, 9, 12, 13, 14.**

The transformation is:  $(\mathbf{a}_{49}, \mathbf{b}_{49}, \mathbf{c}_{49}) = (\mathbf{a}_{132}, \mathbf{b}_{132}, \mathbf{c}_{132}) \begin{pmatrix} 1 & 0 & 0 \\ 0 & 1 & 0 \\ 0 & 0 & 1 \end{pmatrix}, \overrightarrow{O_{132}O_{49}} = \frac{1}{2}\mathbf{a}_{49} + (\frac{1}{2})\mathbf{c}_{49}$

The reduction of higher dimensional irrep:

$$D_{4h} : E_g \rightarrow B_{2g} + B_{3g} \text{ of } D_{2h}.$$

$$D_{4h} : E_u \rightarrow B_{2u} + B_{3u} \text{ of } D_{2h}.$$

The correspondences of irreps at HSPs from original SG to lowered SG:

$$\begin{aligned} n_{GM6}^{49} &= n_{GM8}^{132} + n_{GM9}^{132} n_{GM5}^{49} = n_{GM6}^{132} + n_{GM7}^{132} n_{X6}^{49} = n_{X5}^{132} n_{X5}^{49} = n_{X6}^{132} n_{S6}^{49} = n_{M6}^{132} + n_{M7}^{132} n_{S5}^{49} = n_{M8}^{132} + n_{M9}^{132} n_{R4}^{49} = \\ n_{A5}^{132} n_{R3}^{49} &= n_{A5}^{132} n_{U4}^{49} = n_{R4}^{132} n_{U3}^{49} = n_{R3}^{132} n_{Z4}^{49} = n_{Z5}^{132} n_{Z3}^{49} = n_{Z5}^{132} n_{T4}^{49} = n_{R3}^{132} n_{T3}^{49} = n_{R4}^{132} n_{Y6}^{49} = n_{X6}^{132} n_{Y5}^{49} = n_{X5}^{132} \end{aligned}$$

The lower SG is SG 65 when the preserved operations are: **(sub-SG label is 2) 1, 6, 7, 8, 9, 14, 15, 16.**

The transformation is:  $(\mathbf{a}_{65}, \mathbf{b}_{65}, \mathbf{c}_{65}) = (\mathbf{a}_{132}, \mathbf{b}_{132}, \mathbf{c}_{132}) \begin{pmatrix} 1 & -1 & 0 \\ 1 & 1 & 0 \\ 0 & 0 & 1 \end{pmatrix}, \overrightarrow{O_{132}O_{65}} = \frac{1}{2}\mathbf{c}_{65}$

The reduction of higher dimensional irrep:

$$D_{4h} : E_g \rightarrow B_{2g} + B_{3g} \text{ of } D_{2h}.$$

$$D_{4h} : E_u \rightarrow B_{2u} + B_{3u} \text{ of } D_{2h}.$$

The correspondences of irreps at HSPs from original SG to lowered SG:

$$\begin{aligned} n_{GM6}^{65} &= n_{GM8}^{132} + n_{GM9}^{132} n_{GM5}^{65} = n_{GM6}^{132} + n_{GM7}^{132} n_{Y6}^{65} = n_{M8}^{132} + n_{M9}^{132} n_{Y5}^{65} = n_{M6}^{132} + n_{M7}^{132} n_{S6}^{65} = n_{X6}^{132} n_{S4}^{65} = n_{X5}^{132} n_{S5}^{65} = \\ n_{X6}^{132} n_{S3}^{65} &= n_{X5}^{132} n_{Z6}^{65} = n_{Z5}^{132} n_{Z5}^{65} = n_{Z5}^{132} n_{T6}^{65} = n_{A5}^{132} n_{T5}^{65} = n_{A5}^{132} n_{R6}^{65} = n_{R4}^{132} n_{R4}^{65} = n_{R3}^{132} n_{R5}^{65} = n_{R3}^{132} n_{R3}^{65} = n_{R4}^{132} \end{aligned}$$

The lower SG is SG 84 when the preserved operations are: **(sub-SG label is 3) 1, 2, 3, 6, 9, 10, 11, 14.**

The transformation is:  $(\mathbf{a}_{84}, \mathbf{b}_{84}, \mathbf{c}_{84}) = (\mathbf{a}_{132}, \mathbf{b}_{132}, \mathbf{c}_{132}) \begin{pmatrix} -1 & 0 & 0 \\ 0 & -1 & 0 \\ 0 & 0 & 1 \end{pmatrix}, \overrightarrow{O_{132}O_{84}} = \frac{1}{2}\mathbf{c}_{84}$

The reduction of higher dimensional irrep:

$$D_{4h} : E_g \rightarrow {}^2E_g + {}^1E_g \text{ of } C_{4h}.$$

$$D_{4h} : E_u \rightarrow {}^2E_u + {}^1E_u \text{ of } C_{4h}.$$

The correspondences of irreps at HSPs from original SG to lowered SG:

$$\begin{aligned}
 n_{GM9}^{84} &= n_{GM8}^{132} n_{GM5}^{84} = n_{GM6}^{132} n_{GM11}^{84} = n_{GM8}^{132} n_{GM7}^{84} = n_{GM6}^{132} n_{GM12}^{84} = n_{GM9}^{132} n_{GM8}^{84} = n_{GM7}^{132} n_{GM10}^{84} = n_{GM9}^{132} n_{GM6}^{84} = \\
 n_{GM7}^{132} n_{X6}^{84} &= n_{X6}^{132} n_{X4}^{84} = n_{X5}^{132} n_{X5}^{84} = n_{X6}^{132} n_{X3}^{84} = n_{X5}^{132} n_{M9}^{84} = n_{M8}^{132} n_{M5}^{84} = n_{M6}^{132} n_{M11}^{84} = n_{M8}^{132} n_{M7}^{84} = n_{M6}^{132} n_{M12}^{84} = n_{M9}^{132} \\
 n_{M8}^{84} &= n_{M7}^{132} n_{M10}^{84} = n_{M9}^{132} n_{M6}^{84} = n_{M7}^{132} n_{A4}^{84} = n_{A5}^{132} n_{A3}^{84} = n_{A5}^{132} n_{R4}^{84} = n_{R3}^{132} n_{R6}^{84} = n_{R4}^{132} n_{R3}^{84} = n_{R4}^{132} n_{R5}^{84} = n_{R3}^{132} n_{Z4}^{84} = \\
 n_{Z5}^{132} n_{Z3}^{84} &= n_{Z5}^{132}
 \end{aligned}$$

**45. Lowered SGs by higher-dimensional irreps of pairings in SG 133**

The representative operations of SG/T for SG 133:

$$\begin{aligned}
 1 : (x, y, z), 2 : (\frac{1}{2} - y, x, z + \frac{1}{2}), 3 : (y, \frac{1}{2} - x, z + \frac{1}{2}), 4 : (x, \frac{1}{2} - y, -z), 5 : (\frac{1}{2} - x, y, -z), 6 : (\frac{1}{2} - x, \frac{1}{2} - y, z), \\
 7 : (y, x, \frac{1}{2} - z), 8 : (\frac{1}{2} - y, \frac{1}{2} - x, \frac{1}{2} - z), 9 : (-x, -y, -z), 10 : (y + \frac{1}{2}, -x, \frac{1}{2} - z), 11 : (-y, x + \frac{1}{2}, \frac{1}{2} - z), \\
 12 : (-x, y + \frac{1}{2}, z), 13 : (x + \frac{1}{2}, -y, z), 14 : (x + \frac{1}{2}, y + \frac{1}{2}, -z), 15 : (-y, -x, z + \frac{1}{2}), 16 : (y + \frac{1}{2}, x + \frac{1}{2}, z + \frac{1}{2}).
 \end{aligned}$$

The lower SG is SG 50 when the preserved operations are: **(sub-SG label is 1)** 1, 4, 5, 6, 9, 12, 13, 14.

The transformation is:  $(\mathbf{a}_{50}, \mathbf{b}_{50}, \mathbf{c}_{50}) = (\mathbf{a}_{133}, \mathbf{b}_{133}, \mathbf{c}_{133}) \begin{pmatrix} 1 & 0 & 0 \\ 0 & 1 & 0 \\ 0 & 0 & 1 \end{pmatrix}, \overrightarrow{O_{133}O_{50}} = \frac{1}{2}\mathbf{a}_{50} + (\frac{1}{2})\mathbf{b}_{50}$

The reduction of higher dimensional irrep:

$$D_{4h} : E_g \rightarrow B_{2g} + B_{3g} \text{ of } D_{2h}.$$

$$D_{4h} : E_u \rightarrow B_{2u} + B_{3u} \text{ of } D_{2h}.$$

The correspondences of irreps at HSPs from original SG to lowered SG:

$$\begin{aligned}
 n_{GM6}^{50} &= n_{GM8}^{133} + n_{GM9}^{133} n_{GM5}^{50} = n_{GM6}^{133} + n_{GM7}^{133} n_{X4}^{50} = n_{X3}^{133} n_{X3}^{50} = n_{X4}^{133} n_{S3}^{50} = n_{M3}^{133} n_{S4}^{50} = n_{M5}^{133} n_{R3}^{50} = n_{A5}^{133} + n_{A6}^{133} n_{R4}^{50} = \\
 n_{A7}^{133} + n_{A8}^{133} n_{U4}^{50} &= n_{R3}^{133} n_{U3}^{50} = n_{R4}^{133} n_{Z6}^{50} = n_{Z5}^{133} n_{Z5}^{50} = n_{Z5}^{133} n_{T4}^{50} = n_{R3}^{133} n_{T3}^{50} = n_{R4}^{133} n_{Y4}^{50} = n_{X3}^{133} n_{Y3}^{50} = n_{X4}^{133}
 \end{aligned}$$

The lower SG is SG 68 when the preserved operations are: **(sub-SG label is 2)** 1, 6, 7, 8, 9, 14, 15, 16.

The transformation is:  $(\mathbf{a}_{68}, \mathbf{b}_{68}, \mathbf{c}_{68}) = (\mathbf{a}_{133}, \mathbf{b}_{133}, \mathbf{c}_{133}) \begin{pmatrix} 1 & -1 & 0 \\ 1 & 1 & 0 \\ 0 & 0 & 1 \end{pmatrix}, \overrightarrow{O_{133}O_{68}} = \frac{1}{4}\mathbf{a}_{68} + (\frac{3}{4})\mathbf{b}_{68}$

The reduction of higher dimensional irrep:

$$D_{4h} : E_g \rightarrow B_{2g} + B_{3g} \text{ of } D_{2h}.$$

$$D_{4h} : E_u \rightarrow B_{2u} + B_{3u} \text{ of } D_{2h}.$$

The correspondences of irreps at HSPs from original SG to lowered SG:

$$\begin{aligned}
 n_{GM6}^{68} &= n_{GM8}^{133} + n_{GM9}^{133} n_{GM5}^{68} = n_{GM6}^{133} + n_{GM7}^{133} n_{Y6}^{68} = n_{M5}^{133} n_{Y5}^{68} = n_{M5}^{133} n_{S2}^{68} = n_{X3}^{133} + n_{X4}^{133} n_{Z4}^{68} = n_{Z5}^{133} n_{Z3}^{68} = n_{Z5}^{133} n_{T4}^{68} = \\
 n_{A5}^{133} + n_{A6}^{133} n_{T3}^{68} &= n_{A7}^{133} + n_{A8}^{133} n_{R2}^{68} = n_{R3}^{133} + n_{R4}^{133}
 \end{aligned}$$

The lower SG is SG 86 when the preserved operations are: **(sub-SG label is 3)** 1, 2, 3, 6, 9, 10, 11, 14.

The transformation is:  $(\mathbf{a}_{86}, \mathbf{b}_{86}, \mathbf{c}_{86}) = (\mathbf{a}_{133}, \mathbf{b}_{133}, \mathbf{c}_{133}) \begin{pmatrix} -1 & 0 & 0 \\ 0 & 1 & 0 \\ 0 & 0 & -1 \end{pmatrix}, \overrightarrow{O_{133}O_{86}} = \mathbf{b}_{86} + \mathbf{c}_{86}$

The reduction of higher dimensional irrep:

$$D_{4h} : E_g \rightarrow {}^2E_g + {}^1E_g \text{ of } C_{4h}.$$

$$D_{4h} : E_u \rightarrow {}^2E_u + {}^1E_u \text{ of } C_{4h}.$$

The correspondences of irreps at HSPs from original SG to lowered SG:

$$\begin{aligned}
 n_{GM9}^{86} &= n_{GM8}^{133} n_{GM5}^{86} = n_{GM6}^{133} n_{GM11}^{86} = n_{GM8}^{133} n_{GM7}^{86} = n_{GM6}^{133} n_{GM12}^{86} = n_{GM9}^{133} n_{GM8}^{86} = n_{GM7}^{133} n_{GM10}^{86} = n_{GM9}^{133} n_{GM6}^{86} = \\
 n_{GM7}^{133} n_{X2}^{86} &= n_{X3}^{133} + n_{X4}^{133} n_{M3}^{86} = n_{M5}^{133} n_{M4}^{86} = n_{M5}^{133} n_{A10}^{86} = n_{A8}^{133} n_{A6}^{86} = n_{A6}^{133} n_{A12}^{86} = n_{A6}^{133} n_{A8}^{86} = n_{A8}^{133} n_{A11}^{86} = n_{A5}^{133} n_{A7}^{86} = \\
 n_{A7}^{133} n_{A9}^{86} &= n_{A7}^{133} n_{A5}^{86} = n_{A5}^{133} n_{R2}^{86} = n_{R3}^{133} + n_{R4}^{133} n_{Z4}^{86} = n_{Z5}^{133} n_{Z3}^{86} = n_{Z5}^{133}
 \end{aligned}$$

#### 46. Lowered SGs by higher-dimensional irreps of pairings in SG 134

The representative operations of SG/T for SG 134:

$$1 : (x, y, z), 2 : (\frac{1}{2} - y, x, z + \frac{1}{2}), 3 : (y, \frac{1}{2} - x, z + \frac{1}{2}), 4 : (x, \frac{1}{2} - y, \frac{1}{2} - z), 5 : (\frac{1}{2} - x, y, \frac{1}{2} - z), 6 : (\frac{1}{2} - x, \frac{1}{2} - y, z), 7 : (y, x, -z), 8 : (\frac{1}{2} - y, \frac{1}{2} - x, -z), 9 : (-x, -y, -z), 10 : (y + \frac{1}{2}, -x, \frac{1}{2} - z), 11 : (-y, x + \frac{1}{2}, \frac{1}{2} - z), 12 : (-x, y + \frac{1}{2}, z + \frac{1}{2}), 13 : (x + \frac{1}{2}, -y, z + \frac{1}{2}), 14 : (x + \frac{1}{2}, y + \frac{1}{2}, -z), 15 : (-y, -x, z), 16 : (y + \frac{1}{2}, x + \frac{1}{2}, z).$$

The lower SG is SG 48 when the preserved operations are: **(sub-SG label is 1) 1, 4, 5, 6, 9, 12, 13, 14.**

The transformation is:  $(\mathbf{a}_{48}, \mathbf{b}_{48}, \mathbf{c}_{48}) = (\mathbf{a}_{134}, \mathbf{b}_{134}, \mathbf{c}_{134}) \begin{pmatrix} 0 & 0 & 1 \\ 1 & 0 & 0 \\ 0 & 1 & 0 \end{pmatrix}, \overrightarrow{O_{134}O_{48}} = \mathbf{a}_{48} + (\frac{1}{2})\mathbf{c}_{48}$

The reduction of higher dimensional irrep:

$$D_{4h} : E_g \rightarrow B_{1g} + B_{3g} \text{ of } D_{2h}.$$

$$D_{4h} : E_u \rightarrow B_{1u} + B_{3u} \text{ of } D_{2h}.$$

The correspondences of irreps at HSPs from original SG to lowered SG:

$$\begin{aligned} n_{GM6}^{48} &= n_{GM8}^{134} + n_{GM9}^{134} & n_{GM5}^{48} &= n_{GM6}^{134} + n_{GM7}^{134} & n_{X4}^{48} &= n_{X4}^{134} & n_{X3}^{48} &= n_{X3}^{134} & n_{S3}^{48} &= n_{R3}^{134} & n_{S4}^{48} &= n_{R4}^{134} & n_{R6}^{48} &= n_{A6}^{134} + n_{A7}^{134} & n_{R5}^{48} &= \\ n_{A8}^{134} + n_{A9}^{134} & n_{U3}^{48} &= n_{M5}^{134} & n_{U4}^{48} &= n_{M5}^{134} & n_{Z4}^{48} &= n_{X3}^{134} & n_{Z3}^{48} &= n_{X4}^{134} & n_{T4}^{48} &= n_{R3}^{134} & n_{T3}^{48} &= n_{R4}^{134} & n_{Y4}^{48} &= n_{Z5}^{134} & n_{Y3}^{48} &= n_{Z5}^{134} \end{aligned}$$

The lower SG is SG 67 when the preserved operations are: **(sub-SG label is 2) 1, 6, 7, 8, 9, 14, 15, 16.**

The transformation is:  $(\mathbf{a}_{67}, \mathbf{b}_{67}, \mathbf{c}_{67}) = (\mathbf{a}_{134}, \mathbf{b}_{134}, \mathbf{c}_{134}) \begin{pmatrix} 1 & -1 & 0 \\ 1 & 1 & 0 \\ 0 & 0 & 1 \end{pmatrix}, \overrightarrow{O_{134}O_{67}} = \frac{1}{2}\mathbf{a}_{67} + (\frac{1}{2})\mathbf{b}_{67} + (\frac{1}{2})\mathbf{c}_{67}$

The reduction of higher dimensional irrep:

$$D_{4h} : E_g \rightarrow B_{2g} + B_{3g} \text{ of } D_{2h}.$$

$$D_{4h} : E_u \rightarrow B_{2u} + B_{3u} \text{ of } D_{2h}.$$

The correspondences of irreps at HSPs from original SG to lowered SG:

$$\begin{aligned} n_{GM6}^{67} &= n_{GM8}^{134} + n_{GM9}^{134} & n_{GM5}^{67} &= n_{GM6}^{134} + n_{GM7}^{134} & n_{Y6}^{67} &= n_{M5}^{134} & n_{Y5}^{67} &= n_{M5}^{134} & n_{S2}^{67} &= n_{X3}^{134} + n_{X4}^{134} & n_{Z6}^{67} &= n_{Z5}^{134} & n_{Z5}^{67} &= n_{Z5}^{134} & n_{T6}^{67} &= \\ n_{A6}^{134} + n_{A7}^{134} & n_{T5}^{67} &= n_{A8}^{134} + n_{A9}^{134} & n_{R2}^{67} &= n_{R3}^{134} + n_{R4}^{134} \end{aligned}$$

The lower SG is SG 86 when the preserved operations are: **(sub-SG label is 3) 1, 2, 3, 6, 9, 10, 11, 14.**

The transformation is:  $(\mathbf{a}_{86}, \mathbf{b}_{86}, \mathbf{c}_{86}) = (\mathbf{a}_{134}, \mathbf{b}_{134}, \mathbf{c}_{134}) \begin{pmatrix} -1 & 0 & 0 \\ 0 & 1 & 0 \\ 0 & 0 & -1 \end{pmatrix}, \overrightarrow{O_{134}O_{86}} = \mathbf{b}_{86} + (\frac{1}{2})\mathbf{c}_{86}$

The reduction of higher dimensional irrep:

$$D_{4h} : E_g \rightarrow {}^2E_g + {}^1E_g \text{ of } C_{4h}.$$

$$D_{4h} : E_u \rightarrow {}^2E_u + {}^1E_u \text{ of } C_{4h}.$$

The correspondences of irreps at HSPs from original SG to lowered SG:

$$\begin{aligned} n_{GM9}^{86} &= n_{GM8}^{134} & n_{GM5}^{86} &= n_{GM6}^{134} & n_{GM11}^{86} &= n_{GM8}^{134} & n_{GM7}^{86} &= n_{GM6}^{134} & n_{GM12}^{86} &= n_{GM9}^{134} & n_{GM8}^{86} &= n_{GM7}^{134} & n_{GM10}^{86} &= n_{GM9}^{134} & n_{GM6}^{86} &= \\ n_{GM7}^{134} & n_{X2}^{86} &= n_{X3}^{134} + n_{X4}^{134} & n_{M3}^{86} &= n_{M5}^{134} & n_{M4}^{86} &= n_{M5}^{134} & n_{A10}^{86} &= n_{A7}^{134} & n_{A6}^{86} &= n_{A9}^{134} & n_{A12}^{86} &= n_{A7}^{134} & n_{A8}^{86} &= n_{A9}^{134} & n_{A11}^{86} &= n_{A6}^{134} & n_{A7}^{86} &= \\ n_{A8}^{134} & n_{A9}^{86} &= n_{A6}^{134} & n_{A5}^{86} &= n_{A8}^{134} & n_{R2}^{86} &= n_{R3}^{134} + n_{R4}^{134} & n_{Z4}^{86} &= n_{Z5}^{134} & n_{Z3}^{86} &= n_{Z5}^{134} \end{aligned}$$

#### 47. Lowered SGs by higher-dimensional irreps of pairings in SG 135

The representative operations of SG/T for SG 135:

$$1 : (x, y, z), 2 : (-y, x, z + \frac{1}{2}), 3 : (y, -x, z + \frac{1}{2}), 4 : (x + \frac{1}{2}, \frac{1}{2} - y, -z), 5 : (\frac{1}{2} - x, y + \frac{1}{2}, -z), 6 : (-x, -y, z), 7 : (y + \frac{1}{2}, x + \frac{1}{2}, \frac{1}{2} - z), 8 : (\frac{1}{2} - y, \frac{1}{2} - x, \frac{1}{2} - z), 9 : (-x, -y, -z), 10 : (y, -x, \frac{1}{2} - z), 11 : (-y, x, \frac{1}{2} - z), 12 : (\frac{1}{2} - x, y + \frac{1}{2}, z), 13 : (x + \frac{1}{2}, \frac{1}{2} - y, z), 14 : (x, y, -z), 15 : (\frac{1}{2} - y, \frac{1}{2} - x, z + \frac{1}{2}), 16 : (y + \frac{1}{2}, x + \frac{1}{2}, z + \frac{1}{2}).$$

The lower SG is SG 55 when the preserved operations are: **(sub-SG label is 1) 1, 4, 5, 6, 9, 12, 13, 14.**

$$\text{The transformation is: } (\mathbf{a}_{55}, \mathbf{b}_{55}, \mathbf{c}_{55}) = (\mathbf{a}_{135}, \mathbf{b}_{135}, \mathbf{c}_{135}) \begin{pmatrix} 1 & 0 & 0 \\ 0 & 1 & 0 \\ 0 & 0 & 1 \end{pmatrix}, \overrightarrow{O_{135}O_{55}} = \frac{1}{2}\mathbf{c}_{55}$$

The reduction of higher dimensional irrep:

$$D_{4h} : E_g \rightarrow B_{2g} + B_{3g} \text{ of } D_{2h}.$$

$$D_{4h} : E_u \rightarrow B_{2u} + B_{3u} \text{ of } D_{2h}.$$

The correspondences of irreps at HSPs from original SG to lowered SG:

$$\begin{aligned} n_{GM6}^{55} &= n_{GM8}^{135} + n_{GM9}^{135} & n_{GM5}^{55} &= n_{GM6}^{135} + n_{GM7}^{135} & n_{X4}^{55} &= n_{X4}^{135} & n_{X3}^{55} &= n_{X3}^{135} & n_{S6}^{55} &= n_{M8}^{135} + n_{M9}^{135} & n_{S5}^{55} &= n_{M6}^{135} + n_{M7}^{135} & n_{R6}^{55} &= \\ n_{A5}^{135} & n_{R5}^{55} = n_{A5}^{135} & n_{U4}^{55} &= n_{R4}^{135} & n_{U3}^{55} &= n_{R3}^{135} & n_{Z6}^{55} &= n_{Z5}^{135} & n_{Z5}^{55} &= n_{Z5}^{135} & n_{T4}^{55} &= n_{R4}^{135} & n_{T3}^{55} &= n_{R3}^{135} & n_{Y4}^{55} &= n_{X4}^{135} & n_{Y3}^{55} &= n_{X3}^{135} \end{aligned}$$

The lower SG is SG 66 when the preserved operations are: **(sub-SG label is 2) 1, 6, 7, 8, 9, 14, 15, 16.**

$$\text{The transformation is: } (\mathbf{a}_{66}, \mathbf{b}_{66}, \mathbf{c}_{66}) = (\mathbf{a}_{135}, \mathbf{b}_{135}, \mathbf{c}_{135}) \begin{pmatrix} 1 & -1 & 0 \\ 1 & 1 & 0 \\ 0 & 0 & 1 \end{pmatrix}, \overrightarrow{O_{135}O_{66}} = -\frac{1}{4}\mathbf{a}_{66} + \left(\frac{1}{4}\right)\mathbf{b}_{66} + \left(\frac{1}{2}\right)\mathbf{c}_{66}$$

The reduction of higher dimensional irrep:

$$D_{4h} : E_g \rightarrow B_{2g} + B_{3g} \text{ of } D_{2h}.$$

$$D_{4h} : E_u \rightarrow B_{2u} + B_{3u} \text{ of } D_{2h}.$$

The correspondences of irreps at HSPs from original SG to lowered SG:

$$\begin{aligned} n_{GM6}^{66} &= n_{GM8}^{135} + n_{GM9}^{135} & n_{GM5}^{66} &= n_{GM6}^{135} + n_{GM7}^{135} & n_{Y6}^{66} &= n_{M6}^{135} + n_{M7}^{135} & n_{Y5}^{66} &= n_{M8}^{135} + n_{M9}^{135} & n_{S6}^{66} &= n_{X4}^{135} & n_{S4}^{66} &= n_{X4}^{135} & n_{S5}^{66} &= \\ n_{X3}^{135} & n_{S3}^{66} = n_{X3}^{135} & n_{Z4}^{66} &= n_{Z5}^{135} & n_{Z3}^{66} &= n_{Z5}^{135} & n_{T4}^{66} &= n_{A5}^{135} & n_{T3}^{66} &= n_{A5}^{135} & n_{R6}^{66} &= n_{R4}^{135} & n_{R4}^{66} &= n_{R4}^{135} & n_{R5}^{66} &= n_{R3}^{135} & n_{R3}^{66} &= n_{R3}^{135} \end{aligned}$$

The lower SG is SG 84 when the preserved operations are: **(sub-SG label is 3) 1, 2, 3, 6, 9, 10, 11, 14.**

$$\text{The transformation is: } (\mathbf{a}_{84}, \mathbf{b}_{84}, \mathbf{c}_{84}) = (\mathbf{a}_{135}, \mathbf{b}_{135}, \mathbf{c}_{135}) \begin{pmatrix} -1 & 0 & 0 \\ 0 & -1 & 0 \\ 0 & 0 & 1 \end{pmatrix}, \overrightarrow{O_{135}O_{84}} = \frac{1}{2}\mathbf{a}_{84} + \left(\frac{1}{2}\right)\mathbf{b}_{84} + \left(\frac{1}{2}\right)\mathbf{c}_{84}$$

The reduction of higher dimensional irrep:

$$D_{4h} : E_g \rightarrow {}^2E_g + {}^1E_g \text{ of } C_{4h}.$$

$$D_{4h} : E_u \rightarrow {}^2E_u + {}^1E_u \text{ of } C_{4h}.$$

The correspondences of irreps at HSPs from original SG to lowered SG:

$$\begin{aligned} n_{GM9}^{84} &= n_{GM8}^{135} & n_{GM5}^{84} &= n_{GM6}^{135} & n_{GM11}^{84} &= n_{GM8}^{135} & n_{GM7}^{84} &= n_{GM6}^{135} & n_{GM12}^{84} &= n_{GM9}^{135} & n_{GM8}^{84} &= n_{GM7}^{135} & n_{GM10}^{84} &= n_{GM9}^{135} & n_{GM6}^{84} &= \\ n_{GM7}^{135} & n_{X6}^{84} = n_{X3}^{135} & n_{X4}^{84} &= n_{X3}^{135} & n_{X5}^{84} &= n_{X4}^{135} & n_{X3}^{84} &= n_{X4}^{135} & n_{M9}^{84} &= n_{M9}^{135} & n_{M5}^{84} &= n_{M7}^{135} & n_{M11}^{84} &= n_{M8}^{135} & n_{M7}^{84} &= n_{M6}^{135} & n_{M12}^{84} &= n_{M9}^{135} \\ n_{M8}^{84} &= n_{M7}^{135} & n_{M10}^{84} &= n_{M8}^{135} & n_{M6}^{84} &= n_{M6}^{135} & n_{A4}^{84} &= n_{A5}^{135} & n_{A3}^{84} &= n_{A5}^{135} & n_{R4}^{84} &= n_{R3}^{135} & n_{R6}^{84} &= n_{R3}^{135} & n_{R3}^{84} &= n_{R4}^{135} & n_{R5}^{84} &= n_{R4}^{135} & n_{Z4}^{84} &= \\ n_{Z5}^{135} & n_{Z3}^{84} = n_{Z5}^{135} \end{aligned}$$

#### 48. Lowered SGs by higher-dimensional irreps of pairings in SG 136

The representative operations of SG/T for SG 136:

$$\begin{aligned} 1 : (x, y, z), & 2 : \left(\frac{1}{2} - y, x + \frac{1}{2}, z + \frac{1}{2}\right), & 3 : \left(y + \frac{1}{2}, \frac{1}{2} - x, z + \frac{1}{2}\right), & 4 : \left(x + \frac{1}{2}, \frac{1}{2} - y, \frac{1}{2} - z\right), & 5 : \left(\frac{1}{2} - x, y + \frac{1}{2}, \frac{1}{2} - z\right), \\ 6 : (-x, -y, z), & 7 : (y, x, -z), & 8 : (-y, -x, -z), & 9 : (-x, -y, -z), & 10 : \left(y + \frac{1}{2}, \frac{1}{2} - x, \frac{1}{2} - z\right), & 11 : \left(\frac{1}{2} - y, x + \frac{1}{2}, \frac{1}{2} - z\right), \\ 12 : \left(\frac{1}{2} - x, y + \frac{1}{2}, z + \frac{1}{2}\right), & 13 : \left(x + \frac{1}{2}, \frac{1}{2} - y, z + \frac{1}{2}\right), & 14 : (x, y, -z), & 15 : (-y, -x, z), & 16 : (y, x, z). \end{aligned}$$

The lower SG is SG 58 when the preserved operations are: **(sub-SG label is 1) 1, 4, 5, 6, 9, 12, 13, 14.**

$$\text{The transformation is: } (\mathbf{a}_{58}, \mathbf{b}_{58}, \mathbf{c}_{58}) = (\mathbf{a}_{136}, \mathbf{b}_{136}, \mathbf{c}_{136}) \begin{pmatrix} 1 & 0 & 0 \\ 0 & 1 & 0 \\ 0 & 0 & 1 \end{pmatrix}, \overrightarrow{O_{136}O_{58}} = \frac{1}{2}\mathbf{a}_{58}$$

The reduction of higher dimensional irrep:

$$D_{4h} : E_g \rightarrow B_{2g} + B_{3g} \text{ of } D_{2h}.$$

$$D_{4h} : E_u \rightarrow B_{2u} + B_{3u} \text{ of } D_{2h}.$$

The correspondences of irreps at HSPs from original SG to lowered SG:

$$n_{GM6}^{58} = n_{GM8}^{136} + n_{GM9}^{136} \quad n_{GM5}^{58} = n_{GM6}^{136} + n_{GM7}^{136} \quad n_{X4}^{58} = n_{X4}^{136} \quad n_{X3}^{58} = n_{X3}^{136} \quad n_{S6}^{58} = n_{M6}^{136} + n_{M7}^{136} \quad n_{S5}^{58} = n_{M8}^{136} + n_{M9}^{136} \quad n_{R4}^{58} =$$

$$\begin{aligned} n_{A_5}^{136} n_{R_3}^{58} &= n_{A_5}^{136} n_{U_7}^{58} = n_{R_3}^{136} n_{U_3}^{58} = n_{R_7}^{136} n_{U_6}^{58} = n_{R_4}^{136} n_{U_2}^{58} = n_{R_8}^{136} n_{U_8}^{58} = n_{R_2}^{136} n_{U_4}^{58} = n_{R_6}^{136} n_{U_9}^{58} = n_{R_5}^{136} n_{U_5}^{58} = n_{R_9}^{136} n_{Z_4}^{58} = \\ n_{Z_5}^{136} n_{Z_3}^{58} &= n_{Z_5}^{136} n_{T_8}^{58} = n_{R_8}^{136} n_{T_4}^{58} = n_{R_4}^{136} n_{T_9}^{58} = n_{R_9}^{136} n_{T_5}^{58} = n_{R_5}^{136} n_{T_7}^{58} = n_{R_7}^{136} n_{T_3}^{58} = n_{R_3}^{136} n_{T_6}^{58} = n_{R_6}^{136} n_{T_2}^{58} = n_{R_2}^{136} n_{Y_4}^{58} = \\ n_{X_4}^{136} n_{Y_3}^{58} &= n_{X_3}^{136} \end{aligned}$$

The lower SG is SG 65 when the preserved operations are: **(sub-SG label is 2) 1, 6, 7, 8, 9, 14, 15, 16.**

The transformation is:  $(\mathbf{a}_{65}, \mathbf{b}_{65}, \mathbf{c}_{65}) = (\mathbf{a}_{136}, \mathbf{b}_{136}, \mathbf{c}_{136}) \begin{pmatrix} 1 & -1 & 0 \\ 1 & 1 & 0 \\ 0 & 0 & 1 \end{pmatrix}, \overrightarrow{O_{136}O_{65}} = \frac{1}{2}\mathbf{c}_{65}$

The reduction of higher dimensional irrep:

$$D_{4h} : E_g \rightarrow B_{2g} + B_{3g} \text{ of } D_{2h}.$$

$$D_{4h} : E_u \rightarrow B_{2u} + B_{3u} \text{ of } D_{2h}.$$

The correspondences of irreps at HSPs from original SG to lowered SG:

$$\begin{aligned} n_{GM6}^{65} &= n_{GM8}^{136} + n_{GM9}^{136} \quad n_{GM5}^{65} = n_{GM6}^{136} + n_{GM7}^{136} \quad n_{Y6}^{65} = n_{M8}^{136} + n_{M9}^{136} \quad n_{Y5}^{65} = n_{M6}^{136} + n_{M7}^{136} \quad n_{S6}^{65} = n_{X4}^{136} \quad n_{S4}^{65} = n_{X4}^{136} \quad n_{S5}^{65} = \\ n_{X3}^{136} n_{S3}^{65} &= n_{X3}^{136} n_{Z5}^{65} = n_{Z5}^{136} n_{Z5}^{65} = n_{Z5}^{136} n_{T6}^{65} = n_{A5}^{136} n_{T5}^{65} = n_{A5}^{136} n_{R6}^{65} = n_{R3}^{136} + n_{R5}^{136} \quad n_{R4}^{65} = n_{R7}^{136} + n_{R9}^{136} \quad n_{R5}^{65} = n_{R2}^{136} + n_{R4}^{136} \\ n_{R3}^{65} &= n_{R6}^{136} + n_{R8}^{136} \end{aligned}$$

The lower SG is SG 84 when the preserved operations are: **(sub-SG label is 3) 1, 2, 3, 6, 9, 10, 11, 14.**

The transformation is:  $(\mathbf{a}_{84}, \mathbf{b}_{84}, \mathbf{c}_{84}) = (\mathbf{a}_{136}, \mathbf{b}_{136}, \mathbf{c}_{136}) \begin{pmatrix} -1 & 0 & 0 \\ 0 & -1 & 0 \\ 0 & 0 & 1 \end{pmatrix}, \overrightarrow{O_{136}O_{84}} = \frac{1}{2}\mathbf{b}_{84} + (\frac{1}{2})\mathbf{c}_{84}$

The reduction of higher dimensional irrep:

$$D_{4h} : E_g \rightarrow {}^2E_g + {}^1E_g \text{ of } C_{4h}.$$

$$D_{4h} : E_u \rightarrow {}^2E_u + {}^1E_u \text{ of } C_{4h}.$$

The correspondences of irreps at HSPs from original SG to lowered SG:

$$\begin{aligned} n_{GM9}^{84} &= n_{GM8}^{136} \quad n_{GM5}^{84} = n_{GM6}^{136} \quad n_{GM11}^{84} = n_{GM8}^{136} \quad n_{GM7}^{84} = n_{GM6}^{136} \quad n_{GM12}^{84} = n_{GM9}^{136} \quad n_{GM8}^{84} = n_{GM7}^{136} \quad n_{GM10}^{84} = n_{GM9}^{136} \quad n_{GM6}^{84} = \\ n_{GM7}^{136} n_{X6}^{84} &= n_{X3}^{136} n_{X4}^{84} = n_{X3}^{136} n_{X5}^{84} = n_{X4}^{136} n_{X3}^{84} = n_{X4}^{136} n_{M7}^{84} = n_{M7}^{136} n_{M5}^{84} = n_{M9}^{136} n_{M11}^{84} = n_{M6}^{136} n_{M7}^{84} = n_{M8}^{136} n_{M12}^{84} = n_{M7}^{136} \\ n_{M8}^{84} &= n_{M9}^{136} \quad n_{M10}^{84} = n_{M6}^{136} \quad n_{M6}^{84} = n_{M8}^{136} \quad n_{A4}^{84} = n_{A5}^{136} \quad n_{A3}^{84} = n_{A5}^{136} \quad n_{R4}^{84} = n_{R2}^{136} + n_{R4}^{136} \quad n_{R6}^{84} = n_{R6}^{136} + n_{R8}^{136} \quad n_{R3}^{84} = n_{R3}^{136} + n_{R5}^{136} \\ n_{R5}^{84} &= n_{R7}^{136} + n_{R9}^{136} \quad n_{Z4}^{84} = n_{Z5}^{136} \quad n_{Z3}^{84} = n_{Z5}^{136} \end{aligned}$$

#### 49. Lowered SGs by higher-dimensional irreps of pairings in SG 137

The representative operations of SG/T for SG 137:

$$\begin{aligned} 1 : (x, y, z), \quad 2 : (\frac{1}{2} - y, x, z + \frac{1}{2}), \quad 3 : (y, \frac{1}{2} - x, z + \frac{1}{2}), \quad 4 : (x + \frac{1}{2}, -y, -z), \quad 5 : (-x, y + \frac{1}{2}, -z), \quad 6 : (\frac{1}{2} - x, \frac{1}{2} - y, z), \\ 7 : (y + \frac{1}{2}, x + \frac{1}{2}, \frac{1}{2} - z), \quad 8 : (-y, -x, \frac{1}{2} - z), \quad 9 : (-x, -y, -z), \quad 10 : (y + \frac{1}{2}, -x, \frac{1}{2} - z), \quad 11 : (-y, x + \frac{1}{2}, \frac{1}{2} - z), \\ 12 : (\frac{1}{2} - x, y, z), \quad 13 : (x, \frac{1}{2} - y, z), \quad 14 : (x + \frac{1}{2}, y + \frac{1}{2}, -z), \quad 15 : (\frac{1}{2} - y, \frac{1}{2} - x, z + \frac{1}{2}), \quad 16 : (y, x, z + \frac{1}{2}). \end{aligned}$$

The lower SG is SG 59 when the preserved operations are: **(sub-SG label is 1) 1, 4, 5, 6, 9, 12, 13, 14.**

The transformation is:  $(\mathbf{a}_{59}, \mathbf{b}_{59}, \mathbf{c}_{59}) = (\mathbf{a}_{137}, \mathbf{b}_{137}, \mathbf{c}_{137}) \begin{pmatrix} 1 & 0 & 0 \\ 0 & 1 & 0 \\ 0 & 0 & 1 \end{pmatrix}, \overrightarrow{O_{137}O_{59}} = \frac{1}{2}\mathbf{b}_{59}$

The reduction of higher dimensional irrep:

$$D_{4h} : E_g \rightarrow B_{2g} + B_{3g} \text{ of } D_{2h}.$$

$$D_{4h} : E_u \rightarrow B_{2u} + B_{3u} \text{ of } D_{2h}.$$

The correspondences of irreps at HSPs from original SG to lowered SG:

$$\begin{aligned} n_{GM6}^{59} &= n_{GM8}^{137} + n_{GM9}^{137} \quad n_{GM5}^{59} = n_{GM6}^{137} + n_{GM7}^{137} \quad n_{X4}^{59} = n_{X3}^{137} \quad n_{X3}^{59} = n_{X4}^{137} \quad n_{S3}^{59} = n_{M5}^{137} \quad n_{S4}^{59} = n_{M5}^{137} \quad n_{R3}^{59} = n_{A5}^{137} + n_{A6}^{137} \quad n_{R4}^{59} = \\ n_{A7}^{137} + n_{A8}^{137} \quad n_{U4}^{59} &= n_{R4}^{137} \quad n_{U3}^{59} = n_{R3}^{137} \quad n_{Z6}^{59} = n_{Z5}^{137} \quad n_{Z5}^{59} = n_{Z5}^{137} \quad n_{T4}^{59} = n_{R3}^{137} \quad n_{T3}^{59} = n_{R4}^{137} \quad n_{Y4}^{59} = n_{X3}^{137} \quad n_{Y3}^{59} = n_{X4}^{137} \end{aligned}$$

The lower SG is SG 68 when the preserved operations are: **(sub-SG label is 2) 1, 6, 7, 8, 9, 14, 15, 16.**

The transformation is:  $(\mathbf{a}_{68}, \mathbf{b}_{68}, \mathbf{c}_{68}) = (\mathbf{a}_{137}, \mathbf{b}_{137}, \mathbf{c}_{137}) \begin{pmatrix} 1 & -1 & 0 \\ 1 & 1 & 0 \\ 0 & 0 & 1 \end{pmatrix}, \overrightarrow{O_{137}O_{68}} = \mathbf{b}_{68}$

The reduction of higher dimensional irrep:

$$D_{4h} : E_g \rightarrow B_{2g} + B_{3g} \text{ of } D_{2h}.$$

$$D_{4h} : E_u \rightarrow B_{2u} + B_{3u} \text{ of } D_{2h}.$$

The correspondences of irreps at HSPs from original SG to lowered SG:

$$n_{GM6}^{68} = n_{GM8}^{137} + n_{GM9}^{137} n_{GM5}^{68} = n_{GM6}^{137} + n_{GM7}^{137} n_{Y6}^{68} = n_{M5}^{137} n_{Y5}^{68} = n_{M5}^{137} n_{S2}^{68} = n_{X3}^{137} + n_{X4}^{137} n_{Z4}^{68} = n_{Z5}^{137} n_{Z3}^{68} = n_{Z5}^{137} n_{T4}^{68} =$$

$$n_{A5}^{137} + n_{A6}^{137} n_{T3}^{68} = n_{A7}^{137} + n_{A8}^{137} n_{R2}^{68} = n_{R3}^{137} + n_{R4}^{137}$$

The lower SG is SG 86 when the preserved operations are: **(sub-SG label is 3) 1, 2, 3, 6, 9, 10, 11, 14.**

The transformation is:  $(\mathbf{a}_{86}, \mathbf{b}_{86}, \mathbf{c}_{86}) = (\mathbf{a}_{137}, \mathbf{b}_{137}, \mathbf{c}_{137}) \begin{pmatrix} -1 & 0 & 0 \\ 0 & -1 & 0 \\ 0 & 0 & 1 \end{pmatrix}, \overrightarrow{O_{137}O_{86}} = \frac{1}{2}\mathbf{a}_{86}$

The reduction of higher dimensional irrep:

$$D_{4h} : E_g \rightarrow {}^2E_g + {}^1E_g \text{ of } C_{4h}.$$

$$D_{4h} : E_u \rightarrow {}^2E_u + {}^1E_u \text{ of } C_{4h}.$$

The correspondences of irreps at HSPs from original SG to lowered SG:

$$n_{GM9}^{86} = n_{GM8}^{137} n_{GM5}^{86} = n_{GM6}^{137} n_{GM11}^{86} = n_{GM8}^{137} n_{GM7}^{86} = n_{GM6}^{137} n_{GM12}^{86} = n_{GM9}^{137} n_{GM8}^{86} = n_{GM7}^{137} n_{GM10}^{86} = n_{GM9}^{137} n_{GM6}^{86} =$$

$$n_{GM7}^{137} n_{X2}^{86} = n_{X3}^{137} + n_{X4}^{137} n_{M3}^{86} = n_{M5}^{137} n_{M4}^{86} = n_{M5}^{137} n_{A10}^{86} = n_{A7}^{137} n_{A6}^{86} = n_{A6}^{137} n_{A12}^{86} = n_{A5}^{137} n_{A8}^{86} = n_{A8}^{137} n_{A11}^{86} = n_{A6}^{137} n_{A7}^{86} =$$

$$n_{A7}^{137} n_{A9}^{86} = n_{A8}^{137} n_{A5}^{86} = n_{A5}^{137} n_{R2}^{86} = n_{R3}^{137} + n_{R4}^{137} n_{Z4}^{86} = n_{Z5}^{137} n_{Z3}^{86} = n_{Z5}^{137}$$

**50. Lowered SGs by higher-dimensional irreps of pairings in SG 138**

The representative operations of SG/T for SG 138:

$$1 : (x, y, z), 2 : (\frac{1}{2} - y, x, z + \frac{1}{2}), 3 : (y, \frac{1}{2} - x, z + \frac{1}{2}), 4 : (x + \frac{1}{2}, -y, \frac{1}{2} - z), 5 : (-x, y + \frac{1}{2}, \frac{1}{2} - z), 6 : (\frac{1}{2} - x, \frac{1}{2} - y, z),$$

$$7 : (y + \frac{1}{2}, x + \frac{1}{2}, -z), 8 : (-y, -x, -z), 9 : (-x, -y, -z), 10 : (y + \frac{1}{2}, -x, \frac{1}{2} - z), 11 : (-y, x + \frac{1}{2}, \frac{1}{2} - z),$$

$$12 : (\frac{1}{2} - x, y, z + \frac{1}{2}), 13 : (x, \frac{1}{2} - y, z + \frac{1}{2}), 14 : (x + \frac{1}{2}, y + \frac{1}{2}, -z), 15 : (\frac{1}{2} - y, \frac{1}{2} - x, z), 16 : (y, x, z).$$

The lower SG is SG 56 when the preserved operations are: **(sub-SG label is 1) 1, 4, 5, 6, 9, 12, 13, 14.**

The transformation is:  $(\mathbf{a}_{56}, \mathbf{b}_{56}, \mathbf{c}_{56}) = (\mathbf{a}_{138}, \mathbf{b}_{138}, \mathbf{c}_{138}) \begin{pmatrix} 1 & 0 & 0 \\ 0 & 1 & 0 \\ 0 & 0 & 1 \end{pmatrix}, \overrightarrow{O_{138}O_{56}} = \mathbf{b}_{56} + (\frac{1}{2})\mathbf{c}_{56}$

The reduction of higher dimensional irrep:

$$D_{4h} : E_g \rightarrow B_{2g} + B_{3g} \text{ of } D_{2h}.$$

$$D_{4h} : E_u \rightarrow B_{2u} + B_{3u} \text{ of } D_{2h}.$$

The correspondences of irreps at HSPs from original SG to lowered SG:

$$n_{GM6}^{56} = n_{GM8}^{138} + n_{GM9}^{138} n_{GM5}^{56} = n_{GM6}^{138} + n_{GM7}^{138} n_{Y6}^{56} = n_{M5}^{138} n_{Y5}^{56} = n_{M5}^{138} n_{S3}^{56} = n_{X4}^{138} n_{S4}^{56} = n_{M5}^{138} n_{B6}^{56} = n_{A6}^{138} + n_{A7}^{138} n_{R5}^{56} =$$

$$n_{A8}^{138} + n_{A9}^{138} n_{U3}^{56} = n_{R3}^{138} n_{U4}^{56} = n_{R4}^{138} n_{Z4}^{56} = n_{Z5}^{138} n_{Z3}^{56} = n_{Z5}^{138} n_{T4}^{56} = n_{R3}^{138} n_{T3}^{56} = n_{R4}^{138} n_{Y4}^{56} = n_{X4}^{138} n_{Y3}^{56} = n_{X3}^{138}$$

The lower SG is SG 67 when the preserved operations are: **(sub-SG label is 2) 1, 6, 7, 8, 9, 14, 15, 16.**

The transformation is:  $(\mathbf{a}_{67}, \mathbf{b}_{67}, \mathbf{c}_{67}) = (\mathbf{a}_{138}, \mathbf{b}_{138}, \mathbf{c}_{138}) \begin{pmatrix} 1 & -1 & 0 \\ 1 & 1 & 0 \\ 0 & 0 & 1 \end{pmatrix}, \overrightarrow{O_{138}O_{67}} = \frac{1}{4}\mathbf{a}_{67} + (\frac{3}{4})\mathbf{b}_{67} + (\frac{1}{2})\mathbf{c}_{67}$

The reduction of higher dimensional irrep:

$$D_{4h} : E_g \rightarrow B_{2g} + B_{3g} \text{ of } D_{2h}.$$

$$D_{4h} : E_u \rightarrow B_{2u} + B_{3u} \text{ of } D_{2h}.$$

The correspondences of irreps at HSPs from original SG to lowered SG:

$$n_{GM6}^{67} = n_{GM8}^{138} + n_{GM9}^{138} n_{GM5}^{67} = n_{GM6}^{138} + n_{GM7}^{138} n_{Y6}^{67} = n_{M5}^{138} n_{Y5}^{67} = n_{M5}^{138} n_{S2}^{67} = n_{X3}^{138} + n_{X4}^{138} n_{Z6}^{67} = n_{Z5}^{138} n_{Z5}^{67} = n_{Z5}^{138} n_{T6}^{67} =$$

$$n_{A8}^{138} + n_{A9}^{138} n_{T5}^{67} = n_{A6}^{138} + n_{A7}^{138} n_{R2}^{67} = n_{R3}^{138} + n_{R4}^{138}$$

The lower SG is SG 86 when the preserved operations are: **(sub-SG label is 3) 1, 2, 3, 6, 9, 10, 11, 14.**

The transformation is:  $(\mathbf{a}_{86}, \mathbf{b}_{86}, \mathbf{c}_{86}) = (\mathbf{a}_{138}, \mathbf{b}_{138}, \mathbf{c}_{138}) \begin{pmatrix} -1 & 0 & 0 \\ 0 & -1 & 0 \\ 0 & 0 & 1 \end{pmatrix}, \overrightarrow{O_{138}O_{86}} = \frac{1}{2}\mathbf{a}_{86} + (\frac{1}{2})\mathbf{c}_{86}$

The reduction of higher dimensional irrep:

$$D_{4h} : E_g \rightarrow {}^2E_g + {}^1E_g \text{ of } C_{4h}.$$

$$D_{4h} : E_u \rightarrow {}^2E_u + {}^1E_u \text{ of } C_{4h}.$$

The correspondences of irreps at HSPs from original SG to lowered SG:

$$\begin{aligned} n_{GM9}^{86} &= n_{GM8}^{138} n_{GM5}^{86} = n_{GM6}^{138} n_{GM11}^{86} = n_{GM8}^{138} n_{GM7}^{86} = n_{GM6}^{138} n_{GM12}^{86} = n_{GM9}^{138} n_{GM8}^{86} = n_{GM7}^{138} n_{GM10}^{86} = n_{GM9}^{138} n_{GM6}^{86} = \\ n_{GM7}^{138} n_{X2}^{86} &= n_{X3}^{138} + n_{X4}^{138} n_{M3}^{86} = n_{M5}^{138} n_{M4}^{86} = n_{M5}^{138} n_{A10}^{86} = n_{A9}^{138} n_{A6}^{86} = n_{A7}^{138} n_{A12}^{86} = n_{A8}^{138} n_{A8}^{86} = n_{A6}^{138} n_{A11}^{86} = n_{A9}^{138} n_{A7}^{86} = \\ n_{A7}^{138} n_{A9}^{86} &= n_{A8}^{138} n_{A5}^{86} = n_{A6}^{138} n_{R2}^{86} = n_{R3}^{138} + n_{R4}^{138} n_{Z4}^{86} = n_{Z5}^{138} n_{Z3}^{86} = n_{Z5}^{138} \end{aligned}$$

### 51. Lowered SGs by higher-dimensional irreps of pairings in SG 139

The representative operations of SG/T for SG 139:

$$\begin{aligned} 1 : (x, y, z), 2 : (-y, x, z), 3 : (y, -x, z), 4 : (x, -y, -z), 5 : (-x, y, -z), 6 : (-x, -y, z), 7 : (y, x, -z), 8 : \\ (-y, -x, -z), 9 : (-x, -y, -z), 10 : (y, -x, -z), 11 : (-y, x, -z), 12 : (-x, y, z), 13 : (x, -y, z), 14 : (x, y, -z), \\ 15 : (-y, -x, z), 16 : (y, x, z). \end{aligned}$$

The lower SG is SG 71 when the preserved operations are: **(sub-SG label is 1) 1, 4, 5, 6, 9, 12, 13, 14.**

$$\text{The transformation is: } (\mathbf{a}_{71}, \mathbf{b}_{71}, \mathbf{c}_{71}) = (\mathbf{a}_{139}, \mathbf{b}_{139}, \mathbf{c}_{139}) \begin{pmatrix} 0 & 0 & 1 \\ 1 & 0 & 0 \\ 0 & 1 & 0 \end{pmatrix}, \overrightarrow{O_{139}O_{71}} = -\frac{1}{2}\mathbf{b}_{71}$$

The reduction of higher dimensional irrep:

$$D_{4h} : E_g \rightarrow B_{1g} + B_{3g} \text{ of } D_{2h}.$$

$$D_{4h} : E_u \rightarrow B_{1u} + B_{3u} \text{ of } D_{2h}.$$

The correspondences of irreps at HSPs from original SG to lowered SG:

$$\begin{aligned} n_{GM6}^{71} &= n_{GM8}^{139} + n_{GM9}^{139} n_{GM5}^{71} = n_{GM6}^{139} + n_{GM7}^{139} n_{X6}^{71} = n_{M8}^{139} + n_{M9}^{139} n_{X5}^{71} = n_{M6}^{139} + n_{M7}^{139} n_{T6}^{71} = n_{N4}^{139} n_{T4}^{71} = n_{N6}^{139} n_{T5}^{71} = \\ n_{N3}^{139} n_{T3}^{71} &= n_{N5}^{139} n_{W5}^{71} = n_{P6}^{139} + n_{P7}^{139} n_{R6}^{71} = n_{X6}^{139} n_{R4}^{71} = n_{X5}^{139} n_{R5}^{71} = n_{X6}^{139} n_{R3}^{71} = n_{X5}^{139} n_{S5}^{71} = n_{N4}^{139} n_{S3}^{71} = n_{N6}^{139} n_{S6}^{71} = n_{N3}^{139} \\ n_{S4}^{71} &= n_{N5}^{139} \end{aligned}$$

The lower SG is SG 69 when the preserved operations are: **(sub-SG label is 2) 1, 6, 7, 8, 9, 14, 15, 16.**

$$\text{The transformation is: } (\mathbf{a}_{69}, \mathbf{b}_{69}, \mathbf{c}_{69}) = (\mathbf{a}_{139}, \mathbf{b}_{139}, \mathbf{c}_{139}) \begin{pmatrix} 1 & -1 & 0 \\ 1 & 1 & 0 \\ 0 & 0 & 1 \end{pmatrix}, \overrightarrow{O_{139}O_{69}} = \mathbf{0}$$

The reduction of higher dimensional irrep:

$$D_{4h} : E_g \rightarrow B_{2g} + B_{3g} \text{ of } D_{2h}.$$

$$D_{4h} : E_u \rightarrow B_{2u} + B_{3u} \text{ of } D_{2h}.$$

The correspondences of irreps at HSPs from original SG to lowered SG:

$$\begin{aligned} n_{GM6}^{69} &= n_{GM8}^{139} + n_{GM9}^{139} n_{GM5}^{69} = n_{GM6}^{139} + n_{GM7}^{139} n_{Y6}^{69} = n_{X6}^{139} n_{Y5}^{69} = n_{X5}^{139} n_{L2}^{69} = n_{N5}^{139} + n_{N6}^{139} n_{L3}^{69} = n_{N3}^{139} + n_{N4}^{139} n_{Z6}^{69} = \\ n_{M8}^{139} + n_{M9}^{139} n_{Z5}^{69} &= n_{M6}^{139} + n_{M7}^{139} n_{T6}^{69} = n_{X6}^{139} n_{T5}^{69} = n_{X5}^{139} \end{aligned}$$

The lower SG is SG 87 when the preserved operations are: **(sub-SG label is 3) 1, 2, 3, 6, 9, 10, 11, 14.**

$$\text{The transformation is: } (\mathbf{a}_{87}, \mathbf{b}_{87}, \mathbf{c}_{87}) = (\mathbf{a}_{139}, \mathbf{b}_{139}, \mathbf{c}_{139}) \begin{pmatrix} 0 & 1 & 0 \\ -1 & 0 & 0 \\ 0 & 0 & 1 \end{pmatrix}, \overrightarrow{O_{139}O_{87}} = \mathbf{0}$$

The reduction of higher dimensional irrep:

$$D_{4h} : E_g \rightarrow {}^2E_g + {}^1E_g \text{ of } C_{4h}.$$

$$D_{4h} : E_u \rightarrow {}^2E_u + {}^1E_u \text{ of } C_{4h}.$$

The correspondences of irreps at HSPs from original SG to lowered SG:

$$\begin{aligned} n_{GM9}^{87} &= n_{GM8}^{139} n_{GM5}^{87} = n_{GM6}^{139} n_{GM11}^{87} = n_{GM8}^{139} n_{GM7}^{87} = n_{GM6}^{139} n_{GM12}^{87} = n_{GM9}^{139} n_{GM8}^{87} = n_{GM7}^{139} n_{GM10}^{87} = n_{GM9}^{139} n_{GM6}^{87} = \\ n_{GM7}^{139} n_{M9}^{87} &= n_{M8}^{139} n_{M5}^{87} = n_{M6}^{139} n_{M11}^{87} = n_{M8}^{139} n_{M7}^{87} = n_{M6}^{139} n_{M12}^{87} = n_{M9}^{139} n_{M8}^{87} = n_{M7}^{139} n_{M10}^{87} = n_{M9}^{139} n_{M6}^{87} = n_{M7}^{139} n_{X6}^{87} = \\ n_{X6}^{139} n_{X4}^{87} &= n_{X5}^{139} n_{X5}^{87} = n_{X6}^{139} n_{X3}^{87} = n_{X5}^{139} n_{P7}^{87} = n_{P7}^{139} n_{P8}^{87} = n_{P6}^{139} n_{P5}^{87} = n_{P7}^{139} n_{P6}^{87} = n_{P6}^{139} n_{N2}^{87} = n_{N5}^{139} + n_{N6}^{139} n_{N3}^{87} = \\ n_{N3}^{139} + n_{N4}^{139} \end{aligned}$$

### 52. Lowered SGs by higher-dimensional irreps of pairings in SG 140

The representative operations of SG/T for SG 140:

$$1 : (x, y, z), 2 : (-y, x, z), 3 : (y, -x, z), 4 : (x, -y, \frac{1}{2} - z), 5 : (-x, y, \frac{1}{2} - z), 6 : (-x, -y, z), 7 : (y, x, \frac{1}{2} - z), \\ 8 : (-y, -x, \frac{1}{2} - z), 9 : (-x, -y, -z), 10 : (y, -x, -z), 11 : (-y, x, -z), 12 : (-x, y, z + \frac{1}{2}), 13 : (x, -y, z + \frac{1}{2}), \\ 14 : (x, y, -z), 15 : (-y, -x, z + \frac{1}{2}), 16 : (y, x, z + \frac{1}{2}).$$

The lower SG is SG 72 when the preserved operations are: **(sub-SG label is 1) 1, 4, 5, 6, 9, 12, 13, 14.**

The transformation is:  $(\mathbf{a}_{72}, \mathbf{b}_{72}, \mathbf{c}_{72}) = (\mathbf{a}_{140}, \mathbf{b}_{140}, \mathbf{c}_{140}) \begin{pmatrix} 1 & 0 & 0 \\ 0 & 1 & 0 \\ 0 & 0 & 1 \end{pmatrix}, \overrightarrow{O_{140}O_{72}} = -\mathbf{b}_{72}$

The reduction of higher dimensional irrep:

$$D_{4h} : E_g \rightarrow B_{2g} + B_{3g} \text{ of } D_{2h}.$$

$$D_{4h} : E_u \rightarrow B_{2u} + B_{3u} \text{ of } D_{2h}.$$

The correspondences of irreps at HSPs from original SG to lowered SG:

$$n_{GM6}^{72} = n_{GM8}^{140} + n_{GM9}^{140} \quad n_{GM5}^{72} = n_{GM6}^{140} + n_{GM7}^{140} \quad n_{X6}^{72} = n_{M8}^{140} + n_{M9}^{140} \quad n_{X5}^{72} = n_{M6}^{140} + n_{M7}^{140} \quad n_{T6}^{72} = n_{X6}^{140} \quad n_{T4}^{72} = n_{X5}^{140} \quad n_{T5}^{72} = \\ n_{X6}^{140} \quad n_{T3}^{72} = n_{X5}^{140} \quad n_{W5}^{72} = n_{P6}^{140} + n_{P7}^{140} \quad n_{R2}^{72} = n_{N2}^{140} \quad n_{S2}^{72} = n_{N2}^{140}$$

The lower SG is SG 69 when the preserved operations are: **(sub-SG label is 2) 1, 6, 7, 8, 9, 14, 15, 16.**

The transformation is:  $(\mathbf{a}_{69}, \mathbf{b}_{69}, \mathbf{c}_{69}) = (\mathbf{a}_{140}, \mathbf{b}_{140}, \mathbf{c}_{140}) \begin{pmatrix} 1 & -1 & 0 \\ 1 & 1 & 0 \\ 0 & 0 & 1 \end{pmatrix}, \overrightarrow{O_{140}O_{69}} = -\frac{1}{4}\mathbf{a}_{69} + (-\frac{1}{4})\mathbf{b}_{69}$

The reduction of higher dimensional irrep:

$$D_{4h} : E_g \rightarrow B_{2g} + B_{3g} \text{ of } D_{2h}.$$

$$D_{4h} : E_u \rightarrow B_{2u} + B_{3u} \text{ of } D_{2h}.$$

The correspondences of irreps at HSPs from original SG to lowered SG:

$$n_{GM6}^{69} = n_{GM8}^{140} + n_{GM9}^{140} \quad n_{GM5}^{69} = n_{GM6}^{140} + n_{GM7}^{140} \quad n_{Y6}^{69} = n_{X5}^{140} \quad n_{Y5}^{69} = n_{X6}^{140} \quad n_{L2}^{69} = n_{N2}^{140} \quad n_{L3}^{69} = n_{N2}^{140} \quad n_{Z6}^{69} = n_{M8}^{140} + n_{M9}^{140} \quad n_{Z5}^{69} = \\ n_{M6}^{140} + n_{M7}^{140} \quad n_{T6}^{69} = n_{X5}^{140} \quad n_{T5}^{69} = n_{X6}^{140}$$

The lower SG is SG 87 when the preserved operations are: **(sub-SG label is 3) 1, 2, 3, 6, 9, 10, 11, 14.**

The transformation is:  $(\mathbf{a}_{87}, \mathbf{b}_{87}, \mathbf{c}_{87}) = (\mathbf{a}_{140}, \mathbf{b}_{140}, \mathbf{c}_{140}) \begin{pmatrix} 0 & 1 & 0 \\ -1 & 0 & 0 \\ 0 & 0 & 1 \end{pmatrix}, \overrightarrow{O_{140}O_{87}} = \mathbf{a}_{87}$

The reduction of higher dimensional irrep:

$$D_{4h} : E_g \rightarrow {}^2E_g + {}^1E_g \text{ of } C_{4h}.$$

$$D_{4h} : E_u \rightarrow {}^2E_u + {}^1E_u \text{ of } C_{4h}.$$

The correspondences of irreps at HSPs from original SG to lowered SG:

$$n_{GM9}^{87} = n_{GM8}^{140} \quad n_{GM5}^{87} = n_{GM6}^{140} \quad n_{GM11}^{87} = n_{GM8}^{140} \quad n_{GM7}^{87} = n_{GM6}^{140} \quad n_{GM12}^{87} = n_{GM9}^{140} \quad n_{GM8}^{87} = n_{GM7}^{140} \quad n_{GM10}^{87} = n_{GM9}^{140} \quad n_{GM6}^{87} = \\ n_{GM7}^{140} \quad n_{M9}^{87} = n_{M8}^{140} \quad n_{M5}^{87} = n_{M6}^{140} \quad n_{M11}^{87} = n_{M8}^{140} \quad n_{M7}^{87} = n_{M6}^{140} \quad n_{M12}^{87} = n_{M9}^{140} \quad n_{M8}^{87} = n_{M7}^{140} \quad n_{M10}^{87} = n_{M9}^{140} \quad n_{M6}^{87} = n_{M7}^{140} \quad n_{X6}^{87} = \\ n_{X6}^{140} \quad n_{X4}^{87} = n_{X5}^{140} \quad n_{X5}^{87} = n_{X6}^{140} \quad n_{X3}^{87} = n_{X5}^{140} \quad n_{P7}^{87} = n_{P6}^{140} \quad n_{P8}^{87} = n_{P7}^{140} \quad n_{P5}^{87} = n_{P7}^{140} \quad n_{P6}^{87} = n_{P6}^{140} \quad n_{N2}^{87} = n_{N2}^{140} \quad n_{N3}^{87} = n_{N2}^{140}$$

### 53. Lowered SGs by higher-dimensional irreps of pairings in SG 141

The representative operations of SG/T for SG 141:

$$1 : (x, y, z), 2 : (\frac{1}{4} - y, x + \frac{3}{4}, z + \frac{1}{4}), 3 : (y + \frac{3}{4}, \frac{3}{4} - x, z + \frac{1}{4}), 4 : (x, -y, -z), 5 : (-x, y + \frac{1}{2}, -z), 6 : (-x, \frac{1}{2} - y, z), \\ 7 : (y + \frac{3}{4}, x + \frac{1}{4}, \frac{3}{4} - z), 8 : (\frac{1}{4} - y, \frac{1}{4} - x, \frac{3}{4} - z), 9 : (-x, -y, -z), 10 : (y + \frac{3}{4}, \frac{1}{4} - x, \frac{3}{4} - z), 11 : (\frac{1}{4} - y, x + \frac{1}{4}, \frac{3}{4} - z), \\ 12 : (-x, y, z), 13 : (x, \frac{1}{2} - y, z), 14 : (x, y + \frac{1}{2}, -z), 15 : (\frac{1}{4} - y, \frac{3}{4} - x, z + \frac{1}{4}), 16 : (y + \frac{3}{4}, x + \frac{3}{4}, z + \frac{1}{4}).$$

The lower SG is SG 74 when the preserved operations are: **(sub-SG label is 1) 1, 4, 5, 6, 9, 12, 13, 14.**

$$\text{The transformation is: } (\mathbf{a}_{74}, \mathbf{b}_{74}, \mathbf{c}_{74}) = (\mathbf{a}_{141}, \mathbf{b}_{141}, \mathbf{c}_{141}) \begin{pmatrix} 0 & 1 & 0 \\ 1 & 0 & 0 \\ 0 & 0 & -1 \end{pmatrix}, \overrightarrow{O_{141}O_{74}} = \frac{1}{4}\mathbf{a}_{74} + (-\frac{1}{4})\mathbf{b}_{74} + (\frac{1}{4})\mathbf{c}_{74}$$

The reduction of higher dimensional irrep:

$$D_{4h} : E_g \rightarrow B_{2g} + B_{3g} \text{ of } D_{2h}.$$

$$D_{4h} : E_u \rightarrow B_{2u} + B_{3u} \text{ of } D_{2h}.$$

The correspondences of irreps at HSPs from original SG to lowered SG:

$$\begin{aligned} n_{GM6}^{74} &= n_{GM8}^{141} + n_{GM9}^{141} & n_{GM5}^{74} &= n_{GM6}^{141} + n_{GM7}^{141} & n_{X6}^{74} &= n_{M5}^{141} & n_{X5}^{74} &= n_{M5}^{141} & n_{T2}^{74} &= n_{X3}^{141} + n_{X4}^{141} & n_{W5}^{74} &= n_{P7}^{141} & n_{W4}^{74} &= n_{P3}^{141} + n_{P5}^{141} \\ n_{W2}^{74} &= n_{P4}^{141} + n_{P6}^{141} & n_{W3}^{74} &= n_{P7}^{141} & n_{R6}^{74} &= n_{N6}^{141} & n_{R4}^{74} &= n_{N4}^{141} & n_{R5}^{74} &= n_{N5}^{141} & n_{R3}^{74} &= n_{N3}^{141} & n_{S4}^{74} &= n_{N3}^{141} & n_{S6}^{74} &= n_{N5}^{141} & n_{S3}^{74} &= n_{N4}^{141} & n_{S5}^{74} &= n_{N5}^{141} \end{aligned}$$

The lower SG is SG 70 when the preserved operations are: **(sub-SG label is 2) 1, 6, 7, 8, 9, 14, 15, 16.**

$$\text{The transformation is: } (\mathbf{a}_{70}, \mathbf{b}_{70}, \mathbf{c}_{70}) = (\mathbf{a}_{141}, \mathbf{b}_{141}, \mathbf{c}_{141}) \begin{pmatrix} -1 & 0 & -1 \\ -1 & 0 & 1 \\ 0 & 1 & 0 \end{pmatrix}, \overrightarrow{O_{141}O_{70}} = \frac{1}{4}\mathbf{a}_{70} + (\frac{1}{4})\mathbf{b}_{70} + (\frac{1}{2})\mathbf{c}_{70}$$

The reduction of higher dimensional irrep:

$$D_{4h} : E_g \rightarrow B_{1g} + B_{3g} \text{ of } D_{2h}.$$

$$D_{4h} : E_u \rightarrow B_{1u} + B_{3u} \text{ of } D_{2h}.$$

The correspondences of irreps at HSPs from original SG to lowered SG:

$$\begin{aligned} n_{GM6}^{70} &= n_{GM8}^{141} + n_{GM9}^{141} & n_{GM5}^{70} &= n_{GM6}^{141} + n_{GM7}^{141} & n_{Y4}^{70} &= n_{M5}^{141} & n_{Y3}^{70} &= n_{M5}^{141} & n_{L3}^{70} &= n_{N5}^{141} + n_{N6}^{141} & n_{L2}^{70} &= n_{N3}^{141} + n_{N4}^{141} & n_{Z3}^{70} &= n_{N3}^{141} + n_{N4}^{141} \\ n_{X3}^{141} & n_{Z4}^{70} &= n_{X4}^{141} & n_{T4}^{70} &= n_{X3}^{141} & n_{T3}^{70} &= n_{X4}^{141} \end{aligned}$$

The lower SG is SG 88 when the preserved operations are: **(sub-SG label is 3) 1, 2, 3, 6, 9, 10, 11, 14.**

$$\text{The transformation is: } (\mathbf{a}_{88}, \mathbf{b}_{88}, \mathbf{c}_{88}) = (\mathbf{a}_{141}, \mathbf{b}_{141}, \mathbf{c}_{141}) \begin{pmatrix} 1 & 0 & 0 \\ 0 & 1 & 0 \\ 0 & 0 & 1 \end{pmatrix}, \overrightarrow{O_{141}O_{88}} = \frac{1}{2}\mathbf{a}_{88}$$

The reduction of higher dimensional irrep:

$$D_{4h} : E_g \rightarrow {}^2E_g + {}^1E_g \text{ of } C_{4h}.$$

$$D_{4h} : E_u \rightarrow {}^2E_u + {}^1E_u \text{ of } C_{4h}.$$

The correspondences of irreps at HSPs from original SG to lowered SG:

$$\begin{aligned} n_{GM9}^{88} &= n_{GM8}^{141} & n_{GM5}^{88} &= n_{GM6}^{141} & n_{GM11}^{88} &= n_{GM8}^{141} & n_{GM7}^{88} &= n_{GM6}^{141} & n_{GM12}^{88} &= n_{GM9}^{141} & n_{GM8}^{88} &= n_{GM7}^{141} & n_{GM10}^{88} &= n_{GM9}^{141} & n_{GM6}^{88} &= n_{GM7}^{141} & n_{M4}^{88} &= n_{M5}^{141} & n_{M3}^{88} &= n_{M5}^{141} & n_{X2}^{88} &= n_{X3}^{141} + n_{X4}^{141} & n_{P5}^{88} &= n_{P7}^{141} & n_{P6}^{88} &= n_{P7}^{141} & n_{P7}^{88} &= n_{P3}^{141} + n_{P6}^{141} & n_{P8}^{88} &= n_{P4}^{141} + n_{P5}^{141} & n_{N3}^{88} &= n_{N3}^{141} + n_{N4}^{141} & n_{N2}^{88} &= n_{N5}^{141} + n_{N6}^{141} \end{aligned}$$

#### 54. Lowered SGs by higher-dimensional irreps of pairings in SG 142

The representative operations of SG/T for SG 142:

$$\begin{aligned} 1 : (x, y, z), & 2 : (\frac{1}{4} - y, x + \frac{3}{4}, z + \frac{1}{4}), & 3 : (y + \frac{3}{4}, \frac{3}{4} - x, z + \frac{1}{4}), & 4 : (x + \frac{1}{2}, \frac{1}{2} - y, -z), & 5 : (\frac{1}{2} - x, y, -z), & 6 : (-x, \frac{1}{2} - y, z), \\ 7 : (y + \frac{3}{4}, x + \frac{1}{4}, \frac{1}{4} - z), & 8 : (\frac{1}{4} - y, \frac{1}{4} - x, \frac{1}{4} - z), & 9 : (-x, -y, -z), & 10 : (y + \frac{3}{4}, \frac{1}{4} - x, \frac{3}{4} - z), & 11 : (\frac{1}{4} - y, x + \frac{1}{4}, \frac{3}{4} - z), \\ 12 : (-x, y, z + \frac{1}{2}), & 13 : (x, \frac{1}{2} - y, z + \frac{1}{2}), & 14 : (x, y + \frac{1}{2}, -z), & 15 : (\frac{3}{4} - y, \frac{1}{4} - x, z + \frac{1}{4}), & 16 : (y + \frac{1}{4}, x + \frac{1}{4}, z + \frac{1}{4}). \end{aligned}$$

The lower SG is SG 73 when the preserved operations are: **(sub-SG label is 1) 1, 4, 5, 6, 9, 12, 13, 14.**

$$\text{The transformation is: } (\mathbf{a}_{73}, \mathbf{b}_{73}, \mathbf{c}_{73}) = (\mathbf{a}_{142}, \mathbf{b}_{142}, \mathbf{c}_{142}) \begin{pmatrix} 0 & -1 & 0 \\ -1 & 0 & 0 \\ 0 & 0 & -1 \end{pmatrix}, \overrightarrow{O_{142}O_{73}} = \frac{1}{4}\mathbf{a}_{73} + (-\frac{1}{4})\mathbf{b}_{73} + (\frac{1}{4})\mathbf{c}_{73}$$

The reduction of higher dimensional irrep:

$$D_{4h} : E_g \rightarrow B_{2g} + B_{3g} \text{ of } D_{2h}.$$

$$D_{4h} : E_u \rightarrow B_{2u} + B_{3u} \text{ of } D_{2h}.$$

The correspondences of irreps at HSPs from original SG to lowered SG:

$$n_{GM6}^{73} = n_{GM8}^{142} + n_{GM9}^{142} \quad n_{GM5}^{73} = n_{GM6}^{142} + n_{GM7}^{142} \quad n_{X6}^{73} = n_{M5}^{142} \quad n_{X5}^{73} = n_{M5}^{142} \quad n_{T2}^{73} = n_{X3}^{142} + n_{X4}^{142} \quad n_{W3}^{73} = n_{P7}^{142} \quad n_{W2}^{73} = n_{P4}^{142} + n_{P6}^{142}$$

$$n_{W4}^{73} = n_{P3}^{142} + n_{P5}^{142} \quad n_{W5}^{73} = n_{P7}^{142} \quad n_{R2}^{73} = n_{N2}^{142} \quad n_{S2}^{73} = n_{N2}^{142}$$

The lower SG is SG 70 when the preserved operations are: **(sub-SG label is 2) 1, 6, 7, 8, 9, 14, 15, 16.**

$$\text{The transformation is: } (\mathbf{a}_{70}, \mathbf{b}_{70}, \mathbf{c}_{70}) = (\mathbf{a}_{142}, \mathbf{b}_{142}, \mathbf{c}_{142}) \begin{pmatrix} 1 & 0 & 1 \\ 1 & 0 & -1 \\ 0 & 1 & 0 \end{pmatrix}, \overrightarrow{O_{142}O_{70}} = \frac{1}{4}\mathbf{a}_{70} + \left(\frac{1}{4}\right)\mathbf{b}_{70} + \left(\frac{1}{2}\right)\mathbf{c}_{70}$$

The reduction of higher dimensional irrep:

$$D_{4h} : E_g \rightarrow B_{1g} + B_{3g} \quad \text{of } D_{2h}.$$

$$D_{4h} : E_u \rightarrow B_{1u} + B_{3u} \quad \text{of } D_{2h}.$$

The correspondences of irreps at HSPs from original SG to lowered SG:

$$n_{GM6}^{70} = n_{GM8}^{142} + n_{GM9}^{142} \quad n_{GM5}^{70} = n_{GM6}^{142} + n_{GM7}^{142} \quad n_{Y4}^{70} = n_{M5}^{142} \quad n_{Y3}^{70} = n_{M5}^{142} \quad n_{L3}^{70} = n_{N2}^{142} \quad n_{L2}^{70} = n_{N2}^{142} \quad n_{Z3}^{70} = n_{X4}^{142} \quad n_{Z4}^{70} = n_{X3}^{142} \\ n_{T4}^{70} = n_{X4}^{142} \quad n_{T3}^{70} = n_{X3}^{142}$$

The lower SG is SG 88 when the preserved operations are: **(sub-SG label is 3) 1, 2, 3, 6, 9, 10, 11, 14.**

$$\text{The transformation is: } (\mathbf{a}_{88}, \mathbf{b}_{88}, \mathbf{c}_{88}) = (\mathbf{a}_{142}, \mathbf{b}_{142}, \mathbf{c}_{142}) \begin{pmatrix} 1 & 0 & 0 \\ 0 & 1 & 0 \\ 0 & 0 & 1 \end{pmatrix}, \overrightarrow{O_{142}O_{88}} = \frac{1}{2}\mathbf{a}_{88}$$

The reduction of higher dimensional irrep:

$$D_{4h} : E_g \rightarrow {}^2E_g + {}^1E_g \quad \text{of } C_{4h}.$$

$$D_{4h} : E_u \rightarrow {}^2E_u + {}^1E_u \quad \text{of } C_{4h}.$$

The correspondences of irreps at HSPs from original SG to lowered SG:

$$n_{GM9}^{88} = n_{GM8}^{142} \quad n_{GM5}^{88} = n_{GM6}^{142} \quad n_{GM11}^{88} = n_{GM8}^{142} \quad n_{GM7}^{88} = n_{GM6}^{142} \quad n_{GM12}^{88} = n_{GM9}^{142} \quad n_{GM8}^{88} = n_{GM7}^{142} \quad n_{GM10}^{88} = n_{GM9}^{142} \quad n_{GM6}^{88} = n_{GM7}^{142} \quad n_{M4}^{88} = n_{M5}^{142} \quad n_{M3}^{88} = n_{M5}^{142} \quad n_{X2}^{88} = n_{X3}^{142} + n_{X4}^{142} \quad n_{P5}^{88} = n_{P4}^{142} + n_{P5}^{142} \quad n_{P6}^{88} = n_{P3}^{142} + n_{P6}^{142} \quad n_{P7}^{88} = n_{P7}^{142} \quad n_{P8}^{88} = n_{P7}^{142} \quad n_{N3}^{88} = n_{N2}^{142} \quad n_{N2}^{88} = n_{N2}^{142}$$

### 55. Lowered SGs by higher-dimensional irreps of pairings in SG 149

The representative operations of SG/T for SG 149:

$$1 : (x, y, z), 2 : (-y, x - y, z), 3 : (y - x, -x, z), 4 : (x, x - y, -z), 5 : (y - x, y, -z), 6 : (-y, -x, -z).$$

The lower SG is SG 5 when the preserved operations are: **(sub-SG label is 1) 1, 5.**

$$\text{The transformation is: } (\mathbf{a}_5, \mathbf{b}_5, \mathbf{c}_5) = (\mathbf{a}_{149}, \mathbf{b}_{149}, \mathbf{c}_{149}) \begin{pmatrix} -1 & 1 & 0 \\ 0 & 2 & 0 \\ 0 & 0 & -1 \end{pmatrix}, \overrightarrow{O_{149}O_5} = \frac{1}{2}\mathbf{a}_5$$

The reduction of higher dimensional irrep:

$$D_3 : E \rightarrow A + B \quad \text{of } C_2.$$

The correspondences of irreps at HSPs from original SG to lowered SG:

$$n_{GM4}^5 = n_{GM5}^{149} + n_{GM6}^{149} \quad n_{GM3}^5 = n_{GM4}^{149} + n_{GM6}^{149} \quad n_{Y4}^5 = n_{M4}^{149} \quad n_{Y3}^5 = n_{M3}^{149} \quad n_{V2}^5 = n_{M3}^{149} + n_{M4}^{149} \quad n_{A4}^5 = n_{A5}^{149} + n_{A6}^{149} \quad n_{A3}^5 = n_{A4}^{149} + n_{A6}^{149} \quad n_{M4}^5 = n_{L4}^{149} \quad n_{M3}^5 = n_{L3}^{149} \quad n_{L2}^5 = n_{L3}^{149} + n_{L4}^{149}$$

The lower SG is SG 5 when the preserved operations are: **(sub-SG label is 2) 1, 4.**

$$\text{The transformation is: } (\mathbf{a}_5, \mathbf{b}_5, \mathbf{c}_5) = (\mathbf{a}_{149}, \mathbf{b}_{149}, \mathbf{c}_{149}) \begin{pmatrix} 0 & 2 & 0 \\ -1 & 1 & 0 \\ 0 & 0 & 1 \end{pmatrix}, \overrightarrow{O_{149}O_5} = \frac{1}{2}\mathbf{a}_5$$

The reduction of higher dimensional irrep:

$$D_3 : E \rightarrow A + B \quad \text{of } C_2.$$

The correspondences of irreps at HSPs from original SG to lowered SG:

$$n_{GM4}^5 = n_{GM4}^{149} + n_{GM6}^{149} \quad n_{GM3}^5 = n_{GM5}^{149} + n_{GM6}^{149} \quad n_{Y4}^5 = n_{M3}^{149} \quad n_{Y3}^5 = n_{M4}^{149} \quad n_{V2}^5 = n_{M3}^{149} + n_{M4}^{149} \quad n_{A4}^5 = n_{A4}^{149} + n_{A6}^{149} \quad n_{A3}^5 = n_{A5}^{149} + n_{A6}^{149} \quad n_{M4}^5 = n_{L3}^{149} \quad n_{M3}^5 = n_{L4}^{149} \quad n_{L2}^5 = n_{L3}^{149} + n_{L4}^{149}$$

The lower SG is SG 5 when the preserved operations are: **(sub-SG label is 3) 1, 6.**

The transformation is:  $(\mathbf{a}_5, \mathbf{b}_5, \mathbf{c}_5) = (\mathbf{a}_{149}, \mathbf{b}_{149}, \mathbf{c}_{149}) \begin{pmatrix} -1 & -1 & 0 \\ -1 & 1 & 0 \\ 0 & 0 & -1 \end{pmatrix}, \overrightarrow{O_{149}O_5} = \frac{1}{2}\mathbf{a}_5$

The reduction of higher dimensional irrep:

$$D_3 : E \rightarrow A + B \text{ of } C_2.$$

The correspondences of irreps at HSPs from original SG to lowered SG:

$$\begin{aligned} n_{GM4}^5 &= n_{GM4}^{149} + n_{GM6}^{149} n_{GM3}^5 = n_{GM5}^{149} + n_{GM6}^{149} n_{Y4}^5 = n_{M3}^{149} n_{Y3}^5 = n_{M4}^{149} n_{V2}^5 = n_{M3}^{149} + n_{M4}^{149} n_{A4}^5 = n_{A4}^{149} + n_{A6}^{149} n_{A3}^5 = \\ n_{A5}^{149} + n_{A6}^{149} n_{M4}^5 &= n_{L3}^{149} n_{M3}^5 = n_{L4}^{149} n_{L2}^5 = n_{L3}^{149} + n_{L4}^{149} \end{aligned}$$

The lower SG is SG 143 when the preserved operations are: **(sub-SG label is 4) 1, 2, 3.**

The transformation is:  $(\mathbf{a}_{143}, \mathbf{b}_{143}, \mathbf{c}_{143}) = (\mathbf{a}_{149}, \mathbf{b}_{149}, \mathbf{c}_{149}) \begin{pmatrix} -1 & 1 & 0 \\ -1 & 0 & 0 \\ 0 & 0 & 1 \end{pmatrix}, \overrightarrow{O_{149}O_{143}} = -\frac{1}{3}\mathbf{a}_{143} + (\frac{1}{3})\mathbf{b}_{143}$

The reduction of higher dimensional irrep:

$$D_3 : E \rightarrow {}^2E + {}^1E \text{ of } C_3.$$

The correspondences of irreps at HSPs from original SG to lowered SG:

$$\begin{aligned} n_{GM4}^{143} &= n_{GM4}^{149} + n_{GM5}^{149} n_{GM6}^{143} = n_{GM6}^{149} n_{GM5}^{143} = n_{GM6}^{149} n_{M2}^{143} = n_{M3}^{149} + n_{M4}^{149} n_{K4}^{143} = n_{K6}^{149} n_{K6}^{143} = n_{K5}^{149} n_{K5}^{143} = n_{K4}^{149} n_{A4}^{143} = \\ n_{A4}^{149} + n_{A5}^{149} n_{A6}^{143} &= n_{A6}^{149} n_{A5}^{143} = n_{A6}^{149} n_{L2}^{143} = n_{L3}^{149} + n_{L4}^{149} n_{H4}^{143} = n_{H6}^{149} n_{H6}^{143} = n_{H5}^{149} n_{H5}^{143} = n_{H4}^{149} \end{aligned}$$

## 56. Lowered SGs by higher-dimensional irreps of pairings in SG 150

The representative operations of SG/T for SG 150:

$$1 : (x, y, z), 2 : (-y, x - y, z), 3 : (y - x, -x, z), 4 : (x - y, -y, -z), 5 : (y, x, -z), 6 : (-x, y - x, -z).$$

The lower SG is SG 5 when the preserved operations are: **(sub-SG label is 1) 1, 4.**

The transformation is:  $(\mathbf{a}_5, \mathbf{b}_5, \mathbf{c}_5) = (\mathbf{a}_{150}, \mathbf{b}_{150}, \mathbf{c}_{150}) \begin{pmatrix} -1 & -1 & 0 \\ -2 & 0 & 0 \\ 0 & 0 & -1 \end{pmatrix}, \overrightarrow{O_{150}O_5} = \frac{1}{2}\mathbf{a}_5$

The reduction of higher dimensional irrep:

$$D_3 : E \rightarrow A + B \text{ of } C_2.$$

The correspondences of irreps at HSPs from original SG to lowered SG:

$$\begin{aligned} n_{GM4}^5 &= n_{GM5}^{150} + n_{GM6}^{150} n_{GM3}^5 = n_{GM4}^{150} + n_{GM6}^{150} n_{Y4}^5 = n_{M3}^{150} n_{Y3}^5 = n_{M4}^{150} n_{V2}^5 = n_{M3}^{150} + n_{M4}^{150} n_{A4}^5 = n_{A5}^{150} + n_{A6}^{150} n_{A3}^5 = \\ n_{A5}^{150} + n_{A6}^{150} n_{M4}^5 &= n_{L3}^{150} n_{M3}^5 = n_{L4}^{150} n_{L2}^5 = n_{L3}^{150} + n_{L4}^{150} \end{aligned}$$

The lower SG is SG 5 when the preserved operations are: **(sub-SG label is 2) 1, 6.**

The transformation is:  $(\mathbf{a}_5, \mathbf{b}_5, \mathbf{c}_5) = (\mathbf{a}_{150}, \mathbf{b}_{150}, \mathbf{c}_{150}) \begin{pmatrix} -2 & 0 & 0 \\ -1 & 1 & 0 \\ 0 & 0 & -1 \end{pmatrix}, \overrightarrow{O_{150}O_5} = \frac{1}{2}\mathbf{a}_5$

The reduction of higher dimensional irrep:

$$D_3 : E \rightarrow A + B \text{ of } C_2.$$

The correspondences of irreps at HSPs from original SG to lowered SG:

$$\begin{aligned} n_{GM4}^5 &= n_{GM4}^{150} + n_{GM6}^{150} n_{GM3}^5 = n_{GM5}^{150} + n_{GM6}^{150} n_{Y4}^5 = n_{M3}^{150} n_{Y3}^5 = n_{M4}^{150} n_{V2}^5 = n_{M3}^{150} + n_{M4}^{150} n_{A4}^5 = n_{A5}^{150} + n_{A6}^{150} n_{A3}^5 = \\ n_{A5}^{150} + n_{A6}^{150} n_{M4}^5 &= n_{L3}^{150} n_{M3}^5 = n_{L4}^{150} n_{L2}^5 = n_{L3}^{150} + n_{L4}^{150} \end{aligned}$$

The lower SG is SG 5 when the preserved operations are: **(sub-SG label is 3) 1, 5.**

The transformation is:  $(\mathbf{a}_5, \mathbf{b}_5, \mathbf{c}_5) = (\mathbf{a}_{150}, \mathbf{b}_{150}, \mathbf{c}_{150}) \begin{pmatrix} -1 & 1 & 0 \\ 1 & 1 & 0 \\ 0 & 0 & -1 \end{pmatrix}, \overrightarrow{O_{150}O_5} = \frac{1}{2}\mathbf{a}_5$

The reduction of higher dimensional irrep:

$$D_3 : E \rightarrow A + B \text{ of } C_2.$$

The correspondences of irreps at HSPs from original SG to lowered SG:

$$n_{GM4}^5 = n_{GM5}^{150} + n_{GM6}^{150} n_{GM3}^5 = n_{GM4}^{150} + n_{GM6}^{150} n_{Y4}^5 = n_{M3}^{150} n_{Y3}^5 = n_{M4}^{150} n_{V2}^5 = n_{M3}^{150} + n_{M4}^{150} n_{A4}^5 = n_{A5}^{150} + n_{A6}^{150} n_{A3}^5 =$$

$$n_{A4}^{150} + n_{A6}^{150} n_{M4}^5 = n_{L4}^{150} n_{M3}^5 = n_{L3}^{150} n_{L2}^5 = n_{L3}^{150} + n_{L4}^{150}$$

The lower SG is SG 143 when the preserved operations are: **(sub-SG label is 4) 1, 2, 3.**

$$\text{The transformation is: } (\mathbf{a}_{143}, \mathbf{b}_{143}, \mathbf{c}_{143}) = (\mathbf{a}_{150}, \mathbf{b}_{150}, \mathbf{c}_{150}) \begin{pmatrix} -1 & 1 & 0 \\ -1 & 0 & 0 \\ 0 & 0 & 1 \end{pmatrix}, \overrightarrow{O_{150}O_{143}} = -\frac{1}{3}\mathbf{a}_{143} + \left(\frac{1}{3}\right)\mathbf{b}_{143}$$

The reduction of higher dimensional irrep:

$$D_3 : E \rightarrow {}^2E + {}^1E \text{ of } C_3.$$

The correspondences of irreps at HSPs from original SG to lowered SG:

$$\begin{aligned} n_{GM4}^{143} &= n_{GM4}^{150} + n_{GM5}^{150} n_{GM6}^{143} = n_{GM6}^{150} n_{GM5}^{143} = n_{GM6}^{150} n_{M2}^{143} = n_{M3}^{150} + n_{M4}^{150} n_{K4}^{143} = n_{K6}^{150} n_{K6}^{143} = n_{K6}^{150} n_{K5}^{143} = n_{K4}^{150} + n_{K5}^{150} \\ n_{A4}^{143} &= n_{A4}^{150} + n_{A5}^{150} n_{A6}^{143} = n_{A6}^{150} n_{A5}^{143} = n_{A6}^{150} n_{L2}^{143} = n_{L3}^{150} + n_{L4}^{150} n_{H4}^{143} = n_{H6}^{150} n_{H6}^{143} = n_{H6}^{150} n_{H5}^{143} = n_{H4}^{150} + n_{H5}^{150} \end{aligned}$$

### 57. Lowered SGs by higher-dimensional irreps of pairings in SG 151

The representative operations of SG/T for SG 151:

$$1 : (x, y, z), 2 : (-y, x - y, z + \frac{1}{3}), 3 : (y - x, -x, z + \frac{2}{3}), 4 : (x, x - y, -z), 5 : (y - x, y, \frac{1}{3} - z), 6 : (-y, -x, \frac{2}{3} - z).$$

The lower SG is SG 5 when the preserved operations are: **(sub-SG label is 1) 1, 5.**

$$\text{The transformation is: } (\mathbf{a}_5, \mathbf{b}_5, \mathbf{c}_5) = (\mathbf{a}_{151}, \mathbf{b}_{151}, \mathbf{c}_{151}) \begin{pmatrix} -1 & 1 & 0 \\ 0 & 2 & 0 \\ 0 & 0 & -1 \end{pmatrix}, \overrightarrow{O_{151}O_5} = \frac{1}{2}\mathbf{a}_5 + \left(-\frac{1}{6}\right)\mathbf{c}_5$$

The reduction of higher dimensional irrep:

$$D_3 : E \rightarrow A + B \text{ of } C_2.$$

The correspondences of irreps at HSPs from original SG to lowered SG:

$$\begin{aligned} n_{GM4}^5 &= n_{GM4}^{151} + n_{GM6}^{151} n_{GM3}^5 = n_{GM5}^{151} + n_{GM6}^{151} n_{Y4}^5 = n_{M3}^{151} n_{V2}^5 = n_{M3}^{151} + n_{M4}^{151} n_{A4}^5 = n_{A4}^{151} + n_{A6}^{151} n_{A3}^5 = \\ n_{A5}^{151} + n_{A6}^{151} n_{M4}^5 &= n_{L3}^{151} n_{M3}^5 = n_{L4}^{151} n_{L2}^5 = n_{L3}^{151} + n_{L4}^{151} \end{aligned}$$

The lower SG is SG 5 when the preserved operations are: **(sub-SG label is 2) 1, 4.**

$$\text{The transformation is: } (\mathbf{a}_5, \mathbf{b}_5, \mathbf{c}_5) = (\mathbf{a}_{151}, \mathbf{b}_{151}, \mathbf{c}_{151}) \begin{pmatrix} 0 & 2 & 0 \\ -1 & 1 & 0 \\ 0 & 0 & 1 \end{pmatrix}, \overrightarrow{O_{151}O_5} = \frac{1}{2}\mathbf{a}_5$$

The reduction of higher dimensional irrep:

$$D_3 : E \rightarrow A + B \text{ of } C_2.$$

The correspondences of irreps at HSPs from original SG to lowered SG:

$$\begin{aligned} n_{GM4}^5 &= n_{GM4}^{151} + n_{GM6}^{151} n_{GM3}^5 = n_{GM5}^{151} + n_{GM6}^{151} n_{Y4}^5 = n_{M3}^{151} n_{V2}^5 = n_{M3}^{151} + n_{M4}^{151} n_{A4}^5 = n_{A4}^{151} + n_{A6}^{151} n_{A3}^5 = \\ n_{A5}^{151} + n_{A6}^{151} n_{M4}^5 &= n_{L3}^{151} n_{M3}^5 = n_{L4}^{151} n_{L2}^5 = n_{L3}^{151} + n_{L4}^{151} \end{aligned}$$

The lower SG is SG 5 when the preserved operations are: **(sub-SG label is 3) 1, 6.**

$$\text{The transformation is: } (\mathbf{a}_5, \mathbf{b}_5, \mathbf{c}_5) = (\mathbf{a}_{151}, \mathbf{b}_{151}, \mathbf{c}_{151}) \begin{pmatrix} -1 & -1 & 0 \\ -1 & 1 & 0 \\ 0 & 0 & -1 \end{pmatrix}, \overrightarrow{O_{151}O_5} = \frac{1}{2}\mathbf{a}_5 + \left(\frac{1}{6}\right)\mathbf{c}_5$$

The reduction of higher dimensional irrep:

$$D_3 : E \rightarrow A + B \text{ of } C_2.$$

The correspondences of irreps at HSPs from original SG to lowered SG:

$$\begin{aligned} n_{GM4}^5 &= n_{GM4}^{151} + n_{GM6}^{151} n_{GM3}^5 = n_{GM5}^{151} + n_{GM6}^{151} n_{Y4}^5 = n_{M3}^{151} n_{V2}^5 = n_{M3}^{151} + n_{M4}^{151} n_{A4}^5 = n_{A4}^{151} + n_{A6}^{151} n_{A3}^5 = \\ n_{A5}^{151} + n_{A6}^{151} n_{M4}^5 &= n_{L3}^{151} n_{M3}^5 = n_{L4}^{151} n_{L2}^5 = n_{L3}^{151} + n_{L4}^{151} \end{aligned}$$

The lower SG is SG 144 when the preserved operations are: **(sub-SG label is 4) 1, 2, 3.**

$$\text{The transformation is: } (\mathbf{a}_{144}, \mathbf{b}_{144}, \mathbf{c}_{144}) = (\mathbf{a}_{151}, \mathbf{b}_{151}, \mathbf{c}_{151}) \begin{pmatrix} 1 & -1 & 0 \\ 0 & -1 & 0 \\ 0 & 0 & -1 \end{pmatrix}, \overrightarrow{O_{151}O_{144}} = \frac{1}{3}\mathbf{a}_{144} + \left(\frac{2}{3}\right)\mathbf{b}_{144} + \left(\frac{1}{6}\right)\mathbf{c}_{144}$$

The reduction of higher dimensional irrep:

$$D_3 : E \rightarrow {}^2E + {}^1E \text{ of } C_3.$$

The correspondences of irreps at HSPs from original SG to lowered SG:

$$\begin{aligned} n_{GM4}^{144} &= n_{GM4}^{151} + n_{GM5}^{151} n_{GM6}^{144} = n_{GM6}^{151} n_{GM5}^{144} = n_{GM6}^{151} n_{M2}^{144} = n_{M3}^{151} + n_{M4}^{151} n_{K4}^{144} = n_{K6}^{151} n_{K6}^{144} = n_{K4}^{151} n_{K5}^{144} = n_{K5}^{151} n_{A4}^{144} = \\ n_{A6}^{151} n_{A6}^{144} &= n_{A6}^{151} n_{A5}^{144} = n_{A4}^{151} + n_{A5}^{151} n_{L2}^{144} = n_{L3}^{151} + n_{L4}^{151} n_{H4}^{144} = n_{H5}^{151} n_{H6}^{144} = n_{H6}^{151} n_{H5}^{144} = n_{H4}^{151} \end{aligned}$$

### 58. Lowered SGs by higher-dimensional irreps of pairings in SG 152

The representative operations of SG/T for SG 152:

$$1 : (x, y, z), 2 : (-y, x - y, z + \frac{1}{3}), 3 : (y - x, -x, z + \frac{2}{3}), 4 : (x - y, -y, \frac{2}{3} - z), 5 : (y, x, -z), 6 : (-x, y - x, \frac{1}{3} - z).$$

The lower SG is SG 5 when the preserved operations are: **(sub-SG label is 1) 1, 4.**

$$\text{The transformation is: } (\mathbf{a}_5, \mathbf{b}_5, \mathbf{c}_5) = (\mathbf{a}_{152}, \mathbf{b}_{152}, \mathbf{c}_{152}) \begin{pmatrix} -1 & -1 & 0 \\ -2 & 0 & 0 \\ 0 & 0 & -1 \end{pmatrix}, \overrightarrow{O_{152}O_5} = \frac{1}{2}\mathbf{a}_5 + (-\frac{1}{3})\mathbf{c}_5$$

The reduction of higher dimensional irrep:

$$D_3 : E \rightarrow A + B \text{ of } C_2.$$

The correspondences of irreps at HSPs from original SG to lowered SG:

$$\begin{aligned} n_{GM4}^5 &= n_{GM5}^{152} + n_{GM6}^{152} n_{GM3}^5 = n_{GM4}^{152} + n_{GM6}^{152} n_{Y4}^5 = n_{M4}^{152} n_{Y3}^5 = n_{M3}^{152} n_{V2}^5 = n_{M3}^{152} + n_{M4}^{152} n_{A4}^5 = n_{A5}^{152} + n_{A6}^{152} n_{A3}^5 = \\ n_{A4}^{152} + n_{A6}^{152} n_{M4}^5 &= n_{L3}^{152} n_{M3}^5 = n_{L4}^{152} n_{L2}^5 = n_{L3}^{152} + n_{L4}^{152} \end{aligned}$$

The lower SG is SG 5 when the preserved operations are: **(sub-SG label is 2) 1, 6.**

$$\text{The transformation is: } (\mathbf{a}_5, \mathbf{b}_5, \mathbf{c}_5) = (\mathbf{a}_{152}, \mathbf{b}_{152}, \mathbf{c}_{152}) \begin{pmatrix} -2 & 0 & 0 \\ -1 & 1 & 0 \\ 0 & 0 & -1 \end{pmatrix}, \overrightarrow{O_{152}O_5} = \frac{1}{2}\mathbf{a}_5 + (-\frac{1}{6})\mathbf{c}_5$$

The reduction of higher dimensional irrep:

$$D_3 : E \rightarrow A + B \text{ of } C_2.$$

The correspondences of irreps at HSPs from original SG to lowered SG:

$$\begin{aligned} n_{GM4}^5 &= n_{GM5}^{152} + n_{GM6}^{152} n_{GM3}^5 = n_{GM4}^{152} + n_{GM6}^{152} n_{Y4}^5 = n_{M4}^{152} n_{Y3}^5 = n_{M3}^{152} n_{V2}^5 = n_{M3}^{152} + n_{M4}^{152} n_{A4}^5 = n_{A5}^{152} + n_{A6}^{152} n_{A3}^5 = \\ n_{A4}^{152} + n_{A6}^{152} n_{M4}^5 &= n_{L3}^{152} n_{M3}^5 = n_{L4}^{152} n_{L2}^5 = n_{L3}^{152} + n_{L4}^{152} \end{aligned}$$

The lower SG is SG 5 when the preserved operations are: **(sub-SG label is 3) 1, 5.**

$$\text{The transformation is: } (\mathbf{a}_5, \mathbf{b}_5, \mathbf{c}_5) = (\mathbf{a}_{152}, \mathbf{b}_{152}, \mathbf{c}_{152}) \begin{pmatrix} -1 & 1 & 0 \\ 1 & 1 & 0 \\ 0 & 0 & -1 \end{pmatrix}, \overrightarrow{O_{152}O_5} = \frac{1}{2}\mathbf{a}_5$$

The reduction of higher dimensional irrep:

$$D_3 : E \rightarrow A + B \text{ of } C_2.$$

The correspondences of irreps at HSPs from original SG to lowered SG:

$$\begin{aligned} n_{GM4}^5 &= n_{GM5}^{152} + n_{GM6}^{152} n_{GM3}^5 = n_{GM4}^{152} + n_{GM6}^{152} n_{Y4}^5 = n_{M4}^{152} n_{Y3}^5 = n_{M3}^{152} n_{V2}^5 = n_{M3}^{152} + n_{M4}^{152} n_{A4}^5 = n_{A5}^{152} + n_{A6}^{152} n_{A3}^5 = \\ n_{A4}^{152} + n_{A6}^{152} n_{M4}^5 &= n_{L3}^{152} n_{M3}^5 = n_{L4}^{152} n_{L2}^5 = n_{L3}^{152} + n_{L4}^{152} \end{aligned}$$

The lower SG is SG 144 when the preserved operations are: **(sub-SG label is 4) 1, 2, 3.**

$$\text{The transformation is: } (\mathbf{a}_{144}, \mathbf{b}_{144}, \mathbf{c}_{144}) = (\mathbf{a}_{152}, \mathbf{b}_{152}, \mathbf{c}_{152}) \begin{pmatrix} 1 & -1 & 0 \\ 0 & -1 & 0 \\ 0 & 0 & -1 \end{pmatrix}, \overrightarrow{O_{152}O_{144}} = \frac{1}{3}\mathbf{a}_{144} + (\frac{2}{3})\mathbf{b}_{144}$$

The reduction of higher dimensional irrep:

$$D_3 : E \rightarrow {}^2E + {}^1E \text{ of } C_3.$$

The correspondences of irreps at HSPs from original SG to lowered SG:

$$\begin{aligned} n_{GM4}^{144} &= n_{GM4}^{152} + n_{GM5}^{152} n_{GM6}^{144} = n_{GM6}^{152} n_{GM5}^{144} = n_{GM6}^{152} n_{M2}^{144} = n_{M3}^{152} + n_{M4}^{152} n_{K4}^{144} = n_{K6}^{152} n_{K6}^{144} = n_{K4}^{152} + n_{K5}^{152} n_{K5}^{144} = n_{K6}^{152} \\ n_{A4}^{144} &= n_{A6}^{152} n_{A6}^{144} = n_{A6}^{152} n_{A5}^{144} = n_{A4}^{152} + n_{A5}^{152} n_{L2}^{144} = n_{L3}^{152} + n_{L4}^{152} n_{H4}^{144} = n_{H4}^{152} + n_{H5}^{152} n_{H6}^{144} = n_{H6}^{152} n_{H5}^{144} = n_{H6}^{152} \end{aligned}$$

### 59. Lowered SGs by higher-dimensional irreps of pairings in SG 153

The representative operations of SG/T for SG 153:

$$1 : (x, y, z), 2 : (-y, x - y, z + \frac{2}{3}), 3 : (y - x, -x, z + \frac{1}{3}), 4 : (x, x - y, -z), 5 : (y - x, y, \frac{2}{3} - z), 6 : (-y, -x, \frac{1}{3} - z).$$

The lower SG is SG 5 when the preserved operations are: **(sub-SG label is 1) 1, 5.**

$$\text{The transformation is: } (\mathbf{a}_5, \mathbf{b}_5, \mathbf{c}_5) = (\mathbf{a}_{153}, \mathbf{b}_{153}, \mathbf{c}_{153}) \begin{pmatrix} -1 & 1 & 0 \\ 0 & 2 & 0 \\ 0 & 0 & -1 \end{pmatrix}, \overrightarrow{O_{153}O_5} = \frac{1}{2}\mathbf{a}_5 + (-\frac{1}{3})\mathbf{c}_5$$

The reduction of higher dimensional irrep:

$$D_3 : E \rightarrow A + B \text{ of } C_2.$$

The correspondences of irreps at HSPs from original SG to lowered SG:

$$\begin{aligned} n_{GM4}^5 &= n_{GM5}^{153} + n_{GM6}^{153} & n_{GM3}^5 &= n_{GM4}^{153} + n_{GM6}^{153} & n_{Y4}^5 &= n_{M4}^{153} n_{Y3}^5 = n_{M3}^{153} n_{V2}^5 = n_{M3}^{153} + n_{M4}^{153} n_{A4}^5 = n_{A4}^{153} + n_{A6}^{153} n_{A3}^5 = \\ n_{A5}^{153} + n_{A6}^{153} & n_{M4}^5 = n_{L4}^{153} & n_{M3}^5 &= n_{L3}^{153} & n_{L2}^5 &= n_{L3}^{153} + n_{L4}^{153} \end{aligned}$$

The lower SG is SG 5 when the preserved operations are: **(sub-SG label is 2) 1, 4.**

$$\text{The transformation is: } (\mathbf{a}_5, \mathbf{b}_5, \mathbf{c}_5) = (\mathbf{a}_{153}, \mathbf{b}_{153}, \mathbf{c}_{153}) \begin{pmatrix} 0 & 2 & 0 \\ -1 & 1 & 0 \\ 0 & 0 & 1 \end{pmatrix}, \overrightarrow{O_{153}O_5} = \frac{1}{2}\mathbf{a}_5 + (\frac{1}{2})\mathbf{c}_5$$

The reduction of higher dimensional irrep:

$$D_3 : E \rightarrow A + B \text{ of } C_2.$$

The correspondences of irreps at HSPs from original SG to lowered SG:

$$\begin{aligned} n_{GM4}^5 &= n_{GM4}^{153} + n_{GM6}^{153} & n_{GM3}^5 &= n_{GM5}^{153} + n_{GM6}^{153} & n_{Y4}^5 &= n_{M3}^{153} n_{Y3}^5 = n_{M4}^{153} n_{V2}^5 = n_{M3}^{153} + n_{M4}^{153} n_{A4}^5 = n_{A4}^{153} + n_{A6}^{153} n_{A3}^5 = \\ n_{A5}^{153} + n_{A6}^{153} & n_{M4}^5 = n_{L4}^{153} & n_{M3}^5 &= n_{L3}^{153} & n_{L2}^5 &= n_{L3}^{153} + n_{L4}^{153} \end{aligned}$$

The lower SG is SG 5 when the preserved operations are: **(sub-SG label is 3) 1, 6.**

$$\text{The transformation is: } (\mathbf{a}_5, \mathbf{b}_5, \mathbf{c}_5) = (\mathbf{a}_{153}, \mathbf{b}_{153}, \mathbf{c}_{153}) \begin{pmatrix} -1 & -1 & 0 \\ -1 & 1 & 0 \\ 0 & 0 & -1 \end{pmatrix}, \overrightarrow{O_{153}O_5} = \frac{1}{2}\mathbf{a}_5 + (-\frac{1}{6})\mathbf{c}_5$$

The reduction of higher dimensional irrep:

$$D_3 : E \rightarrow A + B \text{ of } C_2.$$

The correspondences of irreps at HSPs from original SG to lowered SG:

$$\begin{aligned} n_{GM4}^5 &= n_{GM4}^{153} + n_{GM6}^{153} & n_{GM3}^5 &= n_{GM5}^{153} + n_{GM6}^{153} & n_{Y4}^5 &= n_{M3}^{153} n_{Y3}^5 = n_{M4}^{153} n_{V2}^5 = n_{M3}^{153} + n_{M4}^{153} n_{A4}^5 = n_{A4}^{153} + n_{A6}^{153} n_{A3}^5 = \\ n_{A5}^{153} + n_{A6}^{153} & n_{M4}^5 = n_{L4}^{153} & n_{M3}^5 &= n_{L3}^{153} & n_{L2}^5 &= n_{L3}^{153} + n_{L4}^{153} \end{aligned}$$

The lower SG is SG 145 when the preserved operations are: **(sub-SG label is 4) 1, 2, 3.**

$$\text{The transformation is: } (\mathbf{a}_{145}, \mathbf{b}_{145}, \mathbf{c}_{145}) = (\mathbf{a}_{153}, \mathbf{b}_{153}, \mathbf{c}_{153}) \begin{pmatrix} 1 & -1 & 0 \\ 0 & -1 & 0 \\ 0 & 0 & -1 \end{pmatrix}, \overrightarrow{O_{153}O_{145}} = \frac{1}{3}\mathbf{a}_{145} + (\frac{2}{3})\mathbf{b}_{145} + (-\frac{1}{6})\mathbf{c}_{145}$$

The reduction of higher dimensional irrep:

$$D_3 : E \rightarrow {}^2E + {}^1E \text{ of } C_3.$$

The correspondences of irreps at HSPs from original SG to lowered SG:

$$\begin{aligned} n_{GM4}^{145} &= n_{GM4}^{153} + n_{GM5}^{153} & n_{GM6}^{145} &= n_{GM6}^{153} & n_{GM5}^{145} &= n_{GM6}^{153} n_{M2}^{145} = n_{M3}^{153} + n_{M4}^{153} n_{K4}^{145} = n_{K6}^{153} n_{K6}^{145} = n_{K4}^{153} n_{K5}^{145} = n_{K5}^{153} n_{A4}^{145} = \\ n_{A6}^{153} n_{A6}^{145} &= n_{A4}^{153} + n_{A5}^{153} & n_{A5}^{145} &= n_{A6}^{153} n_{L2}^{145} = n_{L3}^{153} + n_{L4}^{153} & n_{H5}^{145} &= n_{H5}^{153} n_{H4}^{145} = n_{H6}^{153} n_{H6}^{145} = n_{H4}^{153} \end{aligned}$$

### 60. Lowered SGs by higher-dimensional irreps of pairings in SG 154

The representative operations of SG/T for SG 154:

$$1 : (x, y, z), 2 : (-y, x - y, z + \frac{2}{3}), 3 : (y - x, -x, z + \frac{1}{3}), 4 : (x - y, -y, \frac{1}{3} - z), 5 : (y, x, -z), 6 : (-x, y - x, \frac{2}{3} - z).$$

The lower SG is SG 5 when the preserved operations are: **(sub-SG label is 1) 1, 4.**

$$\text{The transformation is: } (\mathbf{a}_5, \mathbf{b}_5, \mathbf{c}_5) = (\mathbf{a}_{154}, \mathbf{b}_{154}, \mathbf{c}_{154}) \begin{pmatrix} -1 & -1 & 0 \\ -2 & 0 & 0 \\ 0 & 0 & -1 \end{pmatrix}, \overrightarrow{O_{154}O_5} = \frac{1}{2}\mathbf{a}_5 + (-\frac{1}{6})\mathbf{c}_5$$

The reduction of higher dimensional irrep:

$$D_3 : E \rightarrow A + B \text{ of } C_2.$$

The correspondences of irreps at HSPs from original SG to lowered SG:

$$\begin{aligned} n_{GM4}^5 &= n_{GM5}^{154} + n_{GM6}^{154} & n_{GM3}^5 &= n_{GM4}^{154} + n_{GM6}^{154} & n_{Y4}^5 &= n_{M4}^{154} n_{Y3}^5 = n_{M3}^{154} n_{V2}^5 = n_{M3}^{154} + n_{M4}^{154} n_{A4}^5 = n_{A4}^{154} + n_{A6}^{154} n_{A3}^5 = \\ n_{A5}^{154} + n_{A6}^{154} n_{M4}^5 &= n_{L3}^{154} n_{M3}^5 = n_{L4}^{154} n_{L2}^5 = n_{L3}^{154} + n_{L4}^{154} \end{aligned}$$

The lower SG is SG 5 when the preserved operations are: **(sub-SG label is 2) 1, 6.**

$$\text{The transformation is: } (\mathbf{a}_5, \mathbf{b}_5, \mathbf{c}_5) = (\mathbf{a}_{154}, \mathbf{b}_{154}, \mathbf{c}_{154}) \begin{pmatrix} -2 & 0 & 0 \\ -1 & 1 & 0 \\ 0 & 0 & -1 \end{pmatrix}, \overrightarrow{O_{154}O_5} = \frac{1}{2}\mathbf{a}_5 + (-\frac{1}{3})\mathbf{c}_5$$

The reduction of higher dimensional irrep:

$$D_3 : E \rightarrow A + B \text{ of } C_2.$$

The correspondences of irreps at HSPs from original SG to lowered SG:

$$\begin{aligned} n_{GM4}^5 &= n_{GM5}^{154} + n_{GM6}^{154} & n_{GM3}^5 &= n_{GM4}^{154} + n_{GM6}^{154} & n_{Y4}^5 &= n_{M4}^{154} n_{Y3}^5 = n_{M3}^{154} n_{V2}^5 = n_{M3}^{154} + n_{M4}^{154} n_{A4}^5 = n_{A4}^{154} + n_{A6}^{154} n_{A3}^5 = \\ n_{A5}^{154} + n_{A6}^{154} n_{M4}^5 &= n_{L3}^{154} n_{M3}^5 = n_{L4}^{154} n_{L2}^5 = n_{L3}^{154} + n_{L4}^{154} \end{aligned}$$

The lower SG is SG 5 when the preserved operations are: **(sub-SG label is 3) 1, 5.**

$$\text{The transformation is: } (\mathbf{a}_5, \mathbf{b}_5, \mathbf{c}_5) = (\mathbf{a}_{154}, \mathbf{b}_{154}, \mathbf{c}_{154}) \begin{pmatrix} -1 & 1 & 0 \\ 1 & 1 & 0 \\ 0 & 0 & -1 \end{pmatrix}, \overrightarrow{O_{154}O_5} = \frac{1}{2}\mathbf{a}_5$$

The reduction of higher dimensional irrep:

$$D_3 : E \rightarrow A + B \text{ of } C_2.$$

The correspondences of irreps at HSPs from original SG to lowered SG:

$$\begin{aligned} n_{GM4}^5 &= n_{GM5}^{154} + n_{GM6}^{154} & n_{GM3}^5 &= n_{GM4}^{154} + n_{GM6}^{154} & n_{Y4}^5 &= n_{M4}^{154} n_{Y3}^5 = n_{M3}^{154} n_{V2}^5 = n_{M3}^{154} + n_{M4}^{154} n_{A4}^5 = n_{A5}^{154} + n_{A6}^{154} n_{A3}^5 = \\ n_{A4}^{154} + n_{A6}^{154} n_{M4}^5 &= n_{L4}^{154} n_{M3}^5 = n_{L3}^{154} n_{L2}^5 = n_{L3}^{154} + n_{L4}^{154} \end{aligned}$$

The lower SG is SG 145 when the preserved operations are: **(sub-SG label is 4) 1, 2, 3.**

$$\text{The transformation is: } (\mathbf{a}_{145}, \mathbf{b}_{145}, \mathbf{c}_{145}) = (\mathbf{a}_{154}, \mathbf{b}_{154}, \mathbf{c}_{154}) \begin{pmatrix} 1 & -1 & 0 \\ 0 & -1 & 0 \\ 0 & 0 & -1 \end{pmatrix}, \overrightarrow{O_{154}O_{145}} = \frac{1}{3}\mathbf{a}_{145} + (\frac{2}{3})\mathbf{b}_{145}$$

The reduction of higher dimensional irrep:

$$D_3 : E \rightarrow {}^2E + {}^1E \text{ of } C_3.$$

The correspondences of irreps at HSPs from original SG to lowered SG:

$$\begin{aligned} n_{GM4}^{145} &= n_{GM4}^{154} + n_{GM5}^{154} & n_{GM6}^{145} &= n_{GM6}^{154} & n_{M2}^{145} &= n_{M3}^{154} + n_{M4}^{154} n_{K4}^{145} = n_{K6}^{154} n_{K6}^{145} = n_{K4}^{154} + n_{K5}^{154} n_{K5}^{145} = n_{K6}^{154} \\ n_{A4}^{145} &= n_{A4}^{154} n_{A6}^{145} = n_{A4}^{154} + n_{A5}^{154} & n_{A5}^{145} &= n_{A6}^{154} n_{L2}^{145} = n_{L3}^{154} + n_{L4}^{154} & n_{H5}^{145} &= n_{H6}^{154} n_{H4}^{145} = n_{H6}^{154} n_{H6}^{145} = n_{H4}^{154} + n_{H5}^{154} \end{aligned}$$

### 61. Lowered SGs by higher-dimensional irreps of pairings in SG 155

The representative operations of SG/T for SG 155:

$$1 : (x, y, z), 2 : (z, x, y), 3 : (y, z, x), 4 : (-y, -x, -z), 5 : (-z, -y, -x), 6 : (-x, -z, -y).$$

The lower SG is SG 5 when the preserved operations are: **(sub-SG label is 1) 1, 6.**

The transformation is:  $(\mathbf{a}_5, \mathbf{b}_5, \mathbf{c}_5) = (\mathbf{a}_{155}, \mathbf{b}_{155}, \mathbf{c}_{155}) \begin{pmatrix} -2 & 0 & 1 \\ 1 & 1 & -1 \\ 1 & -1 & -1 \end{pmatrix}, \overrightarrow{O_{155}O_5} = \frac{1}{2}\mathbf{a}_5$

The reduction of higher dimensional irrep:

$D_3 : E \rightarrow A + B$  of  $C_2$ .

The correspondences of irreps at HSPs from original SG to lowered SG:

$$\begin{aligned} n_{GM4}^5 &= n_{GM4}^{155} + n_{GM6}^{155} & n_{GM3}^5 &= n_{GM5}^{155} + n_{GM6}^{155} & n_{Y4}^5 &= n_{F4}^{155} & n_{Y3}^5 &= n_{F3}^{155} & n_{V2}^5 &= n_{F3}^{155} + n_{F4}^{155} & n_{A4}^5 &= n_{T4}^{155} + n_{T6}^{155} & n_{A3}^5 &= n_{T5}^{155} + n_{T6}^{155} \\ n_{M4}^5 &= n_{T5}^{155} + n_{T6}^{155} & n_{M3}^5 &= n_{L3}^{155} & n_{L2}^5 &= n_{L4}^{155} + n_{L4}^{155} \end{aligned}$$

The lower SG is SG 5 when the preserved operations are: **(sub-SG label is 2) 1, 5.**

The transformation is:  $(\mathbf{a}_5, \mathbf{b}_5, \mathbf{c}_5) = (\mathbf{a}_{155}, \mathbf{b}_{155}, \mathbf{c}_{155}) \begin{pmatrix} -1 & 1 & 0 \\ 0 & 0 & -1 \\ -1 & -1 & 0 \end{pmatrix}, \overrightarrow{O_{155}O_5} = \frac{1}{2}\mathbf{a}_5$

The reduction of higher dimensional irrep:

$D_3 : E \rightarrow A + B$  of  $C_2$ .

The correspondences of irreps at HSPs from original SG to lowered SG:

$$\begin{aligned} n_{GM4}^5 &= n_{GM5}^{155} + n_{GM6}^{155} & n_{GM3}^5 &= n_{GM4}^{155} + n_{GM6}^{155} & n_{Y4}^5 &= n_{F3}^{155} & n_{Y3}^5 &= n_{F4}^{155} & n_{V2}^5 &= n_{L3}^{155} + n_{L4}^{155} & n_{A4}^5 &= n_{L4}^{155} & n_{A3}^5 &= n_{L3}^{155} \\ n_{M4}^5 &= n_{T5}^{155} + n_{T6}^{155} & n_{M3}^5 &= n_{T4}^{155} + n_{T6}^{155} & n_{L2}^5 &= n_{F3}^{155} + n_{F4}^{155} \end{aligned}$$

The lower SG is SG 5 when the preserved operations are: **(sub-SG label is 3) 1, 4.**

The transformation is:  $(\mathbf{a}_5, \mathbf{b}_5, \mathbf{c}_5) = (\mathbf{a}_{155}, \mathbf{b}_{155}, \mathbf{c}_{155}) \begin{pmatrix} -1 & -1 & 0 \\ -1 & 1 & 0 \\ 0 & 0 & -1 \end{pmatrix}, \overrightarrow{O_{155}O_5} = \frac{1}{2}\mathbf{a}_5$

The reduction of higher dimensional irrep:

$D_3 : E \rightarrow A + B$  of  $C_2$ .

The correspondences of irreps at HSPs from original SG to lowered SG:

$$\begin{aligned} n_{GM4}^5 &= n_{GM5}^{155} + n_{GM6}^{155} & n_{GM3}^5 &= n_{GM4}^{155} + n_{GM6}^{155} & n_{Y4}^5 &= n_{F3}^{155} & n_{Y3}^5 &= n_{F4}^{155} & n_{V2}^5 &= n_{L3}^{155} + n_{L4}^{155} & n_{A4}^5 &= n_{L4}^{155} & n_{A3}^5 &= n_{L3}^{155} \\ n_{M4}^5 &= n_{T5}^{155} + n_{T6}^{155} & n_{M3}^5 &= n_{T4}^{155} + n_{T6}^{155} & n_{L2}^5 &= n_{F3}^{155} + n_{F4}^{155} \end{aligned}$$

The lower SG is SG 146 when the preserved operations are: **(sub-SG label is 4) 1, 2, 3.**

The transformation is:  $(\mathbf{a}_{146}, \mathbf{b}_{146}, \mathbf{c}_{146}) = (\mathbf{a}_{155}, \mathbf{b}_{155}, \mathbf{c}_{155}) \begin{pmatrix} 0 & 1 & 0 \\ 0 & 0 & 1 \\ 1 & 0 & 0 \end{pmatrix}, \overrightarrow{O_{155}O_{146}} = -\frac{1}{3}\mathbf{a}_{146} + (\frac{2}{3})\mathbf{b}_{146} + (-\frac{1}{3})\mathbf{c}_{146}$

The reduction of higher dimensional irrep:

$D_3 : E \rightarrow {}^2E + {}^1E$  of  $C_3$ .

The correspondences of irreps at HSPs from original SG to lowered SG:

$$\begin{aligned} n_{GM4}^{146} &= n_{GM4}^{155} + n_{GM5}^{155} & n_{GM6}^{146} &= n_{GM6}^{155} & n_{GM5}^{146} &= n_{GM6}^{155} & n_{L2}^{146} &= n_{L3}^{155} + n_{L4}^{155} & n_{F2}^{146} &= n_{F3}^{155} + n_{F4}^{155} & n_{T4}^{146} &= n_{T4}^{155} + n_{T5}^{155} & n_{T6}^{146} &= n_{T6}^{155} \\ n_{T6}^{146} &= n_{T5}^{155} \end{aligned}$$

## 62. Lowered SGs by higher-dimensional irreps of pairings in SG 156

The representative operations of SG/T for SG 156:

$$1 : (x, y, z), 2 : (-y, x - y, z), 3 : (y - x, -x, z), 4 : (y - x, y, z), 5 : (-y, -x, z), 6 : (x, x - y, z).$$

The lower SG is SG 8 when the preserved operations are: **(sub-SG label is 1) 1, 4.**

The transformation is:  $(\mathbf{a}_8, \mathbf{b}_8, \mathbf{c}_8) = (\mathbf{a}_{156}, \mathbf{b}_{156}, \mathbf{c}_{156}) \begin{pmatrix} -1 & -1 & 0 \\ -2 & 0 & 0 \\ 0 & 0 & -1 \end{pmatrix}, \overrightarrow{O_{156}O_8} = \mathbf{0}$

The reduction of higher dimensional irrep:

$C_{3v} : E \rightarrow A' + A''$  of  $C_{1h}$ .

The correspondences of irreps at HSPs from original SG to lowered SG:

$$\begin{aligned} n_{GM4}^8 &= n_{GM5}^{156} + n_{GM6}^{156} & n_{GM3}^8 &= n_{GM4}^{156} + n_{GM6}^{156} & n_{Y4}^8 &= n_{M4}^{156} & n_{Y3}^8 &= n_{M3}^{156} & n_{V2}^8 &= n_{M3}^{156} + n_{M4}^{156} & n_{A4}^8 &= n_{A5}^{156} + n_{A6}^{156} & n_{A3}^8 &= n_{A5}^{156} + n_{A6}^{156} \\ n_{T6}^8 &= n_{T5}^{156} \end{aligned}$$

$$n_{A4}^{156} + n_{A6}^{156} n_{M4}^8 = n_{L4}^{156} n_{M3}^8 = n_{L3}^{156} n_{L2}^8 = n_{L3}^{156} + n_{L4}^{156}$$

The lower SG is SG 8 when the preserved operations are: **(sub-SG label is 2) 1, 6.**

$$\text{The transformation is: } (\mathbf{a}_8, \mathbf{b}_8, \mathbf{c}_8) = (\mathbf{a}_{156}, \mathbf{b}_{156}, \mathbf{c}_{156}) \begin{pmatrix} -2 & 0 & 0 \\ -1 & 1 & 0 \\ 0 & 0 & -1 \end{pmatrix}, \overrightarrow{O_{156}O_8} = \mathbf{0}$$

The reduction of higher dimensional irrep:

$$C_{3v} : E \rightarrow A' + A'' \text{ of } C_{1h}.$$

The correspondences of irreps at HSPs from original SG to lowered SG:

$$n_{GM4}^8 = n_{GM4}^{156} + n_{GM6}^{156} n_{GM3}^8 = n_{GM5}^{156} + n_{GM6}^{156} n_{Y4}^8 = n_{M3}^{156} n_{Y3}^8 = n_{M4}^{156} n_{V2}^8 = n_{M3}^{156} + n_{M4}^{156} n_{A4}^8 = n_{A4}^{156} + n_{A6}^{156} n_{A3}^8 = n_{A5}^{156} + n_{A6}^{156} n_{M4}^8 = n_{L4}^{156} n_{M3}^8 = n_{L3}^{156} n_{L2}^8 = n_{L3}^{156} + n_{L4}^{156}$$

The lower SG is SG 8 when the preserved operations are: **(sub-SG label is 3) 1, 5.**

$$\text{The transformation is: } (\mathbf{a}_8, \mathbf{b}_8, \mathbf{c}_8) = (\mathbf{a}_{156}, \mathbf{b}_{156}, \mathbf{c}_{156}) \begin{pmatrix} -1 & 1 & 0 \\ 1 & 1 & 0 \\ 0 & 0 & -1 \end{pmatrix}, \overrightarrow{O_{156}O_8} = \mathbf{0}$$

The reduction of higher dimensional irrep:

$$C_{3v} : E \rightarrow A' + A'' \text{ of } C_{1h}.$$

The correspondences of irreps at HSPs from original SG to lowered SG:

$$n_{GM4}^8 = n_{GM5}^{156} + n_{GM6}^{156} n_{GM3}^8 = n_{GM4}^{156} + n_{GM6}^{156} n_{Y4}^8 = n_{M4}^{156} n_{Y3}^8 = n_{M3}^{156} n_{V2}^8 = n_{M3}^{156} + n_{M4}^{156} n_{A4}^8 = n_{A5}^{156} + n_{A6}^{156} n_{A3}^8 = n_{A4}^{156} + n_{A6}^{156} n_{M4}^8 = n_{L4}^{156} n_{M3}^8 = n_{L3}^{156} n_{L2}^8 = n_{L3}^{156} + n_{L4}^{156}$$

The lower SG is SG 143 when the preserved operations are: **(sub-SG label is 4) 1, 2, 3.**

$$\text{The transformation is: } (\mathbf{a}_{143}, \mathbf{b}_{143}, \mathbf{c}_{143}) = (\mathbf{a}_{156}, \mathbf{b}_{156}, \mathbf{c}_{156}) \begin{pmatrix} -1 & 1 & 0 \\ -1 & 0 & 0 \\ 0 & 0 & 1 \end{pmatrix}, \overrightarrow{O_{156}O_{143}} = -\frac{1}{3}\mathbf{a}_{143} + \left(\frac{1}{3}\right)\mathbf{b}_{143}$$

The reduction of higher dimensional irrep:

$$C_{3v} : E \rightarrow {}^2E + {}^1E \text{ of } C_3.$$

The correspondences of irreps at HSPs from original SG to lowered SG:

$$n_{GM4}^{143} = n_{GM4}^{156} + n_{GM5}^{156} n_{GM6}^{143} = n_{GM6}^{156} n_{GM5}^{143} = n_{GM6}^{156} n_{M2}^{143} = n_{M3}^{156} + n_{M4}^{156} n_{K4}^{143} = n_{K6}^{156} n_{K6}^{143} = n_{K5}^{156} n_{K5}^{143} = n_{K4}^{156} n_{A4}^{143} = n_{A4}^{156} + n_{A5}^{156} n_{A6}^{143} = n_{A6}^{156} n_{A5}^{143} = n_{A6}^{156} n_{L2}^{143} = n_{L3}^{156} + n_{L4}^{156} n_{H4}^{143} = n_{H6}^{156} n_{H6}^{143} = n_{H5}^{156} n_{H5}^{143} = n_{H4}^{156}$$

### 63. Lowered SGs by higher-dimensional irreps of pairings in SG 157

The representative operations of SG/T for SG 157:

$$1 : (x, y, z), 2 : (-y, x - y, z), 3 : (y - x, -x, z), 4 : (-x, y - x, z), 5 : (x - y, -y, z), 6 : (y, x, z).$$

The lower SG is SG 8 when the preserved operations are: **(sub-SG label is 1) 1, 5.**

$$\text{The transformation is: } (\mathbf{a}_8, \mathbf{b}_8, \mathbf{c}_8) = (\mathbf{a}_{157}, \mathbf{b}_{157}, \mathbf{c}_{157}) \begin{pmatrix} -1 & 1 & 0 \\ 0 & 2 & 0 \\ 0 & 0 & -1 \end{pmatrix}, \overrightarrow{O_{157}O_8} = \mathbf{0}$$

The reduction of higher dimensional irrep:

$$C_{3v} : E \rightarrow A' + A'' \text{ of } C_{1h}.$$

The correspondences of irreps at HSPs from original SG to lowered SG:

$$n_{GM4}^8 = n_{GM5}^{157} + n_{GM6}^{157} n_{GM3}^8 = n_{GM4}^{157} + n_{GM6}^{157} n_{Y4}^8 = n_{M4}^{157} n_{Y3}^8 = n_{M3}^{157} n_{V2}^8 = n_{M3}^{157} + n_{M4}^{157} n_{A4}^8 = n_{A5}^{157} + n_{A6}^{157} n_{A3}^8 = n_{A4}^{157} + n_{A6}^{157} n_{M4}^8 = n_{L4}^{157} n_{M3}^8 = n_{L3}^{157} n_{L2}^8 = n_{L3}^{157} + n_{L4}^{157}$$

The lower SG is SG 8 when the preserved operations are: **(sub-SG label is 2) 1, 4.**

$$\text{The transformation is: } (\mathbf{a}_8, \mathbf{b}_8, \mathbf{c}_8) = (\mathbf{a}_{157}, \mathbf{b}_{157}, \mathbf{c}_{157}) \begin{pmatrix} 0 & 2 & 0 \\ -1 & 1 & 0 \\ 0 & 0 & 1 \end{pmatrix}, \overrightarrow{O_{157}O_8} = \mathbf{0}$$

The reduction of higher dimensional irrep:

$C_{3v} : E \rightarrow A' + A''$  of  $C_{1h}$ .

The correspondences of irreps at HSPs from original SG to lowered SG:

$$\begin{aligned} n_{GM4}^8 &= n_{GM4}^{157} + n_{GM6}^{157} & n_{GM3}^8 &= n_{GM5}^{157} + n_{GM6}^{157} & n_{Y4}^8 &= n_{M3}^{157} n_{Y3}^8 = n_{M4}^{157} n_{V2}^8 = n_{M3}^{157} + n_{M4}^{157} & n_{A4}^8 &= n_{A4}^{157} + n_{A6}^{157} & n_{A3}^8 &= \\ n_{A5}^{157} + n_{A6}^{157} & n_{M4}^8 &= n_{L3}^{157} & n_{M3}^8 &= n_{L4}^{157} & n_{L2}^8 &= n_{L3}^{157} + n_{L4}^{157} \end{aligned}$$

The lower SG is SG 8 when the preserved operations are: **(sub-SG label is 3) 1, 6.**

The transformation is:  $(\mathbf{a}_8, \mathbf{b}_8, \mathbf{c}_8) = (\mathbf{a}_{157}, \mathbf{b}_{157}, \mathbf{c}_{157}) \begin{pmatrix} -1 & -1 & 0 \\ -1 & 1 & 0 \\ 0 & 0 & -1 \end{pmatrix}, \overrightarrow{O_{157}O_8} = \mathbf{0}$

The reduction of higher dimensional irrep:

$C_{3v} : E \rightarrow A' + A''$  of  $C_{1h}$ .

The correspondences of irreps at HSPs from original SG to lowered SG:

$$\begin{aligned} n_{GM4}^8 &= n_{GM4}^{157} + n_{GM6}^{157} & n_{GM3}^8 &= n_{GM5}^{157} + n_{GM6}^{157} & n_{Y4}^8 &= n_{M3}^{157} n_{Y3}^8 = n_{M4}^{157} n_{V2}^8 = n_{M3}^{157} + n_{M4}^{157} & n_{A4}^8 &= n_{A4}^{157} + n_{A6}^{157} & n_{A3}^8 &= \\ n_{A5}^{157} + n_{A6}^{157} & n_{M4}^8 &= n_{L3}^{157} & n_{M3}^8 &= n_{L4}^{157} & n_{L2}^8 &= n_{L3}^{157} + n_{L4}^{157} \end{aligned}$$

The lower SG is SG 143 when the preserved operations are: **(sub-SG label is 4) 1, 2, 3.**

The transformation is:  $(\mathbf{a}_{143}, \mathbf{b}_{143}, \mathbf{c}_{143}) = (\mathbf{a}_{157}, \mathbf{b}_{157}, \mathbf{c}_{157}) \begin{pmatrix} -1 & 1 & 0 \\ -1 & 0 & 0 \\ 0 & 0 & 1 \end{pmatrix}, \overrightarrow{O_{157}O_{143}} = -\frac{1}{3}\mathbf{a}_{143} + (\frac{1}{3})\mathbf{b}_{143}$

The reduction of higher dimensional irrep:

$C_{3v} : E \rightarrow {}^2E + {}^1E$  of  $C_3$ .

The correspondences of irreps at HSPs from original SG to lowered SG:

$$\begin{aligned} n_{GM4}^{143} &= n_{GM4}^{157} + n_{GM5}^{157} & n_{GM6}^{143} &= n_{GM6}^{157} & n_{GM5}^{143} &= n_{GM6}^{157} & n_{M2}^{143} &= n_{M3}^{157} + n_{M4}^{157} & n_{K4}^{143} &= n_{K6}^{157} & n_{K6}^{143} &= n_{K6}^{157} & n_{K5}^{143} &= n_{K4}^{157} + n_{K5}^{157} \\ n_{A4}^{143} &= n_{A4}^{157} + n_{A5}^{157} & n_{A6}^{143} &= n_{A6}^{157} & n_{A5}^{143} &= n_{A6}^{157} & n_{L2}^{143} &= n_{L3}^{157} + n_{L4}^{157} & n_{H4}^{143} &= n_{H6}^{157} & n_{H6}^{143} &= n_{H6}^{157} & n_{H5}^{143} &= n_{H4}^{157} + n_{H5}^{157} \end{aligned}$$

#### 64. Lowered SGs by higher-dimensional irreps of pairings in SG 158

The representative operations of SG/T for SG 158:

$$1 : (x, y, z), 2 : (-y, x - y, z), 3 : (y - x, -x, z), 4 : (y - x, y, z + \frac{1}{2}), 5 : (-y, -x, z + \frac{1}{2}), 6 : (x, x - y, z + \frac{1}{2}).$$

The lower SG is SG 9 when the preserved operations are: **(sub-SG label is 1) 1, 4.**

The transformation is:  $(\mathbf{a}_9, \mathbf{b}_9, \mathbf{c}_9) = (\mathbf{a}_{158}, \mathbf{b}_{158}, \mathbf{c}_{158}) \begin{pmatrix} -1 & -1 & 0 \\ -2 & 0 & 0 \\ 0 & 0 & -1 \end{pmatrix}, \overrightarrow{O_{158}O_9} = \mathbf{0}$

The reduction of higher dimensional irrep:

$C_{3v} : E \rightarrow A' + A''$  of  $C_{1h}$ .

The correspondences of irreps at HSPs from original SG to lowered SG:

$$\begin{aligned} n_{GM4}^9 &= n_{GM5}^{158} + n_{GM6}^{158} & n_{GM3}^9 &= n_{GM4}^{158} + n_{GM6}^{158} & n_{Y4}^9 &= n_{M3}^{158} n_{Y3}^9 = n_{M4}^{158} n_{V2}^9 = n_{M3}^{158} + n_{M4}^{158} & n_{A4}^9 &= n_{A4}^{158} + n_{A6}^{158} & n_{A3}^9 &= \\ n_{A5}^{158} + n_{A6}^{158} & n_{M4}^9 &= n_{L3}^{158} & n_{M3}^9 &= n_{L4}^{158} & n_{L2}^9 &= n_{L3}^{158} + n_{L4}^{158} \end{aligned}$$

The lower SG is SG 9 when the preserved operations are: **(sub-SG label is 2) 1, 6.**

The transformation is:  $(\mathbf{a}_9, \mathbf{b}_9, \mathbf{c}_9) = (\mathbf{a}_{158}, \mathbf{b}_{158}, \mathbf{c}_{158}) \begin{pmatrix} -2 & 0 & 0 \\ -1 & 1 & 0 \\ 0 & 0 & -1 \end{pmatrix}, \overrightarrow{O_{158}O_9} = \mathbf{0}$

The reduction of higher dimensional irrep:

$C_{3v} : E \rightarrow A' + A''$  of  $C_{1h}$ .

The correspondences of irreps at HSPs from original SG to lowered SG:

$$\begin{aligned} n_{GM4}^9 &= n_{GM4}^{158} + n_{GM6}^{158} & n_{GM3}^9 &= n_{GM5}^{158} + n_{GM6}^{158} & n_{Y4}^9 &= n_{M3}^{158} n_{Y3}^9 = n_{M4}^{158} n_{V2}^9 = n_{M3}^{158} + n_{M4}^{158} & n_{A4}^9 &= n_{A4}^{158} + n_{A6}^{158} & n_{A3}^9 &= \\ n_{A4}^{158} + n_{A6}^{158} & n_{M4}^9 &= n_{L4}^{158} & n_{M3}^9 &= n_{L3}^{158} & n_{L2}^9 &= n_{L3}^{158} + n_{L4}^{158} \end{aligned}$$

The lower SG is SG 9 when the preserved operations are: **(sub-SG label is 3) 1, 5.**

The transformation is:  $(\mathbf{a}_9, \mathbf{b}_9, \mathbf{c}_9) = (\mathbf{a}_{158}, \mathbf{b}_{158}, \mathbf{c}_{158}) \begin{pmatrix} -1 & 1 & 0 \\ 1 & 1 & 0 \\ 0 & 0 & -1 \end{pmatrix}, \overrightarrow{O_{158}O_9} = \mathbf{0}$

The reduction of higher dimensional irrep:

$C_{3v} : E \rightarrow A' + A''$  of  $C_{1h}$ .

The correspondences of irreps at HSPs from original SG to lowered SG:

$$\begin{aligned} n_{GM4}^9 &= n_{GM5}^{158} + n_{GM6}^{158} & n_{GM3}^9 &= n_{GM4}^{158} + n_{GM6}^{158} & n_{Y4}^9 &= n_{M4}^{158} & n_{Y3}^9 &= n_{M3}^{158} & n_{V2}^9 &= n_{M3}^{158} + n_{M4}^{158} & n_{A4}^9 &= n_{A4}^{158} + n_{A6}^{158} & n_{A3}^9 &= \\ n_{A5}^{158} + n_{A6}^{158} & n_{M4}^9 &= n_{L3}^{158} & n_{M3}^9 &= n_{L4}^{158} & n_{L2}^9 &= n_{L3}^{158} + n_{L4}^{158} \end{aligned}$$

The lower SG is SG 143 when the preserved operations are: **(sub-SG label is 4) 1, 2, 3.**

The transformation is:  $(\mathbf{a}_{143}, \mathbf{b}_{143}, \mathbf{c}_{143}) = (\mathbf{a}_{158}, \mathbf{b}_{158}, \mathbf{c}_{158}) \begin{pmatrix} -1 & 1 & 0 \\ -1 & 0 & 0 \\ 0 & 0 & 1 \end{pmatrix}, \overrightarrow{O_{158}O_{143}} = -\frac{1}{3}\mathbf{a}_{143} + (\frac{1}{3})\mathbf{b}_{143}$

The reduction of higher dimensional irrep:

$C_{3v} : E \rightarrow {}^2E + {}^1E$  of  $C_3$ .

The correspondences of irreps at HSPs from original SG to lowered SG:

$$\begin{aligned} n_{GM4}^{143} &= n_{GM4}^{158} + n_{GM5}^{158} & n_{GM6}^{143} &= n_{GM6}^{158} & n_{M2}^{143} &= n_{M3}^{158} + n_{M4}^{158} & n_{K4}^{143} &= n_{K6}^{158} & n_{K6}^{143} &= n_{K5}^{158} & n_{K5}^{143} &= n_{K4}^{158} & n_{A4}^{143} &= \\ n_{A4}^{158} + n_{A5}^{158} & n_{A6}^{143} &= n_{A6}^{158} & n_{A5}^{143} &= n_{A6}^{158} & n_{L2}^{143} &= n_{L3}^{158} + n_{L4}^{158} & n_{H4}^{143} &= n_{H6}^{158} & n_{H6}^{143} &= n_{H5}^{158} & n_{H5}^{143} &= n_{H4}^{158} \end{aligned}$$

### 65. Lowered SGs by higher-dimensional irreps of pairings in SG 159

The representative operations of SG/T for SG 159:

$$1 : (x, y, z), 2 : (-y, x - y, z), 3 : (y - x, -x, z), 4 : (-x, y - x, z + \frac{1}{2}), 5 : (x - y, -y, z + \frac{1}{2}), 6 : (y, x, z + \frac{1}{2}).$$

The lower SG is SG 9 when the preserved operations are: **(sub-SG label is 1) 1, 5.**

The transformation is:  $(\mathbf{a}_9, \mathbf{b}_9, \mathbf{c}_9) = (\mathbf{a}_{159}, \mathbf{b}_{159}, \mathbf{c}_{159}) \begin{pmatrix} -1 & 1 & 0 \\ 0 & 2 & 0 \\ 0 & 0 & -1 \end{pmatrix}, \overrightarrow{O_{159}O_9} = \mathbf{0}$

The reduction of higher dimensional irrep:

$C_{3v} : E \rightarrow A' + A''$  of  $C_{1h}$ .

The correspondences of irreps at HSPs from original SG to lowered SG:

$$\begin{aligned} n_{GM4}^9 &= n_{GM4}^{159} + n_{GM6}^{159} & n_{GM3}^9 &= n_{GM5}^{159} + n_{GM6}^{159} & n_{Y4}^9 &= n_{M4}^{159} & n_{Y3}^9 &= n_{M3}^{159} & n_{V2}^9 &= n_{M3}^{159} + n_{M4}^{159} & n_{A4}^9 &= n_{A4}^{159} + n_{A6}^{159} & n_{A3}^9 &= \\ n_{A5}^{159} + n_{A6}^{159} & n_{M4}^9 &= n_{L3}^{159} & n_{M3}^9 &= n_{L4}^{159} & n_{L2}^9 &= n_{L3}^{159} + n_{L4}^{159} \end{aligned}$$

The lower SG is SG 9 when the preserved operations are: **(sub-SG label is 2) 1, 4.**

The transformation is:  $(\mathbf{a}_9, \mathbf{b}_9, \mathbf{c}_9) = (\mathbf{a}_{159}, \mathbf{b}_{159}, \mathbf{c}_{159}) \begin{pmatrix} 0 & 2 & 0 \\ -1 & 1 & 0 \\ 0 & 0 & 1 \end{pmatrix}, \overrightarrow{O_{159}O_9} = \mathbf{0}$

The reduction of higher dimensional irrep:

$C_{3v} : E \rightarrow A' + A''$  of  $C_{1h}$ .

The correspondences of irreps at HSPs from original SG to lowered SG:

$$\begin{aligned} n_{GM4}^9 &= n_{GM4}^{159} + n_{GM6}^{159} & n_{GM3}^9 &= n_{GM5}^{159} + n_{GM6}^{159} & n_{Y4}^9 &= n_{M4}^{159} & n_{Y3}^9 &= n_{M3}^{159} & n_{V2}^9 &= n_{M3}^{159} + n_{M4}^{159} & n_{A4}^9 &= n_{A4}^{159} + n_{A6}^{159} & n_{A3}^9 &= \\ n_{A5}^{159} + n_{A6}^{159} & n_{M4}^9 &= n_{L3}^{159} & n_{M3}^9 &= n_{L4}^{159} & n_{L2}^9 &= n_{L3}^{159} + n_{L4}^{159} \end{aligned}$$

The lower SG is SG 9 when the preserved operations are: **(sub-SG label is 3) 1, 6.**

The transformation is:  $(\mathbf{a}_9, \mathbf{b}_9, \mathbf{c}_9) = (\mathbf{a}_{159}, \mathbf{b}_{159}, \mathbf{c}_{159}) \begin{pmatrix} -1 & -1 & 0 \\ -1 & 1 & 0 \\ 0 & 0 & -1 \end{pmatrix}, \overrightarrow{O_{159}O_9} = \mathbf{0}$

The reduction of higher dimensional irrep:

$C_{3v} : E \rightarrow A' + A''$  of  $C_{1h}$ .

The correspondences of irreps at HSPs from original SG to lowered SG:

$$\begin{aligned} n_{GM4}^9 &= n_{GM4}^{159} + n_{GM6}^{159} & n_{GM3}^9 &= n_{GM5}^{159} + n_{GM6}^{159} & n_{Y4}^9 &= n_{M4}^{159} & n_{Y3}^9 &= n_{M3}^{159} & n_{V2}^9 &= n_{M3}^{159} + n_{M4}^{159} & n_{A4}^9 &= n_{A4}^{159} + n_{A6}^{159} & n_{A3}^9 &= \\ n_{A5}^{159} + n_{A6}^{159} & n_{M4}^9 &= n_{L3}^{159} & n_{M3}^9 &= n_{L4}^{159} & n_{L2}^9 &= n_{L3}^{159} + n_{L4}^{159} \end{aligned}$$

$$n_{A4}^{159} + n_{A6}^{159} n_{M4}^9 = n_{L4}^{159} n_{M3}^9 = n_{L3}^{159} n_{L2}^9 = n_{L3}^{159} + n_{L4}^{159}$$

The lower SG is SG 143 when the preserved operations are: **(sub-SG label is 4) 1, 2, 3.**

$$\text{The transformation is: } (\mathbf{a}_{143}, \mathbf{b}_{143}, \mathbf{c}_{143}) = (\mathbf{a}_{159}, \mathbf{b}_{159}, \mathbf{c}_{159}) \begin{pmatrix} -1 & 1 & 0 \\ -1 & 0 & 0 \\ 0 & 0 & 1 \end{pmatrix}, \overrightarrow{O_{159}O_{143}} = -\frac{1}{3}\mathbf{a}_{143} + \left(\frac{1}{3}\right)\mathbf{b}_{143}$$

The reduction of higher dimensional irrep:

$$C_{3v} : E \rightarrow {}^2E + {}^1E \text{ of } C_3.$$

The correspondences of irreps at HSPs from original SG to lowered SG:

$$\begin{aligned} n_{GM4}^{143} &= n_{GM4}^{159} + n_{GM5}^{159} n_{GM6}^{143} = n_{GM6}^{159} n_{GM5}^{143} = n_{GM6}^{159} n_{M2}^{143} = n_{M3}^{159} + n_{M4}^{159} n_{K4}^{143} = n_{K6}^{159} n_{K6}^{143} = n_{K6}^{159} n_{K5}^{143} = n_{K4}^{159} + n_{K5}^{159} \\ n_{A4}^{143} &= n_{A4}^{159} + n_{A5}^{159} n_{A6}^{143} = n_{A6}^{159} n_{A5}^{143} = n_{A6}^{159} n_{L2}^{143} = n_{L3}^{159} + n_{L4}^{159} n_{H4}^{143} = n_{H6}^{159} n_{H6}^{143} = n_{H6}^{159} n_{H5}^{143} = n_{H4}^{159} + n_{H5}^{159} \end{aligned}$$

## 66. Lowered SGs by higher-dimensional irreps of pairings in SG 160

The representative operations of SG/T for SG 160:

$$1 : (x, y, z), 2 : (z, x, y), 3 : (y, z, x), 4 : (y, x, z), 5 : (z, y, x), 6 : (x, z, y).$$

The lower SG is SG 8 when the preserved operations are: **(sub-SG label is 1) 1, 6.**

$$\text{The transformation is: } (\mathbf{a}_8, \mathbf{b}_8, \mathbf{c}_8) = (\mathbf{a}_{160}, \mathbf{b}_{160}, \mathbf{c}_{160}) \begin{pmatrix} -2 & 0 & 1 \\ 1 & 1 & -1 \\ 1 & -1 & -1 \end{pmatrix}, \overrightarrow{O_{160}O_8} = \mathbf{0}$$

The reduction of higher dimensional irrep:

$$C_{3v} : E \rightarrow A' + A'' \text{ of } C_{1h}.$$

The correspondences of irreps at HSPs from original SG to lowered SG:

$$\begin{aligned} n_{GM4}^8 &= n_{GM4}^{160} + n_{GM6}^{160} n_{GM3}^8 = n_{GM5}^{160} + n_{GM6}^{160} n_{Y4}^8 = n_{F4}^{160} n_{Y3}^8 = n_{F3}^{160} n_{V2}^8 = n_{F3}^{160} + n_{F4}^{160} n_{A4}^8 = n_{T4}^{160} + n_{T6}^{160} n_{A3}^8 = \\ n_{T5}^{160} + n_{T6}^{160} n_{M4}^8 &= n_{L3}^{160} n_{M3}^8 = n_{L4}^{160} n_{L2}^8 = n_{L3}^{160} + n_{L4}^{160} \end{aligned}$$

The lower SG is SG 8 when the preserved operations are: **(sub-SG label is 2) 1, 5.**

$$\text{The transformation is: } (\mathbf{a}_8, \mathbf{b}_8, \mathbf{c}_8) = (\mathbf{a}_{160}, \mathbf{b}_{160}, \mathbf{c}_{160}) \begin{pmatrix} -1 & 1 & 0 \\ 0 & 0 & -1 \\ -1 & -1 & 0 \end{pmatrix}, \overrightarrow{O_{160}O_8} = \mathbf{0}$$

The reduction of higher dimensional irrep:

$$C_{3v} : E \rightarrow A' + A'' \text{ of } C_{1h}.$$

The correspondences of irreps at HSPs from original SG to lowered SG:

$$\begin{aligned} n_{GM4}^8 &= n_{GM5}^{160} + n_{GM6}^{160} n_{GM3}^8 = n_{GM4}^{160} + n_{GM6}^{160} n_{Y4}^8 = n_{F3}^{160} n_{Y3}^8 = n_{F4}^{160} n_{V2}^8 = n_{L3}^{160} + n_{L4}^{160} n_{A4}^8 = n_{L4}^{160} n_{A3}^8 = n_{L3}^{160} \\ n_{M4}^8 &= n_{T5}^{160} + n_{T6}^{160} n_{M3}^8 = n_{T4}^{160} + n_{T6}^{160} n_{L2}^8 = n_{F3}^{160} + n_{F4}^{160} \end{aligned}$$

The lower SG is SG 8 when the preserved operations are: **(sub-SG label is 3) 1, 4.**

$$\text{The transformation is: } (\mathbf{a}_8, \mathbf{b}_8, \mathbf{c}_8) = (\mathbf{a}_{160}, \mathbf{b}_{160}, \mathbf{c}_{160}) \begin{pmatrix} -1 & -1 & 0 \\ -1 & 1 & 0 \\ 0 & 0 & -1 \end{pmatrix}, \overrightarrow{O_{160}O_8} = \mathbf{0}$$

The reduction of higher dimensional irrep:

$$C_{3v} : E \rightarrow A' + A'' \text{ of } C_{1h}.$$

The correspondences of irreps at HSPs from original SG to lowered SG:

$$\begin{aligned} n_{GM4}^8 &= n_{GM5}^{160} + n_{GM6}^{160} n_{GM3}^8 = n_{GM4}^{160} + n_{GM6}^{160} n_{Y4}^8 = n_{F3}^{160} n_{Y3}^8 = n_{F4}^{160} n_{V2}^8 = n_{L3}^{160} + n_{L4}^{160} n_{A4}^8 = n_{L4}^{160} n_{A3}^8 = n_{L3}^{160} \\ n_{M4}^8 &= n_{T5}^{160} + n_{T6}^{160} n_{M3}^8 = n_{T4}^{160} + n_{T6}^{160} n_{L2}^8 = n_{F3}^{160} + n_{F4}^{160} \end{aligned}$$

The lower SG is SG 146 when the preserved operations are: **(sub-SG label is 4) 1, 2, 3.**

$$\text{The transformation is: } (\mathbf{a}_{146}, \mathbf{b}_{146}, \mathbf{c}_{146}) = (\mathbf{a}_{160}, \mathbf{b}_{160}, \mathbf{c}_{160}) \begin{pmatrix} 0 & 1 & 0 \\ 0 & 0 & 1 \\ 1 & 0 & 0 \end{pmatrix}, \overrightarrow{O_{160}O_{146}} = -\frac{1}{3}\mathbf{a}_{146} + \left(\frac{2}{3}\right)\mathbf{b}_{146} + \left(-\frac{1}{3}\right)\mathbf{c}_{146}$$

The reduction of higher dimensional irrep:

$C_{3v} : E \rightarrow {}^2E + {}^1E$  of  $C_3$ .

The correspondences of irreps at HSPs from original SG to lowered SG:

$$n_{GM4}^{146} = n_{GM4}^{160} + n_{GM5}^{160} n_{GM6}^{146} = n_{GM6}^{160} n_{GM5}^{146} = n_{GM6}^{160} n_{L2}^{146} = n_{L3}^{160} + n_{L4}^{160} n_{F2}^{146} = n_{F3}^{160} + n_{F4}^{160} n_{T4}^{146} = n_{T4}^{160} + n_{T5}^{160} n_{T6}^{146} = n_{T6}^{160} n_{T5}^{146} = n_{T6}^{160}$$

### 67. Lowered SGs by higher-dimensional irreps of pairings in SG 161

The representative operations of SG/T for SG 161:

$$1 : (x, y, z), 2 : (z, x, y), 3 : (y, z, x), 4 : (y + \frac{1}{2}, x + \frac{1}{2}, z + \frac{1}{2}), 5 : (z + \frac{1}{2}, y + \frac{1}{2}, x + \frac{1}{2}), 6 : (x + \frac{1}{2}, z + \frac{1}{2}, y + \frac{1}{2}).$$

The lower SG is SG 9 when the preserved operations are: (**sub-SG label is 1**) 1, 6.

$$\text{The transformation is: } (\mathbf{a}_9, \mathbf{b}_9, \mathbf{c}_9) = (\mathbf{a}_{161}, \mathbf{b}_{161}, \mathbf{c}_{161}) \begin{pmatrix} -2 & 0 & 1 \\ 1 & 1 & -1 \\ 1 & -1 & -1 \end{pmatrix}, \overrightarrow{O_{161}O_9} = \mathbf{0}$$

The reduction of higher dimensional irrep:

$C_{3v} : E \rightarrow A' + A''$  of  $C_{1h}$ .

The correspondences of irreps at HSPs from original SG to lowered SG:

$$n_{GM4}^9 = n_{GM4}^{161} + n_{GM6}^{161} n_{GM3}^9 = n_{GM5}^{161} + n_{GM6}^{161} n_{Y4}^9 = n_{F3}^{161} n_{Y3}^9 = n_{F4}^{161} n_{V2}^9 = n_{F3}^{161} + n_{F4}^{161} n_{A4}^9 = n_{T5}^{161} + n_{T6}^{161} n_{A3}^9 = n_{T4}^{161} + n_{T6}^{161} n_{M4}^9 = n_{L3}^{161} n_{M3}^9 = n_{L4}^{161} n_{L2}^9 = n_{L3}^{161} + n_{L4}^{161}$$

The lower SG is SG 9 when the preserved operations are: (**sub-SG label is 2**) 1, 5.

$$\text{The transformation is: } (\mathbf{a}_9, \mathbf{b}_9, \mathbf{c}_9) = (\mathbf{a}_{161}, \mathbf{b}_{161}, \mathbf{c}_{161}) \begin{pmatrix} -1 & 1 & 0 \\ 0 & 0 & -1 \\ -1 & -1 & 0 \end{pmatrix}, \overrightarrow{O_{161}O_9} = -\frac{1}{4}\mathbf{b}_9$$

The reduction of higher dimensional irrep:

$C_{3v} : E \rightarrow A' + A''$  of  $C_{1h}$ .

The correspondences of irreps at HSPs from original SG to lowered SG:

$$n_{GM4}^9 = n_{GM5}^{161} + n_{GM6}^{161} n_{GM3}^9 = n_{GM4}^{161} + n_{GM6}^{161} n_{Y4}^9 = n_{F3}^{161} n_{Y3}^9 = n_{F4}^{161} n_{V2}^9 = n_{L3}^{161} + n_{L4}^{161} n_{A4}^9 = n_{L3}^{161} n_{A3}^9 = n_{L4}^{161} n_{M4}^9 = n_{T4}^{161} + n_{T6}^{161} n_{M3}^9 = n_{T5}^{161} + n_{T6}^{161} n_{L2}^9 = n_{F3}^{161} + n_{F4}^{161}$$

The lower SG is SG 9 when the preserved operations are: (**sub-SG label is 3**) 1, 4.

$$\text{The transformation is: } (\mathbf{a}_9, \mathbf{b}_9, \mathbf{c}_9) = (\mathbf{a}_{161}, \mathbf{b}_{161}, \mathbf{c}_{161}) \begin{pmatrix} -1 & -1 & 0 \\ -1 & 1 & 0 \\ 0 & 0 & -1 \end{pmatrix}, \overrightarrow{O_{161}O_9} = -\frac{1}{4}\mathbf{b}_9$$

The reduction of higher dimensional irrep:

$C_{3v} : E \rightarrow A' + A''$  of  $C_{1h}$ .

The correspondences of irreps at HSPs from original SG to lowered SG:

$$n_{GM4}^9 = n_{GM5}^{161} + n_{GM6}^{161} n_{GM3}^9 = n_{GM4}^{161} + n_{GM6}^{161} n_{Y4}^9 = n_{F3}^{161} n_{Y3}^9 = n_{F4}^{161} n_{V2}^9 = n_{L3}^{161} + n_{L4}^{161} n_{A4}^9 = n_{L3}^{161} n_{A3}^9 = n_{L4}^{161} n_{M4}^9 = n_{T4}^{161} + n_{T6}^{161} n_{M3}^9 = n_{T5}^{161} + n_{T6}^{161} n_{L2}^9 = n_{F3}^{161} + n_{F4}^{161}$$

The lower SG is SG 146 when the preserved operations are: (**sub-SG label is 4**) 1, 2, 3.

$$\text{The transformation is: } (\mathbf{a}_{146}, \mathbf{b}_{146}, \mathbf{c}_{146}) = (\mathbf{a}_{161}, \mathbf{b}_{161}, \mathbf{c}_{161}) \begin{pmatrix} 0 & 1 & 0 \\ 0 & 0 & 1 \\ 1 & 0 & 0 \end{pmatrix}, \overrightarrow{O_{161}O_{146}} = -\frac{1}{3}\mathbf{a}_{146} + (\frac{2}{3})\mathbf{b}_{146} + (-\frac{1}{3})\mathbf{c}_{146}$$

The reduction of higher dimensional irrep:

$C_{3v} : E \rightarrow {}^2E + {}^1E$  of  $C_3$ .

The correspondences of irreps at HSPs from original SG to lowered SG:

$$n_{GM4}^{146} = n_{GM4}^{161} + n_{GM5}^{161} n_{GM6}^{146} = n_{GM6}^{161} n_{GM5}^{146} = n_{GM6}^{161} n_{L2}^{146} = n_{L3}^{161} + n_{L4}^{161} n_{F2}^{146} = n_{F3}^{161} + n_{F4}^{161} n_{T4}^{146} = n_{T4}^{161} + n_{T5}^{161} n_{T6}^{146} = n_{T6}^{161} n_{T5}^{146} = n_{T6}^{161}$$



~~~~~

**69. Lowered SGs by higher-dimensional irreps of pairings in SG 163**

The representative operations of SG/T for SG 163:

$$1 : (x, y, z), 2 : (-y, x - y, z), 3 : (y - x, -x, z), 4 : (x, x - y, \frac{1}{2} - z), 5 : (y - x, y, \frac{1}{2} - z), 6 : (-y, -x, \frac{1}{2} - z), \\ 7 : (-x, -y, -z), 8 : (y, y - x, -z), 9 : (x - y, x, -z), 10 : (-x, y - x, z + \frac{1}{2}), 11 : (x - y, -y, z + \frac{1}{2}), 12 : (y, x, z + \frac{1}{2}).$$

The lower SG is SG 15 when the preserved operations are: **(sub-SG label is 1) 1, 5, 7, 11.**

The transformation is:  $(\mathbf{a}_{15}, \mathbf{b}_{15}, \mathbf{c}_{15}) = (\mathbf{a}_{163}, \mathbf{b}_{163}, \mathbf{c}_{163}) \begin{pmatrix} -1 & 1 & 0 \\ 0 & 2 & 0 \\ 0 & 0 & -1 \end{pmatrix}, \overrightarrow{O_{163}O_{15}} = \frac{1}{2}\mathbf{a}_{15}$

The reduction of higher dimensional irrep:

$$D_{3d} : E_g \rightarrow A_g + B_g \text{ of } C_{2h}.$$

$$D_{3d} : E_u \rightarrow A_u + B_u \text{ of } C_{2h}.$$

The correspondences of irreps at HSPs from original SG to lowered SG:

$$n_{GM6}^{15} = n_{GM6}^{163} + n_{GM9}^{163} \quad n_{GM4}^{15} = n_{GM4}^{163} + n_{GM8}^{163} \quad n_{GM5}^{15} = n_{GM5}^{163} + n_{GM7}^{163} \quad n_{GM3}^{15} = n_{GM5}^{163} + n_{GM8}^{163} \quad n_{Y6}^{15} = n_{M6}^{163} \quad n_{Y4}^{15} = n_{M4}^{163} \\ n_{Y5}^{15} = n_{M5}^{163} \quad n_{Y3}^{15} = n_{M3}^{163} \quad n_{V3}^{15} = n_{M3}^{163} + n_{M4}^{163} \quad n_{V2}^{15} = n_{M5}^{163} + n_{M6}^{163} \quad n_{A2}^{15} = n_{A4}^{163} + n_{A5}^{163} + n_{A6}^{163} \quad n_{M2}^{15} = n_{L2}^{163} \quad n_{L3}^{15} = n_{L2}^{163} \quad n_{L2}^{15} = n_{L2}^{163}$$

~~~~~

The lower SG is SG 15 when the preserved operations are: **(sub-SG label is 2) 1, 4, 7, 10.**

The transformation is:  $(\mathbf{a}_{15}, \mathbf{b}_{15}, \mathbf{c}_{15}) = (\mathbf{a}_{163}, \mathbf{b}_{163}, \mathbf{c}_{163}) \begin{pmatrix} 0 & 2 & 0 \\ -1 & 1 & 0 \\ 0 & 0 & 1 \end{pmatrix}, \overrightarrow{O_{163}O_{15}} = \frac{1}{2}\mathbf{a}_{15}$

The reduction of higher dimensional irrep:

$$D_{3d} : E_g \rightarrow A_g + B_g \text{ of } C_{2h}.$$

$$D_{3d} : E_u \rightarrow A_u + B_u \text{ of } C_{2h}.$$

The correspondences of irreps at HSPs from original SG to lowered SG:

$$n_{GM6}^{15} = n_{GM6}^{163} + n_{GM9}^{163} \quad n_{GM4}^{15} = n_{GM4}^{163} + n_{GM8}^{163} \quad n_{GM5}^{15} = n_{GM7}^{163} + n_{GM9}^{163} \quad n_{GM3}^{15} = n_{GM5}^{163} + n_{GM8}^{163} \quad n_{Y6}^{15} = n_{M5}^{163} \quad n_{Y4}^{15} = n_{M3}^{163} \\ n_{Y5}^{15} = n_{M6}^{163} \quad n_{Y3}^{15} = n_{M4}^{163} \quad n_{V3}^{15} = n_{M3}^{163} + n_{M4}^{163} \quad n_{V2}^{15} = n_{M5}^{163} + n_{M6}^{163} \quad n_{A2}^{15} = n_{A4}^{163} + n_{A5}^{163} + n_{A6}^{163} \quad n_{M2}^{15} = n_{L2}^{163} \quad n_{L3}^{15} = n_{L2}^{163} \quad n_{L2}^{15} = n_{L2}^{163}$$

~~~~~

The lower SG is SG 15 when the preserved operations are: **(sub-SG label is 3) 1, 6, 7, 12.**

The transformation is:  $(\mathbf{a}_{15}, \mathbf{b}_{15}, \mathbf{c}_{15}) = (\mathbf{a}_{163}, \mathbf{b}_{163}, \mathbf{c}_{163}) \begin{pmatrix} -1 & -1 & 0 \\ -1 & 1 & 0 \\ 0 & 0 & -1 \end{pmatrix}, \overrightarrow{O_{163}O_{15}} = \frac{1}{2}\mathbf{a}_{15}$

The reduction of higher dimensional irrep:

$$D_{3d} : E_g \rightarrow A_g + B_g \text{ of } C_{2h}.$$

$$D_{3d} : E_u \rightarrow A_u + B_u \text{ of } C_{2h}.$$

The correspondences of irreps at HSPs from original SG to lowered SG:

$$n_{GM6}^{15} = n_{GM6}^{163} + n_{GM9}^{163} \quad n_{GM4}^{15} = n_{GM4}^{163} + n_{GM8}^{163} \quad n_{GM5}^{15} = n_{GM7}^{163} + n_{GM9}^{163} \quad n_{GM3}^{15} = n_{GM5}^{163} + n_{GM8}^{163} \quad n_{Y6}^{15} = n_{M5}^{163} \quad n_{Y4}^{15} = n_{M3}^{163} \\ n_{Y5}^{15} = n_{M6}^{163} \quad n_{Y3}^{15} = n_{M4}^{163} \quad n_{V3}^{15} = n_{M3}^{163} + n_{M4}^{163} \quad n_{V2}^{15} = n_{M5}^{163} + n_{M6}^{163} \quad n_{A2}^{15} = n_{A4}^{163} + n_{A5}^{163} + n_{A6}^{163} \quad n_{M2}^{15} = n_{L2}^{163} \quad n_{L3}^{15} = n_{L2}^{163} \quad n_{L2}^{15} = n_{L2}^{163}$$

~~~~~

The lower SG is SG 147 when the preserved operations are: **(sub-SG label is 4) 1, 2, 3, 7, 8, 9.**

The transformation is:  $(\mathbf{a}_{147}, \mathbf{b}_{147}, \mathbf{c}_{147}) = (\mathbf{a}_{163}, \mathbf{b}_{163}, \mathbf{c}_{163}) \begin{pmatrix} -1 & 1 & 0 \\ -1 & 0 & 0 \\ 0 & 0 & 1 \end{pmatrix}, \overrightarrow{O_{163}O_{147}} = \frac{1}{2}\mathbf{c}_{147}$

The reduction of higher dimensional irrep:

$$D_{3d} : E_g \rightarrow {}^2E_g + {}^1E_g \text{ of } C_{3i}.$$

$$D_{3d} : E_u \rightarrow {}^1E_u + {}^2E_u \text{ of } C_{3i}.$$

The correspondences of irreps at HSPs from original SG to lowered SG:

$$\begin{aligned}
n_{GM7}^{147} &= n_{GM6}^{163} + n_{GM7}^{163} n_{GM4}^{147} = n_{GM4}^{163} + n_{GM5}^{163} n_{GM9}^{147} = n_{GM9}^{163} n_{GM6}^{147} = n_{GM8}^{163} n_{GM8}^{147} = n_{GM9}^{163} n_{GM5}^{147} = n_{GM8}^{163} n_{M2}^{147} = \\
n_{M5}^{163} + n_{M6}^{163} n_{M3}^{147} &= n_{M3}^{163} + n_{M4}^{163} n_{K4}^{147} = n_{K4}^{163} + n_{K5}^{163} n_{K6}^{147} = n_{K6}^{163} n_{K5}^{147} = n_{K6}^{163} n_{A7}^{147} = n_{A4}^{163} n_{A4}^{147} = n_{A4}^{163} n_{A9}^{147} = n_{A6}^{163} n_{A6}^{147} = \\
n_{A5}^{163} n_{A8}^{147} &= n_{A5}^{163} n_{A5}^{147} = n_{A6}^{163} n_{L2}^{147} = n_{L2}^{163} n_{L3}^{147} = n_{L2}^{163} n_{H4}^{147} = n_{H4}^{163} + n_{H5}^{163} n_{H6}^{147} = n_{H6}^{163} n_{H5}^{147} = n_{H6}^{163}
\end{aligned}$$

### 70. Lowered SGs by higher-dimensional irreps of pairings in SG 164

The representative operations of SG/T for SG 164:

$$1 : (x, y, z), 2 : (-y, x - y, z), 3 : (y - x, -x, z), 4 : (x - y, -y, -z), 5 : (y, x, -z), 6 : (-x, y - x, -z), 7 : (-x, -y, -z), 8 : (y, y - x, -z), 9 : (x - y, x, -z), 10 : (y - x, y, z), 11 : (-y, -x, z), 12 : (x, x - y, z).$$

The lower SG is SG 12 when the preserved operations are: **(sub-SG label is 1) 1, 4, 7, 10.**

$$\text{The transformation is: } (\mathbf{a}_{12}, \mathbf{b}_{12}, \mathbf{c}_{12}) = (\mathbf{a}_{164}, \mathbf{b}_{164}, \mathbf{c}_{164}) \begin{pmatrix} -1 & -1 & 0 \\ -2 & 0 & 0 \\ 0 & 0 & -1 \end{pmatrix}, \overrightarrow{O_{164}O_{12}} = \frac{1}{2}\mathbf{a}_{12}$$

The reduction of higher dimensional irrep:

$$D_{3d} : E_g \rightarrow A_g + B_g \text{ of } C_{2h}.$$

$$D_{3d} : E_u \rightarrow A_u + B_u \text{ of } C_{2h}.$$

The correspondences of irreps at HSPs from original SG to lowered SG:

$$\begin{aligned}
n_{GM6}^{12} &= n_{GM7}^{164} + n_{GM9}^{164} n_{GM4}^{12} = n_{GM5}^{164} + n_{GM8}^{164} n_{GM5}^{12} = n_{GM6}^{164} + n_{GM9}^{164} n_{GM3}^{12} = n_{GM4}^{164} + n_{GM8}^{164} n_{Y6}^{12} = n_{M6}^{164} n_{Y4}^{12} = n_{M3}^{164} \\
n_{Y5}^{12} &= n_{M5}^{164} n_{Y3}^{12} = n_{M3}^{164} n_{V2}^{12} = n_{M3}^{164} + n_{M4}^{164} n_{V3}^{12} = n_{M5}^{164} + n_{M6}^{164} n_{A6}^{12} = n_{A7}^{164} + n_{A9}^{164} n_{A4}^{12} = n_{A5}^{164} + n_{A8}^{164} n_{A5}^{12} = n_{A6}^{164} + n_{A9}^{164} \\
n_{A3}^{12} &= n_{A4}^{164} + n_{A8}^{164} n_{M6}^{12} = n_{L6}^{164} n_{M4}^{12} = n_{L4}^{164} n_{M5}^{12} = n_{L5}^{164} n_{M3}^{12} = n_{L3}^{164} n_{L2}^{12} = n_{L3}^{164} + n_{L4}^{164} n_{L3}^{12} = n_{L5}^{164} + n_{L6}^{164}
\end{aligned}$$

The lower SG is SG 12 when the preserved operations are: **(sub-SG label is 2) 1, 6, 7, 12.**

$$\text{The transformation is: } (\mathbf{a}_{12}, \mathbf{b}_{12}, \mathbf{c}_{12}) = (\mathbf{a}_{164}, \mathbf{b}_{164}, \mathbf{c}_{164}) \begin{pmatrix} -2 & 0 & 0 \\ -1 & 1 & 0 \\ 0 & 0 & -1 \end{pmatrix}, \overrightarrow{O_{164}O_{12}} = \frac{1}{2}\mathbf{a}_{12}$$

The reduction of higher dimensional irrep:

$$D_{3d} : E_g \rightarrow A_g + B_g \text{ of } C_{2h}.$$

$$D_{3d} : E_u \rightarrow A_u + B_u \text{ of } C_{2h}.$$

The correspondences of irreps at HSPs from original SG to lowered SG:

$$\begin{aligned}
n_{GM6}^{12} &= n_{GM6}^{164} + n_{GM9}^{164} n_{GM4}^{12} = n_{GM4}^{164} + n_{GM8}^{164} n_{GM5}^{12} = n_{GM7}^{164} + n_{GM9}^{164} n_{GM3}^{12} = n_{GM5}^{164} + n_{GM8}^{164} n_{Y6}^{12} = n_{M5}^{164} n_{Y4}^{12} = n_{M3}^{164} \\
n_{Y5}^{12} &= n_{M6}^{164} n_{Y3}^{12} = n_{M4}^{164} n_{V2}^{12} = n_{M3}^{164} + n_{M4}^{164} n_{V3}^{12} = n_{M5}^{164} + n_{M6}^{164} n_{A6}^{12} = n_{A7}^{164} + n_{A9}^{164} n_{A4}^{12} = n_{A5}^{164} + n_{A8}^{164} n_{A5}^{12} = n_{A6}^{164} + n_{A9}^{164} \\
n_{A3}^{12} &= n_{A5}^{164} + n_{A8}^{164} n_{M6}^{12} = n_{L5}^{164} n_{M4}^{12} = n_{L3}^{164} n_{M5}^{12} = n_{L6}^{164} n_{M3}^{12} = n_{L4}^{164} n_{L2}^{12} = n_{L3}^{164} + n_{L4}^{164} n_{L3}^{12} = n_{L5}^{164} + n_{L6}^{164}
\end{aligned}$$

The lower SG is SG 12 when the preserved operations are: **(sub-SG label is 3) 1, 5, 7, 11.**

$$\text{The transformation is: } (\mathbf{a}_{12}, \mathbf{b}_{12}, \mathbf{c}_{12}) = (\mathbf{a}_{164}, \mathbf{b}_{164}, \mathbf{c}_{164}) \begin{pmatrix} -1 & 1 & 0 \\ 1 & 1 & 0 \\ 0 & 0 & -1 \end{pmatrix}, \overrightarrow{O_{164}O_{12}} = \frac{1}{2}\mathbf{a}_{12}$$

The reduction of higher dimensional irrep:

$$D_{3d} : E_g \rightarrow A_g + B_g \text{ of } C_{2h}.$$

$$D_{3d} : E_u \rightarrow A_u + B_u \text{ of } C_{2h}.$$

The correspondences of irreps at HSPs from original SG to lowered SG:

$$\begin{aligned}
n_{GM6}^{12} &= n_{GM7}^{164} + n_{GM9}^{164} n_{GM4}^{12} = n_{GM5}^{164} + n_{GM8}^{164} n_{GM5}^{12} = n_{GM6}^{164} + n_{GM9}^{164} n_{GM3}^{12} = n_{GM4}^{164} + n_{GM8}^{164} n_{Y6}^{12} = n_{M6}^{164} n_{Y4}^{12} = n_{M3}^{164} \\
n_{Y5}^{12} &= n_{M5}^{164} n_{Y3}^{12} = n_{M3}^{164} n_{V2}^{12} = n_{M3}^{164} + n_{M4}^{164} n_{V3}^{12} = n_{M5}^{164} + n_{M6}^{164} n_{A6}^{12} = n_{A7}^{164} + n_{A9}^{164} n_{A4}^{12} = n_{A5}^{164} + n_{A8}^{164} n_{A5}^{12} = n_{A6}^{164} + n_{A9}^{164} \\
n_{A3}^{12} &= n_{A4}^{164} + n_{A8}^{164} n_{M6}^{12} = n_{L6}^{164} n_{M4}^{12} = n_{L4}^{164} n_{M5}^{12} = n_{L5}^{164} n_{M3}^{12} = n_{L3}^{164} n_{L2}^{12} = n_{L3}^{164} + n_{L4}^{164} n_{L3}^{12} = n_{L5}^{164} + n_{L6}^{164}
\end{aligned}$$

The lower SG is SG 147 when the preserved operations are: **(sub-SG label is 4) 1, 2, 3, 7, 8, 9.**

$$\text{The transformation is: } (\mathbf{a}_{147}, \mathbf{b}_{147}, \mathbf{c}_{147}) = (\mathbf{a}_{164}, \mathbf{b}_{164}, \mathbf{c}_{164}) \begin{pmatrix} -1 & 1 & 0 \\ -1 & 0 & 0 \\ 0 & 0 & 1 \end{pmatrix}, \overrightarrow{O_{164}O_{147}} = \frac{1}{2}\mathbf{c}_{147}$$

The reduction of higher dimensional irrep:

$$D_{3d} : E_g \rightarrow {}^2E_g + {}^1E_g \text{ of } C_{3i}.$$

$D_{3d} : E_u \rightarrow {}^1E_u + {}^2E_u$  of  $C_{3i}$ .

The correspondences of irreps at HSPs from original SG to lowered SG:

$$\begin{aligned} n_{GM7}^{147} &= n_{GM6}^{164} + n_{GM7}^{164} & n_{GM4}^{147} &= n_{GM4}^{164} + n_{GM5}^{164} & n_{GM9}^{147} &= n_{GM9}^{164} & n_{GM6}^{147} &= n_{GM8}^{164} & n_{GM8}^{147} &= n_{GM9}^{164} & n_{GM5}^{147} &= n_{GM8}^{164} & n_{M2}^{147} &= n_{M5}^{164} + n_{M6}^{164} \\ n_{M5}^{164} + n_{M6}^{164} & n_{M3}^{147} &= n_{M3}^{164} + n_{M4}^{164} & n_{K4}^{147} &= n_{K4}^{164} + n_{K5}^{164} & n_{K6}^{147} &= n_{K6}^{164} & n_{K5}^{147} &= n_{K6}^{164} & n_{A7}^{147} &= n_{A4}^{164} + n_{A5}^{164} & n_{A4}^{147} &= n_{A6}^{164} + n_{A7}^{164} & n_{A9}^{147} &= n_{A8}^{164} + n_{A9}^{164} \\ n_{A8}^{164} & n_{A6}^{147} &= n_{A9}^{164} & n_{A8}^{147} &= n_{A8}^{164} & n_{A5}^{147} &= n_{A9}^{164} & n_{L2}^{147} &= n_{L3}^{164} + n_{L4}^{164} & n_{L3}^{147} &= n_{L5}^{164} + n_{L6}^{164} & n_{H4}^{147} &= n_{H4}^{164} + n_{H5}^{164} & n_{H6}^{147} &= n_{H6}^{164} & n_{H5}^{147} &= n_{H6}^{164} \end{aligned}$$

## 71. Lowered SGs by higher-dimensional irreps of pairings in SG 165

The representative operations of SG/T for SG 165:

$$\begin{aligned} 1 : (x, y, z), 2 : (-y, x - y, z), 3 : (y - x, -x, z), 4 : (x - y, -y, \frac{1}{2} - z), 5 : (y, x, \frac{1}{2} - z), 6 : (-x, y - x, \frac{1}{2} - z), \\ 7 : (-x, -y, -z), 8 : (y, y - x, -z), 9 : (x - y, x, -z), 10 : (y - x, y, z + \frac{1}{2}), 11 : (-y, -x, z + \frac{1}{2}), 12 : (x, x - y, z + \frac{1}{2}). \end{aligned}$$

The lower SG is SG 15 when the preserved operations are: **(sub-SG label is 1) 1, 4, 7, 10.**

The transformation is:  $(\mathbf{a}_{15}, \mathbf{b}_{15}, \mathbf{c}_{15}) = (\mathbf{a}_{165}, \mathbf{b}_{165}, \mathbf{c}_{165}) \begin{pmatrix} -1 & -1 & 0 \\ -2 & 0 & 0 \\ 0 & 0 & -1 \end{pmatrix}, \overrightarrow{O_{165}O_{15}} = \frac{1}{2}\mathbf{a}_{15}$

The reduction of higher dimensional irrep:

$D_{3d} : E_g \rightarrow A_g + B_g$  of  $C_{2h}$ .

$D_{3d} : E_u \rightarrow A_u + B_u$  of  $C_{2h}$ .

The correspondences of irreps at HSPs from original SG to lowered SG:

$$\begin{aligned} n_{GM6}^{15} &= n_{GM7}^{165} + n_{GM9}^{165} & n_{GM4}^{15} &= n_{GM5}^{165} + n_{GM8}^{165} & n_{GM5}^{15} &= n_{GM6}^{165} + n_{GM9}^{165} & n_{GM3}^{15} &= n_{GM4}^{165} + n_{GM8}^{165} & n_{Y6}^{15} &= n_{M6}^{165} & n_{Y4}^{15} &= n_{M3}^{165} \\ n_{Y5}^{15} &= n_{M5}^{165} & n_{Y3}^{15} &= n_{M3}^{165} & n_{V3}^{15} &= n_{M3}^{165} + n_{M4}^{165} & n_{V2}^{15} &= n_{M5}^{165} + n_{M6}^{165} & n_{A2}^{15} &= n_{A4}^{165} + n_{A5}^{165} + n_{A6}^{165} & n_{M2}^{15} &= n_{L2}^{165} & n_{L3}^{15} &= n_{L2}^{165} & n_{L2}^{15} &= n_{L2}^{165} \end{aligned}$$

The lower SG is SG 15 when the preserved operations are: **(sub-SG label is 2) 1, 6, 7, 12.**

The transformation is:  $(\mathbf{a}_{15}, \mathbf{b}_{15}, \mathbf{c}_{15}) = (\mathbf{a}_{165}, \mathbf{b}_{165}, \mathbf{c}_{165}) \begin{pmatrix} -2 & 0 & 0 \\ -1 & 1 & 0 \\ 0 & 0 & -1 \end{pmatrix}, \overrightarrow{O_{165}O_{15}} = \frac{1}{2}\mathbf{a}_{15}$

The reduction of higher dimensional irrep:

$D_{3d} : E_g \rightarrow A_g + B_g$  of  $C_{2h}$ .

$D_{3d} : E_u \rightarrow A_u + B_u$  of  $C_{2h}$ .

The correspondences of irreps at HSPs from original SG to lowered SG:

$$\begin{aligned} n_{GM6}^{15} &= n_{GM7}^{165} + n_{GM9}^{165} & n_{GM4}^{15} &= n_{GM5}^{165} + n_{GM8}^{165} & n_{GM5}^{15} &= n_{GM6}^{165} + n_{GM9}^{165} & n_{GM3}^{15} &= n_{GM4}^{165} + n_{GM8}^{165} & n_{Y6}^{15} &= n_{M6}^{165} & n_{Y4}^{15} &= n_{M3}^{165} \\ n_{Y5}^{15} &= n_{M5}^{165} & n_{Y3}^{15} &= n_{M3}^{165} & n_{V3}^{15} &= n_{M3}^{165} + n_{M4}^{165} & n_{V2}^{15} &= n_{M5}^{165} + n_{M6}^{165} & n_{A2}^{15} &= n_{A4}^{165} + n_{A5}^{165} + n_{A6}^{165} & n_{M2}^{15} &= n_{L2}^{165} & n_{L3}^{15} &= n_{L2}^{165} & n_{L2}^{15} &= n_{L2}^{165} \end{aligned}$$

The lower SG is SG 15 when the preserved operations are: **(sub-SG label is 3) 1, 5, 7, 11.**

The transformation is:  $(\mathbf{a}_{15}, \mathbf{b}_{15}, \mathbf{c}_{15}) = (\mathbf{a}_{165}, \mathbf{b}_{165}, \mathbf{c}_{165}) \begin{pmatrix} -1 & 1 & 0 \\ 1 & 1 & 0 \\ 0 & 0 & -1 \end{pmatrix}, \overrightarrow{O_{165}O_{15}} = \frac{1}{2}\mathbf{a}_{15}$

The reduction of higher dimensional irrep:

$D_{3d} : E_g \rightarrow A_g + B_g$  of  $C_{2h}$ .

$D_{3d} : E_u \rightarrow A_u + B_u$  of  $C_{2h}$ .

The correspondences of irreps at HSPs from original SG to lowered SG:

$$\begin{aligned} n_{GM6}^{15} &= n_{GM7}^{165} + n_{GM9}^{165} & n_{GM4}^{15} &= n_{GM5}^{165} + n_{GM8}^{165} & n_{GM5}^{15} &= n_{GM6}^{165} + n_{GM9}^{165} & n_{GM3}^{15} &= n_{GM4}^{165} + n_{GM8}^{165} & n_{Y6}^{15} &= n_{M6}^{165} & n_{Y4}^{15} &= n_{M3}^{165} \\ n_{Y5}^{15} &= n_{M5}^{165} & n_{Y3}^{15} &= n_{M3}^{165} & n_{V3}^{15} &= n_{M3}^{165} + n_{M4}^{165} & n_{V2}^{15} &= n_{M5}^{165} + n_{M6}^{165} & n_{A2}^{15} &= n_{A4}^{165} + n_{A5}^{165} + n_{A6}^{165} & n_{M2}^{15} &= n_{L2}^{165} & n_{L3}^{15} &= n_{L2}^{165} & n_{L2}^{15} &= n_{L2}^{165} \end{aligned}$$

The lower SG is SG 147 when the preserved operations are: **(sub-SG label is 4) 1, 2, 3, 7, 8, 9.**

The transformation is:  $(\mathbf{a}_{147}, \mathbf{b}_{147}, \mathbf{c}_{147}) = (\mathbf{a}_{165}, \mathbf{b}_{165}, \mathbf{c}_{165}) \begin{pmatrix} -1 & 1 & 0 \\ -1 & 0 & 0 \\ 0 & 0 & 1 \end{pmatrix}, \overrightarrow{O_{165}O_{147}} = \frac{1}{2}\mathbf{c}_{147}$

The reduction of higher dimensional irrep:

$$D_{3d} : E_g \rightarrow {}^2E_g + {}^1E_g \text{ of } C_{3i}.$$

$$D_{3d} : E_u \rightarrow {}^1E_u + {}^2E_u \text{ of } C_{3i}.$$

The correspondences of irreps at HSPs from original SG to lowered SG:

$$\begin{aligned} n_{GM7}^{147} &= n_{GM6}^{165} + n_{GM7}^{165} & n_{GM4}^{147} &= n_{GM4}^{165} + n_{GM5}^{165} & n_{GM9}^{147} &= n_{GM9}^{165} & n_{GM6}^{147} &= n_{GM8}^{165} & n_{GM8}^{147} &= n_{GM9}^{165} & n_{GM5}^{147} &= n_{GM8}^{165} & n_{M2}^{147} &= n_{GM8}^{165} & n_{M2}^{147} &= n_{GM8}^{165} \\ n_{M5}^{165} + n_{M6}^{165} & n_{M3}^{147} &= n_{M3}^{165} + n_{M4}^{165} & n_{K4}^{147} &= n_{K4}^{165} + n_{K5}^{165} & n_{K6}^{147} &= n_{K6}^{165} & n_{K5}^{147} &= n_{K6}^{165} & n_{A7}^{147} &= n_{A4}^{165} & n_{A4}^{147} &= n_{A4}^{165} & n_{A9}^{147} &= n_{A6}^{165} & n_{A6}^{147} &= n_{A6}^{165} \\ n_{A5}^{165} & n_{A8}^{147} &= n_{A5}^{165} & n_{A5}^{147} &= n_{A6}^{165} & n_{L2}^{147} &= n_{L2}^{165} & n_{L3}^{147} &= n_{L2}^{165} & n_{H4}^{147} &= n_{H4}^{165} & n_{H5}^{147} &= n_{H5}^{165} & n_{H6}^{147} &= n_{H6}^{165} \end{aligned}$$

## 72. Lowered SGs by higher-dimensional irreps of pairings in SG 166

The representative operations of SG/T for SG 166:

$$\begin{aligned} 1 : (x, y, z), 2 : (z, x, y), 3 : (y, z, x), 4 : (-y, -x, -z), 5 : (-z, -y, -x), 6 : (-x, -z, -y), 7 : (-x, -y, -z), \\ 8 : (-z, -x, -y), 9 : (-y, -z, -x), 10 : (y, x, z), 11 : (z, y, x), 12 : (x, z, y). \end{aligned}$$

The lower SG is SG 12 when the preserved operations are: **(sub-SG label is 1) 1, 6, 7, 12.**

The transformation is:  $(\mathbf{a}_{12}, \mathbf{b}_{12}, \mathbf{c}_{12}) = (\mathbf{a}_{166}, \mathbf{b}_{166}, \mathbf{c}_{166}) \begin{pmatrix} -2 & 0 & 1 \\ 1 & 1 & -1 \\ 1 & -1 & -1 \end{pmatrix}, \overrightarrow{O_{166}O_{12}} = \frac{1}{2}\mathbf{a}_{12}$

The reduction of higher dimensional irrep:

$$D_{3d} : E_g \rightarrow A_g + B_g \text{ of } C_{2h}.$$

$$D_{3d} : E_u \rightarrow A_u + B_u \text{ of } C_{2h}.$$

The correspondences of irreps at HSPs from original SG to lowered SG:

$$\begin{aligned} n_{GM6}^{12} &= n_{GM6}^{166} + n_{GM9}^{166} & n_{GM4}^{12} &= n_{GM4}^{166} + n_{GM8}^{166} & n_{GM5}^{12} &= n_{GM7}^{166} + n_{GM9}^{166} & n_{GM3}^{12} &= n_{GM6}^{166} + n_{GM8}^{166} & n_{Y6}^{12} &= n_{F6}^{166} & n_{Y4}^{12} &= n_{F4}^{166} & n_{F4}^{12} &= n_{F4}^{166} \\ n_{Y5}^{12} &= n_{F5}^{166} & n_{Y3}^{12} &= n_{F3}^{166} & n_{V2}^{12} &= n_{F3}^{166} + n_{F4}^{166} & n_{V3}^{12} &= n_{F5}^{166} + n_{F6}^{166} & n_{A6}^{12} &= n_{T6}^{166} + n_{T9}^{166} & n_{A4}^{12} &= n_{T4}^{166} + n_{T8}^{166} & n_{A5}^{12} &= n_{T7}^{166} + n_{T9}^{166} \\ n_{A3}^{12} &= n_{T5}^{166} + n_{T8}^{166} & n_{M6}^{12} &= n_{L5}^{166} & n_{M4}^{12} &= n_{L3}^{166} & n_{M5}^{12} &= n_{L6}^{166} & n_{M3}^{12} &= n_{L4}^{166} & n_{L2}^{12} &= n_{L3}^{166} + n_{L4}^{166} & n_{L3}^{12} &= n_{L5}^{166} + n_{L6}^{166} \end{aligned}$$

The lower SG is SG 12 when the preserved operations are: **(sub-SG label is 2) 1, 5, 7, 11.**

The transformation is:  $(\mathbf{a}_{12}, \mathbf{b}_{12}, \mathbf{c}_{12}) = (\mathbf{a}_{166}, \mathbf{b}_{166}, \mathbf{c}_{166}) \begin{pmatrix} -1 & 1 & 0 \\ 0 & 0 & -1 \\ -1 & -1 & 0 \end{pmatrix}, \overrightarrow{O_{166}O_{12}} = \frac{1}{2}\mathbf{a}_{12}$

The reduction of higher dimensional irrep:

$$D_{3d} : E_g \rightarrow A_g + B_g \text{ of } C_{2h}.$$

$$D_{3d} : E_u \rightarrow A_u + B_u \text{ of } C_{2h}.$$

The correspondences of irreps at HSPs from original SG to lowered SG:

$$\begin{aligned} n_{GM6}^{12} &= n_{GM7}^{166} + n_{GM9}^{166} & n_{GM4}^{12} &= n_{GM5}^{166} + n_{GM8}^{166} & n_{GM5}^{12} &= n_{GM6}^{166} + n_{GM9}^{166} & n_{GM3}^{12} &= n_{GM4}^{166} + n_{GM8}^{166} & n_{Y6}^{12} &= n_{F5}^{166} & n_{Y4}^{12} &= n_{F3}^{166} & n_{F3}^{12} &= n_{F3}^{166} \\ n_{Y5}^{12} &= n_{F6}^{166} & n_{Y3}^{12} &= n_{F4}^{166} & n_{V2}^{12} &= n_{L3}^{166} + n_{L4}^{166} & n_{V3}^{12} &= n_{L5}^{166} + n_{L6}^{166} & n_{A6}^{12} &= n_{L6}^{166} & n_{A4}^{12} &= n_{L4}^{166} & n_{A5}^{12} &= n_{L5}^{166} & n_{A3}^{12} &= n_{L3}^{166} & n_{M6}^{12} &= n_{L3}^{166} & n_{M6}^{12} &= n_{L3}^{166} \\ n_{T7}^{166} + n_{T9}^{166} & n_{M4}^{12} &= n_{T5}^{166} + n_{T8}^{166} & n_{M5}^{12} &= n_{T6}^{166} + n_{T9}^{166} & n_{M3}^{12} &= n_{T4}^{166} + n_{T8}^{166} & n_{L2}^{12} &= n_{F3}^{166} + n_{F4}^{166} & n_{L3}^{12} &= n_{F5}^{166} + n_{F6}^{166} \end{aligned}$$

The lower SG is SG 12 when the preserved operations are: **(sub-SG label is 3) 1, 4, 7, 10.**

The transformation is:  $(\mathbf{a}_{12}, \mathbf{b}_{12}, \mathbf{c}_{12}) = (\mathbf{a}_{166}, \mathbf{b}_{166}, \mathbf{c}_{166}) \begin{pmatrix} -1 & -1 & 0 \\ -1 & 1 & 0 \\ 0 & 0 & -1 \end{pmatrix}, \overrightarrow{O_{166}O_{12}} = \frac{1}{2}\mathbf{a}_{12}$

The reduction of higher dimensional irrep:

$$D_{3d} : E_g \rightarrow A_g + B_g \text{ of } C_{2h}.$$

$$D_{3d} : E_u \rightarrow A_u + B_u \text{ of } C_{2h}.$$

The correspondences of irreps at HSPs from original SG to lowered SG:

$$\begin{aligned} n_{GM6}^{12} &= n_{GM7}^{166} + n_{GM9}^{166} & n_{GM4}^{12} &= n_{GM5}^{166} + n_{GM8}^{166} & n_{GM5}^{12} &= n_{GM6}^{166} + n_{GM9}^{166} & n_{GM3}^{12} &= n_{GM4}^{166} + n_{GM8}^{166} & n_{Y6}^{12} &= n_{F5}^{166} & n_{Y4}^{12} &= n_{F3}^{166} & n_{F3}^{12} &= n_{F3}^{166} \\ n_{Y5}^{12} &= n_{F6}^{166} & n_{Y3}^{12} &= n_{F4}^{166} & n_{V2}^{12} &= n_{L3}^{166} + n_{L4}^{166} & n_{V3}^{12} &= n_{L5}^{166} + n_{L6}^{166} & n_{A6}^{12} &= n_{L6}^{166} & n_{A4}^{12} &= n_{L4}^{166} & n_{A5}^{12} &= n_{L5}^{166} & n_{A3}^{12} &= n_{L3}^{166} & n_{M6}^{12} &= n_{L3}^{166} & n_{M6}^{12} &= n_{L3}^{166} \\ n_{T7}^{166} + n_{T9}^{166} & n_{M4}^{12} &= n_{T5}^{166} + n_{T8}^{166} & n_{M5}^{12} &= n_{T6}^{166} + n_{T9}^{166} & n_{M3}^{12} &= n_{T4}^{166} + n_{T8}^{166} & n_{L2}^{12} &= n_{F3}^{166} + n_{F4}^{166} & n_{L3}^{12} &= n_{F5}^{166} + n_{F6}^{166} \end{aligned}$$

The lower SG is SG 148 when the preserved operations are: **(sub-SG label is 4) 1, 2, 3, 7, 8, 9.**

The transformation is:  $(\mathbf{a}_{148}, \mathbf{b}_{148}, \mathbf{c}_{148}) = (\mathbf{a}_{166}, \mathbf{b}_{166}, \mathbf{c}_{166}) \begin{pmatrix} 0 & 1 & 0 \\ 0 & 0 & 1 \\ 1 & 0 & 0 \end{pmatrix}, \overrightarrow{O_{166}O_{148}} = \mathbf{0}$

The reduction of higher dimensional irrep:

$$D_{3d} : E_g \rightarrow {}^2E_g + {}^1E_g \text{ of } C_{3i}.$$

$$D_{3d} : E_u \rightarrow {}^1E_u + {}^2E_u \text{ of } C_{3i}.$$

The correspondences of irreps at HSPs from original SG to lowered SG:

$$\begin{aligned} n_{GM7}^{148} &= n_{GM6}^{166} + n_{GM7}^{166} n_{GM4}^{148} = n_{GM4}^{166} + n_{GM5}^{166} n_{GM9}^{148} = n_{GM9}^{166} n_{GM6}^{148} = n_{GM8}^{166} n_{GM8}^{148} = n_{GM9}^{166} n_{GM5}^{148} = n_{GM8}^{166} n_{L2}^{148} = \\ n_{L5}^{166} + n_{L6}^{166} n_{L3}^{148} &= n_{L3}^{166} + n_{L4}^{166} n_{F2}^{148} = n_{F5}^{166} + n_{F6}^{166} n_{F3}^{148} = n_{F3}^{166} + n_{F4}^{166} n_{T7}^{148} = n_{T6}^{166} + n_{T7}^{166} n_{T4}^{148} = n_{T4}^{166} + n_{T5}^{166} n_{T9}^{148} = n_{T9}^{166} \\ n_{T6}^{148} &= n_{T8}^{166} n_{T8}^{148} = n_{T9}^{166} n_{T5}^{148} = n_{T8}^{166} \end{aligned}$$

### 73. Lowered SGs by higher-dimensional irreps of pairings in SG 167

The representative operations of SG/T for SG 167:

$$\begin{aligned} 1 : (x, y, z), 2 : (z, x, y), 3 : (y, z, x), 4 : (\frac{1}{2} - y, \frac{1}{2} - x, \frac{1}{2} - z), 5 : (\frac{1}{2} - z, \frac{1}{2} - y, \frac{1}{2} - x), 6 : (\frac{1}{2} - x, \frac{1}{2} - z, \frac{1}{2} - y), \\ 7 : (-x, -y, -z), 8 : (-z, -x, -y), 9 : (-y, -z, -x), 10 : (y + \frac{1}{2}, x + \frac{1}{2}, z + \frac{1}{2}), 11 : (z + \frac{1}{2}, y + \frac{1}{2}, x + \frac{1}{2}), \\ 12 : (x + \frac{1}{2}, z + \frac{1}{2}, y + \frac{1}{2}). \end{aligned}$$

The lower SG is SG 15 when the preserved operations are: **(sub-SG label is 1) 1, 6, 7, 12.**

The transformation is:  $(\mathbf{a}_{15}, \mathbf{b}_{15}, \mathbf{c}_{15}) = (\mathbf{a}_{167}, \mathbf{b}_{167}, \mathbf{c}_{167}) \begin{pmatrix} -2 & 0 & 1 \\ 1 & 1 & -1 \\ 1 & -1 & -1 \end{pmatrix}, \overrightarrow{O_{167}O_{15}} = \frac{1}{2}\mathbf{a}_{15}$

The reduction of higher dimensional irrep:

$$D_{3d} : E_g \rightarrow A_g + B_g \text{ of } C_{2h}.$$

$$D_{3d} : E_u \rightarrow A_u + B_u \text{ of } C_{2h}.$$

The correspondences of irreps at HSPs from original SG to lowered SG:

$$\begin{aligned} n_{GM6}^{15} &= n_{GM6}^{167} + n_{GM9}^{167} n_{GM4}^{15} = n_{GM4}^{167} + n_{GM8}^{167} n_{GM5}^{15} = n_{GM7}^{167} + n_{GM9}^{167} n_{GM3}^{15} = n_{GM5}^{167} + n_{GM8}^{167} n_{Y6}^{15} = n_{F6}^{167} n_{Y4}^{15} = n_{F4}^{167} \\ n_{Y5}^{15} &= n_{F5}^{167} n_{Y3}^{15} = n_{F3}^{167} n_{V3}^{15} = n_{F3}^{167} + n_{F4}^{167} n_{V2}^{15} = n_{F5}^{167} + n_{F6}^{167} n_{A2}^{15} = n_{T4}^{167} + n_{T5}^{167} + n_{T6}^{167} n_{M2}^{15} = n_{L2}^{167} n_{L3}^{15} = n_{L2}^{167} n_{L2}^{15} = \\ n_{L2}^{167} \end{aligned}$$

The lower SG is SG 15 when the preserved operations are: **(sub-SG label is 2) 1, 5, 7, 11.**

The transformation is:  $(\mathbf{a}_{15}, \mathbf{b}_{15}, \mathbf{c}_{15}) = (\mathbf{a}_{167}, \mathbf{b}_{167}, \mathbf{c}_{167}) \begin{pmatrix} -1 & 1 & 0 \\ 0 & 0 & -1 \\ -1 & -1 & 0 \end{pmatrix}, \overrightarrow{O_{167}O_{15}} = \frac{1}{4}\mathbf{a}_{15} + (-\frac{1}{4})\mathbf{b}_{15}$

The reduction of higher dimensional irrep:

$$D_{3d} : E_g \rightarrow A_g + B_g \text{ of } C_{2h}.$$

$$D_{3d} : E_u \rightarrow A_u + B_u \text{ of } C_{2h}.$$

The correspondences of irreps at HSPs from original SG to lowered SG:

$$\begin{aligned} n_{GM6}^{15} &= n_{GM7}^{167} + n_{GM9}^{167} n_{GM4}^{15} = n_{GM5}^{167} + n_{GM8}^{167} n_{GM5}^{15} = n_{GM6}^{167} + n_{GM9}^{167} n_{GM3}^{15} = n_{GM4}^{167} + n_{GM8}^{167} n_{Y6}^{15} = n_{F3}^{167} n_{Y4}^{15} = \\ n_{F5}^{167} n_{Y5}^{15} &= n_{F4}^{167} n_{Y3}^{15} = n_{F6}^{167} n_{V3}^{15} = n_{L2}^{167} n_{V2}^{15} = n_{L2}^{167} n_{A2}^{15} = n_{L2}^{167} n_{M2}^{15} = n_{T4}^{167} + n_{T5}^{167} + n_{T6}^{167} n_{L3}^{15} = n_{F5}^{167} + n_{F6}^{167} n_{L2}^{15} = \\ n_{F3}^{167} + n_{F4}^{167} \end{aligned}$$

The lower SG is SG 15 when the preserved operations are: **(sub-SG label is 3) 1, 4, 7, 10.**

The transformation is:  $(\mathbf{a}_{15}, \mathbf{b}_{15}, \mathbf{c}_{15}) = (\mathbf{a}_{167}, \mathbf{b}_{167}, \mathbf{c}_{167}) \begin{pmatrix} -1 & -1 & 0 \\ -1 & 1 & 0 \\ 0 & 0 & -1 \end{pmatrix}, \overrightarrow{O_{167}O_{15}} = \frac{1}{4}\mathbf{a}_{15} + (-\frac{1}{4})\mathbf{b}_{15}$

The reduction of higher dimensional irrep:

$$D_{3d} : E_g \rightarrow A_g + B_g \text{ of } C_{2h}.$$

$$D_{3d} : E_u \rightarrow A_u + B_u \text{ of } C_{2h}.$$

The correspondences of irreps at HSPs from original SG to lowered SG:

$$\begin{aligned} n_{GM6}^{15} &= n_{GM7}^{167} + n_{GM9}^{167} & n_{GM4}^{15} &= n_{GM5}^{167} + n_{GM8}^{167} & n_{GM5}^{15} &= n_{GM6}^{167} + n_{GM9}^{167} & n_{GM3}^{15} &= n_{GM4}^{167} + n_{GM8}^{167} & n_{Y6}^{15} &= n_{F3}^{167} & n_{Y4}^{15} &= \\ n_{F5}^{167} & n_{Y5}^{15} &= n_{F4}^{167} & n_{Y3}^{15} &= n_{F6}^{167} & n_{V3}^{15} &= n_{L2}^{167} & n_{V2}^{15} &= n_{L2}^{167} & n_{A2}^{15} &= n_{L2}^{167} & n_{M2}^{15} &= n_{T4}^{167} + n_{T5}^{167} + n_{T6}^{167} & n_{L3}^{15} &= n_{F5}^{167} + n_{F6}^{167} & n_{L2}^{15} &= \\ n_{F3}^{167} & + n_{F4}^{167} & & & & & & & & & & & & & & & & \end{aligned}$$

The lower SG is SG 148 when the preserved operations are: **(sub-SG label is 4) 1, 2, 3, 7, 8, 9.**

The transformation is:  $(\mathbf{a}_{148}, \mathbf{b}_{148}, \mathbf{c}_{148}) = (\mathbf{a}_{167}, \mathbf{b}_{167}, \mathbf{c}_{167}) \begin{pmatrix} 0 & 1 & 0 \\ 0 & 0 & 1 \\ 1 & 0 & 0 \end{pmatrix}, \overrightarrow{O_{167}O_{148}} = \mathbf{0}$

The reduction of higher dimensional irrep:

$$D_{3d} : E_g \rightarrow {}^2E_g + {}^1E_g \text{ of } C_{3i}.$$

$$D_{3d} : E_u \rightarrow {}^1E_u + {}^2E_u \text{ of } C_{3i}.$$

The correspondences of irreps at HSPs from original SG to lowered SG:

$$\begin{aligned} n_{GM7}^{148} &= n_{GM6}^{167} + n_{GM7}^{167} & n_{GM4}^{148} &= n_{GM4}^{167} + n_{GM5}^{167} & n_{GM9}^{148} &= n_{GM9}^{167} & n_{GM6}^{148} &= n_{GM8}^{167} & n_{GM8}^{148} &= n_{GM9}^{167} & n_{GM5}^{148} &= n_{GM8}^{167} & n_{L2}^{148} &= \\ n_{L2}^{167} & n_{L3}^{148} &= n_{L2}^{167} & n_{F2}^{148} &= n_{F5}^{167} + n_{F6}^{167} & n_{F3}^{148} &= n_{F3}^{167} + n_{F4}^{167} & n_{T7}^{148} &= n_{T4}^{167} & n_{T4}^{148} &= n_{T4}^{167} & n_{T9}^{148} &= n_{T5}^{167} & n_{T6}^{148} &= n_{T6}^{167} & n_{T8}^{148} &= n_{T6}^{167} \\ n_{T5}^{148} &= n_{T5}^{167} & & & & & & & & & & & & & & & & \end{aligned}$$

#### 74. Lowered SGs by higher-dimensional irreps of pairings in SG 177

The representative operations of SG/T for SG 177:

$$\begin{aligned} 1 : (x, y, z), 2 : (x - y, x, z), 3 : (-y, x - y, z), 4 : (-x, -y, z), 5 : (y - x, -x, z), 6 : (y, y - x, z), 7 : (x - y, -y, -z), \\ 8 : (y, x, -z), 9 : (-x, y - x, -z), 10 : (x, x - y, -z), 11 : (y - x, y, -z), 12 : (-y, -x, -z). \end{aligned}$$

The lower SG is SG 21 when the preserved operations are: **(sub-SG label is 1) 1, 4, 11, 7.**

The transformation is:  $(\mathbf{a}_{21}, \mathbf{b}_{21}, \mathbf{c}_{21}) = (\mathbf{a}_{177}, \mathbf{b}_{177}, \mathbf{c}_{177}) \begin{pmatrix} 1 & -1 & 0 \\ 2 & 0 & 0 \\ 0 & 0 & 1 \end{pmatrix}, \overrightarrow{O_{177}O_{21}} = \frac{1}{2}\mathbf{c}_{21}$

The reduction of higher dimensional irrep:

$$D_6 : E_2 \rightarrow A_1 + B_1 \text{ of } D_2.$$

$$D_6 : E_1 \rightarrow B_2 + B_3 \text{ of } D_2.$$

The correspondences of irreps at HSPs from original SG to lowered SG:

$$\begin{aligned} n_{GM5}^{21} &= n_{GM7}^{177} + n_{GM8}^{177} + n_{GM9}^{177} & n_{Y5}^{21} &= n_{M5}^{177} & n_{S4}^{21} &= n_{M5}^{177} & n_{S3}^{21} &= n_{M5}^{177} & n_{Z5}^{21} &= n_{A7}^{177} + n_{A8}^{177} + n_{A9}^{177} & n_{T5}^{21} &= n_{L5}^{177} & n_{R4}^{21} &= n_{L5}^{177} \\ n_{R3}^{21} &= n_{L5}^{177} & & & & & & & & & & & & & & & \end{aligned}$$

The lower SG is SG 21 when the preserved operations are: **(sub-SG label is 2) 1, 4, 9, 10.**

The transformation is:  $(\mathbf{a}_{21}, \mathbf{b}_{21}, \mathbf{c}_{21}) = (\mathbf{a}_{177}, \mathbf{b}_{177}, \mathbf{c}_{177}) \begin{pmatrix} 0 & -2 & 0 \\ 1 & -1 & 0 \\ 0 & 0 & 1 \end{pmatrix}, \overrightarrow{O_{177}O_{21}} = \frac{1}{2}\mathbf{c}_{21}$

The reduction of higher dimensional irrep:

$$D_6 : E_2 \rightarrow A_1 + B_1 \text{ of } D_2.$$

$$D_6 : E_1 \rightarrow B_2 + B_3 \text{ of } D_2.$$

The correspondences of irreps at HSPs from original SG to lowered SG:

$$\begin{aligned} n_{GM5}^{21} &= n_{GM7}^{177} + n_{GM8}^{177} + n_{GM9}^{177} & n_{Y5}^{21} &= n_{M5}^{177} & n_{S4}^{21} &= n_{M5}^{177} & n_{S3}^{21} &= n_{M5}^{177} & n_{Z5}^{21} &= n_{A7}^{177} + n_{A8}^{177} + n_{A9}^{177} & n_{T5}^{21} &= n_{L5}^{177} & n_{R4}^{21} &= n_{L5}^{177} \\ n_{R3}^{21} &= n_{L5}^{177} & & & & & & & & & & & & & & & \end{aligned}$$

The lower SG is SG 21 when the preserved operations are: **(sub-SG label is 3) 1, 4, 12, 8.**

The transformation is:  $(\mathbf{a}_{21}, \mathbf{b}_{21}, \mathbf{c}_{21}) = (\mathbf{a}_{177}, \mathbf{b}_{177}, \mathbf{c}_{177}) \begin{pmatrix} -1 & -1 & 0 \\ 1 & -1 & 0 \\ 0 & 0 & 1 \end{pmatrix}, \overrightarrow{O_{177}O_{21}} = \frac{1}{2}\mathbf{c}_{21}$

The reduction of higher dimensional irrep:

$$D_6 : E_2 \rightarrow A_1 + B_1 \text{ of } D_2.$$

$$D_6 : E_1 \rightarrow B_2 + B_3 \text{ of } D_2.$$

The correspondences of irreps at HSPs from original SG to lowered SG:

$$\begin{aligned} n_{GM5}^{21} &= n_{GM7}^{177} + n_{GM8}^{177} + n_{GM9}^{177} & n_{Y5}^{21} &= n_{M5}^{177} & n_{S4}^{21} &= n_{M5}^{177} & n_{S3}^{21} &= n_{M5}^{177} & n_{Z5}^{21} &= n_{A7}^{177} + n_{A8}^{177} + n_{A9}^{177} & n_{T5}^{21} &= n_{L5}^{177} & n_{R4}^{21} &= n_{L5}^{177} \\ n_{R3}^{21} &= n_{L5}^{177} \end{aligned}$$

The lower SG is SG 168 when the preserved operations are: **(sub-SG label is 4) 1, 2, 6, 3, 5, 4.**

$$\text{The transformation is: } (\mathbf{a}_{168}, \mathbf{b}_{168}, \mathbf{c}_{168}) = (\mathbf{a}_{177}, \mathbf{b}_{177}, \mathbf{c}_{177}) \begin{pmatrix} -1 & 1 & 0 \\ -1 & 0 & 0 \\ 0 & 0 & 1 \end{pmatrix}, \overrightarrow{O_{177}O_{168}} = -\mathbf{a}_{168}$$

The reduction of higher dimensional irrep:

$$D_6 : E_2 \rightarrow {}^1E_2 + {}^2E_2 \text{ of } C_6.$$

$$D_6 : E_1 \rightarrow {}^2E_1 + {}^1E_1 \text{ of } C_6.$$

The correspondences of irreps at HSPs from original SG to lowered SG:

$$\begin{aligned} n_{GM9}^{168} &= n_{GM8}^{177} & n_{GM12}^{168} &= n_{GM8}^{177} & n_{GM8}^{168} &= n_{GM7}^{177} & n_{GM7}^{168} &= n_{GM7}^{177} & n_{GM11}^{168} &= n_{GM9}^{177} & n_{GM10}^{168} &= n_{GM9}^{177} & n_{M3}^{168} &= n_{M5}^{177} & n_{M4}^{168} &= n_{M5}^{177} \\ n_{K4}^{168} &= n_{K4}^{177} + n_{K5}^{177} & n_{K6}^{168} &= n_{K6}^{177} & n_{K5}^{168} &= n_{K6}^{177} & n_{A9}^{168} &= n_{A8}^{177} & n_{A12}^{168} &= n_{A8}^{177} & n_{A8}^{168} &= n_{A7}^{177} & n_{A7}^{168} &= n_{A7}^{177} & n_{A11}^{168} &= n_{A9}^{177} & n_{A10}^{168} &= n_{A9}^{177} \\ n_{L3}^{168} &= n_{L5}^{177} & n_{L4}^{168} &= n_{L5}^{177} & n_{H4}^{168} &= n_{H4}^{177} + n_{H5}^{177} & n_{H6}^{168} &= n_{H6}^{177} & n_{H5}^{168} &= n_{H6}^{177} \end{aligned}$$

### 75. Lowered SGs by higher-dimensional irreps of pairings in SG 178

The representative operations of SG/T for SG 178:

$$\begin{aligned} 1 : (x, y, z), & 2 : (x - y, x, z + \frac{1}{6}), & 3 : (-y, x - y, z + \frac{1}{3}), & 4 : (-x, -y, z + \frac{1}{2}), & 5 : (y - x, -x, z + \frac{2}{3}), & 6 : (y, y - x, z + \frac{5}{6}), \\ 7 : (x - y, -y, -z), & 8 : (y, x, \frac{1}{3} - z), & 9 : (-x, y - x, \frac{2}{3} - z), & 10 : (x, x - y, \frac{1}{6} - z), & 11 : (y - x, y, \frac{1}{2} - z), & 12 : (-y, -x, \frac{5}{6} - z). \end{aligned}$$

The lower SG is SG 20 when the preserved operations are: **(sub-SG label is 1) 1, 4, 11, 7.**

$$\text{The transformation is: } (\mathbf{a}_{20}, \mathbf{b}_{20}, \mathbf{c}_{20}) = (\mathbf{a}_{178}, \mathbf{b}_{178}, \mathbf{c}_{178}) \begin{pmatrix} 1 & 1 & 0 \\ 2 & 0 & 0 \\ 0 & 0 & -1 \end{pmatrix}, \overrightarrow{O_{178}O_{20}} = \frac{1}{4}\mathbf{c}_{20}$$

The reduction of higher dimensional irrep:

$$D_6 : E_2 \rightarrow A_1 + B_1 \text{ of } D_2.$$

$$D_6 : E_1 \rightarrow B_2 + B_3 \text{ of } D_2.$$

The correspondences of irreps at HSPs from original SG to lowered SG:

$$\begin{aligned} n_{GM5}^{20} &= n_{GM7}^{178} + n_{GM8}^{178} + n_{GM9}^{178} & n_{Y5}^{20} &= n_{M5}^{178} & n_{S4}^{20} &= n_{M5}^{178} & n_{S3}^{20} &= n_{M5}^{178} & n_{Z5}^{20} &= n_{A4}^{178} + n_{A8}^{178} & n_{Z4}^{20} &= n_{A6}^{178} + n_{A9}^{178} & n_{Z2}^{20} &= n_{A7}^{178} + n_{A9}^{178} & n_{Z3}^{20} &= n_{A5}^{178} + n_{A8}^{178} & n_{T5}^{20} &= n_{L2}^{178} & n_{T4}^{20} &= n_{L5}^{178} & n_{T2}^{20} &= n_{L3}^{178} & n_{T3}^{20} &= n_{L4}^{178} & n_{R4}^{20} &= n_{L2}^{178} + n_{L4}^{178} & n_{R3}^{20} &= n_{L3}^{178} + n_{L5}^{178} \end{aligned}$$

The lower SG is SG 20 when the preserved operations are: **(sub-SG label is 2) 1, 4, 9, 10.**

$$\text{The transformation is: } (\mathbf{a}_{20}, \mathbf{b}_{20}, \mathbf{c}_{20}) = (\mathbf{a}_{178}, \mathbf{b}_{178}, \mathbf{c}_{178}) \begin{pmatrix} 0 & 2 & 0 \\ 1 & 1 & 0 \\ 0 & 0 & -1 \end{pmatrix}, \overrightarrow{O_{178}O_{20}} = \frac{1}{6}\mathbf{c}_{20}$$

The reduction of higher dimensional irrep:

$$D_6 : E_2 \rightarrow A_1 + B_1 \text{ of } D_2.$$

$$D_6 : E_1 \rightarrow B_2 + B_3 \text{ of } D_2.$$

The correspondences of irreps at HSPs from original SG to lowered SG:

$$\begin{aligned} n_{GM5}^{20} &= n_{GM7}^{178} + n_{GM8}^{178} + n_{GM9}^{178} & n_{Y5}^{20} &= n_{M5}^{178} & n_{S4}^{20} &= n_{M5}^{178} & n_{S3}^{20} &= n_{M5}^{178} & n_{Z5}^{20} &= n_{A4}^{178} + n_{A8}^{178} & n_{Z4}^{20} &= n_{A6}^{178} + n_{A9}^{178} & n_{Z2}^{20} &= n_{A7}^{178} + n_{A9}^{178} & n_{Z3}^{20} &= n_{A5}^{178} + n_{A8}^{178} & n_{T5}^{20} &= n_{L2}^{178} & n_{T4}^{20} &= n_{L5}^{178} & n_{T2}^{20} &= n_{L3}^{178} & n_{T3}^{20} &= n_{L4}^{178} & n_{R4}^{20} &= n_{L2}^{178} + n_{L4}^{178} & n_{R3}^{20} &= n_{L3}^{178} + n_{L5}^{178} \end{aligned}$$

The lower SG is SG 20 when the preserved operations are: **(sub-SG label is 3) 1, 4, 12, 8.**

$$\text{The transformation is: } (\mathbf{a}_{20}, \mathbf{b}_{20}, \mathbf{c}_{20}) = (\mathbf{a}_{178}, \mathbf{b}_{178}, \mathbf{c}_{178}) \begin{pmatrix} -1 & 1 & 0 \\ 1 & 1 & 0 \\ 0 & 0 & -1 \end{pmatrix}, \overrightarrow{O_{178}O_{20}} = \frac{1}{12}\mathbf{c}_{20}$$

The reduction of higher dimensional irrep:

$$D_6 : E_2 \rightarrow A_1 + B_1 \text{ of } D_2.$$

$$D_6 : E_1 \rightarrow B_2 + B_3 \text{ of } D_2.$$

The correspondences of irreps at HSPs from original SG to lowered SG:

$$\begin{aligned} n_{GM5}^{20} &= n_{GM7}^{178} + n_{GM8}^{178} + n_{GM9}^{178} & n_{Y5}^{20} &= n_{M5}^{178} & n_{S4}^{20} &= n_{M5}^{178} & n_{S3}^{20} &= n_{M5}^{178} & n_{Z5}^{20} &= n_{A5}^{178} + n_{A8}^{178} & n_{Z4}^{20} &= n_{A6}^{178} + n_{A9}^{178} & n_{Z2}^{20} &= \\ n_{A7}^{178} + n_{A9}^{178} & n_{Z3}^{20} &= n_{A4}^{178} + n_{A8}^{178} & n_{T5}^{20} &= n_{L4}^{178} & n_{T4}^{20} &= n_{L5}^{178} & n_{T2}^{20} &= n_{L3}^{178} & n_{T3}^{20} &= n_{L2}^{178} & n_{R4}^{20} &= n_{L2}^{178} + n_{L4}^{178} & n_{R3}^{20} &= n_{L3}^{178} + n_{L5}^{178} \end{aligned}$$

The lower SG is SG 169 when the preserved operations are: **(sub-SG label is 4) 1, 2, 6, 3, 5, 4.**

The transformation is:  $(\mathbf{a}_{169}, \mathbf{b}_{169}, \mathbf{c}_{169}) = (\mathbf{a}_{178}, \mathbf{b}_{178}, \mathbf{c}_{178}) \begin{pmatrix} 1 & -1 & 0 \\ 0 & -1 & 0 \\ 0 & 0 & -1 \end{pmatrix}, \overrightarrow{O_{178}O_{169}} = \mathbf{a}_{169} + \mathbf{b}_{169} + (\frac{1}{4})\mathbf{c}_{169}$

The reduction of higher dimensional irrep:

$$D_6 : E_2 \rightarrow {}^1E_2 + {}^2E_2 \text{ of } C_6.$$

$$D_6 : E_1 \rightarrow {}^2E_1 + {}^1E_1 \text{ of } C_6.$$

The correspondences of irreps at HSPs from original SG to lowered SG:

$$\begin{aligned} n_{GM9}^{169} &= n_{GM8}^{178} & n_{GM12}^{169} &= n_{GM8}^{178} & n_{GM8}^{169} &= n_{GM7}^{178} & n_{GM7}^{169} &= n_{GM7}^{178} & n_{GM11}^{169} &= n_{GM9}^{178} & n_{GM10}^{169} &= n_{GM9}^{178} & n_{M3}^{169} &= n_{M5}^{178} & n_{M4}^{169} &= n_{M5}^{178} \\ n_{K4}^{169} &= n_{K4}^{178} + n_{K5}^{178} & n_{K6}^{169} &= n_{K6}^{178} & n_{K5}^{169} &= n_{K6}^{178} & n_{A9}^{169} &= n_{A4}^{178} + n_{A5}^{178} & n_{A12}^{169} &= n_{A9}^{178} & n_{A8}^{169} &= n_{A9}^{178} & n_{A7}^{169} &= n_{A8}^{178} & n_{A11}^{169} &= n_{A8}^{178} & n_{A10}^{169} &= \\ n_{A6}^{178} + n_{A7}^{178} & n_{L3}^{169} &= n_{L2}^{178} + n_{L4}^{178} & n_{L4}^{169} &= n_{L3}^{178} + n_{L5}^{178} & n_{H4}^{169} &= n_{H6}^{178} & n_{H6}^{169} &= n_{H6}^{178} & n_{H5}^{169} &= n_{H4}^{178} + n_{H5}^{178} \end{aligned}$$

## 76. Lowered SGs by higher-dimensional irreps of pairings in SG 179

The representative operations of SG/T for SG 179:

$$\begin{aligned} 1 : (x, y, z), & 2 : (x - y, x, z + \frac{5}{6}), & 3 : (-y, x - y, z + \frac{2}{3}), & 4 : (-x, -y, z + \frac{1}{2}), & 5 : (y - x, -x, z + \frac{1}{3}), & 6 : (y, y - x, z + \frac{1}{6}), \\ 7 : (x - y, -y, -z), & 8 : (y, x, \frac{2}{3} - z), & 9 : (-x, y - x, \frac{1}{3} - z), & 10 : (x, x - y, \frac{5}{6} - z), & 11 : (y - x, y, \frac{1}{2} - z), & 12 : (-y, -x, \frac{1}{6} - z). \end{aligned}$$

The lower SG is SG 20 when the preserved operations are: **(sub-SG label is 1) 1, 4, 11, 7.**

The transformation is:  $(\mathbf{a}_{20}, \mathbf{b}_{20}, \mathbf{c}_{20}) = (\mathbf{a}_{179}, \mathbf{b}_{179}, \mathbf{c}_{179}) \begin{pmatrix} 1 & 1 & 0 \\ 2 & 0 & 0 \\ 0 & 0 & -1 \end{pmatrix}, \overrightarrow{O_{179}O_{20}} = \frac{1}{4}\mathbf{c}_{20}$

The reduction of higher dimensional irrep:

$$D_6 : E_2 \rightarrow A_1 + B_1 \text{ of } D_2.$$

$$D_6 : E_1 \rightarrow B_2 + B_3 \text{ of } D_2.$$

The correspondences of irreps at HSPs from original SG to lowered SG:

$$\begin{aligned} n_{GM5}^{20} &= n_{GM7}^{179} + n_{GM8}^{179} + n_{GM9}^{179} & n_{Y5}^{20} &= n_{M5}^{179} & n_{S4}^{20} &= n_{M5}^{179} & n_{S3}^{20} &= n_{M5}^{179} & n_{Z5}^{20} &= n_{A4}^{179} + n_{A8}^{179} & n_{Z4}^{20} &= n_{A7}^{179} + n_{A9}^{179} & n_{Z2}^{20} &= \\ n_{A6}^{179} + n_{A9}^{179} & n_{Z3}^{20} &= n_{A5}^{179} + n_{A8}^{179} & n_{T5}^{20} &= n_{L4}^{179} & n_{T4}^{20} &= n_{L5}^{179} & n_{T2}^{20} &= n_{L3}^{179} & n_{T3}^{20} &= n_{L2}^{179} & n_{R4}^{20} &= n_{L2}^{179} + n_{L4}^{179} & n_{R3}^{20} &= n_{L3}^{179} + n_{L5}^{179} \end{aligned}$$

The lower SG is SG 20 when the preserved operations are: **(sub-SG label is 2) 1, 4, 9, 10.**

The transformation is:  $(\mathbf{a}_{20}, \mathbf{b}_{20}, \mathbf{c}_{20}) = (\mathbf{a}_{179}, \mathbf{b}_{179}, \mathbf{c}_{179}) \begin{pmatrix} 0 & 2 & 0 \\ 1 & 1 & 0 \\ 0 & 0 & -1 \end{pmatrix}, \overrightarrow{O_{179}O_{20}} = \frac{1}{3}\mathbf{c}_{20}$

The reduction of higher dimensional irrep:

$$D_6 : E_2 \rightarrow A_1 + B_1 \text{ of } D_2.$$

$$D_6 : E_1 \rightarrow B_2 + B_3 \text{ of } D_2.$$

The correspondences of irreps at HSPs from original SG to lowered SG:

$$\begin{aligned} n_{GM5}^{20} &= n_{GM7}^{179} + n_{GM8}^{179} + n_{GM9}^{179} & n_{Y5}^{20} &= n_{M5}^{179} & n_{S4}^{20} &= n_{M5}^{179} & n_{S3}^{20} &= n_{M5}^{179} & n_{Z5}^{20} &= n_{A4}^{179} + n_{A8}^{179} & n_{Z4}^{20} &= n_{A6}^{179} + n_{A9}^{179} & n_{Z2}^{20} &= \\ n_{A7}^{179} + n_{A9}^{179} & n_{Z3}^{20} &= n_{A5}^{179} + n_{A8}^{179} & n_{T5}^{20} &= n_{L4}^{179} & n_{T4}^{20} &= n_{L3}^{179} & n_{T2}^{20} &= n_{L5}^{179} & n_{T3}^{20} &= n_{L2}^{179} & n_{R4}^{20} &= n_{L2}^{179} + n_{L4}^{179} & n_{R3}^{20} &= n_{L3}^{179} + n_{L5}^{179} \end{aligned}$$

The lower SG is SG 20 when the preserved operations are: **(sub-SG label is 3) 1, 4, 12, 8.**

The transformation is:  $(\mathbf{a}_{20}, \mathbf{b}_{20}, \mathbf{c}_{20}) = (\mathbf{a}_{179}, \mathbf{b}_{179}, \mathbf{c}_{179}) \begin{pmatrix} -1 & 1 & 0 \\ 1 & 1 & 0 \\ 0 & 0 & -1 \end{pmatrix}, \overrightarrow{O_{179}O_{20}} = \frac{5}{12}\mathbf{c}_{20}$

The reduction of higher dimensional irrep:

$$D_6 : E_2 \rightarrow A_1 + B_1 \text{ of } D_2.$$

$$D_6 : E_1 \rightarrow B_2 + B_3 \text{ of } D_2.$$

The correspondences of irreps at HSPs from original SG to lowered SG:

$$\begin{aligned} n_{GM5}^{20} &= n_{GM7}^{179} + n_{GM8}^{179} + n_{GM9}^{179} & n_{Y5}^{20} &= n_{M5}^{179} & n_{S4}^{20} &= n_{M5}^{179} & n_{S3}^{20} &= n_{M5}^{179} & n_{Z5}^{20} &= n_{A4}^{179} + n_{A8}^{179} & n_{Z4}^{20} &= n_{A7}^{179} + n_{A9}^{179} & n_{Z2}^{20} &= \\ n_{A6}^{179} + n_{A9}^{179} & n_{Z3}^{20} &= n_{A5}^{179} + n_{A8}^{179} & n_{T5}^{20} &= n_{L4}^{179} & n_{T4}^{20} &= n_{L5}^{179} & n_{T2}^{20} &= n_{L3}^{179} & n_{T3}^{20} &= n_{L2}^{179} & n_{R4}^{20} &= n_{L2}^{179} + n_{L4}^{179} & n_{R3}^{20} &= n_{L3}^{179} + n_{L5}^{179} \end{aligned}$$

The lower SG is SG 170 when the preserved operations are: **(sub-SG label is 4) 1, 2, 6, 3, 5, 4.**

The transformation is:  $(\mathbf{a}_{170}, \mathbf{b}_{170}, \mathbf{c}_{170}) = (\mathbf{a}_{179}, \mathbf{b}_{179}, \mathbf{c}_{179}) \begin{pmatrix} 1 & -1 & 0 \\ 0 & -1 & 0 \\ 0 & 0 & -1 \end{pmatrix}, \overrightarrow{O_{179}O_{170}} = \mathbf{a}_{170} + \mathbf{b}_{170} + (\frac{1}{4})\mathbf{c}_{170}$

The reduction of higher dimensional irrep:

$$D_6 : E_2 \rightarrow {}^1E_2 + {}^2E_2 \text{ of } C_6.$$

$$D_6 : E_1 \rightarrow {}^2E_1 + {}^1E_1 \text{ of } C_6.$$

The correspondences of irreps at HSPs from original SG to lowered SG:

$$\begin{aligned} n_{GM9}^{170} &= n_{GM8}^{179} & n_{GM12}^{170} &= n_{GM8}^{179} & n_{GM8}^{170} &= n_{GM7}^{179} & n_{GM7}^{170} &= n_{GM7}^{179} & n_{GM11}^{170} &= n_{GM9}^{179} & n_{GM10}^{170} &= n_{GM9}^{179} & n_{M3}^{170} &= n_{M5}^{179} & n_{M4}^{170} &= n_{M5}^{179} \\ n_{K4}^{170} &= n_{K4}^{179} + n_{K5}^{179} & n_{K6}^{170} &= n_{K6}^{179} & n_{K5}^{170} &= n_{K6}^{179} & n_{A9}^{170} &= n_{A8}^{179} & n_{A12}^{170} &= n_{A6}^{179} + n_{A7}^{179} & n_{A8}^{170} &= n_{A9}^{179} & n_{A7}^{170} &= n_{A8}^{179} & n_{A11}^{170} &= n_{A4}^{179} + n_{A5}^{179} \\ n_{A10}^{170} &= n_{A9}^{179} & n_{L3}^{170} &= n_{L2}^{179} + n_{L4}^{179} & n_{L4}^{170} &= n_{L3}^{179} + n_{L5}^{179} & n_{H5}^{170} &= n_{H6}^{179} & n_{H4}^{170} &= n_{H4}^{179} + n_{H5}^{179} & n_{H6}^{170} &= n_{H6}^{179} \end{aligned}$$

### 77. Lowered SGs by higher-dimensional irreps of pairings in SG 180

The representative operations of SG/T for SG 180:

$$\begin{aligned} 1 : (x, y, z), & 2 : (x - y, x, z + \frac{1}{3}), & 3 : (-y, x - y, z + \frac{2}{3}), & 4 : (-x, -y, z), & 5 : (y - x, -x, z + \frac{1}{3}), & 6 : (y, y - x, z + \frac{2}{3}), \\ 7 : (x - y, -y, -z), & 8 : (y, x, \frac{2}{3} - z), & 9 : (-x, y - x, \frac{1}{3} - z), & 10 : (x, x - y, \frac{1}{3} - z), & 11 : (y - x, y, -z), & 12 : (-y, -x, \frac{2}{3} - z). \end{aligned}$$

The lower SG is SG 21 when the preserved operations are: **(sub-SG label is 1) 1, 4, 11, 7.**

The transformation is:  $(\mathbf{a}_{21}, \mathbf{b}_{21}, \mathbf{c}_{21}) = (\mathbf{a}_{180}, \mathbf{b}_{180}, \mathbf{c}_{180}) \begin{pmatrix} 1 & -1 & 0 \\ 2 & 0 & 0 \\ 0 & 0 & 1 \end{pmatrix}, \overrightarrow{O_{180}O_{21}} = \frac{1}{2}\mathbf{c}_{21}$

The reduction of higher dimensional irrep:

$$D_6 : E_2 \rightarrow A_1 + B_1 \text{ of } D_2.$$

$$D_6 : E_1 \rightarrow B_2 + B_3 \text{ of } D_2.$$

The correspondences of irreps at HSPs from original SG to lowered SG:

$$\begin{aligned} n_{GM5}^{21} &= n_{GM7}^{180} + n_{GM8}^{180} + n_{GM9}^{180} & n_{Y5}^{21} &= n_{M5}^{180} & n_{S4}^{21} &= n_{M5}^{180} & n_{S3}^{21} &= n_{M5}^{180} & n_{Z5}^{21} &= n_{A7}^{180} + n_{A8}^{180} + n_{A9}^{180} & n_{T5}^{21} &= n_{L5}^{180} & n_{R4}^{21} &= n_{L5}^{180} \\ n_{R3}^{21} &= n_{L5}^{180} \end{aligned}$$

The lower SG is SG 21 when the preserved operations are: **(sub-SG label is 2) 1, 4, 9, 10.**

The transformation is:  $(\mathbf{a}_{21}, \mathbf{b}_{21}, \mathbf{c}_{21}) = (\mathbf{a}_{180}, \mathbf{b}_{180}, \mathbf{c}_{180}) \begin{pmatrix} 0 & -2 & 0 \\ 1 & -1 & 0 \\ 0 & 0 & 1 \end{pmatrix}, \overrightarrow{O_{180}O_{21}} = \frac{2}{3}\mathbf{c}_{21}$

The reduction of higher dimensional irrep:

$$D_6 : E_2 \rightarrow A_1 + B_1 \text{ of } D_2.$$

$$D_6 : E_1 \rightarrow B_2 + B_3 \text{ of } D_2.$$

The correspondences of irreps at HSPs from original SG to lowered SG:

$$\begin{aligned} n_{GM5}^{21} &= n_{GM7}^{180} + n_{GM8}^{180} + n_{GM9}^{180} & n_{Y5}^{21} &= n_{M5}^{180} & n_{S4}^{21} &= n_{M5}^{180} & n_{S3}^{21} &= n_{M5}^{180} & n_{Z5}^{21} &= n_{A7}^{180} + n_{A8}^{180} + n_{A9}^{180} & n_{T5}^{21} &= n_{L5}^{180} & n_{R4}^{21} &= n_{L5}^{180} \\ n_{R3}^{21} &= n_{L5}^{180} \end{aligned}$$

The lower SG is SG 21 when the preserved operations are: **(sub-SG label is 3) 1, 4, 12, 8.**

The transformation is:  $(\mathbf{a}_{21}, \mathbf{b}_{21}, \mathbf{c}_{21}) = (\mathbf{a}_{180}, \mathbf{b}_{180}, \mathbf{c}_{180}) \begin{pmatrix} -1 & -1 & 0 \\ 1 & -1 & 0 \\ 0 & 0 & 1 \end{pmatrix}, \overrightarrow{O_{180}O_{21}} = \frac{5}{6}\mathbf{c}_{21}$

The reduction of higher dimensional irrep:

$$D_6 : E_2 \rightarrow A_1 + B_1 \text{ of } D_2.$$

$$D_6 : E_1 \rightarrow B_2 + B_3 \text{ of } D_2.$$

The correspondences of irreps at HSPs from original SG to lowered SG:

$$\begin{aligned} n_{GM5}^{21} &= n_{GM7}^{180} + n_{GM8}^{180} + n_{GM9}^{180} & n_{Y5}^{21} &= n_{M5}^{180} & n_{S4}^{21} &= n_{M5}^{180} & n_{S3}^{21} &= n_{M5}^{180} & n_{Z5}^{21} &= n_{A7}^{180} + n_{A8}^{180} + n_{A9}^{180} & n_{T5}^{21} &= n_{L5}^{180} & n_{R4}^{21} &= n_{L5}^{180} \\ n_{R3}^{21} &= n_{L5}^{180} \end{aligned}$$

The lower SG is SG 171 when the preserved operations are: **(sub-SG label is 4) 1, 2, 6, 3, 5, 4.**

$$\text{The transformation is: } (\mathbf{a}_{171}, \mathbf{b}_{171}, \mathbf{c}_{171}) = (\mathbf{a}_{180}, \mathbf{b}_{180}, \mathbf{c}_{180}) \begin{pmatrix} 1 & -1 & 0 \\ 0 & -1 & 0 \\ 0 & 0 & -1 \end{pmatrix}, \overrightarrow{O_{180}O_{171}} = \mathbf{a}_{171} + \mathbf{b}_{171}$$

The reduction of higher dimensional irrep:

$$D_6 : E_2 \rightarrow {}^1E_2 + {}^2E_2 \text{ of } C_6.$$

$$D_6 : E_1 \rightarrow {}^2E_1 + {}^1E_1 \text{ of } C_6.$$

The correspondences of irreps at HSPs from original SG to lowered SG:

$$\begin{aligned} n_{GM9}^{171} &= n_{GM8}^{180} & n_{GM12}^{171} &= n_{GM8}^{180} & n_{GM8}^{171} &= n_{GM7}^{180} & n_{GM7}^{171} &= n_{GM7}^{180} & n_{GM11}^{171} &= n_{GM9}^{180} & n_{GM10}^{171} &= n_{GM9}^{180} & n_{M3}^{171} &= n_{M5}^{180} & n_{M4}^{171} &= n_{M5}^{180} \\ n_{K4}^{171} &= n_{K4}^{180} + n_{K5}^{180} & n_{K6}^{171} &= n_{K6}^{180} & n_{K5}^{171} &= n_{K6}^{180} & n_{A9}^{171} &= n_{A9}^{180} & n_{A12}^{171} &= n_{A7}^{180} & n_{A8}^{171} &= n_{A9}^{180} & n_{A7}^{171} &= n_{A8}^{180} & n_{A11}^{171} &= n_{A7}^{180} & n_{A10}^{171} &= n_{A8}^{180} \\ n_{L3}^{171} &= n_{L5}^{180} & n_{L4}^{171} &= n_{L5}^{180} & n_{H5}^{171} &= n_{H6}^{180} & n_{H4}^{171} &= n_{H4}^{180} + n_{H5}^{180} & n_{H6}^{171} &= n_{H6}^{180} \end{aligned}$$

### 78. Lowered SGs by higher-dimensional irreps of pairings in SG 181

The representative operations of SG/T for SG 181:

$$\begin{aligned} 1 : (x, y, z), & 2 : (x - y, x, z + \frac{2}{3}), & 3 : (-y, x - y, z + \frac{1}{3}), & 4 : (-x, -y, z), & 5 : (y - x, -x, z + \frac{2}{3}), & 6 : (y, y - x, z + \frac{1}{3}), \\ 7 : (x - y, -y, -z), & 8 : (y, x, \frac{1}{3} - z), & 9 : (-x, y - x, \frac{2}{3} - z), & 10 : (x, x - y, \frac{2}{3} - z), & 11 : (y - x, y, -z), & 12 : (-y, -x, \frac{1}{3} - z). \end{aligned}$$

The lower SG is SG 21 when the preserved operations are: **(sub-SG label is 1) 1, 4, 11, 7.**

$$\text{The transformation is: } (\mathbf{a}_{21}, \mathbf{b}_{21}, \mathbf{c}_{21}) = (\mathbf{a}_{181}, \mathbf{b}_{181}, \mathbf{c}_{181}) \begin{pmatrix} 1 & -1 & 0 \\ 2 & 0 & 0 \\ 0 & 0 & 1 \end{pmatrix}, \overrightarrow{O_{181}O_{21}} = \frac{1}{2}\mathbf{c}_{21}$$

The reduction of higher dimensional irrep:

$$D_6 : E_2 \rightarrow A_1 + B_1 \text{ of } D_2.$$

$$D_6 : E_1 \rightarrow B_2 + B_3 \text{ of } D_2.$$

The correspondences of irreps at HSPs from original SG to lowered SG:

$$\begin{aligned} n_{GM5}^{21} &= n_{GM7}^{181} + n_{GM8}^{181} + n_{GM9}^{181} & n_{Y5}^{21} &= n_{M5}^{181} & n_{S4}^{21} &= n_{M5}^{181} & n_{S3}^{21} &= n_{M5}^{181} & n_{Z5}^{21} &= n_{A7}^{181} + n_{A8}^{181} + n_{A9}^{181} & n_{T5}^{21} &= n_{L5}^{181} & n_{R4}^{21} &= n_{L5}^{181} \\ n_{R3}^{21} &= n_{L5}^{181} \end{aligned}$$

The lower SG is SG 21 when the preserved operations are: **(sub-SG label is 2) 1, 4, 9, 10.**

$$\text{The transformation is: } (\mathbf{a}_{21}, \mathbf{b}_{21}, \mathbf{c}_{21}) = (\mathbf{a}_{181}, \mathbf{b}_{181}, \mathbf{c}_{181}) \begin{pmatrix} 0 & -2 & 0 \\ 1 & -1 & 0 \\ 0 & 0 & 1 \end{pmatrix}, \overrightarrow{O_{181}O_{21}} = \frac{5}{6}\mathbf{c}_{21}$$

The reduction of higher dimensional irrep:

$$D_6 : E_2 \rightarrow A_1 + B_1 \text{ of } D_2.$$

$$D_6 : E_1 \rightarrow B_2 + B_3 \text{ of } D_2.$$

The correspondences of irreps at HSPs from original SG to lowered SG:

$$\begin{aligned} n_{GM5}^{21} &= n_{GM7}^{181} + n_{GM8}^{181} + n_{GM9}^{181} & n_{Y5}^{21} &= n_{M5}^{181} & n_{S4}^{21} &= n_{M5}^{181} & n_{S3}^{21} &= n_{M5}^{181} & n_{Z5}^{21} &= n_{A7}^{181} + n_{A8}^{181} + n_{A9}^{181} & n_{T5}^{21} &= n_{L5}^{181} & n_{R4}^{21} &= n_{L5}^{181} \\ n_{R3}^{21} &= n_{L5}^{181} \end{aligned}$$

The lower SG is SG 21 when the preserved operations are: **(sub-SG label is 3) 1, 4, 12, 8.**

$$\text{The transformation is: } (\mathbf{a}_{21}, \mathbf{b}_{21}, \mathbf{c}_{21}) = (\mathbf{a}_{181}, \mathbf{b}_{181}, \mathbf{c}_{181}) \begin{pmatrix} -1 & -1 & 0 \\ 1 & -1 & 0 \\ 0 & 0 & 1 \end{pmatrix}, \overrightarrow{O_{181}O_{21}} = \frac{2}{3}\mathbf{c}_{21}$$

The reduction of higher dimensional irrep:

$$D_6 : E_2 \rightarrow A_1 + B_1 \text{ of } D_2.$$

$$D_6 : E_1 \rightarrow B_2 + B_3 \text{ of } D_2.$$

The correspondences of irreps at HSPs from original SG to lowered SG:

$$\begin{aligned} n_{GM5}^{21} &= n_{GM7}^{181} + n_{GM8}^{181} + n_{GM9}^{181} \quad n_{Y5}^{21} = n_{M5}^{181} \quad n_{S4}^{21} = n_{M5}^{181} \quad n_{S3}^{21} = n_{M5}^{181} \quad n_{Z5}^{21} = n_{A7}^{181} + n_{A8}^{181} + n_{A9}^{181} \\ n_{T5}^{21} &= n_{L5}^{181} \quad n_{R4}^{21} = n_{L5}^{181} \quad n_{R3}^{21} = n_{L5}^{181} \end{aligned}$$

The lower SG is SG 172 when the preserved operations are: **(sub-SG label is 4) 1, 2, 6, 3, 5, 4.**

$$\text{The transformation is: } (\mathbf{a}_{172}, \mathbf{b}_{172}, \mathbf{c}_{172}) = (\mathbf{a}_{181}, \mathbf{b}_{181}, \mathbf{c}_{181}) \begin{pmatrix} 1 & -1 & 0 \\ 0 & -1 & 0 \\ 0 & 0 & -1 \end{pmatrix}, \overrightarrow{O_{181}O_{172}} = \mathbf{a}_{172} + \mathbf{b}_{172}$$

The reduction of higher dimensional irrep:

$$D_6 : E_2 \rightarrow {}^1E_2 + {}^2E_2 \text{ of } C_6.$$

$$D_6 : E_1 \rightarrow {}^2E_1 + {}^1E_1 \text{ of } C_6.$$

The correspondences of irreps at HSPs from original SG to lowered SG:

$$\begin{aligned} n_{GM9}^{172} &= n_{GM8}^{181} \quad n_{GM12}^{172} = n_{GM8}^{181} \quad n_{GM8}^{172} = n_{GM7}^{181} \quad n_{GM7}^{172} = n_{GM7}^{181} \quad n_{GM11}^{172} = n_{GM9}^{181} \quad n_{GM10}^{172} = n_{GM9}^{181} \quad n_{M3}^{172} = n_{M5}^{181} \quad n_{M4}^{172} = n_{M5}^{181} \\ n_{K4}^{172} &= n_{K4}^{181} + n_{K5}^{181} \quad n_{K6}^{172} = n_{K6}^{181} \quad n_{K5}^{172} = n_{K6}^{181} \quad n_{A9}^{172} = n_{A7}^{181} \quad n_{A12}^{172} = n_{A9}^{181} \quad n_{A8}^{172} = n_{A8}^{181} \quad n_{A7}^{172} = n_{A9}^{181} \quad n_{A11}^{172} = n_{A8}^{181} \quad n_{A10}^{172} = n_{A7}^{181} \\ n_{L3}^{172} &= n_{L5}^{181} \quad n_{L4}^{172} = n_{L5}^{181} \quad n_{H4}^{172} = n_{H6}^{181} \quad n_{H6}^{172} = n_{H6}^{181} \quad n_{H5}^{172} = n_{H4}^{181} + n_{H5}^{181} \end{aligned}$$

### 79. Lowered SGs by higher-dimensional irreps of pairings in SG 182

The representative operations of SG/T for SG 182:

$$\begin{aligned} 1 : (x, y, z), \quad 2 : (x - y, x, z + \frac{1}{2}), \quad 3 : (-y, x - y, z), \quad 4 : (-x, -y, z + \frac{1}{2}), \quad 5 : (y - x, -x, z), \quad 6 : (y, y - x, z + \frac{1}{2}), \\ 7 : (x - y, -y, -z), \quad 8 : (y, x, -z), \quad 9 : (-x, y - x, -z), \quad 10 : (x, x - y, \frac{1}{2} - z), \quad 11 : (y - x, y, \frac{1}{2} - z), \quad 12 : (-y, -x, \frac{1}{2} - z). \end{aligned}$$

The lower SG is SG 20 when the preserved operations are: **(sub-SG label is 1) 1, 4, 11, 7.**

$$\text{The transformation is: } (\mathbf{a}_{20}, \mathbf{b}_{20}, \mathbf{c}_{20}) = (\mathbf{a}_{182}, \mathbf{b}_{182}, \mathbf{c}_{182}) \begin{pmatrix} 1 & 1 & 0 \\ 2 & 0 & 0 \\ 0 & 0 & -1 \end{pmatrix}, \overrightarrow{O_{182}O_{20}} = \frac{1}{4}\mathbf{c}_{20}$$

The reduction of higher dimensional irrep:

$$D_6 : E_2 \rightarrow A_1 + B_1 \text{ of } D_2.$$

$$D_6 : E_1 \rightarrow B_2 + B_3 \text{ of } D_2.$$

The correspondences of irreps at HSPs from original SG to lowered SG:

$$\begin{aligned} n_{GM5}^{20} &= n_{GM7}^{182} + n_{GM8}^{182} + n_{GM9}^{182} \quad n_{Y5}^{20} = n_{M5}^{182} \quad n_{S4}^{20} = n_{M5}^{182} \quad n_{S3}^{20} = n_{M5}^{182} \quad n_{Z5}^{20} = n_{A4}^{182} + n_{A8}^{182} \quad n_{Z4}^{20} = n_{A7}^{182} + n_{A9}^{182} \quad n_{Z2}^{20} = \\ n_{A6}^{182} + n_{A9}^{182} \quad n_{Z3}^{20} &= n_{A4}^{182} + n_{A8}^{182} \quad n_{T5}^{20} = n_{L4}^{182} \quad n_{T4}^{20} = n_{L3}^{182} \quad n_{T2}^{20} = n_{L5}^{182} \quad n_{T3}^{20} = n_{L2}^{182} \quad n_{R4}^{20} = n_{L2}^{182} + n_{L4}^{182} \quad n_{R3}^{20} = n_{L3}^{182} + n_{L5}^{182} \end{aligned}$$

The lower SG is SG 20 when the preserved operations are: **(sub-SG label is 2) 1, 4, 9, 10.**

$$\text{The transformation is: } (\mathbf{a}_{20}, \mathbf{b}_{20}, \mathbf{c}_{20}) = (\mathbf{a}_{182}, \mathbf{b}_{182}, \mathbf{c}_{182}) \begin{pmatrix} 0 & 2 & 0 \\ 1 & 1 & 0 \\ 0 & 0 & -1 \end{pmatrix}, \overrightarrow{O_{182}O_{20}} = \frac{1}{2}\mathbf{c}_{20}$$

The reduction of higher dimensional irrep:

$$D_6 : E_2 \rightarrow A_1 + B_1 \text{ of } D_2.$$

$$D_6 : E_1 \rightarrow B_2 + B_3 \text{ of } D_2.$$

The correspondences of irreps at HSPs from original SG to lowered SG:

$$\begin{aligned} n_{GM5}^{20} &= n_{GM7}^{182} + n_{GM8}^{182} + n_{GM9}^{182} \quad n_{Y5}^{20} = n_{M5}^{182} \quad n_{S4}^{20} = n_{M5}^{182} \quad n_{S3}^{20} = n_{M5}^{182} \quad n_{Z5}^{20} = n_{A5}^{182} + n_{A8}^{182} \quad n_{Z4}^{20} = n_{A7}^{182} + n_{A9}^{182} \quad n_{Z2}^{20} = \\ n_{A6}^{182} + n_{A9}^{182} \quad n_{Z3}^{20} &= n_{A4}^{182} + n_{A8}^{182} \quad n_{T5}^{20} = n_{L4}^{182} \quad n_{T4}^{20} = n_{L3}^{182} \quad n_{T2}^{20} = n_{L5}^{182} \quad n_{T3}^{20} = n_{L2}^{182} \quad n_{R4}^{20} = n_{L2}^{182} + n_{L4}^{182} \quad n_{R3}^{20} = n_{L3}^{182} + n_{L5}^{182} \end{aligned}$$

The lower SG is SG 20 when the preserved operations are: **(sub-SG label is 3) 1, 4, 12, 8.**

$$\text{The transformation is: } (\mathbf{a}_{20}, \mathbf{b}_{20}, \mathbf{c}_{20}) = (\mathbf{a}_{182}, \mathbf{b}_{182}, \mathbf{c}_{182}) \begin{pmatrix} -1 & 1 & 0 \\ 1 & 1 & 0 \\ 0 & 0 & -1 \end{pmatrix}, \overrightarrow{O_{182}O_{20}} = \frac{1}{4}\mathbf{c}_{20}$$

The reduction of higher dimensional irrep:

$$D_6 : E_2 \rightarrow A_1 + B_1 \text{ of } D_2.$$

$$D_6 : E_1 \rightarrow B_2 + B_3 \text{ of } D_2.$$

The correspondences of irreps at HSPs from original SG to lowered SG:

$$\begin{aligned} n_{GM5}^{20} &= n_{GM7}^{182} + n_{GM8}^{182} + n_{GM9}^{182} & n_{Y5}^{20} &= n_{M5}^{182} & n_{S4}^{20} &= n_{M5}^{182} & n_{S3}^{20} &= n_{M5}^{182} & n_{Z5}^{20} &= n_{A5}^{182} + n_{A8}^{182} & n_{Z4}^{20} &= n_{A6}^{182} + n_{A9}^{182} & n_{Z2}^{20} &= \\ n_{A7}^{182} + n_{A9}^{182} & n_{Z3}^{20} &= n_{A4}^{182} + n_{A8}^{182} & n_{T5}^{20} &= n_{L4}^{182} & n_{T4}^{20} &= n_{L5}^{182} & n_{T2}^{20} &= n_{L3}^{182} & n_{T3}^{20} &= n_{L2}^{182} & n_{R4}^{20} &= n_{L2}^{182} + n_{L4}^{182} & n_{R3}^{20} &= n_{L3}^{182} + n_{L5}^{182} \end{aligned}$$

The lower SG is SG 173 when the preserved operations are: **(sub-SG label is 4) 1, 2, 6, 3, 5, 4.**

The transformation is:  $(\mathbf{a}_{173}, \mathbf{b}_{173}, \mathbf{c}_{173}) = (\mathbf{a}_{182}, \mathbf{b}_{182}, \mathbf{c}_{182}) \begin{pmatrix} 1 & -1 & 0 \\ 0 & -1 & 0 \\ 0 & 0 & -1 \end{pmatrix}, \overrightarrow{O_{182}O_{173}} = \mathbf{a}_{173} + \mathbf{b}_{173} + (\frac{1}{4})\mathbf{c}_{173}$

The reduction of higher dimensional irrep:

$$D_6 : E_2 \rightarrow {}^1E_2 + {}^2E_2 \text{ of } C_6.$$

$$D_6 : E_1 \rightarrow {}^2E_1 + {}^1E_1 \text{ of } C_6.$$

The correspondences of irreps at HSPs from original SG to lowered SG:

$$\begin{aligned} n_{GM9}^{173} &= n_{GM8}^{182} & n_{GM12}^{173} &= n_{GM8}^{182} & n_{GM8}^{173} &= n_{GM7}^{182} & n_{GM7}^{173} &= n_{GM7}^{182} & n_{GM11}^{173} &= n_{GM9}^{182} & n_{GM10}^{173} &= n_{GM9}^{182} & n_{M3}^{173} &= n_{M5}^{182} & n_{M4}^{173} &= n_{M5}^{182} \\ n_{K4}^{173} &= n_{K4}^{182} + n_{K5}^{182} & n_{K6}^{173} &= n_{K6}^{182} & n_{K5}^{173} &= n_{K6}^{182} & n_{A9}^{173} &= n_{A8}^{182} & n_{A12}^{173} &= n_{A9}^{182} & n_{A8}^{173} &= n_{A6}^{182} + n_{A7}^{182} & n_{A7}^{173} &= n_{A4}^{182} + n_{A5}^{182} & n_{A11}^{173} &= n_{A8}^{182} \\ n_{A10}^{173} &= n_{A9}^{182} & n_{L3}^{173} &= n_{L2}^{182} + n_{L4}^{182} & n_{L4}^{173} &= n_{L3}^{182} + n_{L5}^{182} & n_{H4}^{173} &= n_{H4}^{182} + n_{H5}^{182} & n_{H6}^{173} &= n_{H6}^{182} & n_{H5}^{173} &= n_{H6}^{182} \end{aligned}$$

### 80. Lowered SGs by higher-dimensional irreps of pairings in SG 183

The representative operations of SG/T for SG 183:

$$\begin{aligned} &1 : (x, y, z), 2 : (x - y, x, z), 3 : (-y, x - y, z), 4 : (-x, -y, z), 5 : (y - x, -x, z), 6 : (y, y - x, z), 7 : (y - x, y, z), \\ &8 : (-y, -x, z), 9 : (x, x - y, z), 10 : (-x, y - x, z), 11 : (x - y, -y, z), 12 : (y, x, z). \end{aligned}$$

The lower SG is SG 35 when the preserved operations are: **(sub-SG label is 1) 1, 4, 11, 7.**

The transformation is:  $(\mathbf{a}_{35}, \mathbf{b}_{35}, \mathbf{c}_{35}) = (\mathbf{a}_{183}, \mathbf{b}_{183}, \mathbf{c}_{183}) \begin{pmatrix} 1 & -1 & 0 \\ 2 & 0 & 0 \\ 0 & 0 & 1 \end{pmatrix}, \overrightarrow{O_{183}O_{35}} = \mathbf{0}$

The reduction of higher dimensional irrep:

$$C_{6v} : E_2 \rightarrow A_1 + A_2 \text{ of } C_{2v}.$$

$$C_{6v} : E_1 \rightarrow B_1 + B_2 \text{ of } C_{2v}.$$

The correspondences of irreps at HSPs from original SG to lowered SG:

$$\begin{aligned} n_{GM5}^{35} &= n_{GM7}^{183} + n_{GM8}^{183} + n_{GM9}^{183} & n_{Y5}^{35} &= n_{M5}^{183} & n_{S4}^{35} &= n_{M5}^{183} & n_{S3}^{35} &= n_{M5}^{183} & n_{Z5}^{35} &= n_{A7}^{183} + n_{A8}^{183} + n_{A9}^{183} & n_{T5}^{35} &= n_{L5}^{183} & n_{R4}^{35} &= n_{L5}^{183} \\ n_{R3}^{35} &= n_{L5}^{183} \end{aligned}$$

The lower SG is SG 35 when the preserved operations are: **(sub-SG label is 2) 1, 4, 9, 10.**

The transformation is:  $(\mathbf{a}_{35}, \mathbf{b}_{35}, \mathbf{c}_{35}) = (\mathbf{a}_{183}, \mathbf{b}_{183}, \mathbf{c}_{183}) \begin{pmatrix} 0 & -2 & 0 \\ 1 & -1 & 0 \\ 0 & 0 & 1 \end{pmatrix}, \overrightarrow{O_{183}O_{35}} = \mathbf{0}$

The reduction of higher dimensional irrep:

$$C_{6v} : E_2 \rightarrow A_1 + A_2 \text{ of } C_{2v}.$$

$$C_{6v} : E_1 \rightarrow B_1 + B_2 \text{ of } C_{2v}.$$

The correspondences of irreps at HSPs from original SG to lowered SG:

$$\begin{aligned} n_{GM5}^{35} &= n_{GM7}^{183} + n_{GM8}^{183} + n_{GM9}^{183} & n_{Y5}^{35} &= n_{M5}^{183} & n_{S4}^{35} &= n_{M5}^{183} & n_{S3}^{35} &= n_{M5}^{183} & n_{Z5}^{35} &= n_{A7}^{183} + n_{A8}^{183} + n_{A9}^{183} & n_{T5}^{35} &= n_{L5}^{183} & n_{R4}^{35} &= n_{L5}^{183} \\ n_{R3}^{35} &= n_{L5}^{183} \end{aligned}$$

The lower SG is SG 35 when the preserved operations are: **(sub-SG label is 3) 1, 4, 12, 8.**

The transformation is:  $(\mathbf{a}_{35}, \mathbf{b}_{35}, \mathbf{c}_{35}) = (\mathbf{a}_{183}, \mathbf{b}_{183}, \mathbf{c}_{183}) \begin{pmatrix} -1 & -1 & 0 \\ 1 & -1 & 0 \\ 0 & 0 & 1 \end{pmatrix}, \overrightarrow{O_{183}O_{35}} = \mathbf{0}$

The reduction of higher dimensional irrep:

$$C_{6v} : E_2 \rightarrow A_1 + A_2 \text{ of } C_{2v}.$$

$$C_{6v} : E_1 \rightarrow B_1 + B_2 \text{ of } C_{2v}.$$

The correspondences of irreps at HSPs from original SG to lowered SG:

$$n_{GM5}^{35} = n_{GM7}^{183} + n_{GM8}^{183} + n_{GM9}^{183} n_{Y5}^{35} = n_{M5}^{183} n_{S4}^{35} = n_{M5}^{183} n_{S3}^{35} = n_{M5}^{183} n_{Z5}^{35} = n_{A7}^{183} + n_{A8}^{183} + n_{A9}^{183} n_{T5}^{35} = n_{L5}^{183} n_{R4}^{35} = n_{L5}^{183} n_{R3}^{35} = n_{L5}^{183}$$

The lower SG is SG 168 when the preserved operations are: **(sub-SG label is 4) 1, 2, 6, 3, 5, 4.**

$$\text{The transformation is: } (\mathbf{a}_{168}, \mathbf{b}_{168}, \mathbf{c}_{168}) = (\mathbf{a}_{183}, \mathbf{b}_{183}, \mathbf{c}_{183}) \begin{pmatrix} -1 & 1 & 0 \\ -1 & 0 & 0 \\ 0 & 0 & 1 \end{pmatrix}, \overrightarrow{O_{183}O_{168}} = -\mathbf{a}_{168}$$

The reduction of higher dimensional irrep:

$$C_{6v} : E_2 \rightarrow {}^1E_2 + {}^2E_2 \text{ of } C_6.$$

$$C_{6v} : E_1 \rightarrow {}^2E_1 + {}^1E_1 \text{ of } C_6.$$

The correspondences of irreps at HSPs from original SG to lowered SG:

$$n_{GM9}^{168} = n_{GM8}^{183} n_{GM12}^{168} = n_{GM8}^{183} n_{GM8}^{168} = n_{GM7}^{183} n_{GM7}^{168} = n_{GM7}^{183} n_{GM11}^{168} = n_{GM9}^{183} n_{GM10}^{168} = n_{GM9}^{183} n_{M3}^{168} = n_{M5}^{183} n_{M4}^{168} = n_{M5}^{183} n_{K4}^{168} = n_{K4}^{183} + n_{K5}^{183} n_{K6}^{168} = n_{K6}^{183} n_{K5}^{168} = n_{K6}^{183} n_{A9}^{168} = n_{A8}^{183} n_{A12}^{168} = n_{A8}^{183} n_{A8}^{168} = n_{A7}^{183} n_{A7}^{168} = n_{A7}^{183} n_{A11}^{168} = n_{A9}^{183} n_{A10}^{168} = n_{A9}^{183} n_{L3}^{168} = n_{L5}^{183} n_{L4}^{168} = n_{L5}^{183} n_{H4}^{168} = n_{H4}^{183} + n_{H5}^{183} n_{H6}^{168} = n_{H6}^{183} n_{H5}^{168} = n_{H6}^{183}$$

### 81. Lowered SGs by higher-dimensional irreps of pairings in SG 184

The representative operations of SG/T for SG 184:

$$1 : (x, y, z), 2 : (x - y, x, z), 3 : (-y, x - y, z), 4 : (-x, -y, z), 5 : (y - x, -x, z), 6 : (y, y - x, z), 7 : (y - x, y, z + \frac{1}{2}), \\ 8 : (-y, -x, z + \frac{1}{2}), 9 : (x, x - y, z + \frac{1}{2}), 10 : (-x, y - x, z + \frac{1}{2}), 11 : (x - y, -y, z + \frac{1}{2}), 12 : (y, x, z + \frac{1}{2}).$$

The lower SG is SG 37 when the preserved operations are: **(sub-SG label is 1) 1, 4, 11, 7.**

$$\text{The transformation is: } (\mathbf{a}_{37}, \mathbf{b}_{37}, \mathbf{c}_{37}) = (\mathbf{a}_{184}, \mathbf{b}_{184}, \mathbf{c}_{184}) \begin{pmatrix} 1 & -1 & 0 \\ 2 & 0 & 0 \\ 0 & 0 & 1 \end{pmatrix}, \overrightarrow{O_{184}O_{37}} = \mathbf{0}$$

The reduction of higher dimensional irrep:

$$C_{6v} : E_2 \rightarrow A_1 + A_2 \text{ of } C_{2v}.$$

$$C_{6v} : E_1 \rightarrow B_1 + B_2 \text{ of } C_{2v}.$$

The correspondences of irreps at HSPs from original SG to lowered SG:

$$n_{GM5}^{37} = n_{GM7}^{184} + n_{GM8}^{184} + n_{GM9}^{184} n_{Y5}^{37} = n_{M5}^{184} n_{S4}^{37} = n_{M5}^{184} n_{S3}^{37} = n_{M5}^{184} n_{Z5}^{37} = n_{A7}^{184} + n_{A8}^{184} + n_{A9}^{184} n_{T5}^{37} = n_{L5}^{184} n_{R4}^{37} = n_{L5}^{184} n_{R3}^{37} = n_{L5}^{184}$$

The lower SG is SG 37 when the preserved operations are: **(sub-SG label is 2) 1, 4, 9, 10.**

$$\text{The transformation is: } (\mathbf{a}_{37}, \mathbf{b}_{37}, \mathbf{c}_{37}) = (\mathbf{a}_{184}, \mathbf{b}_{184}, \mathbf{c}_{184}) \begin{pmatrix} 0 & -2 & 0 \\ 1 & -1 & 0 \\ 0 & 0 & 1 \end{pmatrix}, \overrightarrow{O_{184}O_{37}} = \mathbf{0}$$

The reduction of higher dimensional irrep:

$$C_{6v} : E_2 \rightarrow A_1 + A_2 \text{ of } C_{2v}.$$

$$C_{6v} : E_1 \rightarrow B_1 + B_2 \text{ of } C_{2v}.$$

The correspondences of irreps at HSPs from original SG to lowered SG:

$$n_{GM5}^{37} = n_{GM7}^{184} + n_{GM8}^{184} + n_{GM9}^{184} n_{Y5}^{37} = n_{M5}^{184} n_{S4}^{37} = n_{M5}^{184} n_{S3}^{37} = n_{M5}^{184} n_{Z5}^{37} = n_{A7}^{184} + n_{A8}^{184} + n_{A9}^{184} n_{T5}^{37} = n_{L5}^{184} n_{R4}^{37} = n_{L5}^{184} n_{R3}^{37} = n_{L5}^{184}$$

The lower SG is SG 37 when the preserved operations are: **(sub-SG label is 3) 1, 4, 12, 8.**

$$\text{The transformation is: } (\mathbf{a}_{37}, \mathbf{b}_{37}, \mathbf{c}_{37}) = (\mathbf{a}_{184}, \mathbf{b}_{184}, \mathbf{c}_{184}) \begin{pmatrix} -1 & -1 & 0 \\ 1 & -1 & 0 \\ 0 & 0 & 1 \end{pmatrix}, \overrightarrow{O_{184}O_{37}} = \mathbf{0}$$

The reduction of higher dimensional irrep:

$$C_{6v} : E_2 \rightarrow A_1 + A_2 \text{ of } C_{2v}.$$

$$C_{6v} : E_1 \rightarrow B_1 + B_2 \text{ of } C_{2v}.$$

The correspondences of irreps at HSPs from original SG to lowered SG:

$$n_{GM5}^{37} = n_{GM7}^{184} + n_{GM8}^{184} + n_{GM9}^{184} n_{Y5}^{37} = n_{M5}^{184} n_{S4}^{37} = n_{M5}^{184} n_{S3}^{37} = n_{M5}^{184} n_{Z5}^{37} = n_{A7}^{184} + n_{A8}^{184} + n_{A9}^{184} n_{T5}^{37} = n_{L5}^{184} n_{R4}^{37} = n_{L5}^{184} n_{R3}^{37} = n_{L5}^{184}$$

The lower SG is SG 168 when the preserved operations are: **(sub-SG label is 4) 1, 2, 6, 3, 5, 4.**

$$\text{The transformation is: } (\mathbf{a}_{168}, \mathbf{b}_{168}, \mathbf{c}_{168}) = (\mathbf{a}_{184}, \mathbf{b}_{184}, \mathbf{c}_{184}) \begin{pmatrix} -1 & 1 & 0 \\ -1 & 0 & 0 \\ 0 & 0 & 1 \end{pmatrix}, \overrightarrow{O_{184}O_{168}} = -\mathbf{a}_{168}$$

The reduction of higher dimensional irrep:

$$C_{6v} : E_2 \rightarrow {}^1E_2 + {}^2E_2 \text{ of } C_6.$$

$$C_{6v} : E_1 \rightarrow {}^2E_1 + {}^1E_1 \text{ of } C_6.$$

The correspondences of irreps at HSPs from original SG to lowered SG:

$$n_{GM9}^{168} = n_{GM8}^{184} n_{GM12}^{168} = n_{GM8}^{184} n_{GM8}^{168} = n_{GM7}^{184} n_{GM7}^{168} = n_{GM7}^{184} n_{GM11}^{168} = n_{GM9}^{184} n_{GM10}^{168} = n_{GM9}^{184} n_{M3}^{168} = n_{M5}^{184} n_{M4}^{168} = n_{M5}^{184} n_{K4}^{168} = n_{K4}^{184} + n_{K5}^{184} n_{K6}^{168} = n_{K6}^{184} n_{K5}^{168} = n_{K6}^{184} n_{A9}^{168} = n_{A8}^{184} n_{A12}^{168} = n_{A8}^{184} n_{A8}^{168} = n_{A7}^{184} n_{A7}^{168} = n_{A7}^{184} n_{A11}^{168} = n_{A9}^{184} n_{A10}^{168} = n_{A9}^{184} n_{L3}^{168} = n_{L5}^{184} n_{L4}^{168} = n_{L5}^{184} n_{H4}^{168} = n_{H4}^{184} + n_{H5}^{184} n_{H6}^{168} = n_{H6}^{184} n_{H5}^{168} = n_{H6}^{184}$$

## 82. Lowered SGs by higher-dimensional irreps of pairings in SG 185

The representative operations of SG/T for SG 185:

$$1 : (x, y, z), 2 : (x - y, x, z + \frac{1}{2}), 3 : (-y, x - y, z), 4 : (-x, -y, z + \frac{1}{2}), 5 : (y - x, -x, z), 6 : (y, y - x, z + \frac{1}{2}), 7 : (y - x, y, z + \frac{1}{2}), 8 : (-y, -x, z + \frac{1}{2}), 9 : (x, x - y, z + \frac{1}{2}), 10 : (-x, y - x, z), 11 : (x - y, -y, z), 12 : (y, x, z).$$

The lower SG is SG 36 when the preserved operations are: **(sub-SG label is 1) 1, 4, 11, 7.**

$$\text{The transformation is: } (\mathbf{a}_{36}, \mathbf{b}_{36}, \mathbf{c}_{36}) = (\mathbf{a}_{185}, \mathbf{b}_{185}, \mathbf{c}_{185}) \begin{pmatrix} 1 & 1 & 0 \\ 2 & 0 & 0 \\ 0 & 0 & -1 \end{pmatrix}, \overrightarrow{O_{185}O_{36}} = \mathbf{0}$$

The reduction of higher dimensional irrep:

$$C_{6v} : E_2 \rightarrow A_1 + A_2 \text{ of } C_{2v}.$$

$$C_{6v} : E_1 \rightarrow B_2 + B_1 \text{ of } C_{2v}.$$

The correspondences of irreps at HSPs from original SG to lowered SG:

$$n_{GM5}^{36} = n_{GM7}^{185} + n_{GM8}^{185} + n_{GM9}^{185} n_{Y5}^{36} = n_{M5}^{185} n_{S4}^{36} = n_{M5}^{185} n_{S3}^{36} = n_{M5}^{185} n_{Z5}^{36} = n_{A7}^{185} + n_{A8}^{185} + n_{A9}^{185} n_{T5}^{36} = n_{L5}^{185} n_{R4}^{36} = n_{L5}^{185} n_{R3}^{36} = n_{L5}^{185}$$

The lower SG is SG 36 when the preserved operations are: **(sub-SG label is 2) 1, 4, 9, 10.**

$$\text{The transformation is: } (\mathbf{a}_{36}, \mathbf{b}_{36}, \mathbf{c}_{36}) = (\mathbf{a}_{185}, \mathbf{b}_{185}, \mathbf{c}_{185}) \begin{pmatrix} 2 & 0 & 0 \\ 1 & -1 & 0 \\ 0 & 0 & -1 \end{pmatrix}, \overrightarrow{O_{185}O_{36}} = \mathbf{0}$$

The reduction of higher dimensional irrep:

$$C_{6v} : E_2 \rightarrow A_1 + A_2 \text{ of } C_{2v}.$$

$$C_{6v} : E_1 \rightarrow B_2 + B_1 \text{ of } C_{2v}.$$

The correspondences of irreps at HSPs from original SG to lowered SG:

$$n_{GM5}^{36} = n_{GM7}^{185} + n_{GM8}^{185} + n_{GM9}^{185} n_{Y5}^{36} = n_{M5}^{185} n_{S4}^{36} = n_{M5}^{185} n_{S3}^{36} = n_{M5}^{185} n_{Z5}^{36} = n_{A7}^{185} + n_{A8}^{185} + n_{A9}^{185} n_{T5}^{36} = n_{L5}^{185} n_{R4}^{36} = n_{L5}^{185} n_{R3}^{36} = n_{L5}^{185}$$

The lower SG is SG 36 when the preserved operations are: **(sub-SG label is 3) 1, 4, 12, 8.**

$$\text{The transformation is: } (\mathbf{a}_{36}, \mathbf{b}_{36}, \mathbf{c}_{36}) = (\mathbf{a}_{185}, \mathbf{b}_{185}, \mathbf{c}_{185}) \begin{pmatrix} -1 & 1 & 0 \\ 1 & 1 & 0 \\ 0 & 0 & -1 \end{pmatrix}, \overrightarrow{O_{185}O_{36}} = \mathbf{0}$$

The reduction of higher dimensional irrep:

$$C_{6v} : E_2 \rightarrow A_1 + A_2 \text{ of } C_{2v}.$$

$$C_{6v} : E_1 \rightarrow B_2 + B_1 \text{ of } C_{2v}.$$

The correspondences of irreps at HSPs from original SG to lowered SG:

$$n_{GM5}^{36} = n_{GM7}^{185} + n_{GM8}^{185} + n_{GM9}^{185} n_{Y5}^{36} = n_{M5}^{185} n_{S4}^{36} = n_{M5}^{185} n_{S3}^{36} = n_{M5}^{185} n_{Z5}^{36} = n_{A7}^{185} + n_{A8}^{185} + n_{A9}^{185} n_{T5}^{36} = n_{L5}^{185} n_{R4}^{36} = n_{L5}^{185} n_{R3}^{36} = n_{L5}^{185}$$

The lower SG is SG 173 when the preserved operations are: **(sub-SG label is 4) 1, 2, 6, 3, 5, 4.**

$$\text{The transformation is: } (\mathbf{a}_{173}, \mathbf{b}_{173}, \mathbf{c}_{173}) = (\mathbf{a}_{185}, \mathbf{b}_{185}, \mathbf{c}_{185}) \begin{pmatrix} 1 & -1 & 0 \\ 0 & -1 & 0 \\ 0 & 0 & -1 \end{pmatrix}, \overrightarrow{O_{185}O_{173}} = \mathbf{a}_{173} + \mathbf{b}_{173}$$

The reduction of higher dimensional irrep:

$$C_{6v} : E_2 \rightarrow {}^1E_2 + {}^2E_2 \text{ of } C_6.$$

$$C_{6v} : E_1 \rightarrow {}^2E_1 + {}^1E_1 \text{ of } C_6.$$

The correspondences of irreps at HSPs from original SG to lowered SG:

$$n_{GM9}^{173} = n_{GM8}^{185} n_{GM12}^{173} = n_{GM8}^{185} n_{GM8}^{173} = n_{GM7}^{185} n_{GM7}^{173} = n_{GM7}^{185} n_{GM11}^{173} = n_{GM9}^{185} n_{GM10}^{173} = n_{GM9}^{185} n_{M3}^{173} = n_{M5}^{185} n_{M4}^{173} = n_{M5}^{185} n_{K4}^{173} = n_{K4}^{185} + n_{K5}^{185} n_{K6}^{173} = n_{K6}^{185} n_{K5}^{173} = n_{K6}^{185} n_{A9}^{173} = n_{A9}^{185} n_{A12}^{173} = n_{A9}^{185} n_{A8}^{173} = n_{A7}^{185} n_{A7}^{173} = n_{A7}^{185} n_{A11}^{173} = n_{A8}^{185} n_{A10}^{173} = n_{A8}^{185} n_{L3}^{173} = n_{L5}^{185} n_{L4}^{173} = n_{L5}^{185} n_{H4}^{173} = n_{H4}^{185} + n_{H5}^{185} n_{H6}^{173} = n_{H6}^{185} n_{H5}^{173} = n_{H6}^{185}$$

### 83. Lowered SGs by higher-dimensional irreps of pairings in SG 186

The representative operations of SG/T for SG 186:

$$1 : (x, y, z), 2 : (x - y, x, z + \frac{1}{2}), 3 : (-y, x - y, z), 4 : (-x, -y, z + \frac{1}{2}), 5 : (y - x, -x, z), 6 : (y, y - x, z + \frac{1}{2}), \\ 7 : (y - x, y, z), 8 : (-y, -x, z), 9 : (x, x - y, z), 10 : (-x, y - x, z + \frac{1}{2}), 11 : (x - y, -y, z + \frac{1}{2}), 12 : (y, x, z + \frac{1}{2}).$$

The lower SG is SG 36 when the preserved operations are: **(sub-SG label is 1) 1, 4, 11, 7.**

$$\text{The transformation is: } (\mathbf{a}_{36}, \mathbf{b}_{36}, \mathbf{c}_{36}) = (\mathbf{a}_{186}, \mathbf{b}_{186}, \mathbf{c}_{186}) \begin{pmatrix} 1 & -1 & 0 \\ 0 & -2 & 0 \\ 0 & 0 & -1 \end{pmatrix}, \overrightarrow{O_{186}O_{36}} = \mathbf{0}$$

The reduction of higher dimensional irrep:

$$C_{6v} : E_2 \rightarrow A_1 + A_2 \text{ of } C_{2v}.$$

$$C_{6v} : E_1 \rightarrow B_2 + B_1 \text{ of } C_{2v}.$$

The correspondences of irreps at HSPs from original SG to lowered SG:

$$n_{GM5}^{36} = n_{GM7}^{186} + n_{GM8}^{186} + n_{GM9}^{186} n_{Y5}^{36} = n_{M5}^{186} n_{S4}^{36} = n_{M5}^{186} n_{S3}^{36} = n_{M5}^{186} n_{Z5}^{36} = n_{A7}^{186} + n_{A8}^{186} + n_{A9}^{186} n_{T5}^{36} = n_{L5}^{186} n_{R4}^{36} = n_{L5}^{186} n_{R3}^{36} = n_{L5}^{186}$$

The lower SG is SG 36 when the preserved operations are: **(sub-SG label is 2) 1, 4, 9, 10.**

$$\text{The transformation is: } (\mathbf{a}_{36}, \mathbf{b}_{36}, \mathbf{c}_{36}) = (\mathbf{a}_{186}, \mathbf{b}_{186}, \mathbf{c}_{186}) \begin{pmatrix} 0 & 2 & 0 \\ 1 & 1 & 0 \\ 0 & 0 & -1 \end{pmatrix}, \overrightarrow{O_{186}O_{36}} = \mathbf{0}$$

The reduction of higher dimensional irrep:

$$C_{6v} : E_2 \rightarrow A_1 + A_2 \text{ of } C_{2v}.$$

$$C_{6v} : E_1 \rightarrow B_2 + B_1 \text{ of } C_{2v}.$$

The correspondences of irreps at HSPs from original SG to lowered SG:

$$n_{GM5}^{36} = n_{GM7}^{186} + n_{GM8}^{186} + n_{GM9}^{186} n_{Y5}^{36} = n_{M5}^{186} n_{S4}^{36} = n_{M5}^{186} n_{S3}^{36} = n_{M5}^{186} n_{Z5}^{36} = n_{A7}^{186} + n_{A8}^{186} + n_{A9}^{186} n_{T5}^{36} = n_{L5}^{186} n_{R4}^{36} = n_{L5}^{186} n_{R3}^{36} = n_{L5}^{186}$$

The lower SG is SG 36 when the preserved operations are: **(sub-SG label is 3) 1, 4, 12, 8.**

$$\text{The transformation is: } (\mathbf{a}_{36}, \mathbf{b}_{36}, \mathbf{c}_{36}) = (\mathbf{a}_{186}, \mathbf{b}_{186}, \mathbf{c}_{186}) \begin{pmatrix} 1 & 1 & 0 \\ 1 & -1 & 0 \\ 0 & 0 & -1 \end{pmatrix}, \overrightarrow{O_{186}O_{36}} = \mathbf{0}$$

The reduction of higher dimensional irrep:

$$C_{6v} : E_2 \rightarrow A_1 + A_2 \text{ of } C_{2v}.$$

$$C_{6v} : E_1 \rightarrow B_2 + B_1 \text{ of } C_{2v}.$$

The correspondences of irreps at HSPs from original SG to lowered SG:

$$n_{GM5}^{36} = n_{GM7}^{186} + n_{GM8}^{186} + n_{GM9}^{186} n_{Y5}^{36} = n_{M5}^{186} n_{S4}^{36} = n_{M5}^{186} n_{S3}^{36} = n_{M5}^{186} n_{Z5}^{36} = n_{A7}^{186} + n_{A8}^{186} + n_{A9}^{186} n_{T5}^{36} = n_{L5}^{186} n_{R4}^{36} = n_{L5}^{186} n_{R3}^{36} = n_{L5}^{186}$$

The lower SG is SG 173 when the preserved operations are: **(sub-SG label is 4) 1, 2, 6, 3, 5, 4.**

$$\text{The transformation is: } (\mathbf{a}_{173}, \mathbf{b}_{173}, \mathbf{c}_{173}) = (\mathbf{a}_{186}, \mathbf{b}_{186}, \mathbf{c}_{186}) \begin{pmatrix} 1 & -1 & 0 \\ 0 & -1 & 0 \\ 0 & 0 & -1 \end{pmatrix}, \overrightarrow{O_{186}O_{173}} = \mathbf{a}_{173} + \mathbf{b}_{173}$$

The reduction of higher dimensional irrep:

$$C_{6v} : E_2 \rightarrow {}^1E_2 + {}^2E_2 \text{ of } C_6.$$

$$C_{6v} : E_1 \rightarrow {}^2E_1 + {}^1E_1 \text{ of } C_6.$$

The correspondences of irreps at HSPs from original SG to lowered SG:

$$n_{GM9}^{173} = n_{GM8}^{186} n_{GM12}^{173} = n_{GM8}^{186} n_{GM8}^{173} = n_{GM7}^{186} n_{GM7}^{173} = n_{GM7}^{186} n_{GM11}^{173} = n_{GM9}^{186} n_{GM10}^{173} = n_{GM9}^{186} n_{M3}^{173} = n_{M5}^{186} n_{M4}^{173} = n_{M5}^{186} n_{K4}^{173} = n_{K4}^{186} + n_{K5}^{186} n_{K6}^{173} = n_{K6}^{186} n_{K5}^{173} = n_{K6}^{186} n_{A9}^{173} = n_{A9}^{186} n_{A12}^{173} = n_{A9}^{186} n_{A8}^{173} = n_{A7}^{186} n_{A7}^{173} = n_{A7}^{186} n_{A11}^{173} = n_{A8}^{186} n_{A10}^{173} = n_{A8}^{186} n_{L3}^{173} = n_{L5}^{186} n_{L4}^{173} = n_{L5}^{186} n_{H4}^{173} = n_{H4}^{186} + n_{H5}^{186} n_{H6}^{173} = n_{H6}^{186} n_{H5}^{173} = n_{H6}^{186}$$

#### 84. Lowered SGs by higher-dimensional irreps of pairings in SG 187

The representative operations of SG/T for SG 187:

$$1 : (x, y, z), 2 : (-y, x - y, z), 3 : (y - x, -x, z), 4 : (x, x - y, -z), 5 : (y - x, y, -z), 6 : (-y, -x, -z), 7 : (y - x, -x, -z), 8 : (x, y, -z), 9 : (-y, x - y, -z), 10 : (y - x, y, z), 11 : (-y, -x, z), 12 : (x, x - y, z).$$

The lower SG is SG 38 when the preserved operations are: **(sub-SG label is 1) 1, 5, 10, 8.**

$$\text{The transformation is: } (\mathbf{a}_{38}, \mathbf{b}_{38}, \mathbf{c}_{38}) = (\mathbf{a}_{187}, \mathbf{b}_{187}, \mathbf{c}_{187}) \begin{pmatrix} 0 & -1 & 1 \\ 0 & 0 & 2 \\ -1 & 0 & 0 \end{pmatrix}, \overrightarrow{O_{187}O_{38}} = \frac{1}{2}\mathbf{a}_{38}$$

The reduction of higher dimensional irrep:

$$D_{3h} : E' \rightarrow A_1 + B_2 \text{ of } C_{2v}.$$

$$D_{3h} : E'' \rightarrow A_2 + B_1 \text{ of } C_{2v}.$$

The correspondences of irreps at HSPs from original SG to lowered SG:

$$n_{GM5}^{38} = n_{GM7}^{187} + n_{GM8}^{187} + n_{GM9}^{187} n_{Y5}^{38} = n_{M5}^{187} n_{S3}^{38} = n_{M5}^{187} n_{S4}^{38} = n_{M5}^{187} n_{Z5}^{38} = n_{A7}^{187} + n_{A8}^{187} + n_{A9}^{187} n_{T5}^{38} = n_{L5}^{187} n_{R3}^{38} = n_{L5}^{187} n_{R4}^{38} = n_{L5}^{187}$$

The lower SG is SG 38 when the preserved operations are: **(sub-SG label is 2) 1, 4, 8, 12.**

$$\text{The transformation is: } (\mathbf{a}_{38}, \mathbf{b}_{38}, \mathbf{c}_{38}) = (\mathbf{a}_{187}, \mathbf{b}_{187}, \mathbf{c}_{187}) \begin{pmatrix} 0 & 0 & 2 \\ 0 & -1 & 1 \\ 1 & 0 & 0 \end{pmatrix}, \overrightarrow{O_{187}O_{38}} = \frac{1}{2}\mathbf{a}_{38}$$

The reduction of higher dimensional irrep:

$$D_{3h} : E' \rightarrow A_1 + B_2 \text{ of } C_{2v}.$$

$$D_{3h} : E'' \rightarrow A_2 + B_1 \text{ of } C_{2v}.$$

The correspondences of irreps at HSPs from original SG to lowered SG:

$$n_{GM5}^{38} = n_{GM7}^{187} + n_{GM8}^{187} + n_{GM9}^{187} n_{Y5}^{38} = n_{M5}^{187} n_{S3}^{38} = n_{M5}^{187} n_{S4}^{38} = n_{M5}^{187} n_{Z5}^{38} = n_{A7}^{187} + n_{A8}^{187} + n_{A9}^{187} n_{T5}^{38} = n_{L5}^{187} n_{R3}^{38} = n_{L5}^{187} n_{R4}^{38} = n_{L5}^{187}$$

The lower SG is SG 38 when the preserved operations are: **(sub-SG label is 3) 1, 6, 11, 8.**

$$\text{The transformation is: } (\mathbf{a}_{38}, \mathbf{b}_{38}, \mathbf{c}_{38}) = (\mathbf{a}_{187}, \mathbf{b}_{187}, \mathbf{c}_{187}) \begin{pmatrix} 0 & 1 & -1 \\ 0 & 1 & 1 \\ 1 & 0 & 0 \end{pmatrix}, \overrightarrow{O_{187}O_{38}} = \frac{1}{2}\mathbf{a}_{38}$$

The reduction of higher dimensional irrep:

$$D_{3h} : E' \rightarrow A_1 + B_2 \text{ of } C_{2v}.$$

$$D_{3h} : E'' \rightarrow A_2 + B_1 \text{ of } C_{2v}.$$

The correspondences of irreps at HSPs from original SG to lowered SG:

$$n_{GM5}^{38} = n_{GM7}^{187} + n_{GM8}^{187} + n_{GM9}^{187} n_{Y5}^{38} = n_{M5}^{187} n_{S3}^{38} = n_{M5}^{187} n_{S4}^{38} = n_{M5}^{187} n_{Z5}^{38} = n_{A7}^{187} + n_{A8}^{187} + n_{A9}^{187} n_{T5}^{38} = n_{L5}^{187} n_{R3}^{38} = n_{L5}^{187} n_{R4}^{38} = n_{L5}^{187}$$

$$n_{R4}^{38} = n_{L5}^{187}$$

The lower SG is SG 174 when the preserved operations are: **(sub-SG label is 4) 1, 7, 9, 2, 3, 8.**

$$\text{The transformation is: } (\mathbf{a}_{174}, \mathbf{b}_{174}, \mathbf{c}_{174}) = (\mathbf{a}_{187}, \mathbf{b}_{187}, \mathbf{c}_{187}) \begin{pmatrix} -1 & 1 & 0 \\ -1 & 0 & 0 \\ 0 & 0 & 1 \end{pmatrix}, \overrightarrow{O_{187}O_{174}} = \frac{1}{3}\mathbf{a}_{174} + \left(\frac{2}{3}\right)\mathbf{b}_{174} + \left(\frac{1}{2}\right)\mathbf{c}_{174}$$

The reduction of higher dimensional irrep:

$$D_{3h} : E' \rightarrow {}^1E' + {}^2E' \text{ of } C_{3h}.$$

$$D_{3h} : E'' \rightarrow {}^2E'' + {}^1E'' \text{ of } C_{3h}.$$

The correspondences of irreps at HSPs from original SG to lowered SG:

$$\begin{aligned} n_{GM8}^{174} &= n_{GM7}^{187} n_{GM7}^{174} = n_{GM7}^{187} n_{GM12}^{174} = n_{GM8}^{187} n_{GM11}^{174} = n_{GM9}^{187} n_{GM9}^{174} = n_{GM8}^{187} n_{GM10}^{174} = n_{GM9}^{187} n_{M3}^{174} = n_{M5}^{187} n_{M4}^{174} = \\ n_{M5}^{187} n_{K8}^{174} &= n_{K10}^{187} n_{K7}^{174} = n_{K9}^{187} n_{K12}^{174} = n_{K8}^{187} n_{K11}^{174} = n_{K7}^{187} n_{K9}^{174} = n_{K11}^{187} n_{K10}^{174} = n_{K12}^{187} n_{A8}^{174} = n_{A7}^{187} n_{A7}^{174} = n_{A7}^{187} n_{A12}^{174} = \\ n_{A9}^{187} n_{A11}^{174} &= n_{A8}^{187} n_{A9}^{174} = n_{A9}^{187} n_{A10}^{174} = n_{A8}^{187} n_{L3}^{174} = n_{L5}^{187} n_{L4}^{174} = n_{L5}^{187} n_{H8}^{174} = n_{H9}^{187} n_{H7}^{174} = n_{H10}^{187} n_{H12}^{174} = n_{H7}^{187} n_{H11}^{174} = n_{H8}^{187} \\ n_{H9}^{174} &= n_{H12}^{187} n_{H10}^{174} = n_{H11}^{187} \end{aligned}$$

### 85. Lowered SGs by higher-dimensional irreps of pairings in SG 188

The representative operations of SG/T for SG 188:

$$1 : (x, y, z), 2 : (-y, x - y, z), 3 : (y - x, -x, z), 4 : (x, x - y, -z), 5 : (y - x, y, -z), 6 : (-y, -x, -z), 7 : (y - x, -x, \frac{1}{2} - z), 8 : (x, y, \frac{1}{2} - z), 9 : (-y, x - y, \frac{1}{2} - z), 10 : (y - x, y, z + \frac{1}{2}), 11 : (-y, -x, z + \frac{1}{2}), 12 : (x, x - y, z + \frac{1}{2}).$$

The lower SG is SG 40 when the preserved operations are: **(sub-SG label is 1) 1, 5, 10, 8.**

$$\text{The transformation is: } (\mathbf{a}_{40}, \mathbf{b}_{40}, \mathbf{c}_{40}) = (\mathbf{a}_{188}, \mathbf{b}_{188}, \mathbf{c}_{188}) \begin{pmatrix} 0 & -1 & 1 \\ 0 & 0 & 2 \\ -1 & 0 & 0 \end{pmatrix}, \overrightarrow{O_{188}O_{40}} = \frac{1}{2}\mathbf{a}_{40}$$

The reduction of higher dimensional irrep:

$$D_{3h} : E' \rightarrow A_1 + B_2 \text{ of } C_{2v}.$$

$$D_{3h} : E'' \rightarrow A_2 + B_1 \text{ of } C_{2v}.$$

The correspondences of irreps at HSPs from original SG to lowered SG:

$$\begin{aligned} n_{GM5}^{40} &= n_{GM7}^{188} + n_{GM8}^{188} + n_{GM9}^{188} n_{Y5}^{40} = n_{M5}^{188} n_{S3}^{40} = n_{M5}^{188} n_{S4}^{40} = n_{M5}^{188} n_{Z3}^{40} = n_{A4}^{188} + n_{A8}^{188} n_{Z5}^{40} = n_{A7}^{188} + n_{A9}^{188} n_{Z2}^{40} = \\ n_{A5}^{188} + n_{A8}^{188} n_{Z4}^{40} &= n_{A6}^{188} + n_{A9}^{188} n_{T3}^{40} = n_{L4}^{188} n_{T5}^{40} = n_{L5}^{188} n_{T2}^{40} = n_{L4}^{188} n_{T4}^{40} = n_{L5}^{188} n_{R3}^{40} = n_{L2}^{188} + n_{L4}^{188} n_{R4}^{40} = n_{L3}^{188} + n_{L5}^{188} \end{aligned}$$

The lower SG is SG 40 when the preserved operations are: **(sub-SG label is 2) 1, 4, 8, 12.**

$$\text{The transformation is: } (\mathbf{a}_{40}, \mathbf{b}_{40}, \mathbf{c}_{40}) = (\mathbf{a}_{188}, \mathbf{b}_{188}, \mathbf{c}_{188}) \begin{pmatrix} 0 & 0 & 2 \\ 0 & -1 & 1 \\ 1 & 0 & 0 \end{pmatrix}, \overrightarrow{O_{188}O_{40}} = \frac{1}{2}\mathbf{a}_{40}$$

The reduction of higher dimensional irrep:

$$D_{3h} : E' \rightarrow A_1 + B_2 \text{ of } C_{2v}.$$

$$D_{3h} : E'' \rightarrow A_2 + B_1 \text{ of } C_{2v}.$$

The correspondences of irreps at HSPs from original SG to lowered SG:

$$\begin{aligned} n_{GM5}^{40} &= n_{GM7}^{188} + n_{GM8}^{188} + n_{GM9}^{188} n_{Y5}^{40} = n_{M5}^{188} n_{S3}^{40} = n_{M5}^{188} n_{S4}^{40} = n_{M5}^{188} n_{Z3}^{40} = n_{A5}^{188} + n_{A8}^{188} n_{Z5}^{40} = n_{A6}^{188} + n_{A9}^{188} n_{Z2}^{40} = \\ n_{A4}^{188} + n_{A8}^{188} n_{Z4}^{40} &= n_{A7}^{188} + n_{A9}^{188} n_{T3}^{40} = n_{L4}^{188} n_{T5}^{40} = n_{L5}^{188} n_{T2}^{40} = n_{L2}^{188} n_{T4}^{40} = n_{L3}^{188} n_{R3}^{40} = n_{L2}^{188} + n_{L4}^{188} n_{R4}^{40} = n_{L3}^{188} + n_{L5}^{188} \end{aligned}$$

The lower SG is SG 40 when the preserved operations are: **(sub-SG label is 3) 1, 6, 11, 8.**

$$\text{The transformation is: } (\mathbf{a}_{40}, \mathbf{b}_{40}, \mathbf{c}_{40}) = (\mathbf{a}_{188}, \mathbf{b}_{188}, \mathbf{c}_{188}) \begin{pmatrix} 0 & 1 & -1 \\ 0 & 1 & 1 \\ 1 & 0 & 0 \end{pmatrix}, \overrightarrow{O_{188}O_{40}} = \frac{1}{2}\mathbf{a}_{40}$$

The reduction of higher dimensional irrep:

$$D_{3h} : E' \rightarrow A_1 + B_2 \text{ of } C_{2v}.$$

$$D_{3h} : E'' \rightarrow A_2 + B_1 \text{ of } C_{2v}.$$

The correspondences of irreps at HSPs from original SG to lowered SG:

$$n_{GM5}^{40} = n_{GM7}^{188} + n_{GM8}^{188} + n_{GM9}^{188} n_{Y5}^{40} = n_{M5}^{188} n_{S3}^{40} = n_{M5}^{188} n_{S4}^{40} = n_{M5}^{188} n_{Z3}^{40} = n_{A5}^{188} + n_{A8}^{188} n_{Z5}^{40} = n_{A6}^{188} + n_{A9}^{188} n_{Z2}^{40} =$$

$$n_{A4}^{188} + n_{A8}^{188} n_{Z4}^{40} = n_{A7}^{188} + n_{A9}^{188} n_{T3}^{40} = n_{L4}^{188} n_{T5}^{40} = n_{L5}^{188} n_{T2}^{40} = n_{L2}^{188} n_{T4}^{40} = n_{L3}^{188} n_{R3}^{40} = n_{L2}^{188} + n_{L4}^{188} n_{R4}^{40} = n_{L3}^{188} + n_{L5}^{188}$$

The lower SG is SG 174 when the preserved operations are: **(sub-SG label is 4) 1, 7, 9, 2, 3, 8.**

$$\text{The transformation is: } (\mathbf{a}_{174}, \mathbf{b}_{174}, \mathbf{c}_{174}) = (\mathbf{a}_{188}, \mathbf{b}_{188}, \mathbf{c}_{188}) \begin{pmatrix} -1 & 1 & 0 \\ -1 & 0 & 0 \\ 0 & 0 & 1 \end{pmatrix}, \overrightarrow{O_{188}O_{174}} = \frac{1}{3}\mathbf{a}_{174} + \left(\frac{2}{3}\right)\mathbf{b}_{174} + \left(\frac{1}{4}\right)\mathbf{c}_{174}$$

The reduction of higher dimensional irrep:

$$D_{3h} : E' \rightarrow {}^1E' + {}^2E' \text{ of } C_{3h}.$$

$$D_{3h} : E'' \rightarrow {}^2E'' + {}^1E'' \text{ of } C_{3h}.$$

The correspondences of irreps at HSPs from original SG to lowered SG:

$$\begin{aligned} n_{GM8}^{174} &= n_{GM7}^{188} n_{GM7}^{174} = n_{GM7}^{188} n_{GM12}^{174} = n_{GM8}^{188} n_{GM11}^{174} = n_{GM9}^{188} n_{GM9}^{174} = n_{GM8}^{188} n_{GM10}^{174} = n_{GM9}^{188} n_{M3}^{174} = n_{M5}^{188} n_{M4}^{174} = n_{M5}^{188} \\ n_{K8}^{174} &= n_{K10}^{188} n_{K7}^{174} = n_{K9}^{188} n_{K12}^{174} = n_{K8}^{188} n_{K11}^{174} = n_{K7}^{188} n_{K9}^{174} = n_{K11}^{188} n_{K10}^{174} = n_{K12}^{188} n_{A8}^{174} = n_{A6}^{188} + n_{A7}^{188} n_{A7}^{174} = n_{A4}^{188} + n_{A5}^{188} \\ n_{A12}^{174} &= n_{A9}^{188} n_{A11}^{174} = n_{A8}^{188} n_{A9}^{174} = n_{A8}^{188} n_{A10}^{174} = n_{A9}^{188} n_{L3}^{174} = n_{L2}^{188} + n_{L4}^{188} n_{L4}^{174} = n_{L3}^{188} + n_{L5}^{188} n_{H8}^{174} = n_{H10}^{188} n_{H7}^{174} = n_{H9}^{188} \\ n_{H12}^{174} &= n_{H8}^{188} n_{H11}^{174} = n_{H7}^{188} n_{H9}^{174} = n_{H11}^{188} n_{H10}^{174} = n_{H12}^{188} \end{aligned}$$

### 86. Lowered SGs by higher-dimensional irreps of pairings in SG 189

The representative operations of SG/T for SG 189:

$$1 : (x, y, z), 2 : (-y, x - y, z), 3 : (y - x, -x, z), 4 : (x - y, -y, -z), 5 : (y, x, -z), 6 : (-x, y - x, -z), 7 : (y - x, -x, -z), 8 : (x, y, -z), 9 : (-y, x - y, -z), 10 : (-x, y - x, z), 11 : (x - y, -y, z), 12 : (y, x, z).$$

The lower SG is SG 38 when the preserved operations are: **(sub-SG label is 1) 1, 4, 8, 11.**

$$\text{The transformation is: } (\mathbf{a}_{38}, \mathbf{b}_{38}, \mathbf{c}_{38}) = (\mathbf{a}_{189}, \mathbf{b}_{189}, \mathbf{c}_{189}) \begin{pmatrix} 0 & 1 & -1 \\ 0 & 2 & 0 \\ 1 & 0 & 0 \end{pmatrix}, \overrightarrow{O_{189}O_{38}} = \frac{1}{2}\mathbf{a}_{38}$$

The reduction of higher dimensional irrep:

$$D_{3h} : E' \rightarrow A_1 + B_2 \text{ of } C_{2v}.$$

$$D_{3h} : E'' \rightarrow A_2 + B_1 \text{ of } C_{2v}.$$

The correspondences of irreps at HSPs from original SG to lowered SG:

$$\begin{aligned} n_{GM5}^{38} &= n_{GM7}^{189} + n_{GM8}^{189} + n_{GM9}^{189} n_{Y5}^{38} = n_{M5}^{189} n_{S3}^{38} = n_{M5}^{189} n_{S4}^{38} = n_{M5}^{189} n_{Z5}^{38} = n_{A7}^{189} + n_{A8}^{189} + n_{A9}^{189} n_{T5}^{38} = n_{L5}^{189} n_{R3}^{38} = n_{L5}^{189} \\ n_{R4}^{38} &= n_{L5}^{189} \end{aligned}$$

The lower SG is SG 38 when the preserved operations are: **(sub-SG label is 2) 1, 6, 10, 8.**

$$\text{The transformation is: } (\mathbf{a}_{38}, \mathbf{b}_{38}, \mathbf{c}_{38}) = (\mathbf{a}_{189}, \mathbf{b}_{189}, \mathbf{c}_{189}) \begin{pmatrix} 0 & 2 & 0 \\ 0 & 1 & 1 \\ 1 & 0 & 0 \end{pmatrix}, \overrightarrow{O_{189}O_{38}} = \frac{1}{2}\mathbf{a}_{38}$$

The reduction of higher dimensional irrep:

$$D_{3h} : E' \rightarrow A_1 + B_2 \text{ of } C_{2v}.$$

$$D_{3h} : E'' \rightarrow A_2 + B_1 \text{ of } C_{2v}.$$

The correspondences of irreps at HSPs from original SG to lowered SG:

$$\begin{aligned} n_{GM5}^{38} &= n_{GM7}^{189} + n_{GM8}^{189} + n_{GM9}^{189} n_{Y5}^{38} = n_{M5}^{189} n_{S3}^{38} = n_{M5}^{189} n_{S4}^{38} = n_{M5}^{189} n_{Z5}^{38} = n_{A7}^{189} + n_{A8}^{189} + n_{A9}^{189} n_{T5}^{38} = n_{L5}^{189} n_{R3}^{38} = n_{L5}^{189} \\ n_{R4}^{38} &= n_{L5}^{189} \end{aligned}$$

The lower SG is SG 38 when the preserved operations are: **(sub-SG label is 3) 1, 5, 8, 12.**

$$\text{The transformation is: } (\mathbf{a}_{38}, \mathbf{b}_{38}, \mathbf{c}_{38}) = (\mathbf{a}_{189}, \mathbf{b}_{189}, \mathbf{c}_{189}) \begin{pmatrix} 0 & 1 & 1 \\ 0 & -1 & 1 \\ 1 & 0 & 0 \end{pmatrix}, \overrightarrow{O_{189}O_{38}} = \frac{1}{2}\mathbf{a}_{38}$$

The reduction of higher dimensional irrep:

$$D_{3h} : E' \rightarrow A_1 + B_2 \text{ of } C_{2v}.$$

$$D_{3h} : E'' \rightarrow A_2 + B_1 \text{ of } C_{2v}.$$

The correspondences of irreps at HSPs from original SG to lowered SG:

$$n_{GM5}^{38} = n_{GM7}^{189} + n_{GM8}^{189} + n_{GM9}^{189} n_{Y5}^{38} = n_{M5}^{189} n_{S3}^{38} = n_{M5}^{189} n_{S4}^{38} = n_{M5}^{189} n_{Z5}^{38} = n_{A7}^{189} + n_{A8}^{189} + n_{A9}^{189} n_{T5}^{38} = n_{L5}^{189} n_{R3}^{38} = n_{L5}^{189}$$

$$n_{R4}^{38} = n_{L5}^{189}$$

The lower SG is SG 174 when the preserved operations are: **(sub-SG label is 4) 1, 7, 9, 2, 3, 8.**

$$\text{The transformation is: } (\mathbf{a}_{174}, \mathbf{b}_{174}, \mathbf{c}_{174}) = (\mathbf{a}_{189}, \mathbf{b}_{189}, \mathbf{c}_{189}) \begin{pmatrix} -1 & 1 & 0 \\ -1 & 0 & 0 \\ 0 & 0 & 1 \end{pmatrix}, \overrightarrow{O_{189}O_{174}} = \frac{1}{3}\mathbf{a}_{174} + \left(\frac{2}{3}\right)\mathbf{b}_{174} + \left(\frac{1}{2}\right)\mathbf{c}_{174}$$

The reduction of higher dimensional irrep:

$$D_{3h} : E' \rightarrow {}^1E' + {}^2E' \text{ of } C_{3h}.$$

$$D_{3h} : E'' \rightarrow {}^2E'' + {}^1E'' \text{ of } C_{3h}.$$

The correspondences of irreps at HSPs from original SG to lowered SG:

$$\begin{aligned} n_{GM8}^{174} &= n_{GM7}^{189} n_{GM7}^{174} = n_{GM7}^{189} n_{GM12}^{174} = n_{GM8}^{189} n_{GM11}^{174} = n_{GM9}^{189} n_{GM9}^{174} = n_{GM8}^{189} n_{GM10}^{174} = n_{GM9}^{189} n_{M3}^{174} = n_{M5}^{189} n_{M4}^{174} = \\ n_{M5}^{189} n_{K8}^{174} &= n_{K9}^{189} n_{K7}^{174} = n_{K8}^{189} n_{K12}^{174} = n_{K7}^{189} n_{K11}^{174} = n_{K9}^{189} n_{K10}^{174} = n_{K8}^{189} n_{A8}^{174} = n_{A7}^{189} n_{A7}^{174} = n_{A7}^{189} n_{A12}^{174} = n_{A9}^{189} n_{A11}^{174} = n_{A8}^{189} n_{A9}^{174} = n_{A9}^{189} n_{A10}^{174} = n_{A8}^{189} n_{L3}^{174} = n_{L5}^{189} n_{L4}^{174} = n_{L5}^{189} n_{H8}^{174} = n_{H8}^{189} n_{H7}^{174} = n_{H9}^{189} n_{H12}^{174} = n_{H7}^{189} n_{H11}^{174} = n_{H7}^{189} n_{H9}^{174} = \\ n_{H8}^{189} n_{H10}^{174} &= n_{H9}^{189} \end{aligned}$$

### 87. Lowered SGs by higher-dimensional irreps of pairings in SG 190

The representative operations of SG/T for SG 190:

$$\begin{aligned} 1 : (x, y, z), 2 : (-y, x - y, z), 3 : (y - x, -x, z), 4 : (x - y, -y, -z), 5 : (y, x, -z), 6 : (-x, y - x, -z), 7 : \\ (y - x, -x, \frac{1}{2} - z), 8 : (x, y, \frac{1}{2} - z), 9 : (-y, x - y, \frac{1}{2} - z), 10 : (-x, y - x, z + \frac{1}{2}), 11 : (x - y, -y, z + \frac{1}{2}), \\ 12 : (y, x, z + \frac{1}{2}). \end{aligned}$$

The lower SG is SG 40 when the preserved operations are: **(sub-SG label is 1) 1, 4, 8, 11.**

$$\text{The transformation is: } (\mathbf{a}_{40}, \mathbf{b}_{40}, \mathbf{c}_{40}) = (\mathbf{a}_{190}, \mathbf{b}_{190}, \mathbf{c}_{190}) \begin{pmatrix} 0 & 1 & -1 \\ 0 & 2 & 0 \\ 1 & 0 & 0 \end{pmatrix}, \overrightarrow{O_{190}O_{40}} = \frac{1}{2}\mathbf{a}_{40}$$

The reduction of higher dimensional irrep:

$$D_{3h} : E' \rightarrow A_1 + B_2 \text{ of } C_{2v}.$$

$$D_{3h} : E'' \rightarrow A_2 + B_1 \text{ of } C_{2v}.$$

The correspondences of irreps at HSPs from original SG to lowered SG:

$$\begin{aligned} n_{GM5}^{40} &= n_{GM7}^{190} + n_{GM8}^{190} + n_{GM9}^{190} n_{Y5}^{40} = n_{M5}^{190} n_{S3}^{40} = n_{M5}^{190} n_{S4}^{40} = n_{M5}^{190} n_{Z3}^{40} = n_{A4}^{190} + n_{A8}^{190} n_{Z5}^{40} = n_{A6}^{190} + n_{A9}^{190} n_{Z2}^{40} = \\ n_{A5}^{190} + n_{A8}^{190} n_{Z4}^{40} &= n_{A6}^{190} + n_{A9}^{190} n_{T3}^{40} = n_{L2}^{190} n_{T5}^{40} = n_{L5}^{190} n_{T2}^{40} = n_{L4}^{190} n_{T4}^{40} = n_{L3}^{190} n_{R3}^{40} = n_{L2}^{190} + n_{L4}^{190} n_{R4}^{40} = n_{L3}^{190} + n_{L5}^{190} \end{aligned}$$

The lower SG is SG 40 when the preserved operations are: **(sub-SG label is 2) 1, 6, 10, 8.**

$$\text{The transformation is: } (\mathbf{a}_{40}, \mathbf{b}_{40}, \mathbf{c}_{40}) = (\mathbf{a}_{190}, \mathbf{b}_{190}, \mathbf{c}_{190}) \begin{pmatrix} 0 & 2 & 0 \\ 0 & 1 & 1 \\ 1 & 0 & 0 \end{pmatrix}, \overrightarrow{O_{190}O_{40}} = \frac{1}{2}\mathbf{a}_{40}$$

The reduction of higher dimensional irrep:

$$D_{3h} : E' \rightarrow A_1 + B_2 \text{ of } C_{2v}.$$

$$D_{3h} : E'' \rightarrow A_2 + B_1 \text{ of } C_{2v}.$$

The correspondences of irreps at HSPs from original SG to lowered SG:

$$\begin{aligned} n_{GM5}^{40} &= n_{GM7}^{190} + n_{GM8}^{190} + n_{GM9}^{190} n_{Y5}^{40} = n_{M5}^{190} n_{S3}^{40} = n_{M5}^{190} n_{S4}^{40} = n_{M5}^{190} n_{Z3}^{40} = n_{A5}^{190} + n_{A8}^{190} n_{Z5}^{40} = n_{A7}^{190} + n_{A9}^{190} n_{Z2}^{40} = \\ n_{A4}^{190} + n_{A8}^{190} n_{Z4}^{40} &= n_{A6}^{190} + n_{A9}^{190} n_{T3}^{40} = n_{L2}^{190} n_{T5}^{40} = n_{L5}^{190} n_{T2}^{40} = n_{L4}^{190} n_{T4}^{40} = n_{L3}^{190} n_{R3}^{40} = n_{L2}^{190} + n_{L4}^{190} n_{R4}^{40} = n_{L3}^{190} + n_{L5}^{190} \end{aligned}$$

The lower SG is SG 40 when the preserved operations are: **(sub-SG label is 3) 1, 5, 8, 12.**

$$\text{The transformation is: } (\mathbf{a}_{40}, \mathbf{b}_{40}, \mathbf{c}_{40}) = (\mathbf{a}_{190}, \mathbf{b}_{190}, \mathbf{c}_{190}) \begin{pmatrix} 0 & 1 & 1 \\ 0 & -1 & 1 \\ 1 & 0 & 0 \end{pmatrix}, \overrightarrow{O_{190}O_{40}} = \frac{1}{2}\mathbf{a}_{40}$$

The reduction of higher dimensional irrep:

$$D_{3h} : E' \rightarrow A_1 + B_2 \text{ of } C_{2v}.$$

$$D_{3h} : E'' \rightarrow A_2 + B_1 \text{ of } C_{2v}.$$

The correspondences of irreps at HSPs from original SG to lowered SG:

$$\begin{aligned} n_{GM5}^{40} &= n_{GM7}^{190} + n_{GM8}^{190} + n_{GM9}^{190} & n_{Y5}^{40} &= n_{M5}^{190} & n_{S3}^{40} &= n_{M5}^{190} & n_{S4}^{40} &= n_{M5}^{190} & n_{Z3}^{40} &= n_{A4}^{190} + n_{A8}^{190} & n_{Z5}^{40} &= n_{A6}^{190} + n_{A9}^{190} & n_{Z2}^{40} &= \\ n_{A5}^{190} + n_{A8}^{190} & n_{Z4}^{40} &= n_{A7}^{190} + n_{A9}^{190} & n_{T3}^{40} &= n_{L4}^{190} & n_{T5}^{40} &= n_{L3}^{190} & n_{T2}^{40} &= n_{L2}^{190} & n_{T4}^{40} &= n_{L5}^{190} & n_{R3}^{40} &= n_{L2}^{190} + n_{L4}^{190} & n_{R4}^{40} &= n_{L3}^{190} + n_{L5}^{190} \end{aligned}$$

The lower SG is SG 174 when the preserved operations are: (**sub-SG label is 4**) 1, 7, 9, 2, 3, 8.

The transformation is:  $(\mathbf{a}_{174}, \mathbf{b}_{174}, \mathbf{c}_{174}) = (\mathbf{a}_{190}, \mathbf{b}_{190}, \mathbf{c}_{190}) \begin{pmatrix} -1 & 1 & 0 \\ -1 & 0 & 0 \\ 0 & 0 & 1 \end{pmatrix}, \overrightarrow{O_{190}O_{174}} = \frac{1}{3}\mathbf{a}_{174} + (\frac{2}{3})\mathbf{b}_{174} + (\frac{1}{4})\mathbf{c}_{174}$

The reduction of higher dimensional irrep:

$$D_{3h} : E' \rightarrow {}^1E' + {}^2E' \text{ of } C_{3h}.$$

$$D_{3h} : E'' \rightarrow {}^2E'' + {}^1E'' \text{ of } C_{3h}.$$

The correspondences of irreps at HSPs from original SG to lowered SG:

$$\begin{aligned} n_{GM8}^{174} &= n_{GM7}^{190} & n_{GM7}^{174} &= n_{GM7}^{190} & n_{GM12}^{174} &= n_{GM8}^{190} & n_{GM11}^{174} &= n_{GM9}^{190} & n_{GM9}^{174} &= n_{GM8}^{190} & n_{GM10}^{174} &= n_{GM9}^{190} & n_{M3}^{174} &= n_{M5}^{190} & n_{M4}^{174} &= n_{M5}^{190} \\ n_{K8}^{174} &= n_{K9}^{190} & n_{K7}^{174} &= n_{K8}^{190} & n_{K12}^{174} &= n_{K7}^{190} & n_{K11}^{174} &= n_{K7}^{190} & n_{K9}^{174} &= n_{K9}^{190} & n_{K10}^{174} &= n_{K8}^{190} & n_{A6}^{174} &= n_{A6}^{190} + n_{A7}^{190} & n_{A7}^{174} &= n_{A4}^{190} + n_{A5}^{190} \\ n_{A12}^{174} &= n_{A9}^{190} & n_{A11}^{174} &= n_{A8}^{190} & n_{A9}^{174} &= n_{A8}^{190} & n_{A10}^{174} &= n_{A9}^{190} & n_{L3}^{174} &= n_{L2}^{190} + n_{L4}^{190} & n_{L4}^{174} &= n_{L3}^{190} + n_{L5}^{190} & n_{H8}^{174} &= n_{H9}^{190} & n_{H7}^{174} &= n_{H8}^{190} \\ n_{H12}^{174} &= n_{H6}^{190} + n_{H7}^{190} & n_{H11}^{174} &= n_{H4}^{190} + n_{H5}^{190} & n_{H9}^{174} &= n_{H8}^{190} & n_{H10}^{174} &= n_{H9}^{190} \end{aligned}$$

### 88. Lowered SGs by higher-dimensional irreps of pairings in SG 191

The representative operations of SG/T for SG 191:

$$\begin{aligned} &1 : (x, y, z), 2 : (x - y, x, z), 3 : (-y, x - y, z), 4 : (-x, -y, z), 5 : (y - x, -x, z), 6 : (y, y - x, z), 7 : (x - y, -y, -z), \\ &8 : (y, x, -z), 9 : (-x, y - x, -z), 10 : (x, x - y, -z), 11 : (y - x, y, -z), 12 : (-y, -x, -z), 13 : (-x, -y, -z), \\ &14 : (y - x, -x, -z), 15 : (y, y - x, -z), 16 : (x, y, -z), 17 : (x - y, x, -z), 18 : (-y, x - y, -z), 19 : (y - x, y, z), \\ &20 : (-y, -x, z), 21 : (x, x - y, z), 22 : (-x, y - x, z), 23 : (x - y, -y, z), 24 : (y, x, z). \end{aligned}$$

The lower SG is SG 65 when the preserved operations are: (**sub-SG label is 1**) 1, 4, 11, 7, 13, 16, 23, 19.

The transformation is:  $(\mathbf{a}_{65}, \mathbf{b}_{65}, \mathbf{c}_{65}) = (\mathbf{a}_{191}, \mathbf{b}_{191}, \mathbf{c}_{191}) \begin{pmatrix} 1 & -1 & 0 \\ 2 & 0 & 0 \\ 0 & 0 & 1 \end{pmatrix}, \overrightarrow{O_{191}O_{65}} = \frac{1}{2}\mathbf{c}_{65}$

The reduction of higher dimensional irrep:

$$D_{6h} : E_{2g} \rightarrow A_g + B_{1g} \text{ of } D_{2h}.$$

$$D_{6h} : E_{1g} \rightarrow B_{2g} + B_{3g} \text{ of } D_{2h}.$$

$$D_{6h} : E_{2u} \rightarrow A_u + B_{1u} \text{ of } D_{2h}.$$

$$D_{6h} : E_{1u} \rightarrow B_{2u} + B_{3u} \text{ of } D_{2h}.$$

The correspondences of irreps at HSPs from original SG to lowered SG:

$$\begin{aligned} n_{GM6}^{65} &= n_{GM10}^{191} + n_{GM11}^{191} + n_{GM12}^{191} & n_{GM5}^{65} &= n_{GM7}^{191} + n_{GM8}^{191} + n_{GM9}^{191} & n_{Y6}^{65} &= n_{M6}^{191} & n_{Y5}^{65} &= n_{M5}^{191} & n_{S6}^{65} &= n_{M6}^{191} & n_{S4}^{65} &= n_{M5}^{191} \\ n_{S5}^{65} &= n_{M6}^{191} & n_{S3}^{65} &= n_{M5}^{191} & n_{Z6}^{65} &= n_{A7}^{191} + n_{A8}^{191} + n_{A9}^{191} & n_{Z5}^{65} &= n_{A10}^{191} + n_{A11}^{191} + n_{A12}^{191} & n_{T6}^{65} &= n_{L5}^{191} & n_{T5}^{65} &= n_{L6}^{191} & n_{R6}^{65} &= n_{L5}^{191} & n_{R4}^{65} &= \\ n_{L6}^{191} & n_{R5}^{65} &= n_{L5}^{191} & n_{R3}^{65} &= n_{L6}^{191} \end{aligned}$$

The lower SG is SG 65 when the preserved operations are: (**sub-SG label is 2**) 1, 4, 9, 10, 13, 16, 21, 22.

The transformation is:  $(\mathbf{a}_{65}, \mathbf{b}_{65}, \mathbf{c}_{65}) = (\mathbf{a}_{191}, \mathbf{b}_{191}, \mathbf{c}_{191}) \begin{pmatrix} 0 & -2 & 0 \\ 1 & -1 & 0 \\ 0 & 0 & 1 \end{pmatrix}, \overrightarrow{O_{191}O_{65}} = \frac{1}{2}\mathbf{c}_{65}$

The reduction of higher dimensional irrep:

$$D_{6h} : E_{2g} \rightarrow A_g + B_{1g} \text{ of } D_{2h}.$$

$$D_{6h} : E_{1g} \rightarrow B_{2g} + B_{3g} \text{ of } D_{2h}.$$

$$D_{6h} : E_{2u} \rightarrow A_u + B_{1u} \text{ of } D_{2h}.$$

$$D_{6h} : E_{1u} \rightarrow B_{2u} + B_{3u} \text{ of } D_{2h}.$$

The correspondences of irreps at HSPs from original SG to lowered SG:

$$\begin{aligned} n_{GM6}^{65} &= n_{GM10}^{191} + n_{GM11}^{191} + n_{GM12}^{191} & n_{GM5}^{65} &= n_{GM7}^{191} + n_{GM8}^{191} + n_{GM9}^{191} & n_{Y6}^{65} &= n_{M6}^{191} & n_{Y5}^{65} &= n_{M5}^{191} & n_{S6}^{65} &= n_{M6}^{191} & n_{S4}^{65} &= n_{M5}^{191} \\ n_{S5}^{65} &= n_{M6}^{191} & n_{S3}^{65} &= n_{M5}^{191} & n_{Z6}^{65} &= n_{A7}^{191} + n_{A8}^{191} + n_{A9}^{191} & n_{Z5}^{65} &= n_{A10}^{191} + n_{A11}^{191} + n_{A12}^{191} & n_{T6}^{65} &= n_{L5}^{191} & n_{T5}^{65} &= n_{L6}^{191} & n_{R6}^{65} &= n_{L5}^{191} & n_{R4}^{65} &= \\ n_{L6}^{191} & n_{R5}^{65} &= n_{L5}^{191} & n_{R3}^{65} &= n_{L6}^{191} \end{aligned}$$

The lower SG is SG 65 when the preserved operations are: **(sub-SG label is 3)** 1, 4, 12, 8, 13, 16, 24, 20.

The transformation is:  $(\mathbf{a}_{65}, \mathbf{b}_{65}, \mathbf{c}_{65}) = (\mathbf{a}_{191}, \mathbf{b}_{191}, \mathbf{c}_{191}) \begin{pmatrix} -1 & -1 & 0 \\ 1 & -1 & 0 \\ 0 & 0 & 1 \end{pmatrix}, \overrightarrow{O_{191}O_{65}} = \frac{1}{2}\mathbf{c}_{65}$

The reduction of higher dimensional irrep:

$$D_{6h} : E_{2g} \rightarrow A_g + B_{1g} \text{ of } D_{2h}.$$

$$D_{6h} : E_{1g} \rightarrow B_{2g} + B_{3g} \text{ of } D_{2h}.$$

$$D_{6h} : E_{2u} \rightarrow A_u + B_{1u} \text{ of } D_{2h}.$$

$$D_{6h} : E_{1u} \rightarrow B_{2u} + B_{3u} \text{ of } D_{2h}.$$

The correspondences of irreps at HSPs from original SG to lowered SG:

$$\begin{aligned} n_{GM6}^{65} &= n_{GM10}^{191} + n_{GM11}^{191} + n_{GM12}^{191} & n_{GM5}^{65} &= n_{GM7}^{191} + n_{GM8}^{191} + n_{GM9}^{191} & n_{Y6}^{65} &= n_{M6}^{191} & n_{Y5}^{65} &= n_{M5}^{191} & n_{S6}^{65} &= n_{M6}^{191} & n_{S4}^{65} &= n_{M5}^{191} \\ n_{S5}^{65} &= n_{M6}^{191} & n_{S3}^{65} &= n_{M5}^{191} & n_{Z6}^{65} &= n_{A7}^{191} + n_{A8}^{191} + n_{A9}^{191} & n_{Z5}^{65} &= n_{A10}^{191} + n_{A11}^{191} + n_{A12}^{191} & n_{T6}^{65} &= n_{L5}^{191} & n_{T5}^{65} &= n_{L6}^{191} & n_{R6}^{65} &= n_{L5}^{191} & n_{R4}^{65} &= n_{L5}^{191} \\ n_{L6}^{191} & n_{R5}^{65} &= n_{L5}^{191} & n_{R3}^{65} &= n_{L6}^{191} \end{aligned}$$

The lower SG is SG 175 when the preserved operations are: **(sub-SG label is 4)** 1, 2, 6, 3, 5, 4, 13, 14, 18, 15, 17, 16.

The transformation is:  $(\mathbf{a}_{175}, \mathbf{b}_{175}, \mathbf{c}_{175}) = (\mathbf{a}_{191}, \mathbf{b}_{191}, \mathbf{c}_{191}) \begin{pmatrix} -1 & 1 & 0 \\ -1 & 0 & 0 \\ 0 & 0 & 1 \end{pmatrix}, \overrightarrow{O_{191}O_{175}} = \frac{1}{2}\mathbf{c}_{175}$

The reduction of higher dimensional irrep:

$$D_{6h} : E_{2g} \rightarrow {}^2E_{2g} + {}^1E_{2g} \text{ of } C_{6h}.$$

$$D_{6h} : E_{1g} \rightarrow {}^2E_{1g} + {}^1E_{1g} \text{ of } C_{6h}.$$

$$D_{6h} : E_{2u} \rightarrow {}^2E_{2u} + {}^1E_{2u} \text{ of } C_{6h}.$$

$$D_{6h} : E_{1u} \rightarrow {}^2E_{1u} + {}^1E_{1u} \text{ of } C_{6h}.$$

The correspondences of irreps at HSPs from original SG to lowered SG:

$$\begin{aligned} n_{GM15}^{175} &= n_{GM11}^{191} & n_{GM9}^{175} &= n_{GM8}^{191} & n_{GM18}^{175} &= n_{GM11}^{191} & n_{GM12}^{175} &= n_{GM8}^{191} & n_{GM14}^{175} &= n_{GM10}^{191} & n_{GM8}^{175} &= n_{GM7}^{191} & n_{GM13}^{175} &= n_{GM10}^{191} \\ n_{GM7}^{175} &= n_{GM7}^{191} & n_{GM17}^{175} &= n_{GM12}^{191} & n_{GM11}^{175} &= n_{GM9}^{191} & n_{GM16}^{175} &= n_{GM12}^{191} & n_{GM10}^{175} &= n_{GM9}^{191} & n_{M5}^{175} &= n_{M6}^{191} & n_{M3}^{175} &= n_{M5}^{191} & n_{M6}^{175} &= n_{M6}^{191} \\ n_{M6}^{191} & n_{M4}^{175} &= n_{M5}^{191} & n_{K8}^{175} &= n_{K7}^{191} & n_{K7}^{175} &= n_{K7}^{191} & n_{K12}^{175} &= n_{K8}^{191} & n_{K11}^{175} &= n_{K9}^{191} & n_{K9}^{175} &= n_{K8}^{191} & n_{K10}^{175} &= n_{K9}^{191} & n_{A15}^{175} &= n_{A8}^{191} & n_{A9}^{175} &= n_{A11}^{191} \\ n_{A18}^{175} &= n_{A8}^{191} & n_{A12}^{175} &= n_{A11}^{191} & n_{A14}^{175} &= n_{A7}^{191} & n_{A8}^{175} &= n_{A10}^{191} & n_{A13}^{175} &= n_{A7}^{191} & n_{A7}^{175} &= n_{A10}^{191} & n_{A17}^{175} &= n_{A9}^{191} & n_{A11}^{175} &= n_{A12}^{191} & n_{A16}^{175} &= n_{A9}^{191} \\ n_{A10}^{175} &= n_{A12}^{191} & n_{L5}^{175} &= n_{L5}^{191} & n_{L3}^{175} &= n_{L6}^{191} & n_{L6}^{175} &= n_{L5}^{191} & n_{L4}^{175} &= n_{L6}^{191} & n_{H8}^{175} &= n_{H7}^{191} & n_{H7}^{175} &= n_{H7}^{191} & n_{H12}^{175} &= n_{H9}^{191} & n_{H11}^{175} &= n_{H8}^{191} & n_{H9}^{175} &= n_{H9}^{191} \\ n_{H9}^{191} & n_{H10}^{175} &= n_{H8}^{191} \end{aligned}$$

### 89. Lowered SGs by higher-dimensional irreps of pairings in SG 192

The representative operations of SG/T for SG 192:

$$\begin{aligned} &1 : (x, y, z), 2 : (x-y, x, z), 3 : (-y, x-y, z), 4 : (-x, -y, z), 5 : (y-x, -x, z), 6 : (y, y-x, z), 7 : (x-y, -y, \frac{1}{2}-z), \\ &8 : (y, x, \frac{1}{2}-z), 9 : (-x, y-x, \frac{1}{2}-z), 10 : (x, x-y, \frac{1}{2}-z), 11 : (y-x, y, \frac{1}{2}-z), 12 : (-y, -x, \frac{1}{2}-z), 13 : (-x, -y, -z), \\ &14 : (y-x, -x, -z), 15 : (y, y-x, -z), 16 : (x, y, -z), 17 : (x-y, x, -z), 18 : (-y, x-y, -z), 19 : (y-x, y, z + \frac{1}{2}), \\ &20 : (-y, -x, z + \frac{1}{2}), 21 : (x, x-y, z + \frac{1}{2}), 22 : (-x, y-x, z + \frac{1}{2}), 23 : (x-y, -y, z + \frac{1}{2}), 24 : (y, x, z + \frac{1}{2}). \end{aligned}$$

The lower SG is SG 66 when the preserved operations are: **(sub-SG label is 1)** 1, 4, 11, 7, 13, 16, 23, 19.

The transformation is:  $(\mathbf{a}_{66}, \mathbf{b}_{66}, \mathbf{c}_{66}) = (\mathbf{a}_{192}, \mathbf{b}_{192}, \mathbf{c}_{192}) \begin{pmatrix} 1 & -1 & 0 \\ 2 & 0 & 0 \\ 0 & 0 & 1 \end{pmatrix}, \overrightarrow{O_{192}O_{66}} = \frac{1}{2}\mathbf{c}_{66}$

The reduction of higher dimensional irrep:

$$D_{6h} : E_{2g} \rightarrow A_g + B_{1g} \text{ of } D_{2h}.$$

$$D_{6h} : E_{1g} \rightarrow B_{2g} + B_{3g} \text{ of } D_{2h}.$$

$$D_{6h} : E_{2u} \rightarrow A_u + B_{1u} \text{ of } D_{2h}.$$

$$D_{6h} : E_{1u} \rightarrow B_{2u} + B_{3u} \text{ of } D_{2h}.$$

The correspondences of irreps at HSPs from original SG to lowered SG:

$$n_{GM6}^{66} = n_{GM10}^{192} + n_{GM11}^{192} + n_{GM12}^{192} \quad n_{GM5}^{66} = n_{GM7}^{192} + n_{GM8}^{192} + n_{GM9}^{192} \quad n_{Y6}^{66} = n_{M6}^{192} \quad n_{Y5}^{66} = n_{M5}^{192} \quad n_{S6}^{66} = n_{M6}^{192} \quad n_{S4}^{66} = n_{M5}^{192}$$

$$n_{S5}^{66} = n_{M6}^{192} n_{S3}^{66} = n_{M5}^{192} n_{Z4}^{66} = n_{A10}^{192} + n_{A11}^{192} + n_{A12}^{192} n_{Z3}^{66} = n_{A7}^{192} + n_{A8}^{192} + n_{A9}^{192} n_{T4}^{66} = n_{L4}^{192} n_{T3}^{66} = n_{L3}^{192} n_{R6}^{66} = n_{L3}^{192} n_{R4}^{66} =$$

$$n_{L4}^{192} n_{R5}^{66} = n_{L4}^{192} n_{R3}^{66} = n_{L3}^{192}$$

The lower SG is SG 66 when the preserved operations are: **(sub-SG label is 2) 1, 4, 9, 10, 13, 16, 21, 22.**

$$\text{The transformation is: } (\mathbf{a}_{66}, \mathbf{b}_{66}, \mathbf{c}_{66}) = (\mathbf{a}_{192}, \mathbf{b}_{192}, \mathbf{c}_{192}) \begin{pmatrix} 0 & -2 & 0 \\ 1 & -1 & 0 \\ 0 & 0 & 1 \end{pmatrix}, \overrightarrow{O_{192}O_{66}} = \frac{1}{2}\mathbf{c}_{66}$$

The reduction of higher dimensional irrep:

$$D_{6h} : E_{2g} \rightarrow A_g + B_{1g} \text{ of } D_{2h}.$$

$$D_{6h} : E_{1g} \rightarrow B_{2g} + B_{3g} \text{ of } D_{2h}.$$

$$D_{6h} : E_{2u} \rightarrow A_u + B_{1u} \text{ of } D_{2h}.$$

$$D_{6h} : E_{1u} \rightarrow B_{2u} + B_{3u} \text{ of } D_{2h}.$$

The correspondences of irreps at HSPs from original SG to lowered SG:

$$n_{GM6}^{66} = n_{GM10}^{192} + n_{GM11}^{192} + n_{GM12}^{192} n_{GM5}^{66} = n_{GM7}^{192} + n_{GM8}^{192} + n_{GM9}^{192} n_{Y6}^{66} = n_{M6}^{192} n_{Y5}^{66} = n_{M5}^{192} n_{S6}^{66} = n_{M6}^{192} n_{S4}^{66} = n_{M5}^{192}$$

$$n_{S5}^{66} = n_{M6}^{192} n_{S3}^{66} = n_{M5}^{192} n_{Z4}^{66} = n_{A10}^{192} + n_{A11}^{192} + n_{A12}^{192} n_{Z3}^{66} = n_{A7}^{192} + n_{A8}^{192} + n_{A9}^{192} n_{T4}^{66} = n_{L4}^{192} n_{T3}^{66} = n_{L3}^{192} n_{R6}^{66} = n_{L3}^{192} n_{R4}^{66} =$$

$$n_{L4}^{192} n_{R5}^{66} = n_{L4}^{192} n_{R3}^{66} = n_{L3}^{192}$$

The lower SG is SG 66 when the preserved operations are: **(sub-SG label is 3) 1, 4, 12, 8, 13, 16, 24, 20.**

$$\text{The transformation is: } (\mathbf{a}_{66}, \mathbf{b}_{66}, \mathbf{c}_{66}) = (\mathbf{a}_{192}, \mathbf{b}_{192}, \mathbf{c}_{192}) \begin{pmatrix} -1 & -1 & 0 \\ 1 & -1 & 0 \\ 0 & 0 & 1 \end{pmatrix}, \overrightarrow{O_{192}O_{66}} = \frac{1}{2}\mathbf{c}_{66}$$

The reduction of higher dimensional irrep:

$$D_{6h} : E_{2g} \rightarrow A_g + B_{1g} \text{ of } D_{2h}.$$

$$D_{6h} : E_{1g} \rightarrow B_{2g} + B_{3g} \text{ of } D_{2h}.$$

$$D_{6h} : E_{2u} \rightarrow A_u + B_{1u} \text{ of } D_{2h}.$$

$$D_{6h} : E_{1u} \rightarrow B_{2u} + B_{3u} \text{ of } D_{2h}.$$

The correspondences of irreps at HSPs from original SG to lowered SG:

$$n_{GM6}^{66} = n_{GM10}^{192} + n_{GM11}^{192} + n_{GM12}^{192} n_{GM5}^{66} = n_{GM7}^{192} + n_{GM8}^{192} + n_{GM9}^{192} n_{Y6}^{66} = n_{M6}^{192} n_{Y5}^{66} = n_{M5}^{192} n_{S6}^{66} = n_{M6}^{192} n_{S4}^{66} = n_{M5}^{192}$$

$$n_{S5}^{66} = n_{M6}^{192} n_{S3}^{66} = n_{M5}^{192} n_{Z4}^{66} = n_{A10}^{192} + n_{A11}^{192} + n_{A12}^{192} n_{Z3}^{66} = n_{A7}^{192} + n_{A8}^{192} + n_{A9}^{192} n_{T4}^{66} = n_{L4}^{192} n_{T3}^{66} = n_{L3}^{192} n_{R6}^{66} = n_{L3}^{192} n_{R4}^{66} =$$

$$n_{L4}^{192} n_{R5}^{66} = n_{L4}^{192} n_{R3}^{66} = n_{L3}^{192}$$

The lower SG is SG 175 when the preserved operations are: **(sub-SG label is 4) 1, 2, 6, 3, 5, 4, 13, 14, 18, 15, 17, 16.**

$$\text{The transformation is: } (\mathbf{a}_{175}, \mathbf{b}_{175}, \mathbf{c}_{175}) = (\mathbf{a}_{192}, \mathbf{b}_{192}, \mathbf{c}_{192}) \begin{pmatrix} -1 & 1 & 0 \\ -1 & 0 & 0 \\ 0 & 0 & 1 \end{pmatrix}, \overrightarrow{O_{192}O_{175}} = \frac{1}{2}\mathbf{c}_{175}$$

The reduction of higher dimensional irrep:

$$D_{6h} : E_{2g} \rightarrow {}^2E_{2g} + {}^1E_{2g} \text{ of } C_{6h}.$$

$$D_{6h} : E_{1g} \rightarrow {}^2E_{1g} + {}^1E_{1g} \text{ of } C_{6h}.$$

$$D_{6h} : E_{2u} \rightarrow {}^2E_{2u} + {}^1E_{2u} \text{ of } C_{6h}.$$

$$D_{6h} : E_{1u} \rightarrow {}^2E_{1u} + {}^1E_{1u} \text{ of } C_{6h}.$$

The correspondences of irreps at HSPs from original SG to lowered SG:

$$n_{GM15}^{175} = n_{GM11}^{192} n_{GM9}^{175} = n_{GM8}^{192} n_{GM18}^{175} = n_{GM11}^{192} n_{GM12}^{175} = n_{GM8}^{192} n_{GM14}^{175} = n_{GM10}^{192} n_{GM8}^{175} = n_{GM7}^{192} n_{GM13}^{175} = n_{GM10}^{192}$$

$$n_{GM7}^{175} = n_{GM7}^{192} n_{GM17}^{175} = n_{GM12}^{192} n_{GM11}^{175} = n_{GM9}^{192} n_{GM16}^{175} = n_{GM12}^{192} n_{GM10}^{175} = n_{GM9}^{192} n_{M5}^{175} = n_{M6}^{192} n_{M3}^{175} = n_{M5}^{192} n_{M6}^{175} =$$

$$n_{M6}^{192} n_{M4}^{175} = n_{M5}^{192} n_{K8}^{175} = n_{K7}^{192} n_{K7}^{175} = n_{K7}^{192} n_{K12}^{175} = n_{K8}^{192} n_{K11}^{175} = n_{K9}^{192} n_{K9}^{175} = n_{K8}^{192} n_{K10}^{175} = n_{K9}^{192} n_{A15}^{175} = n_{A8}^{192} n_{A9}^{175} = n_{A12}^{192}$$

$$n_{A18}^{175} = n_{A12}^{192} n_{A12}^{175} = n_{A8}^{192} n_{A14}^{175} = n_{A10}^{192} n_{A8}^{175} = n_{A7}^{192} n_{A13}^{175} = n_{A7}^{192} n_{A7}^{175} = n_{A10}^{192} n_{A17}^{175} = n_{A9}^{192} n_{A11}^{175} = n_{A11}^{192} n_{A16}^{175} = n_{A11}^{192}$$

$$n_{A10}^{175} = n_{A9}^{192} n_{L5}^{175} = n_{L3}^{192} n_{L3}^{175} = n_{L4}^{192} n_{L6}^{175} = n_{L4}^{192} n_{L4}^{175} = n_{L3}^{192} n_{H8}^{175} = n_{H4}^{192} + n_{H5}^{192} n_{H7}^{175} = n_{H6}^{192} + n_{H7}^{192} n_{H12}^{175} = n_{H8}^{192} n_{H11}^{175} =$$

$$n_{H9}^{192} n_{H9}^{175} = n_{H9}^{192} n_{H10}^{175} = n_{H8}^{192}$$

## 90. Lowered SGs by higher-dimensional irreps of pairings in SG 193

The representative operations of SG/T for SG 193:

$$1 : (x, y, z), 2 : (x - y, x, z + \frac{1}{2}), 3 : (-y, x - y, z), 4 : (-x, -y, z + \frac{1}{2}), 5 : (y - x, -x, z), 6 : (y, y - x, z + \frac{1}{2}), \\ 7 : (x - y, -y, \frac{1}{2} - z), 8 : (y, x, \frac{1}{2} - z), 9 : (-x, y - x, \frac{1}{2} - z), 10 : (x, x - y, -z), 11 : (y - x, y, -z), 12 : (-y, -x, -z), \\ 13 : (-x, -y, -z), 14 : (y - x, -x, \frac{1}{2} - z), 15 : (y, y - x, -z), 16 : (x, y, \frac{1}{2} - z), 17 : (x - y, x, -z), 18 : (-y, x - y, \frac{1}{2} - z), \\ 19 : (y - x, y, z + \frac{1}{2}), 20 : (-y, -x, z + \frac{1}{2}), 21 : (x, x - y, z + \frac{1}{2}), 22 : (-x, y - x, z), 23 : (x - y, -y, z), 24 : (y, x, z).$$

The lower SG is SG 63 when the preserved operations are: **(sub-SG label is 1)** 1, 4, 11, 7, 13, 16, 23, 19.

$$\text{The transformation is: } (\mathbf{a}_{63}, \mathbf{b}_{63}, \mathbf{c}_{63}) = (\mathbf{a}_{193}, \mathbf{b}_{193}, \mathbf{c}_{193}) \begin{pmatrix} 1 & -1 & 0 \\ 2 & 0 & 0 \\ 0 & 0 & 1 \end{pmatrix}, \overrightarrow{O_{193}O_{63}} = \frac{1}{2}\mathbf{c}_{63}$$

The reduction of higher dimensional irrep:

$$D_{6h} : E_{2g} \rightarrow A_g + B_{1g} \text{ of } D_{2h}.$$

$$D_{6h} : E_{1g} \rightarrow B_{2g} + B_{3g} \text{ of } D_{2h}.$$

$$D_{6h} : E_{2u} \rightarrow A_u + B_{1u} \text{ of } D_{2h}.$$

$$D_{6h} : E_{1u} \rightarrow B_{2u} + B_{3u} \text{ of } D_{2h}.$$

The correspondences of irreps at HSPs from original SG to lowered SG:

$$n_{GM6}^{63} = n_{GM10}^{193} + n_{GM11}^{193} + n_{GM12}^{193} \quad n_{GM5}^{63} = n_{GM7}^{193} + n_{GM8}^{193} + n_{GM9}^{193} \quad n_{Y6}^{63} = n_{M6}^{193} \quad n_{Y5}^{63} = n_{M5}^{193} \quad n_{S6}^{63} = n_{M6}^{193} \quad n_{S4}^{63} = n_{M5}^{193} \\ n_{S5}^{63} = n_{M6}^{193} \quad n_{S3}^{63} = n_{M5}^{193} \quad n_{Z4}^{63} = n_{A5}^{193} + n_{A6}^{193} \quad n_{Z3}^{63} = n_{A4}^{193} + n_{A6}^{193} \quad n_{T4}^{63} = n_{L3}^{193} \quad n_{T3}^{63} = n_{L4}^{193} \quad n_{R2}^{63} = n_{L3}^{193} + n_{L4}^{193}$$

The lower SG is SG 63 when the preserved operations are: **(sub-SG label is 2)** 1, 4, 9, 10, 13, 16, 21, 22.

$$\text{The transformation is: } (\mathbf{a}_{63}, \mathbf{b}_{63}, \mathbf{c}_{63}) = (\mathbf{a}_{193}, \mathbf{b}_{193}, \mathbf{c}_{193}) \begin{pmatrix} -2 & 0 & 0 \\ -1 & -1 & 0 \\ 0 & 0 & 1 \end{pmatrix}, \overrightarrow{O_{193}O_{63}} = \frac{1}{2}\mathbf{c}_{63}$$

The reduction of higher dimensional irrep:

$$D_{6h} : E_{2g} \rightarrow A_g + B_{1g} \text{ of } D_{2h}.$$

$$D_{6h} : E_{1g} \rightarrow B_{2g} + B_{3g} \text{ of } D_{2h}.$$

$$D_{6h} : E_{2u} \rightarrow A_u + B_{1u} \text{ of } D_{2h}.$$

$$D_{6h} : E_{1u} \rightarrow B_{2u} + B_{3u} \text{ of } D_{2h}.$$

The correspondences of irreps at HSPs from original SG to lowered SG:

$$n_{GM6}^{63} = n_{GM10}^{193} + n_{GM11}^{193} + n_{GM12}^{193} \quad n_{GM5}^{63} = n_{GM7}^{193} + n_{GM8}^{193} + n_{GM9}^{193} \quad n_{Y6}^{63} = n_{M6}^{193} \quad n_{Y5}^{63} = n_{M5}^{193} \quad n_{S6}^{63} = n_{M6}^{193} \quad n_{S4}^{63} = n_{M5}^{193} \\ n_{S5}^{63} = n_{M6}^{193} \quad n_{S3}^{63} = n_{M5}^{193} \quad n_{Z4}^{63} = n_{A5}^{193} + n_{A6}^{193} \quad n_{Z3}^{63} = n_{A4}^{193} + n_{A6}^{193} \quad n_{T4}^{63} = n_{L3}^{193} \quad n_{T3}^{63} = n_{L4}^{193} \quad n_{R2}^{63} = n_{L3}^{193} + n_{L4}^{193}$$

The lower SG is SG 63 when the preserved operations are: **(sub-SG label is 3)** 1, 4, 12, 8, 13, 16, 24, 20.

$$\text{The transformation is: } (\mathbf{a}_{63}, \mathbf{b}_{63}, \mathbf{c}_{63}) = (\mathbf{a}_{193}, \mathbf{b}_{193}, \mathbf{c}_{193}) \begin{pmatrix} -1 & -1 & 0 \\ 1 & -1 & 0 \\ 0 & 0 & 1 \end{pmatrix}, \overrightarrow{O_{193}O_{63}} = \frac{1}{2}\mathbf{c}_{63}$$

The reduction of higher dimensional irrep:

$$D_{6h} : E_{2g} \rightarrow A_g + B_{1g} \text{ of } D_{2h}.$$

$$D_{6h} : E_{1g} \rightarrow B_{2g} + B_{3g} \text{ of } D_{2h}.$$

$$D_{6h} : E_{2u} \rightarrow A_u + B_{1u} \text{ of } D_{2h}.$$

$$D_{6h} : E_{1u} \rightarrow B_{2u} + B_{3u} \text{ of } D_{2h}.$$

The correspondences of irreps at HSPs from original SG to lowered SG:

$$n_{GM6}^{63} = n_{GM10}^{193} + n_{GM11}^{193} + n_{GM12}^{193} \quad n_{GM5}^{63} = n_{GM7}^{193} + n_{GM8}^{193} + n_{GM9}^{193} \quad n_{Y6}^{63} = n_{M6}^{193} \quad n_{Y5}^{63} = n_{M5}^{193} \quad n_{S6}^{63} = n_{M6}^{193} \quad n_{S4}^{63} = n_{M5}^{193} \\ n_{S5}^{63} = n_{M6}^{193} \quad n_{S3}^{63} = n_{M5}^{193} \quad n_{Z4}^{63} = n_{A4}^{193} + n_{A6}^{193} \quad n_{Z3}^{63} = n_{A5}^{193} + n_{A6}^{193} \quad n_{T4}^{63} = n_{L4}^{193} \quad n_{T3}^{63} = n_{L3}^{193} \quad n_{R2}^{63} = n_{L3}^{193} + n_{L4}^{193}$$

The lower SG is SG 176 when the preserved operations are: **(sub-SG label is 4)** 1, 2, 6, 3, 5, 4, 13, 14, 18, 15, 17, 16.

$$\text{The transformation is: } (\mathbf{a}_{176}, \mathbf{b}_{176}, \mathbf{c}_{176}) = (\mathbf{a}_{193}, \mathbf{b}_{193}, \mathbf{c}_{193}) \begin{pmatrix} -1 & 1 & 0 \\ -1 & 0 & 0 \\ 0 & 0 & 1 \end{pmatrix}, \overrightarrow{O_{193}O_{176}} = \frac{1}{2}\mathbf{c}_{176}$$

The reduction of higher dimensional irrep:

$$D_{6h} : E_{2g} \rightarrow {}^2E_{2g} + {}^1E_{2g} \text{ of } C_{6h}.$$

$$D_{6h} : E_{1g} \rightarrow {}^2E_{1g} + {}^1E_{1g} \text{ of } C_{6h}.$$

$$D_{6h} : E_{2u} \rightarrow {}^2E_{2u} + {}^1E_{2u} \text{ of } C_{6h}.$$

$$D_{6h} : E_{1u} \rightarrow {}^2E_{1u} + {}^1E_{1u} \text{ of } C_{6h}.$$

The correspondences of irreps at HSPs from original SG to lowered SG:

$$n_{GM15}^{176} = n_{GM11}^{193} \quad n_{GM9}^{176} = n_{GM8}^{193} \quad n_{GM18}^{176} = n_{GM11}^{193} \quad n_{GM12}^{176} = n_{GM8}^{193} \quad n_{GM14}^{176} = n_{GM10}^{193} \quad n_{GM8}^{176} = n_{GM7}^{193} \quad n_{GM13}^{176} = n_{GM10}^{193} \\ n_{GM7}^{176} = n_{GM7}^{193} \quad n_{GM17}^{176} = n_{GM12}^{193} \quad n_{GM11}^{176} = n_{GM9}^{193} \quad n_{GM16}^{176} = n_{GM12}^{193} \quad n_{GM10}^{176} = n_{GM9}^{193} \quad n_{M5}^{176} = n_{M6}^{193} \quad n_{M3}^{176} = n_{M5}^{193} \quad n_{M6}^{176} = n_{M6}^{193}$$

$$\begin{aligned}
n_{M4}^{176} &= n_{M3}^{193} n_{K8}^{176} = n_{K7}^{193} n_{K7}^{176} = n_{K7}^{193} n_{K12}^{176} = n_{K8}^{193} n_{K11}^{176} = n_{K9}^{193} n_{K9}^{176} = n_{K8}^{193} n_{K10}^{176} = n_{K9}^{193} n_{A4}^{176} = n_{A4}^{193} + n_{A5}^{193} n_{A6}^{176} = n_{A6}^{193} \\
n_{A5}^{176} &= n_{A6}^{193} n_{L2}^{176} = n_{L3}^{193} + n_{L4}^{193} n_{H7}^{176} = n_{H7}^{193} n_{H8}^{176} = n_{H7}^{193} n_{H12}^{176} = n_{H9}^{193} n_{H11}^{176} = n_{H8}^{193} n_{H10}^{176} = n_{H8}^{193} n_{H9}^{176} = n_{H9}^{193}
\end{aligned}$$

### 91. Lowered SGs by higher-dimensional irreps of pairings in SG 194

The representative operations of SG/T for SG 194:

$$\begin{aligned}
&1 : (x, y, z), 2 : (x - y, x, z + \frac{1}{2}), 3 : (-y, x - y, z), 4 : (-x, -y, z + \frac{1}{2}), 5 : (y - x, -x, z), 6 : (y, y - x, z + \frac{1}{2}), \\
&7 : (x - y, -y, -z), 8 : (y, x, -z), 9 : (-x, y - x, -z), 10 : (x, x - y, \frac{1}{2} - z), 11 : (y - x, y, \frac{1}{2} - z), 12 : (-y, -x, \frac{1}{2} - z), \\
&13 : (-x, -y, -z), 14 : (y - x, -x, \frac{1}{2} - z), 15 : (y, y - x, -z), 16 : (x, y, \frac{1}{2} - z), 17 : (x - y, x, -z), 18 : (-y, x - y, \frac{1}{2} - z), \\
&19 : (y - x, y, z), 20 : (-y, -x, z), 21 : (x, x - y, z), 22 : (-x, y - x, z + \frac{1}{2}), 23 : (x - y, -y, z + \frac{1}{2}), 24 : (y, x, z + \frac{1}{2}).
\end{aligned}$$

The lower SG is SG 63 when the preserved operations are: **(sub-SG label is 1) 1, 4, 11, 7, 13, 16, 23, 19.**

$$\text{The transformation is: } (\mathbf{a}_{63}, \mathbf{b}_{63}, \mathbf{c}_{63}) = (\mathbf{a}_{194}, \mathbf{b}_{194}, \mathbf{c}_{194}) \begin{pmatrix} -1 & -1 & 0 \\ 0 & -2 & 0 \\ 0 & 0 & 1 \end{pmatrix}, \overrightarrow{O_{194}O_{63}} = \frac{1}{2}\mathbf{c}_{63}$$

The reduction of higher dimensional irrep:

$$D_{6h} : E_{2g} \rightarrow A_g + B_{1g} \text{ of } D_{2h}.$$

$$D_{6h} : E_{1g} \rightarrow B_{2g} + B_{3g} \text{ of } D_{2h}.$$

$$D_{6h} : E_{2u} \rightarrow A_u + B_{1u} \text{ of } D_{2h}.$$

$$D_{6h} : E_{1u} \rightarrow B_{2u} + B_{3u} \text{ of } D_{2h}.$$

The correspondences of irreps at HSPs from original SG to lowered SG:

$$\begin{aligned}
n_{GM6}^{63} &= n_{GM10}^{194} + n_{GM11}^{194} + n_{GM12}^{194} n_{GM5}^{63} = n_{GM7}^{194} + n_{GM8}^{194} + n_{GM9}^{194} n_{Y6}^{63} = n_{M6}^{194} n_{Y5}^{63} = n_{M5}^{194} n_{S6}^{63} = n_{M6}^{194} n_{S4}^{63} = n_{M5}^{194} \\
n_{S5}^{63} &= n_{M6}^{194} n_{S3}^{63} = n_{M5}^{194} n_{Z4}^{63} = n_{A4}^{194} + n_{A6}^{194} n_{Z3}^{63} = n_{A5}^{194} + n_{A6}^{194} n_{T4}^{63} = n_{L3}^{194} n_{T3}^{63} = n_{L4}^{194} n_{R2}^{63} = n_{L3}^{194} + n_{L4}^{194}
\end{aligned}$$

The lower SG is SG 63 when the preserved operations are: **(sub-SG label is 2) 1, 4, 9, 10, 13, 16, 21, 22.**

$$\text{The transformation is: } (\mathbf{a}_{63}, \mathbf{b}_{63}, \mathbf{c}_{63}) = (\mathbf{a}_{194}, \mathbf{b}_{194}, \mathbf{c}_{194}) \begin{pmatrix} 0 & -2 & 0 \\ 1 & -1 & 0 \\ 0 & 0 & 1 \end{pmatrix}, \overrightarrow{O_{194}O_{63}} = \frac{1}{2}\mathbf{c}_{63}$$

The reduction of higher dimensional irrep:

$$D_{6h} : E_{2g} \rightarrow A_g + B_{1g} \text{ of } D_{2h}.$$

$$D_{6h} : E_{1g} \rightarrow B_{2g} + B_{3g} \text{ of } D_{2h}.$$

$$D_{6h} : E_{2u} \rightarrow A_u + B_{1u} \text{ of } D_{2h}.$$

$$D_{6h} : E_{1u} \rightarrow B_{2u} + B_{3u} \text{ of } D_{2h}.$$

The correspondences of irreps at HSPs from original SG to lowered SG:

$$\begin{aligned}
n_{GM6}^{63} &= n_{GM10}^{194} + n_{GM11}^{194} + n_{GM12}^{194} n_{GM5}^{63} = n_{GM7}^{194} + n_{GM8}^{194} + n_{GM9}^{194} n_{Y6}^{63} = n_{M6}^{194} n_{Y5}^{63} = n_{M5}^{194} n_{S6}^{63} = n_{M6}^{194} n_{S4}^{63} = n_{M5}^{194} \\
n_{S5}^{63} &= n_{M6}^{194} n_{S3}^{63} = n_{M5}^{194} n_{Z4}^{63} = n_{A5}^{194} + n_{A6}^{194} n_{Z3}^{63} = n_{A4}^{194} + n_{A6}^{194} n_{T4}^{63} = n_{L4}^{194} n_{T3}^{63} = n_{L3}^{194} n_{R2}^{63} = n_{L3}^{194} + n_{L4}^{194}
\end{aligned}$$

The lower SG is SG 63 when the preserved operations are: **(sub-SG label is 3) 1, 4, 12, 8, 13, 16, 24, 20.**

$$\text{The transformation is: } (\mathbf{a}_{63}, \mathbf{b}_{63}, \mathbf{c}_{63}) = (\mathbf{a}_{194}, \mathbf{b}_{194}, \mathbf{c}_{194}) \begin{pmatrix} -1 & 1 & 0 \\ -1 & -1 & 0 \\ 0 & 0 & 1 \end{pmatrix}, \overrightarrow{O_{194}O_{63}} = \frac{1}{2}\mathbf{c}_{63}$$

The reduction of higher dimensional irrep:

$$D_{6h} : E_{2g} \rightarrow A_g + B_{1g} \text{ of } D_{2h}.$$

$$D_{6h} : E_{1g} \rightarrow B_{2g} + B_{3g} \text{ of } D_{2h}.$$

$$D_{6h} : E_{2u} \rightarrow A_u + B_{1u} \text{ of } D_{2h}.$$

$$D_{6h} : E_{1u} \rightarrow B_{2u} + B_{3u} \text{ of } D_{2h}.$$

The correspondences of irreps at HSPs from original SG to lowered SG:

$$\begin{aligned}
n_{GM6}^{63} &= n_{GM10}^{194} + n_{GM11}^{194} + n_{GM12}^{194} n_{GM5}^{63} = n_{GM7}^{194} + n_{GM8}^{194} + n_{GM9}^{194} n_{Y6}^{63} = n_{M6}^{194} n_{Y5}^{63} = n_{M5}^{194} n_{S6}^{63} = n_{M6}^{194} n_{S4}^{63} = n_{M5}^{194} \\
n_{S5}^{63} &= n_{M6}^{194} n_{S3}^{63} = n_{M5}^{194} n_{Z4}^{63} = n_{A5}^{194} + n_{A6}^{194} n_{Z3}^{63} = n_{A4}^{194} + n_{A6}^{194} n_{T4}^{63} = n_{L4}^{194} n_{T3}^{63} = n_{L3}^{194} n_{R2}^{63} = n_{L3}^{194} + n_{L4}^{194}
\end{aligned}$$

The lower SG is SG 176 when the preserved operations are: **(sub-SG label is 4) 1, 2, 6, 3, 5, 4, 13, 14, 18, 15, 17, 16.**

The transformation is:  $(\mathbf{a}_{176}, \mathbf{b}_{176}, \mathbf{c}_{176}) = (\mathbf{a}_{194}, \mathbf{b}_{194}, \mathbf{c}_{194}) \begin{pmatrix} -1 & 1 & 0 \\ -1 & 0 & 0 \\ 0 & 0 & 1 \end{pmatrix}, \overrightarrow{O_{194}O_{176}} = \frac{1}{2}\mathbf{c}_{176}$

The reduction of higher dimensional irrep:

$$D_{6h} : E_{2g} \rightarrow {}^2E_{2g} + {}^1E_{2g} \text{ of } C_{6h}.$$

$$D_{6h} : E_{1g} \rightarrow {}^2E_{1g} + {}^1E_{1g} \text{ of } C_{6h}.$$

$$D_{6h} : E_{2u} \rightarrow {}^2E_{2u} + {}^1E_{2u} \text{ of } C_{6h}.$$

$$D_{6h} : E_{1u} \rightarrow {}^2E_{1u} + {}^1E_{1u} \text{ of } C_{6h}.$$

The correspondences of irreps at HSPs from original SG to lowered SG:

$$\begin{aligned} n_{GM15}^{176} &= n_{GM11}^{194} n_{GM9}^{176} = n_{GM8}^{194} n_{GM18}^{176} = n_{GM11}^{194} n_{GM12}^{176} = n_{GM8}^{194} n_{GM14}^{176} = n_{GM10}^{194} n_{GM8}^{176} = n_{GM7}^{194} n_{GM13}^{176} = n_{GM10}^{194} \\ n_{GM7}^{176} &= n_{GM7}^{194} n_{GM17}^{176} = n_{GM12}^{194} n_{GM11}^{176} = n_{GM9}^{194} n_{GM16}^{176} = n_{GM12}^{194} n_{GM10}^{176} = n_{GM9}^{194} n_{M5}^{176} = n_{M6}^{194} n_{M3}^{176} = n_{M5}^{194} n_{M6}^{176} = n_{M6}^{194} \\ n_{M4}^{176} &= n_{M5}^{194} n_{K8}^{176} = n_{K7}^{194} n_{K7}^{176} = n_{K7}^{194} n_{K12}^{176} = n_{K8}^{194} n_{K11}^{176} = n_{K9}^{194} n_{K9}^{176} = n_{K8}^{194} n_{K10}^{176} = n_{K9}^{194} n_{A4}^{176} = n_{A4}^{194} + n_{A5}^{194} n_{A6}^{176} = n_{A6}^{194} \\ n_{A5}^{176} &= n_{A6}^{194} n_{L2}^{176} = n_{L3}^{194} + n_{L4}^{194} n_{H7}^{176} = n_{H6}^{194} + n_{H7}^{194} n_{H8}^{176} = n_{H4}^{194} + n_{H5}^{194} n_{H12}^{176} = n_{H8}^{194} n_{H11}^{176} = n_{H9}^{194} n_{H10}^{176} = n_{H8}^{194} n_{H9}^{176} = \end{aligned}$$

## 92. Lowered SGs by higher-dimensional irreps of pairings in SG 195

The representative operations of SG/T for SG 195:

$$1 : (x, y, z), 2 : (x, -y, -z), 3 : (-x, y, -z), 4 : (-x, -y, z), 5 : (z, x, y), 6 : (y, z, x), 7 : (-y, z, -x), 8 : (-z, -x, y), \\ 9 : (-y, -z, x), 10 : (z, -x, -y), 11 : (y, -z, -x), 12 : (-z, x, -y).$$

The lower SG is SG 16 when the preserved operations are: **(sub-SG label is 1) 1, 2, 3, 4.**

The transformation is:  $(\mathbf{a}_{16}, \mathbf{b}_{16}, \mathbf{c}_{16}) = (\mathbf{a}_{195}, \mathbf{b}_{195}, \mathbf{c}_{195}) \begin{pmatrix} 0 & 0 & 1 \\ 1 & 0 & 0 \\ 0 & 1 & 0 \end{pmatrix}, \overrightarrow{O_{195}O_{16}} = \frac{1}{2}\mathbf{a}_{16} + (\frac{1}{2})\mathbf{c}_{16}$

The reduction of higher dimensional irrep:

$$T : T \rightarrow B_1 + B_2 + B_3 \text{ of } D_2.$$

The correspondences of irreps at HSPs from original SG to lowered SG:

$$\begin{aligned} n_{GM5}^{16} &= n_{GM5}^{195} + n_{GM6}^{195} + n_{GM7}^{195} n_{X5}^{16} = n_{X5}^{195} n_{S5}^{16} = n_{M5}^{195} n_{R5}^{16} = n_{R5}^{195} + n_{R6}^{195} + n_{R7}^{195} n_{U5}^{16} = n_{M5}^{195} n_{Z5}^{16} = n_{X5}^{195} n_{T5}^{16} = n_{M5}^{195} \\ n_{Y5}^{16} &= n_{X5}^{195} \end{aligned}$$

The lower SG is SG 146 when the preserved operations are: **(sub-SG label is 2) 1, 5, 6.**

The transformation is:  $(\mathbf{a}_{146}, \mathbf{b}_{146}, \mathbf{c}_{146}) = (\mathbf{a}_{195}, \mathbf{b}_{195}, \mathbf{c}_{195}) \begin{pmatrix} 0 & 1 & 0 \\ 0 & 0 & 1 \\ 1 & 0 & 0 \end{pmatrix}, \overrightarrow{O_{195}O_{146}} = -\frac{1}{3}\mathbf{a}_{146} + (\frac{2}{3})\mathbf{b}_{146} + (-\frac{1}{3})\mathbf{c}_{146}$

The reduction of higher dimensional irrep:

$$T : T \rightarrow A + {}^2E + {}^1E \text{ of } C_3.$$

The correspondences of irreps at HSPs from original SG to lowered SG:

$$\begin{aligned} n_{GM4}^{146} &= n_{GM6}^{195} + n_{GM7}^{195} n_{GM6}^{146} = n_{GM5}^{195} + n_{GM6}^{195} n_{GM5}^{146} = n_{GM5}^{195} + n_{GM7}^{195} n_{L2}^{146} = 2n_{X5}^{195} n_{F2}^{146} = 2n_{M5}^{195} n_{T4}^{146} = n_{R6}^{195} + n_{R7}^{195} \\ n_{T6}^{146} &= n_{R5}^{195} + n_{R6}^{195} n_{T5}^{146} = n_{R5}^{195} + n_{R7}^{195} \end{aligned}$$

The lower SG is SG 146 when the preserved operations are: **(sub-SG label is 3) 1, 12, 11.**

The transformation is:  $(\mathbf{a}_{146}, \mathbf{b}_{146}, \mathbf{c}_{146}) = (\mathbf{a}_{195}, \mathbf{b}_{195}, \mathbf{c}_{195}) \begin{pmatrix} 0 & -1 & 0 \\ 0 & 0 & -1 \\ 1 & 0 & 0 \end{pmatrix}, \overrightarrow{O_{195}O_{146}} = -\frac{1}{3}\mathbf{a}_{146} + (\frac{2}{3})\mathbf{b}_{146} + (-\frac{1}{3})\mathbf{c}_{146}$

The reduction of higher dimensional irrep:

$$T : T \rightarrow A + {}^2E + {}^1E \text{ of } C_3.$$

The correspondences of irreps at HSPs from original SG to lowered SG:

$$\begin{aligned} n_{GM4}^{146} &= n_{GM6}^{195} + n_{GM7}^{195} n_{GM6}^{146} = n_{GM5}^{195} + n_{GM6}^{195} n_{GM5}^{146} = n_{GM5}^{195} + n_{GM7}^{195} n_{L2}^{146} = 2n_{X5}^{195} n_{F2}^{146} = 2n_{M5}^{195} n_{T4}^{146} = n_{R6}^{195} + n_{R7}^{195} \\ n_{T6}^{146} &= n_{R5}^{195} + n_{R6}^{195} n_{T5}^{146} = n_{R5}^{195} + n_{R7}^{195} \end{aligned}$$

The lower SG is SG 146 when the preserved operations are: **(sub-SG label is 4) 1, 8, 7.**

The transformation is:  $(\mathbf{a}_{146}, \mathbf{b}_{146}, \mathbf{c}_{146}) = (\mathbf{a}_{195}, \mathbf{b}_{195}, \mathbf{c}_{195}) \begin{pmatrix} 1 & 0 & 0 \\ 0 & -1 & 0 \\ 0 & 0 & -1 \end{pmatrix}, \overrightarrow{O_{195}O_{146}} = -\frac{1}{3}\mathbf{a}_{146} + (\frac{2}{3})\mathbf{b}_{146} + (-\frac{1}{3})\mathbf{c}_{146}$

The reduction of higher dimensional irrep:

$T: T \rightarrow A + {}^2E + {}^1E$  of  $C_3$ .

The correspondences of irreps at HSPs from original SG to lowered SG:

$$\begin{aligned} n_{GM4}^{146} &= n_{GM6}^{195} + n_{GM7}^{195} n_{GM6}^{146} = n_{GM5}^{195} + n_{GM6}^{195} n_{GM5}^{146} = n_{GM5}^{195} + n_{GM7}^{195} n_{L2}^{146} = 2n_{X5}^{195} n_{F2}^{146} = 2n_{M5}^{195} n_{T4}^{146} = n_{R6}^{195} + n_{R7}^{195} \\ n_{T6}^{146} &= n_{R5}^{195} + n_{R6}^{195} n_{T5}^{146} = n_{R5}^{195} + n_{R7}^{195} \end{aligned}$$

The lower SG is SG 146 when the preserved operations are: **(sub-SG label is 5) 1, 10, 9.**

The transformation is:  $(\mathbf{a}_{146}, \mathbf{b}_{146}, \mathbf{c}_{146}) = (\mathbf{a}_{195}, \mathbf{b}_{195}, \mathbf{c}_{195}) \begin{pmatrix} -1 & 0 & 0 \\ 0 & 1 & 0 \\ 0 & 0 & -1 \end{pmatrix}, \overrightarrow{O_{195}O_{146}} = -\frac{1}{3}\mathbf{a}_{146} + (\frac{2}{3})\mathbf{b}_{146} + (-\frac{1}{3})\mathbf{c}_{146}$

The reduction of higher dimensional irrep:

$T: T \rightarrow A + {}^2E + {}^1E$  of  $C_3$ .

The correspondences of irreps at HSPs from original SG to lowered SG:

$$\begin{aligned} n_{GM4}^{146} &= n_{GM6}^{195} + n_{GM7}^{195} n_{GM6}^{146} = n_{GM5}^{195} + n_{GM6}^{195} n_{GM5}^{146} = n_{GM5}^{195} + n_{GM7}^{195} n_{L2}^{146} = 2n_{X5}^{195} n_{F2}^{146} = 2n_{M5}^{195} n_{T4}^{146} = n_{R6}^{195} + n_{R7}^{195} \\ n_{T6}^{146} &= n_{R5}^{195} + n_{R6}^{195} n_{T5}^{146} = n_{R5}^{195} + n_{R7}^{195} \end{aligned}$$

### 93. Lowered SGs by higher-dimensional irreps of pairings in SG 196

The representative operations of SG/T for SG 196:

$$1: (x, y, z), 2: (x, -y, -z), 3: (-x, y, -z), 4: (-x, -y, z), 5: (z, x, y), 6: (y, z, x), 7: (-y, z, -x), 8: (-z, -x, y), 9: (-y, -z, x), 10: (z, -x, -y), 11: (y, -z, -x), 12: (-z, x, -y).$$

The lower SG is SG 22 when the preserved operations are: **(sub-SG label is 1) 1, 2, 3, 4.**

The transformation is:  $(\mathbf{a}_{22}, \mathbf{b}_{22}, \mathbf{c}_{22}) = (\mathbf{a}_{196}, \mathbf{b}_{196}, \mathbf{c}_{196}) \begin{pmatrix} 0 & 0 & 1 \\ 1 & 0 & 0 \\ 0 & 1 & 0 \end{pmatrix}, \overrightarrow{O_{196}O_{22}} = \frac{1}{4}\mathbf{a}_{22} + (-\frac{1}{4})\mathbf{b}_{22} + (-\frac{1}{4})\mathbf{c}_{22}$

The reduction of higher dimensional irrep:

$T: T \rightarrow B_1 + B_2 + B_3$  of  $D_2$ .

The correspondences of irreps at HSPs from original SG to lowered SG:

$$n_{GM5}^{22} = n_{GM5}^{196} + n_{GM6}^{196} n_{Y5}^{22} = n_{X5}^{196} n_{L2}^{22} = n_{L4}^{196} + n_{L5}^{196} + n_{L6}^{196} n_{Z5}^{22} = n_{X5}^{196} n_{T5}^{22} = n_{X5}^{196}$$

The lower SG is SG 146 when the preserved operations are: **(sub-SG label is 2) 1, 5, 6.**

The transformation is:  $(\mathbf{a}_{146}, \mathbf{b}_{146}, \mathbf{c}_{146}) = (\mathbf{a}_{196}, \mathbf{b}_{196}, \mathbf{c}_{196}) \begin{pmatrix} \frac{1}{2} & 0 & \frac{1}{2} \\ \frac{1}{2} & \frac{1}{2} & 0 \\ 0 & \frac{1}{2} & \frac{1}{2} \end{pmatrix}, \overrightarrow{O_{196}O_{146}} = -\frac{1}{3}\mathbf{a}_{146} + (\frac{2}{3})\mathbf{b}_{146} + (-\frac{1}{3})\mathbf{c}_{146}$

The reduction of higher dimensional irrep:

$T: T \rightarrow A + {}^2E + {}^1E$  of  $C_3$ .

The correspondences of irreps at HSPs from original SG to lowered SG:

$$\begin{aligned} n_{GM4}^{146} &= n_{GM6}^{196} + n_{GM7}^{196} n_{GM6}^{146} = n_{GM5}^{196} + n_{GM6}^{196} n_{GM5}^{146} = n_{GM5}^{196} + n_{GM7}^{196} n_{L2}^{146} = n_{L4}^{196} + n_{L5}^{196} + n_{L6}^{196} n_{F2}^{146} = 2n_{X5}^{196} n_{T4}^{146} = \\ n_{L4}^{196} n_{T6}^{146} &= n_{L6}^{196} n_{T5}^{146} = n_{L5}^{196} \end{aligned}$$

The lower SG is SG 146 when the preserved operations are: **(sub-SG label is 3) 1, 12, 11.**

The transformation is:  $(\mathbf{a}_{146}, \mathbf{b}_{146}, \mathbf{c}_{146}) = (\mathbf{a}_{196}, \mathbf{b}_{196}, \mathbf{c}_{196}) \begin{pmatrix} -\frac{1}{2} & -\frac{1}{2} & 0 \\ 0 & -\frac{1}{2} & -\frac{1}{2} \\ \frac{1}{2} & 0 & \frac{1}{2} \end{pmatrix}, \overrightarrow{O_{196}O_{146}} = -\frac{1}{3}\mathbf{a}_{146} + (\frac{2}{3})\mathbf{b}_{146} + (-\frac{1}{3})\mathbf{c}_{146}$

The reduction of higher dimensional irrep:

$T: T \rightarrow A + {}^2E + {}^1E$  of  $C_3$ .

The correspondences of irreps at HSPs from original SG to lowered SG:

$$n_{GM4}^{146} = n_{GM6}^{196} + n_{GM7}^{196} n_{GM6}^{146} = n_{GM5}^{196} + n_{GM6}^{196} n_{GM5}^{146} = n_{GM5}^{196} + n_{GM7}^{196} n_{L2}^{146} = n_{L4}^{196} + n_{L5}^{196} + n_{L6}^{196} n_{F2}^{146} = 2n_{X5}^{196} n_{T4}^{146} =$$

$$n_{L4}^{196} n_{T6}^{146} = n_{L6}^{196} n_{T5}^{146} = n_{L5}^{196}$$

The lower SG is SG 146 when the preserved operations are: **(sub-SG label is 4) 1, 8, 7.**

$$\text{The transformation is: } (\mathbf{a}_{146}, \mathbf{b}_{146}, \mathbf{c}_{146}) = (\mathbf{a}_{196}, \mathbf{b}_{196}, \mathbf{c}_{196}) \begin{pmatrix} \frac{1}{2} & 0 & \frac{1}{2} \\ -\frac{1}{2} & -\frac{1}{2} & 0 \\ 0 & -\frac{1}{2} & -\frac{1}{2} \end{pmatrix}, \overrightarrow{O_{196}O_{146}} = -\frac{1}{3}\mathbf{a}_{146} + \left(\frac{2}{3}\right)\mathbf{b}_{146} + \left(-\frac{1}{3}\right)\mathbf{c}_{146}$$

The reduction of higher dimensional irrep:

$$T : T \rightarrow A + {}^2E + {}^1E \text{ of } C_3.$$

The correspondences of irreps at HSPs from original SG to lowered SG:

$$n_{GM4}^{146} = n_{GM6}^{196} + n_{GM7}^{196} n_{GM6}^{146} = n_{GM5}^{196} + n_{GM6}^{196} n_{GM5}^{146} = n_{GM5}^{196} + n_{GM7}^{196} n_{L2}^{146} = n_{L4}^{196} + n_{L5}^{196} + n_{L6}^{196} n_{F2}^{146} = 2n_{X5}^{196} n_{T4}^{146} = n_{L4}^{196} n_{T6}^{146} = n_{L6}^{196} n_{T5}^{146} = n_{L5}^{196}$$

The lower SG is SG 146 when the preserved operations are: **(sub-SG label is 5) 1, 10, 9.**

$$\text{The transformation is: } (\mathbf{a}_{146}, \mathbf{b}_{146}, \mathbf{c}_{146}) = (\mathbf{a}_{196}, \mathbf{b}_{196}, \mathbf{c}_{196}) \begin{pmatrix} -\frac{1}{2} & -\frac{1}{2} & 0 \\ 0 & \frac{1}{2} & \frac{1}{2} \\ -\frac{1}{2} & 0 & -\frac{1}{2} \end{pmatrix}, \overrightarrow{O_{196}O_{146}} = -\frac{1}{3}\mathbf{a}_{146} + \left(\frac{2}{3}\right)\mathbf{b}_{146} + \left(-\frac{1}{3}\right)\mathbf{c}_{146}$$

The reduction of higher dimensional irrep:

$$T : T \rightarrow A + {}^2E + {}^1E \text{ of } C_3.$$

The correspondences of irreps at HSPs from original SG to lowered SG:

$$n_{GM4}^{146} = n_{GM6}^{196} + n_{GM7}^{196} n_{GM6}^{146} = n_{GM5}^{196} + n_{GM6}^{196} n_{GM5}^{146} = n_{GM5}^{196} + n_{GM7}^{196} n_{L2}^{146} = n_{L4}^{196} + n_{L5}^{196} + n_{L6}^{196} n_{F2}^{146} = 2n_{X5}^{196} n_{T4}^{146} = n_{L4}^{196} n_{T6}^{146} = n_{L6}^{196} n_{T5}^{146} = n_{L5}^{196}$$

#### 94. Lowered SGs by higher-dimensional irreps of pairings in SG 197

The representative operations of SG/T for SG 197:

$$1 : (x, y, z), 2 : (x, -y, -z), 3 : (-x, y, -z), 4 : (-x, -y, z), 5 : (z, x, y), 6 : (y, z, x), 7 : (-y, z, -x), 8 : (-z, -x, y), 9 : (-y, -z, x), 10 : (z, -x, -y), 11 : (y, -z, -x), 12 : (-z, x, -y).$$

The lower SG is SG 23 when the preserved operations are: **(sub-SG label is 1) 1, 2, 3, 4.**

$$\text{The transformation is: } (\mathbf{a}_{23}, \mathbf{b}_{23}, \mathbf{c}_{23}) = (\mathbf{a}_{197}, \mathbf{b}_{197}, \mathbf{c}_{197}) \begin{pmatrix} 0 & 0 & 1 \\ 1 & 0 & 0 \\ 0 & 1 & 0 \end{pmatrix}, \overrightarrow{O_{197}O_{23}} = -\frac{1}{2}\mathbf{b}_{23}$$

The reduction of higher dimensional irrep:

$$T : T \rightarrow B_1 + B_2 + B_3 \text{ of } D_2.$$

The correspondences of irreps at HSPs from original SG to lowered SG:

$$n_{GM5}^{23} = n_{GM5}^{197} + n_{GM6}^{197} + n_{GM7}^{197} n_{X5}^{23} = n_{H5}^{197} + n_{H6}^{197} + n_{H7}^{197} n_{T4}^{23} = n_{N3}^{197} n_{T3}^{23} = n_{N4}^{197} n_{W5}^{23} = n_{P5}^{197} + n_{P6}^{197} + n_{P7}^{197} n_{R4}^{23} = n_{N4}^{197} n_{R3}^{23} = n_{N3}^{197} n_{S3}^{23} = n_{N4}^{197} n_{S4}^{23} = n_{N3}^{197}$$

The lower SG is SG 146 when the preserved operations are: **(sub-SG label is 2) 1, 5, 6.**

$$\text{The transformation is: } (\mathbf{a}_{146}, \mathbf{b}_{146}, \mathbf{c}_{146}) = (\mathbf{a}_{197}, \mathbf{b}_{197}, \mathbf{c}_{197}) \begin{pmatrix} \frac{1}{2} & -\frac{1}{2} & \frac{1}{2} \\ \frac{1}{2} & \frac{1}{2} & -\frac{1}{2} \\ -\frac{1}{2} & \frac{1}{2} & \frac{1}{2} \end{pmatrix}, \overrightarrow{O_{197}O_{146}} = -\frac{1}{3}\mathbf{a}_{146} + \left(\frac{2}{3}\right)\mathbf{b}_{146} + \left(-\frac{1}{3}\right)\mathbf{c}_{146}$$

The reduction of higher dimensional irrep:

$$T : T \rightarrow A + {}^2E + {}^1E \text{ of } C_3.$$

The correspondences of irreps at HSPs from original SG to lowered SG:

$$n_{GM4}^{146} = n_{GM6}^{197} + n_{GM7}^{197} n_{GM6}^{146} = n_{GM5}^{197} + n_{GM6}^{197} n_{GM5}^{146} = n_{GM5}^{197} + n_{GM7}^{197} n_{L2}^{146} = n_{N3}^{197} + n_{N4}^{197} n_{F2}^{146} = n_{N3}^{197} + n_{N4}^{197} n_{T4}^{146} = n_{H6}^{197} + n_{H7}^{197} n_{T6}^{146} = n_{H5}^{197} + n_{H6}^{197} n_{T5}^{146} = n_{H5}^{197} + n_{H7}^{197}$$

The lower SG is SG 146 when the preserved operations are: **(sub-SG label is 3) 1, 12, 11.**

$$\text{The transformation is: } (\mathbf{a}_{146}, \mathbf{b}_{146}, \mathbf{c}_{146}) = (\mathbf{a}_{197}, \mathbf{b}_{197}, \mathbf{c}_{197}) \begin{pmatrix} -\frac{1}{2} & -\frac{1}{2} & \frac{1}{2} \\ \frac{1}{2} & -\frac{1}{2} & -\frac{1}{2} \\ \frac{1}{2} & -\frac{1}{2} & \frac{1}{2} \end{pmatrix}, \overrightarrow{O_{197}O_{146}} = -\frac{1}{3}\mathbf{a}_{146} + \left(\frac{2}{3}\right)\mathbf{b}_{146} + \left(-\frac{1}{3}\right)\mathbf{c}_{146}$$

The reduction of higher dimensional irrep:

$T : T \rightarrow A + {}^2E + {}^1E$  of  $C_3$ .

The correspondences of irreps at HSPs from original SG to lowered SG:

$$\begin{aligned} n_{GM4}^{146} &= n_{GM6}^{197} + n_{GM7}^{197} n_{GM6}^{146} = n_{GM5}^{197} + n_{GM6}^{197} n_{GM5}^{146} = n_{GM5}^{197} + n_{GM7}^{197} n_{L2}^{146} = n_{N3}^{197} + n_{N4}^{197} n_{F2}^{146} = n_{N3}^{197} + n_{N4}^{197} n_{T4}^{146} = \\ n_{H6}^{197} + n_{H7}^{197} n_{T6}^{146} &= n_{H5}^{197} + n_{H6}^{197} n_{T5}^{146} = n_{H5}^{197} + n_{H7}^{197} \end{aligned}$$

The lower SG is SG 146 when the preserved operations are: **(sub-SG label is 4) 1, 8, 7.**

$$\text{The transformation is: } (\mathbf{a}_{146}, \mathbf{b}_{146}, \mathbf{c}_{146}) = (\mathbf{a}_{197}, \mathbf{b}_{197}, \mathbf{c}_{197}) \begin{pmatrix} \frac{1}{2} & -\frac{1}{2} & \frac{1}{2} \\ -\frac{1}{2} & -\frac{1}{2} & \frac{1}{2} \\ \frac{1}{2} & -\frac{1}{2} & -\frac{1}{2} \end{pmatrix}, \overrightarrow{O_{197}O_{146}} = -\frac{1}{3}\mathbf{a}_{146} + \left(\frac{2}{3}\right)\mathbf{b}_{146} + \left(-\frac{1}{3}\right)\mathbf{c}_{146}$$

The reduction of higher dimensional irrep:

$T : T \rightarrow A + {}^2E + {}^1E$  of  $C_3$ .

The correspondences of irreps at HSPs from original SG to lowered SG:

$$\begin{aligned} n_{GM4}^{146} &= n_{GM6}^{197} + n_{GM7}^{197} n_{GM6}^{146} = n_{GM5}^{197} + n_{GM6}^{197} n_{GM5}^{146} = n_{GM5}^{197} + n_{GM7}^{197} n_{L2}^{146} = n_{N3}^{197} + n_{N4}^{197} n_{F2}^{146} = n_{N3}^{197} + n_{N4}^{197} n_{T4}^{146} = \\ n_{H6}^{197} + n_{H7}^{197} n_{T6}^{146} &= n_{H5}^{197} + n_{H6}^{197} n_{T5}^{146} = n_{H5}^{197} + n_{H7}^{197} \end{aligned}$$

The lower SG is SG 146 when the preserved operations are: **(sub-SG label is 5) 1, 10, 9.**

$$\text{The transformation is: } (\mathbf{a}_{146}, \mathbf{b}_{146}, \mathbf{c}_{146}) = (\mathbf{a}_{197}, \mathbf{b}_{197}, \mathbf{c}_{197}) \begin{pmatrix} -\frac{1}{2} & -\frac{1}{2} & \frac{1}{2} \\ -\frac{1}{2} & \frac{1}{2} & \frac{1}{2} \\ -\frac{1}{2} & \frac{1}{2} & -\frac{1}{2} \end{pmatrix}, \overrightarrow{O_{197}O_{146}} = -\frac{1}{3}\mathbf{a}_{146} + \left(\frac{2}{3}\right)\mathbf{b}_{146} + \left(-\frac{1}{3}\right)\mathbf{c}_{146}$$

The reduction of higher dimensional irrep:

$T : T \rightarrow A + {}^2E + {}^1E$  of  $C_3$ .

The correspondences of irreps at HSPs from original SG to lowered SG:

$$\begin{aligned} n_{GM4}^{146} &= n_{GM6}^{197} + n_{GM7}^{197} n_{GM6}^{146} = n_{GM5}^{197} + n_{GM6}^{197} n_{GM5}^{146} = n_{GM5}^{197} + n_{GM7}^{197} n_{L2}^{146} = n_{N3}^{197} + n_{N4}^{197} n_{F2}^{146} = n_{N3}^{197} + n_{N4}^{197} n_{T4}^{146} = \\ n_{H6}^{197} + n_{H7}^{197} n_{T6}^{146} &= n_{H5}^{197} + n_{H6}^{197} n_{T5}^{146} = n_{H5}^{197} + n_{H7}^{197} \end{aligned}$$

## 95. Lowered SGs by higher-dimensional irreps of pairings in SG 198

The representative operations of SG/T for SG 198:

$$\begin{aligned} 1 : (x, y, z), 2 : (x + \frac{1}{2}, \frac{1}{2} - y, -z), 3 : (-x, y + \frac{1}{2}, \frac{1}{2} - z), 4 : (\frac{1}{2} - x, -y, z + \frac{1}{2}), 5 : (z, x, y), 6 : (y, z, x), \\ 7 : (-y, z + \frac{1}{2}, \frac{1}{2} - x), 8 : (\frac{1}{2} - z, -x, y + \frac{1}{2}), 9 : (\frac{1}{2} - y, -z, x + \frac{1}{2}), 10 : (z + \frac{1}{2}, \frac{1}{2} - x, -y), 11 : (y + \frac{1}{2}, \frac{1}{2} - z, -x), \\ 12 : (-z, x + \frac{1}{2}, \frac{1}{2} - y). \end{aligned}$$

The lower SG is SG 19 when the preserved operations are: **(sub-SG label is 1) 1, 2, 3, 4.**

$$\text{The transformation is: } (\mathbf{a}_{19}, \mathbf{b}_{19}, \mathbf{c}_{19}) = (\mathbf{a}_{198}, \mathbf{b}_{198}, \mathbf{c}_{198}) \begin{pmatrix} 0 & 0 & -1 \\ 0 & -1 & 0 \\ -1 & 0 & 0 \end{pmatrix}, \overrightarrow{O_{198}O_{19}} = \frac{1}{4}\mathbf{a}_{19} + \left(-\frac{1}{4}\right)\mathbf{b}_{19} + \left(\frac{1}{4}\right)\mathbf{c}_{19}$$

The reduction of higher dimensional irrep:

$T : T \rightarrow B_1 + B_3 + B_2$  of  $D_2$ .

The correspondences of irreps at HSPs from original SG to lowered SG:

$$\begin{aligned} n_{GM5}^{19} &= n_{GM5}^{198} + n_{GM6}^{198} n_{GM5}^{19} = n_{X4}^{198} n_{X5}^{19} = n_{X3}^{198} n_{X3}^{19} = n_{X5}^{198} n_{X2}^{19} = n_{X2}^{198} n_{S5}^{19} = n_{M5}^{198} n_{R3}^{19} = n_{R7}^{198} n_{R2}^{19} = \\ n_{R4}^{198} + n_{R5}^{198} + n_{R6}^{198} n_{R4}^{19} &= n_{R7}^{198} n_{R5}^{19} = n_{R7}^{198} n_{U5}^{19} = n_{M5}^{198} n_{Z4}^{19} = n_{X5}^{198} n_{Z5}^{19} = n_{X4}^{198} n_{Z3}^{19} = n_{X3}^{198} n_{Z2}^{19} = n_{X2}^{198} n_{T5}^{19} = n_{M5}^{198} n_{Y3}^{19} = \\ n_{X3}^{198} n_{Y2}^{19} &= n_{X5}^{198} n_{Y4}^{19} = n_{X4}^{198} n_{Y5}^{19} = n_{X2}^{198} \end{aligned}$$

The lower SG is SG 146 when the preserved operations are: **(sub-SG label is 2) 1, 5, 6.**

$$\text{The transformation is: } (\mathbf{a}_{146}, \mathbf{b}_{146}, \mathbf{c}_{146}) = (\mathbf{a}_{198}, \mathbf{b}_{198}, \mathbf{c}_{198}) \begin{pmatrix} 0 & 1 & 0 \\ 0 & 0 & 1 \\ 1 & 0 & 0 \end{pmatrix}, \overrightarrow{O_{198}O_{146}} = -\frac{1}{3}\mathbf{a}_{146} + \left(\frac{2}{3}\right)\mathbf{b}_{146} + \left(-\frac{1}{3}\right)\mathbf{c}_{146}$$

The reduction of higher dimensional irrep:

$T : T \rightarrow A + {}^2E + {}^1E$  of  $C_3$ .

The correspondences of irreps at HSPs from original SG to lowered SG:

$$\begin{aligned} n_{GM4}^{146} &= n_{GM6}^{198} + n_{GM7}^{198} n_{GM6}^{146} = n_{GM5}^{198} + n_{GM6}^{198} n_{GM5}^{146} = n_{GM5}^{198} + n_{GM7}^{198} n_{L2}^{146} = n_{X2}^{198} + n_{X3}^{198} + n_{X4}^{198} + n_{X5}^{198} n_{F2}^{146} = 2n_{M5}^{198} \\ n_{T4}^{146} &= n_{R4}^{198} + n_{R7}^{198} n_{T6}^{146} = n_{R6}^{198} + n_{R7}^{198} n_{T5}^{146} = n_{R5}^{198} + n_{R7}^{198} \end{aligned}$$

The lower SG is SG 146 when the preserved operations are: **(sub-SG label is 3) 1, 12, 11.**

$$\text{The transformation is: } (\mathbf{a}_{146}, \mathbf{b}_{146}, \mathbf{c}_{146}) = (\mathbf{a}_{198}, \mathbf{b}_{198}, \mathbf{c}_{198}) \begin{pmatrix} 0 & -1 & 0 \\ 0 & 0 & -1 \\ 1 & 0 & 0 \end{pmatrix}, \overrightarrow{O_{198}O_{146}} = -\frac{1}{2}\mathbf{a}_{146} + \left(\frac{1}{2}\right)\mathbf{b}_{146}$$

The reduction of higher dimensional irrep:

$$T : T \rightarrow A + {}^2E + {}^1E \text{ of } C_3.$$

The correspondences of irreps at HSPs from original SG to lowered SG:

$$\begin{aligned} n_{GM4}^{146} &= n_{GM6}^{198} + n_{GM7}^{198} n_{GM6}^{146} = n_{GM5}^{198} + n_{GM6}^{198} n_{GM5}^{146} = n_{GM5}^{198} + n_{GM7}^{198} n_{L2}^{146} = n_{X2}^{198} + n_{X3}^{198} + n_{X4}^{198} + n_{X5}^{198} n_{F2}^{146} = 2n_{M5}^{198} \\ n_{T4}^{146} &= n_{R4}^{198} + n_{R7}^{198} n_{T6}^{146} = n_{R6}^{198} + n_{R7}^{198} n_{T5}^{146} = n_{R5}^{198} + n_{R7}^{198} \end{aligned}$$

The lower SG is SG 146 when the preserved operations are: **(sub-SG label is 4) 1, 8, 7.**

$$\text{The transformation is: } (\mathbf{a}_{146}, \mathbf{b}_{146}, \mathbf{c}_{146}) = (\mathbf{a}_{198}, \mathbf{b}_{198}, \mathbf{c}_{198}) \begin{pmatrix} 1 & 0 & 0 \\ 0 & -1 & 0 \\ 0 & 0 & -1 \end{pmatrix}, \overrightarrow{O_{198}O_{146}} = -\frac{1}{6}\mathbf{a}_{146} + \left(\frac{5}{6}\right)\mathbf{b}_{146} + \left(-\frac{2}{3}\right)\mathbf{c}_{146}$$

The reduction of higher dimensional irrep:

$$T : T \rightarrow A + {}^2E + {}^1E \text{ of } C_3.$$

The correspondences of irreps at HSPs from original SG to lowered SG:

$$\begin{aligned} n_{GM4}^{146} &= n_{GM6}^{198} + n_{GM7}^{198} n_{GM6}^{146} = n_{GM5}^{198} + n_{GM6}^{198} n_{GM5}^{146} = n_{GM5}^{198} + n_{GM7}^{198} n_{L2}^{146} = n_{X2}^{198} + n_{X3}^{198} + n_{X4}^{198} + n_{X5}^{198} n_{F2}^{146} = 2n_{M5}^{198} \\ n_{T4}^{146} &= n_{R4}^{198} + n_{R7}^{198} n_{T6}^{146} = n_{R6}^{198} + n_{R7}^{198} n_{T5}^{146} = n_{R5}^{198} + n_{R7}^{198} \end{aligned}$$

The lower SG is SG 146 when the preserved operations are: **(sub-SG label is 5) 1, 10, 9.**

$$\text{The transformation is: } (\mathbf{a}_{146}, \mathbf{b}_{146}, \mathbf{c}_{146}) = (\mathbf{a}_{198}, \mathbf{b}_{198}, \mathbf{c}_{198}) \begin{pmatrix} -1 & 0 & 0 \\ 0 & 1 & 0 \\ 0 & 0 & -1 \end{pmatrix}, \overrightarrow{O_{198}O_{146}} = -\frac{2}{3}\mathbf{a}_{146} + \left(\frac{5}{6}\right)\mathbf{b}_{146} + \left(-\frac{1}{6}\right)\mathbf{c}_{146}$$

The reduction of higher dimensional irrep:

$$T : T \rightarrow A + {}^2E + {}^1E \text{ of } C_3.$$

The correspondences of irreps at HSPs from original SG to lowered SG:

$$\begin{aligned} n_{GM4}^{146} &= n_{GM6}^{198} + n_{GM7}^{198} n_{GM6}^{146} = n_{GM5}^{198} + n_{GM6}^{198} n_{GM5}^{146} = n_{GM5}^{198} + n_{GM7}^{198} n_{L2}^{146} = n_{X2}^{198} + n_{X3}^{198} + n_{X4}^{198} + n_{X5}^{198} n_{F2}^{146} = 2n_{M5}^{198} \\ n_{T4}^{146} &= n_{R4}^{198} + n_{R7}^{198} n_{T6}^{146} = n_{R6}^{198} + n_{R7}^{198} n_{T5}^{146} = n_{R5}^{198} + n_{R7}^{198} \end{aligned}$$

## 96. Lowered SGs by higher-dimensional irreps of pairings in SG 199

The representative operations of SG/T for SG 199:

$$\begin{aligned} 1 : (x, y, z), 2 : (x, -y, \frac{1}{2} - z), 3 : (\frac{1}{2} - x, y, -z), 4 : (-x, \frac{1}{2} - y, z), 5 : (z, x, y), 6 : (y, z, x), 7 : (\frac{1}{2} - y, z, -x), \\ 8 : (-z, \frac{1}{2} - x, y), 9 : (-y, \frac{1}{2} - z, x), 10 : (z, -x, \frac{1}{2} - y), 11 : (y, -z, \frac{1}{2} - x), 12 : (\frac{1}{2} - z, x, -y). \end{aligned}$$

The lower SG is SG 24 when the preserved operations are: **(sub-SG label is 1) 1, 2, 3, 4.**

$$\text{The transformation is: } (\mathbf{a}_{24}, \mathbf{b}_{24}, \mathbf{c}_{24}) = (\mathbf{a}_{199}, \mathbf{b}_{199}, \mathbf{c}_{199}) \begin{pmatrix} 0 & -1 & 0 \\ 0 & 0 & -1 \\ 1 & 0 & 0 \end{pmatrix}, \overrightarrow{O_{199}O_{24}} = -\frac{1}{2}\mathbf{b}_{24}$$

The reduction of higher dimensional irrep:

$$T : T \rightarrow B_1 + B_2 + B_3 \text{ of } D_2.$$

The correspondences of irreps at HSPs from original SG to lowered SG:

$$\begin{aligned} n_{GM5}^{24} &= n_{GM5}^{199} + n_{GM6}^{199} n_{GM5}^{24} = n_{H5}^{199} + n_{H6}^{199} + n_{H7}^{199} n_{T3}^{24} = n_{N4}^{199} n_{T4}^{24} = n_{N3}^{199} n_{W3}^{24} = n_{P7}^{199} n_{W2}^{24} = n_{P7}^{199} n_{W4}^{24} = \\ n_{P4}^{199} + n_{P5}^{199} + n_{P6}^{199} n_{W5}^{24} &= n_{P7}^{199} n_{R3}^{24} = n_{N4}^{199} n_{R4}^{24} = n_{N3}^{199} n_{S4}^{24} = n_{N4}^{199} n_{S3}^{24} = n_{N3}^{199} \end{aligned}$$

The lower SG is SG 146 when the preserved operations are: **(sub-SG label is 2) 1, 5, 6.**

The transformation is:  $(\mathbf{a}_{146}, \mathbf{b}_{146}, \mathbf{c}_{146}) = (\mathbf{a}_{199}, \mathbf{b}_{199}, \mathbf{c}_{199}) \begin{pmatrix} \frac{1}{2} & -\frac{1}{2} & \frac{1}{2} \\ \frac{1}{2} & \frac{1}{2} & -\frac{1}{2} \\ -\frac{1}{2} & \frac{1}{2} & \frac{1}{2} \end{pmatrix}, \overrightarrow{O_{199}O_{146}} = -\frac{1}{3}\mathbf{a}_{146} + (\frac{2}{3})\mathbf{b}_{146} + (-\frac{1}{3})\mathbf{c}_{146}$

The reduction of higher dimensional irrep:

$T : T \rightarrow A + {}^2E + {}^1E$  of  $C_3$ .

The correspondences of irreps at HSPs from original SG to lowered SG:

$$\begin{aligned} n_{GM4}^{146} &= n_{GM6}^{199} + n_{GM7}^{199} & n_{GM6}^{146} &= n_{GM5}^{199} + n_{GM6}^{199} & n_{GM5}^{146} &= n_{GM5}^{199} + n_{GM7}^{199} & n_{L2}^{146} &= n_{N3}^{199} + n_{N4}^{199} & n_{F2}^{146} &= n_{N3}^{199} + n_{N4}^{199} & n_{T4}^{146} &= \\ n_{H6}^{199} + n_{H7}^{199} & n_{T6}^{146} &= n_{H5}^{199} + n_{H6}^{199} & n_{T5}^{146} &= n_{H5}^{199} + n_{H7}^{199} \end{aligned}$$

The lower SG is SG 146 when the preserved operations are: **(sub-SG label is 3) 1, 12, 11.**

The transformation is:  $(\mathbf{a}_{146}, \mathbf{b}_{146}, \mathbf{c}_{146}) = (\mathbf{a}_{199}, \mathbf{b}_{199}, \mathbf{c}_{199}) \begin{pmatrix} -\frac{1}{2} & \frac{1}{2} & \frac{1}{2} \\ \frac{1}{2} & \frac{1}{2} & -\frac{1}{2} \\ -\frac{1}{2} & \frac{1}{2} & -\frac{1}{2} \end{pmatrix}, \overrightarrow{O_{199}O_{146}} = -\frac{1}{2}\mathbf{a}_{146} + (\frac{1}{2})\mathbf{b}_{146}$

The reduction of higher dimensional irrep:

$T : T \rightarrow A + {}^2E + {}^1E$  of  $C_3$ .

The correspondences of irreps at HSPs from original SG to lowered SG:

$$\begin{aligned} n_{GM4}^{146} &= n_{GM6}^{199} + n_{GM7}^{199} & n_{GM6}^{146} &= n_{GM5}^{199} + n_{GM6}^{199} & n_{GM5}^{146} &= n_{GM5}^{199} + n_{GM7}^{199} & n_{L2}^{146} &= n_{N3}^{199} + n_{N4}^{199} & n_{F2}^{146} &= n_{N3}^{199} + n_{N4}^{199} & n_{T4}^{146} &= \\ n_{H6}^{199} + n_{H7}^{199} & n_{T6}^{146} &= n_{H5}^{199} + n_{H6}^{199} & n_{T5}^{146} &= n_{H5}^{199} + n_{H7}^{199} \end{aligned}$$

The lower SG is SG 146 when the preserved operations are: **(sub-SG label is 4) 1, 8, 7.**

The transformation is:  $(\mathbf{a}_{146}, \mathbf{b}_{146}, \mathbf{c}_{146}) = (\mathbf{a}_{199}, \mathbf{b}_{199}, \mathbf{c}_{199}) \begin{pmatrix} \frac{1}{2} & -\frac{1}{2} & \frac{1}{2} \\ -\frac{1}{2} & -\frac{1}{2} & \frac{1}{2} \\ \frac{1}{2} & -\frac{1}{2} & -\frac{1}{2} \end{pmatrix}, \overrightarrow{O_{199}O_{146}} = -\frac{1}{3}\mathbf{a}_{146} + (\frac{1}{6})\mathbf{b}_{146} + (\frac{1}{6})\mathbf{c}_{146}$

The reduction of higher dimensional irrep:

$T : T \rightarrow A + {}^2E + {}^1E$  of  $C_3$ .

The correspondences of irreps at HSPs from original SG to lowered SG:

$$\begin{aligned} n_{GM4}^{146} &= n_{GM6}^{199} + n_{GM7}^{199} & n_{GM6}^{146} &= n_{GM5}^{199} + n_{GM6}^{199} & n_{GM5}^{146} &= n_{GM5}^{199} + n_{GM7}^{199} & n_{L2}^{146} &= n_{N3}^{199} + n_{N4}^{199} & n_{F2}^{146} &= n_{N3}^{199} + n_{N4}^{199} & n_{T4}^{146} &= \\ n_{H6}^{199} + n_{H7}^{199} & n_{T6}^{146} &= n_{H5}^{199} + n_{H6}^{199} & n_{T5}^{146} &= n_{H5}^{199} + n_{H7}^{199} \end{aligned}$$

The lower SG is SG 146 when the preserved operations are: **(sub-SG label is 5) 1, 10, 9.**

The transformation is:  $(\mathbf{a}_{146}, \mathbf{b}_{146}, \mathbf{c}_{146}) = (\mathbf{a}_{199}, \mathbf{b}_{199}, \mathbf{c}_{199}) \begin{pmatrix} -\frac{1}{2} & -\frac{1}{2} & \frac{1}{2} \\ -\frac{1}{2} & \frac{1}{2} & \frac{1}{2} \\ -\frac{1}{2} & \frac{1}{2} & -\frac{1}{2} \end{pmatrix}, \overrightarrow{O_{199}O_{146}} = -\frac{1}{2}\mathbf{a}_{146} + (\frac{1}{2})\mathbf{b}_{146}$

The reduction of higher dimensional irrep:

$T : T \rightarrow A + {}^2E + {}^1E$  of  $C_3$ .

The correspondences of irreps at HSPs from original SG to lowered SG:

$$\begin{aligned} n_{GM4}^{146} &= n_{GM6}^{199} + n_{GM7}^{199} & n_{GM6}^{146} &= n_{GM5}^{199} + n_{GM6}^{199} & n_{GM5}^{146} &= n_{GM5}^{199} + n_{GM7}^{199} & n_{L2}^{146} &= n_{N3}^{199} + n_{N4}^{199} & n_{F2}^{146} &= n_{N3}^{199} + n_{N4}^{199} & n_{T4}^{146} &= \\ n_{H6}^{199} + n_{H7}^{199} & n_{T6}^{146} &= n_{H5}^{199} + n_{H6}^{199} & n_{T5}^{146} &= n_{H5}^{199} + n_{H7}^{199} \end{aligned}$$

## 97. Lowered SGs by higher-dimensional irreps of pairings in SG 200

The representative operations of SG/T for SG 200:

1 :  $(x, y, z)$ , 2 :  $(x, -y, -z)$ , 3 :  $(-x, y, -z)$ , 4 :  $(-x, -y, z)$ , 5 :  $(z, x, y)$ , 6 :  $(y, z, x)$ , 7 :  $(-y, z, -x)$ , 8 :  $(-z, -x, y)$ ,  
 9 :  $(-y, -z, x)$ , 10 :  $(z, -x, -y)$ , 11 :  $(y, -z, -x)$ , 12 :  $(-z, x, -y)$ , 13 :  $(-x, -y, -z)$ , 14 :  $(-x, y, z)$ , 15 :  $(x, -y, z)$ ,  
 16 :  $(x, y, -z)$ , 17 :  $(-z, -x, -y)$ , 18 :  $(-y, -z, -x)$ , 19 :  $(y, -z, x)$ , 20 :  $(z, x, -y)$ , 21 :  $(y, z, -x)$ , 22 :  $(-z, x, y)$ ,  
 23 :  $(-y, z, x)$ , 24 :  $(z, -x, y)$ .

The lower SG is SG 47 when the preserved operations are: **(sub-SG label is 1) 1, 2, 3, 4, 13, 14, 15, 16.**

The transformation is:  $(\mathbf{a}_{47}, \mathbf{b}_{47}, \mathbf{c}_{47}) = (\mathbf{a}_{200}, \mathbf{b}_{200}, \mathbf{c}_{200}) \begin{pmatrix} 0 & 0 & 1 \\ 1 & 0 & 0 \\ 0 & 1 & 0 \end{pmatrix}, \overrightarrow{O_{200}O_{47}} = \frac{1}{2}\mathbf{a}_{47} + (\frac{1}{2})\mathbf{c}_{47}$

The reduction of higher dimensional irrep:

$$T_h : T_g \rightarrow B_{2g} + B_{1g} + B_{3g} \text{ of } D_{2h}.$$

$$T_h : T_u \rightarrow B_{2u} + B_{1u} + B_{3u} \text{ of } D_{2h}.$$

The correspondences of irreps at HSPs from original SG to lowered SG:

$$\begin{aligned} n_{GM6}^{47} &= n_{GM10}^{200} + n_{GM8}^{200} + n_{GM9}^{200} & n_{GM5}^{47} &= n_{GM5}^{200} + n_{GM6}^{200} + n_{GM7}^{200} & n_{X6}^{47} &= n_{X5}^{200} & n_{X5}^{47} &= n_{X5}^{200} & n_{X6}^{47} &= n_{X6}^{200} & n_{S6}^{47} &= n_{M5}^{200} & n_{S5}^{47} &= n_{M6}^{200} & n_{R6}^{47} &= n_{R6}^{200} \\ n_{R10}^{200} + n_{R8}^{200} + n_{R9}^{200} & n_{R5}^{47} &= n_{R5}^{200} + n_{R6}^{200} & + n_{R7}^{200} & n_{U6}^{47} &= n_{M6}^{200} & n_{U5}^{47} &= n_{M5}^{200} & n_{Z6}^{47} &= n_{X5}^{200} & n_{Z5}^{47} &= n_{X6}^{200} & n_{T6}^{47} &= n_{M5}^{200} & n_{T5}^{47} &= n_{M6}^{200} \\ n_{Y6}^{47} &= n_{X6}^{200} & n_{Y5}^{47} &= n_{X5}^{200} \end{aligned}$$

The lower SG is SG 148 when the preserved operations are: **(sub-SG label is 2) 1, 5, 6, 13, 17, 18.**

$$\text{The transformation is: } (\mathbf{a}_{148}, \mathbf{b}_{148}, \mathbf{c}_{148}) = (\mathbf{a}_{200}, \mathbf{b}_{200}, \mathbf{c}_{200}) \begin{pmatrix} 0 & 1 & 0 \\ 0 & 0 & 1 \\ 1 & 0 & 0 \end{pmatrix}, \overrightarrow{O_{200}O_{148}} = \mathbf{0}$$

The reduction of higher dimensional irrep:

$$T_h : T_g \rightarrow A_g + {}^2E_g + {}^1E_g \text{ of } C_{3i}.$$

$$T_h : T_u \rightarrow {}^1E_u + A_u + {}^2E_u \text{ of } C_{3i}.$$

The correspondences of irreps at HSPs from original SG to lowered SG:

$$\begin{aligned} n_{GM7}^{148} &= n_{GM10}^{200} + n_{GM9}^{200} & n_{GM4}^{148} &= n_{GM6}^{200} + n_{GM7}^{200} & n_{GM9}^{148} &= n_{GM8}^{200} + n_{GM9}^{200} & n_{GM6}^{148} &= n_{GM5}^{200} + n_{GM6}^{200} & n_{GM8}^{148} &= n_{GM10}^{200} + n_{GM8}^{200} \\ n_{GM5}^{148} &= n_{GM5}^{200} + n_{GM7}^{200} & n_{L2}^{148} &= 2n_{X6}^{200} & n_{L3}^{148} &= 2n_{X5}^{200} & n_{F2}^{148} &= 2n_{M6}^{200} & n_{F3}^{148} &= 2n_{M5}^{200} & n_{T7}^{148} &= n_{R10}^{200} + n_{R9}^{200} & n_{T4}^{148} &= n_{R6}^{200} + n_{R7}^{200} \\ n_{T9}^{148} &= n_{R8}^{200} + n_{R9}^{200} & n_{T6}^{148} &= n_{R5}^{200} + n_{R6}^{200} & n_{T8}^{148} &= n_{R10}^{200} + n_{R8}^{200} & n_{T5}^{148} &= n_{R5}^{200} + n_{R7}^{200} \end{aligned}$$

The lower SG is SG 148 when the preserved operations are: **(sub-SG label is 3) 1, 12, 11, 13, 24, 23.**

$$\text{The transformation is: } (\mathbf{a}_{148}, \mathbf{b}_{148}, \mathbf{c}_{148}) = (\mathbf{a}_{200}, \mathbf{b}_{200}, \mathbf{c}_{200}) \begin{pmatrix} 0 & -1 & 0 \\ 0 & 0 & -1 \\ 1 & 0 & 0 \end{pmatrix}, \overrightarrow{O_{200}O_{148}} = \mathbf{0}$$

The reduction of higher dimensional irrep:

$$T_h : T_g \rightarrow A_g + {}^2E_g + {}^1E_g \text{ of } C_{3i}.$$

$$T_h : T_u \rightarrow {}^1E_u + A_u + {}^2E_u \text{ of } C_{3i}.$$

The correspondences of irreps at HSPs from original SG to lowered SG:

$$\begin{aligned} n_{GM7}^{148} &= n_{GM10}^{200} + n_{GM9}^{200} & n_{GM4}^{148} &= n_{GM6}^{200} + n_{GM7}^{200} & n_{GM9}^{148} &= n_{GM8}^{200} + n_{GM9}^{200} & n_{GM6}^{148} &= n_{GM5}^{200} + n_{GM6}^{200} & n_{GM8}^{148} &= n_{GM10}^{200} + n_{GM8}^{200} \\ n_{GM5}^{148} &= n_{GM5}^{200} + n_{GM7}^{200} & n_{L2}^{148} &= 2n_{X6}^{200} & n_{L3}^{148} &= 2n_{X5}^{200} & n_{F2}^{148} &= 2n_{M6}^{200} & n_{F3}^{148} &= 2n_{M5}^{200} & n_{T7}^{148} &= n_{R10}^{200} + n_{R9}^{200} & n_{T4}^{148} &= n_{R6}^{200} + n_{R7}^{200} \\ n_{T9}^{148} &= n_{R8}^{200} + n_{R9}^{200} & n_{T6}^{148} &= n_{R5}^{200} + n_{R6}^{200} & n_{T8}^{148} &= n_{R10}^{200} + n_{R8}^{200} & n_{T5}^{148} &= n_{R5}^{200} + n_{R7}^{200} \end{aligned}$$

The lower SG is SG 148 when the preserved operations are: **(sub-SG label is 4) 1, 8, 7, 13, 20, 19.**

$$\text{The transformation is: } (\mathbf{a}_{148}, \mathbf{b}_{148}, \mathbf{c}_{148}) = (\mathbf{a}_{200}, \mathbf{b}_{200}, \mathbf{c}_{200}) \begin{pmatrix} 1 & 0 & 0 \\ 0 & -1 & 0 \\ 0 & 0 & -1 \end{pmatrix}, \overrightarrow{O_{200}O_{148}} = \mathbf{0}$$

The reduction of higher dimensional irrep:

$$T_h : T_g \rightarrow A_g + {}^2E_g + {}^1E_g \text{ of } C_{3i}.$$

$$T_h : T_u \rightarrow {}^1E_u + A_u + {}^2E_u \text{ of } C_{3i}.$$

The correspondences of irreps at HSPs from original SG to lowered SG:

$$\begin{aligned} n_{GM7}^{148} &= n_{GM10}^{200} + n_{GM9}^{200} & n_{GM4}^{148} &= n_{GM6}^{200} + n_{GM7}^{200} & n_{GM9}^{148} &= n_{GM8}^{200} + n_{GM9}^{200} & n_{GM6}^{148} &= n_{GM5}^{200} + n_{GM6}^{200} & n_{GM8}^{148} &= n_{GM10}^{200} + n_{GM8}^{200} \\ n_{GM5}^{148} &= n_{GM5}^{200} + n_{GM7}^{200} & n_{L2}^{148} &= 2n_{X6}^{200} & n_{L3}^{148} &= 2n_{X5}^{200} & n_{F2}^{148} &= 2n_{M6}^{200} & n_{F3}^{148} &= 2n_{M5}^{200} & n_{T7}^{148} &= n_{R10}^{200} + n_{R9}^{200} & n_{T4}^{148} &= n_{R6}^{200} + n_{R7}^{200} \\ n_{T9}^{148} &= n_{R8}^{200} + n_{R9}^{200} & n_{T6}^{148} &= n_{R5}^{200} + n_{R6}^{200} & n_{T8}^{148} &= n_{R10}^{200} + n_{R8}^{200} & n_{T5}^{148} &= n_{R5}^{200} + n_{R7}^{200} \end{aligned}$$

The lower SG is SG 148 when the preserved operations are: **(sub-SG label is 5) 1, 10, 9, 13, 22, 21.**

$$\text{The transformation is: } (\mathbf{a}_{148}, \mathbf{b}_{148}, \mathbf{c}_{148}) = (\mathbf{a}_{200}, \mathbf{b}_{200}, \mathbf{c}_{200}) \begin{pmatrix} -1 & 0 & 0 \\ 0 & 1 & 0 \\ 0 & 0 & -1 \end{pmatrix}, \overrightarrow{O_{200}O_{148}} = \mathbf{0}$$

The reduction of higher dimensional irrep:

$$T_h : T_g \rightarrow A_g + {}^2E_g + {}^1E_g \text{ of } C_{3i}.$$

$$T_h : T_u \rightarrow {}^1E_u + A_u + {}^2E_u \text{ of } C_{3i}.$$

The correspondences of irreps at HSPs from original SG to lowered SG:

$$\begin{aligned} n_{GM7}^{148} &= n_{GM10}^{200} + n_{GM9}^{200} & n_{GM4}^{148} &= n_{GM6}^{200} + n_{GM7}^{200} & n_{GM9}^{148} &= n_{GM8}^{200} + n_{GM9}^{200} & n_{GM6}^{148} &= n_{GM5}^{200} + n_{GM6}^{200} & n_{GM8}^{148} &= n_{GM10}^{200} + n_{GM8}^{200} \\ n_{GM5}^{148} &= n_{GM5}^{200} + n_{GM7}^{200} & n_{L2}^{148} &= 2n_{X6}^{200} & n_{L3}^{148} &= 2n_{X5}^{200} & n_{F2}^{148} &= 2n_{M6}^{200} & n_{F3}^{148} &= 2n_{M5}^{200} & n_{T7}^{148} &= n_{R10}^{200} + n_{R9}^{200} & n_{T4}^{148} &= n_{R6}^{200} + n_{R7}^{200} \\ n_{T9}^{148} &= n_{R8}^{200} + n_{R9}^{200} & n_{T6}^{148} &= n_{R5}^{200} + n_{R6}^{200} & n_{T8}^{148} &= n_{R10}^{200} + n_{R8}^{200} & n_{T5}^{148} &= n_{R5}^{200} + n_{R7}^{200} \end{aligned}$$

98. Lowered SGs by higher-dimensional irreps of pairings in SG 201

The representative operations of SG/T for SG 201:

$$\begin{aligned}
 &1 : (x, y, z), 2 : (x, \frac{1}{2} - y, \frac{1}{2} - z), 3 : (\frac{1}{2} - x, y, \frac{1}{2} - z), 4 : (\frac{1}{2} - x, \frac{1}{2} - y, z), 5 : (z, x, y), 6 : (y, z, x), 7 : (\frac{1}{2} - y, z, \frac{1}{2} - x), \\
 &8 : (\frac{1}{2} - z, \frac{1}{2} - x, y), 9 : (\frac{1}{2} - y, \frac{1}{2} - z, x), 10 : (z, \frac{1}{2} - x, \frac{1}{2} - y), 11 : (y, \frac{1}{2} - z, \frac{1}{2} - x), 12 : (\frac{1}{2} - z, x, \frac{1}{2} - y), \\
 &13 : (-x, -y, -z), 14 : (-x, y + \frac{1}{2}, z + \frac{1}{2}), 15 : (x + \frac{1}{2}, -y, z + \frac{1}{2}), 16 : (x + \frac{1}{2}, y + \frac{1}{2}, -z), 17 : (-z, -x, -y), \\
 &18 : (-y, -z, -x), 19 : (y + \frac{1}{2}, -z, x + \frac{1}{2}), 20 : (z + \frac{1}{2}, x + \frac{1}{2}, -y), 21 : (y + \frac{1}{2}, z + \frac{1}{2}, -x), 22 : (-z, x + \frac{1}{2}, y + \frac{1}{2}), \\
 &23 : (-y, z + \frac{1}{2}, x + \frac{1}{2}), 24 : (z + \frac{1}{2}, -x, y + \frac{1}{2}).
 \end{aligned}$$

The lower SG is SG 48 when the preserved operations are: **(sub-SG label is 1)** 1, 2, 3, 4, 13, 14, 15, 16.

The transformation is:  $(\mathbf{a}_{48}, \mathbf{b}_{48}, \mathbf{c}_{48}) = (\mathbf{a}_{201}, \mathbf{b}_{201}, \mathbf{c}_{201}) \begin{pmatrix} 0 & 0 & 1 \\ 1 & 0 & 0 \\ 0 & 1 & 0 \end{pmatrix}, \overrightarrow{O_{201}O_{48}} = \frac{1}{2}\mathbf{a}_{48} + (\frac{1}{2})\mathbf{c}_{48}$

The reduction of higher dimensional irrep:

$$T_h : T_g \rightarrow B_{2g} + B_{1g} + B_{3g} \text{ of } D_{2h}.$$

$$T_h : T_u \rightarrow B_{2u} + B_{1u} + B_{3u} \text{ of } D_{2h}.$$

The correspondences of irreps at HSPs from original SG to lowered SG:

$$\begin{aligned}
 n_{GM6}^{48} &= n_{GM10}^{201} + n_{GM8}^{201} + n_{GM9}^{201} \quad n_{GM5}^{48} = n_{GM5}^{201} + n_{GM6}^{201} + n_{GM7}^{201} \quad n_{X4}^{48} = n_{X3}^{201} \quad n_{X3}^{48} = n_{X4}^{201} \quad n_{S3}^{48} = n_{M3}^{201} \quad n_{S4}^{48} = n_{M4}^{201} \quad n_{R6}^{48} = \\
 n_{R10}^{201} + n_{R8}^{201} + n_{R9}^{201} \quad n_{R5}^{48} &= n_{R5}^{201} + n_{R6}^{201} + n_{R7}^{201} \quad n_{U3}^{48} = n_{M3}^{201} \quad n_{U4}^{48} = n_{M4}^{201} \quad n_{Z4}^{48} = n_{X3}^{201} \quad n_{Z3}^{48} = n_{X4}^{201} \quad n_{T4}^{48} = n_{M4}^{201} \quad n_{T3}^{48} = n_{M3}^{201} \\
 n_{Y4}^{48} &= n_{X4}^{201} \quad n_{Y3}^{48} = n_{X3}^{201}
 \end{aligned}$$

The lower SG is SG 148 when the preserved operations are: **(sub-SG label is 2)** 1, 5, 6, 13, 17, 18.

The transformation is:  $(\mathbf{a}_{148}, \mathbf{b}_{148}, \mathbf{c}_{148}) = (\mathbf{a}_{201}, \mathbf{b}_{201}, \mathbf{c}_{201}) \begin{pmatrix} 0 & 1 & 0 \\ 0 & 0 & 1 \\ 1 & 0 & 0 \end{pmatrix}, \overrightarrow{O_{201}O_{148}} = \mathbf{0}$

The reduction of higher dimensional irrep:

$$T_h : T_g \rightarrow A_g + {}^2E_g + {}^1E_g \text{ of } C_{3i}.$$

$$T_h : T_u \rightarrow {}^1E_u + A_u + {}^2E_u \text{ of } C_{3i}.$$

The correspondences of irreps at HSPs from original SG to lowered SG:

$$\begin{aligned}
 n_{GM7}^{148} &= n_{GM10}^{201} + n_{GM9}^{201} \quad n_{GM4}^{148} = n_{GM6}^{201} + n_{GM7}^{201} \quad n_{GM9}^{148} = n_{GM8}^{201} + n_{GM9}^{201} \quad n_{GM6}^{148} = n_{GM5}^{201} + n_{GM6}^{201} \quad n_{GM8}^{148} = n_{GM10}^{201} + n_{GM8}^{201} \\
 n_{GM5}^{148} &= n_{GM5}^{201} + n_{GM7}^{201} \quad n_{L2}^{148} = n_{X3}^{201} + n_{X4}^{201} \quad n_{L3}^{148} = n_{X3}^{201} + n_{X4}^{201} \quad n_{F2}^{148} = n_{M3}^{201} + n_{M4}^{201} \quad n_{F3}^{148} = n_{M3}^{201} + n_{M4}^{201} \quad n_{T7}^{148} = n_{R10}^{201} + n_{R9}^{201} \\
 n_{T4}^{148} &= n_{R6}^{201} + n_{R7}^{201} \quad n_{T9}^{148} = n_{R8}^{201} + n_{R9}^{201} \quad n_{T6}^{148} = n_{R5}^{201} + n_{R6}^{201} \quad n_{T8}^{148} = n_{R10}^{201} + n_{R8}^{201} \quad n_{T5}^{148} = n_{R5}^{201} + n_{R7}^{201}
 \end{aligned}$$

The lower SG is SG 148 when the preserved operations are: **(sub-SG label is 3)** 1, 12, 11, 13, 24, 23.

The transformation is:  $(\mathbf{a}_{148}, \mathbf{b}_{148}, \mathbf{c}_{148}) = (\mathbf{a}_{201}, \mathbf{b}_{201}, \mathbf{c}_{201}) \begin{pmatrix} 0 & -1 & 0 \\ 0 & 0 & -1 \\ 1 & 0 & 0 \end{pmatrix}, \overrightarrow{O_{201}O_{148}} = \frac{1}{2}\mathbf{b}_{148} + (\frac{1}{2})\mathbf{c}_{148}$

The reduction of higher dimensional irrep:

$$T_h : T_g \rightarrow A_g + {}^2E_g + {}^1E_g \text{ of } C_{3i}.$$

$$T_h : T_u \rightarrow {}^1E_u + A_u + {}^2E_u \text{ of } C_{3i}.$$

The correspondences of irreps at HSPs from original SG to lowered SG:

$$\begin{aligned}
 n_{GM7}^{148} &= n_{GM10}^{201} + n_{GM9}^{201} \quad n_{GM4}^{148} = n_{GM6}^{201} + n_{GM7}^{201} \quad n_{GM9}^{148} = n_{GM8}^{201} + n_{GM9}^{201} \quad n_{GM6}^{148} = n_{GM5}^{201} + n_{GM6}^{201} \quad n_{GM8}^{148} = n_{GM10}^{201} + n_{GM8}^{201} \\
 n_{GM5}^{148} &= n_{GM5}^{201} + n_{GM7}^{201} \quad n_{L2}^{148} = n_{X3}^{201} + n_{X4}^{201} \quad n_{L3}^{148} = n_{X3}^{201} + n_{X4}^{201} \quad n_{F2}^{148} = n_{M3}^{201} + n_{M4}^{201} \quad n_{F3}^{148} = n_{M3}^{201} + n_{M4}^{201} \quad n_{T7}^{148} = n_{R10}^{201} + n_{R9}^{201} \\
 n_{T4}^{148} &= n_{R6}^{201} + n_{R7}^{201} \quad n_{T9}^{148} = n_{R8}^{201} + n_{R9}^{201} \quad n_{T6}^{148} = n_{R5}^{201} + n_{R6}^{201} \quad n_{T8}^{148} = n_{R10}^{201} + n_{R8}^{201} \quad n_{T5}^{148} = n_{R5}^{201} + n_{R7}^{201}
 \end{aligned}$$

The lower SG is SG 148 when the preserved operations are: **(sub-SG label is 4)** 1, 8, 7, 13, 20, 19.

The transformation is:  $(\mathbf{a}_{148}, \mathbf{b}_{148}, \mathbf{c}_{148}) = (\mathbf{a}_{201}, \mathbf{b}_{201}, \mathbf{c}_{201}) \begin{pmatrix} 1 & 0 & 0 \\ 0 & -1 & 0 \\ 0 & 0 & -1 \end{pmatrix}, \overrightarrow{O_{201}O_{148}} = \frac{1}{2}\mathbf{b}_{148} + (\frac{1}{2})\mathbf{c}_{148}$

The reduction of higher dimensional irrep:

$$T_h : T_g \rightarrow A_g + {}^2E_g + {}^1E_g \text{ of } C_{3i}.$$

$$T_h : T_u \rightarrow {}^1E_u + A_u + {}^2E_u \text{ of } C_{3i}.$$

The correspondences of irreps at HSPs from original SG to lowered SG:

$$n_{GM7}^{148} = n_{GM10}^{201} + n_{GM9}^{201} \quad n_{GM4}^{148} = n_{GM6}^{201} + n_{GM7}^{201} \quad n_{GM9}^{148} = n_{GM8}^{201} + n_{GM9}^{201} \quad n_{GM6}^{148} = n_{GM5}^{201} + n_{GM6}^{201} \quad n_{GM8}^{148} = n_{GM10}^{201} + n_{GM8}^{201}$$

$$\begin{aligned} n_{GM5}^{148} &= n_{GM5}^{201} + n_{GM7}^{201} n_{L2}^{148} = n_{X3}^{201} + n_{X4}^{201} n_{L3}^{148} = n_{X3}^{201} + n_{X4}^{201} n_{F2}^{148} = n_{M3}^{201} + n_{M4}^{201} n_{F3}^{148} = n_{M3}^{201} + n_{M4}^{201} n_{T7}^{148} = n_{R10}^{201} + n_{R9}^{201} \\ n_{T4}^{148} &= n_{R6}^{201} + n_{R7}^{201} n_{T9}^{148} = n_{R8}^{201} + n_{R9}^{201} n_{T6}^{148} = n_{R5}^{201} + n_{R6}^{201} n_{T8}^{148} = n_{R10}^{201} + n_{R8}^{201} n_{T5}^{148} = n_{R5}^{201} + n_{R7}^{201} \end{aligned}$$

The lower SG is SG 148 when the preserved operations are: **(sub-SG label is 5) 1, 10, 9, 13, 22, 21.**

The transformation is:  $(\mathbf{a}_{148}, \mathbf{b}_{148}, \mathbf{c}_{148}) = (\mathbf{a}_{201}, \mathbf{b}_{201}, \mathbf{c}_{201}) \begin{pmatrix} -1 & 0 & 0 \\ 0 & 1 & 0 \\ 0 & 0 & -1 \end{pmatrix}, \overrightarrow{O_{201}O_{148}} = \frac{1}{2}\mathbf{b}_{148}$

The reduction of higher dimensional irrep:

$$T_h : \mathbf{T}_g \rightarrow A_g + {}^2E_g + {}^1E_g \text{ of } C_{3i}.$$

$$T_h : \mathbf{T}_u \rightarrow {}^1E_u + A_u + {}^2E_u \text{ of } C_{3i}.$$

The correspondences of irreps at HSPs from original SG to lowered SG:

$$\begin{aligned} n_{GM7}^{148} &= n_{GM10}^{201} + n_{GM9}^{201} n_{GM4}^{148} = n_{GM6}^{201} + n_{GM7}^{201} n_{GM9}^{148} = n_{GM8}^{201} + n_{GM9}^{201} n_{GM6}^{148} = n_{GM5}^{201} + n_{GM6}^{201} n_{GM8}^{148} = n_{GM10}^{201} + n_{GM8}^{201} \\ n_{GM5}^{148} &= n_{GM5}^{201} + n_{GM7}^{201} n_{L2}^{148} = n_{X3}^{201} + n_{X4}^{201} n_{L3}^{148} = n_{X3}^{201} + n_{X4}^{201} n_{F2}^{148} = n_{M3}^{201} + n_{M4}^{201} n_{F3}^{148} = n_{M3}^{201} + n_{M4}^{201} n_{T7}^{148} = n_{R6}^{201} + n_{R7}^{201} \\ n_{T4}^{148} &= n_{R10}^{201} + n_{R9}^{201} n_{T9}^{148} = n_{R5}^{201} + n_{R6}^{201} n_{T6}^{148} = n_{R8}^{201} + n_{R9}^{201} n_{T8}^{148} = n_{R5}^{201} + n_{R7}^{201} n_{T5}^{148} = n_{R10}^{201} + n_{R8}^{201} \end{aligned}$$

### 99. Lowered SGs by higher-dimensional irreps of pairings in SG 202

The representative operations of SG/T for SG 202:

$$\begin{aligned} &1 : (x, y, z), 2 : (x, -y, -z), 3 : (-x, y, -z), 4 : (-x, -y, z), 5 : (z, x, y), 6 : (y, z, x), 7 : (-y, z, -x), 8 : (-z, -x, y), \\ &9 : (-y, -z, x), 10 : (z, -x, -y), 11 : (y, -z, -x), 12 : (-z, x, -y), 13 : (-x, -y, -z), 14 : (-x, y, z), 15 : (x, -y, z), \\ &16 : (x, y, -z), 17 : (-z, -x, -y), 18 : (-y, -z, -x), 19 : (y, -z, x), 20 : (z, x, -y), 21 : (y, z, -x), 22 : (-z, x, y), \\ &23 : (-y, z, x), 24 : (z, -x, y). \end{aligned}$$

The lower SG is SG 69 when the preserved operations are: **(sub-SG label is 1) 1, 2, 3, 4, 13, 14, 15, 16.**

The transformation is:  $(\mathbf{a}_{69}, \mathbf{b}_{69}, \mathbf{c}_{69}) = (\mathbf{a}_{202}, \mathbf{b}_{202}, \mathbf{c}_{202}) \begin{pmatrix} 0 & 0 & 1 \\ 1 & 0 & 0 \\ 0 & 1 & 0 \end{pmatrix}, \overrightarrow{O_{202}O_{69}} = \mathbf{0}$

The reduction of higher dimensional irrep:

$$T_h : \mathbf{T}_g \rightarrow B_{2g} + B_{1g} + B_{3g} \text{ of } D_{2h}.$$

$$T_h : \mathbf{T}_u \rightarrow B_{2u} + B_{1u} + B_{3u} \text{ of } D_{2h}.$$

The correspondences of irreps at HSPs from original SG to lowered SG:

$$\begin{aligned} n_{GM6}^{69} &= n_{GM10}^{202} + n_{GM8}^{202} + n_{GM9}^{202} n_{GM5}^{69} = n_{GM5}^{202} + n_{GM6}^{202} + n_{GM7}^{202} n_{Y6}^{69} = n_{X6}^{202} n_{Y5}^{69} = n_{X5}^{202} n_{L2}^{69} = n_{L7}^{202} + n_{L8}^{202} + n_{L9}^{202} \\ n_{L3}^{69} &= n_{L4}^{202} + n_{L5}^{202} + n_{L6}^{202} n_{Z6}^{69} = n_{X6}^{202} n_{Z5}^{69} = n_{X5}^{202} n_{T6}^{69} = n_{X6}^{202} n_{T5}^{69} = n_{X5}^{202} \end{aligned}$$

The lower SG is SG 148 when the preserved operations are: **(sub-SG label is 2) 1, 5, 6, 13, 17, 18.**

The transformation is:  $(\mathbf{a}_{148}, \mathbf{b}_{148}, \mathbf{c}_{148}) = (\mathbf{a}_{202}, \mathbf{b}_{202}, \mathbf{c}_{202}) \begin{pmatrix} \frac{1}{2} & 0 & \frac{1}{2} \\ \frac{1}{2} & \frac{1}{2} & 0 \\ 0 & \frac{1}{2} & \frac{1}{2} \end{pmatrix}, \overrightarrow{O_{202}O_{148}} = \mathbf{0}$

The reduction of higher dimensional irrep:

$$T_h : \mathbf{T}_g \rightarrow A_g + {}^2E_g + {}^1E_g \text{ of } C_{3i}.$$

$$T_h : \mathbf{T}_u \rightarrow {}^1E_u + A_u + {}^2E_u \text{ of } C_{3i}.$$

The correspondences of irreps at HSPs from original SG to lowered SG:

$$\begin{aligned} n_{GM7}^{148} &= n_{GM10}^{202} + n_{GM9}^{202} n_{GM4}^{148} = n_{GM6}^{202} + n_{GM7}^{202} n_{GM9}^{148} = n_{GM8}^{202} + n_{GM9}^{202} n_{GM6}^{148} = n_{GM5}^{202} + n_{GM6}^{202} n_{GM8}^{148} = n_{GM10}^{202} + n_{GM8}^{202} \\ n_{GM5}^{148} &= n_{GM5}^{202} + n_{GM7}^{202} n_{L2}^{148} = n_{L7}^{202} + n_{L8}^{202} + n_{L9}^{202} n_{L3}^{148} = n_{L4}^{202} + n_{L5}^{202} + n_{L6}^{202} n_{F2}^{148} = 2n_{X6}^{202} n_{F3}^{148} = 2n_{X5}^{202} n_{T7}^{148} = n_{L7}^{202} \\ n_{T4}^{148} &= n_{L4}^{202} n_{T9}^{148} = n_{L9}^{202} n_{T6}^{148} = n_{L6}^{202} n_{T8}^{148} = n_{L8}^{202} n_{T5}^{148} = n_{L5}^{202} \end{aligned}$$

The lower SG is SG 148 when the preserved operations are: **(sub-SG label is 3) 1, 12, 11, 13, 24, 23.**

The transformation is:  $(\mathbf{a}_{148}, \mathbf{b}_{148}, \mathbf{c}_{148}) = (\mathbf{a}_{202}, \mathbf{b}_{202}, \mathbf{c}_{202}) \begin{pmatrix} -\frac{1}{2} & -\frac{1}{2} & 0 \\ 0 & -\frac{1}{2} & -\frac{1}{2} \\ \frac{1}{2} & 0 & \frac{1}{2} \end{pmatrix}, \overrightarrow{O_{202}O_{148}} = \mathbf{0}$

The reduction of higher dimensional irrep:

$$T_h : \mathbf{T}_g \rightarrow A_g + {}^2E_g + {}^1E_g \text{ of } C_{3i}.$$

$T_h : T_u \rightarrow {}^1E_u + A_u + {}^2E_u$  of  $C_{3i}$ .

The correspondences of irreps at HSPs from original SG to lowered SG:

$$\begin{aligned} n_{GM7}^{148} &= n_{GM10}^{202} + n_{GM9}^{202} n_{GM4}^{148} = n_{GM6}^{202} + n_{GM7}^{202} n_{GM9}^{148} = n_{GM8}^{202} + n_{GM9}^{202} n_{GM6}^{148} = n_{GM5}^{202} + n_{GM6}^{202} n_{GM8}^{148} = n_{GM10}^{202} + n_{GM8}^{202} \\ n_{GM5}^{148} &= n_{GM5}^{202} + n_{GM7}^{202} n_{L2}^{148} = n_{L7}^{202} + n_{L8}^{202} + n_{L9}^{202} n_{L3}^{148} = n_{L4}^{202} + n_{L5}^{202} + n_{L6}^{202} n_{F2}^{148} = 2n_{X6}^{202} n_{F3}^{148} = 2n_{X5}^{202} n_{T7}^{148} = n_{L7}^{202} \\ n_{T4}^{148} &= n_{L4}^{202} n_{T9}^{148} = n_{L9}^{202} n_{T6}^{148} = n_{L6}^{202} n_{T8}^{148} = n_{L8}^{202} n_{T5}^{148} = n_{L5}^{202} \end{aligned}$$

The lower SG is SG 148 when the preserved operations are: **(sub-SG label is 4)** 1, 8, 7, 13, 20, 19.

The transformation is:  $(\mathbf{a}_{148}, \mathbf{b}_{148}, \mathbf{c}_{148}) = (\mathbf{a}_{202}, \mathbf{b}_{202}, \mathbf{c}_{202}) \begin{pmatrix} \frac{1}{2} & 0 & \frac{1}{2} \\ -\frac{1}{2} & -\frac{1}{2} & 0 \\ 0 & -\frac{1}{2} & -\frac{1}{2} \end{pmatrix}, \overrightarrow{O_{202}O_{148}} = \mathbf{0}$

The reduction of higher dimensional irrep:

$T_h : T_g \rightarrow A_g + {}^2E_g + {}^1E_g$  of  $C_{3i}$ .

$T_h : T_u \rightarrow {}^1E_u + A_u + {}^2E_u$  of  $C_{3i}$ .

The correspondences of irreps at HSPs from original SG to lowered SG:

$$\begin{aligned} n_{GM7}^{148} &= n_{GM10}^{202} + n_{GM9}^{202} n_{GM4}^{148} = n_{GM6}^{202} + n_{GM7}^{202} n_{GM9}^{148} = n_{GM8}^{202} + n_{GM9}^{202} n_{GM6}^{148} = n_{GM5}^{202} + n_{GM6}^{202} n_{GM8}^{148} = n_{GM10}^{202} + n_{GM8}^{202} \\ n_{GM5}^{148} &= n_{GM5}^{202} + n_{GM7}^{202} n_{L2}^{148} = n_{L7}^{202} + n_{L8}^{202} + n_{L9}^{202} n_{L3}^{148} = n_{L4}^{202} + n_{L5}^{202} + n_{L6}^{202} n_{F2}^{148} = 2n_{X6}^{202} n_{F3}^{148} = 2n_{X5}^{202} n_{T7}^{148} = n_{L7}^{202} \\ n_{T4}^{148} &= n_{L4}^{202} n_{T9}^{148} = n_{L9}^{202} n_{T6}^{148} = n_{L6}^{202} n_{T8}^{148} = n_{L8}^{202} n_{T5}^{148} = n_{L5}^{202} \end{aligned}$$

The lower SG is SG 148 when the preserved operations are: **(sub-SG label is 5)** 1, 10, 9, 13, 22, 21.

The transformation is:  $(\mathbf{a}_{148}, \mathbf{b}_{148}, \mathbf{c}_{148}) = (\mathbf{a}_{202}, \mathbf{b}_{202}, \mathbf{c}_{202}) \begin{pmatrix} -\frac{1}{2} & -\frac{1}{2} & 0 \\ 0 & \frac{1}{2} & \frac{1}{2} \\ -\frac{1}{2} & 0 & -\frac{1}{2} \end{pmatrix}, \overrightarrow{O_{202}O_{148}} = \mathbf{0}$

The reduction of higher dimensional irrep:

$T_h : T_g \rightarrow A_g + {}^2E_g + {}^1E_g$  of  $C_{3i}$ .

$T_h : T_u \rightarrow {}^1E_u + A_u + {}^2E_u$  of  $C_{3i}$ .

The correspondences of irreps at HSPs from original SG to lowered SG:

$$\begin{aligned} n_{GM7}^{148} &= n_{GM10}^{202} + n_{GM9}^{202} n_{GM4}^{148} = n_{GM6}^{202} + n_{GM7}^{202} n_{GM9}^{148} = n_{GM8}^{202} + n_{GM9}^{202} n_{GM6}^{148} = n_{GM5}^{202} + n_{GM6}^{202} n_{GM8}^{148} = n_{GM10}^{202} + n_{GM8}^{202} \\ n_{GM5}^{148} &= n_{GM5}^{202} + n_{GM7}^{202} n_{L2}^{148} = n_{L7}^{202} + n_{L8}^{202} + n_{L9}^{202} n_{L3}^{148} = n_{L4}^{202} + n_{L5}^{202} + n_{L6}^{202} n_{F2}^{148} = 2n_{X6}^{202} n_{F3}^{148} = 2n_{X5}^{202} n_{T7}^{148} = n_{L7}^{202} \\ n_{T4}^{148} &= n_{L4}^{202} n_{T9}^{148} = n_{L9}^{202} n_{T6}^{148} = n_{L6}^{202} n_{T8}^{148} = n_{L8}^{202} n_{T5}^{148} = n_{L5}^{202} \end{aligned}$$

**100. Lowered SGs by higher-dimensional irreps of pairings in SG 203**

The representative operations of SG/T for SG 203:

1 :  $(x, y, z)$ , 2 :  $(x, \frac{3}{4} - y, \frac{3}{4} - z)$ , 3 :  $(\frac{3}{4} - x, y, \frac{3}{4} - z)$ , 4 :  $(\frac{3}{4} - x, \frac{3}{4} - y, z)$ , 5 :  $(z, x, y)$ , 6 :  $(y, z, x)$ , 7 :  $(\frac{3}{4} - y, z, \frac{3}{4} - x)$ ,  
 8 :  $(\frac{3}{4} - z, \frac{3}{4} - x, y)$ , 9 :  $(\frac{3}{4} - y, \frac{3}{4} - z, x)$ , 10 :  $(z, \frac{3}{4} - x, \frac{3}{4} - y)$ , 11 :  $(y, \frac{3}{4} - z, \frac{3}{4} - x)$ , 12 :  $(\frac{3}{4} - z, x, \frac{3}{4} - y)$ ,  
 13 :  $(-x, -y, -z)$ , 14 :  $(-x, y + \frac{1}{4}, z + \frac{1}{4})$ , 15 :  $(x + \frac{1}{4}, -y, z + \frac{1}{4})$ , 16 :  $(x + \frac{1}{4}, y + \frac{1}{4}, -z)$ , 17 :  $(-z, -x, -y)$ ,  
 18 :  $(-y, -z, -x)$ , 19 :  $(y + \frac{1}{4}, -z, x + \frac{1}{4})$ , 20 :  $(z + \frac{1}{4}, x + \frac{1}{4}, -y)$ , 21 :  $(y + \frac{1}{4}, z + \frac{1}{4}, -x)$ , 22 :  $(-z, x + \frac{1}{4}, y + \frac{1}{4})$ ,  
 23 :  $(-y, z + \frac{1}{4}, x + \frac{1}{4})$ , 24 :  $(z + \frac{1}{4}, -x, y + \frac{1}{4})$ .

The lower SG is SG 70 when the preserved operations are: **(sub-SG label is 1)** 1, 2, 3, 4, 13, 14, 15, 16.

The transformation is:  $(\mathbf{a}_{70}, \mathbf{b}_{70}, \mathbf{c}_{70}) = (\mathbf{a}_{203}, \mathbf{b}_{203}, \mathbf{c}_{203}) \begin{pmatrix} 0 & 1 & 0 \\ 1 & 0 & 0 \\ 0 & 0 & -1 \end{pmatrix}, \overrightarrow{O_{203}O_{70}} = \frac{1}{4}\mathbf{a}_{70} + (\frac{1}{4})\mathbf{b}_{70} + (\frac{1}{2})\mathbf{c}_{70}$

The reduction of higher dimensional irrep:

$T_h : T_g \rightarrow B_{1g} + B_{2g} + B_{3g}$  of  $D_{2h}$ .

$T_h : T_u \rightarrow B_{1u} + B_{2u} + B_{3u}$  of  $D_{2h}$ .

The correspondences of irreps at HSPs from original SG to lowered SG:

$$\begin{aligned} n_{GM6}^{70} &= n_{GM10}^{203} + n_{GM8}^{203} + n_{GM9}^{203} n_{GM5}^{70} = n_{GM5}^{203} + n_{GM6}^{203} + n_{GM7}^{203} n_{Y4}^{70} = n_{X3}^{203} n_{Y3}^{70} = n_{X4}^{203} n_{L3}^{70} = n_{L4}^{203} + n_{L5}^{203} + n_{L6}^{203} \\ n_{L2}^{70} &= n_{L7}^{203} + n_{L8}^{203} + n_{L9}^{203} n_{Z3}^{70} = n_{X4}^{203} n_{Z4}^{70} = n_{X3}^{203} n_{T4}^{70} = n_{X3}^{203} n_{T3}^{70} = n_{X4}^{203} \end{aligned}$$

The lower SG is SG 148 when the preserved operations are: **(sub-SG label is 2)** 1, 5, 6, 13, 17, 18.

The transformation is:  $(\mathbf{a}_{148}, \mathbf{b}_{148}, \mathbf{c}_{148}) = (\mathbf{a}_{203}, \mathbf{b}_{203}, \mathbf{c}_{203}) \begin{pmatrix} \frac{1}{2} & 0 & \frac{1}{2} \\ \frac{1}{2} & \frac{1}{2} & 0 \\ 0 & \frac{1}{2} & \frac{1}{2} \end{pmatrix}, \overrightarrow{O_{203}O_{148}} = \mathbf{0}$

The reduction of higher dimensional irrep:

$$T_h : T_g \rightarrow A_g + {}^2E_g + {}^1E_g \text{ of } C_{3i}.$$

$$T_h : T_u \rightarrow {}^1E_u + A_u + {}^2E_u \text{ of } C_{3i}.$$

The correspondences of irreps at HSPs from original SG to lowered SG:

$$\begin{aligned} n_{GM7}^{148} &= n_{GM10}^{203} + n_{GM9}^{203} & n_{GM4}^{148} &= n_{GM6}^{203} + n_{GM7}^{203} & n_{GM9}^{148} &= n_{GM8}^{203} + n_{GM9}^{203} & n_{GM6}^{148} &= n_{GM5}^{203} + n_{GM6}^{203} & n_{GM8}^{148} &= n_{GM10}^{203} + n_{GM8}^{203} \\ n_{GM5}^{148} &= n_{GM5}^{203} + n_{GM7}^{203} & n_{L2}^{148} &= n_{L4}^{203} + n_{L5}^{203} + n_{L6}^{203} & n_{L3}^{148} &= n_{L7}^{203} + n_{L8}^{203} + n_{L9}^{203} & n_{F2}^{148} &= n_{X3}^{203} + n_{X4}^{203} & n_{F3}^{148} &= n_{X3}^{203} + n_{X4}^{203} \\ n_{T7}^{148} &= n_{L7}^{203} & n_{T4}^{148} &= n_{L4}^{203} & n_{T9}^{148} &= n_{L9}^{203} & n_{T6}^{148} &= n_{L6}^{203} & n_{T8}^{148} &= n_{L8}^{203} & n_{T5}^{148} &= n_{L5}^{203} \end{aligned}$$

The lower SG is SG 148 when the preserved operations are: **(sub-SG label is 3)** 1, 12, 11, 13, 24, 23.

The transformation is:  $(\mathbf{a}_{148}, \mathbf{b}_{148}, \mathbf{c}_{148}) = (\mathbf{a}_{203}, \mathbf{b}_{203}, \mathbf{c}_{203}) \begin{pmatrix} -\frac{1}{2} & -\frac{1}{2} & 0 \\ 0 & -\frac{1}{2} & -\frac{1}{2} \\ \frac{1}{2} & 0 & \frac{1}{2} \end{pmatrix}, \overrightarrow{O_{203}O_{148}} = \frac{1}{2}\mathbf{b}_{148}$

The reduction of higher dimensional irrep:

$$T_h : T_g \rightarrow A_g + {}^2E_g + {}^1E_g \text{ of } C_{3i}.$$

$$T_h : T_u \rightarrow {}^1E_u + A_u + {}^2E_u \text{ of } C_{3i}.$$

The correspondences of irreps at HSPs from original SG to lowered SG:

$$\begin{aligned} n_{GM7}^{148} &= n_{GM10}^{203} + n_{GM9}^{203} & n_{GM4}^{148} &= n_{GM6}^{203} + n_{GM7}^{203} & n_{GM9}^{148} &= n_{GM8}^{203} + n_{GM9}^{203} & n_{GM6}^{148} &= n_{GM5}^{203} + n_{GM6}^{203} & n_{GM8}^{148} &= n_{GM10}^{203} + n_{GM8}^{203} \\ n_{GM5}^{148} &= n_{GM5}^{203} + n_{GM7}^{203} & n_{L2}^{148} &= n_{L4}^{203} + n_{L5}^{203} + n_{L6}^{203} & n_{L3}^{148} &= n_{L7}^{203} + n_{L8}^{203} + n_{L9}^{203} & n_{F2}^{148} &= n_{X3}^{203} + n_{X4}^{203} & n_{F3}^{148} &= n_{X3}^{203} + n_{X4}^{203} \\ n_{T7}^{148} &= n_{L7}^{203} & n_{T4}^{148} &= n_{L4}^{203} & n_{T9}^{148} &= n_{L9}^{203} & n_{T6}^{148} &= n_{L6}^{203} & n_{T8}^{148} &= n_{L8}^{203} & n_{T5}^{148} &= n_{L5}^{203} \end{aligned}$$

The lower SG is SG 148 when the preserved operations are: **(sub-SG label is 4)** 1, 8, 7, 13, 20, 19.

The transformation is:  $(\mathbf{a}_{148}, \mathbf{b}_{148}, \mathbf{c}_{148}) = (\mathbf{a}_{203}, \mathbf{b}_{203}, \mathbf{c}_{203}) \begin{pmatrix} \frac{1}{2} & 0 & \frac{1}{2} \\ -\frac{1}{2} & -\frac{1}{2} & 0 \\ 0 & -\frac{1}{2} & -\frac{1}{2} \end{pmatrix}, \overrightarrow{O_{203}O_{148}} = \frac{1}{2}\mathbf{b}_{148}$

The reduction of higher dimensional irrep:

$$T_h : T_g \rightarrow A_g + {}^2E_g + {}^1E_g \text{ of } C_{3i}.$$

$$T_h : T_u \rightarrow {}^1E_u + A_u + {}^2E_u \text{ of } C_{3i}.$$

The correspondences of irreps at HSPs from original SG to lowered SG:

$$\begin{aligned} n_{GM7}^{148} &= n_{GM10}^{203} + n_{GM9}^{203} & n_{GM4}^{148} &= n_{GM6}^{203} + n_{GM7}^{203} & n_{GM9}^{148} &= n_{GM8}^{203} + n_{GM9}^{203} & n_{GM6}^{148} &= n_{GM5}^{203} + n_{GM6}^{203} & n_{GM8}^{148} &= n_{GM10}^{203} + n_{GM8}^{203} \\ n_{GM5}^{148} &= n_{GM5}^{203} + n_{GM7}^{203} & n_{L2}^{148} &= n_{L4}^{203} + n_{L5}^{203} + n_{L6}^{203} & n_{L3}^{148} &= n_{L7}^{203} + n_{L8}^{203} + n_{L9}^{203} & n_{F2}^{148} &= n_{X3}^{203} + n_{X4}^{203} & n_{F3}^{148} &= n_{X3}^{203} + n_{X4}^{203} \\ n_{T7}^{148} &= n_{L7}^{203} & n_{T4}^{148} &= n_{L4}^{203} & n_{T9}^{148} &= n_{L9}^{203} & n_{T6}^{148} &= n_{L6}^{203} & n_{T8}^{148} &= n_{L8}^{203} & n_{T5}^{148} &= n_{L5}^{203} \end{aligned}$$

The lower SG is SG 148 when the preserved operations are: **(sub-SG label is 5)** 1, 10, 9, 13, 22, 21.

The transformation is:  $(\mathbf{a}_{148}, \mathbf{b}_{148}, \mathbf{c}_{148}) = (\mathbf{a}_{203}, \mathbf{b}_{203}, \mathbf{c}_{203}) \begin{pmatrix} -\frac{1}{2} & -\frac{1}{2} & 0 \\ 0 & \frac{1}{2} & \frac{1}{2} \\ -\frac{1}{2} & 0 & -\frac{1}{2} \end{pmatrix}, \overrightarrow{O_{203}O_{148}} = \frac{1}{2}\mathbf{b}_{148} + (\frac{1}{2})\mathbf{c}_{148}$

The reduction of higher dimensional irrep:

$$T_h : T_g \rightarrow A_g + {}^2E_g + {}^1E_g \text{ of } C_{3i}.$$

$$T_h : T_u \rightarrow {}^1E_u + A_u + {}^2E_u \text{ of } C_{3i}.$$

The correspondences of irreps at HSPs from original SG to lowered SG:

$$\begin{aligned} n_{GM7}^{148} &= n_{GM10}^{203} + n_{GM9}^{203} & n_{GM4}^{148} &= n_{GM6}^{203} + n_{GM7}^{203} & n_{GM9}^{148} &= n_{GM8}^{203} + n_{GM9}^{203} & n_{GM6}^{148} &= n_{GM5}^{203} + n_{GM6}^{203} & n_{GM8}^{148} &= n_{GM10}^{203} + n_{GM8}^{203} \\ n_{GM5}^{148} &= n_{GM5}^{203} + n_{GM7}^{203} & n_{L2}^{148} &= n_{L7}^{203} + n_{L8}^{203} + n_{L9}^{203} & n_{L3}^{148} &= n_{L4}^{203} + n_{L5}^{203} + n_{L6}^{203} & n_{F2}^{148} &= n_{X3}^{203} + n_{X4}^{203} & n_{F3}^{148} &= n_{X3}^{203} + n_{X4}^{203} \\ n_{T7}^{148} &= n_{L4}^{203} & n_{T4}^{148} &= n_{L7}^{203} & n_{T9}^{148} &= n_{L6}^{203} & n_{T6}^{148} &= n_{L9}^{203} & n_{T8}^{148} &= n_{L5}^{203} & n_{T5}^{148} &= n_{L8}^{203} \end{aligned}$$

### 101. Lowered SGs by higher-dimensional irreps of pairings in SG 204

The representative operations of SG/T for SG 204:

$$\begin{aligned} &1 : (x, y, z), 2 : (x, -y, -z), 3 : (-x, y, -z), 4 : (-x, -y, z), 5 : (z, x, y), 6 : (y, z, x), 7 : (-y, z, -x), 8 : (-z, -x, y), \\ &9 : (-y, -z, x), 10 : (z, -x, -y), 11 : (y, -z, -x), 12 : (-z, x, -y), 13 : (-x, -y, -z), 14 : (-x, y, z), 15 : (x, -y, z), \end{aligned}$$

16 :  $(x, y, -z)$ , 17 :  $(-z, -x, -y)$ , 18 :  $(-y, -z, -x)$ , 19 :  $(y, -z, x)$ , 20 :  $(z, x, -y)$ , 21 :  $(y, z, -x)$ , 22 :  $(-z, x, y)$ ,  
 23 :  $(-y, z, x)$ , 24 :  $(z, -x, y)$ .

The lower SG is SG 71 when the preserved operations are: **(sub-SG label is 1)** 1, 2, 3, 4, 13, 14, 15, 16.

The transformation is:  $(\mathbf{a}_{71}, \mathbf{b}_{71}, \mathbf{c}_{71}) = (\mathbf{a}_{204}, \mathbf{b}_{204}, \mathbf{c}_{204}) \begin{pmatrix} 0 & 0 & 1 \\ 1 & 0 & 0 \\ 0 & 1 & 0 \end{pmatrix}, \overrightarrow{O_{204}O_{71}} = -\frac{1}{2}\mathbf{b}_{71}$

The reduction of higher dimensional irrep:

$T_h : T_g \rightarrow B_{2g} + B_{1g} + B_{3g}$  of  $D_{2h}$ .

$T_h : T_u \rightarrow B_{2u} + B_{1u} + B_{3u}$  of  $D_{2h}$ .

The correspondences of irreps at HSPs from original SG to lowered SG:

$$\begin{aligned} n_{GM6}^{71} &= n_{GM10}^{204} + n_{GM8}^{204} + n_{GM9}^{204} & n_{GM5}^{71} &= n_{GM5}^{204} + n_{GM6}^{204} + n_{GM7}^{204} & n_{X6}^{71} &= n_{H10}^{204} + n_{H8}^{204} + n_{H9}^{204} & n_{X5}^{71} &= n_{H5}^{204} + n_{H6}^{204} + n_{H7}^{204} \\ n_{T6}^{71} &= n_{N3}^{204} & n_{T4}^{71} &= n_{N5}^{204} & n_{T5}^{71} &= n_{N4}^{204} & n_{T3}^{71} &= n_{N6}^{204} & n_{W5}^{71} &= n_{P5}^{204} + n_{P6}^{204} + n_{P7}^{204} & n_{R6}^{71} &= n_{N6}^{204} & n_{R4}^{71} &= n_{N4}^{204} & n_{R5}^{71} &= n_{N5}^{204} & n_{R3}^{71} &= n_{N3}^{204} \\ n_{S5}^{71} &= n_{N4}^{204} & n_{S3}^{71} &= n_{N6}^{204} & n_{S6}^{71} &= n_{N3}^{204} & n_{S4}^{71} &= n_{N5}^{204} \end{aligned}$$

The lower SG is SG 148 when the preserved operations are: **(sub-SG label is 2)** 1, 5, 6, 13, 17, 18.

The transformation is:  $(\mathbf{a}_{148}, \mathbf{b}_{148}, \mathbf{c}_{148}) = (\mathbf{a}_{204}, \mathbf{b}_{204}, \mathbf{c}_{204}) \begin{pmatrix} \frac{1}{2} & -\frac{1}{2} & \frac{1}{2} \\ \frac{1}{2} & \frac{1}{2} & -\frac{1}{2} \\ -\frac{1}{2} & \frac{1}{2} & \frac{1}{2} \end{pmatrix}, \overrightarrow{O_{204}O_{148}} = \mathbf{0}$

The reduction of higher dimensional irrep:

$T_h : T_g \rightarrow A_g + {}^2E_g + {}^1E_g$  of  $C_{3i}$ .

$T_h : T_u \rightarrow {}^1E_u + A_u + {}^2E_u$  of  $C_{3i}$ .

The correspondences of irreps at HSPs from original SG to lowered SG:

$$\begin{aligned} n_{GM7}^{148} &= n_{GM10}^{204} + n_{GM9}^{204} & n_{GM4}^{148} &= n_{GM6}^{204} + n_{GM7}^{204} & n_{GM9}^{148} &= n_{GM8}^{204} + n_{GM9}^{204} & n_{GM6}^{148} &= n_{GM5}^{204} + n_{GM6}^{204} & n_{GM8}^{148} &= n_{GM10}^{204} + n_{GM8}^{204} \\ n_{GM5}^{148} &= n_{GM5}^{204} + n_{GM7}^{204} & n_{L2}^{148} &= n_{N5}^{204} + n_{N6}^{204} & n_{L3}^{148} &= n_{N3}^{204} + n_{N4}^{204} & n_{F2}^{148} &= n_{N5}^{204} + n_{N6}^{204} & n_{F3}^{148} &= n_{N3}^{204} + n_{N4}^{204} & n_{T7}^{148} &= n_{H10}^{204} + n_{H9}^{204} \\ n_{T4}^{148} &= n_{H6}^{204} + n_{H7}^{204} & n_{T9}^{148} &= n_{H8}^{204} + n_{H9}^{204} & n_{T6}^{148} &= n_{H5}^{204} + n_{H6}^{204} & n_{T8}^{148} &= n_{H10}^{204} + n_{H8}^{204} & n_{T5}^{148} &= n_{H5}^{204} + n_{H7}^{204} \end{aligned}$$

The lower SG is SG 148 when the preserved operations are: **(sub-SG label is 3)** 1, 12, 11, 13, 24, 23.

The transformation is:  $(\mathbf{a}_{148}, \mathbf{b}_{148}, \mathbf{c}_{148}) = (\mathbf{a}_{204}, \mathbf{b}_{204}, \mathbf{c}_{204}) \begin{pmatrix} -\frac{1}{2} & -\frac{1}{2} & \frac{1}{2} \\ \frac{1}{2} & -\frac{1}{2} & -\frac{1}{2} \\ \frac{1}{2} & -\frac{1}{2} & \frac{1}{2} \end{pmatrix}, \overrightarrow{O_{204}O_{148}} = \mathbf{0}$

The reduction of higher dimensional irrep:

$T_h : T_g \rightarrow A_g + {}^2E_g + {}^1E_g$  of  $C_{3i}$ .

$T_h : T_u \rightarrow {}^1E_u + A_u + {}^2E_u$  of  $C_{3i}$ .

The correspondences of irreps at HSPs from original SG to lowered SG:

$$\begin{aligned} n_{GM7}^{148} &= n_{GM10}^{204} + n_{GM9}^{204} & n_{GM4}^{148} &= n_{GM6}^{204} + n_{GM7}^{204} & n_{GM9}^{148} &= n_{GM8}^{204} + n_{GM9}^{204} & n_{GM6}^{148} &= n_{GM5}^{204} + n_{GM6}^{204} & n_{GM8}^{148} &= n_{GM10}^{204} + n_{GM8}^{204} \\ n_{GM5}^{148} &= n_{GM5}^{204} + n_{GM7}^{204} & n_{L2}^{148} &= n_{N5}^{204} + n_{N6}^{204} & n_{L3}^{148} &= n_{N3}^{204} + n_{N4}^{204} & n_{F2}^{148} &= n_{N5}^{204} + n_{N6}^{204} & n_{F3}^{148} &= n_{N3}^{204} + n_{N4}^{204} & n_{T7}^{148} &= n_{H10}^{204} + n_{H9}^{204} \\ n_{T4}^{148} &= n_{H6}^{204} + n_{H7}^{204} & n_{T9}^{148} &= n_{H8}^{204} + n_{H9}^{204} & n_{T6}^{148} &= n_{H5}^{204} + n_{H6}^{204} & n_{T8}^{148} &= n_{H10}^{204} + n_{H8}^{204} & n_{T5}^{148} &= n_{H5}^{204} + n_{H7}^{204} \end{aligned}$$

The lower SG is SG 148 when the preserved operations are: **(sub-SG label is 4)** 1, 8, 7, 13, 20, 19.

The transformation is:  $(\mathbf{a}_{148}, \mathbf{b}_{148}, \mathbf{c}_{148}) = (\mathbf{a}_{204}, \mathbf{b}_{204}, \mathbf{c}_{204}) \begin{pmatrix} \frac{1}{2} & -\frac{1}{2} & \frac{1}{2} \\ -\frac{1}{2} & -\frac{1}{2} & \frac{1}{2} \\ \frac{1}{2} & -\frac{1}{2} & -\frac{1}{2} \end{pmatrix}, \overrightarrow{O_{204}O_{148}} = \mathbf{0}$

The reduction of higher dimensional irrep:

$T_h : T_g \rightarrow A_g + {}^2E_g + {}^1E_g$  of  $C_{3i}$ .

$T_h : T_u \rightarrow {}^1E_u + A_u + {}^2E_u$  of  $C_{3i}$ .

The correspondences of irreps at HSPs from original SG to lowered SG:

$$\begin{aligned} n_{GM7}^{148} &= n_{GM10}^{204} + n_{GM9}^{204} & n_{GM4}^{148} &= n_{GM6}^{204} + n_{GM7}^{204} & n_{GM9}^{148} &= n_{GM8}^{204} + n_{GM9}^{204} & n_{GM6}^{148} &= n_{GM5}^{204} + n_{GM6}^{204} & n_{GM8}^{148} &= n_{GM10}^{204} + n_{GM8}^{204} \\ n_{GM5}^{148} &= n_{GM5}^{204} + n_{GM7}^{204} & n_{L2}^{148} &= n_{N5}^{204} + n_{N6}^{204} & n_{L3}^{148} &= n_{N3}^{204} + n_{N4}^{204} & n_{F2}^{148} &= n_{N5}^{204} + n_{N6}^{204} & n_{F3}^{148} &= n_{N3}^{204} + n_{N4}^{204} & n_{T7}^{148} &= n_{H10}^{204} + n_{H9}^{204} \\ n_{T4}^{148} &= n_{H6}^{204} + n_{H7}^{204} & n_{T9}^{148} &= n_{H8}^{204} + n_{H9}^{204} & n_{T6}^{148} &= n_{H5}^{204} + n_{H6}^{204} & n_{T8}^{148} &= n_{H10}^{204} + n_{H8}^{204} & n_{T5}^{148} &= n_{H5}^{204} + n_{H7}^{204} \end{aligned}$$

The lower SG is SG 148 when the preserved operations are: **(sub-SG label is 5)** 1, 10, 9, 13, 22, 21.

The transformation is:  $(\mathbf{a}_{148}, \mathbf{b}_{148}, \mathbf{c}_{148}) = (\mathbf{a}_{204}, \mathbf{b}_{204}, \mathbf{c}_{204}) \begin{pmatrix} -\frac{1}{2} & -\frac{1}{2} & \frac{1}{2} \\ -\frac{1}{2} & \frac{1}{2} & \frac{1}{2} \\ -\frac{1}{2} & \frac{1}{2} & -\frac{1}{2} \end{pmatrix}, \overrightarrow{O_{204}O_{148}} = \mathbf{0}$

The reduction of higher dimensional irrep:

$$T_h : T_g \rightarrow A_g + {}^2E_g + {}^1E_g \text{ of } C_{3i}.$$

$$T_h : T_u \rightarrow {}^1E_u + A_u + {}^2E_u \text{ of } C_{3i}.$$

The correspondences of irreps of HSPs from original SG to lowered SG:

$$\begin{aligned} n_{GM7}^{148} &= n_{GM10}^{204} + n_{GM9}^{204} n_{GM4}^{148} = n_{GM6}^{204} + n_{GM7}^{204} n_{GM9}^{148} = n_{GM8}^{204} + n_{GM9}^{204} n_{GM6}^{148} = n_{GM5}^{204} + n_{GM6}^{204} n_{GM8}^{148} = n_{GM10}^{204} + n_{GM8}^{204} \\ n_{GM5}^{148} &= n_{GM5}^{204} + n_{GM7}^{204} n_{L2}^{148} = n_{N5}^{204} + n_{N6}^{204} n_{L3}^{148} = n_{N3}^{204} + n_{N4}^{204} n_{F2}^{148} = n_{N5}^{204} + n_{N6}^{204} n_{F3}^{148} = n_{N3}^{204} + n_{N4}^{204} n_{T7}^{148} = n_{H10}^{204} + n_{H9}^{204} \\ n_{T4}^{148} &= n_{H6}^{204} + n_{H7}^{204} n_{T9}^{148} = n_{H8}^{204} + n_{H9}^{204} n_{T6}^{148} = n_{H5}^{204} + n_{H6}^{204} n_{T8}^{148} = n_{H10}^{204} + n_{H8}^{204} n_{T5}^{148} = n_{H5}^{204} + n_{H7}^{204} \end{aligned}$$

## 102. Lowered SGs by higher-dimensional irreps of pairings in SG 205

The representative operations of SG/T for SG 205:

$$\begin{aligned} 1 : (x, y, z), 2 : (x + \frac{1}{2}, \frac{1}{2} - y, -z), 3 : (-x, y + \frac{1}{2}, \frac{1}{2} - z), 4 : (\frac{1}{2} - x, -y, z + \frac{1}{2}), 5 : (z, x, y), 6 : (y, z, x), \\ 7 : (-y, z + \frac{1}{2}, \frac{1}{2} - x), 8 : (\frac{1}{2} - z, -x, y + \frac{1}{2}), 9 : (\frac{1}{2} - y, -z, x + \frac{1}{2}), 10 : (z + \frac{1}{2}, \frac{1}{2} - x, -y), 11 : (y + \frac{1}{2}, \frac{1}{2} - z, -x), \\ 12 : (-z, x + \frac{1}{2}, \frac{1}{2} - y), 13 : (-x, -y, -z), 14 : (\frac{1}{2} - x, y + \frac{1}{2}, z), 15 : (x, \frac{1}{2} - y, z + \frac{1}{2}), 16 : (x + \frac{1}{2}, y, \frac{1}{2} - z), 17 : \\ (-z, -x, -y), 18 : (-y, -z, -x), 19 : (y, \frac{1}{2} - z, x + \frac{1}{2}), 20 : (z + \frac{1}{2}, x, \frac{1}{2} - y), 21 : (y + \frac{1}{2}, z, \frac{1}{2} - x), 22 : (\frac{1}{2} - z, x + \frac{1}{2}, y), \\ 23 : (\frac{1}{2} - y, z + \frac{1}{2}, x), 24 : (z, \frac{1}{2} - x, y + \frac{1}{2}). \end{aligned}$$

The lower SG is SG 61 when the preserved operations are: (**sub-SG label is 1**) 1, 2, 3, 4, 13, 14, 15, 16.

$$\text{The transformation is: } (\mathbf{a}_{61}, \mathbf{b}_{61}, \mathbf{c}_{61}) = (\mathbf{a}_{205}, \mathbf{b}_{205}, \mathbf{c}_{205}) \begin{pmatrix} 0 & 0 & -1 \\ 1 & 0 & 0 \\ 0 & -1 & 0 \end{pmatrix}, \overrightarrow{O_{205}O_{61}} = \frac{1}{2}\mathbf{a}_{61} + (\frac{1}{2})\mathbf{b}_{61}$$

The reduction of higher dimensional irrep:

$$T_h : T_g \rightarrow B_{1g} + B_{2g} + B_{3g} \text{ of } D_{2h}.$$

$$T_h : T_u \rightarrow B_{1u} + B_{2u} + B_{3u} \text{ of } D_{2h}.$$

The correspondences of irreps at HSPs from original SG to lowered SG:

$$\begin{aligned} n_{GM6}^{61} &= n_{GM10}^{205} + n_{GM8}^{205} + n_{GM9}^{205} n_{GM5}^{61} = n_{GM5}^{205} + n_{GM6}^{205} + n_{GM7}^{205} n_{X4}^{61} = n_{X4}^{205} n_{X3}^{61} = n_{X3}^{205} n_{S3}^{61} = n_{M3}^{205} n_{S4}^{61} = n_{M4}^{205} n_{R7}^{61} = \\ n_{R11}^{205} n_{R3}^{61} &= n_{R10}^{205} n_{R6}^{61} = n_{R11}^{205} n_{R2}^{61} = n_{R10}^{205} n_{R8}^{61} = n_{R11}^{205} n_{R4}^{61} = n_{R10}^{205} n_{R9}^{61} = n_{R7}^{205} + n_{R8}^{205} + n_{R9}^{205} n_{R5}^{61} = n_{R4}^{205} + n_{R5}^{205} + n_{R6}^{205} \\ n_{U4}^{61} &= n_{M3}^{205} n_{U3}^{61} = n_{M4}^{205} n_{Z4}^{61} = n_{X4}^{205} n_{Z3}^{61} = n_{X3}^{205} n_{T3}^{61} = n_{M4}^{205} n_{T4}^{61} = n_{M3}^{205} n_{Y4}^{61} = n_{X4}^{205} n_{Y3}^{61} = n_{X3}^{205} \end{aligned}$$

The lower SG is SG 148 when the preserved operations are: (**sub-SG label is 2**) 1, 5, 6, 13, 17, 18.

$$\text{The transformation is: } (\mathbf{a}_{148}, \mathbf{b}_{148}, \mathbf{c}_{148}) = (\mathbf{a}_{205}, \mathbf{b}_{205}, \mathbf{c}_{205}) \begin{pmatrix} 0 & 1 & 0 \\ 0 & 0 & 1 \\ 1 & 0 & 0 \end{pmatrix}, \overrightarrow{O_{205}O_{148}} = \mathbf{0}$$

The reduction of higher dimensional irrep:

$$T_h : T_g \rightarrow A_g + {}^2E_g + {}^1E_g \text{ of } C_{3i}.$$

$$T_h : T_u \rightarrow {}^1E_u + A_u + {}^2E_u \text{ of } C_{3i}.$$

The correspondences of irreps at HSPs from original SG to lowered SG:

$$\begin{aligned} n_{GM7}^{148} &= n_{GM10}^{205} + n_{GM9}^{205} n_{GM4}^{148} = n_{GM6}^{205} + n_{GM7}^{205} n_{GM9}^{148} = n_{GM8}^{205} + n_{GM9}^{205} n_{GM6}^{148} = n_{GM5}^{205} + n_{GM6}^{205} n_{GM8}^{148} = n_{GM10}^{205} + n_{GM8}^{205} \\ n_{GM5}^{148} &= n_{GM5}^{205} + n_{GM7}^{205} n_{L2}^{148} = n_{X3}^{205} + n_{X4}^{205} n_{L3}^{148} = n_{X3}^{205} + n_{X4}^{205} n_{F2}^{148} = n_{M3}^{205} + n_{M4}^{205} n_{F3}^{148} = n_{M3}^{205} + n_{M4}^{205} n_{T7}^{148} = n_{R11}^{205} + n_{R7}^{205} \\ n_{T4}^{148} &= n_{R10}^{205} + n_{R4}^{205} n_{T9}^{148} = n_{R11}^{205} + n_{R9}^{205} n_{T6}^{148} = n_{R10}^{205} + n_{R6}^{205} n_{T8}^{148} = n_{R11}^{205} + n_{R8}^{205} n_{T5}^{148} = n_{R10}^{205} + n_{R5}^{205} \end{aligned}$$

The lower SG is SG 148 when the preserved operations are: (**sub-SG label is 3**) 1, 12, 11, 13, 24, 23.

$$\text{The transformation is: } (\mathbf{a}_{148}, \mathbf{b}_{148}, \mathbf{c}_{148}) = (\mathbf{a}_{205}, \mathbf{b}_{205}, \mathbf{c}_{205}) \begin{pmatrix} 0 & 1 & 0 \\ 1 & 0 & 0 \\ 0 & 0 & -1 \end{pmatrix}, \overrightarrow{O_{205}O_{148}} = \frac{1}{2}\mathbf{b}_{148} + (\frac{1}{2})\mathbf{c}_{148}$$

The reduction of higher dimensional irrep:

$$T_h : T_g \rightarrow A_g + {}^2E_g + {}^1E_g \text{ of } C_{3i}.$$

$$T_h : T_u \rightarrow {}^1E_u + A_u + {}^2E_u \text{ of } C_{3i}.$$

The correspondences of irreps at HSPs from original SG to lowered SG:

$$\begin{aligned} n_{GM7}^{148} &= n_{GM10}^{205} + n_{GM9}^{205} n_{GM4}^{148} = n_{GM6}^{205} + n_{GM7}^{205} n_{GM9}^{148} = n_{GM8}^{205} + n_{GM9}^{205} n_{GM6}^{148} = n_{GM5}^{205} + n_{GM6}^{205} n_{GM8}^{148} = n_{GM10}^{205} + n_{GM8}^{205} \\ n_{GM5}^{148} &= n_{GM5}^{205} + n_{GM7}^{205} n_{L2}^{148} = n_{X3}^{205} + n_{X4}^{205} n_{L3}^{148} = n_{X3}^{205} + n_{X4}^{205} n_{F2}^{148} = n_{M3}^{205} + n_{M4}^{205} n_{F3}^{148} = n_{M3}^{205} + n_{M4}^{205} n_{T7}^{148} = n_{R11}^{205} + n_{R7}^{205} \\ n_{T4}^{148} &= n_{R10}^{205} + n_{R4}^{205} n_{T9}^{148} = n_{R11}^{205} + n_{R8}^{205} n_{T6}^{148} = n_{R10}^{205} + n_{R5}^{205} n_{T8}^{148} = n_{R11}^{205} + n_{R9}^{205} n_{T5}^{148} = n_{R10}^{205} + n_{R6}^{205} \end{aligned}$$

The lower SG is SG 148 when the preserved operations are: **(sub-SG label is 4) 1, 8, 7, 13, 20, 19.**

The transformation is:  $(\mathbf{a}_{148}, \mathbf{b}_{148}, \mathbf{c}_{148}) = (\mathbf{a}_{205}, \mathbf{b}_{205}, \mathbf{c}_{205}) \begin{pmatrix} 0 & 0 & -1 \\ 0 & 1 & 0 \\ 1 & 0 & 0 \end{pmatrix}, \overrightarrow{O_{205}O_{148}} = \frac{1}{2}\mathbf{b}_{148} + (\frac{1}{2})\mathbf{c}_{148}$

The reduction of higher dimensional irrep:

$T_h : T_g \rightarrow A_g + {}^2E_g + {}^1E_g$  of  $C_{3i}$ .

$T_h : T_u \rightarrow {}^1E_u + A_u + {}^2E_u$  of  $C_{3i}$ .

The correspondences of irreps at HSPs from original SG to lowered SG:

$$\begin{aligned} n_{GM7}^{148} &= n_{GM10}^{205} + n_{GM9}^{205} n_{GM4}^{148} = n_{GM6}^{205} + n_{GM7}^{205} n_{GM9}^{148} = n_{GM10}^{205} + n_{GM8}^{205} n_{GM6}^{148} = n_{GM5}^{205} + n_{GM7}^{205} n_{GM8}^{148} = n_{GM8}^{205} + n_{GM9}^{205} \\ n_{GM5}^{148} &= n_{GM5}^{205} + n_{GM6}^{205} n_{L2}^{148} = n_{X3}^{205} + n_{X4}^{205} n_{L3}^{148} = n_{X3}^{205} + n_{X4}^{205} n_{F2}^{148} = n_{M3}^{205} + n_{M4}^{205} n_{F3}^{148} = n_{M3}^{205} + n_{M4}^{205} n_{T7}^{148} = n_{R11}^{205} + n_{R7}^{205} \\ n_{T4}^{148} &= n_{R10}^{205} + n_{R4}^{205} n_{T9}^{148} = n_{R11}^{205} + n_{R8}^{205} n_{T6}^{148} = n_{R10}^{205} + n_{R5}^{205} n_{T8}^{148} = n_{R11}^{205} + n_{R9}^{205} n_{T5}^{148} = n_{R10}^{205} + n_{R6}^{205} \end{aligned}$$

The lower SG is SG 148 when the preserved operations are: **(sub-SG label is 5) 1, 10, 9, 13, 22, 21.**

The transformation is:  $(\mathbf{a}_{148}, \mathbf{b}_{148}, \mathbf{c}_{148}) = (\mathbf{a}_{205}, \mathbf{b}_{205}, \mathbf{c}_{205}) \begin{pmatrix} -1 & 0 & 0 \\ 0 & 1 & 0 \\ 0 & 0 & -1 \end{pmatrix}, \overrightarrow{O_{205}O_{148}} = \frac{1}{2}\mathbf{b}_{148} + (\frac{1}{2})\mathbf{c}_{148}$

The reduction of higher dimensional irrep:

$T_h : T_g \rightarrow A_g + {}^2E_g + {}^1E_g$  of  $C_{3i}$ .

$T_h : T_u \rightarrow {}^1E_u + A_u + {}^2E_u$  of  $C_{3i}$ .

The correspondences of irreps at HSPs from original SG to lowered SG:

$$\begin{aligned} n_{GM7}^{148} &= n_{GM10}^{205} + n_{GM9}^{205} n_{GM4}^{148} = n_{GM6}^{205} + n_{GM7}^{205} n_{GM9}^{148} = n_{GM8}^{205} + n_{GM9}^{205} n_{GM6}^{148} = n_{GM5}^{205} + n_{GM6}^{205} n_{GM8}^{148} = n_{GM10}^{205} + n_{GM8}^{205} \\ n_{GM5}^{148} &= n_{GM5}^{205} + n_{GM7}^{205} n_{L2}^{148} = n_{X3}^{205} + n_{X4}^{205} n_{L3}^{148} = n_{X3}^{205} + n_{X4}^{205} n_{F2}^{148} = n_{M3}^{205} + n_{M4}^{205} n_{F3}^{148} = n_{M3}^{205} + n_{M4}^{205} n_{T7}^{148} = n_{R11}^{205} + n_{R7}^{205} \\ n_{T4}^{148} &= n_{R10}^{205} + n_{R4}^{205} n_{T9}^{148} = n_{R11}^{205} + n_{R9}^{205} n_{T6}^{148} = n_{R10}^{205} + n_{R6}^{205} n_{T8}^{148} = n_{R11}^{205} + n_{R8}^{205} n_{T5}^{148} = n_{R10}^{205} + n_{R5}^{205} \end{aligned}$$

**103. Lowered SGs by higher-dimensional irreps of pairings in SG 206**

The representative operations of SG/T for SG 206:

1 :  $(x, y, z)$ , 2 :  $(x, -y, \frac{1}{2} - z)$ , 3 :  $(\frac{1}{2} - x, y, -z)$ , 4 :  $(-x, \frac{1}{2} - y, z)$ , 5 :  $(z, x, y)$ , 6 :  $(y, z, x)$ , 7 :  $(\frac{1}{2} - y, z, -x)$ ,  
 8 :  $(-z, \frac{1}{2} - x, y)$ , 9 :  $(-y, \frac{1}{2} - z, x)$ , 10 :  $(z, -x, \frac{1}{2} - y)$ , 11 :  $(y, -z, \frac{1}{2} - x)$ , 12 :  $(\frac{1}{2} - z, x, -y)$ , 13 :  $(-x, -y, -z)$ ,  
 14 :  $(-x, y, z + \frac{1}{2})$ , 15 :  $(x + \frac{1}{2}, -y, z)$ , 16 :  $(x, y + \frac{1}{2}, -z)$ , 17 :  $(-z, -x, -y)$ , 18 :  $(-y, -z, -x)$ , 19 :  $(y + \frac{1}{2}, -z, x)$ ,  
 20 :  $(z, x + \frac{1}{2}, -y)$ , 21 :  $(y, z + \frac{1}{2}, -x)$ , 22 :  $(-z, x, y + \frac{1}{2})$ , 23 :  $(-y, z, x + \frac{1}{2})$ , 24 :  $(z + \frac{1}{2}, -x, y)$ .

The lower SG is SG 73 when the preserved operations are: **(sub-SG label is 1) 1, 2, 3, 4, 13, 14, 15, 16.**

The transformation is:  $(\mathbf{a}_{73}, \mathbf{b}_{73}, \mathbf{c}_{73}) = (\mathbf{a}_{206}, \mathbf{b}_{206}, \mathbf{c}_{206}) \begin{pmatrix} 0 & 1 & 0 \\ 1 & 0 & 0 \\ 0 & 0 & -1 \end{pmatrix}, \overrightarrow{O_{206}O_{73}} = \frac{1}{4}\mathbf{a}_{73} + (-\frac{1}{4})\mathbf{b}_{73} + (\frac{1}{4})\mathbf{c}_{73}$

The reduction of higher dimensional irrep:

$T_h : T_g \rightarrow B_{2g} + B_{1g} + B_{3g}$  of  $D_{2h}$ .

$T_h : T_u \rightarrow B_{2u} + B_{1u} + B_{3u}$  of  $D_{2h}$ .

The correspondences of irreps at HSPs from original SG to lowered SG:

$$\begin{aligned} n_{GM6}^{73} &= n_{GM10}^{206} + n_{GM8}^{206} + n_{GM9}^{206} n_{GM5}^{73} = n_{GM5}^{206} + n_{GM6}^{206} + n_{GM7}^{206} n_{X6}^{73} = n_{H5}^{206} + n_{H6}^{206} + n_{H7}^{206} n_{X5}^{73} = n_{H10}^{206} + n_{H8}^{206} + n_{H9}^{206} \\ n_{T2}^{73} &= n_{N2}^{206} n_{W3}^{73} = n_{P4}^{206} + n_{P5}^{206} + n_{P6}^{206} n_{W2}^{73} = n_{P7}^{206} n_{W4}^{73} = n_{P7}^{206} n_{W5}^{73} = n_{P7}^{206} n_{R2}^{73} = n_{N2}^{206} n_{S2}^{73} = n_{N2}^{206} \end{aligned}$$

The lower SG is SG 148 when the preserved operations are: **(sub-SG label is 2) 1, 5, 6, 13, 17, 18.**

The transformation is:  $(\mathbf{a}_{148}, \mathbf{b}_{148}, \mathbf{c}_{148}) = (\mathbf{a}_{206}, \mathbf{b}_{206}, \mathbf{c}_{206}) \begin{pmatrix} \frac{1}{2} & -\frac{1}{2} & \frac{1}{2} \\ \frac{1}{2} & \frac{1}{2} & -\frac{1}{2} \\ -\frac{1}{2} & \frac{1}{2} & \frac{1}{2} \end{pmatrix}, \overrightarrow{O_{206}O_{148}} = \mathbf{0}$

The reduction of higher dimensional irrep:

$T_h : T_g \rightarrow A_g + {}^2E_g + {}^1E_g$  of  $C_{3i}$ .

$T_h : T_u \rightarrow {}^1E_u + A_u + {}^2E_u$  of  $C_{3i}$ .

The correspondences of irreps at HSPs from original SG to lowered SG:

$$\begin{aligned} n_{GM7}^{148} &= n_{GM10}^{206} + n_{GM9}^{206} n_{GM4}^{148} = n_{GM6}^{206} + n_{GM7}^{206} n_{GM9}^{148} = n_{GM8}^{206} + n_{GM9}^{206} n_{GM6}^{148} = n_{GM5}^{206} + n_{GM6}^{206} n_{GM8}^{148} = n_{GM10}^{206} + n_{GM8}^{206} \\ n_{GM5}^{148} &= n_{GM5}^{206} + n_{GM7}^{206} n_{L2}^{148} = n_{N2}^{206} n_{L3}^{148} = n_{N2}^{206} n_{F2}^{148} = n_{N2}^{206} n_{F3}^{148} = n_{N2}^{206} n_{T7}^{148} = n_{H10}^{206} + n_{H9}^{206} n_{T4}^{148} = n_{H6}^{206} + n_{H7}^{206} n_{T9}^{148} = \\ n_{H8}^{206} + n_{H9}^{206} n_{T6}^{148} &= n_{H5}^{206} + n_{H6}^{206} n_{T8}^{148} = n_{H10}^{206} + n_{H8}^{206} n_{T5}^{148} = n_{H5}^{206} + n_{H7}^{206} \end{aligned}$$

The lower SG is SG 148 when the preserved operations are: **(sub-SG label is 3)** 1, 12, 11, 13, 24, 23.

The transformation is:  $(\mathbf{a}_{148}, \mathbf{b}_{148}, \mathbf{c}_{148}) = (\mathbf{a}_{206}, \mathbf{b}_{206}, \mathbf{c}_{206}) \begin{pmatrix} -\frac{1}{2} & -\frac{1}{2} & \frac{1}{2} \\ \frac{1}{2} & -\frac{1}{2} & -\frac{1}{2} \\ \frac{1}{2} & -\frac{1}{2} & \frac{1}{2} \end{pmatrix}, \overrightarrow{O_{206}O_{148}} = \frac{1}{2}\mathbf{b}_{148} + (\frac{1}{2})\mathbf{c}_{148}$

The reduction of higher dimensional irrep:

$$\begin{aligned} T_h : \mathbf{T}_g &\rightarrow A_g + {}^2E_g + {}^1E_g \text{ of } C_{3i}. \\ T_h : \mathbf{T}_u &\rightarrow {}^1E_u + A_u + {}^2E_u \text{ of } C_{3i}. \end{aligned}$$

The correspondences of irreps at HSPs from original SG to lowered SG:

$$\begin{aligned} n_{GM7}^{148} &= n_{GM10}^{206} + n_{GM9}^{206} n_{GM4}^{148} = n_{GM6}^{206} + n_{GM7}^{206} n_{GM9}^{148} = n_{GM8}^{206} + n_{GM9}^{206} n_{GM6}^{148} = n_{GM5}^{206} + n_{GM6}^{206} n_{GM8}^{148} = n_{GM10}^{206} + n_{GM8}^{206} \\ n_{GM5}^{148} &= n_{GM5}^{206} + n_{GM7}^{206} n_{L2}^{148} = n_{N2}^{206} n_{L3}^{148} = n_{N2}^{206} n_{F2}^{148} = n_{N2}^{206} n_{F3}^{148} = n_{N2}^{206} n_{T7}^{148} = n_{H10}^{206} + n_{H9}^{206} n_{T4}^{148} = n_{H6}^{206} + n_{H7}^{206} n_{T9}^{148} = \\ n_{H8}^{206} + n_{H9}^{206} n_{T6}^{148} &= n_{H5}^{206} + n_{H6}^{206} n_{T8}^{148} = n_{H10}^{206} + n_{H8}^{206} n_{T5}^{148} = n_{H5}^{206} + n_{H7}^{206} \end{aligned}$$

The lower SG is SG 148 when the preserved operations are: **(sub-SG label is 4)** 1, 8, 7, 13, 20, 19.

The transformation is:  $(\mathbf{a}_{148}, \mathbf{b}_{148}, \mathbf{c}_{148}) = (\mathbf{a}_{206}, \mathbf{b}_{206}, \mathbf{c}_{206}) \begin{pmatrix} \frac{1}{2} & -\frac{1}{2} & \frac{1}{2} \\ -\frac{1}{2} & -\frac{1}{2} & \frac{1}{2} \\ \frac{1}{2} & -\frac{1}{2} & -\frac{1}{2} \end{pmatrix}, \overrightarrow{O_{206}O_{148}} = \frac{1}{2}\mathbf{b}_{148} + (\frac{1}{2})\mathbf{c}_{148}$

The reduction of higher dimensional irrep:

$$\begin{aligned} T_h : \mathbf{T}_g &\rightarrow A_g + {}^2E_g + {}^1E_g \text{ of } C_{3i}. \\ T_h : \mathbf{T}_u &\rightarrow {}^1E_u + A_u + {}^2E_u \text{ of } C_{3i}. \end{aligned}$$

The correspondences of irreps at HSPs from original SG to lowered SG:

$$\begin{aligned} n_{GM7}^{148} &= n_{GM10}^{206} + n_{GM9}^{206} n_{GM4}^{148} = n_{GM6}^{206} + n_{GM7}^{206} n_{GM9}^{148} = n_{GM8}^{206} + n_{GM9}^{206} n_{GM6}^{148} = n_{GM5}^{206} + n_{GM6}^{206} n_{GM8}^{148} = n_{GM10}^{206} + n_{GM8}^{206} \\ n_{GM5}^{148} &= n_{GM5}^{206} + n_{GM7}^{206} n_{L2}^{148} = n_{N2}^{206} n_{L3}^{148} = n_{N2}^{206} n_{F2}^{148} = n_{N2}^{206} n_{F3}^{148} = n_{N2}^{206} n_{T7}^{148} = n_{H10}^{206} + n_{H9}^{206} n_{T4}^{148} = n_{H6}^{206} + n_{H7}^{206} n_{T9}^{148} = \\ n_{H8}^{206} + n_{H9}^{206} n_{T6}^{148} &= n_{H5}^{206} + n_{H6}^{206} n_{T8}^{148} = n_{H10}^{206} + n_{H8}^{206} n_{T5}^{148} = n_{H5}^{206} + n_{H7}^{206} \end{aligned}$$

The lower SG is SG 148 when the preserved operations are: **(sub-SG label is 5)** 1, 10, 9, 13, 22, 21.

The transformation is:  $(\mathbf{a}_{148}, \mathbf{b}_{148}, \mathbf{c}_{148}) = (\mathbf{a}_{206}, \mathbf{b}_{206}, \mathbf{c}_{206}) \begin{pmatrix} -\frac{1}{2} & \frac{1}{2} & \frac{1}{2} \\ -\frac{1}{2} & -\frac{1}{2} & \frac{1}{2} \\ \frac{1}{2} & -\frac{1}{2} & \frac{1}{2} \end{pmatrix}, \overrightarrow{O_{206}O_{148}} = \frac{1}{2}\mathbf{b}_{148} + (\frac{1}{2})\mathbf{c}_{148}$

The reduction of higher dimensional irrep:

$$\begin{aligned} T_h : \mathbf{T}_g &\rightarrow A_g + {}^2E_g + {}^1E_g \text{ of } C_{3i}. \\ T_h : \mathbf{T}_u &\rightarrow {}^1E_u + A_u + {}^2E_u \text{ of } C_{3i}. \end{aligned}$$

The correspondences of irreps at HSPs from original SG to lowered SG:

$$\begin{aligned} n_{GM7}^{148} &= n_{GM10}^{206} + n_{GM9}^{206} n_{GM4}^{148} = n_{GM6}^{206} + n_{GM7}^{206} n_{GM9}^{148} = n_{GM10}^{206} + n_{GM8}^{206} n_{GM6}^{148} = n_{GM5}^{206} + n_{GM7}^{206} n_{GM8}^{148} = n_{GM8}^{206} + n_{GM9}^{206} \\ n_{GM5}^{148} &= n_{GM5}^{206} + n_{GM6}^{206} n_{L2}^{148} = n_{N2}^{206} n_{L3}^{148} = n_{N2}^{206} n_{F2}^{148} = n_{N2}^{206} n_{F3}^{148} = n_{N2}^{206} n_{T7}^{148} = n_{H10}^{206} + n_{H9}^{206} n_{T4}^{148} = n_{H6}^{206} + n_{H7}^{206} n_{T9}^{148} = \\ n_{H10}^{206} + n_{H8}^{206} n_{T6}^{148} &= n_{H5}^{206} + n_{H7}^{206} n_{T8}^{148} = n_{H8}^{206} + n_{H9}^{206} n_{T5}^{148} = n_{H5}^{206} + n_{H6}^{206} \end{aligned}$$

**104. Lowered SGs by higher-dimensional irreps of pairings in SG 207**

The representative operations of SG/T for SG 207:

$$\begin{aligned} &1 : (x, y, z), 2 : (x, -z, y), 3 : (x, z, -y), 4 : (z, y, -x), 5 : (-z, y, x), 6 : (-y, x, z), 7 : (y, -x, z), 8 : (x, -y, -z), \\ &9 : (-x, y, -z), 10 : (-x, -y, z), 11 : (y, x, -z), 12 : (-y, -x, -z), 13 : (-x, z, y), 14 : (-x, -z, -y), 15 : (z, -y, x), \\ &16 : (-z, -y, -x), 17 : (z, x, y), 18 : (y, z, x), 19 : (-y, z, -x), 20 : (-z, -x, y), 21 : (-y, -z, x), 22 : (z, -x, -y), \\ &23 : (y, -z, -x), 24 : (-z, x, -y). \end{aligned}$$

The lower SG is SG 16 when the preserved operations are: **(sub-SG label is 1)** 1, 8, 9, 10.

The transformation is:  $(\mathbf{a}_{16}, \mathbf{b}_{16}, \mathbf{c}_{16}) = (\mathbf{a}_{207}, \mathbf{b}_{207}, \mathbf{c}_{207}) \begin{pmatrix} 0 & 0 & 1 \\ 1 & 0 & 0 \\ 0 & 1 & 0 \end{pmatrix}, \overrightarrow{O_{207}O_{16}} = \frac{1}{2}\mathbf{a}_{16} + (\frac{1}{2})\mathbf{c}_{16}$

The reduction of higher dimensional irrep:

$$O : T_1 \rightarrow B_1 + B_2 + B_3 \text{ of } D_2.$$

$$O : T_2 \rightarrow B_1 + B_2 + B_3 \text{ of } D_2.$$

The correspondences of irreps at HSPs from original SG to lowered SG:

$$\begin{aligned} n_{GM5}^{16} &= n_{GM6}^{207} + n_{GM7}^{207} + 2n_{GM8}^{207} & n_{X5}^{16} &= n_{X6}^{207} + n_{X7}^{207} & n_{S5}^{16} &= n_{M6}^{207} + n_{M7}^{207} & n_{R5}^{16} &= n_{R6}^{207} + n_{R7}^{207} + 2n_{R8}^{207} \\ n_{Z5}^{16} &= n_{X6}^{207} + n_{X7}^{207} & n_{T5}^{16} &= n_{M6}^{207} + n_{M7}^{207} & n_{Y5}^{16} &= n_{X6}^{207} + n_{X7}^{207} \end{aligned}$$

The lower SG is SG 21 when the preserved operations are: **(sub-SG label is 2) 1, 8, 13, 14.**

The transformation is:  $(\mathbf{a}_{21}, \mathbf{b}_{21}, \mathbf{c}_{21}) = (\mathbf{a}_{207}, \mathbf{b}_{207}, \mathbf{c}_{207}) \begin{pmatrix} 0 & 0 & 1 \\ 1 & -1 & 0 \\ 1 & 1 & 0 \end{pmatrix}, \overrightarrow{O_{207}O_{21}} = \frac{1}{2}\mathbf{c}_{21}$

The reduction of higher dimensional irrep:

$$O : T_1 \rightarrow B_1 + B_2 + B_3 \text{ of } D_2.$$

$$O : T_2 \rightarrow A_1 + B_2 + B_3 \text{ of } D_2.$$

The correspondences of irreps at HSPs from original SG to lowered SG:

$$\begin{aligned} n_{GM5}^{21} &= n_{GM6}^{207} + n_{GM7}^{207} + 2n_{GM8}^{207} & n_{Y5}^{21} &= n_{M6}^{207} + n_{M7}^{207} & n_{S4}^{21} &= n_{X6}^{207} + n_{X7}^{207} & n_{S3}^{21} &= n_{X6}^{207} + n_{X7}^{207} & n_{Z5}^{21} &= n_{X6}^{207} + n_{X7}^{207} \\ n_{R4}^{21} &= n_{M6}^{207} + n_{M7}^{207} & n_{R3}^{21} &= n_{M6}^{207} + n_{M7}^{207} \end{aligned}$$

The lower SG is SG 21 when the preserved operations are: **(sub-SG label is 3) 1, 9, 16, 15.**

The transformation is:  $(\mathbf{a}_{21}, \mathbf{b}_{21}, \mathbf{c}_{21}) = (\mathbf{a}_{207}, \mathbf{b}_{207}, \mathbf{c}_{207}) \begin{pmatrix} -1 & 1 & 0 \\ 0 & 0 & 1 \\ 1 & 1 & 0 \end{pmatrix}, \overrightarrow{O_{207}O_{21}} = \frac{1}{2}\mathbf{c}_{21}$

The reduction of higher dimensional irrep:

$$O : T_1 \rightarrow B_1 + B_2 + B_3 \text{ of } D_2.$$

$$O : T_2 \rightarrow A_1 + B_2 + B_3 \text{ of } D_2.$$

The correspondences of irreps at HSPs from original SG to lowered SG:

$$\begin{aligned} n_{GM5}^{21} &= n_{GM6}^{207} + n_{GM7}^{207} + 2n_{GM8}^{207} & n_{Y5}^{21} &= n_{M6}^{207} + n_{M7}^{207} & n_{S4}^{21} &= n_{X6}^{207} + n_{X7}^{207} & n_{S3}^{21} &= n_{X6}^{207} + n_{X7}^{207} & n_{Z5}^{21} &= n_{X6}^{207} + n_{X7}^{207} \\ n_{R4}^{21} &= n_{M6}^{207} + n_{M7}^{207} & n_{R3}^{21} &= n_{M6}^{207} + n_{M7}^{207} \end{aligned}$$

The lower SG is SG 21 when the preserved operations are: **(sub-SG label is 4) 1, 10, 11, 12.**

The transformation is:  $(\mathbf{a}_{21}, \mathbf{b}_{21}, \mathbf{c}_{21}) = (\mathbf{a}_{207}, \mathbf{b}_{207}, \mathbf{c}_{207}) \begin{pmatrix} 1 & -1 & 0 \\ 1 & 1 & 0 \\ 0 & 0 & 1 \end{pmatrix}, \overrightarrow{O_{207}O_{21}} = \frac{1}{2}\mathbf{c}_{21}$

The reduction of higher dimensional irrep:

$$O : T_1 \rightarrow B_1 + B_2 + B_3 \text{ of } D_2.$$

$$O : T_2 \rightarrow A_1 + B_2 + B_3 \text{ of } D_2.$$

The correspondences of irreps at HSPs from original SG to lowered SG:

$$\begin{aligned} n_{GM5}^{21} &= n_{GM6}^{207} + n_{GM7}^{207} + 2n_{GM8}^{207} & n_{Y5}^{21} &= n_{M6}^{207} + n_{M7}^{207} & n_{S4}^{21} &= n_{X6}^{207} + n_{X7}^{207} & n_{S3}^{21} &= n_{X6}^{207} + n_{X7}^{207} & n_{Z5}^{21} &= n_{X6}^{207} + n_{X7}^{207} \\ n_{R4}^{21} &= n_{M6}^{207} + n_{M7}^{207} & n_{R3}^{21} &= n_{M6}^{207} + n_{M7}^{207} \end{aligned}$$

The lower SG is SG 75 when the preserved operations are: **(sub-SG label is 5) 1, 6, 7, 10.**

The transformation is:  $(\mathbf{a}_{75}, \mathbf{b}_{75}, \mathbf{c}_{75}) = (\mathbf{a}_{207}, \mathbf{b}_{207}, \mathbf{c}_{207}) \begin{pmatrix} -1 & 0 & 0 \\ 0 & -1 & 0 \\ 0 & 0 & 1 \end{pmatrix}, \overrightarrow{O_{207}O_{75}} = -\frac{1}{2}\mathbf{a}_{75} + (\frac{1}{2})\mathbf{b}_{75}$

The reduction of higher dimensional irrep:

$$O : T_1 \rightarrow A + {}^2E + {}^1E \text{ of } C_4.$$

$$O : T_2 \rightarrow {}^2E + B + {}^1E \text{ of } C_4.$$

The correspondences of irreps at HSPs from original SG to lowered SG:

$$\begin{aligned} n_{GM5}^{75} &= n_{GM7}^{207} + n_{GM8}^{207} & n_{GM7}^{75} &= n_{GM7}^{207} + n_{GM8}^{207} & n_{GM8}^{75} &= n_{GM6}^{207} + n_{GM8}^{207} & n_{GM6}^{75} &= n_{GM6}^{207} + n_{GM8}^{207} & n_{X4}^{75} &= n_{X6}^{207} + n_{X7}^{207} \\ n_{X6}^{75} &= n_{X7}^{207} & n_{M5}^{75} &= n_{M7}^{207} & n_{M7}^{75} &= n_{M7}^{207} & n_{M8}^{75} &= n_{M6}^{207} & n_{M6}^{75} &= n_{M6}^{207} & n_{A5}^{75} &= n_{R6}^{207} + n_{R8}^{207} & n_{A7}^{75} &= n_{R6}^{207} + n_{R8}^{207} & n_{A8}^{75} &= n_{R7}^{207} + n_{R8}^{207} \\ n_{A6}^{75} &= n_{R7}^{207} + n_{R8}^{207} & n_{R4}^{75} &= n_{M6}^{207} + n_{M7}^{207} & n_{R3}^{75} &= n_{M6}^{207} + n_{M7}^{207} & n_{Z5}^{75} &= n_{X7}^{207} & n_{Z7}^{75} &= n_{X7}^{207} & n_{Z8}^{75} &= n_{X6}^{207} & n_{Z6}^{75} &= n_{X6}^{207} \end{aligned}$$

The lower SG is SG 75 when the preserved operations are: **(sub-SG label is 6) 1, 2, 3, 8.**

The transformation is:  $(\mathbf{a}_{75}, \mathbf{b}_{75}, \mathbf{c}_{75}) = (\mathbf{a}_{207}, \mathbf{b}_{207}, \mathbf{c}_{207}) \begin{pmatrix} 0 & 0 & 1 \\ -1 & 0 & 0 \\ 0 & -1 & 0 \end{pmatrix}, \overrightarrow{O_{207}O_{75}} = -\frac{1}{2}\mathbf{a}_{75} + (\frac{1}{2})\mathbf{b}_{75}$

The reduction of higher dimensional irrep:

$O : T_1 \rightarrow A + {}^2E + {}^1E$  of  $C_4$ .

$O : T_2 \rightarrow {}^2E + B + {}^1E$  of  $C_4$ .

The correspondences of irreps at HSPs from original SG to lowered SG:

$$\begin{aligned} n_{GM5}^{75} &= n_{GM7}^{207} + n_{GM8}^{207} & n_{GM7}^{75} &= n_{GM7}^{207} + n_{GM8}^{207} & n_{GM8}^{75} &= n_{GM6}^{207} + n_{GM8}^{207} & n_{GM6}^{75} &= n_{GM6}^{207} + n_{GM8}^{207} & n_{X4}^{75} &= n_{X6}^{207} + n_{X7}^{207} & n_{X3}^{75} &= \\ n_{X6}^{207} + n_{X7}^{207} & n_{M5}^{75} &= n_{M7}^{207} & n_{M7}^{75} &= n_{M7}^{207} & n_{M8}^{75} &= n_{M6}^{207} & n_{M6}^{75} &= n_{M6}^{207} & n_{A5}^{75} &= n_{R6}^{207} + n_{R8}^{207} & n_{A7}^{75} &= n_{R6}^{207} + n_{R8}^{207} & n_{A8}^{75} &= n_{R7}^{207} + n_{R8}^{207} \\ n_{A6}^{75} &= n_{R7}^{207} + n_{R8}^{207} & n_{R4}^{75} &= n_{M6}^{207} + n_{M7}^{207} & n_{R3}^{75} &= n_{M6}^{207} + n_{M7}^{207} & n_{Z5}^{75} &= n_{X7}^{207} & n_{Z7}^{75} &= n_{X7}^{207} & n_{Z8}^{75} &= n_{X6}^{207} & n_{Z6}^{75} &= n_{X6}^{207} \end{aligned}$$

The lower SG is SG 75 when the preserved operations are: **(sub-SG label is 7) 1, 4, 5, 9.**

The transformation is:  $(\mathbf{a}_{75}, \mathbf{b}_{75}, \mathbf{c}_{75}) = (\mathbf{a}_{207}, \mathbf{b}_{207}, \mathbf{c}_{207}) \begin{pmatrix} -1 & 0 & 0 \\ 0 & 0 & 1 \\ 0 & 1 & 0 \end{pmatrix}, \overrightarrow{O_{207}O_{75}} = -\frac{1}{2}\mathbf{a}_{75} + (\frac{1}{2})\mathbf{b}_{75}$

The reduction of higher dimensional irrep:

$O : T_1 \rightarrow A + {}^2E + {}^1E$  of  $C_4$ .

$O : T_2 \rightarrow {}^2E + B + {}^1E$  of  $C_4$ .

The correspondences of irreps at HSPs from original SG to lowered SG:

$$\begin{aligned} n_{GM5}^{75} &= n_{GM7}^{207} + n_{GM8}^{207} & n_{GM7}^{75} &= n_{GM7}^{207} + n_{GM8}^{207} & n_{GM8}^{75} &= n_{GM6}^{207} + n_{GM8}^{207} & n_{GM6}^{75} &= n_{GM6}^{207} + n_{GM8}^{207} & n_{X4}^{75} &= n_{X6}^{207} + n_{X7}^{207} & n_{X3}^{75} &= \\ n_{X6}^{207} + n_{X7}^{207} & n_{M5}^{75} &= n_{M7}^{207} & n_{M7}^{75} &= n_{M7}^{207} & n_{M8}^{75} &= n_{M6}^{207} & n_{M6}^{75} &= n_{M6}^{207} & n_{A5}^{75} &= n_{R6}^{207} + n_{R8}^{207} & n_{A7}^{75} &= n_{R6}^{207} + n_{R8}^{207} & n_{A8}^{75} &= n_{R7}^{207} + n_{R8}^{207} \\ n_{A6}^{75} &= n_{R7}^{207} + n_{R8}^{207} & n_{R4}^{75} &= n_{M6}^{207} + n_{M7}^{207} & n_{R3}^{75} &= n_{M6}^{207} + n_{M7}^{207} & n_{Z5}^{75} &= n_{X7}^{207} & n_{Z7}^{75} &= n_{X7}^{207} & n_{Z8}^{75} &= n_{X6}^{207} & n_{Z6}^{75} &= n_{X6}^{207} \end{aligned}$$

The lower SG is SG 89 when the preserved operations are: **(sub-SG label is 8) 1, 6, 7, 10, 8, 9, 11, 12.**

The transformation is:  $(\mathbf{a}_{89}, \mathbf{b}_{89}, \mathbf{c}_{89}) = (\mathbf{a}_{207}, \mathbf{b}_{207}, \mathbf{c}_{207}) \begin{pmatrix} -1 & 0 & 0 \\ 0 & -1 & 0 \\ 0 & 0 & 1 \end{pmatrix}, \overrightarrow{O_{207}O_{89}} = \frac{1}{2}\mathbf{c}_{89}$

The reduction of higher dimensional irrep:

$O : E \rightarrow A_1 + B_1$  of  $D_4$ .

The correspondences of irreps at HSPs from original SG to lowered SG:

$$\begin{aligned} n_{GM6}^{89} &= n_{GM7}^{207} + n_{GM8}^{207} & n_{GM7}^{89} &= n_{GM6}^{207} + n_{GM8}^{207} & n_{X5}^{89} &= n_{X6}^{207} + n_{X7}^{207} & n_{M6}^{89} &= n_{M6}^{207} & n_{M7}^{89} &= n_{M7}^{207} & n_{A6}^{89} &= n_{R7}^{207} + n_{R8}^{207} & n_{A7}^{89} &= \\ n_{R6}^{207} + n_{R8}^{207} & n_{R5}^{89} &= n_{M6}^{207} + n_{M7}^{207} & n_{Z6}^{89} &= n_{X7}^{207} & n_{Z7}^{89} &= n_{X6}^{207} \end{aligned}$$

The lower SG is SG 89 when the preserved operations are: **(sub-SG label is 9) 1, 2, 3, 8, 9, 10, 13, 14.**

The transformation is:  $(\mathbf{a}_{89}, \mathbf{b}_{89}, \mathbf{c}_{89}) = (\mathbf{a}_{207}, \mathbf{b}_{207}, \mathbf{c}_{207}) \begin{pmatrix} 0 & 0 & 1 \\ -1 & 0 & 0 \\ 0 & -1 & 0 \end{pmatrix}, \overrightarrow{O_{207}O_{89}} = \frac{1}{2}\mathbf{c}_{89}$

The reduction of higher dimensional irrep:

$O : E \rightarrow A_1 + B_1$  of  $D_4$ .

The correspondences of irreps at HSPs from original SG to lowered SG:

$$\begin{aligned} n_{GM6}^{89} &= n_{GM7}^{207} + n_{GM8}^{207} & n_{GM7}^{89} &= n_{GM6}^{207} + n_{GM8}^{207} & n_{X5}^{89} &= n_{X6}^{207} + n_{X7}^{207} & n_{M6}^{89} &= n_{M6}^{207} & n_{M7}^{89} &= n_{M7}^{207} & n_{A6}^{89} &= n_{R7}^{207} + n_{R8}^{207} & n_{A7}^{89} &= \\ n_{R6}^{207} + n_{R8}^{207} & n_{R5}^{89} &= n_{M6}^{207} + n_{M7}^{207} & n_{Z6}^{89} &= n_{X7}^{207} & n_{Z7}^{89} &= n_{X6}^{207} \end{aligned}$$

The lower SG is SG 89 when the preserved operations are: **(sub-SG label is 10) 1, 4, 5, 9, 10, 8, 16, 15.**

The transformation is:  $(\mathbf{a}_{89}, \mathbf{b}_{89}, \mathbf{c}_{89}) = (\mathbf{a}_{207}, \mathbf{b}_{207}, \mathbf{c}_{207}) \begin{pmatrix} -1 & 0 & 0 \\ 0 & 0 & 1 \\ 0 & 1 & 0 \end{pmatrix}, \overrightarrow{O_{207}O_{89}} = \frac{1}{2}\mathbf{c}_{89}$

The reduction of higher dimensional irrep:

$O : E \rightarrow A_1 + B_1$  of  $D_4$ .

The correspondences of irreps at HSPs from original SG to lowered SG:

$$\begin{aligned} n_{GM6}^{89} &= n_{GM7}^{207} + n_{GM8}^{207} & n_{GM7}^{89} &= n_{GM6}^{207} + n_{GM8}^{207} & n_{X5}^{89} &= n_{X6}^{207} + n_{X7}^{207} & n_{M6}^{89} &= n_{M6}^{207} & n_{M7}^{89} &= n_{M7}^{207} & n_{A6}^{89} &= n_{R7}^{207} + n_{R8}^{207} & n_{A7}^{89} &= \\ n_{R6}^{207} + n_{R8}^{207} & n_{R5}^{89} &= n_{M6}^{207} + n_{M7}^{207} & n_{Z6}^{89} &= n_{X7}^{207} & n_{Z7}^{89} &= n_{X6}^{207} \end{aligned}$$

The lower SG is SG 146 when the preserved operations are: **(sub-SG label is 11) 1, 17, 18.**

The transformation is:  $(\mathbf{a}_{146}, \mathbf{b}_{146}, \mathbf{c}_{146}) = (\mathbf{a}_{207}, \mathbf{b}_{207}, \mathbf{c}_{207}) \begin{pmatrix} 0 & 1 & 0 \\ 0 & 0 & 1 \\ 1 & 0 & 0 \end{pmatrix}, \overrightarrow{O_{207}O_{146}} = -\frac{1}{3}\mathbf{a}_{146} + (\frac{2}{3})\mathbf{b}_{146} + (-\frac{1}{3})\mathbf{c}_{146}$

The reduction of higher dimensional irrep:

$$O : T_1 \rightarrow A + {}^2E + {}^1E \text{ of } C_3.$$

$$O : T_2 \rightarrow A + {}^2E + {}^1E \text{ of } C_3.$$

The correspondences of irreps at HSPs from original SG to lowered SG:

$$\begin{aligned} n_{GM4}^{146} &= 2n_{GM8}^{207} \quad n_{GM6}^{146} = n_{GM6}^{207} + n_{GM7}^{207} + n_{GM8}^{207} \quad n_{GM5}^{146} = n_{GM6}^{207} + n_{GM7}^{207} + n_{GM8}^{207} \quad n_{L2}^{146} = 2n_{X6}^{207} + 2n_{X7}^{207} \quad n_{F2}^{146} = \\ 2n_{M6}^{207} + 2n_{M7}^{207} \quad n_{T4}^{146} &= 2n_{R8}^{207} \quad n_{T6}^{146} = n_{R6}^{207} + n_{R7}^{207} + n_{R8}^{207} \quad n_{T5}^{146} = n_{R6}^{207} + n_{R7}^{207} + n_{R8}^{207} \end{aligned}$$

The lower SG is SG 146 when the preserved operations are: **(sub-SG label is 12) 1, 24, 23.**

$$\text{The transformation is: } (\mathbf{a}_{146}, \mathbf{b}_{146}, \mathbf{c}_{146}) = (\mathbf{a}_{207}, \mathbf{b}_{207}, \mathbf{c}_{207}) \begin{pmatrix} 0 & -1 & 0 \\ 0 & 0 & -1 \\ 1 & 0 & 0 \end{pmatrix}, \overrightarrow{O_{207}O_{146}} = -\frac{1}{3}\mathbf{a}_{146} + \left(\frac{2}{3}\right)\mathbf{b}_{146} + \left(-\frac{1}{3}\right)\mathbf{c}_{146}$$

The reduction of higher dimensional irrep:

$$O : T_1 \rightarrow A + {}^2E + {}^1E \text{ of } C_3.$$

$$O : T_2 \rightarrow A + {}^2E + {}^1E \text{ of } C_3.$$

The correspondences of irreps at HSPs from original SG to lowered SG:

$$\begin{aligned} n_{GM4}^{146} &= 2n_{GM8}^{207} \quad n_{GM6}^{146} = n_{GM6}^{207} + n_{GM7}^{207} + n_{GM8}^{207} \quad n_{GM5}^{146} = n_{GM6}^{207} + n_{GM7}^{207} + n_{GM8}^{207} \quad n_{L2}^{146} = 2n_{X6}^{207} + 2n_{X7}^{207} \quad n_{F2}^{146} = \\ 2n_{M6}^{207} + 2n_{M7}^{207} \quad n_{T4}^{146} &= 2n_{R8}^{207} \quad n_{T6}^{146} = n_{R6}^{207} + n_{R7}^{207} + n_{R8}^{207} \quad n_{T5}^{146} = n_{R6}^{207} + n_{R7}^{207} + n_{R8}^{207} \end{aligned}$$

The lower SG is SG 146 when the preserved operations are: **(sub-SG label is 13) 1, 20, 19.**

$$\text{The transformation is: } (\mathbf{a}_{146}, \mathbf{b}_{146}, \mathbf{c}_{146}) = (\mathbf{a}_{207}, \mathbf{b}_{207}, \mathbf{c}_{207}) \begin{pmatrix} 1 & 0 & 0 \\ 0 & -1 & 0 \\ 0 & 0 & -1 \end{pmatrix}, \overrightarrow{O_{207}O_{146}} = -\frac{1}{3}\mathbf{a}_{146} + \left(\frac{2}{3}\right)\mathbf{b}_{146} + \left(-\frac{1}{3}\right)\mathbf{c}_{146}$$

The reduction of higher dimensional irrep:

$$O : T_1 \rightarrow A + {}^2E + {}^1E \text{ of } C_3.$$

$$O : T_2 \rightarrow A + {}^2E + {}^1E \text{ of } C_3.$$

The correspondences of irreps at HSPs from original SG to lowered SG:

$$\begin{aligned} n_{GM4}^{146} &= 2n_{GM8}^{207} \quad n_{GM6}^{146} = n_{GM6}^{207} + n_{GM7}^{207} + n_{GM8}^{207} \quad n_{GM5}^{146} = n_{GM6}^{207} + n_{GM7}^{207} + n_{GM8}^{207} \quad n_{L2}^{146} = 2n_{X6}^{207} + 2n_{X7}^{207} \quad n_{F2}^{146} = \\ 2n_{M6}^{207} + 2n_{M7}^{207} \quad n_{T4}^{146} &= 2n_{R8}^{207} \quad n_{T6}^{146} = n_{R6}^{207} + n_{R7}^{207} + n_{R8}^{207} \quad n_{T5}^{146} = n_{R6}^{207} + n_{R7}^{207} + n_{R8}^{207} \end{aligned}$$

The lower SG is SG 146 when the preserved operations are: **(sub-SG label is 14) 1, 22, 21.**

$$\text{The transformation is: } (\mathbf{a}_{146}, \mathbf{b}_{146}, \mathbf{c}_{146}) = (\mathbf{a}_{207}, \mathbf{b}_{207}, \mathbf{c}_{207}) \begin{pmatrix} -1 & 0 & 0 \\ 0 & 1 & 0 \\ 0 & 0 & -1 \end{pmatrix}, \overrightarrow{O_{207}O_{146}} = -\frac{1}{3}\mathbf{a}_{146} + \left(\frac{2}{3}\right)\mathbf{b}_{146} + \left(-\frac{1}{3}\right)\mathbf{c}_{146}$$

The reduction of higher dimensional irrep:

$$O : T_1 \rightarrow A + {}^2E + {}^1E \text{ of } C_3.$$

$$O : T_2 \rightarrow A + {}^2E + {}^1E \text{ of } C_3.$$

The correspondences of irreps at HSPs from original SG to lowered SG:

$$\begin{aligned} n_{GM4}^{146} &= 2n_{GM8}^{207} \quad n_{GM6}^{146} = n_{GM6}^{207} + n_{GM7}^{207} + n_{GM8}^{207} \quad n_{GM5}^{146} = n_{GM6}^{207} + n_{GM7}^{207} + n_{GM8}^{207} \quad n_{L2}^{146} = 2n_{X6}^{207} + 2n_{X7}^{207} \quad n_{F2}^{146} = \\ 2n_{M6}^{207} + 2n_{M7}^{207} \quad n_{T4}^{146} &= 2n_{R8}^{207} \quad n_{T6}^{146} = n_{R6}^{207} + n_{R7}^{207} + n_{R8}^{207} \quad n_{T5}^{146} = n_{R6}^{207} + n_{R7}^{207} + n_{R8}^{207} \end{aligned}$$

The lower SG is SG 195 when the preserved operations are: **(sub-SG label is 15) 1, 8, 9, 10, 17, 24, 20, 22, 18, 23, 19, 21.**

$$\text{The transformation is: } (\mathbf{a}_{195}, \mathbf{b}_{195}, \mathbf{c}_{195}) = (\mathbf{a}_{207}, \mathbf{b}_{207}, \mathbf{c}_{207}) \begin{pmatrix} 0 & 0 & 1 \\ 1 & 0 & 0 \\ 0 & 1 & 0 \end{pmatrix}, \overrightarrow{O_{207}O_{195}} = \mathbf{0}$$

The reduction of higher dimensional irrep:

$$O : E \rightarrow {}^1E + {}^2E \text{ of } T.$$

The correspondences of irreps at HSPs from original SG to lowered SG:

$$\begin{aligned} n_{GM6}^{195} &= n_{GM8}^{207} \quad n_{GM7}^{195} = n_{GM8}^{207} \quad n_{GM5}^{195} = n_{GM6}^{207} + n_{GM7}^{207} \quad n_{X5}^{195} = n_{X6}^{207} + n_{X7}^{207} \quad n_{M5}^{195} = n_{M6}^{207} + n_{M7}^{207} \quad n_{R6}^{195} = n_{R8}^{207} \quad n_{R7}^{195} = n_{R8}^{207} \\ n_{R5}^{195} &= n_{R6}^{207} + n_{R7}^{207} \end{aligned}$$

### 105. Lowered SGs by higher-dimensional irreps of pairings in SG 208

The representative operations of SG/T for SG 208:

$$\begin{aligned}
& 1 : (x, y, z), 2 : (x + \frac{1}{2}, \frac{1}{2} - z, y + \frac{1}{2}), 3 : (x + \frac{1}{2}, z + \frac{1}{2}, \frac{1}{2} - y), 4 : (z + \frac{1}{2}, y + \frac{1}{2}, \frac{1}{2} - x), 5 : (\frac{1}{2} - z, y + \frac{1}{2}, x + \frac{1}{2}), \\
& 6 : (\frac{1}{2} - y, x + \frac{1}{2}, z + \frac{1}{2}), 7 : (y + \frac{1}{2}, \frac{1}{2} - x, z + \frac{1}{2}), 8 : (x, -y, -z), 9 : (-x, y, -z), 10 : (-x, -y, z), 11 : (y + \frac{1}{2}, x + \frac{1}{2}, \frac{1}{2} - z), \\
& 12 : (\frac{1}{2} - y, \frac{1}{2} - x, \frac{1}{2} - z), 13 : (\frac{1}{2} - x, z + \frac{1}{2}, y + \frac{1}{2}), 14 : (\frac{1}{2} - x, \frac{1}{2} - z, \frac{1}{2} - y), 15 : (z + \frac{1}{2}, \frac{1}{2} - y, x + \frac{1}{2}), 16 : (\frac{1}{2} - z, \frac{1}{2} - y, \frac{1}{2} - x), \\
& 17 : (z, x, y), 18 : (y, z, x), 19 : (-y, z, -x), 20 : (-z, -x, y), 21 : (-y, -z, x), 22 : (z, -x, -y), 23 : (y, -z, -x), \\
& 24 : (-z, x, -y).
\end{aligned}$$

The lower SG is SG 16 when the preserved operations are: **(sub-SG label is 1) 1, 8, 9, 10.**

The transformation is:  $(\mathbf{a}_{16}, \mathbf{b}_{16}, \mathbf{c}_{16}) = (\mathbf{a}_{208}, \mathbf{b}_{208}, \mathbf{c}_{208}) \begin{pmatrix} 0 & 0 & 1 \\ 1 & 0 & 0 \\ 0 & 1 & 0 \end{pmatrix}, \overrightarrow{O_{208}O_{16}} = \frac{1}{2}\mathbf{a}_{16} + (\frac{1}{2})\mathbf{c}_{16}$

The reduction of higher dimensional irrep:

$$O : T_1 \rightarrow B_1 + B_2 + B_3 \quad \text{of} \quad D_2.$$

$$O : T_2 \rightarrow B_1 + B_2 + B_3 \quad \text{of} \quad D_2.$$

The correspondences of irreps at HSPs from original SG to lowered SG:

$$\begin{aligned}
n_{GM5}^{16} &= n_{GM6}^{208} + n_{GM7}^{208} + 2n_{GM8}^{208} & n_{X5}^{16} &= n_{X6}^{208} + n_{X7}^{208} & n_{S5}^{16} &= n_{M6}^{208} + n_{M7}^{208} & n_{R5}^{16} &= n_{R6}^{208} + n_{R7}^{208} + 2n_{R8}^{208} & n_{U5}^{16} &= n_{M6}^{208} + n_{M7}^{208} \\
n_{Z5}^{16} &= n_{X6}^{208} + n_{X7}^{208} & n_{T5}^{16} &= n_{M6}^{208} + n_{M7}^{208} & n_{Y5}^{16} &= n_{X6}^{208} + n_{X7}^{208}
\end{aligned}$$

The lower SG is SG 21 when the preserved operations are: **(sub-SG label is 2) 1, 8, 13, 14.**

The transformation is:  $(\mathbf{a}_{21}, \mathbf{b}_{21}, \mathbf{c}_{21}) = (\mathbf{a}_{208}, \mathbf{b}_{208}, \mathbf{c}_{208}) \begin{pmatrix} 0 & 0 & 1 \\ 1 & -1 & 0 \\ 1 & 1 & 0 \end{pmatrix}, \overrightarrow{O_{208}O_{21}} = \frac{1}{4}\mathbf{a}_{21} + (\frac{1}{4})\mathbf{b}_{21} + (\frac{1}{4})\mathbf{c}_{21}$

The reduction of higher dimensional irrep:

$$O : T_1 \rightarrow B_1 + B_2 + B_3 \quad \text{of} \quad D_2.$$

$$O : T_2 \rightarrow A_1 + B_2 + B_3 \quad \text{of} \quad D_2.$$

The correspondences of irreps at HSPs from original SG to lowered SG:

$$\begin{aligned}
n_{GM5}^{21} &= n_{GM6}^{208} + n_{GM7}^{208} + 2n_{GM8}^{208} & n_{Y5}^{21} &= n_{M6}^{208} + n_{M7}^{208} & n_{S4}^{21} &= n_{X6}^{208} + n_{X7}^{208} & n_{S3}^{21} &= n_{X6}^{208} + n_{X7}^{208} & n_{Z5}^{21} &= n_{X6}^{208} + n_{X7}^{208} & n_{T5}^{21} &= \\
n_{R6}^{208} + n_{R7}^{208} + 2n_{R8}^{208} & n_{R4}^{21} &= n_{M6}^{208} + n_{M7}^{208} & n_{R3}^{21} &= n_{M6}^{208} + n_{M7}^{208}
\end{aligned}$$

The lower SG is SG 21 when the preserved operations are: **(sub-SG label is 3) 1, 9, 16, 15.**

The transformation is:  $(\mathbf{a}_{21}, \mathbf{b}_{21}, \mathbf{c}_{21}) = (\mathbf{a}_{208}, \mathbf{b}_{208}, \mathbf{c}_{208}) \begin{pmatrix} -1 & -1 & 0 \\ 0 & 0 & 1 \\ -1 & 1 & 0 \end{pmatrix}, \overrightarrow{O_{208}O_{21}} = \frac{1}{4}\mathbf{a}_{21} + (\frac{1}{4})\mathbf{b}_{21} + (\frac{1}{4})\mathbf{c}_{21}$

The reduction of higher dimensional irrep:

$$O : T_1 \rightarrow B_1 + B_2 + B_3 \quad \text{of} \quad D_2.$$

$$O : T_2 \rightarrow A_1 + B_2 + B_3 \quad \text{of} \quad D_2.$$

The correspondences of irreps at HSPs from original SG to lowered SG:

$$\begin{aligned}
n_{GM5}^{21} &= n_{GM6}^{208} + n_{GM7}^{208} + 2n_{GM8}^{208} & n_{Y5}^{21} &= n_{M6}^{208} + n_{M7}^{208} & n_{S4}^{21} &= n_{X6}^{208} + n_{X7}^{208} & n_{S3}^{21} &= n_{X6}^{208} + n_{X7}^{208} & n_{Z5}^{21} &= n_{X6}^{208} + n_{X7}^{208} & n_{T5}^{21} &= \\
n_{R6}^{208} + n_{R7}^{208} + 2n_{R8}^{208} & n_{R4}^{21} &= n_{M6}^{208} + n_{M7}^{208} & n_{R3}^{21} &= n_{M6}^{208} + n_{M7}^{208}
\end{aligned}$$

The lower SG is SG 21 when the preserved operations are: **(sub-SG label is 4) 1, 10, 11, 12.**

The transformation is:  $(\mathbf{a}_{21}, \mathbf{b}_{21}, \mathbf{c}_{21}) = (\mathbf{a}_{208}, \mathbf{b}_{208}, \mathbf{c}_{208}) \begin{pmatrix} -1 & -1 & 0 \\ 1 & -1 & 0 \\ 0 & 0 & 1 \end{pmatrix}, \overrightarrow{O_{208}O_{21}} = \frac{1}{4}\mathbf{a}_{21} + (\frac{1}{4})\mathbf{b}_{21} + (\frac{3}{4})\mathbf{c}_{21}$

The reduction of higher dimensional irrep:

$$O : T_1 \rightarrow B_1 + B_2 + B_3 \quad \text{of} \quad D_2.$$

$$O : T_2 \rightarrow A_1 + B_2 + B_3 \quad \text{of} \quad D_2.$$

The correspondences of irreps at HSPs from original SG to lowered SG:

$$\begin{aligned}
n_{GM5}^{21} &= n_{GM6}^{208} + n_{GM7}^{208} + 2n_{GM8}^{208} & n_{Y5}^{21} &= n_{M6}^{208} + n_{M7}^{208} & n_{S4}^{21} &= n_{X6}^{208} + n_{X7}^{208} & n_{S3}^{21} &= n_{X6}^{208} + n_{X7}^{208} & n_{Z5}^{21} &= n_{X6}^{208} + n_{X7}^{208} & n_{T5}^{21} &= \\
n_{R6}^{208} + n_{R7}^{208} + 2n_{R8}^{208} & n_{R4}^{21} &= n_{M6}^{208} + n_{M7}^{208} & n_{R3}^{21} &= n_{M6}^{208} + n_{M7}^{208}
\end{aligned}$$

The lower SG is SG 77 when the preserved operations are: **(sub-SG label is 5) 1, 6, 7, 10.**

The transformation is:  $(\mathbf{a}_{77}, \mathbf{b}_{77}, \mathbf{c}_{77}) = (\mathbf{a}_{208}, \mathbf{b}_{208}, \mathbf{c}_{208}) \begin{pmatrix} -1 & 0 & 0 \\ 0 & -1 & 0 \\ 0 & 0 & 1 \end{pmatrix}, \overrightarrow{O_{208}O_{77}} = \frac{1}{2}\mathbf{b}_{77}$

The reduction of higher dimensional irrep:

$$O : T_1 \rightarrow A + {}^2E + {}^1E \quad \text{of} \quad C_4.$$

$O : T_2 \rightarrow {}^2E + B + {}^1E$  of  $C_4$ .

The correspondences of irreps at HSPs from original SG to lowered SG:

$$\begin{aligned} n_{GM5}^{77} &= n_{GM7}^{208} + n_{GM8}^{208} & n_{GM7}^{77} &= n_{GM7}^{208} + n_{GM8}^{208} & n_{GM8}^{77} &= n_{GM6}^{208} + n_{GM8}^{208} & n_{GM6}^{77} &= n_{GM6}^{208} + n_{GM8}^{208} & n_{X4}^{77} &= n_{X6}^{208} + n_{X7}^{208} & n_{X3}^{77} &= n_{X6}^{208} + n_{X7}^{208} \\ n_{X6}^{208} + n_{X7}^{208} & n_{M5}^{77} = n_{M7}^{208} & n_{M7}^{77} &= n_{M7}^{208} & n_{M8}^{77} &= n_{M6}^{208} & n_{M6}^{77} &= n_{M6}^{208} & n_{A5}^{77} &= n_{R7}^{208} + n_{R8}^{208} & n_{A8}^{77} &= n_{R6}^{208} + n_{R8}^{208} \\ n_{A6}^{77} &= n_{R7}^{208} + n_{R8}^{208} & n_{R4}^{77} &= n_{M6}^{208} + n_{M7}^{208} & n_{R3}^{77} &= n_{M6}^{208} + n_{M7}^{208} & n_{Z6}^{77} &= n_{X6}^{208} & n_{Z8}^{77} &= n_{X7}^{208} & n_{Z7}^{77} &= n_{X6}^{208} & n_{Z5}^{77} &= n_{X7}^{208} \end{aligned}$$

The lower SG is SG 77 when the preserved operations are: **(sub-SG label is 6) 1, 2, 3, 8.**

The transformation is:  $(\mathbf{a}_{77}, \mathbf{b}_{77}, \mathbf{c}_{77}) = (\mathbf{a}_{208}, \mathbf{b}_{208}, \mathbf{c}_{208}) \begin{pmatrix} 0 & 0 & -1 \\ -1 & 0 & 0 \\ 0 & 1 & 0 \end{pmatrix}, \overrightarrow{O_{208}O_{77}} = \frac{1}{2}\mathbf{a}_{77} + \mathbf{b}_{77}$

The reduction of higher dimensional irrep:

$O : T_1 \rightarrow A + {}^2E + {}^1E$  of  $C_4$ .

$O : T_2 \rightarrow {}^2E + B + {}^1E$  of  $C_4$ .

The correspondences of irreps at HSPs from original SG to lowered SG:

$$\begin{aligned} n_{GM5}^{77} &= n_{GM7}^{208} + n_{GM8}^{208} & n_{GM7}^{77} &= n_{GM7}^{208} + n_{GM8}^{208} & n_{GM8}^{77} &= n_{GM6}^{208} + n_{GM8}^{208} & n_{GM6}^{77} &= n_{GM6}^{208} + n_{GM8}^{208} & n_{X4}^{77} &= n_{X6}^{208} + n_{X7}^{208} & n_{X3}^{77} &= n_{X6}^{208} + n_{X7}^{208} \\ n_{X6}^{208} + n_{X7}^{208} & n_{M5}^{77} = n_{M7}^{208} & n_{M7}^{77} &= n_{M7}^{208} & n_{M8}^{77} &= n_{M6}^{208} & n_{M6}^{77} &= n_{M6}^{208} & n_{A5}^{77} &= n_{R6}^{208} + n_{R8}^{208} & n_{A8}^{77} &= n_{R7}^{208} + n_{R8}^{208} \\ n_{A6}^{77} &= n_{R7}^{208} + n_{R8}^{208} & n_{R4}^{77} &= n_{M6}^{208} + n_{M7}^{208} & n_{R3}^{77} &= n_{M6}^{208} + n_{M7}^{208} & n_{Z6}^{77} &= n_{X6}^{208} & n_{Z8}^{77} &= n_{X7}^{208} & n_{Z7}^{77} &= n_{X6}^{208} & n_{Z5}^{77} &= n_{X7}^{208} \end{aligned}$$

The lower SG is SG 77 when the preserved operations are: **(sub-SG label is 7) 1, 4, 5, 9.**

The transformation is:  $(\mathbf{a}_{77}, \mathbf{b}_{77}, \mathbf{c}_{77}) = (\mathbf{a}_{208}, \mathbf{b}_{208}, \mathbf{c}_{208}) \begin{pmatrix} -1 & 0 & 0 \\ 0 & 0 & -1 \\ 0 & -1 & 0 \end{pmatrix}, \overrightarrow{O_{208}O_{77}} = \mathbf{a}_{77} + (\frac{1}{2})\mathbf{b}_{77}$

The reduction of higher dimensional irrep:

$O : T_1 \rightarrow A + {}^2E + {}^1E$  of  $C_4$ .

$O : T_2 \rightarrow {}^2E + B + {}^1E$  of  $C_4$ .

The correspondences of irreps at HSPs from original SG to lowered SG:

$$\begin{aligned} n_{GM5}^{77} &= n_{GM7}^{208} + n_{GM8}^{208} & n_{GM7}^{77} &= n_{GM7}^{208} + n_{GM8}^{208} & n_{GM8}^{77} &= n_{GM6}^{208} + n_{GM8}^{208} & n_{GM6}^{77} &= n_{GM6}^{208} + n_{GM8}^{208} & n_{X4}^{77} &= n_{X6}^{208} + n_{X7}^{208} & n_{X3}^{77} &= n_{X6}^{208} + n_{X7}^{208} \\ n_{X6}^{208} + n_{X7}^{208} & n_{M5}^{77} = n_{M7}^{208} & n_{M7}^{77} &= n_{M7}^{208} & n_{M8}^{77} &= n_{M6}^{208} & n_{M6}^{77} &= n_{M6}^{208} & n_{A5}^{77} &= n_{R6}^{208} + n_{R8}^{208} & n_{A8}^{77} &= n_{R7}^{208} + n_{R8}^{208} \\ n_{A6}^{77} &= n_{R7}^{208} + n_{R8}^{208} & n_{R4}^{77} &= n_{M6}^{208} + n_{M7}^{208} & n_{R3}^{77} &= n_{M6}^{208} + n_{M7}^{208} & n_{Z6}^{77} &= n_{X6}^{208} & n_{Z8}^{77} &= n_{X7}^{208} & n_{Z7}^{77} &= n_{X6}^{208} & n_{Z5}^{77} &= n_{X7}^{208} \end{aligned}$$

The lower SG is SG 93 when the preserved operations are: **(sub-SG label is 8) 1, 6, 7, 10, 8, 9, 11, 12.**

The transformation is:  $(\mathbf{a}_{93}, \mathbf{b}_{93}, \mathbf{c}_{93}) = (\mathbf{a}_{208}, \mathbf{b}_{208}, \mathbf{c}_{208}) \begin{pmatrix} -1 & 0 & 0 \\ 0 & -1 & 0 \\ 0 & 0 & 1 \end{pmatrix}, \overrightarrow{O_{208}O_{93}} = \frac{1}{2}\mathbf{b}_{93} + (\frac{1}{2})\mathbf{c}_{93}$

The reduction of higher dimensional irrep:

$O : E \rightarrow A_1 + B_1$  of  $D_4$ .

The correspondences of irreps at HSPs from original SG to lowered SG:

$$\begin{aligned} n_{GM6}^{93} &= n_{GM7}^{208} + n_{GM8}^{208} & n_{GM7}^{93} &= n_{GM6}^{208} + n_{GM8}^{208} & n_{X5}^{93} &= n_{X6}^{208} + n_{X7}^{208} & n_{M6}^{93} &= n_{M7}^{208} & n_{M7}^{93} &= n_{M6}^{208} & n_{A6}^{93} &= n_{R7}^{208} + n_{R8}^{208} & n_{A7}^{93} &= n_{R6}^{208} + n_{R8}^{208} \\ n_{R6}^{208} + n_{R8}^{208} & n_{R5}^{93} = n_{M6}^{208} + n_{M7}^{208} & n_{Z7}^{93} &= n_{X6}^{208} & n_{Z6}^{93} &= n_{X7}^{208} \end{aligned}$$

The lower SG is SG 93 when the preserved operations are: **(sub-SG label is 9) 1, 2, 3, 8, 9, 10, 13, 14.**

The transformation is:  $(\mathbf{a}_{93}, \mathbf{b}_{93}, \mathbf{c}_{93}) = (\mathbf{a}_{208}, \mathbf{b}_{208}, \mathbf{c}_{208}) \begin{pmatrix} 0 & 0 & 1 \\ -1 & 0 & 0 \\ 0 & -1 & 0 \end{pmatrix}, \overrightarrow{O_{208}O_{93}} = \frac{1}{2}\mathbf{b}_{93} + (\frac{1}{2})\mathbf{c}_{93}$

The reduction of higher dimensional irrep:

$O : E \rightarrow A_1 + B_1$  of  $D_4$ .

The correspondences of irreps at HSPs from original SG to lowered SG:

$$\begin{aligned} n_{GM6}^{93} &= n_{GM7}^{208} + n_{GM8}^{208} & n_{GM7}^{93} &= n_{GM6}^{208} + n_{GM8}^{208} & n_{X5}^{93} &= n_{X6}^{208} + n_{X7}^{208} & n_{M6}^{93} &= n_{M7}^{208} & n_{M7}^{93} &= n_{M6}^{208} & n_{A6}^{93} &= n_{R7}^{208} + n_{R8}^{208} & n_{A7}^{93} &= n_{R6}^{208} + n_{R8}^{208} \\ n_{R6}^{208} + n_{R8}^{208} & n_{R5}^{93} = n_{M6}^{208} + n_{M7}^{208} & n_{Z7}^{93} &= n_{X6}^{208} & n_{Z6}^{93} &= n_{X7}^{208} \end{aligned}$$

The lower SG is SG 93 when the preserved operations are: **(sub-SG label is 10) 1, 4, 5, 9, 10, 8, 16, 15.**

The transformation is:  $(\mathbf{a}_{93}, \mathbf{b}_{93}, \mathbf{c}_{93}) = (\mathbf{a}_{208}, \mathbf{b}_{208}, \mathbf{c}_{208}) \begin{pmatrix} -1 & 0 & 0 \\ 0 & 0 & 1 \\ 0 & 1 & 0 \end{pmatrix}, \overrightarrow{O_{208}O_{93}} = \frac{1}{2}\mathbf{b}_{93} + (\frac{1}{2})\mathbf{c}_{93}$

The reduction of higher dimensional irrep:

$O : E \rightarrow A_1 + B_1$  of  $D_4$ .

The correspondences of irreps at HSPs from original SG to lowered SG:

$$\begin{aligned} n_{GM6}^{93} &= n_{GM7}^{208} + n_{GM8}^{208} & n_{GM7}^{93} &= n_{GM6}^{208} + n_{GM8}^{208} & n_{X5}^{93} &= n_{X6}^{208} + n_{X7}^{208} & n_{M6}^{93} &= n_{M7}^{208} & n_{M7}^{93} &= n_{M6}^{208} & n_{A6}^{93} &= n_{R6}^{208} + n_{R8}^{208} & n_{A7}^{93} &= n_{R6}^{208} + n_{R8}^{208} \end{aligned}$$

$$n_{R7}^{208} + n_{R8}^{208} n_{R5}^{93} = n_{M6}^{208} + n_{M7}^{208} n_{Z7}^{93} = n_{X6}^{208} n_{Z6}^{93} = n_{X7}^{208}$$

The lower SG is SG 146 when the preserved operations are: **(sub-SG label is 11)** 1, 17, 18.

$$\text{The transformation is: } (\mathbf{a}_{146}, \mathbf{b}_{146}, \mathbf{c}_{146}) = (\mathbf{a}_{208}, \mathbf{b}_{208}, \mathbf{c}_{208}) \begin{pmatrix} 0 & 1 & 0 \\ 0 & 0 & 1 \\ 1 & 0 & 0 \end{pmatrix}, \overrightarrow{O_{208}O_{146}} = -\frac{1}{3}\mathbf{a}_{146} + \left(\frac{2}{3}\right)\mathbf{b}_{146} + \left(-\frac{1}{3}\right)\mathbf{c}_{146}$$

The reduction of higher dimensional irrep:

$$O : T_1 \rightarrow A + {}^2E + {}^1E \text{ of } C_3.$$

$$O : T_2 \rightarrow A + {}^2E + {}^1E \text{ of } C_3.$$

The correspondences of irreps at HSPs from original SG to lowered SG:

$$n_{GM4}^{146} = 2n_{GM8}^{208} n_{GM6}^{146} = n_{GM6}^{208} + n_{GM7}^{208} + n_{GM8}^{208} n_{GM5}^{146} = n_{GM6}^{208} + n_{GM7}^{208} + n_{GM8}^{208} n_{L2}^{146} = 2n_{X6}^{208} + 2n_{X7}^{208} n_{F2}^{146} = 2n_{M6}^{208} + 2n_{M7}^{208} n_{T4}^{146} = 2n_{R8}^{208} n_{T6}^{146} = n_{R6}^{208} + n_{R7}^{208} + n_{R8}^{208} n_{T5}^{146} = n_{R6}^{208} + n_{R7}^{208} + n_{R8}^{208}$$

The lower SG is SG 146 when the preserved operations are: **(sub-SG label is 12)** 1, 24, 23.

$$\text{The transformation is: } (\mathbf{a}_{146}, \mathbf{b}_{146}, \mathbf{c}_{146}) = (\mathbf{a}_{208}, \mathbf{b}_{208}, \mathbf{c}_{208}) \begin{pmatrix} 0 & -1 & 0 \\ 0 & 0 & -1 \\ 1 & 0 & 0 \end{pmatrix}, \overrightarrow{O_{208}O_{146}} = -\frac{1}{3}\mathbf{a}_{146} + \left(\frac{2}{3}\right)\mathbf{b}_{146} + \left(-\frac{1}{3}\right)\mathbf{c}_{146}$$

The reduction of higher dimensional irrep:

$$O : T_1 \rightarrow A + {}^2E + {}^1E \text{ of } C_3.$$

$$O : T_2 \rightarrow A + {}^2E + {}^1E \text{ of } C_3.$$

The correspondences of irreps at HSPs from original SG to lowered SG:

$$n_{GM4}^{146} = 2n_{GM8}^{208} n_{GM6}^{146} = n_{GM6}^{208} + n_{GM7}^{208} + n_{GM8}^{208} n_{GM5}^{146} = n_{GM6}^{208} + n_{GM7}^{208} + n_{GM8}^{208} n_{L2}^{146} = 2n_{X6}^{208} + 2n_{X7}^{208} n_{F2}^{146} = 2n_{M6}^{208} + 2n_{M7}^{208} n_{T4}^{146} = 2n_{R8}^{208} n_{T6}^{146} = n_{R6}^{208} + n_{R7}^{208} + n_{R8}^{208} n_{T5}^{146} = n_{R6}^{208} + n_{R7}^{208} + n_{R8}^{208}$$

The lower SG is SG 146 when the preserved operations are: **(sub-SG label is 13)** 1, 20, 19.

$$\text{The transformation is: } (\mathbf{a}_{146}, \mathbf{b}_{146}, \mathbf{c}_{146}) = (\mathbf{a}_{208}, \mathbf{b}_{208}, \mathbf{c}_{208}) \begin{pmatrix} 1 & 0 & 0 \\ 0 & -1 & 0 \\ 0 & 0 & -1 \end{pmatrix}, \overrightarrow{O_{208}O_{146}} = -\frac{1}{3}\mathbf{a}_{146} + \left(\frac{2}{3}\right)\mathbf{b}_{146} + \left(-\frac{1}{3}\right)\mathbf{c}_{146}$$

The reduction of higher dimensional irrep:

$$O : T_1 \rightarrow A + {}^2E + {}^1E \text{ of } C_3.$$

$$O : T_2 \rightarrow A + {}^2E + {}^1E \text{ of } C_3.$$

The correspondences of irreps at HSPs from original SG to lowered SG:

$$n_{GM4}^{146} = 2n_{GM8}^{208} n_{GM6}^{146} = n_{GM6}^{208} + n_{GM7}^{208} + n_{GM8}^{208} n_{GM5}^{146} = n_{GM6}^{208} + n_{GM7}^{208} + n_{GM8}^{208} n_{L2}^{146} = 2n_{X6}^{208} + 2n_{X7}^{208} n_{F2}^{146} = 2n_{M6}^{208} + 2n_{M7}^{208} n_{T4}^{146} = 2n_{R8}^{208} n_{T6}^{146} = n_{R6}^{208} + n_{R7}^{208} + n_{R8}^{208} n_{T5}^{146} = n_{R6}^{208} + n_{R7}^{208} + n_{R8}^{208}$$

The lower SG is SG 146 when the preserved operations are: **(sub-SG label is 14)** 1, 22, 21.

$$\text{The transformation is: } (\mathbf{a}_{146}, \mathbf{b}_{146}, \mathbf{c}_{146}) = (\mathbf{a}_{208}, \mathbf{b}_{208}, \mathbf{c}_{208}) \begin{pmatrix} -1 & 0 & 0 \\ 0 & 1 & 0 \\ 0 & 0 & -1 \end{pmatrix}, \overrightarrow{O_{208}O_{146}} = -\frac{1}{3}\mathbf{a}_{146} + \left(\frac{2}{3}\right)\mathbf{b}_{146} + \left(-\frac{1}{3}\right)\mathbf{c}_{146}$$

The reduction of higher dimensional irrep:

$$O : T_1 \rightarrow A + {}^2E + {}^1E \text{ of } C_3.$$

$$O : T_2 \rightarrow A + {}^2E + {}^1E \text{ of } C_3.$$

The correspondences of irreps at HSPs from original SG to lowered SG:

$$n_{GM4}^{146} = 2n_{GM8}^{208} n_{GM6}^{146} = n_{GM6}^{208} + n_{GM7}^{208} + n_{GM8}^{208} n_{GM5}^{146} = n_{GM6}^{208} + n_{GM7}^{208} + n_{GM8}^{208} n_{L2}^{146} = 2n_{X6}^{208} + 2n_{X7}^{208} n_{F2}^{146} = 2n_{M6}^{208} + 2n_{M7}^{208} n_{T4}^{146} = 2n_{R8}^{208} n_{T6}^{146} = n_{R6}^{208} + n_{R7}^{208} + n_{R8}^{208} n_{T5}^{146} = n_{R6}^{208} + n_{R7}^{208} + n_{R8}^{208}$$

The lower SG is SG 195 when the preserved operations are: **(sub-SG label is 15)** 1, 8, 9, 10, 17, 24, 20, 22, 18, 23, 19, 21.

$$\text{The transformation is: } (\mathbf{a}_{195}, \mathbf{b}_{195}, \mathbf{c}_{195}) = (\mathbf{a}_{208}, \mathbf{b}_{208}, \mathbf{c}_{208}) \begin{pmatrix} 0 & 0 & 1 \\ 1 & 0 & 0 \\ 0 & 1 & 0 \end{pmatrix}, \overrightarrow{O_{208}O_{195}} = \mathbf{0}$$

The reduction of higher dimensional irrep:

$$O : E \rightarrow {}^1E + {}^2E \text{ of } T.$$

The correspondences of irreps at HSPs from original SG to lowered SG:

$$n_{GM6}^{195} = n_{GM8}^{208} n_{GM7}^{195} = n_{GM8}^{208} n_{GM5}^{195} = n_{GM6}^{208} + n_{GM7}^{208} n_{X5}^{195} = n_{X6}^{208} + n_{X7}^{208} n_{M5}^{195} = n_{M6}^{208} + n_{M7}^{208} n_{R6}^{195} = n_{R8}^{208} n_{R7}^{195} = n_{R8}^{208}$$

$$n_{R5}^{195} = n_{R6}^{208} + n_{R7}^{208}$$

## 106. Lowered SGs by higher-dimensional irreps of pairings in SG 209

The representative operations of SG/T for SG 209:

$$1 : (x, y, z), 2 : (x, -z, y), 3 : (x, z, -y), 4 : (z, y, -x), 5 : (-z, y, x), 6 : (-y, x, z), 7 : (y, -x, z), 8 : (x, -y, -z), \\ 9 : (-x, y, -z), 10 : (-x, -y, z), 11 : (y, x, -z), 12 : (-y, -x, -z), 13 : (-x, z, y), 14 : (-x, -z, -y), 15 : (z, -y, x), \\ 16 : (-z, -y, -x), 17 : (z, x, y), 18 : (y, z, x), 19 : (-y, z, -x), 20 : (-z, -x, y), 21 : (-y, -z, x), 22 : (z, -x, -y), \\ 23 : (y, -z, -x), 24 : (-z, x, -y).$$

The lower SG is SG 22 when the preserved operations are: **(sub-SG label is 1) 1, 8, 9, 10.**

$$\text{The transformation is: } (\mathbf{a}_{22}, \mathbf{b}_{22}, \mathbf{c}_{22}) = (\mathbf{a}_{209}, \mathbf{b}_{209}, \mathbf{c}_{209}) \begin{pmatrix} 0 & 0 & 1 \\ 1 & 0 & 0 \\ 0 & 1 & 0 \end{pmatrix}, \overrightarrow{O_{209}O_{22}} = \frac{1}{4}\mathbf{a}_{22} + (-\frac{1}{4})\mathbf{b}_{22} + (-\frac{1}{4})\mathbf{c}_{22}$$

The reduction of higher dimensional irrep:

$$O : T_1 \rightarrow B_1 + B_2 + B_3 \text{ of } D_2.$$

$$O : T_2 \rightarrow B_1 + B_2 + B_3 \text{ of } D_2.$$

The correspondences of irreps at HSPs from original SG to lowered SG:

$$n_{GM5}^{22} = n_{GM6}^{209} + n_{GM7}^{209} + 2n_{GM8}^{209} \quad n_{Y5}^{22} = n_{X6}^{209} + n_{X7}^{209} \quad n_{L2}^{22} = n_{L4}^{209} + n_{L5}^{209} + 2n_{L6}^{209} \quad n_{Z5}^{22} = n_{X6}^{209} + n_{X7}^{209} \quad n_{T5}^{22} = n_{X6}^{209} + n_{X7}^{209}$$

The lower SG is SG 23 when the preserved operations are: **(sub-SG label is 2) 1, 8, 13, 14.**

$$\text{The transformation is: } (\mathbf{a}_{23}, \mathbf{b}_{23}, \mathbf{c}_{23}) = (\mathbf{a}_{209}, \mathbf{b}_{209}, \mathbf{c}_{209}) \begin{pmatrix} 0 & 0 & 1 \\ \frac{1}{2} & -\frac{1}{2} & 0 \\ \frac{1}{2} & \frac{1}{2} & 0 \end{pmatrix}, \overrightarrow{O_{209}O_{23}} = -\frac{1}{2}\mathbf{b}_{23}$$

The reduction of higher dimensional irrep:

$$O : T_1 \rightarrow B_1 + B_2 + B_3 \text{ of } D_2.$$

$$O : T_2 \rightarrow A_1 + B_2 + B_3 \text{ of } D_2.$$

The correspondences of irreps at HSPs from original SG to lowered SG:

$$n_{GM5}^{23} = n_{GM6}^{209} + n_{GM7}^{209} + 2n_{GM8}^{209} \quad n_{X5}^{23} = n_{X6}^{209} + n_{X7}^{209} \quad n_{T4}^{23} = n_{X6}^{209} + n_{X7}^{209} \quad n_{T3}^{23} = n_{X6}^{209} + n_{X7}^{209} \quad n_{W5}^{23} = n_{W5}^{209} \quad n_{R4}^{23} = n_{L5}^{209} + n_{L6}^{209} \\ n_{R3}^{23} = n_{L4}^{209} + n_{L6}^{209} \quad n_{S3}^{23} = n_{L4}^{209} + n_{L6}^{209} \quad n_{S4}^{23} = n_{L5}^{209} + n_{L6}^{209}$$

The lower SG is SG 23 when the preserved operations are: **(sub-SG label is 3) 1, 9, 16, 15.**

$$\text{The transformation is: } (\mathbf{a}_{23}, \mathbf{b}_{23}, \mathbf{c}_{23}) = (\mathbf{a}_{209}, \mathbf{b}_{209}, \mathbf{c}_{209}) \begin{pmatrix} -\frac{1}{2} & \frac{1}{2} & 0 \\ 0 & 0 & 1 \\ \frac{1}{2} & \frac{1}{2} & 0 \end{pmatrix}, \overrightarrow{O_{209}O_{23}} = -\frac{1}{2}\mathbf{b}_{23}$$

The reduction of higher dimensional irrep:

$$O : T_1 \rightarrow B_1 + B_2 + B_3 \text{ of } D_2.$$

$$O : T_2 \rightarrow A_1 + B_2 + B_3 \text{ of } D_2.$$

The correspondences of irreps at HSPs from original SG to lowered SG:

$$n_{GM5}^{23} = n_{GM6}^{209} + n_{GM7}^{209} + 2n_{GM8}^{209} \quad n_{X5}^{23} = n_{X6}^{209} + n_{X7}^{209} \quad n_{T4}^{23} = n_{X6}^{209} + n_{X7}^{209} \quad n_{T3}^{23} = n_{X6}^{209} + n_{X7}^{209} \quad n_{W5}^{23} = n_{W5}^{209} \quad n_{R4}^{23} = n_{L5}^{209} + n_{L6}^{209} \\ n_{R3}^{23} = n_{L4}^{209} + n_{L6}^{209} \quad n_{S3}^{23} = n_{L4}^{209} + n_{L6}^{209} \quad n_{S4}^{23} = n_{L5}^{209} + n_{L6}^{209}$$

The lower SG is SG 23 when the preserved operations are: **(sub-SG label is 4) 1, 10, 11, 12.**

$$\text{The transformation is: } (\mathbf{a}_{23}, \mathbf{b}_{23}, \mathbf{c}_{23}) = (\mathbf{a}_{209}, \mathbf{b}_{209}, \mathbf{c}_{209}) \begin{pmatrix} \frac{1}{2} & -\frac{1}{2} & 0 \\ \frac{1}{2} & \frac{1}{2} & 0 \\ 0 & 0 & 1 \end{pmatrix}, \overrightarrow{O_{209}O_{23}} = -\frac{1}{2}\mathbf{b}_{23}$$

The reduction of higher dimensional irrep:

$$O : T_1 \rightarrow B_1 + B_2 + B_3 \text{ of } D_2.$$

$$O : T_2 \rightarrow A_1 + B_2 + B_3 \text{ of } D_2.$$

The correspondences of irreps at HSPs from original SG to lowered SG:

$$n_{GM5}^{23} = n_{GM6}^{209} + n_{GM7}^{209} + 2n_{GM8}^{209} \quad n_{X5}^{23} = n_{X6}^{209} + n_{X7}^{209} \quad n_{T4}^{23} = n_{X6}^{209} + n_{X7}^{209} \quad n_{T3}^{23} = n_{X6}^{209} + n_{X7}^{209} \quad n_{W5}^{23} = n_{W5}^{209} \quad n_{R4}^{23} = n_{L5}^{209} + n_{L6}^{209} \\ n_{R3}^{23} = n_{L4}^{209} + n_{L6}^{209} \quad n_{S3}^{23} = n_{L4}^{209} + n_{L6}^{209} \quad n_{S4}^{23} = n_{L5}^{209} + n_{L6}^{209}$$

The lower SG is SG 79 when the preserved operations are: **(sub-SG label is 5) 1, 6, 7, 10.**

$$\text{The transformation is: } (\mathbf{a}_{79}, \mathbf{b}_{79}, \mathbf{c}_{79}) = (\mathbf{a}_{209}, \mathbf{b}_{209}, \mathbf{c}_{209}) \begin{pmatrix} \frac{1}{2} & \frac{1}{2} & 0 \\ -\frac{1}{2} & \frac{1}{2} & 0 \\ 0 & 0 & 1 \end{pmatrix}, \overrightarrow{O_{209}O_{79}} = \frac{1}{2}\mathbf{a}_{79} + (\frac{1}{2})\mathbf{b}_{79}$$

The reduction of higher dimensional irrep:

$$\begin{aligned} \text{O} : T_1 &\rightarrow \text{A} + {}^2\text{E} + {}^1\text{E} \text{ of } C_4. \\ \text{O} : T_2 &\rightarrow {}^2\text{E} + \text{B} + {}^1\text{E} \text{ of } C_4. \end{aligned}$$

The correspondences of irreps at HSPs from original SG to lowered SG:

$$\begin{aligned} n_{GM5}^{79} &= n_{GM7}^{209} + n_{GM8}^{209} \quad n_{GM7}^{79} = n_{GM7}^{209} + n_{GM8}^{209} \quad n_{GM8}^{79} = n_{GM6}^{209} + n_{GM8}^{209} \quad n_{GM6}^{79} = n_{GM6}^{209} + n_{GM8}^{209} \quad n_{M5}^{79} = n_{X7}^{209} \quad n_{M7}^{79} = n_{X7}^{209} \\ n_{M8}^{79} &= n_{X6}^{209} \quad n_{M6}^{79} = n_{X6}^{209} \quad n_{X4}^{79} = n_{X6}^{209} + n_{X7}^{209} \quad n_{X3}^{79} = n_{X6}^{209} + n_{X7}^{209} \quad n_{P4}^{79} = n_{W5}^{209} \quad n_{P3}^{79} = n_{W5}^{209} \quad n_{N2}^{79} = n_{L4}^{209} + n_{L5}^{209} + 2n_{L6}^{209} \end{aligned}$$

The lower SG is SG 79 when the preserved operations are: **(sub-SG label is 6) 1, 2, 3, 8.**

$$\text{The transformation is: } (\mathbf{a}_{79}, \mathbf{b}_{79}, \mathbf{c}_{79}) = (\mathbf{a}_{209}, \mathbf{b}_{209}, \mathbf{c}_{209}) \begin{pmatrix} 0 & 0 & 1 \\ -\frac{1}{2} & \frac{1}{2} & 0 \\ -\frac{1}{2} & -\frac{1}{2} & 0 \end{pmatrix}, \overrightarrow{O_{209}O_{79}} = \frac{1}{2}\mathbf{a}_{79} + \left(\frac{1}{2}\right)\mathbf{b}_{79}$$

The reduction of higher dimensional irrep:

$$\begin{aligned} \text{O} : T_1 &\rightarrow \text{A} + {}^2\text{E} + {}^1\text{E} \text{ of } C_4. \\ \text{O} : T_2 &\rightarrow {}^2\text{E} + \text{B} + {}^1\text{E} \text{ of } C_4. \end{aligned}$$

The correspondences of irreps at HSPs from original SG to lowered SG:

$$\begin{aligned} n_{GM5}^{79} &= n_{GM7}^{209} + n_{GM8}^{209} \quad n_{GM7}^{79} = n_{GM7}^{209} + n_{GM8}^{209} \quad n_{GM8}^{79} = n_{GM6}^{209} + n_{GM8}^{209} \quad n_{GM6}^{79} = n_{GM6}^{209} + n_{GM8}^{209} \quad n_{M5}^{79} = n_{X7}^{209} \quad n_{M7}^{79} = n_{X7}^{209} \\ n_{M8}^{79} &= n_{X6}^{209} \quad n_{M6}^{79} = n_{X6}^{209} \quad n_{X4}^{79} = n_{X6}^{209} + n_{X7}^{209} \quad n_{X3}^{79} = n_{X6}^{209} + n_{X7}^{209} \quad n_{P4}^{79} = n_{W5}^{209} \quad n_{P3}^{79} = n_{W5}^{209} \quad n_{N2}^{79} = n_{L4}^{209} + n_{L5}^{209} + 2n_{L6}^{209} \end{aligned}$$

The lower SG is SG 79 when the preserved operations are: **(sub-SG label is 7) 1, 4, 5, 9.**

$$\text{The transformation is: } (\mathbf{a}_{79}, \mathbf{b}_{79}, \mathbf{c}_{79}) = (\mathbf{a}_{209}, \mathbf{b}_{209}, \mathbf{c}_{209}) \begin{pmatrix} \frac{1}{2} & -\frac{1}{2} & 0 \\ 0 & 0 & 1 \\ -\frac{1}{2} & -\frac{1}{2} & 0 \end{pmatrix}, \overrightarrow{O_{209}O_{79}} = \frac{1}{2}\mathbf{a}_{79} + \left(\frac{1}{2}\right)\mathbf{b}_{79}$$

The reduction of higher dimensional irrep:

$$\begin{aligned} \text{O} : T_1 &\rightarrow \text{A} + {}^2\text{E} + {}^1\text{E} \text{ of } C_4. \\ \text{O} : T_2 &\rightarrow {}^2\text{E} + \text{B} + {}^1\text{E} \text{ of } C_4. \end{aligned}$$

The correspondences of irreps at HSPs from original SG to lowered SG:

$$\begin{aligned} n_{GM5}^{79} &= n_{GM7}^{209} + n_{GM8}^{209} \quad n_{GM7}^{79} = n_{GM7}^{209} + n_{GM8}^{209} \quad n_{GM8}^{79} = n_{GM6}^{209} + n_{GM8}^{209} \quad n_{GM6}^{79} = n_{GM6}^{209} + n_{GM8}^{209} \quad n_{M5}^{79} = n_{X7}^{209} \quad n_{M7}^{79} = n_{X7}^{209} \\ n_{M8}^{79} &= n_{X6}^{209} \quad n_{M6}^{79} = n_{X6}^{209} \quad n_{X4}^{79} = n_{X6}^{209} + n_{X7}^{209} \quad n_{X3}^{79} = n_{X6}^{209} + n_{X7}^{209} \quad n_{P4}^{79} = n_{W5}^{209} \quad n_{P3}^{79} = n_{W5}^{209} \quad n_{N2}^{79} = n_{L4}^{209} + n_{L5}^{209} + 2n_{L6}^{209} \end{aligned}$$

The lower SG is SG 97 when the preserved operations are: **(sub-SG label is 8) 1, 6, 7, 10, 8, 9, 11, 12.**

$$\text{The transformation is: } (\mathbf{a}_{97}, \mathbf{b}_{97}, \mathbf{c}_{97}) = (\mathbf{a}_{209}, \mathbf{b}_{209}, \mathbf{c}_{209}) \begin{pmatrix} \frac{1}{2} & \frac{1}{2} & 0 \\ -\frac{1}{2} & \frac{1}{2} & 0 \\ 0 & 0 & 1 \end{pmatrix}, \overrightarrow{O_{209}O_{97}} = \mathbf{0}$$

The reduction of higher dimensional irrep:

$$\text{O} : \text{E} \rightarrow A_1 + B_2 \text{ of } D_4.$$

The correspondences of irreps at HSPs from original SG to lowered SG:

$$\begin{aligned} n_{GM6}^{97} &= n_{GM7}^{209} + n_{GM8}^{209} \quad n_{GM7}^{97} = n_{GM6}^{209} + n_{GM8}^{209} \quad n_{M6}^{97} = n_{X7}^{209} \quad n_{M7}^{97} = n_{X6}^{209} \quad n_{X5}^{97} = n_{X6}^{209} + n_{X7}^{209} \quad n_{P5}^{97} = n_{W5}^{209} \quad n_{N4}^{97} = n_{L5}^{209} + n_{L6}^{209} \\ n_{N3}^{97} &= n_{L4}^{209} + n_{L6}^{209} \end{aligned}$$

The lower SG is SG 97 when the preserved operations are: **(sub-SG label is 9) 1, 2, 3, 8, 9, 10, 13, 14.**

$$\text{The transformation is: } (\mathbf{a}_{97}, \mathbf{b}_{97}, \mathbf{c}_{97}) = (\mathbf{a}_{209}, \mathbf{b}_{209}, \mathbf{c}_{209}) \begin{pmatrix} 0 & 0 & 1 \\ -\frac{1}{2} & \frac{1}{2} & 0 \\ -\frac{1}{2} & -\frac{1}{2} & 0 \end{pmatrix}, \overrightarrow{O_{209}O_{97}} = \mathbf{0}$$

The reduction of higher dimensional irrep:

$$\text{O} : \text{E} \rightarrow A_1 + B_2 \text{ of } D_4.$$

The correspondences of irreps at HSPs from original SG to lowered SG:

$$\begin{aligned} n_{GM6}^{97} &= n_{GM7}^{209} + n_{GM8}^{209} \quad n_{GM7}^{97} = n_{GM6}^{209} + n_{GM8}^{209} \quad n_{M6}^{97} = n_{X7}^{209} \quad n_{M7}^{97} = n_{X6}^{209} \quad n_{X5}^{97} = n_{X6}^{209} + n_{X7}^{209} \quad n_{P5}^{97} = n_{W5}^{209} \quad n_{N4}^{97} = n_{L5}^{209} + n_{L6}^{209} \\ n_{N3}^{97} &= n_{L4}^{209} + n_{L6}^{209} \end{aligned}$$

The lower SG is SG 97 when the preserved operations are: **(sub-SG label is 10) 1, 4, 5, 9, 10, 8, 16, 15.**

$$\text{The transformation is: } (\mathbf{a}_{97}, \mathbf{b}_{97}, \mathbf{c}_{97}) = (\mathbf{a}_{209}, \mathbf{b}_{209}, \mathbf{c}_{209}) \begin{pmatrix} \frac{1}{2} & -\frac{1}{2} & 0 \\ 0 & 0 & 1 \\ -\frac{1}{2} & -\frac{1}{2} & 0 \end{pmatrix}, \overrightarrow{O_{209}O_{97}} = \mathbf{0}$$

The reduction of higher dimensional irrep:

$$\text{O} : \text{E} \rightarrow A_1 + B_2 \text{ of } D_4.$$

The correspondences of irreps at HSPs from original SG to lowered SG:

$$\begin{aligned} n_{GM6}^{97} &= n_{GM7}^{209} + n_{GM8}^{209} \quad n_{GM7}^{97} = n_{GM6}^{209} + n_{GM8}^{209} \quad n_{M6}^{97} = n_{X7}^{209} \quad n_{M7}^{97} = n_{X6}^{209} \quad n_{X5}^{97} = n_{X6}^{209} + n_{X7}^{209} \quad n_{P5}^{97} = n_{W5}^{209} \quad n_{N4}^{97} = n_{L5}^{209} + n_{L6}^{209} \\ n_{N3}^{97} &= n_{L4}^{209} + n_{L6}^{209} \end{aligned}$$

The lower SG is SG 146 when the preserved operations are: **(sub-SG label is 11) 1, 17, 18.**

$$\text{The transformation is: } (\mathbf{a}_{146}, \mathbf{b}_{146}, \mathbf{c}_{146}) = (\mathbf{a}_{209}, \mathbf{b}_{209}, \mathbf{c}_{209}) \begin{pmatrix} \frac{1}{2} & 0 & \frac{1}{2} \\ \frac{1}{2} & \frac{1}{2} & 0 \\ 0 & \frac{1}{2} & \frac{1}{2} \end{pmatrix}, \overrightarrow{O_{209}O_{146}} = -\frac{1}{3}\mathbf{a}_{146} + \left(\frac{2}{3}\right)\mathbf{b}_{146} + \left(-\frac{1}{3}\right)\mathbf{c}_{146}$$

The reduction of higher dimensional irrep:

$$O : T_1 \rightarrow A + {}^2E + {}^1E \text{ of } C_3.$$

$$O : T_2 \rightarrow A + {}^2E + {}^1E \text{ of } C_3.$$

The correspondences of irreps at HSPs from original SG to lowered SG:

$$\begin{aligned} n_{GM4}^{146} &= 2n_{GM8}^{209} & n_{GM6}^{146} &= n_{GM6}^{209} + n_{GM7}^{209} + n_{GM8}^{209} & n_{GM5}^{146} &= n_{GM6}^{209} + n_{GM7}^{209} + n_{GM8}^{209} & n_{L2}^{146} &= n_{L4}^{209} + n_{L5}^{209} + 2n_{L6}^{209} & n_{F2}^{146} &= \\ 2n_{X6}^{209} + 2n_{X7}^{209} & n_{T4}^{146} &= n_{L4}^{209} + n_{L5}^{209} & n_{T6}^{146} &= n_{L6}^{209} & n_{T5}^{146} &= n_{L6}^{209} \end{aligned}$$

The lower SG is SG 146 when the preserved operations are: **(sub-SG label is 12) 1, 24, 23.**

$$\text{The transformation is: } (\mathbf{a}_{146}, \mathbf{b}_{146}, \mathbf{c}_{146}) = (\mathbf{a}_{209}, \mathbf{b}_{209}, \mathbf{c}_{209}) \begin{pmatrix} -\frac{1}{2} & -\frac{1}{2} & 0 \\ 0 & -\frac{1}{2} & -\frac{1}{2} \\ \frac{1}{2} & 0 & \frac{1}{2} \end{pmatrix}, \overrightarrow{O_{209}O_{146}} = -\frac{1}{3}\mathbf{a}_{146} + \left(\frac{2}{3}\right)\mathbf{b}_{146} + \left(-\frac{1}{3}\right)\mathbf{c}_{146}$$

The reduction of higher dimensional irrep:

$$O : T_1 \rightarrow A + {}^2E + {}^1E \text{ of } C_3.$$

$$O : T_2 \rightarrow A + {}^2E + {}^1E \text{ of } C_3.$$

The correspondences of irreps at HSPs from original SG to lowered SG:

$$\begin{aligned} n_{GM4}^{146} &= 2n_{GM8}^{209} & n_{GM6}^{146} &= n_{GM6}^{209} + n_{GM7}^{209} + n_{GM8}^{209} & n_{GM5}^{146} &= n_{GM6}^{209} + n_{GM7}^{209} + n_{GM8}^{209} & n_{L2}^{146} &= n_{L4}^{209} + n_{L5}^{209} + 2n_{L6}^{209} & n_{F2}^{146} &= \\ 2n_{X6}^{209} + 2n_{X7}^{209} & n_{T4}^{146} &= n_{L4}^{209} + n_{L5}^{209} & n_{T6}^{146} &= n_{L6}^{209} & n_{T5}^{146} &= n_{L6}^{209} \end{aligned}$$

The lower SG is SG 146 when the preserved operations are: **(sub-SG label is 13) 1, 20, 19.**

$$\text{The transformation is: } (\mathbf{a}_{146}, \mathbf{b}_{146}, \mathbf{c}_{146}) = (\mathbf{a}_{209}, \mathbf{b}_{209}, \mathbf{c}_{209}) \begin{pmatrix} \frac{1}{2} & 0 & \frac{1}{2} \\ -\frac{1}{2} & -\frac{1}{2} & 0 \\ 0 & -\frac{1}{2} & -\frac{1}{2} \end{pmatrix}, \overrightarrow{O_{209}O_{146}} = -\frac{1}{3}\mathbf{a}_{146} + \left(\frac{2}{3}\right)\mathbf{b}_{146} + \left(-\frac{1}{3}\right)\mathbf{c}_{146}$$

The reduction of higher dimensional irrep:

$$O : T_1 \rightarrow A + {}^2E + {}^1E \text{ of } C_3.$$

$$O : T_2 \rightarrow A + {}^2E + {}^1E \text{ of } C_3.$$

The correspondences of irreps at HSPs from original SG to lowered SG:

$$\begin{aligned} n_{GM4}^{146} &= 2n_{GM8}^{209} & n_{GM6}^{146} &= n_{GM6}^{209} + n_{GM7}^{209} + n_{GM8}^{209} & n_{GM5}^{146} &= n_{GM6}^{209} + n_{GM7}^{209} + n_{GM8}^{209} & n_{L2}^{146} &= n_{L4}^{209} + n_{L5}^{209} + 2n_{L6}^{209} & n_{F2}^{146} &= \\ 2n_{X6}^{209} + 2n_{X7}^{209} & n_{T4}^{146} &= n_{L4}^{209} + n_{L5}^{209} & n_{T6}^{146} &= n_{L6}^{209} & n_{T5}^{146} &= n_{L6}^{209} \end{aligned}$$

The lower SG is SG 146 when the preserved operations are: **(sub-SG label is 14) 1, 22, 21.**

$$\text{The transformation is: } (\mathbf{a}_{146}, \mathbf{b}_{146}, \mathbf{c}_{146}) = (\mathbf{a}_{209}, \mathbf{b}_{209}, \mathbf{c}_{209}) \begin{pmatrix} -\frac{1}{2} & -\frac{1}{2} & 0 \\ 0 & \frac{1}{2} & \frac{1}{2} \\ -\frac{1}{2} & 0 & -\frac{1}{2} \end{pmatrix}, \overrightarrow{O_{209}O_{146}} = -\frac{1}{3}\mathbf{a}_{146} + \left(\frac{2}{3}\right)\mathbf{b}_{146} + \left(-\frac{1}{3}\right)\mathbf{c}_{146}$$

The reduction of higher dimensional irrep:

$$O : T_1 \rightarrow A + {}^2E + {}^1E \text{ of } C_3.$$

$$O : T_2 \rightarrow A + {}^2E + {}^1E \text{ of } C_3.$$

The correspondences of irreps at HSPs from original SG to lowered SG:

$$\begin{aligned} n_{GM4}^{146} &= 2n_{GM8}^{209} & n_{GM6}^{146} &= n_{GM6}^{209} + n_{GM7}^{209} + n_{GM8}^{209} & n_{GM5}^{146} &= n_{GM6}^{209} + n_{GM7}^{209} + n_{GM8}^{209} & n_{L2}^{146} &= n_{L4}^{209} + n_{L5}^{209} + 2n_{L6}^{209} & n_{F2}^{146} &= \\ 2n_{X6}^{209} + 2n_{X7}^{209} & n_{T4}^{146} &= n_{L4}^{209} + n_{L5}^{209} & n_{T6}^{146} &= n_{L6}^{209} & n_{T5}^{146} &= n_{L6}^{209} \end{aligned}$$

The lower SG is SG 196 when the preserved operations are: **(sub-SG label is 15) 1, 8, 9, 10, 17, 24, 20, 22, 18, 23, 19, 21.**

$$\text{The transformation is: } (\mathbf{a}_{196}, \mathbf{b}_{196}, \mathbf{c}_{196}) = (\mathbf{a}_{209}, \mathbf{b}_{209}, \mathbf{c}_{209}) \begin{pmatrix} 0 & 0 & 1 \\ 1 & 0 & 0 \\ 0 & 1 & 0 \end{pmatrix}, \overrightarrow{O_{209}O_{196}} = \frac{1}{4}\mathbf{a}_{196} + \left(\frac{1}{4}\right)\mathbf{b}_{196} + \left(\frac{1}{4}\right)\mathbf{c}_{196}$$

The reduction of higher dimensional irrep:

$$O : E \rightarrow {}^1E + {}^2E \text{ of } T.$$

The correspondences of irreps at HSPs from original SG to lowered SG:

$$\begin{aligned} n_{GM6}^{196} &= n_{GM8}^{209} & n_{GM7}^{196} &= n_{GM8}^{209} & n_{GM5}^{196} &= n_{GM6}^{209} + n_{GM7}^{209} & n_{X5}^{196} &= n_{X6}^{209} + n_{X7}^{209} & n_{L4}^{196} &= n_{L4}^{209} + n_{L5}^{209} & n_{L6}^{196} &= n_{L6}^{209} & n_{L5}^{196} &= n_{L6}^{209} \\ n_{W4}^{196} &= n_{W5}^{209} & n_{W3}^{196} &= n_{W5}^{209} \end{aligned}$$

## 107. Lowered SGs by higher-dimensional irreps of pairings in SG 210

The representative operations of SG/T for SG 210:

$$1 : (x, y, z), 2 : (x + \frac{1}{4}, \frac{1}{4} - z, y + \frac{1}{4}), 3 : (x + \frac{1}{4}, z + \frac{1}{4}, \frac{1}{4} - y), 4 : (z + \frac{1}{4}, y + \frac{1}{4}, \frac{1}{4} - x), 5 : (\frac{1}{4} - z, y + \frac{1}{4}, x + \frac{1}{4}), \\ 6 : (\frac{1}{4} - y, x + \frac{1}{4}, z + \frac{1}{4}), 7 : (y + \frac{1}{4}, \frac{1}{4} - x, z + \frac{1}{4}), 8 : (x, -y, -z), 9 : (-x, y, -z), 10 : (-x, -y, z), 11 : (y + \frac{1}{4}, x + \frac{1}{4}, \frac{1}{4} - z), \\ 12 : (\frac{1}{4} - y, \frac{1}{4} - x, \frac{1}{4} - z), 13 : (\frac{1}{4} - x, z + \frac{1}{4}, y + \frac{1}{4}), 14 : (\frac{1}{4} - x, \frac{1}{4} - z, \frac{1}{4} - y), 15 : (z + \frac{1}{4}, \frac{1}{4} - y, x + \frac{1}{4}), 16 : (\frac{1}{4} - z, \frac{1}{4} - y, \frac{1}{4} - x), \\ 17 : (z, x, y), 18 : (y, z, x), 19 : (-y, z, -x), 20 : (-z, -x, y), 21 : (-y, -z, x), 22 : (z, -x, -y), 23 : (y, -z, -x), \\ 24 : (-z, x, -y).$$

The lower SG is SG 22 when the preserved operations are: **(sub-SG label is 1) 1, 8, 9, 10.**

$$\text{The transformation is: } (\mathbf{a}_{22}, \mathbf{b}_{22}, \mathbf{c}_{22}) = (\mathbf{a}_{210}, \mathbf{b}_{210}, \mathbf{c}_{210}) \begin{pmatrix} 0 & 0 & 1 \\ 1 & 0 & 0 \\ 0 & 1 & 0 \end{pmatrix}, \overrightarrow{O_{210}O_{22}} = \frac{1}{4}\mathbf{a}_{22} + (-\frac{1}{4})\mathbf{b}_{22} + (-\frac{1}{4})\mathbf{c}_{22}$$

The reduction of higher dimensional irrep:

$$O : T_1 \rightarrow B_1 + B_2 + B_3 \text{ of } D_2.$$

$$O : T_2 \rightarrow B_1 + B_2 + B_3 \text{ of } D_2.$$

The correspondences of irreps at HSPs from original SG to lowered SG:

$$n_{GM5}^{22} = n_{GM6}^{210} + n_{GM7}^{210} + 2n_{GM8}^{210} \quad n_{Y5}^{22} = n_{X6}^{210} + n_{X7}^{210} \quad n_{L2}^{22} = n_{L4}^{210} + n_{L5}^{210} + 2n_{L6}^{210} \quad n_{Z5}^{22} = n_{X6}^{210} + n_{X7}^{210} \quad n_{T5}^{22} = n_{X6}^{210} + n_{X7}^{210}$$

The lower SG is SG 24 when the preserved operations are: **(sub-SG label is 2) 1, 8, 13, 14.**

$$\text{The transformation is: } (\mathbf{a}_{24}, \mathbf{b}_{24}, \mathbf{c}_{24}) = (\mathbf{a}_{210}, \mathbf{b}_{210}, \mathbf{c}_{210}) \begin{pmatrix} 0 & 0 & -1 \\ \frac{1}{2} & \frac{1}{2} & 0 \\ \frac{1}{2} & -\frac{1}{2} & 0 \end{pmatrix}, \overrightarrow{O_{210}O_{24}} = -\frac{1}{4}\mathbf{b}_{24} + (\frac{3}{8})\mathbf{c}_{24}$$

The reduction of higher dimensional irrep:

$$O : T_1 \rightarrow B_1 + B_2 + B_3 \text{ of } D_2.$$

$$O : T_2 \rightarrow A_1 + B_2 + B_3 \text{ of } D_2.$$

The correspondences of irreps at HSPs from original SG to lowered SG:

$$n_{GM5}^{24} = n_{GM6}^{210} + n_{GM7}^{210} + 2n_{GM8}^{210} \quad n_{X5}^{24} = n_{X6}^{210} + n_{X7}^{210} \quad n_{T3}^{24} = n_{L5}^{210} + n_{L6}^{210} \quad n_{T4}^{24} = n_{L4}^{210} + n_{L6}^{210} \quad n_{W3}^{24} = n_{W5}^{210} \quad n_{W2}^{24} = n_{W4}^{210} \\ n_{W4}^{24} = n_{W2}^{210} \quad n_{W5}^{24} = n_{W3}^{210} \quad n_{R3}^{24} = n_{L4}^{210} + n_{L6}^{210} \quad n_{R4}^{24} = n_{L5}^{210} + n_{L6}^{210} \quad n_{S4}^{24} = n_{L4}^{210} + n_{L6}^{210} \quad n_{S3}^{24} = n_{L5}^{210} + n_{L6}^{210}$$

The lower SG is SG 24 when the preserved operations are: **(sub-SG label is 3) 1, 9, 16, 15.**

$$\text{The transformation is: } (\mathbf{a}_{24}, \mathbf{b}_{24}, \mathbf{c}_{24}) = (\mathbf{a}_{210}, \mathbf{b}_{210}, \mathbf{c}_{210}) \begin{pmatrix} 0 & \frac{1}{2} & \frac{1}{2} \\ -1 & 0 & 0 \\ 0 & -\frac{1}{2} & \frac{1}{2} \end{pmatrix}, \overrightarrow{O_{210}O_{24}} = \frac{1}{8}\mathbf{a}_{24} + (-\frac{1}{2})\mathbf{b}_{24} + (\frac{1}{4})\mathbf{c}_{24}$$

The reduction of higher dimensional irrep:

$$O : T_1 \rightarrow B_1 + B_2 + B_3 \text{ of } D_2.$$

$$O : T_2 \rightarrow A_1 + B_1 + B_2 \text{ of } D_2.$$

The correspondences of irreps at HSPs from original SG to lowered SG:

$$n_{GM5}^{24} = n_{GM6}^{210} + n_{GM7}^{210} + 2n_{GM8}^{210} \quad n_{X5}^{24} = n_{X6}^{210} + n_{X7}^{210} \quad n_{T3}^{24} = n_{L5}^{210} + n_{L6}^{210} \quad n_{T4}^{24} = n_{L4}^{210} + n_{L6}^{210} \quad n_{W3}^{24} = n_{W5}^{210} \quad n_{W2}^{24} = n_{W4}^{210} \\ n_{W4}^{24} = n_{W2}^{210} \quad n_{W5}^{24} = n_{W3}^{210} \quad n_{R3}^{24} = n_{L5}^{210} + n_{L6}^{210} \quad n_{R4}^{24} = n_{L4}^{210} + n_{L6}^{210} \quad n_{S4}^{24} = n_{L5}^{210} + n_{L6}^{210} \quad n_{S3}^{24} = n_{L4}^{210} + n_{L6}^{210}$$

The lower SG is SG 24 when the preserved operations are: **(sub-SG label is 4) 1, 10, 11, 12.**

$$\text{The transformation is: } (\mathbf{a}_{24}, \mathbf{b}_{24}, \mathbf{c}_{24}) = (\mathbf{a}_{210}, \mathbf{b}_{210}, \mathbf{c}_{210}) \begin{pmatrix} 0 & \frac{1}{2} & -\frac{1}{2} \\ 0 & \frac{1}{2} & \frac{1}{2} \\ 1 & 0 & 0 \end{pmatrix}, \overrightarrow{O_{210}O_{24}} = \frac{1}{8}\mathbf{a}_{24} + (-\frac{1}{2})\mathbf{b}_{24} + (\frac{1}{4})\mathbf{c}_{24}$$

The reduction of higher dimensional irrep:

$$O : T_1 \rightarrow B_1 + B_2 + B_3 \text{ of } D_2.$$

$$O : T_2 \rightarrow A_1 + B_1 + B_2 \text{ of } D_2.$$

The correspondences of irreps at HSPs from original SG to lowered SG:

$$n_{GM5}^{24} = n_{GM6}^{210} + n_{GM7}^{210} + 2n_{GM8}^{210} \quad n_{X5}^{24} = n_{X6}^{210} + n_{X7}^{210} \quad n_{T3}^{24} = n_{L5}^{210} + n_{L6}^{210} \quad n_{T4}^{24} = n_{L4}^{210} + n_{L6}^{210} \quad n_{W3}^{24} = n_{W5}^{210} \quad n_{W2}^{24} = n_{W4}^{210} \\ n_{W4}^{24} = n_{W2}^{210} \quad n_{W5}^{24} = n_{W3}^{210} \quad n_{R3}^{24} = n_{L5}^{210} + n_{L6}^{210} \quad n_{R4}^{24} = n_{L4}^{210} + n_{L6}^{210} \quad n_{S4}^{24} = n_{L5}^{210} + n_{L6}^{210} \quad n_{S3}^{24} = n_{L4}^{210} + n_{L6}^{210}$$

The lower SG is SG 80 when the preserved operations are: **(sub-SG label is 5) 1, 6, 7, 10.**

The transformation is:  $(\mathbf{a}_{80}, \mathbf{b}_{80}, \mathbf{c}_{80}) = (\mathbf{a}_{210}, \mathbf{b}_{210}, \mathbf{c}_{210}) \begin{pmatrix} \frac{1}{2} & \frac{1}{2} & 0 \\ -\frac{1}{2} & \frac{1}{2} & 0 \\ 0 & 0 & 1 \end{pmatrix}, \overrightarrow{O_{210}O_{80}} = \frac{1}{2}\mathbf{a}_{80} + (-\frac{1}{2})\mathbf{b}_{80}$

The reduction of higher dimensional irrep:

$$O : T_1 \rightarrow A + {}^2E + {}^1E \text{ of } C_4.$$

$$O : T_2 \rightarrow {}^2E + B + {}^1E \text{ of } C_4.$$

The correspondences of irreps at HSPs from original SG to lowered SG:

$$\begin{aligned} n_{GM5}^{80} &= n_{GM7}^{210} + n_{GM8}^{210} & n_{GM7}^{80} &= n_{GM7}^{210} + n_{GM8}^{210} & n_{GM8}^{80} &= n_{GM6}^{210} + n_{GM8}^{210} & n_{GM6}^{80} &= n_{GM6}^{210} + n_{GM8}^{210} & n_{M7}^{80} &= n_{X7}^{210} & n_{M5}^{80} &= \\ n_{X7}^{210} n_{M6}^{80} &= n_{X6}^{210} n_{M8}^{80} &= n_{X6}^{210} n_{X4}^{80} &= n_{X6}^{210} + n_{X7}^{210} & n_{X3}^{80} &= n_{X6}^{210} + n_{X7}^{210} & n_{P4}^{80} &= n_{W3}^{210} + n_{W5}^{210} & n_{P3}^{80} &= n_{W2}^{210} + n_{W4}^{210} & n_{N2}^{80} &= \\ n_{L4}^{210} + n_{L5}^{210} + 2n_{L6}^{210} & & & & & & & & & & & \end{aligned}$$

The lower SG is SG 80 when the preserved operations are: **(sub-SG label is 6) 1, 2, 3, 8.**

The transformation is:  $(\mathbf{a}_{80}, \mathbf{b}_{80}, \mathbf{c}_{80}) = (\mathbf{a}_{210}, \mathbf{b}_{210}, \mathbf{c}_{210}) \begin{pmatrix} 0 & 0 & 1 \\ -\frac{1}{2} & \frac{1}{2} & 0 \\ -\frac{1}{2} & -\frac{1}{2} & 0 \end{pmatrix}, \overrightarrow{O_{210}O_{80}} = \frac{1}{2}\mathbf{a}_{80}$

The reduction of higher dimensional irrep:

$$O : T_1 \rightarrow A + {}^2E + {}^1E \text{ of } C_4.$$

$$O : T_2 \rightarrow {}^2E + B + {}^1E \text{ of } C_4.$$

The correspondences of irreps at HSPs from original SG to lowered SG:

$$\begin{aligned} n_{GM5}^{80} &= n_{GM7}^{210} + n_{GM8}^{210} & n_{GM7}^{80} &= n_{GM7}^{210} + n_{GM8}^{210} & n_{GM8}^{80} &= n_{GM6}^{210} + n_{GM8}^{210} & n_{GM6}^{80} &= n_{GM6}^{210} + n_{GM8}^{210} & n_{M7}^{80} &= n_{X7}^{210} & n_{M5}^{80} &= \\ n_{X7}^{210} n_{M6}^{80} &= n_{X6}^{210} n_{M8}^{80} &= n_{X6}^{210} n_{X4}^{80} &= n_{X6}^{210} + n_{X7}^{210} & n_{X3}^{80} &= n_{X6}^{210} + n_{X7}^{210} & n_{P4}^{80} &= n_{W3}^{210} + n_{W5}^{210} & n_{P3}^{80} &= n_{W2}^{210} + n_{W4}^{210} & n_{N2}^{80} &= \\ n_{L4}^{210} + n_{L5}^{210} + 2n_{L6}^{210} & & & & & & & & & & & \end{aligned}$$

The lower SG is SG 80 when the preserved operations are: **(sub-SG label is 7) 1, 4, 5, 9.**

The transformation is:  $(\mathbf{a}_{80}, \mathbf{b}_{80}, \mathbf{c}_{80}) = (\mathbf{a}_{210}, \mathbf{b}_{210}, \mathbf{c}_{210}) \begin{pmatrix} \frac{1}{2} & -\frac{1}{2} & 0 \\ 0 & 0 & 1 \\ -\frac{1}{2} & -\frac{1}{2} & 0 \end{pmatrix}, \overrightarrow{O_{210}O_{80}} = \frac{1}{2}\mathbf{a}_{80} + (\frac{1}{2})\mathbf{b}_{80}$

The reduction of higher dimensional irrep:

$$O : T_1 \rightarrow A + {}^2E + {}^1E \text{ of } C_4.$$

$$O : T_2 \rightarrow {}^2E + B + {}^1E \text{ of } C_4.$$

The correspondences of irreps at HSPs from original SG to lowered SG:

$$\begin{aligned} n_{GM5}^{80} &= n_{GM7}^{210} + n_{GM8}^{210} & n_{GM7}^{80} &= n_{GM7}^{210} + n_{GM8}^{210} & n_{GM8}^{80} &= n_{GM6}^{210} + n_{GM8}^{210} & n_{GM6}^{80} &= n_{GM6}^{210} + n_{GM8}^{210} & n_{M7}^{80} &= n_{X7}^{210} & n_{M5}^{80} &= \\ n_{X7}^{210} n_{M6}^{80} &= n_{X6}^{210} n_{M8}^{80} &= n_{X6}^{210} n_{X4}^{80} &= n_{X6}^{210} + n_{X7}^{210} & n_{X3}^{80} &= n_{X6}^{210} + n_{X7}^{210} & n_{P4}^{80} &= n_{W3}^{210} + n_{W5}^{210} & n_{P3}^{80} &= n_{W2}^{210} + n_{W4}^{210} & n_{N2}^{80} &= \\ n_{L4}^{210} + n_{L5}^{210} + 2n_{L6}^{210} & & & & & & & & & & & \end{aligned}$$

The lower SG is SG 98 when the preserved operations are: **(sub-SG label is 8) 1, 6, 7, 10, 8, 9, 11, 12.**

The transformation is:  $(\mathbf{a}_{98}, \mathbf{b}_{98}, \mathbf{c}_{98}) = (\mathbf{a}_{210}, \mathbf{b}_{210}, \mathbf{c}_{210}) \begin{pmatrix} -\frac{1}{2} & \frac{1}{2} & 0 \\ -\frac{1}{2} & -\frac{1}{2} & 0 \\ 0 & 0 & 1 \end{pmatrix}, \overrightarrow{O_{210}O_{98}} = \frac{1}{2}\mathbf{a}_{98} + (\frac{1}{4})\mathbf{c}_{98}$

The reduction of higher dimensional irrep:

$$O : E \rightarrow A_1 + B_2 \text{ of } D_4.$$

The correspondences of irreps at HSPs from original SG to lowered SG:

$$\begin{aligned} n_{GM6}^{98} &= n_{GM7}^{210} + n_{GM8}^{210} & n_{GM7}^{98} &= n_{GM6}^{210} + n_{GM8}^{210} & n_{M6}^{98} &= n_{X7}^{210} & n_{M7}^{98} &= n_{X6}^{210} & n_{X5}^{98} &= n_{X6}^{210} + n_{X7}^{210} & n_{P2}^{98} &= n_{W4}^{210} & n_{P3}^{98} &= n_{W5}^{210} \\ n_{P5}^{98} &= n_{W3}^{210} & n_{P4}^{98} &= n_{W2}^{210} & n_{N3}^{98} &= n_{L5}^{210} + n_{L6}^{210} & n_{N4}^{98} &= n_{L4}^{210} + n_{L6}^{210} & & & & & & \end{aligned}$$

The lower SG is SG 98 when the preserved operations are: **(sub-SG label is 9) 1, 2, 3, 8, 9, 10, 13, 14.**

The transformation is:  $(\mathbf{a}_{98}, \mathbf{b}_{98}, \mathbf{c}_{98}) = (\mathbf{a}_{210}, \mathbf{b}_{210}, \mathbf{c}_{210}) \begin{pmatrix} 0 & 0 & -1 \\ -\frac{1}{2} & \frac{1}{2} & 0 \\ \frac{1}{2} & \frac{1}{2} & 0 \end{pmatrix}, \overrightarrow{O_{210}O_{98}} = \frac{1}{2}\mathbf{a}_{98} + (\frac{1}{4})\mathbf{c}_{98}$

The reduction of higher dimensional irrep:

$$O : E \rightarrow A_1 + B_2 \text{ of } D_4.$$

The correspondences of irreps at HSPs from original SG to lowered SG:

$$\begin{aligned} n_{GM6}^{98} &= n_{GM7}^{210} + n_{GM8}^{210} & n_{GM7}^{98} &= n_{GM6}^{210} + n_{GM8}^{210} & n_{M6}^{98} &= n_{X7}^{210} & n_{M7}^{98} &= n_{X6}^{210} & n_{X5}^{98} &= n_{X6}^{210} + n_{X7}^{210} & n_{P2}^{98} &= n_{W4}^{210} & n_{P3}^{98} &= n_{W5}^{210} \\ n_{P5}^{98} &= n_{W3}^{210} & n_{P4}^{98} &= n_{W2}^{210} & n_{N3}^{98} &= n_{L5}^{210} + n_{L6}^{210} & n_{N4}^{98} &= n_{L4}^{210} + n_{L6}^{210} & & & & & & \end{aligned}$$

The lower SG is SG 98 when the preserved operations are: **(sub-SG label is 10) 1, 4, 5, 9, 10, 8, 16, 15.**

The transformation is:  $(\mathbf{a}_{98}, \mathbf{b}_{98}, \mathbf{c}_{98}) = (\mathbf{a}_{210}, \mathbf{b}_{210}, \mathbf{c}_{210}) \begin{pmatrix} -\frac{1}{2} & -\frac{1}{2} & 0 \\ 0 & 0 & -1 \\ \frac{1}{2} & -\frac{1}{2} & 0 \end{pmatrix}, \overrightarrow{O_{210}O_{98}} = \frac{1}{2}\mathbf{a}_{98} + (\frac{1}{4})\mathbf{c}_{98}$

The reduction of higher dimensional irrep:

$O : E \rightarrow A_1 + B_2$  of  $D_4$ .

The correspondences of irreps at HSPs from original SG to lowered SG:

$$\begin{aligned} n_{GM6}^{98} &= n_{GM7}^{210} + n_{GM8}^{210} & n_{GM7}^{98} &= n_{GM6}^{210} + n_{GM8}^{210} & n_{M6}^{98} &= n_{X7}^{210} & n_{M7}^{98} &= n_{X6}^{210} & n_{X5}^{98} &= n_{X6}^{210} + n_{X7}^{210} & n_{P2}^{98} &= n_{W4}^{210} & n_{P3}^{98} &= n_{W5}^{210} \\ n_{P5}^{98} &= n_{W3}^{210} & n_{P4}^{98} &= n_{W2}^{210} & n_{N3}^{98} &= n_{L5}^{210} + n_{L6}^{210} & n_{N4}^{98} &= n_{L4}^{210} + n_{L6}^{210} \end{aligned}$$

The lower SG is SG 146 when the preserved operations are: **(sub-SG label is 11) 1, 17, 18.**

The transformation is:  $(\mathbf{a}_{146}, \mathbf{b}_{146}, \mathbf{c}_{146}) = (\mathbf{a}_{210}, \mathbf{b}_{210}, \mathbf{c}_{210}) \begin{pmatrix} \frac{1}{2} & 0 & \frac{1}{2} \\ \frac{1}{2} & \frac{1}{2} & 0 \\ 0 & \frac{1}{2} & \frac{1}{2} \end{pmatrix}, \overrightarrow{O_{210}O_{146}} = -\frac{1}{3}\mathbf{a}_{146} + (\frac{2}{3})\mathbf{b}_{146} + (-\frac{1}{3})\mathbf{c}_{146}$

The reduction of higher dimensional irrep:

$O : T_1 \rightarrow A + {}^2E + {}^1E$  of  $C_3$ .

$O : T_2 \rightarrow A + {}^2E + {}^1E$  of  $C_3$ .

The correspondences of irreps at HSPs from original SG to lowered SG:

$$\begin{aligned} n_{GM4}^{146} &= 2n_{GM8}^{210} & n_{GM6}^{146} &= n_{GM6}^{210} + n_{GM7}^{210} + n_{GM8}^{210} & n_{GM5}^{146} &= n_{GM6}^{210} + n_{GM7}^{210} + n_{GM8}^{210} & n_{L2}^{146} &= n_{L4}^{210} + n_{L5}^{210} + 2n_{L6}^{210} & n_{F2}^{146} &= \\ 2n_{X6}^{210} + 2n_{X7}^{210} & n_{T4}^{146} &= n_{L4}^{210} + n_{L5}^{210} & n_{T6}^{146} &= n_{L6}^{210} & n_{T5}^{146} &= n_{L6}^{210} \end{aligned}$$

The lower SG is SG 146 when the preserved operations are: **(sub-SG label is 12) 1, 24, 23.**

The transformation is:  $(\mathbf{a}_{146}, \mathbf{b}_{146}, \mathbf{c}_{146}) = (\mathbf{a}_{210}, \mathbf{b}_{210}, \mathbf{c}_{210}) \begin{pmatrix} -\frac{1}{2} & -\frac{1}{2} & 0 \\ 0 & -\frac{1}{2} & -\frac{1}{2} \\ \frac{1}{2} & 0 & \frac{1}{2} \end{pmatrix}, \overrightarrow{O_{210}O_{146}} = -\frac{1}{3}\mathbf{a}_{146} + (\frac{2}{3})\mathbf{b}_{146} + (-\frac{1}{3})\mathbf{c}_{146}$

The reduction of higher dimensional irrep:

$O : T_1 \rightarrow A + {}^2E + {}^1E$  of  $C_3$ .

$O : T_2 \rightarrow A + {}^2E + {}^1E$  of  $C_3$ .

The correspondences of irreps at HSPs from original SG to lowered SG:

$$\begin{aligned} n_{GM4}^{146} &= 2n_{GM8}^{210} & n_{GM6}^{146} &= n_{GM6}^{210} + n_{GM7}^{210} + n_{GM8}^{210} & n_{GM5}^{146} &= n_{GM6}^{210} + n_{GM7}^{210} + n_{GM8}^{210} & n_{L2}^{146} &= n_{L4}^{210} + n_{L5}^{210} + 2n_{L6}^{210} & n_{F2}^{146} &= \\ 2n_{X6}^{210} + 2n_{X7}^{210} & n_{T4}^{146} &= n_{L4}^{210} + n_{L5}^{210} & n_{T6}^{146} &= n_{L6}^{210} & n_{T5}^{146} &= n_{L6}^{210} \end{aligned}$$

The lower SG is SG 146 when the preserved operations are: **(sub-SG label is 13) 1, 20, 19.**

The transformation is:  $(\mathbf{a}_{146}, \mathbf{b}_{146}, \mathbf{c}_{146}) = (\mathbf{a}_{210}, \mathbf{b}_{210}, \mathbf{c}_{210}) \begin{pmatrix} \frac{1}{2} & 0 & \frac{1}{2} \\ -\frac{1}{2} & -\frac{1}{2} & 0 \\ 0 & -\frac{1}{2} & -\frac{1}{2} \end{pmatrix}, \overrightarrow{O_{210}O_{146}} = -\frac{1}{3}\mathbf{a}_{146} + (\frac{2}{3})\mathbf{b}_{146} + (-\frac{1}{3})\mathbf{c}_{146}$

The reduction of higher dimensional irrep:

$O : T_1 \rightarrow A + {}^2E + {}^1E$  of  $C_3$ .

$O : T_2 \rightarrow A + {}^2E + {}^1E$  of  $C_3$ .

The correspondences of irreps at HSPs from original SG to lowered SG:

$$\begin{aligned} n_{GM4}^{146} &= 2n_{GM8}^{210} & n_{GM6}^{146} &= n_{GM6}^{210} + n_{GM7}^{210} + n_{GM8}^{210} & n_{GM5}^{146} &= n_{GM6}^{210} + n_{GM7}^{210} + n_{GM8}^{210} & n_{L2}^{146} &= n_{L4}^{210} + n_{L5}^{210} + 2n_{L6}^{210} & n_{F2}^{146} &= \\ 2n_{X6}^{210} + 2n_{X7}^{210} & n_{T4}^{146} &= n_{L4}^{210} + n_{L5}^{210} & n_{T6}^{146} &= n_{L6}^{210} & n_{T5}^{146} &= n_{L6}^{210} \end{aligned}$$

The lower SG is SG 146 when the preserved operations are: **(sub-SG label is 14) 1, 22, 21.**

The transformation is:  $(\mathbf{a}_{146}, \mathbf{b}_{146}, \mathbf{c}_{146}) = (\mathbf{a}_{210}, \mathbf{b}_{210}, \mathbf{c}_{210}) \begin{pmatrix} -\frac{1}{2} & -\frac{1}{2} & 0 \\ 0 & \frac{1}{2} & \frac{1}{2} \\ -\frac{1}{2} & 0 & -\frac{1}{2} \end{pmatrix}, \overrightarrow{O_{210}O_{146}} = -\frac{1}{3}\mathbf{a}_{146} + (\frac{2}{3})\mathbf{b}_{146} + (-\frac{1}{3})\mathbf{c}_{146}$

The reduction of higher dimensional irrep:

$O : T_1 \rightarrow A + {}^2E + {}^1E$  of  $C_3$ .

$O : T_2 \rightarrow A + {}^2E + {}^1E$  of  $C_3$ .

The correspondences of irreps at HSPs from original SG to lowered SG:

$$\begin{aligned} n_{GM4}^{146} &= 2n_{GM8}^{210} & n_{GM6}^{146} &= n_{GM6}^{210} + n_{GM7}^{210} + n_{GM8}^{210} & n_{GM5}^{146} &= n_{GM6}^{210} + n_{GM7}^{210} + n_{GM8}^{210} & n_{L2}^{146} &= n_{L4}^{210} + n_{L5}^{210} + 2n_{L6}^{210} & n_{F2}^{146} &= \\ 2n_{X6}^{210} + 2n_{X7}^{210} & n_{T4}^{146} &= n_{L4}^{210} + n_{L5}^{210} & n_{T6}^{146} &= n_{L6}^{210} & n_{T5}^{146} &= n_{L6}^{210} \end{aligned}$$

The lower SG is SG 196 when the preserved operations are: **(sub-SG label is 15) 1, 8, 9, 10, 17, 24, 20, 22, 18, 23, 19, 21.**

The transformation is:  $(\mathbf{a}_{196}, \mathbf{b}_{196}, \mathbf{c}_{196}) = (\mathbf{a}_{210}, \mathbf{b}_{210}, \mathbf{c}_{210}) \begin{pmatrix} 0 & 0 & 1 \\ 1 & 0 & 0 \\ 0 & 1 & 0 \end{pmatrix}, \overrightarrow{O_{210}O_{196}} = \frac{1}{4}\mathbf{a}_{196} + (\frac{1}{4})\mathbf{b}_{196} + (\frac{1}{4})\mathbf{c}_{196}$

The reduction of higher dimensional irrep:

$O : E \rightarrow {}^1E + {}^2E$  of  $T$ .

The correspondences of irreps at HSPs from original SG to lowered SG:

$$\begin{aligned} n_{GM6}^{196} &= n_{GM8}^{210} n_{GM7}^{196} = n_{GM8}^{210} n_{GM5}^{196} = n_{GM6}^{210} + n_{GM7}^{210} n_{X5}^{196} = n_{X6}^{210} + n_{X7}^{210} n_{L4}^{196} = n_{L4}^{210} + n_{L5}^{210} n_{L6}^{196} = n_{L6}^{210} n_{L5}^{196} = n_{L6}^{210} \\ n_{W4}^{196} &= n_{W2}^{210} + n_{W4}^{210} n_{W3}^{196} = n_{W3}^{210} + n_{W5}^{210} \end{aligned}$$

### 108. Lowered SGs by higher-dimensional irreps of pairings in SG 211

The representative operations of SG/T for SG 211:

$$\begin{aligned} 1 : (x, y, z), 2 : (x, -z, y), 3 : (x, z, -y), 4 : (z, y, -x), 5 : (-z, y, x), 6 : (-y, x, z), 7 : (y, -x, z), 8 : (x, -y, -z), \\ 9 : (-x, y, -z), 10 : (-x, -y, z), 11 : (y, x, -z), 12 : (-y, -x, -z), 13 : (-x, z, y), 14 : (-x, -z, -y), 15 : (z, -y, x), \\ 16 : (-z, -y, -x), 17 : (z, x, y), 18 : (y, z, x), 19 : (-y, z, -x), 20 : (-z, -x, y), 21 : (-y, -z, x), 22 : (z, -x, -y), \\ 23 : (y, -z, -x), 24 : (-z, x, -y). \end{aligned}$$

The lower SG is SG 23 when the preserved operations are: **(sub-SG label is 1) 1, 8, 9, 10.**

The transformation is:  $(\mathbf{a}_{23}, \mathbf{b}_{23}, \mathbf{c}_{23}) = (\mathbf{a}_{211}, \mathbf{b}_{211}, \mathbf{c}_{211}) \begin{pmatrix} 0 & 0 & 1 \\ 1 & 0 & 0 \\ 0 & 1 & 0 \end{pmatrix}, \overrightarrow{O_{211}O_{23}} = -\frac{1}{2}\mathbf{b}_{23}$

The reduction of higher dimensional irrep:

$O : T_1 \rightarrow B_1 + B_2 + B_3$  of  $D_2$ .

$O : T_2 \rightarrow B_1 + B_2 + B_3$  of  $D_2$ .

The correspondences of irreps at HSPs from original SG to lowered SG:

$$\begin{aligned} n_{GM5}^{23} &= n_{GM6}^{211} + n_{GM7}^{211} + 2n_{GM8}^{211} n_{X5}^{23} = n_{H6}^{211} + n_{H7}^{211} + 2n_{H8}^{211} n_{T4}^{23} = n_{N5}^{211} n_{T3}^{23} = n_{N5}^{211} n_{W5}^{23} = n_{P5}^{211} + n_{P6}^{211} + n_{P7}^{211} n_{R4}^{23} = \\ n_{N5}^{211} n_{R3}^{23} &= n_{N5}^{211} n_{S3}^{23} = n_{N5}^{211} n_{S4}^{23} = n_{N5}^{211} \end{aligned}$$

The lower SG is SG 22 when the preserved operations are: **(sub-SG label is 2) 1, 8, 13, 14.**

The transformation is:  $(\mathbf{a}_{22}, \mathbf{b}_{22}, \mathbf{c}_{22}) = (\mathbf{a}_{211}, \mathbf{b}_{211}, \mathbf{c}_{211}) \begin{pmatrix} 0 & 0 & 1 \\ 1 & -1 & 0 \\ 1 & 1 & 0 \end{pmatrix}, \overrightarrow{O_{211}O_{22}} = \frac{1}{4}\mathbf{a}_{22} + (-\frac{1}{4})\mathbf{b}_{22} + (-\frac{1}{4})\mathbf{c}_{22}$

The reduction of higher dimensional irrep:

$O : T_1 \rightarrow B_1 + B_2 + B_3$  of  $D_2$ .

$O : T_2 \rightarrow A_1 + B_2 + B_3$  of  $D_2$ .

The correspondences of irreps at HSPs from original SG to lowered SG:

$$n_{GM5}^{22} = n_{GM6}^{211} + n_{GM7}^{211} + 2n_{GM8}^{211} n_{Y5}^{22} = n_{N5}^{211} n_{L2}^{22} = 2n_{N5}^{211} n_{Z5}^{22} = n_{H6}^{211} + n_{H7}^{211} + 2n_{H8}^{211} n_{T5}^{22} = n_{N5}^{211}$$

The lower SG is SG 22 when the preserved operations are: **(sub-SG label is 3) 1, 9, 16, 15.**

The transformation is:  $(\mathbf{a}_{22}, \mathbf{b}_{22}, \mathbf{c}_{22}) = (\mathbf{a}_{211}, \mathbf{b}_{211}, \mathbf{c}_{211}) \begin{pmatrix} -1 & 1 & 0 \\ 0 & 0 & 1 \\ 1 & 1 & 0 \end{pmatrix}, \overrightarrow{O_{211}O_{22}} = \frac{1}{4}\mathbf{a}_{22} + (-\frac{1}{4})\mathbf{b}_{22} + (-\frac{1}{4})\mathbf{c}_{22}$

The reduction of higher dimensional irrep:

$O : T_1 \rightarrow B_1 + B_2 + B_3$  of  $D_2$ .

$O : T_2 \rightarrow A_1 + B_2 + B_3$  of  $D_2$ .

The correspondences of irreps at HSPs from original SG to lowered SG:

$$n_{GM5}^{22} = n_{GM6}^{211} + n_{GM7}^{211} + 2n_{GM8}^{211} n_{Y5}^{22} = n_{N5}^{211} n_{L2}^{22} = 2n_{N5}^{211} n_{Z5}^{22} = n_{H6}^{211} + n_{H7}^{211} + 2n_{H8}^{211} n_{T5}^{22} = n_{N5}^{211}$$

The lower SG is SG 22 when the preserved operations are: **(sub-SG label is 4) 1, 10, 11, 12.**

The transformation is:  $(\mathbf{a}_{22}, \mathbf{b}_{22}, \mathbf{c}_{22}) = (\mathbf{a}_{211}, \mathbf{b}_{211}, \mathbf{c}_{211}) \begin{pmatrix} 1 & -1 & 0 \\ 1 & 1 & 0 \\ 0 & 0 & 1 \end{pmatrix}, \overrightarrow{O_{211}O_{22}} = \frac{1}{4}\mathbf{a}_{22} + (-\frac{1}{4})\mathbf{b}_{22} + (-\frac{1}{4})\mathbf{c}_{22}$

The reduction of higher dimensional irrep:

$O : T_1 \rightarrow B_1 + B_2 + B_3$  of  $D_2$ .

$O : T_2 \rightarrow A_1 + B_2 + B_3$  of  $D_2$ .

The correspondences of irreps at HSPs from original SG to lowered SG:

$$n_{GM5}^{22} = n_{GM6}^{211} + n_{GM7}^{211} + 2n_{GM8}^{211} \quad n_{Y5}^{22} = n_{N5}^{211} \quad n_{L2}^{22} = 2n_{N5}^{211} \quad n_{Z5}^{22} = n_{H6}^{211} + n_{H7}^{211} + 2n_{H8}^{211} \quad n_{T5}^{22} = n_{N5}^{211}$$

The lower SG is SG 79 when the preserved operations are: **(sub-SG label is 5) 1, 6, 7, 10.**

$$\text{The transformation is: } (\mathbf{a}_{79}, \mathbf{b}_{79}, \mathbf{c}_{79}) = (\mathbf{a}_{211}, \mathbf{b}_{211}, \mathbf{c}_{211}) \begin{pmatrix} 0 & 1 & 0 \\ -1 & 0 & 0 \\ 0 & 0 & 1 \end{pmatrix}, \overrightarrow{O_{211}O_{79}} = \frac{1}{2}\mathbf{a}_{79} + \left(\frac{1}{2}\right)\mathbf{b}_{79}$$

The reduction of higher dimensional irrep:

$$O : T_1 \rightarrow A + {}^2E + {}^1E \quad \text{of } C_4.$$

$$O : T_2 \rightarrow {}^2E + B + {}^1E \quad \text{of } C_4.$$

The correspondences of irreps at HSPs from original SG to lowered SG:

$$\begin{aligned} n_{GM5}^{79} &= n_{GM7}^{211} + n_{GM8}^{211} & n_{GM7}^{79} &= n_{GM7}^{211} + n_{GM8}^{211} & n_{GM8}^{79} &= n_{GM6}^{211} + n_{GM8}^{211} & n_{GM6}^{79} &= n_{GM6}^{211} + n_{GM8}^{211} & n_{M5}^{79} &= n_{H7}^{211} + n_{H8}^{211} \\ n_{M7}^{79} &= n_{H7}^{211} + n_{H8}^{211} & n_{M8}^{79} &= n_{H6}^{211} + n_{H8}^{211} & n_{M6}^{79} &= n_{H6}^{211} + n_{H8}^{211} & n_{X4}^{79} &= n_{N5}^{211} & n_{X3}^{79} &= n_{N5}^{211} & n_{P4}^{79} &= n_{P5}^{211} + n_{P6}^{211} + n_{P7}^{211} \\ n_{P5}^{79} &+ n_{P6}^{211} + n_{P7}^{211} & n_{N2}^{79} &= 2n_{N5}^{211} \end{aligned}$$

The lower SG is SG 79 when the preserved operations are: **(sub-SG label is 6) 1, 2, 3, 8.**

$$\text{The transformation is: } (\mathbf{a}_{79}, \mathbf{b}_{79}, \mathbf{c}_{79}) = (\mathbf{a}_{211}, \mathbf{b}_{211}, \mathbf{c}_{211}) \begin{pmatrix} 0 & 0 & 1 \\ 0 & 1 & 0 \\ -1 & 0 & 0 \end{pmatrix}, \overrightarrow{O_{211}O_{79}} = \frac{1}{2}\mathbf{a}_{79} + \left(\frac{1}{2}\right)\mathbf{b}_{79}$$

The reduction of higher dimensional irrep:

$$O : T_1 \rightarrow A + {}^2E + {}^1E \quad \text{of } C_4.$$

$$O : T_2 \rightarrow {}^2E + B + {}^1E \quad \text{of } C_4.$$

The correspondences of irreps at HSPs from original SG to lowered SG:

$$\begin{aligned} n_{GM5}^{79} &= n_{GM7}^{211} + n_{GM8}^{211} & n_{GM7}^{79} &= n_{GM7}^{211} + n_{GM8}^{211} & n_{GM8}^{79} &= n_{GM6}^{211} + n_{GM8}^{211} & n_{GM6}^{79} &= n_{GM6}^{211} + n_{GM8}^{211} & n_{M5}^{79} &= n_{H7}^{211} + n_{H8}^{211} \\ n_{M7}^{79} &= n_{H7}^{211} + n_{H8}^{211} & n_{M8}^{79} &= n_{H6}^{211} + n_{H8}^{211} & n_{M6}^{79} &= n_{H6}^{211} + n_{H8}^{211} & n_{X4}^{79} &= n_{N5}^{211} & n_{X3}^{79} &= n_{N5}^{211} & n_{P4}^{79} &= n_{P5}^{211} + n_{P6}^{211} + n_{P7}^{211} \\ n_{P5}^{79} &+ n_{P6}^{211} + n_{P7}^{211} & n_{N2}^{79} &= 2n_{N5}^{211} \end{aligned}$$

The lower SG is SG 79 when the preserved operations are: **(sub-SG label is 7) 1, 4, 5, 9.**

$$\text{The transformation is: } (\mathbf{a}_{79}, \mathbf{b}_{79}, \mathbf{c}_{79}) = (\mathbf{a}_{211}, \mathbf{b}_{211}, \mathbf{c}_{211}) \begin{pmatrix} 0 & -1 & 0 \\ 0 & 0 & 1 \\ -1 & 0 & 0 \end{pmatrix}, \overrightarrow{O_{211}O_{79}} = \frac{1}{2}\mathbf{a}_{79} + \left(\frac{1}{2}\right)\mathbf{b}_{79}$$

The reduction of higher dimensional irrep:

$$O : T_1 \rightarrow A + {}^2E + {}^1E \quad \text{of } C_4.$$

$$O : T_2 \rightarrow {}^2E + B + {}^1E \quad \text{of } C_4.$$

The correspondences of irreps at HSPs from original SG to lowered SG:

$$\begin{aligned} n_{GM5}^{79} &= n_{GM7}^{211} + n_{GM8}^{211} & n_{GM7}^{79} &= n_{GM7}^{211} + n_{GM8}^{211} & n_{GM8}^{79} &= n_{GM6}^{211} + n_{GM8}^{211} & n_{GM6}^{79} &= n_{GM6}^{211} + n_{GM8}^{211} & n_{M5}^{79} &= n_{H7}^{211} + n_{H8}^{211} \\ n_{M7}^{79} &= n_{H7}^{211} + n_{H8}^{211} & n_{M8}^{79} &= n_{H6}^{211} + n_{H8}^{211} & n_{M6}^{79} &= n_{H6}^{211} + n_{H8}^{211} & n_{X4}^{79} &= n_{N5}^{211} & n_{X3}^{79} &= n_{N5}^{211} & n_{P4}^{79} &= n_{P5}^{211} + n_{P6}^{211} + n_{P7}^{211} \\ n_{P5}^{79} &+ n_{P6}^{211} + n_{P7}^{211} & n_{N2}^{79} &= 2n_{N5}^{211} \end{aligned}$$

The lower SG is SG 97 when the preserved operations are: **(sub-SG label is 8) 1, 6, 7, 10, 8, 9, 11, 12.**

$$\text{The transformation is: } (\mathbf{a}_{97}, \mathbf{b}_{97}, \mathbf{c}_{97}) = (\mathbf{a}_{211}, \mathbf{b}_{211}, \mathbf{c}_{211}) \begin{pmatrix} 0 & 1 & 0 \\ -1 & 0 & 0 \\ 0 & 0 & 1 \end{pmatrix}, \overrightarrow{O_{211}O_{97}} = \mathbf{0}$$

The reduction of higher dimensional irrep:

$$O : E \rightarrow A_1 + B_1 \quad \text{of } D_4.$$

The correspondences of irreps at HSPs from original SG to lowered SG:

$$\begin{aligned} n_{GM6}^{97} &= n_{GM7}^{211} + n_{GM8}^{211} & n_{GM7}^{97} &= n_{GM6}^{211} + n_{GM8}^{211} & n_{M6}^{97} &= n_{H7}^{211} + n_{H8}^{211} & n_{M7}^{97} &= n_{H6}^{211} + n_{H8}^{211} & n_{X5}^{97} &= n_{N5}^{211} & n_{P5}^{97} &= n_{P5}^{211} + n_{P6}^{211} + n_{P7}^{211} \\ n_{N4}^{97} &= n_{N5}^{211} & n_{N3}^{97} &= n_{N5}^{211} \end{aligned}$$

The lower SG is SG 97 when the preserved operations are: **(sub-SG label is 9) 1, 2, 3, 8, 9, 10, 13, 14.**

$$\text{The transformation is: } (\mathbf{a}_{97}, \mathbf{b}_{97}, \mathbf{c}_{97}) = (\mathbf{a}_{211}, \mathbf{b}_{211}, \mathbf{c}_{211}) \begin{pmatrix} 0 & 0 & 1 \\ 0 & 1 & 0 \\ -1 & 0 & 0 \end{pmatrix}, \overrightarrow{O_{211}O_{97}} = \mathbf{0}$$

The reduction of higher dimensional irrep:

$$O : E \rightarrow A_1 + B_1 \quad \text{of } D_4.$$

The correspondences of irreps at HSPs from original SG to lowered SG:

$$\begin{aligned} n_{GM6}^{97} &= n_{GM7}^{211} + n_{GM8}^{211} & n_{GM7}^{97} &= n_{GM6}^{211} + n_{GM8}^{211} & n_{M6}^{97} &= n_{H7}^{211} + n_{H8}^{211} & n_{M7}^{97} &= n_{H6}^{211} + n_{H8}^{211} & n_{X5}^{97} &= n_{N5}^{211} & n_{P5}^{97} &= n_{P5}^{211} + n_{P6}^{211} + n_{P7}^{211} \\ n_{N4}^{97} &= n_{N5}^{211} & n_{N3}^{97} &= n_{N5}^{211} \end{aligned}$$

The lower SG is SG 97 when the preserved operations are: **(sub-SG label is 10)** 1, 4, 5, 9, 10, 8, 16, 15.

The transformation is:  $(\mathbf{a}_{97}, \mathbf{b}_{97}, \mathbf{c}_{97}) = (\mathbf{a}_{211}, \mathbf{b}_{211}, \mathbf{c}_{211}) \begin{pmatrix} 0 & -1 & 0 \\ 0 & 0 & 1 \\ -1 & 0 & 0 \end{pmatrix}, \overrightarrow{O_{211}O_{97}} = \mathbf{0}$

The reduction of higher dimensional irrep:

$$O : E \rightarrow A_1 + B_1 \text{ of } D_4.$$

The correspondences of irreps at HSPs from original SG to lowered SG:

$$\begin{aligned} n_{GM6}^{97} &= n_{GM7}^{211} + n_{GM8}^{211} n_{GM7}^{97} = n_{GM6}^{211} + n_{GM8}^{211} n_{M6}^{97} = n_{H7}^{211} + n_{H8}^{211} n_{M7}^{97} = n_{H6}^{211} + n_{H8}^{211} n_{X5}^{97} = n_{N5}^{211} n_{P5}^{97} = n_{P5}^{211} + n_{P6}^{211} + n_{P7}^{211} \\ n_{N4}^{97} &= n_{N5}^{211} n_{N3}^{97} = n_{N5}^{211} \end{aligned}$$

The lower SG is SG 146 when the preserved operations are: **(sub-SG label is 11)** 1, 17, 18.

The transformation is:  $(\mathbf{a}_{146}, \mathbf{b}_{146}, \mathbf{c}_{146}) = (\mathbf{a}_{211}, \mathbf{b}_{211}, \mathbf{c}_{211}) \begin{pmatrix} \frac{1}{2} & -\frac{1}{2} & \frac{1}{2} \\ \frac{1}{2} & \frac{1}{2} & -\frac{1}{2} \\ -\frac{1}{2} & \frac{1}{2} & \frac{1}{2} \end{pmatrix}, \overrightarrow{O_{211}O_{146}} = -\frac{1}{3}\mathbf{a}_{146} + (\frac{2}{3})\mathbf{b}_{146} + (-\frac{1}{3})\mathbf{c}_{146}$

The reduction of higher dimensional irrep:

$$O : T_1 \rightarrow A + {}^2E + {}^1E \text{ of } C_3.$$

$$O : T_2 \rightarrow A + {}^2E + {}^1E \text{ of } C_3.$$

The correspondences of irreps at HSPs from original SG to lowered SG:

$$\begin{aligned} n_{GM4}^{146} &= 2n_{GM8}^{211} n_{GM6}^{146} = n_{GM6}^{211} + n_{GM7}^{211} + n_{GM8}^{211} n_{GM5}^{146} = n_{GM6}^{211} + n_{GM7}^{211} + n_{GM8}^{211} n_{L2}^{146} = 2n_{N5}^{211} n_{F2}^{146} = 2n_{N5}^{211} n_{T4}^{146} = \\ 2n_{H8}^{211} n_{T6}^{146} &= n_{H6}^{211} + n_{H7}^{211} + n_{H8}^{211} n_{T5}^{146} = n_{H6}^{211} + n_{H7}^{211} + n_{H8}^{211} \end{aligned}$$

The lower SG is SG 146 when the preserved operations are: **(sub-SG label is 12)** 1, 24, 23.

The transformation is:  $(\mathbf{a}_{146}, \mathbf{b}_{146}, \mathbf{c}_{146}) = (\mathbf{a}_{211}, \mathbf{b}_{211}, \mathbf{c}_{211}) \begin{pmatrix} -\frac{1}{2} & -\frac{1}{2} & \frac{1}{2} \\ \frac{1}{2} & -\frac{1}{2} & -\frac{1}{2} \\ \frac{1}{2} & -\frac{1}{2} & \frac{1}{2} \end{pmatrix}, \overrightarrow{O_{211}O_{146}} = -\frac{1}{3}\mathbf{a}_{146} + (\frac{2}{3})\mathbf{b}_{146} + (-\frac{1}{3})\mathbf{c}_{146}$

The reduction of higher dimensional irrep:

$$O : T_1 \rightarrow A + {}^2E + {}^1E \text{ of } C_3.$$

$$O : T_2 \rightarrow A + {}^2E + {}^1E \text{ of } C_3.$$

The correspondences of irreps at HSPs from original SG to lowered SG:

$$\begin{aligned} n_{GM4}^{146} &= 2n_{GM8}^{211} n_{GM6}^{146} = n_{GM6}^{211} + n_{GM7}^{211} + n_{GM8}^{211} n_{GM5}^{146} = n_{GM6}^{211} + n_{GM7}^{211} + n_{GM8}^{211} n_{L2}^{146} = 2n_{N5}^{211} n_{F2}^{146} = 2n_{N5}^{211} n_{T4}^{146} = \\ 2n_{H8}^{211} n_{T6}^{146} &= n_{H6}^{211} + n_{H7}^{211} + n_{H8}^{211} n_{T5}^{146} = n_{H6}^{211} + n_{H7}^{211} + n_{H8}^{211} \end{aligned}$$

The lower SG is SG 146 when the preserved operations are: **(sub-SG label is 13)** 1, 20, 19.

The transformation is:  $(\mathbf{a}_{146}, \mathbf{b}_{146}, \mathbf{c}_{146}) = (\mathbf{a}_{211}, \mathbf{b}_{211}, \mathbf{c}_{211}) \begin{pmatrix} \frac{1}{2} & -\frac{1}{2} & \frac{1}{2} \\ -\frac{1}{2} & -\frac{1}{2} & \frac{1}{2} \\ \frac{1}{2} & -\frac{1}{2} & -\frac{1}{2} \end{pmatrix}, \overrightarrow{O_{211}O_{146}} = -\frac{1}{3}\mathbf{a}_{146} + (\frac{2}{3})\mathbf{b}_{146} + (-\frac{1}{3})\mathbf{c}_{146}$

The reduction of higher dimensional irrep:

$$O : T_1 \rightarrow A + {}^2E + {}^1E \text{ of } C_3.$$

$$O : T_2 \rightarrow A + {}^2E + {}^1E \text{ of } C_3.$$

The correspondences of irreps at HSPs from original SG to lowered SG:

$$\begin{aligned} n_{GM4}^{146} &= 2n_{GM8}^{211} n_{GM6}^{146} = n_{GM6}^{211} + n_{GM7}^{211} + n_{GM8}^{211} n_{GM5}^{146} = n_{GM6}^{211} + n_{GM7}^{211} + n_{GM8}^{211} n_{L2}^{146} = 2n_{N5}^{211} n_{F2}^{146} = 2n_{N5}^{211} n_{T4}^{146} = \\ 2n_{H8}^{211} n_{T6}^{146} &= n_{H6}^{211} + n_{H7}^{211} + n_{H8}^{211} n_{T5}^{146} = n_{H6}^{211} + n_{H7}^{211} + n_{H8}^{211} \end{aligned}$$

The lower SG is SG 146 when the preserved operations are: **(sub-SG label is 14)** 1, 22, 21.

The transformation is:  $(\mathbf{a}_{146}, \mathbf{b}_{146}, \mathbf{c}_{146}) = (\mathbf{a}_{211}, \mathbf{b}_{211}, \mathbf{c}_{211}) \begin{pmatrix} -\frac{1}{2} & -\frac{1}{2} & \frac{1}{2} \\ -\frac{1}{2} & \frac{1}{2} & \frac{1}{2} \\ -\frac{1}{2} & \frac{1}{2} & -\frac{1}{2} \end{pmatrix}, \overrightarrow{O_{211}O_{146}} = -\frac{1}{3}\mathbf{a}_{146} + (\frac{2}{3})\mathbf{b}_{146} + (-\frac{1}{3})\mathbf{c}_{146}$

The reduction of higher dimensional irrep:

$$O : T_1 \rightarrow A + {}^2E + {}^1E \text{ of } C_3.$$

$$O : T_2 \rightarrow A + {}^2E + {}^1E \text{ of } C_3.$$

The correspondences of irreps at HSPs from original SG to lowered SG:

$$\begin{aligned} n_{GM4}^{146} &= 2n_{GM8}^{211} n_{GM6}^{146} = n_{GM6}^{211} + n_{GM7}^{211} + n_{GM8}^{211} n_{GM5}^{146} = n_{GM6}^{211} + n_{GM7}^{211} + n_{GM8}^{211} n_{L2}^{146} = 2n_{N5}^{211} n_{F2}^{146} = 2n_{N5}^{211} n_{T4}^{146} = \\ 2n_{H8}^{211} n_{T6}^{146} &= n_{H6}^{211} + n_{H7}^{211} + n_{H8}^{211} n_{T5}^{146} = n_{H6}^{211} + n_{H7}^{211} + n_{H8}^{211} \end{aligned}$$

The lower SG is SG 197 when the preserved operations are: **(sub-SG label is 15)** 1, 8, 9, 10, 17, 24, 20, 22, 18, 23, 19, 21.

The transformation is:  $(\mathbf{a}_{197}, \mathbf{b}_{197}, \mathbf{c}_{197}) = (\mathbf{a}_{211}, \mathbf{b}_{211}, \mathbf{c}_{211}) \begin{pmatrix} 0 & 0 & 1 \\ 1 & 0 & 0 \\ 0 & 1 & 0 \end{pmatrix}, \overrightarrow{O_{211}O_{197}} = \mathbf{0}$

The reduction of higher dimensional irrep:

$$O : E \rightarrow {}^1E + {}^2E \text{ of } T.$$

The correspondences of irreps at HSPs from original SG to lowered SG:

$$n_{GM6}^{197} = n_{GM8}^{211} n_{GM7}^{197} = n_{GM8}^{211} n_{GM5}^{197} = n_{GM6}^{211} + n_{GM7}^{211} n_{H6}^{197} = n_{H8}^{211} n_{H7}^{197} = n_{H8}^{211} n_{H5}^{197} = n_{H6}^{211} + n_{H7}^{211} n_{N4}^{197} = n_{N5}^{211} n_{N3}^{197} = n_{N5}^{211} n_{P6}^{197} = n_{P6}^{211} n_{P7}^{197} = n_{P7}^{211} n_{P5}^{197} = n_{P5}^{211}$$

**109. Lowered SGs by higher-dimensional irreps of pairings in SG 212**

The representative operations of SG/T for SG 212:

$$1 : (x, y, z), 2 : (x + \frac{3}{4}, \frac{3}{4} - z, y + \frac{1}{4}), 3 : (x + \frac{1}{4}, z + \frac{3}{4}, \frac{3}{4} - y), 4 : (z + \frac{1}{4}, y + \frac{3}{4}, \frac{3}{4} - x), 5 : (\frac{3}{4} - z, y + \frac{1}{4}, x + \frac{3}{4}),$$

$$6 : (\frac{3}{4} - y, x + \frac{1}{4}, z + \frac{3}{4}), 7 : (y + \frac{3}{4}, \frac{3}{4} - x, z + \frac{1}{4}), 8 : (x + \frac{1}{2}, \frac{1}{2} - y, -z), 9 : (-x, y + \frac{1}{2}, \frac{1}{2} - z), 10 : (\frac{1}{2} - x, -y, z + \frac{1}{2}),$$

$$11 : (y + \frac{1}{4}, x + \frac{3}{4}, \frac{3}{4} - z), 12 : (\frac{1}{4} - y, \frac{1}{4} - x, \frac{1}{4} - z), 13 : (\frac{3}{4} - x, z + \frac{1}{4}, y + \frac{3}{4}), 14 : (\frac{1}{4} - x, \frac{1}{4} - z, \frac{1}{4} - y), 15 : (z + \frac{3}{4}, \frac{3}{4} - y, x + \frac{1}{4}),$$

$$16 : (\frac{1}{4} - z, \frac{1}{4} - y, \frac{1}{4} - x), 17 : (z, x, y), 18 : (y, z, x), 19 : (-y, z + \frac{1}{2}, \frac{1}{2} - x), 20 : (\frac{1}{2} - z, -x, y + \frac{1}{2}), 21 : (\frac{1}{2} - y, -z, x + \frac{1}{2}),$$

$$22 : (z + \frac{1}{2}, \frac{1}{2} - x, -y), 23 : (y + \frac{1}{2}, \frac{1}{2} - z, -x), 24 : (-z, x + \frac{1}{2}, \frac{1}{2} - y).$$

The lower SG is SG 19 when the preserved operations are: (sub-SG label is 1) 1, 8, 9, 10.

The transformation is:  $(\mathbf{a}_{19}, \mathbf{b}_{19}, \mathbf{c}_{19}) = (\mathbf{a}_{212}, \mathbf{b}_{212}, \mathbf{c}_{212}) \begin{pmatrix} -1 & 0 & 0 \\ 0 & 0 & 1 \\ 0 & 1 & 0 \end{pmatrix}, \overrightarrow{O_{212}O_{19}} = \frac{1}{4}\mathbf{a}_{19} + (-\frac{1}{4})\mathbf{b}_{19} + (\frac{3}{4})\mathbf{c}_{19}$

The reduction of higher dimensional irrep:

$$O : T_1 \rightarrow B_1 + B_3 + B_2 \text{ of } D_2.$$

$$O : T_2 \rightarrow B_1 + B_3 + B_2 \text{ of } D_2.$$

The correspondences of irreps at HSPs from original SG to lowered SG:

$$n_{GM5}^{19} = n_{GM6}^{212} + n_{GM7}^{212} + 2n_{GM8}^{212} n_{X4}^{19} = n_{X4}^{212} + n_{X6}^{212} n_{X5}^{19} = n_{X3}^{212} + n_{X5}^{212} n_{X3}^{19} = n_{X7}^{212} n_{X2}^{19} = n_{X7}^{212} n_{S5}^{19} = n_{M6}^{212} + n_{M7}^{212}$$

$$n_{R3}^{19} = n_{R4}^{212} + n_{R5}^{212} + 2n_{R6}^{212} n_{R2}^{19} = n_{R7}^{212} + n_{R8}^{212} n_{R4}^{19} = n_{R7}^{212} + n_{R8}^{212} n_{R5}^{19} = n_{R7}^{212} + n_{R8}^{212} n_{U5}^{19} = n_{M6}^{212} + n_{M7}^{212} n_{Z4}^{19} = n_{X7}^{212} n_{Z5}^{19} =$$

$$n_{X3}^{212} + n_{X5}^{212} n_{Z3}^{19} = n_{X4}^{212} + n_{X6}^{212} n_{Z2}^{19} = n_{X7}^{212} n_{T5}^{19} = n_{M6}^{212} + n_{M7}^{212} n_{Y3}^{19} = n_{X4}^{212} + n_{X6}^{212} n_{Y2}^{19} = n_{X7}^{212} n_{Y4}^{19} = n_{X3}^{212} + n_{X5}^{212} n_{Y5}^{19} =$$

$$n_{X7}^{212}$$

The lower SG is SG 20 when the preserved operations are: (sub-SG label is 2) 1, 8, 13, 14.

The transformation is:  $(\mathbf{a}_{20}, \mathbf{b}_{20}, \mathbf{c}_{20}) = (\mathbf{a}_{212}, \mathbf{b}_{212}, \mathbf{c}_{212}) \begin{pmatrix} 0 & 0 & -1 \\ 1 & 1 & 0 \\ 1 & -1 & 0 \end{pmatrix}, \overrightarrow{O_{212}O_{20}} = \frac{1}{8}\mathbf{a}_{20} + (\frac{1}{8})\mathbf{b}_{20} + (\frac{5}{8})\mathbf{c}_{20}$

The reduction of higher dimensional irrep:

$$O : T_1 \rightarrow B_1 + B_2 + B_3 \text{ of } D_2.$$

$$O : T_2 \rightarrow A_1 + B_2 + B_3 \text{ of } D_2.$$

The correspondences of irreps at HSPs from original SG to lowered SG:

$$n_{GM5}^{20} = n_{GM6}^{212} + n_{GM7}^{212} + 2n_{GM8}^{212} n_{Y5}^{20} = n_{M6}^{212} + n_{M7}^{212} n_{S4}^{20} = n_{X3}^{212} + n_{X5}^{212} + n_{X7}^{212} n_{S3}^{20} = n_{X4}^{212} + n_{X6}^{212} + n_{X7}^{212} n_{Z5}^{20} = n_{X5}^{212} + n_{X6}^{212}$$

$$n_{Z4}^{20} = n_{X7}^{212} n_{Z2}^{20} = n_{X7}^{212} n_{Z3}^{20} = n_{X3}^{212} + n_{X4}^{212} n_{T5}^{20} = n_{R4}^{212} + n_{R6}^{212} + n_{R8}^{212} n_{T4}^{20} = n_{R7}^{212} + n_{R8}^{212} n_{T2}^{20} = n_{R7}^{212} + n_{R8}^{212} n_{T3}^{20} =$$

$$n_{R5}^{212} + n_{R6}^{212} + n_{R8}^{212} n_{R4}^{20} = n_{M6}^{212} + n_{M7}^{212} n_{R3}^{20} = n_{M6}^{212} + n_{M7}^{212}$$

The lower SG is SG 20 when the preserved operations are: (sub-SG label is 3) 1, 9, 16, 15.

The transformation is:  $(\mathbf{a}_{20}, \mathbf{b}_{20}, \mathbf{c}_{20}) = (\mathbf{a}_{212}, \mathbf{b}_{212}, \mathbf{c}_{212}) \begin{pmatrix} -1 & 1 & 0 \\ 0 & 0 & 1 \\ 1 & 1 & 0 \end{pmatrix}, \overrightarrow{O_{212}O_{20}} = \frac{1}{8}\mathbf{a}_{20} + (\frac{1}{8})\mathbf{b}_{20} + (\frac{1}{8})\mathbf{c}_{20}$

The reduction of higher dimensional irrep:

$$O : T_1 \rightarrow B_1 + B_2 + B_3 \text{ of } D_2.$$

$$O : T_2 \rightarrow A_1 + B_2 + B_3 \text{ of } D_2.$$

The correspondences of irreps at HSPs from original SG to lowered SG:

$$n_{GM5}^{20} = n_{GM6}^{212} + n_{GM7}^{212} + 2n_{GM8}^{212} n_{Y5}^{20} = n_{M6}^{212} + n_{M7}^{212} n_{S4}^{20} = n_{X3}^{212} + n_{X5}^{212} + n_{X7}^{212} n_{S3}^{20} = n_{X4}^{212} + n_{X6}^{212} + n_{X7}^{212} n_{Z5}^{20} = n_{X5}^{212} + n_{X6}^{212}$$

$$n_{Z4}^{20} = n_{X7}^{212} n_{Z2}^{20} = n_{X7}^{212} n_{Z3}^{20} = n_{X3}^{212} + n_{X4}^{212} n_{T5}^{20} = n_{R4}^{212} + n_{R6}^{212} + n_{R8}^{212} n_{T4}^{20} = n_{R7}^{212} + n_{R8}^{212} n_{T2}^{20} = n_{R7}^{212} + n_{R8}^{212} n_{T3}^{20} =$$

$$n_{R5}^{212} + n_{R6}^{212} + n_{R8}^{212} n_{R4}^{20} = n_{M6}^{212} + n_{M7}^{212} n_{R3}^{20} = n_{M6}^{212} + n_{M7}^{212}$$

The lower SG is SG 20 when the preserved operations are: **(sub-SG label is 4) 1, 10, 11, 12.**

$$\text{The transformation is: } (\mathbf{a}_{20}, \mathbf{b}_{20}, \mathbf{c}_{20}) = (\mathbf{a}_{212}, \mathbf{b}_{212}, \mathbf{c}_{212}) \begin{pmatrix} 1 & -1 & 0 \\ -1 & -1 & 0 \\ 0 & 0 & -1 \end{pmatrix}, \overrightarrow{O_{212}O_{20}} = \frac{1}{8}\mathbf{a}_{20} + (-\frac{1}{8})\mathbf{b}_{20} + (-\frac{1}{8})\mathbf{c}_{20}$$

The reduction of higher dimensional irrep:

$$O : T_1 \rightarrow B_1 + B_2 + B_3 \text{ of } D_2.$$

$$O : T_2 \rightarrow A_1 + B_2 + B_3 \text{ of } D_2.$$

The correspondences of irreps at HSPs from original SG to lowered SG:

$$\begin{aligned} n_{GM5}^{20} &= n_{GM6}^{212} + n_{GM7}^{212} + 2n_{GM8}^{212} & n_{Y5}^{20} &= n_{M6}^{212} + n_{M7}^{212} & n_{S4}^{20} &= n_{X3}^{212} + n_{X5}^{212} + n_{X7}^{212} & n_{S3}^{20} &= n_{X4}^{212} + n_{X6}^{212} + n_{X7}^{212} & n_{Z5}^{20} &= n_{X3}^{212} + n_{X4}^{212} \\ n_{Z4}^{20} &= n_{X7}^{212} & n_{Z2}^{20} &= n_{X7}^{212} & n_{Z3}^{20} &= n_{X5}^{212} + n_{X6}^{212} & n_{T5}^{20} &= n_{R5}^{212} + n_{R6}^{212} + n_{R8}^{212} & n_{T4}^{20} &= n_{R7}^{212} + n_{R8}^{212} & n_{T2}^{20} &= n_{R7}^{212} + n_{R8}^{212} & n_{T3}^{20} &= \\ n_{R4}^{212} + n_{R6}^{212} + n_{R7}^{212} & n_{R4}^{20} &= n_{M6}^{212} + n_{M7}^{212} & n_{R3}^{20} &= n_{M6}^{212} + n_{M7}^{212} \end{aligned}$$

The lower SG is SG 78 when the preserved operations are: **(sub-SG label is 5) 1, 6, 7, 10.**

$$\text{The transformation is: } (\mathbf{a}_{78}, \mathbf{b}_{78}, \mathbf{c}_{78}) = (\mathbf{a}_{212}, \mathbf{b}_{212}, \mathbf{c}_{212}) \begin{pmatrix} -1 & 0 & 0 \\ 0 & -1 & 0 \\ 0 & 0 & 1 \end{pmatrix}, \overrightarrow{O_{212}O_{78}} = -\frac{1}{4}\mathbf{a}_{78} + (\frac{1}{2})\mathbf{b}_{78}$$

The reduction of higher dimensional irrep:

$$O : T_1 \rightarrow A + {}^2E + {}^1E \text{ of } C_4.$$

$$O : T_2 \rightarrow {}^2E + B + {}^1E \text{ of } C_4.$$

The correspondences of irreps at HSPs from original SG to lowered SG:

$$\begin{aligned} n_{GM5}^{78} &= n_{GM7}^{212} + n_{GM8}^{212} & n_{GM7}^{78} &= n_{GM7}^{212} + n_{GM8}^{212} & n_{GM8}^{78} &= n_{GM6}^{212} + n_{GM8}^{212} & n_{GM6}^{78} &= n_{GM6}^{212} + n_{GM8}^{212} & n_{X4}^{78} &= n_{X3}^{212} + n_{X5}^{212} + n_{X7}^{212} \\ n_{X3}^{78} &= n_{X4}^{212} + n_{X6}^{212} + n_{X7}^{212} & n_{M5}^{78} &= n_{M6}^{212} & n_{M7}^{78} &= n_{M7}^{212} & n_{M8}^{78} &= n_{M6}^{212} & n_{M6}^{78} &= n_{M7}^{212} & n_{A5}^{78} &= n_{R5}^{212} + n_{R6}^{212} + n_{R7}^{212} & n_{A7}^{78} &= n_{R7}^{212} + n_{R8}^{212} \\ n_{A8}^{78} &= n_{R7}^{212} + n_{R8}^{212} & n_{A6}^{78} &= n_{R4}^{212} + n_{R6}^{212} + n_{R8}^{212} & n_{R4}^{78} &= n_{M6}^{212} + n_{M7}^{212} & n_{R3}^{78} &= n_{M6}^{212} + n_{M7}^{212} & n_{Z7}^{78} &= n_{X3}^{212} + n_{X6}^{212} & n_{Z6}^{78} &= n_{X7}^{212} & n_{Z5}^{78} &= \\ n_{X7}^{212} & n_{Z8}^{78} &= n_{X4}^{212} + n_{X5}^{212} \end{aligned}$$

The lower SG is SG 78 when the preserved operations are: **(sub-SG label is 6) 1, 2, 3, 8.**

$$\text{The transformation is: } (\mathbf{a}_{78}, \mathbf{b}_{78}, \mathbf{c}_{78}) = (\mathbf{a}_{212}, \mathbf{b}_{212}, \mathbf{c}_{212}) \begin{pmatrix} 0 & 0 & -1 \\ -1 & 0 & 0 \\ 0 & 1 & 0 \end{pmatrix}, \overrightarrow{O_{212}O_{78}} = \frac{1}{4}\mathbf{a}_{78} + \mathbf{b}_{78}$$

The reduction of higher dimensional irrep:

$$O : T_1 \rightarrow A + {}^2E + {}^1E \text{ of } C_4.$$

$$O : T_2 \rightarrow {}^2E + B + {}^1E \text{ of } C_4.$$

The correspondences of irreps at HSPs from original SG to lowered SG:

$$\begin{aligned} n_{GM5}^{78} &= n_{GM7}^{212} + n_{GM8}^{212} & n_{GM7}^{78} &= n_{GM7}^{212} + n_{GM8}^{212} & n_{GM8}^{78} &= n_{GM6}^{212} + n_{GM8}^{212} & n_{GM6}^{78} &= n_{GM6}^{212} + n_{GM8}^{212} & n_{X4}^{78} &= n_{X3}^{212} + n_{X5}^{212} + n_{X7}^{212} \\ n_{X3}^{78} &= n_{X4}^{212} + n_{X6}^{212} + n_{X7}^{212} & n_{M5}^{78} &= n_{M6}^{212} & n_{M7}^{78} &= n_{M7}^{212} & n_{M8}^{78} &= n_{M6}^{212} & n_{M6}^{78} &= n_{M7}^{212} & n_{A5}^{78} &= n_{R5}^{212} + n_{R6}^{212} + n_{R7}^{212} & n_{A7}^{78} &= n_{R7}^{212} + n_{R8}^{212} \\ n_{A8}^{78} &= n_{R7}^{212} + n_{R8}^{212} & n_{A6}^{78} &= n_{R4}^{212} + n_{R6}^{212} + n_{R8}^{212} & n_{R4}^{78} &= n_{M6}^{212} + n_{M7}^{212} & n_{R3}^{78} &= n_{M6}^{212} + n_{M7}^{212} & n_{Z7}^{78} &= n_{X3}^{212} + n_{X6}^{212} & n_{Z6}^{78} &= n_{X7}^{212} & n_{Z5}^{78} &= \\ n_{X7}^{212} & n_{Z8}^{78} &= n_{X4}^{212} + n_{X5}^{212} \end{aligned}$$

The lower SG is SG 78 when the preserved operations are: **(sub-SG label is 7) 1, 4, 5, 9.**

$$\text{The transformation is: } (\mathbf{a}_{78}, \mathbf{b}_{78}, \mathbf{c}_{78}) = (\mathbf{a}_{212}, \mathbf{b}_{212}, \mathbf{c}_{212}) \begin{pmatrix} -1 & 0 & 0 \\ 0 & 0 & -1 \\ 0 & -1 & 0 \end{pmatrix}, \overrightarrow{O_{212}O_{78}} = \mathbf{a}_{78} + (\frac{1}{4})\mathbf{b}_{78}$$

The reduction of higher dimensional irrep:

$$O : T_1 \rightarrow A + {}^2E + {}^1E \text{ of } C_4.$$

$$O : T_2 \rightarrow {}^2E + B + {}^1E \text{ of } C_4.$$

The correspondences of irreps at HSPs from original SG to lowered SG:

$$\begin{aligned} n_{GM5}^{78} &= n_{GM7}^{212} + n_{GM8}^{212} & n_{GM7}^{78} &= n_{GM7}^{212} + n_{GM8}^{212} & n_{GM8}^{78} &= n_{GM6}^{212} + n_{GM8}^{212} & n_{GM6}^{78} &= n_{GM6}^{212} + n_{GM8}^{212} & n_{X4}^{78} &= n_{X3}^{212} + n_{X5}^{212} + n_{X7}^{212} \\ n_{X3}^{78} &= n_{X4}^{212} + n_{X6}^{212} + n_{X7}^{212} & n_{M5}^{78} &= n_{M6}^{212} & n_{M7}^{78} &= n_{M7}^{212} & n_{M8}^{78} &= n_{M6}^{212} & n_{M6}^{78} &= n_{M7}^{212} & n_{A5}^{78} &= n_{R5}^{212} + n_{R6}^{212} + n_{R7}^{212} & n_{A7}^{78} &= n_{R7}^{212} + n_{R8}^{212} \\ n_{A8}^{78} &= n_{R7}^{212} + n_{R8}^{212} & n_{A6}^{78} &= n_{R4}^{212} + n_{R6}^{212} + n_{R8}^{212} & n_{R4}^{78} &= n_{M6}^{212} + n_{M7}^{212} & n_{R3}^{78} &= n_{M6}^{212} + n_{M7}^{212} & n_{Z7}^{78} &= n_{X3}^{212} + n_{X6}^{212} & n_{Z6}^{78} &= n_{X7}^{212} & n_{Z5}^{78} &= \\ n_{X7}^{212} & n_{Z8}^{78} &= n_{X4}^{212} + n_{X5}^{212} \end{aligned}$$

The lower SG is SG 96 when the preserved operations are: **(sub-SG label is 8) 1, 6, 7, 10, 8, 9, 11, 12.**

$$\text{The transformation is: } (\mathbf{a}_{96}, \mathbf{b}_{96}, \mathbf{c}_{96}) = (\mathbf{a}_{212}, \mathbf{b}_{212}, \mathbf{c}_{212}) \begin{pmatrix} 0 & -1 & 0 \\ -1 & 0 & 0 \\ 0 & 0 & -1 \end{pmatrix}, \overrightarrow{O_{212}O_{96}} = \frac{1}{2}\mathbf{a}_{96} + (\frac{1}{4})\mathbf{b}_{96} + (\frac{1}{8})\mathbf{c}_{96}$$

The reduction of higher dimensional irrep:

$$O : E \rightarrow A_1 + B_1 \text{ of } D_4.$$

The correspondences of irreps at HSPs from original SG to lowered SG:

$$\begin{aligned} n_{GM6}^{96} &= n_{GM7}^{212} + n_{GM8}^{212} & n_{GM7}^{96} &= n_{GM6}^{212} + n_{GM8}^{212} & n_{X3}^{96} &= n_{X3}^{212} + n_{X5}^{212} & n_{X4}^{96} &= n_{X4}^{212} + n_{X6}^{212} & n_{X5}^{96} &= n_{X7}^{212} & n_{X6}^{96} &= n_{X7}^{212} & n_{M6}^{96} &= n_{M6}^{212} + n_{M7}^{212} \\ n_{M7}^{96} &= n_{M6}^{212} & n_{A6}^{96} &= n_{R7}^{212} & n_{A4}^{96} &= n_{R5}^{212} + n_{R6}^{212} & n_{A3}^{96} &= n_{R8}^{212} & n_{A5}^{96} &= n_{R4}^{212} + n_{R6}^{212} & n_{A7}^{96} &= n_{R7}^{212} + n_{R8}^{212} & n_{R5}^{96} &= n_{M6}^{212} + n_{M7}^{212} \\ n_{Z3}^{96} &= n_{X3}^{212} & n_{Z5}^{96} &= n_{X6}^{212} & n_{Z6}^{96} &= n_{X5}^{212} & n_{Z4}^{96} &= n_{X4}^{212} & n_{Z7}^{96} &= n_{X7}^{212} \end{aligned}$$

The lower SG is SG 96 when the preserved operations are: **(sub-SG label is 9)** 1, 2, 3, 8, 9, 10, 13, 14.

$$\text{The transformation is: } (\mathbf{a}_{96}, \mathbf{b}_{96}, \mathbf{c}_{96}) = (\mathbf{a}_{212}, \mathbf{b}_{212}, \mathbf{c}_{212}) \begin{pmatrix} 0 & 0 & -1 \\ -1 & 0 & 0 \\ 0 & 1 & 0 \end{pmatrix}, \overrightarrow{O_{212}O_{96}} = \frac{1}{4}\mathbf{a}_{96} + \left(\frac{1}{2}\right)\mathbf{b}_{96} + \left(\frac{3}{8}\right)\mathbf{c}_{96}$$

The reduction of higher dimensional irrep:

$$O : E \rightarrow A_1 + B_1 \text{ of } D_4.$$

The correspondences of irreps at HSPs from original SG to lowered SG:

$$\begin{aligned} n_{GM6}^{96} &= n_{GM7}^{212} + n_{GM8}^{212} & n_{GM7}^{96} &= n_{GM6}^{212} + n_{GM8}^{212} & n_{X3}^{96} &= n_{X4}^{212} + n_{X6}^{212} & n_{X4}^{96} &= n_{X3}^{212} + n_{X5}^{212} & n_{X5}^{96} &= n_{X7}^{212} & n_{X6}^{96} &= n_{X7}^{212} & n_{M6}^{96} &= n_{M6}^{212} + n_{M7}^{212} \\ n_{M7}^{96} &= n_{M6}^{212} & n_{A6}^{96} &= n_{R8}^{212} & n_{A4}^{96} &= n_{R4}^{212} + n_{R6}^{212} & n_{A3}^{96} &= n_{R7}^{212} & n_{A5}^{96} &= n_{R5}^{212} + n_{R6}^{212} & n_{A7}^{96} &= n_{R7}^{212} + n_{R8}^{212} & n_{R5}^{96} &= n_{M6}^{212} + n_{M7}^{212} \\ n_{Z3}^{96} &= n_{X6}^{212} & n_{Z5}^{96} &= n_{X3}^{212} & n_{Z6}^{96} &= n_{X4}^{212} & n_{Z4}^{96} &= n_{X5}^{212} & n_{Z7}^{96} &= n_{X7}^{212} \end{aligned}$$

The lower SG is SG 96 when the preserved operations are: **(sub-SG label is 10)** 1, 4, 5, 9, 10, 8, 16, 15.

$$\text{The transformation is: } (\mathbf{a}_{96}, \mathbf{b}_{96}, \mathbf{c}_{96}) = (\mathbf{a}_{212}, \mathbf{b}_{212}, \mathbf{c}_{212}) \begin{pmatrix} 1 & 0 & 0 \\ 0 & 0 & 1 \\ 0 & -1 & 0 \end{pmatrix}, \overrightarrow{O_{212}O_{96}} = \frac{1}{2}\mathbf{a}_{96} + \left(\frac{1}{4}\right)\mathbf{b}_{96} + \left(\frac{5}{8}\right)\mathbf{c}_{96}$$

The reduction of higher dimensional irrep:

$$O : E \rightarrow A_1 + B_1 \text{ of } D_4.$$

The correspondences of irreps at HSPs from original SG to lowered SG:

$$\begin{aligned} n_{GM6}^{96} &= n_{GM7}^{212} + n_{GM8}^{212} & n_{GM7}^{96} &= n_{GM6}^{212} + n_{GM8}^{212} & n_{X3}^{96} &= n_{X4}^{212} + n_{X6}^{212} & n_{X4}^{96} &= n_{X3}^{212} + n_{X5}^{212} & n_{X5}^{96} &= n_{X7}^{212} & n_{X6}^{96} &= n_{X7}^{212} & n_{M6}^{96} &= n_{M6}^{212} + n_{M7}^{212} \\ n_{M7}^{96} &= n_{M6}^{212} & n_{A6}^{96} &= n_{R8}^{212} & n_{A4}^{96} &= n_{R4}^{212} + n_{R6}^{212} & n_{A3}^{96} &= n_{R7}^{212} & n_{A5}^{96} &= n_{R5}^{212} + n_{R6}^{212} & n_{A7}^{96} &= n_{R7}^{212} + n_{R8}^{212} & n_{R5}^{96} &= n_{M6}^{212} + n_{M7}^{212} \\ n_{Z3}^{96} &= n_{X6}^{212} & n_{Z5}^{96} &= n_{X3}^{212} & n_{Z6}^{96} &= n_{X4}^{212} & n_{Z4}^{96} &= n_{X5}^{212} & n_{Z7}^{96} &= n_{X7}^{212} \end{aligned}$$

The lower SG is SG 146 when the preserved operations are: **(sub-SG label is 11)** 1, 17, 18.

$$\text{The transformation is: } (\mathbf{a}_{146}, \mathbf{b}_{146}, \mathbf{c}_{146}) = (\mathbf{a}_{212}, \mathbf{b}_{212}, \mathbf{c}_{212}) \begin{pmatrix} 0 & 1 & 0 \\ 0 & 0 & 1 \\ 1 & 0 & 0 \end{pmatrix}, \overrightarrow{O_{212}O_{146}} = -\frac{1}{3}\mathbf{a}_{146} + \left(\frac{2}{3}\right)\mathbf{b}_{146} + \left(-\frac{1}{3}\right)\mathbf{c}_{146}$$

The reduction of higher dimensional irrep:

$$O : T_1 \rightarrow A + {}^2E + {}^1E \text{ of } C_3.$$

$$O : T_2 \rightarrow A + {}^2E + {}^1E \text{ of } C_3.$$

The correspondences of irreps at HSPs from original SG to lowered SG:

$$\begin{aligned} n_{GM4}^{146} &= 2n_{GM8}^{212} & n_{GM6}^{146} &= n_{GM6}^{212} + n_{GM7}^{212} + n_{GM8}^{212} & n_{GM5}^{146} &= n_{GM6}^{212} + n_{GM7}^{212} + n_{GM8}^{212} & n_{L2}^{146} &= n_{X3}^{212} + n_{X4}^{212} + n_{X5}^{212} + n_{X6}^{212} + 2n_{X7}^{212} \\ n_{F2}^{146} &= 2n_{M6}^{212} + 2n_{M7}^{212} & n_{T4}^{146} &= n_{R4}^{212} + n_{R5}^{212} + n_{R7}^{212} + n_{R8}^{212} & n_{T6}^{146} &= n_{R6}^{212} + n_{R7}^{212} + n_{R8}^{212} & n_{T5}^{146} &= n_{R6}^{212} + n_{R7}^{212} + n_{R8}^{212} \end{aligned}$$

The lower SG is SG 146 when the preserved operations are: **(sub-SG label is 12)** 1, 24, 23.

$$\text{The transformation is: } (\mathbf{a}_{146}, \mathbf{b}_{146}, \mathbf{c}_{146}) = (\mathbf{a}_{212}, \mathbf{b}_{212}, \mathbf{c}_{212}) \begin{pmatrix} 0 & -1 & 0 \\ 0 & 0 & -1 \\ 1 & 0 & 0 \end{pmatrix}, \overrightarrow{O_{212}O_{146}} = -\frac{1}{6}\mathbf{a}_{146} + \left(\frac{5}{6}\right)\mathbf{b}_{146} + \left(-\frac{2}{3}\right)\mathbf{c}_{146}$$

The reduction of higher dimensional irrep:

$$O : T_1 \rightarrow A + {}^2E + {}^1E \text{ of } C_3.$$

$$O : T_2 \rightarrow A + {}^2E + {}^1E \text{ of } C_3.$$

The correspondences of irreps at HSPs from original SG to lowered SG:

$$\begin{aligned} n_{GM4}^{146} &= 2n_{GM8}^{212} & n_{GM6}^{146} &= n_{GM6}^{212} + n_{GM7}^{212} + n_{GM8}^{212} & n_{GM5}^{146} &= n_{GM6}^{212} + n_{GM7}^{212} + n_{GM8}^{212} & n_{L2}^{146} &= n_{X3}^{212} + n_{X4}^{212} + n_{X5}^{212} + n_{X6}^{212} + 2n_{X7}^{212} \\ n_{F2}^{146} &= 2n_{M6}^{212} + 2n_{M7}^{212} & n_{T4}^{146} &= n_{R4}^{212} + n_{R5}^{212} + n_{R7}^{212} + n_{R8}^{212} & n_{T6}^{146} &= n_{R6}^{212} + n_{R7}^{212} + n_{R8}^{212} & n_{T5}^{146} &= n_{R6}^{212} + n_{R7}^{212} + n_{R8}^{212} \end{aligned}$$

The lower SG is SG 146 when the preserved operations are: **(sub-SG label is 13)** 1, 20, 19.

$$\text{The transformation is: } (\mathbf{a}_{146}, \mathbf{b}_{146}, \mathbf{c}_{146}) = (\mathbf{a}_{212}, \mathbf{b}_{212}, \mathbf{c}_{212}) \begin{pmatrix} 0 & 0 & -1 \\ 0 & 1 & 0 \\ 1 & 0 & 0 \end{pmatrix}, \overrightarrow{O_{212}O_{146}} = \frac{1}{2}\mathbf{b}_{146} + \left(-\frac{1}{2}\right)\mathbf{c}_{146}$$

The reduction of higher dimensional irrep:

$$O : T_1 \rightarrow A + {}^2E + {}^1E \text{ of } C_3.$$

$$O : T_2 \rightarrow A + {}^2E + {}^1E \text{ of } C_3.$$

The correspondences of irreps at HSPs from original SG to lowered SG:

$$n_{GM4}^{146} = 2n_{GM8}^{212} \quad n_{GM6}^{146} = n_{GM6}^{212} + n_{GM7}^{212} + n_{GM8}^{212} \quad n_{GM5}^{146} = n_{GM6}^{212} + n_{GM7}^{212} + n_{GM8}^{212} \quad n_{L2}^{146} = n_{X3}^{212} + n_{X4}^{212} + n_{X5}^{212} + n_{X6}^{212} + 2n_{X7}^{212}$$

$$n_{F2}^{146} = 2n_{M6}^{212} + 2n_{M7}^{212} n_{T4}^{146} = n_{R4}^{212} + n_{R5}^{212} + n_{R7}^{212} + n_{R8}^{212} n_{T6}^{146} = n_{R6}^{212} + n_{R7}^{212} + n_{R8}^{212} n_{T5}^{146} = n_{R6}^{212} + n_{R7}^{212} + n_{R8}^{212}$$

The lower SG is SG 146 when the preserved operations are: **(sub-SG label is 14) 1, 22, 21.**

$$\text{The transformation is: } (\mathbf{a}_{146}, \mathbf{b}_{146}, \mathbf{c}_{146}) = (\mathbf{a}_{212}, \mathbf{b}_{212}, \mathbf{c}_{212}) \begin{pmatrix} -1 & 0 & 0 \\ 0 & 1 & 0 \\ 0 & 0 & -1 \end{pmatrix}, \overrightarrow{O_{212}O_{146}} = -\frac{2}{3}\mathbf{a}_{146} + \left(\frac{5}{6}\right)\mathbf{b}_{146} + \left(-\frac{1}{6}\right)\mathbf{c}_{146}$$

The reduction of higher dimensional irrep:

$$O : T_1 \rightarrow A + {}^2E + {}^1E \text{ of } C_3.$$

$$O : T_2 \rightarrow A + {}^2E + {}^1E \text{ of } C_3.$$

The correspondences of irreps at HSPs from original SG to lowered SG:

$$n_{GM4}^{146} = 2n_{GM8}^{212} n_{GM6}^{146} = n_{GM6}^{212} + n_{GM7}^{212} + n_{GM8}^{212} n_{GM5}^{146} = n_{GM6}^{212} + n_{GM7}^{212} + n_{GM8}^{212} n_{L2}^{146} = n_{X3}^{212} + n_{X4}^{212} + n_{X5}^{212} + n_{X6}^{212} + 2n_{X7}^{212}$$

$$n_{F2}^{146} = 2n_{M6}^{212} + 2n_{M7}^{212} n_{T4}^{146} = n_{R4}^{212} + n_{R5}^{212} + n_{R7}^{212} + n_{R8}^{212} n_{T6}^{146} = n_{R6}^{212} + n_{R7}^{212} + n_{R8}^{212} n_{T5}^{146} = n_{R6}^{212} + n_{R7}^{212} + n_{R8}^{212}$$

The lower SG is SG 198 when the preserved operations are: **(sub-SG label is 15) 1, 8, 9, 10, 17, 24, 20, 22, 18, 23, 19, 21.**

$$\text{The transformation is: } (\mathbf{a}_{198}, \mathbf{b}_{198}, \mathbf{c}_{198}) = (\mathbf{a}_{212}, \mathbf{b}_{212}, \mathbf{c}_{212}) \begin{pmatrix} 0 & 0 & -1 \\ 1 & 0 & 0 \\ 0 & -1 & 0 \end{pmatrix}, \overrightarrow{O_{212}O_{198}} = -\frac{1}{2}\mathbf{c}_{198}$$

The reduction of higher dimensional irrep:

$$O : E \rightarrow {}^1E + {}^2E \text{ of } T.$$

The correspondences of irreps at HSPs from original SG to lowered SG:

$$n_{GM6}^{198} = n_{GM8}^{212} n_{GM7}^{198} = n_{GM8}^{212} n_{GM5}^{198} = n_{GM6}^{212} + n_{GM7}^{212} n_{X3}^{198} = n_{X3}^{212} + n_{X5}^{212} n_{X4}^{198} = n_{X4}^{212} + n_{X6}^{212} n_{X5}^{198} = n_{X7}^{212} n_{X2}^{198} = n_{X7}^{212}$$

$$n_{M5}^{198} = n_{M6}^{212} + n_{M7}^{212} n_{R4}^{198} = n_{R4}^{212} + n_{R5}^{212} n_{R6}^{198} = n_{R6}^{212} n_{R5}^{198} = n_{R6}^{212} n_{R7}^{198} = n_{R7}^{212} + n_{R8}^{212}$$

### 110. Lowered SGs by higher-dimensional irreps of pairings in SG 213

The representative operations of SG/T for SG 213:

$$\begin{aligned} &1 : (x, y, z), 2 : (x + \frac{1}{4}, \frac{1}{4} - z, y + \frac{3}{4}), 3 : (x + \frac{3}{4}, z + \frac{1}{4}, \frac{1}{4} - y), 4 : (z + \frac{3}{4}, y + \frac{1}{4}, \frac{1}{4} - x), 5 : (\frac{1}{4} - z, y + \frac{3}{4}, x + \frac{1}{4}), \\ &6 : (\frac{1}{4} - y, x + \frac{3}{4}, z + \frac{1}{4}), 7 : (y + \frac{1}{4}, \frac{1}{4} - x, z + \frac{3}{4}), 8 : (x + \frac{1}{2}, \frac{1}{2} - y, -z), 9 : (-x, y + \frac{1}{2}, \frac{1}{2} - z), 10 : (\frac{1}{2} - x, -y, z + \frac{1}{2}), \\ &11 : (y + \frac{3}{4}, x + \frac{1}{4}, \frac{1}{4} - z), 12 : (\frac{3}{4} - y, \frac{3}{4} - x, \frac{3}{4} - z), 13 : (\frac{1}{4} - x, z + \frac{3}{4}, y + \frac{1}{4}), 14 : (\frac{3}{4} - x, \frac{3}{4} - z, \frac{3}{4} - y), 15 : (z + \frac{1}{4}, \frac{1}{4} - y, x + \frac{3}{4}), \\ &16 : (\frac{3}{4} - z, \frac{3}{4} - y, \frac{3}{4} - x), 17 : (z, x, y), 18 : (y, z, x), 19 : (-y, z + \frac{1}{2}, \frac{1}{2} - x), 20 : (\frac{1}{2} - z, -x, y + \frac{1}{2}), 21 : (\frac{1}{2} - y, -z, x + \frac{1}{2}), \\ &22 : (z + \frac{1}{2}, \frac{1}{2} - x, -y), 23 : (y + \frac{1}{2}, \frac{1}{2} - z, -x), 24 : (-z, x + \frac{1}{2}, \frac{1}{2} - y). \end{aligned}$$

The lower SG is SG 19 when the preserved operations are: **(sub-SG label is 1) 1, 8, 9, 10.**

$$\text{The transformation is: } (\mathbf{a}_{19}, \mathbf{b}_{19}, \mathbf{c}_{19}) = (\mathbf{a}_{213}, \mathbf{b}_{213}, \mathbf{c}_{213}) \begin{pmatrix} -1 & 0 & 0 \\ 0 & 0 & 1 \\ 0 & 1 & 0 \end{pmatrix}, \overrightarrow{O_{213}O_{19}} = \frac{1}{4}\mathbf{a}_{19} + \left(-\frac{1}{4}\right)\mathbf{b}_{19} + \left(\frac{3}{4}\right)\mathbf{c}_{19}$$

The reduction of higher dimensional irrep:

$$O : T_1 \rightarrow B_1 + B_3 + B_2 \text{ of } D_2.$$

$$O : T_2 \rightarrow B_1 + B_3 + B_2 \text{ of } D_2.$$

The correspondences of irreps at HSPs from original SG to lowered SG:

$$n_{GM5}^{19} = n_{GM6}^{213} + n_{GM7}^{213} + 2n_{GM8}^{213} n_{X4}^{19} = n_{X7}^{213} n_{X5}^{19} = n_{X7}^{213} n_{X3}^{19} = n_{X3}^{213} + n_{X5}^{213} n_{X2}^{19} = n_{X4}^{213} + n_{X6}^{213} n_{S5}^{19} = n_{M6}^{213} + n_{M7}^{213} n_{R3}^{19} =$$

$$n_{R4}^{213} + n_{R5}^{213} + 2n_{R6}^{213} n_{R2}^{19} = n_{R7}^{213} + n_{R8}^{213} n_{R4}^{19} = n_{R7}^{213} + n_{R8}^{213} n_{R5}^{19} = n_{R7}^{213} + n_{R8}^{213} n_{J5}^{19} = n_{M6}^{213} + n_{M7}^{213} n_{Z1}^{19} = n_{X4}^{213} + n_{X6}^{213} n_{Z5}^{19} =$$

$$n_{X7}^{213} n_{Z3}^{19} = n_{X7}^{213} n_{Z2}^{19} = n_{X3}^{213} + n_{X5}^{213} n_{T5}^{19} = n_{M6}^{213} + n_{M7}^{213} n_{Y3}^{19} = n_{X7}^{213} n_{Y2}^{19} = n_{X4}^{213} + n_{X6}^{213} n_{Y4}^{19} = n_{X7}^{213} n_{Y5}^{19} = n_{X3}^{213} + n_{X5}^{213}$$

The lower SG is SG 20 when the preserved operations are: **(sub-SG label is 2) 1, 8, 13, 14.**

$$\text{The transformation is: } (\mathbf{a}_{20}, \mathbf{b}_{20}, \mathbf{c}_{20}) = (\mathbf{a}_{213}, \mathbf{b}_{213}, \mathbf{c}_{213}) \begin{pmatrix} 0 & 0 & -1 \\ -1 & -1 & 0 \\ -1 & 1 & 0 \end{pmatrix}, \overrightarrow{O_{213}O_{20}} = \frac{1}{8}\mathbf{a}_{20} + \left(\frac{1}{8}\right)\mathbf{b}_{20} + \left(\frac{3}{8}\right)\mathbf{c}_{20}$$

The reduction of higher dimensional irrep:

$$O : T_1 \rightarrow B_1 + B_2 + B_3 \text{ of } D_2.$$

$$O : T_2 \rightarrow A_1 + B_2 + B_3 \text{ of } D_2.$$

The correspondences of irreps at HSPs from original SG to lowered SG:

$$\begin{aligned} n_{GM5}^{20} &= n_{GM6}^{213} + n_{GM7}^{213} + 2n_{GM8}^{213} & n_{Y5}^{20} &= n_{M6}^{213} + n_{M7}^{213} & n_{S4}^{20} &= n_{X4}^{213} + n_{X6}^{213} + n_{X7}^{213} & n_{S3}^{20} &= n_{X3}^{213} + n_{X5}^{213} + n_{X7}^{213} & n_{Z5}^{20} &= n_{X7}^{213} \\ n_{Z4}^{20} &= n_{X5}^{213} + n_{X6}^{213} & n_{Z2}^{20} &= n_{X3}^{213} + n_{X4}^{213} & n_{Z3}^{20} &= n_{X7}^{213} & n_{T5}^{20} &= n_{R7}^{213} + n_{R8}^{213} & n_{T4}^{20} &= n_{R4}^{213} + n_{R6}^{213} + n_{R7}^{213} & n_{T2}^{20} &= n_{R5}^{213} + n_{R6}^{213} + n_{R8}^{213} \\ n_{T3}^{20} &= n_{R7}^{213} + n_{R8}^{213} & n_{R4}^{20} &= n_{M6}^{213} + n_{M7}^{213} & n_{R3}^{20} &= n_{M6}^{213} + n_{M7}^{213} \end{aligned}$$

The lower SG is SG 20 when the preserved operations are: **(sub-SG label is 3) 1, 9, 16, 15.**

The transformation is:  $(\mathbf{a}_{20}, \mathbf{b}_{20}, \mathbf{c}_{20}) = (\mathbf{a}_{213}, \mathbf{b}_{213}, \mathbf{c}_{213}) \begin{pmatrix} -1 & -1 & 0 \\ 0 & 0 & 1 \\ -1 & 1 & 0 \end{pmatrix}, \overrightarrow{O_{213}O_{20}} = \frac{1}{8}\mathbf{a}_{20} + (\frac{3}{8})\mathbf{b}_{20} + (\frac{1}{8})\mathbf{c}_{20}$

The reduction of higher dimensional irrep:

$$O : T_1 \rightarrow B_1 + B_2 + B_3 \quad \text{of} \quad D_2.$$

$$O : T_2 \rightarrow A_1 + B_2 + B_3 \quad \text{of} \quad D_2.$$

The correspondences of irreps at HSPs from original SG to lowered SG:

$$\begin{aligned} n_{GM5}^{20} &= n_{GM6}^{213} + n_{GM7}^{213} + 2n_{GM8}^{213} & n_{Y5}^{20} &= n_{M6}^{213} + n_{M7}^{213} & n_{S4}^{20} &= n_{X3}^{213} + n_{X5}^{213} + n_{X7}^{213} & n_{S3}^{20} &= n_{X4}^{213} + n_{X6}^{213} + n_{X7}^{213} & n_{Z5}^{20} &= n_{X7}^{213} \\ n_{Z4}^{20} &= n_{X3}^{213} + n_{X6}^{213} & n_{Z2}^{20} &= n_{X5}^{213} + n_{X6}^{213} & n_{Z3}^{20} &= n_{X7}^{213} & n_{T5}^{20} &= n_{R7}^{213} + n_{R8}^{213} & n_{T4}^{20} &= n_{R5}^{213} + n_{R6}^{213} + n_{R8}^{213} & n_{T2}^{20} &= n_{R4}^{213} + n_{R6}^{213} + n_{R7}^{213} \\ n_{T3}^{20} &= n_{R7}^{213} + n_{R8}^{213} & n_{R4}^{20} &= n_{M6}^{213} + n_{M7}^{213} & n_{R3}^{20} &= n_{M6}^{213} + n_{M7}^{213} \end{aligned}$$

The lower SG is SG 20 when the preserved operations are: **(sub-SG label is 4) 1, 10, 11, 12.**

The transformation is:  $(\mathbf{a}_{20}, \mathbf{b}_{20}, \mathbf{c}_{20}) = (\mathbf{a}_{213}, \mathbf{b}_{213}, \mathbf{c}_{213}) \begin{pmatrix} 1 & -1 & 0 \\ -1 & -1 & 0 \\ 0 & 0 & -1 \end{pmatrix}, \overrightarrow{O_{213}O_{20}} = \frac{3}{8}\mathbf{a}_{20} + (\frac{1}{8})\mathbf{b}_{20} + (\frac{1}{8})\mathbf{c}_{20}$

The reduction of higher dimensional irrep:

$$O : T_1 \rightarrow B_1 + B_2 + B_3 \quad \text{of} \quad D_2.$$

$$O : T_2 \rightarrow A_1 + B_2 + B_3 \quad \text{of} \quad D_2.$$

The correspondences of irreps at HSPs from original SG to lowered SG:

$$\begin{aligned} n_{GM5}^{20} &= n_{GM6}^{213} + n_{GM7}^{213} + 2n_{GM8}^{213} & n_{Y5}^{20} &= n_{M6}^{213} + n_{M7}^{213} & n_{S4}^{20} &= n_{X3}^{213} + n_{X5}^{213} + n_{X7}^{213} & n_{S3}^{20} &= n_{X3}^{213} + n_{X5}^{213} + n_{X7}^{213} & n_{Z5}^{20} &= n_{X7}^{213} \\ n_{Z4}^{20} &= n_{X3}^{213} + n_{X6}^{213} & n_{Z2}^{20} &= n_{X3}^{213} + n_{X4}^{213} & n_{Z3}^{20} &= n_{X7}^{213} & n_{T5}^{20} &= n_{R7}^{213} + n_{R8}^{213} & n_{T4}^{20} &= n_{R4}^{213} + n_{R6}^{213} + n_{R7}^{213} & n_{T2}^{20} &= n_{R5}^{213} + n_{R6}^{213} + n_{R8}^{213} \\ n_{T3}^{20} &= n_{R7}^{213} + n_{R8}^{213} & n_{R4}^{20} &= n_{M6}^{213} + n_{M7}^{213} & n_{R3}^{20} &= n_{M6}^{213} + n_{M7}^{213} \end{aligned}$$

The lower SG is SG 76 when the preserved operations are: **(sub-SG label is 5) 1, 6, 7, 10.**

The transformation is:  $(\mathbf{a}_{76}, \mathbf{b}_{76}, \mathbf{c}_{76}) = (\mathbf{a}_{213}, \mathbf{b}_{213}, \mathbf{c}_{213}) \begin{pmatrix} -1 & 0 & 0 \\ 0 & 1 & 0 \\ 0 & 0 & -1 \end{pmatrix}, \overrightarrow{O_{213}O_{76}} = \frac{3}{4}\mathbf{a}_{76}$

The reduction of higher dimensional irrep:

$$O : T_1 \rightarrow A + {}^2E + {}^1E \quad \text{of} \quad C_4.$$

$$O : T_2 \rightarrow {}^2E + B + {}^1E \quad \text{of} \quad C_4.$$

The correspondences of irreps at HSPs from original SG to lowered SG:

$$\begin{aligned} n_{GM5}^{76} &= n_{GM7}^{213} + n_{GM8}^{213} & n_{GM7}^{76} &= n_{GM7}^{213} + n_{GM8}^{213} & n_{GM8}^{76} &= n_{GM6}^{213} + n_{GM8}^{213} & n_{GM6}^{76} &= n_{GM6}^{213} + n_{GM8}^{213} & n_{X4}^{76} &= n_{X3}^{213} + n_{X5}^{213} + n_{X7}^{213} \\ n_{X3}^{76} &= n_{X4}^{213} + n_{X6}^{213} + n_{X7}^{213} & n_{M5}^{76} &= n_{M7}^{213} & n_{M7}^{76} &= n_{M6}^{213} & n_{M8}^{76} &= n_{M7}^{213} & n_{M6}^{76} &= n_{M6}^{213} & n_{A6}^{76} &= n_{R7}^{213} + n_{R8}^{213} & n_{A7}^{76} &= n_{R5}^{213} + n_{R6}^{213} + n_{R7}^{213} \\ n_{A8}^{76} &= n_{R4}^{213} + n_{R6}^{213} + n_{R8}^{213} & n_{A5}^{76} &= n_{R7}^{213} + n_{R8}^{213} & n_{R4}^{76} &= n_{M6}^{213} + n_{M7}^{213} & n_{R3}^{76} &= n_{M6}^{213} + n_{M7}^{213} & n_{Z8}^{76} &= n_{X7}^{213} & n_{Z5}^{76} &= n_{X4}^{213} + n_{X5}^{213} & n_{Z6}^{76} &= n_{X3}^{213} + n_{X6}^{213} \\ n_{X3}^{76} + n_{X6}^{76} &= n_{X7}^{213} \end{aligned}$$

The lower SG is SG 76 when the preserved operations are: **(sub-SG label is 6) 1, 2, 3, 8.**

The transformation is:  $(\mathbf{a}_{76}, \mathbf{b}_{76}, \mathbf{c}_{76}) = (\mathbf{a}_{213}, \mathbf{b}_{213}, \mathbf{c}_{213}) \begin{pmatrix} 0 & 0 & -1 \\ -1 & 0 & 0 \\ 0 & 1 & 0 \end{pmatrix}, \overrightarrow{O_{213}O_{76}} = \frac{3}{4}\mathbf{a}_{76} + \mathbf{b}_{76}$

The reduction of higher dimensional irrep:

$$O : T_1 \rightarrow A + {}^2E + {}^1E \quad \text{of} \quad C_4.$$

$$O : T_2 \rightarrow {}^2E + B + {}^1E \quad \text{of} \quad C_4.$$

The correspondences of irreps at HSPs from original SG to lowered SG:

$$\begin{aligned} n_{GM5}^{76} &= n_{GM7}^{213} + n_{GM8}^{213} & n_{GM7}^{76} &= n_{GM7}^{213} + n_{GM8}^{213} & n_{GM8}^{76} &= n_{GM6}^{213} + n_{GM8}^{213} & n_{GM6}^{76} &= n_{GM6}^{213} + n_{GM8}^{213} & n_{X4}^{76} &= n_{X3}^{213} + n_{X5}^{213} + n_{X7}^{213} \\ n_{X3}^{76} &= n_{X4}^{213} + n_{X6}^{213} + n_{X7}^{213} & n_{M5}^{76} &= n_{M7}^{213} & n_{M7}^{76} &= n_{M6}^{213} & n_{M8}^{76} &= n_{M7}^{213} & n_{M6}^{76} &= n_{M6}^{213} & n_{A6}^{76} &= n_{R7}^{213} + n_{R8}^{213} & n_{A7}^{76} &= n_{R5}^{213} + n_{R6}^{213} + n_{R7}^{213} \\ n_{A8}^{76} &= n_{R4}^{213} + n_{R6}^{213} + n_{R8}^{213} & n_{A5}^{76} &= n_{R7}^{213} + n_{R8}^{213} & n_{R4}^{76} &= n_{M6}^{213} + n_{M7}^{213} & n_{R3}^{76} &= n_{M6}^{213} + n_{M7}^{213} & n_{Z8}^{76} &= n_{X7}^{213} & n_{Z5}^{76} &= n_{X4}^{213} + n_{X5}^{213} & n_{Z6}^{76} &= n_{X3}^{213} + n_{X6}^{213} \\ n_{X3}^{76} + n_{X6}^{76} &= n_{X7}^{213} \end{aligned}$$

The lower SG is SG 76 when the preserved operations are: **(sub-SG label is 7) 1, 4, 5, 9.**

The transformation is:  $(\mathbf{a}_{76}, \mathbf{b}_{76}, \mathbf{c}_{76}) = (\mathbf{a}_{213}, \mathbf{b}_{213}, \mathbf{c}_{213}) \begin{pmatrix} -1 & 0 & 0 \\ 0 & 0 & -1 \\ 0 & -1 & 0 \end{pmatrix}, \overrightarrow{O_{213}O_{76}} = \frac{1}{2}\mathbf{a}_{76} + (\frac{1}{4})\mathbf{b}_{76}$

The reduction of higher dimensional irrep:

$O : T_1 \rightarrow A + {}^2E + {}^1E$  of  $C_4$ .

$O : T_2 \rightarrow {}^2E + B + {}^1E$  of  $C_4$ .

The correspondences of irreps at HSPs from original SG to lowered SG:

$$\begin{aligned} n_{GM5}^{76} &= n_{GM7}^{213} + n_{GM8}^{213} & n_{GM7}^{76} &= n_{GM7}^{213} + n_{GM8}^{213} & n_{GM8}^{76} &= n_{GM6}^{213} + n_{GM8}^{213} & n_{GM6}^{76} &= n_{GM6}^{213} + n_{GM8}^{213} & n_{X4}^{76} &= n_{X4}^{213} + n_{X6}^{213} + n_{X7}^{213} \\ n_{X3}^{76} &= n_{X3}^{213} + n_{X5}^{213} + n_{X7}^{213} & n_{M5}^{76} &= n_{M6}^{213} n_{M7}^{76} = n_{M7}^{213} n_{M8}^{76} = n_{M6}^{213} n_{M6}^{76} = n_{M7}^{213} n_{A6}^{76} = n_{R7}^{213} + n_{R8}^{213} & n_{A7}^{76} &= n_{R4}^{213} + n_{R6}^{213} + n_{R8}^{213} \\ n_{A8}^{76} &= n_{R5}^{213} + n_{R6}^{213} + n_{R7}^{213} & n_{A5}^{76} &= n_{R7}^{213} + n_{R8}^{213} & n_{R4}^{76} &= n_{M6}^{213} + n_{M7}^{213} & n_{R3}^{76} &= n_{M6}^{213} + n_{M7}^{213} & n_{Z8}^{76} &= n_{X7}^{213} n_{Z5}^{76} = n_{X4}^{213} + n_{X5}^{213} n_{Z6}^{76} = \\ n_{X3}^{213} + n_{X6}^{213} & n_{Z7}^{76} = n_{X7}^{213} \end{aligned}$$

The lower SG is SG 92 when the preserved operations are: **(sub-SG label is 8)** 1, 6, 7, 10, 8, 9, 11, 12.

The transformation is:  $(\mathbf{a}_{92}, \mathbf{b}_{92}, \mathbf{c}_{92}) = (\mathbf{a}_{213}, \mathbf{b}_{213}, \mathbf{c}_{213}) \begin{pmatrix} 1 & 0 & 0 \\ 0 & -1 & 0 \\ 0 & 0 & -1 \end{pmatrix}, \overrightarrow{O_{213}O_{92}} = \frac{3}{4}\mathbf{a}_{92} + (\frac{1}{8})\mathbf{c}_{92}$

The reduction of higher dimensional irrep:

$O : E \rightarrow A_1 + B_1$  of  $D_4$ .

The correspondences of irreps at HSPs from original SG to lowered SG:

$$\begin{aligned} n_{GM6}^{92} &= n_{GM7}^{213} + n_{GM8}^{213} & n_{GM7}^{92} &= n_{GM6}^{213} + n_{GM8}^{213} & n_{X3}^{92} &= n_{X7}^{213} n_{X4}^{92} = n_{X7}^{213} n_{X2}^{92} = n_{X4}^{213} + n_{X6}^{213} & n_{X5}^{92} &= n_{X3}^{213} + n_{X5}^{213} & n_{M6}^{92} &= \\ n_{M7}^{92} &= n_{M6}^{213} n_{M7}^{92} = n_{R5}^{213} + n_{R6}^{213} & n_{A6}^{92} &= n_{R7}^{213} n_{A5}^{92} = n_{R4}^{213} + n_{R6}^{213} & n_{A3}^{92} &= n_{R8}^{213} n_{A7}^{92} = n_{R7}^{213} + n_{R8}^{213} & n_{R5}^{92} &= n_{M6}^{213} + n_{M7}^{213} \\ n_{Z6}^{92} &= n_{X5}^{213} n_{Z4}^{92} = n_{X4}^{213} n_{Z3}^{92} = n_{X3}^{213} n_{Z5}^{92} = n_{X6}^{213} n_{Z7}^{92} = n_{X7}^{213} \end{aligned}$$

The lower SG is SG 92 when the preserved operations are: **(sub-SG label is 9)** 1, 2, 3, 8, 9, 10, 13, 14.

The transformation is:  $(\mathbf{a}_{92}, \mathbf{b}_{92}, \mathbf{c}_{92}) = (\mathbf{a}_{213}, \mathbf{b}_{213}, \mathbf{c}_{213}) \begin{pmatrix} 0 & 0 & -1 \\ 0 & 1 & 0 \\ 1 & 0 & 0 \end{pmatrix}, \overrightarrow{O_{213}O_{92}} = \frac{1}{2}\mathbf{a}_{92} + (\frac{1}{4})\mathbf{b}_{92} + (-\frac{1}{8})\mathbf{c}_{92}$

The reduction of higher dimensional irrep:

$O : E \rightarrow A_1 + B_1$  of  $D_4$ .

The correspondences of irreps at HSPs from original SG to lowered SG:

$$\begin{aligned} n_{GM6}^{92} &= n_{GM7}^{213} + n_{GM8}^{213} & n_{GM7}^{92} &= n_{GM6}^{213} + n_{GM8}^{213} & n_{X3}^{92} &= n_{X7}^{213} n_{X4}^{92} = n_{X7}^{213} n_{X2}^{92} = n_{X4}^{213} + n_{X6}^{213} & n_{X5}^{92} &= n_{X3}^{213} + n_{X5}^{213} & n_{M6}^{92} &= \\ n_{M7}^{92} &= n_{M6}^{213} n_{M7}^{92} = n_{R5}^{213} + n_{R6}^{213} & n_{A6}^{92} &= n_{R7}^{213} n_{A5}^{92} = n_{R4}^{213} + n_{R6}^{213} & n_{A3}^{92} &= n_{R8}^{213} n_{A7}^{92} = n_{R7}^{213} + n_{R8}^{213} & n_{R5}^{92} &= n_{M6}^{213} + n_{M7}^{213} \\ n_{Z6}^{92} &= n_{X5}^{213} n_{Z4}^{92} = n_{X4}^{213} n_{Z3}^{92} = n_{X3}^{213} n_{Z5}^{92} = n_{X6}^{213} n_{Z7}^{92} = n_{X7}^{213} \end{aligned}$$

The lower SG is SG 92 when the preserved operations are: **(sub-SG label is 10)** 1, 4, 5, 9, 10, 8, 16, 15.

The transformation is:  $(\mathbf{a}_{92}, \mathbf{b}_{92}, \mathbf{c}_{92}) = (\mathbf{a}_{213}, \mathbf{b}_{213}, \mathbf{c}_{213}) \begin{pmatrix} 1 & 0 & 0 \\ 0 & 0 & 1 \\ 0 & -1 & 0 \end{pmatrix}, \overrightarrow{O_{213}O_{92}} = \frac{1}{2}\mathbf{a}_{92} + (-\frac{1}{4})\mathbf{b}_{92} + (\frac{3}{8})\mathbf{c}_{92}$

The reduction of higher dimensional irrep:

$O : E \rightarrow A_1 + B_1$  of  $D_4$ .

The correspondences of irreps at HSPs from original SG to lowered SG:

$$\begin{aligned} n_{GM6}^{92} &= n_{GM7}^{213} + n_{GM8}^{213} & n_{GM7}^{92} &= n_{GM6}^{213} + n_{GM8}^{213} & n_{X3}^{92} &= n_{X7}^{213} n_{X4}^{92} = n_{X7}^{213} n_{X2}^{92} = n_{X4}^{213} + n_{X6}^{213} & n_{X5}^{92} &= n_{X3}^{213} + n_{X5}^{213} & n_{M6}^{92} &= \\ n_{M7}^{92} &= n_{M6}^{213} n_{M7}^{92} = n_{R5}^{213} + n_{R6}^{213} & n_{A6}^{92} &= n_{R7}^{213} n_{A5}^{92} = n_{R4}^{213} + n_{R6}^{213} & n_{A3}^{92} &= n_{R8}^{213} n_{A7}^{92} = n_{R7}^{213} + n_{R8}^{213} & n_{R5}^{92} &= n_{M6}^{213} + n_{M7}^{213} \\ n_{Z6}^{92} &= n_{X5}^{213} n_{Z4}^{92} = n_{X4}^{213} n_{Z3}^{92} = n_{X3}^{213} n_{Z5}^{92} = n_{X6}^{213} n_{Z7}^{92} = n_{X7}^{213} \end{aligned}$$

The lower SG is SG 146 when the preserved operations are: **(sub-SG label is 11)** 1, 17, 18.

The transformation is:  $(\mathbf{a}_{146}, \mathbf{b}_{146}, \mathbf{c}_{146}) = (\mathbf{a}_{213}, \mathbf{b}_{213}, \mathbf{c}_{213}) \begin{pmatrix} 0 & 1 & 0 \\ 0 & 0 & 1 \\ 1 & 0 & 0 \end{pmatrix}, \overrightarrow{O_{213}O_{146}} = -\frac{1}{3}\mathbf{a}_{146} + (\frac{2}{3})\mathbf{b}_{146} + (-\frac{1}{3})\mathbf{c}_{146}$

The reduction of higher dimensional irrep:

$O : T_1 \rightarrow A + {}^2E + {}^1E$  of  $C_3$ .

$O : T_2 \rightarrow A + {}^2E + {}^1E$  of  $C_3$ .

The correspondences of irreps at HSPs from original SG to lowered SG:

$$\begin{aligned} n_{GM4}^{146} &= 2n_{GM8}^{213} & n_{GM6}^{146} &= n_{GM6}^{213} + n_{GM7}^{213} + n_{GM8}^{213} & n_{GM5}^{146} &= n_{GM6}^{213} + n_{GM7}^{213} + n_{GM8}^{213} & n_{L2}^{146} &= n_{X3}^{213} + n_{X4}^{213} + n_{X5}^{213} + n_{X6}^{213} + 2n_{X7}^{213} \\ n_{F2}^{146} &= 2n_{M6}^{213} + 2n_{M7}^{213} & n_{T4}^{146} &= n_{R4}^{213} + n_{R5}^{213} + n_{R7}^{213} + n_{R8}^{213} & n_{T6}^{146} &= n_{R6}^{213} + n_{R7}^{213} + n_{R8}^{213} & n_{T5}^{146} &= n_{R6}^{213} + n_{R7}^{213} + n_{R8}^{213} \end{aligned}$$

The lower SG is SG 146 when the preserved operations are: **(sub-SG label is 12)** 1, 24, 23.

The transformation is:  $(\mathbf{a}_{146}, \mathbf{b}_{146}, \mathbf{c}_{146}) = (\mathbf{a}_{213}, \mathbf{b}_{213}, \mathbf{c}_{213}) \begin{pmatrix} 0 & -1 & 0 \\ 0 & 0 & -1 \\ 1 & 0 & 0 \end{pmatrix}, \overrightarrow{O_{213}O_{146}} = -\frac{1}{6}\mathbf{a}_{146} + (\frac{5}{6})\mathbf{b}_{146} + (-\frac{2}{3})\mathbf{c}_{146}$

The reduction of higher dimensional irrep:

$$O : T_1 \rightarrow A + {}^2E + {}^1E \text{ of } C_3.$$

$$O : T_2 \rightarrow A + {}^2E + {}^1E \text{ of } C_3.$$

The correspondences of irreps at HSPs from original SG to lowered SG:

$$\begin{aligned} n_{GM4}^{146} &= 2n_{GM8}^{213} & n_{GM6}^{146} &= n_{GM6}^{213} + n_{GM7}^{213} + n_{GM8}^{213} & n_{GM5}^{146} &= n_{GM6}^{213} + n_{GM7}^{213} + n_{GM8}^{213} & n_{L2}^{146} &= n_{X3}^{213} + n_{X4}^{213} + n_{X5}^{213} + n_{X6}^{213} + 2n_{X7}^{213} \\ n_{F2}^{146} &= 2n_{M6}^{213} + 2n_{M7}^{213} & n_{T4}^{146} &= n_{R4}^{213} + n_{R5}^{213} + n_{R7}^{213} + n_{R8}^{213} & n_{T6}^{146} &= n_{R6}^{213} + n_{R7}^{213} + n_{R8}^{213} & n_{T5}^{146} &= n_{R6}^{213} + n_{R7}^{213} + n_{R8}^{213} \end{aligned}$$

The lower SG is SG 146 when the preserved operations are: (**sub-SG label is 13**) 1, 20, 19.

The transformation is:  $(\mathbf{a}_{146}, \mathbf{b}_{146}, \mathbf{c}_{146}) = (\mathbf{a}_{213}, \mathbf{b}_{213}, \mathbf{c}_{213}) \begin{pmatrix} 0 & 0 & -1 \\ 0 & 1 & 0 \\ 1 & 0 & 0 \end{pmatrix}, \overrightarrow{O_{213}O_{146}} = \frac{1}{2}\mathbf{b}_{146} + (-\frac{1}{2})\mathbf{c}_{146}$

The reduction of higher dimensional irrep:

$$O : T_1 \rightarrow A + {}^2E + {}^1E \text{ of } C_3.$$

$$O : T_2 \rightarrow A + {}^2E + {}^1E \text{ of } C_3.$$

The correspondences of irreps at HSPs from original SG to lowered SG:

$$\begin{aligned} n_{GM4}^{146} &= 2n_{GM8}^{213} & n_{GM6}^{146} &= n_{GM6}^{213} + n_{GM7}^{213} + n_{GM8}^{213} & n_{GM5}^{146} &= n_{GM6}^{213} + n_{GM7}^{213} + n_{GM8}^{213} & n_{L2}^{146} &= n_{X3}^{213} + n_{X4}^{213} + n_{X5}^{213} + n_{X6}^{213} + 2n_{X7}^{213} \\ n_{F2}^{146} &= 2n_{M6}^{213} + 2n_{M7}^{213} & n_{T4}^{146} &= n_{R4}^{213} + n_{R5}^{213} + n_{R7}^{213} + n_{R8}^{213} & n_{T6}^{146} &= n_{R6}^{213} + n_{R7}^{213} + n_{R8}^{213} & n_{T5}^{146} &= n_{R6}^{213} + n_{R7}^{213} + n_{R8}^{213} \end{aligned}$$

The lower SG is SG 146 when the preserved operations are: (**sub-SG label is 14**) 1, 22, 21.

The transformation is:  $(\mathbf{a}_{146}, \mathbf{b}_{146}, \mathbf{c}_{146}) = (\mathbf{a}_{213}, \mathbf{b}_{213}, \mathbf{c}_{213}) \begin{pmatrix} -1 & 0 & 0 \\ 0 & 1 & 0 \\ 0 & 0 & -1 \end{pmatrix}, \overrightarrow{O_{213}O_{146}} = -\frac{2}{3}\mathbf{a}_{146} + (\frac{5}{6})\mathbf{b}_{146} + (-\frac{1}{6})\mathbf{c}_{146}$

The reduction of higher dimensional irrep:

$$O : T_1 \rightarrow A + {}^2E + {}^1E \text{ of } C_3.$$

$$O : T_2 \rightarrow A + {}^2E + {}^1E \text{ of } C_3.$$

The correspondences of irreps at HSPs from original SG to lowered SG:

$$\begin{aligned} n_{GM4}^{146} &= 2n_{GM8}^{213} & n_{GM6}^{146} &= n_{GM6}^{213} + n_{GM7}^{213} + n_{GM8}^{213} & n_{GM5}^{146} &= n_{GM6}^{213} + n_{GM7}^{213} + n_{GM8}^{213} & n_{L2}^{146} &= n_{X3}^{213} + n_{X4}^{213} + n_{X5}^{213} + n_{X6}^{213} + 2n_{X7}^{213} \\ n_{F2}^{146} &= 2n_{M6}^{213} + 2n_{M7}^{213} & n_{T4}^{146} &= n_{R4}^{213} + n_{R5}^{213} + n_{R7}^{213} + n_{R8}^{213} & n_{T6}^{146} &= n_{R6}^{213} + n_{R7}^{213} + n_{R8}^{213} & n_{T5}^{146} &= n_{R6}^{213} + n_{R7}^{213} + n_{R8}^{213} \end{aligned}$$

The lower SG is SG 198 when the preserved operations are: (**sub-SG label is 15**) 1, 8, 9, 10, 17, 24, 20, 22, 18, 23, 19, 21.

The transformation is:  $(\mathbf{a}_{198}, \mathbf{b}_{198}, \mathbf{c}_{198}) = (\mathbf{a}_{213}, \mathbf{b}_{213}, \mathbf{c}_{213}) \begin{pmatrix} 0 & 0 & -1 \\ 1 & 0 & 0 \\ 0 & -1 & 0 \end{pmatrix}, \overrightarrow{O_{213}O_{198}} = -\frac{1}{2}\mathbf{c}_{198}$

The reduction of higher dimensional irrep:

$$O : E \rightarrow {}^1E + {}^2E \text{ of } T.$$

The correspondences of irreps at HSPs from original SG to lowered SG:

$$\begin{aligned} n_{GM6}^{198} &= n_{GM8}^{213} & n_{GM7}^{198} &= n_{GM8}^{213} & n_{GM5}^{198} &= n_{GM6}^{213} + n_{GM7}^{213} & n_{X3}^{198} &= n_{X7}^{213} & n_{X4}^{198} &= n_{X7}^{213} & n_{X5}^{198} &= n_{X3}^{213} + n_{X5}^{213} & n_{X2}^{198} &= n_{X4}^{213} + n_{X6}^{213} \\ n_{M5}^{198} &= n_{M6}^{213} + n_{M7}^{213} & n_{R4}^{198} &= n_{R4}^{213} & n_{R5}^{198} &= n_{R6}^{213} & n_{R6}^{198} &= n_{R6}^{213} & n_{R7}^{198} &= n_{R7}^{213} & n_{R8}^{198} &= n_{R8}^{213} \end{aligned}$$

### 111. Lowered SGs by higher-dimensional irreps of pairings in SG 214

The representative operations of SG/T for SG 214:

$$\begin{aligned} 1 : (x, y, z), & 2 : (x + \frac{1}{4}, \frac{1}{4} - z, y + \frac{3}{4}), & 3 : (x + \frac{3}{4}, z + \frac{1}{4}, \frac{1}{4} - y), & 4 : (z + \frac{3}{4}, y + \frac{1}{4}, \frac{1}{4} - x), & 5 : (\frac{1}{4} - z, y + \frac{3}{4}, x + \frac{1}{4}), \\ 6 : (\frac{1}{4} - y, x + \frac{3}{4}, z + \frac{1}{4}), & 7 : (y + \frac{1}{4}, \frac{1}{4} - x, z + \frac{3}{4}), & 8 : (x, -y, \frac{1}{2} - z), & 9 : (\frac{1}{2} - x, y, -z), & 10 : (-x, \frac{1}{2} - y, z), \\ 11 : (y + \frac{3}{4}, x + \frac{1}{4}, \frac{1}{4} - z), & 12 : (\frac{1}{4} - y, \frac{1}{4} - x, \frac{1}{4} - z), & 13 : (\frac{1}{4} - x, z + \frac{3}{4}, y + \frac{1}{4}), & 14 : (\frac{1}{4} - x, \frac{1}{4} - z, \frac{1}{4} - y), \\ 15 : (z + \frac{1}{4}, \frac{1}{4} - y, x + \frac{3}{4}), & 16 : (\frac{1}{4} - z, \frac{1}{4} - y, \frac{1}{4} - x), & 17 : (z, x, y), & 18 : (y, z, x), & 19 : (\frac{1}{2} - y, z, -x), & 20 : (-z, \frac{1}{2} - x, y), \\ 21 : (-y, \frac{1}{2} - z, x), & 22 : (z, -x, \frac{1}{2} - y), & 23 : (y, -z, \frac{1}{2} - x), & 24 : (\frac{1}{2} - z, x, -y). \end{aligned}$$

The lower SG is SG 24 when the preserved operations are: **(sub-SG label is 1) 1, 8, 9, 10.**

$$\text{The transformation is: } (\mathbf{a}_{24}, \mathbf{b}_{24}, \mathbf{c}_{24}) = (\mathbf{a}_{214}, \mathbf{b}_{214}, \mathbf{c}_{214}) \begin{pmatrix} 0 & 0 & 1 \\ 1 & 0 & 0 \\ 0 & 1 & 0 \end{pmatrix}, \overrightarrow{O_{214}O_{24}} = \frac{1}{2}\mathbf{c}_{24}$$

The reduction of higher dimensional irrep:

$$O : T_1 \rightarrow B_1 + B_2 + B_3 \text{ of } D_2.$$

$$O : T_2 \rightarrow B_1 + B_2 + B_3 \text{ of } D_2.$$

The correspondences of irreps at HSPs from original SG to lowered SG:

$$\begin{aligned} n_{GM5}^{24} &= n_{GM6}^{214} + n_{GM7}^{214} + 2n_{GM8}^{214} & n_{X5}^{24} &= n_{H6}^{214} + n_{H7}^{214} + 2n_{H8}^{214} & n_{T3}^{24} &= n_{N5}^{214} & n_{T4}^{24} &= n_{N5}^{214} & n_{W3}^{24} &= n_{P4}^{214} + n_{P5}^{214} + n_{P6}^{214} & n_{W2}^{24} &= \\ n_{P7}^{214} n_{W4}^{24} &= n_{P7}^{214} n_{W5}^{24} = n_{P7}^{214} n_{R3}^{24} &= n_{N5}^{214} n_{R4}^{24} &= n_{N5}^{214} n_{S4}^{24} &= n_{N5}^{214} n_{S3}^{24} &= n_{N5}^{214} \end{aligned}$$

The lower SG is SG 22 when the preserved operations are: **(sub-SG label is 2) 1, 8, 13, 14.**

$$\text{The transformation is: } (\mathbf{a}_{22}, \mathbf{b}_{22}, \mathbf{c}_{22}) = (\mathbf{a}_{214}, \mathbf{b}_{214}, \mathbf{c}_{214}) \begin{pmatrix} 0 & 1 & 0 \\ -1 & 0 & 1 \\ 1 & 0 & 1 \end{pmatrix}, \overrightarrow{O_{214}O_{22}} = \frac{1}{8}\mathbf{a}_{22} + (-\frac{3}{8})\mathbf{b}_{22} + (\frac{1}{8})\mathbf{c}_{22}$$

The reduction of higher dimensional irrep:

$$O : T_1 \rightarrow B_1 + B_2 + B_3 \text{ of } D_2.$$

$$O : T_2 \rightarrow A_1 + B_1 + B_3 \text{ of } D_2.$$

The correspondences of irreps at HSPs from original SG to lowered SG:

$$n_{GM5}^{22} = n_{GM6}^{214} + n_{GM7}^{214} + 2n_{GM8}^{214} \quad n_{Y5}^{22} = n_{H6}^{214} + n_{H7}^{214} + 2n_{H8}^{214} \quad n_{L2}^{22} = 2n_{N5}^{214} \quad n_{Z5}^{22} = n_{N5}^{214} \quad n_{T5}^{22} = n_{N5}^{214}$$

The lower SG is SG 22 when the preserved operations are: **(sub-SG label is 3) 1, 9, 16, 15.**

$$\text{The transformation is: } (\mathbf{a}_{22}, \mathbf{b}_{22}, \mathbf{c}_{22}) = (\mathbf{a}_{214}, \mathbf{b}_{214}, \mathbf{c}_{214}) \begin{pmatrix} -1 & 1 & 0 \\ 0 & 0 & 1 \\ 1 & 1 & 0 \end{pmatrix}, \overrightarrow{O_{214}O_{22}} = \frac{1}{8}\mathbf{a}_{22} + (-\frac{1}{8})\mathbf{b}_{22} + (-\frac{1}{8})\mathbf{c}_{22}$$

The reduction of higher dimensional irrep:

$$O : T_1 \rightarrow B_1 + B_2 + B_3 \text{ of } D_2.$$

$$O : T_2 \rightarrow A_1 + B_2 + B_3 \text{ of } D_2.$$

The correspondences of irreps at HSPs from original SG to lowered SG:

$$n_{GM5}^{22} = n_{GM6}^{214} + n_{GM7}^{214} + 2n_{GM8}^{214} \quad n_{Y5}^{22} = n_{N5}^{214} \quad n_{L2}^{22} = 2n_{N5}^{214} \quad n_{Z5}^{22} = n_{H6}^{214} + n_{H7}^{214} + 2n_{H8}^{214} \quad n_{T5}^{22} = n_{N5}^{214}$$

The lower SG is SG 22 when the preserved operations are: **(sub-SG label is 4) 1, 10, 11, 12.**

$$\text{The transformation is: } (\mathbf{a}_{22}, \mathbf{b}_{22}, \mathbf{c}_{22}) = (\mathbf{a}_{214}, \mathbf{b}_{214}, \mathbf{c}_{214}) \begin{pmatrix} 1 & -1 & 0 \\ 1 & 1 & 0 \\ 0 & 0 & 1 \end{pmatrix}, \overrightarrow{O_{214}O_{22}} = \frac{3}{8}\mathbf{a}_{22} + (-\frac{1}{8})\mathbf{b}_{22} + (-\frac{1}{8})\mathbf{c}_{22}$$

The reduction of higher dimensional irrep:

$$O : T_1 \rightarrow B_1 + B_2 + B_3 \text{ of } D_2.$$

$$O : T_2 \rightarrow A_1 + B_2 + B_3 \text{ of } D_2.$$

The correspondences of irreps at HSPs from original SG to lowered SG:

$$n_{GM5}^{22} = n_{GM6}^{214} + n_{GM7}^{214} + 2n_{GM8}^{214} \quad n_{Y5}^{22} = n_{N5}^{214} \quad n_{L2}^{22} = 2n_{N5}^{214} \quad n_{Z5}^{22} = n_{H6}^{214} + n_{H7}^{214} + 2n_{H8}^{214} \quad n_{T5}^{22} = n_{N5}^{214}$$

The lower SG is SG 80 when the preserved operations are: **(sub-SG label is 5) 1, 6, 7, 10.**

$$\text{The transformation is: } (\mathbf{a}_{80}, \mathbf{b}_{80}, \mathbf{c}_{80}) = (\mathbf{a}_{214}, \mathbf{b}_{214}, \mathbf{c}_{214}) \begin{pmatrix} 0 & 1 & 0 \\ -1 & 0 & 0 \\ 0 & 0 & 1 \end{pmatrix}, \overrightarrow{O_{214}O_{80}} = \frac{3}{4}\mathbf{a}_{80} + (\frac{1}{2})\mathbf{b}_{80}$$

The reduction of higher dimensional irrep:

$$O : T_1 \rightarrow A + {}^2E + {}^1E \text{ of } C_4.$$

$$O : T_2 \rightarrow {}^2E + B + {}^1E \text{ of } C_4.$$

The correspondences of irreps at HSPs from original SG to lowered SG:

$$\begin{aligned} n_{GM5}^{80} &= n_{GM7}^{214} + n_{GM8}^{214} & n_{GM7}^{80} &= n_{GM7}^{214} + n_{GM8}^{214} & n_{GM8}^{80} &= n_{GM6}^{214} + n_{GM8}^{214} & n_{GM6}^{80} &= n_{GM6}^{214} + n_{GM8}^{214} & n_{M7}^{80} &= n_{H6}^{214} + n_{H8}^{214} \\ n_{M5}^{80} &= n_{H6}^{214} + n_{H8}^{214} & n_{M6}^{80} &= n_{H7}^{214} + n_{H8}^{214} & n_{M8}^{80} &= n_{H7}^{214} + n_{H8}^{214} & n_{X4}^{80} &= n_{N5}^{214} & n_{X3}^{80} &= n_{N5}^{214} & n_{P4}^{80} &= n_{P4}^{214} + n_{P5}^{214} + n_{P6}^{214} + n_{P7}^{214} \\ n_{P3}^{80} &= 2n_{P7}^{214} & n_{N2}^{80} &= 2n_{N5}^{214} \end{aligned}$$

The lower SG is SG 80 when the preserved operations are: **(sub-SG label is 6) 1, 2, 3, 8.**

$$\text{The transformation is: } (\mathbf{a}_{80}, \mathbf{b}_{80}, \mathbf{c}_{80}) = (\mathbf{a}_{214}, \mathbf{b}_{214}, \mathbf{c}_{214}) \begin{pmatrix} 0 & 0 & 1 \\ 0 & 1 & 0 \\ -1 & 0 & 0 \end{pmatrix}, \overrightarrow{O_{214}O_{80}} = \frac{3}{4}\mathbf{a}_{80} + (\frac{1}{2})\mathbf{b}_{80}$$

The reduction of higher dimensional irrep:

$$O : T_1 \rightarrow A + {}^2E + {}^1E \text{ of } C_4.$$

$$O : T_2 \rightarrow {}^2E + B + {}^1E \text{ of } C_4.$$

The correspondences of irreps at HSPs from original SG to lowered SG:

$$\begin{aligned} n_{GM5}^{80} &= n_{GM7}^{214} + n_{GM8}^{214} & n_{GM7}^{80} &= n_{GM7}^{214} + n_{GM8}^{214} & n_{GM8}^{80} &= n_{GM6}^{214} + n_{GM8}^{214} & n_{GM6}^{80} &= n_{GM6}^{214} + n_{GM8}^{214} & n_{M7}^{80} &= n_{H6}^{214} + n_{H8}^{214} \\ n_{M5}^{80} &= n_{H6}^{214} + n_{H8}^{214} & n_{M6}^{80} &= n_{H7}^{214} + n_{H8}^{214} & n_{M8}^{80} &= n_{H7}^{214} + n_{H8}^{214} & n_{X4}^{80} &= n_{N5}^{214} & n_{X3}^{80} &= n_{N5}^{214} & n_{P4}^{80} &= n_{P4}^{214} + n_{P5}^{214} + n_{P6}^{214} + n_{P7}^{214} \\ n_{P3}^{80} &= 2n_{P7}^{214} & n_{N2}^{80} &= 2n_{N5}^{214} \end{aligned}$$

The lower SG is SG 80 when the preserved operations are: **(sub-SG label is 7) 1, 4, 5, 9.**

$$\text{The transformation is: } (\mathbf{a}_{80}, \mathbf{b}_{80}, \mathbf{c}_{80}) = (\mathbf{a}_{214}, \mathbf{b}_{214}, \mathbf{c}_{214}) \begin{pmatrix} 0 & -1 & 0 \\ 0 & 0 & 1 \\ -1 & 0 & 0 \end{pmatrix}, \overrightarrow{O_{214}O_{80}} = \mathbf{a}_{80} + (-\frac{1}{4})\mathbf{b}_{80}$$

The reduction of higher dimensional irrep:

$$O : T_1 \rightarrow A + {}^2E + {}^1E \text{ of } C_4.$$

$$O : T_2 \rightarrow {}^2E + B + {}^1E \text{ of } C_4.$$

The correspondences of irreps at HSPs from original SG to lowered SG:

$$\begin{aligned} n_{GM5}^{80} &= n_{GM7}^{214} + n_{GM8}^{214} & n_{GM7}^{80} &= n_{GM7}^{214} + n_{GM8}^{214} & n_{GM8}^{80} &= n_{GM6}^{214} + n_{GM8}^{214} & n_{GM6}^{80} &= n_{GM6}^{214} + n_{GM8}^{214} & n_{M7}^{80} &= n_{H6}^{214} + n_{H8}^{214} \\ n_{M5}^{80} &= n_{H6}^{214} + n_{H8}^{214} & n_{M6}^{80} &= n_{H7}^{214} + n_{H8}^{214} & n_{M8}^{80} &= n_{H7}^{214} + n_{H8}^{214} & n_{X4}^{80} &= n_{N5}^{214} & n_{X3}^{80} &= n_{N5}^{214} & n_{P4}^{80} &= n_{P4}^{214} + n_{P5}^{214} + n_{P6}^{214} + n_{P7}^{214} \\ n_{P3}^{80} &= 2n_{P7}^{214} & n_{N2}^{80} &= 2n_{N5}^{214} \end{aligned}$$

The lower SG is SG 98 when the preserved operations are: **(sub-SG label is 8) 1, 6, 7, 10, 8, 9, 11, 12.**

$$\text{The transformation is: } (\mathbf{a}_{98}, \mathbf{b}_{98}, \mathbf{c}_{98}) = (\mathbf{a}_{214}, \mathbf{b}_{214}, \mathbf{c}_{214}) \begin{pmatrix} 0 & 1 & 0 \\ -1 & 0 & 0 \\ 0 & 0 & 1 \end{pmatrix}, \overrightarrow{O_{214}O_{98}} = \frac{1}{4}\mathbf{a}_{98} + (\frac{3}{8})\mathbf{c}_{98}$$

The reduction of higher dimensional irrep:

$$O : E \rightarrow A_1 + B_1 \text{ of } D_4.$$

The correspondences of irreps at HSPs from original SG to lowered SG:

$$\begin{aligned} n_{GM6}^{98} &= n_{GM7}^{214} + n_{GM8}^{214} & n_{GM7}^{98} &= n_{GM6}^{214} + n_{GM8}^{214} & n_{M6}^{98} &= n_{H6}^{214} + n_{H8}^{214} & n_{M7}^{98} &= n_{H7}^{214} + n_{H8}^{214} & n_{X5}^{98} &= n_{N5}^{214} & n_{P2}^{98} &= n_{P7}^{214} & n_{P3}^{98} &= n_{P4}^{214} + n_{P5}^{214} + n_{P6}^{214} \\ n_{P5}^{98} &= n_{P7}^{214} & n_{P4}^{98} &= n_{P7}^{214} & n_{N3}^{98} &= n_{N5}^{214} & n_{N4}^{98} &= n_{N5}^{214} \end{aligned}$$

The lower SG is SG 98 when the preserved operations are: **(sub-SG label is 9) 1, 2, 3, 8, 9, 10, 13, 14.**

$$\text{The transformation is: } (\mathbf{a}_{98}, \mathbf{b}_{98}, \mathbf{c}_{98}) = (\mathbf{a}_{214}, \mathbf{b}_{214}, \mathbf{c}_{214}) \begin{pmatrix} 0 & 0 & 1 \\ 0 & 1 & 0 \\ -1 & 0 & 0 \end{pmatrix}, \overrightarrow{O_{214}O_{98}} = \frac{1}{4}\mathbf{a}_{98} + (\frac{3}{8})\mathbf{c}_{98}$$

The reduction of higher dimensional irrep:

$$O : E \rightarrow A_1 + B_1 \text{ of } D_4.$$

The correspondences of irreps at HSPs from original SG to lowered SG:

$$\begin{aligned} n_{GM6}^{98} &= n_{GM7}^{214} + n_{GM8}^{214} & n_{GM7}^{98} &= n_{GM6}^{214} + n_{GM8}^{214} & n_{M6}^{98} &= n_{H6}^{214} + n_{H8}^{214} & n_{M7}^{98} &= n_{H7}^{214} + n_{H8}^{214} & n_{X5}^{98} &= n_{N5}^{214} & n_{P2}^{98} &= n_{P7}^{214} & n_{P3}^{98} &= n_{P4}^{214} + n_{P5}^{214} + n_{P6}^{214} \\ n_{P5}^{98} &= n_{P7}^{214} & n_{P4}^{98} &= n_{P7}^{214} & n_{N3}^{98} &= n_{N5}^{214} & n_{N4}^{98} &= n_{N5}^{214} \end{aligned}$$

The lower SG is SG 98 when the preserved operations are: **(sub-SG label is 10) 1, 4, 5, 9, 10, 8, 16, 15.**

$$\text{The transformation is: } (\mathbf{a}_{98}, \mathbf{b}_{98}, \mathbf{c}_{98}) = (\mathbf{a}_{214}, \mathbf{b}_{214}, \mathbf{c}_{214}) \begin{pmatrix} 0 & -1 & 0 \\ 0 & 0 & -1 \\ 1 & 0 & 0 \end{pmatrix}, \overrightarrow{O_{214}O_{98}} = \frac{1}{2}\mathbf{a}_{98} + (-\frac{1}{4})\mathbf{b}_{98} + (\frac{1}{8})\mathbf{c}_{98}$$

The reduction of higher dimensional irrep:

$$O : E \rightarrow A_1 + B_1 \text{ of } D_4.$$

The correspondences of irreps at HSPs from original SG to lowered SG:

$$\begin{aligned} n_{GM6}^{98} &= n_{GM7}^{214} + n_{GM8}^{214} & n_{GM7}^{98} &= n_{GM6}^{214} + n_{GM8}^{214} & n_{M6}^{98} &= n_{H6}^{214} + n_{H8}^{214} & n_{M7}^{98} &= n_{H7}^{214} + n_{H8}^{214} & n_{X5}^{98} &= n_{N5}^{214} & n_{P2}^{98} &= n_{P7}^{214} & n_{P3}^{98} &= n_{P4}^{214} + n_{P5}^{214} + n_{P6}^{214} \\ n_{P5}^{98} &= n_{P7}^{214} & n_{P4}^{98} &= n_{P7}^{214} & n_{N3}^{98} &= n_{N5}^{214} & n_{N4}^{98} &= n_{N5}^{214} \end{aligned}$$

The lower SG is SG 146 when the preserved operations are: **(sub-SG label is 11) 1, 17, 18.**

$$\text{The transformation is: } (\mathbf{a}_{146}, \mathbf{b}_{146}, \mathbf{c}_{146}) = (\mathbf{a}_{214}, \mathbf{b}_{214}, \mathbf{c}_{214}) \begin{pmatrix} \frac{1}{2} & -\frac{1}{2} & \frac{1}{2} \\ \frac{1}{2} & \frac{1}{2} & -\frac{1}{2} \\ -\frac{1}{2} & \frac{1}{2} & \frac{1}{2} \end{pmatrix}, \overrightarrow{O_{214}O_{146}} = -\frac{1}{3}\mathbf{a}_{146} + (\frac{2}{3})\mathbf{b}_{146} + (-\frac{1}{3})\mathbf{c}_{146}$$

The reduction of higher dimensional irrep:

$$O : T_1 \rightarrow A + {}^2E + {}^1E \text{ of } C_3.$$

$$O : T_2 \rightarrow A + {}^2E + {}^1E \text{ of } C_3.$$

The correspondences of irreps at HSPs from original SG to lowered SG:

$$n_{GM4}^{146} = 2n_{GM8}^{214} \quad n_{GM6}^{146} = n_{GM6}^{214} + n_{GM7}^{214} + n_{GM8}^{214} \quad n_{GM5}^{146} = n_{GM6}^{214} + n_{GM7}^{214} + n_{GM8}^{214} \quad n_{L2}^{146} = 2n_{N5}^{214} \quad n_{F2}^{146} = 2n_{N5}^{214} \quad n_{T4}^{146} =$$

$$2n_{H8}^{214} n_{T6}^{146} = n_{H6}^{214} + n_{H7}^{214} + n_{H8}^{214} n_{T5}^{146} = n_{H6}^{214} + n_{H7}^{214} + n_{H8}^{214}$$

The lower SG is SG 146 when the preserved operations are: **(sub-SG label is 12) 1, 24, 23.**

$$\text{The transformation is: } (\mathbf{a}_{146}, \mathbf{b}_{146}, \mathbf{c}_{146}) = (\mathbf{a}_{214}, \mathbf{b}_{214}, \mathbf{c}_{214}) \begin{pmatrix} -\frac{1}{2} & -\frac{1}{2} & \frac{1}{2} \\ \frac{1}{2} & -\frac{1}{2} & -\frac{1}{2} \\ \frac{1}{2} & -\frac{1}{2} & \frac{1}{2} \end{pmatrix}, \overrightarrow{O_{214}O_{146}} = -\frac{1}{3}\mathbf{a}_{146} + \left(\frac{1}{6}\right)\mathbf{b}_{146} + \left(\frac{1}{6}\right)\mathbf{c}_{146}$$

The reduction of higher dimensional irrep:

$$O : T_1 \rightarrow A + {}^2E + {}^1E \text{ of } C_3.$$

$$O : T_2 \rightarrow A + {}^2E + {}^1E \text{ of } C_3.$$

The correspondences of irreps at HSPs from original SG to lowered SG:

$$n_{GM4}^{146} = 2n_{GM8}^{214} n_{GM6}^{146} = n_{GM6}^{214} + n_{GM7}^{214} + n_{GM8}^{214} n_{GM5}^{146} = n_{GM6}^{214} + n_{GM7}^{214} + n_{GM8}^{214} n_{L2}^{146} = 2n_{N5}^{214} n_{F2}^{146} = 2n_{N5}^{214} n_{T4}^{146} = 2n_{H8}^{214} n_{T6}^{146} = n_{H6}^{214} + n_{H7}^{214} + n_{H8}^{214} n_{T5}^{146} = n_{H6}^{214} + n_{H7}^{214} + n_{H8}^{214}$$

The lower SG is SG 146 when the preserved operations are: **(sub-SG label is 13) 1, 20, 19.**

$$\text{The transformation is: } (\mathbf{a}_{146}, \mathbf{b}_{146}, \mathbf{c}_{146}) = (\mathbf{a}_{214}, \mathbf{b}_{214}, \mathbf{c}_{214}) \begin{pmatrix} \frac{1}{2} & -\frac{1}{2} & \frac{1}{2} \\ -\frac{1}{2} & -\frac{1}{2} & \frac{1}{2} \\ \frac{1}{2} & -\frac{1}{2} & -\frac{1}{2} \end{pmatrix}, \overrightarrow{O_{214}O_{146}} = -\frac{1}{3}\mathbf{a}_{146} + \left(\frac{1}{6}\right)\mathbf{b}_{146} + \left(\frac{1}{6}\right)\mathbf{c}_{146}$$

The reduction of higher dimensional irrep:

$$O : T_1 \rightarrow A + {}^2E + {}^1E \text{ of } C_3.$$

$$O : T_2 \rightarrow A + {}^2E + {}^1E \text{ of } C_3.$$

The correspondences of irreps at HSPs from original SG to lowered SG:

$$n_{GM4}^{146} = 2n_{GM8}^{214} n_{GM6}^{146} = n_{GM6}^{214} + n_{GM7}^{214} + n_{GM8}^{214} n_{GM5}^{146} = n_{GM6}^{214} + n_{GM7}^{214} + n_{GM8}^{214} n_{L2}^{146} = 2n_{N5}^{214} n_{F2}^{146} = 2n_{N5}^{214} n_{T4}^{146} = 2n_{H8}^{214} n_{T6}^{146} = n_{H6}^{214} + n_{H7}^{214} + n_{H8}^{214} n_{T5}^{146} = n_{H6}^{214} + n_{H7}^{214} + n_{H8}^{214}$$

The lower SG is SG 146 when the preserved operations are: **(sub-SG label is 14) 1, 22, 21.**

$$\text{The transformation is: } (\mathbf{a}_{146}, \mathbf{b}_{146}, \mathbf{c}_{146}) = (\mathbf{a}_{214}, \mathbf{b}_{214}, \mathbf{c}_{214}) \begin{pmatrix} -\frac{1}{2} & -\frac{1}{2} & \frac{1}{2} \\ -\frac{1}{2} & \frac{1}{2} & \frac{1}{2} \\ -\frac{1}{2} & \frac{1}{2} & -\frac{1}{2} \end{pmatrix}, \overrightarrow{O_{214}O_{146}} = -\frac{1}{2}\mathbf{a}_{146} + \left(\frac{1}{2}\right)\mathbf{b}_{146}$$

The reduction of higher dimensional irrep:

$$O : T_1 \rightarrow A + {}^2E + {}^1E \text{ of } C_3.$$

$$O : T_2 \rightarrow A + {}^2E + {}^1E \text{ of } C_3.$$

The correspondences of irreps at HSPs from original SG to lowered SG:

$$n_{GM4}^{146} = 2n_{GM8}^{214} n_{GM6}^{146} = n_{GM6}^{214} + n_{GM7}^{214} + n_{GM8}^{214} n_{GM5}^{146} = n_{GM6}^{214} + n_{GM7}^{214} + n_{GM8}^{214} n_{L2}^{146} = 2n_{N5}^{214} n_{F2}^{146} = 2n_{N5}^{214} n_{T4}^{146} = 2n_{H8}^{214} n_{T6}^{146} = n_{H6}^{214} + n_{H7}^{214} + n_{H8}^{214} n_{T5}^{146} = n_{H6}^{214} + n_{H7}^{214} + n_{H8}^{214}$$

The lower SG is SG 199 when the preserved operations are: **(sub-SG label is 15) 1, 8, 9, 10, 17, 24, 20, 22, 18, 23, 19, 21.**

$$\text{The transformation is: } (\mathbf{a}_{199}, \mathbf{b}_{199}, \mathbf{c}_{199}) = (\mathbf{a}_{214}, \mathbf{b}_{214}, \mathbf{c}_{214}) \begin{pmatrix} 0 & 0 & -1 \\ 1 & 0 & 0 \\ 0 & -1 & 0 \end{pmatrix}, \overrightarrow{O_{214}O_{199}} = \frac{1}{2}\mathbf{a}_{199} + \left(-\frac{1}{2}\right)\mathbf{b}_{199}$$

The reduction of higher dimensional irrep:

$$O : E \rightarrow {}^1E + {}^2E \text{ of } T.$$

The correspondences of irreps at HSPs from original SG to lowered SG:

$$n_{GM6}^{199} = n_{GM8}^{214} n_{GM7}^{199} = n_{GM8}^{214} n_{GM5}^{199} = n_{GM6}^{214} + n_{GM7}^{214} n_{H6}^{199} = n_{GM8}^{214} n_{H7}^{199} = n_{H8}^{214} n_{H5}^{199} = n_{H6}^{214} + n_{H7}^{214} n_{N3}^{199} = n_{N5}^{214} n_{N4}^{199} = n_{N5}^{214} n_{P4}^{199} = n_{P4}^{214} n_{P6}^{199} = n_{P6}^{214} n_{P5}^{199} = n_{P5}^{214} n_{P7}^{199} = n_{P7}^{214}$$

## 112. Lowered SGs by higher-dimensional irreps of pairings in SG 215

The representative operations of SG/T for SG 215:

$$1 : (x, y, z), 2 : (x, -y, -z), 3 : (-x, y, -z), 4 : (-x, -y, z), 5 : (z, x, y), 6 : (y, z, x), 7 : (-y, z, -x), 8 : (-z, -x, y), 9 : (-y, -z, x), 10 : (z, -x, -y), 11 : (y, -z, -x), 12 : (-z, x, -y), 13 : (-x, z, -y), 14 : (-x, -z, y), 15 : (-z, -y, x), 16 : (z, -y, -x), 17 : (y, -x, -z), 18 : (-y, x, -z), 19 : (-y, -x, z), 20 : (y, x, z), 21 : (x, -z, -y), 22 : (x, z, y),$$

$$23 : (-z, y, -x), 24 : (z, y, x).$$

The lower SG is SG 16 when the preserved operations are: **(sub-SG label is 1) 1, 2, 3, 4.**

$$\text{The transformation is: } (\mathbf{a}_{16}, \mathbf{b}_{16}, \mathbf{c}_{16}) = (\mathbf{a}_{215}, \mathbf{b}_{215}, \mathbf{c}_{215}) \begin{pmatrix} 0 & 0 & 1 \\ 1 & 0 & 0 \\ 0 & 1 & 0 \end{pmatrix}, \overrightarrow{O_{215}O_{16}} = \frac{1}{2}\mathbf{a}_{16} + \left(\frac{1}{2}\right)\mathbf{c}_{16}$$

The reduction of higher dimensional irrep:

$$T_d : T_1 \rightarrow B_1 + B_2 + B_3 \text{ of } D_2.$$

$$T_d : T_2 \rightarrow B_1 + B_2 + B_3 \text{ of } D_2.$$

The correspondences of irreps at HSPs from original SG to lowered SG:

$$\begin{aligned} n_{GM5}^{16} &= n_{GM6}^{215} + n_{GM7}^{215} + 2n_{GM8}^{215} n_{X5}^{16} = n_{X6}^{215} + n_{X7}^{215} n_{S5}^{16} = n_{M6}^{215} + n_{M7}^{215} n_{R5}^{16} = n_{R6}^{215} + n_{R7}^{215} + 2n_{R8}^{215} n_{U5}^{16} = n_{M6}^{215} + n_{M7}^{215} \\ n_{Z5}^{16} &= n_{X6}^{215} + n_{X7}^{215} n_{T5}^{16} = n_{M6}^{215} + n_{M7}^{215} n_{Y5}^{16} = n_{X6}^{215} + n_{X7}^{215} \end{aligned}$$

The lower SG is SG 35 when the preserved operations are: **(sub-SG label is 2) 1, 4, 19, 20.**

$$\text{The transformation is: } (\mathbf{a}_{35}, \mathbf{b}_{35}, \mathbf{c}_{35}) = (\mathbf{a}_{215}, \mathbf{b}_{215}, \mathbf{c}_{215}) \begin{pmatrix} 1 & -1 & 0 \\ 1 & 1 & 0 \\ 0 & 0 & 1 \end{pmatrix}, \overrightarrow{O_{215}O_{35}} = \mathbf{0}$$

The reduction of higher dimensional irrep:

$$T_d : T_1 \rightarrow A_2 + B_1 + B_2 \text{ of } C_{2v}.$$

$$T_d : T_2 \rightarrow A_1 + B_1 + B_2 \text{ of } C_{2v}.$$

The correspondences of irreps at HSPs from original SG to lowered SG:

$$\begin{aligned} n_{GM5}^{35} &= n_{GM6}^{215} + n_{GM7}^{215} + 2n_{GM8}^{215} n_{Y5}^{35} = n_{M6}^{215} + n_{M7}^{215} n_{S4}^{35} = n_{X6}^{215} + n_{X7}^{215} n_{S3}^{35} = n_{X6}^{215} + n_{X7}^{215} n_{Z5}^{35} = n_{X6}^{215} + n_{X7}^{215} n_{T5}^{35} = \\ n_{R6}^{215} + n_{R7}^{215} + 2n_{R8}^{215} n_{R4}^{35} &= n_{M6}^{215} + n_{M7}^{215} n_{R3}^{35} = n_{M6}^{215} + n_{M7}^{215} \end{aligned}$$

The lower SG is SG 35 when the preserved operations are: **(sub-SG label is 3) 1, 2, 21, 22.**

$$\text{The transformation is: } (\mathbf{a}_{35}, \mathbf{b}_{35}, \mathbf{c}_{35}) = (\mathbf{a}_{215}, \mathbf{b}_{215}, \mathbf{c}_{215}) \begin{pmatrix} 0 & 0 & 1 \\ 1 & -1 & 0 \\ 1 & 1 & 0 \end{pmatrix}, \overrightarrow{O_{215}O_{35}} = \mathbf{0}$$

The reduction of higher dimensional irrep:

$$T_d : T_1 \rightarrow A_2 + B_1 + B_2 \text{ of } C_{2v}.$$

$$T_d : T_2 \rightarrow A_1 + B_1 + B_2 \text{ of } C_{2v}.$$

The correspondences of irreps at HSPs from original SG to lowered SG:

$$\begin{aligned} n_{GM5}^{35} &= n_{GM6}^{215} + n_{GM7}^{215} + 2n_{GM8}^{215} n_{Y5}^{35} = n_{M6}^{215} + n_{M7}^{215} n_{S4}^{35} = n_{X6}^{215} + n_{X7}^{215} n_{S3}^{35} = n_{X6}^{215} + n_{X7}^{215} n_{Z5}^{35} = n_{X6}^{215} + n_{X7}^{215} n_{T5}^{35} = \\ n_{R6}^{215} + n_{R7}^{215} + 2n_{R8}^{215} n_{R4}^{35} &= n_{M6}^{215} + n_{M7}^{215} n_{R3}^{35} = n_{M6}^{215} + n_{M7}^{215} \end{aligned}$$

The lower SG is SG 35 when the preserved operations are: **(sub-SG label is 4) 1, 3, 24, 23.**

$$\text{The transformation is: } (\mathbf{a}_{35}, \mathbf{b}_{35}, \mathbf{c}_{35}) = (\mathbf{a}_{215}, \mathbf{b}_{215}, \mathbf{c}_{215}) \begin{pmatrix} -1 & 1 & 0 \\ 0 & 0 & 1 \\ 1 & 1 & 0 \end{pmatrix}, \overrightarrow{O_{215}O_{35}} = \mathbf{0}$$

The reduction of higher dimensional irrep:

$$T_d : T_1 \rightarrow A_2 + B_1 + B_2 \text{ of } C_{2v}.$$

$$T_d : T_2 \rightarrow A_1 + B_1 + B_2 \text{ of } C_{2v}.$$

The correspondences of irreps at HSPs from original SG to lowered SG:

$$\begin{aligned} n_{GM5}^{35} &= n_{GM6}^{215} + n_{GM7}^{215} + 2n_{GM8}^{215} n_{Y5}^{35} = n_{M6}^{215} + n_{M7}^{215} n_{S4}^{35} = n_{X6}^{215} + n_{X7}^{215} n_{S3}^{35} = n_{X6}^{215} + n_{X7}^{215} n_{Z5}^{35} = n_{X6}^{215} + n_{X7}^{215} n_{T5}^{35} = \\ n_{R6}^{215} + n_{R7}^{215} + 2n_{R8}^{215} n_{R4}^{35} &= n_{M6}^{215} + n_{M7}^{215} n_{R3}^{35} = n_{M6}^{215} + n_{M7}^{215} \end{aligned}$$

The lower SG is SG 81 when the preserved operations are: **(sub-SG label is 5) 1, 17, 18, 4.**

$$\text{The transformation is: } (\mathbf{a}_{81}, \mathbf{b}_{81}, \mathbf{c}_{81}) = (\mathbf{a}_{215}, \mathbf{b}_{215}, \mathbf{c}_{215}) \begin{pmatrix} -1 & 0 & 0 \\ 0 & -1 & 0 \\ 0 & 0 & 1 \end{pmatrix}, \overrightarrow{O_{215}O_{81}} = \frac{1}{2}\mathbf{a}_{81} + \left(\frac{1}{2}\right)\mathbf{b}_{81} + \left(\frac{1}{2}\right)\mathbf{c}_{81}$$

The reduction of higher dimensional irrep:

$$T_d : T_1 \rightarrow A + {}^2E + {}^1E \text{ of } S_4.$$

$$T_d : T_2 \rightarrow {}^2E + B + {}^1E \text{ of } S_4.$$

The correspondences of irreps at HSPs from original SG to lowered SG:

$$\begin{aligned} n_{GM7}^{81} &= n_{GM7}^{215} + n_{GM8}^{215} n_{GM8}^{81} = n_{GM6}^{215} + n_{GM8}^{215} n_{GM5}^{81} = n_{GM7}^{215} + n_{GM8}^{215} n_{GM6}^{81} = n_{GM6}^{215} + n_{GM8}^{215} n_{X4}^{81} = n_{X6}^{215} + n_{X7}^{215} n_{X3}^{81} = \\ n_{X6}^{215} + n_{X7}^{215} n_{M7}^{81} &= n_{M7}^{215} n_{M8}^{81} = n_{M6}^{215} n_{M5}^{81} = n_{M7}^{215} n_{M6}^{81} = n_{M6}^{215} n_{A7}^{81} = n_{R7}^{215} + n_{R8}^{215} n_{A8}^{81} = n_{R6}^{215} + n_{R8}^{215} n_{A5}^{81} = n_{R7}^{215} + n_{R8}^{215} \end{aligned}$$

$$n_{A6}^{81} = n_{R6}^{215} + n_{R8}^{215} \quad n_{R4}^{81} = n_{M6}^{215} + n_{M7}^{215} \quad n_{R3}^{81} = n_{M6}^{215} + n_{M7}^{215} \quad n_{Z7}^{81} = n_{X7}^{215} \quad n_{Z8}^{81} = n_{X6}^{215} \quad n_{Z5}^{81} = n_{X7}^{215} \quad n_{Z6}^{81} = n_{X6}^{215}$$

The lower SG is SG 81 when the preserved operations are: **(sub-SG label is 6) 1, 13, 14, 2.**

$$\text{The transformation is: } (\mathbf{a}_{81}, \mathbf{b}_{81}, \mathbf{c}_{81}) = (\mathbf{a}_{215}, \mathbf{b}_{215}, \mathbf{c}_{215}) \begin{pmatrix} 0 & 0 & 1 \\ -1 & 0 & 0 \\ 0 & -1 & 0 \end{pmatrix}, \overrightarrow{O_{215}O_{81}} = \frac{1}{2}\mathbf{a}_{81} + \left(\frac{1}{2}\right)\mathbf{b}_{81} + \left(\frac{1}{2}\right)\mathbf{c}_{81}$$

The reduction of higher dimensional irrep:

$$T_d : T_1 \rightarrow A + {}^2E + {}^1E \quad \text{of } S_4.$$

$$T_d : T_2 \rightarrow {}^2E + B + {}^1E \quad \text{of } S_4.$$

The correspondences of irreps at HSPs from original SG to lowered SG:

$$\begin{aligned} n_{GM7}^{81} &= n_{GM7}^{215} + n_{GM8}^{215} \quad n_{GM8}^{81} = n_{GM6}^{215} + n_{GM8}^{215} \quad n_{GM5}^{81} = n_{GM7}^{215} + n_{GM8}^{215} \quad n_{GM6}^{81} = n_{GM6}^{215} + n_{GM8}^{215} \quad n_{X4}^{81} = n_{X6}^{215} + n_{X7}^{215} \quad n_{X3}^{81} = \\ n_{X6}^{215} + n_{X7}^{215} \quad n_{M7}^{81} &= n_{M7}^{215} \quad n_{M8}^{81} = n_{M6}^{215} \quad n_{M5}^{81} = n_{M7}^{215} \quad n_{M6}^{81} = n_{M6}^{215} \quad n_{A7}^{81} = n_{R7}^{215} + n_{R8}^{215} \quad n_{A8}^{81} = n_{R6}^{215} + n_{R8}^{215} \quad n_{A5}^{81} = n_{R7}^{215} + n_{R8}^{215} \\ n_{A6}^{81} &= n_{R6}^{215} + n_{R8}^{215} \quad n_{R4}^{81} = n_{M6}^{215} + n_{M7}^{215} \quad n_{R3}^{81} = n_{M6}^{215} + n_{M7}^{215} \quad n_{Z7}^{81} = n_{X7}^{215} \quad n_{Z8}^{81} = n_{X6}^{215} \quad n_{Z5}^{81} = n_{X7}^{215} \quad n_{Z6}^{81} = n_{X6}^{215} \end{aligned}$$

The lower SG is SG 81 when the preserved operations are: **(sub-SG label is 7) 1, 15, 16, 3.**

$$\text{The transformation is: } (\mathbf{a}_{81}, \mathbf{b}_{81}, \mathbf{c}_{81}) = (\mathbf{a}_{215}, \mathbf{b}_{215}, \mathbf{c}_{215}) \begin{pmatrix} -1 & 0 & 0 \\ 0 & 0 & 1 \\ 0 & 1 & 0 \end{pmatrix}, \overrightarrow{O_{215}O_{81}} = \frac{1}{2}\mathbf{a}_{81} + \left(\frac{1}{2}\right)\mathbf{b}_{81} + \left(\frac{1}{2}\right)\mathbf{c}_{81}$$

The reduction of higher dimensional irrep:

$$T_d : T_1 \rightarrow A + {}^2E + {}^1E \quad \text{of } S_4.$$

$$T_d : T_2 \rightarrow {}^2E + B + {}^1E \quad \text{of } S_4.$$

The correspondences of irreps at HSPs from original SG to lowered SG:

$$\begin{aligned} n_{GM7}^{81} &= n_{GM7}^{215} + n_{GM8}^{215} \quad n_{GM8}^{81} = n_{GM6}^{215} + n_{GM8}^{215} \quad n_{GM5}^{81} = n_{GM7}^{215} + n_{GM8}^{215} \quad n_{GM6}^{81} = n_{GM6}^{215} + n_{GM8}^{215} \quad n_{X4}^{81} = n_{X6}^{215} + n_{X7}^{215} \quad n_{X3}^{81} = \\ n_{X6}^{215} + n_{X7}^{215} \quad n_{M7}^{81} &= n_{M7}^{215} \quad n_{M8}^{81} = n_{M6}^{215} \quad n_{M5}^{81} = n_{M7}^{215} \quad n_{M6}^{81} = n_{M6}^{215} \quad n_{A7}^{81} = n_{R7}^{215} + n_{R8}^{215} \quad n_{A8}^{81} = n_{R6}^{215} + n_{R8}^{215} \quad n_{A5}^{81} = n_{R7}^{215} + n_{R8}^{215} \\ n_{A6}^{81} &= n_{R6}^{215} + n_{R8}^{215} \quad n_{R4}^{81} = n_{M6}^{215} + n_{M7}^{215} \quad n_{R3}^{81} = n_{M6}^{215} + n_{M7}^{215} \quad n_{Z7}^{81} = n_{X7}^{215} \quad n_{Z8}^{81} = n_{X6}^{215} \quad n_{Z5}^{81} = n_{X7}^{215} \quad n_{Z6}^{81} = n_{X6}^{215} \end{aligned}$$

The lower SG is SG 111 when the preserved operations are: **(sub-SG label is 8) 1, 18, 17, 4, 2, 3, 19, 20.**

$$\text{The transformation is: } (\mathbf{a}_{111}, \mathbf{b}_{111}, \mathbf{c}_{111}) = (\mathbf{a}_{215}, \mathbf{b}_{215}, \mathbf{c}_{215}) \begin{pmatrix} -1 & 0 & 0 \\ 0 & 1 & 0 \\ 0 & 0 & -1 \end{pmatrix}, \overrightarrow{O_{215}O_{111}} = \frac{1}{2}\mathbf{a}_{111} + \left(\frac{1}{2}\right)\mathbf{b}_{111} + \left(\frac{1}{2}\right)\mathbf{c}_{111}$$

The reduction of higher dimensional irrep:

$$T_d : E \rightarrow A_1 + B_1 \quad \text{of } D_{2d}.$$

The correspondences of irreps at HSPs from original SG to lowered SG:

$$\begin{aligned} n_{GM6}^{111} &= n_{GM7}^{215} + n_{GM8}^{215} \quad n_{GM7}^{111} = n_{GM6}^{215} + n_{GM8}^{215} \quad n_{X5}^{111} = n_{X6}^{215} + n_{X7}^{215} \quad n_{M6}^{111} = n_{M7}^{215} \quad n_{M7}^{111} = n_{M6}^{215} \quad n_{A6}^{111} = n_{R7}^{215} + n_{R8}^{215} \quad n_{A7}^{111} = \\ n_{R6}^{215} + n_{R8}^{215} \quad n_{R5}^{111} &= n_{M6}^{215} + n_{M7}^{215} \quad n_{Z6}^{111} = n_{X7}^{215} \quad n_{Z7}^{111} = n_{X6}^{215} \end{aligned}$$

The lower SG is SG 111 when the preserved operations are: **(sub-SG label is 9) 1, 14, 13, 2, 3, 4, 21, 22.**

$$\text{The transformation is: } (\mathbf{a}_{111}, \mathbf{b}_{111}, \mathbf{c}_{111}) = (\mathbf{a}_{215}, \mathbf{b}_{215}, \mathbf{c}_{215}) \begin{pmatrix} 0 & 0 & -1 \\ -1 & 0 & 0 \\ 0 & 1 & 0 \end{pmatrix}, \overrightarrow{O_{215}O_{111}} = \frac{1}{2}\mathbf{a}_{111} + \left(\frac{1}{2}\right)\mathbf{b}_{111} + \left(\frac{1}{2}\right)\mathbf{c}_{111}$$

The reduction of higher dimensional irrep:

$$T_d : E \rightarrow A_1 + B_1 \quad \text{of } D_{2d}.$$

The correspondences of irreps at HSPs from original SG to lowered SG:

$$\begin{aligned} n_{GM6}^{111} &= n_{GM7}^{215} + n_{GM8}^{215} \quad n_{GM7}^{111} = n_{GM6}^{215} + n_{GM8}^{215} \quad n_{X5}^{111} = n_{X6}^{215} + n_{X7}^{215} \quad n_{M6}^{111} = n_{M7}^{215} \quad n_{M7}^{111} = n_{M6}^{215} \quad n_{A6}^{111} = n_{R7}^{215} + n_{R8}^{215} \quad n_{A7}^{111} = \\ n_{R6}^{215} + n_{R8}^{215} \quad n_{R5}^{111} &= n_{M6}^{215} + n_{M7}^{215} \quad n_{Z6}^{111} = n_{X7}^{215} \quad n_{Z7}^{111} = n_{X6}^{215} \end{aligned}$$

The lower SG is SG 111 when the preserved operations are: **(sub-SG label is 10) 1, 16, 15, 3, 4, 2, 24, 23.**

$$\text{The transformation is: } (\mathbf{a}_{111}, \mathbf{b}_{111}, \mathbf{c}_{111}) = (\mathbf{a}_{215}, \mathbf{b}_{215}, \mathbf{c}_{215}) \begin{pmatrix} -1 & 0 & 0 \\ 0 & 0 & -1 \\ 0 & -1 & 0 \end{pmatrix}, \overrightarrow{O_{215}O_{111}} = \frac{1}{2}\mathbf{a}_{111} + \left(\frac{1}{2}\right)\mathbf{b}_{111} + \left(\frac{1}{2}\right)\mathbf{c}_{111}$$

The reduction of higher dimensional irrep:

$$T_d : E \rightarrow A_1 + B_1 \quad \text{of } D_{2d}.$$

The correspondences of irreps at HSPs from original SG to lowered SG:

$$\begin{aligned} n_{GM6}^{111} &= n_{GM7}^{215} + n_{GM8}^{215} \quad n_{GM7}^{111} = n_{GM6}^{215} + n_{GM8}^{215} \quad n_{X5}^{111} = n_{X6}^{215} + n_{X7}^{215} \quad n_{M6}^{111} = n_{M7}^{215} \quad n_{M7}^{111} = n_{M6}^{215} \quad n_{A6}^{111} = n_{R7}^{215} + n_{R8}^{215} \quad n_{A7}^{111} = \\ n_{R6}^{215} + n_{R8}^{215} \quad n_{R5}^{111} &= n_{M6}^{215} + n_{M7}^{215} \quad n_{Z6}^{111} = n_{X7}^{215} \quad n_{Z7}^{111} = n_{X6}^{215} \end{aligned}$$

The lower SG is SG 146 when the preserved operations are: **(sub-SG label is 11) 1, 5, 6.**

The transformation is:  $(\mathbf{a}_{146}, \mathbf{b}_{146}, \mathbf{c}_{146}) = (\mathbf{a}_{215}, \mathbf{b}_{215}, \mathbf{c}_{215}) \begin{pmatrix} 0 & 1 & 0 \\ 0 & 0 & 1 \\ 1 & 0 & 0 \end{pmatrix}, \overrightarrow{O_{215}O_{146}} = -\frac{1}{3}\mathbf{a}_{146} + (\frac{2}{3})\mathbf{b}_{146} + (-\frac{1}{3})\mathbf{c}_{146}$

The reduction of higher dimensional irrep:

$$T_d : T_1 \rightarrow A + {}^2E + {}^1E \text{ of } C_3.$$

$$T_d : T_2 \rightarrow A + {}^2E + {}^1E \text{ of } C_3.$$

The correspondences of irreps at HSPs from original SG to lowered SG:

$$n_{GM4}^{146} = 2n_{GM8}^{215} \quad n_{GM6}^{146} = n_{GM6}^{215} + n_{GM7}^{215} + n_{GM8}^{215} \quad n_{GM5}^{146} = n_{GM6}^{215} + n_{GM7}^{215} + n_{GM8}^{215} \quad n_{L2}^{146} = 2n_{X6}^{215} + 2n_{X7}^{215} \quad n_{F2}^{146} = 2n_{M6}^{215} + 2n_{M7}^{215} \quad n_{T4}^{146} = 2n_{R8}^{215} \quad n_{T6}^{146} = n_{R6}^{215} + n_{R7}^{215} + n_{R8}^{215} \quad n_{T5}^{146} = n_{R6}^{215} + n_{R7}^{215} + n_{R8}^{215}$$

The lower SG is SG 146 when the preserved operations are: **(sub-SG label is 12) 1, 12, 11.**

The transformation is:  $(\mathbf{a}_{146}, \mathbf{b}_{146}, \mathbf{c}_{146}) = (\mathbf{a}_{215}, \mathbf{b}_{215}, \mathbf{c}_{215}) \begin{pmatrix} 0 & -1 & 0 \\ 0 & 0 & -1 \\ 1 & 0 & 0 \end{pmatrix}, \overrightarrow{O_{215}O_{146}} = -\frac{1}{3}\mathbf{a}_{146} + (\frac{2}{3})\mathbf{b}_{146} + (-\frac{1}{3})\mathbf{c}_{146}$

The reduction of higher dimensional irrep:

$$T_d : T_1 \rightarrow A + {}^2E + {}^1E \text{ of } C_3.$$

$$T_d : T_2 \rightarrow A + {}^2E + {}^1E \text{ of } C_3.$$

The correspondences of irreps at HSPs from original SG to lowered SG:

$$n_{GM4}^{146} = 2n_{GM8}^{215} \quad n_{GM6}^{146} = n_{GM6}^{215} + n_{GM7}^{215} + n_{GM8}^{215} \quad n_{GM5}^{146} = n_{GM6}^{215} + n_{GM7}^{215} + n_{GM8}^{215} \quad n_{L2}^{146} = 2n_{X6}^{215} + 2n_{X7}^{215} \quad n_{F2}^{146} = 2n_{M6}^{215} + 2n_{M7}^{215} \quad n_{T4}^{146} = 2n_{R8}^{215} \quad n_{T6}^{146} = n_{R6}^{215} + n_{R7}^{215} + n_{R8}^{215} \quad n_{T5}^{146} = n_{R6}^{215} + n_{R7}^{215} + n_{R8}^{215}$$

The lower SG is SG 146 when the preserved operations are: **(sub-SG label is 13) 1, 8, 7.**

The transformation is:  $(\mathbf{a}_{146}, \mathbf{b}_{146}, \mathbf{c}_{146}) = (\mathbf{a}_{215}, \mathbf{b}_{215}, \mathbf{c}_{215}) \begin{pmatrix} 1 & 0 & 0 \\ 0 & -1 & 0 \\ 0 & 0 & -1 \end{pmatrix}, \overrightarrow{O_{215}O_{146}} = -\frac{1}{3}\mathbf{a}_{146} + (\frac{2}{3})\mathbf{b}_{146} + (-\frac{1}{3})\mathbf{c}_{146}$

The reduction of higher dimensional irrep:

$$T_d : T_1 \rightarrow A + {}^2E + {}^1E \text{ of } C_3.$$

$$T_d : T_2 \rightarrow A + {}^2E + {}^1E \text{ of } C_3.$$

The correspondences of irreps at HSPs from original SG to lowered SG:

$$n_{GM4}^{146} = 2n_{GM8}^{215} \quad n_{GM6}^{146} = n_{GM6}^{215} + n_{GM7}^{215} + n_{GM8}^{215} \quad n_{GM5}^{146} = n_{GM6}^{215} + n_{GM7}^{215} + n_{GM8}^{215} \quad n_{L2}^{146} = 2n_{X6}^{215} + 2n_{X7}^{215} \quad n_{F2}^{146} = 2n_{M6}^{215} + 2n_{M7}^{215} \quad n_{T4}^{146} = 2n_{R8}^{215} \quad n_{T6}^{146} = n_{R6}^{215} + n_{R7}^{215} + n_{R8}^{215} \quad n_{T5}^{146} = n_{R6}^{215} + n_{R7}^{215} + n_{R8}^{215}$$

The lower SG is SG 146 when the preserved operations are: **(sub-SG label is 14) 1, 10, 9.**

The transformation is:  $(\mathbf{a}_{146}, \mathbf{b}_{146}, \mathbf{c}_{146}) = (\mathbf{a}_{215}, \mathbf{b}_{215}, \mathbf{c}_{215}) \begin{pmatrix} -1 & 0 & 0 \\ 0 & 1 & 0 \\ 0 & 0 & -1 \end{pmatrix}, \overrightarrow{O_{215}O_{146}} = -\frac{1}{3}\mathbf{a}_{146} + (\frac{2}{3})\mathbf{b}_{146} + (-\frac{1}{3})\mathbf{c}_{146}$

The reduction of higher dimensional irrep:

$$T_d : T_1 \rightarrow A + {}^2E + {}^1E \text{ of } C_3.$$

$$T_d : T_2 \rightarrow A + {}^2E + {}^1E \text{ of } C_3.$$

The correspondences of irreps at HSPs from original SG to lowered SG:

$$n_{GM4}^{146} = 2n_{GM8}^{215} \quad n_{GM6}^{146} = n_{GM6}^{215} + n_{GM7}^{215} + n_{GM8}^{215} \quad n_{GM5}^{146} = n_{GM6}^{215} + n_{GM7}^{215} + n_{GM8}^{215} \quad n_{L2}^{146} = 2n_{X6}^{215} + 2n_{X7}^{215} \quad n_{F2}^{146} = 2n_{M6}^{215} + 2n_{M7}^{215} \quad n_{T4}^{146} = 2n_{R8}^{215} \quad n_{T6}^{146} = n_{R6}^{215} + n_{R7}^{215} + n_{R8}^{215} \quad n_{T5}^{146} = n_{R6}^{215} + n_{R7}^{215} + n_{R8}^{215}$$

The lower SG is SG 195 when the preserved operations are: **(sub-SG label is 15) 1, 2, 3, 4, 5, 12, 8, 10, 6, 11, 7, 9.**

The transformation is:  $(\mathbf{a}_{195}, \mathbf{b}_{195}, \mathbf{c}_{195}) = (\mathbf{a}_{215}, \mathbf{b}_{215}, \mathbf{c}_{215}) \begin{pmatrix} 0 & 0 & 1 \\ 1 & 0 & 0 \\ 0 & 1 & 0 \end{pmatrix}, \overrightarrow{O_{215}O_{195}} = \mathbf{0}$

The reduction of higher dimensional irrep:

$$T_d : E \rightarrow {}^1E + {}^2E \text{ of } T.$$

The correspondences of irreps at HSPs from original SG to lowered SG:

$$n_{GM6}^{195} = n_{GM8}^{215} \quad n_{GM7}^{195} = n_{GM8}^{215} \quad n_{GM5}^{195} = n_{GM6}^{215} + n_{GM7}^{215} \quad n_{X5}^{195} = n_{X6}^{215} + n_{X7}^{215} \quad n_{M5}^{195} = n_{M6}^{215} + n_{M7}^{215} \quad n_{R6}^{195} = n_{R8}^{215} \quad n_{R7}^{195} = n_{R8}^{215} \quad n_{R5}^{195} = n_{R6}^{215} + n_{R7}^{215}$$

### 113. Lowered SGs by higher-dimensional irreps of pairings in SG 216

The representative operations of SG/T for SG 216:

$$1 : (x, y, z), 2 : (x, -y, -z), 3 : (-x, y, -z), 4 : (-x, -y, z), 5 : (z, x, y), 6 : (y, z, x), 7 : (-y, z, -x), 8 : (-z, -x, y), \\ 9 : (-y, -z, x), 10 : (z, -x, -y), 11 : (y, -z, -x), 12 : (-z, x, -y), 13 : (-x, z, -y), 14 : (-x, -z, y), 15 : (-z, -y, x), \\ 16 : (z, -y, -x), 17 : (y, -x, -z), 18 : (-y, x, -z), 19 : (-y, -x, z), 20 : (y, x, z), 21 : (x, -z, -y), 22 : (x, z, y), \\ 23 : (-z, y, -x), 24 : (z, y, x).$$

The lower SG is SG 22 when the preserved operations are: **(sub-SG label is 1) 1, 2, 3, 4.**

$$\text{The transformation is: } (\mathbf{a}_{22}, \mathbf{b}_{22}, \mathbf{c}_{22}) = (\mathbf{a}_{216}, \mathbf{b}_{216}, \mathbf{c}_{216}) \begin{pmatrix} 0 & 0 & 1 \\ 1 & 0 & 0 \\ 0 & 1 & 0 \end{pmatrix}, \overrightarrow{O_{216}O_{22}} = \frac{1}{4}\mathbf{a}_{22} + (-\frac{1}{4})\mathbf{b}_{22} + (-\frac{1}{4})\mathbf{c}_{22}$$

The reduction of higher dimensional irrep:

$$T_d : T_1 \rightarrow B_1 + B_2 + B_3 \text{ of } D_2.$$

$$T_d : T_2 \rightarrow B_1 + B_2 + B_3 \text{ of } D_2.$$

The correspondences of irreps at HSPs from original SG to lowered SG:

$$n_{GM5}^{22} = n_{GM6}^{216} + n_{GM7}^{216} + 2n_{GM8}^{216} \quad n_{Y5}^{22} = n_{X6}^{216} + n_{X7}^{216} \quad n_{L2}^{22} = n_{L4}^{216} + n_{L5}^{216} + 2n_{L6}^{216} \quad n_{Z5}^{22} = n_{X6}^{216} + n_{X7}^{216} \quad n_{T5}^{22} = n_{X6}^{216} + n_{X7}^{216}$$

The lower SG is SG 44 when the preserved operations are: **(sub-SG label is 2) 1, 4, 19, 20.**

$$\text{The transformation is: } (\mathbf{a}_{44}, \mathbf{b}_{44}, \mathbf{c}_{44}) = (\mathbf{a}_{216}, \mathbf{b}_{216}, \mathbf{c}_{216}) \begin{pmatrix} \frac{1}{2} & -\frac{1}{2} & 0 \\ \frac{1}{2} & \frac{1}{2} & 0 \\ 0 & 0 & 1 \end{pmatrix}, \overrightarrow{O_{216}O_{44}} = -\frac{1}{2}\mathbf{b}_{44}$$

The reduction of higher dimensional irrep:

$$T_d : T_1 \rightarrow A_2 + B_1 + B_2 \text{ of } C_{2v}.$$

$$T_d : T_2 \rightarrow A_1 + B_1 + B_2 \text{ of } C_{2v}.$$

The correspondences of irreps at HSPs from original SG to lowered SG:

$$n_{GM5}^{44} = n_{GM6}^{216} + n_{GM7}^{216} + 2n_{GM8}^{216} \quad n_{X5}^{44} = n_{X6}^{216} + n_{X7}^{216} \quad n_{T4}^{44} = n_{X6}^{216} + n_{X7}^{216} \quad n_{T3}^{44} = n_{X6}^{216} + n_{X7}^{216} \quad n_{W4}^{44} = n_{W7}^{216} + n_{W8}^{216} \quad n_{W3}^{44} = \\ n_{W5}^{216} + n_{W6}^{216} \quad n_{R4}^{44} = n_{L5}^{216} + n_{L6}^{216} \quad n_{R3}^{44} = n_{L4}^{216} + n_{L6}^{216} \quad n_{S3}^{44} = n_{L5}^{216} + n_{L6}^{216} \quad n_{S4}^{44} = n_{L4}^{216} + n_{L6}^{216}$$

The lower SG is SG 44 when the preserved operations are: **(sub-SG label is 3) 1, 2, 21, 22.**

$$\text{The transformation is: } (\mathbf{a}_{44}, \mathbf{b}_{44}, \mathbf{c}_{44}) = (\mathbf{a}_{216}, \mathbf{b}_{216}, \mathbf{c}_{216}) \begin{pmatrix} 0 & 0 & 1 \\ \frac{1}{2} & -\frac{1}{2} & 0 \\ \frac{1}{2} & \frac{1}{2} & 0 \end{pmatrix}, \overrightarrow{O_{216}O_{44}} = -\frac{1}{2}\mathbf{b}_{44}$$

The reduction of higher dimensional irrep:

$$T_d : T_1 \rightarrow A_2 + B_1 + B_2 \text{ of } C_{2v}.$$

$$T_d : T_2 \rightarrow A_1 + B_1 + B_2 \text{ of } C_{2v}.$$

The correspondences of irreps at HSPs from original SG to lowered SG:

$$n_{GM5}^{44} = n_{GM6}^{216} + n_{GM7}^{216} + 2n_{GM8}^{216} \quad n_{X5}^{44} = n_{X6}^{216} + n_{X7}^{216} \quad n_{T4}^{44} = n_{X6}^{216} + n_{X7}^{216} \quad n_{T3}^{44} = n_{X6}^{216} + n_{X7}^{216} \quad n_{W4}^{44} = n_{W7}^{216} + n_{W8}^{216} \quad n_{W3}^{44} = \\ n_{W5}^{216} + n_{W6}^{216} \quad n_{R4}^{44} = n_{L5}^{216} + n_{L6}^{216} \quad n_{R3}^{44} = n_{L4}^{216} + n_{L6}^{216} \quad n_{S3}^{44} = n_{L5}^{216} + n_{L6}^{216} \quad n_{S4}^{44} = n_{L4}^{216} + n_{L6}^{216}$$

The lower SG is SG 44 when the preserved operations are: **(sub-SG label is 4) 1, 3, 24, 23.**

$$\text{The transformation is: } (\mathbf{a}_{44}, \mathbf{b}_{44}, \mathbf{c}_{44}) = (\mathbf{a}_{216}, \mathbf{b}_{216}, \mathbf{c}_{216}) \begin{pmatrix} -\frac{1}{2} & \frac{1}{2} & 0 \\ 0 & 0 & 1 \\ \frac{1}{2} & \frac{1}{2} & 0 \end{pmatrix}, \overrightarrow{O_{216}O_{44}} = -\frac{1}{2}\mathbf{b}_{44}$$

The reduction of higher dimensional irrep:

$$T_d : T_1 \rightarrow A_2 + B_1 + B_2 \text{ of } C_{2v}.$$

$$T_d : T_2 \rightarrow A_1 + B_1 + B_2 \text{ of } C_{2v}.$$

The correspondences of irreps at HSPs from original SG to lowered SG:

$$n_{GM5}^{44} = n_{GM6}^{216} + n_{GM7}^{216} + 2n_{GM8}^{216} \quad n_{X5}^{44} = n_{X6}^{216} + n_{X7}^{216} \quad n_{T4}^{44} = n_{X6}^{216} + n_{X7}^{216} \quad n_{T3}^{44} = n_{X6}^{216} + n_{X7}^{216} \quad n_{W4}^{44} = n_{W7}^{216} + n_{W8}^{216} \quad n_{W3}^{44} = \\ n_{W5}^{216} + n_{W6}^{216} \quad n_{R4}^{44} = n_{L5}^{216} + n_{L6}^{216} \quad n_{R3}^{44} = n_{L4}^{216} + n_{L6}^{216} \quad n_{S3}^{44} = n_{L5}^{216} + n_{L6}^{216} \quad n_{S4}^{44} = n_{L4}^{216} + n_{L6}^{216}$$

The lower SG is SG 82 when the preserved operations are: **(sub-SG label is 5) 1, 17, 18, 4.**

$$\text{The transformation is: } (\mathbf{a}_{82}, \mathbf{b}_{82}, \mathbf{c}_{82}) = (\mathbf{a}_{216}, \mathbf{b}_{216}, \mathbf{c}_{216}) \begin{pmatrix} \frac{1}{2} & \frac{1}{2} & 0 \\ -\frac{1}{2} & \frac{1}{2} & 0 \\ 0 & 0 & 1 \end{pmatrix}, \overrightarrow{O_{216}O_{82}} = \frac{1}{2}\mathbf{a}_{82} + (-\frac{1}{2})\mathbf{b}_{82}$$

The reduction of higher dimensional irrep:

$$T_d : T_1 \rightarrow A + {}^2E + {}^1E \text{ of } S_4.$$

$$T_d : T_2 \rightarrow {}^2E + B + {}^1E \text{ of } S_4.$$

The correspondences of irreps at HSPs from original SG to lowered SG:

$$\begin{aligned} n_{GM7}^{82} &= n_{GM7}^{216} + n_{GM8}^{216} n_{GM8}^{82} = n_{GM6}^{216} + n_{GM8}^{216} n_{GM5}^{82} = n_{GM7}^{216} + n_{GM8}^{216} n_{GM6}^{82} = n_{GM6}^{216} + n_{GM8}^{216} n_{M7}^{82} = n_{X6}^{216} n_{M8}^{82} = n_{X7}^{216} \\ n_{M5}^{82} &= n_{X6}^{216} n_{M6}^{82} = n_{X7}^{216} n_{X4}^{82} = n_{X6}^{216} + n_{X7}^{216} n_{X3}^{82} = n_{X6}^{216} + n_{X7}^{216} n_{P7}^{82} = n_{W8}^{216} n_{P8}^{82} = n_{W7}^{216} n_{P5}^{82} = n_{W6}^{216} n_{P6}^{82} = n_{W5}^{216} n_{N2}^{82} = \\ &n_{L4}^{216} + n_{L5}^{216} + 2n_{L6}^{216} \end{aligned}$$

The lower SG is SG 82 when the preserved operations are: **(sub-SG label is 6) 1, 13, 14, 2.**

$$\text{The transformation is: } (\mathbf{a}_{82}, \mathbf{b}_{82}, \mathbf{c}_{82}) = (\mathbf{a}_{216}, \mathbf{b}_{216}, \mathbf{c}_{216}) \begin{pmatrix} 0 & 0 & 1 \\ -\frac{1}{2} & \frac{1}{2} & 0 \\ -\frac{1}{2} & -\frac{1}{2} & 0 \end{pmatrix}, \overrightarrow{O_{216}O_{82}} = \frac{1}{2}\mathbf{a}_{82} + (-\frac{1}{2})\mathbf{b}_{82}$$

The reduction of higher dimensional irrep:

$$T_d : T_1 \rightarrow A + {}^2E + {}^1E \text{ of } S_4.$$

$$T_d : T_2 \rightarrow {}^2E + B + {}^1E \text{ of } S_4.$$

The correspondences of irreps at HSPs from original SG to lowered SG:

$$\begin{aligned} n_{GM7}^{82} &= n_{GM7}^{216} + n_{GM8}^{216} n_{GM8}^{82} = n_{GM6}^{216} + n_{GM8}^{216} n_{GM5}^{82} = n_{GM7}^{216} + n_{GM8}^{216} n_{GM6}^{82} = n_{GM6}^{216} + n_{GM8}^{216} n_{M7}^{82} = n_{X6}^{216} n_{M8}^{82} = n_{X7}^{216} \\ n_{M5}^{82} &= n_{X6}^{216} n_{M6}^{82} = n_{X7}^{216} n_{X4}^{82} = n_{X6}^{216} + n_{X7}^{216} n_{X3}^{82} = n_{X6}^{216} + n_{X7}^{216} n_{P7}^{82} = n_{W8}^{216} n_{P8}^{82} = n_{W7}^{216} n_{P5}^{82} = n_{W6}^{216} n_{P6}^{82} = n_{W5}^{216} n_{N2}^{82} = \\ &n_{L4}^{216} + n_{L5}^{216} + 2n_{L6}^{216} \end{aligned}$$

The lower SG is SG 82 when the preserved operations are: **(sub-SG label is 7) 1, 15, 16, 3.**

$$\text{The transformation is: } (\mathbf{a}_{82}, \mathbf{b}_{82}, \mathbf{c}_{82}) = (\mathbf{a}_{216}, \mathbf{b}_{216}, \mathbf{c}_{216}) \begin{pmatrix} \frac{1}{2} & -\frac{1}{2} & 0 \\ 0 & 0 & 1 \\ -\frac{1}{2} & -\frac{1}{2} & 0 \end{pmatrix}, \overrightarrow{O_{216}O_{82}} = \frac{1}{2}\mathbf{a}_{82} + (-\frac{1}{2})\mathbf{b}_{82}$$

The reduction of higher dimensional irrep:

$$T_d : T_1 \rightarrow A + {}^2E + {}^1E \text{ of } S_4.$$

$$T_d : T_2 \rightarrow {}^2E + B + {}^1E \text{ of } S_4.$$

The correspondences of irreps at HSPs from original SG to lowered SG:

$$\begin{aligned} n_{GM7}^{82} &= n_{GM7}^{216} + n_{GM8}^{216} n_{GM8}^{82} = n_{GM6}^{216} + n_{GM8}^{216} n_{GM5}^{82} = n_{GM7}^{216} + n_{GM8}^{216} n_{GM6}^{82} = n_{GM6}^{216} + n_{GM8}^{216} n_{M7}^{82} = n_{X6}^{216} n_{M8}^{82} = n_{X7}^{216} \\ n_{M5}^{82} &= n_{X6}^{216} n_{M6}^{82} = n_{X7}^{216} n_{X4}^{82} = n_{X6}^{216} + n_{X7}^{216} n_{X3}^{82} = n_{X6}^{216} + n_{X7}^{216} n_{P7}^{82} = n_{W8}^{216} n_{P8}^{82} = n_{W7}^{216} n_{P5}^{82} = n_{W6}^{216} n_{P6}^{82} = n_{W5}^{216} n_{N2}^{82} = \\ &n_{L4}^{216} + n_{L5}^{216} + 2n_{L6}^{216} \end{aligned}$$

The lower SG is SG 119 when the preserved operations are: **(sub-SG label is 8) 1, 18, 17, 4, 2, 3, 19, 20.**

$$\text{The transformation is: } (\mathbf{a}_{119}, \mathbf{b}_{119}, \mathbf{c}_{119}) = (\mathbf{a}_{216}, \mathbf{b}_{216}, \mathbf{c}_{216}) \begin{pmatrix} \frac{1}{2} & -\frac{1}{2} & 0 \\ -\frac{1}{2} & -\frac{1}{2} & 0 \\ 0 & 0 & -1 \end{pmatrix}, \overrightarrow{O_{216}O_{119}} = \frac{1}{2}\mathbf{a}_{119} + (-\frac{1}{2})\mathbf{b}_{119}$$

The reduction of higher dimensional irrep:

$$T_d : E \rightarrow A_1 + B_1 \text{ of } D_{2d}.$$

The correspondences of irreps at HSPs from original SG to lowered SG:

$$\begin{aligned} n_{GM6}^{119} &= n_{GM7}^{216} + n_{GM8}^{216} n_{GM7}^{119} = n_{GM6}^{216} + n_{GM8}^{216} n_{M6}^{119} = n_{X6}^{216} n_{M7}^{119} = n_{X7}^{216} n_{X5}^{119} = n_{X6}^{216} + n_{X7}^{216} n_{P7}^{119} = n_{W6}^{216} n_{P8}^{119} = n_{W5}^{216} \\ n_{P5}^{119} &= n_{W8}^{216} n_{P6}^{119} = n_{W7}^{216} n_{N4}^{119} = n_{L5}^{216} + n_{L6}^{216} n_{N3}^{119} = n_{L4}^{216} + n_{L6}^{216} \end{aligned}$$

The lower SG is SG 119 when the preserved operations are: **(sub-SG label is 9) 1, 14, 13, 2, 3, 4, 21, 22.**

$$\text{The transformation is: } (\mathbf{a}_{119}, \mathbf{b}_{119}, \mathbf{c}_{119}) = (\mathbf{a}_{216}, \mathbf{b}_{216}, \mathbf{c}_{216}) \begin{pmatrix} 0 & 0 & -1 \\ -\frac{1}{2} & -\frac{1}{2} & 0 \\ -\frac{1}{2} & \frac{1}{2} & 0 \end{pmatrix}, \overrightarrow{O_{216}O_{119}} = \frac{1}{2}\mathbf{a}_{119} + (-\frac{1}{2})\mathbf{b}_{119}$$

The reduction of higher dimensional irrep:

$$T_d : E \rightarrow A_1 + B_1 \text{ of } D_{2d}.$$

The correspondences of irreps at HSPs from original SG to lowered SG:

$$\begin{aligned} n_{GM6}^{119} &= n_{GM7}^{216} + n_{GM8}^{216} n_{GM7}^{119} = n_{GM6}^{216} + n_{GM8}^{216} n_{M6}^{119} = n_{X6}^{216} n_{M7}^{119} = n_{X7}^{216} n_{X5}^{119} = n_{X6}^{216} + n_{X7}^{216} n_{P7}^{119} = n_{W8}^{216} n_{P8}^{119} = n_{W7}^{216} \\ n_{P5}^{119} &= n_{W6}^{216} n_{P6}^{119} = n_{W5}^{216} n_{N4}^{119} = n_{L5}^{216} + n_{L6}^{216} n_{N3}^{119} = n_{L4}^{216} + n_{L6}^{216} \end{aligned}$$

The lower SG is SG 119 when the preserved operations are: **(sub-SG label is 10) 1, 16, 15, 3, 4, 2, 24, 23.**

$$\text{The transformation is: } (\mathbf{a}_{119}, \mathbf{b}_{119}, \mathbf{c}_{119}) = (\mathbf{a}_{216}, \mathbf{b}_{216}, \mathbf{c}_{216}) \begin{pmatrix} \frac{1}{2} & \frac{1}{2} & 0 \\ 0 & 0 & -1 \\ -\frac{1}{2} & \frac{1}{2} & 0 \end{pmatrix}, \overrightarrow{O_{216}O_{119}} = \frac{1}{2}\mathbf{a}_{119} + (-\frac{1}{2})\mathbf{b}_{119}$$

The reduction of higher dimensional irrep:

$$T_d : E \rightarrow A_1 + B_1 \text{ of } D_{2d}.$$

The correspondences of irreps at HSPs from original SG to lowered SG:

$$\begin{aligned} n_{GM6}^{119} &= n_{GM7}^{216} + n_{GM8}^{216} & n_{GM7}^{119} &= n_{GM6}^{216} + n_{GM8}^{216} & n_{M6}^{119} &= n_{X6}^{216} & n_{M7}^{119} &= n_{X7}^{216} & n_{X5}^{119} &= n_{X6}^{216} + n_{X7}^{216} & n_{P7}^{119} &= n_{W6}^{216} & n_{P8}^{119} &= n_{W5}^{216} \\ n_{P5}^{119} &= n_{W8}^{216} & n_{P6}^{119} &= n_{W7}^{216} & n_{N4}^{119} &= n_{L5}^{216} + n_{L6}^{216} & n_{N3}^{119} &= n_{L4}^{216} + n_{L6}^{216} \end{aligned}$$

The lower SG is SG 146 when the preserved operations are: **(sub-SG label is 11) 1, 5, 6.**

$$\text{The transformation is: } (\mathbf{a}_{146}, \mathbf{b}_{146}, \mathbf{c}_{146}) = (\mathbf{a}_{216}, \mathbf{b}_{216}, \mathbf{c}_{216}) \begin{pmatrix} \frac{1}{2} & 0 & \frac{1}{2} \\ \frac{1}{2} & \frac{1}{2} & 0 \\ 0 & \frac{1}{2} & \frac{1}{2} \end{pmatrix}, \overrightarrow{O_{216}O_{146}} = -\frac{1}{3}\mathbf{a}_{146} + \left(\frac{2}{3}\right)\mathbf{b}_{146} + \left(-\frac{1}{3}\right)\mathbf{c}_{146}$$

The reduction of higher dimensional irrep:

$$T_d : T_1 \rightarrow A + {}^2E + {}^1E \text{ of } C_3.$$

$$T_d : T_2 \rightarrow A + {}^2E + {}^1E \text{ of } C_3.$$

The correspondences of irreps at HSPs from original SG to lowered SG:

$$\begin{aligned} n_{GM4}^{146} &= 2n_{GM8}^{216} & n_{GM6}^{146} &= n_{GM6}^{216} + n_{GM7}^{216} + n_{GM8}^{216} & n_{GM5}^{146} &= n_{GM6}^{216} + n_{GM7}^{216} + n_{GM8}^{216} & n_{L2}^{146} &= n_{L4}^{216} + n_{L5}^{216} + 2n_{L6}^{216} & n_{F2}^{146} &= \\ 2n_{X6}^{216} + 2n_{X7}^{216} & n_{T4}^{146} &= n_{L4}^{216} + n_{L5}^{216} & n_{T6}^{146} &= n_{L6}^{216} & n_{T5}^{146} &= n_{L6}^{216} \end{aligned}$$

The lower SG is SG 146 when the preserved operations are: **(sub-SG label is 12) 1, 12, 11.**

$$\text{The transformation is: } (\mathbf{a}_{146}, \mathbf{b}_{146}, \mathbf{c}_{146}) = (\mathbf{a}_{216}, \mathbf{b}_{216}, \mathbf{c}_{216}) \begin{pmatrix} -\frac{1}{2} & -\frac{1}{2} & 0 \\ 0 & -\frac{1}{2} & -\frac{1}{2} \\ \frac{1}{2} & 0 & \frac{1}{2} \end{pmatrix}, \overrightarrow{O_{216}O_{146}} = -\frac{1}{3}\mathbf{a}_{146} + \left(\frac{2}{3}\right)\mathbf{b}_{146} + \left(-\frac{1}{3}\right)\mathbf{c}_{146}$$

The reduction of higher dimensional irrep:

$$T_d : T_1 \rightarrow A + {}^2E + {}^1E \text{ of } C_3.$$

$$T_d : T_2 \rightarrow A + {}^2E + {}^1E \text{ of } C_3.$$

The correspondences of irreps at HSPs from original SG to lowered SG:

$$\begin{aligned} n_{GM4}^{146} &= 2n_{GM8}^{216} & n_{GM6}^{146} &= n_{GM6}^{216} + n_{GM7}^{216} + n_{GM8}^{216} & n_{GM5}^{146} &= n_{GM6}^{216} + n_{GM7}^{216} + n_{GM8}^{216} & n_{L2}^{146} &= n_{L4}^{216} + n_{L5}^{216} + 2n_{L6}^{216} & n_{F2}^{146} &= \\ 2n_{X6}^{216} + 2n_{X7}^{216} & n_{T4}^{146} &= n_{L4}^{216} + n_{L5}^{216} & n_{T6}^{146} &= n_{L6}^{216} & n_{T5}^{146} &= n_{L6}^{216} \end{aligned}$$

The lower SG is SG 146 when the preserved operations are: **(sub-SG label is 13) 1, 8, 7.**

$$\text{The transformation is: } (\mathbf{a}_{146}, \mathbf{b}_{146}, \mathbf{c}_{146}) = (\mathbf{a}_{216}, \mathbf{b}_{216}, \mathbf{c}_{216}) \begin{pmatrix} \frac{1}{2} & 0 & \frac{1}{2} \\ -\frac{1}{2} & -\frac{1}{2} & 0 \\ 0 & -\frac{1}{2} & -\frac{1}{2} \end{pmatrix}, \overrightarrow{O_{216}O_{146}} = -\frac{1}{3}\mathbf{a}_{146} + \left(\frac{2}{3}\right)\mathbf{b}_{146} + \left(-\frac{1}{3}\right)\mathbf{c}_{146}$$

The reduction of higher dimensional irrep:

$$T_d : T_1 \rightarrow A + {}^2E + {}^1E \text{ of } C_3.$$

$$T_d : T_2 \rightarrow A + {}^2E + {}^1E \text{ of } C_3.$$

The correspondences of irreps at HSPs from original SG to lowered SG:

$$\begin{aligned} n_{GM4}^{146} &= 2n_{GM8}^{216} & n_{GM6}^{146} &= n_{GM6}^{216} + n_{GM7}^{216} + n_{GM8}^{216} & n_{GM5}^{146} &= n_{GM6}^{216} + n_{GM7}^{216} + n_{GM8}^{216} & n_{L2}^{146} &= n_{L4}^{216} + n_{L5}^{216} + 2n_{L6}^{216} & n_{F2}^{146} &= \\ 2n_{X6}^{216} + 2n_{X7}^{216} & n_{T4}^{146} &= n_{L4}^{216} + n_{L5}^{216} & n_{T6}^{146} &= n_{L6}^{216} & n_{T5}^{146} &= n_{L6}^{216} \end{aligned}$$

The lower SG is SG 146 when the preserved operations are: **(sub-SG label is 14) 1, 10, 9.**

$$\text{The transformation is: } (\mathbf{a}_{146}, \mathbf{b}_{146}, \mathbf{c}_{146}) = (\mathbf{a}_{216}, \mathbf{b}_{216}, \mathbf{c}_{216}) \begin{pmatrix} -\frac{1}{2} & -\frac{1}{2} & 0 \\ 0 & \frac{1}{2} & \frac{1}{2} \\ -\frac{1}{2} & 0 & -\frac{1}{2} \end{pmatrix}, \overrightarrow{O_{216}O_{146}} = -\frac{1}{3}\mathbf{a}_{146} + \left(\frac{2}{3}\right)\mathbf{b}_{146} + \left(-\frac{1}{3}\right)\mathbf{c}_{146}$$

The reduction of higher dimensional irrep:

$$T_d : T_1 \rightarrow A + {}^2E + {}^1E \text{ of } C_3.$$

$$T_d : T_2 \rightarrow A + {}^2E + {}^1E \text{ of } C_3.$$

The correspondences of irreps at HSPs from original SG to lowered SG:

$$\begin{aligned} n_{GM4}^{146} &= 2n_{GM8}^{216} & n_{GM6}^{146} &= n_{GM6}^{216} + n_{GM7}^{216} + n_{GM8}^{216} & n_{GM5}^{146} &= n_{GM6}^{216} + n_{GM7}^{216} + n_{GM8}^{216} & n_{L2}^{146} &= n_{L4}^{216} + n_{L5}^{216} + 2n_{L6}^{216} & n_{F2}^{146} &= \\ 2n_{X6}^{216} + 2n_{X7}^{216} & n_{T4}^{146} &= n_{L4}^{216} + n_{L5}^{216} & n_{T6}^{146} &= n_{L6}^{216} & n_{T5}^{146} &= n_{L6}^{216} \end{aligned}$$

The lower SG is SG 196 when the preserved operations are: **(sub-SG label is 15) 1, 2, 3, 4, 5, 12, 8, 10, 6, 11, 7, 9.**

$$\text{The transformation is: } (\mathbf{a}_{196}, \mathbf{b}_{196}, \mathbf{c}_{196}) = (\mathbf{a}_{216}, \mathbf{b}_{216}, \mathbf{c}_{216}) \begin{pmatrix} 0 & 0 & 1 \\ 1 & 0 & 0 \\ 0 & 1 & 0 \end{pmatrix}, \overrightarrow{O_{216}O_{196}} = \frac{1}{4}\mathbf{a}_{196} + \left(\frac{1}{4}\right)\mathbf{b}_{196} + \left(\frac{1}{4}\right)\mathbf{c}_{196}$$

The reduction of higher dimensional irrep:

$$T_d : E \rightarrow {}^1E + {}^2E \text{ of } T.$$

The correspondences of irreps at HSPs from original SG to lowered SG:

$$\begin{aligned} n_{GM6}^{196} &= n_{GM8}^{216} & n_{GM7}^{196} &= n_{GM8}^{216} & n_{GM5}^{196} &= n_{GM6}^{216} + n_{GM7}^{216} & n_{X5}^{196} &= n_{X6}^{216} + n_{X7}^{216} & n_{L4}^{196} &= n_{L4}^{216} + n_{L5}^{216} & n_{L6}^{196} &= n_{L6}^{216} & n_{L5}^{196} &= n_{L6}^{216} \\ n_{W4}^{196} &= n_{W5}^{216} + n_{W6}^{216} & n_{W3}^{196} &= n_{W7}^{216} + n_{W8}^{216} \end{aligned}$$

#### 114. Lowered SGs by higher-dimensional irreps of pairings in SG 217

The representative operations of SG/T for SG 217:

$$\begin{aligned}
 &1 : (x, y, z), 2 : (x, -y, -z), 3 : (-x, y, -z), 4 : (-x, -y, z), 5 : (z, x, y), 6 : (y, z, x), 7 : (-y, z, -x), 8 : (-z, -x, y), \\
 &9 : (-y, -z, x), 10 : (z, -x, -y), 11 : (y, -z, -x), 12 : (-z, x, -y), 13 : (-x, z, -y), 14 : (-x, -z, y), 15 : (-z, -y, x), \\
 &16 : (z, -y, -x), 17 : (y, -x, -z), 18 : (-y, x, -z), 19 : (-y, -x, z), 20 : (y, x, z), 21 : (x, -z, -y), 22 : (x, z, y), \\
 &23 : (-z, y, -x), 24 : (z, y, x).
 \end{aligned}$$

The lower SG is SG 23 when the preserved operations are: **(sub-SG label is 1) 1, 2, 3, 4.**

$$\text{The transformation is: } (\mathbf{a}_{23}, \mathbf{b}_{23}, \mathbf{c}_{23}) = (\mathbf{a}_{217}, \mathbf{b}_{217}, \mathbf{c}_{217}) \begin{pmatrix} 0 & 0 & 1 \\ 1 & 0 & 0 \\ 0 & 1 & 0 \end{pmatrix}, \overrightarrow{O_{217}O_{23}} = -\frac{1}{2}\mathbf{b}_{23}$$

The reduction of higher dimensional irrep:

$$T_d : T_1 \rightarrow B_1 + B_2 + B_3 \text{ of } D_2.$$

$$T_d : T_2 \rightarrow B_1 + B_2 + B_3 \text{ of } D_2.$$

The correspondences of irreps at HSPs from original SG to lowered SG:

$$\begin{aligned}
 n_{GM5}^{23} &= n_{GM6}^{217} + n_{GM7}^{217} + 2n_{GM8}^{217} \quad n_{X5}^{23} = n_{H6}^{217} + n_{H7}^{217} + 2n_{H8}^{217} \quad n_{T4}^{23} = n_{N5}^{217} \quad n_{T3}^{23} = n_{N5}^{217} \quad n_{W5}^{23} = n_{P6}^{217} + n_{P7}^{217} + 2n_{P8}^{217} \quad n_{R4}^{23} = \\
 n_{N5}^{217} \quad n_{R3}^{23} &= n_{N5}^{217} \quad n_{S3}^{23} = n_{N5}^{217} \quad n_{S4}^{23} = n_{N5}^{217}
 \end{aligned}$$

The lower SG is SG 42 when the preserved operations are: **(sub-SG label is 2) 1, 4, 19, 20.**

$$\text{The transformation is: } (\mathbf{a}_{42}, \mathbf{b}_{42}, \mathbf{c}_{42}) = (\mathbf{a}_{217}, \mathbf{b}_{217}, \mathbf{c}_{217}) \begin{pmatrix} 1 & -1 & 0 \\ 1 & 1 & 0 \\ 0 & 0 & 1 \end{pmatrix}, \overrightarrow{O_{217}O_{42}} = \mathbf{0}$$

The reduction of higher dimensional irrep:

$$T_d : T_1 \rightarrow A_2 + B_1 + B_2 \text{ of } C_{2v}.$$

$$T_d : T_2 \rightarrow A_1 + B_1 + B_2 \text{ of } C_{2v}.$$

The correspondences of irreps at HSPs from original SG to lowered SG:

$$n_{GM5}^{42} = n_{GM6}^{217} + n_{GM7}^{217} + 2n_{GM8}^{217} \quad n_{Y5}^{42} = n_{N5}^{217} \quad n_{L2}^{42} = 2n_{N5}^{217} \quad n_{Z5}^{42} = n_{H6}^{217} + n_{H7}^{217} + 2n_{H8}^{217} \quad n_{T5}^{42} = n_{N5}^{217}$$

The lower SG is SG 42 when the preserved operations are: **(sub-SG label is 3) 1, 2, 21, 22.**

$$\text{The transformation is: } (\mathbf{a}_{42}, \mathbf{b}_{42}, \mathbf{c}_{42}) = (\mathbf{a}_{217}, \mathbf{b}_{217}, \mathbf{c}_{217}) \begin{pmatrix} 0 & 0 & 1 \\ 1 & -1 & 0 \\ 1 & 1 & 0 \end{pmatrix}, \overrightarrow{O_{217}O_{42}} = \mathbf{0}$$

The reduction of higher dimensional irrep:

$$T_d : T_1 \rightarrow A_2 + B_1 + B_2 \text{ of } C_{2v}.$$

$$T_d : T_2 \rightarrow A_1 + B_1 + B_2 \text{ of } C_{2v}.$$

The correspondences of irreps at HSPs from original SG to lowered SG:

$$n_{GM5}^{42} = n_{GM6}^{217} + n_{GM7}^{217} + 2n_{GM8}^{217} \quad n_{Y5}^{42} = n_{N5}^{217} \quad n_{L2}^{42} = 2n_{N5}^{217} \quad n_{Z5}^{42} = n_{H6}^{217} + n_{H7}^{217} + 2n_{H8}^{217} \quad n_{T5}^{42} = n_{N5}^{217}$$

The lower SG is SG 42 when the preserved operations are: **(sub-SG label is 4) 1, 3, 24, 23.**

$$\text{The transformation is: } (\mathbf{a}_{42}, \mathbf{b}_{42}, \mathbf{c}_{42}) = (\mathbf{a}_{217}, \mathbf{b}_{217}, \mathbf{c}_{217}) \begin{pmatrix} -1 & 1 & 0 \\ 0 & 0 & 1 \\ 1 & 1 & 0 \end{pmatrix}, \overrightarrow{O_{217}O_{42}} = \mathbf{0}$$

The reduction of higher dimensional irrep:

$$T_d : T_1 \rightarrow A_2 + B_1 + B_2 \text{ of } C_{2v}.$$

$$T_d : T_2 \rightarrow A_1 + B_1 + B_2 \text{ of } C_{2v}.$$

The correspondences of irreps at HSPs from original SG to lowered SG:

$$n_{GM5}^{42} = n_{GM6}^{217} + n_{GM7}^{217} + 2n_{GM8}^{217} \quad n_{Y5}^{42} = n_{N5}^{217} \quad n_{L2}^{42} = 2n_{N5}^{217} \quad n_{Z5}^{42} = n_{H6}^{217} + n_{H7}^{217} + 2n_{H8}^{217} \quad n_{T5}^{42} = n_{N5}^{217}$$

The lower SG is SG 82 when the preserved operations are: **(sub-SG label is 5) 1, 17, 18, 4.**

The transformation is:  $(\mathbf{a}_{82}, \mathbf{b}_{82}, \mathbf{c}_{82}) = (\mathbf{a}_{217}, \mathbf{b}_{217}, \mathbf{c}_{217}) \begin{pmatrix} 0 & 1 & 0 \\ -1 & 0 & 0 \\ 0 & 0 & 1 \end{pmatrix}, \overrightarrow{O_{217}O_{82}} = \frac{1}{2}\mathbf{a}_{82} + (-\frac{1}{2})\mathbf{b}_{82}$

The reduction of higher dimensional irrep:

$$T_d : T_1 \rightarrow A + {}^2E + {}^1E \text{ of } S_4.$$

$$T_d : T_2 \rightarrow {}^2E + B + {}^1E \text{ of } S_4.$$

The correspondences of irreps at HSPs from original SG to lowered SG:

$$\begin{aligned} n_{GM7}^{82} &= n_{GM7}^{217} + n_{GM8}^{217} & n_{GM8}^{82} &= n_{GM6}^{217} + n_{GM8}^{217} & n_{GM5}^{82} &= n_{GM7}^{217} + n_{GM8}^{217} & n_{GM6}^{82} &= n_{GM6}^{217} + n_{GM8}^{217} & n_{M7}^{82} &= n_{H7}^{217} + n_{H8}^{217} \\ n_{M8}^{82} &= n_{H6}^{217} + n_{H8}^{217} & n_{M5}^{82} &= n_{H7}^{217} + n_{H8}^{217} & n_{M6}^{82} &= n_{H6}^{217} + n_{H8}^{217} & n_{X4}^{82} &= n_{N5}^{217} & n_{X3}^{82} &= n_{N5}^{217} & n_{P7}^{82} &= n_{P6}^{217} + n_{P8}^{217} & n_{P8}^{82} &= n_{P7}^{217} + n_{P8}^{217} \\ n_{P5}^{82} &= n_{P6}^{217} + n_{P8}^{217} & n_{P6}^{82} &= n_{P7}^{217} + n_{P8}^{217} & n_{N2}^{82} &= 2n_{N5}^{217} \end{aligned}$$

The lower SG is SG 82 when the preserved operations are: **(sub-SG label is 6) 1, 13, 14, 2.**

The transformation is:  $(\mathbf{a}_{82}, \mathbf{b}_{82}, \mathbf{c}_{82}) = (\mathbf{a}_{217}, \mathbf{b}_{217}, \mathbf{c}_{217}) \begin{pmatrix} 0 & 0 & 1 \\ 0 & 1 & 0 \\ -1 & 0 & 0 \end{pmatrix}, \overrightarrow{O_{217}O_{82}} = \frac{1}{2}\mathbf{a}_{82} + (-\frac{1}{2})\mathbf{b}_{82}$

The reduction of higher dimensional irrep:

$$T_d : T_1 \rightarrow A + {}^2E + {}^1E \text{ of } S_4.$$

$$T_d : T_2 \rightarrow {}^2E + B + {}^1E \text{ of } S_4.$$

The correspondences of irreps at HSPs from original SG to lowered SG:

$$\begin{aligned} n_{GM7}^{82} &= n_{GM7}^{217} + n_{GM8}^{217} & n_{GM8}^{82} &= n_{GM6}^{217} + n_{GM8}^{217} & n_{GM5}^{82} &= n_{GM7}^{217} + n_{GM8}^{217} & n_{GM6}^{82} &= n_{GM6}^{217} + n_{GM8}^{217} & n_{M7}^{82} &= n_{H7}^{217} + n_{H8}^{217} \\ n_{M8}^{82} &= n_{H6}^{217} + n_{H8}^{217} & n_{M5}^{82} &= n_{H7}^{217} + n_{H8}^{217} & n_{M6}^{82} &= n_{H6}^{217} + n_{H8}^{217} & n_{X4}^{82} &= n_{N5}^{217} & n_{X3}^{82} &= n_{N5}^{217} & n_{P7}^{82} &= n_{P6}^{217} + n_{P8}^{217} & n_{P8}^{82} &= n_{P7}^{217} + n_{P8}^{217} \\ n_{P5}^{82} &= n_{P6}^{217} + n_{P8}^{217} & n_{P6}^{82} &= n_{P7}^{217} + n_{P8}^{217} & n_{N2}^{82} &= 2n_{N5}^{217} \end{aligned}$$

The lower SG is SG 82 when the preserved operations are: **(sub-SG label is 7) 1, 15, 16, 3.**

The transformation is:  $(\mathbf{a}_{82}, \mathbf{b}_{82}, \mathbf{c}_{82}) = (\mathbf{a}_{217}, \mathbf{b}_{217}, \mathbf{c}_{217}) \begin{pmatrix} 0 & -1 & 0 \\ 0 & 0 & 1 \\ -1 & 0 & 0 \end{pmatrix}, \overrightarrow{O_{217}O_{82}} = \frac{1}{2}\mathbf{a}_{82} + (-\frac{1}{2})\mathbf{b}_{82}$

The reduction of higher dimensional irrep:

$$T_d : T_1 \rightarrow A + {}^2E + {}^1E \text{ of } S_4.$$

$$T_d : T_2 \rightarrow {}^2E + B + {}^1E \text{ of } S_4.$$

The correspondences of irreps at HSPs from original SG to lowered SG:

$$\begin{aligned} n_{GM7}^{82} &= n_{GM7}^{217} + n_{GM8}^{217} & n_{GM8}^{82} &= n_{GM6}^{217} + n_{GM8}^{217} & n_{GM5}^{82} &= n_{GM7}^{217} + n_{GM8}^{217} & n_{GM6}^{82} &= n_{GM6}^{217} + n_{GM8}^{217} & n_{M7}^{82} &= n_{H7}^{217} + n_{H8}^{217} \\ n_{M8}^{82} &= n_{H6}^{217} + n_{H8}^{217} & n_{M5}^{82} &= n_{H7}^{217} + n_{H8}^{217} & n_{M6}^{82} &= n_{H6}^{217} + n_{H8}^{217} & n_{X4}^{82} &= n_{N5}^{217} & n_{X3}^{82} &= n_{N5}^{217} & n_{P7}^{82} &= n_{P6}^{217} + n_{P8}^{217} & n_{P8}^{82} &= n_{P7}^{217} + n_{P8}^{217} \\ n_{P5}^{82} &= n_{P6}^{217} + n_{P8}^{217} & n_{P6}^{82} &= n_{P7}^{217} + n_{P8}^{217} & n_{N2}^{82} &= 2n_{N5}^{217} \end{aligned}$$

The lower SG is SG 121 when the preserved operations are: **(sub-SG label is 8) 1, 18, 17, 4, 2, 3, 19, 20.**

The transformation is:  $(\mathbf{a}_{121}, \mathbf{b}_{121}, \mathbf{c}_{121}) = (\mathbf{a}_{217}, \mathbf{b}_{217}, \mathbf{c}_{217}) \begin{pmatrix} 0 & -1 & 0 \\ -1 & 0 & 0 \\ 0 & 0 & -1 \end{pmatrix}, \overrightarrow{O_{217}O_{121}} = \frac{1}{2}\mathbf{a}_{121} + (-\frac{1}{2})\mathbf{b}_{121}$

The reduction of higher dimensional irrep:

$$T_d : E \rightarrow A_1 + B_1 \text{ of } D_{2d}.$$

The correspondences of irreps at HSPs from original SG to lowered SG:

$$\begin{aligned} n_{GM6}^{121} &= n_{GM7}^{217} + n_{GM8}^{217} & n_{GM7}^{121} &= n_{GM6}^{217} + n_{GM8}^{217} & n_{M6}^{121} &= n_{H7}^{217} + n_{H8}^{217} & n_{M7}^{121} &= n_{H6}^{217} + n_{H8}^{217} & n_{X5}^{121} &= n_{N5}^{217} & n_{P6}^{121} &= n_{P6}^{217} + n_{P8}^{217} \\ n_{P7}^{121} &= n_{P7}^{217} + n_{P8}^{217} & n_{N4}^{121} &= n_{N5}^{217} & n_{N3}^{121} &= n_{N5}^{217} \end{aligned}$$

The lower SG is SG 121 when the preserved operations are: **(sub-SG label is 9) 1, 14, 13, 2, 3, 4, 21, 22.**

The transformation is:  $(\mathbf{a}_{121}, \mathbf{b}_{121}, \mathbf{c}_{121}) = (\mathbf{a}_{217}, \mathbf{b}_{217}, \mathbf{c}_{217}) \begin{pmatrix} 0 & 0 & -1 \\ 0 & -1 & 0 \\ -1 & 0 & 0 \end{pmatrix}, \overrightarrow{O_{217}O_{121}} = \frac{1}{2}\mathbf{a}_{121} + (-\frac{1}{2})\mathbf{b}_{121}$

The reduction of higher dimensional irrep:

$$T_d : E \rightarrow A_1 + B_1 \text{ of } D_{2d}.$$

The correspondences of irreps at HSPs from original SG to lowered SG:

$$\begin{aligned} n_{GM6}^{121} &= n_{GM7}^{217} + n_{GM8}^{217} & n_{GM7}^{121} &= n_{GM6}^{217} + n_{GM8}^{217} & n_{M6}^{121} &= n_{H7}^{217} + n_{H8}^{217} & n_{M7}^{121} &= n_{H6}^{217} + n_{H8}^{217} & n_{X5}^{121} &= n_{N5}^{217} & n_{P6}^{121} &= n_{P6}^{217} + n_{P8}^{217} \\ n_{P7}^{121} &= n_{P7}^{217} + n_{P8}^{217} & n_{N4}^{121} &= n_{N5}^{217} & n_{N3}^{121} &= n_{N5}^{217} \end{aligned}$$

The lower SG is SG 121 when the preserved operations are: **(sub-SG label is 10) 1, 16, 15, 3, 4, 2, 24, 23.**

The transformation is:  $(\mathbf{a}_{121}, \mathbf{b}_{121}, \mathbf{c}_{121}) = (\mathbf{a}_{217}, \mathbf{b}_{217}, \mathbf{c}_{217}) \begin{pmatrix} 0 & 1 & 0 \\ 0 & 0 & -1 \\ -1 & 0 & 0 \end{pmatrix}, \overrightarrow{O_{217}O_{121}} = \frac{1}{2}\mathbf{a}_{121} + (-\frac{1}{2})\mathbf{b}_{121}$

The reduction of higher dimensional irrep:

$$T_d : E \rightarrow A_1 + B_1 \text{ of } D_{2d}.$$

The correspondences of irreps at HSPs from original SG to lowered SG:

$$\begin{aligned} n_{GM6}^{121} &= n_{GM7}^{217} + n_{GM8}^{217} & n_{GM7}^{121} &= n_{GM6}^{217} + n_{GM8}^{217} & n_{M6}^{121} &= n_{H7}^{217} + n_{H8}^{217} & n_{M7}^{121} &= n_{H6}^{217} + n_{H8}^{217} & n_{X5}^{121} &= n_{N5}^{217} & n_{P6}^{121} &= n_{P6}^{217} + n_{P8}^{217} \\ n_{P7}^{121} &= n_{P7}^{217} + n_{P8}^{217} & n_{N4}^{121} &= n_{N5}^{217} & n_{N3}^{121} &= n_{N5}^{217} \end{aligned}$$

The lower SG is SG 146 when the preserved operations are: **(sub-SG label is 11) 1, 5, 6.**

The transformation is:  $(\mathbf{a}_{146}, \mathbf{b}_{146}, \mathbf{c}_{146}) = (\mathbf{a}_{217}, \mathbf{b}_{217}, \mathbf{c}_{217}) \begin{pmatrix} \frac{1}{2} & -\frac{1}{2} & \frac{1}{2} \\ \frac{1}{2} & \frac{1}{2} & -\frac{1}{2} \\ -\frac{1}{2} & \frac{1}{2} & \frac{1}{2} \end{pmatrix}, \overrightarrow{O_{217}O_{146}} = -\frac{1}{3}\mathbf{a}_{146} + (\frac{2}{3})\mathbf{b}_{146} + (-\frac{1}{3})\mathbf{c}_{146}$

The reduction of higher dimensional irrep:

$$T_d : T_1 \rightarrow A + {}^2E + {}^1E \text{ of } C_3.$$

$$T_d : T_2 \rightarrow A + {}^2E + {}^1E \text{ of } C_3.$$

The correspondences of irreps at HSPs from original SG to lowered SG:

$$\begin{aligned} n_{GM4}^{146} &= 2n_{GM8}^{217} & n_{GM6}^{146} &= n_{GM6}^{217} + n_{GM7}^{217} + n_{GM8}^{217} & n_{GM5}^{146} &= n_{GM6}^{217} + n_{GM7}^{217} + n_{GM8}^{217} & n_{L2}^{146} &= 2n_{N5}^{217} & n_{F2}^{146} &= 2n_{N5}^{217} & n_{T4}^{146} &= 2n_{N5}^{217} \\ 2n_{H8}^{217} n_{T6}^{146} &= n_{H6}^{217} + n_{H7}^{217} + n_{H8}^{217} & n_{T5}^{146} &= n_{H6}^{217} + n_{H7}^{217} + n_{H8}^{217} \end{aligned}$$

The lower SG is SG 146 when the preserved operations are: **(sub-SG label is 12) 1, 12, 11.**

The transformation is:  $(\mathbf{a}_{146}, \mathbf{b}_{146}, \mathbf{c}_{146}) = (\mathbf{a}_{217}, \mathbf{b}_{217}, \mathbf{c}_{217}) \begin{pmatrix} -\frac{1}{2} & -\frac{1}{2} & \frac{1}{2} \\ \frac{1}{2} & -\frac{1}{2} & -\frac{1}{2} \\ \frac{1}{2} & -\frac{1}{2} & \frac{1}{2} \end{pmatrix}, \overrightarrow{O_{217}O_{146}} = -\frac{1}{3}\mathbf{a}_{146} + (\frac{2}{3})\mathbf{b}_{146} + (-\frac{1}{3})\mathbf{c}_{146}$

The reduction of higher dimensional irrep:

$$T_d : T_1 \rightarrow A + {}^2E + {}^1E \text{ of } C_3.$$

$$T_d : T_2 \rightarrow A + {}^2E + {}^1E \text{ of } C_3.$$

The correspondences of irreps at HSPs from original SG to lowered SG:

$$\begin{aligned} n_{GM4}^{146} &= 2n_{GM8}^{217} & n_{GM6}^{146} &= n_{GM6}^{217} + n_{GM7}^{217} + n_{GM8}^{217} & n_{GM5}^{146} &= n_{GM6}^{217} + n_{GM7}^{217} + n_{GM8}^{217} & n_{L2}^{146} &= 2n_{N5}^{217} & n_{F2}^{146} &= 2n_{N5}^{217} & n_{T4}^{146} &= 2n_{N5}^{217} \\ 2n_{H8}^{217} n_{T6}^{146} &= n_{H6}^{217} + n_{H7}^{217} + n_{H8}^{217} & n_{T5}^{146} &= n_{H6}^{217} + n_{H7}^{217} + n_{H8}^{217} \end{aligned}$$

The lower SG is SG 146 when the preserved operations are: **(sub-SG label is 13) 1, 8, 7.**

The transformation is:  $(\mathbf{a}_{146}, \mathbf{b}_{146}, \mathbf{c}_{146}) = (\mathbf{a}_{217}, \mathbf{b}_{217}, \mathbf{c}_{217}) \begin{pmatrix} \frac{1}{2} & -\frac{1}{2} & \frac{1}{2} \\ -\frac{1}{2} & -\frac{1}{2} & \frac{1}{2} \\ \frac{1}{2} & -\frac{1}{2} & -\frac{1}{2} \end{pmatrix}, \overrightarrow{O_{217}O_{146}} = -\frac{1}{3}\mathbf{a}_{146} + (\frac{2}{3})\mathbf{b}_{146} + (-\frac{1}{3})\mathbf{c}_{146}$

The reduction of higher dimensional irrep:

$$T_d : T_1 \rightarrow A + {}^2E + {}^1E \text{ of } C_3.$$

$$T_d : T_2 \rightarrow A + {}^2E + {}^1E \text{ of } C_3.$$

The correspondences of irreps at HSPs from original SG to lowered SG:

$$\begin{aligned} n_{GM4}^{146} &= 2n_{GM8}^{217} & n_{GM6}^{146} &= n_{GM6}^{217} + n_{GM7}^{217} + n_{GM8}^{217} & n_{GM5}^{146} &= n_{GM6}^{217} + n_{GM7}^{217} + n_{GM8}^{217} & n_{L2}^{146} &= 2n_{N5}^{217} & n_{F2}^{146} &= 2n_{N5}^{217} & n_{T4}^{146} &= 2n_{N5}^{217} \\ 2n_{H8}^{217} n_{T6}^{146} &= n_{H6}^{217} + n_{H7}^{217} + n_{H8}^{217} & n_{T5}^{146} &= n_{H6}^{217} + n_{H7}^{217} + n_{H8}^{217} \end{aligned}$$

The lower SG is SG 146 when the preserved operations are: **(sub-SG label is 14) 1, 10, 9.**

The transformation is:  $(\mathbf{a}_{146}, \mathbf{b}_{146}, \mathbf{c}_{146}) = (\mathbf{a}_{217}, \mathbf{b}_{217}, \mathbf{c}_{217}) \begin{pmatrix} -\frac{1}{2} & -\frac{1}{2} & \frac{1}{2} \\ -\frac{1}{2} & \frac{1}{2} & \frac{1}{2} \\ -\frac{1}{2} & \frac{1}{2} & -\frac{1}{2} \end{pmatrix}, \overrightarrow{O_{217}O_{146}} = -\frac{1}{3}\mathbf{a}_{146} + (\frac{2}{3})\mathbf{b}_{146} + (-\frac{1}{3})\mathbf{c}_{146}$

The reduction of higher dimensional irrep:

$$T_d : T_1 \rightarrow A + {}^2E + {}^1E \text{ of } C_3.$$

$$T_d : T_2 \rightarrow A + {}^2E + {}^1E \text{ of } C_3.$$

The correspondences of irreps at HSPs from original SG to lowered SG:

$$\begin{aligned} n_{GM4}^{146} &= 2n_{GM8}^{217} & n_{GM6}^{146} &= n_{GM6}^{217} + n_{GM7}^{217} + n_{GM8}^{217} & n_{GM5}^{146} &= n_{GM6}^{217} + n_{GM7}^{217} + n_{GM8}^{217} & n_{L2}^{146} &= 2n_{N5}^{217} & n_{F2}^{146} &= 2n_{N5}^{217} & n_{T4}^{146} &= 2n_{N5}^{217} \\ 2n_{H8}^{217} n_{T6}^{146} &= n_{H6}^{217} + n_{H7}^{217} + n_{H8}^{217} & n_{T5}^{146} &= n_{H6}^{217} + n_{H7}^{217} + n_{H8}^{217} \end{aligned}$$

The lower SG is SG 197 when the preserved operations are: **(sub-SG label is 15) 1, 2, 3, 4, 5, 12, 8, 10, 6, 11, 7, 9.**

The transformation is:  $(\mathbf{a}_{197}, \mathbf{b}_{197}, \mathbf{c}_{197}) = (\mathbf{a}_{217}, \mathbf{b}_{217}, \mathbf{c}_{217}) \begin{pmatrix} 0 & 0 & 1 \\ 1 & 0 & 0 \\ 0 & 1 & 0 \end{pmatrix}, \overrightarrow{O_{217}O_{197}} = \mathbf{0}$

The reduction of higher dimensional irrep:

$T_d : E \rightarrow {}^1E + {}^2E$  of T.

The correspondences of irreps at HSPs from original SG to lowered SG:

$$n_{GM6}^{197} = n_{GM8}^{217} n_{GM7}^{197} = n_{GM8}^{217} n_{GM5}^{197} = n_{GM6}^{217} + n_{GM7}^{217} n_{H6}^{197} = n_{H8}^{217} n_{H7}^{197} = n_{H8}^{217} n_{H5}^{197} = n_{H6}^{217} + n_{H7}^{217} n_{N4}^{197} = n_{N5}^{217} n_{N3}^{197} =$$

$$n_{N5}^{217} n_{P6}^{197} = n_{P8}^{217} n_{P7}^{197} = n_{P8}^{217} n_{P5}^{197} = n_{P6}^{217} + n_{P7}^{217}$$

**115. Lowered SGs by higher-dimensional irreps of pairings in SG 218**

The representative operations of SG/T for SG 218:

1 :  $(x, y, z)$ , 2 :  $(x, -y, -z)$ , 3 :  $(-x, y, -z)$ , 4 :  $(-x, -y, z)$ , 5 :  $(z, x, y)$ , 6 :  $(y, z, x)$ , 7 :  $(-y, z, -x)$ , 8 :  $(-z, -x, y)$ ,  
 9 :  $(-y, -z, x)$ , 10 :  $(z, -x, -y)$ , 11 :  $(y, -z, -x)$ , 12 :  $(-z, x, -y)$ , 13 :  $(\frac{1}{2} - x, z + \frac{1}{2}, \frac{1}{2} - y)$ , 14 :  $(\frac{1}{2} - x, \frac{1}{2} - z, y + \frac{1}{2})$ ,  
 15 :  $(\frac{1}{2} - z, \frac{1}{2} - y, x + \frac{1}{2})$ , 16 :  $(z + \frac{1}{2}, \frac{1}{2} - y, \frac{1}{2} - x)$ , 17 :  $(y + \frac{1}{2}, \frac{1}{2} - x, \frac{1}{2} - z)$ , 18 :  $(\frac{1}{2} - y, x + \frac{1}{2}, \frac{1}{2} - z)$ ,  
 19 :  $(\frac{1}{2} - y, \frac{1}{2} - x, z + \frac{1}{2})$ , 20 :  $(y + \frac{1}{2}, x + \frac{1}{2}, z + \frac{1}{2})$ , 21 :  $(x + \frac{1}{2}, \frac{1}{2} - z, \frac{1}{2} - y)$ , 22 :  $(x + \frac{1}{2}, z + \frac{1}{2}, y + \frac{1}{2})$ ,  
 23 :  $(\frac{1}{2} - z, y + \frac{1}{2}, \frac{1}{2} - x)$ , 24 :  $(z + \frac{1}{2}, y + \frac{1}{2}, x + \frac{1}{2})$ .

The lower SG is SG 16 when the preserved operations are: (sub-SG label is 1) 1, 2, 3, 4.

The transformation is:  $(\mathbf{a}_{16}, \mathbf{b}_{16}, \mathbf{c}_{16}) = (\mathbf{a}_{218}, \mathbf{b}_{218}, \mathbf{c}_{218}) \begin{pmatrix} 0 & 0 & 1 \\ 1 & 0 & 0 \\ 0 & 1 & 0 \end{pmatrix}$ ,  $\overrightarrow{O_{218}O_{16}} = \frac{1}{2}\mathbf{a}_{16} + (\frac{1}{2})\mathbf{c}_{16}$

The reduction of higher dimensional irrep:

$T_d : T_1 \rightarrow B_1 + B_2 + B_3$  of  $D_2$ .

$T_d : T_2 \rightarrow B_1 + B_2 + B_3$  of  $D_2$ .

The correspondences of irreps at HSPs from original SG to lowered SG:

$$n_{GM5}^{16} = n_{GM6}^{218} + n_{GM7}^{218} + 2n_{GM8}^{218} n_{X5}^{16} = n_{M6}^{218} + n_{M7}^{218} n_{S5}^{16} = n_{M6}^{218} + n_{M7}^{218} n_{R5}^{16} = n_{R6}^{218} + n_{R7}^{218} + 2n_{R8}^{218} n_{U5}^{16} = n_{M6}^{218} + n_{M7}^{218}$$

$$n_{Z5}^{16} = n_{X6}^{218} + n_{X7}^{218} n_{T5}^{16} = n_{M6}^{218} + n_{M7}^{218} n_{Y5}^{16} = n_{X6}^{218} + n_{X7}^{218}$$

The lower SG is SG 37 when the preserved operations are: (sub-SG label is 2) 1, 4, 19, 20.

The transformation is:  $(\mathbf{a}_{37}, \mathbf{b}_{37}, \mathbf{c}_{37}) = (\mathbf{a}_{218}, \mathbf{b}_{218}, \mathbf{c}_{218}) \begin{pmatrix} 1 & -1 & 0 \\ 1 & 1 & 0 \\ 0 & 0 & 1 \end{pmatrix}$ ,  $\overrightarrow{O_{218}O_{37}} = \frac{1}{4}\mathbf{a}_{37} + (\frac{1}{4})\mathbf{b}_{37}$

The reduction of higher dimensional irrep:

$T_d : T_1 \rightarrow A_2 + B_1 + B_2$  of  $C_{2v}$ .

$T_d : T_2 \rightarrow A_1 + B_1 + B_2$  of  $C_{2v}$ .

The correspondences of irreps at HSPs from original SG to lowered SG:

$$n_{GM5}^{37} = n_{GM6}^{218} + n_{GM7}^{218} + 2n_{GM8}^{218} n_{Y5}^{37} = n_{M6}^{218} + n_{M7}^{218} n_{S4}^{37} = n_{X6}^{218} + n_{X7}^{218} n_{S3}^{37} = n_{X6}^{218} + n_{X7}^{218} n_{Z5}^{37} = n_{X6}^{218} + n_{X7}^{218} n_{T5}^{37} =$$

$$n_{R6}^{218} + n_{R7}^{218} + 2n_{R8}^{218} n_{R4}^{37} = n_{M6}^{218} + n_{M7}^{218} n_{R3}^{37} = n_{M6}^{218} + n_{M7}^{218}$$

The lower SG is SG 37 when the preserved operations are: (sub-SG label is 3) 1, 2, 21, 22.

The transformation is:  $(\mathbf{a}_{37}, \mathbf{b}_{37}, \mathbf{c}_{37}) = (\mathbf{a}_{218}, \mathbf{b}_{218}, \mathbf{c}_{218}) \begin{pmatrix} 0 & 0 & 1 \\ 1 & -1 & 0 \\ 1 & 1 & 0 \end{pmatrix}$ ,  $\overrightarrow{O_{218}O_{37}} = \frac{1}{4}\mathbf{a}_{37} + (\frac{1}{4})\mathbf{b}_{37}$

The reduction of higher dimensional irrep:

$T_d : T_1 \rightarrow A_2 + B_1 + B_2$  of  $C_{2v}$ .

$T_d : T_2 \rightarrow A_1 + B_1 + B_2$  of  $C_{2v}$ .

The correspondences of irreps at HSPs from original SG to lowered SG:

$$n_{GM5}^{37} = n_{GM6}^{218} + n_{GM7}^{218} + 2n_{GM8}^{218} n_{Y5}^{37} = n_{M6}^{218} + n_{M7}^{218} n_{S4}^{37} = n_{X6}^{218} + n_{X7}^{218} n_{S3}^{37} = n_{X6}^{218} + n_{X7}^{218} n_{Z5}^{37} = n_{X6}^{218} + n_{X7}^{218} n_{T5}^{37} =$$

$$n_{R6}^{218} + n_{R7}^{218} + 2n_{R8}^{218} n_{R4}^{37} = n_{M6}^{218} + n_{M7}^{218} n_{R3}^{37} = n_{M6}^{218} + n_{M7}^{218}$$

The lower SG is SG 37 when the preserved operations are: (sub-SG label is 4) 1, 3, 24, 23.

The transformation is:  $(\mathbf{a}_{37}, \mathbf{b}_{37}, \mathbf{c}_{37}) = (\mathbf{a}_{218}, \mathbf{b}_{218}, \mathbf{c}_{218}) \begin{pmatrix} -1 & 1 & 0 \\ 0 & 0 & 1 \\ 1 & 1 & 0 \end{pmatrix}$ ,  $\overrightarrow{O_{218}O_{37}} = \frac{1}{4}\mathbf{a}_{37} + (\frac{1}{4})\mathbf{b}_{37}$

The reduction of higher dimensional irrep:

$$T_d : T_1 \rightarrow A_2 + B_1 + B_2 \text{ of } C_{2v}.$$

$$T_d : T_2 \rightarrow A_1 + B_1 + B_2 \text{ of } C_{2v}.$$

The correspondences of irreps at HSPs from original SG to lowered SG:

$$\begin{aligned} n_{GM5}^{37} &= n_{GM6}^{218} + n_{GM7}^{218} + 2n_{GM8}^{218} \quad n_{X5}^{37} = n_{M6}^{218} + n_{M7}^{218} \quad n_{S4}^{37} = n_{X6}^{218} + n_{X7}^{218} \quad n_{S3}^{37} = n_{X6}^{218} + n_{X7}^{218} \quad n_{Z5}^{37} = n_{X6}^{218} + n_{X7}^{218} \quad n_{T5}^{37} = \\ & n_{R6}^{218} + n_{R7}^{218} + 2n_{R8}^{218} \quad n_{R4}^{37} = n_{M6}^{218} + n_{M7}^{218} \quad n_{R3}^{37} = n_{M6}^{218} + n_{M7}^{218} \end{aligned}$$

The lower SG is SG 81 when the preserved operations are: **(sub-SG label is 5) 1, 17, 18, 4.**

$$\text{The transformation is: } (\mathbf{a}_{81}, \mathbf{b}_{81}, \mathbf{c}_{81}) = (\mathbf{a}_{218}, \mathbf{b}_{218}, \mathbf{c}_{218}) \begin{pmatrix} -1 & 0 & 0 \\ 0 & -1 & 0 \\ 0 & 0 & 1 \end{pmatrix}, \overrightarrow{O_{218}O_{81}} = \frac{1}{2}\mathbf{a}_{81} + \left(\frac{1}{4}\right)\mathbf{c}_{81}$$

The reduction of higher dimensional irrep:

$$T_d : T_1 \rightarrow A + {}^2E + {}^1E \text{ of } S_4.$$

$$T_d : T_2 \rightarrow {}^2E + B + {}^1E \text{ of } S_4.$$

The correspondences of irreps at HSPs from original SG to lowered SG:

$$\begin{aligned} n_{GM7}^{81} &= n_{GM7}^{218} + n_{GM8}^{218} \quad n_{GM8}^{81} = n_{GM6}^{218} + n_{GM8}^{218} \quad n_{GM5}^{81} = n_{GM7}^{218} + n_{GM8}^{218} \quad n_{GM6}^{81} = n_{GM6}^{218} + n_{GM8}^{218} \quad n_{X4}^{81} = n_{X6}^{218} + n_{X7}^{218} \quad n_{X3}^{81} = \\ & n_{X6}^{218} + n_{X7}^{218} \quad n_{M7}^{81} = n_{M6}^{218} \quad n_{M8}^{81} = n_{M7}^{218} \quad n_{M5}^{81} = n_{M6}^{218} \quad n_{M6}^{81} = n_{M7}^{218} \quad n_{A7}^{81} = n_{R7}^{218} + n_{R8}^{218} \quad n_{A8}^{81} = n_{R6}^{218} + n_{R8}^{218} \quad n_{A5}^{81} = n_{R6}^{218} + n_{R8}^{218} \\ & n_{A6}^{81} = n_{R7}^{218} + n_{R8}^{218} \quad n_{R4}^{81} = n_{M6}^{218} + n_{M7}^{218} \quad n_{R3}^{81} = n_{M6}^{218} + n_{M7}^{218} \quad n_{Z7}^{81} = n_{X6}^{218} \quad n_{Z8}^{81} = n_{X7}^{218} \quad n_{Z5}^{81} = n_{X6}^{218} \quad n_{Z6}^{81} = n_{X7}^{218} \end{aligned}$$

The lower SG is SG 81 when the preserved operations are: **(sub-SG label is 6) 1, 13, 14, 2.**

$$\text{The transformation is: } (\mathbf{a}_{81}, \mathbf{b}_{81}, \mathbf{c}_{81}) = (\mathbf{a}_{218}, \mathbf{b}_{218}, \mathbf{c}_{218}) \begin{pmatrix} 0 & 0 & 1 \\ -1 & 0 & 0 \\ 0 & -1 & 0 \end{pmatrix}, \overrightarrow{O_{218}O_{81}} = \frac{1}{2}\mathbf{b}_{81} + \left(\frac{3}{4}\right)\mathbf{c}_{81}$$

The reduction of higher dimensional irrep:

$$T_d : T_1 \rightarrow A + {}^2E + {}^1E \text{ of } S_4.$$

$$T_d : T_2 \rightarrow {}^2E + B + {}^1E \text{ of } S_4.$$

The correspondences of irreps at HSPs from original SG to lowered SG:

$$\begin{aligned} n_{GM7}^{81} &= n_{GM7}^{218} + n_{GM8}^{218} \quad n_{GM8}^{81} = n_{GM6}^{218} + n_{GM8}^{218} \quad n_{GM5}^{81} = n_{GM7}^{218} + n_{GM8}^{218} \quad n_{GM6}^{81} = n_{GM6}^{218} + n_{GM8}^{218} \quad n_{X4}^{81} = n_{X6}^{218} + n_{X7}^{218} \quad n_{X3}^{81} = \\ & n_{X6}^{218} + n_{X7}^{218} \quad n_{M7}^{81} = n_{M6}^{218} \quad n_{M8}^{81} = n_{M7}^{218} \quad n_{M5}^{81} = n_{M6}^{218} \quad n_{M6}^{81} = n_{M7}^{218} \quad n_{A7}^{81} = n_{R7}^{218} + n_{R8}^{218} \quad n_{A8}^{81} = n_{R6}^{218} + n_{R8}^{218} \quad n_{A5}^{81} = n_{R6}^{218} + n_{R8}^{218} \\ & n_{A6}^{81} = n_{R7}^{218} + n_{R8}^{218} \quad n_{R4}^{81} = n_{M6}^{218} + n_{M7}^{218} \quad n_{R3}^{81} = n_{M6}^{218} + n_{M7}^{218} \quad n_{Z7}^{81} = n_{X6}^{218} \quad n_{Z8}^{81} = n_{X7}^{218} \quad n_{Z5}^{81} = n_{X6}^{218} \quad n_{Z6}^{81} = n_{X7}^{218} \end{aligned}$$

The lower SG is SG 81 when the preserved operations are: **(sub-SG label is 7) 1, 15, 16, 3.**

$$\text{The transformation is: } (\mathbf{a}_{81}, \mathbf{b}_{81}, \mathbf{c}_{81}) = (\mathbf{a}_{218}, \mathbf{b}_{218}, \mathbf{c}_{218}) \begin{pmatrix} -1 & 0 & 0 \\ 0 & 0 & 1 \\ 0 & 1 & 0 \end{pmatrix}, \overrightarrow{O_{218}O_{81}} = \frac{1}{2}\mathbf{a}_{81} + \left(\frac{3}{4}\right)\mathbf{c}_{81}$$

The reduction of higher dimensional irrep:

$$T_d : T_1 \rightarrow A + {}^2E + {}^1E \text{ of } S_4.$$

$$T_d : T_2 \rightarrow {}^2E + B + {}^1E \text{ of } S_4.$$

The correspondences of irreps at HSPs from original SG to lowered SG:

$$\begin{aligned} n_{GM7}^{81} &= n_{GM7}^{218} + n_{GM8}^{218} \quad n_{GM8}^{81} = n_{GM6}^{218} + n_{GM8}^{218} \quad n_{GM5}^{81} = n_{GM7}^{218} + n_{GM8}^{218} \quad n_{GM6}^{81} = n_{GM6}^{218} + n_{GM8}^{218} \quad n_{X4}^{81} = n_{X6}^{218} + n_{X7}^{218} \quad n_{X3}^{81} = \\ & n_{X6}^{218} + n_{X7}^{218} \quad n_{M7}^{81} = n_{M6}^{218} \quad n_{M8}^{81} = n_{M7}^{218} \quad n_{M5}^{81} = n_{M6}^{218} \quad n_{M6}^{81} = n_{M7}^{218} \quad n_{A7}^{81} = n_{R7}^{218} + n_{R8}^{218} \quad n_{A8}^{81} = n_{R6}^{218} + n_{R8}^{218} \quad n_{A5}^{81} = n_{R6}^{218} + n_{R8}^{218} \\ & n_{A6}^{81} = n_{R7}^{218} + n_{R8}^{218} \quad n_{R4}^{81} = n_{M6}^{218} + n_{M7}^{218} \quad n_{R3}^{81} = n_{M6}^{218} + n_{M7}^{218} \quad n_{Z7}^{81} = n_{X6}^{218} \quad n_{Z8}^{81} = n_{X7}^{218} \quad n_{Z5}^{81} = n_{X6}^{218} \quad n_{Z6}^{81} = n_{X7}^{218} \end{aligned}$$

The lower SG is SG 112 when the preserved operations are: **(sub-SG label is 8) 1, 18, 17, 4, 2, 3, 19, 20.**

$$\text{The transformation is: } (\mathbf{a}_{112}, \mathbf{b}_{112}, \mathbf{c}_{112}) = (\mathbf{a}_{218}, \mathbf{b}_{218}, \mathbf{c}_{218}) \begin{pmatrix} -1 & 0 & 0 \\ 0 & 1 & 0 \\ 0 & 0 & -1 \end{pmatrix}, \overrightarrow{O_{218}O_{112}} = \frac{1}{2}\mathbf{b}_{112} + \left(\frac{3}{4}\right)\mathbf{c}_{112}$$

The reduction of higher dimensional irrep:

$$T_d : E \rightarrow A_1 + B_1 \text{ of } D_{2d}.$$

The correspondences of irreps at HSPs from original SG to lowered SG:

$$\begin{aligned} n_{GM6}^{112} &= n_{GM7}^{218} + n_{GM8}^{218} \quad n_{GM7}^{112} = n_{GM6}^{218} + n_{GM8}^{218} \quad n_{X5}^{112} = n_{X6}^{218} + n_{X7}^{218} \quad n_{M6}^{112} = n_{M7}^{218} \quad n_{M7}^{112} = n_{M6}^{218} \quad n_{A6}^{112} = n_{R6}^{218} + n_{R8}^{218} \quad n_{A7}^{112} = \\ & n_{R7}^{218} + n_{R8}^{218} \quad n_{R5}^{112} = n_{M6}^{218} + n_{M7}^{218} \quad n_{Z6}^{112} = n_{X6}^{218} \quad n_{Z7}^{112} = n_{X7}^{218} \end{aligned}$$

The lower SG is SG 112 when the preserved operations are: **(sub-SG label is 9) 1, 14, 13, 2, 3, 4, 21, 22.**

$$\text{The transformation is: } (\mathbf{a}_{112}, \mathbf{b}_{112}, \mathbf{c}_{112}) = (\mathbf{a}_{218}, \mathbf{b}_{218}, \mathbf{c}_{218}) \begin{pmatrix} 0 & 0 & -1 \\ -1 & 0 & 0 \\ 0 & 1 & 0 \end{pmatrix}, \overrightarrow{O_{218}O_{112}} = \frac{1}{2}\mathbf{a}_{112} + \left(\frac{1}{4}\right)\mathbf{c}_{112}$$

The reduction of higher dimensional irrep:

$T_d : E \rightarrow A_1 + B_1$  of  $D_{2d}$ .

The correspondences of irreps at HSPs from original SG to lowered SG:

$$\begin{aligned} n_{GM6}^{112} &= n_{GM7}^{218} + n_{GM8}^{218} & n_{GM7}^{112} &= n_{GM6}^{218} + n_{GM8}^{218} & n_{X5}^{112} &= n_{X6}^{218} + n_{X7}^{218} & n_{M6}^{112} &= n_{M6}^{218} & n_{M7}^{112} &= n_{M7}^{218} & n_{A6}^{112} &= n_{R6}^{218} + n_{R8}^{218} & n_{A7}^{112} &= \\ n_{R7}^{218} + n_{R8}^{218} & n_{R5}^{112} &= n_{M6}^{218} + n_{M7}^{218} & n_{Z6}^{112} &= n_{X6}^{218} & n_{Z7}^{112} &= n_{X7}^{218} \end{aligned}$$

The lower SG is SG 112 when the preserved operations are: (**sub-SG label is 10**) 1, 16, 15, 3, 4, 2, 24, 23.

$$\text{The transformation is: } (\mathbf{a}_{112}, \mathbf{b}_{112}, \mathbf{c}_{112}) = (\mathbf{a}_{218}, \mathbf{b}_{218}, \mathbf{c}_{218}) \begin{pmatrix} -1 & 0 & 0 \\ 0 & 0 & -1 \\ 0 & -1 & 0 \end{pmatrix}, \overrightarrow{O_{218}O_{112}} = \frac{1}{2}\mathbf{b}_{112} + \left(\frac{1}{4}\right)\mathbf{c}_{112}$$

The reduction of higher dimensional irrep:

$T_d : E \rightarrow A_1 + B_1$  of  $D_{2d}$ .

The correspondences of irreps at HSPs from original SG to lowered SG:

$$\begin{aligned} n_{GM6}^{112} &= n_{GM7}^{218} + n_{GM8}^{218} & n_{GM7}^{112} &= n_{GM6}^{218} + n_{GM8}^{218} & n_{X5}^{112} &= n_{X6}^{218} + n_{X7}^{218} & n_{M6}^{112} &= n_{M6}^{218} & n_{M7}^{112} &= n_{M7}^{218} & n_{A6}^{112} &= n_{R6}^{218} + n_{R8}^{218} & n_{A7}^{112} &= \\ n_{R7}^{218} + n_{R8}^{218} & n_{R5}^{112} &= n_{M6}^{218} + n_{M7}^{218} & n_{Z6}^{112} &= n_{X6}^{218} & n_{Z7}^{112} &= n_{X7}^{218} \end{aligned}$$

The lower SG is SG 146 when the preserved operations are: (**sub-SG label is 11**) 1, 5, 6.

$$\text{The transformation is: } (\mathbf{a}_{146}, \mathbf{b}_{146}, \mathbf{c}_{146}) = (\mathbf{a}_{218}, \mathbf{b}_{218}, \mathbf{c}_{218}) \begin{pmatrix} 0 & 1 & 0 \\ 0 & 0 & 1 \\ 1 & 0 & 0 \end{pmatrix}, \overrightarrow{O_{218}O_{146}} = -\frac{1}{3}\mathbf{a}_{146} + \left(\frac{2}{3}\right)\mathbf{b}_{146} + \left(-\frac{1}{3}\right)\mathbf{c}_{146}$$

The reduction of higher dimensional irrep:

$T_d : T_1 \rightarrow A + {}^2E + {}^1E$  of  $C_3$ .

$T_d : T_2 \rightarrow A + {}^2E + {}^1E$  of  $C_3$ .

The correspondences of irreps at HSPs from original SG to lowered SG:

$$\begin{aligned} n_{GM4}^{146} &= 2n_{GM8}^{218} & n_{GM6}^{146} &= n_{GM6}^{218} + n_{GM7}^{218} + n_{GM8}^{218} & n_{GM5}^{146} &= n_{GM6}^{218} + n_{GM7}^{218} + n_{GM8}^{218} & n_{L2}^{146} &= 2n_{X6}^{218} + 2n_{X7}^{218} & n_{F2}^{146} &= \\ 2n_{M6}^{218} + 2n_{M7}^{218} & n_{T4}^{146} &= 2n_{R8}^{218} & n_{T6}^{146} &= n_{R6}^{218} + n_{R7}^{218} + n_{R8}^{218} & n_{T5}^{146} &= n_{R6}^{218} + n_{R7}^{218} + n_{R8}^{218} \end{aligned}$$

The lower SG is SG 146 when the preserved operations are: (**sub-SG label is 12**) 1, 12, 11.

$$\text{The transformation is: } (\mathbf{a}_{146}, \mathbf{b}_{146}, \mathbf{c}_{146}) = (\mathbf{a}_{218}, \mathbf{b}_{218}, \mathbf{c}_{218}) \begin{pmatrix} 0 & -1 & 0 \\ 0 & 0 & -1 \\ 1 & 0 & 0 \end{pmatrix}, \overrightarrow{O_{218}O_{146}} = -\frac{1}{3}\mathbf{a}_{146} + \left(\frac{2}{3}\right)\mathbf{b}_{146} + \left(-\frac{1}{3}\right)\mathbf{c}_{146}$$

The reduction of higher dimensional irrep:

$T_d : T_1 \rightarrow A + {}^2E + {}^1E$  of  $C_3$ .

$T_d : T_2 \rightarrow A + {}^2E + {}^1E$  of  $C_3$ .

The correspondences of irreps at HSPs from original SG to lowered SG:

$$\begin{aligned} n_{GM4}^{146} &= 2n_{GM8}^{218} & n_{GM6}^{146} &= n_{GM6}^{218} + n_{GM7}^{218} + n_{GM8}^{218} & n_{GM5}^{146} &= n_{GM6}^{218} + n_{GM7}^{218} + n_{GM8}^{218} & n_{L2}^{146} &= 2n_{X6}^{218} + 2n_{X7}^{218} & n_{F2}^{146} &= \\ 2n_{M6}^{218} + 2n_{M7}^{218} & n_{T4}^{146} &= 2n_{R8}^{218} & n_{T6}^{146} &= n_{R6}^{218} + n_{R7}^{218} + n_{R8}^{218} & n_{T5}^{146} &= n_{R6}^{218} + n_{R7}^{218} + n_{R8}^{218} \end{aligned}$$

The lower SG is SG 146 when the preserved operations are: (**sub-SG label is 13**) 1, 8, 7.

$$\text{The transformation is: } (\mathbf{a}_{146}, \mathbf{b}_{146}, \mathbf{c}_{146}) = (\mathbf{a}_{218}, \mathbf{b}_{218}, \mathbf{c}_{218}) \begin{pmatrix} 1 & 0 & 0 \\ 0 & -1 & 0 \\ 0 & 0 & -1 \end{pmatrix}, \overrightarrow{O_{218}O_{146}} = -\frac{1}{3}\mathbf{a}_{146} + \left(\frac{2}{3}\right)\mathbf{b}_{146} + \left(-\frac{1}{3}\right)\mathbf{c}_{146}$$

The reduction of higher dimensional irrep:

$T_d : T_1 \rightarrow A + {}^2E + {}^1E$  of  $C_3$ .

$T_d : T_2 \rightarrow A + {}^2E + {}^1E$  of  $C_3$ .

The correspondences of irreps at HSPs from original SG to lowered SG:

$$\begin{aligned} n_{GM4}^{146} &= 2n_{GM8}^{218} & n_{GM6}^{146} &= n_{GM6}^{218} + n_{GM7}^{218} + n_{GM8}^{218} & n_{GM5}^{146} &= n_{GM6}^{218} + n_{GM7}^{218} + n_{GM8}^{218} & n_{L2}^{146} &= 2n_{X6}^{218} + 2n_{X7}^{218} & n_{F2}^{146} &= \\ 2n_{M6}^{218} + 2n_{M7}^{218} & n_{T4}^{146} &= 2n_{R8}^{218} & n_{T6}^{146} &= n_{R6}^{218} + n_{R7}^{218} + n_{R8}^{218} & n_{T5}^{146} &= n_{R6}^{218} + n_{R7}^{218} + n_{R8}^{218} \end{aligned}$$

The lower SG is SG 146 when the preserved operations are: (**sub-SG label is 14**) 1, 10, 9.

$$\text{The transformation is: } (\mathbf{a}_{146}, \mathbf{b}_{146}, \mathbf{c}_{146}) = (\mathbf{a}_{218}, \mathbf{b}_{218}, \mathbf{c}_{218}) \begin{pmatrix} -1 & 0 & 0 \\ 0 & 1 & 0 \\ 0 & 0 & -1 \end{pmatrix}, \overrightarrow{O_{218}O_{146}} = -\frac{1}{3}\mathbf{a}_{146} + \left(\frac{2}{3}\right)\mathbf{b}_{146} + \left(-\frac{1}{3}\right)\mathbf{c}_{146}$$

The reduction of higher dimensional irrep:

$T_d : T_1 \rightarrow A + {}^2E + {}^1E$  of  $C_3$ .

$T_d : T_2 \rightarrow A + {}^2E + {}^1E$  of  $C_3$ .

The correspondences of irreps at HSPs from original SG to lowered SG:

$$\begin{aligned} n_{GM4}^{146} &= 2n_{GM8}^{218} & n_{GM6}^{146} &= n_{GM6}^{218} + n_{GM7}^{218} + n_{GM8}^{218} & n_{GM5}^{146} &= n_{GM6}^{218} + n_{GM7}^{218} + n_{GM8}^{218} & n_{L2}^{146} &= 2n_{X6}^{218} + 2n_{X7}^{218} & n_{F2}^{146} &= \\ 2n_{M6}^{218} + 2n_{M7}^{218} & n_{T4}^{146} &= 2n_{R8}^{218} & n_{T6}^{146} &= n_{R6}^{218} + n_{R7}^{218} + n_{R8}^{218} & n_{T5}^{146} &= n_{R6}^{218} + n_{R7}^{218} + n_{R8}^{218} \end{aligned}$$

The lower SG is SG 195 when the preserved operations are: **(sub-SG label is 15)** 1, 2, 3, 4, 5, 12, 8, 10, 6, 11, 7, 9.

The transformation is:  $(\mathbf{a}_{195}, \mathbf{b}_{195}, \mathbf{c}_{195}) = (\mathbf{a}_{218}, \mathbf{b}_{218}, \mathbf{c}_{218}) \begin{pmatrix} 0 & 0 & 1 \\ 1 & 0 & 0 \\ 0 & 1 & 0 \end{pmatrix}, \overrightarrow{O_{218}O_{195}} = \mathbf{0}$

The reduction of higher dimensional irrep:

$$T_d : E \rightarrow {}^1E + {}^2E \text{ of } T.$$

The correspondences of irreps at HSPs from original SG to lowered SG:

$$\begin{aligned} n_{GM6}^{195} &= n_{GM8}^{218} n_{GM7}^{195} = n_{GM8}^{218} n_{GM5}^{195} = n_{GM6}^{218} + n_{GM7}^{218} n_{X5}^{195} = n_{X6}^{218} + n_{X7}^{218} n_{M5}^{195} = n_{M6}^{218} + n_{M7}^{218} n_{R6}^{195} = n_{R8}^{218} n_{R7}^{195} = n_{R8}^{218} \\ n_{R5}^{195} &= n_{R6}^{218} + n_{R7}^{218} \end{aligned}$$

### 116. Lowered SGs by higher-dimensional irreps of pairings in SG 219

The representative operations of SG/T for SG 219:

$$\begin{aligned} &1 : (x, y, z), 2 : (x, -y, -z), 3 : (-x, y, -z), 4 : (-x, -y, z), 5 : (z, x, y), 6 : (y, z, x), 7 : (-y, z, -x), 8 : (-z, -x, y), \\ &9 : (-y, -z, x), 10 : (z, -x, -y), 11 : (y, -z, -x), 12 : (-z, x, -y), 13 : (\frac{1}{2} - x, z + \frac{1}{2}, \frac{1}{2} - y), 14 : (\frac{1}{2} - x, \frac{1}{2} - z, y + \frac{1}{2}), \\ &15 : (\frac{1}{2} - z, \frac{1}{2} - y, x + \frac{1}{2}), 16 : (z + \frac{1}{2}, \frac{1}{2} - y, \frac{1}{2} - x), 17 : (y + \frac{1}{2}, \frac{1}{2} - x, \frac{1}{2} - z), 18 : (\frac{1}{2} - y, x + \frac{1}{2}, \frac{1}{2} - z), \\ &19 : (\frac{1}{2} - y, \frac{1}{2} - x, z + \frac{1}{2}), 20 : (y + \frac{1}{2}, x + \frac{1}{2}, z + \frac{1}{2}), 21 : (x + \frac{1}{2}, \frac{1}{2} - z, \frac{1}{2} - y), 22 : (x + \frac{1}{2}, z + \frac{1}{2}, y + \frac{1}{2}), \\ &23 : (\frac{1}{2} - z, y + \frac{1}{2}, \frac{1}{2} - x), 24 : (z + \frac{1}{2}, y + \frac{1}{2}, x + \frac{1}{2}). \end{aligned}$$

The lower SG is SG 22 when the preserved operations are: **(sub-SG label is 1)** 1, 2, 3, 4.

The transformation is:  $(\mathbf{a}_{22}, \mathbf{b}_{22}, \mathbf{c}_{22}) = (\mathbf{a}_{219}, \mathbf{b}_{219}, \mathbf{c}_{219}) \begin{pmatrix} 0 & 0 & 1 \\ 1 & 0 & 0 \\ 0 & 1 & 0 \end{pmatrix}, \overrightarrow{O_{219}O_{22}} = \frac{1}{4}\mathbf{a}_{22} + (-\frac{1}{4})\mathbf{b}_{22} + (-\frac{1}{4})\mathbf{c}_{22}$

The reduction of higher dimensional irrep:

$$T_d : T_1 \rightarrow B_1 + B_2 + B_3 \text{ of } D_2.$$

$$T_d : T_2 \rightarrow B_1 + B_2 + B_3 \text{ of } D_2.$$

The correspondences of irreps at HSPs from original SG to lowered SG:

$$n_{GM5}^{22} = n_{GM6}^{219} + n_{GM7}^{219} + 2n_{GM8}^{219} n_{Y5}^{22} = n_{X6}^{219} + n_{X7}^{219} n_{L2}^{22} = n_{L4}^{219} + n_{L5}^{219} + 2n_{L6}^{219} n_{Z5}^{22} = n_{X6}^{219} + n_{X7}^{219} n_{T5}^{22} = n_{X6}^{219} + n_{X7}^{219}$$

The lower SG is SG 45 when the preserved operations are: **(sub-SG label is 2)** 1, 4, 19, 20.

The transformation is:  $(\mathbf{a}_{45}, \mathbf{b}_{45}, \mathbf{c}_{45}) = (\mathbf{a}_{219}, \mathbf{b}_{219}, \mathbf{c}_{219}) \begin{pmatrix} \frac{1}{2} & -\frac{1}{2} & 0 \\ \frac{1}{2} & \frac{1}{2} & 0 \\ 0 & 0 & 1 \end{pmatrix}, \overrightarrow{O_{219}O_{45}} = -\frac{1}{2}\mathbf{b}_{45}$

The reduction of higher dimensional irrep:

$$T_d : T_1 \rightarrow A_2 + B_1 + B_2 \text{ of } C_{2v}.$$

$$T_d : T_2 \rightarrow A_1 + B_1 + B_2 \text{ of } C_{2v}.$$

The correspondences of irreps at HSPs from original SG to lowered SG:

$$\begin{aligned} n_{GM5}^{45} &= n_{GM6}^{219} + n_{GM7}^{219} + 2n_{GM8}^{219} n_{X5}^{45} = n_{X6}^{219} + n_{X7}^{219} n_{T4}^{45} = n_{X6}^{219} + n_{X7}^{219} n_{T3}^{45} = n_{X6}^{219} + n_{X7}^{219} n_{W4}^{45} = n_{W7}^{219} + n_{W8}^{219} n_{W3}^{45} = \\ n_{W5}^{219} + n_{W6}^{219} n_{R4}^{45} &= n_{L5}^{219} + n_{L6}^{219} n_{R3}^{45} = n_{L4}^{219} + n_{L6}^{219} n_{S4}^{45} = n_{L5}^{219} + n_{L6}^{219} n_{S3}^{45} = n_{L4}^{219} + n_{L6}^{219} \end{aligned}$$

The lower SG is SG 45 when the preserved operations are: **(sub-SG label is 3)** 1, 2, 21, 22.

The transformation is:  $(\mathbf{a}_{45}, \mathbf{b}_{45}, \mathbf{c}_{45}) = (\mathbf{a}_{219}, \mathbf{b}_{219}, \mathbf{c}_{219}) \begin{pmatrix} 0 & 0 & 1 \\ \frac{1}{2} & -\frac{1}{2} & 0 \\ \frac{1}{2} & \frac{1}{2} & 0 \end{pmatrix}, \overrightarrow{O_{219}O_{45}} = -\frac{1}{2}\mathbf{b}_{45}$

The reduction of higher dimensional irrep:

$$T_d : T_1 \rightarrow A_2 + B_1 + B_2 \text{ of } C_{2v}.$$

$$T_d : T_2 \rightarrow A_1 + B_1 + B_2 \text{ of } C_{2v}.$$

The correspondences of irreps at HSPs from original SG to lowered SG:

$$\begin{aligned} n_{GM5}^{45} &= n_{GM6}^{219} + n_{GM7}^{219} + 2n_{GM8}^{219} n_{X5}^{45} = n_{X6}^{219} + n_{X7}^{219} n_{T4}^{45} = n_{X6}^{219} + n_{X7}^{219} n_{T3}^{45} = n_{X6}^{219} + n_{X7}^{219} n_{W4}^{45} = n_{W7}^{219} + n_{W8}^{219} n_{W3}^{45} = \\ n_{W5}^{219} + n_{W6}^{219} n_{R4}^{45} &= n_{L5}^{219} + n_{L6}^{219} n_{R3}^{45} = n_{L4}^{219} + n_{L6}^{219} n_{S4}^{45} = n_{L5}^{219} + n_{L6}^{219} n_{S3}^{45} = n_{L4}^{219} + n_{L6}^{219} \end{aligned}$$

The lower SG is SG 45 when the preserved operations are: **(sub-SG label is 4) 1, 3, 24, 23.**

The transformation is:  $(\mathbf{a}_{45}, \mathbf{b}_{45}, \mathbf{c}_{45}) = (\mathbf{a}_{219}, \mathbf{b}_{219}, \mathbf{c}_{219}) \begin{pmatrix} -\frac{1}{2} & \frac{1}{2} & 0 \\ 0 & 0 & 1 \\ \frac{1}{2} & \frac{1}{2} & 0 \end{pmatrix}, \overrightarrow{O_{219}O_{45}} = -\frac{1}{2}\mathbf{b}_{45}$

The reduction of higher dimensional irrep:

$$T_d: T_1 \rightarrow A_2 + B_1 + B_2 \text{ of } C_{2v}.$$

$$T_d: T_2 \rightarrow A_1 + B_1 + B_2 \text{ of } C_{2v}.$$

The correspondences of irreps at HSPs from original SG to lowered SG:

$$\begin{aligned} n_{GM5}^{45} &= n_{GM6}^{219} + n_{GM7}^{219} + 2n_{GM8}^{219} & n_{X5}^{45} &= n_{X6}^{219} + n_{X7}^{219} & n_{T4}^{45} &= n_{X6}^{219} + n_{X7}^{219} & n_{T3}^{45} &= n_{X6}^{219} + n_{X7}^{219} & n_{W4}^{45} &= n_{W5}^{219} + n_{W6}^{219} & n_{W3}^{45} &= \\ n_{W7}^{219} + n_{W8}^{219} & n_{R4}^{45} &= n_{L4}^{219} + n_{L6}^{219} & n_{R3}^{45} &= n_{L5}^{219} + n_{L6}^{219} & n_{S4}^{45} &= n_{L4}^{219} + n_{L6}^{219} & n_{S3}^{45} &= n_{L5}^{219} + n_{L6}^{219} \end{aligned}$$

The lower SG is SG 82 when the preserved operations are: **(sub-SG label is 5) 1, 17, 18, 4.**

The transformation is:  $(\mathbf{a}_{82}, \mathbf{b}_{82}, \mathbf{c}_{82}) = (\mathbf{a}_{219}, \mathbf{b}_{219}, \mathbf{c}_{219}) \begin{pmatrix} \frac{1}{2} & \frac{1}{2} & 0 \\ -\frac{1}{2} & \frac{1}{2} & 0 \\ 0 & 0 & 1 \end{pmatrix}, \overrightarrow{O_{219}O_{82}} = \frac{1}{2}\mathbf{a}_{82}$

The reduction of higher dimensional irrep:

$$T_d: T_1 \rightarrow A + {}^2E + {}^1E \text{ of } S_4.$$

$$T_d: T_2 \rightarrow {}^2E + B + {}^1E \text{ of } S_4.$$

The correspondences of irreps at HSPs from original SG to lowered SG:

$$\begin{aligned} n_{GM7}^{82} &= n_{GM7}^{219} + n_{GM8}^{219} & n_{GM8}^{82} &= n_{GM6}^{219} + n_{GM8}^{219} & n_{GM5}^{82} &= n_{GM7}^{219} + n_{GM8}^{219} & n_{GM6}^{82} &= n_{GM6}^{219} + n_{GM8}^{219} & n_{M7}^{82} &= n_{X6}^{219} & n_{M8}^{82} &= n_{X7}^{219} \\ n_{M5}^{82} &= n_{X7}^{219} & n_{M6}^{82} &= n_{X6}^{219} & n_{X4}^{82} &= n_{X6}^{219} + n_{X7}^{219} & n_{X3}^{82} &= n_{X6}^{219} + n_{X7}^{219} & n_{P7}^{82} &= n_{W6}^{219} & n_{P8}^{82} &= n_{W5}^{219} & n_{P5}^{82} &= n_{W7}^{219} & n_{P6}^{82} &= n_{W8}^{219} & n_{N2}^{82} &= \\ n_{L4}^{219} + n_{L5}^{219} & + 2n_{L6}^{219} \end{aligned}$$

The lower SG is SG 82 when the preserved operations are: **(sub-SG label is 6) 1, 13, 14, 2.**

The transformation is:  $(\mathbf{a}_{82}, \mathbf{b}_{82}, \mathbf{c}_{82}) = (\mathbf{a}_{219}, \mathbf{b}_{219}, \mathbf{c}_{219}) \begin{pmatrix} 0 & 0 & 1 \\ -\frac{1}{2} & \frac{1}{2} & 0 \\ -\frac{1}{2} & -\frac{1}{2} & 0 \end{pmatrix}, \overrightarrow{O_{219}O_{82}} = \frac{1}{4}\mathbf{c}_{82}$

The reduction of higher dimensional irrep:

$$T_d: T_1 \rightarrow A + {}^2E + {}^1E \text{ of } S_4.$$

$$T_d: T_2 \rightarrow {}^2E + B + {}^1E \text{ of } S_4.$$

The correspondences of irreps at HSPs from original SG to lowered SG:

$$\begin{aligned} n_{GM7}^{82} &= n_{GM7}^{219} + n_{GM8}^{219} & n_{GM8}^{82} &= n_{GM6}^{219} + n_{GM8}^{219} & n_{GM5}^{82} &= n_{GM7}^{219} + n_{GM8}^{219} & n_{GM6}^{82} &= n_{GM6}^{219} + n_{GM8}^{219} & n_{M7}^{82} &= n_{X6}^{219} & n_{M8}^{82} &= n_{X7}^{219} \\ n_{M5}^{82} &= n_{X7}^{219} & n_{M6}^{82} &= n_{X6}^{219} & n_{X4}^{82} &= n_{X6}^{219} + n_{X7}^{219} & n_{X3}^{82} &= n_{X6}^{219} + n_{X7}^{219} & n_{P7}^{82} &= n_{W6}^{219} & n_{P8}^{82} &= n_{W5}^{219} & n_{P5}^{82} &= n_{W7}^{219} & n_{P6}^{82} &= n_{W8}^{219} & n_{N2}^{82} &= \\ n_{L4}^{219} + n_{L5}^{219} & + 2n_{L6}^{219} \end{aligned}$$

The lower SG is SG 82 when the preserved operations are: **(sub-SG label is 7) 1, 15, 16, 3.**

The transformation is:  $(\mathbf{a}_{82}, \mathbf{b}_{82}, \mathbf{c}_{82}) = (\mathbf{a}_{219}, \mathbf{b}_{219}, \mathbf{c}_{219}) \begin{pmatrix} \frac{1}{2} & -\frac{1}{2} & 0 \\ 0 & 0 & 1 \\ -\frac{1}{2} & -\frac{1}{2} & 0 \end{pmatrix}, \overrightarrow{O_{219}O_{82}} = \frac{1}{2}\mathbf{a}_{82} + (-\frac{1}{2})\mathbf{b}_{82} + (\frac{1}{4})\mathbf{c}_{82}$

The reduction of higher dimensional irrep:

$$T_d: T_1 \rightarrow A + {}^2E + {}^1E \text{ of } S_4.$$

$$T_d: T_2 \rightarrow {}^2E + B + {}^1E \text{ of } S_4.$$

The correspondences of irreps at HSPs from original SG to lowered SG:

$$\begin{aligned} n_{GM7}^{82} &= n_{GM7}^{219} + n_{GM8}^{219} & n_{GM8}^{82} &= n_{GM6}^{219} + n_{GM8}^{219} & n_{GM5}^{82} &= n_{GM7}^{219} + n_{GM8}^{219} & n_{GM6}^{82} &= n_{GM6}^{219} + n_{GM8}^{219} & n_{M7}^{82} &= n_{X6}^{219} & n_{M8}^{82} &= n_{X7}^{219} \\ n_{M5}^{82} &= n_{X7}^{219} & n_{M6}^{82} &= n_{X6}^{219} & n_{X4}^{82} &= n_{X6}^{219} + n_{X7}^{219} & n_{X3}^{82} &= n_{X6}^{219} + n_{X7}^{219} & n_{P7}^{82} &= n_{W6}^{219} & n_{P8}^{82} &= n_{W5}^{219} & n_{P5}^{82} &= n_{W7}^{219} & n_{P6}^{82} &= n_{W8}^{219} & n_{N2}^{82} &= \\ n_{L4}^{219} + n_{L5}^{219} & + 2n_{L6}^{219} \end{aligned}$$

The lower SG is SG 120 when the preserved operations are: **(sub-SG label is 8) 1, 18, 17, 4, 2, 3, 19, 20.**

The transformation is:  $(\mathbf{a}_{120}, \mathbf{b}_{120}, \mathbf{c}_{120}) = (\mathbf{a}_{219}, \mathbf{b}_{219}, \mathbf{c}_{219}) \begin{pmatrix} \frac{1}{2} & -\frac{1}{2} & 0 \\ -\frac{1}{2} & -\frac{1}{2} & 0 \\ 0 & 0 & -1 \end{pmatrix}, \overrightarrow{O_{219}O_{120}} = \frac{1}{2}\mathbf{a}_{120} + (-)\mathbf{b}_{120}$

The reduction of higher dimensional irrep:

$$T_d: E \rightarrow A_1 + B_1 \text{ of } D_{2d}.$$

The correspondences of irreps at HSPs from original SG to lowered SG:

$$\begin{aligned} n_{GM6}^{120} &= n_{GM7}^{219} + n_{GM8}^{219} & n_{GM7}^{120} &= n_{GM6}^{219} + n_{GM8}^{219} & n_{GM5}^{120} &= n_{X6}^{219} & n_{GM4}^{120} &= n_{X7}^{219} & n_{M6}^{120} &= n_{X6}^{219} & n_{M7}^{120} &= n_{X7}^{219} & n_{M5}^{120} &= n_{W6}^{219} & n_{M4}^{120} &= n_{W7}^{219} & n_{M3}^{120} &= n_{W8}^{219} \\ n_{P5}^{120} &= n_{W6}^{219} & n_{P6}^{120} &= n_{W5}^{219} & n_{N4}^{120} &= n_{L5}^{219} + n_{L6}^{219} & n_{N3}^{120} &= n_{L4}^{219} + n_{L6}^{219} \end{aligned}$$

The lower SG is SG 120 when the preserved operations are: **(sub-SG label is 9)** 1, 14, 13, 2, 3, 4, 21, 22.

$$\text{The transformation is: } (\mathbf{a}_{120}, \mathbf{b}_{120}, \mathbf{c}_{120}) = (\mathbf{a}_{219}, \mathbf{b}_{219}, \mathbf{c}_{219}) \begin{pmatrix} 0 & 0 & -1 \\ -\frac{1}{2} & -\frac{1}{2} & 0 \\ -\frac{1}{2} & \frac{1}{2} & 0 \end{pmatrix}, \overrightarrow{O_{219}O_{120}} = \frac{1}{2}\mathbf{a}_{120} + (-\frac{1}{2})\mathbf{b}_{120} + (-\frac{1}{4})\mathbf{c}_{120}$$

The reduction of higher dimensional irrep:

$$T_d : E \rightarrow A_1 + B_1 \text{ of } D_{2d}.$$

The correspondences of irreps at HSPs from original SG to lowered SG:

$$\begin{aligned} n_{GM6}^{120} &= n_{GM7}^{219} + n_{GM8}^{219} & n_{GM7}^{120} &= n_{GM6}^{219} + n_{GM8}^{219} & n_{M6}^{120} &= n_{X6}^{219} & n_{M7}^{120} &= n_{X7}^{219} & n_{X5}^{120} &= n_{X6}^{219} + n_{X7}^{219} & n_{P7}^{120} &= n_{W8}^{219} & n_{P8}^{120} &= n_{W7}^{219} \\ n_{P5}^{120} &= n_{W6}^{219} & n_{P6}^{120} &= n_{W5}^{219} & n_{N4}^{120} &= n_{L4}^{219} + n_{L6}^{219} & n_{N3}^{120} &= n_{L5}^{219} + n_{L6}^{219} \end{aligned}$$

The lower SG is SG 120 when the preserved operations are: **(sub-SG label is 10)** 1, 16, 15, 3, 4, 2, 24, 23.

$$\text{The transformation is: } (\mathbf{a}_{120}, \mathbf{b}_{120}, \mathbf{c}_{120}) = (\mathbf{a}_{219}, \mathbf{b}_{219}, \mathbf{c}_{219}) \begin{pmatrix} \frac{1}{2} & \frac{1}{2} & 0 \\ 0 & 0 & -1 \\ -\frac{1}{2} & \frac{1}{2} & 0 \end{pmatrix}, \overrightarrow{O_{219}O_{120}} = \mathbf{a}_{120} + (-\frac{1}{4})\mathbf{c}_{120}$$

The reduction of higher dimensional irrep:

$$T_d : E \rightarrow A_1 + B_1 \text{ of } D_{2d}.$$

The correspondences of irreps at HSPs from original SG to lowered SG:

$$\begin{aligned} n_{GM6}^{120} &= n_{GM7}^{219} + n_{GM8}^{219} & n_{GM7}^{120} &= n_{GM6}^{219} + n_{GM8}^{219} & n_{M6}^{120} &= n_{X6}^{219} & n_{M7}^{120} &= n_{X7}^{219} & n_{X5}^{120} &= n_{X6}^{219} + n_{X7}^{219} & n_{P7}^{120} &= n_{W6}^{219} & n_{P8}^{120} &= n_{W5}^{219} \\ n_{P5}^{120} &= n_{W8}^{219} & n_{P6}^{120} &= n_{W7}^{219} & n_{N4}^{120} &= n_{L5}^{219} + n_{L6}^{219} & n_{N3}^{120} &= n_{L4}^{219} + n_{L6}^{219} \end{aligned}$$

The lower SG is SG 146 when the preserved operations are: **(sub-SG label is 11)** 1, 5, 6.

$$\text{The transformation is: } (\mathbf{a}_{146}, \mathbf{b}_{146}, \mathbf{c}_{146}) = (\mathbf{a}_{219}, \mathbf{b}_{219}, \mathbf{c}_{219}) \begin{pmatrix} \frac{1}{2} & 0 & \frac{1}{2} \\ \frac{1}{2} & \frac{1}{2} & 0 \\ 0 & \frac{1}{2} & \frac{1}{2} \end{pmatrix}, \overrightarrow{O_{219}O_{146}} = -\frac{1}{3}\mathbf{a}_{146} + (\frac{2}{3})\mathbf{b}_{146} + (-\frac{1}{3})\mathbf{c}_{146}$$

The reduction of higher dimensional irrep:

$$T_d : T_1 \rightarrow A + {}^2E + {}^1E \text{ of } C_3.$$

$$T_d : T_2 \rightarrow A + {}^2E + {}^1E \text{ of } C_3.$$

The correspondences of irreps at HSPs from original SG to lowered SG:

$$\begin{aligned} n_{GM4}^{146} &= 2n_{GM8}^{219} & n_{GM6}^{146} &= n_{GM6}^{219} + n_{GM7}^{219} + n_{GM8}^{219} & n_{GM5}^{146} &= n_{GM6}^{219} + n_{GM7}^{219} + n_{GM8}^{219} & n_{L2}^{146} &= n_{L4}^{219} + n_{L5}^{219} + 2n_{L6}^{219} & n_{F2}^{146} &= 2n_{X6}^{219} + 2n_{X7}^{219} \\ n_{T4}^{146} &= n_{L4}^{219} + n_{L5}^{219} & n_{T6}^{146} &= n_{L6}^{219} & n_{T5}^{146} &= n_{L6}^{219} \end{aligned}$$

The lower SG is SG 146 when the preserved operations are: **(sub-SG label is 12)** 1, 12, 11.

$$\text{The transformation is: } (\mathbf{a}_{146}, \mathbf{b}_{146}, \mathbf{c}_{146}) = (\mathbf{a}_{219}, \mathbf{b}_{219}, \mathbf{c}_{219}) \begin{pmatrix} -\frac{1}{2} & -\frac{1}{2} & 0 \\ 0 & -\frac{1}{2} & -\frac{1}{2} \\ \frac{1}{2} & 0 & \frac{1}{2} \end{pmatrix}, \overrightarrow{O_{219}O_{146}} = -\frac{1}{3}\mathbf{a}_{146} + (\frac{2}{3})\mathbf{b}_{146} + (-\frac{1}{3})\mathbf{c}_{146}$$

The reduction of higher dimensional irrep:

$$T_d : T_1 \rightarrow A + {}^2E + {}^1E \text{ of } C_3.$$

$$T_d : T_2 \rightarrow A + {}^2E + {}^1E \text{ of } C_3.$$

The correspondences of irreps at HSPs from original SG to lowered SG:

$$\begin{aligned} n_{GM4}^{146} &= 2n_{GM8}^{219} & n_{GM6}^{146} &= n_{GM6}^{219} + n_{GM7}^{219} + n_{GM8}^{219} & n_{GM5}^{146} &= n_{GM6}^{219} + n_{GM7}^{219} + n_{GM8}^{219} & n_{L2}^{146} &= n_{L4}^{219} + n_{L5}^{219} + 2n_{L6}^{219} & n_{F2}^{146} &= 2n_{X6}^{219} + 2n_{X7}^{219} \\ n_{T4}^{146} &= n_{L4}^{219} + n_{L5}^{219} & n_{T6}^{146} &= n_{L6}^{219} & n_{T5}^{146} &= n_{L6}^{219} \end{aligned}$$

The lower SG is SG 146 when the preserved operations are: **(sub-SG label is 13)** 1, 8, 7.

$$\text{The transformation is: } (\mathbf{a}_{146}, \mathbf{b}_{146}, \mathbf{c}_{146}) = (\mathbf{a}_{219}, \mathbf{b}_{219}, \mathbf{c}_{219}) \begin{pmatrix} \frac{1}{2} & 0 & \frac{1}{2} \\ -\frac{1}{2} & -\frac{1}{2} & 0 \\ 0 & -\frac{1}{2} & -\frac{1}{2} \end{pmatrix}, \overrightarrow{O_{219}O_{146}} = -\frac{1}{3}\mathbf{a}_{146} + (\frac{2}{3})\mathbf{b}_{146} + (-\frac{1}{3})\mathbf{c}_{146}$$

The reduction of higher dimensional irrep:

$$T_d : T_1 \rightarrow A + {}^2E + {}^1E \text{ of } C_3.$$

$$T_d : T_2 \rightarrow A + {}^2E + {}^1E \text{ of } C_3.$$

The correspondences of irreps at HSPs from original SG to lowered SG:

$$\begin{aligned} n_{GM4}^{146} &= 2n_{GM8}^{219} & n_{GM6}^{146} &= n_{GM6}^{219} + n_{GM7}^{219} + n_{GM8}^{219} & n_{GM5}^{146} &= n_{GM6}^{219} + n_{GM7}^{219} + n_{GM8}^{219} & n_{L2}^{146} &= n_{L4}^{219} + n_{L5}^{219} + 2n_{L6}^{219} & n_{F2}^{146} &= 2n_{X6}^{219} + 2n_{X7}^{219} \\ n_{T4}^{146} &= n_{L4}^{219} + n_{L5}^{219} & n_{T6}^{146} &= n_{L6}^{219} & n_{T5}^{146} &= n_{L6}^{219} \end{aligned}$$

The lower SG is SG 146 when the preserved operations are: **(sub-SG label is 14)** 1, 10, 9.

$$\text{The transformation is: } (\mathbf{a}_{146}, \mathbf{b}_{146}, \mathbf{c}_{146}) = (\mathbf{a}_{219}, \mathbf{b}_{219}, \mathbf{c}_{219}) \begin{pmatrix} -\frac{1}{2} & -\frac{1}{2} & 0 \\ 0 & \frac{1}{2} & \frac{1}{2} \\ -\frac{1}{2} & 0 & -\frac{1}{2} \end{pmatrix}, \overrightarrow{O_{219}O_{146}} = -\frac{1}{3}\mathbf{a}_{146} + (\frac{2}{3})\mathbf{b}_{146} + (-\frac{1}{3})\mathbf{c}_{146}$$

The reduction of higher dimensional irrep:

$$T_d : T_1 \rightarrow A + {}^2E + {}^1E \text{ of } C_3.$$

$$T_d : T_2 \rightarrow A + {}^2E + {}^1E \text{ of } C_3.$$

The correspondences of irreps at HSPs from original SG to lowered SG:

$$n_{GM4}^{146} = 2n_{GM8}^{219} \quad n_{GM6}^{146} = n_{GM6}^{219} + n_{GM7}^{219} + n_{GM8}^{219} \quad n_{GM5}^{146} = n_{GM6}^{219} + n_{GM7}^{219} + n_{GM8}^{219} \quad n_{L2}^{146} = n_{L4}^{219} + n_{L5}^{219} + 2n_{L6}^{219} \quad n_{F2}^{146} = 2n_{X6}^{219} + 2n_{X7}^{219} \quad n_{T4}^{146} = n_{L4}^{219} + n_{L5}^{219} \quad n_{T6}^{146} = n_{L6}^{219} \quad n_{T5}^{146} = n_{L6}^{219}$$

The lower SG is SG 196 when the preserved operations are: **(sub-SG label is 15) 1, 2, 3, 4, 5, 12, 8, 10, 6, 11, 7, 9.**

The transformation is:  $(\mathbf{a}_{196}, \mathbf{b}_{196}, \mathbf{c}_{196}) = (\mathbf{a}_{219}, \mathbf{b}_{219}, \mathbf{c}_{219}) \begin{pmatrix} 0 & 0 & 1 \\ 1 & 0 & 0 \\ 0 & 1 & 0 \end{pmatrix}, \overrightarrow{O_{219}O_{196}} = \frac{1}{4}\mathbf{a}_{196} + (\frac{1}{4})\mathbf{b}_{196} + (\frac{1}{4})\mathbf{c}_{196}$

The reduction of higher dimensional irrep:

$$T_d : E \rightarrow {}^1E + {}^2E \text{ of } T.$$

The correspondences of irreps at HSPs from original SG to lowered SG:

$$n_{GM6}^{196} = n_{GM8}^{219} \quad n_{GM7}^{196} = n_{GM8}^{219} \quad n_{GM5}^{196} = n_{GM6}^{219} + n_{GM7}^{219} \quad n_{X5}^{196} = n_{X6}^{219} + n_{X7}^{219} \quad n_{L4}^{196} = n_{L4}^{219} + n_{L5}^{219} \quad n_{L6}^{196} = n_{L6}^{219} \quad n_{L5}^{196} = n_{L6}^{219} \quad n_{W4}^{196} = n_{W5}^{219} + n_{W6}^{219} \quad n_{W3}^{196} = n_{W7}^{219} + n_{W8}^{219}$$

**117. Lowered SGs by higher-dimensional irreps of pairings in SG 220**

The representative operations of SG/T for SG 220:

1 :  $(x, y, z)$ , 2 :  $(x, -y, \frac{1}{2} - z)$ , 3 :  $(\frac{1}{2} - x, y, -z)$ , 4 :  $(-x, \frac{1}{2} - y, z)$ , 5 :  $(z, x, y)$ , 6 :  $(y, z, x)$ , 7 :  $(\frac{1}{2} - y, z, -x)$ ,  
 8 :  $(-z, \frac{1}{2} - x, y)$ , 9 :  $(-y, \frac{1}{2} - z, x)$ , 10 :  $(z, -x, \frac{1}{2} - y)$ , 11 :  $(y, -z, \frac{1}{2} - x)$ , 12 :  $(\frac{1}{2} - z, x, -y)$ , 13 :  $(\frac{1}{4} - x, z + \frac{1}{4}, \frac{3}{4} - y)$ ,  
 14 :  $(\frac{3}{4} - x, \frac{1}{4} - z, y + \frac{1}{4})$ , 15 :  $(\frac{3}{4} - z, \frac{1}{4} - y, x + \frac{1}{4})$ , 16 :  $(z + \frac{1}{4}, \frac{3}{4} - y, \frac{1}{4} - x)$ , 17 :  $(y + \frac{1}{4}, \frac{3}{4} - x, \frac{1}{4} - z)$ , 18 :  $(\frac{1}{4} - y, x + \frac{1}{4}, \frac{3}{4} - z)$ ,  
 19 :  $(\frac{3}{4} - y, \frac{1}{4} - x, z + \frac{1}{4})$ , 20 :  $(y + \frac{1}{4}, x + \frac{1}{4}, z + \frac{1}{4})$ , 21 :  $(x + \frac{1}{4}, \frac{3}{4} - z, \frac{1}{4} - y)$ , 22 :  $(x + \frac{1}{4}, z + \frac{1}{4}, y + \frac{1}{4})$ , 23 :  $(\frac{1}{4} - z, y + \frac{1}{4}, \frac{3}{4} - x)$ ,  
 24 :  $(z + \frac{1}{4}, y + \frac{1}{4}, x + \frac{1}{4})$ .

The lower SG is SG 24 when the preserved operations are: **(sub-SG label is 1) 1, 2, 3, 4.**

The transformation is:  $(\mathbf{a}_{24}, \mathbf{b}_{24}, \mathbf{c}_{24}) = (\mathbf{a}_{220}, \mathbf{b}_{220}, \mathbf{c}_{220}) \begin{pmatrix} 0 & 0 & 1 \\ 1 & 0 & 0 \\ 0 & 1 & 0 \end{pmatrix}, \overrightarrow{O_{220}O_{24}} = \frac{1}{2}\mathbf{c}_{24}$

The reduction of higher dimensional irrep:

$$T_d : T_1 \rightarrow B_1 + B_2 + B_3 \text{ of } D_2.$$

$$T_d : T_2 \rightarrow B_1 + B_2 + B_3 \text{ of } D_2.$$

The correspondences of irreps at HSPs from original SG to lowered SG:

$$n_{GM5}^{24} = n_{GM6}^{220} + n_{GM7}^{220} + 2n_{GM8}^{220} \quad n_{X5}^{24} = n_{H6}^{220} + n_{H7}^{220} + 2n_{H8}^{220} \quad n_{T3}^{24} = n_{N2}^{220} + n_{N4}^{220} \quad n_{T4}^{24} = n_{N3}^{220} + n_{N5}^{220} \quad n_{W3}^{24} = n_{P4}^{220} + n_{P5}^{220} + 2n_{P6}^{220} \\ n_{W2}^{24} = n_{P7}^{220} + n_{P8}^{220} \quad n_{W4}^{24} = n_{P7}^{220} + n_{P8}^{220} \quad n_{W5}^{24} = n_{P7}^{220} + n_{P8}^{220} \quad n_{R3}^{24} = n_{N3}^{220} + n_{N5}^{220} \quad n_{R4}^{24} = n_{N2}^{220} + n_{N4}^{220} \quad n_{S4}^{24} = n_{N2}^{220} + n_{N4}^{220} \quad n_{S3}^{24} = n_{N3}^{220} + n_{N5}^{220}$$

The lower SG is SG 43 when the preserved operations are: **(sub-SG label is 2) 1, 4, 19, 20.**

The transformation is:  $(\mathbf{a}_{43}, \mathbf{b}_{43}, \mathbf{c}_{43}) = (\mathbf{a}_{220}, \mathbf{b}_{220}, \mathbf{c}_{220}) \begin{pmatrix} 1 & -1 & 0 \\ 1 & 1 & 0 \\ 0 & 0 & 1 \end{pmatrix}, \overrightarrow{O_{220}O_{43}} = \frac{3}{8}\mathbf{a}_{43} + (-\frac{1}{8})\mathbf{b}_{43}$

The reduction of higher dimensional irrep:

$$T_d : T_1 \rightarrow A_2 + B_1 + B_2 \text{ of } C_{2v}.$$

$$T_d : T_2 \rightarrow A_1 + B_1 + B_2 \text{ of } C_{2v}.$$

The correspondences of irreps at HSPs from original SG to lowered SG:

$$n_{GM5}^{43} = n_{GM6}^{220} + n_{GM7}^{220} + 2n_{GM8}^{220} \quad n_{Y5}^{43} = n_{N2}^{220} \quad n_{Y3}^{43} = n_{N4}^{220} \quad n_{Y4}^{43} = n_{N5}^{220} \quad n_{Y2}^{43} = n_{N3}^{220} \quad n_{L2}^{43} = n_{N2}^{220} + n_{N3}^{220} + n_{N4}^{220} + n_{N5}^{220} \quad n_{Z5}^{43} = n_{H6}^{220} + n_{H7}^{220} + 2n_{H8}^{220} \quad n_{T5}^{43} = n_{N4}^{220} \quad n_{T3}^{43} = n_{N2}^{220} \quad n_{T4}^{43} = n_{N5}^{220} \quad n_{T2}^{43} = n_{N3}^{220}$$

The lower SG is SG 43 when the preserved operations are: **(sub-SG label is 3) 1, 2, 21, 22.**

The transformation is:  $(\mathbf{a}_{43}, \mathbf{b}_{43}, \mathbf{c}_{43}) = (\mathbf{a}_{220}, \mathbf{b}_{220}, \mathbf{c}_{220}) \begin{pmatrix} 0 & 0 & 1 \\ 1 & -1 & 0 \\ 1 & 1 & 0 \end{pmatrix}, \overrightarrow{O_{220}O_{43}} = \frac{3}{8}\mathbf{a}_{43} + (-\frac{1}{8})\mathbf{b}_{43}$

The reduction of higher dimensional irrep:

$$T_d: T_1 \rightarrow A_2 + B_1 + B_2 \text{ of } C_{2v}.$$

$$T_d: T_2 \rightarrow A_1 + B_1 + B_2 \text{ of } C_{2v}.$$

The correspondences of irreps at HSPs from original SG to lowered SG:

$$\begin{aligned} n_{GM5}^{43} &= n_{GM6}^{220} + n_{GM7}^{220} + 2n_{GM8}^{220} & n_{Y5}^{43} &= n_{N2}^{220} & n_{Y3}^{43} &= n_{N4}^{220} & n_{Y4}^{43} &= n_{N5}^{220} & n_{Y2}^{43} &= n_{N3}^{220} & n_{L2}^{43} &= n_{N2}^{220} + n_{N3}^{220} + n_{N4}^{220} + n_{N5}^{220} & n_{Z5}^{43} &= \\ n_{H6}^{220} + n_{H7}^{220} + 2n_{H8}^{220} & n_{T5}^{43} &= n_{N4}^{220} & n_{T3}^{43} &= n_{N2}^{220} & n_{T4}^{43} &= n_{N5}^{220} & n_{T2}^{43} &= n_{N3}^{220} \end{aligned}$$

The lower SG is SG 43 when the preserved operations are: **(sub-SG label is 4) 1, 3, 24, 23.**

The transformation is:  $(\mathbf{a}_{43}, \mathbf{b}_{43}, \mathbf{c}_{43}) = (\mathbf{a}_{220}, \mathbf{b}_{220}, \mathbf{c}_{220}) \begin{pmatrix} 1 & 1 & 0 \\ 0 & 0 & 1 \\ 1 & -1 & 0 \end{pmatrix}, \overrightarrow{O_{220}O_{43}} = \frac{3}{8}\mathbf{a}_{43} + (-\frac{1}{8})\mathbf{b}_{43}$

The reduction of higher dimensional irrep:

$$T_d: T_1 \rightarrow A_2 + B_1 + B_2 \text{ of } C_{2v}.$$

$$T_d: T_2 \rightarrow A_1 + B_1 + B_2 \text{ of } C_{2v}.$$

The correspondences of irreps at HSPs from original SG to lowered SG:

$$\begin{aligned} n_{GM5}^{43} &= n_{GM6}^{220} + n_{GM7}^{220} + 2n_{GM8}^{220} & n_{Y5}^{43} &= n_{N2}^{220} & n_{Y3}^{43} &= n_{N4}^{220} & n_{Y4}^{43} &= n_{N5}^{220} & n_{Y2}^{43} &= n_{N3}^{220} & n_{L2}^{43} &= n_{N2}^{220} + n_{N3}^{220} + n_{N4}^{220} + n_{N5}^{220} & n_{Z5}^{43} &= \\ n_{H6}^{220} + n_{H7}^{220} + 2n_{H8}^{220} & n_{T5}^{43} &= n_{N4}^{220} & n_{T3}^{43} &= n_{N2}^{220} & n_{T4}^{43} &= n_{N5}^{220} & n_{T2}^{43} &= n_{N3}^{220} \end{aligned}$$

The lower SG is SG 82 when the preserved operations are: **(sub-SG label is 5) 1, 17, 18, 4.**

The transformation is:  $(\mathbf{a}_{82}, \mathbf{b}_{82}, \mathbf{c}_{82}) = (\mathbf{a}_{220}, \mathbf{b}_{220}, \mathbf{c}_{220}) \begin{pmatrix} 0 & 1 & 0 \\ -1 & 0 & 0 \\ 0 & 0 & 1 \end{pmatrix}, \overrightarrow{O_{220}O_{82}} = \frac{3}{4}\mathbf{a}_{82} + (-\frac{1}{2})\mathbf{b}_{82} + (\frac{1}{8})\mathbf{c}_{82}$

The reduction of higher dimensional irrep:

$$T_d: T_1 \rightarrow A + {}^2E + {}^1E \text{ of } S_4.$$

$$T_d: T_2 \rightarrow {}^2E + B + {}^1E \text{ of } S_4.$$

The correspondences of irreps at HSPs from original SG to lowered SG:

$$\begin{aligned} n_{GM7}^{82} &= n_{GM7}^{220} + n_{GM8}^{220} & n_{GM8}^{82} &= n_{GM6}^{220} + n_{GM8}^{220} & n_{GM5}^{82} &= n_{GM7}^{220} + n_{GM8}^{220} & n_{GM6}^{82} &= n_{GM6}^{220} + n_{GM8}^{220} & n_{M7}^{82} &= n_{H6}^{220} + n_{H8}^{220} \\ n_{M8}^{82} &= n_{H7}^{220} + n_{H8}^{220} & n_{M5}^{82} &= n_{H7}^{220} + n_{H8}^{220} & n_{M6}^{82} &= n_{H6}^{220} + n_{H8}^{220} & n_{X4}^{82} &= n_{N2}^{220} + n_{N4}^{220} & n_{X3}^{82} &= n_{N3}^{220} + n_{N5}^{220} & n_{P7}^{82} &= n_{P4}^{220} + n_{P6}^{220} + n_{P7}^{220} \\ n_{P8}^{82} &= n_{P5}^{220} + n_{P6}^{220} + n_{P8}^{220} & n_{P5}^{82} &= n_{P7}^{220} + n_{P8}^{220} & n_{P6}^{82} &= n_{P7}^{220} + n_{P8}^{220} & n_{N2}^{82} &= n_{N2}^{220} + n_{N3}^{220} + n_{N4}^{220} + n_{N5}^{220} \end{aligned}$$

The lower SG is SG 82 when the preserved operations are: **(sub-SG label is 6) 1, 13, 14, 2.**

The transformation is:  $(\mathbf{a}_{82}, \mathbf{b}_{82}, \mathbf{c}_{82}) = (\mathbf{a}_{220}, \mathbf{b}_{220}, \mathbf{c}_{220}) \begin{pmatrix} 0 & 0 & 1 \\ 0 & 1 & 0 \\ -1 & 0 & 0 \end{pmatrix}, \overrightarrow{O_{220}O_{82}} = \frac{3}{4}\mathbf{a}_{82} + (-\frac{1}{2})\mathbf{b}_{82} + (\frac{1}{8})\mathbf{c}_{82}$

The reduction of higher dimensional irrep:

$$T_d: T_1 \rightarrow A + {}^2E + {}^1E \text{ of } S_4.$$

$$T_d: T_2 \rightarrow {}^2E + B + {}^1E \text{ of } S_4.$$

The correspondences of irreps at HSPs from original SG to lowered SG:

$$\begin{aligned} n_{GM7}^{82} &= n_{GM7}^{220} + n_{GM8}^{220} & n_{GM8}^{82} &= n_{GM6}^{220} + n_{GM8}^{220} & n_{GM5}^{82} &= n_{GM7}^{220} + n_{GM8}^{220} & n_{GM6}^{82} &= n_{GM6}^{220} + n_{GM8}^{220} & n_{M7}^{82} &= n_{H6}^{220} + n_{H8}^{220} \\ n_{M8}^{82} &= n_{H7}^{220} + n_{H8}^{220} & n_{M5}^{82} &= n_{H7}^{220} + n_{H8}^{220} & n_{M6}^{82} &= n_{H6}^{220} + n_{H8}^{220} & n_{X4}^{82} &= n_{N2}^{220} + n_{N4}^{220} & n_{X3}^{82} &= n_{N3}^{220} + n_{N5}^{220} & n_{P7}^{82} &= n_{P4}^{220} + n_{P6}^{220} + n_{P7}^{220} \\ n_{P8}^{82} &= n_{P5}^{220} + n_{P6}^{220} + n_{P8}^{220} & n_{P5}^{82} &= n_{P7}^{220} + n_{P8}^{220} & n_{P6}^{82} &= n_{P7}^{220} + n_{P8}^{220} & n_{N2}^{82} &= n_{N2}^{220} + n_{N3}^{220} + n_{N4}^{220} + n_{N5}^{220} \end{aligned}$$

The lower SG is SG 82 when the preserved operations are: **(sub-SG label is 7) 1, 15, 16, 3.**

The transformation is:  $(\mathbf{a}_{82}, \mathbf{b}_{82}, \mathbf{c}_{82}) = (\mathbf{a}_{220}, \mathbf{b}_{220}, \mathbf{c}_{220}) \begin{pmatrix} 0 & -1 & 0 \\ 0 & 0 & 1 \\ -1 & 0 & 0 \end{pmatrix}, \overrightarrow{O_{220}O_{82}} = \frac{1}{2}\mathbf{a}_{82} + (-\frac{3}{4})\mathbf{b}_{82} + (-\frac{1}{8})\mathbf{c}_{82}$

The reduction of higher dimensional irrep:

$$T_d: T_1 \rightarrow A + {}^2E + {}^1E \text{ of } S_4.$$

$$T_d: T_2 \rightarrow {}^2E + B + {}^1E \text{ of } S_4.$$

The correspondences of irreps at HSPs from original SG to lowered SG:

$$\begin{aligned} n_{GM7}^{82} &= n_{GM7}^{220} + n_{GM8}^{220} & n_{GM8}^{82} &= n_{GM6}^{220} + n_{GM8}^{220} & n_{GM5}^{82} &= n_{GM7}^{220} + n_{GM8}^{220} & n_{GM6}^{82} &= n_{GM6}^{220} + n_{GM8}^{220} & n_{M7}^{82} &= n_{H6}^{220} + n_{H8}^{220} \\ n_{M8}^{82} &= n_{H7}^{220} + n_{H8}^{220} & n_{M5}^{82} &= n_{H7}^{220} + n_{H8}^{220} & n_{M6}^{82} &= n_{H6}^{220} + n_{H8}^{220} & n_{X4}^{82} &= n_{N2}^{220} + n_{N4}^{220} & n_{X3}^{82} &= n_{N3}^{220} + n_{N5}^{220} & n_{P7}^{82} &= n_{P4}^{220} + n_{P6}^{220} + n_{P7}^{220} \\ n_{P8}^{82} &= n_{P5}^{220} + n_{P6}^{220} + n_{P8}^{220} & n_{P5}^{82} &= n_{P7}^{220} + n_{P8}^{220} & n_{P6}^{82} &= n_{P7}^{220} + n_{P8}^{220} & n_{N2}^{82} &= n_{N2}^{220} + n_{N3}^{220} + n_{N4}^{220} + n_{N5}^{220} \end{aligned}$$

The lower SG is SG 122 when the preserved operations are: **(sub-SG label is 8) 1, 18, 17, 4, 2, 3, 19, 20.**

The transformation is:  $(\mathbf{a}_{122}, \mathbf{b}_{122}, \mathbf{c}_{122}) = (\mathbf{a}_{220}, \mathbf{b}_{220}, \mathbf{c}_{220}) \begin{pmatrix} 1 & 0 & 0 \\ 0 & 1 & 0 \\ 0 & 0 & 1 \end{pmatrix}, \overrightarrow{O_{220}O_{122}} = \frac{1}{2}\mathbf{a}_{122} + (-\frac{3}{4})\mathbf{b}_{122} + (\frac{1}{8})\mathbf{c}_{122}$

The reduction of higher dimensional irrep:

$$T_d : E \rightarrow A_1 + B_1 \text{ of } D_{2d}.$$

The correspondences of irreps at HSPs from original SG to lowered SG:

$$\begin{aligned} n_{GM6}^{122} &= n_{GM7}^{220} + n_{GM8}^{220} & n_{GM7}^{122} &= n_{GM6}^{220} + n_{GM8}^{220} & n_{M6}^{122} &= n_{H7}^{220} + n_{H8}^{220} & n_{M7}^{122} &= n_{H6}^{220} + n_{H8}^{220} & n_{X5}^{122} &= n_{N2}^{220} & n_{X3}^{122} &= n_{N4}^{220} & n_{X2}^{122} &= n_{N5}^{220} \\ n_{N3}^{122} &= n_{N5}^{220} & n_{P3}^{122} &= n_{P4}^{220} + n_{P6}^{220} & n_{P6}^{122} &= n_{P5}^{220} + n_{P6}^{220} & n_{P5}^{122} &= n_{P7}^{220} & n_{P4}^{122} &= n_{P8}^{220} & n_{P7}^{122} &= n_{P7}^{220} + n_{P8}^{220} & n_{N3}^{122} &= n_{N3}^{220} + n_{N5}^{220} \\ n_{N4}^{122} &= n_{N2}^{220} + n_{N4}^{220} \end{aligned}$$

The lower SG is SG 122 when the preserved operations are: **(sub-SG label is 9)** 1, 14, 13, 2, 3, 4, 21, 22.

The transformation is:  $(\mathbf{a}_{122}, \mathbf{b}_{122}, \mathbf{c}_{122}) = (\mathbf{a}_{220}, \mathbf{b}_{220}, \mathbf{c}_{220}) \begin{pmatrix} 0 & 0 & -1 \\ -1 & 0 & 0 \\ 0 & 1 & 0 \end{pmatrix}, \overrightarrow{O_{220}O_{122}} = -\frac{1}{2}\mathbf{a}_{122} + (-\frac{1}{4})\mathbf{b}_{122} + (\frac{1}{8})\mathbf{c}_{122}$

The reduction of higher dimensional irrep:

$$T_d : E \rightarrow A_1 + B_1 \text{ of } D_{2d}.$$

The correspondences of irreps at HSPs from original SG to lowered SG:

$$\begin{aligned} n_{GM6}^{122} &= n_{GM7}^{220} + n_{GM8}^{220} & n_{GM7}^{122} &= n_{GM6}^{220} + n_{GM8}^{220} & n_{M6}^{122} &= n_{H7}^{220} + n_{H8}^{220} & n_{M7}^{122} &= n_{H6}^{220} + n_{H8}^{220} & n_{X5}^{122} &= n_{N2}^{220} & n_{X3}^{122} &= n_{N4}^{220} & n_{X2}^{122} &= n_{N5}^{220} \\ n_{N3}^{122} &= n_{N5}^{220} & n_{P3}^{122} &= n_{P8}^{220} & n_{P6}^{122} &= n_{P7}^{220} & n_{P5}^{122} &= n_{P5}^{220} + n_{P6}^{220} & n_{P4}^{122} &= n_{P4}^{220} + n_{P6}^{220} & n_{P7}^{122} &= n_{P7}^{220} + n_{P8}^{220} & n_{N3}^{122} &= n_{N2}^{220} + n_{N4}^{220} \\ n_{N4}^{122} &= n_{N3}^{220} + n_{N5}^{220} \end{aligned}$$

The lower SG is SG 122 when the preserved operations are: **(sub-SG label is 10)** 1, 16, 15, 3, 4, 2, 24, 23.

The transformation is:  $(\mathbf{a}_{122}, \mathbf{b}_{122}, \mathbf{c}_{122}) = (\mathbf{a}_{220}, \mathbf{b}_{220}, \mathbf{c}_{220}) \begin{pmatrix} -1 & 0 & 0 \\ 0 & 0 & 1 \\ 0 & 1 & 0 \end{pmatrix}, \overrightarrow{O_{220}O_{122}} = \frac{1}{4}\mathbf{a}_{122} + (-\frac{1}{2})\mathbf{b}_{122} + (-\frac{1}{8})\mathbf{c}_{122}$

The reduction of higher dimensional irrep:

$$T_d : E \rightarrow A_1 + B_1 \text{ of } D_{2d}.$$

The correspondences of irreps at HSPs from original SG to lowered SG:

$$\begin{aligned} n_{GM6}^{122} &= n_{GM7}^{220} + n_{GM8}^{220} & n_{GM7}^{122} &= n_{GM6}^{220} + n_{GM8}^{220} & n_{M6}^{122} &= n_{H6}^{220} + n_{H8}^{220} & n_{M7}^{122} &= n_{H7}^{220} + n_{H8}^{220} & n_{X5}^{122} &= n_{N2}^{220} & n_{X3}^{122} &= n_{N4}^{220} & n_{X2}^{122} &= n_{N5}^{220} \\ n_{N2}^{122} &= n_{N4}^{220} & n_{P3}^{122} &= n_{P5}^{220} + n_{P6}^{220} & n_{P6}^{122} &= n_{P4}^{220} + n_{P6}^{220} & n_{P5}^{122} &= n_{P8}^{220} & n_{P4}^{122} &= n_{P7}^{220} & n_{P7}^{122} &= n_{P7}^{220} + n_{P8}^{220} & n_{N3}^{122} &= n_{N2}^{220} + n_{N4}^{220} \\ n_{N4}^{122} &= n_{N3}^{220} + n_{N5}^{220} \end{aligned}$$

The lower SG is SG 146 when the preserved operations are: **(sub-SG label is 11)** 1, 5, 6.

The transformation is:  $(\mathbf{a}_{146}, \mathbf{b}_{146}, \mathbf{c}_{146}) = (\mathbf{a}_{220}, \mathbf{b}_{220}, \mathbf{c}_{220}) \begin{pmatrix} \frac{1}{2} & -\frac{1}{2} & \frac{1}{2} \\ \frac{1}{2} & \frac{1}{2} & -\frac{1}{2} \\ -\frac{1}{2} & \frac{1}{2} & \frac{1}{2} \end{pmatrix}, \overrightarrow{O_{220}O_{146}} = -\frac{1}{3}\mathbf{a}_{146} + (\frac{2}{3})\mathbf{b}_{146} + (-\frac{1}{3})\mathbf{c}_{146}$

The reduction of higher dimensional irrep:

$$T_d : T_1 \rightarrow A + {}^2E + {}^1E \text{ of } C_3.$$

$$T_d : T_2 \rightarrow A + {}^2E + {}^1E \text{ of } C_3.$$

The correspondences of irreps at HSPs from original SG to lowered SG:

$$\begin{aligned} n_{GM4}^{146} &= 2n_{GM8}^{220} & n_{GM6}^{146} &= n_{GM6}^{220} + n_{GM7}^{220} + n_{GM8}^{220} & n_{GM5}^{146} &= n_{GM6}^{220} + n_{GM7}^{220} + n_{GM8}^{220} & n_{L2}^{146} &= n_{N2}^{220} + n_{N3}^{220} + n_{N4}^{220} + n_{N5}^{220} \\ n_{F2}^{146} &= n_{N2}^{220} + n_{N3}^{220} + n_{N4}^{220} + n_{N5}^{220} & n_{T4}^{146} &= 2n_{H8}^{220} & n_{T6}^{146} &= n_{H6}^{220} + n_{H7}^{220} + n_{H8}^{220} & n_{T5}^{146} &= n_{H6}^{220} + n_{H7}^{220} + n_{H8}^{220} \end{aligned}$$

The lower SG is SG 146 when the preserved operations are: **(sub-SG label is 12)** 1, 12, 11.

The transformation is:  $(\mathbf{a}_{146}, \mathbf{b}_{146}, \mathbf{c}_{146}) = (\mathbf{a}_{220}, \mathbf{b}_{220}, \mathbf{c}_{220}) \begin{pmatrix} -\frac{1}{2} & -\frac{1}{2} & \frac{1}{2} \\ \frac{1}{2} & -\frac{1}{2} & -\frac{1}{2} \\ \frac{1}{2} & -\frac{1}{2} & \frac{1}{2} \end{pmatrix}, \overrightarrow{O_{220}O_{146}} = -\frac{1}{3}\mathbf{a}_{146} + (\frac{1}{6})\mathbf{b}_{146} + (\frac{1}{6})\mathbf{c}_{146}$

The reduction of higher dimensional irrep:

$$T_d : T_1 \rightarrow A + {}^2E + {}^1E \text{ of } C_3.$$

$$T_d : T_2 \rightarrow A + {}^2E + {}^1E \text{ of } C_3.$$

The correspondences of irreps at HSPs from original SG to lowered SG:

$$\begin{aligned} n_{GM4}^{146} &= 2n_{GM8}^{220} & n_{GM6}^{146} &= n_{GM6}^{220} + n_{GM7}^{220} + n_{GM8}^{220} & n_{GM5}^{146} &= n_{GM6}^{220} + n_{GM7}^{220} + n_{GM8}^{220} & n_{L2}^{146} &= n_{N2}^{220} + n_{N3}^{220} + n_{N4}^{220} + n_{N5}^{220} \\ n_{F2}^{146} &= n_{N2}^{220} + n_{N3}^{220} + n_{N4}^{220} + n_{N5}^{220} & n_{T4}^{146} &= 2n_{H8}^{220} & n_{T6}^{146} &= n_{H6}^{220} + n_{H7}^{220} + n_{H8}^{220} & n_{T5}^{146} &= n_{H6}^{220} + n_{H7}^{220} + n_{H8}^{220} \end{aligned}$$

The lower SG is SG 146 when the preserved operations are: **(sub-SG label is 13)** 1, 8, 7.

The transformation is:  $(\mathbf{a}_{146}, \mathbf{b}_{146}, \mathbf{c}_{146}) = (\mathbf{a}_{220}, \mathbf{b}_{220}, \mathbf{c}_{220}) \begin{pmatrix} \frac{1}{2} & -\frac{1}{2} & \frac{1}{2} \\ -\frac{1}{2} & -\frac{1}{2} & \frac{1}{2} \\ \frac{1}{2} & -\frac{1}{2} & -\frac{1}{2} \end{pmatrix}, \overrightarrow{O_{220}O_{146}} = -\frac{1}{3}\mathbf{a}_{146} + (\frac{1}{6})\mathbf{b}_{146} + (\frac{1}{6})\mathbf{c}_{146}$

The reduction of higher dimensional irrep:

$$T_d : T_1 \rightarrow A + {}^2E + {}^1E \text{ of } C_3.$$

$$T_d : T_2 \rightarrow A + {}^2E + {}^1E \text{ of } C_3.$$

The correspondences of irreps at HSPs from original SG to lowered SG:

$$\begin{aligned} n_{GM4}^{146} &= 2n_{GM8}^{220} n_{GM6}^{146} = n_{GM6}^{220} + n_{GM7}^{220} + n_{GM8}^{220} n_{L2}^{146} = n_{N2}^{220} + n_{N3}^{220} + n_{N4}^{220} + n_{N5}^{220} \\ n_{F2}^{146} &= n_{N2}^{220} + n_{N3}^{220} + n_{N4}^{220} + n_{N5}^{220} n_{T4}^{146} = 2n_{H8}^{220} n_{T6}^{146} = n_{H6}^{220} + n_{H7}^{220} + n_{H8}^{220} n_{T5}^{146} = n_{H6}^{220} + n_{H7}^{220} + n_{H8}^{220} \end{aligned}$$

The lower SG is SG 146 when the preserved operations are: **(sub-SG label is 14)** 1, 10, 9.

$$\text{The transformation is: } (\mathbf{a}_{146}, \mathbf{b}_{146}, \mathbf{c}_{146}) = (\mathbf{a}_{220}, \mathbf{b}_{220}, \mathbf{c}_{220}) \begin{pmatrix} -\frac{1}{2} & -\frac{1}{2} & \frac{1}{2} \\ -\frac{1}{2} & \frac{1}{2} & \frac{1}{2} \\ -\frac{1}{2} & \frac{1}{2} & -\frac{1}{2} \end{pmatrix}, \overrightarrow{O_{220}O_{146}} = -\frac{1}{2}\mathbf{a}_{146} + \left(\frac{1}{2}\right)\mathbf{b}_{146}$$

The reduction of higher dimensional irrep:

$$T_d : T_1 \rightarrow A + {}^2E + {}^1E \text{ of } C_3.$$

$$T_d : T_2 \rightarrow A + {}^2E + {}^1E \text{ of } C_3.$$

The correspondences of irreps at HSPs from original SG to lowered SG:

$$\begin{aligned} n_{GM4}^{146} &= 2n_{GM8}^{220} n_{GM6}^{146} = n_{GM6}^{220} + n_{GM7}^{220} + n_{GM8}^{220} n_{L2}^{146} = n_{N2}^{220} + n_{N3}^{220} + n_{N4}^{220} + n_{N5}^{220} \\ n_{F2}^{146} &= n_{N2}^{220} + n_{N3}^{220} + n_{N4}^{220} + n_{N5}^{220} n_{T4}^{146} = 2n_{H8}^{220} n_{T6}^{146} = n_{H6}^{220} + n_{H7}^{220} + n_{H8}^{220} n_{T5}^{146} = n_{H6}^{220} + n_{H7}^{220} + n_{H8}^{220} \end{aligned}$$

The lower SG is SG 199 when the preserved operations are: **(sub-SG label is 15)** 1, 2, 3, 4, 5, 12, 8, 10, 6, 11, 7, 9.

$$\text{The transformation is: } (\mathbf{a}_{199}, \mathbf{b}_{199}, \mathbf{c}_{199}) = (\mathbf{a}_{220}, \mathbf{b}_{220}, \mathbf{c}_{220}) \begin{pmatrix} 0 & 0 & -1 \\ 1 & 0 & 0 \\ 0 & -1 & 0 \end{pmatrix}, \overrightarrow{O_{220}O_{199}} = \frac{1}{2}\mathbf{a}_{199} + \left(-\frac{1}{2}\right)\mathbf{b}_{199}$$

The reduction of higher dimensional irrep:

$$T_d : E \rightarrow {}^1E + {}^2E \text{ of } T.$$

The correspondences of irreps at HSPs from original SG to lowered SG:

$$\begin{aligned} n_{GM6}^{199} &= n_{GM8}^{220} n_{GM7}^{199} = n_{GM8}^{220} n_{GM5}^{199} = n_{GM6}^{220} + n_{GM7}^{220} n_{H6}^{199} = n_{H8}^{220} n_{H7}^{199} = n_{H8}^{220} n_{H5}^{199} = n_{H6}^{220} + n_{H7}^{220} n_{N3}^{199} = n_{N2}^{220} + n_{N4}^{220} \\ n_{N4}^{199} &= n_{N3}^{220} + n_{N5}^{220} n_{P4}^{199} = n_{P4}^{220} + n_{P5}^{220} n_{P6}^{199} = n_{P6}^{220} n_{P5}^{199} = n_{P6}^{220} n_{P7}^{199} = n_{P7}^{220} + n_{P8}^{220} \end{aligned}$$

### 118. Lowered SGs by higher-dimensional irreps of pairings in SG 221

The representative operations of SG/T for SG 221:

$$\begin{aligned} &1 : (x, y, z), 2 : (x, -z, y), 3 : (x, z, -y), 4 : (z, y, -x), 5 : (-z, y, x), 6 : (-y, x, z), 7 : (y, -x, z), 8 : (x, -y, -z), \\ &9 : (-x, y, -z), 10 : (-x, -y, z), 11 : (y, x, -z), 12 : (-y, -x, -z), 13 : (-x, z, y), 14 : (-x, -z, -y), 15 : (z, -y, x), \\ &16 : (-z, -y, -x), 17 : (z, x, y), 18 : (y, z, x), 19 : (-y, z, -x), 20 : (-z, -x, y), 21 : (-y, -z, x), 22 : (z, -x, -y), 23 : \\ &(y, -z, -x), 24 : (-z, x, -y), 25 : (-x, -y, -z), 26 : (-x, z, -y), 27 : (-x, -z, y), 28 : (-z, -y, x), 29 : (z, -y, -x), \\ &30 : (y, -x, -z), 31 : (-y, x, -z), 32 : (-x, y, z), 33 : (x, -y, z), 34 : (x, y, -z), 35 : (-y, -x, z), 36 : (y, x, z), \\ &37 : (x, -z, -y), 38 : (x, z, y), 39 : (-z, y, -x), 40 : (z, y, x), 41 : (-z, -x, -y), 42 : (-y, -z, -x), 43 : (y, -z, x), \\ &44 : (z, x, -y), 45 : (y, z, -x), 46 : (-z, x, y), 47 : (-y, z, x), 48 : (z, -x, y). \end{aligned}$$

The lower SG is SG 47 when the preserved operations are: **(sub-SG label is 1)** 1, 8, 9, 10, 25, 32, 33, 34.

$$\text{The transformation is: } (\mathbf{a}_{47}, \mathbf{b}_{47}, \mathbf{c}_{47}) = (\mathbf{a}_{221}, \mathbf{b}_{221}, \mathbf{c}_{221}) \begin{pmatrix} 0 & 0 & 1 \\ 1 & 0 & 0 \\ 0 & 1 & 0 \end{pmatrix}, \overrightarrow{O_{221}O_{47}} = \frac{1}{2}\mathbf{a}_{47} + \left(\frac{1}{2}\right)\mathbf{c}_{47}$$

The reduction of higher dimensional irrep:

$$O_h : T_{1g} \rightarrow B_{2g} + B_{1g} + B_{3g} \text{ of } D_{2h}.$$

$$O_h : T_{2g} \rightarrow B_{2g} + B_{1g} + B_{3g} \text{ of } D_{2h}.$$

$$O_h : T_{1u} \rightarrow B_{2u} + B_{1u} + B_{3u} \text{ of } D_{2h}.$$

$$O_h : T_{2u} \rightarrow B_{2u} + B_{1u} + B_{3u} \text{ of } D_{2h}.$$

The correspondences of irreps at HSPs from original SG to lowered SG:

$$\begin{aligned} n_{GM6}^{47} &= 2n_{GM11}^{221} + n_{GM8}^{221} + n_{GM9}^{221} n_{GM5}^{47} = 2n_{GM10}^{221} + n_{GM6}^{221} + n_{GM7}^{221} n_{X6}^{47} = n_{X6}^{221} + n_{X7}^{221} n_{X5}^{47} = n_{X8}^{221} + n_{X9}^{221} n_{S6}^{47} = \\ &n_{M6}^{221} + n_{M7}^{221} n_{S5}^{47} = n_{M8}^{221} + n_{M9}^{221} n_{R6}^{47} = 2n_{R11}^{221} + n_{R8}^{221} + n_{R9}^{221} n_{R5}^{47} = 2n_{R10}^{221} + n_{R6}^{221} + n_{R7}^{221} n_{U6}^{47} = n_{M8}^{221} + n_{M9}^{221} n_{U5}^{47} = n_{M6}^{221} + n_{M7}^{221} \\ &n_{Z6}^{47} = n_{X6}^{221} + n_{X7}^{221} n_{Z5}^{47} = n_{X8}^{221} + n_{X9}^{221} n_{T6}^{47} = n_{M6}^{221} + n_{M7}^{221} n_{T5}^{47} = n_{M8}^{221} + n_{M9}^{221} n_{Y6}^{47} = n_{X8}^{221} + n_{X9}^{221} n_{Y5}^{47} = n_{X6}^{221} + n_{X7}^{221} \end{aligned}$$

The lower SG is SG 65 when the preserved operations are: **(sub-SG label is 2)** 1, 8, 13, 14, 25, 32, 37, 38.

The transformation is:  $(\mathbf{a}_{65}, \mathbf{b}_{65}, \mathbf{c}_{65}) = (\mathbf{a}_{221}, \mathbf{b}_{221}, \mathbf{c}_{221}) \begin{pmatrix} 0 & 0 & 1 \\ 1 & -1 & 0 \\ 1 & 1 & 0 \end{pmatrix}, \overrightarrow{O_{221}O_{65}} = \frac{1}{2}\mathbf{c}_{65}$

The reduction of higher dimensional irrep:

$$O_h : T_{1g} \rightarrow B_{2g} + B_{1g} + B_{3g} \text{ of } D_{2h}.$$

$$O_h : T_{2g} \rightarrow A_g + B_{2g} + B_{3g} \text{ of } D_{2h}.$$

$$O_h : T_{1u} \rightarrow B_{2u} + B_{1u} + B_{3u} \text{ of } D_{2h}.$$

$$O_h : T_{2u} \rightarrow A_u + B_{2u} + B_{3u} \text{ of } D_{2h}.$$

The correspondences of irreps at HSPs from original SG to lowered SG:

$$\begin{aligned} n_{GM6}^{65} &= 2n_{GM11}^{221} + n_{GM8}^{221} + n_{GM9}^{221} & n_{GM5}^{65} &= 2n_{GM10}^{221} + n_{GM6}^{221} + n_{GM7}^{221} & n_{Y6}^{65} &= n_{M8}^{221} + n_{M9}^{221} & n_{Y5}^{65} &= n_{M6}^{221} + n_{M7}^{221} & n_{S6}^{65} &= \\ n_{X8}^{221} + n_{X9}^{221} & n_{S4}^{65} &= n_{X6}^{221} + n_{X7}^{221} & n_{S5}^{65} &= n_{X8}^{221} + n_{X9}^{221} & n_{S3}^{65} &= n_{X6}^{221} + n_{X7}^{221} & n_{Z6}^{65} &= n_{X6}^{221} + n_{X7}^{221} & n_{Z5}^{65} &= n_{X8}^{221} + n_{X9}^{221} & n_{T6}^{65} &= \\ 2n_{R10}^{221} + n_{R6}^{221} + n_{R7}^{221} & n_{T5}^{65} &= 2n_{R11}^{221} + n_{R8}^{221} + n_{R9}^{221} & n_{R6}^{65} &= n_{M6}^{221} + n_{M7}^{221} & n_{R4}^{65} &= n_{M8}^{221} + n_{M9}^{221} & n_{R5}^{65} &= n_{M6}^{221} + n_{M7}^{221} & n_{R3}^{65} &= \\ n_{M8}^{221} + n_{M9}^{221} & & & & & & & & & & & & & \end{aligned}$$

The lower SG is SG 65 when the preserved operations are: **(sub-SG label is 3)** 1, 9, 16, 15, 25, 33, 40, 39.

The transformation is:  $(\mathbf{a}_{65}, \mathbf{b}_{65}, \mathbf{c}_{65}) = (\mathbf{a}_{221}, \mathbf{b}_{221}, \mathbf{c}_{221}) \begin{pmatrix} -1 & 1 & 0 \\ 0 & 0 & 1 \\ 1 & 1 & 0 \end{pmatrix}, \overrightarrow{O_{221}O_{65}} = \frac{1}{2}\mathbf{c}_{65}$

The reduction of higher dimensional irrep:

$$O_h : T_{1g} \rightarrow B_{2g} + B_{1g} + B_{3g} \text{ of } D_{2h}.$$

$$O_h : T_{2g} \rightarrow A_g + B_{2g} + B_{3g} \text{ of } D_{2h}.$$

$$O_h : T_{1u} \rightarrow B_{2u} + B_{1u} + B_{3u} \text{ of } D_{2h}.$$

$$O_h : T_{2u} \rightarrow A_u + B_{2u} + B_{3u} \text{ of } D_{2h}.$$

The correspondences of irreps at HSPs from original SG to lowered SG:

$$\begin{aligned} n_{GM6}^{65} &= 2n_{GM11}^{221} + n_{GM8}^{221} + n_{GM9}^{221} & n_{GM5}^{65} &= 2n_{GM10}^{221} + n_{GM6}^{221} + n_{GM7}^{221} & n_{Y6}^{65} &= n_{M8}^{221} + n_{M9}^{221} & n_{Y5}^{65} &= n_{M6}^{221} + n_{M7}^{221} & n_{S6}^{65} &= \\ n_{X8}^{221} + n_{X9}^{221} & n_{S4}^{65} &= n_{X6}^{221} + n_{X7}^{221} & n_{S5}^{65} &= n_{X8}^{221} + n_{X9}^{221} & n_{S3}^{65} &= n_{X6}^{221} + n_{X7}^{221} & n_{Z6}^{65} &= n_{X6}^{221} + n_{X7}^{221} & n_{Z5}^{65} &= n_{X8}^{221} + n_{X9}^{221} & n_{T6}^{65} &= \\ 2n_{R10}^{221} + n_{R6}^{221} + n_{R7}^{221} & n_{T5}^{65} &= 2n_{R11}^{221} + n_{R8}^{221} + n_{R9}^{221} & n_{R6}^{65} &= n_{M6}^{221} + n_{M7}^{221} & n_{R4}^{65} &= n_{M8}^{221} + n_{M9}^{221} & n_{R5}^{65} &= n_{M6}^{221} + n_{M7}^{221} & n_{R3}^{65} &= \\ n_{M8}^{221} + n_{M9}^{221} & & & & & & & & & & & & & \end{aligned}$$

The lower SG is SG 65 when the preserved operations are: **(sub-SG label is 4)** 1, 10, 11, 12, 25, 34, 35, 36.

The transformation is:  $(\mathbf{a}_{65}, \mathbf{b}_{65}, \mathbf{c}_{65}) = (\mathbf{a}_{221}, \mathbf{b}_{221}, \mathbf{c}_{221}) \begin{pmatrix} 1 & -1 & 0 \\ 1 & 1 & 0 \\ 0 & 0 & 1 \end{pmatrix}, \overrightarrow{O_{221}O_{65}} = \frac{1}{2}\mathbf{c}_{65}$

The reduction of higher dimensional irrep:

$$O_h : T_{1g} \rightarrow B_{2g} + B_{1g} + B_{3g} \text{ of } D_{2h}.$$

$$O_h : T_{2g} \rightarrow A_g + B_{2g} + B_{3g} \text{ of } D_{2h}.$$

$$O_h : T_{1u} \rightarrow B_{2u} + B_{1u} + B_{3u} \text{ of } D_{2h}.$$

$$O_h : T_{2u} \rightarrow A_u + B_{2u} + B_{3u} \text{ of } D_{2h}.$$

The correspondences of irreps at HSPs from original SG to lowered SG:

$$\begin{aligned} n_{GM6}^{65} &= 2n_{GM11}^{221} + n_{GM8}^{221} + n_{GM9}^{221} & n_{GM5}^{65} &= 2n_{GM10}^{221} + n_{GM6}^{221} + n_{GM7}^{221} & n_{Y6}^{65} &= n_{M8}^{221} + n_{M9}^{221} & n_{Y5}^{65} &= n_{M6}^{221} + n_{M7}^{221} & n_{S6}^{65} &= \\ n_{X8}^{221} + n_{X9}^{221} & n_{S4}^{65} &= n_{X6}^{221} + n_{X7}^{221} & n_{S5}^{65} &= n_{X8}^{221} + n_{X9}^{221} & n_{S3}^{65} &= n_{X6}^{221} + n_{X7}^{221} & n_{Z6}^{65} &= n_{X6}^{221} + n_{X7}^{221} & n_{Z5}^{65} &= n_{X8}^{221} + n_{X9}^{221} & n_{T6}^{65} &= \\ 2n_{R10}^{221} + n_{R6}^{221} + n_{R7}^{221} & n_{T5}^{65} &= 2n_{R11}^{221} + n_{R8}^{221} + n_{R9}^{221} & n_{R6}^{65} &= n_{M6}^{221} + n_{M7}^{221} & n_{R4}^{65} &= n_{M8}^{221} + n_{M9}^{221} & n_{R5}^{65} &= n_{M6}^{221} + n_{M7}^{221} & n_{R3}^{65} &= \\ n_{M8}^{221} + n_{M9}^{221} & & & & & & & & & & & & & \end{aligned}$$

The lower SG is SG 83 when the preserved operations are: **(sub-SG label is 5)** 1, 6, 7, 10, 25, 30, 31, 34.

The transformation is:  $(\mathbf{a}_{83}, \mathbf{b}_{83}, \mathbf{c}_{83}) = (\mathbf{a}_{221}, \mathbf{b}_{221}, \mathbf{c}_{221}) \begin{pmatrix} -1 & 0 & 0 \\ 0 & -1 & 0 \\ 0 & 0 & 1 \end{pmatrix}, \overrightarrow{O_{221}O_{83}} = \frac{1}{2}\mathbf{c}_{83}$

The reduction of higher dimensional irrep:

$$O_h : T_{1g} \rightarrow A_g + {}^2E_g + {}^1E_g \text{ of } C_{4h}.$$

$$O_h : T_{2g} \rightarrow {}^2E_g + B_g + {}^1E_g \text{ of } C_{4h}.$$

$$O_h : T_{1u} \rightarrow A_u + {}^2E_u + {}^1E_u \text{ of } C_{4h}.$$

$$O_h : T_{2u} \rightarrow {}^2E_u + B_u + {}^1E_u \text{ of } C_{4h}.$$

The correspondences of irreps at HSPs from original SG to lowered SG:

$$\begin{aligned} n_{GM9}^{83} &= n_{GM11}^{221} + n_{GM9}^{221} & n_{GM5}^{83} &= n_{GM10}^{221} + n_{GM7}^{221} & n_{GM11}^{83} &= n_{GM11}^{221} + n_{GM9}^{221} & n_{GM7}^{83} &= n_{GM10}^{221} + n_{GM7}^{221} & n_{GM12}^{83} &= \\ n_{GM11}^{221} + n_{GM8}^{221} & n_{GM8}^{83} &= n_{GM10}^{221} + n_{GM6}^{221} & n_{GM10}^{83} &= n_{GM11}^{221} + n_{GM8}^{221} & n_{GM6}^{83} &= n_{GM10}^{221} + n_{GM6}^{221} & n_{X6}^{83} &= n_{X8}^{221} + n_{X9}^{221} & n_{X4}^{83} &= \end{aligned}$$

$$\begin{aligned}
 n_{X6}^{221} + n_{X7}^{221} n_{X5}^{83} &= n_{X8}^{221} + n_{X9}^{221} n_{X3}^{83} = n_{X6}^{221} + n_{X7}^{221} n_{M9}^{83} = n_{M8}^{221} n_{M5}^{83} = n_{M6}^{221} n_{M11}^{83} = n_{M8}^{221} n_{M7}^{83} = n_{M6}^{221} n_{M12}^{83} = n_{M9}^{221} \\
 n_{M8}^{83} &= n_{M7}^{221} n_{M10}^{83} = n_{M9}^{221} n_{M6}^{83} = n_{M7}^{221} n_{A9}^{83} = n_{R10}^{221} + n_{R7}^{221} n_{A5}^{83} = n_{R11}^{221} + n_{R9}^{221} n_{A11}^{83} = n_{R10}^{221} + n_{R7}^{221} n_{A7}^{83} = n_{R11}^{221} + n_{R9}^{221} \\
 n_{A12}^{83} &= n_{R10}^{221} + n_{R6}^{221} n_{A8}^{83} = n_{R11}^{221} + n_{R8}^{221} n_{A10}^{83} = n_{R10}^{221} + n_{R6}^{221} n_{A6}^{83} = n_{R11}^{221} + n_{R8}^{221} n_{R6}^{83} = n_{M6}^{221} + n_{M7}^{221} n_{R4}^{83} = n_{M8}^{221} + n_{M9}^{221} \\
 n_{R5}^{83} &= n_{M6}^{221} + n_{M7}^{221} n_{R3}^{83} = n_{M8}^{221} + n_{M9}^{221} n_{Z9}^{83} = n_{X7}^{221} n_{Z5}^{83} = n_{X9}^{221} n_{Z11}^{83} = n_{X7}^{221} n_{Z7}^{83} = n_{X9}^{221} n_{Z12}^{83} = n_{X6}^{221} n_{Z8}^{83} = n_{X8}^{221} n_{Z10}^{83} = \\
 n_{X6}^{221} n_{Z6}^{83} &= n_{X8}^{221}
 \end{aligned}$$

The lower SG is SG 83 when the preserved operations are: **(sub-SG label is 6)** 1, 2, 3, 8, 25, 26, 27, 32.

The transformation is:  $(\mathbf{a}_{83}, \mathbf{b}_{83}, \mathbf{c}_{83}) = (\mathbf{a}_{221}, \mathbf{b}_{221}, \mathbf{c}_{221}) \begin{pmatrix} 0 & 0 & 1 \\ -1 & 0 & 0 \\ 0 & -1 & 0 \end{pmatrix}, \overrightarrow{O_{221}O_{83}} = \frac{1}{2}\mathbf{c}_{83}$

The reduction of higher dimensional irrep:

$$\begin{aligned}
 O_h : T_{1g} &\rightarrow A_g + {}^2E_g + {}^1E_g \text{ of } C_{4h}. \\
 O_h : T_{2g} &\rightarrow {}^2E_g + B_g + {}^1E_g \text{ of } C_{4h}. \\
 O_h : T_{1u} &\rightarrow A_u + {}^2E_u + {}^1E_u \text{ of } C_{4h}. \\
 O_h : T_{2u} &\rightarrow {}^2E_u + B_u + {}^1E_u \text{ of } C_{4h}.
 \end{aligned}$$

The correspondences of irreps at HSPs from original SG to lowered SG:

$$\begin{aligned}
 n_{GM9}^{83} &= n_{GM11}^{221} + n_{GM9}^{221} n_{GM5}^{83} = n_{GM10}^{221} + n_{GM7}^{221} n_{GM11}^{83} = n_{GM11}^{221} + n_{GM9}^{221} n_{GM7}^{83} = n_{GM10}^{221} + n_{GM7}^{221} n_{GM12}^{83} = \\
 n_{GM11}^{221} + n_{GM8}^{221} n_{GM8}^{83} &= n_{GM10}^{221} + n_{GM6}^{221} n_{GM10}^{83} = n_{GM11}^{221} + n_{GM8}^{221} n_{GM6}^{83} = n_{GM10}^{221} + n_{GM6}^{221} n_{X6}^{83} = n_{X8}^{221} + n_{X9}^{221} n_{X4}^{83} = \\
 n_{X6}^{221} + n_{X7}^{221} n_{X5}^{83} &= n_{X8}^{221} + n_{X9}^{221} n_{X3}^{83} = n_{X6}^{221} + n_{X7}^{221} n_{M9}^{83} = n_{M8}^{221} n_{M5}^{83} = n_{M6}^{221} n_{M11}^{83} = n_{M8}^{221} n_{M7}^{83} = n_{M6}^{221} n_{M12}^{83} = n_{M9}^{221} \\
 n_{M8}^{83} &= n_{M7}^{221} n_{M10}^{83} = n_{M9}^{221} n_{M6}^{83} = n_{M7}^{221} n_{A9}^{83} = n_{R10}^{221} + n_{R7}^{221} n_{A5}^{83} = n_{R11}^{221} + n_{R9}^{221} n_{A11}^{83} = n_{R10}^{221} + n_{R7}^{221} n_{A7}^{83} = n_{R11}^{221} + n_{R9}^{221} \\
 n_{A12}^{83} &= n_{R10}^{221} + n_{R6}^{221} n_{A8}^{83} = n_{R11}^{221} + n_{R8}^{221} n_{A10}^{83} = n_{R10}^{221} + n_{R6}^{221} n_{A6}^{83} = n_{R11}^{221} + n_{R8}^{221} n_{R6}^{83} = n_{M6}^{221} + n_{M7}^{221} n_{R4}^{83} = n_{M8}^{221} + n_{M9}^{221} \\
 n_{R5}^{83} &= n_{M6}^{221} + n_{M7}^{221} n_{R3}^{83} = n_{M8}^{221} + n_{M9}^{221} n_{Z9}^{83} = n_{X7}^{221} n_{Z5}^{83} = n_{X9}^{221} n_{Z11}^{83} = n_{X7}^{221} n_{Z7}^{83} = n_{X9}^{221} n_{Z12}^{83} = n_{X6}^{221} n_{Z8}^{83} = n_{X8}^{221} n_{Z10}^{83} = \\
 n_{X6}^{221} n_{Z6}^{83} &= n_{X8}^{221}
 \end{aligned}$$

The lower SG is SG 83 when the preserved operations are: **(sub-SG label is 7)** 1, 4, 5, 9, 25, 28, 29, 33.

The transformation is:  $(\mathbf{a}_{83}, \mathbf{b}_{83}, \mathbf{c}_{83}) = (\mathbf{a}_{221}, \mathbf{b}_{221}, \mathbf{c}_{221}) \begin{pmatrix} -1 & 0 & 0 \\ 0 & 0 & 1 \\ 0 & 1 & 0 \end{pmatrix}, \overrightarrow{O_{221}O_{83}} = \frac{1}{2}\mathbf{c}_{83}$

The reduction of higher dimensional irrep:

$$\begin{aligned}
 O_h : T_{1g} &\rightarrow A_g + {}^2E_g + {}^1E_g \text{ of } C_{4h}. \\
 O_h : T_{2g} &\rightarrow {}^2E_g + B_g + {}^1E_g \text{ of } C_{4h}. \\
 O_h : T_{1u} &\rightarrow A_u + {}^2E_u + {}^1E_u \text{ of } C_{4h}. \\
 O_h : T_{2u} &\rightarrow {}^2E_u + B_u + {}^1E_u \text{ of } C_{4h}.
 \end{aligned}$$

The correspondences of irreps at HSPs from original SG to lowered SG:

$$\begin{aligned}
 n_{GM9}^{83} &= n_{GM11}^{221} + n_{GM9}^{221} n_{GM5}^{83} = n_{GM10}^{221} + n_{GM7}^{221} n_{GM11}^{83} = n_{GM11}^{221} + n_{GM9}^{221} n_{GM7}^{83} = n_{GM10}^{221} + n_{GM7}^{221} n_{GM12}^{83} = \\
 n_{GM11}^{221} + n_{GM8}^{221} n_{GM8}^{83} &= n_{GM10}^{221} + n_{GM6}^{221} n_{GM10}^{83} = n_{GM11}^{221} + n_{GM8}^{221} n_{GM6}^{83} = n_{GM10}^{221} + n_{GM6}^{221} n_{X6}^{83} = n_{X8}^{221} + n_{X9}^{221} n_{X4}^{83} = \\
 n_{X6}^{221} + n_{X7}^{221} n_{X5}^{83} &= n_{X8}^{221} + n_{X9}^{221} n_{X3}^{83} = n_{X6}^{221} + n_{X7}^{221} n_{M9}^{83} = n_{M8}^{221} n_{M5}^{83} = n_{M6}^{221} n_{M11}^{83} = n_{M8}^{221} n_{M7}^{83} = n_{M6}^{221} n_{M12}^{83} = n_{M9}^{221} \\
 n_{M8}^{83} &= n_{M7}^{221} n_{M10}^{83} = n_{M9}^{221} n_{M6}^{83} = n_{M7}^{221} n_{A9}^{83} = n_{R10}^{221} + n_{R7}^{221} n_{A5}^{83} = n_{R11}^{221} + n_{R9}^{221} n_{A11}^{83} = n_{R10}^{221} + n_{R7}^{221} n_{A7}^{83} = n_{R11}^{221} + n_{R9}^{221} \\
 n_{A12}^{83} &= n_{R10}^{221} + n_{R6}^{221} n_{A8}^{83} = n_{R11}^{221} + n_{R8}^{221} n_{A10}^{83} = n_{R10}^{221} + n_{R6}^{221} n_{A6}^{83} = n_{R11}^{221} + n_{R8}^{221} n_{R6}^{83} = n_{M6}^{221} + n_{M7}^{221} n_{R4}^{83} = n_{M8}^{221} + n_{M9}^{221} \\
 n_{R5}^{83} &= n_{M6}^{221} + n_{M7}^{221} n_{R3}^{83} = n_{M8}^{221} + n_{M9}^{221} n_{Z9}^{83} = n_{X7}^{221} n_{Z5}^{83} = n_{X9}^{221} n_{Z11}^{83} = n_{X7}^{221} n_{Z7}^{83} = n_{X9}^{221} n_{Z12}^{83} = n_{X6}^{221} n_{Z8}^{83} = n_{X8}^{221} n_{Z10}^{83} = \\
 n_{X6}^{221} n_{Z6}^{83} &= n_{X8}^{221}
 \end{aligned}$$

The lower SG is SG 123 when the preserved operations are: **(sub-SG label is 8)** 1, 6, 7, 10, 8, 9, 11, 12, 25, 30, 31, 34, 32, 33, 35, 36.

The transformation is:  $(\mathbf{a}_{123}, \mathbf{b}_{123}, \mathbf{c}_{123}) = (\mathbf{a}_{221}, \mathbf{b}_{221}, \mathbf{c}_{221}) \begin{pmatrix} -1 & 0 & 0 \\ 0 & -1 & 0 \\ 0 & 0 & 1 \end{pmatrix}, \overrightarrow{O_{221}O_{123}} = \frac{1}{2}\mathbf{c}_{123}$

The reduction of higher dimensional irrep:

$$\begin{aligned}
 O_h : E_g &\rightarrow A_{1g} + B_{1g} \text{ of } D_{4h}. \\
 O_h : E_u &\rightarrow A_{1u} + B_{1u} \text{ of } D_{4h}.
 \end{aligned}$$

The correspondences of irreps at HSPs from original SG to lowered SG:

$$\begin{aligned}
 n_{GM8}^{123} &= n_{GM11}^{221} + n_{GM9}^{221} n_{GM6}^{123} = n_{GM10}^{221} + n_{GM7}^{221} n_{GM9}^{123} = n_{GM11}^{221} + n_{GM8}^{221} n_{GM7}^{123} = n_{GM10}^{221} + n_{GM6}^{221} n_{X6}^{123} = n_{X8}^{221} + n_{X9}^{221} \\
 n_{X5}^{123} &= n_{X6}^{221} + n_{X7}^{221} n_{M8}^{123} = n_{M8}^{221} n_{M6}^{123} = n_{M6}^{221} n_{M9}^{123} = n_{M7}^{221} n_{A8}^{123} = n_{R10}^{221} + n_{R7}^{221} n_{A6}^{123} = n_{R11}^{221} + n_{R9}^{221} n_{A9}^{123} = \\
 n_{R10}^{221} + n_{R6}^{221} n_{A7}^{123} &= n_{R11}^{221} + n_{R8}^{221} n_{R6}^{123} = n_{M6}^{221} + n_{M7}^{221} n_{R5}^{123} = n_{M8}^{221} + n_{M9}^{221} n_{Z8}^{123} = n_{X7}^{221} n_{Z6}^{123} = n_{X9}^{221} n_{Z9}^{123} = n_{X6}^{221} n_{Z7}^{123} = n_{X8}^{221}
 \end{aligned}$$

The lower SG is SG 123 when the preserved operations are: **(sub-SG label is 9)** 1, 2, 3, 8, 9, 10, 13, 14, 25, 26, 27, 32, 33, 34, 37, 38.

The transformation is:  $(\mathbf{a}_{123}, \mathbf{b}_{123}, \mathbf{c}_{123}) = (\mathbf{a}_{221}, \mathbf{b}_{221}, \mathbf{c}_{221}) \begin{pmatrix} 0 & 0 & 1 \\ -1 & 0 & 0 \\ 0 & -1 & 0 \end{pmatrix}, \overrightarrow{O_{221}O_{123}} = \frac{1}{2}\mathbf{c}_{123}$

The reduction of higher dimensional irrep:

$$O_h : E_g \rightarrow A_{1g} + B_{1g} \text{ of } D_{4h}.$$

$$O_h : E_u \rightarrow A_{1u} + B_{1u} \text{ of } D_{4h}.$$

The correspondences of irreps at HSPs from original SG to lowered SG:

$$\begin{aligned} n_{GM8}^{123} &= n_{GM11}^{221} + n_{GM9}^{221} & n_{GM6}^{123} &= n_{GM10}^{221} + n_{GM7}^{221} & n_{GM9}^{123} &= n_{GM11}^{221} + n_{GM8}^{221} & n_{GM7}^{123} &= n_{GM10}^{221} + n_{GM6}^{221} & n_{X6}^{123} &= n_{X8}^{221} + n_{X9}^{221} \\ n_{X5}^{123} &= n_{X6}^{221} + n_{X7}^{221} & n_{M8}^{123} &= n_{M8}^{221} & n_{M6}^{123} &= n_{M6}^{221} & n_{M9}^{123} &= n_{M9}^{221} & n_{M7}^{123} &= n_{M7}^{221} & n_{A8}^{123} &= n_{R10}^{221} + n_{R7}^{221} & n_{A6}^{123} &= n_{R11}^{221} + n_{R9}^{221} & n_{A9}^{123} &= n_{R10}^{221} + n_{R6}^{221} & n_{A7}^{123} &= n_{R11}^{221} + n_{R8}^{221} & n_{R6}^{123} &= n_{M6}^{221} + n_{M7}^{221} & n_{R5}^{123} &= n_{M8}^{221} + n_{M9}^{221} & n_{Z8}^{123} &= n_{X7}^{221} & n_{Z6}^{123} &= n_{X9}^{221} & n_{Z9}^{123} &= n_{X6}^{221} & n_{Z7}^{123} &= n_{X8}^{221} \end{aligned}$$

The lower SG is SG 123 when the preserved operations are: **(sub-SG label is 10)** 1, 4, 5, 9, 10, 8, 16, 15, 25, 28, 29, 33, 34, 32, 40, 39.

The transformation is:  $(\mathbf{a}_{123}, \mathbf{b}_{123}, \mathbf{c}_{123}) = (\mathbf{a}_{221}, \mathbf{b}_{221}, \mathbf{c}_{221}) \begin{pmatrix} -1 & 0 & 0 \\ 0 & 0 & 1 \\ 0 & 1 & 0 \end{pmatrix}, \overrightarrow{O_{221}O_{123}} = \frac{1}{2}\mathbf{c}_{123}$

The reduction of higher dimensional irrep:

$$O_h : E_g \rightarrow A_{1g} + B_{1g} \text{ of } D_{4h}.$$

$$O_h : E_u \rightarrow A_{1u} + B_{1u} \text{ of } D_{4h}.$$

The correspondences of irreps at HSPs from original SG to lowered SG:

$$\begin{aligned} n_{GM8}^{123} &= n_{GM11}^{221} + n_{GM9}^{221} & n_{GM6}^{123} &= n_{GM10}^{221} + n_{GM7}^{221} & n_{GM9}^{123} &= n_{GM11}^{221} + n_{GM8}^{221} & n_{GM7}^{123} &= n_{GM10}^{221} + n_{GM6}^{221} & n_{X6}^{123} &= n_{X8}^{221} + n_{X9}^{221} \\ n_{X5}^{123} &= n_{X6}^{221} + n_{X7}^{221} & n_{M8}^{123} &= n_{M8}^{221} & n_{M6}^{123} &= n_{M6}^{221} & n_{M9}^{123} &= n_{M9}^{221} & n_{M7}^{123} &= n_{M7}^{221} & n_{A8}^{123} &= n_{R10}^{221} + n_{R7}^{221} & n_{A6}^{123} &= n_{R11}^{221} + n_{R9}^{221} & n_{A9}^{123} &= n_{R10}^{221} + n_{R6}^{221} & n_{A7}^{123} &= n_{R11}^{221} + n_{R8}^{221} & n_{R6}^{123} &= n_{M6}^{221} + n_{M7}^{221} & n_{R5}^{123} &= n_{M8}^{221} + n_{M9}^{221} & n_{Z8}^{123} &= n_{X7}^{221} & n_{Z6}^{123} &= n_{X9}^{221} & n_{Z9}^{123} &= n_{X6}^{221} & n_{Z7}^{123} &= n_{X8}^{221} \end{aligned}$$

The lower SG is SG 148 when the preserved operations are: **(sub-SG label is 11)** 1, 17, 18, 25, 41, 42.

The transformation is:  $(\mathbf{a}_{148}, \mathbf{b}_{148}, \mathbf{c}_{148}) = (\mathbf{a}_{221}, \mathbf{b}_{221}, \mathbf{c}_{221}) \begin{pmatrix} 0 & 1 & 0 \\ 0 & 0 & 1 \\ 1 & 0 & 0 \end{pmatrix}, \overrightarrow{O_{221}O_{148}} = \mathbf{0}$

The reduction of higher dimensional irrep:

$$O_h : T_{1g} \rightarrow A_g + {}^2E_g + {}^1E_g \text{ of } C_{3i}.$$

$$O_h : T_{2g} \rightarrow A_g + {}^2E_g + {}^1E_g \text{ of } C_{3i}.$$

$$O_h : T_{1u} \rightarrow {}^1E_u + A_u + {}^2E_u \text{ of } C_{3i}.$$

$$O_h : T_{2u} \rightarrow {}^1E_u + A_u + {}^2E_u \text{ of } C_{3i}.$$

The correspondences of irreps at HSPs from original SG to lowered SG:

$$\begin{aligned} n_{GM7}^{148} &= 2n_{GM11}^{221} & n_{GM4}^{148} &= 2n_{GM10}^{221} & n_{GM9}^{148} &= n_{GM11}^{221} + n_{GM8}^{221} + n_{GM9}^{221} & n_{GM6}^{148} &= n_{GM10}^{221} + n_{GM6}^{221} + n_{GM7}^{221} & n_{GM8}^{148} &= n_{GM10}^{221} + n_{GM6}^{221} + n_{GM7}^{221} & n_{GM8}^{148} &= n_{GM10}^{221} + n_{GM6}^{221} + n_{GM7}^{221} \\ n_{GM11}^{221} + n_{GM8}^{221} + n_{GM9}^{221} & & n_{GM5}^{148} &= n_{GM10}^{221} + n_{GM6}^{221} + n_{GM7}^{221} & n_{L2}^{148} &= 2n_{X8}^{221} + 2n_{X9}^{221} & n_{L3}^{148} &= 2n_{X6}^{221} + 2n_{X7}^{221} & n_{F2}^{148} &= 2n_{M8}^{221} + 2n_{M9}^{221} \\ n_{F3}^{148} &= 2n_{M6}^{221} + 2n_{M7}^{221} & n_{T7}^{148} &= 2n_{R11}^{221} & n_{T4}^{148} &= 2n_{R10}^{221} & n_{T9}^{148} &= n_{R11}^{221} + n_{R8}^{221} + n_{R9}^{221} & n_{T6}^{148} &= n_{R10}^{221} + n_{R6}^{221} + n_{R7}^{221} & n_{T8}^{148} &= n_{R10}^{221} + n_{R6}^{221} + n_{R7}^{221} \\ n_{R11}^{221} + n_{R8}^{221} + n_{R9}^{221} & & n_{T5}^{148} &= n_{R10}^{221} + n_{R6}^{221} + n_{R7}^{221} \end{aligned}$$

The lower SG is SG 148 when the preserved operations are: **(sub-SG label is 12)** 1, 24, 23, 25, 48, 47.

The transformation is:  $(\mathbf{a}_{148}, \mathbf{b}_{148}, \mathbf{c}_{148}) = (\mathbf{a}_{221}, \mathbf{b}_{221}, \mathbf{c}_{221}) \begin{pmatrix} 0 & -1 & 0 \\ 0 & 0 & -1 \\ 1 & 0 & 0 \end{pmatrix}, \overrightarrow{O_{221}O_{148}} = \mathbf{0}$

The reduction of higher dimensional irrep:

$$O_h : T_{1g} \rightarrow A_g + {}^2E_g + {}^1E_g \text{ of } C_{3i}.$$

$$O_h : T_{2g} \rightarrow A_g + {}^2E_g + {}^1E_g \text{ of } C_{3i}.$$

$$O_h : T_{1u} \rightarrow {}^1E_u + A_u + {}^2E_u \text{ of } C_{3i}.$$

$$O_h : T_{2u} \rightarrow {}^1E_u + A_u + {}^2E_u \text{ of } C_{3i}.$$

The correspondences of irreps at HSPs from original SG to lowered SG:

$$\begin{aligned} n_{GM7}^{148} &= 2n_{GM11}^{221} & n_{GM4}^{148} &= 2n_{GM10}^{221} & n_{GM9}^{148} &= n_{GM11}^{221} + n_{GM8}^{221} + n_{GM9}^{221} & n_{GM6}^{148} &= n_{GM10}^{221} + n_{GM6}^{221} + n_{GM7}^{221} & n_{GM8}^{148} &= n_{GM10}^{221} + n_{GM6}^{221} + n_{GM7}^{221} \\ n_{GM11}^{221} + n_{GM8}^{221} + n_{GM9}^{221} & & n_{GM5}^{148} &= n_{GM10}^{221} + n_{GM6}^{221} + n_{GM7}^{221} & n_{L2}^{148} &= 2n_{X8}^{221} + 2n_{X9}^{221} & n_{L3}^{148} &= 2n_{X6}^{221} + 2n_{X7}^{221} & n_{F2}^{148} &= 2n_{M8}^{221} + 2n_{M9}^{221} \\ n_{F3}^{148} &= 2n_{M6}^{221} + 2n_{M7}^{221} & n_{T7}^{148} &= 2n_{R11}^{221} & n_{T4}^{148} &= 2n_{R10}^{221} & n_{T9}^{148} &= n_{R11}^{221} + n_{R8}^{221} + n_{R9}^{221} & n_{T6}^{148} &= n_{R10}^{221} + n_{R6}^{221} + n_{R7}^{221} & n_{T8}^{148} &= n_{R10}^{221} + n_{R6}^{221} + n_{R7}^{221} \\ n_{R11}^{221} + n_{R8}^{221} + n_{R9}^{221} & & n_{T5}^{148} &= n_{R10}^{221} + n_{R6}^{221} + n_{R7}^{221} \end{aligned}$$

The lower SG is SG 148 when the preserved operations are: **(sub-SG label is 13)** 1, 20, 19, 25, 44, 43.

The transformation is:  $(\mathbf{a}_{148}, \mathbf{b}_{148}, \mathbf{c}_{148}) = (\mathbf{a}_{221}, \mathbf{b}_{221}, \mathbf{c}_{221}) \begin{pmatrix} 1 & 0 & 0 \\ 0 & -1 & 0 \\ 0 & 0 & -1 \end{pmatrix}, \overrightarrow{O_{221}O_{148}} = \mathbf{0}$

The reduction of higher dimensional irrep:

$$O_h : T_{1g} \rightarrow A_g + {}^2E_g + {}^1E_g \text{ of } C_{3i}.$$

$$O_h : T_{2g} \rightarrow A_g + {}^2E_g + {}^1E_g \text{ of } C_{3i}.$$

$$O_h : T_{1u} \rightarrow {}^1E_u + A_u + {}^2E_u \text{ of } C_{3i}.$$

$$O_h : T_{2u} \rightarrow {}^1E_u + A_u + {}^2E_u \text{ of } C_{3i}.$$

The correspondences of irreps at HSPs from original SG to lowered SG:

$$\begin{aligned} n_{GM7}^{148} &= 2n_{GM11}^{221} n_{GM4}^{148} = 2n_{GM10}^{221} n_{GM9}^{148} = n_{GM11}^{221} + n_{GM8}^{221} + n_{GM9}^{221} n_{GM6}^{148} = n_{GM10}^{221} + n_{GM6}^{221} + n_{GM7}^{221} n_{GM8}^{148} = \\ n_{GM11}^{221} + n_{GM8}^{221} + n_{GM9}^{221} n_{GM5}^{148} &= n_{GM10}^{221} + n_{GM6}^{221} + n_{GM7}^{221} n_{L2}^{148} = 2n_{X8}^{221} + 2n_{X9}^{221} n_{L3}^{148} = 2n_{X6}^{221} + 2n_{X7}^{221} n_{F2}^{148} = 2n_{M8}^{221} + 2n_{M9}^{221} \\ n_{F3}^{148} &= 2n_{M6}^{221} + 2n_{M7}^{221} n_{T7}^{148} = 2n_{R11}^{221} n_{T4}^{148} = 2n_{R10}^{221} n_{T9}^{148} = n_{R11}^{221} + n_{R8}^{221} + n_{R9}^{221} n_{T6}^{148} = n_{R10}^{221} + n_{R6}^{221} + n_{R7}^{221} n_{T8}^{148} = \\ n_{R11}^{221} + n_{R8}^{221} + n_{R9}^{221} n_{T5}^{148} &= n_{R10}^{221} + n_{R6}^{221} + n_{R7}^{221} \end{aligned}$$

The lower SG is SG 148 when the preserved operations are: (**sub-SG label is 14**) 1, 22, 21, 25, 46, 45.

$$\text{The transformation is: } (\mathbf{a}_{148}, \mathbf{b}_{148}, \mathbf{c}_{148}) = (\mathbf{a}_{221}, \mathbf{b}_{221}, \mathbf{c}_{221}) \begin{pmatrix} -1 & 0 & 0 \\ 0 & 1 & 0 \\ 0 & 0 & -1 \end{pmatrix}, \overrightarrow{O_{221}O_{148}} = \mathbf{0}$$

The reduction of higher dimensional irrep:

$$O_h : T_{1g} \rightarrow A_g + {}^2E_g + {}^1E_g \text{ of } C_{3i}.$$

$$O_h : T_{2g} \rightarrow A_g + {}^2E_g + {}^1E_g \text{ of } C_{3i}.$$

$$O_h : T_{1u} \rightarrow {}^1E_u + A_u + {}^2E_u \text{ of } C_{3i}.$$

$$O_h : T_{2u} \rightarrow {}^1E_u + A_u + {}^2E_u \text{ of } C_{3i}.$$

The correspondences of irreps at HSPs from original SG to lowered SG:

$$\begin{aligned} n_{GM7}^{148} &= 2n_{GM11}^{221} n_{GM4}^{148} = 2n_{GM10}^{221} n_{GM9}^{148} = n_{GM11}^{221} + n_{GM8}^{221} + n_{GM9}^{221} n_{GM6}^{148} = n_{GM10}^{221} + n_{GM6}^{221} + n_{GM7}^{221} n_{GM8}^{148} = \\ n_{GM11}^{221} + n_{GM8}^{221} + n_{GM9}^{221} n_{GM5}^{148} &= n_{GM10}^{221} + n_{GM6}^{221} + n_{GM7}^{221} n_{L2}^{148} = 2n_{X8}^{221} + 2n_{X9}^{221} n_{L3}^{148} = 2n_{X6}^{221} + 2n_{X7}^{221} n_{F2}^{148} = 2n_{M8}^{221} + 2n_{M9}^{221} \\ n_{F3}^{148} &= 2n_{M6}^{221} + 2n_{M7}^{221} n_{T7}^{148} = 2n_{R11}^{221} n_{T4}^{148} = 2n_{R10}^{221} n_{T9}^{148} = n_{R11}^{221} + n_{R8}^{221} + n_{R9}^{221} n_{T6}^{148} = n_{R10}^{221} + n_{R6}^{221} + n_{R7}^{221} n_{T8}^{148} = \\ n_{R11}^{221} + n_{R8}^{221} + n_{R9}^{221} n_{T5}^{148} &= n_{R10}^{221} + n_{R6}^{221} + n_{R7}^{221} \end{aligned}$$

The lower SG is SG 200 when the preserved operations are: (**sub-SG label is 15**) 1, 8, 9, 10, 17, 24, 20, 22, 18, 23, 19, 21, 25, 32, 33, 34, 41, 48, 44, 46, 42, 47, 43, 45.

$$\text{The transformation is: } (\mathbf{a}_{200}, \mathbf{b}_{200}, \mathbf{c}_{200}) = (\mathbf{a}_{221}, \mathbf{b}_{221}, \mathbf{c}_{221}) \begin{pmatrix} 0 & 0 & 1 \\ 1 & 0 & 0 \\ 0 & 1 & 0 \end{pmatrix}, \overrightarrow{O_{221}O_{200}} = \mathbf{0}$$

The reduction of higher dimensional irrep:

$$O_h : E_g \rightarrow {}^1E_g + {}^2E_g \text{ of } T_h.$$

$$O_h : E_u \rightarrow {}^1E_u + {}^2E_u \text{ of } T_h.$$

The correspondences of irreps at HSPs from original SG to lowered SG:

$$\begin{aligned} n_{GM9}^{200} &= n_{GM11}^{221} n_{GM6}^{200} = n_{GM10}^{221} n_{GM10}^{200} = n_{GM11}^{221} n_{GM7}^{200} = n_{GM10}^{221} n_{GM8}^{200} = n_{GM8}^{221} + n_{GM9}^{221} n_{GM5}^{200} = n_{GM6}^{221} + n_{GM7}^{221} n_{X6}^{200} = \\ n_{X8}^{221} + n_{X9}^{221} n_{X5}^{200} &= n_{X6}^{221} + n_{X7}^{221} n_{M6}^{200} = n_{M8}^{221} + n_{M9}^{221} n_{M5}^{200} = n_{M6}^{221} + n_{M7}^{221} n_{R9}^{200} = n_{R11}^{221} n_{R6}^{200} = n_{R10}^{221} n_{R10}^{200} = n_{R11}^{221} n_{R7}^{200} = \\ n_{R10}^{221} n_{R8}^{200} &= n_{R8}^{221} + n_{R9}^{221} n_{R5}^{200} = n_{R6}^{221} + n_{R7}^{221} \end{aligned}$$

### 119. Lowered SGs by higher-dimensional irreps of pairings in SG 222

The representative operations of SG/T for SG 222:

$$\begin{aligned} 1 : (x, y, z), 2 : (x, \frac{1}{2} - z, y), 3 : (x, z, \frac{1}{2} - y), 4 : (z, y, \frac{1}{2} - x), 5 : (\frac{1}{2} - z, y, x), 6 : (\frac{1}{2} - y, x, z), 7 : (y, \frac{1}{2} - x, z), \\ 8 : (x, \frac{1}{2} - y, \frac{1}{2} - z), 9 : (\frac{1}{2} - x, y, \frac{1}{2} - z), 10 : (\frac{1}{2} - x, \frac{1}{2} - y, z), 11 : (y, x, \frac{1}{2} - z), 12 : (\frac{1}{2} - y, \frac{1}{2} - x, \frac{1}{2} - z), \\ 13 : (\frac{1}{2} - x, z, y), 14 : (\frac{1}{2} - x, \frac{1}{2} - z, \frac{1}{2} - y), 15 : (z, \frac{1}{2} - y, x), 16 : (\frac{1}{2} - z, \frac{1}{2} - y, \frac{1}{2} - x), 17 : (z, x, y), 18 : (y, z, x), \\ 19 : (\frac{1}{2} - y, z, \frac{1}{2} - x), 20 : (\frac{1}{2} - z, \frac{1}{2} - x, y), 21 : (\frac{1}{2} - y, \frac{1}{2} - z, x), 22 : (z, \frac{1}{2} - x, \frac{1}{2} - y), 23 : (y, \frac{1}{2} - z, \frac{1}{2} - x), 24 : \\ (\frac{1}{2} - z, x, \frac{1}{2} - y), 25 : (-x, -y, -z), 26 : (-x, z + \frac{1}{2}, -y), 27 : (-x, -z, y + \frac{1}{2}), 28 : (-z, -y, x + \frac{1}{2}), 29 : (z + \frac{1}{2}, -y, -x), \\ 30 : (y + \frac{1}{2}, -x, -z), 31 : (-y, x + \frac{1}{2}, -z), 32 : (-x, y + \frac{1}{2}, z + \frac{1}{2}), 33 : (x + \frac{1}{2}, -y, z + \frac{1}{2}), 34 : (x + \frac{1}{2}, y + \frac{1}{2}, -z), \\ 35 : (-y, -x, z + \frac{1}{2}), 36 : (y + \frac{1}{2}, x + \frac{1}{2}, z + \frac{1}{2}), 37 : (x + \frac{1}{2}, -z, -y), 38 : (x + \frac{1}{2}, z + \frac{1}{2}, y + \frac{1}{2}), 39 : (-z, y + \frac{1}{2}, -x), \\ 40 : (z + \frac{1}{2}, y + \frac{1}{2}, x + \frac{1}{2}), 41 : (-z, -x, -y), 42 : (-y, -z, -x), 43 : (y + \frac{1}{2}, -z, x + \frac{1}{2}), 44 : (z + \frac{1}{2}, x + \frac{1}{2}, -y), \end{aligned}$$

$$45 : (y + \frac{1}{2}, z + \frac{1}{2}, -x), 46 : (-z, x + \frac{1}{2}, y + \frac{1}{2}), 47 : (-y, z + \frac{1}{2}, x + \frac{1}{2}), 48 : (z + \frac{1}{2}, -x, y + \frac{1}{2}).$$

The lower SG is SG 48 when the preserved operations are: **(sub-SG label is 1) 1, 8, 9, 10, 25, 32, 33, 34.**

$$\text{The transformation is: } (\mathbf{a}_{48}, \mathbf{b}_{48}, \mathbf{c}_{48}) = (\mathbf{a}_{222}, \mathbf{b}_{222}, \mathbf{c}_{222}) \begin{pmatrix} 0 & 0 & 1 \\ 1 & 0 & 0 \\ 0 & 1 & 0 \end{pmatrix}, \overrightarrow{O_{222}O_{48}} = \frac{1}{2}\mathbf{a}_{48} + (\frac{1}{2})\mathbf{c}_{48}$$

The reduction of higher dimensional irrep:

$$O_h : T_{1g} \rightarrow B_{2g} + B_{1g} + B_{3g} \text{ of } D_{2h}.$$

$$O_h : T_{2g} \rightarrow B_{2g} + B_{1g} + B_{3g} \text{ of } D_{2h}.$$

$$O_h : T_{1u} \rightarrow B_{2u} + B_{1u} + B_{3u} \text{ of } D_{2h}.$$

$$O_h : T_{2u} \rightarrow B_{2u} + B_{1u} + B_{3u} \text{ of } D_{2h}.$$

The correspondences of irreps at HSPs from original SG to lowered SG:

$$\begin{aligned} n_{GM6}^{48} &= 2n_{GM11}^{222} + n_{GM8}^{222} + n_{GM9}^{222} \quad n_{GM5}^{48} = 2n_{GM10}^{222} + n_{GM6}^{222} + n_{GM7}^{222} \quad n_{X4}^{48} = n_{X5}^{222} + n_{X6}^{222} \quad n_{X3}^{48} = n_{X7}^{222} + n_{X8}^{222} \quad n_{S3}^{48} = \\ n_{M5}^{222} n_{S4}^{48} &= n_{M5}^{222} n_{R6}^{48} = n_{R5}^{222} + n_{R6}^{222} + n_{R7}^{222} \quad n_{R5}^{48} = n_{R5}^{222} + n_{R6}^{222} + n_{R7}^{222} \quad n_{U3}^{48} = n_{M5}^{222} n_{U4}^{48} = n_{M5}^{222} n_{Z4}^{48} = n_{X5}^{222} + n_{X6}^{222} \quad n_{Z3}^{48} = \\ n_{X7}^{222} + n_{X8}^{222} \quad n_{T4}^{48} &= n_{M5}^{222} n_{T3}^{48} = n_{M5}^{222} n_{Y4}^{48} = n_{X7}^{222} + n_{X8}^{222} \quad n_{Y3}^{48} = n_{X5}^{222} + n_{X6}^{222} \end{aligned}$$

The lower SG is SG 68 when the preserved operations are: **(sub-SG label is 2) 1, 8, 13, 14, 25, 32, 37, 38.**

$$\text{The transformation is: } (\mathbf{a}_{68}, \mathbf{b}_{68}, \mathbf{c}_{68}) = (\mathbf{a}_{222}, \mathbf{b}_{222}, \mathbf{c}_{222}) \begin{pmatrix} 0 & 0 & 1 \\ -1 & -1 & 0 \\ 1 & -1 & 0 \end{pmatrix}, \overrightarrow{O_{222}O_{68}} = \frac{1}{2}\mathbf{b}_{68} + (\frac{1}{2})\mathbf{c}_{68}$$

The reduction of higher dimensional irrep:

$$O_h : T_{1g} \rightarrow B_{2g} + B_{1g} + B_{3g} \text{ of } D_{2h}.$$

$$O_h : T_{2g} \rightarrow A_g + B_{2g} + B_{3g} \text{ of } D_{2h}.$$

$$O_h : T_{1u} \rightarrow B_{2u} + B_{1u} + B_{3u} \text{ of } D_{2h}.$$

$$O_h : T_{2u} \rightarrow A_u + B_{2u} + B_{3u} \text{ of } D_{2h}.$$

The correspondences of irreps at HSPs from original SG to lowered SG:

$$\begin{aligned} n_{GM6}^{68} &= 2n_{GM11}^{222} + n_{GM8}^{222} + n_{GM9}^{222} \quad n_{GM5}^{68} = 2n_{GM10}^{222} + n_{GM6}^{222} + n_{GM7}^{222} \quad n_{Y6}^{68} = n_{M5}^{222} n_{Y5}^{68} = n_{M5}^{222} n_{S2}^{68} = n_{X5}^{222} + n_{X6}^{222} + n_{X7}^{222} + n_{X8}^{222} \\ n_{Z4}^{68} &= n_{X5}^{222} + n_{X6}^{222} \quad n_{Z3}^{68} = n_{X7}^{222} + n_{X8}^{222} \quad n_{T4}^{68} = n_{R5}^{222} + n_{R6}^{222} + n_{R7}^{222} \quad n_{T3}^{68} = n_{R5}^{222} + n_{R6}^{222} + n_{R7}^{222} \quad n_{R2}^{68} = 2n_{M5}^{222} \end{aligned}$$

The lower SG is SG 68 when the preserved operations are: **(sub-SG label is 3) 1, 9, 16, 15, 25, 33, 40, 39.**

$$\text{The transformation is: } (\mathbf{a}_{68}, \mathbf{b}_{68}, \mathbf{c}_{68}) = (\mathbf{a}_{222}, \mathbf{b}_{222}, \mathbf{c}_{222}) \begin{pmatrix} -1 & 1 & 0 \\ 0 & 0 & 1 \\ 1 & 1 & 0 \end{pmatrix}, \overrightarrow{O_{222}O_{68}} = \frac{1}{2}\mathbf{b}_{68} + (\frac{1}{2})\mathbf{c}_{68}$$

The reduction of higher dimensional irrep:

$$O_h : T_{1g} \rightarrow B_{2g} + B_{1g} + B_{3g} \text{ of } D_{2h}.$$

$$O_h : T_{2g} \rightarrow A_g + B_{2g} + B_{3g} \text{ of } D_{2h}.$$

$$O_h : T_{1u} \rightarrow B_{2u} + B_{1u} + B_{3u} \text{ of } D_{2h}.$$

$$O_h : T_{2u} \rightarrow A_u + B_{2u} + B_{3u} \text{ of } D_{2h}.$$

The correspondences of irreps at HSPs from original SG to lowered SG:

$$\begin{aligned} n_{GM6}^{68} &= 2n_{GM11}^{222} + n_{GM8}^{222} + n_{GM9}^{222} \quad n_{GM5}^{68} = 2n_{GM10}^{222} + n_{GM6}^{222} + n_{GM7}^{222} \quad n_{Y6}^{68} = n_{M5}^{222} n_{Y5}^{68} = n_{M5}^{222} n_{S2}^{68} = n_{X5}^{222} + n_{X6}^{222} + n_{X7}^{222} + n_{X8}^{222} \\ n_{Z4}^{68} &= n_{X5}^{222} + n_{X6}^{222} \quad n_{Z3}^{68} = n_{X7}^{222} + n_{X8}^{222} \quad n_{T4}^{68} = n_{R5}^{222} + n_{R6}^{222} + n_{R7}^{222} \quad n_{T3}^{68} = n_{R5}^{222} + n_{R6}^{222} + n_{R7}^{222} \quad n_{R2}^{68} = 2n_{M5}^{222} \end{aligned}$$

The lower SG is SG 68 when the preserved operations are: **(sub-SG label is 4) 1, 10, 11, 12, 25, 34, 35, 36.**

$$\text{The transformation is: } (\mathbf{a}_{68}, \mathbf{b}_{68}, \mathbf{c}_{68}) = (\mathbf{a}_{222}, \mathbf{b}_{222}, \mathbf{c}_{222}) \begin{pmatrix} -1 & -1 & 0 \\ 1 & -1 & 0 \\ 0 & 0 & 1 \end{pmatrix}, \overrightarrow{O_{222}O_{68}} = \frac{1}{2}\mathbf{b}_{68} + (\frac{1}{2})\mathbf{c}_{68}$$

The reduction of higher dimensional irrep:

$$O_h : T_{1g} \rightarrow B_{2g} + B_{1g} + B_{3g} \text{ of } D_{2h}.$$

$$O_h : T_{2g} \rightarrow A_g + B_{2g} + B_{3g} \text{ of } D_{2h}.$$

$$O_h : T_{1u} \rightarrow B_{2u} + B_{1u} + B_{3u} \text{ of } D_{2h}.$$

$$O_h : T_{2u} \rightarrow A_u + B_{2u} + B_{3u} \text{ of } D_{2h}.$$

The correspondences of irreps at HSPs from original SG to lowered SG:

$$\begin{aligned} n_{GM6}^{68} &= 2n_{GM11}^{222} + n_{GM8}^{222} + n_{GM9}^{222} \quad n_{GM5}^{68} = 2n_{GM10}^{222} + n_{GM6}^{222} + n_{GM7}^{222} \quad n_{Y6}^{68} = n_{M5}^{222} n_{Y5}^{68} = n_{M5}^{222} n_{S2}^{68} = n_{X5}^{222} + n_{X6}^{222} + n_{X7}^{222} + n_{X8}^{222} \\ n_{Z4}^{68} &= n_{X5}^{222} + n_{X6}^{222} \quad n_{Z3}^{68} = n_{X7}^{222} + n_{X8}^{222} \quad n_{T4}^{68} = n_{R5}^{222} + n_{R6}^{222} + n_{R7}^{222} \quad n_{T3}^{68} = n_{R5}^{222} + n_{R6}^{222} + n_{R7}^{222} \quad n_{R2}^{68} = 2n_{M5}^{222} \end{aligned}$$

The lower SG is SG 85 when the preserved operations are: **(sub-SG label is 5) 1, 6, 7, 10, 25, 30, 31, 34.**

The transformation is:  $(\mathbf{a}_{85}, \mathbf{b}_{85}, \mathbf{c}_{85}) = (\mathbf{a}_{222}, \mathbf{b}_{222}, \mathbf{c}_{222}) \begin{pmatrix} -1 & 0 & 0 \\ 0 & -1 & 0 \\ 0 & 0 & 1 \end{pmatrix}, \overrightarrow{O_{222}O_{85}} = \frac{1}{2}\mathbf{c}_{85}$

The reduction of higher dimensional irrep:

$$O_h : T_{1g} \rightarrow A_g + {}^2E_g + {}^1E_g \text{ of } C_{4h}.$$

$$O_h : T_{2g} \rightarrow {}^2E_g + B_g + {}^1E_g \text{ of } C_{4h}.$$

$$O_h : T_{1u} \rightarrow A_u + {}^2E_u + {}^1E_u \text{ of } C_{4h}.$$

$$O_h : T_{2u} \rightarrow {}^2E_u + B_u + {}^1E_u \text{ of } C_{4h}.$$

The correspondences of irreps at HSPs from original SG to lowered SG:

$$\begin{aligned} n_{GM9}^{85} &= n_{GM11}^{222} + n_{GM9}^{222} n_{GM5}^{85} = n_{GM10}^{222} + n_{GM7}^{222} n_{GM11}^{85} = n_{GM11}^{222} + n_{GM9}^{222} n_{GM7}^{85} = n_{GM10}^{222} + n_{GM7}^{222} n_{GM12}^{85} = \\ n_{GM11}^{222} + n_{GM8}^{222} n_{GM8}^{85} &= n_{GM10}^{222} + n_{GM6}^{222} n_{GM10}^{85} = n_{GM11}^{222} + n_{GM8}^{222} n_{GM6}^{85} = n_{GM10}^{222} + n_{GM6}^{222} n_{X2}^{85} = n_{X5}^{222} + n_{X6}^{222} + n_{X7}^{222} + n_{X8}^{222} \\ n_{M3}^{85} &= n_{M5}^{222} n_{M4}^{85} = n_{M5}^{222} n_{A3}^{85} = n_{R5}^{222} + n_{R6}^{222} + n_{R7}^{222} n_{A4}^{85} = n_{R5}^{222} + n_{R6}^{222} + n_{R7}^{222} n_{R2}^{85} = 2n_{M5}^{222} n_{Z9}^{85} = n_{X6}^{222} n_{Z5}^{85} = n_{X8}^{222} n_{Z11}^{85} = \\ n_{X8}^{222} n_{Z7}^{85} &= n_{X6}^{222} n_{Z12}^{85} = n_{X7}^{222} n_{Z8}^{85} = n_{X5}^{222} n_{Z10}^{85} = n_{X5}^{222} n_{Z6}^{85} = n_{X7}^{222} \end{aligned}$$

The lower SG is SG 85 when the preserved operations are: **(sub-SG label is 6)** 1, 2, 3, 8, 25, 26, 27, 32.

The transformation is:  $(\mathbf{a}_{85}, \mathbf{b}_{85}, \mathbf{c}_{85}) = (\mathbf{a}_{222}, \mathbf{b}_{222}, \mathbf{c}_{222}) \begin{pmatrix} 0 & 0 & 1 \\ -1 & 0 & 0 \\ 0 & -1 & 0 \end{pmatrix}, \overrightarrow{O_{222}O_{85}} = \frac{1}{2}\mathbf{c}_{85}$

The reduction of higher dimensional irrep:

$$O_h : T_{1g} \rightarrow A_g + {}^2E_g + {}^1E_g \text{ of } C_{4h}.$$

$$O_h : T_{2g} \rightarrow {}^2E_g + B_g + {}^1E_g \text{ of } C_{4h}.$$

$$O_h : T_{1u} \rightarrow A_u + {}^2E_u + {}^1E_u \text{ of } C_{4h}.$$

$$O_h : T_{2u} \rightarrow {}^2E_u + B_u + {}^1E_u \text{ of } C_{4h}.$$

The correspondences of irreps at HSPs from original SG to lowered SG:

$$\begin{aligned} n_{GM9}^{85} &= n_{GM11}^{222} + n_{GM9}^{222} n_{GM5}^{85} = n_{GM10}^{222} + n_{GM7}^{222} n_{GM11}^{85} = n_{GM11}^{222} + n_{GM9}^{222} n_{GM7}^{85} = n_{GM10}^{222} + n_{GM7}^{222} n_{GM12}^{85} = \\ n_{GM11}^{222} + n_{GM8}^{222} n_{GM8}^{85} &= n_{GM10}^{222} + n_{GM6}^{222} n_{GM10}^{85} = n_{GM11}^{222} + n_{GM8}^{222} n_{GM6}^{85} = n_{GM10}^{222} + n_{GM6}^{222} n_{X2}^{85} = n_{X5}^{222} + n_{X6}^{222} + n_{X7}^{222} + n_{X8}^{222} \\ n_{M3}^{85} &= n_{M5}^{222} n_{M4}^{85} = n_{M5}^{222} n_{A3}^{85} = n_{R5}^{222} + n_{R6}^{222} + n_{R7}^{222} n_{A4}^{85} = n_{R5}^{222} + n_{R6}^{222} + n_{R7}^{222} n_{R2}^{85} = 2n_{M5}^{222} n_{Z9}^{85} = n_{X6}^{222} n_{Z5}^{85} = n_{X8}^{222} n_{Z11}^{85} = \\ n_{X8}^{222} n_{Z7}^{85} &= n_{X6}^{222} n_{Z12}^{85} = n_{X7}^{222} n_{Z8}^{85} = n_{X5}^{222} n_{Z10}^{85} = n_{X5}^{222} n_{Z6}^{85} = n_{X7}^{222} \end{aligned}$$

The lower SG is SG 85 when the preserved operations are: **(sub-SG label is 7)** 1, 4, 5, 9, 25, 28, 29, 33.

The transformation is:  $(\mathbf{a}_{85}, \mathbf{b}_{85}, \mathbf{c}_{85}) = (\mathbf{a}_{222}, \mathbf{b}_{222}, \mathbf{c}_{222}) \begin{pmatrix} -1 & 0 & 0 \\ 0 & 0 & -1 \\ 0 & -1 & 0 \end{pmatrix}, \overrightarrow{O_{222}O_{85}} = \frac{1}{2}\mathbf{c}_{85}$

The reduction of higher dimensional irrep:

$$O_h : T_{1g} \rightarrow A_g + {}^2E_g + {}^1E_g \text{ of } C_{4h}.$$

$$O_h : T_{2g} \rightarrow {}^2E_g + B_g + {}^1E_g \text{ of } C_{4h}.$$

$$O_h : T_{1u} \rightarrow A_u + {}^2E_u + {}^1E_u \text{ of } C_{4h}.$$

$$O_h : T_{2u} \rightarrow {}^2E_u + B_u + {}^1E_u \text{ of } C_{4h}.$$

The correspondences of irreps at HSPs from original SG to lowered SG:

$$\begin{aligned} n_{GM9}^{85} &= n_{GM11}^{222} + n_{GM9}^{222} n_{GM5}^{85} = n_{GM10}^{222} + n_{GM7}^{222} n_{GM11}^{85} = n_{GM11}^{222} + n_{GM9}^{222} n_{GM7}^{85} = n_{GM10}^{222} + n_{GM7}^{222} n_{GM12}^{85} = \\ n_{GM11}^{222} + n_{GM8}^{222} n_{GM8}^{85} &= n_{GM10}^{222} + n_{GM6}^{222} n_{GM10}^{85} = n_{GM11}^{222} + n_{GM8}^{222} n_{GM6}^{85} = n_{GM10}^{222} + n_{GM6}^{222} n_{X2}^{85} = n_{X5}^{222} + n_{X6}^{222} + n_{X7}^{222} + n_{X8}^{222} \\ n_{M3}^{85} &= n_{M5}^{222} n_{M4}^{85} = n_{M5}^{222} n_{A3}^{85} = n_{R5}^{222} + n_{R6}^{222} + n_{R7}^{222} n_{A4}^{85} = n_{R5}^{222} + n_{R6}^{222} + n_{R7}^{222} n_{R2}^{85} = 2n_{M5}^{222} n_{Z9}^{85} = n_{X6}^{222} n_{Z5}^{85} = n_{X8}^{222} n_{Z11}^{85} = \\ n_{X6}^{222} n_{Z7}^{85} &= n_{X8}^{222} n_{Z12}^{85} = n_{X5}^{222} n_{Z8}^{85} = n_{X7}^{222} n_{Z10}^{85} = n_{X7}^{222} n_{Z6}^{85} = n_{X5}^{222} \end{aligned}$$

The lower SG is SG 126 when the preserved operations are: **(sub-SG label is 8)** 1, 6, 7, 10, 8, 9, 11, 12, 25, 30, 31, 34, 32, 33, 35, 36.

The transformation is:  $(\mathbf{a}_{126}, \mathbf{b}_{126}, \mathbf{c}_{126}) = (\mathbf{a}_{222}, \mathbf{b}_{222}, \mathbf{c}_{222}) \begin{pmatrix} -1 & 0 & 0 \\ 0 & -1 & 0 \\ 0 & 0 & 1 \end{pmatrix}, \overrightarrow{O_{222}O_{126}} = \frac{1}{2}\mathbf{a}_{126} + (\frac{1}{2})\mathbf{b}_{126} + (\frac{1}{2})\mathbf{c}_{126}$

The reduction of higher dimensional irrep:

$$O_h : E_g \rightarrow A_{1g} + B_{1g} \text{ of } D_{4h}.$$

$$O_h : E_u \rightarrow A_{1u} + B_{1u} \text{ of } D_{4h}.$$

The correspondences of irreps at HSPs from original SG to lowered SG:

$$\begin{aligned} n_{GM8}^{126} &= n_{GM11}^{222} + n_{GM9}^{222} n_{GM6}^{126} = n_{GM10}^{222} + n_{GM7}^{222} n_{GM9}^{126} = n_{GM11}^{222} + n_{GM8}^{222} n_{GM7}^{126} = n_{GM10}^{222} + n_{GM6}^{222} n_{X4}^{126} = n_{X7}^{222} + n_{X8}^{222} \\ n_{X3}^{126} &= n_{X5}^{222} + n_{X6}^{222} n_{M5}^{126} = n_{M5}^{222} n_{A5}^{126} = n_{R5}^{222} + n_{R6}^{222} + n_{R7}^{222} n_{R4}^{126} = n_{M5}^{222} n_{R3}^{126} = n_{M5}^{222} n_{Z5}^{126} = n_{X8}^{222} n_{Z7}^{126} = n_{X6}^{222} n_{Z8}^{126} = n_{X5}^{222} \\ n_{Z6}^{126} &= n_{X7}^{222} \end{aligned}$$

The lower SG is SG 126 when the preserved operations are: **(sub-SG label is 9)** 1, 2, 3, 8, 9, 10, 13, 14, 25, 26, 27, 32, 33, 34,

37, 38.

The transformation is:  $(\mathbf{a}_{126}, \mathbf{b}_{126}, \mathbf{c}_{126}) = (\mathbf{a}_{222}, \mathbf{b}_{222}, \mathbf{c}_{222}) \begin{pmatrix} 0 & 0 & 1 \\ -1 & 0 & 0 \\ 0 & -1 & 0 \end{pmatrix}, \overrightarrow{O_{222}O_{126}} = \frac{1}{2}\mathbf{a}_{126} + (\frac{1}{2})\mathbf{b}_{126} + (\frac{1}{2})\mathbf{c}_{126}$

The reduction of higher dimensional irrep:

$$O_h : E_g \rightarrow A_{1g} + B_{1g} \text{ of } D_{4h}.$$

$$O_h : E_u \rightarrow A_{1u} + B_{1u} \text{ of } D_{4h}.$$

The correspondences of irreps at HSPs from original SG to lowered SG:

$$\begin{aligned} n_{GM8}^{126} &= n_{GM11}^{222} + n_{GM9}^{222} & n_{GM6}^{126} &= n_{GM10}^{222} + n_{GM7}^{222} & n_{GM9}^{126} &= n_{GM11}^{222} + n_{GM8}^{222} & n_{GM7}^{126} &= n_{GM10}^{222} + n_{GM6}^{222} & n_{X4}^{126} &= n_{X7}^{222} + n_{X8}^{222} \\ n_{X3}^{126} &= n_{X5}^{222} + n_{X6}^{222} & n_{M5}^{126} &= n_{M5}^{222} & n_{A5}^{126} &= n_{R5}^{222} + n_{R6}^{222} + n_{R7}^{222} & n_{R4}^{126} &= n_{M5}^{222} n_{R3}^{126} = n_{M5}^{222} n_{Z5}^{222} = n_{X8}^{222} n_{Z7}^{222} & n_{Z6}^{126} &= n_{X6}^{222} n_{Z8}^{222} = n_{X5}^{222} \\ n_{Z6}^{126} &= n_{X7}^{222} \end{aligned}$$

The lower SG is SG 126 when the preserved operations are: **(sub-SG label is 10)** 1, 4, 5, 9, 10, 8, 16, 15, 25, 28, 29, 33, 34, 32, 40, 39.

The transformation is:  $(\mathbf{a}_{126}, \mathbf{b}_{126}, \mathbf{c}_{126}) = (\mathbf{a}_{222}, \mathbf{b}_{222}, \mathbf{c}_{222}) \begin{pmatrix} -1 & 0 & 0 \\ 0 & 0 & -1 \\ 0 & -1 & 0 \end{pmatrix}, \overrightarrow{O_{222}O_{126}} = \frac{1}{2}\mathbf{a}_{126} + (\frac{1}{2})\mathbf{b}_{126} + (\frac{1}{2})\mathbf{c}_{126}$

The reduction of higher dimensional irrep:

$$O_h : E_g \rightarrow A_{1g} + B_{1g} \text{ of } D_{4h}.$$

$$O_h : E_u \rightarrow A_{1u} + B_{1u} \text{ of } D_{4h}.$$

The correspondences of irreps at HSPs from original SG to lowered SG:

$$\begin{aligned} n_{GM8}^{126} &= n_{GM11}^{222} + n_{GM9}^{222} & n_{GM6}^{126} &= n_{GM10}^{222} + n_{GM7}^{222} & n_{GM9}^{126} &= n_{GM11}^{222} + n_{GM8}^{222} & n_{GM7}^{126} &= n_{GM10}^{222} + n_{GM6}^{222} & n_{X4}^{126} &= n_{X7}^{222} + n_{X8}^{222} \\ n_{X3}^{126} &= n_{X5}^{222} + n_{X6}^{222} & n_{M5}^{126} &= n_{M5}^{222} & n_{A5}^{126} &= n_{R5}^{222} + n_{R6}^{222} + n_{R7}^{222} & n_{R4}^{126} &= n_{M5}^{222} n_{R3}^{126} = n_{M5}^{222} n_{Z5}^{222} = n_{X6}^{222} n_{Z7}^{222} & n_{Z6}^{126} &= n_{X6}^{222} n_{Z8}^{222} = n_{X5}^{222} \\ n_{Z6}^{126} &= n_{X5}^{222} \end{aligned}$$

The lower SG is SG 148 when the preserved operations are: **(sub-SG label is 11)** 1, 17, 18, 25, 41, 42.

The transformation is:  $(\mathbf{a}_{148}, \mathbf{b}_{148}, \mathbf{c}_{148}) = (\mathbf{a}_{222}, \mathbf{b}_{222}, \mathbf{c}_{222}) \begin{pmatrix} 0 & 1 & 0 \\ 0 & 0 & 1 \\ 1 & 0 & 0 \end{pmatrix}, \overrightarrow{O_{222}O_{148}} = \mathbf{0}$

The reduction of higher dimensional irrep:

$$O_h : T_{1g} \rightarrow A_g + {}^2E_g + {}^1E_g \text{ of } C_{3i}.$$

$$O_h : T_{2g} \rightarrow A_g + {}^2E_g + {}^1E_g \text{ of } C_{3i}.$$

$$O_h : T_{1u} \rightarrow {}^1E_u + A_u + {}^2E_u \text{ of } C_{3i}.$$

$$O_h : T_{2u} \rightarrow {}^1E_u + A_u + {}^2E_u \text{ of } C_{3i}.$$

The correspondences of irreps at HSPs from original SG to lowered SG:

$$\begin{aligned} n_{GM7}^{148} &= 2n_{GM11}^{222} & n_{GM4}^{148} &= 2n_{GM10}^{222} & n_{GM9}^{148} &= n_{GM11}^{222} + n_{GM8}^{222} + n_{GM9}^{222} & n_{GM6}^{148} &= n_{GM10}^{222} + n_{GM6}^{222} + n_{GM7}^{222} & n_{GM8}^{148} &= \\ n_{GM11}^{222} + n_{GM8}^{222} + n_{GM9}^{222} & n_{GM5}^{148} &= n_{GM10}^{222} + n_{GM6}^{222} + n_{GM7}^{222} & n_{L2}^{148} &= n_{X5}^{222} + n_{X6}^{222} + n_{X7}^{222} + n_{X8}^{222} & n_{L3}^{148} &= n_{X5}^{222} + n_{X6}^{222} + n_{X7}^{222} + n_{X8}^{222} \\ n_{F2}^{148} &= 2n_{M5}^{222} & n_{F3}^{148} &= 2n_{M5}^{222} & n_{T7}^{148} &= n_{R6}^{222} + n_{R7}^{222} & n_{T4}^{148} &= n_{R6}^{222} + n_{R7}^{222} & n_{T9}^{148} &= n_{R5}^{222} + n_{R7}^{222} & n_{T6}^{148} &= n_{R5}^{222} + n_{R6}^{222} & n_{T8}^{148} &= n_{R5}^{222} + n_{R6}^{222} \\ n_{T5}^{148} &= n_{R5}^{222} + n_{R7}^{222} \end{aligned}$$

The lower SG is SG 148 when the preserved operations are: **(sub-SG label is 12)** 1, 24, 23, 25, 48, 47.

The transformation is:  $(\mathbf{a}_{148}, \mathbf{b}_{148}, \mathbf{c}_{148}) = (\mathbf{a}_{222}, \mathbf{b}_{222}, \mathbf{c}_{222}) \begin{pmatrix} 0 & -1 & 0 \\ 0 & 0 & -1 \\ 1 & 0 & 0 \end{pmatrix}, \overrightarrow{O_{222}O_{148}} = \frac{1}{2}\mathbf{b}_{148} + (\frac{1}{2})\mathbf{c}_{148}$

The reduction of higher dimensional irrep:

$$O_h : T_{1g} \rightarrow A_g + {}^2E_g + {}^1E_g \text{ of } C_{3i}.$$

$$O_h : T_{2g} \rightarrow A_g + {}^2E_g + {}^1E_g \text{ of } C_{3i}.$$

$$O_h : T_{1u} \rightarrow {}^1E_u + A_u + {}^2E_u \text{ of } C_{3i}.$$

$$O_h : T_{2u} \rightarrow {}^1E_u + A_u + {}^2E_u \text{ of } C_{3i}.$$

The correspondences of irreps at HSPs from original SG to lowered SG:

$$\begin{aligned} n_{GM7}^{148} &= 2n_{GM11}^{222} & n_{GM4}^{148} &= 2n_{GM10}^{222} & n_{GM9}^{148} &= n_{GM11}^{222} + n_{GM8}^{222} + n_{GM9}^{222} & n_{GM6}^{148} &= n_{GM10}^{222} + n_{GM6}^{222} + n_{GM7}^{222} & n_{GM8}^{148} &= \\ n_{GM11}^{222} + n_{GM8}^{222} + n_{GM9}^{222} & n_{GM5}^{148} &= n_{GM10}^{222} + n_{GM6}^{222} + n_{GM7}^{222} & n_{L2}^{148} &= n_{X5}^{222} + n_{X6}^{222} + n_{X7}^{222} + n_{X8}^{222} & n_{L3}^{148} &= n_{X5}^{222} + n_{X6}^{222} + n_{X7}^{222} + n_{X8}^{222} \\ n_{F2}^{148} &= 2n_{M5}^{222} & n_{F3}^{148} &= 2n_{M5}^{222} & n_{T7}^{148} &= n_{R6}^{222} + n_{R7}^{222} & n_{T4}^{148} &= n_{R6}^{222} + n_{R7}^{222} & n_{T9}^{148} &= n_{R5}^{222} + n_{R7}^{222} & n_{T6}^{148} &= n_{R5}^{222} + n_{R6}^{222} & n_{T8}^{148} &= n_{R5}^{222} + n_{R6}^{222} \\ n_{T5}^{148} &= n_{R5}^{222} + n_{R7}^{222} \end{aligned}$$

The lower SG is SG 148 when the preserved operations are: **(sub-SG label is 13)** 1, 20, 19, 25, 44, 43.

The transformation is:  $(\mathbf{a}_{148}, \mathbf{b}_{148}, \mathbf{c}_{148}) = (\mathbf{a}_{222}, \mathbf{b}_{222}, \mathbf{c}_{222}) \begin{pmatrix} 1 & 0 & 0 \\ 0 & -1 & 0 \\ 0 & 0 & -1 \end{pmatrix}, \overrightarrow{O_{222}O_{148}} = \frac{1}{2}\mathbf{b}_{148} + (\frac{1}{2})\mathbf{c}_{148}$

The reduction of higher dimensional irrep:

$$O_h : T_{1g} \rightarrow A_g + {}^2E_g + {}^1E_g \text{ of } C_{3i}.$$

$$O_h : T_{2g} \rightarrow A_g + {}^2E_g + {}^1E_g \text{ of } C_{3i}.$$

$$O_h : T_{1u} \rightarrow {}^1E_u + A_u + {}^2E_u \text{ of } C_{3i}.$$

$$O_h : T_{2u} \rightarrow {}^1E_u + A_u + {}^2E_u \text{ of } C_{3i}.$$

The correspondences of irreps at HSPs from original SG to lowered SG:

$$\begin{aligned} n_{GM7}^{148} &= 2n_{GM11}^{222} n_{GM4}^{148} = 2n_{GM10}^{222} n_{GM9}^{148} = n_{GM11}^{222} + n_{GM8}^{222} + n_{GM9}^{222} n_{GM6}^{148} = n_{GM10}^{222} + n_{GM6}^{222} + n_{GM7}^{222} n_{GM8}^{148} = \\ n_{GM11}^{222} + n_{GM8}^{222} + n_{GM9}^{222} n_{GM5}^{148} &= n_{GM10}^{222} + n_{GM6}^{222} + n_{GM7}^{222} n_{L2}^{148} = n_{X5}^{222} + n_{X6}^{222} + n_{X7}^{222} + n_{X8}^{222} n_{L3}^{148} = n_{X5}^{222} + n_{X6}^{222} + n_{X7}^{222} + n_{X8}^{222} \\ n_{F2}^{148} &= 2n_{M5}^{222} n_{F3}^{148} = 2n_{M5}^{222} n_{T7}^{148} = n_{R6}^{222} + n_{R7}^{222} n_{T4}^{148} = n_{R6}^{222} + n_{R7}^{222} n_{T9}^{148} = n_{R5}^{222} + n_{R7}^{222} n_{T6}^{148} = n_{R5}^{222} + n_{R6}^{222} n_{T8}^{148} = n_{R5}^{222} + n_{R6}^{222} \\ n_{T5}^{148} &= n_{R5}^{222} + n_{R7}^{222} \end{aligned}$$

The lower SG is SG 148 when the preserved operations are: **(sub-SG label is 14)** 1, 22, 21, 25, 46, 45.

The transformation is:  $(\mathbf{a}_{148}, \mathbf{b}_{148}, \mathbf{c}_{148}) = (\mathbf{a}_{222}, \mathbf{b}_{222}, \mathbf{c}_{222}) \begin{pmatrix} -1 & 0 & 0 \\ 0 & 1 & 0 \\ 0 & 0 & -1 \end{pmatrix}, \overrightarrow{O_{222}O_{148}} = \frac{1}{2}\mathbf{b}_{148}$

The reduction of higher dimensional irrep:

$$O_h : T_{1g} \rightarrow A_g + {}^2E_g + {}^1E_g \text{ of } C_{3i}.$$

$$O_h : T_{2g} \rightarrow A_g + {}^2E_g + {}^1E_g \text{ of } C_{3i}.$$

$$O_h : T_{1u} \rightarrow {}^1E_u + A_u + {}^2E_u \text{ of } C_{3i}.$$

$$O_h : T_{2u} \rightarrow {}^1E_u + A_u + {}^2E_u \text{ of } C_{3i}.$$

The correspondences of irreps at HSPs from original SG to lowered SG:

$$\begin{aligned} n_{GM7}^{148} &= 2n_{GM11}^{222} n_{GM4}^{148} = 2n_{GM10}^{222} n_{GM9}^{148} = n_{GM11}^{222} + n_{GM8}^{222} + n_{GM9}^{222} n_{GM6}^{148} = n_{GM10}^{222} + n_{GM6}^{222} + n_{GM7}^{222} n_{GM8}^{148} = \\ n_{GM11}^{222} + n_{GM8}^{222} + n_{GM9}^{222} n_{GM5}^{148} &= n_{GM10}^{222} + n_{GM6}^{222} + n_{GM7}^{222} n_{L2}^{148} = n_{X5}^{222} + n_{X6}^{222} + n_{X7}^{222} + n_{X8}^{222} n_{L3}^{148} = n_{X5}^{222} + n_{X6}^{222} + n_{X7}^{222} + n_{X8}^{222} \\ n_{F2}^{148} &= 2n_{M5}^{222} n_{F3}^{148} = 2n_{M5}^{222} n_{T7}^{148} = n_{R6}^{222} + n_{R7}^{222} n_{T4}^{148} = n_{R6}^{222} + n_{R7}^{222} n_{T9}^{148} = n_{R5}^{222} + n_{R6}^{222} n_{T6}^{148} = n_{R5}^{222} + n_{R6}^{222} n_{T8}^{148} = n_{R5}^{222} + n_{R6}^{222} \\ n_{T5}^{148} &= n_{R5}^{222} + n_{R6}^{222} \end{aligned}$$

The lower SG is SG 201 when the preserved operations are: **(sub-SG label is 15)** 1, 8, 9, 10, 17, 24, 20, 22, 18, 23, 19, 21, 25, 32, 33, 34, 41, 48, 44, 46, 42, 47, 43, 45.

The transformation is:  $(\mathbf{a}_{201}, \mathbf{b}_{201}, \mathbf{c}_{201}) = (\mathbf{a}_{222}, \mathbf{b}_{222}, \mathbf{c}_{222}) \begin{pmatrix} 0 & 0 & -1 \\ 1 & 0 & 0 \\ 0 & -1 & 0 \end{pmatrix}, \overrightarrow{O_{222}O_{201}} = \frac{1}{2}\mathbf{b}_{201} + (\frac{1}{2})\mathbf{c}_{201}$

The reduction of higher dimensional irrep:

$$O_h : E_g \rightarrow {}^1E_g + {}^2E_g \text{ of } T_h.$$

$$O_h : E_u \rightarrow {}^1E_u + {}^2E_u \text{ of } T_h.$$

The correspondences of irreps at HSPs from original SG to lowered SG:

$$\begin{aligned} n_{GM9}^{201} &= n_{GM11}^{222} n_{GM6}^{201} = n_{GM10}^{222} n_{GM10}^{201} = n_{GM11}^{222} n_{GM7}^{201} = n_{GM10}^{222} n_{GM8}^{201} = n_{GM8}^{222} + n_{GM9}^{222} n_{GM5}^{201} = n_{GM6}^{222} + n_{GM7}^{222} n_{X4}^{201} = \\ n_{X7}^{222} + n_{X8}^{222} n_{X3}^{201} &= n_{X5}^{222} + n_{X6}^{222} n_{M3}^{201} = n_{M5}^{222} n_{M4}^{201} = n_{M5}^{222} n_{R9}^{201} = n_{R7}^{222} n_{R6}^{201} = n_{R6}^{222} n_{R10}^{201} = n_{R6}^{222} n_{R7}^{201} = n_{R7}^{222} n_{R8}^{201} = n_{R5}^{222} \\ n_{R5}^{201} &= n_{R5}^{222} \end{aligned}$$

## 120. Lowered SGs by higher-dimensional irreps of pairings in SG 223

The representative operations of SG/T for SG 223:

$$\begin{aligned} 1 : (x, y, z), 2 : (x + \frac{1}{2}, \frac{1}{2} - z, y + \frac{1}{2}), 3 : (x + \frac{1}{2}, z + \frac{1}{2}, \frac{1}{2} - y), 4 : (z + \frac{1}{2}, y + \frac{1}{2}, \frac{1}{2} - x), 5 : (\frac{1}{2} - z, y + \frac{1}{2}, x + \frac{1}{2}), \\ 6 : (\frac{1}{2} - y, x + \frac{1}{2}, z + \frac{1}{2}), 7 : (y + \frac{1}{2}, \frac{1}{2} - x, z + \frac{1}{2}), 8 : (x, -y, -z), 9 : (-x, y, -z), 10 : (-x, -y, z), 11 : (y + \frac{1}{2}, x + \frac{1}{2}, \frac{1}{2} - z), \\ 12 : (\frac{1}{2} - y, \frac{1}{2} - x, \frac{1}{2} - z), 13 : (\frac{1}{2} - x, z + \frac{1}{2}, y + \frac{1}{2}), 14 : (\frac{1}{2} - x, \frac{1}{2} - z, \frac{1}{2} - y), 15 : (z + \frac{1}{2}, \frac{1}{2} - y, x + \frac{1}{2}), 16 : (\frac{1}{2} - z, \frac{1}{2} - y, \frac{1}{2} - x), \\ 17 : (z, x, y), 18 : (y, z, x), 19 : (-y, z, -x), 20 : (-z, -x, y), 21 : (-y, -z, x), 22 : (z, -x, -y), 23 : (y, -z, -x), \\ 24 : (-z, x, -y), 25 : (-x, -y, -z), 26 : (\frac{1}{2} - x, z + \frac{1}{2}, \frac{1}{2} - y), 27 : (\frac{1}{2} - x, \frac{1}{2} - z, y + \frac{1}{2}), 28 : (\frac{1}{2} - z, \frac{1}{2} - y, x + \frac{1}{2}), \\ 29 : (z + \frac{1}{2}, \frac{1}{2} - y, \frac{1}{2} - x), 30 : (y + \frac{1}{2}, \frac{1}{2} - x, \frac{1}{2} - z), 31 : (\frac{1}{2} - y, x + \frac{1}{2}, \frac{1}{2} - z), 32 : (-x, y, z), 33 : (x, -y, z), \end{aligned}$$

$$\begin{aligned}
34 : (x, y, -z), 35 : (\frac{1}{2} - y, \frac{1}{2} - x, z + \frac{1}{2}), 36 : (y + \frac{1}{2}, x + \frac{1}{2}, z + \frac{1}{2}), 37 : (x + \frac{1}{2}, \frac{1}{2} - z, \frac{1}{2} - y), 38 : (x + \frac{1}{2}, z + \frac{1}{2}, y + \frac{1}{2}), \\
39 : (\frac{1}{2} - z, y + \frac{1}{2}, \frac{1}{2} - x), 40 : (z + \frac{1}{2}, y + \frac{1}{2}, x + \frac{1}{2}), 41 : (-z, -x, -y), 42 : (-y, -z, -x), 43 : (y, -z, x), 44 : (z, x, -y), \\
45 : (y, z, -x), 46 : (-z, x, y), 47 : (-y, z, x), 48 : (z, -x, y).
\end{aligned}$$

The lower SG is SG 47 when the preserved operations are: **(sub-SG label is 1) 1, 8, 9, 10, 25, 32, 33, 34.**

The transformation is:  $(\mathbf{a}_{47}, \mathbf{b}_{47}, \mathbf{c}_{47}) = (\mathbf{a}_{223}, \mathbf{b}_{223}, \mathbf{c}_{223}) \begin{pmatrix} 0 & 0 & 1 \\ 1 & 0 & 0 \\ 0 & 1 & 0 \end{pmatrix}, \overrightarrow{O_{223}O_{47}} = \frac{1}{2}\mathbf{a}_{47} + (\frac{1}{2})\mathbf{c}_{47}$

The reduction of higher dimensional irrep:

$$O_h : T_{1g} \rightarrow B_{2g} + B_{1g} + B_{3g} \text{ of } D_{2h}.$$

$$O_h : T_{2g} \rightarrow B_{2g} + B_{1g} + B_{3g} \text{ of } D_{2h}.$$

$$O_h : T_{1u} \rightarrow B_{2u} + B_{1u} + B_{3u} \text{ of } D_{2h}.$$

$$O_h : T_{2u} \rightarrow B_{2u} + B_{1u} + B_{3u} \text{ of } D_{2h}.$$

The correspondences of irreps at HSPs from original SG to lowered SG:

$$\begin{aligned}
n_{GM6}^{47} &= 2n_{GM11}^{223} + n_{GM8}^{223} + n_{GM9}^{223} n_{GM5}^{47} = 2n_{GM10}^{223} + n_{GM6}^{223} + n_{GM7}^{223} n_{X6}^{47} = n_{X5}^{223} n_{X5}^{47} = n_{X5}^{223} n_{S6}^{47} = n_{M6}^{223} + n_{M7}^{223} n_{S5}^{47} = \\
n_{M8}^{223} + n_{M9}^{223} n_{R6}^{47} &= n_{R5}^{223} + n_{R6}^{223} + n_{R7}^{223} n_{R5}^{47} = n_{R5}^{223} + n_{R6}^{223} + n_{R7}^{223} n_{U6}^{47} = n_{M8}^{223} + n_{M9}^{223} n_{U5}^{47} = n_{M6}^{223} + n_{M7}^{223} n_{Z6}^{47} = n_{X5}^{223} n_{Z5}^{47} = \\
n_{X5}^{223} n_{T6}^{47} &= n_{M6}^{223} + n_{M7}^{223} n_{T5}^{47} = n_{M8}^{223} + n_{M9}^{223} n_{Y6}^{47} = n_{X5}^{223} n_{Y5}^{47} = n_{X5}^{223}
\end{aligned}$$

The lower SG is SG 66 when the preserved operations are: **(sub-SG label is 2) 1, 8, 13, 14, 25, 32, 37, 38.**

The transformation is:  $(\mathbf{a}_{66}, \mathbf{b}_{66}, \mathbf{c}_{66}) = (\mathbf{a}_{223}, \mathbf{b}_{223}, \mathbf{c}_{223}) \begin{pmatrix} 0 & 0 & 1 \\ 1 & -1 & 0 \\ 1 & 1 & 0 \end{pmatrix}, \overrightarrow{O_{223}O_{66}} = \frac{1}{4}\mathbf{a}_{66} + (\frac{1}{4})\mathbf{b}_{66} + (\frac{1}{2})\mathbf{c}_{66}$

The reduction of higher dimensional irrep:

$$O_h : T_{1g} \rightarrow B_{2g} + B_{1g} + B_{3g} \text{ of } D_{2h}.$$

$$O_h : T_{2g} \rightarrow A_g + B_{2g} + B_{3g} \text{ of } D_{2h}.$$

$$O_h : T_{1u} \rightarrow B_{2u} + B_{1u} + B_{3u} \text{ of } D_{2h}.$$

$$O_h : T_{2u} \rightarrow A_u + B_{2u} + B_{3u} \text{ of } D_{2h}.$$

The correspondences of irreps at HSPs from original SG to lowered SG:

$$\begin{aligned}
n_{GM6}^{66} &= 2n_{GM11}^{223} + n_{GM8}^{223} + n_{GM9}^{223} n_{GM5}^{66} = 2n_{GM10}^{223} + n_{GM6}^{223} + n_{GM7}^{223} n_{Y6}^{66} = n_{M6}^{223} + n_{M7}^{223} n_{Y5}^{66} = n_{M8}^{223} + n_{M9}^{223} n_{S6}^{66} = n_{X5}^{223} \\
n_{S4}^{66} &= n_{X5}^{223} n_{S5}^{66} = n_{X5}^{223} n_{S3}^{66} = n_{X5}^{223} n_{Z4}^{66} = n_{X5}^{223} n_{Z3}^{66} = n_{X5}^{223} n_{T4}^{66} = n_{R5}^{223} + n_{R6}^{223} + n_{R7}^{223} n_{T3}^{66} = n_{R5}^{223} + n_{R6}^{223} + n_{R7}^{223} n_{R6}^{66} = \\
n_{M8}^{223} + n_{M9}^{223} n_{R4}^{66} &= n_{M6}^{223} + n_{M7}^{223} n_{R5}^{66} = n_{M8}^{223} + n_{M9}^{223} n_{R3}^{66} = n_{M6}^{223} + n_{M7}^{223}
\end{aligned}$$

The lower SG is SG 66 when the preserved operations are: **(sub-SG label is 3) 1, 9, 16, 15, 25, 33, 40, 39.**

The transformation is:  $(\mathbf{a}_{66}, \mathbf{b}_{66}, \mathbf{c}_{66}) = (\mathbf{a}_{223}, \mathbf{b}_{223}, \mathbf{c}_{223}) \begin{pmatrix} -1 & 1 & 0 \\ 0 & 0 & 1 \\ 1 & 1 & 0 \end{pmatrix}, \overrightarrow{O_{223}O_{66}} = \frac{1}{4}\mathbf{a}_{66} + (\frac{1}{4})\mathbf{b}_{66} + (\frac{1}{2})\mathbf{c}_{66}$

The reduction of higher dimensional irrep:

$$O_h : T_{1g} \rightarrow B_{2g} + B_{1g} + B_{3g} \text{ of } D_{2h}.$$

$$O_h : T_{2g} \rightarrow A_g + B_{2g} + B_{3g} \text{ of } D_{2h}.$$

$$O_h : T_{1u} \rightarrow B_{2u} + B_{1u} + B_{3u} \text{ of } D_{2h}.$$

$$O_h : T_{2u} \rightarrow A_u + B_{2u} + B_{3u} \text{ of } D_{2h}.$$

The correspondences of irreps at HSPs from original SG to lowered SG:

$$\begin{aligned}
n_{GM6}^{66} &= 2n_{GM11}^{223} + n_{GM8}^{223} + n_{GM9}^{223} n_{GM5}^{66} = 2n_{GM10}^{223} + n_{GM6}^{223} + n_{GM7}^{223} n_{Y6}^{66} = n_{M6}^{223} + n_{M7}^{223} n_{Y5}^{66} = n_{M8}^{223} + n_{M9}^{223} n_{S6}^{66} = n_{X5}^{223} \\
n_{S4}^{66} &= n_{X5}^{223} n_{S5}^{66} = n_{X5}^{223} n_{S3}^{66} = n_{X5}^{223} n_{Z4}^{66} = n_{X5}^{223} n_{Z3}^{66} = n_{X5}^{223} n_{T4}^{66} = n_{R5}^{223} + n_{R6}^{223} + n_{R7}^{223} n_{T3}^{66} = n_{R5}^{223} + n_{R6}^{223} + n_{R7}^{223} n_{R6}^{66} = \\
n_{M8}^{223} + n_{M9}^{223} n_{R4}^{66} &= n_{M6}^{223} + n_{M7}^{223} n_{R5}^{66} = n_{M8}^{223} + n_{M9}^{223} n_{R3}^{66} = n_{M6}^{223} + n_{M7}^{223}
\end{aligned}$$

The lower SG is SG 66 when the preserved operations are: **(sub-SG label is 4) 1, 10, 11, 12, 25, 34, 35, 36.**

The transformation is:  $(\mathbf{a}_{66}, \mathbf{b}_{66}, \mathbf{c}_{66}) = (\mathbf{a}_{223}, \mathbf{b}_{223}, \mathbf{c}_{223}) \begin{pmatrix} 1 & -1 & 0 \\ 1 & 1 & 0 \\ 0 & 0 & 1 \end{pmatrix}, \overrightarrow{O_{223}O_{66}} = \frac{1}{4}\mathbf{a}_{66} + (\frac{1}{4})\mathbf{b}_{66} + (\frac{1}{2})\mathbf{c}_{66}$

The reduction of higher dimensional irrep:

$$O_h : T_{1g} \rightarrow B_{2g} + B_{1g} + B_{3g} \text{ of } D_{2h}.$$

$$O_h : T_{2g} \rightarrow A_g + B_{2g} + B_{3g} \text{ of } D_{2h}.$$

$$O_h : T_{1u} \rightarrow B_{2u} + B_{1u} + B_{3u} \text{ of } D_{2h}.$$

$$O_h : T_{2u} \rightarrow A_u + B_{2u} + B_{3u} \text{ of } D_{2h}.$$

The correspondences of irreps at HSPs from original SG to lowered SG:

$$\begin{aligned}
n_{GM6}^{66} &= 2n_{GM11}^{223} + n_{GM8}^{223} + n_{GM9}^{223} n_{GM5}^{66} = 2n_{GM10}^{223} + n_{GM6}^{223} + n_{GM7}^{223} n_{Y6}^{66} = n_{M6}^{223} + n_{M7}^{223} n_{Y5}^{66} = n_{M8}^{223} + n_{M9}^{223} n_{S6}^{66} = n_{X5}^{223} \\
n_{S4}^{66} &= n_{X5}^{223} n_{S5}^{66} = n_{X5}^{223} n_{S3}^{66} = n_{X5}^{223} n_{Z4}^{66} = n_{X5}^{223} n_{Z3}^{66} = n_{X5}^{223} n_{T4}^{66} = n_{R5}^{223} + n_{R6}^{223} + n_{R7}^{223} n_{T3}^{66} = n_{R5}^{223} + n_{R6}^{223} + n_{R7}^{223} n_{R6}^{66} = \\
n_{M8}^{223} + n_{M9}^{223} n_{R4}^{66} &= n_{M6}^{223} + n_{M7}^{223} n_{R5}^{66} = n_{M8}^{223} + n_{M9}^{223} n_{R3}^{66} = n_{M6}^{223} + n_{M7}^{223}
\end{aligned}$$

The lower SG is SG 84 when the preserved operations are: **(sub-SG label is 5)** 1, 6, 7, 10, 25, 30, 31, 34.

The transformation is:  $(\mathbf{a}_{84}, \mathbf{b}_{84}, \mathbf{c}_{84}) = (\mathbf{a}_{223}, \mathbf{b}_{223}, \mathbf{c}_{223}) \begin{pmatrix} -1 & 0 & 0 \\ 0 & -1 & 0 \\ 0 & 0 & 1 \end{pmatrix}, \overrightarrow{O_{223}O_{84}} = \frac{1}{2}\mathbf{b}_{84} + (\frac{1}{2})\mathbf{c}_{84}$

The reduction of higher dimensional irrep:

$$O_h : T_{1g} \rightarrow A_g + {}^2E_g + {}^1E_g \text{ of } C_{4h}.$$

$$O_h : T_{2g} \rightarrow {}^2E_g + B_g + {}^1E_g \text{ of } C_{4h}.$$

$$O_h : T_{1u} \rightarrow A_u + {}^2E_u + {}^1E_u \text{ of } C_{4h}.$$

$$O_h : T_{2u} \rightarrow {}^2E_u + B_u + {}^1E_u \text{ of } C_{4h}.$$

The correspondences of irreps at HSPs from original SG to lowered SG:

$$\begin{aligned}
n_{GM9}^{84} &= n_{GM11}^{223} + n_{GM9}^{223} n_{GM5}^{84} = n_{GM10}^{223} + n_{GM7}^{223} n_{GM11}^{84} = n_{GM11}^{223} + n_{GM9}^{223} n_{GM7}^{84} = n_{GM10}^{223} + n_{GM7}^{223} n_{GM12}^{84} = \\
n_{GM11}^{223} + n_{GM8}^{223} n_{GM8}^{84} &= n_{GM10}^{223} + n_{GM6}^{223} n_{GM10}^{84} = n_{GM11}^{223} + n_{GM8}^{223} n_{GM6}^{84} = n_{GM10}^{223} + n_{GM6}^{223} n_{X6}^{84} = n_{X5}^{223} n_{X4}^{84} = n_{X5}^{223} \\
n_{X5}^{84} &= n_{X5}^{223} n_{X3}^{84} = n_{X5}^{223} n_{M9}^{84} = n_{M7}^{223} n_{M5}^{84} = n_{M9}^{223} n_{M11}^{84} = n_{M7}^{223} n_{M7}^{84} = n_{M9}^{223} n_{M12}^{84} = n_{M6}^{223} n_{M8}^{84} = n_{M8}^{223} n_{M10}^{84} = n_{M6}^{223} \\
n_{M6}^{84} &= n_{M8}^{223} n_{A4}^{84} = n_{R5}^{223} + n_{R6}^{223} + n_{R7}^{223} n_{A3}^{84} = n_{R5}^{223} + n_{R6}^{223} + n_{R7}^{223} n_{R4}^{84} = n_{M6}^{223} + n_{M7}^{223} n_{R6}^{84} = n_{M8}^{223} + n_{M9}^{223} n_{R3}^{84} = n_{M6}^{223} + n_{M7}^{223} \\
n_{R5}^{84} &= n_{M8}^{223} + n_{M9}^{223} n_{Z4}^{84} = n_{X5}^{223} n_{Z3}^{84} = n_{X5}^{223}
\end{aligned}$$

The lower SG is SG 84 when the preserved operations are: **(sub-SG label is 6)** 1, 2, 3, 8, 25, 26, 27, 32.

The transformation is:  $(\mathbf{a}_{84}, \mathbf{b}_{84}, \mathbf{c}_{84}) = (\mathbf{a}_{223}, \mathbf{b}_{223}, \mathbf{c}_{223}) \begin{pmatrix} 0 & 0 & 1 \\ -1 & 0 & 0 \\ 0 & -1 & 0 \end{pmatrix}, \overrightarrow{O_{223}O_{84}} = \frac{1}{2}\mathbf{b}_{84} + (\frac{1}{2})\mathbf{c}_{84}$

The reduction of higher dimensional irrep:

$$O_h : T_{1g} \rightarrow A_g + {}^2E_g + {}^1E_g \text{ of } C_{4h}.$$

$$O_h : T_{2g} \rightarrow {}^2E_g + B_g + {}^1E_g \text{ of } C_{4h}.$$

$$O_h : T_{1u} \rightarrow A_u + {}^2E_u + {}^1E_u \text{ of } C_{4h}.$$

$$O_h : T_{2u} \rightarrow {}^2E_u + B_u + {}^1E_u \text{ of } C_{4h}.$$

The correspondences of irreps at HSPs from original SG to lowered SG:

$$\begin{aligned}
n_{GM9}^{84} &= n_{GM11}^{223} + n_{GM9}^{223} n_{GM5}^{84} = n_{GM10}^{223} + n_{GM7}^{223} n_{GM11}^{84} = n_{GM11}^{223} + n_{GM9}^{223} n_{GM7}^{84} = n_{GM10}^{223} + n_{GM7}^{223} n_{GM12}^{84} = \\
n_{GM11}^{223} + n_{GM8}^{223} n_{GM8}^{84} &= n_{GM10}^{223} + n_{GM6}^{223} n_{GM10}^{84} = n_{GM11}^{223} + n_{GM8}^{223} n_{GM6}^{84} = n_{GM10}^{223} + n_{GM6}^{223} n_{X6}^{84} = n_{X5}^{223} n_{X4}^{84} = n_{X5}^{223} \\
n_{X5}^{84} &= n_{X5}^{223} n_{X3}^{84} = n_{X5}^{223} n_{M9}^{84} = n_{M7}^{223} n_{M5}^{84} = n_{M9}^{223} n_{M11}^{84} = n_{M7}^{223} n_{M7}^{84} = n_{M9}^{223} n_{M12}^{84} = n_{M6}^{223} n_{M8}^{84} = n_{M8}^{223} n_{M10}^{84} = n_{M6}^{223} \\
n_{M6}^{84} &= n_{M8}^{223} n_{A4}^{84} = n_{R5}^{223} + n_{R6}^{223} + n_{R7}^{223} n_{A3}^{84} = n_{R5}^{223} + n_{R6}^{223} + n_{R7}^{223} n_{R4}^{84} = n_{M6}^{223} + n_{M7}^{223} n_{R6}^{84} = n_{M8}^{223} + n_{M9}^{223} n_{R3}^{84} = n_{M6}^{223} + n_{M7}^{223} \\
n_{R5}^{84} &= n_{M8}^{223} + n_{M9}^{223} n_{Z4}^{84} = n_{X5}^{223} n_{Z3}^{84} = n_{X5}^{223}
\end{aligned}$$

The lower SG is SG 84 when the preserved operations are: **(sub-SG label is 7)** 1, 4, 5, 9, 25, 28, 29, 33.

The transformation is:  $(\mathbf{a}_{84}, \mathbf{b}_{84}, \mathbf{c}_{84}) = (\mathbf{a}_{223}, \mathbf{b}_{223}, \mathbf{c}_{223}) \begin{pmatrix} -1 & 0 & 0 \\ 0 & 0 & 1 \\ 0 & 1 & 0 \end{pmatrix}, \overrightarrow{O_{223}O_{84}} = \frac{1}{2}\mathbf{b}_{84} + (\frac{1}{2})\mathbf{c}_{84}$

The reduction of higher dimensional irrep:

$$O_h : T_{1g} \rightarrow A_g + {}^2E_g + {}^1E_g \text{ of } C_{4h}.$$

$$O_h : T_{2g} \rightarrow {}^2E_g + B_g + {}^1E_g \text{ of } C_{4h}.$$

$$O_h : T_{1u} \rightarrow A_u + {}^2E_u + {}^1E_u \text{ of } C_{4h}.$$

$$O_h : T_{2u} \rightarrow {}^2E_u + B_u + {}^1E_u \text{ of } C_{4h}.$$

The correspondences of irreps at HSPs from original SG to lowered SG:

$$\begin{aligned}
n_{GM9}^{84} &= n_{GM11}^{223} + n_{GM9}^{223} n_{GM5}^{84} = n_{GM10}^{223} + n_{GM7}^{223} n_{GM11}^{84} = n_{GM11}^{223} + n_{GM9}^{223} n_{GM7}^{84} = n_{GM10}^{223} + n_{GM7}^{223} n_{GM12}^{84} = \\
n_{GM11}^{223} + n_{GM8}^{223} n_{GM8}^{84} &= n_{GM10}^{223} + n_{GM6}^{223} n_{GM10}^{84} = n_{GM11}^{223} + n_{GM8}^{223} n_{GM6}^{84} = n_{GM10}^{223} + n_{GM6}^{223} n_{X6}^{84} = n_{X5}^{223} n_{X4}^{84} = n_{X5}^{223} \\
n_{X5}^{84} &= n_{X5}^{223} n_{X3}^{84} = n_{X5}^{223} n_{M9}^{84} = n_{M7}^{223} n_{M5}^{84} = n_{M9}^{223} n_{M11}^{84} = n_{M7}^{223} n_{M7}^{84} = n_{M9}^{223} n_{M12}^{84} = n_{M6}^{223} n_{M8}^{84} = n_{M8}^{223} n_{M10}^{84} = n_{M6}^{223} \\
n_{M6}^{84} &= n_{M8}^{223} n_{A4}^{84} = n_{R5}^{223} + n_{R6}^{223} + n_{R7}^{223} n_{A3}^{84} = n_{R5}^{223} + n_{R6}^{223} + n_{R7}^{223} n_{R4}^{84} = n_{M6}^{223} + n_{M7}^{223} n_{R6}^{84} = n_{M8}^{223} + n_{M9}^{223} n_{R3}^{84} = n_{M6}^{223} + n_{M7}^{223} \\
n_{R5}^{84} &= n_{M8}^{223} + n_{M9}^{223} n_{Z4}^{84} = n_{X5}^{223} n_{Z3}^{84} = n_{X5}^{223}
\end{aligned}$$

The lower SG is SG 131 when the preserved operations are: **(sub-SG label is 8)** 1, 6, 7, 10, 8, 9, 11, 12, 25, 30, 31, 34, 32, 33, 35, 36.

The transformation is:  $(\mathbf{a}_{131}, \mathbf{b}_{131}, \mathbf{c}_{131}) = (\mathbf{a}_{223}, \mathbf{b}_{223}, \mathbf{c}_{223}) \begin{pmatrix} -1 & 0 & 0 \\ 0 & -1 & 0 \\ 0 & 0 & 1 \end{pmatrix}, \overrightarrow{O_{223}O_{131}} = \frac{1}{2}\mathbf{b}_{131} + (\frac{1}{2})\mathbf{c}_{131}$

The reduction of higher dimensional irrep:

$$O_h : E_g \rightarrow A_{1g} + B_{1g} \text{ of } D_{4h}.$$

$$O_h : E_u \rightarrow A_{1u} + B_{1u} \text{ of } D_{4h}.$$

The correspondences of irreps at HSPs from original SG to lowered SG:

$$\begin{aligned} n_{GM8}^{131} &= n_{GM11}^{223} + n_{GM9}^{223} & n_{GM6}^{131} &= n_{GM10}^{223} + n_{GM7}^{223} & n_{GM9}^{131} &= n_{GM11}^{223} + n_{GM8}^{223} & n_{GM7}^{131} &= n_{GM10}^{223} + n_{GM6}^{223} & n_{X6}^{131} &= n_{X5}^{223} & n_{X5}^{131} &= n_{X5}^{223} \\ n_{X5}^{223} n_{M8}^{131} &= n_{M7}^{223} n_{M6}^{131} & n_{M6}^{223} n_{M9}^{131} &= n_{M9}^{223} n_{M9}^{131} & n_{M6}^{223} n_{M7}^{131} &= n_{M8}^{223} n_{A5}^{131} & n_{R5}^{223} &+ n_{R6}^{223} &+ n_{R7}^{223} & n_{R5}^{131} &= n_{M6}^{223} &+ n_{M7}^{223} & n_{R6}^{131} &= n_{M8}^{223} &+ n_{M9}^{223} \\ n_{Z5}^{131} &= n_{X5}^{223} \end{aligned}$$

The lower SG is SG 131 when the preserved operations are: (**sub-SG label is 9**) 1, 2, 3, 8, 9, 10, 13, 14, 25, 26, 27, 32, 33, 34, 37, 38.

$$\text{The transformation is: } (\mathbf{a}_{131}, \mathbf{b}_{131}, \mathbf{c}_{131}) = (\mathbf{a}_{223}, \mathbf{b}_{223}, \mathbf{c}_{223}) \begin{pmatrix} 0 & 0 & 1 \\ -1 & 0 & 0 \\ 0 & -1 & 0 \end{pmatrix}, \overrightarrow{O_{223}O_{131}} = \frac{1}{2}\mathbf{b}_{131} + \left(\frac{1}{2}\right)\mathbf{c}_{131}$$

The reduction of higher dimensional irrep:

$$O_h : E_g \rightarrow A_{1g} + B_{1g} \text{ of } D_{4h}.$$

$$O_h : E_u \rightarrow A_{1u} + B_{1u} \text{ of } D_{4h}.$$

The correspondences of irreps at HSPs from original SG to lowered SG:

$$\begin{aligned} n_{GM8}^{131} &= n_{GM11}^{223} + n_{GM9}^{223} & n_{GM6}^{131} &= n_{GM10}^{223} + n_{GM7}^{223} & n_{GM9}^{131} &= n_{GM11}^{223} + n_{GM8}^{223} & n_{GM7}^{131} &= n_{GM10}^{223} + n_{GM6}^{223} & n_{X6}^{131} &= n_{X5}^{223} & n_{X5}^{131} &= n_{X5}^{223} \\ n_{X5}^{223} n_{M8}^{131} &= n_{M7}^{223} n_{M6}^{131} & n_{M6}^{223} n_{M9}^{131} &= n_{M9}^{223} n_{M9}^{131} & n_{M6}^{223} n_{M7}^{131} &= n_{M8}^{223} n_{A5}^{131} & n_{R5}^{223} &+ n_{R6}^{223} &+ n_{R7}^{223} & n_{R5}^{131} &= n_{M6}^{223} &+ n_{M7}^{223} & n_{R6}^{131} &= n_{M8}^{223} &+ n_{M9}^{223} \\ n_{Z5}^{131} &= n_{X5}^{223} \end{aligned}$$

The lower SG is SG 131 when the preserved operations are: (**sub-SG label is 10**) 1, 4, 5, 9, 10, 8, 16, 15, 25, 28, 29, 33, 34, 32, 40, 39.

$$\text{The transformation is: } (\mathbf{a}_{131}, \mathbf{b}_{131}, \mathbf{c}_{131}) = (\mathbf{a}_{223}, \mathbf{b}_{223}, \mathbf{c}_{223}) \begin{pmatrix} -1 & 0 & 0 \\ 0 & 0 & 1 \\ 0 & 1 & 0 \end{pmatrix}, \overrightarrow{O_{223}O_{131}} = \frac{1}{2}\mathbf{b}_{131} + \left(\frac{1}{2}\right)\mathbf{c}_{131}$$

The reduction of higher dimensional irrep:

$$O_h : E_g \rightarrow A_{1g} + B_{1g} \text{ of } D_{4h}.$$

$$O_h : E_u \rightarrow A_{1u} + B_{1u} \text{ of } D_{4h}.$$

The correspondences of irreps at HSPs from original SG to lowered SG:

$$\begin{aligned} n_{GM8}^{131} &= n_{GM11}^{223} + n_{GM9}^{223} & n_{GM6}^{131} &= n_{GM10}^{223} + n_{GM7}^{223} & n_{GM9}^{131} &= n_{GM11}^{223} + n_{GM8}^{223} & n_{GM7}^{131} &= n_{GM10}^{223} + n_{GM6}^{223} & n_{X6}^{131} &= n_{X5}^{223} & n_{X5}^{131} &= n_{X5}^{223} \\ n_{X5}^{223} n_{M8}^{131} &= n_{M6}^{223} n_{M6}^{131} & n_{M6}^{223} n_{M9}^{131} &= n_{M8}^{223} n_{M9}^{131} & n_{M6}^{223} n_{M7}^{131} &= n_{M9}^{223} n_{A5}^{131} & n_{R5}^{223} &+ n_{R6}^{223} &+ n_{R7}^{223} & n_{R5}^{131} &= n_{M6}^{223} &+ n_{M7}^{223} & n_{R6}^{131} &= n_{M8}^{223} &+ n_{M9}^{223} \\ n_{Z5}^{131} &= n_{X5}^{223} \end{aligned}$$

The lower SG is SG 148 when the preserved operations are: (**sub-SG label is 11**) 1, 17, 18, 25, 41, 42.

$$\text{The transformation is: } (\mathbf{a}_{148}, \mathbf{b}_{148}, \mathbf{c}_{148}) = (\mathbf{a}_{223}, \mathbf{b}_{223}, \mathbf{c}_{223}) \begin{pmatrix} 0 & 1 & 0 \\ 0 & 0 & 1 \\ 1 & 0 & 0 \end{pmatrix}, \overrightarrow{O_{223}O_{148}} = \mathbf{0}$$

The reduction of higher dimensional irrep:

$$O_h : T_{1g} \rightarrow A_g + {}^2E_g + {}^1E_g \text{ of } C_{3i}.$$

$$O_h : T_{2g} \rightarrow A_g + {}^2E_g + {}^1E_g \text{ of } C_{3i}.$$

$$O_h : T_{1u} \rightarrow {}^1E_u + A_u + {}^2E_u \text{ of } C_{3i}.$$

$$O_h : T_{2u} \rightarrow {}^1E_u + A_u + {}^2E_u \text{ of } C_{3i}.$$

The correspondences of irreps at HSPs from original SG to lowered SG:

$$\begin{aligned} n_{GM7}^{148} &= 2n_{GM11}^{223} & n_{GM4}^{148} &= 2n_{GM10}^{223} & n_{GM9}^{148} &= n_{GM11}^{223} + n_{GM8}^{223} + n_{GM9}^{223} & n_{GM6}^{148} &= n_{GM10}^{223} + n_{GM6}^{223} + n_{GM7}^{223} & n_{GM8}^{148} &= n_{GM11}^{223} + n_{GM8}^{223} + n_{GM9}^{223} & n_{GM7}^{148} &= n_{GM10}^{223} + n_{GM6}^{223} + n_{GM7}^{223} & n_{L2}^{148} &= 2n_{X5}^{223} & n_{L3}^{148} &= 2n_{X5}^{223} & n_{F2}^{148} &= 2n_{M8}^{223} + 2n_{M9}^{223} & n_{F3}^{148} &= 2n_{M6}^{223} + 2n_{M7}^{223} & n_{T7}^{148} &= n_{R6}^{223} + n_{R7}^{223} & n_{T4}^{148} &= n_{R6}^{223} + n_{R7}^{223} & n_{T9}^{148} &= n_{R5}^{223} + n_{R7}^{223} & n_{T6}^{148} &= n_{R5}^{223} + n_{R6}^{223} & n_{T8}^{148} &= n_{R5}^{223} + n_{R6}^{223} & n_{T5}^{148} &= n_{R5}^{223} + n_{R6}^{223} \\ n_{R5}^{223} &+ n_{R7}^{223} \end{aligned}$$

The lower SG is SG 148 when the preserved operations are: (**sub-SG label is 12**) 1, 24, 23, 25, 48, 47.

$$\text{The transformation is: } (\mathbf{a}_{148}, \mathbf{b}_{148}, \mathbf{c}_{148}) = (\mathbf{a}_{223}, \mathbf{b}_{223}, \mathbf{c}_{223}) \begin{pmatrix} 0 & -1 & 0 \\ 0 & 0 & -1 \\ 1 & 0 & 0 \end{pmatrix}, \overrightarrow{O_{223}O_{148}} = \mathbf{0}$$

The reduction of higher dimensional irrep:

$$O_h : T_{1g} \rightarrow A_g + {}^2E_g + {}^1E_g \text{ of } C_{3i}.$$

$$O_h : T_{2g} \rightarrow A_g + {}^2E_g + {}^1E_g \text{ of } C_{3i}.$$

$$O_h : T_{1u} \rightarrow {}^1E_u + A_u + {}^2E_u \text{ of } C_{3i}.$$

$$O_h : T_{2u} \rightarrow {}^1E_u + A_u + {}^2E_u \text{ of } C_{3i}.$$

The correspondences of irreps at HSPs from original SG to lowered SG:

$$\begin{aligned}
 n_{GM7}^{148} &= 2n_{GM11}^{223} n_{GM4}^{148} = 2n_{GM10}^{223} n_{GM9}^{148} = n_{GM11}^{223} + n_{GM8}^{223} + n_{GM9}^{223} n_{GM6}^{148} = n_{GM10}^{223} + n_{GM6}^{223} + n_{GM7}^{223} n_{GM8}^{148} = \\
 n_{GM11}^{223} + n_{GM8}^{223} + n_{GM9}^{223} n_{GM5}^{148} &= n_{GM10}^{223} + n_{GM6}^{223} + n_{GM7}^{223} n_{L2}^{148} = 2n_{X5}^{223} n_{L3}^{148} = 2n_{X5}^{223} n_{F2}^{148} = 2n_{M8}^{223} + 2n_{M9}^{223} n_{F3}^{148} = \\
 2n_{M6}^{223} + 2n_{M7}^{223} n_{T7}^{148} &= n_{R6}^{223} + n_{R7}^{223} n_{T4}^{148} = n_{R6}^{223} + n_{R7}^{223} n_{T9}^{148} = n_{R5}^{223} + n_{R7}^{223} n_{T6}^{148} = n_{R5}^{223} + n_{R6}^{223} n_{T8}^{148} = n_{R5}^{223} + n_{R6}^{223} n_{T5}^{148} = \\
 n_{R5}^{223} + n_{R7}^{223}
 \end{aligned}$$

The lower SG is SG 148 when the preserved operations are: **(sub-SG label is 13)** 1, 20, 19, 25, 44, 43.

The transformation is:  $(\mathbf{a}_{148}, \mathbf{b}_{148}, \mathbf{c}_{148}) = (\mathbf{a}_{223}, \mathbf{b}_{223}, \mathbf{c}_{223}) \begin{pmatrix} 1 & 0 & 0 \\ 0 & -1 & 0 \\ 0 & 0 & -1 \end{pmatrix}, \overrightarrow{O_{223}O_{148}} = \mathbf{0}$

The reduction of higher dimensional irrep:

$$\begin{aligned}
 O_h : T_{1g} &\rightarrow A_g + {}^2E_g + {}^1E_g \text{ of } C_{3i}. \\
 O_h : T_{2g} &\rightarrow A_g + {}^2E_g + {}^1E_g \text{ of } C_{3i}. \\
 O_h : T_{1u} &\rightarrow {}^1E_u + A_u + {}^2E_u \text{ of } C_{3i}. \\
 O_h : T_{2u} &\rightarrow {}^1E_u + A_u + {}^2E_u \text{ of } C_{3i}.
 \end{aligned}$$

The correspondences of irreps at HSPs from original SG to lowered SG:

$$\begin{aligned}
 n_{GM7}^{148} &= 2n_{GM11}^{223} n_{GM4}^{148} = 2n_{GM10}^{223} n_{GM9}^{148} = n_{GM11}^{223} + n_{GM8}^{223} + n_{GM9}^{223} n_{GM6}^{148} = n_{GM10}^{223} + n_{GM6}^{223} + n_{GM7}^{223} n_{GM8}^{148} = \\
 n_{GM11}^{223} + n_{GM8}^{223} + n_{GM9}^{223} n_{GM5}^{148} &= n_{GM10}^{223} + n_{GM6}^{223} + n_{GM7}^{223} n_{L2}^{148} = 2n_{X5}^{223} n_{L3}^{148} = 2n_{X5}^{223} n_{F2}^{148} = 2n_{M8}^{223} + 2n_{M9}^{223} n_{F3}^{148} = \\
 2n_{M6}^{223} + 2n_{M7}^{223} n_{T7}^{148} &= n_{R6}^{223} + n_{R7}^{223} n_{T4}^{148} = n_{R6}^{223} + n_{R7}^{223} n_{T9}^{148} = n_{R5}^{223} + n_{R7}^{223} n_{T6}^{148} = n_{R5}^{223} + n_{R6}^{223} n_{T8}^{148} = n_{R5}^{223} + n_{R6}^{223} n_{T5}^{148} = \\
 n_{R5}^{223} + n_{R7}^{223}
 \end{aligned}$$

The lower SG is SG 148 when the preserved operations are: **(sub-SG label is 14)** 1, 22, 21, 25, 46, 45.

The transformation is:  $(\mathbf{a}_{148}, \mathbf{b}_{148}, \mathbf{c}_{148}) = (\mathbf{a}_{223}, \mathbf{b}_{223}, \mathbf{c}_{223}) \begin{pmatrix} -1 & 0 & 0 \\ 0 & 1 & 0 \\ 0 & 0 & -1 \end{pmatrix}, \overrightarrow{O_{223}O_{148}} = \mathbf{0}$

The reduction of higher dimensional irrep:

$$\begin{aligned}
 O_h : T_{1g} &\rightarrow A_g + {}^2E_g + {}^1E_g \text{ of } C_{3i}. \\
 O_h : T_{2g} &\rightarrow A_g + {}^2E_g + {}^1E_g \text{ of } C_{3i}. \\
 O_h : T_{1u} &\rightarrow {}^1E_u + A_u + {}^2E_u \text{ of } C_{3i}. \\
 O_h : T_{2u} &\rightarrow {}^1E_u + A_u + {}^2E_u \text{ of } C_{3i}.
 \end{aligned}$$

The correspondences of irreps at HSPs from original SG to lowered SG:

$$\begin{aligned}
 n_{GM7}^{148} &= 2n_{GM11}^{223} n_{GM4}^{148} = 2n_{GM10}^{223} n_{GM9}^{148} = n_{GM11}^{223} + n_{GM8}^{223} + n_{GM9}^{223} n_{GM6}^{148} = n_{GM10}^{223} + n_{GM6}^{223} + n_{GM7}^{223} n_{GM8}^{148} = \\
 n_{GM11}^{223} + n_{GM8}^{223} + n_{GM9}^{223} n_{GM5}^{148} &= n_{GM10}^{223} + n_{GM6}^{223} + n_{GM7}^{223} n_{L2}^{148} = 2n_{X5}^{223} n_{L3}^{148} = 2n_{X5}^{223} n_{F2}^{148} = 2n_{M8}^{223} + 2n_{M9}^{223} n_{F3}^{148} = \\
 2n_{M6}^{223} + 2n_{M7}^{223} n_{T7}^{148} &= n_{R6}^{223} + n_{R7}^{223} n_{T4}^{148} = n_{R6}^{223} + n_{R7}^{223} n_{T9}^{148} = n_{R5}^{223} + n_{R7}^{223} n_{T6}^{148} = n_{R5}^{223} + n_{R6}^{223} n_{T8}^{148} = n_{R5}^{223} + n_{R6}^{223} n_{T5}^{148} = \\
 n_{R5}^{223} + n_{R7}^{223}
 \end{aligned}$$

The lower SG is SG 200 when the preserved operations are: **(sub-SG label is 15)** 1, 8, 9, 10, 17, 24, 20, 22, 18, 23, 19, 21, 25, 32, 33, 34, 41, 48, 44, 46, 42, 47, 43, 45.

The transformation is:  $(\mathbf{a}_{200}, \mathbf{b}_{200}, \mathbf{c}_{200}) = (\mathbf{a}_{223}, \mathbf{b}_{223}, \mathbf{c}_{223}) \begin{pmatrix} 0 & 0 & 1 \\ 1 & 0 & 0 \\ 0 & 1 & 0 \end{pmatrix}, \overrightarrow{O_{223}O_{200}} = \mathbf{0}$

The reduction of higher dimensional irrep:

$$\begin{aligned}
 O_h : E_g &\rightarrow {}^1E_g + {}^2E_g \text{ of } T_h. \\
 O_h : E_u &\rightarrow {}^1E_u + {}^2E_u \text{ of } T_h.
 \end{aligned}$$

The correspondences of irreps at HSPs from original SG to lowered SG:

$$\begin{aligned}
 n_{GM9}^{200} &= n_{GM11}^{223} n_{GM6}^{200} = n_{GM10}^{223} n_{GM10}^{200} = n_{GM11}^{223} n_{GM7}^{200} = n_{GM10}^{223} n_{GM8}^{200} = n_{GM8}^{223} + n_{GM9}^{223} n_{GM5}^{200} = n_{GM6}^{223} + n_{GM7}^{223} n_{X6}^{200} = \\
 n_{X5}^{223} n_{X5}^{200} &= n_{X5}^{223} n_{M6}^{200} = n_{M8}^{223} + n_{M9}^{223} n_{M5}^{200} = n_{M6}^{223} + n_{M7}^{223} n_{R9}^{200} = n_{R7}^{223} n_{R6}^{200} = n_{R6}^{223} n_{R10}^{200} = n_{R6}^{223} n_{R7}^{200} = n_{R7}^{223} n_{R8}^{200} = n_{R5}^{223} \\
 n_{R5}^{200} &= n_{R5}^{223}
 \end{aligned}$$

**121. Lowered SGs by higher-dimensional irreps of pairings in SG 224**

The representative operations of SG/T for SG 224:

$$\begin{aligned}
& 1 : (x, y, z), 2 : (x + \frac{1}{2}, -z, y + \frac{1}{2}), 3 : (x + \frac{1}{2}, z + \frac{1}{2}, -y), 4 : (z + \frac{1}{2}, y + \frac{1}{2}, -x), 5 : (-z, y + \frac{1}{2}, x + \frac{1}{2}), \\
& 6 : (-y, x + \frac{1}{2}, z + \frac{1}{2}), 7 : (y + \frac{1}{2}, -x, z + \frac{1}{2}), 8 : (x, \frac{1}{2} - y, \frac{1}{2} - z), 9 : (\frac{1}{2} - x, y, \frac{1}{2} - z), 10 : (\frac{1}{2} - x, \frac{1}{2} - y, z), \\
& 11 : (y + \frac{1}{2}, x + \frac{1}{2}, -z), 12 : (-y, -x, -z), 13 : (-x, z + \frac{1}{2}, y + \frac{1}{2}), 14 : (-x, -z, -y), 15 : (z + \frac{1}{2}, -y, x + \frac{1}{2}), \\
& 16 : (-z, -y, -x), 17 : (z, x, y), 18 : (y, z, x), 19 : (\frac{1}{2} - y, z, \frac{1}{2} - x), 20 : (\frac{1}{2} - z, \frac{1}{2} - x, y), 21 : (\frac{1}{2} - y, \frac{1}{2} - z, x), \\
& 22 : (z, \frac{1}{2} - x, \frac{1}{2} - y), 23 : (y, \frac{1}{2} - z, \frac{1}{2} - x), 24 : (\frac{1}{2} - z, x, \frac{1}{2} - y), 25 : (-x, -y, -z), 26 : (\frac{1}{2} - x, z, \frac{1}{2} - y), \\
& 27 : (\frac{1}{2} - x, \frac{1}{2} - z, y), 28 : (\frac{1}{2} - z, \frac{1}{2} - y, x), 29 : (z, \frac{1}{2} - y, \frac{1}{2} - x), 30 : (y, \frac{1}{2} - x, \frac{1}{2} - z), 31 : (\frac{1}{2} - y, x, \frac{1}{2} - z), \\
& 32 : (-x, y + \frac{1}{2}, z + \frac{1}{2}), 33 : (x + \frac{1}{2}, -y, z + \frac{1}{2}), 34 : (x + \frac{1}{2}, y + \frac{1}{2}, -z), 35 : (\frac{1}{2} - y, \frac{1}{2} - x, z), 36 : (y, x, z), \\
& 37 : (x, \frac{1}{2} - z, \frac{1}{2} - y), 38 : (x, z, y), 39 : (\frac{1}{2} - z, y, \frac{1}{2} - x), 40 : (z, y, x), 41 : (-z, -x, -y), 42 : (-y, -z, -x), \\
& 43 : (y + \frac{1}{2}, -z, x + \frac{1}{2}), 44 : (z + \frac{1}{2}, x + \frac{1}{2}, -y), 45 : (y + \frac{1}{2}, z + \frac{1}{2}, -x), 46 : (-z, x + \frac{1}{2}, y + \frac{1}{2}), 47 : (-y, z + \frac{1}{2}, x + \frac{1}{2}), \\
& 48 : (z + \frac{1}{2}, -x, y + \frac{1}{2}).
\end{aligned}$$

The lower SG is SG 48 when the preserved operations are: **(sub-SG label is 1) 1, 8, 9, 10, 25, 32, 33, 34.**

The transformation is:  $(\mathbf{a}_{48}, \mathbf{b}_{48}, \mathbf{c}_{48}) = (\mathbf{a}_{224}, \mathbf{b}_{224}, \mathbf{c}_{224}) \begin{pmatrix} 0 & 0 & 1 \\ 1 & 0 & 0 \\ 0 & 1 & 0 \end{pmatrix}, \overrightarrow{O_{224}O_{48}} = \frac{1}{2}\mathbf{a}_{48} + (\frac{1}{2})\mathbf{c}_{48}$

The reduction of higher dimensional irrep:

$$O_h : T_{1g} \rightarrow B_{2g} + B_{1g} + B_{3g} \text{ of } D_{2h}.$$

$$O_h : T_{2g} \rightarrow B_{2g} + B_{1g} + B_{3g} \text{ of } D_{2h}.$$

$$O_h : T_{1u} \rightarrow B_{2u} + B_{1u} + B_{3u} \text{ of } D_{2h}.$$

$$O_h : T_{2u} \rightarrow B_{2u} + B_{1u} + B_{3u} \text{ of } D_{2h}.$$

The correspondences of irreps at HSPs from original SG to lowered SG:

$$\begin{aligned}
n_{GM6}^{48} &= 2n_{GM11}^{224} + n_{GM8}^{224} + n_{GM9}^{224} \quad n_{GM5}^{48} = 2n_{GM10}^{224} + n_{GM6}^{224} + n_{GM7}^{224} \quad n_{X4}^{48} = n_{X5}^{224} \quad n_{X3}^{48} = n_{X5}^{224} \quad n_{S3}^{48} = n_{M5}^{224} \quad n_{S4}^{48} = n_{M5}^{224} \\
n_{R6}^{48} &= 2n_{R11}^{224} + n_{R8}^{224} + n_{R9}^{224} \quad n_{R5}^{48} = 2n_{R10}^{224} + n_{R6}^{224} + n_{R7}^{224} \quad n_{U3}^{48} = n_{M5}^{224} \quad n_{U4}^{48} = n_{M5}^{224} \quad n_{Z4}^{48} = n_{X5}^{224} \quad n_{Z3}^{48} = n_{X5}^{224} \quad n_{T4}^{48} = n_{M5}^{224} \quad n_{T3}^{48} = n_{M5}^{224} \\
n_{M5}^{224} n_{Y4}^{48} &= n_{X5}^{224} n_{Y3}^{48} = n_{X5}^{224}
\end{aligned}$$

The lower SG is SG 67 when the preserved operations are: **(sub-SG label is 2) 1, 8, 13, 14, 25, 32, 37, 38.**

The transformation is:  $(\mathbf{a}_{67}, \mathbf{b}_{67}, \mathbf{c}_{67}) = (\mathbf{a}_{224}, \mathbf{b}_{224}, \mathbf{c}_{224}) \begin{pmatrix} 0 & 0 & 1 \\ 1 & -1 & 0 \\ 1 & 1 & 0 \end{pmatrix}, \overrightarrow{O_{224}O_{67}} = \frac{1}{4}\mathbf{a}_{67} + (\frac{1}{4})\mathbf{b}_{67} + (\frac{1}{2})\mathbf{c}_{67}$

The reduction of higher dimensional irrep:

$$O_h : T_{1g} \rightarrow B_{2g} + B_{1g} + B_{3g} \text{ of } D_{2h}.$$

$$O_h : T_{2g} \rightarrow A_g + B_{2g} + B_{3g} \text{ of } D_{2h}.$$

$$O_h : T_{1u} \rightarrow B_{2u} + B_{1u} + B_{3u} \text{ of } D_{2h}.$$

$$O_h : T_{2u} \rightarrow A_u + B_{2u} + B_{3u} \text{ of } D_{2h}.$$

The correspondences of irreps at HSPs from original SG to lowered SG:

$$\begin{aligned}
n_{GM6}^{67} &= 2n_{GM11}^{224} + n_{GM8}^{224} + n_{GM9}^{224} \quad n_{GM5}^{67} = 2n_{GM10}^{224} + n_{GM6}^{224} + n_{GM7}^{224} \quad n_{Y6}^{67} = n_{M5}^{224} \quad n_{Y5}^{67} = n_{M5}^{224} \quad n_{S2}^{67} = 2n_{X5}^{224} \quad n_{Z6}^{67} = n_{X5}^{224} \\
n_{Z5}^{67} &= n_{X5}^{224} \quad n_{T6}^{67} = 2n_{R11}^{224} + n_{R8}^{224} + n_{R9}^{224} \quad n_{T5}^{67} = 2n_{R10}^{224} + n_{R6}^{224} + n_{R7}^{224} \quad n_{R2}^{67} = 2n_{M5}^{224}
\end{aligned}$$

The lower SG is SG 67 when the preserved operations are: **(sub-SG label is 3) 1, 9, 16, 15, 25, 33, 40, 39.**

The transformation is:  $(\mathbf{a}_{67}, \mathbf{b}_{67}, \mathbf{c}_{67}) = (\mathbf{a}_{224}, \mathbf{b}_{224}, \mathbf{c}_{224}) \begin{pmatrix} 1 & 1 & 0 \\ 0 & 0 & 1 \\ 1 & -1 & 0 \end{pmatrix}, \overrightarrow{O_{224}O_{67}} = \frac{1}{4}\mathbf{a}_{67} + (\frac{1}{4})\mathbf{b}_{67} + (\frac{1}{2})\mathbf{c}_{67}$

The reduction of higher dimensional irrep:

$$O_h : T_{1g} \rightarrow B_{2g} + B_{1g} + B_{3g} \text{ of } D_{2h}.$$

$$O_h : T_{2g} \rightarrow A_g + B_{2g} + B_{3g} \text{ of } D_{2h}.$$

$$O_h : T_{1u} \rightarrow B_{2u} + B_{1u} + B_{3u} \text{ of } D_{2h}.$$

$$O_h : T_{2u} \rightarrow A_u + B_{2u} + B_{3u} \text{ of } D_{2h}.$$

The correspondences of irreps at HSPs from original SG to lowered SG:

$$\begin{aligned}
n_{GM6}^{67} &= 2n_{GM11}^{224} + n_{GM8}^{224} + n_{GM9}^{224} \quad n_{GM5}^{67} = 2n_{GM10}^{224} + n_{GM6}^{224} + n_{GM7}^{224} \quad n_{Y6}^{67} = n_{M5}^{224} \quad n_{Y5}^{67} = n_{M5}^{224} \quad n_{S2}^{67} = 2n_{X5}^{224} \quad n_{Z6}^{67} = n_{X5}^{224} \\
n_{Z5}^{67} &= n_{X5}^{224} \quad n_{T6}^{67} = 2n_{R11}^{224} + n_{R8}^{224} + n_{R9}^{224} \quad n_{T5}^{67} = 2n_{R10}^{224} + n_{R6}^{224} + n_{R7}^{224} \quad n_{R2}^{67} = 2n_{M5}^{224}
\end{aligned}$$

The lower SG is SG 67 when the preserved operations are: **(sub-SG label is 4) 1, 10, 11, 12, 25, 34, 35, 36.**

The transformation is:  $(\mathbf{a}_{67}, \mathbf{b}_{67}, \mathbf{c}_{67}) = (\mathbf{a}_{224}, \mathbf{b}_{224}, \mathbf{c}_{224}) \begin{pmatrix} 1 & -1 & 0 \\ 1 & 1 & 0 \\ 0 & 0 & 1 \end{pmatrix}, \overrightarrow{O_{224}O_{67}} = \frac{1}{4}\mathbf{a}_{67} + (\frac{1}{4})\mathbf{b}_{67} + (\frac{1}{2})\mathbf{c}_{67}$

The reduction of higher dimensional irrep:

$$O_h : T_{1g} \rightarrow B_{2g} + B_{1g} + B_{3g} \text{ of } D_{2h}.$$

$$O_h : T_{2g} \rightarrow A_g + B_{2g} + B_{3g} \text{ of } D_{2h}.$$

$$O_h : T_{1u} \rightarrow B_{2u} + B_{1u} + B_{3u} \text{ of } D_{2h}.$$

$$O_h : T_{2u} \rightarrow A_u + B_{2u} + B_{3u} \text{ of } D_{2h}.$$

The correspondences of irreps at HSPs from original SG to lowered SG:

$$\begin{aligned} n_{GM6}^{67} &= 2n_{GM11}^{224} + n_{GM8}^{224} + n_{GM9}^{224} n_{GM5}^{67} = 2n_{GM10}^{224} + n_{GM6}^{224} + n_{GM7}^{224} n_{Y6}^{67} = n_{M5}^{224} n_{Y5}^{67} = n_{M5}^{224} n_{S2}^{67} = 2n_{X5}^{224} n_{Z6}^{67} = n_{X5}^{224} \\ n_{Z5}^{67} &= n_{X5}^{224} n_{T6}^{67} = 2n_{R11}^{224} + n_{R8}^{224} + n_{R9}^{224} n_{T5}^{67} = 2n_{R10}^{224} + n_{R6}^{224} + n_{R7}^{224} n_{R2}^{67} = 2n_{M5}^{224} \end{aligned}$$

The lower SG is SG 86 when the preserved operations are: **(sub-SG label is 5)** 1, 6, 7, 10, 25, 30, 31, 34.

$$\text{The transformation is: } (\mathbf{a}_{86}, \mathbf{b}_{86}, \mathbf{c}_{86}) = (\mathbf{a}_{224}, \mathbf{b}_{224}, \mathbf{c}_{224}) \begin{pmatrix} -1 & 0 & 0 \\ 0 & 1 & 0 \\ 0 & 0 & -1 \end{pmatrix}, \overrightarrow{O_{224}O_{86}} = \frac{1}{2}\mathbf{b}_{86} + \left(\frac{1}{2}\right)\mathbf{c}_{86}$$

The reduction of higher dimensional irrep:

$$O_h : T_{1g} \rightarrow A_g + {}^2E_g + {}^1E_g \text{ of } C_{4h}.$$

$$O_h : T_{2g} \rightarrow {}^2E_g + B_g + {}^1E_g \text{ of } C_{4h}.$$

$$O_h : T_{1u} \rightarrow A_u + {}^2E_u + {}^1E_u \text{ of } C_{4h}.$$

$$O_h : T_{2u} \rightarrow {}^2E_u + B_u + {}^1E_u \text{ of } C_{4h}.$$

The correspondences of irreps at HSPs from original SG to lowered SG:

$$\begin{aligned} n_{GM9}^{86} &= n_{GM11}^{224} + n_{GM9}^{224} n_{GM5}^{86} = n_{GM10}^{224} + n_{GM7}^{224} n_{GM11}^{86} = n_{GM11}^{224} + n_{GM9}^{224} n_{GM7}^{86} = n_{GM10}^{224} + n_{GM7}^{224} n_{GM12}^{86} = \\ n_{GM11}^{224} + n_{GM8}^{224} n_{GM8}^{86} &= n_{GM10}^{224} + n_{GM6}^{224} n_{GM10}^{86} = n_{GM11}^{224} + n_{GM8}^{224} n_{GM6}^{86} = n_{GM10}^{224} + n_{GM6}^{224} n_{X2}^{86} = 2n_{X5}^{224} n_{M3}^{86} = n_{M5}^{224} \\ n_{M4}^{86} &= n_{M5}^{224} n_{A10}^{86} = n_{R11}^{224} + n_{R9}^{224} n_{A6}^{86} = n_{R10}^{224} + n_{R7}^{224} n_{A12}^{86} = n_{R11}^{224} + n_{R9}^{224} n_{A8}^{86} = n_{R10}^{224} + n_{R7}^{224} n_{A11}^{86} = n_{R11}^{224} + n_{R8}^{224} n_{A7}^{86} = \\ n_{R10}^{224} + n_{R6}^{224} n_{A9}^{86} &= n_{R11}^{224} + n_{R8}^{224} n_{A5}^{86} = n_{R10}^{224} + n_{R6}^{224} n_{R2}^{86} = 2n_{M5}^{224} n_{Z4}^{86} = n_{X5}^{224} n_{Z3}^{86} = n_{X5}^{224} \end{aligned}$$

The lower SG is SG 86 when the preserved operations are: **(sub-SG label is 6)** 1, 2, 3, 8, 25, 26, 27, 32.

$$\text{The transformation is: } (\mathbf{a}_{86}, \mathbf{b}_{86}, \mathbf{c}_{86}) = (\mathbf{a}_{224}, \mathbf{b}_{224}, \mathbf{c}_{224}) \begin{pmatrix} 0 & 0 & -1 \\ -1 & 0 & 0 \\ 0 & 1 & 0 \end{pmatrix}, \overrightarrow{O_{224}O_{86}} = \frac{1}{2}\mathbf{b}_{86} + \left(\frac{1}{2}\right)\mathbf{c}_{86}$$

The reduction of higher dimensional irrep:

$$O_h : T_{1g} \rightarrow A_g + {}^2E_g + {}^1E_g \text{ of } C_{4h}.$$

$$O_h : T_{2g} \rightarrow {}^2E_g + B_g + {}^1E_g \text{ of } C_{4h}.$$

$$O_h : T_{1u} \rightarrow A_u + {}^2E_u + {}^1E_u \text{ of } C_{4h}.$$

$$O_h : T_{2u} \rightarrow {}^2E_u + B_u + {}^1E_u \text{ of } C_{4h}.$$

The correspondences of irreps at HSPs from original SG to lowered SG:

$$\begin{aligned} n_{GM9}^{86} &= n_{GM11}^{224} + n_{GM9}^{224} n_{GM5}^{86} = n_{GM10}^{224} + n_{GM7}^{224} n_{GM11}^{86} = n_{GM11}^{224} + n_{GM9}^{224} n_{GM7}^{86} = n_{GM10}^{224} + n_{GM7}^{224} n_{GM12}^{86} = \\ n_{GM11}^{224} + n_{GM8}^{224} n_{GM8}^{86} &= n_{GM10}^{224} + n_{GM6}^{224} n_{GM10}^{86} = n_{GM11}^{224} + n_{GM8}^{224} n_{GM6}^{86} = n_{GM10}^{224} + n_{GM6}^{224} n_{X2}^{86} = 2n_{X5}^{224} n_{M3}^{86} = n_{M5}^{224} \\ n_{M4}^{86} &= n_{M5}^{224} n_{A10}^{86} = n_{R11}^{224} + n_{R9}^{224} n_{A6}^{86} = n_{R10}^{224} + n_{R7}^{224} n_{A12}^{86} = n_{R11}^{224} + n_{R9}^{224} n_{A8}^{86} = n_{R10}^{224} + n_{R7}^{224} n_{A11}^{86} = n_{R11}^{224} + n_{R8}^{224} n_{A7}^{86} = \\ n_{R10}^{224} + n_{R6}^{224} n_{A9}^{86} &= n_{R11}^{224} + n_{R8}^{224} n_{A5}^{86} = n_{R10}^{224} + n_{R6}^{224} n_{R2}^{86} = 2n_{M5}^{224} n_{Z4}^{86} = n_{X5}^{224} n_{Z3}^{86} = n_{X5}^{224} \end{aligned}$$

The lower SG is SG 86 when the preserved operations are: **(sub-SG label is 7)** 1, 4, 5, 9, 25, 28, 29, 33.

$$\text{The transformation is: } (\mathbf{a}_{86}, \mathbf{b}_{86}, \mathbf{c}_{86}) = (\mathbf{a}_{224}, \mathbf{b}_{224}, \mathbf{c}_{224}) \begin{pmatrix} -1 & 0 & 0 \\ 0 & 0 & 1 \\ 0 & 1 & 0 \end{pmatrix}, \overrightarrow{O_{224}O_{86}} = \frac{1}{2}\mathbf{b}_{86} + \left(\frac{1}{2}\right)\mathbf{c}_{86}$$

The reduction of higher dimensional irrep:

$$O_h : T_{1g} \rightarrow A_g + {}^2E_g + {}^1E_g \text{ of } C_{4h}.$$

$$O_h : T_{2g} \rightarrow {}^2E_g + B_g + {}^1E_g \text{ of } C_{4h}.$$

$$O_h : T_{1u} \rightarrow A_u + {}^2E_u + {}^1E_u \text{ of } C_{4h}.$$

$$O_h : T_{2u} \rightarrow {}^2E_u + B_u + {}^1E_u \text{ of } C_{4h}.$$

The correspondences of irreps at HSPs from original SG to lowered SG:

$$\begin{aligned} n_{GM9}^{86} &= n_{GM11}^{224} + n_{GM9}^{224} n_{GM5}^{86} = n_{GM10}^{224} + n_{GM7}^{224} n_{GM11}^{86} = n_{GM11}^{224} + n_{GM9}^{224} n_{GM7}^{86} = n_{GM10}^{224} + n_{GM7}^{224} n_{GM12}^{86} = \\ n_{GM11}^{224} + n_{GM8}^{224} n_{GM8}^{86} &= n_{GM10}^{224} + n_{GM6}^{224} n_{GM10}^{86} = n_{GM11}^{224} + n_{GM8}^{224} n_{GM6}^{86} = n_{GM10}^{224} + n_{GM6}^{224} n_{X2}^{86} = 2n_{X5}^{224} n_{M3}^{86} = n_{M5}^{224} \\ n_{M4}^{86} &= n_{M5}^{224} n_{A10}^{86} = n_{R11}^{224} + n_{R8}^{224} n_{A6}^{86} = n_{R10}^{224} + n_{R6}^{224} n_{A12}^{86} = n_{R11}^{224} + n_{R8}^{224} n_{A8}^{86} = n_{R10}^{224} + n_{R6}^{224} n_{A11}^{86} = n_{R11}^{224} + n_{R9}^{224} n_{A7}^{86} = \\ n_{R10}^{224} + n_{R7}^{224} n_{A9}^{86} &= n_{R11}^{224} + n_{R9}^{224} n_{A5}^{86} = n_{R10}^{224} + n_{R7}^{224} n_{R2}^{86} = 2n_{M5}^{224} n_{Z4}^{86} = n_{X5}^{224} n_{Z3}^{86} = n_{X5}^{224} \end{aligned}$$

The lower SG is SG 134 when the preserved operations are: **(sub-SG label is 8)** 1, 6, 7, 10, 8, 9, 11, 12, 25, 30, 31, 34, 32, 33, 35, 36.

The transformation is:  $(\mathbf{a}_{134}, \mathbf{b}_{134}, \mathbf{c}_{134}) = (\mathbf{a}_{224}, \mathbf{b}_{224}, \mathbf{c}_{224}) \begin{pmatrix} -1 & 0 & 0 \\ 0 & 1 & 0 \\ 0 & 0 & -1 \end{pmatrix}, \overrightarrow{O_{224}O_{134}} = \frac{1}{2}\mathbf{c}_{134}$

The reduction of higher dimensional irrep:

$$O_h : E_g \rightarrow A_{1g} + B_{1g} \text{ of } D_{4h}.$$

$$O_h : E_u \rightarrow A_{1u} + B_{1u} \text{ of } D_{4h}.$$

The correspondences of irreps at HSPs from original SG to lowered SG:

$$\begin{aligned} n_{GM8}^{134} &= n_{GM11}^{224} + n_{GM9}^{224} & n_{GM6}^{134} &= n_{GM10}^{224} + n_{GM7}^{224} & n_{GM9}^{134} &= n_{GM11}^{224} + n_{GM8}^{224} & n_{GM7}^{134} &= n_{GM10}^{224} + n_{GM6}^{224} & n_{X4}^{134} &= n_{X5}^{224} & n_{X3}^{134} &= n_{X5}^{224} \\ n_{X5}^{224} n_{M5}^{134} &= n_{M5}^{224} n_{A9}^{134} & &= n_{R10}^{224} + n_{R6}^{224} & n_{A7}^{134} &= n_{R11}^{224} + n_{R8}^{224} & n_{A8}^{134} &= n_{R10}^{224} + n_{R7}^{224} & n_{A6}^{134} &= n_{R11}^{224} + n_{R9}^{224} & n_{R4}^{134} &= n_{M5}^{224} n_{R3}^{134} \\ n_{M5}^{224} n_{Z5}^{134} &= n_{X5}^{224} & & & & & & & & & & \end{aligned}$$

The lower SG is SG 134 when the preserved operations are: (**sub-SG label is 9**) 1, 2, 3, 8, 9, 10, 13, 14, 25, 26, 27, 32, 33, 34, 37, 38.

The transformation is:  $(\mathbf{a}_{134}, \mathbf{b}_{134}, \mathbf{c}_{134}) = (\mathbf{a}_{224}, \mathbf{b}_{224}, \mathbf{c}_{224}) \begin{pmatrix} 0 & 0 & -1 \\ -1 & 0 & 0 \\ 0 & 1 & 0 \end{pmatrix}, \overrightarrow{O_{224}O_{134}} = \frac{1}{2}\mathbf{c}_{134}$

The reduction of higher dimensional irrep:

$$O_h : E_g \rightarrow A_{1g} + B_{1g} \text{ of } D_{4h}.$$

$$O_h : E_u \rightarrow A_{1u} + B_{1u} \text{ of } D_{4h}.$$

The correspondences of irreps at HSPs from original SG to lowered SG:

$$\begin{aligned} n_{GM8}^{134} &= n_{GM11}^{224} + n_{GM9}^{224} & n_{GM6}^{134} &= n_{GM10}^{224} + n_{GM7}^{224} & n_{GM9}^{134} &= n_{GM11}^{224} + n_{GM8}^{224} & n_{GM7}^{134} &= n_{GM10}^{224} + n_{GM6}^{224} & n_{X4}^{134} &= n_{X5}^{224} & n_{X3}^{134} &= n_{X5}^{224} \\ n_{X5}^{224} n_{M5}^{134} &= n_{M5}^{224} n_{A9}^{134} & &= n_{R10}^{224} + n_{R6}^{224} & n_{A7}^{134} &= n_{R11}^{224} + n_{R8}^{224} & n_{A8}^{134} &= n_{R10}^{224} + n_{R7}^{224} & n_{A6}^{134} &= n_{R11}^{224} + n_{R9}^{224} & n_{R4}^{134} &= n_{M5}^{224} n_{R3}^{134} \\ n_{M5}^{224} n_{Z5}^{134} &= n_{X5}^{224} & & & & & & & & & & \end{aligned}$$

The lower SG is SG 134 when the preserved operations are: (**sub-SG label is 10**) 1, 4, 5, 9, 10, 8, 16, 15, 25, 28, 29, 33, 34, 32, 40, 39.

The transformation is:  $(\mathbf{a}_{134}, \mathbf{b}_{134}, \mathbf{c}_{134}) = (\mathbf{a}_{224}, \mathbf{b}_{224}, \mathbf{c}_{224}) \begin{pmatrix} -1 & 0 & 0 \\ 0 & 0 & 1 \\ 0 & 1 & 0 \end{pmatrix}, \overrightarrow{O_{224}O_{134}} = \frac{1}{2}\mathbf{c}_{134}$

The reduction of higher dimensional irrep:

$$O_h : E_g \rightarrow A_{1g} + B_{1g} \text{ of } D_{4h}.$$

$$O_h : E_u \rightarrow A_{1u} + B_{1u} \text{ of } D_{4h}.$$

The correspondences of irreps at HSPs from original SG to lowered SG:

$$\begin{aligned} n_{GM8}^{134} &= n_{GM11}^{224} + n_{GM9}^{224} & n_{GM6}^{134} &= n_{GM10}^{224} + n_{GM7}^{224} & n_{GM9}^{134} &= n_{GM11}^{224} + n_{GM8}^{224} & n_{GM7}^{134} &= n_{GM10}^{224} + n_{GM6}^{224} & n_{X4}^{134} &= n_{X5}^{224} & n_{X3}^{134} &= n_{X5}^{224} \\ n_{X5}^{224} n_{M5}^{134} &= n_{M5}^{224} n_{A9}^{134} & &= n_{R10}^{224} + n_{R6}^{224} & n_{A7}^{134} &= n_{R11}^{224} + n_{R8}^{224} & n_{A8}^{134} &= n_{R10}^{224} + n_{R6}^{224} & n_{A6}^{134} &= n_{R11}^{224} + n_{R8}^{224} & n_{R4}^{134} &= n_{M5}^{224} n_{R3}^{134} \\ n_{M5}^{224} n_{Z5}^{134} &= n_{X5}^{224} & & & & & & & & & & \end{aligned}$$

The lower SG is SG 148 when the preserved operations are: (**sub-SG label is 11**) 1, 17, 18, 25, 41, 42.

The transformation is:  $(\mathbf{a}_{148}, \mathbf{b}_{148}, \mathbf{c}_{148}) = (\mathbf{a}_{224}, \mathbf{b}_{224}, \mathbf{c}_{224}) \begin{pmatrix} 0 & 1 & 0 \\ 0 & 0 & 1 \\ 1 & 0 & 0 \end{pmatrix}, \overrightarrow{O_{224}O_{148}} = \mathbf{0}$

The reduction of higher dimensional irrep:

$$O_h : T_{1g} \rightarrow A_g + {}^2E_g + {}^1E_g \text{ of } C_{3i}.$$

$$O_h : T_{2g} \rightarrow A_g + {}^2E_g + {}^1E_g \text{ of } C_{3i}.$$

$$O_h : T_{1u} \rightarrow {}^1E_u + A_u + {}^2E_u \text{ of } C_{3i}.$$

$$O_h : T_{2u} \rightarrow {}^1E_u + A_u + {}^2E_u \text{ of } C_{3i}.$$

The correspondences of irreps at HSPs from original SG to lowered SG:

$$\begin{aligned} n_{GM7}^{148} &= 2n_{GM11}^{224} & n_{GM4}^{148} &= 2n_{GM10}^{224} & n_{GM9}^{148} &= n_{GM11}^{224} + n_{GM8}^{224} + n_{GM9}^{224} & n_{GM6}^{148} &= n_{GM10}^{224} + n_{GM6}^{224} + n_{GM7}^{224} & n_{GM8}^{148} &= 2n_{GM11}^{224} & n_{GM5}^{148} &= 2n_{GM10}^{224} \\ n_{GM11}^{224} + n_{GM8}^{224} + n_{GM9}^{224} & & n_{GM5}^{148} &= n_{GM10}^{224} + n_{GM6}^{224} + n_{GM7}^{224} & n_{L2}^{148} &= 2n_{X5}^{224} & n_{L3}^{148} &= 2n_{X5}^{224} & n_{F2}^{148} &= 2n_{M5}^{224} & n_{F3}^{148} &= 2n_{M5}^{224} \\ n_{T7}^{148} &= 2n_{R11}^{224} & n_{T4}^{148} &= 2n_{R10}^{224} & n_{T9}^{148} &= n_{R11}^{224} + n_{R8}^{224} + n_{R9}^{224} & n_{T6}^{148} &= n_{R10}^{224} + n_{R6}^{224} + n_{R7}^{224} & n_{T8}^{148} &= n_{R11}^{224} + n_{R8}^{224} + n_{R9}^{224} & n_{T5}^{148} &= n_{R10}^{224} + n_{R6}^{224} + n_{R7}^{224} \end{aligned}$$

The lower SG is SG 148 when the preserved operations are: (**sub-SG label is 12**) 1, 24, 23, 25, 48, 47.

The transformation is:  $(\mathbf{a}_{148}, \mathbf{b}_{148}, \mathbf{c}_{148}) = (\mathbf{a}_{224}, \mathbf{b}_{224}, \mathbf{c}_{224}) \begin{pmatrix} 0 & -1 & 0 \\ 0 & 0 & -1 \\ 1 & 0 & 0 \end{pmatrix}, \overrightarrow{O_{224}O_{148}} = \frac{1}{2}\mathbf{b}_{148} + (\frac{1}{2})\mathbf{c}_{148}$

The reduction of higher dimensional irrep:

$$O_h : T_{1g} \rightarrow A_g + {}^2E_g + {}^1E_g \text{ of } C_{3i}.$$

$$O_h : T_{2g} \rightarrow A_g + {}^2E_g + {}^1E_g \text{ of } C_{3i}.$$

$$O_h : T_{1u} \rightarrow {}^1E_u + A_u + {}^2E_u \text{ of } C_{3i}.$$

$$O_h : T_{2u} \rightarrow {}^1E_u + A_u + {}^2E_u \text{ of } C_{3i}.$$

The correspondences of irreps at HSPs from original SG to lowered SG:

$$\begin{aligned} n_{GM7}^{148} &= 2n_{GM11}^{224} n_{GM4}^{148} = 2n_{GM10}^{224} n_{GM9}^{148} = n_{GM11}^{224} + n_{GM8}^{224} + n_{GM9}^{224} n_{GM6}^{148} = n_{GM10}^{224} + n_{GM6}^{224} + n_{GM7}^{224} n_{GM8}^{148} = \\ n_{GM11}^{224} + n_{GM8}^{224} + n_{GM9}^{224} n_{GM5}^{148} &= n_{GM10}^{224} + n_{GM6}^{224} + n_{GM7}^{224} n_{L2}^{148} = 2n_{X5}^{224} n_{L3}^{148} = 2n_{X5}^{224} n_{F2}^{148} = 2n_{M5}^{224} n_{F3}^{148} = 2n_{M5}^{224} \\ n_{T7}^{148} &= 2n_{R11}^{224} n_{T4}^{148} = 2n_{R10}^{224} n_{T9}^{148} = n_{R11}^{224} + n_{R8}^{224} + n_{R9}^{224} n_{T6}^{148} = n_{R10}^{224} + n_{R6}^{224} + n_{R7}^{224} n_{T8}^{148} = n_{R11}^{224} + n_{R8}^{224} + n_{R9}^{224} n_{T5}^{148} = \\ n_{R10}^{224} + n_{R6}^{224} + n_{R7}^{224} \end{aligned}$$

The lower SG is SG 148 when the preserved operations are: (**sub-SG label is 13**) 1, 20, 19, 25, 44, 43.

$$\text{The transformation is: } (\mathbf{a}_{148}, \mathbf{b}_{148}, \mathbf{c}_{148}) = (\mathbf{a}_{224}, \mathbf{b}_{224}, \mathbf{c}_{224}) \begin{pmatrix} 1 & 0 & 0 \\ 0 & -1 & 0 \\ 0 & 0 & -1 \end{pmatrix}, \overrightarrow{O_{224}O_{148}} = \frac{1}{2}\mathbf{b}_{148} + \left(\frac{1}{2}\right)\mathbf{c}_{148}$$

The reduction of higher dimensional irrep:

$$O_h : T_{1g} \rightarrow A_g + {}^2E_g + {}^1E_g \text{ of } C_{3i}.$$

$$O_h : T_{2g} \rightarrow A_g + {}^2E_g + {}^1E_g \text{ of } C_{3i}.$$

$$O_h : T_{1u} \rightarrow {}^1E_u + A_u + {}^2E_u \text{ of } C_{3i}.$$

$$O_h : T_{2u} \rightarrow {}^1E_u + A_u + {}^2E_u \text{ of } C_{3i}.$$

The correspondences of irreps at HSPs from original SG to lowered SG:

$$\begin{aligned} n_{GM7}^{148} &= 2n_{GM11}^{224} n_{GM4}^{148} = 2n_{GM10}^{224} n_{GM9}^{148} = n_{GM11}^{224} + n_{GM8}^{224} + n_{GM9}^{224} n_{GM6}^{148} = n_{GM10}^{224} + n_{GM6}^{224} + n_{GM7}^{224} n_{GM8}^{148} = \\ n_{GM11}^{224} + n_{GM8}^{224} + n_{GM9}^{224} n_{GM5}^{148} &= n_{GM10}^{224} + n_{GM6}^{224} + n_{GM7}^{224} n_{L2}^{148} = 2n_{X5}^{224} n_{L3}^{148} = 2n_{X5}^{224} n_{F2}^{148} = 2n_{M5}^{224} n_{F3}^{148} = 2n_{M5}^{224} \\ n_{T7}^{148} &= 2n_{R11}^{224} n_{T4}^{148} = 2n_{R10}^{224} n_{T9}^{148} = n_{R11}^{224} + n_{R8}^{224} + n_{R9}^{224} n_{T6}^{148} = n_{R10}^{224} + n_{R6}^{224} + n_{R7}^{224} n_{T8}^{148} = n_{R11}^{224} + n_{R8}^{224} + n_{R9}^{224} n_{T5}^{148} = \\ n_{R10}^{224} + n_{R6}^{224} + n_{R7}^{224} \end{aligned}$$

The lower SG is SG 148 when the preserved operations are: (**sub-SG label is 14**) 1, 22, 21, 25, 46, 45.

$$\text{The transformation is: } (\mathbf{a}_{148}, \mathbf{b}_{148}, \mathbf{c}_{148}) = (\mathbf{a}_{224}, \mathbf{b}_{224}, \mathbf{c}_{224}) \begin{pmatrix} -1 & 0 & 0 \\ 0 & 1 & 0 \\ 0 & 0 & -1 \end{pmatrix}, \overrightarrow{O_{224}O_{148}} = \frac{1}{2}\mathbf{b}_{148}$$

The reduction of higher dimensional irrep:

$$O_h : T_{1g} \rightarrow A_g + {}^2E_g + {}^1E_g \text{ of } C_{3i}.$$

$$O_h : T_{2g} \rightarrow A_g + {}^2E_g + {}^1E_g \text{ of } C_{3i}.$$

$$O_h : T_{1u} \rightarrow {}^1E_u + A_u + {}^2E_u \text{ of } C_{3i}.$$

$$O_h : T_{2u} \rightarrow {}^1E_u + A_u + {}^2E_u \text{ of } C_{3i}.$$

The correspondences of irreps at HSPs from original SG to lowered SG:

$$\begin{aligned} n_{GM7}^{148} &= 2n_{GM11}^{224} n_{GM4}^{148} = 2n_{GM10}^{224} n_{GM9}^{148} = n_{GM11}^{224} + n_{GM8}^{224} + n_{GM9}^{224} n_{GM6}^{148} = n_{GM10}^{224} + n_{GM6}^{224} + n_{GM7}^{224} n_{GM8}^{148} = \\ n_{GM11}^{224} + n_{GM8}^{224} + n_{GM9}^{224} n_{GM5}^{148} &= n_{GM10}^{224} + n_{GM6}^{224} + n_{GM7}^{224} n_{L2}^{148} = 2n_{X5}^{224} n_{L3}^{148} = 2n_{X5}^{224} n_{F2}^{148} = 2n_{M5}^{224} n_{F3}^{148} = 2n_{M5}^{224} \\ n_{T7}^{148} &= 2n_{R10}^{224} n_{T4}^{148} = 2n_{R11}^{224} n_{T9}^{148} = n_{R10}^{224} + n_{R6}^{224} + n_{R7}^{224} n_{T6}^{148} = n_{R11}^{224} + n_{R8}^{224} + n_{R9}^{224} n_{T8}^{148} = n_{R10}^{224} + n_{R6}^{224} + n_{R7}^{224} n_{T5}^{148} = \\ n_{R11}^{224} + n_{R8}^{224} + n_{R9}^{224} \end{aligned}$$

The lower SG is SG 201 when the preserved operations are: (**sub-SG label is 15**) 1, 8, 9, 10, 17, 24, 20, 22, 18, 23, 19, 21, 25, 32, 33, 34, 41, 48, 44, 46, 42, 47, 43, 45.

$$\text{The transformation is: } (\mathbf{a}_{201}, \mathbf{b}_{201}, \mathbf{c}_{201}) = (\mathbf{a}_{224}, \mathbf{b}_{224}, \mathbf{c}_{224}) \begin{pmatrix} 0 & 0 & -1 \\ 1 & 0 & 0 \\ 0 & -1 & 0 \end{pmatrix}, \overrightarrow{O_{224}O_{201}} = \frac{1}{2}\mathbf{b}_{201} + \left(\frac{1}{2}\right)\mathbf{c}_{201}$$

The reduction of higher dimensional irrep:

$$O_h : E_g \rightarrow {}^1E_g + {}^2E_g \text{ of } T_h.$$

$$O_h : E_u \rightarrow {}^1E_u + {}^2E_u \text{ of } T_h.$$

The correspondences of irreps at HSPs from original SG to lowered SG:

$$\begin{aligned} n_{GM9}^{201} &= n_{GM11}^{224} n_{GM6}^{201} = n_{GM10}^{224} n_{GM10}^{201} = n_{GM11}^{224} n_{GM7}^{201} = n_{GM10}^{224} n_{GM8}^{201} = n_{GM8}^{224} + n_{GM9}^{224} n_{GM5}^{201} = n_{GM6}^{224} + n_{GM7}^{224} n_{X4}^{201} = \\ n_{X5}^{224} n_{X3}^{201} &= n_{X5}^{224} n_{M3}^{201} = n_{M5}^{224} n_{M4}^{201} = n_{M5}^{224} n_{R9}^{201} = n_{R11}^{224} n_{R6}^{201} = n_{R10}^{224} n_{R10}^{201} = n_{R11}^{224} n_{R7}^{201} = n_{R10}^{224} n_{R8}^{201} = n_{R8}^{224} + n_{R9}^{224} n_{R5}^{201} = \\ n_{R6}^{224} + n_{R7}^{224} \end{aligned}$$

122. Lowered SGs by higher-dimensional irreps of pairings in SG 225

The representative operations of SG/T for SG 225:

1 : (x, y, z), 2 : (x, -z, y), 3 : (x, z, -y), 4 : (z, y, -x), 5 : (-z, y, x), 6 : (-y, x, z), 7 : (y, -x, z), 8 : (x, -y, -z),  
 9 : (-x, y, -z), 10 : (-x, -y, z), 11 : (y, x, -z), 12 : (-y, -x, -z), 13 : (-x, z, y), 14 : (-x, -z, -y), 15 : (z, -y, x),  
 16 : (-z, -y, -x), 17 : (z, x, y), 18 : (y, z, x), 19 : (-y, z, -x), 20 : (-z, -x, y), 21 : (-y, -z, x), 22 : (z, -x, -y), 23 :  
 (y, -z, -x), 24 : (-z, x, -y), 25 : (-x, -y, -z), 26 : (-x, z, -y), 27 : (-x, -z, y), 28 : (-z, -y, x), 29 : (z, -y, -x),  
 30 : (y, -x, -z), 31 : (-y, x, -z), 32 : (-x, y, z), 33 : (x, -y, z), 34 : (x, y, -z), 35 : (-y, -x, z), 36 : (y, x, z),  
 37 : (x, -z, -y), 38 : (x, z, y), 39 : (-z, y, -x), 40 : (z, y, x), 41 : (-z, -x, -y), 42 : (-y, -z, -x), 43 : (y, -z, x),  
 44 : (z, x, -y), 45 : (y, z, -x), 46 : (-z, x, y), 47 : (-y, z, x), 48 : (z, -x, y).

The lower SG is SG 69 when the preserved operations are: **(sub-SG label is 1) 1, 8, 9, 10, 25, 32, 33, 34.**

The transformation is:  $(\mathbf{a}_{69}, \mathbf{b}_{69}, \mathbf{c}_{69}) = (\mathbf{a}_{225}, \mathbf{b}_{225}, \mathbf{c}_{225}) \begin{pmatrix} 0 & 0 & 1 \\ 1 & 0 & 0 \\ 0 & 1 & 0 \end{pmatrix}, \overrightarrow{O_{225}O_{69}} = \mathbf{0}$

The reduction of higher dimensional irrep:

$O_h : T_{1g} \rightarrow B_{2g} + B_{1g} + B_{3g}$  of  $D_{2h}$ .

$O_h : T_{2g} \rightarrow B_{2g} + B_{1g} + B_{3g}$  of  $D_{2h}$ .

$O_h : T_{1u} \rightarrow B_{2u} + B_{1u} + B_{3u}$  of  $D_{2h}$ .

$O_h : T_{2u} \rightarrow B_{2u} + B_{1u} + B_{3u}$  of  $D_{2h}$ .

The correspondences of irreps at HSPs from original SG to lowered SG:

$$\begin{aligned} n_{GM6}^{69} &= 2n_{GM11}^{225} + n_{GM8}^{225} + n_{GM9}^{225} & n_{GM5}^{69} &= 2n_{GM10}^{225} + n_{GM6}^{225} + n_{GM7}^{225} & n_{X6}^{69} &= n_{X8}^{225} + n_{X9}^{225} & n_{Y5}^{69} &= n_{X6}^{225} + n_{X7}^{225} & n_{L2}^{69} &= \\ n_{L6}^{225} + n_{L7}^{225} + 2n_{L9}^{225} & & n_{L3}^{69} &= n_{L4}^{225} + n_{L5}^{225} + 2n_{L8}^{225} & n_{Z6}^{69} &= n_{X8}^{225} + n_{X9}^{225} & n_{Z5}^{69} &= n_{X6}^{225} + n_{X7}^{225} & n_{T6}^{69} &= n_{X8}^{225} + n_{X9}^{225} & n_{T5}^{69} &= n_{X6}^{225} + n_{X7}^{225} \end{aligned}$$

The lower SG is SG 71 when the preserved operations are: **(sub-SG label is 2) 1, 8, 13, 14, 25, 32, 37, 38.**

The transformation is:  $(\mathbf{a}_{71}, \mathbf{b}_{71}, \mathbf{c}_{71}) = (\mathbf{a}_{225}, \mathbf{b}_{225}, \mathbf{c}_{225}) \begin{pmatrix} 0 & 0 & 1 \\ \frac{1}{2} & -\frac{1}{2} & 0 \\ \frac{1}{2} & \frac{1}{2} & 0 \end{pmatrix}, \overrightarrow{O_{225}O_{71}} = -\frac{1}{2}\mathbf{b}_{71}$

The reduction of higher dimensional irrep:

$O_h : T_{1g} \rightarrow B_{2g} + B_{1g} + B_{3g}$  of  $D_{2h}$ .

$O_h : T_{2g} \rightarrow A_g + B_{2g} + B_{3g}$  of  $D_{2h}$ .

$O_h : T_{1u} \rightarrow B_{2u} + B_{1u} + B_{3u}$  of  $D_{2h}$ .

$O_h : T_{2u} \rightarrow A_u + B_{2u} + B_{3u}$  of  $D_{2h}$ .

The correspondences of irreps at HSPs from original SG to lowered SG:

$$\begin{aligned} n_{GM6}^{71} &= 2n_{GM11}^{225} + n_{GM8}^{225} + n_{GM9}^{225} & n_{GM5}^{71} &= 2n_{GM10}^{225} + n_{GM6}^{225} + n_{GM7}^{225} & n_{X6}^{71} &= n_{X8}^{225} + n_{X9}^{225} & n_{X5}^{71} &= n_{X6}^{225} + n_{X7}^{225} & n_{T6}^{71} &= \\ n_{X6}^{225} + n_{X7}^{225} & & n_{T4}^{71} &= n_{X8}^{225} + n_{X9}^{225} & n_{T5}^{71} &= n_{X6}^{225} + n_{X7}^{225} & n_{T3}^{71} &= n_{X8}^{225} + n_{X9}^{225} & n_{W5}^{71} &= n_{W6}^{225} + n_{W7}^{225} & n_{R6}^{71} &= n_{L7}^{225} + n_{L9}^{225} & n_{R4}^{71} &= \\ n_{L5}^{225} + n_{L8}^{225} & & n_{R5}^{71} &= n_{L6}^{225} + n_{L9}^{225} & n_{R3}^{71} &= n_{L4}^{225} + n_{L8}^{225} & n_{S5}^{71} &= n_{L4}^{225} + n_{L8}^{225} & n_{S3}^{71} &= n_{L6}^{225} + n_{L9}^{225} & n_{S6}^{71} &= n_{L5}^{225} + n_{L8}^{225} & n_{S4}^{71} &= \\ n_{L7}^{225} + n_{L9}^{225} & & & & & & & & & & & & & & \end{aligned}$$

The lower SG is SG 71 when the preserved operations are: **(sub-SG label is 3) 1, 9, 16, 15, 25, 33, 40, 39.**

The transformation is:  $(\mathbf{a}_{71}, \mathbf{b}_{71}, \mathbf{c}_{71}) = (\mathbf{a}_{225}, \mathbf{b}_{225}, \mathbf{c}_{225}) \begin{pmatrix} -\frac{1}{2} & \frac{1}{2} & 0 \\ 0 & 0 & 1 \\ \frac{1}{2} & \frac{1}{2} & 0 \end{pmatrix}, \overrightarrow{O_{225}O_{71}} = -\frac{1}{2}\mathbf{b}_{71}$

The reduction of higher dimensional irrep:

$O_h : T_{1g} \rightarrow B_{2g} + B_{1g} + B_{3g}$  of  $D_{2h}$ .

$O_h : T_{2g} \rightarrow A_g + B_{2g} + B_{3g}$  of  $D_{2h}$ .

$O_h : T_{1u} \rightarrow B_{2u} + B_{1u} + B_{3u}$  of  $D_{2h}$ .

$O_h : T_{2u} \rightarrow A_u + B_{2u} + B_{3u}$  of  $D_{2h}$ .

The correspondences of irreps at HSPs from original SG to lowered SG:

$$\begin{aligned} n_{GM6}^{71} &= 2n_{GM11}^{225} + n_{GM8}^{225} + n_{GM9}^{225} & n_{GM5}^{71} &= 2n_{GM10}^{225} + n_{GM6}^{225} + n_{GM7}^{225} & n_{X6}^{71} &= n_{X8}^{225} + n_{X9}^{225} & n_{X5}^{71} &= n_{X6}^{225} + n_{X7}^{225} & n_{T6}^{71} &= \\ n_{X6}^{225} + n_{X7}^{225} & & n_{T4}^{71} &= n_{X8}^{225} + n_{X9}^{225} & n_{T5}^{71} &= n_{X6}^{225} + n_{X7}^{225} & n_{T3}^{71} &= n_{X8}^{225} + n_{X9}^{225} & n_{W5}^{71} &= n_{W6}^{225} + n_{W7}^{225} & n_{R6}^{71} &= n_{L7}^{225} + n_{L9}^{225} & n_{R4}^{71} &= \\ n_{L5}^{225} + n_{L8}^{225} & & n_{R5}^{71} &= n_{L6}^{225} + n_{L9}^{225} & n_{R3}^{71} &= n_{L4}^{225} + n_{L8}^{225} & n_{S5}^{71} &= n_{L4}^{225} + n_{L8}^{225} & n_{S3}^{71} &= n_{L6}^{225} + n_{L9}^{225} & n_{S6}^{71} &= n_{L5}^{225} + n_{L8}^{225} & n_{S4}^{71} &= \\ n_{L7}^{225} + n_{L9}^{225} & & & & & & & & & & & & & & \end{aligned}$$

The lower SG is SG 71 when the preserved operations are: **(sub-SG label is 4) 1, 10, 11, 12, 25, 34, 35, 36.**

The transformation is:  $(\mathbf{a}_{71}, \mathbf{b}_{71}, \mathbf{c}_{71}) = (\mathbf{a}_{225}, \mathbf{b}_{225}, \mathbf{c}_{225}) \begin{pmatrix} \frac{1}{2} & -\frac{1}{2} & 0 \\ \frac{1}{2} & \frac{1}{2} & 0 \\ 0 & 0 & 1 \end{pmatrix}, \overrightarrow{O_{225}O_{71}} = -\frac{1}{2}\mathbf{b}_{71}$

The reduction of higher dimensional irrep:

$$O_h : T_{1g} \rightarrow B_{2g} + B_{1g} + B_{3g} \text{ of } D_{2h}.$$

$$O_h : T_{2g} \rightarrow A_g + B_{2g} + B_{3g} \text{ of } D_{2h}.$$

$$O_h : T_{1u} \rightarrow B_{2u} + B_{1u} + B_{3u} \text{ of } D_{2h}.$$

$$O_h : T_{2u} \rightarrow A_u + B_{2u} + B_{3u} \text{ of } D_{2h}.$$

The correspondences of irreps at HSPs from original SG to lowered SG:

$$\begin{aligned} n_{GM6}^{71} &= 2n_{GM11}^{225} + n_{GM8}^{225} + n_{GM9}^{225} n_{GM5}^{71} = 2n_{GM10}^{225} + n_{GM6}^{225} + n_{GM7}^{225} n_{X6}^{71} = n_{X8}^{225} + n_{X9}^{225} n_{X5}^{71} = n_{X6}^{225} + n_{X7}^{225} n_{T6}^{71} = \\ n_{X6}^{225} + n_{X7}^{225} n_{T4}^{71} &= n_{X8}^{225} + n_{X9}^{225} n_{T5}^{71} = n_{X6}^{225} + n_{X7}^{225} n_{T3}^{71} = n_{X8}^{225} + n_{X9}^{225} n_{W5}^{71} = n_{W6}^{225} + n_{W7}^{225} n_{R6}^{71} = n_{L7}^{225} + n_{L9}^{225} n_{R4}^{71} = \\ n_{L5}^{225} + n_{L8}^{225} n_{R5}^{71} &= n_{L6}^{225} + n_{L9}^{225} n_{R3}^{71} = n_{L4}^{225} + n_{L8}^{225} n_{S5}^{71} = n_{L4}^{225} + n_{L8}^{225} n_{S3}^{71} = n_{L6}^{225} + n_{L9}^{225} n_{S6}^{71} = n_{L5}^{225} + n_{L8}^{225} n_{S4}^{71} = \\ n_{L7}^{225} + n_{L9}^{225} & \end{aligned}$$

The lower SG is SG 87 when the preserved operations are: **(sub-SG label is 5) 1, 6, 7, 10, 25, 30, 31, 34.**

The transformation is:  $(\mathbf{a}_{87}, \mathbf{b}_{87}, \mathbf{c}_{87}) = (\mathbf{a}_{225}, \mathbf{b}_{225}, \mathbf{c}_{225}) \begin{pmatrix} \frac{1}{2} & \frac{1}{2} & 0 \\ -\frac{1}{2} & \frac{1}{2} & 0 \\ 0 & 0 & 1 \end{pmatrix}, \overrightarrow{O_{225}O_{87}} = \mathbf{0}$

The reduction of higher dimensional irrep:

$$O_h : T_{1g} \rightarrow A_g + {}^2E_g + {}^1E_g \text{ of } C_{4h}.$$

$$O_h : T_{2g} \rightarrow {}^2E_g + B_g + {}^1E_g \text{ of } C_{4h}.$$

$$O_h : T_{1u} \rightarrow A_u + {}^2E_u + {}^1E_u \text{ of } C_{4h}.$$

$$O_h : T_{2u} \rightarrow {}^2E_u + B_u + {}^1E_u \text{ of } C_{4h}.$$

The correspondences of irreps at HSPs from original SG to lowered SG:

$$\begin{aligned} n_{GM9}^{87} &= n_{GM11}^{225} + n_{GM9}^{225} n_{GM5}^{87} = n_{GM10}^{225} + n_{GM7}^{225} n_{GM11}^{87} = n_{GM11}^{225} + n_{GM9}^{225} n_{GM7}^{87} = n_{GM10}^{225} + n_{GM7}^{225} n_{GM12}^{87} = \\ n_{GM11}^{225} + n_{GM8}^{225} n_{GM8}^{87} &= n_{GM10}^{225} + n_{GM6}^{225} n_{GM10}^{87} = n_{GM11}^{225} + n_{GM8}^{225} n_{GM6}^{87} = n_{GM10}^{225} + n_{GM6}^{225} n_{M9}^{87} = n_{X9}^{225} n_{M5}^{87} = n_{X7}^{225} \\ n_{M11}^{87} &= n_{X9}^{225} n_{M7}^{87} = n_{X7}^{225} n_{M12}^{87} = n_{X8}^{225} n_{M8}^{87} = n_{X6}^{225} n_{M10}^{87} = n_{X8}^{225} n_{M6}^{87} = n_{X6}^{225} n_{X6}^{87} = n_{X8}^{225} + n_{X9}^{225} n_{X4}^{87} = n_{X6}^{225} + n_{X7}^{225} \\ n_{X5}^{87} &= n_{X8}^{225} + n_{X9}^{225} n_{X3}^{87} = n_{X6}^{225} + n_{X7}^{225} n_{P7}^{87} = n_{W6}^{225} n_{P8}^{87} = n_{W7}^{225} n_{P5}^{87} = n_{W6}^{225} n_{P6}^{87} = n_{W7}^{225} n_{N2}^{87} = n_{L6}^{225} + n_{L7}^{225} + 2n_{L9}^{225} n_{N3}^{87} = \\ n_{L4}^{225} + n_{L5}^{225} + 2n_{L8}^{225} & \end{aligned}$$

The lower SG is SG 87 when the preserved operations are: **(sub-SG label is 6) 1, 2, 3, 8, 25, 26, 27, 32.**

The transformation is:  $(\mathbf{a}_{87}, \mathbf{b}_{87}, \mathbf{c}_{87}) = (\mathbf{a}_{225}, \mathbf{b}_{225}, \mathbf{c}_{225}) \begin{pmatrix} 0 & 0 & 1 \\ -\frac{1}{2} & \frac{1}{2} & 0 \\ -\frac{1}{2} & -\frac{1}{2} & 0 \end{pmatrix}, \overrightarrow{O_{225}O_{87}} = \mathbf{0}$

The reduction of higher dimensional irrep:

$$O_h : T_{1g} \rightarrow A_g + {}^2E_g + {}^1E_g \text{ of } C_{4h}.$$

$$O_h : T_{2g} \rightarrow {}^2E_g + B_g + {}^1E_g \text{ of } C_{4h}.$$

$$O_h : T_{1u} \rightarrow A_u + {}^2E_u + {}^1E_u \text{ of } C_{4h}.$$

$$O_h : T_{2u} \rightarrow {}^2E_u + B_u + {}^1E_u \text{ of } C_{4h}.$$

The correspondences of irreps at HSPs from original SG to lowered SG:

$$\begin{aligned} n_{GM9}^{87} &= n_{GM11}^{225} + n_{GM9}^{225} n_{GM5}^{87} = n_{GM10}^{225} + n_{GM7}^{225} n_{GM11}^{87} = n_{GM11}^{225} + n_{GM9}^{225} n_{GM7}^{87} = n_{GM10}^{225} + n_{GM7}^{225} n_{GM12}^{87} = \\ n_{GM11}^{225} + n_{GM8}^{225} n_{GM8}^{87} &= n_{GM10}^{225} + n_{GM6}^{225} n_{GM10}^{87} = n_{GM11}^{225} + n_{GM8}^{225} n_{GM6}^{87} = n_{GM10}^{225} + n_{GM6}^{225} n_{M9}^{87} = n_{X9}^{225} n_{M5}^{87} = n_{X7}^{225} \\ n_{M11}^{87} &= n_{X9}^{225} n_{M7}^{87} = n_{X7}^{225} n_{M12}^{87} = n_{X8}^{225} n_{M8}^{87} = n_{X6}^{225} n_{M10}^{87} = n_{X8}^{225} n_{M6}^{87} = n_{X6}^{225} n_{X6}^{87} = n_{X8}^{225} + n_{X9}^{225} n_{X4}^{87} = n_{X6}^{225} + n_{X7}^{225} \\ n_{X5}^{87} &= n_{X8}^{225} + n_{X9}^{225} n_{X3}^{87} = n_{X6}^{225} + n_{X7}^{225} n_{P7}^{87} = n_{W6}^{225} n_{P8}^{87} = n_{W7}^{225} n_{P5}^{87} = n_{W6}^{225} n_{P6}^{87} = n_{W7}^{225} n_{N2}^{87} = n_{L6}^{225} + n_{L7}^{225} + 2n_{L9}^{225} n_{N3}^{87} = \\ n_{L4}^{225} + n_{L5}^{225} + 2n_{L8}^{225} & \end{aligned}$$

The lower SG is SG 87 when the preserved operations are: **(sub-SG label is 7) 1, 4, 5, 9, 25, 28, 29, 33.**

The transformation is:  $(\mathbf{a}_{87}, \mathbf{b}_{87}, \mathbf{c}_{87}) = (\mathbf{a}_{225}, \mathbf{b}_{225}, \mathbf{c}_{225}) \begin{pmatrix} \frac{1}{2} & -\frac{1}{2} & 0 \\ 0 & 0 & 1 \\ -\frac{1}{2} & -\frac{1}{2} & 0 \end{pmatrix}, \overrightarrow{O_{225}O_{87}} = \mathbf{0}$

The reduction of higher dimensional irrep:

$$O_h : T_{1g} \rightarrow A_g + {}^2E_g + {}^1E_g \text{ of } C_{4h}.$$

$$O_h : T_{2g} \rightarrow {}^2E_g + B_g + {}^1E_g \text{ of } C_{4h}.$$

$$O_h : T_{1u} \rightarrow A_u + {}^2E_u + {}^1E_u \text{ of } C_{4h}.$$

$$O_h : T_{2u} \rightarrow {}^2E_u + B_u + {}^1E_u \text{ of } C_{4h}.$$

The correspondences of irreps at HSPs from original SG to lowered SG:

$$\begin{aligned} n_{GM9}^{87} &= n_{GM11}^{225} + n_{GM9}^{225} n_{GM5}^{87} = n_{GM10}^{225} + n_{GM7}^{225} n_{GM11}^{87} = n_{GM11}^{225} + n_{GM9}^{225} n_{GM7}^{87} = n_{GM10}^{225} + n_{GM7}^{225} n_{GM12}^{87} = \\ n_{GM11}^{225} + n_{GM8}^{225} n_{GM8}^{87} &= n_{GM10}^{225} + n_{GM6}^{225} n_{GM10}^{87} = n_{GM11}^{225} + n_{GM8}^{225} n_{GM6}^{87} = n_{GM10}^{225} + n_{GM6}^{225} n_{M9}^{87} = n_{X9}^{225} n_{M5}^{87} = n_{X7}^{225} \end{aligned}$$

$$\begin{aligned} n_{M11}^{87} &= n_{X9}^{225} n_{M7}^{87} = n_{X7}^{225} n_{M12}^{87} = n_{X8}^{225} n_{M8}^{87} = n_{X6}^{225} n_{M10}^{87} = n_{X8}^{225} n_{M6}^{87} = n_{X6}^{225} n_{X6}^{87} = n_{X8}^{225} + n_{X9}^{225} n_{X4}^{87} = n_{X6}^{225} + n_{X7}^{225} \\ n_{X5}^{87} &= n_{X8}^{225} + n_{X9}^{225} n_{X3}^{87} = n_{X6}^{225} + n_{X7}^{225} n_{P7}^{87} = n_{W6}^{225} n_{P8}^{87} = n_{W7}^{225} n_{P5}^{87} = n_{W6}^{225} n_{P6}^{87} = n_{W7}^{225} n_{N2}^{87} = n_{L6}^{225} + n_{L7}^{225} + 2n_{L9}^{225} n_{N3}^{87} = \\ n_{L4}^{225} + n_{L5}^{225} + 2n_{L8}^{225} \end{aligned}$$

The lower SG is SG 139 when the preserved operations are: (**sub-SG label is 8**) 1, 6, 7, 10, 8, 9, 11, 12, 25, 30, 31, 34, 32, 33, 35, 36.

$$\text{The transformation is: } (\mathbf{a}_{139}, \mathbf{b}_{139}, \mathbf{c}_{139}) = (\mathbf{a}_{225}, \mathbf{b}_{225}, \mathbf{c}_{225}) \begin{pmatrix} \frac{1}{2} & \frac{1}{2} & 0 \\ -\frac{1}{2} & \frac{1}{2} & 0 \\ 0 & 0 & 1 \end{pmatrix}, \overrightarrow{O_{225}O_{139}} = \mathbf{0}$$

The reduction of higher dimensional irrep:

$$O_h : E_g \rightarrow A_{1g} + B_{2g} \text{ of } D_{4h}.$$

$$O_h : E_u \rightarrow A_{1u} + B_{2u} \text{ of } D_{4h}.$$

The correspondences of irreps at HSPs from original SG to lowered SG:

$$\begin{aligned} n_{GM8}^{139} &= n_{GM11}^{225} + n_{GM9}^{225} n_{GM6}^{139} = n_{GM10}^{225} + n_{GM7}^{225} n_{GM9}^{139} = n_{GM11}^{225} + n_{GM8}^{225} n_{GM7}^{139} = n_{GM10}^{225} + n_{GM6}^{225} n_{M8}^{139} = n_{X9}^{225} n_{M6}^{139} = \\ n_{X7}^{225} n_{M9}^{139} &= n_{X8}^{225} n_{M7}^{139} = n_{X6}^{225} n_{X6}^{139} = n_{X8}^{225} + n_{X9}^{225} n_{X5}^{139} = n_{X6}^{225} + n_{X7}^{225} n_{P7}^{139} = n_{W6}^{225} n_{P6}^{139} = n_{W7}^{225} n_{N6}^{139} = n_{L7}^{225} + n_{L9}^{225} n_{N4}^{139} = \\ n_{L5}^{225} + n_{L8}^{225} n_{N5}^{139} &= n_{L6}^{225} + n_{L9}^{225} n_{N3}^{139} = n_{L4}^{225} + n_{L8}^{225} \end{aligned}$$

The lower SG is SG 139 when the preserved operations are: (**sub-SG label is 9**) 1, 2, 3, 8, 9, 10, 13, 14, 25, 26, 27, 32, 33, 34, 37, 38.

$$\text{The transformation is: } (\mathbf{a}_{139}, \mathbf{b}_{139}, \mathbf{c}_{139}) = (\mathbf{a}_{225}, \mathbf{b}_{225}, \mathbf{c}_{225}) \begin{pmatrix} 0 & 0 & 1 \\ -\frac{1}{2} & \frac{1}{2} & 0 \\ -\frac{1}{2} & -\frac{1}{2} & 0 \end{pmatrix}, \overrightarrow{O_{225}O_{139}} = \mathbf{0}$$

The reduction of higher dimensional irrep:

$$O_h : E_g \rightarrow A_{1g} + B_{2g} \text{ of } D_{4h}.$$

$$O_h : E_u \rightarrow A_{1u} + B_{2u} \text{ of } D_{4h}.$$

The correspondences of irreps at HSPs from original SG to lowered SG:

$$\begin{aligned} n_{GM8}^{139} &= n_{GM11}^{225} + n_{GM9}^{225} n_{GM6}^{139} = n_{GM10}^{225} + n_{GM7}^{225} n_{GM9}^{139} = n_{GM11}^{225} + n_{GM8}^{225} n_{GM7}^{139} = n_{GM10}^{225} + n_{GM6}^{225} n_{M8}^{139} = n_{X9}^{225} n_{M6}^{139} = \\ n_{X7}^{225} n_{M9}^{139} &= n_{X8}^{225} n_{M7}^{139} = n_{X6}^{225} n_{X6}^{139} = n_{X8}^{225} + n_{X9}^{225} n_{X5}^{139} = n_{X6}^{225} + n_{X7}^{225} n_{P7}^{139} = n_{W6}^{225} n_{P6}^{139} = n_{W7}^{225} n_{N6}^{139} = n_{L7}^{225} + n_{L9}^{225} n_{N4}^{139} = \\ n_{L5}^{225} + n_{L8}^{225} n_{N5}^{139} &= n_{L6}^{225} + n_{L9}^{225} n_{N3}^{139} = n_{L4}^{225} + n_{L8}^{225} \end{aligned}$$

The lower SG is SG 139 when the preserved operations are: (**sub-SG label is 10**) 1, 4, 5, 9, 10, 8, 16, 15, 25, 28, 29, 33, 34, 32, 40, 39.

$$\text{The transformation is: } (\mathbf{a}_{139}, \mathbf{b}_{139}, \mathbf{c}_{139}) = (\mathbf{a}_{225}, \mathbf{b}_{225}, \mathbf{c}_{225}) \begin{pmatrix} \frac{1}{2} & -\frac{1}{2} & 0 \\ 0 & 0 & 1 \\ -\frac{1}{2} & -\frac{1}{2} & 0 \end{pmatrix}, \overrightarrow{O_{225}O_{139}} = \mathbf{0}$$

The reduction of higher dimensional irrep:

$$O_h : E_g \rightarrow A_{1g} + B_{2g} \text{ of } D_{4h}.$$

$$O_h : E_u \rightarrow A_{1u} + B_{2u} \text{ of } D_{4h}.$$

The correspondences of irreps at HSPs from original SG to lowered SG:

$$\begin{aligned} n_{GM8}^{139} &= n_{GM11}^{225} + n_{GM9}^{225} n_{GM6}^{139} = n_{GM10}^{225} + n_{GM7}^{225} n_{GM9}^{139} = n_{GM11}^{225} + n_{GM8}^{225} n_{GM7}^{139} = n_{GM10}^{225} + n_{GM6}^{225} n_{M8}^{139} = n_{X9}^{225} n_{M6}^{139} = \\ n_{X7}^{225} n_{M9}^{139} &= n_{X8}^{225} n_{M7}^{139} = n_{X6}^{225} n_{X6}^{139} = n_{X8}^{225} + n_{X9}^{225} n_{X5}^{139} = n_{X6}^{225} + n_{X7}^{225} n_{P7}^{139} = n_{W6}^{225} n_{P6}^{139} = n_{W7}^{225} n_{N6}^{139} = n_{L7}^{225} + n_{L9}^{225} n_{N4}^{139} = \\ n_{L5}^{225} + n_{L8}^{225} n_{N5}^{139} &= n_{L6}^{225} + n_{L9}^{225} n_{N3}^{139} = n_{L4}^{225} + n_{L8}^{225} \end{aligned}$$

The lower SG is SG 148 when the preserved operations are: (**sub-SG label is 11**) 1, 17, 18, 25, 41, 42.

$$\text{The transformation is: } (\mathbf{a}_{148}, \mathbf{b}_{148}, \mathbf{c}_{148}) = (\mathbf{a}_{225}, \mathbf{b}_{225}, \mathbf{c}_{225}) \begin{pmatrix} \frac{1}{2} & 0 & \frac{1}{2} \\ \frac{1}{2} & \frac{1}{2} & 0 \\ \frac{1}{2} & \frac{1}{2} & 0 \\ 0 & \frac{1}{2} & \frac{1}{2} \end{pmatrix}, \overrightarrow{O_{225}O_{148}} = \mathbf{0}$$

The reduction of higher dimensional irrep:

$$O_h : T_{1g} \rightarrow A_g + {}^2E_g + {}^1E_g \text{ of } C_{3i}.$$

$$O_h : T_{2g} \rightarrow A_g + {}^2E_g + {}^1E_g \text{ of } C_{3i}.$$

$$O_h : T_{1u} \rightarrow {}^1E_u + A_u + {}^2E_u \text{ of } C_{3i}.$$

$$O_h : T_{2u} \rightarrow {}^1E_u + A_u + {}^2E_u \text{ of } C_{3i}.$$

The correspondences of irreps at HSPs from original SG to lowered SG:

$$\begin{aligned} n_{GM7}^{148} &= 2n_{GM11}^{225} n_{GM4}^{148} = 2n_{GM10}^{225} n_{GM9}^{148} = n_{GM11}^{225} + n_{GM8}^{225} + n_{GM9}^{225} n_{GM6}^{148} = n_{GM10}^{225} + n_{GM6}^{225} + n_{GM7}^{225} n_{GM8}^{148} = \\ n_{GM11}^{225} + n_{GM8}^{225} + n_{GM9}^{225} n_{GM5}^{148} &= n_{GM10}^{225} + n_{GM6}^{225} + n_{GM7}^{225} n_{L2}^{148} = n_{L6}^{225} + n_{L7}^{225} + 2n_{L9}^{225} n_{L3}^{148} = n_{L4}^{225} + n_{L5}^{225} + 2n_{L8}^{225} n_{F2}^{148} = \\ 2n_{X8}^{225} + 2n_{X9}^{225} n_{F3}^{148} &= 2n_{X6}^{225} + 2n_{X7}^{225} n_{T7}^{148} = n_{L6}^{225} + n_{L7}^{225} n_{T4}^{148} = n_{L4}^{225} + n_{L5}^{225} n_{T9}^{148} = n_{L9}^{225} n_{T6}^{148} = n_{L8}^{225} n_{T8}^{148} = n_{L9}^{225} n_{T5}^{148} = \\ n_{L8}^{225} \end{aligned}$$

The lower SG is SG 148 when the preserved operations are: **(sub-SG label is 12)** 1, 24, 23, 25, 48, 47.

$$\text{The transformation is: } (\mathbf{a}_{148}, \mathbf{b}_{148}, \mathbf{c}_{148}) = (\mathbf{a}_{225}, \mathbf{b}_{225}, \mathbf{c}_{225}) \begin{pmatrix} -\frac{1}{2} & -\frac{1}{2} & 0 \\ 0 & -\frac{1}{2} & -\frac{1}{2} \\ \frac{1}{2} & 0 & \frac{1}{2} \end{pmatrix}, \overrightarrow{O_{225}O_{148}} = \mathbf{0}$$

The reduction of higher dimensional irrep:

$$O_h : T_{1g} \rightarrow A_g + {}^2E_g + {}^1E_g \text{ of } C_{3i}.$$

$$O_h : T_{2g} \rightarrow A_g + {}^2E_g + {}^1E_g \text{ of } C_{3i}.$$

$$O_h : T_{1u} \rightarrow {}^1E_u + A_u + {}^2E_u \text{ of } C_{3i}.$$

$$O_h : T_{2u} \rightarrow {}^1E_u + A_u + {}^2E_u \text{ of } C_{3i}.$$

The correspondences of irreps at HSPs from original SG to lowered SG:

$$\begin{aligned} n_{GM7}^{148} &= 2n_{GM11}^{225} n_{GM4}^{148} = 2n_{GM10}^{225} n_{GM9}^{148} = n_{GM11}^{225} + n_{GM8}^{225} + n_{GM9}^{225} n_{GM6}^{148} = n_{GM10}^{225} + n_{GM6}^{225} + n_{GM7}^{225} n_{GM8}^{148} = \\ n_{GM11}^{225} + n_{GM8}^{225} + n_{GM9}^{225} n_{GM5}^{148} &= n_{GM10}^{225} + n_{GM6}^{225} + n_{GM7}^{225} n_{L2}^{148} = n_{L6}^{225} + n_{L7}^{225} + 2n_{L9}^{225} n_{L3}^{148} = n_{L4}^{225} + n_{L5}^{225} + 2n_{L8}^{225} n_{F2}^{148} = \\ 2n_{X8}^{225} + 2n_{X9}^{225} n_{F3}^{148} &= 2n_{X6}^{225} + 2n_{X7}^{225} n_{T7}^{148} = n_{L6}^{225} + n_{L7}^{225} n_{T4}^{148} = n_{L4}^{225} + n_{L5}^{225} n_{T9}^{148} = n_{L9}^{225} n_{T6}^{148} = n_{L8}^{225} n_{T8}^{148} = n_{L9}^{225} n_{T5}^{148} = \\ n_{L8}^{225} \end{aligned}$$

The lower SG is SG 148 when the preserved operations are: **(sub-SG label is 13)** 1, 20, 19, 25, 44, 43.

$$\text{The transformation is: } (\mathbf{a}_{148}, \mathbf{b}_{148}, \mathbf{c}_{148}) = (\mathbf{a}_{225}, \mathbf{b}_{225}, \mathbf{c}_{225}) \begin{pmatrix} \frac{1}{2} & 0 & \frac{1}{2} \\ -\frac{1}{2} & -\frac{1}{2} & 0 \\ 0 & -\frac{1}{2} & -\frac{1}{2} \end{pmatrix}, \overrightarrow{O_{225}O_{148}} = \mathbf{0}$$

The reduction of higher dimensional irrep:

$$O_h : T_{1g} \rightarrow A_g + {}^2E_g + {}^1E_g \text{ of } C_{3i}.$$

$$O_h : T_{2g} \rightarrow A_g + {}^2E_g + {}^1E_g \text{ of } C_{3i}.$$

$$O_h : T_{1u} \rightarrow {}^1E_u + A_u + {}^2E_u \text{ of } C_{3i}.$$

$$O_h : T_{2u} \rightarrow {}^1E_u + A_u + {}^2E_u \text{ of } C_{3i}.$$

The correspondences of irreps at HSPs from original SG to lowered SG:

$$\begin{aligned} n_{GM7}^{148} &= 2n_{GM11}^{225} n_{GM4}^{148} = 2n_{GM10}^{225} n_{GM9}^{148} = n_{GM11}^{225} + n_{GM8}^{225} + n_{GM9}^{225} n_{GM6}^{148} = n_{GM10}^{225} + n_{GM6}^{225} + n_{GM7}^{225} n_{GM8}^{148} = \\ n_{GM11}^{225} + n_{GM8}^{225} + n_{GM9}^{225} n_{GM5}^{148} &= n_{GM10}^{225} + n_{GM6}^{225} + n_{GM7}^{225} n_{L2}^{148} = n_{L6}^{225} + n_{L7}^{225} + 2n_{L9}^{225} n_{L3}^{148} = n_{L4}^{225} + n_{L5}^{225} + 2n_{L8}^{225} n_{F2}^{148} = \\ 2n_{X8}^{225} + 2n_{X9}^{225} n_{F3}^{148} &= 2n_{X6}^{225} + 2n_{X7}^{225} n_{T7}^{148} = n_{L6}^{225} + n_{L7}^{225} n_{T4}^{148} = n_{L4}^{225} + n_{L5}^{225} n_{T9}^{148} = n_{L9}^{225} n_{T6}^{148} = n_{L8}^{225} n_{T8}^{148} = n_{L9}^{225} n_{T5}^{148} = \\ n_{L8}^{225} \end{aligned}$$

The lower SG is SG 148 when the preserved operations are: **(sub-SG label is 14)** 1, 22, 21, 25, 46, 45.

$$\text{The transformation is: } (\mathbf{a}_{148}, \mathbf{b}_{148}, \mathbf{c}_{148}) = (\mathbf{a}_{225}, \mathbf{b}_{225}, \mathbf{c}_{225}) \begin{pmatrix} -\frac{1}{2} & -\frac{1}{2} & 0 \\ 0 & \frac{1}{2} & \frac{1}{2} \\ -\frac{1}{2} & 0 & -\frac{1}{2} \end{pmatrix}, \overrightarrow{O_{225}O_{148}} = \mathbf{0}$$

The reduction of higher dimensional irrep:

$$O_h : T_{1g} \rightarrow A_g + {}^2E_g + {}^1E_g \text{ of } C_{3i}.$$

$$O_h : T_{2g} \rightarrow A_g + {}^2E_g + {}^1E_g \text{ of } C_{3i}.$$

$$O_h : T_{1u} \rightarrow {}^1E_u + A_u + {}^2E_u \text{ of } C_{3i}.$$

$$O_h : T_{2u} \rightarrow {}^1E_u + A_u + {}^2E_u \text{ of } C_{3i}.$$

The correspondences of irreps at HSPs from original SG to lowered SG:

$$\begin{aligned} n_{GM7}^{148} &= 2n_{GM11}^{225} n_{GM4}^{148} = 2n_{GM10}^{225} n_{GM9}^{148} = n_{GM11}^{225} + n_{GM8}^{225} + n_{GM9}^{225} n_{GM6}^{148} = n_{GM10}^{225} + n_{GM6}^{225} + n_{GM7}^{225} n_{GM8}^{148} = \\ n_{GM11}^{225} + n_{GM8}^{225} + n_{GM9}^{225} n_{GM5}^{148} &= n_{GM10}^{225} + n_{GM6}^{225} + n_{GM7}^{225} n_{L2}^{148} = n_{L6}^{225} + n_{L7}^{225} + 2n_{L9}^{225} n_{L3}^{148} = n_{L4}^{225} + n_{L5}^{225} + 2n_{L8}^{225} n_{F2}^{148} = \\ 2n_{X8}^{225} + 2n_{X9}^{225} n_{F3}^{148} &= 2n_{X6}^{225} + 2n_{X7}^{225} n_{T7}^{148} = n_{L6}^{225} + n_{L7}^{225} n_{T4}^{148} = n_{L4}^{225} + n_{L5}^{225} n_{T9}^{148} = n_{L9}^{225} n_{T6}^{148} = n_{L8}^{225} n_{T8}^{148} = n_{L9}^{225} n_{T5}^{148} = \\ n_{L8}^{225} \end{aligned}$$

The lower SG is SG 202 when the preserved operations are: **(sub-SG label is 15)** 1, 8, 9, 10, 17, 24, 20, 22, 18, 23, 19, 21, 25, 32, 33, 34, 41, 48, 44, 46, 42, 47, 43, 45.

$$\text{The transformation is: } (\mathbf{a}_{202}, \mathbf{b}_{202}, \mathbf{c}_{202}) = (\mathbf{a}_{225}, \mathbf{b}_{225}, \mathbf{c}_{225}) \begin{pmatrix} 0 & 0 & 1 \\ 1 & 0 & 0 \\ 0 & 1 & 0 \end{pmatrix}, \overrightarrow{O_{225}O_{202}} = \mathbf{0}$$

The reduction of higher dimensional irrep:

$$O_h : E_g \rightarrow {}^1E_g + {}^2E_g \text{ of } T_h.$$

$$O_h : E_u \rightarrow {}^1E_u + {}^2E_u \text{ of } T_h.$$

The correspondences of irreps at HSPs from original SG to lowered SG:

$$\begin{aligned} n_{GM9}^{202} &= n_{GM11}^{225} n_{GM6}^{202} = n_{GM10}^{225} n_{GM10}^{202} = n_{GM11}^{225} n_{GM7}^{202} = n_{GM10}^{225} n_{GM8}^{202} = n_{GM8}^{225} + n_{GM9}^{225} n_{GM5}^{202} = n_{GM6}^{225} + n_{GM7}^{225} n_{X6}^{202} = \\ n_{GM11}^{225} + n_{GM8}^{225} + n_{GM9}^{225} n_{X5}^{202} &= n_{GM10}^{225} + n_{GM7}^{225} n_{L7}^{202} = n_{L6}^{225} + n_{L7}^{225} n_{L4}^{202} = n_{L4}^{225} + n_{L5}^{225} n_{L9}^{202} = n_{L9}^{225} n_{L6}^{202} = n_{L8}^{225} n_{L8}^{202} = n_{L9}^{225} n_{L5}^{202} = n_{L8}^{225} n_{L5}^{202} = \\ n_{W5}^{202} &= n_{W6}^{225} + n_{W7}^{225} \end{aligned}$$

123. Lowered SGs by higher-dimensional irreps of pairings in SG 226

The representative operations of SG/T for SG 226:

$$\begin{aligned}
 &1 : (x, y, z), 2 : (x + \frac{1}{2}, \frac{1}{2} - z, y + \frac{1}{2}), 3 : (x + \frac{1}{2}, z + \frac{1}{2}, \frac{1}{2} - y), 4 : (z + \frac{1}{2}, y + \frac{1}{2}, \frac{1}{2} - x), 5 : (\frac{1}{2} - z, y + \frac{1}{2}, x + \frac{1}{2}), \\
 &6 : (\frac{1}{2} - y, x + \frac{1}{2}, z + \frac{1}{2}), 7 : (y + \frac{1}{2}, \frac{1}{2} - x, z + \frac{1}{2}), 8 : (x, -y, -z), 9 : (-x, y, -z), 10 : (-x, -y, z), 11 : (y + \frac{1}{2}, x + \frac{1}{2}, \frac{1}{2} - z), \\
 &12 : (\frac{1}{2} - y, \frac{1}{2} - x, \frac{1}{2} - z), 13 : (\frac{1}{2} - x, z + \frac{1}{2}, y + \frac{1}{2}), 14 : (\frac{1}{2} - x, \frac{1}{2} - z, \frac{1}{2} - y), 15 : (z + \frac{1}{2}, \frac{1}{2} - y, x + \frac{1}{2}), 16 : (\frac{1}{2} - z, \frac{1}{2} - y, \frac{1}{2} - x), \\
 &17 : (z, x, y), 18 : (y, z, x), 19 : (-y, z, -x), 20 : (-z, -x, y), 21 : (-y, -z, x), 22 : (z, -x, -y), 23 : (y, -z, -x), \\
 &24 : (-z, x, -y), 25 : (-x, -y, -z), 26 : (\frac{1}{2} - x, z + \frac{1}{2}, \frac{1}{2} - y), 27 : (\frac{1}{2} - x, \frac{1}{2} - z, y + \frac{1}{2}), 28 : (\frac{1}{2} - z, \frac{1}{2} - y, x + \frac{1}{2}), \\
 &29 : (z + \frac{1}{2}, \frac{1}{2} - y, \frac{1}{2} - x), 30 : (y + \frac{1}{2}, \frac{1}{2} - x, \frac{1}{2} - z), 31 : (\frac{1}{2} - y, x + \frac{1}{2}, \frac{1}{2} - z), 32 : (-x, y, z), 33 : (x, -y, z), \\
 &34 : (x, y, -z), 35 : (\frac{1}{2} - y, \frac{1}{2} - x, z + \frac{1}{2}), 36 : (y + \frac{1}{2}, x + \frac{1}{2}, z + \frac{1}{2}), 37 : (x + \frac{1}{2}, \frac{1}{2} - z, \frac{1}{2} - y), 38 : (x + \frac{1}{2}, z + \frac{1}{2}, y + \frac{1}{2}), \\
 &39 : (\frac{1}{2} - z, y + \frac{1}{2}, \frac{1}{2} - x), 40 : (z + \frac{1}{2}, y + \frac{1}{2}, x + \frac{1}{2}), 41 : (-z, -x, -y), 42 : (-y, -z, -x), 43 : (y, -z, x), 44 : (z, x, -y), \\
 &45 : (y, z, -x), 46 : (-z, x, y), 47 : (-y, z, x), 48 : (z, -x, y).
 \end{aligned}$$

The lower SG is SG 69 when the preserved operations are: (sub-SG label is 1) 1, 8, 9, 10, 25, 32, 33, 34.

The transformation is:  $(\mathbf{a}_{69}, \mathbf{b}_{69}, \mathbf{c}_{69}) = (\mathbf{a}_{226}, \mathbf{b}_{226}, \mathbf{c}_{226}) \begin{pmatrix} 0 & 0 & 1 \\ 1 & 0 & 0 \\ 0 & 1 & 0 \end{pmatrix}, \overrightarrow{O_{226}O_{69}} = \mathbf{0}$

The reduction of higher dimensional irrep:

$$\begin{aligned}
 O_h : T_{1g} &\rightarrow B_{2g} + B_{1g} + B_{3g} \text{ of } D_{2h}. \\
 O_h : T_{2g} &\rightarrow B_{2g} + B_{1g} + B_{3g} \text{ of } D_{2h}. \\
 O_h : T_{1u} &\rightarrow B_{2u} + B_{1u} + B_{3u} \text{ of } D_{2h}. \\
 O_h : T_{2u} &\rightarrow B_{2u} + B_{1u} + B_{3u} \text{ of } D_{2h}.
 \end{aligned}$$

The correspondences of irreps at HSPs from original SG to lowered SG:

$$\begin{aligned}
 n_{GM6}^{69} &= 2n_{GM11}^{226} + n_{GM8}^{226} + n_{GM9}^{226} \quad n_{GM5}^{69} = 2n_{GM10}^{226} + n_{GM6}^{226} + n_{GM7}^{226} \quad n_{Y6}^{69} = n_{X8}^{226} + n_{X9}^{226} \quad n_{Y5}^{69} = n_{X6}^{226} + n_{X7}^{226} \quad n_{L2}^{69} = \\
 n_{L4}^{226} + n_{L5}^{226} + n_{L6}^{226} \quad n_{L3}^{69} &= n_{L4}^{226} + n_{L5}^{226} + n_{L6}^{226} \quad n_{Z6}^{69} = n_{X8}^{226} + n_{X9}^{226} \quad n_{Z5}^{69} = n_{X6}^{226} + n_{X7}^{226} \quad n_{T6}^{69} = n_{X8}^{226} + n_{X9}^{226} \quad n_{T5}^{69} = n_{X6}^{226} + n_{X7}^{226}
 \end{aligned}$$

The lower SG is SG 72 when the preserved operations are: (sub-SG label is 2) 1, 8, 13, 14, 25, 32, 37, 38.

The transformation is:  $(\mathbf{a}_{72}, \mathbf{b}_{72}, \mathbf{c}_{72}) = (\mathbf{a}_{226}, \mathbf{b}_{226}, \mathbf{c}_{226}) \begin{pmatrix} 0 & 0 & 1 \\ \frac{1}{2} & -\frac{1}{2} & 0 \\ \frac{1}{2} & \frac{1}{2} & 0 \end{pmatrix}, \overrightarrow{O_{226}O_{72}} = -\frac{1}{2}\mathbf{b}_{72}$

The reduction of higher dimensional irrep:

$$\begin{aligned}
 O_h : T_{1g} &\rightarrow B_{2g} + B_{1g} + B_{3g} \text{ of } D_{2h}. \\
 O_h : T_{2g} &\rightarrow A_g + B_{2g} + B_{3g} \text{ of } D_{2h}. \\
 O_h : T_{1u} &\rightarrow B_{2u} + B_{1u} + B_{3u} \text{ of } D_{2h}. \\
 O_h : T_{2u} &\rightarrow A_u + B_{2u} + B_{3u} \text{ of } D_{2h}.
 \end{aligned}$$

The correspondences of irreps at HSPs from original SG to lowered SG:

$$\begin{aligned}
 n_{GM6}^{72} &= 2n_{GM11}^{226} + n_{GM8}^{226} + n_{GM9}^{226} \quad n_{GM5}^{72} = 2n_{GM10}^{226} + n_{GM6}^{226} + n_{GM7}^{226} \quad n_{X6}^{72} = n_{X8}^{226} + n_{X9}^{226} \quad n_{X5}^{72} = n_{X6}^{226} + n_{X7}^{226} \quad n_{T6}^{72} = \\
 n_{X6}^{226} + n_{X7}^{226} \quad n_{T4}^{72} &= n_{X8}^{226} + n_{X9}^{226} \quad n_{T5}^{72} = n_{X6}^{226} + n_{X7}^{226} \quad n_{T3}^{72} = n_{X8}^{226} + n_{X9}^{226} \quad n_{W5}^{72} = n_{W6}^{226} + n_{W7}^{226} \quad n_{R2}^{72} = n_{L4}^{226} + n_{L5}^{226} + n_{L6}^{226} \quad n_{S2}^{72} = \\
 n_{L4}^{226} + n_{L5}^{226} + n_{L6}^{226}
 \end{aligned}$$

The lower SG is SG 72 when the preserved operations are: (sub-SG label is 3) 1, 9, 16, 15, 25, 33, 40, 39.

The transformation is:  $(\mathbf{a}_{72}, \mathbf{b}_{72}, \mathbf{c}_{72}) = (\mathbf{a}_{226}, \mathbf{b}_{226}, \mathbf{c}_{226}) \begin{pmatrix} -\frac{1}{2} & \frac{1}{2} & 0 \\ 0 & 0 & 1 \\ \frac{1}{2} & \frac{1}{2} & 0 \end{pmatrix}, \overrightarrow{O_{226}O_{72}} = -\frac{1}{2}\mathbf{b}_{72}$

The reduction of higher dimensional irrep:

$$\begin{aligned}
 O_h : T_{1g} &\rightarrow B_{2g} + B_{1g} + B_{3g} \text{ of } D_{2h}. \\
 O_h : T_{2g} &\rightarrow A_g + B_{2g} + B_{3g} \text{ of } D_{2h}. \\
 O_h : T_{1u} &\rightarrow B_{2u} + B_{1u} + B_{3u} \text{ of } D_{2h}. \\
 O_h : T_{2u} &\rightarrow A_u + B_{2u} + B_{3u} \text{ of } D_{2h}.
 \end{aligned}$$

The correspondences of irreps at HSPs from original SG to lowered SG:

$$n_{GM6}^{72} = 2n_{GM11}^{226} + n_{GM8}^{226} + n_{GM9}^{226} \quad n_{GM5}^{72} = 2n_{GM10}^{226} + n_{GM6}^{226} + n_{GM7}^{226} \quad n_{X6}^{72} = n_{X8}^{226} + n_{X9}^{226} \quad n_{X5}^{72} = n_{X6}^{226} + n_{X7}^{226} \quad n_{T6}^{72} =$$

$$n_{X6}^{226} + n_{X7}^{226} n_{T4}^{72} = n_{X8}^{226} + n_{X9}^{226} n_{T5}^{72} = n_{X6}^{226} + n_{X7}^{226} n_{T3}^{72} = n_{X8}^{226} + n_{X9}^{226} n_{W5}^{72} = n_{W6}^{226} + n_{W7}^{226} n_{R2}^{72} = n_{L4}^{226} + n_{L5}^{226} + n_{L6}^{226} n_{S2}^{72} =$$

The lower SG is SG 72 when the preserved operations are: **(sub-SG label is 4) 1, 10, 11, 12, 25, 34, 35, 36.**

$$\text{The transformation is: } (\mathbf{a}_{72}, \mathbf{b}_{72}, \mathbf{c}_{72}) = (\mathbf{a}_{226}, \mathbf{b}_{226}, \mathbf{c}_{226}) \begin{pmatrix} \frac{1}{2} & -\frac{1}{2} & 0 \\ \frac{1}{2} & \frac{1}{2} & 0 \\ 0 & 0 & 1 \end{pmatrix}, \overrightarrow{O_{226}O_{72}} = -\frac{1}{2}\mathbf{b}_{72}$$

The reduction of higher dimensional irrep:

$$O_h : T_{1g} \rightarrow B_{2g} + B_{1g} + B_{3g} \text{ of } D_{2h}.$$

$$O_h : T_{2g} \rightarrow A_g + B_{2g} + B_{3g} \text{ of } D_{2h}.$$

$$O_h : T_{1u} \rightarrow B_{2u} + B_{1u} + B_{3u} \text{ of } D_{2h}.$$

$$O_h : T_{2u} \rightarrow A_u + B_{2u} + B_{3u} \text{ of } D_{2h}.$$

The correspondences of irreps at HSPs from original SG to lowered SG:

$$n_{GM6}^{72} = 2n_{GM11}^{226} + n_{GM8}^{226} + n_{GM9}^{226} n_{GM5}^{72} = 2n_{GM10}^{226} + n_{GM6}^{226} + n_{GM7}^{226} n_{X6}^{72} = n_{X8}^{226} + n_{X9}^{226} n_{X5}^{72} = n_{X6}^{226} + n_{X7}^{226} n_{T6}^{72} =$$

$$n_{X6}^{226} + n_{X7}^{226} n_{T4}^{72} = n_{X8}^{226} + n_{X9}^{226} n_{T5}^{72} = n_{X6}^{226} + n_{X7}^{226} n_{T3}^{72} = n_{X8}^{226} + n_{X9}^{226} n_{W5}^{72} = n_{W6}^{226} + n_{W7}^{226} n_{R2}^{72} = n_{L4}^{226} + n_{L5}^{226} + n_{L6}^{226} n_{S2}^{72} =$$

$$n_{L4}^{226} + n_{L5}^{226} + n_{L6}^{226}$$

The lower SG is SG 87 when the preserved operations are: **(sub-SG label is 5) 1, 6, 7, 10, 25, 30, 31, 34.**

$$\text{The transformation is: } (\mathbf{a}_{87}, \mathbf{b}_{87}, \mathbf{c}_{87}) = (\mathbf{a}_{226}, \mathbf{b}_{226}, \mathbf{c}_{226}) \begin{pmatrix} \frac{1}{2} & \frac{1}{2} & 0 \\ -\frac{1}{2} & \frac{1}{2} & 0 \\ 0 & 0 & 1 \end{pmatrix}, \overrightarrow{O_{226}O_{87}} = \frac{1}{2}\mathbf{a}_{87}$$

The reduction of higher dimensional irrep:

$$O_h : T_{1g} \rightarrow A_g + {}^2E_g + {}^1E_g \text{ of } C_{4h}.$$

$$O_h : T_{2g} \rightarrow {}^2E_g + B_g + {}^1E_g \text{ of } C_{4h}.$$

$$O_h : T_{1u} \rightarrow A_u + {}^2E_u + {}^1E_u \text{ of } C_{4h}.$$

$$O_h : T_{2u} \rightarrow {}^2E_u + B_u + {}^1E_u \text{ of } C_{4h}.$$

The correspondences of irreps at HSPs from original SG to lowered SG:

$$n_{GM9}^{87} = n_{GM11}^{226} + n_{GM9}^{226} n_{GM5}^{87} = n_{GM10}^{226} + n_{GM7}^{226} n_{GM11}^{87} = n_{GM11}^{226} + n_{GM9}^{226} n_{GM7}^{87} = n_{GM10}^{226} + n_{GM7}^{226} n_{GM12}^{87} =$$

$$n_{GM11}^{226} + n_{GM8}^{226} n_{GM8}^{87} = n_{GM10}^{226} + n_{GM6}^{226} n_{GM10}^{87} = n_{GM11}^{226} + n_{GM8}^{226} n_{GM6}^{87} = n_{GM10}^{226} + n_{GM6}^{226} n_{M9}^{87} = n_{X8}^{226} n_{M5}^{87} = n_{X6}^{226}$$

$$n_{M11}^{87} = n_{X8}^{226} n_{M7}^{87} = n_{X6}^{226} n_{M12}^{87} = n_{X9}^{226} n_{M8}^{87} = n_{X7}^{226} n_{M10}^{87} = n_{X9}^{226} n_{M6}^{87} = n_{X7}^{226} n_{X6}^{87} = n_{X6}^{226} + n_{X7}^{226} n_{X4}^{87} = n_{X8}^{226} + n_{X9}^{226}$$

$$n_{X5}^{87} = n_{X6}^{226} + n_{X7}^{226} n_{X3}^{87} = n_{X8}^{226} + n_{X9}^{226} n_{P7}^{87} = n_{W7}^{226} n_{P8}^{87} = n_{W6}^{226} n_{P5}^{87} = n_{W6}^{226} n_{P6}^{87} = n_{W7}^{226} n_{N2}^{87} = n_{L4}^{226} + n_{L5}^{226} + n_{L6}^{226} n_{N3}^{87} =$$

$$n_{L4}^{226} + n_{L5}^{226} + n_{L6}^{226}$$

The lower SG is SG 87 when the preserved operations are: **(sub-SG label is 6) 1, 2, 3, 8, 25, 26, 27, 32.**

$$\text{The transformation is: } (\mathbf{a}_{87}, \mathbf{b}_{87}, \mathbf{c}_{87}) = (\mathbf{a}_{226}, \mathbf{b}_{226}, \mathbf{c}_{226}) \begin{pmatrix} 0 & 0 & 1 \\ -\frac{1}{2} & \frac{1}{2} & 0 \\ -\frac{1}{2} & -\frac{1}{2} & 0 \end{pmatrix}, \overrightarrow{O_{226}O_{87}} = \frac{1}{2}\mathbf{a}_{87}$$

The reduction of higher dimensional irrep:

$$O_h : T_{1g} \rightarrow A_g + {}^2E_g + {}^1E_g \text{ of } C_{4h}.$$

$$O_h : T_{2g} \rightarrow {}^2E_g + B_g + {}^1E_g \text{ of } C_{4h}.$$

$$O_h : T_{1u} \rightarrow A_u + {}^2E_u + {}^1E_u \text{ of } C_{4h}.$$

$$O_h : T_{2u} \rightarrow {}^2E_u + B_u + {}^1E_u \text{ of } C_{4h}.$$

The correspondences of irreps at HSPs from original SG to lowered SG:

$$n_{GM9}^{87} = n_{GM11}^{226} + n_{GM9}^{226} n_{GM5}^{87} = n_{GM10}^{226} + n_{GM7}^{226} n_{GM11}^{87} = n_{GM11}^{226} + n_{GM9}^{226} n_{GM7}^{87} = n_{GM10}^{226} + n_{GM7}^{226} n_{GM12}^{87} =$$

$$n_{GM11}^{226} + n_{GM8}^{226} n_{GM8}^{87} = n_{GM10}^{226} + n_{GM6}^{226} n_{GM10}^{87} = n_{GM11}^{226} + n_{GM8}^{226} n_{GM6}^{87} = n_{GM10}^{226} + n_{GM6}^{226} n_{M9}^{87} = n_{X8}^{226} n_{M5}^{87} = n_{X6}^{226}$$

$$n_{M11}^{87} = n_{X8}^{226} n_{M7}^{87} = n_{X6}^{226} n_{M12}^{87} = n_{X9}^{226} n_{M8}^{87} = n_{X7}^{226} n_{M10}^{87} = n_{X9}^{226} n_{M6}^{87} = n_{X7}^{226} n_{X6}^{87} = n_{X6}^{226} + n_{X7}^{226} n_{X4}^{87} = n_{X8}^{226} + n_{X9}^{226}$$

$$n_{X5}^{87} = n_{X6}^{226} + n_{X7}^{226} n_{X3}^{87} = n_{X8}^{226} + n_{X9}^{226} n_{P7}^{87} = n_{W6}^{226} n_{P8}^{87} = n_{W7}^{226} n_{P5}^{87} = n_{W7}^{226} n_{P6}^{87} = n_{W6}^{226} n_{N2}^{87} = n_{L4}^{226} + n_{L5}^{226} + n_{L6}^{226} n_{N3}^{87} =$$

$$n_{L4}^{226} + n_{L5}^{226} + n_{L6}^{226}$$

The lower SG is SG 87 when the preserved operations are: **(sub-SG label is 7) 1, 4, 5, 9, 25, 28, 29, 33.**

$$\text{The transformation is: } (\mathbf{a}_{87}, \mathbf{b}_{87}, \mathbf{c}_{87}) = (\mathbf{a}_{226}, \mathbf{b}_{226}, \mathbf{c}_{226}) \begin{pmatrix} \frac{1}{2} & -\frac{1}{2} & 0 \\ 0 & 0 & 1 \\ -\frac{1}{2} & -\frac{1}{2} & 0 \end{pmatrix}, \overrightarrow{O_{226}O_{87}} = \frac{1}{2}\mathbf{a}_{87}$$

The reduction of higher dimensional irrep:

$$O_h : T_{1g} \rightarrow A_g + {}^2E_g + {}^1E_g \text{ of } C_{4h}.$$

$$O_h : T_{2g} \rightarrow {}^2E_g + B_g + {}^1E_g \text{ of } C_{4h}.$$

$$O_h : T_{1u} \rightarrow A_u + {}^2E_u + {}^1E_u \text{ of } C_{4h}.$$

$$O_h : T_{2u} \rightarrow {}^2E_u + B_u + {}^1E_u \text{ of } C_{4h}.$$

The correspondences of irreps at HSPs from original SG to lowered SG:

$$\begin{aligned}
 n_{GM9}^{87} &= n_{GM11}^{226} + n_{GM9}^{226} & n_{GM5}^{87} &= n_{GM10}^{226} + n_{GM7}^{226} & n_{GM11}^{87} &= n_{GM11}^{226} + n_{GM9}^{226} & n_{GM7}^{87} &= n_{GM10}^{226} + n_{GM7}^{226} & n_{GM12}^{87} &= n_{GM11}^{226} + n_{GM8}^{226} & n_{GM12}^{87} &= n_{GM11}^{226} + n_{GM8}^{226} \\
 n_{GM11}^{226} + n_{GM8}^{226} & & n_{GM8}^{87} &= n_{GM10}^{226} + n_{GM6}^{226} & n_{GM10}^{87} &= n_{GM11}^{226} + n_{GM8}^{226} & n_{GM6}^{87} &= n_{GM10}^{226} + n_{GM6}^{226} & n_{M9}^{87} &= n_{X8}^{226} & n_{M5}^{87} &= n_{X6}^{226} \\
 n_{M11}^{87} &= n_{X8}^{226} & n_{M7}^{87} &= n_{X6}^{226} & n_{M12}^{87} &= n_{X9}^{226} & n_{M8}^{87} &= n_{X7}^{226} & n_{M10}^{87} &= n_{X9}^{226} & n_{M6}^{87} &= n_{X7}^{226} & n_{X6}^{87} &= n_{X8}^{226} + n_{X9}^{226} \\
 n_{X5}^{87} &= n_{X6}^{226} + n_{X7}^{226} & n_{X3}^{87} &= n_{X8}^{226} + n_{X9}^{226} & n_{P7}^{87} &= n_{W7}^{226} & n_{P8}^{87} &= n_{W6}^{226} & n_{P5}^{87} &= n_{W6}^{226} & n_{P6}^{87} &= n_{W7}^{226} & n_{N2}^{87} &= n_{L4}^{226} + n_{L5}^{226} + n_{L6}^{226} & n_{N3}^{87} &= n_{L4}^{226} + n_{L5}^{226} + n_{L6}^{226}
 \end{aligned}$$

The lower SG is SG 140 when the preserved operations are: **(sub-SG label is 8)** 1, 6, 7, 10, 8, 9, 11, 12, 25, 30, 31, 34, 32, 33, 35, 36.

The transformation is:  $(\mathbf{a}_{140}, \mathbf{b}_{140}, \mathbf{c}_{140}) = (\mathbf{a}_{226}, \mathbf{b}_{226}, \mathbf{c}_{226}) \begin{pmatrix} \frac{1}{2} & \frac{1}{2} & 0 \\ -\frac{1}{2} & \frac{1}{2} & 0 \\ 0 & 0 & 1 \end{pmatrix}, \overrightarrow{O_{226}O_{140}} = \frac{1}{2}\mathbf{b}_{140}$

The reduction of higher dimensional irrep:

$$O_h : E_g \rightarrow A_{1g} + B_{2g} \text{ of } D_{4h}.$$

$$O_h : E_u \rightarrow A_{1u} + B_{2u} \text{ of } D_{4h}.$$

The correspondences of irreps at HSPs from original SG to lowered SG:

$$\begin{aligned}
 n_{GM8}^{140} &= n_{GM11}^{226} + n_{GM9}^{226} & n_{GM6}^{140} &= n_{GM10}^{226} + n_{GM7}^{226} & n_{GM9}^{140} &= n_{GM11}^{226} + n_{GM8}^{226} & n_{GM7}^{140} &= n_{GM10}^{226} + n_{GM6}^{226} & n_{M8}^{140} &= n_{X8}^{226} & n_{M6}^{140} &= n_{X6}^{226} \\
 n_{X6}^{140} & & n_{M9}^{140} &= n_{X9}^{226} & n_{M7}^{140} &= n_{X7}^{226} & n_{X6}^{140} &= n_{X6}^{226} + n_{X7}^{226} & n_{X5}^{140} &= n_{X8}^{226} + n_{X9}^{226} & n_{P7}^{140} &= n_{W7}^{226} & n_{P6}^{140} &= n_{W6}^{226} & n_{N2}^{140} &= n_{L4}^{226} + n_{L5}^{226} + n_{L6}^{226}
 \end{aligned}$$

The lower SG is SG 140 when the preserved operations are: **(sub-SG label is 9)** 1, 2, 3, 8, 9, 10, 13, 14, 25, 26, 27, 32, 33, 34, 37, 38.

The transformation is:  $(\mathbf{a}_{140}, \mathbf{b}_{140}, \mathbf{c}_{140}) = (\mathbf{a}_{226}, \mathbf{b}_{226}, \mathbf{c}_{226}) \begin{pmatrix} 0 & 0 & 1 \\ -\frac{1}{2} & \frac{1}{2} & 0 \\ -\frac{1}{2} & -\frac{1}{2} & 0 \end{pmatrix}, \overrightarrow{O_{226}O_{140}} = \frac{1}{2}\mathbf{b}_{140}$

The reduction of higher dimensional irrep:

$$O_h : E_g \rightarrow A_{1g} + B_{2g} \text{ of } D_{4h}.$$

$$O_h : E_u \rightarrow A_{1u} + B_{2u} \text{ of } D_{4h}.$$

The correspondences of irreps at HSPs from original SG to lowered SG:

$$\begin{aligned}
 n_{GM8}^{140} &= n_{GM11}^{226} + n_{GM9}^{226} & n_{GM6}^{140} &= n_{GM10}^{226} + n_{GM7}^{226} & n_{GM9}^{140} &= n_{GM11}^{226} + n_{GM8}^{226} & n_{GM7}^{140} &= n_{GM10}^{226} + n_{GM6}^{226} & n_{M8}^{140} &= n_{X8}^{226} & n_{M6}^{140} &= n_{X6}^{226} \\
 n_{X6}^{140} & & n_{M9}^{140} &= n_{X9}^{226} & n_{M7}^{140} &= n_{X7}^{226} & n_{X6}^{140} &= n_{X6}^{226} + n_{X7}^{226} & n_{X5}^{140} &= n_{X8}^{226} + n_{X9}^{226} & n_{P7}^{140} &= n_{W7}^{226} & n_{P6}^{140} &= n_{W6}^{226} & n_{N2}^{140} &= n_{L4}^{226} + n_{L5}^{226} + n_{L6}^{226}
 \end{aligned}$$

The lower SG is SG 140 when the preserved operations are: **(sub-SG label is 10)** 1, 4, 5, 9, 10, 8, 16, 15, 25, 28, 29, 33, 34, 32, 40, 39.

The transformation is:  $(\mathbf{a}_{140}, \mathbf{b}_{140}, \mathbf{c}_{140}) = (\mathbf{a}_{226}, \mathbf{b}_{226}, \mathbf{c}_{226}) \begin{pmatrix} \frac{1}{2} & -\frac{1}{2} & 0 \\ 0 & 0 & 1 \\ -\frac{1}{2} & -\frac{1}{2} & 0 \end{pmatrix}, \overrightarrow{O_{226}O_{140}} = \frac{1}{2}\mathbf{b}_{140}$

The reduction of higher dimensional irrep:

$$O_h : E_g \rightarrow A_{1g} + B_{2g} \text{ of } D_{4h}.$$

$$O_h : E_u \rightarrow A_{1u} + B_{2u} \text{ of } D_{4h}.$$

The correspondences of irreps at HSPs from original SG to lowered SG:

$$\begin{aligned}
 n_{GM8}^{140} &= n_{GM11}^{226} + n_{GM9}^{226} & n_{GM6}^{140} &= n_{GM10}^{226} + n_{GM7}^{226} & n_{GM9}^{140} &= n_{GM11}^{226} + n_{GM8}^{226} & n_{GM7}^{140} &= n_{GM10}^{226} + n_{GM6}^{226} & n_{M8}^{140} &= n_{X8}^{226} & n_{M6}^{140} &= n_{X6}^{226} \\
 n_{X6}^{140} & & n_{M9}^{140} &= n_{X9}^{226} & n_{M7}^{140} &= n_{X7}^{226} & n_{X6}^{140} &= n_{X6}^{226} + n_{X7}^{226} & n_{X5}^{140} &= n_{X8}^{226} + n_{X9}^{226} & n_{P7}^{140} &= n_{W7}^{226} & n_{P6}^{140} &= n_{W6}^{226} & n_{N2}^{140} &= n_{L4}^{226} + n_{L5}^{226} + n_{L6}^{226}
 \end{aligned}$$

The lower SG is SG 148 when the preserved operations are: **(sub-SG label is 11)** 1, 17, 18, 25, 41, 42.

The transformation is:  $(\mathbf{a}_{148}, \mathbf{b}_{148}, \mathbf{c}_{148}) = (\mathbf{a}_{226}, \mathbf{b}_{226}, \mathbf{c}_{226}) \begin{pmatrix} \frac{1}{2} & 0 & \frac{1}{2} \\ \frac{1}{2} & \frac{1}{2} & 0 \\ 0 & \frac{1}{2} & \frac{1}{2} \end{pmatrix}, \overrightarrow{O_{226}O_{148}} = \mathbf{0}$

The reduction of higher dimensional irrep:

$$O_h : T_{1g} \rightarrow A_g + {}^2E_g + {}^1E_g \text{ of } C_{3i}.$$

$$O_h : T_{2g} \rightarrow A_g + {}^2E_g + {}^1E_g \text{ of } C_{3i}.$$

$$O_h : T_{1u} \rightarrow {}^1E_u + A_u + {}^2E_u \text{ of } C_{3i}.$$

$$O_h : T_{2u} \rightarrow {}^1E_u + A_u + {}^2E_u \text{ of } C_{3i}.$$

The correspondences of irreps at HSPs from original SG to lowered SG:

$$\begin{aligned}
 n_{GM7}^{148} &= 2n_{GM11}^{226} & n_{GM4}^{148} &= 2n_{GM10}^{226} & n_{GM9}^{148} &= n_{GM11}^{226} + n_{GM8}^{226} + n_{GM9}^{226} & n_{GM6}^{148} &= n_{GM10}^{226} + n_{GM6}^{226} + n_{GM7}^{226} & n_{GM8}^{148} &= n_{GM11}^{226} + n_{GM8}^{226} \\
 n_{GM11}^{226} + n_{GM8}^{226} + n_{GM9}^{226} & & n_{GM5}^{148} &= n_{GM10}^{226} + n_{GM6}^{226} + n_{GM7}^{226} & n_{L2}^{148} &= n_{L4}^{226} + n_{L5}^{226} + n_{L6}^{226} & n_{L3}^{148} &= n_{L4}^{226} + n_{L5}^{226} + n_{L6}^{226} & n_{F2}^{148} &= 2n_{X8}^{226} + 2n_{X9}^{226} \\
 n_{F3}^{148} &= 2n_{X6}^{226} + 2n_{X7}^{226} & n_{T7}^{148} &= n_{L4}^{226} & n_{T4}^{148} &= n_{L4}^{226} & n_{T9}^{148} &= n_{L5}^{226} & n_{T6}^{148} &= n_{L6}^{226} & n_{T8}^{148} &= n_{L6}^{226} & n_{T5}^{148} &= n_{L5}^{226}
 \end{aligned}$$

The lower SG is SG 148 when the preserved operations are: **(sub-SG label is 12)** 1, 24, 23, 25, 48, 47.



## 124. Lowered SGs by higher-dimensional irreps of pairings in SG 227

The representative operations of SG/T for SG 227:

$$\begin{aligned}
 &1 : (x, y, z), 2 : (x + \frac{1}{4}, -z, y + \frac{1}{4}), 3 : (x + \frac{1}{4}, z + \frac{1}{4}, -y), 4 : (z + \frac{1}{4}, y + \frac{1}{4}, -x), 5 : (-z, y + \frac{1}{4}, x + \frac{1}{4}), \\
 &6 : (-y, x + \frac{1}{4}, z + \frac{1}{4}), 7 : (y + \frac{1}{4}, -x, z + \frac{1}{4}), 8 : (x, \frac{1}{4} - y, \frac{1}{4} - z), 9 : (\frac{1}{4} - x, y, \frac{1}{4} - z), 10 : (\frac{1}{4} - x, \frac{1}{4} - y, z), \\
 &11 : (y + \frac{1}{4}, x + \frac{1}{4}, -z), 12 : (-y, -x, -z), 13 : (-x, z + \frac{1}{4}, y + \frac{1}{4}), 14 : (-x, -z, -y), 15 : (z + \frac{1}{4}, -y, x + \frac{1}{4}), \\
 &16 : (-z, -y, -x), 17 : (z, x, y), 18 : (y, z, x), 19 : (\frac{1}{4} - y, z, \frac{1}{4} - x), 20 : (\frac{1}{4} - z, \frac{1}{4} - x, y), 21 : (\frac{1}{4} - y, \frac{1}{4} - z, x), \\
 &22 : (z, \frac{1}{4} - x, \frac{1}{4} - y), 23 : (y, \frac{1}{4} - z, \frac{1}{4} - x), 24 : (\frac{1}{4} - z, x, \frac{1}{4} - y), 25 : (-x, -y, -z), 26 : (\frac{1}{4} - x, z, \frac{1}{4} - y), \\
 &27 : (\frac{1}{4} - x, \frac{1}{4} - z, y), 28 : (\frac{1}{4} - z, \frac{1}{4} - y, x), 29 : (z, \frac{1}{4} - y, \frac{1}{4} - x), 30 : (y, \frac{1}{4} - x, \frac{1}{4} - z), 31 : (\frac{1}{4} - y, x, \frac{1}{4} - z), \\
 &32 : (-x, y + \frac{1}{4}, z + \frac{1}{4}), 33 : (x + \frac{1}{4}, -y, z + \frac{1}{4}), 34 : (x + \frac{1}{4}, y + \frac{1}{4}, -z), 35 : (\frac{1}{4} - y, \frac{1}{4} - x, z), 36 : (y, x, z), \\
 &37 : (x, \frac{1}{4} - z, \frac{1}{4} - y), 38 : (x, z, y), 39 : (\frac{1}{4} - z, y, \frac{1}{4} - x), 40 : (z, y, x), 41 : (-z, -x, -y), 42 : (-y, -z, -x), \\
 &43 : (y + \frac{1}{4}, -z, x + \frac{1}{4}), 44 : (z + \frac{1}{4}, x + \frac{1}{4}, -y), 45 : (y + \frac{1}{4}, z + \frac{1}{4}, -x), 46 : (-z, x + \frac{1}{4}, y + \frac{1}{4}), 47 : (-y, z + \frac{1}{4}, x + \frac{1}{4}), \\
 &48 : (z + \frac{1}{4}, -x, y + \frac{1}{4}).
 \end{aligned}$$

The lower SG is SG 70 when the preserved operations are: **(sub-SG label is 1) 1, 8, 9, 10, 25, 32, 33, 34.**

$$\text{The transformation is: } (\mathbf{a}_{70}, \mathbf{b}_{70}, \mathbf{c}_{70}) = (\mathbf{a}_{227}, \mathbf{b}_{227}, \mathbf{c}_{227}) \begin{pmatrix} 0 & 1 & 0 \\ 1 & 0 & 0 \\ 0 & 0 & -1 \end{pmatrix}, \overrightarrow{O_{227}O_{70}} = \frac{1}{4}\mathbf{a}_{70} + (\frac{1}{4})\mathbf{b}_{70} + (\frac{1}{2})\mathbf{c}_{70}$$

The reduction of higher dimensional irrep:

$$O_h : T_{1g} \rightarrow B_{1g} + B_{2g} + B_{3g} \text{ of } D_{2h}.$$

$$O_h : T_{2g} \rightarrow B_{1g} + B_{2g} + B_{3g} \text{ of } D_{2h}.$$

$$O_h : T_{1u} \rightarrow B_{1u} + B_{2u} + B_{3u} \text{ of } D_{2h}.$$

$$O_h : T_{2u} \rightarrow B_{1u} + B_{2u} + B_{3u} \text{ of } D_{2h}.$$

The correspondences of irreps at HSPs from original SG to lowered SG:

$$\begin{aligned}
 n_{GM6}^{70} &= 2n_{GM11}^{227} + n_{GM8}^{227} + n_{GM9}^{227} \quad n_{GM5}^{70} = 2n_{GM10}^{227} + n_{GM6}^{227} + n_{GM7}^{227} \quad n_{Y4}^{70} = n_{X5}^{227} \quad n_{Y3}^{70} = n_{X5}^{227} \quad n_{L3}^{70} = n_{L4}^{227} + n_{L5}^{227} + 2n_{L8}^{227} \\
 n_{L2}^{70} &= n_{L6}^{227} + n_{L7}^{227} + 2n_{L9}^{227} \quad n_{Z3}^{70} = n_{X5}^{227} \quad n_{Z4}^{70} = n_{X5}^{227} \quad n_{T4}^{70} = n_{X5}^{227} \quad n_{T3}^{70} = n_{X5}^{227}
 \end{aligned}$$

The lower SG is SG 74 when the preserved operations are: **(sub-SG label is 2) 1, 8, 13, 14, 25, 32, 37, 38.**

$$\text{The transformation is: } (\mathbf{a}_{74}, \mathbf{b}_{74}, \mathbf{c}_{74}) = (\mathbf{a}_{227}, \mathbf{b}_{227}, \mathbf{c}_{227}) \begin{pmatrix} 0 & 0 & 1 \\ \frac{1}{2} & -\frac{1}{2} & 0 \\ \frac{1}{2} & \frac{1}{2} & 0 \end{pmatrix}, \overrightarrow{O_{227}O_{74}} = \frac{1}{4}\mathbf{a}_{74} + (-\frac{1}{4})\mathbf{b}_{74} + (\frac{1}{4})\mathbf{c}_{74}$$

The reduction of higher dimensional irrep:

$$O_h : T_{1g} \rightarrow B_{2g} + B_{1g} + B_{3g} \text{ of } D_{2h}.$$

$$O_h : T_{2g} \rightarrow A_g + B_{2g} + B_{3g} \text{ of } D_{2h}.$$

$$O_h : T_{1u} \rightarrow B_{2u} + B_{1u} + B_{3u} \text{ of } D_{2h}.$$

$$O_h : T_{2u} \rightarrow A_u + B_{2u} + B_{3u} \text{ of } D_{2h}.$$

The correspondences of irreps at HSPs from original SG to lowered SG:

$$\begin{aligned}
 n_{GM6}^{74} &= 2n_{GM11}^{227} + n_{GM8}^{227} + n_{GM9}^{227} \quad n_{GM5}^{74} = 2n_{GM10}^{227} + n_{GM6}^{227} + n_{GM7}^{227} \quad n_{X6}^{74} = n_{X5}^{227} \quad n_{X5}^{74} = n_{X5}^{227} \quad n_{T2}^{74} = 2n_{X5}^{227} \quad n_{W5}^{74} = n_{W7}^{227} \\
 n_{W4}^{74} &= n_{W4}^{227} + n_{W6}^{227} \quad n_{W2}^{74} = n_{W3}^{227} + n_{W5}^{227} \quad n_{W3}^{74} = n_{W7}^{227} \quad n_{R6}^{74} = n_{L4}^{227} + n_{L8}^{227} \quad n_{R4}^{74} = n_{L6}^{227} + n_{L9}^{227} \quad n_{R5}^{74} = n_{L5}^{227} + n_{L8}^{227} \quad n_{R3}^{74} = \\
 n_{L7}^{227} + n_{L9}^{227} \quad n_{S4}^{74} &= n_{L7}^{227} + n_{L9}^{227} \quad n_{S6}^{74} = n_{L5}^{227} + n_{L8}^{227} \quad n_{S3}^{74} = n_{L6}^{227} + n_{L9}^{227} \quad n_{S5}^{74} = n_{L4}^{227} + n_{L8}^{227}
 \end{aligned}$$

The lower SG is SG 74 when the preserved operations are: **(sub-SG label is 3) 1, 9, 16, 15, 25, 33, 40, 39.**

$$\text{The transformation is: } (\mathbf{a}_{74}, \mathbf{b}_{74}, \mathbf{c}_{74}) = (\mathbf{a}_{227}, \mathbf{b}_{227}, \mathbf{c}_{227}) \begin{pmatrix} \frac{1}{2} & \frac{1}{2} & 0 \\ 0 & 0 & 1 \\ \frac{1}{2} & -\frac{1}{2} & 0 \end{pmatrix}, \overrightarrow{O_{227}O_{74}} = \frac{1}{4}\mathbf{a}_{74} + (-\frac{1}{4})\mathbf{b}_{74} + (\frac{1}{4})\mathbf{c}_{74}$$

The reduction of higher dimensional irrep:

$$O_h : T_{1g} \rightarrow B_{2g} + B_{1g} + B_{3g} \text{ of } D_{2h}.$$

$$O_h : T_{2g} \rightarrow A_g + B_{2g} + B_{3g} \text{ of } D_{2h}.$$

$$O_h : T_{1u} \rightarrow B_{2u} + B_{1u} + B_{3u} \text{ of } D_{2h}.$$

$$O_h : T_{2u} \rightarrow A_u + B_{2u} + B_{3u} \text{ of } D_{2h}.$$

The correspondences of irreps at HSPs from original SG to lowered SG:

$$\begin{aligned}
 n_{GM6}^{74} &= 2n_{GM11}^{227} + n_{GM8}^{227} + n_{GM9}^{227} \quad n_{GM5}^{74} = 2n_{GM10}^{227} + n_{GM6}^{227} + n_{GM7}^{227} \quad n_{X6}^{74} = n_{X5}^{227} \quad n_{X5}^{74} = n_{X5}^{227} \quad n_{T2}^{74} = 2n_{X5}^{227} \quad n_{W5}^{74} = n_{W7}^{227} \\
 n_{W4}^{74} &= n_{W4}^{227} + n_{W6}^{227} \quad n_{W2}^{74} = n_{W3}^{227} + n_{W5}^{227} \quad n_{W3}^{74} = n_{W7}^{227} \quad n_{R6}^{74} = n_{L4}^{227} + n_{L8}^{227} \quad n_{R4}^{74} = n_{L6}^{227} + n_{L9}^{227} \quad n_{R5}^{74} = n_{L5}^{227} + n_{L8}^{227} \quad n_{R3}^{74} = \\
 n_{L7}^{227} + n_{L9}^{227} \quad n_{S4}^{74} &= n_{L7}^{227} + n_{L9}^{227} \quad n_{S6}^{74} = n_{L5}^{227} + n_{L8}^{227} \quad n_{S3}^{74} = n_{L6}^{227} + n_{L9}^{227} \quad n_{S5}^{74} = n_{L4}^{227} + n_{L8}^{227}
 \end{aligned}$$

The lower SG is SG 74 when the preserved operations are: **(sub-SG label is 4) 1, 10, 11, 12, 25, 34, 35, 36.**

The transformation is:  $(\mathbf{a}_{74}, \mathbf{b}_{74}, \mathbf{c}_{74}) = (\mathbf{a}_{227}, \mathbf{b}_{227}, \mathbf{c}_{227}) \begin{pmatrix} \frac{1}{2} & -\frac{1}{2} & 0 \\ \frac{1}{2} & \frac{1}{2} & 0 \\ 0 & 0 & 1 \end{pmatrix}, \overrightarrow{O_{227}O_{74}} = \frac{1}{4}\mathbf{a}_{74} + (-\frac{1}{4})\mathbf{b}_{74} + (\frac{1}{4})\mathbf{c}_{74}$

The reduction of higher dimensional irrep:

$$O_h : T_{1g} \rightarrow B_{2g} + B_{1g} + B_{3g} \text{ of } D_{2h}.$$

$$O_h : T_{2g} \rightarrow A_g + B_{2g} + B_{3g} \text{ of } D_{2h}.$$

$$O_h : T_{1u} \rightarrow B_{2u} + B_{1u} + B_{3u} \text{ of } D_{2h}.$$

$$O_h : T_{2u} \rightarrow A_u + B_{2u} + B_{3u} \text{ of } D_{2h}.$$

The correspondences of irreps at HSPs from original SG to lowered SG:

$$\begin{aligned} n_{GM6}^{74} &= 2n_{GM11}^{227} + n_{GM8}^{227} + n_{GM9}^{227} n_{GM5}^{74} = 2n_{GM10}^{227} + n_{GM6}^{227} + n_{GM7}^{227} n_{X6}^{74} = n_{X5}^{227} n_{X5}^{74} = n_{X5}^{227} n_{T2}^{74} = 2n_{X5}^{227} n_{W5}^{74} = n_{W7}^{227} \\ n_{W4}^{74} &= n_{W4}^{227} + n_{W6}^{227} n_{W2}^{74} = n_{W3}^{227} + n_{W5}^{227} n_{W3}^{74} = n_{W7}^{227} n_{R6}^{74} = n_{L4}^{227} + n_{L8}^{227} n_{R4}^{74} = n_{L6}^{227} + n_{L9}^{227} n_{R5}^{74} = n_{L5}^{227} + n_{L8}^{227} n_{R3}^{74} = \\ n_{L7}^{227} + n_{L9}^{227} n_{S4}^{74} &= n_{L7}^{227} + n_{L9}^{227} n_{S6}^{74} = n_{L5}^{227} + n_{L8}^{227} n_{S3}^{74} = n_{L6}^{227} + n_{L9}^{227} n_{S5}^{74} = n_{L4}^{227} + n_{L8}^{227} \end{aligned}$$

The lower SG is SG 88 when the preserved operations are: **(sub-SG label is 5) 1, 6, 7, 10, 25, 30, 31, 34.**

The transformation is:  $(\mathbf{a}_{88}, \mathbf{b}_{88}, \mathbf{c}_{88}) = (\mathbf{a}_{227}, \mathbf{b}_{227}, \mathbf{c}_{227}) \begin{pmatrix} -\frac{1}{2} & \frac{1}{2} & 0 \\ \frac{1}{2} & \frac{1}{2} & 0 \\ 0 & 0 & -1 \end{pmatrix}, \overrightarrow{O_{227}O_{88}} = \frac{1}{2}\mathbf{a}_{88}$

The reduction of higher dimensional irrep:

$$O_h : T_{1g} \rightarrow A_g + {}^2E_g + {}^1E_g \text{ of } C_{4h}.$$

$$O_h : T_{2g} \rightarrow {}^2E_g + B_g + {}^1E_g \text{ of } C_{4h}.$$

$$O_h : T_{1u} \rightarrow A_u + {}^2E_u + {}^1E_u \text{ of } C_{4h}.$$

$$O_h : T_{2u} \rightarrow {}^2E_u + B_u + {}^1E_u \text{ of } C_{4h}.$$

The correspondences of irreps at HSPs from original SG to lowered SG:

$$\begin{aligned} n_{GM9}^{88} &= n_{GM11}^{227} + n_{GM9}^{227} n_{GM5}^{88} = n_{GM10}^{227} + n_{GM7}^{227} n_{GM11}^{88} = n_{GM11}^{227} + n_{GM9}^{227} n_{GM7}^{88} = n_{GM10}^{227} + n_{GM7}^{227} n_{GM12}^{88} = \\ n_{GM11}^{227} + n_{GM8}^{227} n_{GM8}^{88} &= n_{GM10}^{227} + n_{GM6}^{227} n_{GM10}^{88} = n_{GM11}^{227} + n_{GM8}^{227} n_{GM6}^{88} = n_{GM10}^{227} + n_{GM6}^{227} n_{M4}^{88} = n_{X5}^{227} n_{M3}^{88} = n_{X5}^{227} \\ n_{X2}^{88} &= 2n_{X5}^{227} n_{P5}^{88} = n_{W7}^{227} n_{P6}^{88} = n_{W7}^{227} n_{P7}^{88} = n_{W5}^{227} + n_{W6}^{227} n_{P8}^{88} = n_{W3}^{227} + n_{W4}^{227} n_{N3}^{88} = n_{L6}^{227} + n_{L7}^{227} + 2n_{L9}^{227} n_{N2}^{88} = \\ n_{L4}^{227} + n_{L5}^{227} + 2n_{L8}^{227} \end{aligned}$$

The lower SG is SG 88 when the preserved operations are: **(sub-SG label is 6) 1, 2, 3, 8, 25, 26, 27, 32.**

The transformation is:  $(\mathbf{a}_{88}, \mathbf{b}_{88}, \mathbf{c}_{88}) = (\mathbf{a}_{227}, \mathbf{b}_{227}, \mathbf{c}_{227}) \begin{pmatrix} 0 & 0 & 1 \\ -\frac{1}{2} & -\frac{1}{2} & 0 \\ \frac{1}{2} & -\frac{1}{2} & 0 \end{pmatrix}, \overrightarrow{O_{227}O_{88}} = \frac{1}{2}\mathbf{a}_{88}$

The reduction of higher dimensional irrep:

$$O_h : T_{1g} \rightarrow A_g + {}^2E_g + {}^1E_g \text{ of } C_{4h}.$$

$$O_h : T_{2g} \rightarrow {}^2E_g + B_g + {}^1E_g \text{ of } C_{4h}.$$

$$O_h : T_{1u} \rightarrow A_u + {}^2E_u + {}^1E_u \text{ of } C_{4h}.$$

$$O_h : T_{2u} \rightarrow {}^2E_u + B_u + {}^1E_u \text{ of } C_{4h}.$$

The correspondences of irreps at HSPs from original SG to lowered SG:

$$\begin{aligned} n_{GM9}^{88} &= n_{GM11}^{227} + n_{GM9}^{227} n_{GM5}^{88} = n_{GM10}^{227} + n_{GM7}^{227} n_{GM11}^{88} = n_{GM11}^{227} + n_{GM9}^{227} n_{GM7}^{88} = n_{GM10}^{227} + n_{GM7}^{227} n_{GM12}^{88} = \\ n_{GM11}^{227} + n_{GM8}^{227} n_{GM8}^{88} &= n_{GM10}^{227} + n_{GM6}^{227} n_{GM10}^{88} = n_{GM11}^{227} + n_{GM8}^{227} n_{GM6}^{88} = n_{GM10}^{227} + n_{GM6}^{227} n_{M4}^{88} = n_{X5}^{227} n_{M3}^{88} = n_{X5}^{227} \\ n_{X2}^{88} &= 2n_{X5}^{227} n_{P5}^{88} = n_{W7}^{227} n_{P6}^{88} = n_{W7}^{227} n_{P7}^{88} = n_{W5}^{227} + n_{W6}^{227} n_{P8}^{88} = n_{W3}^{227} + n_{W4}^{227} n_{N3}^{88} = n_{L6}^{227} + n_{L7}^{227} + 2n_{L9}^{227} n_{N2}^{88} = \\ n_{L4}^{227} + n_{L5}^{227} + 2n_{L8}^{227} \end{aligned}$$

The lower SG is SG 88 when the preserved operations are: **(sub-SG label is 7) 1, 4, 5, 9, 25, 28, 29, 33.**

The transformation is:  $(\mathbf{a}_{88}, \mathbf{b}_{88}, \mathbf{c}_{88}) = (\mathbf{a}_{227}, \mathbf{b}_{227}, \mathbf{c}_{227}) \begin{pmatrix} \frac{1}{2} & -\frac{1}{2} & 0 \\ 0 & 0 & 1 \\ -\frac{1}{2} & -\frac{1}{2} & 0 \end{pmatrix}, \overrightarrow{O_{227}O_{88}} = \frac{1}{2}\mathbf{a}_{88}$

The reduction of higher dimensional irrep:

$$O_h : T_{1g} \rightarrow A_g + {}^2E_g + {}^1E_g \text{ of } C_{4h}.$$

$$O_h : T_{2g} \rightarrow {}^2E_g + B_g + {}^1E_g \text{ of } C_{4h}.$$

$$O_h : T_{1u} \rightarrow A_u + {}^2E_u + {}^1E_u \text{ of } C_{4h}.$$

$$O_h : T_{2u} \rightarrow {}^2E_u + B_u + {}^1E_u \text{ of } C_{4h}.$$

The correspondences of irreps at HSPs from original SG to lowered SG:

$$\begin{aligned} n_{GM9}^{88} &= n_{GM11}^{227} + n_{GM9}^{227} n_{GM5}^{88} = n_{GM10}^{227} + n_{GM7}^{227} n_{GM11}^{88} = n_{GM11}^{227} + n_{GM9}^{227} n_{GM7}^{88} = n_{GM10}^{227} + n_{GM7}^{227} n_{GM12}^{88} = \\ n_{GM11}^{227} + n_{GM8}^{227} n_{GM8}^{88} &= n_{GM10}^{227} + n_{GM6}^{227} n_{GM10}^{88} = n_{GM11}^{227} + n_{GM8}^{227} n_{GM6}^{88} = n_{GM10}^{227} + n_{GM6}^{227} n_{M4}^{88} = n_{X5}^{227} n_{M3}^{88} = n_{X5}^{227} \\ n_{X2}^{88} &= 2n_{X5}^{227} n_{P5}^{88} = n_{W7}^{227} n_{P6}^{88} = n_{W7}^{227} n_{P7}^{88} = n_{W5}^{227} + n_{W6}^{227} n_{P8}^{88} = n_{W3}^{227} + n_{W4}^{227} n_{N3}^{88} = n_{L6}^{227} + n_{L7}^{227} + 2n_{L9}^{227} n_{N2}^{88} = \\ n_{L4}^{227} + n_{L5}^{227} + 2n_{L8}^{227} \end{aligned}$$

$$n_{LA}^{227} + n_{L5}^{227} + 2n_{L8}^{227}$$

The lower SG is SG 141 when the preserved operations are: (**sub-SG label is 8**) 1, 6, 7, 10, 8, 9, 11, 12, 25, 30, 31, 34, 32, 33, 35, 36.

The transformation is:  $(\mathbf{a}_{141}, \mathbf{b}_{141}, \mathbf{c}_{141}) = (\mathbf{a}_{227}, \mathbf{b}_{227}, \mathbf{c}_{227}) \begin{pmatrix} \frac{1}{2} & \frac{1}{2} & 0 \\ -\frac{1}{2} & \frac{1}{2} & 0 \\ 0 & 0 & 1 \end{pmatrix}, \overrightarrow{O_{227}O_{141}} = \frac{1}{2}\mathbf{a}_{141}$

The reduction of higher dimensional irrep:

$$O_h : E_g \rightarrow A_{1g} + B_{2g} \text{ of } D_{4h}.$$

$$O_h : E_u \rightarrow A_{1u} + B_{2u} \text{ of } D_{4h}.$$

The correspondences of irreps at HSPs from original SG to lowered SG:

$$\begin{aligned} n_{GM8}^{141} &= n_{GM11}^{227} + n_{GM9}^{227} & n_{GM6}^{141} &= n_{GM10}^{227} + n_{GM7}^{227} & n_{GM9}^{141} &= n_{GM11}^{227} + n_{GM8}^{227} & n_{GM7}^{141} &= n_{GM10}^{227} + n_{GM6}^{227} & n_{M5}^{141} &= n_{X5}^{227} & n_{X3}^{141} &= n_{X5}^{227} \\ n_{X5}^{227} n_{X4}^{141} &= n_{X5}^{227} n_{P5}^{141} & n_{W5}^{227} n_{P3}^{141} &= n_{W3}^{227} n_{P4}^{141} & n_{W6}^{227} n_{P6}^{141} &= n_{W4}^{227} n_{P7}^{141} & n_{W7}^{227} n_{N6}^{141} &= n_{L7}^{227} + n_{L9}^{227} & n_{N4}^{141} &= n_{L5}^{227} + n_{L8}^{227} \\ n_{N5}^{141} &= n_{L6}^{227} + n_{L9}^{227} & n_{N3}^{141} &= n_{L4}^{227} + n_{L8}^{227} \end{aligned}$$

The lower SG is SG 141 when the preserved operations are: (**sub-SG label is 9**) 1, 2, 3, 8, 9, 10, 13, 14, 25, 26, 27, 32, 33, 34, 37, 38.

The transformation is:  $(\mathbf{a}_{141}, \mathbf{b}_{141}, \mathbf{c}_{141}) = (\mathbf{a}_{227}, \mathbf{b}_{227}, \mathbf{c}_{227}) \begin{pmatrix} 0 & 0 & 1 \\ \frac{1}{2} & \frac{1}{2} & 0 \\ -\frac{1}{2} & \frac{1}{2} & 0 \end{pmatrix}, \overrightarrow{O_{227}O_{141}} = \frac{1}{2}\mathbf{a}_{141}$

The reduction of higher dimensional irrep:

$$O_h : E_g \rightarrow A_{1g} + B_{2g} \text{ of } D_{4h}.$$

$$O_h : E_u \rightarrow A_{1u} + B_{2u} \text{ of } D_{4h}.$$

The correspondences of irreps at HSPs from original SG to lowered SG:

$$\begin{aligned} n_{GM8}^{141} &= n_{GM11}^{227} + n_{GM9}^{227} & n_{GM6}^{141} &= n_{GM10}^{227} + n_{GM7}^{227} & n_{GM9}^{141} &= n_{GM11}^{227} + n_{GM8}^{227} & n_{GM7}^{141} &= n_{GM10}^{227} + n_{GM6}^{227} & n_{M5}^{141} &= n_{X5}^{227} & n_{X3}^{141} &= n_{X5}^{227} \\ n_{X5}^{227} n_{X4}^{141} &= n_{X5}^{227} n_{P5}^{141} & n_{W5}^{227} n_{P3}^{141} &= n_{W3}^{227} n_{P4}^{141} & n_{W6}^{227} n_{P6}^{141} &= n_{W4}^{227} n_{P7}^{141} & n_{W7}^{227} n_{N6}^{141} &= n_{L7}^{227} + n_{L9}^{227} & n_{N4}^{141} &= n_{L5}^{227} + n_{L8}^{227} \\ n_{N5}^{141} &= n_{L6}^{227} + n_{L9}^{227} & n_{N3}^{141} &= n_{L4}^{227} + n_{L8}^{227} \end{aligned}$$

The lower SG is SG 141 when the preserved operations are: (**sub-SG label is 10**) 1, 4, 5, 9, 10, 8, 16, 15, 25, 28, 29, 33, 34, 32, 40, 39.

The transformation is:  $(\mathbf{a}_{141}, \mathbf{b}_{141}, \mathbf{c}_{141}) = (\mathbf{a}_{227}, \mathbf{b}_{227}, \mathbf{c}_{227}) \begin{pmatrix} -\frac{1}{2} & -\frac{1}{2} & 0 \\ 0 & 0 & -1 \\ \frac{1}{2} & -\frac{1}{2} & 0 \end{pmatrix}, \overrightarrow{O_{227}O_{141}} = \frac{1}{2}\mathbf{a}_{141}$

The reduction of higher dimensional irrep:

$$O_h : E_g \rightarrow A_{1g} + B_{2g} \text{ of } D_{4h}.$$

$$O_h : E_u \rightarrow A_{1u} + B_{2u} \text{ of } D_{4h}.$$

The correspondences of irreps at HSPs from original SG to lowered SG:

$$\begin{aligned} n_{GM8}^{141} &= n_{GM11}^{227} + n_{GM9}^{227} & n_{GM6}^{141} &= n_{GM10}^{227} + n_{GM7}^{227} & n_{GM9}^{141} &= n_{GM11}^{227} + n_{GM8}^{227} & n_{GM7}^{141} &= n_{GM10}^{227} + n_{GM6}^{227} & n_{M5}^{141} &= n_{X5}^{227} & n_{X3}^{141} &= n_{X5}^{227} \\ n_{X5}^{227} n_{X4}^{141} &= n_{X5}^{227} n_{P5}^{141} & n_{W5}^{227} n_{P3}^{141} &= n_{W3}^{227} n_{P4}^{141} & n_{W6}^{227} n_{P6}^{141} &= n_{W4}^{227} n_{P7}^{141} & n_{W7}^{227} n_{N6}^{141} &= n_{L7}^{227} + n_{L9}^{227} & n_{N4}^{141} &= n_{L5}^{227} + n_{L8}^{227} \\ n_{N5}^{141} &= n_{L6}^{227} + n_{L9}^{227} & n_{N3}^{141} &= n_{L4}^{227} + n_{L8}^{227} \end{aligned}$$

The lower SG is SG 148 when the preserved operations are: (**sub-SG label is 11**) 1, 17, 18, 25, 41, 42.

The transformation is:  $(\mathbf{a}_{148}, \mathbf{b}_{148}, \mathbf{c}_{148}) = (\mathbf{a}_{227}, \mathbf{b}_{227}, \mathbf{c}_{227}) \begin{pmatrix} \frac{1}{2} & 0 & \frac{1}{2} \\ \frac{1}{2} & \frac{1}{2} & 0 \\ 0 & \frac{1}{2} & \frac{1}{2} \end{pmatrix}, \overrightarrow{O_{227}O_{148}} = \mathbf{0}$

The reduction of higher dimensional irrep:

$$O_h : T_{1g} \rightarrow A_g + {}^2E_g + {}^1E_g \text{ of } C_{3i}.$$

$$O_h : T_{2g} \rightarrow A_g + {}^2E_g + {}^1E_g \text{ of } C_{3i}.$$

$$O_h : T_{1u} \rightarrow {}^1E_u + A_u + {}^2E_u \text{ of } C_{3i}.$$

$$O_h : T_{2u} \rightarrow {}^1E_u + A_u + {}^2E_u \text{ of } C_{3i}.$$

The correspondences of irreps at HSPs from original SG to lowered SG:

$$\begin{aligned} n_{GM7}^{148} &= 2n_{GM11}^{227} & n_{GM4}^{148} &= 2n_{GM10}^{227} & n_{GM9}^{148} &= n_{GM11}^{227} + n_{GM8}^{227} & n_{GM9}^{148} &= n_{GM11}^{227} + n_{GM8}^{227} & n_{GM6}^{148} &= n_{GM10}^{227} + n_{GM6}^{227} + n_{GM7}^{227} & n_{GM8}^{148} &= n_{GM11}^{227} + n_{GM8}^{227} \\ n_{GM11}^{227} + n_{GM8}^{227} &+ n_{GM9}^{227} & n_{GM5}^{148} &= n_{GM10}^{227} + n_{GM6}^{227} + n_{GM7}^{227} & n_{L2}^{148} &= n_{L4}^{227} + n_{L5}^{227} + 2n_{L8}^{227} & n_{L3}^{148} &= n_{L6}^{227} + n_{L7}^{227} + 2n_{L9}^{227} & n_{F2}^{148} &= n_{L5}^{227} + n_{L8}^{227} \\ 2n_{X5}^{227} n_{F3}^{148} &= 2n_{X5}^{227} n_{T7}^{148} & n_{L6}^{227} &+ n_{L7}^{227} & n_{T4}^{148} &= n_{L4}^{227} + n_{L5}^{227} & n_{T9}^{148} &= n_{L9}^{227} & n_{T6}^{148} &= n_{L8}^{227} & n_{T8}^{148} &= n_{L9}^{227} & n_{T5}^{148} &= n_{L8}^{227} \end{aligned}$$

The lower SG is SG 148 when the preserved operations are: (**sub-SG label is 12**) 1, 24, 23, 25, 48, 47.

The transformation is:  $(\mathbf{a}_{148}, \mathbf{b}_{148}, \mathbf{c}_{148}) = (\mathbf{a}_{227}, \mathbf{b}_{227}, \mathbf{c}_{227}) \begin{pmatrix} -\frac{1}{2} & -\frac{1}{2} & 0 \\ 0 & -\frac{1}{2} & -\frac{1}{2} \\ \frac{1}{2} & 0 & \frac{1}{2} \end{pmatrix}, \overrightarrow{O_{227}O_{148}} = \frac{1}{2}\mathbf{b}_{148}$

The reduction of higher dimensional irrep:

$$O_h : T_{1g} \rightarrow A_g + {}^2E_g + {}^1E_g \text{ of } C_{3i}.$$

$$O_h : T_{2g} \rightarrow A_g + {}^2E_g + {}^1E_g \text{ of } C_{3i}.$$

$$O_h : T_{1u} \rightarrow {}^1E_u + A_u + {}^2E_u \text{ of } C_{3i}.$$

$$O_h : T_{2u} \rightarrow {}^1E_u + A_u + {}^2E_u \text{ of } C_{3i}.$$

The correspondences of irreps at HSPs from original SG to lowered SG:

$$\begin{aligned} n_{GM7}^{148} &= 2n_{GM11}^{227} n_{GM4}^{148} = 2n_{GM10}^{227} n_{GM9}^{148} = n_{GM11}^{227} + n_{GM8}^{227} + n_{GM9}^{227} n_{GM6}^{148} = n_{GM10}^{227} + n_{GM6}^{227} + n_{GM7}^{227} n_{GM8}^{148} = \\ n_{GM11}^{227} + n_{GM8}^{227} + n_{GM9}^{227} n_{GM5}^{148} &= n_{GM10}^{227} + n_{GM6}^{227} + n_{GM7}^{227} n_{L2}^{148} = n_{L4}^{227} + n_{L5}^{227} + 2n_{L8}^{227} n_{L3}^{148} = n_{L6}^{227} + n_{L7}^{227} + 2n_{L9}^{227} n_{F2}^{148} = \\ 2n_{X5}^{227} n_{F3}^{148} &= 2n_{X5}^{227} n_{T7}^{148} = n_{L6}^{227} + n_{L7}^{227} n_{T4}^{148} = n_{L4}^{227} + n_{L5}^{227} n_{T9}^{148} = n_{L9}^{227} n_{T6}^{148} = n_{L8}^{227} n_{T8}^{148} = n_{L9}^{227} n_{T5}^{148} = n_{L8}^{227} \end{aligned}$$

The lower SG is SG 148 when the preserved operations are: **(sub-SG label is 13)** 1, 20, 19, 25, 44, 43.

The transformation is:  $(\mathbf{a}_{148}, \mathbf{b}_{148}, \mathbf{c}_{148}) = (\mathbf{a}_{227}, \mathbf{b}_{227}, \mathbf{c}_{227}) \begin{pmatrix} \frac{1}{2} & 0 & \frac{1}{2} \\ -\frac{1}{2} & -\frac{1}{2} & 0 \\ 0 & -\frac{1}{2} & -\frac{1}{2} \end{pmatrix}, \overrightarrow{O_{227}O_{148}} = \frac{1}{2}\mathbf{b}_{148}$

The reduction of higher dimensional irrep:

$$O_h : T_{1g} \rightarrow A_g + {}^2E_g + {}^1E_g \text{ of } C_{3i}.$$

$$O_h : T_{2g} \rightarrow A_g + {}^2E_g + {}^1E_g \text{ of } C_{3i}.$$

$$O_h : T_{1u} \rightarrow {}^1E_u + A_u + {}^2E_u \text{ of } C_{3i}.$$

$$O_h : T_{2u} \rightarrow {}^1E_u + A_u + {}^2E_u \text{ of } C_{3i}.$$

The correspondences of irreps at HSPs from original SG to lowered SG:

$$\begin{aligned} n_{GM7}^{148} &= 2n_{GM11}^{227} n_{GM4}^{148} = 2n_{GM10}^{227} n_{GM9}^{148} = n_{GM11}^{227} + n_{GM8}^{227} + n_{GM9}^{227} n_{GM6}^{148} = n_{GM10}^{227} + n_{GM6}^{227} + n_{GM7}^{227} n_{GM8}^{148} = \\ n_{GM11}^{227} + n_{GM8}^{227} + n_{GM9}^{227} n_{GM5}^{148} &= n_{GM10}^{227} + n_{GM6}^{227} + n_{GM7}^{227} n_{L2}^{148} = n_{L4}^{227} + n_{L5}^{227} + 2n_{L8}^{227} n_{L3}^{148} = n_{L6}^{227} + n_{L7}^{227} + 2n_{L9}^{227} n_{F2}^{148} = \\ 2n_{X5}^{227} n_{F3}^{148} &= 2n_{X5}^{227} n_{T7}^{148} = n_{L6}^{227} + n_{L7}^{227} n_{T4}^{148} = n_{L4}^{227} + n_{L5}^{227} n_{T9}^{148} = n_{L9}^{227} n_{T6}^{148} = n_{L8}^{227} n_{T8}^{148} = n_{L9}^{227} n_{T5}^{148} = n_{L8}^{227} \end{aligned}$$

The lower SG is SG 148 when the preserved operations are: **(sub-SG label is 14)** 1, 22, 21, 25, 46, 45.

The transformation is:  $(\mathbf{a}_{148}, \mathbf{b}_{148}, \mathbf{c}_{148}) = (\mathbf{a}_{227}, \mathbf{b}_{227}, \mathbf{c}_{227}) \begin{pmatrix} -\frac{1}{2} & -\frac{1}{2} & 0 \\ 0 & \frac{1}{2} & \frac{1}{2} \\ -\frac{1}{2} & 0 & -\frac{1}{2} \end{pmatrix}, \overrightarrow{O_{227}O_{148}} = \frac{1}{2}\mathbf{b}_{148} + (\frac{1}{2})\mathbf{c}_{148}$

The reduction of higher dimensional irrep:

$$O_h : T_{1g} \rightarrow A_g + {}^2E_g + {}^1E_g \text{ of } C_{3i}.$$

$$O_h : T_{2g} \rightarrow A_g + {}^2E_g + {}^1E_g \text{ of } C_{3i}.$$

$$O_h : T_{1u} \rightarrow {}^1E_u + A_u + {}^2E_u \text{ of } C_{3i}.$$

$$O_h : T_{2u} \rightarrow {}^1E_u + A_u + {}^2E_u \text{ of } C_{3i}.$$

The correspondences of irreps at HSPs from original SG to lowered SG:

$$\begin{aligned} n_{GM7}^{148} &= 2n_{GM11}^{227} n_{GM4}^{148} = 2n_{GM10}^{227} n_{GM9}^{148} = n_{GM11}^{227} + n_{GM8}^{227} + n_{GM9}^{227} n_{GM6}^{148} = n_{GM10}^{227} + n_{GM6}^{227} + n_{GM7}^{227} n_{GM8}^{148} = \\ n_{GM11}^{227} + n_{GM8}^{227} + n_{GM9}^{227} n_{GM5}^{148} &= n_{GM10}^{227} + n_{GM6}^{227} + n_{GM7}^{227} n_{L2}^{148} = n_{L6}^{227} + n_{L7}^{227} + 2n_{L9}^{227} n_{L3}^{148} = n_{L4}^{227} + n_{L5}^{227} + 2n_{L8}^{227} n_{F2}^{148} = \\ 2n_{X5}^{227} n_{F3}^{148} &= 2n_{X5}^{227} n_{T7}^{148} = n_{L6}^{227} + n_{L7}^{227} n_{T4}^{148} = n_{L4}^{227} + n_{L5}^{227} n_{T9}^{148} = n_{L9}^{227} n_{T6}^{148} = n_{L8}^{227} n_{T8}^{148} = n_{L9}^{227} n_{T5}^{148} = n_{L8}^{227} \end{aligned}$$

The lower SG is SG 203 when the preserved operations are: **(sub-SG label is 15)** 1, 8, 9, 10, 17, 24, 20, 22, 18, 23, 19, 21, 25, 32, 33, 34, 41, 48, 44, 46, 42, 47, 43, 45.

The transformation is:  $(\mathbf{a}_{203}, \mathbf{b}_{203}, \mathbf{c}_{203}) = (\mathbf{a}_{227}, \mathbf{b}_{227}, \mathbf{c}_{227}) \begin{pmatrix} 0 & 0 & -1 \\ 1 & 0 & 0 \\ 0 & -1 & 0 \end{pmatrix}, \overrightarrow{O_{227}O_{203}} = \frac{1}{2}\mathbf{a}_{203} + (\frac{1}{4})\mathbf{b}_{203} + (\frac{1}{4})\mathbf{c}_{203}$

The reduction of higher dimensional irrep:

$$O_h : E_g \rightarrow {}^1E_g + {}^2E_g \text{ of } T_h.$$

$$O_h : E_u \rightarrow {}^1E_u + {}^2E_u \text{ of } T_h.$$

The correspondences of irreps at HSPs from original SG to lowered SG:

$$\begin{aligned} n_{GM9}^{203} &= n_{GM11}^{227} n_{GM6}^{203} = n_{GM10}^{227} n_{GM10}^{203} = n_{GM11}^{227} n_{GM7}^{203} = n_{GM10}^{227} n_{GM8}^{203} = n_{GM8}^{227} + n_{GM9}^{227} n_{GM5}^{203} = n_{GM6}^{227} + n_{GM7}^{227} n_{X4}^{203} = \\ n_{X3}^{227} n_{X3}^{203} &= n_{X5}^{227} n_{L7}^{203} = n_{L4}^{227} + n_{L5}^{227} n_{L4}^{203} = n_{L6}^{227} + n_{L7}^{227} n_{L9}^{203} = n_{L8}^{227} n_{L6}^{203} = n_{L9}^{227} n_{L8}^{203} = n_{L8}^{227} n_{L5}^{203} = n_{L9}^{227} n_{W2}^{203} = n_{W7}^{227} \\ n_{W4}^{203} &= n_{W7}^{227} n_{W3}^{203} = n_{W4}^{227} + n_{W5}^{227} n_{W5}^{203} = n_{W3}^{227} + n_{W6}^{227} \end{aligned}$$

125. Lowered SGs by higher-dimensional irreps of pairings in SG 228

The representative operations of SG/T for SG 228:

$$\begin{aligned}
 &1 : (x, y, z), 2 : (x + \frac{1}{4}, \frac{1}{2} - z, y + \frac{1}{4}), 3 : (x + \frac{1}{4}, z + \frac{1}{4}, \frac{1}{2} - y), 4 : (z + \frac{1}{4}, y + \frac{1}{4}, \frac{1}{2} - x), 5 : (\frac{1}{2} - z, y + \frac{1}{4}, x + \frac{1}{4}), \\
 &6 : (\frac{1}{2} - y, x + \frac{1}{4}, z + \frac{1}{4}), 7 : (y + \frac{1}{4}, \frac{1}{2} - x, z + \frac{1}{4}), 8 : (x, \frac{1}{4} - y, \frac{1}{4} - z), 9 : (\frac{1}{4} - x, y, \frac{1}{4} - z), 10 : (\frac{1}{4} - x, \frac{1}{4} - y, z), \\
 &11 : (y + \frac{1}{4}, x + \frac{1}{4}, \frac{1}{2} - z), 12 : (\frac{1}{2} - y, \frac{1}{2} - x, \frac{1}{2} - z), 13 : (\frac{1}{2} - x, z + \frac{1}{4}, y + \frac{1}{4}), 14 : (\frac{1}{2} - x, \frac{1}{2} - z, \frac{1}{2} - y), 15 : (z + \frac{1}{4}, \frac{1}{2} - y, x + \frac{1}{4}), \\
 &16 : (\frac{1}{2} - z, \frac{1}{2} - y, \frac{1}{2} - x), 17 : (z, x, y), 18 : (y, z, x), 19 : (\frac{1}{4} - y, z, \frac{1}{4} - x), 20 : (\frac{1}{4} - z, \frac{1}{4} - x, y), 21 : (\frac{1}{4} - y, \frac{1}{4} - z, x), \\
 &22 : (z, \frac{1}{4} - x, \frac{1}{4} - y), 23 : (y, \frac{1}{4} - z, \frac{1}{4} - x), 24 : (\frac{1}{4} - z, x, \frac{1}{4} - y), 25 : (-x, -y, -z), 26 : (\frac{1}{4} - x, z + \frac{1}{2}, \frac{1}{4} - y), \\
 &27 : (\frac{1}{4} - x, \frac{1}{4} - z, y + \frac{1}{2}), 28 : (\frac{1}{4} - z, \frac{1}{4} - y, x + \frac{1}{2}), 29 : (z + \frac{1}{2}, \frac{1}{4} - y, \frac{1}{4} - x), 30 : (y + \frac{1}{2}, \frac{1}{4} - x, \frac{1}{4} - z), 31 : (\frac{1}{4} - y, x + \frac{1}{2}, \frac{1}{4} - z), \\
 &32 : (-x, y + \frac{1}{4}, z + \frac{1}{4}), 33 : (x + \frac{1}{4}, -y, z + \frac{1}{4}), 34 : (x + \frac{1}{4}, y + \frac{1}{4}, -z), 35 : (\frac{1}{4} - y, \frac{1}{4} - x, z + \frac{1}{2}), 36 : (y + \frac{1}{2}, x + \frac{1}{2}, z + \frac{1}{2}), \\
 &37 : (x + \frac{1}{2}, \frac{1}{4} - z, \frac{1}{4} - y), 38 : (x + \frac{1}{2}, z + \frac{1}{2}, y + \frac{1}{2}), 39 : (\frac{1}{4} - z, y + \frac{1}{2}, \frac{1}{4} - x), 40 : (z + \frac{1}{2}, y + \frac{1}{2}, x + \frac{1}{2}), 41 : (-z, -x, -y), \\
 &42 : (-y, -z, -x), 43 : (y + \frac{1}{4}, -z, x + \frac{1}{4}), 44 : (z + \frac{1}{4}, x + \frac{1}{4}, -y), 45 : (y + \frac{1}{4}, z + \frac{1}{4}, -x), 46 : (-z, x + \frac{1}{4}, y + \frac{1}{4}), \\
 &47 : (-y, z + \frac{1}{4}, x + \frac{1}{4}), 48 : (z + \frac{1}{4}, -x, y + \frac{1}{4}).
 \end{aligned}$$

The lower SG is SG 70 when the preserved operations are: **(sub-SG label is 1) 1, 8, 9, 10, 25, 32, 33, 34.**

The transformation is:  $(\mathbf{a}_{70}, \mathbf{b}_{70}, \mathbf{c}_{70}) = (\mathbf{a}_{228}, \mathbf{b}_{228}, \mathbf{c}_{228}) \begin{pmatrix} 0 & 1 & 0 \\ 1 & 0 & 0 \\ 0 & 0 & -1 \end{pmatrix}, \overrightarrow{O_{228}O_{70}} = \frac{1}{4}\mathbf{a}_{70} + (\frac{1}{4})\mathbf{b}_{70} + (\frac{1}{2})\mathbf{c}_{70}$

The reduction of higher dimensional irrep:

$$\begin{aligned}
 O_h : T_{1g} &\rightarrow B_{1g} + B_{2g} + B_{3g} \text{ of } D_{2h}. \\
 O_h : T_{2g} &\rightarrow B_{1g} + B_{2g} + B_{3g} \text{ of } D_{2h}. \\
 O_h : T_{1u} &\rightarrow B_{1u} + B_{2u} + B_{3u} \text{ of } D_{2h}. \\
 O_h : T_{2u} &\rightarrow B_{1u} + B_{2u} + B_{3u} \text{ of } D_{2h}.
 \end{aligned}$$

The correspondences of irreps at HSPs from original SG to lowered SG:

$$\begin{aligned}
 n_{GM6}^{70} &= 2n_{GM11}^{228} + n_{GM8}^{228} + n_{GM9}^{228} \quad n_{GM5}^{70} = 2n_{GM10}^{228} + n_{GM6}^{228} + n_{GM7}^{228} \quad n_{Y4}^{70} = n_{X5}^{228} \quad n_{Y3}^{70} = n_{X5}^{228} \quad n_{L3}^{70} = n_{L4}^{228} + n_{L5}^{228} + n_{L6}^{228} \\
 n_{L2}^{70} &= n_{L4}^{228} + n_{L5}^{228} + n_{L6}^{228} \quad n_{Z3}^{70} = n_{X5}^{228} \quad n_{Z4}^{70} = n_{X5}^{228} \quad n_{T4}^{70} = n_{X5}^{228} \quad n_{T3}^{70} = n_{X5}^{228}
 \end{aligned}$$

The lower SG is SG 73 when the preserved operations are: **(sub-SG label is 2) 1, 8, 13, 14, 25, 32, 37, 38.**

The transformation is:  $(\mathbf{a}_{73}, \mathbf{b}_{73}, \mathbf{c}_{73}) = (\mathbf{a}_{228}, \mathbf{b}_{228}, \mathbf{c}_{228}) \begin{pmatrix} 0 & 0 & 1 \\ \frac{1}{2} & -\frac{1}{2} & 0 \\ \frac{1}{2} & \frac{1}{2} & 0 \end{pmatrix}, \overrightarrow{O_{228}O_{73}} = \frac{1}{4}\mathbf{a}_{73} + (-\frac{1}{4})\mathbf{b}_{73} + (\frac{1}{4})\mathbf{c}_{73}$

The reduction of higher dimensional irrep:

$$\begin{aligned}
 O_h : T_{1g} &\rightarrow B_{2g} + B_{1g} + B_{3g} \text{ of } D_{2h}. \\
 O_h : T_{2g} &\rightarrow A_g + B_{2g} + B_{3g} \text{ of } D_{2h}. \\
 O_h : T_{1u} &\rightarrow B_{2u} + B_{1u} + B_{3u} \text{ of } D_{2h}. \\
 O_h : T_{2u} &\rightarrow A_u + B_{2u} + B_{3u} \text{ of } D_{2h}.
 \end{aligned}$$

The correspondences of irreps at HSPs from original SG to lowered SG:

$$\begin{aligned}
 n_{GM6}^{73} &= 2n_{GM11}^{228} + n_{GM8}^{228} + n_{GM9}^{228} \quad n_{GM5}^{73} = 2n_{GM10}^{228} + n_{GM6}^{228} + n_{GM7}^{228} \quad n_{X6}^{73} = n_{X5}^{228} \quad n_{X5}^{73} = n_{X5}^{228} \quad n_{T2}^{73} = 2n_{X5}^{228} \quad n_{W3}^{73} = n_{W7}^{228} \\
 n_{W2}^{73} &= n_{W4}^{228} + n_{W6}^{228} \quad n_{W4}^{73} = n_{W3}^{228} + n_{W5}^{228} \quad n_{W5}^{73} = n_{W7}^{228} \quad n_{R2}^{73} = n_{L4}^{228} + n_{L5}^{228} + n_{L6}^{228} \quad n_{S2}^{73} = n_{L4}^{228} + n_{L5}^{228} + n_{L6}^{228}
 \end{aligned}$$

The lower SG is SG 73 when the preserved operations are: **(sub-SG label is 3) 1, 9, 16, 15, 25, 33, 40, 39.**

The transformation is:  $(\mathbf{a}_{73}, \mathbf{b}_{73}, \mathbf{c}_{73}) = (\mathbf{a}_{228}, \mathbf{b}_{228}, \mathbf{c}_{228}) \begin{pmatrix} -\frac{1}{2} & 0 & -\frac{1}{2} \\ 0 & 1 & 0 \\ \frac{1}{2} & 0 & -\frac{1}{2} \end{pmatrix}, \overrightarrow{O_{228}O_{73}} = \frac{1}{4}\mathbf{a}_{73} + (-\frac{1}{4})\mathbf{b}_{73} + (\frac{1}{4})\mathbf{c}_{73}$

The reduction of higher dimensional irrep:

$$\begin{aligned}
 O_h : T_{1g} &\rightarrow B_{2g} + B_{1g} + B_{3g} \text{ of } D_{2h}. \\
 O_h : T_{2g} &\rightarrow A_g + B_{1g} + B_{3g} \text{ of } D_{2h}. \\
 O_h : T_{1u} &\rightarrow B_{2u} + B_{1u} + B_{3u} \text{ of } D_{2h}. \\
 O_h : T_{2u} &\rightarrow A_u + B_{1u} + B_{3u} \text{ of } D_{2h}.
 \end{aligned}$$

The correspondences of irreps at HSPs from original SG to lowered SG:

$$\begin{aligned}
 n_{GM6}^{73} &= 2n_{GM11}^{228} + n_{GM8}^{228} + n_{GM9}^{228} \quad n_{GM5}^{73} = 2n_{GM10}^{228} + n_{GM6}^{228} + n_{GM7}^{228} \quad n_{X6}^{73} = n_{X5}^{228} \quad n_{X5}^{73} = n_{X5}^{228} \quad n_{T2}^{73} = n_{L4}^{228} + n_{L5}^{228} + n_{L6}^{228} \\
 n_{W3}^{73} &= n_{W3}^{228} + n_{W5}^{228} \quad n_{W2}^{73} = n_{W7}^{228} \quad n_{W4}^{73} = n_{W4}^{228} + n_{W6}^{228} \quad n_{W5}^{73} = n_{W7}^{228} \quad n_{R2}^{73} = 2n_{X5}^{228} \quad n_{S2}^{73} = n_{L4}^{228} + n_{L5}^{228} + n_{L6}^{228}
 \end{aligned}$$

The lower SG is SG 73 when the preserved operations are: **(sub-SG label is 4) 1, 10, 11, 12, 25, 34, 35, 36.**

The transformation is:  $(\mathbf{a}_{73}, \mathbf{b}_{73}, \mathbf{c}_{73}) = (\mathbf{a}_{228}, \mathbf{b}_{228}, \mathbf{c}_{228}) \begin{pmatrix} \frac{1}{2} & -\frac{1}{2} & 0 \\ \frac{1}{2} & \frac{1}{2} & 0 \\ 0 & 0 & 1 \end{pmatrix}, \overrightarrow{O_{228}O_{73}} = \frac{1}{4}\mathbf{a}_{73} + (-\frac{1}{4})\mathbf{b}_{73} + (\frac{1}{4})\mathbf{c}_{73}$

The reduction of higher dimensional irrep:

- $O_h : T_{1g} \rightarrow B_{2g} + B_{1g} + B_{3g}$  of  $D_{2h}$ .
- $O_h : T_{2g} \rightarrow A_g + B_{2g} + B_{3g}$  of  $D_{2h}$ .
- $O_h : T_{1u} \rightarrow B_{2u} + B_{1u} + B_{3u}$  of  $D_{2h}$ .
- $O_h : T_{2u} \rightarrow A_u + B_{2u} + B_{3u}$  of  $D_{2h}$ .

The correspondences of irreps at HSPs from original SG to lowered SG:

$$\begin{aligned} n_{GM6}^{73} &= 2n_{GM11}^{228} + n_{GM8}^{228} + n_{GM9}^{228} \quad n_{GM5}^{73} = 2n_{GM10}^{228} + n_{GM6}^{228} + n_{GM7}^{228} \quad n_{X6}^{73} = n_{X5}^{228} \quad n_{X5}^{73} = n_{X5}^{228} \quad n_{T2}^{73} = 2n_{X5}^{228} \quad n_{W3}^{73} = n_{W2}^{228} \\ n_{W2}^{73} &= n_{W4}^{228} + n_{W6}^{228} \quad n_{W4}^{73} = n_{W3}^{228} + n_{W5}^{228} \quad n_{W5}^{73} = n_{W7}^{228} \quad n_{R2}^{73} = n_{L4}^{228} + n_{L5}^{228} + n_{L6}^{228} \quad n_{S2}^{73} = n_{L4}^{228} + n_{L5}^{228} + n_{L6}^{228} \end{aligned}$$

The lower SG is SG 88 when the preserved operations are: **(sub-SG label is 5)** 1, 6, 7, 10, 25, 30, 31, 34.

The transformation is:  $(\mathbf{a}_{88}, \mathbf{b}_{88}, \mathbf{c}_{88}) = (\mathbf{a}_{228}, \mathbf{b}_{228}, \mathbf{c}_{228}) \begin{pmatrix} \frac{1}{2} & \frac{1}{2} & 0 \\ -\frac{1}{2} & \frac{1}{2} & 0 \\ 0 & 0 & 1 \end{pmatrix}, \overrightarrow{O_{228}O_{88}} = \frac{1}{2}\mathbf{a}_{88}$

The reduction of higher dimensional irrep:

- $O_h : T_{1g} \rightarrow A_g + {}^2E_g + {}^1E_g$  of  $C_{4h}$ .
- $O_h : T_{2g} \rightarrow {}^2E_g + B_g + {}^1E_g$  of  $C_{4h}$ .
- $O_h : T_{1u} \rightarrow A_u + {}^2E_u + {}^1E_u$  of  $C_{4h}$ .
- $O_h : T_{2u} \rightarrow {}^2E_u + B_u + {}^1E_u$  of  $C_{4h}$ .

The correspondences of irreps at HSPs from original SG to lowered SG:

$$\begin{aligned} n_{GM9}^{88} &= n_{GM11}^{228} + n_{GM9}^{228} \quad n_{GM5}^{88} = n_{GM10}^{228} + n_{GM7}^{228} \quad n_{GM11}^{88} = n_{GM11}^{228} + n_{GM9}^{228} \quad n_{GM7}^{88} = n_{GM10}^{228} + n_{GM7}^{228} \quad n_{GM12}^{88} = \\ n_{GM11}^{228} + n_{GM8}^{228} \quad n_{GM8}^{88} &= n_{GM10}^{228} + n_{GM6}^{228} \quad n_{GM10}^{88} = n_{GM11}^{228} + n_{GM8}^{228} \quad n_{GM6}^{88} = n_{GM10}^{228} + n_{GM6}^{228} \quad n_{M4}^{88} = n_{X5}^{228} \quad n_{M3}^{88} = \\ n_{X5}^{228} \quad n_{X2}^{88} &= 2n_{X5}^{228} \quad n_{P5}^{88} = n_{W3}^{228} + n_{W4}^{228} \quad n_{P6}^{88} = n_{W5}^{228} + n_{W6}^{228} \quad n_{P7}^{88} = n_{W7}^{228} \quad n_{P8}^{88} = n_{W7}^{228} \quad n_{N3}^{88} = n_{L4}^{228} + n_{L5}^{228} + n_{L6}^{228} \quad n_{N2}^{88} = \\ n_{L4}^{228} + n_{L5}^{228} + n_{L6}^{228} \end{aligned}$$

The lower SG is SG 88 when the preserved operations are: **(sub-SG label is 6)** 1, 2, 3, 8, 25, 26, 27, 32.

The transformation is:  $(\mathbf{a}_{88}, \mathbf{b}_{88}, \mathbf{c}_{88}) = (\mathbf{a}_{228}, \mathbf{b}_{228}, \mathbf{c}_{228}) \begin{pmatrix} 0 & 0 & 1 \\ \frac{1}{2} & \frac{1}{2} & 0 \\ -\frac{1}{2} & \frac{1}{2} & 0 \end{pmatrix}, \overrightarrow{O_{228}O_{88}} = \frac{1}{2}\mathbf{a}_{88}$

The reduction of higher dimensional irrep:

- $O_h : T_{1g} \rightarrow A_g + {}^2E_g + {}^1E_g$  of  $C_{4h}$ .
- $O_h : T_{2g} \rightarrow {}^2E_g + B_g + {}^1E_g$  of  $C_{4h}$ .
- $O_h : T_{1u} \rightarrow A_u + {}^2E_u + {}^1E_u$  of  $C_{4h}$ .
- $O_h : T_{2u} \rightarrow {}^2E_u + B_u + {}^1E_u$  of  $C_{4h}$ .

The correspondences of irreps at HSPs from original SG to lowered SG:

$$\begin{aligned} n_{GM9}^{88} &= n_{GM11}^{228} + n_{GM9}^{228} \quad n_{GM5}^{88} = n_{GM10}^{228} + n_{GM7}^{228} \quad n_{GM11}^{88} = n_{GM11}^{228} + n_{GM9}^{228} \quad n_{GM7}^{88} = n_{GM10}^{228} + n_{GM7}^{228} \quad n_{GM12}^{88} = \\ n_{GM11}^{228} + n_{GM8}^{228} \quad n_{GM8}^{88} &= n_{GM10}^{228} + n_{GM6}^{228} \quad n_{GM10}^{88} = n_{GM11}^{228} + n_{GM8}^{228} \quad n_{GM6}^{88} = n_{GM10}^{228} + n_{GM6}^{228} \quad n_{M4}^{88} = n_{X5}^{228} \quad n_{M3}^{88} = \\ n_{X5}^{228} \quad n_{X2}^{88} &= 2n_{X5}^{228} \quad n_{P5}^{88} = n_{W3}^{228} + n_{W4}^{228} \quad n_{P6}^{88} = n_{W5}^{228} + n_{W6}^{228} \quad n_{P7}^{88} = n_{W7}^{228} \quad n_{P8}^{88} = n_{W7}^{228} \quad n_{N3}^{88} = n_{L4}^{228} + n_{L5}^{228} + n_{L6}^{228} \quad n_{N2}^{88} = \\ n_{L4}^{228} + n_{L5}^{228} + n_{L6}^{228} \end{aligned}$$

The lower SG is SG 88 when the preserved operations are: **(sub-SG label is 7)** 1, 4, 5, 9, 25, 28, 29, 33.

The transformation is:  $(\mathbf{a}_{88}, \mathbf{b}_{88}, \mathbf{c}_{88}) = (\mathbf{a}_{228}, \mathbf{b}_{228}, \mathbf{c}_{228}) \begin{pmatrix} -\frac{1}{2} & -\frac{1}{2} & 0 \\ 0 & 0 & -1 \\ \frac{1}{2} & -\frac{1}{2} & 0 \end{pmatrix}, \overrightarrow{O_{228}O_{88}} = \frac{1}{2}\mathbf{a}_{88}$

The reduction of higher dimensional irrep:

- $O_h : T_{1g} \rightarrow A_g + {}^2E_g + {}^1E_g$  of  $C_{4h}$ .
- $O_h : T_{2g} \rightarrow {}^2E_g + B_g + {}^1E_g$  of  $C_{4h}$ .
- $O_h : T_{1u} \rightarrow A_u + {}^2E_u + {}^1E_u$  of  $C_{4h}$ .
- $O_h : T_{2u} \rightarrow {}^2E_u + B_u + {}^1E_u$  of  $C_{4h}$ .

The correspondences of irreps at HSPs from original SG to lowered SG:

$$\begin{aligned} n_{GM9}^{88} &= n_{GM11}^{228} + n_{GM9}^{228} \quad n_{GM5}^{88} = n_{GM10}^{228} + n_{GM7}^{228} \quad n_{GM11}^{88} = n_{GM11}^{228} + n_{GM9}^{228} \quad n_{GM7}^{88} = n_{GM10}^{228} + n_{GM7}^{228} \quad n_{GM12}^{88} = \\ n_{GM11}^{228} + n_{GM8}^{228} \quad n_{GM8}^{88} &= n_{GM10}^{228} + n_{GM6}^{228} \quad n_{GM10}^{88} = n_{GM11}^{228} + n_{GM8}^{228} \quad n_{GM6}^{88} = n_{GM10}^{228} + n_{GM6}^{228} \quad n_{M4}^{88} = n_{X5}^{228} \quad n_{M3}^{88} = \\ n_{X5}^{228} \quad n_{X2}^{88} &= 2n_{X5}^{228} \quad n_{P5}^{88} = n_{W3}^{228} + n_{W4}^{228} \quad n_{P6}^{88} = n_{W5}^{228} + n_{W6}^{228} \quad n_{P7}^{88} = n_{W7}^{228} \quad n_{P8}^{88} = n_{W7}^{228} \quad n_{N3}^{88} = n_{L4}^{228} + n_{L5}^{228} + n_{L6}^{228} \quad n_{N2}^{88} = \\ n_{L4}^{228} + n_{L5}^{228} + n_{L6}^{228} \end{aligned}$$

The lower SG is SG 142 when the preserved operations are: **(sub-SG label is 8)** 1, 6, 7, 10, 8, 9, 11, 12, 25, 30, 31, 34, 32, 33,

35, 36.

The transformation is:  $(\mathbf{a}_{142}, \mathbf{b}_{142}, \mathbf{c}_{142}) = (\mathbf{a}_{228}, \mathbf{b}_{228}, \mathbf{c}_{228}) \begin{pmatrix} -\frac{1}{2} & -\frac{1}{2} & 0 \\ \frac{1}{2} & -\frac{1}{2} & 0 \\ 0 & 0 & 1 \end{pmatrix}, \overrightarrow{O_{228}O_{142}} = -\frac{1}{2}\mathbf{a}_{142}$

The reduction of higher dimensional irrep:

$$O_h : E_g \rightarrow A_{1g} + B_{2g} \text{ of } D_{4h}.$$

$$O_h : E_u \rightarrow A_{1u} + B_{2u} \text{ of } D_{4h}.$$

The correspondences of irreps at HSPs from original SG to lowered SG:

$$\begin{aligned} n_{GM8}^{142} &= n_{GM11}^{228} + n_{GM9}^{228} & n_{GM6}^{142} &= n_{GM10}^{228} + n_{GM7}^{228} & n_{GM9}^{142} &= n_{GM11}^{228} + n_{GM8}^{228} & n_{GM7}^{142} &= n_{GM10}^{228} + n_{GM6}^{228} & n_{M5}^{142} &= n_{X5}^{228} & n_{X3}^{142} &= \\ n_{X5}^{228} & n_{X4}^{142} &= n_{X5}^{228} & n_{P3}^{142} &= n_{W3}^{228} & n_{P5}^{142} &= n_{W5}^{228} & n_{P6}^{142} &= n_{W4}^{228} & n_{P4}^{142} &= n_{W6}^{228} & n_{P7}^{142} &= n_{W7}^{228} & n_{N2}^{142} &= n_{L4}^{228} + n_{L5}^{228} + n_{L6}^{228} \end{aligned}$$

The lower SG is SG 142 when the preserved operations are: (**sub-SG label is 9**) 1, 2, 3, 8, 9, 10, 13, 14, 25, 26, 27, 32, 33, 34, 37, 38.

The transformation is:  $(\mathbf{a}_{142}, \mathbf{b}_{142}, \mathbf{c}_{142}) = (\mathbf{a}_{228}, \mathbf{b}_{228}, \mathbf{c}_{228}) \begin{pmatrix} 0 & 0 & 1 \\ -\frac{1}{2} & -\frac{1}{2} & 0 \\ \frac{1}{2} & -\frac{1}{2} & 0 \end{pmatrix}, \overrightarrow{O_{228}O_{142}} = -\frac{1}{2}\mathbf{a}_{142}$

The reduction of higher dimensional irrep:

$$O_h : E_g \rightarrow A_{1g} + B_{2g} \text{ of } D_{4h}.$$

$$O_h : E_u \rightarrow A_{1u} + B_{2u} \text{ of } D_{4h}.$$

The correspondences of irreps at HSPs from original SG to lowered SG:

$$\begin{aligned} n_{GM8}^{142} &= n_{GM11}^{228} + n_{GM9}^{228} & n_{GM6}^{142} &= n_{GM10}^{228} + n_{GM7}^{228} & n_{GM9}^{142} &= n_{GM11}^{228} + n_{GM8}^{228} & n_{GM7}^{142} &= n_{GM10}^{228} + n_{GM6}^{228} & n_{M5}^{142} &= n_{X5}^{228} & n_{X3}^{142} &= \\ n_{X5}^{228} & n_{X4}^{142} &= n_{X5}^{228} & n_{P3}^{142} &= n_{W3}^{228} & n_{P5}^{142} &= n_{W5}^{228} & n_{P6}^{142} &= n_{W4}^{228} & n_{P4}^{142} &= n_{W6}^{228} & n_{P7}^{142} &= n_{W7}^{228} & n_{N2}^{142} &= n_{L4}^{228} + n_{L5}^{228} + n_{L6}^{228} \end{aligned}$$

The lower SG is SG 142 when the preserved operations are: (**sub-SG label is 10**) 1, 4, 5, 9, 10, 8, 16, 15, 25, 28, 29, 33, 34, 32, 40, 39.

The transformation is:  $(\mathbf{a}_{142}, \mathbf{b}_{142}, \mathbf{c}_{142}) = (\mathbf{a}_{228}, \mathbf{b}_{228}, \mathbf{c}_{228}) \begin{pmatrix} \frac{1}{2} & \frac{1}{2} & 0 \\ 0 & 0 & -1 \\ -\frac{1}{2} & \frac{1}{2} & 0 \end{pmatrix}, \overrightarrow{O_{228}O_{142}} = -\frac{1}{2}\mathbf{a}_{142}$

The reduction of higher dimensional irrep:

$$O_h : E_g \rightarrow A_{1g} + B_{2g} \text{ of } D_{4h}.$$

$$O_h : E_u \rightarrow A_{1u} + B_{2u} \text{ of } D_{4h}.$$

The correspondences of irreps at HSPs from original SG to lowered SG:

$$\begin{aligned} n_{GM8}^{142} &= n_{GM11}^{228} + n_{GM9}^{228} & n_{GM6}^{142} &= n_{GM10}^{228} + n_{GM7}^{228} & n_{GM9}^{142} &= n_{GM11}^{228} + n_{GM8}^{228} & n_{GM7}^{142} &= n_{GM10}^{228} + n_{GM6}^{228} & n_{M5}^{142} &= n_{X5}^{228} & n_{X3}^{142} &= \\ n_{X5}^{228} & n_{X4}^{142} &= n_{X5}^{228} & n_{P3}^{142} &= n_{W3}^{228} & n_{P5}^{142} &= n_{W5}^{228} & n_{P6}^{142} &= n_{W4}^{228} & n_{P4}^{142} &= n_{W6}^{228} & n_{P7}^{142} &= n_{W7}^{228} & n_{N2}^{142} &= n_{L4}^{228} + n_{L5}^{228} + n_{L6}^{228} \end{aligned}$$

The lower SG is SG 148 when the preserved operations are: (**sub-SG label is 11**) 1, 17, 18, 25, 41, 42.

The transformation is:  $(\mathbf{a}_{148}, \mathbf{b}_{148}, \mathbf{c}_{148}) = (\mathbf{a}_{228}, \mathbf{b}_{228}, \mathbf{c}_{228}) \begin{pmatrix} \frac{1}{2} & 0 & \frac{1}{2} \\ \frac{1}{2} & \frac{1}{2} & 0 \\ 0 & \frac{1}{2} & \frac{1}{2} \end{pmatrix}, \overrightarrow{O_{228}O_{148}} = \mathbf{0}$

The reduction of higher dimensional irrep:

$$O_h : T_{1g} \rightarrow A_g + {}^2E_g + {}^1E_g \text{ of } C_{3i}.$$

$$O_h : T_{2g} \rightarrow A_g + {}^2E_g + {}^1E_g \text{ of } C_{3i}.$$

$$O_h : T_{1u} \rightarrow {}^1E_u + A_u + {}^2E_u \text{ of } C_{3i}.$$

$$O_h : T_{2u} \rightarrow {}^1E_u + A_u + {}^2E_u \text{ of } C_{3i}.$$

The correspondences of irreps at HSPs from original SG to lowered SG:

$$\begin{aligned} n_{GM7}^{148} &= 2n_{GM11}^{228} & n_{GM4}^{148} &= 2n_{GM10}^{228} & n_{GM9}^{148} &= n_{GM11}^{228} + n_{GM8}^{228} + n_{GM9}^{228} & n_{GM6}^{148} &= n_{GM10}^{228} + n_{GM6}^{228} + n_{GM7}^{228} & n_{GM8}^{148} &= \\ n_{GM11}^{228} & + n_{GM8}^{228} + n_{GM9}^{228} & n_{GM5}^{148} &= n_{GM10}^{228} + n_{GM6}^{228} + n_{GM7}^{228} & n_{L2}^{148} &= n_{L4}^{228} + n_{L5}^{228} + n_{L6}^{228} & n_{L3}^{148} &= n_{L4}^{228} + n_{L5}^{228} + n_{L6}^{228} & n_{F2}^{148} &= \\ 2n_{X5}^{228} & n_{F3}^{148} &= 2n_{X5}^{228} & n_{T7}^{148} &= n_{L4}^{228} & n_{T4}^{148} &= n_{L4}^{228} & n_{T9}^{148} &= n_{L5}^{228} & n_{T6}^{148} &= n_{L6}^{228} & n_{T8}^{148} &= n_{L6}^{228} & n_{T5}^{148} &= n_{L5}^{228} \end{aligned}$$

The lower SG is SG 148 when the preserved operations are: (**sub-SG label is 12**) 1, 24, 23, 25, 48, 47.

The transformation is:  $(\mathbf{a}_{148}, \mathbf{b}_{148}, \mathbf{c}_{148}) = (\mathbf{a}_{228}, \mathbf{b}_{228}, \mathbf{c}_{228}) \begin{pmatrix} -\frac{1}{2} & -\frac{1}{2} & 0 \\ 0 & -\frac{1}{2} & -\frac{1}{2} \\ \frac{1}{2} & 0 & \frac{1}{2} \end{pmatrix}, \overrightarrow{O_{228}O_{148}} = \frac{1}{2}\mathbf{b}_{148}$

The reduction of higher dimensional irrep:

$$O_h : T_{1g} \rightarrow A_g + {}^2E_g + {}^1E_g \text{ of } C_{3i}.$$

$$O_h : T_{2g} \rightarrow A_g + {}^2E_g + {}^1E_g \text{ of } C_{3i}.$$

$$O_h : T_{1u} \rightarrow {}^1E_u + A_u + {}^2E_u \text{ of } C_{3i}.$$

$$O_h : T_{2u} \rightarrow {}^1E_u + A_u + {}^2E_u \text{ of } C_{3i}.$$

The correspondences of irreps at HSPs from original SG to lowered SG:

$$\begin{aligned} n_{GM7}^{148} &= 2n_{GM11}^{228} n_{GM4}^{148} = 2n_{GM10}^{228} n_{GM9}^{148} = n_{GM11}^{228} + n_{GM8}^{228} + n_{GM9}^{228} n_{GM6}^{148} = n_{GM10}^{228} + n_{GM6}^{228} + n_{GM7}^{228} n_{GM8}^{148} = \\ n_{GM11}^{228} + n_{GM8}^{228} + n_{GM9}^{228} n_{GM5}^{148} &= n_{GM10}^{228} + n_{GM6}^{228} + n_{GM7}^{228} n_{L2}^{148} = n_{L4}^{228} + n_{L5}^{228} + n_{L6}^{228} n_{L3}^{148} = n_{L4}^{228} + n_{L5}^{228} + n_{L6}^{228} n_{F2}^{148} = \\ 2n_{X5}^{228} n_{F3}^{148} &= 2n_{X5}^{228} n_{T7}^{148} = n_{L4}^{228} n_{T4}^{148} = n_{L4}^{228} n_{T9}^{148} = n_{L5}^{228} n_{T6}^{148} = n_{L6}^{228} n_{T8}^{148} = n_{L6}^{228} n_{T5}^{148} = n_{L5}^{228} \end{aligned}$$

The lower SG is SG 148 when the preserved operations are: **(sub-SG label is 13)** 1, 20, 19, 25, 44, 43.

The transformation is:  $(\mathbf{a}_{148}, \mathbf{b}_{148}, \mathbf{c}_{148}) = (\mathbf{a}_{228}, \mathbf{b}_{228}, \mathbf{c}_{228}) \begin{pmatrix} \frac{1}{2} & 0 & \frac{1}{2} \\ -\frac{1}{2} & -\frac{1}{2} & 0 \\ 0 & -\frac{1}{2} & -\frac{1}{2} \end{pmatrix}, \overrightarrow{O_{228}O_{148}} = \frac{1}{2}\mathbf{b}_{148}$

The reduction of higher dimensional irrep:

$$\begin{aligned} O_h : T_{1g} &\rightarrow A_g + {}^2E_g + {}^1E_g \text{ of } C_{3i}. \\ O_h : T_{2g} &\rightarrow A_g + {}^2E_g + {}^1E_g \text{ of } C_{3i}. \\ O_h : T_{1u} &\rightarrow {}^1E_u + A_u + {}^2E_u \text{ of } C_{3i}. \\ O_h : T_{2u} &\rightarrow {}^1E_u + A_u + {}^2E_u \text{ of } C_{3i}. \end{aligned}$$

The correspondences of irreps at HSPs from original SG to lowered SG:

$$\begin{aligned} n_{GM7}^{148} &= 2n_{GM11}^{228} n_{GM4}^{148} = 2n_{GM10}^{228} n_{GM9}^{148} = n_{GM11}^{228} + n_{GM8}^{228} + n_{GM9}^{228} n_{GM6}^{148} = n_{GM10}^{228} + n_{GM6}^{228} + n_{GM7}^{228} n_{GM8}^{148} = \\ n_{GM11}^{228} + n_{GM8}^{228} + n_{GM9}^{228} n_{GM5}^{148} &= n_{GM10}^{228} + n_{GM6}^{228} + n_{GM7}^{228} n_{L2}^{148} = n_{L4}^{228} + n_{L5}^{228} + n_{L6}^{228} n_{L3}^{148} = n_{L4}^{228} + n_{L5}^{228} + n_{L6}^{228} n_{F2}^{148} = \\ 2n_{X5}^{228} n_{F3}^{148} &= 2n_{X5}^{228} n_{T7}^{148} = n_{L4}^{228} n_{T4}^{148} = n_{L4}^{228} n_{T9}^{148} = n_{L5}^{228} n_{T6}^{148} = n_{L6}^{228} n_{T8}^{148} = n_{L6}^{228} n_{T5}^{148} = n_{L5}^{228} \end{aligned}$$

The lower SG is SG 148 when the preserved operations are: **(sub-SG label is 14)** 1, 22, 21, 25, 46, 45.

The transformation is:  $(\mathbf{a}_{148}, \mathbf{b}_{148}, \mathbf{c}_{148}) = (\mathbf{a}_{228}, \mathbf{b}_{228}, \mathbf{c}_{228}) \begin{pmatrix} -\frac{1}{2} & -\frac{1}{2} & 0 \\ 0 & \frac{1}{2} & \frac{1}{2} \\ -\frac{1}{2} & 0 & -\frac{1}{2} \end{pmatrix}, \overrightarrow{O_{228}O_{148}} = \frac{1}{2}\mathbf{b}_{148} + (\frac{1}{2})\mathbf{c}_{148}$

The reduction of higher dimensional irrep:

$$\begin{aligned} O_h : T_{1g} &\rightarrow A_g + {}^2E_g + {}^1E_g \text{ of } C_{3i}. \\ O_h : T_{2g} &\rightarrow A_g + {}^2E_g + {}^1E_g \text{ of } C_{3i}. \\ O_h : T_{1u} &\rightarrow {}^1E_u + A_u + {}^2E_u \text{ of } C_{3i}. \\ O_h : T_{2u} &\rightarrow {}^1E_u + A_u + {}^2E_u \text{ of } C_{3i}. \end{aligned}$$

The correspondences of irreps at HSPs from original SG to lowered SG:

$$\begin{aligned} n_{GM7}^{148} &= 2n_{GM11}^{228} n_{GM4}^{148} = 2n_{GM10}^{228} n_{GM9}^{148} = n_{GM11}^{228} + n_{GM8}^{228} + n_{GM9}^{228} n_{GM6}^{148} = n_{GM10}^{228} + n_{GM6}^{228} + n_{GM7}^{228} n_{GM8}^{148} = \\ n_{GM11}^{228} + n_{GM8}^{228} + n_{GM9}^{228} n_{GM5}^{148} &= n_{GM10}^{228} + n_{GM6}^{228} + n_{GM7}^{228} n_{L2}^{148} = n_{L4}^{228} + n_{L5}^{228} + n_{L6}^{228} n_{L3}^{148} = n_{L4}^{228} + n_{L5}^{228} + n_{L6}^{228} n_{F2}^{148} = \\ 2n_{X5}^{228} n_{F3}^{148} &= 2n_{X5}^{228} n_{T7}^{148} = n_{L4}^{228} n_{T4}^{148} = n_{L4}^{228} n_{T9}^{148} = n_{L5}^{228} n_{T6}^{148} = n_{L5}^{228} n_{T8}^{148} = n_{L5}^{228} n_{T5}^{148} = n_{L6}^{228} \end{aligned}$$

The lower SG is SG 203 when the preserved operations are: **(sub-SG label is 15)** 1, 8, 9, 10, 17, 24, 20, 22, 18, 23, 19, 21, 25, 32, 33, 34, 41, 48, 44, 46, 42, 47, 43, 45.

The transformation is:  $(\mathbf{a}_{203}, \mathbf{b}_{203}, \mathbf{c}_{203}) = (\mathbf{a}_{228}, \mathbf{b}_{228}, \mathbf{c}_{228}) \begin{pmatrix} 0 & 0 & -1 \\ 1 & 0 & 0 \\ 0 & -1 & 0 \end{pmatrix}, \overrightarrow{O_{228}O_{203}} = \frac{1}{2}\mathbf{a}_{203} + (\frac{1}{4})\mathbf{b}_{203} + (\frac{1}{4})\mathbf{c}_{203}$

The reduction of higher dimensional irrep:

$$\begin{aligned} O_h : E_g &\rightarrow {}^1E_g + {}^2E_g \text{ of } T_h. \\ O_h : E_u &\rightarrow {}^1E_u + {}^2E_u \text{ of } T_h. \end{aligned}$$

The correspondences of irreps at HSPs from original SG to lowered SG:

$$\begin{aligned} n_{GM9}^{203} &= n_{GM11}^{228} n_{GM6}^{203} = n_{GM10}^{228} n_{GM10}^{203} = n_{GM11}^{228} n_{GM7}^{203} = n_{GM10}^{228} n_{GM8}^{203} = n_{GM8}^{228} + n_{GM9}^{228} n_{GM5}^{203} = n_{GM6}^{228} + n_{GM7}^{228} n_{X4}^{203} = \\ n_{GM11}^{228} n_{X3}^{203} &= n_{X5}^{228} n_{L7}^{203} = n_{L4}^{228} n_{L4}^{203} = n_{L4}^{228} n_{L9}^{203} = n_{L6}^{228} n_{L6}^{203} = n_{L5}^{228} n_{L8}^{203} = n_{L5}^{228} n_{L5}^{203} = n_{L6}^{228} n_{W2}^{203} = n_{W7}^{228} n_{W4}^{203} = n_{W7}^{228} \\ n_{W3}^{203} &= n_{W3}^{228} + n_{W6}^{228} n_{W5}^{203} = n_{W4}^{228} + n_{W5}^{228} \end{aligned}$$

**126. Lowered SGs by higher-dimensional irreps of pairings in SG 229**

The representative operations of SG/T for SG 229:

$$\begin{aligned} 1 : (x, y, z), 2 : (x, -z, y), 3 : (x, z, -y), 4 : (z, y, -x), 5 : (-z, y, x), 6 : (-y, x, z), 7 : (y, -x, z), 8 : (x, -y, -z), \\ 9 : (-x, y, -z), 10 : (-x, -y, z), 11 : (y, x, -z), 12 : (-y, -x, -z), 13 : (-x, z, y), 14 : (-x, -z, -y), 15 : (z, -y, x), \\ 16 : (-z, -y, -x), 17 : (z, x, y), 18 : (y, z, x), 19 : (-y, z, -x), 20 : (-z, -x, y), 21 : (-y, -z, x), 22 : (z, -x, -y), 23 : \end{aligned}$$

(y, -z, -x), 24 : (-z, x, -y), 25 : (-x, -y, -z), 26 : (-x, z, -y), 27 : (-x, -z, y), 28 : (-z, -y, x), 29 : (z, -y, -x),  
 30 : (y, -x, -z), 31 : (-y, x, -z), 32 : (-x, y, z), 33 : (x, -y, z), 34 : (x, y, -z), 35 : (-y, -x, z), 36 : (y, x, z),  
 37 : (x, -z, -y), 38 : (x, z, y), 39 : (-z, y, -x), 40 : (z, y, x), 41 : (-z, -x, -y), 42 : (-y, -z, -x), 43 : (y, -z, x),  
 44 : (z, x, -y), 45 : (y, z, -x), 46 : (-z, x, y), 47 : (-y, z, x), 48 : (z, -x, y).

The lower SG is SG 71 when the preserved operations are: **(sub-SG label is 1) 1, 8, 9, 10, 25, 32, 33, 34.**

The transformation is:  $(\mathbf{a}_{71}, \mathbf{b}_{71}, \mathbf{c}_{71}) = (\mathbf{a}_{229}, \mathbf{b}_{229}, \mathbf{c}_{229}) \begin{pmatrix} 0 & 0 & 1 \\ 1 & 0 & 0 \\ 0 & 1 & 0 \end{pmatrix}, \overrightarrow{O_{229}O_{71}} = -\frac{1}{2}\mathbf{b}_{71}$

The reduction of higher dimensional irrep:

$$O_h : T_{1g} \rightarrow B_{2g} + B_{1g} + B_{3g} \text{ of } D_{2h}.$$

$$O_h : T_{2g} \rightarrow B_{2g} + B_{1g} + B_{3g} \text{ of } D_{2h}.$$

$$O_h : T_{1u} \rightarrow B_{2u} + B_{1u} + B_{3u} \text{ of } D_{2h}.$$

$$O_h : T_{2u} \rightarrow B_{2u} + B_{1u} + B_{3u} \text{ of } D_{2h}.$$

The correspondences of irreps at HSPs from original SG to lowered SG:

$$\begin{aligned} n_{GM6}^{71} &= 2n_{GM11}^{229} + n_{GM8}^{229} + n_{GM9}^{229} & n_{GM5}^{71} &= 2n_{GM10}^{229} + n_{GM6}^{229} + n_{GM7}^{229} & n_{X6}^{71} &= 2n_{H11}^{229} + n_{H8}^{229} + n_{H9}^{229} & n_{X5}^{71} &= 2n_{H10}^{229} + n_{H6}^{229} + n_{H7}^{229} \\ n_{T6}^{71} &= n_{N5}^{229} & n_{T4}^{71} &= n_{N6}^{229} & n_{T5}^{71} &= n_{N5}^{229} & n_{T3}^{71} &= n_{N6}^{229} & n_{W5}^{71} &= n_{P6}^{229} + n_{P7}^{229} + 2n_{P8}^{229} & n_{R6}^{71} &= n_{N6}^{229} & n_{R4}^{71} &= n_{N5}^{229} & n_{R5}^{71} &= n_{N6}^{229} & n_{R3}^{71} &= n_{N5}^{229} \end{aligned}$$

The lower SG is SG 69 when the preserved operations are: **(sub-SG label is 2) 1, 8, 13, 14, 25, 32, 37, 38.**

The transformation is:  $(\mathbf{a}_{69}, \mathbf{b}_{69}, \mathbf{c}_{69}) = (\mathbf{a}_{229}, \mathbf{b}_{229}, \mathbf{c}_{229}) \begin{pmatrix} 0 & 0 & 1 \\ 1 & -1 & 0 \\ 1 & 1 & 0 \end{pmatrix}, \overrightarrow{O_{229}O_{69}} = \mathbf{0}$

The reduction of higher dimensional irrep:

$$O_h : T_{1g} \rightarrow B_{2g} + B_{1g} + B_{3g} \text{ of } D_{2h}.$$

$$O_h : T_{2g} \rightarrow A_g + B_{2g} + B_{3g} \text{ of } D_{2h}.$$

$$O_h : T_{1u} \rightarrow B_{2u} + B_{1u} + B_{3u} \text{ of } D_{2h}.$$

$$O_h : T_{2u} \rightarrow A_u + B_{2u} + B_{3u} \text{ of } D_{2h}.$$

The correspondences of irreps at HSPs from original SG to lowered SG:

$$\begin{aligned} n_{GM6}^{69} &= 2n_{GM11}^{229} + n_{GM8}^{229} + n_{GM9}^{229} & n_{GM5}^{69} &= 2n_{GM10}^{229} + n_{GM6}^{229} + n_{GM7}^{229} & n_{Y6}^{69} &= n_{N6}^{229} & n_{Y5}^{69} &= n_{N5}^{229} & n_{L2}^{69} &= 2n_{N6}^{229} & n_{L3}^{69} &= 2n_{N5}^{229} \\ n_{Z6}^{69} &= 2n_{H11}^{229} + n_{H8}^{229} + n_{H9}^{229} & n_{Z5}^{69} &= 2n_{H10}^{229} + n_{H6}^{229} + n_{H7}^{229} & n_{T6}^{69} &= n_{N6}^{229} & n_{T5}^{69} &= n_{N5}^{229} \end{aligned}$$

The lower SG is SG 69 when the preserved operations are: **(sub-SG label is 3) 1, 9, 16, 15, 25, 33, 40, 39.**

The transformation is:  $(\mathbf{a}_{69}, \mathbf{b}_{69}, \mathbf{c}_{69}) = (\mathbf{a}_{229}, \mathbf{b}_{229}, \mathbf{c}_{229}) \begin{pmatrix} -1 & 1 & 0 \\ 0 & 0 & 1 \\ 1 & 1 & 0 \end{pmatrix}, \overrightarrow{O_{229}O_{69}} = \mathbf{0}$

The reduction of higher dimensional irrep:

$$O_h : T_{1g} \rightarrow B_{2g} + B_{1g} + B_{3g} \text{ of } D_{2h}.$$

$$O_h : T_{2g} \rightarrow A_g + B_{2g} + B_{3g} \text{ of } D_{2h}.$$

$$O_h : T_{1u} \rightarrow B_{2u} + B_{1u} + B_{3u} \text{ of } D_{2h}.$$

$$O_h : T_{2u} \rightarrow A_u + B_{2u} + B_{3u} \text{ of } D_{2h}.$$

The correspondences of irreps at HSPs from original SG to lowered SG:

$$\begin{aligned} n_{GM6}^{69} &= 2n_{GM11}^{229} + n_{GM8}^{229} + n_{GM9}^{229} & n_{GM5}^{69} &= 2n_{GM10}^{229} + n_{GM6}^{229} + n_{GM7}^{229} & n_{Y6}^{69} &= n_{N6}^{229} & n_{Y5}^{69} &= n_{N5}^{229} & n_{L2}^{69} &= 2n_{N6}^{229} & n_{L3}^{69} &= 2n_{N5}^{229} \\ n_{Z6}^{69} &= 2n_{H11}^{229} + n_{H8}^{229} + n_{H9}^{229} & n_{Z5}^{69} &= 2n_{H10}^{229} + n_{H6}^{229} + n_{H7}^{229} & n_{T6}^{69} &= n_{N6}^{229} & n_{T5}^{69} &= n_{N5}^{229} \end{aligned}$$

The lower SG is SG 69 when the preserved operations are: **(sub-SG label is 4) 1, 10, 11, 12, 25, 34, 35, 36.**

The transformation is:  $(\mathbf{a}_{69}, \mathbf{b}_{69}, \mathbf{c}_{69}) = (\mathbf{a}_{229}, \mathbf{b}_{229}, \mathbf{c}_{229}) \begin{pmatrix} 1 & -1 & 0 \\ 1 & 1 & 0 \\ 0 & 0 & 1 \end{pmatrix}, \overrightarrow{O_{229}O_{69}} = \mathbf{0}$

The reduction of higher dimensional irrep:

$$O_h : T_{1g} \rightarrow B_{2g} + B_{1g} + B_{3g} \text{ of } D_{2h}.$$

$$O_h : T_{2g} \rightarrow A_g + B_{2g} + B_{3g} \text{ of } D_{2h}.$$

$$O_h : T_{1u} \rightarrow B_{2u} + B_{1u} + B_{3u} \text{ of } D_{2h}.$$

$$O_h : T_{2u} \rightarrow A_u + B_{2u} + B_{3u} \text{ of } D_{2h}.$$

The correspondences of irreps at HSPs from original SG to lowered SG:

$$\begin{aligned} n_{GM6}^{69} &= 2n_{GM11}^{229} + n_{GM8}^{229} + n_{GM9}^{229} & n_{GM5}^{69} &= 2n_{GM10}^{229} + n_{GM6}^{229} + n_{GM7}^{229} & n_{Y6}^{69} &= n_{N6}^{229} & n_{Y5}^{69} &= n_{N5}^{229} & n_{L2}^{69} &= 2n_{N6}^{229} & n_{L3}^{69} &= 2n_{N5}^{229} \end{aligned}$$

$$n_{Z6}^{69} = 2n_{H11}^{229} + n_{H8}^{229} + n_{H9}^{229} \quad n_{Z5}^{69} = 2n_{H10}^{229} + n_{H6}^{229} + n_{H7}^{229} \quad n_{T6}^{69} = n_{N6}^{229} \quad n_{T5}^{69} = n_{N5}^{229}$$

The lower SG is SG 87 when the preserved operations are: **(sub-SG label is 5)** 1, 6, 7, 10, 25, 30, 31, 34.

$$\text{The transformation is: } (\mathbf{a}_{87}, \mathbf{b}_{87}, \mathbf{c}_{87}) = (\mathbf{a}_{229}, \mathbf{b}_{229}, \mathbf{c}_{229}) \begin{pmatrix} 0 & 1 & 0 \\ -1 & 0 & 0 \\ 0 & 0 & 1 \end{pmatrix}, \overrightarrow{O_{229}O_{87}} = \mathbf{0}$$

The reduction of higher dimensional irrep:

$$O_h : T_{1g} \rightarrow A_g + {}^2E_g + {}^1E_g \quad \text{of } C_{4h}.$$

$$O_h : T_{2g} \rightarrow {}^2E_g + B_g + {}^1E_g \quad \text{of } C_{4h}.$$

$$O_h : T_{1u} \rightarrow A_u + {}^2E_u + {}^1E_u \quad \text{of } C_{4h}.$$

$$O_h : T_{2u} \rightarrow {}^2E_u + B_u + {}^1E_u \quad \text{of } C_{4h}.$$

The correspondences of irreps at HSPs from original SG to lowered SG:

$$\begin{aligned} n_{GM9}^{87} &= n_{GM11}^{229} + n_{GM9}^{229} \quad n_{GM5}^{87} = n_{GM10}^{229} + n_{GM7}^{229} \quad n_{GM11}^{87} = n_{GM11}^{229} + n_{GM9}^{229} \quad n_{GM7}^{87} = n_{GM10}^{229} + n_{GM7}^{229} \quad n_{GM12}^{87} = \\ n_{GM11}^{229} + n_{GM8}^{229} \quad n_{GM8}^{87} &= n_{GM10}^{229} + n_{GM6}^{229} \quad n_{GM10}^{87} = n_{GM11}^{229} + n_{GM8}^{229} \quad n_{GM6}^{87} = n_{GM10}^{229} + n_{GM6}^{229} \quad n_{M9}^{87} = n_{H11}^{229} + n_{H9}^{229} \quad n_{M5}^{87} = \\ n_{H10}^{229} + n_{H7}^{229} \quad n_{M11}^{87} &= n_{H11}^{229} + n_{H9}^{229} \quad n_{M7}^{87} = n_{H10}^{229} + n_{H7}^{229} \quad n_{M12}^{87} = n_{H11}^{229} + n_{H8}^{229} \quad n_{M8}^{87} = n_{H10}^{229} + n_{H6}^{229} \quad n_{M10}^{87} = n_{H11}^{229} + n_{H8}^{229} \\ n_{M6}^{87} &= n_{H10}^{229} + n_{H6}^{229} \quad n_{X6}^{87} = n_{N6}^{229} \quad n_{X4}^{87} = n_{N5}^{229} \quad n_{X5}^{87} = n_{N6}^{229} \quad n_{X3}^{87} = n_{N5}^{229} \quad n_{P7}^{87} = n_{P7}^{229} + n_{P8}^{229} \quad n_{P8}^{87} = n_{P6}^{229} + n_{P8}^{229} \\ n_{P7}^{229} + n_{P8}^{229} \quad n_{P6}^{87} &= n_{P6}^{229} + n_{P8}^{229} \quad n_{N2}^{87} = 2n_{N6}^{229} \quad n_{N3}^{87} = 2n_{N5}^{229} \end{aligned}$$

The lower SG is SG 87 when the preserved operations are: **(sub-SG label is 6)** 1, 2, 3, 8, 25, 26, 27, 32.

$$\text{The transformation is: } (\mathbf{a}_{87}, \mathbf{b}_{87}, \mathbf{c}_{87}) = (\mathbf{a}_{229}, \mathbf{b}_{229}, \mathbf{c}_{229}) \begin{pmatrix} 0 & 0 & 1 \\ 0 & 1 & 0 \\ -1 & 0 & 0 \end{pmatrix}, \overrightarrow{O_{229}O_{87}} = \mathbf{0}$$

The reduction of higher dimensional irrep:

$$O_h : T_{1g} \rightarrow A_g + {}^2E_g + {}^1E_g \quad \text{of } C_{4h}.$$

$$O_h : T_{2g} \rightarrow {}^2E_g + B_g + {}^1E_g \quad \text{of } C_{4h}.$$

$$O_h : T_{1u} \rightarrow A_u + {}^2E_u + {}^1E_u \quad \text{of } C_{4h}.$$

$$O_h : T_{2u} \rightarrow {}^2E_u + B_u + {}^1E_u \quad \text{of } C_{4h}.$$

The correspondences of irreps at HSPs from original SG to lowered SG:

$$\begin{aligned} n_{GM9}^{87} &= n_{GM11}^{229} + n_{GM9}^{229} \quad n_{GM5}^{87} = n_{GM10}^{229} + n_{GM7}^{229} \quad n_{GM11}^{87} = n_{GM11}^{229} + n_{GM9}^{229} \quad n_{GM7}^{87} = n_{GM10}^{229} + n_{GM7}^{229} \quad n_{GM12}^{87} = \\ n_{GM11}^{229} + n_{GM8}^{229} \quad n_{GM8}^{87} &= n_{GM10}^{229} + n_{GM6}^{229} \quad n_{GM10}^{87} = n_{GM11}^{229} + n_{GM8}^{229} \quad n_{GM6}^{87} = n_{GM10}^{229} + n_{GM6}^{229} \quad n_{M9}^{87} = n_{H11}^{229} + n_{H9}^{229} \quad n_{M5}^{87} = \\ n_{H10}^{229} + n_{H7}^{229} \quad n_{M11}^{87} &= n_{H11}^{229} + n_{H9}^{229} \quad n_{M7}^{87} = n_{H10}^{229} + n_{H7}^{229} \quad n_{M12}^{87} = n_{H11}^{229} + n_{H8}^{229} \quad n_{M8}^{87} = n_{H10}^{229} + n_{H6}^{229} \quad n_{M10}^{87} = n_{H11}^{229} + n_{H8}^{229} \\ n_{M6}^{87} &= n_{H10}^{229} + n_{H6}^{229} \quad n_{X6}^{87} = n_{N6}^{229} \quad n_{X4}^{87} = n_{N5}^{229} \quad n_{X5}^{87} = n_{N6}^{229} \quad n_{X3}^{87} = n_{N5}^{229} \quad n_{P7}^{87} = n_{P7}^{229} + n_{P8}^{229} \quad n_{P8}^{87} = n_{P6}^{229} + n_{P8}^{229} \\ n_{P7}^{229} + n_{P8}^{229} \quad n_{P6}^{87} &= n_{P6}^{229} + n_{P8}^{229} \quad n_{N2}^{87} = 2n_{N6}^{229} \quad n_{N3}^{87} = 2n_{N5}^{229} \end{aligned}$$

The lower SG is SG 87 when the preserved operations are: **(sub-SG label is 7)** 1, 4, 5, 9, 25, 28, 29, 33.

$$\text{The transformation is: } (\mathbf{a}_{87}, \mathbf{b}_{87}, \mathbf{c}_{87}) = (\mathbf{a}_{229}, \mathbf{b}_{229}, \mathbf{c}_{229}) \begin{pmatrix} 0 & -1 & 0 \\ 0 & 0 & 1 \\ -1 & 0 & 0 \end{pmatrix}, \overrightarrow{O_{229}O_{87}} = \mathbf{0}$$

The reduction of higher dimensional irrep:

$$O_h : T_{1g} \rightarrow A_g + {}^2E_g + {}^1E_g \quad \text{of } C_{4h}.$$

$$O_h : T_{2g} \rightarrow {}^2E_g + B_g + {}^1E_g \quad \text{of } C_{4h}.$$

$$O_h : T_{1u} \rightarrow A_u + {}^2E_u + {}^1E_u \quad \text{of } C_{4h}.$$

$$O_h : T_{2u} \rightarrow {}^2E_u + B_u + {}^1E_u \quad \text{of } C_{4h}.$$

The correspondences of irreps at HSPs from original SG to lowered SG:

$$\begin{aligned} n_{GM9}^{87} &= n_{GM11}^{229} + n_{GM9}^{229} \quad n_{GM5}^{87} = n_{GM10}^{229} + n_{GM7}^{229} \quad n_{GM11}^{87} = n_{GM11}^{229} + n_{GM9}^{229} \quad n_{GM7}^{87} = n_{GM10}^{229} + n_{GM7}^{229} \quad n_{GM12}^{87} = \\ n_{GM11}^{229} + n_{GM8}^{229} \quad n_{GM8}^{87} &= n_{GM10}^{229} + n_{GM6}^{229} \quad n_{GM10}^{87} = n_{GM11}^{229} + n_{GM8}^{229} \quad n_{GM6}^{87} = n_{GM10}^{229} + n_{GM6}^{229} \quad n_{M9}^{87} = n_{H11}^{229} + n_{H9}^{229} \quad n_{M5}^{87} = \\ n_{H10}^{229} + n_{H7}^{229} \quad n_{M11}^{87} &= n_{H11}^{229} + n_{H9}^{229} \quad n_{M7}^{87} = n_{H10}^{229} + n_{H7}^{229} \quad n_{M12}^{87} = n_{H11}^{229} + n_{H8}^{229} \quad n_{M8}^{87} = n_{H10}^{229} + n_{H6}^{229} \quad n_{M10}^{87} = n_{H11}^{229} + n_{H8}^{229} \\ n_{M6}^{87} &= n_{H10}^{229} + n_{H6}^{229} \quad n_{X6}^{87} = n_{N6}^{229} \quad n_{X4}^{87} = n_{N5}^{229} \quad n_{X5}^{87} = n_{N6}^{229} \quad n_{X3}^{87} = n_{N5}^{229} \quad n_{P7}^{87} = n_{P7}^{229} + n_{P8}^{229} \quad n_{P8}^{87} = n_{P6}^{229} + n_{P8}^{229} \\ n_{P7}^{229} + n_{P8}^{229} \quad n_{P6}^{87} &= n_{P6}^{229} + n_{P8}^{229} \quad n_{N2}^{87} = 2n_{N6}^{229} \quad n_{N3}^{87} = 2n_{N5}^{229} \end{aligned}$$

The lower SG is SG 139 when the preserved operations are: **(sub-SG label is 8)** 1, 6, 7, 10, 8, 9, 11, 12, 25, 30, 31, 34, 32, 33, 35, 36.

$$\text{The transformation is: } (\mathbf{a}_{139}, \mathbf{b}_{139}, \mathbf{c}_{139}) = (\mathbf{a}_{229}, \mathbf{b}_{229}, \mathbf{c}_{229}) \begin{pmatrix} 0 & 1 & 0 \\ -1 & 0 & 0 \\ 0 & 0 & 1 \end{pmatrix}, \overrightarrow{O_{229}O_{139}} = \mathbf{0}$$

The reduction of higher dimensional irrep:

$$O_h : E_g \rightarrow A_{1g} + B_{1g} \quad \text{of } D_{4h}.$$

$$O_h : E_u \rightarrow A_{1u} + B_{1u} \quad \text{of } D_{4h}.$$

The correspondences of irreps at HSPs from original SG to lowered SG:

$$\begin{aligned} n_{GM8}^{139} &= n_{GM11}^{229} + n_{GM9}^{229} n_{GM6}^{139} = n_{GM10}^{229} + n_{GM7}^{229} n_{GM9}^{139} = n_{GM11}^{229} + n_{GM8}^{229} n_{GM7}^{139} = n_{GM10}^{229} + n_{GM6}^{229} n_{M8}^{139} = n_{H11}^{229} + n_{H9}^{229} \\ n_{M6}^{139} &= n_{H10}^{229} + n_{H7}^{229} n_{M9}^{139} = n_{H11}^{229} + n_{H8}^{229} n_{M7}^{139} = n_{H10}^{229} + n_{H6}^{229} n_{X6}^{139} = n_{N6}^{229} n_{X5}^{139} = n_{N5}^{229} n_{P7}^{139} = n_{P7}^{229} + n_{P8}^{229} n_{P6}^{139} = \\ n_{P6}^{229} + n_{P8}^{229} n_{N6}^{139} &= n_{N6}^{229} n_{N4}^{139} = n_{N5}^{229} n_{N5}^{139} = n_{N6}^{229} n_{N3}^{139} = n_{N5}^{229} \end{aligned}$$

The lower SG is SG 139 when the preserved operations are: (**sub-SG label is 9**) 1, 2, 3, 8, 9, 10, 13, 14, 25, 26, 27, 32, 33, 34, 37, 38.

$$\text{The transformation is: } (\mathbf{a}_{139}, \mathbf{b}_{139}, \mathbf{c}_{139}) = (\mathbf{a}_{229}, \mathbf{b}_{229}, \mathbf{c}_{229}) \begin{pmatrix} 0 & 0 & 1 \\ 0 & 1 & 0 \\ -1 & 0 & 0 \end{pmatrix}, \overrightarrow{O_{229}O_{139}} = \mathbf{0}$$

The reduction of higher dimensional irrep:

$$O_h : E_g \rightarrow A_{1g} + B_{1g} \text{ of } D_{4h}.$$

$$O_h : E_u \rightarrow A_{1u} + B_{1u} \text{ of } D_{4h}.$$

The correspondences of irreps at HSPs from original SG to lowered SG:

$$\begin{aligned} n_{GM8}^{139} &= n_{GM11}^{229} + n_{GM9}^{229} n_{GM6}^{139} = n_{GM10}^{229} + n_{GM7}^{229} n_{GM9}^{139} = n_{GM11}^{229} + n_{GM8}^{229} n_{GM7}^{139} = n_{GM10}^{229} + n_{GM6}^{229} n_{M8}^{139} = n_{H11}^{229} + n_{H9}^{229} \\ n_{M6}^{139} &= n_{H10}^{229} + n_{H7}^{229} n_{M9}^{139} = n_{H11}^{229} + n_{H8}^{229} n_{M7}^{139} = n_{H10}^{229} + n_{H6}^{229} n_{X6}^{139} = n_{N6}^{229} n_{X5}^{139} = n_{N5}^{229} n_{P7}^{139} = n_{P7}^{229} + n_{P8}^{229} n_{P6}^{139} = \\ n_{P6}^{229} + n_{P8}^{229} n_{N6}^{139} &= n_{N6}^{229} n_{N4}^{139} = n_{N5}^{229} n_{N5}^{139} = n_{N6}^{229} n_{N3}^{139} = n_{N5}^{229} \end{aligned}$$

The lower SG is SG 139 when the preserved operations are: (**sub-SG label is 10**) 1, 4, 5, 9, 10, 8, 16, 15, 25, 28, 29, 33, 34, 32, 40, 39.

$$\text{The transformation is: } (\mathbf{a}_{139}, \mathbf{b}_{139}, \mathbf{c}_{139}) = (\mathbf{a}_{229}, \mathbf{b}_{229}, \mathbf{c}_{229}) \begin{pmatrix} 0 & -1 & 0 \\ 0 & 0 & 1 \\ -1 & 0 & 0 \end{pmatrix}, \overrightarrow{O_{229}O_{139}} = \mathbf{0}$$

The reduction of higher dimensional irrep:

$$O_h : E_g \rightarrow A_{1g} + B_{1g} \text{ of } D_{4h}.$$

$$O_h : E_u \rightarrow A_{1u} + B_{1u} \text{ of } D_{4h}.$$

The correspondences of irreps at HSPs from original SG to lowered SG:

$$\begin{aligned} n_{GM8}^{139} &= n_{GM11}^{229} + n_{GM9}^{229} n_{GM6}^{139} = n_{GM10}^{229} + n_{GM7}^{229} n_{GM9}^{139} = n_{GM11}^{229} + n_{GM8}^{229} n_{GM7}^{139} = n_{GM10}^{229} + n_{GM6}^{229} n_{M8}^{139} = n_{H11}^{229} + n_{H9}^{229} \\ n_{M6}^{139} &= n_{H10}^{229} + n_{H7}^{229} n_{M9}^{139} = n_{H11}^{229} + n_{H8}^{229} n_{M7}^{139} = n_{H10}^{229} + n_{H6}^{229} n_{X6}^{139} = n_{N6}^{229} n_{X5}^{139} = n_{N5}^{229} n_{P7}^{139} = n_{P7}^{229} + n_{P8}^{229} n_{P6}^{139} = \\ n_{P6}^{229} + n_{P8}^{229} n_{N6}^{139} &= n_{N6}^{229} n_{N4}^{139} = n_{N5}^{229} n_{N5}^{139} = n_{N6}^{229} n_{N3}^{139} = n_{N5}^{229} \end{aligned}$$

The lower SG is SG 148 when the preserved operations are: (**sub-SG label is 11**) 1, 17, 18, 25, 41, 42.

$$\text{The transformation is: } (\mathbf{a}_{148}, \mathbf{b}_{148}, \mathbf{c}_{148}) = (\mathbf{a}_{229}, \mathbf{b}_{229}, \mathbf{c}_{229}) \begin{pmatrix} \frac{1}{2} & -\frac{1}{2} & \frac{1}{2} \\ \frac{1}{2} & \frac{1}{2} & -\frac{1}{2} \\ -\frac{1}{2} & \frac{1}{2} & \frac{1}{2} \end{pmatrix}, \overrightarrow{O_{229}O_{148}} = \mathbf{0}$$

The reduction of higher dimensional irrep:

$$O_h : T_{1g} \rightarrow A_g + {}^2E_g + {}^1E_g \text{ of } C_{3i}.$$

$$O_h : T_{2g} \rightarrow A_g + {}^2E_g + {}^1E_g \text{ of } C_{3i}.$$

$$O_h : T_{1u} \rightarrow {}^1E_u + A_u + {}^2E_u \text{ of } C_{3i}.$$

$$O_h : T_{2u} \rightarrow {}^1E_u + A_u + {}^2E_u \text{ of } C_{3i}.$$

The correspondences of irreps at HSPs from original SG to lowered SG:

$$\begin{aligned} n_{GM7}^{148} &= 2n_{GM11}^{229} n_{GM4}^{148} = 2n_{GM10}^{229} n_{GM9}^{148} = n_{GM11}^{229} + n_{GM8}^{229} + n_{GM9}^{229} n_{GM6}^{148} = n_{GM10}^{229} + n_{GM6}^{229} + n_{GM7}^{229} n_{GM8}^{148} = \\ n_{GM11}^{229} + n_{GM8}^{229} + n_{GM9}^{229} n_{GM5}^{148} &= n_{GM10}^{229} + n_{GM6}^{229} + n_{GM7}^{229} n_{L2}^{148} = 2n_{N6}^{229} n_{L3}^{148} = 2n_{N5}^{229} n_{F2}^{148} = 2n_{N6}^{229} n_{F3}^{148} = 2n_{N5}^{229} \\ n_{T7}^{148} &= 2n_{H11}^{229} n_{T4}^{148} = 2n_{H10}^{229} n_{T9}^{148} = n_{H11}^{229} + n_{H8}^{229} + n_{H9}^{229} n_{T6}^{148} = n_{H10}^{229} + n_{H6}^{229} + n_{H7}^{229} n_{T8}^{148} = n_{H11}^{229} + n_{H8}^{229} + n_{H9}^{229} n_{T5}^{148} = \\ n_{H10}^{229} + n_{H6}^{229} + n_{H7}^{229} \end{aligned}$$

The lower SG is SG 148 when the preserved operations are: (**sub-SG label is 12**) 1, 24, 23, 25, 48, 47.

$$\text{The transformation is: } (\mathbf{a}_{148}, \mathbf{b}_{148}, \mathbf{c}_{148}) = (\mathbf{a}_{229}, \mathbf{b}_{229}, \mathbf{c}_{229}) \begin{pmatrix} -\frac{1}{2} & -\frac{1}{2} & \frac{1}{2} \\ \frac{1}{2} & -\frac{1}{2} & -\frac{1}{2} \\ \frac{1}{2} & -\frac{1}{2} & \frac{1}{2} \end{pmatrix}, \overrightarrow{O_{229}O_{148}} = \mathbf{0}$$

The reduction of higher dimensional irrep:

$$O_h : T_{1g} \rightarrow A_g + {}^2E_g + {}^1E_g \text{ of } C_{3i}.$$

$$O_h : T_{2g} \rightarrow A_g + {}^2E_g + {}^1E_g \text{ of } C_{3i}.$$

$$O_h : T_{1u} \rightarrow {}^1E_u + A_u + {}^2E_u \text{ of } C_{3i}.$$

$$O_h : T_{2u} \rightarrow {}^1E_u + A_u + {}^2E_u \text{ of } C_{3i}.$$

The correspondences of irreps at HSPs from original SG to lowered SG:

$$\begin{aligned} n_{GM7}^{148} &= 2n_{GM11}^{229} n_{GM4}^{148} = 2n_{GM10}^{229} n_{GM9}^{148} = n_{GM11}^{229} + n_{GM8}^{229} + n_{GM9}^{229} n_{GM6}^{148} = n_{GM10}^{229} + n_{GM6}^{229} + n_{GM7}^{229} n_{GM8}^{148} = \\ n_{GM11}^{229} + n_{GM8}^{229} + n_{GM9}^{229} n_{GM5}^{148} &= n_{GM10}^{229} + n_{GM6}^{229} + n_{GM7}^{229} n_{L2}^{148} = 2n_{N6}^{229} n_{L3}^{148} = 2n_{N5}^{229} n_{F2}^{148} = 2n_{N6}^{229} n_{F3}^{148} = 2n_{N5}^{229} \end{aligned}$$

$$n_{T7}^{148} = 2n_{H11}^{229} n_{T4}^{148} = 2n_{H10}^{229} n_{T9}^{148} = n_{H11}^{229} + n_{H8}^{229} + n_{H9}^{229} n_{T6}^{148} = n_{H10}^{229} + n_{H6}^{229} + n_{H7}^{229} n_{T8}^{148} = n_{H11}^{229} + n_{H8}^{229} + n_{H9}^{229} n_{T5}^{148} = n_{H10}^{229} + n_{H6}^{229} + n_{H7}^{229}$$

The lower SG is SG 148 when the preserved operations are: **(sub-SG label is 13)** 1, 20, 19, 25, 44, 43.

The transformation is:  $(\mathbf{a}_{148}, \mathbf{b}_{148}, \mathbf{c}_{148}) = (\mathbf{a}_{229}, \mathbf{b}_{229}, \mathbf{c}_{229}) \begin{pmatrix} \frac{1}{2} & -\frac{1}{2} & \frac{1}{2} \\ -\frac{1}{2} & -\frac{1}{2} & \frac{1}{2} \\ \frac{1}{2} & -\frac{1}{2} & -\frac{1}{2} \end{pmatrix}, \overrightarrow{O_{229}O_{148}} = \mathbf{0}$

The reduction of higher dimensional irrep:

$$O_h : T_{1g} \rightarrow A_g + {}^2E_g + {}^1E_g \text{ of } C_{3i}.$$

$$O_h : T_{2g} \rightarrow A_g + {}^2E_g + {}^1E_g \text{ of } C_{3i}.$$

$$O_h : T_{1u} \rightarrow {}^1E_u + A_u + {}^2E_u \text{ of } C_{3i}.$$

$$O_h : T_{2u} \rightarrow {}^1E_u + A_u + {}^2E_u \text{ of } C_{3i}.$$

The correspondences of irreps at HSPs from original SG to lowered SG:

$$n_{GM7}^{148} = 2n_{GM11}^{229} n_{GM4}^{148} = 2n_{GM10}^{229} n_{GM9}^{148} = n_{GM11}^{229} + n_{GM8}^{229} + n_{GM9}^{229} n_{GM6}^{148} = n_{GM10}^{229} + n_{GM6}^{229} + n_{GM7}^{229} n_{GM8}^{148} = n_{GM11}^{229} + n_{GM8}^{229} + n_{GM9}^{229} n_{GM5}^{148} = n_{GM10}^{229} + n_{GM6}^{229} + n_{GM7}^{229} n_{L2}^{148} = 2n_{N6}^{229} n_{L3}^{148} = 2n_{N5}^{229} n_{F2}^{148} = 2n_{N6}^{229} n_{F3}^{148} = 2n_{N5}^{229} n_{T7}^{148} = 2n_{H11}^{229} n_{T4}^{148} = 2n_{H10}^{229} n_{T9}^{148} = n_{H11}^{229} + n_{H8}^{229} + n_{H9}^{229} n_{T6}^{148} = n_{H10}^{229} + n_{H6}^{229} + n_{H7}^{229} n_{T8}^{148} = n_{H11}^{229} + n_{H8}^{229} + n_{H9}^{229} n_{T5}^{148} = n_{H10}^{229} + n_{H6}^{229} + n_{H7}^{229}$$

The lower SG is SG 148 when the preserved operations are: **(sub-SG label is 14)** 1, 22, 21, 25, 46, 45.

The transformation is:  $(\mathbf{a}_{148}, \mathbf{b}_{148}, \mathbf{c}_{148}) = (\mathbf{a}_{229}, \mathbf{b}_{229}, \mathbf{c}_{229}) \begin{pmatrix} -\frac{1}{2} & -\frac{1}{2} & \frac{1}{2} \\ -\frac{1}{2} & \frac{1}{2} & \frac{1}{2} \\ -\frac{1}{2} & \frac{1}{2} & -\frac{1}{2} \end{pmatrix}, \overrightarrow{O_{229}O_{148}} = \mathbf{0}$

The reduction of higher dimensional irrep:

$$O_h : T_{1g} \rightarrow A_g + {}^2E_g + {}^1E_g \text{ of } C_{3i}.$$

$$O_h : T_{2g} \rightarrow A_g + {}^2E_g + {}^1E_g \text{ of } C_{3i}.$$

$$O_h : T_{1u} \rightarrow {}^1E_u + A_u + {}^2E_u \text{ of } C_{3i}.$$

$$O_h : T_{2u} \rightarrow {}^1E_u + A_u + {}^2E_u \text{ of } C_{3i}.$$

The correspondences of irreps at HSPs from original SG to lowered SG:

$$n_{GM7}^{148} = 2n_{GM11}^{229} n_{GM4}^{148} = 2n_{GM10}^{229} n_{GM9}^{148} = n_{GM11}^{229} + n_{GM8}^{229} + n_{GM9}^{229} n_{GM6}^{148} = n_{GM10}^{229} + n_{GM6}^{229} + n_{GM7}^{229} n_{GM8}^{148} = n_{GM11}^{229} + n_{GM8}^{229} + n_{GM9}^{229} n_{GM5}^{148} = n_{GM10}^{229} + n_{GM6}^{229} + n_{GM7}^{229} n_{L2}^{148} = 2n_{N6}^{229} n_{L3}^{148} = 2n_{N5}^{229} n_{F2}^{148} = 2n_{N6}^{229} n_{F3}^{148} = 2n_{N5}^{229} n_{T7}^{148} = 2n_{H11}^{229} n_{T4}^{148} = 2n_{H10}^{229} n_{T9}^{148} = n_{H11}^{229} + n_{H8}^{229} + n_{H9}^{229} n_{T6}^{148} = n_{H10}^{229} + n_{H6}^{229} + n_{H7}^{229} n_{T8}^{148} = n_{H11}^{229} + n_{H8}^{229} + n_{H9}^{229} n_{T5}^{148} = n_{H10}^{229} + n_{H6}^{229} + n_{H7}^{229}$$

The lower SG is SG 204 when the preserved operations are: **(sub-SG label is 15)** 1, 8, 9, 10, 17, 24, 20, 22, 18, 23, 19, 21, 25, 32, 33, 34, 41, 48, 44, 46, 42, 47, 43, 45.

The transformation is:  $(\mathbf{a}_{204}, \mathbf{b}_{204}, \mathbf{c}_{204}) = (\mathbf{a}_{229}, \mathbf{b}_{229}, \mathbf{c}_{229}) \begin{pmatrix} 0 & 0 & 1 \\ 1 & 0 & 0 \\ 0 & 1 & 0 \end{pmatrix}, \overrightarrow{O_{229}O_{204}} = \mathbf{0}$

The reduction of higher dimensional irrep:

$$O_h : E_g \rightarrow {}^1E_g + {}^2E_g \text{ of } T_h.$$

$$O_h : E_u \rightarrow {}^1E_u + {}^2E_u \text{ of } T_h.$$

The correspondences of irreps at HSPs from original SG to lowered SG:

$$n_{GM9}^{204} = n_{GM11}^{229} n_{GM6}^{204} = n_{GM10}^{229} n_{GM10}^{204} = n_{GM11}^{229} n_{GM7}^{204} = n_{GM10}^{229} n_{GM8}^{204} = n_{GM8}^{229} + n_{GM9}^{229} n_{GM5}^{204} = n_{GM6}^{229} + n_{GM7}^{229} n_{H9}^{204} = n_{H11}^{229} n_{H6}^{204} = n_{H10}^{229} n_{H10}^{204} = n_{H11}^{229} n_{H7}^{204} = n_{H10}^{229} n_{H8}^{204} = n_{H8}^{229} + n_{H9}^{229} n_{H5}^{204} = n_{H6}^{229} + n_{H7}^{229} n_{N6}^{204} = n_{N6}^{229} n_{N4}^{204} = n_{N5}^{229} n_{N5}^{204} = n_{N6}^{229} n_{N3}^{204} = n_{N5}^{229} n_{P6}^{204} = n_{P8}^{229} n_{P7}^{204} = n_{P8}^{229} n_{P5}^{204} = n_{P6}^{229} + n_{P7}^{229}$$

**127. Lowered SGs by higher-dimensional irreps of pairings in SG 230**

The representative operations of SG/T for SG 230:

$$1 : (x, y, z), 2 : (x + \frac{1}{4}, \frac{1}{4} - z, y + \frac{3}{4}), 3 : (x + \frac{3}{4}, z + \frac{1}{4}, \frac{1}{4} - y), 4 : (z + \frac{3}{4}, y + \frac{1}{4}, \frac{1}{4} - x), 5 : (\frac{1}{4} - z, y + \frac{3}{4}, x + \frac{1}{4}), 6 : (\frac{1}{4} - y, x + \frac{3}{4}, z + \frac{1}{4}), 7 : (y + \frac{1}{4}, \frac{1}{4} - x, z + \frac{3}{4}), 8 : (x, -y, \frac{1}{2} - z), 9 : (\frac{1}{2} - x, y, -z), 10 : (-x, \frac{1}{2} - y, z),$$

$$\begin{aligned}
&11 : (y + \frac{3}{4}, x + \frac{1}{4}, \frac{1}{4} - z), 12 : (\frac{1}{4} - y, \frac{1}{4} - x, \frac{1}{4} - z), 13 : (\frac{1}{4} - x, z + \frac{3}{4}, y + \frac{1}{4}), 14 : (\frac{1}{4} - x, \frac{1}{4} - z, \frac{1}{4} - y), \\
&15 : (z + \frac{1}{4}, \frac{1}{4} - y, x + \frac{3}{4}), 16 : (\frac{1}{4} - z, \frac{1}{4} - y, \frac{1}{4} - x), 17 : (z, x, y), 18 : (y, z, x), 19 : (\frac{1}{2} - y, z, -x), 20 : (-z, \frac{1}{2} - x, y), \\
&21 : (-y, \frac{1}{2} - z, x), 22 : (z, -x, \frac{1}{2} - y), 23 : (y, -z, \frac{1}{2} - x), 24 : (\frac{1}{2} - z, x, -y), 25 : (-x, -y, -z), 26 : (\frac{1}{4} - x, z + \frac{1}{4}, \frac{3}{4} - y), \\
&27 : (\frac{3}{4} - x, \frac{1}{4} - z, y + \frac{1}{4}), 28 : (\frac{3}{4} - z, \frac{1}{4} - y, x + \frac{1}{4}), 29 : (z + \frac{1}{4}, \frac{3}{4} - y, \frac{1}{4} - x), 30 : (y + \frac{1}{4}, \frac{3}{4} - x, \frac{1}{4} - z), 31 : (\frac{1}{4} - y, x + \frac{1}{4}, \frac{3}{4} - z), \\
&32 : (-x, y, z + \frac{1}{2}), 33 : (x + \frac{1}{2}, -y, z), 34 : (x, y + \frac{1}{2}, -z), 35 : (\frac{3}{4} - y, \frac{1}{4} - x, z + \frac{1}{4}), 36 : (y + \frac{1}{4}, x + \frac{1}{4}, z + \frac{1}{4}), \\
&37 : (x + \frac{1}{4}, \frac{3}{4} - z, \frac{1}{4} - y), 38 : (x + \frac{1}{4}, z + \frac{1}{4}, y + \frac{1}{4}), 39 : (\frac{1}{4} - z, y + \frac{1}{4}, \frac{3}{4} - x), 40 : (z + \frac{1}{4}, y + \frac{1}{4}, x + \frac{1}{4}), 41 : (-z, -x, -y), \\
&42 : (-y, -z, -x), 43 : (y + \frac{1}{2}, -z, x), 44 : (z, x + \frac{1}{2}, -y), 45 : (y, z + \frac{1}{2}, -x), 46 : (-z, x, y + \frac{1}{2}), 47 : (-y, z, x + \frac{1}{2}), \\
&48 : (z + \frac{1}{2}, -x, y).
\end{aligned}$$

The lower SG is SG 73 when the preserved operations are: **(sub-SG label is 1) 1, 8, 9, 10, 25, 32, 33, 34.**

The transformation is:  $(\mathbf{a}_{73}, \mathbf{b}_{73}, \mathbf{c}_{73}) = (\mathbf{a}_{230}, \mathbf{b}_{230}, \mathbf{c}_{230}) \begin{pmatrix} 0 & 1 & 0 \\ 1 & 0 & 0 \\ 0 & 0 & -1 \end{pmatrix}, \overrightarrow{O_{230}O_{73}} = \frac{1}{4}\mathbf{a}_{73} + (-\frac{1}{4})\mathbf{b}_{73} + (\frac{1}{4})\mathbf{c}_{73}$

The reduction of higher dimensional irrep:

$$O_h : T_{1g} \rightarrow B_{2g} + B_{1g} + B_{3g} \text{ of } D_{2h}.$$

$$O_h : T_{2g} \rightarrow B_{2g} + B_{1g} + B_{3g} \text{ of } D_{2h}.$$

$$O_h : T_{1u} \rightarrow B_{2u} + B_{1u} + B_{3u} \text{ of } D_{2h}.$$

$$O_h : T_{2u} \rightarrow B_{2u} + B_{1u} + B_{3u} \text{ of } D_{2h}.$$

The correspondences of irreps at HSPs from original SG to lowered SG:

$$\begin{aligned}
n_{GM6}^{73} &= 2n_{GM11}^{230} + n_{GM8}^{230} + n_{GM9}^{230} \quad n_{GM5}^{73} = 2n_{GM10}^{230} + n_{GM6}^{230} + n_{GM7}^{230} \quad n_{X6}^{73} = n_{H5}^{230} + n_{H6}^{230} + n_{H7}^{230} \quad n_{X5}^{73} = n_{H5}^{230} + n_{H6}^{230} + n_{H7}^{230} \\
n_{T2}^{73} &= n_{N3}^{230} + n_{N4}^{230} \quad n_{W3}^{73} = n_{P4}^{230} + n_{P5}^{230} + 2n_{P6}^{230} \quad n_{W2}^{73} = n_{P7}^{230} + n_{P8}^{230} \quad n_{W4}^{73} = n_{P7}^{230} + n_{P8}^{230} \quad n_{W5}^{73} = n_{P7}^{230} + n_{P8}^{230} \quad n_{R2}^{73} = n_{N3}^{230} + n_{N4}^{230} \\
n_{S2}^{73} &= n_{N3}^{230} + n_{N4}^{230}
\end{aligned}$$

The lower SG is SG 70 when the preserved operations are: **(sub-SG label is 2) 1, 8, 13, 14, 25, 32, 37, 38.**

The transformation is:  $(\mathbf{a}_{70}, \mathbf{b}_{70}, \mathbf{c}_{70}) = (\mathbf{a}_{230}, \mathbf{b}_{230}, \mathbf{c}_{230}) \begin{pmatrix} 0 & 1 & 0 \\ 1 & 0 & 1 \\ 1 & 0 & -1 \end{pmatrix}, \overrightarrow{O_{230}O_{70}} = \frac{1}{4}\mathbf{a}_{70} + (\frac{1}{4})\mathbf{b}_{70} + (\frac{1}{2})\mathbf{c}_{70}$

The reduction of higher dimensional irrep:

$$O_h : T_{1g} \rightarrow B_{1g} + B_{2g} + B_{3g} \text{ of } D_{2h}.$$

$$O_h : T_{2g} \rightarrow A_g + B_{1g} + B_{3g} \text{ of } D_{2h}.$$

$$O_h : T_{1u} \rightarrow B_{1u} + B_{2u} + B_{3u} \text{ of } D_{2h}.$$

$$O_h : T_{2u} \rightarrow A_u + B_{1u} + B_{3u} \text{ of } D_{2h}.$$

The correspondences of irreps at HSPs from original SG to lowered SG:

$$\begin{aligned}
n_{GM6}^{70} &= 2n_{GM11}^{230} + n_{GM8}^{230} + n_{GM9}^{230} \quad n_{GM5}^{70} = 2n_{GM10}^{230} + n_{GM6}^{230} + n_{GM7}^{230} \quad n_{Y4}^{70} = n_{H5}^{230} + n_{H6}^{230} + n_{H7}^{230} \quad n_{Y3}^{70} = n_{H5}^{230} + n_{H6}^{230} + n_{H7}^{230} \\
n_{L3}^{70} &= n_{N3}^{230} + n_{N4}^{230} \quad n_{L2}^{70} = n_{N3}^{230} + n_{N4}^{230} \quad n_{Z3}^{70} = n_{N4}^{230} \quad n_{Z4}^{70} = n_{N3}^{230} \quad n_{T4}^{70} = n_{N4}^{230} \quad n_{T3}^{70} = n_{N3}^{230}
\end{aligned}$$

The lower SG is SG 70 when the preserved operations are: **(sub-SG label is 3) 1, 9, 16, 15, 25, 33, 40, 39.**

The transformation is:  $(\mathbf{a}_{70}, \mathbf{b}_{70}, \mathbf{c}_{70}) = (\mathbf{a}_{230}, \mathbf{b}_{230}, \mathbf{c}_{230}) \begin{pmatrix} -1 & 0 & 1 \\ 0 & -1 & 0 \\ 1 & 0 & 1 \end{pmatrix}, \overrightarrow{O_{230}O_{70}} = \frac{1}{4}\mathbf{a}_{70} + (\frac{1}{4})\mathbf{b}_{70} + (\frac{1}{2})\mathbf{c}_{70}$

The reduction of higher dimensional irrep:

$$O_h : T_{1g} \rightarrow B_{1g} + B_{2g} + B_{3g} \text{ of } D_{2h}.$$

$$O_h : T_{2g} \rightarrow A_g + B_{1g} + B_{3g} \text{ of } D_{2h}.$$

$$O_h : T_{1u} \rightarrow B_{1u} + B_{2u} + B_{3u} \text{ of } D_{2h}.$$

$$O_h : T_{2u} \rightarrow A_u + B_{1u} + B_{3u} \text{ of } D_{2h}.$$

The correspondences of irreps at HSPs from original SG to lowered SG:

$$\begin{aligned}
n_{GM6}^{70} &= 2n_{GM11}^{230} + n_{GM8}^{230} + n_{GM9}^{230} \quad n_{GM5}^{70} = 2n_{GM10}^{230} + n_{GM6}^{230} + n_{GM7}^{230} \quad n_{Y4}^{70} = n_{H5}^{230} + n_{H6}^{230} + n_{H7}^{230} \quad n_{Y3}^{70} = n_{H5}^{230} + n_{H6}^{230} + n_{H7}^{230} \\
n_{L3}^{70} &= n_{N3}^{230} + n_{N4}^{230} \quad n_{L2}^{70} = n_{N3}^{230} + n_{N4}^{230} \quad n_{Z3}^{70} = n_{N4}^{230} \quad n_{Z4}^{70} = n_{N3}^{230} \quad n_{T4}^{70} = n_{N4}^{230} \quad n_{T3}^{70} = n_{N3}^{230}
\end{aligned}$$

The lower SG is SG 70 when the preserved operations are: **(sub-SG label is 4) 1, 10, 11, 12, 25, 34, 35, 36.**

The transformation is:  $(\mathbf{a}_{70}, \mathbf{b}_{70}, \mathbf{c}_{70}) = (\mathbf{a}_{230}, \mathbf{b}_{230}, \mathbf{c}_{230}) \begin{pmatrix} 1 & 0 & 1 \\ 1 & 0 & -1 \\ 0 & 1 & 0 \end{pmatrix}, \overrightarrow{O_{230}O_{70}} = \frac{1}{4}\mathbf{a}_{70} + (\frac{1}{4})\mathbf{b}_{70} + (\frac{1}{2})\mathbf{c}_{70}$

The reduction of higher dimensional irrep:

$$O_h : T_{1g} \rightarrow B_{1g} + B_{2g} + B_{3g} \text{ of } D_{2h}.$$

$$O_h : T_{2g} \rightarrow A_g + B_{1g} + B_{3g} \text{ of } D_{2h}.$$

$$O_h : T_{1u} \rightarrow B_{1u} + B_{2u} + B_{3u} \text{ of } D_{2h}.$$

$$O_h : T_{2u} \rightarrow A_u + B_{1u} + B_{3u} \text{ of } D_{2h}.$$

The correspondences of irreps at HSPs from original SG to lowered SG:

$$\begin{aligned} n_{GM6}^{70} &= 2n_{GM11}^{230} + n_{GM8}^{230} + n_{GM9}^{230} n_{GM5}^{70} = 2n_{GM10}^{230} + n_{GM6}^{230} + n_{GM7}^{230} n_{Y4}^{70} = n_{H5}^{230} + n_{H6}^{230} + n_{H7}^{230} n_{Y3}^{70} = n_{H5}^{230} + n_{H6}^{230} + n_{H7}^{230} \\ n_{L3}^{70} &= n_{N3}^{230} + n_{N4}^{230} n_{L2}^{70} = n_{N3}^{230} + n_{N4}^{230} n_{Z3}^{70} = n_{N4}^{230} n_{Z4}^{70} = n_{N3}^{230} n_{T4}^{70} = n_{N4}^{230} n_{T3}^{70} = n_{N3}^{230} \end{aligned}$$

The lower SG is SG 88 when the preserved operations are: **(sub-SG label is 5)** 1, 6, 7, 10, 25, 30, 31, 34.

$$\text{The transformation is: } (\mathbf{a}_{88}, \mathbf{b}_{88}, \mathbf{c}_{88}) = (\mathbf{a}_{230}, \mathbf{b}_{230}, \mathbf{c}_{230}) \begin{pmatrix} 1 & 0 & 0 \\ 0 & 1 & 0 \\ 0 & 0 & 1 \end{pmatrix}, \overrightarrow{O_{230}O_{88}} = \frac{1}{2}\mathbf{a}_{88}$$

The reduction of higher dimensional irrep:

$$O_h : T_{1g} \rightarrow A_g + {}^2E_g + {}^1E_g \text{ of } C_{4h}.$$

$$O_h : T_{2g} \rightarrow {}^2E_g + B_g + {}^1E_g \text{ of } C_{4h}.$$

$$O_h : T_{1u} \rightarrow A_u + {}^2E_u + {}^1E_u \text{ of } C_{4h}.$$

$$O_h : T_{2u} \rightarrow {}^2E_u + B_u + {}^1E_u \text{ of } C_{4h}.$$

The correspondences of irreps at HSPs from original SG to lowered SG:

$$\begin{aligned} n_{GM9}^{88} &= n_{GM11}^{230} + n_{GM9}^{230} n_{GM5}^{88} = n_{GM10}^{230} + n_{GM7}^{230} n_{GM11}^{88} = n_{GM11}^{230} + n_{GM9}^{230} n_{GM7}^{88} = n_{GM10}^{230} + n_{GM7}^{230} n_{GM12}^{88} = \\ n_{GM11}^{230} + n_{GM8}^{230} n_{GM8}^{88} &= n_{GM10}^{230} + n_{GM6}^{230} n_{GM10}^{88} = n_{GM11}^{230} + n_{GM8}^{230} n_{GM6}^{88} = n_{GM10}^{230} + n_{GM6}^{230} n_{M4}^{88} = n_{H5}^{230} + n_{H6}^{230} + n_{H7}^{230} \\ n_{M3}^{88} &= n_{H5}^{230} + n_{H6}^{230} + n_{H7}^{230} n_{X2}^{88} = n_{N3}^{230} + n_{N4}^{230} n_{P5}^{88} = n_{P4}^{230} + n_{P6}^{230} + n_{P8}^{230} n_{P6}^{88} = n_{P5}^{230} + n_{P6}^{230} + n_{P7}^{230} n_{P7}^{88} = n_{P7}^{230} + n_{P8}^{230} \\ n_{P8}^{88} &= n_{P7}^{230} + n_{P8}^{230} n_{N3}^{88} = n_{N3}^{230} + n_{N4}^{230} n_{N2}^{88} = n_{N3}^{230} + n_{N4}^{230} \end{aligned}$$

The lower SG is SG 88 when the preserved operations are: **(sub-SG label is 6)** 1, 2, 3, 8, 25, 26, 27, 32.

$$\text{The transformation is: } (\mathbf{a}_{88}, \mathbf{b}_{88}, \mathbf{c}_{88}) = (\mathbf{a}_{230}, \mathbf{b}_{230}, \mathbf{c}_{230}) \begin{pmatrix} 0 & 0 & 1 \\ 1 & 0 & 0 \\ 0 & 1 & 0 \end{pmatrix}, \overrightarrow{O_{230}O_{88}} = \frac{1}{2}\mathbf{a}_{88}$$

The reduction of higher dimensional irrep:

$$O_h : T_{1g} \rightarrow A_g + {}^2E_g + {}^1E_g \text{ of } C_{4h}.$$

$$O_h : T_{2g} \rightarrow {}^2E_g + B_g + {}^1E_g \text{ of } C_{4h}.$$

$$O_h : T_{1u} \rightarrow A_u + {}^2E_u + {}^1E_u \text{ of } C_{4h}.$$

$$O_h : T_{2u} \rightarrow {}^2E_u + B_u + {}^1E_u \text{ of } C_{4h}.$$

The correspondences of irreps at HSPs from original SG to lowered SG:

$$\begin{aligned} n_{GM9}^{88} &= n_{GM11}^{230} + n_{GM9}^{230} n_{GM5}^{88} = n_{GM10}^{230} + n_{GM7}^{230} n_{GM11}^{88} = n_{GM11}^{230} + n_{GM9}^{230} n_{GM7}^{88} = n_{GM10}^{230} + n_{GM7}^{230} n_{GM12}^{88} = \\ n_{GM11}^{230} + n_{GM8}^{230} n_{GM8}^{88} &= n_{GM10}^{230} + n_{GM6}^{230} n_{GM10}^{88} = n_{GM11}^{230} + n_{GM8}^{230} n_{GM6}^{88} = n_{GM10}^{230} + n_{GM6}^{230} n_{M4}^{88} = n_{H5}^{230} + n_{H6}^{230} + n_{H7}^{230} \\ n_{M3}^{88} &= n_{H5}^{230} + n_{H6}^{230} + n_{H7}^{230} n_{X2}^{88} = n_{N3}^{230} + n_{N4}^{230} n_{P5}^{88} = n_{P4}^{230} + n_{P6}^{230} + n_{P8}^{230} n_{P6}^{88} = n_{P5}^{230} + n_{P6}^{230} + n_{P7}^{230} n_{P7}^{88} = n_{P7}^{230} + n_{P8}^{230} \\ n_{P8}^{88} &= n_{P7}^{230} + n_{P8}^{230} n_{N3}^{88} = n_{N3}^{230} + n_{N4}^{230} n_{N2}^{88} = n_{N3}^{230} + n_{N4}^{230} \end{aligned}$$

The lower SG is SG 88 when the preserved operations are: **(sub-SG label is 7)** 1, 4, 5, 9, 25, 28, 29, 33.

$$\text{The transformation is: } (\mathbf{a}_{88}, \mathbf{b}_{88}, \mathbf{c}_{88}) = (\mathbf{a}_{230}, \mathbf{b}_{230}, \mathbf{c}_{230}) \begin{pmatrix} 0 & -1 & 0 \\ 0 & 0 & -1 \\ 1 & 0 & 0 \end{pmatrix}, \overrightarrow{O_{230}O_{88}} = \frac{1}{2}\mathbf{a}_{88}$$

The reduction of higher dimensional irrep:

$$O_h : T_{1g} \rightarrow A_g + {}^2E_g + {}^1E_g \text{ of } C_{4h}.$$

$$O_h : T_{2g} \rightarrow {}^2E_g + B_g + {}^1E_g \text{ of } C_{4h}.$$

$$O_h : T_{1u} \rightarrow A_u + {}^2E_u + {}^1E_u \text{ of } C_{4h}.$$

$$O_h : T_{2u} \rightarrow {}^2E_u + B_u + {}^1E_u \text{ of } C_{4h}.$$

The correspondences of irreps at HSPs from original SG to lowered SG:

$$\begin{aligned} n_{GM9}^{88} &= n_{GM11}^{230} + n_{GM9}^{230} n_{GM5}^{88} = n_{GM10}^{230} + n_{GM7}^{230} n_{GM11}^{88} = n_{GM11}^{230} + n_{GM9}^{230} n_{GM7}^{88} = n_{GM10}^{230} + n_{GM7}^{230} n_{GM12}^{88} = \\ n_{GM11}^{230} + n_{GM8}^{230} n_{GM8}^{88} &= n_{GM10}^{230} + n_{GM6}^{230} n_{GM10}^{88} = n_{GM11}^{230} + n_{GM8}^{230} n_{GM6}^{88} = n_{GM10}^{230} + n_{GM6}^{230} n_{M4}^{88} = n_{H5}^{230} + n_{H6}^{230} + n_{H7}^{230} \\ n_{M3}^{88} &= n_{H5}^{230} + n_{H6}^{230} + n_{H7}^{230} n_{X2}^{88} = n_{N3}^{230} + n_{N4}^{230} n_{P5}^{88} = n_{P4}^{230} + n_{P6}^{230} + n_{P8}^{230} n_{P6}^{88} = n_{P5}^{230} + n_{P6}^{230} + n_{P7}^{230} n_{P7}^{88} = n_{P7}^{230} + n_{P8}^{230} \\ n_{P8}^{88} &= n_{P7}^{230} + n_{P8}^{230} n_{N3}^{88} = n_{N3}^{230} + n_{N4}^{230} n_{N2}^{88} = n_{N3}^{230} + n_{N4}^{230} \end{aligned}$$

The lower SG is SG 142 when the preserved operations are: **(sub-SG label is 8)** 1, 6, 7, 10, 8, 9, 11, 12, 25, 30, 31, 34, 32, 33, 35, 36.

$$\text{The transformation is: } (\mathbf{a}_{142}, \mathbf{b}_{142}, \mathbf{c}_{142}) = (\mathbf{a}_{230}, \mathbf{b}_{230}, \mathbf{c}_{230}) \begin{pmatrix} -1 & 0 & 0 \\ 0 & -1 & 0 \\ 0 & 0 & 1 \end{pmatrix}, \overrightarrow{O_{230}O_{142}} = -\frac{1}{2}\mathbf{a}_{142}$$

The reduction of higher dimensional irrep:

$$O_h : E_g \rightarrow A_{1g} + B_{1g} \text{ of } D_{4h}.$$

$$O_h : E_u \rightarrow A_{1u} + B_{1u} \text{ of } D_{4h}.$$

The correspondences of irreps at HSPs from original SG to lowered SG:

$$\begin{aligned} n_{GM8}^{142} &= n_{GM11}^{230} + n_{GM9}^{230} n_{GM6}^{142} = n_{GM10}^{230} + n_{GM7}^{230} n_{GM9}^{142} = n_{GM11}^{230} + n_{GM8}^{230} n_{GM7}^{142} = n_{GM10}^{230} + n_{GM6}^{230} n_{M5}^{142} = n_{H5}^{230} + n_{H6}^{230} + n_{H7}^{230} \\ n_{X3}^{142} &= n_{N3}^{230} n_{X4}^{142} = n_{N4}^{230} n_{P3}^{142} = n_{P4}^{230} + n_{P6}^{230} n_{P5}^{142} = n_{P5}^{230} + n_{P6}^{230} n_{P6}^{142} = n_{P8}^{230} n_{P4}^{142} = n_{P7}^{230} n_{P7}^{142} = n_{P7}^{230} + n_{P8}^{230} n_{N2}^{142} = \\ & n_{N3}^{230} + n_{N4}^{230} \end{aligned}$$

The lower SG is SG 142 when the preserved operations are: (**sub-SG label is 9**) 1, 2, 3, 8, 9, 10, 13, 14, 25, 26, 27, 32, 33, 34, 37, 38.

$$\text{The transformation is: } (\mathbf{a}_{142}, \mathbf{b}_{142}, \mathbf{c}_{142}) = (\mathbf{a}_{230}, \mathbf{b}_{230}, \mathbf{c}_{230}) \begin{pmatrix} 0 & 0 & 1 \\ -1 & 0 & 0 \\ 0 & -1 & 0 \end{pmatrix}, \overrightarrow{O_{230}O_{142}} = -\frac{1}{2}\mathbf{a}_{142}$$

The reduction of higher dimensional irrep:

$$O_h : E_g \rightarrow A_{1g} + B_{1g} \text{ of } D_{4h}.$$

$$O_h : E_u \rightarrow A_{1u} + B_{1u} \text{ of } D_{4h}.$$

The correspondences of irreps at HSPs from original SG to lowered SG:

$$\begin{aligned} n_{GM8}^{142} &= n_{GM11}^{230} + n_{GM9}^{230} n_{GM6}^{142} = n_{GM10}^{230} + n_{GM7}^{230} n_{GM9}^{142} = n_{GM11}^{230} + n_{GM8}^{230} n_{GM7}^{142} = n_{GM10}^{230} + n_{GM6}^{230} n_{M5}^{142} = n_{H5}^{230} + n_{H6}^{230} + n_{H7}^{230} \\ n_{X3}^{142} &= n_{N3}^{230} n_{X4}^{142} = n_{N4}^{230} n_{P3}^{142} = n_{P4}^{230} + n_{P6}^{230} n_{P5}^{142} = n_{P5}^{230} + n_{P6}^{230} n_{P6}^{142} = n_{P8}^{230} n_{P4}^{142} = n_{P7}^{230} n_{P7}^{142} = n_{P7}^{230} + n_{P8}^{230} n_{N2}^{142} = \\ & n_{N3}^{230} + n_{N4}^{230} \end{aligned}$$

The lower SG is SG 142 when the preserved operations are: (**sub-SG label is 10**) 1, 4, 5, 9, 10, 8, 16, 15, 25, 28, 29, 33, 34, 32, 40, 39.

$$\text{The transformation is: } (\mathbf{a}_{142}, \mathbf{b}_{142}, \mathbf{c}_{142}) = (\mathbf{a}_{230}, \mathbf{b}_{230}, \mathbf{c}_{230}) \begin{pmatrix} 0 & 1 & 0 \\ 0 & 0 & -1 \\ -1 & 0 & 0 \end{pmatrix}, \overrightarrow{O_{230}O_{142}} = -\frac{1}{2}\mathbf{a}_{142}$$

The reduction of higher dimensional irrep:

$$O_h : E_g \rightarrow A_{1g} + B_{1g} \text{ of } D_{4h}.$$

$$O_h : E_u \rightarrow A_{1u} + B_{1u} \text{ of } D_{4h}.$$

The correspondences of irreps at HSPs from original SG to lowered SG:

$$\begin{aligned} n_{GM8}^{142} &= n_{GM11}^{230} + n_{GM9}^{230} n_{GM6}^{142} = n_{GM10}^{230} + n_{GM7}^{230} n_{GM9}^{142} = n_{GM11}^{230} + n_{GM8}^{230} n_{GM7}^{142} = n_{GM10}^{230} + n_{GM6}^{230} n_{M5}^{142} = n_{H5}^{230} + n_{H6}^{230} + n_{H7}^{230} \\ n_{X3}^{142} &= n_{N3}^{230} n_{X4}^{142} = n_{N4}^{230} n_{P3}^{142} = n_{P7}^{230} n_{P5}^{142} = n_{P8}^{230} n_{P6}^{142} = n_{P5}^{230} + n_{P6}^{230} n_{P4}^{142} = n_{P4}^{230} + n_{P6}^{230} n_{P7}^{142} = n_{P7}^{230} + n_{P8}^{230} n_{N2}^{142} = \\ & n_{N3}^{230} + n_{N4}^{230} \end{aligned}$$

The lower SG is SG 148 when the preserved operations are: (**sub-SG label is 11**) 1, 17, 18, 25, 41, 42.

$$\text{The transformation is: } (\mathbf{a}_{148}, \mathbf{b}_{148}, \mathbf{c}_{148}) = (\mathbf{a}_{230}, \mathbf{b}_{230}, \mathbf{c}_{230}) \begin{pmatrix} \frac{1}{2} & -\frac{1}{2} & \frac{1}{2} \\ \frac{1}{2} & \frac{1}{2} & -\frac{1}{2} \\ -\frac{1}{2} & \frac{1}{2} & \frac{1}{2} \end{pmatrix}, \overrightarrow{O_{230}O_{148}} = \mathbf{0}$$

The reduction of higher dimensional irrep:

$$O_h : T_{1g} \rightarrow A_g + {}^2E_g + {}^1E_g \text{ of } C_{3i}.$$

$$O_h : T_{2g} \rightarrow A_g + {}^2E_g + {}^1E_g \text{ of } C_{3i}.$$

$$O_h : T_{1u} \rightarrow {}^1E_u + A_u + {}^2E_u \text{ of } C_{3i}.$$

$$O_h : T_{2u} \rightarrow {}^1E_u + A_u + {}^2E_u \text{ of } C_{3i}.$$

The correspondences of irreps at HSPs from original SG to lowered SG:

$$\begin{aligned} n_{GM7}^{148} &= 2n_{GM11}^{230} n_{GM4}^{148} = 2n_{GM10}^{230} n_{GM9}^{148} = n_{GM11}^{230} + n_{GM8}^{230} + n_{GM9}^{230} n_{GM6}^{148} = n_{GM10}^{230} + n_{GM6}^{230} + n_{GM7}^{230} n_{L2}^{148} = n_{N3}^{230} + n_{N4}^{230} n_{L3}^{148} = n_{N3}^{230} + n_{N4}^{230} n_{F2}^{148} = n_{N3}^{230} + n_{N4}^{230} \\ n_{F3}^{148} &= n_{N3}^{230} + n_{N4}^{230} n_{T7}^{148} = n_{H6}^{230} + n_{H7}^{230} n_{T4}^{148} = n_{H6}^{230} + n_{H7}^{230} n_{T9}^{148} = n_{H5}^{230} + n_{H7}^{230} n_{T6}^{148} = n_{H5}^{230} + n_{H6}^{230} n_{T8}^{148} = n_{H5}^{230} + n_{H6}^{230} \\ n_{T5}^{148} &= n_{H5}^{230} + n_{H7}^{230} \end{aligned}$$

The lower SG is SG 148 when the preserved operations are: (**sub-SG label is 12**) 1, 24, 23, 25, 48, 47.

$$\text{The transformation is: } (\mathbf{a}_{148}, \mathbf{b}_{148}, \mathbf{c}_{148}) = (\mathbf{a}_{230}, \mathbf{b}_{230}, \mathbf{c}_{230}) \begin{pmatrix} -\frac{1}{2} & -\frac{1}{2} & \frac{1}{2} \\ \frac{1}{2} & -\frac{1}{2} & -\frac{1}{2} \\ \frac{1}{2} & -\frac{1}{2} & \frac{1}{2} \end{pmatrix}, \overrightarrow{O_{230}O_{148}} = \frac{1}{2}\mathbf{b}_{148} + \left(\frac{1}{2}\right)\mathbf{c}_{148}$$

The reduction of higher dimensional irrep:

$$O_h : T_{1g} \rightarrow A_g + {}^2E_g + {}^1E_g \text{ of } C_{3i}.$$

$$O_h : T_{2g} \rightarrow A_g + {}^2E_g + {}^1E_g \text{ of } C_{3i}.$$

$$O_h : T_{1u} \rightarrow {}^1E_u + A_u + {}^2E_u \text{ of } C_{3i}.$$

$$O_h : T_{2u} \rightarrow {}^1E_u + A_u + {}^2E_u \text{ of } C_{3i}.$$

The correspondences of irreps at HSPs from original SG to lowered SG:

$$\begin{aligned}
 n_{GM7}^{148} &= 2n_{GM11}^{230} n_{GM4}^{148} = 2n_{GM10}^{230} n_{GM9}^{148} = n_{GM11}^{230} + n_{GM8}^{230} + n_{GM9}^{230} n_{GM6}^{148} = n_{GM10}^{230} + n_{GM6}^{230} + n_{GM7}^{230} n_{GM8}^{148} = \\
 n_{GM11}^{230} + n_{GM8}^{230} + n_{GM9}^{230} n_{GM5}^{148} &= n_{GM10}^{230} + n_{GM6}^{230} + n_{GM7}^{230} n_{L2}^{148} = n_{N3}^{230} + n_{N4}^{230} n_{L3}^{148} = n_{N3}^{230} + n_{N4}^{230} n_{F2}^{148} = n_{N3}^{230} + n_{N4}^{230} \\
 n_{F3}^{148} &= n_{N3}^{230} + n_{N4}^{230} n_{T7}^{148} = n_{H6}^{230} + n_{H7}^{230} n_{T4}^{148} = n_{H6}^{230} + n_{H7}^{230} n_{T9}^{148} = n_{H5}^{230} + n_{H7}^{230} n_{T6}^{148} = n_{H5}^{230} + n_{H6}^{230} n_{T8}^{148} = n_{H5}^{230} + n_{H6}^{230} \\
 n_{T5}^{148} &= n_{H5}^{230} + n_{H7}^{230}
 \end{aligned}$$

The lower SG is SG 148 when the preserved operations are: **(sub-SG label is 13)** 1, 20, 19, 25, 44, 43.

The transformation is:  $(\mathbf{a}_{148}, \mathbf{b}_{148}, \mathbf{c}_{148}) = (\mathbf{a}_{230}, \mathbf{b}_{230}, \mathbf{c}_{230}) \begin{pmatrix} \frac{1}{2} & -\frac{1}{2} & \frac{1}{2} \\ -\frac{1}{2} & -\frac{1}{2} & \frac{1}{2} \\ \frac{1}{2} & -\frac{1}{2} & -\frac{1}{2} \end{pmatrix}, \overrightarrow{O_{230}O_{148}} = \frac{1}{2}\mathbf{b}_{148} + (\frac{1}{2})\mathbf{c}_{148}$

The reduction of higher dimensional irrep:

$$\begin{aligned}
 O_h : T_{1g} &\rightarrow A_g + {}^2E_g + {}^1E_g \text{ of } C_{3i}. \\
 O_h : T_{2g} &\rightarrow A_g + {}^2E_g + {}^1E_g \text{ of } C_{3i}. \\
 O_h : T_{1u} &\rightarrow {}^1E_u + A_u + {}^2E_u \text{ of } C_{3i}. \\
 O_h : T_{2u} &\rightarrow {}^1E_u + A_u + {}^2E_u \text{ of } C_{3i}.
 \end{aligned}$$

The correspondences of irreps at HSPs from original SG to lowered SG:

$$\begin{aligned}
 n_{GM7}^{148} &= 2n_{GM11}^{230} n_{GM4}^{148} = 2n_{GM10}^{230} n_{GM9}^{148} = n_{GM11}^{230} + n_{GM8}^{230} + n_{GM9}^{230} n_{GM6}^{148} = n_{GM10}^{230} + n_{GM6}^{230} + n_{GM7}^{230} n_{GM8}^{148} = \\
 n_{GM11}^{230} + n_{GM8}^{230} + n_{GM9}^{230} n_{GM5}^{148} &= n_{GM10}^{230} + n_{GM6}^{230} + n_{GM7}^{230} n_{L2}^{148} = n_{N3}^{230} + n_{N4}^{230} n_{L3}^{148} = n_{N3}^{230} + n_{N4}^{230} n_{F2}^{148} = n_{N3}^{230} + n_{N4}^{230} \\
 n_{F3}^{148} &= n_{N3}^{230} + n_{N4}^{230} n_{T7}^{148} = n_{H6}^{230} + n_{H7}^{230} n_{T4}^{148} = n_{H6}^{230} + n_{H7}^{230} n_{T9}^{148} = n_{H5}^{230} + n_{H7}^{230} n_{T6}^{148} = n_{H5}^{230} + n_{H6}^{230} n_{T8}^{148} = n_{H5}^{230} + n_{H6}^{230} \\
 n_{T5}^{148} &= n_{H5}^{230} + n_{H7}^{230}
 \end{aligned}$$

The lower SG is SG 148 when the preserved operations are: **(sub-SG label is 14)** 1, 22, 21, 25, 46, 45.

The transformation is:  $(\mathbf{a}_{148}, \mathbf{b}_{148}, \mathbf{c}_{148}) = (\mathbf{a}_{230}, \mathbf{b}_{230}, \mathbf{c}_{230}) \begin{pmatrix} -\frac{1}{2} & \frac{1}{2} & \frac{1}{2} \\ -\frac{1}{2} & -\frac{1}{2} & \frac{1}{2} \\ \frac{1}{2} & -\frac{1}{2} & \frac{1}{2} \end{pmatrix}, \overrightarrow{O_{230}O_{148}} = \frac{1}{2}\mathbf{b}_{148} + (\frac{1}{2})\mathbf{c}_{148}$

The reduction of higher dimensional irrep:

$$\begin{aligned}
 O_h : T_{1g} &\rightarrow A_g + {}^2E_g + {}^1E_g \text{ of } C_{3i}. \\
 O_h : T_{2g} &\rightarrow A_g + {}^2E_g + {}^1E_g \text{ of } C_{3i}. \\
 O_h : T_{1u} &\rightarrow {}^1E_u + A_u + {}^2E_u \text{ of } C_{3i}. \\
 O_h : T_{2u} &\rightarrow {}^1E_u + A_u + {}^2E_u \text{ of } C_{3i}.
 \end{aligned}$$

The correspondences of irreps at HSPs from original SG to lowered SG:

$$\begin{aligned}
 n_{GM7}^{148} &= 2n_{GM11}^{230} n_{GM4}^{148} = 2n_{GM10}^{230} n_{GM9}^{148} = n_{GM11}^{230} + n_{GM8}^{230} + n_{GM9}^{230} n_{GM6}^{148} = n_{GM10}^{230} + n_{GM6}^{230} + n_{GM7}^{230} n_{GM8}^{148} = \\
 n_{GM11}^{230} + n_{GM8}^{230} + n_{GM9}^{230} n_{GM5}^{148} &= n_{GM10}^{230} + n_{GM6}^{230} + n_{GM7}^{230} n_{L2}^{148} = n_{N3}^{230} + n_{N4}^{230} n_{L3}^{148} = n_{N3}^{230} + n_{N4}^{230} n_{F2}^{148} = n_{N3}^{230} + n_{N4}^{230} \\
 n_{F3}^{148} &= n_{N3}^{230} + n_{N4}^{230} n_{T7}^{148} = n_{H6}^{230} + n_{H7}^{230} n_{T4}^{148} = n_{H6}^{230} + n_{H7}^{230} n_{T9}^{148} = n_{H5}^{230} + n_{H7}^{230} n_{T6}^{148} = n_{H5}^{230} + n_{H6}^{230} n_{T8}^{148} = n_{H5}^{230} + n_{H7}^{230} \\
 n_{T5}^{148} &= n_{H5}^{230} + n_{H6}^{230}
 \end{aligned}$$

The lower SG is SG 206 when the preserved operations are: **(sub-SG label is 15)** 1, 8, 9, 10, 17, 24, 20, 22, 18, 23, 19, 21, 25, 32, 33, 34, 41, 48, 44, 46, 42, 47, 43, 45.

The transformation is:  $(\mathbf{a}_{206}, \mathbf{b}_{206}, \mathbf{c}_{206}) = (\mathbf{a}_{230}, \mathbf{b}_{230}, \mathbf{c}_{230}) \begin{pmatrix} 0 & 0 & -1 \\ -1 & 0 & 0 \\ 0 & 1 & 0 \end{pmatrix}, \overrightarrow{O_{230}O_{206}} = \frac{1}{2}\mathbf{a}_{206}$

The reduction of higher dimensional irrep:

$$\begin{aligned}
 O_h : E_g &\rightarrow {}^1E_g + {}^2E_g \text{ of } T_h. \\
 O_h : E_u &\rightarrow {}^1E_u + {}^2E_u \text{ of } T_h.
 \end{aligned}$$

The correspondences of irreps at HSPs from original SG to lowered SG:

$$\begin{aligned}
 n_{GM9}^{206} &= n_{GM11}^{230} n_{GM6}^{206} = n_{GM10}^{230} n_{GM10}^{206} = n_{GM11}^{230} n_{GM7}^{206} = n_{GM10}^{230} n_{GM8}^{206} = n_{GM8}^{230} + n_{GM9}^{230} n_{GM5}^{206} = n_{GM6}^{230} + n_{GM7}^{230} n_{H9}^{206} = \\
 n_{H7}^{230} n_{H6}^{206} &= n_{H6}^{230} n_{H10}^{206} = n_{H6}^{230} n_{H7}^{206} = n_{H7}^{230} n_{H8}^{206} = n_{H5}^{230} n_{H5}^{206} = n_{H5}^{230} n_{N2}^{206} = n_{N3}^{230} + n_{N4}^{230} n_{P4}^{206} = n_{P4}^{230} + n_{P5}^{230} n_{P6}^{206} = n_{P6}^{230} \\
 n_{P5}^{206} &= n_{P6}^{230} n_{P7}^{206} = n_{P7}^{230} + n_{P8}^{230}
 \end{aligned}$$

[1] Manfred Sigrist and Kazuo Ueda, "Phenomenological theory of unconventional superconductivity," *Rev. Mod. Phys.* **63**, 239–311 (1991).
